# Supplementary material for: An analogue of the Robin inequality of the second type for odd integers
Source: arXiv:2202.08390 ancillary file (2022-03-21)
Supplement: Supplementary file 1 [file robintable.pdf]

# Numerical Table for “An analogue of the Robin inequality of the second type for odd integers”

February 17, 2022

## Contents

|          |                |           |
|----------|----------------|-----------|
| <b>1</b> | <b>Table 1</b> | <b>1</b>  |
| <b>2</b> | <b>Table 2</b> | <b>3</b>  |
| <b>3</b> | <b>Table 3</b> | <b>3</b>  |
| <b>4</b> | <b>Table 4</b> | <b>4</b>  |
| <b>5</b> | <b>Table 5</b> | <b>54</b> |

In the following we give some tables which are used to complete the proof of the theorem. Table 1 may be not so long. Table 2 and Table 3 are short. But Table 4 and Table 5 are quite long. The author never recommends to print out them.

## 1 Table 1

In the legend of the table,  $N$  stands for odd colossally abundant number such that the largest prime factor is  $p_k$ . Thus in the first entry of the table the odd colossally abundant number which is treat there is  $3^6 \cdot 5^4 \cdot 7^3 \cdot 11^2 \cdot 13^2 \cdot 17^2 \cdot 19^2 \cdot 23^1 \cdot 29 \cdots 251$ .

There are some distinct odd colossally abundant numbers which have same prime number as their largest prime factor. In such case there are more than two entries in the table. For example, there are 3 rows whose left most entries are 31. The reason is that there are 3 odd colossally abundant numbers :  $3^3 \cdot 5^2 \cdot 7 \cdot 11 \cdots 31$  (the bottom),  $3^3 \cdot 5^2 \cdot 7^2 \cdot 11 \cdots 31$  (the middle) and  $3^4 \cdot 5^2 \cdot 7^2 \cdot 11 \cdots 31$  (the top).

Table 1: Table for Corollary 3.6 (1)

| $p_k$ | $\frac{19.5}{20} \frac{\sigma(N)}{N}$ | $\frac{e^\gamma}{2} \log \log N$ | $\frac{0.5}{20} \frac{\sigma(N)}{N}$ | $\frac{0.7399\dots}{\log \log N}$ |
|-------|---------------------------------------|----------------------------------|--------------------------------------|-----------------------------------|
| 251   | 4.797623                              | 4.939500                         | 0.123016                             | 0.133396                          |
| 241   | 4.778585                              | 4.920098                         | 0.122528                             | 0.133922                          |
| 239   | 4.758839                              | 4.900411                         | 0.122022                             | 0.134460                          |

| $p_k$ | $\frac{19.5}{20} \frac{\sigma(N)}{N}$ | $\frac{e^\gamma}{2} \log \log N$ | $\frac{0.5}{20} \frac{\sigma(N)}{N}$ | $\frac{0.7399...}{\log \log N}$ |
|-------|---------------------------------------|----------------------------------|--------------------------------------|---------------------------------|
| 233   | 4.739010                              | 4.880310                         | 0.121513                             | 0.135014                        |
| 229   | 4.718758                              | 4.859841                         | 0.120994                             | 0.135582                        |
| 229   | 4.712716                              | 4.853706                         | 0.120839                             | 0.135754                        |
| 227   | 4.692226                              | 4.832677                         | 0.120313                             | 0.136344                        |
| 223   | 4.671646                              | 4.811174                         | 0.119786                             | 0.136954                        |
| 211   | 4.650791                              | 4.789212                         | 0.119251                             | 0.137582                        |
| 211   | 4.646536                              | 4.784683                         | 0.119142                             | 0.137712                        |
| 199   | 4.624618                              | 4.762285                         | 0.118580                             | 0.138360                        |
| 199   | 4.612480                              | 4.749717                         | 0.118269                             | 0.138726                        |
| 197   | 4.589418                              | 4.726668                         | 0.117677                             | 0.139402                        |
| 193   | 4.566239                              | 4.703052                         | 0.117083                             | 0.140102                        |
| 191   | 4.542701                              | 4.678888                         | 0.116480                             | 0.140826                        |
| 181   | 4.519042                              | 4.654100                         | 0.115873                             | 0.141576                        |
| 179   | 4.494212                              | 4.628867                         | 0.115236                             | 0.142348                        |
| 173   | 4.469244                              | 4.602955                         | 0.114596                             | 0.143149                        |
| 167   | 4.443558                              | 4.576444                         | 0.113937                             | 0.143978                        |
| 167   | 4.429084                              | 4.561525                         | 0.113566                             | 0.144449                        |
| 163   | 4.402721                              | 4.533925                         | 0.112890                             | 0.145328                        |
| 157   | 4.375875                              | 4.505579                         | 0.112202                             | 0.146243                        |
| 151   | 4.348179                              | 4.476520                         | 0.111492                             | 0.147192                        |
| 151   | 4.337309                              | 4.465079                         | 0.111213                             | 0.147569                        |
| 149   | 4.308774                              | 4.434883                         | 0.110481                             | 0.148574                        |
| 139   | 4.280049                              | 4.403712                         | 0.109745                             | 0.149626                        |
| 137   | 4.249477                              | 4.371867                         | 0.108961                             | 0.150715                        |
| 131   | 4.218684                              | 4.338940                         | 0.108171                             | 0.151859                        |
| 127   | 4.186724                              | 4.305065                         | 0.107352                             | 0.153054                        |
| 113   | 4.154015                              | 4.270080                         | 0.106513                             | 0.154308                        |
| 109   | 4.117577                              | 4.234559                         | 0.105579                             | 0.155602                        |
| 107   | 4.080144                              | 4.197850                         | 0.104619                             | 0.156963                        |
| 103   | 4.042365                              | 4.159717                         | 0.103650                             | 0.158402                        |
| 101   | 4.003496                              | 4.120210                         | 0.102654                             | 0.159921                        |
| 97    | 3.964246                              | 4.079048                         | 0.101647                             | 0.161535                        |
| 97    | 3.942584                              | 4.055321                         | 0.101092                             | 0.162480                        |
| 89    | 3.902353                              | 4.011367                         | 0.100060                             | 0.164260                        |
| 83    | 3.858994                              | 3.966022                         | 0.098949                             | 0.166138                        |
| 83    | 3.848392                              | 3.954563                         | 0.098677                             | 0.166620                        |
| 79    | 3.802578                              | 3.906923                         | 0.097502                             | 0.168651                        |
| 73    | 3.755046                              | 3.857168                         | 0.096283                             | 0.170827                        |
| 73    | 3.726812                              | 3.828634                         | 0.095559                             | 0.172100                        |
| 71    | 3.676450                              | 3.775179                         | 0.094268                             | 0.174537                        |
| 67    | 3.625388                              | 3.718690                         | 0.092959                             | 0.177188                        |
| 61    | 3.572074                              | 3.659222                         | 0.091592                             | 0.180068                        |
| 59    | 3.514459                              | 3.596970                         | 0.090114                             | 0.183184                        |
| 59    | 3.491931                              | 3.571360                         | 0.089537                             | 0.184498                        |

| $p_k$ | $\frac{19.5}{20} \frac{\sigma(N)}{N}$ | $\frac{e^\gamma}{2} \log \log N$ | $\frac{0.5}{20} \frac{\sigma(N)}{N}$ | $\frac{0.7399...}{\log \log N}$ |
|-------|---------------------------------------|----------------------------------|--------------------------------------|---------------------------------|
| 53    | 3.433732                              | 3.502978                         | 0.088044                             | 0.188099                        |
| 47    | 3.370144                              | 3.430934                         | 0.086414                             | 0.192049                        |
| 43    | 3.299933                              | 3.355020                         | 0.084614                             | 0.196395                        |
| 41    | 3.224935                              | 3.274035                         | 0.082691                             | 0.201253                        |
| 37    | 3.148150                              | 3.186126                         | 0.080722                             | 0.206805                        |
| 31    | 3.065304                              | 3.091425                         | 0.078598                             | 0.213140                        |
| 31    | 3.039971                              | 3.060494                         | 0.077948                             | 0.215295                        |
| 31    | 2.986638                              | 3.002923                         | 0.076580                             | 0.219422                        |
| 29    | 2.893306                              | 2.891253                         | 0.074187                             | 0.227897                        |

## 2 Table 2

About the table, see the notices before Table 1.

Table 2: Table for Corollary 3.6 (2)

| $p_k$ | $\frac{19.0}{20} \frac{\sigma(N)}{N}$ | $\frac{e^\gamma}{2} \log \log N$ | $\frac{1.0}{20} \frac{\sigma(N)}{N}$ | $\frac{0.7399...}{\log \log N}$ |
|-------|---------------------------------------|----------------------------------|--------------------------------------|---------------------------------|
| 59    | 3.424345                              | 3.596970                         | 0.180229                             | 0.183184                        |
| 59    | 3.402394                              | 3.571360                         | 0.179073                             | 0.184498                        |
| 53    | 3.345688                              | 3.502978                         | 0.176089                             | 0.188099                        |
| 47    | 3.283730                              | 3.430934                         | 0.172828                             | 0.192049                        |
| 43    | 3.215319                              | 3.355020                         | 0.169227                             | 0.196395                        |
| 41    | 3.142244                              | 3.274035                         | 0.165381                             | 0.201253                        |
| 37    | 3.067429                              | 3.186126                         | 0.161444                             | 0.206805                        |
| 31    | 2.986707                              | 3.091425                         | 0.157195                             | 0.213140                        |
| 31    | 2.962023                              | 3.060494                         | 0.155896                             | 0.215295                        |
| 31    | 2.910058                              | 3.002923                         | 0.153161                             | 0.219422                        |
| 29    | 2.819119                              | 2.891253                         | 0.148375                             | 0.227897                        |
| 23    | 2.725148                              | 2.766208                         | 0.143429                             | 0.238199                        |
| 19    | 2.611600                              | 2.631507                         | 0.137453                             | 0.250392                        |
| 17    | 2.481020                              | 2.483264                         | 0.130580                             | 0.265339                        |
| 13    | 2.343186                              | 2.312727                         | 0.123326                             | 0.284905                        |

## 3 Table 3

About the table, see the notices before Table 1.

Table 3: Table for Corollary 3.6 (3)

| $p_k$ | $\frac{19.0}{20} \frac{\sigma(N)}{N}$ | $\frac{e^\gamma}{2} \log \log N$ | $\frac{1.0}{20} \frac{\sigma(N)}{N}$ | $\frac{0.7399...}{\log \log N}$ |
|-------|---------------------------------------|----------------------------------|--------------------------------------|---------------------------------|
| 19    | 2.487238                              | 2.631507                         | 0.261815                             | 0.250392                        |
| 17    | 2.362876                              | 2.483264                         | 0.248724                             | 0.265339                        |
| 13    | 2.231605                              | 2.312727                         | 0.234906                             | 0.284905                        |

| $p_k$ | $\frac{19.0}{20} \frac{\sigma(N)}{N}$ | $\frac{e^\gamma}{2} \log \log N$ | $\frac{1.0}{20} \frac{\sigma(N)}{N}$ | $\frac{0.7399\dots}{\log \log N}$ |
|-------|---------------------------------------|----------------------------------|--------------------------------------|-----------------------------------|
| 13    | 2.159618                              | 2.198990                         | 0.227328                             | 0.299641                          |
| 13    | 2.105628                              | 2.112070                         | 0.221645                             | 0.311972                          |
| 11    | 1.955226                              | 1.868412                         | 0.205813                             | 0.352657                          |

## 4 Table 4

In the table below,  $p_k$  stands for the  $k$ -th prime and  $N'_k = \prod_{i=2}^k p_i$ .

Table 4: Comparison with  $\frac{N}{\varphi(N)}$

| $k$  | $p_k$ | $\frac{\sigma(N'_k)}{N'_k}$ | $\frac{N'_k}{\varphi(N'_k)}$ | $\frac{e^\gamma}{2} \log \log N'_k + \frac{0.73\dots}{\log \log N'_k}$ |
|------|-------|-----------------------------|------------------------------|------------------------------------------------------------------------|
| 2262 | 19997 | 7.152698                    | 8.824246                     | 8.885457                                                               |
| 2261 | 19993 | 7.152340                    | 8.823805                     | 8.885015                                                               |
| 2260 | 19991 | 7.151982                    | 8.823364                     | 8.884573                                                               |
| 2259 | 19979 | 7.151625                    | 8.822922                     | 8.884131                                                               |
| 2258 | 19973 | 7.151267                    | 8.822481                     | 8.883689                                                               |
| 2257 | 19963 | 7.150909                    | 8.822039                     | 8.883247                                                               |
| 2256 | 19961 | 7.150550                    | 8.821597                     | 8.882804                                                               |
| 2255 | 19949 | 7.150192                    | 8.821155                     | 8.882361                                                               |
| 2254 | 19937 | 7.149834                    | 8.820713                     | 8.881918                                                               |
| 2253 | 19927 | 7.149475                    | 8.820271                     | 8.881475                                                               |
| 2252 | 19919 | 7.149116                    | 8.819828                     | 8.881031                                                               |
| 2251 | 19913 | 7.148757                    | 8.819385                     | 8.880587                                                               |
| 2250 | 19891 | 7.148398                    | 8.818942                     | 8.880144                                                               |
| 2249 | 19889 | 7.148039                    | 8.818499                     | 8.879699                                                               |
| 2248 | 19867 | 7.147680                    | 8.818055                     | 8.879255                                                               |
| 2247 | 19861 | 7.147320                    | 8.817612                     | 8.878811                                                               |
| 2246 | 19853 | 7.146960                    | 8.817168                     | 8.878366                                                               |
| 2245 | 19843 | 7.146600                    | 8.816724                     | 8.877921                                                               |
| 2244 | 19841 | 7.146240                    | 8.816279                     | 8.877476                                                               |
| 2243 | 19819 | 7.145880                    | 8.815835                     | 8.877031                                                               |
| 2242 | 19813 | 7.145519                    | 8.815390                     | 8.876585                                                               |
| 2241 | 19801 | 7.145159                    | 8.814945                     | 8.876140                                                               |
| 2240 | 19793 | 7.144798                    | 8.814500                     | 8.875694                                                               |
| 2239 | 19777 | 7.144437                    | 8.814055                     | 8.875248                                                               |
| 2238 | 19763 | 7.144076                    | 8.813609                     | 8.874801                                                               |
| 2237 | 19759 | 7.143714                    | 8.813163                     | 8.874355                                                               |
| 2236 | 19753 | 7.143353                    | 8.812717                     | 8.873908                                                               |
| 2235 | 19751 | 7.142991                    | 8.812271                     | 8.873461                                                               |
| 2234 | 19739 | 7.142629                    | 8.811825                     | 8.873014                                                               |
| 2233 | 19727 | 7.142268                    | 8.811378                     | 8.872567                                                               |
| 2232 | 19717 | 7.141906                    | 8.810932                     | 8.872119                                                               |
| 2231 | 19709 | 7.141543                    | 8.810485                     | 8.871672                                                               |

| $k$  | $p_k$ | $\frac{\sigma(N'_k)}{N'_k}$ | $\frac{N'_k}{\varphi(N'_k)}$ | $\frac{e^\gamma}{2} \log \log N'_k + \frac{0.73\dots}{\log \log N'_k}$ |
|------|-------|-----------------------------|------------------------------|------------------------------------------------------------------------|
| 2230 | 19699 | 7.141181                    | 8.810038                     | 8.871224                                                               |
| 2229 | 19697 | 7.140819                    | 8.809590                     | 8.870776                                                               |
| 2228 | 19687 | 7.140456                    | 8.809143                     | 8.870327                                                               |
| 2227 | 19681 | 7.140093                    | 8.808696                     | 8.869879                                                               |
| 2226 | 19661 | 7.139731                    | 8.808248                     | 8.869430                                                               |
| 2225 | 19609 | 7.139367                    | 8.807800                     | 8.868981                                                               |
| 2224 | 19603 | 7.139003                    | 8.807351                     | 8.868532                                                               |
| 2223 | 19597 | 7.138639                    | 8.806902                     | 8.868083                                                               |
| 2222 | 19583 | 7.138275                    | 8.806452                     | 8.867633                                                               |
| 2221 | 19577 | 7.137910                    | 8.806003                     | 8.867184                                                               |
| 2220 | 19571 | 7.137546                    | 8.805553                     | 8.866734                                                               |
| 2219 | 19559 | 7.137181                    | 8.805103                     | 8.866284                                                               |
| 2218 | 19553 | 7.136816                    | 8.804653                     | 8.865833                                                               |
| 2217 | 19543 | 7.136451                    | 8.804202                     | 8.865383                                                               |
| 2216 | 19541 | 7.136086                    | 8.803752                     | 8.864932                                                               |
| 2215 | 19531 | 7.135721                    | 8.803301                     | 8.864481                                                               |
| 2214 | 19507 | 7.135356                    | 8.802851                     | 8.864030                                                               |
| 2213 | 19501 | 7.134990                    | 8.802399                     | 8.863578                                                               |
| 2212 | 19489 | 7.134624                    | 8.801948                     | 8.863127                                                               |
| 2211 | 19483 | 7.134258                    | 8.801496                     | 8.862675                                                               |
| 2210 | 19477 | 7.133892                    | 8.801045                     | 8.862223                                                               |
| 2209 | 19471 | 7.133526                    | 8.800593                     | 8.861771                                                               |
| 2208 | 19469 | 7.133159                    | 8.800141                     | 8.861319                                                               |
| 2207 | 19463 | 7.132793                    | 8.799689                     | 8.860866                                                               |
| 2206 | 19457 | 7.132426                    | 8.799237                     | 8.860413                                                               |
| 2205 | 19447 | 7.132060                    | 8.798784                     | 8.859960                                                               |
| 2204 | 19441 | 7.131693                    | 8.798332                     | 8.859507                                                               |
| 2203 | 19433 | 7.131326                    | 8.797879                     | 8.859053                                                               |
| 2202 | 19429 | 7.130959                    | 8.797427                     | 8.858599                                                               |
| 2201 | 19427 | 7.130592                    | 8.796974                     | 8.858146                                                               |
| 2200 | 19423 | 7.130225                    | 8.796521                     | 8.857691                                                               |
| 2199 | 19421 | 7.129858                    | 8.796068                     | 8.857237                                                               |
| 2198 | 19417 | 7.129491                    | 8.795615                     | 8.856782                                                               |
| 2197 | 19403 | 7.129124                    | 8.795162                     | 8.856328                                                               |
| 2196 | 19391 | 7.128757                    | 8.794709                     | 8.855872                                                               |
| 2195 | 19387 | 7.128389                    | 8.794255                     | 8.855417                                                               |
| 2194 | 19381 | 7.128021                    | 8.793802                     | 8.854962                                                               |
| 2193 | 19379 | 7.127654                    | 8.793348                     | 8.854506                                                               |
| 2192 | 19373 | 7.127286                    | 8.792894                     | 8.854050                                                               |
| 2191 | 19333 | 7.126918                    | 8.792440                     | 8.853594                                                               |
| 2190 | 19319 | 7.126549                    | 8.791986                     | 8.853138                                                               |
| 2189 | 19309 | 7.126180                    | 8.791530                     | 8.852681                                                               |
| 2188 | 19301 | 7.125811                    | 8.791075                     | 8.852224                                                               |
| 2187 | 19289 | 7.125442                    | 8.790620                     | 8.851768                                                               |

| $k$  | $p_k$ | $\frac{\sigma(N'_k)}{N'_k}$ | $\frac{N'_k}{\varphi(N'_k)}$ | $\frac{e^\gamma}{2} \log \log N'_k + \frac{0.73\dots}{\log \log N'_k}$ |
|------|-------|-----------------------------|------------------------------|------------------------------------------------------------------------|
| 2186 | 19273 | 7.125073                    | 8.790164                     | 8.851310                                                               |
| 2185 | 19267 | 7.124703                    | 8.789708                     | 8.850853                                                               |
| 2184 | 19259 | 7.124333                    | 8.789252                     | 8.850396                                                               |
| 2183 | 19249 | 7.123963                    | 8.788795                     | 8.849938                                                               |
| 2182 | 19237 | 7.123593                    | 8.788339                     | 8.849480                                                               |
| 2181 | 19231 | 7.123223                    | 8.787882                     | 8.849022                                                               |
| 2180 | 19219 | 7.122853                    | 8.787425                     | 8.848563                                                               |
| 2179 | 19213 | 7.122482                    | 8.786968                     | 8.848105                                                               |
| 2178 | 19211 | 7.122111                    | 8.786510                     | 8.847646                                                               |
| 2177 | 19207 | 7.121741                    | 8.786053                     | 8.847187                                                               |
| 2176 | 19183 | 7.121370                    | 8.785595                     | 8.846727                                                               |
| 2175 | 19181 | 7.120999                    | 8.785137                     | 8.846268                                                               |
| 2174 | 19163 | 7.120627                    | 8.784679                     | 8.845808                                                               |
| 2173 | 19157 | 7.120256                    | 8.784221                     | 8.845348                                                               |
| 2172 | 19141 | 7.119884                    | 8.783763                     | 8.844888                                                               |
| 2171 | 19139 | 7.119512                    | 8.783304                     | 8.844428                                                               |
| 2170 | 19121 | 7.119140                    | 8.782845                     | 8.843967                                                               |
| 2169 | 19087 | 7.118768                    | 8.782385                     | 8.843506                                                               |
| 2168 | 19081 | 7.118395                    | 8.781925                     | 8.843046                                                               |
| 2167 | 19079 | 7.118022                    | 8.781465                     | 8.842584                                                               |
| 2166 | 19073 | 7.117649                    | 8.781005                     | 8.842123                                                               |
| 2165 | 19069 | 7.117276                    | 8.780544                     | 8.841661                                                               |
| 2164 | 19051 | 7.116903                    | 8.780084                     | 8.841200                                                               |
| 2163 | 19037 | 7.116529                    | 8.779623                     | 8.840738                                                               |
| 2162 | 19031 | 7.116155                    | 8.779162                     | 8.840275                                                               |
| 2161 | 19013 | 7.115781                    | 8.778701                     | 8.839813                                                               |
| 2160 | 19009 | 7.115407                    | 8.778239                     | 8.839350                                                               |
| 2159 | 19001 | 7.115033                    | 8.777777                     | 8.838887                                                               |
| 2158 | 18979 | 7.114658                    | 8.777315                     | 8.838424                                                               |
| 2157 | 18973 | 7.114284                    | 8.776853                     | 8.837961                                                               |
| 2156 | 18959 | 7.113909                    | 8.776390                     | 8.837497                                                               |
| 2155 | 18947 | 7.113533                    | 8.775927                     | 8.837034                                                               |
| 2154 | 18919 | 7.113158                    | 8.775464                     | 8.836570                                                               |
| 2153 | 18917 | 7.112782                    | 8.775000                     | 8.836105                                                               |
| 2152 | 18913 | 7.112406                    | 8.774536                     | 8.835641                                                               |
| 2151 | 18911 | 7.112030                    | 8.774072                     | 8.835176                                                               |
| 2150 | 18899 | 7.111654                    | 8.773608                     | 8.834712                                                               |
| 2149 | 18869 | 7.111278                    | 8.773144                     | 8.834247                                                               |
| 2148 | 18859 | 7.110901                    | 8.772679                     | 8.833781                                                               |
| 2147 | 18839 | 7.110524                    | 8.772214                     | 8.833316                                                               |
| 2146 | 18803 | 7.110146                    | 8.771748                     | 8.832850                                                               |
| 2145 | 18797 | 7.109768                    | 8.771282                     | 8.832384                                                               |
| 2144 | 18793 | 7.109390                    | 8.770815                     | 8.831918                                                               |
| 2143 | 18787 | 7.109012                    | 8.770348                     | 8.831452                                                               |

| $k$  | $p_k$ | $\frac{\sigma(N'_k)}{N'_k}$ | $\frac{N'_k}{\varphi(N'_k)}$ | $\frac{e^\gamma}{2} \log \log N'_k + \frac{0.73\dots}{\log \log N'_k}$ |
|------|-------|-----------------------------|------------------------------|------------------------------------------------------------------------|
| 2142 | 18773 | 7.108633                    | 8.769882                     | 8.830986                                                               |
| 2141 | 18757 | 7.108255                    | 8.769414                     | 8.830519                                                               |
| 2140 | 18749 | 7.107876                    | 8.768947                     | 8.830052                                                               |
| 2139 | 18743 | 7.107497                    | 8.768479                     | 8.829585                                                               |
| 2138 | 18731 | 7.107117                    | 8.768011                     | 8.829117                                                               |
| 2137 | 18719 | 7.106738                    | 8.767543                     | 8.828650                                                               |
| 2136 | 18713 | 7.106358                    | 8.767075                     | 8.828182                                                               |
| 2135 | 18701 | 7.105979                    | 8.766606                     | 8.827714                                                               |
| 2134 | 18691 | 7.105599                    | 8.766138                     | 8.827246                                                               |
| 2133 | 18679 | 7.105219                    | 8.765669                     | 8.826777                                                               |
| 2132 | 18671 | 7.104838                    | 8.765199                     | 8.826309                                                               |
| 2131 | 18661 | 7.104458                    | 8.764730                     | 8.825840                                                               |
| 2130 | 18637 | 7.104077                    | 8.764260                     | 8.825371                                                               |
| 2129 | 18617 | 7.103696                    | 8.763790                     | 8.824901                                                               |
| 2128 | 18593 | 7.103314                    | 8.763319                     | 8.824432                                                               |
| 2127 | 18587 | 7.102932                    | 8.762848                     | 8.823962                                                               |
| 2126 | 18583 | 7.102550                    | 8.762376                     | 8.823492                                                               |
| 2125 | 18553 | 7.102168                    | 8.761905                     | 8.823022                                                               |
| 2124 | 18541 | 7.101785                    | 8.761433                     | 8.822551                                                               |
| 2123 | 18539 | 7.101402                    | 8.760960                     | 8.822081                                                               |
| 2122 | 18523 | 7.101019                    | 8.760488                     | 8.821610                                                               |
| 2121 | 18521 | 7.100636                    | 8.760015                     | 8.821139                                                               |
| 2120 | 18517 | 7.100252                    | 8.759542                     | 8.820668                                                               |
| 2119 | 18503 | 7.099869                    | 8.759069                     | 8.820196                                                               |
| 2118 | 18493 | 7.099485                    | 8.758595                     | 8.819724                                                               |
| 2117 | 18481 | 7.099101                    | 8.758122                     | 8.819252                                                               |
| 2116 | 18461 | 7.098717                    | 8.757648                     | 8.818780                                                               |
| 2115 | 18457 | 7.098333                    | 8.757173                     | 8.818308                                                               |
| 2114 | 18451 | 7.097948                    | 8.756699                     | 8.817835                                                               |
| 2113 | 18443 | 7.097564                    | 8.756224                     | 8.817362                                                               |
| 2112 | 18439 | 7.097179                    | 8.755749                     | 8.816889                                                               |
| 2111 | 18433 | 7.096794                    | 8.755275                     | 8.816416                                                               |
| 2110 | 18427 | 7.096409                    | 8.754800                     | 8.815942                                                               |
| 2109 | 18413 | 7.096024                    | 8.754324                     | 8.815468                                                               |
| 2108 | 18401 | 7.095638                    | 8.753849                     | 8.814994                                                               |
| 2107 | 18397 | 7.095253                    | 8.753373                     | 8.814520                                                               |
| 2106 | 18379 | 7.094867                    | 8.752898                     | 8.814046                                                               |
| 2105 | 18371 | 7.094481                    | 8.752421                     | 8.813571                                                               |
| 2104 | 18367 | 7.094095                    | 8.751945                     | 8.813096                                                               |
| 2103 | 18353 | 7.093709                    | 8.751468                     | 8.812621                                                               |
| 2102 | 18341 | 7.093322                    | 8.750991                     | 8.812145                                                               |
| 2101 | 18329 | 7.092936                    | 8.750514                     | 8.811670                                                               |
| 2100 | 18313 | 7.092549                    | 8.750037                     | 8.811194                                                               |
| 2099 | 18311 | 7.092161                    | 8.749559                     | 8.810718                                                               |

| $k$  | $p_k$ | $\frac{\sigma(N'_k)}{N'_k}$ | $\frac{N'_k}{\varphi(N'_k)}$ | $\frac{e^\gamma}{2} \log \log N'_k + \frac{0.73\dots}{\log \log N'_k}$ |
|------|-------|-----------------------------|------------------------------|------------------------------------------------------------------------|
| 2098 | 18307 | 7.091774                    | 8.749081                     | 8.810242                                                               |
| 2097 | 18301 | 7.091387                    | 8.748603                     | 8.809765                                                               |
| 2096 | 18289 | 7.090999                    | 8.748125                     | 8.809288                                                               |
| 2095 | 18287 | 7.090612                    | 8.747647                     | 8.808811                                                               |
| 2094 | 18269 | 7.090224                    | 8.747169                     | 8.808334                                                               |
| 2093 | 18257 | 7.089836                    | 8.746690                     | 8.807856                                                               |
| 2092 | 18253 | 7.089447                    | 8.746211                     | 8.807379                                                               |
| 2091 | 18251 | 7.089059                    | 8.745732                     | 8.806901                                                               |
| 2090 | 18233 | 7.088671                    | 8.745252                     | 8.806422                                                               |
| 2089 | 18229 | 7.088282                    | 8.744773                     | 8.805944                                                               |
| 2088 | 18223 | 7.087893                    | 8.744293                     | 8.805465                                                               |
| 2087 | 18217 | 7.087504                    | 8.743813                     | 8.804986                                                               |
| 2086 | 18211 | 7.087115                    | 8.743333                     | 8.804507                                                               |
| 2085 | 18199 | 7.086726                    | 8.742853                     | 8.804028                                                               |
| 2084 | 18191 | 7.086337                    | 8.742373                     | 8.803548                                                               |
| 2083 | 18181 | 7.085947                    | 8.741892                     | 8.803068                                                               |
| 2082 | 18169 | 7.085557                    | 8.741411                     | 8.802588                                                               |
| 2081 | 18149 | 7.085167                    | 8.740930                     | 8.802108                                                               |
| 2080 | 18143 | 7.084777                    | 8.740449                     | 8.801627                                                               |
| 2079 | 18133 | 7.084387                    | 8.739967                     | 8.801146                                                               |
| 2078 | 18131 | 7.083996                    | 8.739485                     | 8.800665                                                               |
| 2077 | 18127 | 7.083605                    | 8.739003                     | 8.800184                                                               |
| 2076 | 18121 | 7.083214                    | 8.738521                     | 8.799703                                                               |
| 2075 | 18119 | 7.082824                    | 8.738038                     | 8.799221                                                               |
| 2074 | 18097 | 7.082433                    | 8.737556                     | 8.798739                                                               |
| 2073 | 18089 | 7.082041                    | 8.737073                     | 8.798257                                                               |
| 2072 | 18077 | 7.081650                    | 8.736590                     | 8.797774                                                               |
| 2071 | 18061 | 7.081258                    | 8.736107                     | 8.797291                                                               |
| 2070 | 18059 | 7.080866                    | 8.735623                     | 8.796808                                                               |
| 2069 | 18049 | 7.080474                    | 8.735140                     | 8.796325                                                               |
| 2068 | 18047 | 7.080082                    | 8.734656                     | 8.795842                                                               |
| 2067 | 18043 | 7.079689                    | 8.734172                     | 8.795358                                                               |
| 2066 | 18041 | 7.079297                    | 8.733688                     | 8.794874                                                               |
| 2065 | 18013 | 7.078905                    | 8.733204                     | 8.794390                                                               |
| 2064 | 17989 | 7.078512                    | 8.732719                     | 8.793906                                                               |
| 2063 | 17987 | 7.078118                    | 8.732233                     | 8.793421                                                               |
| 2062 | 17981 | 7.077725                    | 8.731748                     | 8.792936                                                               |
| 2061 | 17977 | 7.077331                    | 8.731262                     | 8.792451                                                               |
| 2060 | 17971 | 7.076937                    | 8.730776                     | 8.791966                                                               |
| 2059 | 17959 | 7.076544                    | 8.730291                     | 8.791480                                                               |
| 2058 | 17957 | 7.076150                    | 8.729805                     | 8.790994                                                               |
| 2057 | 17939 | 7.075756                    | 8.729318                     | 8.790508                                                               |
| 2056 | 17929 | 7.075361                    | 8.728832                     | 8.790022                                                               |
| 2055 | 17923 | 7.074967                    | 8.728345                     | 8.789535                                                               |



| $k$  | $p_k$ | $\frac{\sigma(N'_k)}{N'_k}$ | $\frac{N'_k}{\varphi(N'_k)}$ | $\frac{e^\gamma}{2} \log \log N'_k + \frac{0.73\dots}{\log \log N'_k}$ |
|------|-------|-----------------------------|------------------------------|------------------------------------------------------------------------|
| 2054 | 17921 | 7.074572                    | 8.727858                     | 8.789049                                                               |
| 2053 | 17911 | 7.074177                    | 8.727371                     | 8.788561                                                               |
| 2052 | 17909 | 7.073782                    | 8.726884                     | 8.788074                                                               |
| 2051 | 17903 | 7.073387                    | 8.726396                     | 8.787587                                                               |
| 2050 | 17891 | 7.072992                    | 8.725909                     | 8.787099                                                               |
| 2049 | 17881 | 7.072597                    | 8.725421                     | 8.786611                                                               |
| 2048 | 17863 | 7.072201                    | 8.724933                     | 8.786122                                                               |
| 2047 | 17851 | 7.071805                    | 8.724445                     | 8.785634                                                               |
| 2046 | 17839 | 7.071409                    | 8.723956                     | 8.785145                                                               |
| 2045 | 17837 | 7.071013                    | 8.723467                     | 8.784656                                                               |
| 2044 | 17827 | 7.070617                    | 8.722978                     | 8.784167                                                               |
| 2043 | 17807 | 7.070220                    | 8.722489                     | 8.783677                                                               |
| 2042 | 17791 | 7.069823                    | 8.721999                     | 8.783188                                                               |
| 2041 | 17789 | 7.069426                    | 8.721509                     | 8.782698                                                               |
| 2040 | 17783 | 7.069028                    | 8.721018                     | 8.782207                                                               |
| 2039 | 17761 | 7.068631                    | 8.720528                     | 8.781717                                                               |
| 2038 | 17749 | 7.068233                    | 8.720037                     | 8.781226                                                               |
| 2037 | 17747 | 7.067835                    | 8.719546                     | 8.780735                                                               |
| 2036 | 17737 | 7.067436                    | 8.719054                     | 8.780244                                                               |
| 2035 | 17729 | 7.067038                    | 8.718563                     | 8.779753                                                               |
| 2034 | 17713 | 7.066639                    | 8.718071                     | 8.779261                                                               |
| 2033 | 17707 | 7.066240                    | 8.717579                     | 8.778769                                                               |
| 2032 | 17683 | 7.065841                    | 8.717086                     | 8.778277                                                               |
| 2031 | 17681 | 7.065442                    | 8.716593                     | 8.777785                                                               |
| 2030 | 17669 | 7.065042                    | 8.716100                     | 8.777292                                                               |
| 2029 | 17659 | 7.064642                    | 8.715607                     | 8.776799                                                               |
| 2028 | 17657 | 7.064242                    | 8.715114                     | 8.776306                                                               |
| 2027 | 17627 | 7.063842                    | 8.714620                     | 8.775813                                                               |
| 2026 | 17623 | 7.063441                    | 8.714126                     | 8.775319                                                               |
| 2025 | 17609 | 7.063041                    | 8.713631                     | 8.774825                                                               |
| 2024 | 17599 | 7.062640                    | 8.713136                     | 8.774331                                                               |
| 2023 | 17597 | 7.062238                    | 8.712641                     | 8.773837                                                               |
| 2022 | 17581 | 7.061837                    | 8.712146                     | 8.773342                                                               |
| 2021 | 17579 | 7.061435                    | 8.711651                     | 8.772847                                                               |
| 2020 | 17573 | 7.061034                    | 8.711155                     | 8.772352                                                               |
| 2019 | 17569 | 7.060632                    | 8.710659                     | 8.771857                                                               |
| 2018 | 17551 | 7.060230                    | 8.710163                     | 8.771361                                                               |
| 2017 | 17539 | 7.059828                    | 8.709667                     | 8.770865                                                               |
| 2016 | 17519 | 7.059425                    | 8.709171                     | 8.770369                                                               |
| 2015 | 17509 | 7.059022                    | 8.708673                     | 8.769873                                                               |
| 2014 | 17497 | 7.058619                    | 8.708176                     | 8.769377                                                               |
| 2013 | 17491 | 7.058216                    | 8.707678                     | 8.768880                                                               |
| 2012 | 17489 | 7.057812                    | 8.707181                     | 8.768383                                                               |
| 2011 | 17483 | 7.057409                    | 8.706683                     | 8.767885                                                               |

| $k$  | $p_k$ | $\frac{\sigma(N'_k)}{N'_k}$ | $\frac{N'_k}{\varphi(N'_k)}$ | $\frac{e^\gamma}{2} \log \log N'_k + \frac{0.73\dots}{\log \log N'_k}$ |
|------|-------|-----------------------------|------------------------------|------------------------------------------------------------------------|
| 2010 | 17477 | 7.057005                    | 8.706185                     | 8.767388                                                               |
| 2009 | 17471 | 7.056601                    | 8.705687                     | 8.766890                                                               |
| 2008 | 17467 | 7.056198                    | 8.705188                     | 8.766392                                                               |
| 2007 | 17449 | 7.055794                    | 8.704690                     | 8.765893                                                               |
| 2006 | 17443 | 7.055389                    | 8.704191                     | 8.765395                                                               |
| 2005 | 17431 | 7.054985                    | 8.703692                     | 8.764896                                                               |
| 2004 | 17419 | 7.054580                    | 8.703193                     | 8.764397                                                               |
| 2003 | 17417 | 7.054175                    | 8.702693                     | 8.763897                                                               |
| 2002 | 17401 | 7.053770                    | 8.702193                     | 8.763398                                                               |
| 2001 | 17393 | 7.053365                    | 8.701693                     | 8.762898                                                               |
| 2000 | 17389 | 7.052959                    | 8.701193                     | 8.762397                                                               |
| 1999 | 17387 | 7.052554                    | 8.700693                     | 8.761897                                                               |
| 1998 | 17383 | 7.052148                    | 8.700192                     | 8.761396                                                               |
| 1997 | 17377 | 7.051742                    | 8.699692                     | 8.760895                                                               |
| 1996 | 17359 | 7.051337                    | 8.699191                     | 8.760394                                                               |
| 1995 | 17351 | 7.050930                    | 8.698690                     | 8.759893                                                               |
| 1994 | 17341 | 7.050524                    | 8.698189                     | 8.759391                                                               |
| 1993 | 17333 | 7.050118                    | 8.697687                     | 8.758889                                                               |
| 1992 | 17327 | 7.049711                    | 8.697185                     | 8.758387                                                               |
| 1991 | 17321 | 7.049304                    | 8.696683                     | 8.757884                                                               |
| 1990 | 17317 | 7.048897                    | 8.696181                     | 8.757381                                                               |
| 1989 | 17299 | 7.048490                    | 8.695679                     | 8.756878                                                               |
| 1988 | 17293 | 7.048083                    | 8.695176                     | 8.756375                                                               |
| 1987 | 17291 | 7.047675                    | 8.694673                     | 8.755871                                                               |
| 1986 | 17257 | 7.047267                    | 8.694171                     | 8.755368                                                               |
| 1985 | 17239 | 7.046859                    | 8.693667                     | 8.754864                                                               |
| 1984 | 17231 | 7.046450                    | 8.693163                     | 8.754359                                                               |
| 1983 | 17209 | 7.046041                    | 8.692658                     | 8.753855                                                               |
| 1982 | 17207 | 7.045632                    | 8.692153                     | 8.753350                                                               |
| 1981 | 17203 | 7.045223                    | 8.691648                     | 8.752845                                                               |
| 1980 | 17191 | 7.044813                    | 8.691143                     | 8.752340                                                               |
| 1979 | 17189 | 7.044403                    | 8.690637                     | 8.751834                                                               |
| 1978 | 17183 | 7.043993                    | 8.690131                     | 8.751328                                                               |
| 1977 | 17167 | 7.043584                    | 8.689626                     | 8.750822                                                               |
| 1976 | 17159 | 7.043173                    | 8.689119                     | 8.750316                                                               |
| 1975 | 17137 | 7.042763                    | 8.688613                     | 8.749809                                                               |
| 1974 | 17123 | 7.042352                    | 8.688106                     | 8.749302                                                               |
| 1973 | 17117 | 7.041941                    | 8.687599                     | 8.748795                                                               |
| 1972 | 17107 | 7.041529                    | 8.687091                     | 8.748288                                                               |
| 1971 | 17099 | 7.041118                    | 8.686583                     | 8.747780                                                               |
| 1970 | 17093 | 7.040706                    | 8.686075                     | 8.747272                                                               |
| 1969 | 17077 | 7.040294                    | 8.685567                     | 8.746764                                                               |
| 1968 | 17053 | 7.039882                    | 8.685058                     | 8.746256                                                               |
| 1967 | 17047 | 7.039469                    | 8.684549                     | 8.745747                                                               |

| $k$  | $p_k$ | $\frac{\sigma(N'_k)}{N'_k}$ | $\frac{N'_k}{\varphi(N'_k)}$ | $\frac{e^\gamma}{2} \log \log N'_k + \frac{0.73\dots}{\log \log N'_k}$ |
|------|-------|-----------------------------|------------------------------|------------------------------------------------------------------------|
| 1966 | 17041 | 7.039056                    | 8.684040                     | 8.745238                                                               |
| 1965 | 17033 | 7.038643                    | 8.683530                     | 8.744729                                                               |
| 1964 | 17029 | 7.038230                    | 8.683020                     | 8.744220                                                               |
| 1963 | 17027 | 7.037817                    | 8.682510                     | 8.743710                                                               |
| 1962 | 17021 | 7.037403                    | 8.682001                     | 8.743200                                                               |
| 1961 | 17011 | 7.036990                    | 8.681490                     | 8.742690                                                               |
| 1960 | 16993 | 7.036576                    | 8.680980                     | 8.742179                                                               |
| 1959 | 16987 | 7.036162                    | 8.680469                     | 8.741668                                                               |
| 1958 | 16981 | 7.035748                    | 8.679958                     | 8.741157                                                               |
| 1957 | 16979 | 7.035334                    | 8.679447                     | 8.740646                                                               |
| 1956 | 16963 | 7.034919                    | 8.678936                     | 8.740134                                                               |
| 1955 | 16943 | 7.034505                    | 8.678424                     | 8.739622                                                               |
| 1954 | 16937 | 7.034089                    | 8.677912                     | 8.739110                                                               |
| 1953 | 16931 | 7.033674                    | 8.677400                     | 8.738598                                                               |
| 1952 | 16927 | 7.033259                    | 8.676887                     | 8.738085                                                               |
| 1951 | 16921 | 7.032843                    | 8.676375                     | 8.737572                                                               |
| 1950 | 16903 | 7.032428                    | 8.675862                     | 8.737059                                                               |
| 1949 | 16901 | 7.032012                    | 8.675349                     | 8.736545                                                               |
| 1948 | 16889 | 7.031596                    | 8.674835                     | 8.736032                                                               |
| 1947 | 16883 | 7.031179                    | 8.674322                     | 8.735518                                                               |
| 1946 | 16879 | 7.030763                    | 8.673808                     | 8.735003                                                               |
| 1945 | 16871 | 7.030346                    | 8.673294                     | 8.734489                                                               |
| 1944 | 16843 | 7.029930                    | 8.672780                     | 8.733974                                                               |
| 1943 | 16831 | 7.029512                    | 8.672265                     | 8.733459                                                               |
| 1942 | 16829 | 7.029095                    | 8.671750                     | 8.732943                                                               |
| 1941 | 16823 | 7.028677                    | 8.671234                     | 8.732428                                                               |
| 1940 | 16811 | 7.028259                    | 8.670719                     | 8.731912                                                               |
| 1939 | 16787 | 7.027841                    | 8.670203                     | 8.731396                                                               |
| 1938 | 16763 | 7.027423                    | 8.669687                     | 8.730879                                                               |
| 1937 | 16759 | 7.027003                    | 8.669169                     | 8.730362                                                               |
| 1936 | 16747 | 7.026584                    | 8.668652                     | 8.729846                                                               |
| 1935 | 16741 | 7.026164                    | 8.668135                     | 8.729328                                                               |
| 1934 | 16729 | 7.025745                    | 8.667617                     | 8.728811                                                               |
| 1933 | 16703 | 7.025325                    | 8.667099                     | 8.728293                                                               |
| 1932 | 16699 | 7.024904                    | 8.666580                     | 8.727775                                                               |
| 1931 | 16693 | 7.024484                    | 8.666061                     | 8.727257                                                               |
| 1930 | 16691 | 7.024063                    | 8.665542                     | 8.726738                                                               |
| 1929 | 16673 | 7.023642                    | 8.665022                     | 8.726219                                                               |
| 1928 | 16661 | 7.023221                    | 8.664503                     | 8.725700                                                               |
| 1927 | 16657 | 7.022799                    | 8.663983                     | 8.725181                                                               |
| 1926 | 16651 | 7.022378                    | 8.663463                     | 8.724661                                                               |
| 1925 | 16649 | 7.021956                    | 8.662942                     | 8.724141                                                               |
| 1924 | 16633 | 7.021534                    | 8.662422                     | 8.723621                                                               |
| 1923 | 16631 | 7.021112                    | 8.661901                     | 8.723101                                                               |

| $k$  | $p_k$ | $\frac{\sigma(N'_k)}{N'_k}$ | $\frac{N'_k}{\varphi(N'_k)}$ | $\frac{e^\gamma}{2} \log \log N'_k + \frac{0.73\dots}{\log \log N'_k}$ |
|------|-------|-----------------------------|------------------------------|------------------------------------------------------------------------|
| 1922 | 16619 | 7.020690                    | 8.661380                     | 8.722580                                                               |
| 1921 | 16607 | 7.020268                    | 8.660859                     | 8.722059                                                               |
| 1920 | 16603 | 7.019845                    | 8.660338                     | 8.721538                                                               |
| 1919 | 16573 | 7.019422                    | 8.659816                     | 8.721016                                                               |
| 1918 | 16567 | 7.018999                    | 8.659293                     | 8.720494                                                               |
| 1917 | 16561 | 7.018575                    | 8.658771                     | 8.719972                                                               |
| 1916 | 16553 | 7.018151                    | 8.658248                     | 8.719450                                                               |
| 1915 | 16547 | 7.017727                    | 8.657725                     | 8.718927                                                               |
| 1914 | 16529 | 7.017303                    | 8.657202                     | 8.718404                                                               |
| 1913 | 16519 | 7.016879                    | 8.656678                     | 8.717881                                                               |
| 1912 | 16493 | 7.016454                    | 8.656154                     | 8.717357                                                               |
| 1911 | 16487 | 7.016028                    | 8.655629                     | 8.716833                                                               |
| 1910 | 16481 | 7.015603                    | 8.655104                     | 8.716309                                                               |
| 1909 | 16477 | 7.015177                    | 8.654579                     | 8.715785                                                               |
| 1908 | 16453 | 7.014752                    | 8.654054                     | 8.715261                                                               |
| 1907 | 16451 | 7.014325                    | 8.653528                     | 8.714736                                                               |
| 1906 | 16447 | 7.013899                    | 8.653002                     | 8.714211                                                               |
| 1905 | 16433 | 7.013472                    | 8.652476                     | 8.713685                                                               |
| 1904 | 16427 | 7.013046                    | 8.651949                     | 8.713159                                                               |
| 1903 | 16421 | 7.012619                    | 8.651422                     | 8.712633                                                               |
| 1902 | 16417 | 7.012192                    | 8.650895                     | 8.712107                                                               |
| 1901 | 16411 | 7.011765                    | 8.650368                     | 8.711580                                                               |
| 1900 | 16381 | 7.011337                    | 8.649841                     | 8.711054                                                               |
| 1899 | 16369 | 7.010909                    | 8.649313                     | 8.710526                                                               |
| 1898 | 16363 | 7.010481                    | 8.648785                     | 8.709999                                                               |
| 1897 | 16361 | 7.010053                    | 8.648256                     | 8.709471                                                               |
| 1896 | 16349 | 7.009624                    | 8.647728                     | 8.708943                                                               |
| 1895 | 16339 | 7.009196                    | 8.647199                     | 8.708415                                                               |
| 1894 | 16333 | 7.008767                    | 8.646670                     | 8.707887                                                               |
| 1893 | 16319 | 7.008338                    | 8.646140                     | 8.707358                                                               |
| 1892 | 16301 | 7.007908                    | 8.645610                     | 8.706829                                                               |
| 1891 | 16273 | 7.007478                    | 8.645080                     | 8.706299                                                               |
| 1890 | 16267 | 7.007048                    | 8.644549                     | 8.705770                                                               |
| 1889 | 16253 | 7.006617                    | 8.644017                     | 8.705240                                                               |
| 1888 | 16249 | 7.006186                    | 8.643486                     | 8.704710                                                               |
| 1887 | 16231 | 7.005755                    | 8.642954                     | 8.704179                                                               |
| 1886 | 16229 | 7.005323                    | 8.642421                     | 8.703648                                                               |
| 1885 | 16223 | 7.004891                    | 8.641889                     | 8.703117                                                               |
| 1884 | 16217 | 7.004460                    | 8.641356                     | 8.702586                                                               |
| 1883 | 16193 | 7.004028                    | 8.640823                     | 8.702054                                                               |
| 1882 | 16189 | 7.003595                    | 8.640289                     | 8.701523                                                               |
| 1881 | 16187 | 7.003163                    | 8.639756                     | 8.700990                                                               |
| 1880 | 16183 | 7.002730                    | 8.639222                     | 8.700458                                                               |
| 1879 | 16141 | 7.002297                    | 8.638688                     | 8.699925                                                               |

| $k$  | $p_k$ | $\frac{\sigma(N'_k)}{N'_k}$ | $\frac{N'_k}{\varphi(N'_k)}$ | $\frac{e^\gamma}{2} \log \log N'_k + \frac{0.73\dots}{\log \log N'_k}$ |
|------|-------|-----------------------------|------------------------------|------------------------------------------------------------------------|
| 1878 | 16139 | 7.001864                    | 8.638153                     | 8.699392                                                               |
| 1877 | 16127 | 7.001430                    | 8.637618                     | 8.698859                                                               |
| 1876 | 16111 | 7.000996                    | 8.637082                     | 8.698325                                                               |
| 1875 | 16103 | 7.000561                    | 8.636546                     | 8.697791                                                               |
| 1874 | 16097 | 7.000126                    | 8.636010                     | 8.697257                                                               |
| 1873 | 16091 | 6.999692                    | 8.635473                     | 8.696723                                                               |
| 1872 | 16087 | 6.999257                    | 8.634936                     | 8.696188                                                               |
| 1871 | 16073 | 6.998822                    | 8.634400                     | 8.695653                                                               |
| 1870 | 16069 | 6.998386                    | 8.633862                     | 8.695118                                                               |
| 1869 | 16067 | 6.997951                    | 8.633325                     | 8.694582                                                               |
| 1868 | 16063 | 6.997515                    | 8.632788                     | 8.694046                                                               |
| 1867 | 16061 | 6.997080                    | 8.632250                     | 8.693510                                                               |
| 1866 | 16057 | 6.996644                    | 8.631713                     | 8.692973                                                               |
| 1865 | 16033 | 6.996208                    | 8.631175                     | 8.692437                                                               |
| 1864 | 16007 | 6.995772                    | 8.630637                     | 8.691899                                                               |
| 1863 | 16001 | 6.995335                    | 8.630098                     | 8.691362                                                               |
| 1862 | 15991 | 6.994898                    | 8.629559                     | 8.690824                                                               |
| 1861 | 15973 | 6.994460                    | 8.629019                     | 8.690286                                                               |
| 1860 | 15971 | 6.994022                    | 8.628479                     | 8.689748                                                               |
| 1859 | 15959 | 6.993585                    | 8.627938                     | 8.689210                                                               |
| 1858 | 15937 | 6.993146                    | 8.627398                     | 8.688671                                                               |
| 1857 | 15923 | 6.992708                    | 8.626856                     | 8.688132                                                               |
| 1856 | 15919 | 6.992268                    | 8.626315                     | 8.687592                                                               |
| 1855 | 15913 | 6.991829                    | 8.625773                     | 8.687053                                                               |
| 1854 | 15907 | 6.991390                    | 8.625231                     | 8.686513                                                               |
| 1853 | 15901 | 6.990950                    | 8.624688                     | 8.685972                                                               |
| 1852 | 15889 | 6.990511                    | 8.624146                     | 8.685432                                                               |
| 1851 | 15887 | 6.990071                    | 8.623603                     | 8.684891                                                               |
| 1850 | 15881 | 6.989631                    | 8.623060                     | 8.684350                                                               |
| 1849 | 15877 | 6.989191                    | 8.622517                     | 8.683808                                                               |
| 1848 | 15859 | 6.988751                    | 8.621974                     | 8.683266                                                               |
| 1847 | 15823 | 6.988310                    | 8.621431                     | 8.682724                                                               |
| 1846 | 15817 | 6.987868                    | 8.620886                     | 8.682182                                                               |
| 1845 | 15809 | 6.987427                    | 8.620341                     | 8.681639                                                               |
| 1844 | 15803 | 6.986985                    | 8.619796                     | 8.681096                                                               |
| 1843 | 15797 | 6.986542                    | 8.619250                     | 8.680553                                                               |
| 1842 | 15791 | 6.986100                    | 8.618704                     | 8.680009                                                               |
| 1841 | 15787 | 6.985658                    | 8.618159                     | 8.679465                                                               |
| 1840 | 15773 | 6.985215                    | 8.617613                     | 8.678921                                                               |
| 1839 | 15767 | 6.984773                    | 8.617066                     | 8.678377                                                               |
| 1838 | 15761 | 6.984330                    | 8.616520                     | 8.677832                                                               |
| 1837 | 15749 | 6.983886                    | 8.615973                     | 8.677287                                                               |
| 1836 | 15739 | 6.983443                    | 8.615426                     | 8.676741                                                               |
| 1835 | 15737 | 6.982999                    | 8.614879                     | 8.676196                                                               |

| $k$  | $p_k$ | $\frac{\sigma(N'_k)}{N'_k}$ | $\frac{N'_k}{\varphi(N'_k)}$ | $\frac{e^\gamma}{2} \log \log N'_k + \frac{0.73\dots}{\log \log N'_k}$ |
|------|-------|-----------------------------|------------------------------|------------------------------------------------------------------------|
| 1834 | 15733 | 6.982556                    | 8.614331                     | 8.675650                                                               |
| 1833 | 15731 | 6.982112                    | 8.613784                     | 8.675103                                                               |
| 1832 | 15727 | 6.981668                    | 8.613236                     | 8.674557                                                               |
| 1831 | 15683 | 6.981224                    | 8.612689                     | 8.674009                                                               |
| 1830 | 15679 | 6.980779                    | 8.612139                     | 8.673462                                                               |
| 1829 | 15671 | 6.980334                    | 8.611590                     | 8.672915                                                               |
| 1828 | 15667 | 6.979888                    | 8.611041                     | 8.672367                                                               |
| 1827 | 15661 | 6.979443                    | 8.610491                     | 8.671819                                                               |
| 1826 | 15649 | 6.978997                    | 8.609941                     | 8.671270                                                               |
| 1825 | 15647 | 6.978551                    | 8.609391                     | 8.670722                                                               |
| 1824 | 15643 | 6.978105                    | 8.608841                     | 8.670172                                                               |
| 1823 | 15641 | 6.977659                    | 8.608290                     | 8.669623                                                               |
| 1822 | 15629 | 6.977213                    | 8.607740                     | 8.669073                                                               |
| 1821 | 15619 | 6.976767                    | 8.607189                     | 8.668523                                                               |
| 1820 | 15607 | 6.976320                    | 8.606638                     | 8.667973                                                               |
| 1819 | 15601 | 6.975873                    | 8.606087                     | 8.667422                                                               |
| 1818 | 15583 | 6.975426                    | 8.605535                     | 8.666871                                                               |
| 1817 | 15581 | 6.974979                    | 8.604983                     | 8.666320                                                               |
| 1816 | 15569 | 6.974531                    | 8.604431                     | 8.665768                                                               |
| 1815 | 15559 | 6.974083                    | 8.603878                     | 8.665216                                                               |
| 1814 | 15551 | 6.973635                    | 8.603325                     | 8.664664                                                               |
| 1813 | 15541 | 6.973186                    | 8.602772                     | 8.664112                                                               |
| 1812 | 15527 | 6.972738                    | 8.602218                     | 8.663559                                                               |
| 1811 | 15511 | 6.972289                    | 8.601664                     | 8.663006                                                               |
| 1810 | 15497 | 6.971839                    | 8.601110                     | 8.662452                                                               |
| 1809 | 15493 | 6.971389                    | 8.600555                     | 8.661898                                                               |
| 1808 | 15473 | 6.970939                    | 8.599999                     | 8.661344                                                               |
| 1807 | 15467 | 6.970489                    | 8.599444                     | 8.660790                                                               |
| 1806 | 15461 | 6.970038                    | 8.598888                     | 8.660235                                                               |
| 1805 | 15451 | 6.969587                    | 8.598331                     | 8.659680                                                               |
| 1804 | 15443 | 6.969136                    | 8.597775                     | 8.659125                                                               |
| 1803 | 15439 | 6.968685                    | 8.597218                     | 8.658570                                                               |
| 1802 | 15427 | 6.968234                    | 8.596661                     | 8.658014                                                               |
| 1801 | 15413 | 6.967782                    | 8.596104                     | 8.657457                                                               |
| 1800 | 15401 | 6.967330                    | 8.595546                     | 8.656901                                                               |
| 1799 | 15391 | 6.966878                    | 8.594988                     | 8.656344                                                               |
| 1798 | 15383 | 6.966425                    | 8.594430                     | 8.655787                                                               |
| 1797 | 15377 | 6.965972                    | 8.593871                     | 8.655229                                                               |
| 1796 | 15373 | 6.965519                    | 8.593312                     | 8.654672                                                               |
| 1795 | 15361 | 6.965066                    | 8.592753                     | 8.654113                                                               |
| 1794 | 15359 | 6.964613                    | 8.592194                     | 8.653555                                                               |
| 1793 | 15349 | 6.964159                    | 8.591634                     | 8.652996                                                               |
| 1792 | 15331 | 6.963706                    | 8.591075                     | 8.652437                                                               |
| 1791 | 15329 | 6.963251                    | 8.590514                     | 8.651878                                                               |

| $k$  | $p_k$ | $\frac{\sigma(N'_k)}{N'_k}$ | $\frac{N'_k}{\varphi(N'_k)}$ | $\frac{e^\gamma}{2} \log \log N'_k + \frac{0.73\dots}{\log \log N'_k}$ |
|------|-------|-----------------------------|------------------------------|------------------------------------------------------------------------|
| 1790 | 15319 | 6.962797                    | 8.589954                     | 8.651318                                                               |
| 1789 | 15313 | 6.962343                    | 8.589393                     | 8.650758                                                               |
| 1788 | 15307 | 6.961888                    | 8.588832                     | 8.650197                                                               |
| 1787 | 15299 | 6.961433                    | 8.588271                     | 8.649637                                                               |
| 1786 | 15289 | 6.960978                    | 8.587710                     | 8.649076                                                               |
| 1785 | 15287 | 6.960523                    | 8.587148                     | 8.648514                                                               |
| 1784 | 15277 | 6.960068                    | 8.586586                     | 8.647953                                                               |
| 1783 | 15271 | 6.959612                    | 8.586024                     | 8.647391                                                               |
| 1782 | 15269 | 6.959157                    | 8.585462                     | 8.646828                                                               |
| 1781 | 15263 | 6.958701                    | 8.584900                     | 8.646265                                                               |
| 1780 | 15259 | 6.958245                    | 8.584337                     | 8.645702                                                               |
| 1779 | 15241 | 6.957789                    | 8.583775                     | 8.645139                                                               |
| 1778 | 15233 | 6.957332                    | 8.583212                     | 8.644575                                                               |
| 1777 | 15227 | 6.956876                    | 8.582648                     | 8.644011                                                               |
| 1776 | 15217 | 6.956419                    | 8.582084                     | 8.643447                                                               |
| 1775 | 15199 | 6.955962                    | 8.581520                     | 8.642882                                                               |
| 1774 | 15193 | 6.955504                    | 8.580956                     | 8.642317                                                               |
| 1773 | 15187 | 6.955046                    | 8.580391                     | 8.641752                                                               |
| 1772 | 15173 | 6.954588                    | 8.579826                     | 8.641186                                                               |
| 1771 | 15161 | 6.954130                    | 8.579261                     | 8.640620                                                               |
| 1770 | 15149 | 6.953671                    | 8.578695                     | 8.640054                                                               |
| 1769 | 15139 | 6.953212                    | 8.578128                     | 8.639487                                                               |
| 1768 | 15137 | 6.952753                    | 8.577562                     | 8.638921                                                               |
| 1767 | 15131 | 6.952294                    | 8.576995                     | 8.638353                                                               |
| 1766 | 15121 | 6.951834                    | 8.576428                     | 8.637786                                                               |
| 1765 | 15107 | 6.951375                    | 8.575861                     | 8.637218                                                               |
| 1764 | 15101 | 6.950915                    | 8.575293                     | 8.636650                                                               |
| 1763 | 15091 | 6.950454                    | 8.574726                     | 8.636081                                                               |
| 1762 | 15083 | 6.949994                    | 8.574157                     | 8.635512                                                               |
| 1761 | 15077 | 6.949533                    | 8.573589                     | 8.634943                                                               |
| 1760 | 15073 | 6.949072                    | 8.573020                     | 8.634373                                                               |
| 1759 | 15061 | 6.948611                    | 8.572452                     | 8.633803                                                               |
| 1758 | 15053 | 6.948150                    | 8.571882                     | 8.633233                                                               |
| 1757 | 15031 | 6.947688                    | 8.571313                     | 8.632662                                                               |
| 1756 | 15017 | 6.947226                    | 8.570743                     | 8.632091                                                               |
| 1755 | 15013 | 6.946764                    | 8.570172                     | 8.631520                                                               |
| 1754 | 14983 | 6.946301                    | 8.569601                     | 8.630949                                                               |
| 1753 | 14969 | 6.945837                    | 8.569029                     | 8.630377                                                               |
| 1752 | 14957 | 6.945373                    | 8.568457                     | 8.629805                                                               |
| 1751 | 14951 | 6.944909                    | 8.567884                     | 8.629232                                                               |
| 1750 | 14947 | 6.944444                    | 8.567311                     | 8.628660                                                               |
| 1749 | 14939 | 6.943980                    | 8.566738                     | 8.628086                                                               |
| 1748 | 14929 | 6.943515                    | 8.566164                     | 8.627513                                                               |
| 1747 | 14923 | 6.943050                    | 8.565590                     | 8.626939                                                               |

| $k$  | $p_k$ | $\frac{\sigma(N'_k)}{N'_k}$ | $\frac{N'_k}{\varphi(N'_k)}$ | $\frac{e^\gamma}{2} \log \log N'_k + \frac{0.73\dots}{\log \log N'_k}$ |
|------|-------|-----------------------------|------------------------------|------------------------------------------------------------------------|
| 1746 | 14897 | 6.942585                    | 8.565016                     | 8.626365                                                               |
| 1745 | 14891 | 6.942119                    | 8.564441                     | 8.625791                                                               |
| 1744 | 14887 | 6.941653                    | 8.563866                     | 8.625216                                                               |
| 1743 | 14879 | 6.941186                    | 8.563291                     | 8.624641                                                               |
| 1742 | 14869 | 6.940720                    | 8.562715                     | 8.624065                                                               |
| 1741 | 14867 | 6.940253                    | 8.562140                     | 8.623489                                                               |
| 1740 | 14851 | 6.939786                    | 8.561564                     | 8.622913                                                               |
| 1739 | 14843 | 6.939319                    | 8.560987                     | 8.622337                                                               |
| 1738 | 14831 | 6.938852                    | 8.560410                     | 8.621760                                                               |
| 1737 | 14827 | 6.938384                    | 8.559833                     | 8.621183                                                               |
| 1736 | 14821 | 6.937916                    | 8.559256                     | 8.620605                                                               |
| 1735 | 14813 | 6.937448                    | 8.558678                     | 8.620027                                                               |
| 1734 | 14797 | 6.936979                    | 8.558101                     | 8.619449                                                               |
| 1733 | 14783 | 6.936511                    | 8.557522                     | 8.618871                                                               |
| 1732 | 14779 | 6.936041                    | 8.556943                     | 8.618292                                                               |
| 1731 | 14771 | 6.935572                    | 8.556364                     | 8.617712                                                               |
| 1730 | 14767 | 6.935103                    | 8.555785                     | 8.617133                                                               |
| 1729 | 14759 | 6.934633                    | 8.555206                     | 8.616553                                                               |
| 1728 | 14753 | 6.934163                    | 8.554626                     | 8.615973                                                               |
| 1727 | 14747 | 6.933693                    | 8.554046                     | 8.615392                                                               |
| 1726 | 14741 | 6.933223                    | 8.553466                     | 8.614811                                                               |
| 1725 | 14737 | 6.932753                    | 8.552886                     | 8.614230                                                               |
| 1724 | 14731 | 6.932282                    | 8.552305                     | 8.613648                                                               |
| 1723 | 14723 | 6.931812                    | 8.551725                     | 8.613066                                                               |
| 1722 | 14717 | 6.931341                    | 8.551144                     | 8.612484                                                               |
| 1721 | 14713 | 6.930870                    | 8.550563                     | 8.611901                                                               |
| 1720 | 14699 | 6.930399                    | 8.549982                     | 8.611318                                                               |
| 1719 | 14683 | 6.929928                    | 8.549400                     | 8.610734                                                               |
| 1718 | 14669 | 6.929456                    | 8.548818                     | 8.610150                                                               |
| 1717 | 14657 | 6.928983                    | 8.548235                     | 8.609566                                                               |
| 1716 | 14653 | 6.928511                    | 8.547652                     | 8.608982                                                               |
| 1715 | 14639 | 6.928038                    | 8.547069                     | 8.608397                                                               |
| 1714 | 14633 | 6.927565                    | 8.546485                     | 8.607812                                                               |
| 1713 | 14629 | 6.927091                    | 8.545901                     | 8.607226                                                               |
| 1712 | 14627 | 6.926618                    | 8.545317                     | 8.606640                                                               |
| 1711 | 14621 | 6.926144                    | 8.544732                     | 8.606054                                                               |
| 1710 | 14593 | 6.925671                    | 8.544148                     | 8.605467                                                               |
| 1709 | 14591 | 6.925196                    | 8.543562                     | 8.604880                                                               |
| 1708 | 14563 | 6.924721                    | 8.542977                     | 8.604293                                                               |
| 1707 | 14561 | 6.924246                    | 8.542390                     | 8.603706                                                               |
| 1706 | 14557 | 6.923770                    | 8.541804                     | 8.603118                                                               |
| 1705 | 14551 | 6.923295                    | 8.541217                     | 8.602529                                                               |
| 1704 | 14549 | 6.922819                    | 8.540630                     | 8.601941                                                               |
| 1703 | 14543 | 6.922343                    | 8.540043                     | 8.601352                                                               |



| $k$  | $p_k$ | $\frac{\sigma(N'_k)}{N'_k}$ | $\frac{N'_k}{\varphi(N'_k)}$ | $\frac{e^\gamma}{2} \log \log N'_k + \frac{0.73\dots}{\log \log N'_k}$ |
|------|-------|-----------------------------|------------------------------|------------------------------------------------------------------------|
| 1702 | 14537 | 6.921867                    | 8.539456                     | 8.600762                                                               |
| 1701 | 14533 | 6.921391                    | 8.538868                     | 8.600172                                                               |
| 1700 | 14519 | 6.920915                    | 8.538281                     | 8.599582                                                               |
| 1699 | 14503 | 6.920438                    | 8.537692                     | 8.598992                                                               |
| 1698 | 14489 | 6.919961                    | 8.537104                     | 8.598401                                                               |
| 1697 | 14479 | 6.919484                    | 8.536515                     | 8.597810                                                               |
| 1696 | 14461 | 6.919006                    | 8.535925                     | 8.597218                                                               |
| 1695 | 14449 | 6.918527                    | 8.535335                     | 8.596626                                                               |
| 1694 | 14447 | 6.918049                    | 8.534744                     | 8.596034                                                               |
| 1693 | 14437 | 6.917570                    | 8.534153                     | 8.595441                                                               |
| 1692 | 14431 | 6.917091                    | 8.533562                     | 8.594849                                                               |
| 1691 | 14423 | 6.916611                    | 8.532971                     | 8.594255                                                               |
| 1690 | 14419 | 6.916132                    | 8.532379                     | 8.593662                                                               |
| 1689 | 14411 | 6.915652                    | 8.531787                     | 8.593068                                                               |
| 1688 | 14407 | 6.915172                    | 8.531195                     | 8.592473                                                               |
| 1687 | 14401 | 6.914692                    | 8.530603                     | 8.591878                                                               |
| 1686 | 14389 | 6.914212                    | 8.530011                     | 8.591283                                                               |
| 1685 | 14387 | 6.913732                    | 8.529418                     | 8.590688                                                               |
| 1684 | 14369 | 6.913251                    | 8.528825                     | 8.590092                                                               |
| 1683 | 14347 | 6.912770                    | 8.528232                     | 8.589495                                                               |
| 1682 | 14341 | 6.912288                    | 8.527637                     | 8.588899                                                               |
| 1681 | 14327 | 6.911806                    | 8.527043                     | 8.588302                                                               |
| 1680 | 14323 | 6.911324                    | 8.526447                     | 8.587705                                                               |
| 1679 | 14321 | 6.910841                    | 8.525852                     | 8.587107                                                               |
| 1678 | 14303 | 6.910359                    | 8.525257                     | 8.586509                                                               |
| 1677 | 14293 | 6.909876                    | 8.524661                     | 8.585911                                                               |
| 1676 | 14281 | 6.909392                    | 8.524064                     | 8.585312                                                               |
| 1675 | 14251 | 6.908909                    | 8.523467                     | 8.584713                                                               |
| 1674 | 14249 | 6.908424                    | 8.522869                     | 8.584113                                                               |
| 1673 | 14243 | 6.907939                    | 8.522271                     | 8.583514                                                               |
| 1672 | 14221 | 6.907454                    | 8.521673                     | 8.582913                                                               |
| 1671 | 14207 | 6.906968                    | 8.521074                     | 8.582313                                                               |
| 1670 | 14197 | 6.906482                    | 8.520474                     | 8.581712                                                               |
| 1669 | 14177 | 6.905996                    | 8.519874                     | 8.581111                                                               |
| 1668 | 14173 | 6.905509                    | 8.519273                     | 8.580510                                                               |
| 1667 | 14159 | 6.905022                    | 8.518672                     | 8.579908                                                               |
| 1666 | 14153 | 6.904534                    | 8.518070                     | 8.579305                                                               |
| 1665 | 14149 | 6.904046                    | 8.517468                     | 8.578703                                                               |
| 1664 | 14143 | 6.903558                    | 8.516866                     | 8.578100                                                               |
| 1663 | 14107 | 6.903070                    | 8.516264                     | 8.577496                                                               |
| 1662 | 14087 | 6.902581                    | 8.515660                     | 8.576893                                                               |
| 1661 | 14083 | 6.902091                    | 8.515056                     | 8.576289                                                               |
| 1660 | 14081 | 6.901601                    | 8.514451                     | 8.575684                                                               |
| 1659 | 14071 | 6.901111                    | 8.513846                     | 8.575080                                                               |

| $k$  | $p_k$ | $\frac{\sigma(N'_k)}{N'_k}$ | $\frac{N'_k}{\varphi(N'_k)}$ | $\frac{e^\gamma}{2} \log \log N'_k + \frac{0.73\dots}{\log \log N'_k}$ |
|------|-------|-----------------------------|------------------------------|------------------------------------------------------------------------|
| 1658 | 14057 | 6.900620                    | 8.513241                     | 8.574475                                                               |
| 1657 | 14051 | 6.900129                    | 8.512636                     | 8.573869                                                               |
| 1656 | 14033 | 6.899638                    | 8.512030                     | 8.573263                                                               |
| 1655 | 14029 | 6.899147                    | 8.511423                     | 8.572657                                                               |
| 1654 | 14011 | 6.898655                    | 8.510817                     | 8.572050                                                               |
| 1653 | 14009 | 6.898163                    | 8.510209                     | 8.571443                                                               |
| 1652 | 13999 | 6.897670                    | 8.509602                     | 8.570836                                                               |
| 1651 | 13997 | 6.897178                    | 8.508994                     | 8.570228                                                               |
| 1650 | 13967 | 6.896685                    | 8.508386                     | 8.569620                                                               |
| 1649 | 13963 | 6.896191                    | 8.507777                     | 8.569012                                                               |
| 1648 | 13933 | 6.895697                    | 8.507167                     | 8.568403                                                               |
| 1647 | 13931 | 6.895202                    | 8.506557                     | 8.567794                                                               |
| 1646 | 13921 | 6.894707                    | 8.505946                     | 8.567185                                                               |
| 1645 | 13913 | 6.894212                    | 8.505335                     | 8.566575                                                               |
| 1644 | 13907 | 6.893717                    | 8.504724                     | 8.565964                                                               |
| 1643 | 13903 | 6.893221                    | 8.504112                     | 8.565354                                                               |
| 1642 | 13901 | 6.892725                    | 8.503501                     | 8.564743                                                               |
| 1641 | 13883 | 6.892229                    | 8.502889                     | 8.564131                                                               |
| 1640 | 13879 | 6.891733                    | 8.502277                     | 8.563519                                                               |
| 1639 | 13877 | 6.891236                    | 8.501664                     | 8.562907                                                               |
| 1638 | 13873 | 6.890740                    | 8.501051                     | 8.562295                                                               |
| 1637 | 13859 | 6.890243                    | 8.500438                     | 8.561682                                                               |
| 1636 | 13841 | 6.889746                    | 8.499825                     | 8.561068                                                               |
| 1635 | 13831 | 6.889248                    | 8.499211                     | 8.560454                                                               |
| 1634 | 13829 | 6.888750                    | 8.498597                     | 8.559840                                                               |
| 1633 | 13807 | 6.888252                    | 8.497982                     | 8.559226                                                               |
| 1632 | 13799 | 6.887753                    | 8.497366                     | 8.558611                                                               |
| 1631 | 13789 | 6.887254                    | 8.496751                     | 8.557996                                                               |
| 1630 | 13781 | 6.886755                    | 8.496134                     | 8.557380                                                               |
| 1629 | 13763 | 6.886255                    | 8.495518                     | 8.556764                                                               |
| 1628 | 13759 | 6.885755                    | 8.494901                     | 8.556148                                                               |
| 1627 | 13757 | 6.885254                    | 8.494283                     | 8.555531                                                               |
| 1626 | 13751 | 6.884754                    | 8.493666                     | 8.554914                                                               |
| 1625 | 13729 | 6.884253                    | 8.493048                     | 8.554296                                                               |
| 1624 | 13723 | 6.883752                    | 8.492430                     | 8.553678                                                               |
| 1623 | 13721 | 6.883250                    | 8.491811                     | 8.553060                                                               |
| 1622 | 13711 | 6.882749                    | 8.491192                     | 8.552441                                                               |
| 1621 | 13709 | 6.882247                    | 8.490573                     | 8.551822                                                               |
| 1620 | 13697 | 6.881745                    | 8.489953                     | 8.551202                                                               |
| 1619 | 13693 | 6.881242                    | 8.489333                     | 8.550582                                                               |
| 1618 | 13691 | 6.880740                    | 8.488713                     | 8.549962                                                               |
| 1617 | 13687 | 6.880237                    | 8.488093                     | 8.549341                                                               |
| 1616 | 13681 | 6.879735                    | 8.487473                     | 8.548720                                                               |
| 1615 | 13679 | 6.879232                    | 8.486853                     | 8.548098                                                               |

| $k$  | $p_k$ | $\frac{\sigma(N'_k)}{N'_k}$ | $\frac{N'_k}{\varphi(N'_k)}$ | $\frac{e^\gamma}{2} \log \log N'_k + \frac{0.73\dots}{\log \log N'_k}$ |
|------|-------|-----------------------------|------------------------------|------------------------------------------------------------------------|
| 1614 | 13669 | 6.878729                    | 8.486232                     | 8.547476                                                               |
| 1613 | 13649 | 6.878226                    | 8.485612                     | 8.546854                                                               |
| 1612 | 13633 | 6.877722                    | 8.484990                     | 8.546231                                                               |
| 1611 | 13627 | 6.877217                    | 8.484367                     | 8.545608                                                               |
| 1610 | 13619 | 6.876713                    | 8.483745                     | 8.544984                                                               |
| 1609 | 13613 | 6.876208                    | 8.483122                     | 8.544360                                                               |
| 1608 | 13597 | 6.875703                    | 8.482499                     | 8.543736                                                               |
| 1607 | 13591 | 6.875197                    | 8.481875                     | 8.543111                                                               |
| 1606 | 13577 | 6.874691                    | 8.481251                     | 8.542486                                                               |
| 1605 | 13567 | 6.874185                    | 8.480626                     | 8.541861                                                               |
| 1604 | 13553 | 6.873678                    | 8.480001                     | 8.541235                                                               |
| 1603 | 13537 | 6.873171                    | 8.479375                     | 8.540608                                                               |
| 1602 | 13523 | 6.872664                    | 8.478749                     | 8.539982                                                               |
| 1601 | 13513 | 6.872155                    | 8.478122                     | 8.539355                                                               |
| 1600 | 13499 | 6.871647                    | 8.477495                     | 8.538727                                                               |
| 1599 | 13487 | 6.871138                    | 8.476867                     | 8.538100                                                               |
| 1598 | 13477 | 6.870628                    | 8.476238                     | 8.537471                                                               |
| 1597 | 13469 | 6.870119                    | 8.475609                     | 8.536843                                                               |
| 1596 | 13463 | 6.869609                    | 8.474980                     | 8.536214                                                               |
| 1595 | 13457 | 6.869098                    | 8.474350                     | 8.535584                                                               |
| 1594 | 13451 | 6.868588                    | 8.473721                     | 8.534955                                                               |
| 1593 | 13441 | 6.868077                    | 8.473091                     | 8.534324                                                               |
| 1592 | 13421 | 6.867566                    | 8.472460                     | 8.533694                                                               |
| 1591 | 13417 | 6.867055                    | 8.471829                     | 8.533063                                                               |
| 1590 | 13411 | 6.866543                    | 8.471198                     | 8.532431                                                               |
| 1589 | 13399 | 6.866031                    | 8.470566                     | 8.531799                                                               |
| 1588 | 13397 | 6.865519                    | 8.469934                     | 8.531167                                                               |
| 1587 | 13381 | 6.865006                    | 8.469301                     | 8.530534                                                               |
| 1586 | 13367 | 6.864493                    | 8.468669                     | 8.529901                                                               |
| 1585 | 13339 | 6.863980                    | 8.468035                     | 8.529268                                                               |
| 1584 | 13337 | 6.863465                    | 8.467400                     | 8.528634                                                               |
| 1583 | 13331 | 6.862951                    | 8.466765                     | 8.528000                                                               |
| 1582 | 13327 | 6.862436                    | 8.466130                     | 8.527365                                                               |
| 1581 | 13313 | 6.861921                    | 8.465495                     | 8.526730                                                               |
| 1580 | 13309 | 6.861406                    | 8.464859                     | 8.526095                                                               |
| 1579 | 13297 | 6.860890                    | 8.464223                     | 8.525459                                                               |
| 1578 | 13291 | 6.860374                    | 8.463586                     | 8.524823                                                               |
| 1577 | 13267 | 6.859858                    | 8.462950                     | 8.524186                                                               |
| 1576 | 13259 | 6.859341                    | 8.462312                     | 8.523549                                                               |
| 1575 | 13249 | 6.858824                    | 8.461673                     | 8.522911                                                               |
| 1574 | 13241 | 6.858306                    | 8.461035                     | 8.522274                                                               |
| 1573 | 13229 | 6.857788                    | 8.460396                     | 8.521635                                                               |
| 1572 | 13219 | 6.857270                    | 8.459756                     | 8.520997                                                               |
| 1571 | 13217 | 6.856751                    | 8.459116                     | 8.520357                                                               |

| $k$  | $p_k$ | $\frac{\sigma(N'_k)}{N'_k}$ | $\frac{N'_k}{\varphi(N'_k)}$ | $\frac{e^\gamma}{2} \log \log N'_k + \frac{0.73\dots}{\log \log N'_k}$ |
|------|-------|-----------------------------|------------------------------|------------------------------------------------------------------------|
| 1570 | 13187 | 6.856232                    | 8.458476                     | 8.519718                                                               |
| 1569 | 13183 | 6.855712                    | 8.457835                     | 8.519078                                                               |
| 1568 | 13177 | 6.855192                    | 8.457193                     | 8.518438                                                               |
| 1567 | 13171 | 6.854672                    | 8.456551                     | 8.517797                                                               |
| 1566 | 13163 | 6.854152                    | 8.455909                     | 8.517156                                                               |
| 1565 | 13159 | 6.853631                    | 8.455267                     | 8.516514                                                               |
| 1564 | 13151 | 6.853110                    | 8.454624                     | 8.515872                                                               |
| 1563 | 13147 | 6.852589                    | 8.453982                     | 8.515230                                                               |
| 1562 | 13127 | 6.852068                    | 8.453339                     | 8.514587                                                               |
| 1561 | 13121 | 6.851546                    | 8.452695                     | 8.513943                                                               |
| 1560 | 13109 | 6.851024                    | 8.452050                     | 8.513300                                                               |
| 1559 | 13103 | 6.850501                    | 8.451406                     | 8.512656                                                               |
| 1558 | 13099 | 6.849979                    | 8.450761                     | 8.512011                                                               |
| 1557 | 13093 | 6.849456                    | 8.450115                     | 8.511366                                                               |
| 1556 | 13063 | 6.848933                    | 8.449470                     | 8.510721                                                               |
| 1555 | 13049 | 6.848408                    | 8.448823                     | 8.510075                                                               |
| 1554 | 13043 | 6.847884                    | 8.448176                     | 8.509429                                                               |
| 1553 | 13037 | 6.847359                    | 8.447528                     | 8.508782                                                               |
| 1552 | 13033 | 6.846833                    | 8.446880                     | 8.508135                                                               |
| 1551 | 13009 | 6.846308                    | 8.446232                     | 8.507487                                                               |
| 1550 | 13007 | 6.845782                    | 8.445583                     | 8.506840                                                               |
| 1549 | 13003 | 6.845256                    | 8.444933                     | 8.506191                                                               |
| 1548 | 13001 | 6.844729                    | 8.444284                     | 8.505542                                                               |
| 1547 | 12983 | 6.844203                    | 8.443634                     | 8.504893                                                               |
| 1546 | 12979 | 6.843676                    | 8.442984                     | 8.504244                                                               |
| 1545 | 12973 | 6.843148                    | 8.442334                     | 8.503593                                                               |
| 1544 | 12967 | 6.842621                    | 8.441683                     | 8.502943                                                               |
| 1543 | 12959 | 6.842093                    | 8.441032                     | 8.502292                                                               |
| 1542 | 12953 | 6.841565                    | 8.440380                     | 8.501641                                                               |
| 1541 | 12941 | 6.841037                    | 8.439729                     | 8.500989                                                               |
| 1540 | 12923 | 6.840509                    | 8.439077                     | 8.500336                                                               |
| 1539 | 12919 | 6.839979                    | 8.438424                     | 8.499684                                                               |
| 1538 | 12917 | 6.839450                    | 8.437770                     | 8.499031                                                               |
| 1537 | 12911 | 6.838920                    | 8.437117                     | 8.498377                                                               |
| 1536 | 12907 | 6.838391                    | 8.436464                     | 8.497723                                                               |
| 1535 | 12899 | 6.837861                    | 8.435810                     | 8.497068                                                               |
| 1534 | 12893 | 6.837331                    | 8.435156                     | 8.496413                                                               |
| 1533 | 12889 | 6.836801                    | 8.434502                     | 8.495758                                                               |
| 1532 | 12853 | 6.836270                    | 8.433847                     | 8.495102                                                               |
| 1531 | 12841 | 6.835738                    | 8.433191                     | 8.494446                                                               |
| 1530 | 12829 | 6.835206                    | 8.432535                     | 8.493789                                                               |
| 1529 | 12823 | 6.834673                    | 8.431877                     | 8.493132                                                               |
| 1528 | 12821 | 6.834140                    | 8.431220                     | 8.492475                                                               |
| 1527 | 12809 | 6.833607                    | 8.430562                     | 8.491817                                                               |

| $k$  | $p_k$ | $\frac{\sigma(N'_k)}{N'_k}$ | $\frac{N'_k}{\varphi(N'_k)}$ | $\frac{e^\gamma}{2} \log \log N'_k + \frac{0.73\dots}{\log \log N'_k}$ |
|------|-------|-----------------------------|------------------------------|------------------------------------------------------------------------|
| 1526 | 12799 | 6.833074                    | 8.429904                     | 8.491159                                                               |
| 1525 | 12791 | 6.832540                    | 8.429245                     | 8.490500                                                               |
| 1524 | 12781 | 6.832006                    | 8.428586                     | 8.489841                                                               |
| 1523 | 12763 | 6.831472                    | 8.427927                     | 8.489181                                                               |
| 1522 | 12757 | 6.830936                    | 8.427266                     | 8.488521                                                               |
| 1521 | 12743 | 6.830401                    | 8.426606                     | 8.487860                                                               |
| 1520 | 12739 | 6.829865                    | 8.425945                     | 8.487199                                                               |
| 1519 | 12721 | 6.829329                    | 8.425283                     | 8.486538                                                               |
| 1518 | 12713 | 6.828792                    | 8.424621                     | 8.485876                                                               |
| 1517 | 12703 | 6.828255                    | 8.423958                     | 8.485214                                                               |
| 1516 | 12697 | 6.827717                    | 8.423295                     | 8.484551                                                               |
| 1515 | 12689 | 6.827180                    | 8.422632                     | 8.483888                                                               |
| 1514 | 12671 | 6.826642                    | 8.421968                     | 8.483224                                                               |
| 1513 | 12659 | 6.826103                    | 8.421303                     | 8.482560                                                               |
| 1512 | 12653 | 6.825564                    | 8.420638                     | 8.481896                                                               |
| 1511 | 12647 | 6.825024                    | 8.419972                     | 8.481231                                                               |
| 1510 | 12641 | 6.824485                    | 8.419307                     | 8.480565                                                               |
| 1509 | 12637 | 6.823945                    | 8.418641                     | 8.479899                                                               |
| 1508 | 12619 | 6.823405                    | 8.417974                     | 8.479233                                                               |
| 1507 | 12613 | 6.822864                    | 8.417307                     | 8.478566                                                               |
| 1506 | 12611 | 6.822323                    | 8.416640                     | 8.477899                                                               |
| 1505 | 12601 | 6.821783                    | 8.415973                     | 8.477231                                                               |
| 1504 | 12589 | 6.821241                    | 8.415305                     | 8.476563                                                               |
| 1503 | 12583 | 6.820699                    | 8.414636                     | 8.475895                                                               |
| 1502 | 12577 | 6.820157                    | 8.413968                     | 8.475225                                                               |
| 1501 | 12569 | 6.819615                    | 8.413299                     | 8.474556                                                               |
| 1500 | 12553 | 6.819073                    | 8.412629                     | 8.473886                                                               |
| 1499 | 12547 | 6.818529                    | 8.411959                     | 8.473215                                                               |
| 1498 | 12541 | 6.817986                    | 8.411289                     | 8.472545                                                               |
| 1497 | 12539 | 6.817442                    | 8.410618                     | 8.471873                                                               |
| 1496 | 12527 | 6.816899                    | 8.409947                     | 8.471201                                                               |
| 1495 | 12517 | 6.816355                    | 8.409276                     | 8.470529                                                               |
| 1494 | 12511 | 6.815810                    | 8.408604                     | 8.469856                                                               |
| 1493 | 12503 | 6.815265                    | 8.407932                     | 8.469183                                                               |
| 1492 | 12497 | 6.814720                    | 8.407259                     | 8.468509                                                               |
| 1491 | 12491 | 6.814175                    | 8.406587                     | 8.467835                                                               |
| 1490 | 12487 | 6.813630                    | 8.405914                     | 8.467160                                                               |
| 1489 | 12479 | 6.813084                    | 8.405240                     | 8.466485                                                               |
| 1488 | 12473 | 6.812538                    | 8.404567                     | 8.465809                                                               |
| 1487 | 12457 | 6.811992                    | 8.403893                     | 8.465133                                                               |
| 1486 | 12451 | 6.811445                    | 8.403218                     | 8.464457                                                               |
| 1485 | 12437 | 6.810898                    | 8.402544                     | 8.463780                                                               |
| 1484 | 12433 | 6.810350                    | 8.401868                     | 8.463102                                                               |
| 1483 | 12421 | 6.809803                    | 8.401192                     | 8.462424                                                               |

| $k$  | $p_k$ | $\frac{\sigma(N'_k)}{N'_k}$ | $\frac{N'_k}{\varphi(N'_k)}$ | $\frac{e^\gamma}{2} \log \log N'_k + \frac{0.73\dots}{\log \log N'_k}$ |
|------|-------|-----------------------------|------------------------------|------------------------------------------------------------------------|
| 1482 | 12413 | 6.809255                    | 8.400516                     | 8.461746                                                               |
| 1481 | 12409 | 6.808706                    | 8.399839                     | 8.461067                                                               |
| 1480 | 12401 | 6.808157                    | 8.399162                     | 8.460388                                                               |
| 1479 | 12391 | 6.807608                    | 8.398485                     | 8.459708                                                               |
| 1478 | 12379 | 6.807059                    | 8.397807                     | 8.459027                                                               |
| 1477 | 12377 | 6.806509                    | 8.397129                     | 8.458347                                                               |
| 1476 | 12373 | 6.805959                    | 8.396450                     | 8.457665                                                               |
| 1475 | 12347 | 6.805409                    | 8.395772                     | 8.456983                                                               |
| 1474 | 12343 | 6.804858                    | 8.395092                     | 8.456301                                                               |
| 1473 | 12329 | 6.804307                    | 8.394411                     | 8.455619                                                               |
| 1472 | 12323 | 6.803755                    | 8.393731                     | 8.454935                                                               |
| 1471 | 12301 | 6.803203                    | 8.393049                     | 8.454252                                                               |
| 1470 | 12289 | 6.802650                    | 8.392367                     | 8.453568                                                               |
| 1469 | 12281 | 6.802096                    | 8.391684                     | 8.452883                                                               |
| 1468 | 12277 | 6.801543                    | 8.391001                     | 8.452198                                                               |
| 1467 | 12269 | 6.800989                    | 8.390317                     | 8.451513                                                               |
| 1466 | 12263 | 6.800434                    | 8.389634                     | 8.450827                                                               |
| 1465 | 12253 | 6.799880                    | 8.388949                     | 8.450141                                                               |
| 1464 | 12251 | 6.799325                    | 8.388265                     | 8.449454                                                               |
| 1463 | 12241 | 6.798770                    | 8.387580                     | 8.448766                                                               |
| 1462 | 12239 | 6.798215                    | 8.386895                     | 8.448078                                                               |
| 1461 | 12227 | 6.797659                    | 8.386210                     | 8.447390                                                               |
| 1460 | 12211 | 6.797103                    | 8.385524                     | 8.446701                                                               |
| 1459 | 12203 | 6.796547                    | 8.384837                     | 8.446011                                                               |
| 1458 | 12197 | 6.795990                    | 8.384150                     | 8.445322                                                               |
| 1457 | 12163 | 6.795433                    | 8.383463                     | 8.444631                                                               |
| 1456 | 12161 | 6.794874                    | 8.382773                     | 8.443941                                                               |
| 1455 | 12157 | 6.794315                    | 8.382084                     | 8.443249                                                               |
| 1454 | 12149 | 6.793757                    | 8.381394                     | 8.442558                                                               |
| 1453 | 12143 | 6.793197                    | 8.380705                     | 8.441865                                                               |
| 1452 | 12119 | 6.792638                    | 8.380014                     | 8.441173                                                               |
| 1451 | 12113 | 6.792078                    | 8.379323                     | 8.440480                                                               |
| 1450 | 12109 | 6.791517                    | 8.378631                     | 8.439786                                                               |
| 1449 | 12107 | 6.790956                    | 8.377939                     | 8.439092                                                               |
| 1448 | 12101 | 6.790395                    | 8.377247                     | 8.438397                                                               |
| 1447 | 12097 | 6.789834                    | 8.376555                     | 8.437702                                                               |
| 1446 | 12073 | 6.789273                    | 8.375863                     | 8.437006                                                               |
| 1445 | 12071 | 6.788711                    | 8.375169                     | 8.436310                                                               |
| 1444 | 12049 | 6.788148                    | 8.374475                     | 8.435613                                                               |
| 1443 | 12043 | 6.787585                    | 8.373780                     | 8.434916                                                               |
| 1442 | 12041 | 6.787021                    | 8.373085                     | 8.434219                                                               |
| 1441 | 12037 | 6.786458                    | 8.372389                     | 8.433521                                                               |
| 1440 | 12011 | 6.785894                    | 8.371694                     | 8.432822                                                               |
| 1439 | 12007 | 6.785329                    | 8.370997                     | 8.432123                                                               |

| $k$  | $p_k$ | $\frac{\sigma(N'_k)}{N'_k}$ | $\frac{N'_k}{\varphi(N'_k)}$ | $\frac{e^\gamma}{2} \log \log N'_k + \frac{0.73\dots}{\log \log N'_k}$ |
|------|-------|-----------------------------|------------------------------|------------------------------------------------------------------------|
| 1438 | 11987 | 6.784764                    | 8.370299                     | 8.431423                                                               |
| 1437 | 11981 | 6.784198                    | 8.369601                     | 8.430723                                                               |
| 1436 | 11971 | 6.783632                    | 8.368903                     | 8.430023                                                               |
| 1435 | 11969 | 6.783065                    | 8.368203                     | 8.429322                                                               |
| 1434 | 11959 | 6.782498                    | 8.367504                     | 8.428620                                                               |
| 1433 | 11953 | 6.781931                    | 8.366805                     | 8.427918                                                               |
| 1432 | 11941 | 6.781364                    | 8.366105                     | 8.427216                                                               |
| 1431 | 11939 | 6.780796                    | 8.365404                     | 8.426513                                                               |
| 1430 | 11933 | 6.780228                    | 8.364703                     | 8.425809                                                               |
| 1429 | 11927 | 6.779660                    | 8.364002                     | 8.425105                                                               |
| 1428 | 11923 | 6.779092                    | 8.363301                     | 8.424400                                                               |
| 1427 | 11909 | 6.778523                    | 8.362600                     | 8.423695                                                               |
| 1426 | 11903 | 6.777954                    | 8.361897                     | 8.422989                                                               |
| 1425 | 11897 | 6.777385                    | 8.361195                     | 8.422283                                                               |
| 1424 | 11887 | 6.776815                    | 8.360492                     | 8.421577                                                               |
| 1423 | 11867 | 6.776245                    | 8.359789                     | 8.420869                                                               |
| 1422 | 11863 | 6.775674                    | 8.359084                     | 8.420162                                                               |
| 1421 | 11839 | 6.775103                    | 8.358380                     | 8.419454                                                               |
| 1420 | 11833 | 6.774531                    | 8.357674                     | 8.418745                                                               |
| 1419 | 11831 | 6.773958                    | 8.356967                     | 8.418036                                                               |
| 1418 | 11827 | 6.773386                    | 8.356261                     | 8.417326                                                               |
| 1417 | 11821 | 6.772813                    | 8.355555                     | 8.416616                                                               |
| 1416 | 11813 | 6.772240                    | 8.354848                     | 8.415905                                                               |
| 1415 | 11807 | 6.771667                    | 8.354140                     | 8.415194                                                               |
| 1414 | 11801 | 6.771093                    | 8.353433                     | 8.414482                                                               |
| 1413 | 11789 | 6.770520                    | 8.352725                     | 8.413770                                                               |
| 1412 | 11783 | 6.769945                    | 8.352017                     | 8.413057                                                               |
| 1411 | 11779 | 6.769371                    | 8.351308                     | 8.412343                                                               |
| 1410 | 11777 | 6.768796                    | 8.350599                     | 8.411629                                                               |
| 1409 | 11743 | 6.768222                    | 8.349890                     | 8.410915                                                               |
| 1408 | 11731 | 6.767645                    | 8.349179                     | 8.410200                                                               |
| 1407 | 11719 | 6.767068                    | 8.348467                     | 8.409485                                                               |
| 1406 | 11717 | 6.766491                    | 8.347754                     | 8.408769                                                               |
| 1405 | 11701 | 6.765914                    | 8.347042                     | 8.408052                                                               |
| 1404 | 11699 | 6.765335                    | 8.346329                     | 8.407335                                                               |
| 1403 | 11689 | 6.764757                    | 8.345615                     | 8.406618                                                               |
| 1402 | 11681 | 6.764179                    | 8.344901                     | 8.405900                                                               |
| 1401 | 11677 | 6.763600                    | 8.344187                     | 8.405181                                                               |
| 1400 | 11657 | 6.763020                    | 8.343472                     | 8.404462                                                               |
| 1399 | 11633 | 6.762440                    | 8.342757                     | 8.403743                                                               |
| 1398 | 11621 | 6.761859                    | 8.342039                     | 8.403023                                                               |
| 1397 | 11617 | 6.761277                    | 8.341322                     | 8.402302                                                               |
| 1396 | 11597 | 6.760695                    | 8.340604                     | 8.401581                                                               |
| 1395 | 11593 | 6.760112                    | 8.339884                     | 8.400860                                                               |

| $k$  | $p_k$ | $\frac{\sigma(N'_k)}{N'_k}$ | $\frac{N'_k}{\varphi(N'_k)}$ | $\frac{e^\gamma}{2} \log \log N'_k + \frac{0.73\dots}{\log \log N'_k}$ |
|------|-------|-----------------------------|------------------------------|------------------------------------------------------------------------|
| 1394 | 11587 | 6.759529                    | 8.339165                     | 8.400138                                                               |
| 1393 | 11579 | 6.758946                    | 8.338445                     | 8.399415                                                               |
| 1392 | 11551 | 6.758362                    | 8.337725                     | 8.398692                                                               |
| 1391 | 11549 | 6.757777                    | 8.337003                     | 8.397968                                                               |
| 1390 | 11527 | 6.757192                    | 8.336281                     | 8.397244                                                               |
| 1389 | 11519 | 6.756606                    | 8.335558                     | 8.396520                                                               |
| 1388 | 11503 | 6.756019                    | 8.334835                     | 8.395795                                                               |
| 1387 | 11497 | 6.755432                    | 8.334110                     | 8.395069                                                               |
| 1386 | 11491 | 6.754845                    | 8.333385                     | 8.394343                                                               |
| 1385 | 11489 | 6.754257                    | 8.332660                     | 8.393616                                                               |
| 1384 | 11483 | 6.753669                    | 8.331935                     | 8.392889                                                               |
| 1383 | 11471 | 6.753081                    | 8.331209                     | 8.392161                                                               |
| 1382 | 11467 | 6.752492                    | 8.330483                     | 8.391433                                                               |
| 1381 | 11447 | 6.751903                    | 8.329756                     | 8.390704                                                               |
| 1380 | 11443 | 6.751314                    | 8.329029                     | 8.389974                                                               |
| 1379 | 11437 | 6.750724                    | 8.328301                     | 8.389244                                                               |
| 1378 | 11423 | 6.750133                    | 8.327573                     | 8.388514                                                               |
| 1377 | 11411 | 6.749543                    | 8.326844                     | 8.387783                                                               |
| 1376 | 11399 | 6.748951                    | 8.326114                     | 8.387051                                                               |
| 1375 | 11393 | 6.748359                    | 8.325383                     | 8.386319                                                               |
| 1374 | 11383 | 6.747767                    | 8.324653                     | 8.385586                                                               |
| 1373 | 11369 | 6.747174                    | 8.323921                     | 8.384853                                                               |
| 1372 | 11353 | 6.746581                    | 8.323189                     | 8.384119                                                               |
| 1371 | 11351 | 6.745987                    | 8.322456                     | 8.383385                                                               |
| 1370 | 11329 | 6.745392                    | 8.321723                     | 8.382650                                                               |
| 1369 | 11321 | 6.744797                    | 8.320988                     | 8.381915                                                               |
| 1368 | 11317 | 6.744201                    | 8.320253                     | 8.381179                                                               |
| 1367 | 11311 | 6.743605                    | 8.319518                     | 8.380443                                                               |
| 1366 | 11299 | 6.743009                    | 8.318783                     | 8.379706                                                               |
| 1365 | 11287 | 6.742412                    | 8.318046                     | 8.378968                                                               |
| 1364 | 11279 | 6.741815                    | 8.317309                     | 8.378230                                                               |
| 1363 | 11273 | 6.741217                    | 8.316572                     | 8.377492                                                               |
| 1362 | 11261 | 6.740619                    | 8.315834                     | 8.376752                                                               |
| 1361 | 11257 | 6.740021                    | 8.315096                     | 8.376013                                                               |
| 1360 | 11251 | 6.739422                    | 8.314357                     | 8.375272                                                               |
| 1359 | 11243 | 6.738823                    | 8.313618                     | 8.374532                                                               |
| 1358 | 11239 | 6.738224                    | 8.312879                     | 8.373790                                                               |
| 1357 | 11213 | 6.737625                    | 8.312139                     | 8.373048                                                               |
| 1356 | 11197 | 6.737024                    | 8.311398                     | 8.372305                                                               |
| 1355 | 11177 | 6.736422                    | 8.310655                     | 8.371562                                                               |
| 1354 | 11173 | 6.735819                    | 8.309912                     | 8.370819                                                               |
| 1353 | 11171 | 6.735217                    | 8.309168                     | 8.370075                                                               |
| 1352 | 11161 | 6.734614                    | 8.308424                     | 8.369330                                                               |
| 1351 | 11159 | 6.734010                    | 8.307680                     | 8.368585                                                               |



| $k$  | $p_k$ | $\frac{\sigma(N'_k)}{N'_k}$ | $\frac{N'_k}{\varphi(N'_k)}$ | $\frac{e^\gamma}{2} \log \log N'_k + \frac{0.73\dots}{\log \log N'_k}$ |
|------|-------|-----------------------------|------------------------------|------------------------------------------------------------------------|
| 1350 | 11149 | 6.733407                    | 8.306935                     | 8.367839                                                               |
| 1349 | 11131 | 6.732803                    | 8.306190                     | 8.367093                                                               |
| 1348 | 11119 | 6.732198                    | 8.305444                     | 8.366346                                                               |
| 1347 | 11117 | 6.731593                    | 8.304697                     | 8.365598                                                               |
| 1346 | 11113 | 6.730987                    | 8.303950                     | 8.364850                                                               |
| 1345 | 11093 | 6.730382                    | 8.303203                     | 8.364102                                                               |
| 1344 | 11087 | 6.729775                    | 8.302454                     | 8.363352                                                               |
| 1343 | 11083 | 6.729168                    | 8.301705                     | 8.362603                                                               |
| 1342 | 11071 | 6.728561                    | 8.300956                     | 8.361852                                                               |
| 1341 | 11069 | 6.727953                    | 8.300207                     | 8.361101                                                               |
| 1340 | 11059 | 6.727346                    | 8.299457                     | 8.360350                                                               |
| 1339 | 11057 | 6.726737                    | 8.298706                     | 8.359598                                                               |
| 1338 | 11047 | 6.726129                    | 8.297956                     | 8.358845                                                               |
| 1337 | 11027 | 6.725520                    | 8.297205                     | 8.358091                                                               |
| 1336 | 11003 | 6.724910                    | 8.296452                     | 8.357338                                                               |
| 1335 | 10993 | 6.724299                    | 8.295698                     | 8.356583                                                               |
| 1334 | 10987 | 6.723688                    | 8.294944                     | 8.355829                                                               |
| 1333 | 10979 | 6.723076                    | 8.294189                     | 8.355073                                                               |
| 1332 | 10973 | 6.722463                    | 8.293433                     | 8.354317                                                               |
| 1331 | 10957 | 6.721851                    | 8.292677                     | 8.353560                                                               |
| 1330 | 10949 | 6.721237                    | 8.291920                     | 8.352803                                                               |
| 1329 | 10939 | 6.720624                    | 8.291163                     | 8.352045                                                               |
| 1328 | 10937 | 6.720009                    | 8.290405                     | 8.351287                                                               |
| 1327 | 10909 | 6.719395                    | 8.289647                     | 8.350528                                                               |
| 1326 | 10903 | 6.718779                    | 8.288887                     | 8.349769                                                               |
| 1325 | 10891 | 6.718163                    | 8.288127                     | 8.349009                                                               |
| 1324 | 10889 | 6.717546                    | 8.287366                     | 8.348248                                                               |
| 1323 | 10883 | 6.716929                    | 8.286605                     | 8.347487                                                               |
| 1322 | 10867 | 6.716312                    | 8.285844                     | 8.346725                                                               |
| 1321 | 10861 | 6.715694                    | 8.285081                     | 8.345963                                                               |
| 1320 | 10859 | 6.715076                    | 8.284318                     | 8.345200                                                               |
| 1319 | 10853 | 6.714457                    | 8.283555                     | 8.344436                                                               |
| 1318 | 10847 | 6.713839                    | 8.282792                     | 8.343672                                                               |
| 1317 | 10837 | 6.713220                    | 8.282028                     | 8.342907                                                               |
| 1316 | 10831 | 6.712600                    | 8.281264                     | 8.342141                                                               |
| 1315 | 10799 | 6.711981                    | 8.280500                     | 8.341375                                                               |
| 1314 | 10789 | 6.711359                    | 8.279733                     | 8.340609                                                               |
| 1313 | 10781 | 6.710737                    | 8.278965                     | 8.339842                                                               |
| 1312 | 10771 | 6.710115                    | 8.278198                     | 8.339074                                                               |
| 1311 | 10753 | 6.709492                    | 8.277429                     | 8.338306                                                               |
| 1310 | 10739 | 6.708868                    | 8.276659                     | 8.337537                                                               |
| 1309 | 10733 | 6.708243                    | 8.275888                     | 8.336768                                                               |
| 1308 | 10729 | 6.707618                    | 8.275117                     | 8.335998                                                               |
| 1307 | 10723 | 6.706993                    | 8.274346                     | 8.335227                                                               |

| $k$  | $p_k$ | $\frac{\sigma(N'_k)}{N'_k}$ | $\frac{N'_k}{\varphi(N'_k)}$ | $\frac{e^\gamma}{2} \log \log N'_k + \frac{0.73\dots}{\log \log N'_k}$ |
|------|-------|-----------------------------|------------------------------|------------------------------------------------------------------------|
| 1306 | 10711 | 6.706368                    | 8.273574                     | 8.334456                                                               |
| 1305 | 10709 | 6.705742                    | 8.272802                     | 8.333684                                                               |
| 1304 | 10691 | 6.705116                    | 8.272030                     | 8.332912                                                               |
| 1303 | 10687 | 6.704489                    | 8.271256                     | 8.332138                                                               |
| 1302 | 10667 | 6.703861                    | 8.270482                     | 8.331365                                                               |
| 1301 | 10663 | 6.703233                    | 8.269707                     | 8.330591                                                               |
| 1300 | 10657 | 6.702604                    | 8.268931                     | 8.329816                                                               |
| 1299 | 10651 | 6.701975                    | 8.268155                     | 8.329040                                                               |
| 1298 | 10639 | 6.701346                    | 8.267379                     | 8.328264                                                               |
| 1297 | 10631 | 6.700716                    | 8.266602                     | 8.327487                                                               |
| 1296 | 10627 | 6.700086                    | 8.265824                     | 8.326710                                                               |
| 1295 | 10613 | 6.699456                    | 8.265046                     | 8.325932                                                               |
| 1294 | 10607 | 6.698825                    | 8.264267                     | 8.325154                                                               |
| 1293 | 10601 | 6.698193                    | 8.263488                     | 8.324374                                                               |
| 1292 | 10597 | 6.697561                    | 8.262709                     | 8.323595                                                               |
| 1291 | 10589 | 6.696929                    | 8.261929                     | 8.322814                                                               |
| 1290 | 10567 | 6.696297                    | 8.261149                     | 8.322033                                                               |
| 1289 | 10559 | 6.695663                    | 8.260367                     | 8.321251                                                               |
| 1288 | 10531 | 6.695029                    | 8.259585                     | 8.320469                                                               |
| 1287 | 10529 | 6.694394                    | 8.258801                     | 8.319686                                                               |
| 1286 | 10513 | 6.693758                    | 8.258016                     | 8.318903                                                               |
| 1285 | 10501 | 6.693121                    | 8.257231                     | 8.318119                                                               |
| 1284 | 10499 | 6.692484                    | 8.256444                     | 8.317335                                                               |
| 1283 | 10487 | 6.691846                    | 8.255658                     | 8.316549                                                               |
| 1282 | 10477 | 6.691208                    | 8.254871                     | 8.315763                                                               |
| 1281 | 10463 | 6.690570                    | 8.254083                     | 8.314977                                                               |
| 1280 | 10459 | 6.689930                    | 8.253294                     | 8.314190                                                               |
| 1279 | 10457 | 6.689291                    | 8.252505                     | 8.313402                                                               |
| 1278 | 10453 | 6.688651                    | 8.251716                     | 8.312614                                                               |
| 1277 | 10433 | 6.688011                    | 8.250926                     | 8.311825                                                               |
| 1276 | 10429 | 6.687370                    | 8.250135                     | 8.311035                                                               |
| 1275 | 10427 | 6.686729                    | 8.249344                     | 8.310245                                                               |
| 1274 | 10399 | 6.686088                    | 8.248553                     | 8.309454                                                               |
| 1273 | 10391 | 6.685445                    | 8.247760                     | 8.308662                                                               |
| 1272 | 10369 | 6.684802                    | 8.246966                     | 8.307870                                                               |
| 1271 | 10357 | 6.684157                    | 8.246171                     | 8.307078                                                               |
| 1270 | 10343 | 6.683512                    | 8.245375                     | 8.306284                                                               |
| 1269 | 10337 | 6.682866                    | 8.244577                     | 8.305491                                                               |
| 1268 | 10333 | 6.682219                    | 8.243780                     | 8.304696                                                               |
| 1267 | 10331 | 6.681573                    | 8.242982                     | 8.303901                                                               |
| 1266 | 10321 | 6.680926                    | 8.242184                     | 8.303105                                                               |
| 1265 | 10313 | 6.680279                    | 8.241386                     | 8.302308                                                               |
| 1264 | 10303 | 6.679631                    | 8.240586                     | 8.301511                                                               |
| 1263 | 10301 | 6.678983                    | 8.239787                     | 8.300713                                                               |

| $k$  | $p_k$ | $\frac{\sigma(N'_k)}{N'_k}$ | $\frac{N'_k}{\varphi(N'_k)}$ | $\frac{e^\gamma}{2} \log \log N'_k + \frac{0.73\dots}{\log \log N'_k}$ |
|------|-------|-----------------------------|------------------------------|------------------------------------------------------------------------|
| 1262 | 10289 | 6.678334                    | 8.238987                     | 8.299915                                                               |
| 1261 | 10273 | 6.677685                    | 8.238186                     | 8.299116                                                               |
| 1260 | 10271 | 6.677036                    | 8.237384                     | 8.298316                                                               |
| 1259 | 10267 | 6.676385                    | 8.236582                     | 8.297516                                                               |
| 1258 | 10259 | 6.675735                    | 8.235780                     | 8.296715                                                               |
| 1257 | 10253 | 6.675085                    | 8.234977                     | 8.295913                                                               |
| 1256 | 10247 | 6.674434                    | 8.234174                     | 8.295110                                                               |
| 1255 | 10243 | 6.673782                    | 8.233370                     | 8.294307                                                               |
| 1254 | 10223 | 6.673131                    | 8.232566                     | 8.293503                                                               |
| 1253 | 10211 | 6.672478                    | 8.231761                     | 8.292699                                                               |
| 1252 | 10193 | 6.671825                    | 8.230955                     | 8.291894                                                               |
| 1251 | 10181 | 6.671170                    | 8.230147                     | 8.291088                                                               |
| 1250 | 10177 | 6.670515                    | 8.229339                     | 8.290282                                                               |
| 1249 | 10169 | 6.669860                    | 8.228530                     | 8.289475                                                               |
| 1248 | 10163 | 6.669204                    | 8.227721                     | 8.288668                                                               |
| 1247 | 10159 | 6.668548                    | 8.226912                     | 8.287859                                                               |
| 1246 | 10151 | 6.667891                    | 8.226102                     | 8.287050                                                               |
| 1245 | 10141 | 6.667235                    | 8.225292                     | 8.286241                                                               |
| 1244 | 10139 | 6.666577                    | 8.224480                     | 8.285430                                                               |
| 1243 | 10133 | 6.665920                    | 8.223669                     | 8.284619                                                               |
| 1242 | 10111 | 6.665262                    | 8.222858                     | 8.283807                                                               |
| 1241 | 10103 | 6.664603                    | 8.222044                     | 8.282995                                                               |
| 1240 | 10099 | 6.663943                    | 8.221231                     | 8.282182                                                               |
| 1239 | 10093 | 6.663283                    | 8.220417                     | 8.281368                                                               |
| 1238 | 10091 | 6.662623                    | 8.219602                     | 8.280554                                                               |
| 1237 | 10079 | 6.661963                    | 8.218788                     | 8.279739                                                               |
| 1236 | 10069 | 6.661302                    | 8.217972                     | 8.278923                                                               |
| 1235 | 10067 | 6.660641                    | 8.217156                     | 8.278107                                                               |
| 1234 | 10061 | 6.659979                    | 8.216340                     | 8.277290                                                               |
| 1233 | 10039 | 6.659317                    | 8.215523                     | 8.276472                                                               |
| 1232 | 10037 | 6.658654                    | 8.214705                     | 8.275653                                                               |
| 1231 | 10009 | 6.657991                    | 8.213886                     | 8.274834                                                               |
| 1230 | 10007 | 6.657325                    | 8.213066                     | 8.274014                                                               |
| 1229 | 9973  | 6.656660                    | 8.212245                     | 8.273194                                                               |
| 1228 | 9967  | 6.655993                    | 8.211421                     | 8.272373                                                               |
| 1227 | 9949  | 6.655325                    | 8.210598                     | 8.271551                                                               |
| 1226 | 9941  | 6.654656                    | 8.209772                     | 8.270729                                                               |
| 1225 | 9931  | 6.653987                    | 8.208946                     | 8.269906                                                               |
| 1224 | 9929  | 6.653317                    | 8.208120                     | 8.269083                                                               |
| 1223 | 9923  | 6.652647                    | 8.207293                     | 8.268258                                                               |
| 1222 | 9907  | 6.651977                    | 8.206466                     | 8.267433                                                               |
| 1221 | 9901  | 6.651305                    | 8.205638                     | 8.266608                                                               |
| 1220 | 9887  | 6.650633                    | 8.204809                     | 8.265781                                                               |
| 1219 | 9883  | 6.649961                    | 8.203979                     | 8.264954                                                               |

| $k$  | $p_k$ | $\frac{\sigma(N'_k)}{N'_k}$ | $\frac{N'_k}{\varphi(N'_k)}$ | $\frac{e^\gamma}{2} \log \log N'_k + \frac{0.73\dots}{\log \log N'_k}$ |
|------|-------|-----------------------------|------------------------------|------------------------------------------------------------------------|
| 1218 | 9871  | 6.649288                    | 8.203149                     | 8.264126                                                               |
| 1217 | 9859  | 6.648615                    | 8.202318                     | 8.263298                                                               |
| 1216 | 9857  | 6.647940                    | 8.201486                     | 8.262469                                                               |
| 1215 | 9851  | 6.647266                    | 8.200654                     | 8.261639                                                               |
| 1214 | 9839  | 6.646591                    | 8.199821                     | 8.260808                                                               |
| 1213 | 9833  | 6.645916                    | 8.198988                     | 8.259977                                                               |
| 1212 | 9829  | 6.645240                    | 8.198154                     | 8.259145                                                               |
| 1211 | 9817  | 6.644564                    | 8.197320                     | 8.258312                                                               |
| 1210 | 9811  | 6.643887                    | 8.196485                     | 8.257479                                                               |
| 1209 | 9803  | 6.643210                    | 8.195650                     | 8.256645                                                               |
| 1208 | 9791  | 6.642532                    | 8.194814                     | 8.255810                                                               |
| 1207 | 9787  | 6.641854                    | 8.193977                     | 8.254975                                                               |
| 1206 | 9781  | 6.641175                    | 8.193139                     | 8.254138                                                               |
| 1205 | 9769  | 6.640497                    | 8.192302                     | 8.253301                                                               |
| 1204 | 9767  | 6.639817                    | 8.191463                     | 8.252463                                                               |
| 1203 | 9749  | 6.639137                    | 8.190624                     | 8.251625                                                               |
| 1202 | 9743  | 6.638456                    | 8.189784                     | 8.250786                                                               |
| 1201 | 9739  | 6.637775                    | 8.188944                     | 8.249946                                                               |
| 1200 | 9733  | 6.637093                    | 8.188103                     | 8.249105                                                               |
| 1199 | 9721  | 6.636412                    | 8.187262                     | 8.248264                                                               |
| 1198 | 9719  | 6.635729                    | 8.186419                     | 8.247422                                                               |
| 1197 | 9697  | 6.635046                    | 8.185577                     | 8.246579                                                               |
| 1196 | 9689  | 6.634362                    | 8.184733                     | 8.245736                                                               |
| 1195 | 9679  | 6.633677                    | 8.183888                     | 8.244892                                                               |
| 1194 | 9677  | 6.632992                    | 8.183043                     | 8.244047                                                               |
| 1193 | 9661  | 6.632307                    | 8.182197                     | 8.243201                                                               |
| 1192 | 9649  | 6.631620                    | 8.181350                     | 8.242355                                                               |
| 1191 | 9643  | 6.630933                    | 8.180502                     | 8.241508                                                               |
| 1190 | 9631  | 6.630245                    | 8.179654                     | 8.240660                                                               |
| 1189 | 9629  | 6.629557                    | 8.178805                     | 8.239811                                                               |
| 1188 | 9623  | 6.628869                    | 8.177955                     | 8.238962                                                               |
| 1187 | 9619  | 6.628180                    | 8.177105                     | 8.238112                                                               |
| 1186 | 9613  | 6.627491                    | 8.176255                     | 8.237261                                                               |
| 1185 | 9601  | 6.626802                    | 8.175405                     | 8.236410                                                               |
| 1184 | 9587  | 6.626111                    | 8.174553                     | 8.235558                                                               |
| 1183 | 9551  | 6.625420                    | 8.173701                     | 8.234705                                                               |
| 1182 | 9547  | 6.624727                    | 8.172845                     | 8.233851                                                               |
| 1181 | 9539  | 6.624033                    | 8.171989                     | 8.232997                                                               |
| 1180 | 9533  | 6.623339                    | 8.171132                     | 8.232142                                                               |
| 1179 | 9521  | 6.622644                    | 8.170275                     | 8.231286                                                               |
| 1178 | 9511  | 6.621948                    | 8.169417                     | 8.230430                                                               |
| 1177 | 9497  | 6.621252                    | 8.168558                     | 8.229573                                                               |
| 1176 | 9491  | 6.620555                    | 8.167698                     | 8.228715                                                               |
| 1175 | 9479  | 6.619858                    | 8.166837                     | 8.227856                                                               |

| $k$  | $p_k$ | $\frac{\sigma(N'_k)}{N'_k}$ | $\frac{N'_k}{\varphi(N'_k)}$ | $\frac{e^\gamma}{2} \log \log N'_k + \frac{0.73\dots}{\log \log N'_k}$ |
|------|-------|-----------------------------|------------------------------|------------------------------------------------------------------------|
| 1174 | 9473  | 6.619159                    | 8.165976                     | 8.226997                                                               |
| 1173 | 9467  | 6.618461                    | 8.165113                     | 8.226137                                                               |
| 1172 | 9463  | 6.617762                    | 8.164251                     | 8.225276                                                               |
| 1171 | 9461  | 6.617062                    | 8.163388                     | 8.224414                                                               |
| 1170 | 9439  | 6.616363                    | 8.162525                     | 8.223551                                                               |
| 1169 | 9437  | 6.615662                    | 8.161661                     | 8.222688                                                               |
| 1168 | 9433  | 6.614961                    | 8.160796                     | 8.221824                                                               |
| 1167 | 9431  | 6.614260                    | 8.159931                     | 8.220959                                                               |
| 1166 | 9421  | 6.613559                    | 8.159065                     | 8.220094                                                               |
| 1165 | 9419  | 6.612857                    | 8.158199                     | 8.219228                                                               |
| 1164 | 9413  | 6.612155                    | 8.157333                     | 8.218360                                                               |
| 1163 | 9403  | 6.611452                    | 8.156467                     | 8.217492                                                               |
| 1162 | 9397  | 6.610749                    | 8.155599                     | 8.216624                                                               |
| 1161 | 9391  | 6.610046                    | 8.154731                     | 8.215754                                                               |
| 1160 | 9377  | 6.609342                    | 8.153863                     | 8.214884                                                               |
| 1159 | 9371  | 6.608637                    | 8.152993                     | 8.214013                                                               |
| 1158 | 9349  | 6.607932                    | 8.152123                     | 8.213141                                                               |
| 1157 | 9343  | 6.607225                    | 8.151251                     | 8.212268                                                               |
| 1156 | 9341  | 6.606518                    | 8.150379                     | 8.211395                                                               |
| 1155 | 9337  | 6.605811                    | 8.149506                     | 8.210521                                                               |
| 1154 | 9323  | 6.605104                    | 8.148634                     | 8.209646                                                               |
| 1153 | 9319  | 6.604395                    | 8.147760                     | 8.208770                                                               |
| 1152 | 9311  | 6.603687                    | 8.146885                     | 8.207894                                                               |
| 1151 | 9293  | 6.602978                    | 8.146010                     | 8.207016                                                               |
| 1150 | 9283  | 6.602267                    | 8.145134                     | 8.206139                                                               |
| 1149 | 9281  | 6.601556                    | 8.144256                     | 8.205260                                                               |
| 1148 | 9277  | 6.600845                    | 8.143379                     | 8.204380                                                               |
| 1147 | 9257  | 6.600133                    | 8.142501                     | 8.203500                                                               |
| 1146 | 9241  | 6.599420                    | 8.141621                     | 8.202619                                                               |
| 1145 | 9239  | 6.598706                    | 8.140740                     | 8.201737                                                               |
| 1144 | 9227  | 6.597992                    | 8.139859                     | 8.200854                                                               |
| 1143 | 9221  | 6.597277                    | 8.138977                     | 8.199971                                                               |
| 1142 | 9209  | 6.596562                    | 8.138094                     | 8.199086                                                               |
| 1141 | 9203  | 6.595846                    | 8.137211                     | 8.198201                                                               |
| 1140 | 9199  | 6.595129                    | 8.136326                     | 8.197316                                                               |
| 1139 | 9187  | 6.594412                    | 8.135442                     | 8.196429                                                               |
| 1138 | 9181  | 6.593694                    | 8.134556                     | 8.195541                                                               |
| 1137 | 9173  | 6.592976                    | 8.133670                     | 8.194653                                                               |
| 1136 | 9161  | 6.592258                    | 8.132784                     | 8.193764                                                               |
| 1135 | 9157  | 6.591538                    | 8.131896                     | 8.192874                                                               |
| 1134 | 9151  | 6.590818                    | 8.131008                     | 8.191984                                                               |
| 1133 | 9137  | 6.590098                    | 8.130119                     | 8.191092                                                               |
| 1132 | 9133  | 6.589377                    | 8.129230                     | 8.190200                                                               |
| 1131 | 9127  | 6.588656                    | 8.128339                     | 8.189307                                                               |

| $k$  | $p_k$ | $\frac{\sigma(N'_k)}{N'_k}$ | $\frac{N'_k}{\varphi(N'_k)}$ | $\frac{e^\gamma}{2} \log \log N'_k + \frac{0.73\dots}{\log \log N'_k}$ |
|------|-------|-----------------------------|------------------------------|------------------------------------------------------------------------|
| 1130 | 9109  | 6.587934                    | 8.127449                     | 8.188413                                                               |
| 1129 | 9103  | 6.587211                    | 8.126557                     | 8.187518                                                               |
| 1128 | 9091  | 6.586487                    | 8.125664                     | 8.186622                                                               |
| 1127 | 9067  | 6.585763                    | 8.124770                     | 8.185726                                                               |
| 1126 | 9059  | 6.585036                    | 8.123874                     | 8.184829                                                               |
| 1125 | 9049  | 6.584310                    | 8.122977                     | 8.183931                                                               |
| 1124 | 9043  | 6.583582                    | 8.122080                     | 8.183033                                                               |
| 1123 | 9041  | 6.582854                    | 8.121181                     | 8.182133                                                               |
| 1122 | 9029  | 6.582126                    | 8.120283                     | 8.181233                                                               |
| 1121 | 9013  | 6.581397                    | 8.119384                     | 8.180332                                                               |
| 1120 | 9011  | 6.580667                    | 8.118483                     | 8.179430                                                               |
| 1119 | 9007  | 6.579937                    | 8.117582                     | 8.178527                                                               |
| 1118 | 9001  | 6.579206                    | 8.116681                     | 8.177623                                                               |
| 1117 | 8999  | 6.578475                    | 8.115779                     | 8.176719                                                               |
| 1116 | 8971  | 6.577744                    | 8.114877                     | 8.175813                                                               |
| 1115 | 8969  | 6.577011                    | 8.113973                     | 8.174907                                                               |
| 1114 | 8963  | 6.576278                    | 8.113068                     | 8.174000                                                               |
| 1113 | 8951  | 6.575544                    | 8.112163                     | 8.173093                                                               |
| 1112 | 8941  | 6.574810                    | 8.111256                     | 8.172184                                                               |
| 1111 | 8933  | 6.574075                    | 8.110349                     | 8.171275                                                               |
| 1110 | 8929  | 6.573339                    | 8.109441                     | 8.170364                                                               |
| 1109 | 8923  | 6.572603                    | 8.108533                     | 8.169453                                                               |
| 1108 | 8893  | 6.571866                    | 8.107624                     | 8.168541                                                               |
| 1107 | 8887  | 6.571127                    | 8.106713                     | 8.167628                                                               |
| 1106 | 8867  | 6.570388                    | 8.105800                     | 8.166715                                                               |
| 1105 | 8863  | 6.569647                    | 8.104886                     | 8.165801                                                               |
| 1104 | 8861  | 6.568906                    | 8.103972                     | 8.164885                                                               |
| 1103 | 8849  | 6.568165                    | 8.103057                     | 8.163969                                                               |
| 1102 | 8839  | 6.567423                    | 8.102142                     | 8.163052                                                               |
| 1101 | 8837  | 6.566680                    | 8.101225                     | 8.162135                                                               |
| 1100 | 8831  | 6.565937                    | 8.100308                     | 8.161216                                                               |
| 1099 | 8821  | 6.565193                    | 8.099391                     | 8.160297                                                               |
| 1098 | 8819  | 6.564449                    | 8.098473                     | 8.159376                                                               |
| 1097 | 8807  | 6.563705                    | 8.097554                     | 8.158455                                                               |
| 1096 | 8803  | 6.562960                    | 8.096635                     | 8.157533                                                               |
| 1095 | 8783  | 6.562214                    | 8.095715                     | 8.156610                                                               |
| 1094 | 8779  | 6.561467                    | 8.094794                     | 8.155686                                                               |
| 1093 | 8761  | 6.560720                    | 8.093871                     | 8.154761                                                               |
| 1092 | 8753  | 6.559971                    | 8.092948                     | 8.153836                                                               |
| 1091 | 8747  | 6.559222                    | 8.092023                     | 8.152909                                                               |
| 1090 | 8741  | 6.558472                    | 8.091098                     | 8.151982                                                               |
| 1089 | 8737  | 6.557722                    | 8.090172                     | 8.151054                                                               |
| 1088 | 8731  | 6.556971                    | 8.089246                     | 8.150125                                                               |
| 1087 | 8719  | 6.556220                    | 8.088320                     | 8.149195                                                               |

| $k$  | $p_k$ | $\frac{\sigma(N'_k)}{N'_k}$ | $\frac{N'_k}{\varphi(N'_k)}$ | $\frac{e^\gamma}{2} \log \log N'_k + \frac{0.73\dots}{\log \log N'_k}$ |
|------|-------|-----------------------------|------------------------------|------------------------------------------------------------------------|
| 1086 | 8713  | 6.555468                    | 8.087392                     | 8.148264                                                               |
| 1085 | 8707  | 6.554716                    | 8.086464                     | 8.147332                                                               |
| 1084 | 8699  | 6.553963                    | 8.085535                     | 8.146399                                                               |
| 1083 | 8693  | 6.553210                    | 8.084606                     | 8.145466                                                               |
| 1082 | 8689  | 6.552456                    | 8.083676                     | 8.144531                                                               |
| 1081 | 8681  | 6.551702                    | 8.082745                     | 8.143596                                                               |
| 1080 | 8677  | 6.550947                    | 8.081814                     | 8.142660                                                               |
| 1079 | 8669  | 6.550193                    | 8.080883                     | 8.141722                                                               |
| 1078 | 8663  | 6.549437                    | 8.079951                     | 8.140784                                                               |
| 1077 | 8647  | 6.548681                    | 8.079018                     | 8.139845                                                               |
| 1076 | 8641  | 6.547924                    | 8.078084                     | 8.138905                                                               |
| 1075 | 8629  | 6.547166                    | 8.077149                     | 8.137964                                                               |
| 1074 | 8627  | 6.546408                    | 8.076213                     | 8.137023                                                               |
| 1073 | 8623  | 6.545649                    | 8.075277                     | 8.136080                                                               |
| 1072 | 8609  | 6.544890                    | 8.074340                     | 8.135136                                                               |
| 1071 | 8599  | 6.544130                    | 8.073402                     | 8.134192                                                               |
| 1070 | 8597  | 6.543369                    | 8.072463                     | 8.133247                                                               |
| 1069 | 8581  | 6.542608                    | 8.071524                     | 8.132300                                                               |
| 1068 | 8573  | 6.541845                    | 8.070584                     | 8.131353                                                               |
| 1067 | 8563  | 6.541082                    | 8.069642                     | 8.130405                                                               |
| 1066 | 8543  | 6.540319                    | 8.068700                     | 8.129456                                                               |
| 1065 | 8539  | 6.539553                    | 8.067756                     | 8.128506                                                               |
| 1064 | 8537  | 6.538787                    | 8.066811                     | 8.127556                                                               |
| 1063 | 8527  | 6.538021                    | 8.065866                     | 8.126604                                                               |
| 1062 | 8521  | 6.537255                    | 8.064920                     | 8.125651                                                               |
| 1061 | 8513  | 6.536488                    | 8.063973                     | 8.124698                                                               |
| 1060 | 8501  | 6.535720                    | 8.063026                     | 8.123743                                                               |
| 1059 | 8467  | 6.534951                    | 8.062078                     | 8.122788                                                               |
| 1058 | 8461  | 6.534180                    | 8.061125                     | 8.121832                                                               |
| 1057 | 8447  | 6.533407                    | 8.060173                     | 8.120875                                                               |
| 1056 | 8443  | 6.532634                    | 8.059219                     | 8.119917                                                               |
| 1055 | 8431  | 6.531860                    | 8.058264                     | 8.118958                                                               |
| 1054 | 8429  | 6.531086                    | 8.057308                     | 8.117999                                                               |
| 1053 | 8423  | 6.530311                    | 8.056352                     | 8.117038                                                               |
| 1052 | 8419  | 6.529536                    | 8.055396                     | 8.116076                                                               |
| 1051 | 8389  | 6.528760                    | 8.054439                     | 8.115114                                                               |
| 1050 | 8387  | 6.527982                    | 8.053479                     | 8.114150                                                               |
| 1049 | 8377  | 6.527204                    | 8.052519                     | 8.113186                                                               |
| 1048 | 8369  | 6.526425                    | 8.051557                     | 8.112220                                                               |
| 1047 | 8363  | 6.525645                    | 8.050595                     | 8.111254                                                               |
| 1046 | 8353  | 6.524865                    | 8.049633                     | 8.110287                                                               |
| 1045 | 8329  | 6.524084                    | 8.048669                     | 8.109319                                                               |
| 1044 | 8317  | 6.523301                    | 8.047703                     | 8.108350                                                               |
| 1043 | 8311  | 6.522516                    | 8.046735                     | 8.107380                                                               |

| $k$  | $p_k$ | $\frac{\sigma(N'_k)}{N'_k}$ | $\frac{N'_k}{\varphi(N'_k)}$ | $\frac{e^\gamma}{2} \log \log N'_k + \frac{0.73\dots}{\log \log N'_k}$ |
|------|-------|-----------------------------|------------------------------|------------------------------------------------------------------------|
| 1042 | 8297  | 6.521732                    | 8.045767                     | 8.106409                                                               |
| 1041 | 8293  | 6.520946                    | 8.044797                     | 8.105437                                                               |
| 1040 | 8291  | 6.520159                    | 8.043827                     | 8.104465                                                               |
| 1039 | 8287  | 6.519373                    | 8.042857                     | 8.103491                                                               |
| 1038 | 8273  | 6.518587                    | 8.041886                     | 8.102516                                                               |
| 1037 | 8269  | 6.517799                    | 8.040914                     | 8.101540                                                               |
| 1036 | 8263  | 6.517011                    | 8.039942                     | 8.100564                                                               |
| 1035 | 8243  | 6.516222                    | 8.038969                     | 8.099586                                                               |
| 1034 | 8237  | 6.515432                    | 8.037994                     | 8.098608                                                               |
| 1033 | 8233  | 6.514641                    | 8.037018                     | 8.097628                                                               |
| 1032 | 8231  | 6.513849                    | 8.036042                     | 8.096647                                                               |
| 1031 | 8221  | 6.513058                    | 8.035065                     | 8.095666                                                               |
| 1030 | 8219  | 6.512266                    | 8.034088                     | 8.094683                                                               |
| 1029 | 8209  | 6.511474                    | 8.033110                     | 8.093699                                                               |
| 1028 | 8191  | 6.510681                    | 8.032132                     | 8.092715                                                               |
| 1027 | 8179  | 6.509886                    | 8.031151                     | 8.091729                                                               |
| 1026 | 8171  | 6.509090                    | 8.030169                     | 8.090743                                                               |
| 1025 | 8167  | 6.508294                    | 8.029186                     | 8.089755                                                               |
| 1024 | 8161  | 6.507497                    | 8.028203                     | 8.088767                                                               |
| 1023 | 8147  | 6.506699                    | 8.027220                     | 8.087778                                                               |
| 1022 | 8123  | 6.505901                    | 8.026234                     | 8.086787                                                               |
| 1021 | 8117  | 6.505100                    | 8.025246                     | 8.085796                                                               |
| 1020 | 8111  | 6.504299                    | 8.024258                     | 8.084804                                                               |
| 1019 | 8101  | 6.503497                    | 8.023268                     | 8.083810                                                               |
| 1018 | 8093  | 6.502694                    | 8.022278                     | 8.082816                                                               |
| 1017 | 8089  | 6.501891                    | 8.021287                     | 8.081821                                                               |
| 1016 | 8087  | 6.501087                    | 8.020295                     | 8.080824                                                               |
| 1015 | 8081  | 6.500283                    | 8.019303                     | 8.079827                                                               |
| 1014 | 8069  | 6.499479                    | 8.018311                     | 8.078829                                                               |
| 1013 | 8059  | 6.498674                    | 8.017317                     | 8.077829                                                               |
| 1012 | 8053  | 6.497867                    | 8.016322                     | 8.076829                                                               |
| 1011 | 8039  | 6.497061                    | 8.015327                     | 8.075827                                                               |
| 1010 | 8017  | 6.496253                    | 8.014330                     | 8.074825                                                               |
| 1009 | 8011  | 6.495442                    | 8.013330                     | 8.073821                                                               |
| 1008 | 8009  | 6.494632                    | 8.012330                     | 8.072817                                                               |
| 1007 | 7993  | 6.493821                    | 8.011329                     | 8.071812                                                               |
| 1006 | 7963  | 6.493008                    | 8.010327                     | 8.070805                                                               |
| 1005 | 7951  | 6.492193                    | 8.009321                     | 8.069798                                                               |
| 1004 | 7949  | 6.491377                    | 8.008314                     | 8.068790                                                               |
| 1003 | 7937  | 6.490560                    | 8.007306                     | 8.067781                                                               |
| 1002 | 7933  | 6.489743                    | 8.006298                     | 8.066771                                                               |
| 1001 | 7927  | 6.488925                    | 8.005288                     | 8.065760                                                               |
| 1000 | 7919  | 6.488106                    | 8.004278                     | 8.064747                                                               |
| 999  | 7907  | 6.487287                    | 8.003268                     | 8.063734                                                               |



| $k$ | $p_k$ | $\frac{\sigma(N'_k)}{N'_k}$ | $\frac{N'_k}{\varphi(N'_k)}$ | $\frac{e^\gamma}{2} \log \log N'_k + \frac{0.73\dots}{\log \log N'_k}$ |
|-----|-------|-----------------------------|------------------------------|------------------------------------------------------------------------|
| 998 | 7901  | 6.486467                    | 8.002255                     | 8.062719                                                               |
| 997 | 7883  | 6.485646                    | 8.001243                     | 8.061704                                                               |
| 996 | 7879  | 6.484823                    | 8.000228                     | 8.060688                                                               |
| 995 | 7877  | 6.484000                    | 7.999212                     | 8.059670                                                               |
| 994 | 7873  | 6.483177                    | 7.998197                     | 8.058651                                                               |
| 993 | 7867  | 6.482354                    | 7.997181                     | 8.057632                                                               |
| 992 | 7853  | 6.481530                    | 7.996164                     | 8.056611                                                               |
| 991 | 7841  | 6.480705                    | 7.995146                     | 8.055589                                                               |
| 990 | 7829  | 6.479878                    | 7.994126                     | 8.054566                                                               |
| 989 | 7823  | 6.479051                    | 7.993105                     | 8.053542                                                               |
| 988 | 7817  | 6.478222                    | 7.992084                     | 8.052517                                                               |
| 987 | 7793  | 6.477394                    | 7.991061                     | 8.051491                                                               |
| 986 | 7789  | 6.476563                    | 7.990036                     | 8.050464                                                               |
| 985 | 7759  | 6.475731                    | 7.989010                     | 8.049436                                                               |
| 984 | 7757  | 6.474897                    | 7.987980                     | 8.048408                                                               |
| 983 | 7753  | 6.474062                    | 7.986951                     | 8.047378                                                               |
| 982 | 7741  | 6.473227                    | 7.985920                     | 8.046347                                                               |
| 981 | 7727  | 6.472391                    | 7.984889                     | 8.045315                                                               |
| 980 | 7723  | 6.471554                    | 7.983855                     | 8.044281                                                               |
| 979 | 7717  | 6.470716                    | 7.982822                     | 8.043247                                                               |
| 978 | 7703  | 6.469877                    | 7.981787                     | 8.042212                                                               |
| 977 | 7699  | 6.469038                    | 7.980751                     | 8.041175                                                               |
| 976 | 7691  | 6.468197                    | 7.979714                     | 8.040138                                                               |
| 975 | 7687  | 6.467357                    | 7.978677                     | 8.039099                                                               |
| 974 | 7681  | 6.466515                    | 7.977639                     | 8.038059                                                               |
| 973 | 7673  | 6.465674                    | 7.976600                     | 8.037018                                                               |
| 972 | 7669  | 6.464831                    | 7.975561                     | 8.035976                                                               |
| 971 | 7649  | 6.463988                    | 7.974521                     | 8.034933                                                               |
| 970 | 7643  | 6.463143                    | 7.973478                     | 8.033889                                                               |
| 969 | 7639  | 6.462298                    | 7.972435                     | 8.032844                                                               |
| 968 | 7621  | 6.461452                    | 7.971391                     | 8.031797                                                               |
| 967 | 7607  | 6.460604                    | 7.970345                     | 8.030750                                                               |
| 966 | 7603  | 6.459755                    | 7.969297                     | 8.029701                                                               |
| 965 | 7591  | 6.458905                    | 7.968249                     | 8.028652                                                               |
| 964 | 7589  | 6.458055                    | 7.967200                     | 8.027601                                                               |
| 963 | 7583  | 6.457204                    | 7.966150                     | 8.026549                                                               |
| 962 | 7577  | 6.456352                    | 7.965099                     | 8.025496                                                               |
| 961 | 7573  | 6.455500                    | 7.964048                     | 8.024442                                                               |
| 960 | 7561  | 6.454648                    | 7.962996                     | 8.023386                                                               |
| 959 | 7559  | 6.453794                    | 7.961943                     | 8.022330                                                               |
| 958 | 7549  | 6.452941                    | 7.960890                     | 8.021272                                                               |
| 957 | 7547  | 6.452086                    | 7.959835                     | 8.020213                                                               |
| 956 | 7541  | 6.451231                    | 7.958781                     | 8.019153                                                               |
| 955 | 7537  | 6.450376                    | 7.957725                     | 8.018092                                                               |

| $k$ | $p_k$ | $\frac{\sigma(N'_k)}{N'_k}$ | $\frac{N'_k}{\varphi(N'_k)}$ | $\frac{e^\gamma}{2} \log \log N'_k + \frac{0.73\dots}{\log \log N'_k}$ |
|-----|-------|-----------------------------|------------------------------|------------------------------------------------------------------------|
| 954 | 7529  | 6.449520                    | 7.956669                     | 8.017029                                                               |
| 953 | 7523  | 6.448664                    | 7.955613                     | 8.015966                                                               |
| 952 | 7517  | 6.447807                    | 7.954555                     | 8.014901                                                               |
| 951 | 7507  | 6.446949                    | 7.953497                     | 8.013835                                                               |
| 950 | 7499  | 6.446090                    | 7.952437                     | 8.012767                                                               |
| 949 | 7489  | 6.445231                    | 7.951377                     | 8.011699                                                               |
| 948 | 7487  | 6.444370                    | 7.950315                     | 8.010630                                                               |
| 947 | 7481  | 6.443510                    | 7.949253                     | 8.009559                                                               |
| 946 | 7477  | 6.442648                    | 7.948191                     | 8.008487                                                               |
| 945 | 7459  | 6.441787                    | 7.947128                     | 8.007414                                                               |
| 944 | 7457  | 6.440923                    | 7.946062                     | 8.006340                                                               |
| 943 | 7451  | 6.440060                    | 7.944997                     | 8.005264                                                               |
| 942 | 7433  | 6.439196                    | 7.943930                     | 8.004188                                                               |
| 941 | 7417  | 6.438329                    | 7.942862                     | 8.003110                                                               |
| 940 | 7411  | 6.437461                    | 7.941791                     | 8.002031                                                               |
| 939 | 7393  | 6.436593                    | 7.940719                     | 8.000951                                                               |
| 938 | 7369  | 6.435722                    | 7.939645                     | 7.999870                                                               |
| 937 | 7351  | 6.434849                    | 7.938568                     | 7.998788                                                               |
| 936 | 7349  | 6.433974                    | 7.937488                     | 7.997705                                                               |
| 935 | 7333  | 6.433099                    | 7.936408                     | 7.996621                                                               |
| 934 | 7331  | 6.432221                    | 7.935325                     | 7.995536                                                               |
| 933 | 7321  | 6.431344                    | 7.934243                     | 7.994449                                                               |
| 932 | 7309  | 6.430466                    | 7.933159                     | 7.993361                                                               |
| 931 | 7307  | 6.429586                    | 7.932074                     | 7.992272                                                               |
| 930 | 7297  | 6.428706                    | 7.930988                     | 7.991182                                                               |
| 929 | 7283  | 6.427825                    | 7.929901                     | 7.990091                                                               |
| 928 | 7253  | 6.426943                    | 7.928812                     | 7.988998                                                               |
| 927 | 7247  | 6.426057                    | 7.927719                     | 7.987905                                                               |
| 926 | 7243  | 6.425170                    | 7.926625                     | 7.986810                                                               |
| 925 | 7237  | 6.424283                    | 7.925531                     | 7.985714                                                               |
| 924 | 7229  | 6.423396                    | 7.924436                     | 7.984617                                                               |
| 923 | 7219  | 6.422507                    | 7.923340                     | 7.983519                                                               |
| 922 | 7213  | 6.421618                    | 7.922242                     | 7.982419                                                               |
| 921 | 7211  | 6.420728                    | 7.921144                     | 7.981318                                                               |
| 920 | 7207  | 6.419837                    | 7.920045                     | 7.980216                                                               |
| 919 | 7193  | 6.418947                    | 7.918946                     | 7.979113                                                               |
| 918 | 7187  | 6.418054                    | 7.917845                     | 7.978008                                                               |
| 917 | 7177  | 6.417162                    | 7.916744                     | 7.976902                                                               |
| 916 | 7159  | 6.416268                    | 7.915641                     | 7.975795                                                               |
| 915 | 7151  | 6.415371                    | 7.914535                     | 7.974687                                                               |
| 914 | 7129  | 6.414474                    | 7.913428                     | 7.973577                                                               |
| 913 | 7127  | 6.413575                    | 7.912318                     | 7.972467                                                               |
| 912 | 7121  | 6.412675                    | 7.911208                     | 7.971355                                                               |
| 911 | 7109  | 6.411775                    | 7.910097                     | 7.970242                                                               |

| $k$ | $p_k$ | $\frac{\sigma(N'_k)}{N'_k}$ | $\frac{N'_k}{\varphi(N'_k)}$ | $\frac{e^\gamma}{2} \log \log N'_k + \frac{0.73\dots}{\log \log N'_k}$ |
|-----|-------|-----------------------------|------------------------------|------------------------------------------------------------------------|
| 910 | 7103  | 6.410873                    | 7.908984                     | 7.969127                                                               |
| 909 | 7079  | 6.409970                    | 7.907871                     | 7.968012                                                               |
| 908 | 7069  | 6.409065                    | 7.906754                     | 7.966895                                                               |
| 907 | 7057  | 6.408159                    | 7.905635                     | 7.965777                                                               |
| 906 | 7043  | 6.407251                    | 7.904515                     | 7.964658                                                               |
| 905 | 7039  | 6.406341                    | 7.903393                     | 7.963538                                                               |
| 904 | 7027  | 6.405431                    | 7.902270                     | 7.962416                                                               |
| 903 | 7019  | 6.404520                    | 7.901145                     | 7.961293                                                               |
| 902 | 7013  | 6.403607                    | 7.900020                     | 7.960169                                                               |
| 901 | 7001  | 6.402694                    | 7.898893                     | 7.959044                                                               |
| 900 | 6997  | 6.401780                    | 7.897765                     | 7.957917                                                               |
| 899 | 6991  | 6.400865                    | 7.896636                     | 7.956789                                                               |
| 898 | 6983  | 6.399950                    | 7.895507                     | 7.955660                                                               |
| 897 | 6977  | 6.399033                    | 7.894376                     | 7.954529                                                               |
| 896 | 6971  | 6.398116                    | 7.893244                     | 7.953398                                                               |
| 895 | 6967  | 6.397199                    | 7.892112                     | 7.952264                                                               |
| 894 | 6961  | 6.396280                    | 7.890979                     | 7.951130                                                               |
| 893 | 6959  | 6.395362                    | 7.889846                     | 7.949994                                                               |
| 892 | 6949  | 6.394443                    | 7.888712                     | 7.948856                                                               |
| 891 | 6947  | 6.393523                    | 7.887577                     | 7.947717                                                               |
| 890 | 6917  | 6.392603                    | 7.886441                     | 7.946577                                                               |
| 889 | 6911  | 6.391679                    | 7.885301                     | 7.945436                                                               |
| 888 | 6907  | 6.390754                    | 7.884160                     | 7.944294                                                               |
| 887 | 6899  | 6.389829                    | 7.883019                     | 7.943150                                                               |
| 886 | 6883  | 6.388903                    | 7.881876                     | 7.942005                                                               |
| 885 | 6871  | 6.387975                    | 7.880731                     | 7.940858                                                               |
| 884 | 6869  | 6.387045                    | 7.879584                     | 7.939711                                                               |
| 883 | 6863  | 6.386115                    | 7.878437                     | 7.938562                                                               |
| 882 | 6857  | 6.385185                    | 7.877289                     | 7.937411                                                               |
| 881 | 6841  | 6.384254                    | 7.876140                     | 7.936259                                                               |
| 880 | 6833  | 6.383321                    | 7.874989                     | 7.935106                                                               |
| 879 | 6829  | 6.382387                    | 7.873836                     | 7.933952                                                               |
| 878 | 6827  | 6.381452                    | 7.872683                     | 7.932796                                                               |
| 877 | 6823  | 6.380518                    | 7.871530                     | 7.931639                                                               |
| 876 | 6803  | 6.379583                    | 7.870377                     | 7.930480                                                               |
| 875 | 6793  | 6.378645                    | 7.869220                     | 7.929320                                                               |
| 874 | 6791  | 6.377706                    | 7.868061                     | 7.928159                                                               |
| 873 | 6781  | 6.376767                    | 7.866903                     | 7.926996                                                               |
| 872 | 6779  | 6.375827                    | 7.865742                     | 7.925832                                                               |
| 871 | 6763  | 6.374886                    | 7.864582                     | 7.924666                                                               |
| 870 | 6761  | 6.373944                    | 7.863419                     | 7.923500                                                               |
| 869 | 6737  | 6.373001                    | 7.862256                     | 7.922331                                                               |
| 868 | 6733  | 6.372056                    | 7.861089                     | 7.921162                                                               |
| 867 | 6719  | 6.371109                    | 7.859922                     | 7.919991                                                               |

| $k$ | $p_k$ | $\frac{\sigma(N'_k)}{N'_k}$ | $\frac{N'_k}{\varphi(N'_k)}$ | $\frac{e^\gamma}{2} \log \log N'_k + \frac{0.73\dots}{\log \log N'_k}$ |
|-----|-------|-----------------------------|------------------------------|------------------------------------------------------------------------|
| 866 | 6709  | 6.370161                    | 7.858752                     | 7.918819                                                               |
| 865 | 6703  | 6.369212                    | 7.857580                     | 7.917645                                                               |
| 864 | 6701  | 6.368262                    | 7.856408                     | 7.916471                                                               |
| 863 | 6691  | 6.367312                    | 7.855236                     | 7.915294                                                               |
| 862 | 6689  | 6.366360                    | 7.854062                     | 7.914116                                                               |
| 861 | 6679  | 6.365409                    | 7.852888                     | 7.912937                                                               |
| 860 | 6673  | 6.364456                    | 7.851712                     | 7.911756                                                               |
| 859 | 6661  | 6.363502                    | 7.850535                     | 7.910574                                                               |
| 858 | 6659  | 6.362547                    | 7.849357                     | 7.909391                                                               |
| 857 | 6653  | 6.361591                    | 7.848178                     | 7.908205                                                               |
| 856 | 6637  | 6.360635                    | 7.846998                     | 7.907019                                                               |
| 855 | 6619  | 6.359677                    | 7.845816                     | 7.905831                                                               |
| 854 | 6607  | 6.358717                    | 7.844631                     | 7.904642                                                               |
| 853 | 6599  | 6.357754                    | 7.843443                     | 7.903452                                                               |
| 852 | 6581  | 6.356791                    | 7.842255                     | 7.902260                                                               |
| 851 | 6577  | 6.355825                    | 7.841063                     | 7.901067                                                               |
| 850 | 6571  | 6.354859                    | 7.839871                     | 7.899872                                                               |
| 849 | 6569  | 6.353892                    | 7.838678                     | 7.898676                                                               |
| 848 | 6563  | 6.352925                    | 7.837484                     | 7.897478                                                               |
| 847 | 6553  | 6.351957                    | 7.836290                     | 7.896279                                                               |
| 846 | 6551  | 6.350988                    | 7.835094                     | 7.895079                                                               |
| 845 | 6547  | 6.350019                    | 7.833898                     | 7.893876                                                               |
| 844 | 6529  | 6.349049                    | 7.832702                     | 7.892673                                                               |
| 843 | 6521  | 6.348076                    | 7.831502                     | 7.891468                                                               |
| 842 | 6491  | 6.347103                    | 7.830301                     | 7.890261                                                               |
| 841 | 6481  | 6.346125                    | 7.829095                     | 7.889054                                                               |
| 840 | 6473  | 6.345146                    | 7.827887                     | 7.887845                                                               |
| 839 | 6469  | 6.344166                    | 7.826678                     | 7.886634                                                               |
| 838 | 6451  | 6.343186                    | 7.825468                     | 7.885422                                                               |
| 837 | 6449  | 6.342203                    | 7.824255                     | 7.884209                                                               |
| 836 | 6427  | 6.341219                    | 7.823041                     | 7.882994                                                               |
| 835 | 6421  | 6.340233                    | 7.821824                     | 7.881778                                                               |
| 834 | 6397  | 6.339246                    | 7.820606                     | 7.880560                                                               |
| 833 | 6389  | 6.338255                    | 7.819383                     | 7.879341                                                               |
| 832 | 6379  | 6.337263                    | 7.818160                     | 7.878121                                                               |
| 831 | 6373  | 6.336270                    | 7.816934                     | 7.876899                                                               |
| 830 | 6367  | 6.335275                    | 7.815707                     | 7.875676                                                               |
| 829 | 6361  | 6.334281                    | 7.814480                     | 7.874451                                                               |
| 828 | 6359  | 6.333285                    | 7.813251                     | 7.873224                                                               |
| 827 | 6353  | 6.332289                    | 7.812023                     | 7.871996                                                               |
| 826 | 6343  | 6.331293                    | 7.810793                     | 7.870766                                                               |
| 825 | 6337  | 6.330295                    | 7.809562                     | 7.869535                                                               |
| 824 | 6329  | 6.329296                    | 7.808329                     | 7.868302                                                               |
| 823 | 6323  | 6.328296                    | 7.807095                     | 7.867068                                                               |

| $k$ | $p_k$ | $\frac{\sigma(N'_k)}{N'_k}$ | $\frac{N'_k}{\varphi(N'_k)}$ | $\frac{e^\gamma}{2} \log \log N'_k + \frac{0.73\dots}{\log \log N'_k}$ |
|-----|-------|-----------------------------|------------------------------|------------------------------------------------------------------------|
| 822 | 6317  | 6.327295                    | 7.805861                     | 7.865832                                                               |
| 821 | 6311  | 6.326294                    | 7.804625                     | 7.864594                                                               |
| 820 | 6301  | 6.325292                    | 7.803388                     | 7.863355                                                               |
| 819 | 6299  | 6.324288                    | 7.802150                     | 7.862115                                                               |
| 818 | 6287  | 6.323284                    | 7.800911                     | 7.860872                                                               |
| 817 | 6277  | 6.322278                    | 7.799671                     | 7.859628                                                               |
| 816 | 6271  | 6.321271                    | 7.798428                     | 7.858383                                                               |
| 815 | 6269  | 6.320263                    | 7.797184                     | 7.857136                                                               |
| 814 | 6263  | 6.319255                    | 7.795941                     | 7.855887                                                               |
| 813 | 6257  | 6.318247                    | 7.794696                     | 7.854637                                                               |
| 812 | 6247  | 6.317237                    | 7.793450                     | 7.853385                                                               |
| 811 | 6229  | 6.316226                    | 7.792203                     | 7.852131                                                               |
| 810 | 6221  | 6.315212                    | 7.790952                     | 7.850876                                                               |
| 809 | 6217  | 6.314197                    | 7.789699                     | 7.849620                                                               |
| 808 | 6211  | 6.313182                    | 7.788446                     | 7.848362                                                               |
| 807 | 6203  | 6.312165                    | 7.787192                     | 7.847102                                                               |
| 806 | 6199  | 6.311148                    | 7.785937                     | 7.845840                                                               |
| 805 | 6197  | 6.310130                    | 7.784681                     | 7.844577                                                               |
| 804 | 6173  | 6.309112                    | 7.783425                     | 7.843312                                                               |
| 803 | 6163  | 6.308090                    | 7.782164                     | 7.842046                                                               |
| 802 | 6151  | 6.307067                    | 7.780901                     | 7.840778                                                               |
| 801 | 6143  | 6.306041                    | 7.779636                     | 7.839509                                                               |
| 800 | 6133  | 6.305015                    | 7.778370                     | 7.838238                                                               |
| 799 | 6131  | 6.303987                    | 7.777101                     | 7.836965                                                               |
| 798 | 6121  | 6.302959                    | 7.775833                     | 7.835691                                                               |
| 797 | 6113  | 6.301930                    | 7.774563                     | 7.834415                                                               |
| 796 | 6101  | 6.300899                    | 7.773291                     | 7.833137                                                               |
| 795 | 6091  | 6.299866                    | 7.772017                     | 7.831858                                                               |
| 794 | 6089  | 6.298832                    | 7.770741                     | 7.830577                                                               |
| 793 | 6079  | 6.297798                    | 7.769464                     | 7.829295                                                               |
| 792 | 6073  | 6.296762                    | 7.768186                     | 7.828011                                                               |
| 791 | 6067  | 6.295725                    | 7.766907                     | 7.826725                                                               |
| 790 | 6053  | 6.294688                    | 7.765627                     | 7.825437                                                               |
| 789 | 6047  | 6.293648                    | 7.764344                     | 7.824148                                                               |
| 788 | 6043  | 6.292607                    | 7.763060                     | 7.822857                                                               |
| 787 | 6037  | 6.291566                    | 7.761775                     | 7.821564                                                               |
| 786 | 6029  | 6.290524                    | 7.760490                     | 7.820270                                                               |
| 785 | 6011  | 6.289481                    | 7.759203                     | 7.818973                                                               |
| 784 | 6007  | 6.288435                    | 7.757912                     | 7.817676                                                               |
| 783 | 5987  | 6.287388                    | 7.756620                     | 7.816376                                                               |
| 782 | 5981  | 6.286338                    | 7.755325                     | 7.815075                                                               |
| 781 | 5953  | 6.285287                    | 7.754028                     | 7.813773                                                               |
| 780 | 5939  | 6.284232                    | 7.752725                     | 7.812469                                                               |
| 779 | 5927  | 6.283174                    | 7.751420                     | 7.811163                                                               |

| $k$ | $p_k$ | $\frac{\sigma(N'_k)}{N'_k}$ | $\frac{N'_k}{\varphi(N'_k)}$ | $\frac{e^\gamma}{2} \log \log N'_k + \frac{0.73\dots}{\log \log N'_k}$ |
|-----|-------|-----------------------------|------------------------------|------------------------------------------------------------------------|
| 778 | 5923  | 6.282114                    | 7.750112                     | 7.809856                                                               |
| 777 | 5903  | 6.281053                    | 7.748804                     | 7.808547                                                               |
| 776 | 5897  | 6.279990                    | 7.747491                     | 7.807237                                                               |
| 775 | 5881  | 6.278925                    | 7.746177                     | 7.805925                                                               |
| 774 | 5879  | 6.277857                    | 7.744860                     | 7.804611                                                               |
| 773 | 5869  | 6.276790                    | 7.743543                     | 7.803296                                                               |
| 772 | 5867  | 6.275720                    | 7.742223                     | 7.801978                                                               |
| 771 | 5861  | 6.274651                    | 7.740904                     | 7.800659                                                               |
| 770 | 5857  | 6.273580                    | 7.739583                     | 7.799338                                                               |
| 769 | 5851  | 6.272510                    | 7.738262                     | 7.798015                                                               |
| 768 | 5849  | 6.271438                    | 7.736939                     | 7.796691                                                               |
| 767 | 5843  | 6.270366                    | 7.735616                     | 7.795364                                                               |
| 766 | 5839  | 6.269293                    | 7.734292                     | 7.794035                                                               |
| 765 | 5827  | 6.268219                    | 7.732968                     | 7.792705                                                               |
| 764 | 5821  | 6.267144                    | 7.731641                     | 7.791373                                                               |
| 763 | 5813  | 6.266067                    | 7.730312                     | 7.790039                                                               |
| 762 | 5807  | 6.264989                    | 7.728983                     | 7.788703                                                               |
| 761 | 5801  | 6.263911                    | 7.727652                     | 7.787366                                                               |
| 760 | 5791  | 6.262831                    | 7.726320                     | 7.786026                                                               |
| 759 | 5783  | 6.261750                    | 7.724985                     | 7.784685                                                               |
| 758 | 5779  | 6.260667                    | 7.723650                     | 7.783342                                                               |
| 757 | 5749  | 6.259584                    | 7.722313                     | 7.781997                                                               |
| 756 | 5743  | 6.258495                    | 7.720970                     | 7.780651                                                               |
| 755 | 5741  | 6.257406                    | 7.719625                     | 7.779302                                                               |
| 754 | 5737  | 6.256316                    | 7.718281                     | 7.777952                                                               |
| 753 | 5717  | 6.255226                    | 7.716935                     | 7.776600                                                               |
| 752 | 5711  | 6.254132                    | 7.715586                     | 7.775246                                                               |
| 751 | 5701  | 6.253037                    | 7.714235                     | 7.773891                                                               |
| 750 | 5693  | 6.251940                    | 7.712881                     | 7.772534                                                               |
| 749 | 5689  | 6.250842                    | 7.711527                     | 7.771174                                                               |
| 748 | 5683  | 6.249744                    | 7.710171                     | 7.769813                                                               |
| 747 | 5669  | 6.248644                    | 7.708814                     | 7.768450                                                               |
| 746 | 5659  | 6.247542                    | 7.707455                     | 7.767085                                                               |
| 745 | 5657  | 6.246438                    | 7.706093                     | 7.765718                                                               |
| 744 | 5653  | 6.245334                    | 7.704730                     | 7.764350                                                               |
| 743 | 5651  | 6.244230                    | 7.703367                     | 7.762979                                                               |
| 742 | 5647  | 6.243125                    | 7.702004                     | 7.761606                                                               |
| 741 | 5641  | 6.242020                    | 7.700640                     | 7.760231                                                               |
| 740 | 5639  | 6.240913                    | 7.699275                     | 7.758854                                                               |
| 739 | 5623  | 6.239807                    | 7.697910                     | 7.757475                                                               |
| 738 | 5591  | 6.238697                    | 7.696541                     | 7.756095                                                               |
| 737 | 5581  | 6.237582                    | 7.695164                     | 7.754713                                                               |
| 736 | 5573  | 6.236464                    | 7.693785                     | 7.753329                                                               |
| 735 | 5569  | 6.235345                    | 7.692405                     | 7.751943                                                               |

| $k$ | $p_k$ | $\frac{\sigma(N'_k)}{N'_k}$ | $\frac{N'_k}{\varphi(N'_k)}$ | $\frac{e^\gamma}{2} \log \log N'_k + \frac{0.73\dots}{\log \log N'_k}$ |
|-----|-------|-----------------------------|------------------------------|------------------------------------------------------------------------|
| 734 | 5563  | 6.234226                    | 7.691024                     | 7.750555                                                               |
| 733 | 5557  | 6.233105                    | 7.689641                     | 7.749166                                                               |
| 732 | 5531  | 6.231984                    | 7.688257                     | 7.747774                                                               |
| 731 | 5527  | 6.230857                    | 7.686867                     | 7.746381                                                               |
| 730 | 5521  | 6.229730                    | 7.685476                     | 7.744985                                                               |
| 729 | 5519  | 6.228602                    | 7.684084                     | 7.743588                                                               |
| 728 | 5507  | 6.227474                    | 7.682692                     | 7.742188                                                               |
| 727 | 5503  | 6.226343                    | 7.681297                     | 7.740787                                                               |
| 726 | 5501  | 6.225212                    | 7.679901                     | 7.739383                                                               |
| 725 | 5483  | 6.224080                    | 7.678505                     | 7.737978                                                               |
| 724 | 5479  | 6.222945                    | 7.677105                     | 7.736570                                                               |
| 723 | 5477  | 6.221810                    | 7.675703                     | 7.735161                                                               |
| 722 | 5471  | 6.220674                    | 7.674302                     | 7.733749                                                               |
| 721 | 5449  | 6.219537                    | 7.672899                     | 7.732335                                                               |
| 720 | 5443  | 6.218396                    | 7.671491                     | 7.730920                                                               |
| 719 | 5441  | 6.217254                    | 7.670082                     | 7.729503                                                               |
| 718 | 5437  | 6.216111                    | 7.668672                     | 7.728083                                                               |
| 717 | 5431  | 6.214968                    | 7.667262                     | 7.726661                                                               |
| 716 | 5419  | 6.213824                    | 7.665850                     | 7.725237                                                               |
| 715 | 5417  | 6.212678                    | 7.664435                     | 7.723811                                                               |
| 714 | 5413  | 6.211531                    | 7.663020                     | 7.722383                                                               |
| 713 | 5407  | 6.210384                    | 7.661605                     | 7.720953                                                               |
| 712 | 5399  | 6.209235                    | 7.660188                     | 7.719520                                                               |
| 711 | 5393  | 6.208085                    | 7.658769                     | 7.718086                                                               |
| 710 | 5387  | 6.206934                    | 7.657349                     | 7.716649                                                               |
| 709 | 5381  | 6.205783                    | 7.655927                     | 7.715210                                                               |
| 708 | 5351  | 6.204629                    | 7.654505                     | 7.713769                                                               |
| 707 | 5347  | 6.203470                    | 7.653074                     | 7.712326                                                               |
| 706 | 5333  | 6.202310                    | 7.651643                     | 7.710882                                                               |
| 705 | 5323  | 6.201147                    | 7.650208                     | 7.709435                                                               |
| 704 | 5309  | 6.199983                    | 7.648771                     | 7.707987                                                               |
| 703 | 5303  | 6.198815                    | 7.647330                     | 7.706536                                                               |
| 702 | 5297  | 6.197646                    | 7.645888                     | 7.705083                                                               |
| 701 | 5281  | 6.196477                    | 7.644445                     | 7.703628                                                               |
| 700 | 5279  | 6.195303                    | 7.642997                     | 7.702171                                                               |
| 699 | 5273  | 6.194130                    | 7.641549                     | 7.700712                                                               |
| 698 | 5261  | 6.192956                    | 7.640100                     | 7.699251                                                               |
| 697 | 5237  | 6.191779                    | 7.638648                     | 7.697787                                                               |
| 696 | 5233  | 6.190597                    | 7.637189                     | 7.696322                                                               |
| 695 | 5231  | 6.189414                    | 7.635730                     | 7.694855                                                               |
| 694 | 5227  | 6.188231                    | 7.634270                     | 7.693385                                                               |
| 693 | 5209  | 6.187047                    | 7.632810                     | 7.691913                                                               |
| 692 | 5197  | 6.185860                    | 7.631344                     | 7.690439                                                               |
| 691 | 5189  | 6.184670                    | 7.629876                     | 7.688963                                                               |

| $k$ | $p_k$ | $\frac{\sigma(N'_k)}{N'_k}$ | $\frac{N'_k}{\varphi(N'_k)}$ | $\frac{e^\gamma}{2} \log \log N'_k + \frac{0.73\dots}{\log \log N'_k}$ |
|-----|-------|-----------------------------|------------------------------|------------------------------------------------------------------------|
| 690 | 5179  | 6.183478                    | 7.628405                     | 7.687484                                                               |
| 689 | 5171  | 6.182284                    | 7.626932                     | 7.686004                                                               |
| 688 | 5167  | 6.181089                    | 7.625458                     | 7.684521                                                               |
| 687 | 5153  | 6.179893                    | 7.623982                     | 7.683036                                                               |
| 686 | 5147  | 6.178694                    | 7.622502                     | 7.681549                                                               |
| 685 | 5119  | 6.177494                    | 7.621021                     | 7.680060                                                               |
| 684 | 5113  | 6.176287                    | 7.619532                     | 7.678569                                                               |
| 683 | 5107  | 6.175079                    | 7.618042                     | 7.677076                                                               |
| 682 | 5101  | 6.173870                    | 7.616551                     | 7.675580                                                               |
| 681 | 5099  | 6.172660                    | 7.615057                     | 7.674082                                                               |
| 680 | 5087  | 6.171450                    | 7.613564                     | 7.672582                                                               |
| 679 | 5081  | 6.170237                    | 7.612067                     | 7.671080                                                               |
| 678 | 5077  | 6.169023                    | 7.610569                     | 7.669575                                                               |
| 677 | 5059  | 6.167808                    | 7.609070                     | 7.668067                                                               |
| 676 | 5051  | 6.166589                    | 7.607566                     | 7.666558                                                               |
| 675 | 5039  | 6.165368                    | 7.606060                     | 7.665047                                                               |
| 674 | 5023  | 6.164145                    | 7.604550                     | 7.663533                                                               |
| 673 | 5021  | 6.162918                    | 7.603037                     | 7.662017                                                               |
| 672 | 5011  | 6.161691                    | 7.601522                     | 7.660499                                                               |
| 671 | 5009  | 6.160462                    | 7.600005                     | 7.658978                                                               |
| 670 | 5003  | 6.159232                    | 7.598488                     | 7.657455                                                               |
| 669 | 4999  | 6.158001                    | 7.596969                     | 7.655930                                                               |
| 668 | 4993  | 6.156770                    | 7.595450                     | 7.654402                                                               |
| 667 | 4987  | 6.155537                    | 7.593928                     | 7.652872                                                               |
| 666 | 4973  | 6.154303                    | 7.592406                     | 7.651339                                                               |
| 665 | 4969  | 6.153065                    | 7.590879                     | 7.649804                                                               |
| 664 | 4967  | 6.151827                    | 7.589351                     | 7.648266                                                               |
| 663 | 4957  | 6.150589                    | 7.587823                     | 7.646726                                                               |
| 662 | 4951  | 6.149349                    | 7.586293                     | 7.645183                                                               |
| 661 | 4943  | 6.148107                    | 7.584760                     | 7.643638                                                               |
| 660 | 4937  | 6.146863                    | 7.583226                     | 7.642091                                                               |
| 659 | 4933  | 6.145618                    | 7.581690                     | 7.640541                                                               |
| 658 | 4931  | 6.144373                    | 7.580153                     | 7.638989                                                               |
| 657 | 4919  | 6.143127                    | 7.578616                     | 7.637434                                                               |
| 656 | 4909  | 6.141878                    | 7.577075                     | 7.635876                                                               |
| 655 | 4903  | 6.140627                    | 7.575531                     | 7.634316                                                               |
| 654 | 4889  | 6.139375                    | 7.573986                     | 7.632754                                                               |
| 653 | 4877  | 6.138120                    | 7.572437                     | 7.631190                                                               |
| 652 | 4871  | 6.136861                    | 7.570884                     | 7.629623                                                               |
| 651 | 4861  | 6.135602                    | 7.569330                     | 7.628053                                                               |
| 650 | 4831  | 6.134340                    | 7.567773                     | 7.626481                                                               |
| 649 | 4817  | 6.133070                    | 7.566207                     | 7.624908                                                               |
| 648 | 4813  | 6.131797                    | 7.564636                     | 7.623332                                                               |
| 647 | 4801  | 6.130524                    | 7.563064                     | 7.621754                                                               |



| $k$ | $p_k$ | $\frac{\sigma(N'_k)}{N'_k}$ | $\frac{N'_k}{\varphi(N'_k)}$ | $\frac{e^\gamma}{2} \log \log N'_k + \frac{0.73\dots}{\log \log N'_k}$ |
|-----|-------|-----------------------------|------------------------------|------------------------------------------------------------------------|
| 646 | 4799  | 6.129247                    | 7.561489                     | 7.620173                                                               |
| 645 | 4793  | 6.127970                    | 7.559913                     | 7.618589                                                               |
| 644 | 4789  | 6.126692                    | 7.558336                     | 7.617003                                                               |
| 643 | 4787  | 6.125413                    | 7.556758                     | 7.615414                                                               |
| 642 | 4783  | 6.124133                    | 7.555179                     | 7.613822                                                               |
| 641 | 4759  | 6.122853                    | 7.553599                     | 7.612228                                                               |
| 640 | 4751  | 6.121567                    | 7.552012                     | 7.610632                                                               |
| 639 | 4733  | 6.120279                    | 7.550423                     | 7.609033                                                               |
| 638 | 4729  | 6.118986                    | 7.548827                     | 7.607432                                                               |
| 637 | 4723  | 6.117692                    | 7.547231                     | 7.605828                                                               |
| 636 | 4721  | 6.116397                    | 7.545633                     | 7.604221                                                               |
| 635 | 4703  | 6.115102                    | 7.544035                     | 7.602612                                                               |
| 634 | 4691  | 6.113802                    | 7.542431                     | 7.601000                                                               |
| 633 | 4679  | 6.112499                    | 7.540823                     | 7.599386                                                               |
| 632 | 4673  | 6.111193                    | 7.539211                     | 7.597770                                                               |
| 631 | 4663  | 6.109885                    | 7.537598                     | 7.596151                                                               |
| 630 | 4657  | 6.108575                    | 7.535981                     | 7.594529                                                               |
| 629 | 4651  | 6.107264                    | 7.534363                     | 7.592904                                                               |
| 628 | 4649  | 6.105951                    | 7.532743                     | 7.591277                                                               |
| 627 | 4643  | 6.104638                    | 7.531123                     | 7.589647                                                               |
| 626 | 4639  | 6.103324                    | 7.529501                     | 7.588014                                                               |
| 625 | 4637  | 6.102008                    | 7.527878                     | 7.586378                                                               |
| 624 | 4621  | 6.100693                    | 7.526254                     | 7.584739                                                               |
| 623 | 4603  | 6.099373                    | 7.524626                     | 7.583098                                                               |
| 622 | 4597  | 6.098048                    | 7.522991                     | 7.581455                                                               |
| 621 | 4591  | 6.096722                    | 7.521354                     | 7.579808                                                               |
| 620 | 4583  | 6.095394                    | 7.519716                     | 7.578159                                                               |
| 619 | 4567  | 6.094064                    | 7.518075                     | 7.576508                                                               |
| 618 | 4561  | 6.092730                    | 7.516429                     | 7.574853                                                               |
| 617 | 4549  | 6.091395                    | 7.514781                     | 7.573196                                                               |
| 616 | 4547  | 6.090056                    | 7.513129                     | 7.571537                                                               |
| 615 | 4523  | 6.088717                    | 7.511477                     | 7.569874                                                               |
| 614 | 4519  | 6.087371                    | 7.509816                     | 7.568209                                                               |
| 613 | 4517  | 6.086024                    | 7.508154                     | 7.566541                                                               |
| 612 | 4513  | 6.084677                    | 7.506492                     | 7.564870                                                               |
| 611 | 4507  | 6.083329                    | 7.504829                     | 7.563197                                                               |
| 610 | 4493  | 6.081980                    | 7.503164                     | 7.561520                                                               |
| 609 | 4483  | 6.080626                    | 7.501494                     | 7.559841                                                               |
| 608 | 4481  | 6.079270                    | 7.499820                     | 7.558158                                                               |
| 607 | 4463  | 6.077914                    | 7.498147                     | 7.556473                                                               |
| 606 | 4457  | 6.076552                    | 7.496467                     | 7.554786                                                               |
| 605 | 4451  | 6.075189                    | 7.494785                     | 7.553095                                                               |
| 604 | 4447  | 6.073825                    | 7.493101                     | 7.551401                                                               |
| 603 | 4441  | 6.072459                    | 7.491416                     | 7.549705                                                               |

| $k$ | $p_k$ | $\frac{\sigma(N'_k)}{N'_k}$ | $\frac{N'_k}{\varphi(N'_k)}$ | $\frac{e^\gamma}{2} \log \log N'_k + \frac{0.73\dots}{\log \log N'_k}$ |
|-----|-------|-----------------------------|------------------------------|------------------------------------------------------------------------|
| 602 | 4423  | 6.071092                    | 7.489729                     | 7.548005                                                               |
| 601 | 4421  | 6.069720                    | 7.488036                     | 7.546303                                                               |
| 600 | 4409  | 6.068347                    | 7.486342                     | 7.544598                                                               |
| 599 | 4397  | 6.066971                    | 7.484644                     | 7.542890                                                               |
| 598 | 4391  | 6.065592                    | 7.482942                     | 7.541179                                                               |
| 597 | 4373  | 6.064211                    | 7.481238                     | 7.539465                                                               |
| 596 | 4363  | 6.062824                    | 7.479527                     | 7.537749                                                               |
| 595 | 4357  | 6.061435                    | 7.477813                     | 7.536030                                                               |
| 594 | 4349  | 6.060044                    | 7.476096                     | 7.534307                                                               |
| 593 | 4339  | 6.058651                    | 7.474377                     | 7.532582                                                               |
| 592 | 4337  | 6.057255                    | 7.472655                     | 7.530854                                                               |
| 591 | 4327  | 6.055859                    | 7.470932                     | 7.529123                                                               |
| 590 | 4297  | 6.054459                    | 7.469205                     | 7.527388                                                               |
| 589 | 4289  | 6.053051                    | 7.467467                     | 7.525652                                                               |
| 588 | 4283  | 6.051640                    | 7.465726                     | 7.523913                                                               |
| 587 | 4273  | 6.050227                    | 7.463983                     | 7.522170                                                               |
| 586 | 4271  | 6.048811                    | 7.462236                     | 7.520425                                                               |
| 585 | 4261  | 6.047396                    | 7.460489                     | 7.518676                                                               |
| 584 | 4259  | 6.045977                    | 7.458738                     | 7.516924                                                               |
| 583 | 4253  | 6.044557                    | 7.456986                     | 7.515169                                                               |
| 582 | 4243  | 6.043136                    | 7.455233                     | 7.513410                                                               |
| 581 | 4241  | 6.041713                    | 7.453476                     | 7.511649                                                               |
| 580 | 4231  | 6.040288                    | 7.451719                     | 7.509884                                                               |
| 579 | 4229  | 6.038861                    | 7.449957                     | 7.508116                                                               |
| 578 | 4219  | 6.037433                    | 7.448196                     | 7.506345                                                               |
| 577 | 4217  | 6.036003                    | 7.446430                     | 7.504570                                                               |
| 576 | 4211  | 6.034572                    | 7.444665                     | 7.502792                                                               |
| 575 | 4201  | 6.033139                    | 7.442897                     | 7.501011                                                               |
| 574 | 4177  | 6.031703                    | 7.441125                     | 7.499227                                                               |
| 573 | 4159  | 6.030260                    | 7.439343                     | 7.497440                                                               |
| 572 | 4157  | 6.028810                    | 7.437555                     | 7.495651                                                               |
| 571 | 4153  | 6.027360                    | 7.435766                     | 7.493858                                                               |
| 570 | 4139  | 6.025909                    | 7.433975                     | 7.492062                                                               |
| 569 | 4133  | 6.024453                    | 7.432179                     | 7.490263                                                               |
| 568 | 4129  | 6.022996                    | 7.430381                     | 7.488460                                                               |
| 567 | 4127  | 6.021538                    | 7.428581                     | 7.486654                                                               |
| 566 | 4111  | 6.020079                    | 7.426781                     | 7.484844                                                               |
| 565 | 4099  | 6.018615                    | 7.424975                     | 7.483032                                                               |
| 564 | 4093  | 6.017147                    | 7.423163                     | 7.481216                                                               |
| 563 | 4091  | 6.015677                    | 7.421350                     | 7.479397                                                               |
| 562 | 4079  | 6.014207                    | 7.419536                     | 7.477574                                                               |
| 561 | 4073  | 6.012733                    | 7.417717                     | 7.475749                                                               |
| 560 | 4057  | 6.011257                    | 7.415895                     | 7.473919                                                               |
| 559 | 4051  | 6.009776                    | 7.414067                     | 7.472087                                                               |

| $k$ | $p_k$ | $\frac{\sigma(N'_k)}{N'_k}$ | $\frac{N'_k}{\varphi(N'_k)}$ | $\frac{e^\gamma}{2} \log \log N'_k + \frac{0.73\dots}{\log \log N'_k}$ |
|-----|-------|-----------------------------|------------------------------|------------------------------------------------------------------------|
| 558 | 4049  | 6.008293                    | 7.412237                     | 7.470251                                                               |
| 557 | 4027  | 6.006809                    | 7.410407                     | 7.468412                                                               |
| 556 | 4021  | 6.005318                    | 7.408566                     | 7.466570                                                               |
| 555 | 4019  | 6.003825                    | 7.406724                     | 7.464724                                                               |
| 554 | 4013  | 6.002331                    | 7.404881                     | 7.462875                                                               |
| 553 | 4007  | 6.000836                    | 7.403036                     | 7.461022                                                               |
| 552 | 4003  | 5.999339                    | 7.401188                     | 7.459165                                                               |
| 551 | 4001  | 5.997841                    | 7.399339                     | 7.457305                                                               |
| 550 | 3989  | 5.996342                    | 7.397490                     | 7.455441                                                               |
| 549 | 3967  | 5.994839                    | 7.395636                     | 7.453574                                                               |
| 548 | 3947  | 5.993328                    | 7.393771                     | 7.451704                                                               |
| 547 | 3943  | 5.991810                    | 7.391898                     | 7.449831                                                               |
| 546 | 3931  | 5.990291                    | 7.390023                     | 7.447955                                                               |
| 545 | 3929  | 5.988767                    | 7.388143                     | 7.446075                                                               |
| 544 | 3923  | 5.987244                    | 7.386263                     | 7.444191                                                               |
| 543 | 3919  | 5.985718                    | 7.384380                     | 7.442304                                                               |
| 542 | 3917  | 5.984191                    | 7.382496                     | 7.440413                                                               |
| 541 | 3911  | 5.982663                    | 7.380611                     | 7.438517                                                               |
| 540 | 3907  | 5.981134                    | 7.378724                     | 7.436619                                                               |
| 539 | 3889  | 5.979604                    | 7.376835                     | 7.434716                                                               |
| 538 | 3881  | 5.978066                    | 7.374939                     | 7.432810                                                               |
| 537 | 3877  | 5.976527                    | 7.373038                     | 7.430901                                                               |
| 536 | 3863  | 5.974985                    | 7.371137                     | 7.428987                                                               |
| 535 | 3853  | 5.973439                    | 7.369228                     | 7.427070                                                               |
| 534 | 3851  | 5.971889                    | 7.367316                     | 7.425150                                                               |
| 533 | 3847  | 5.970339                    | 7.365403                     | 7.423226                                                               |
| 532 | 3833  | 5.968787                    | 7.363488                     | 7.421298                                                               |
| 531 | 3823  | 5.967230                    | 7.361567                     | 7.419366                                                               |
| 530 | 3821  | 5.965670                    | 7.359642                     | 7.417431                                                               |
| 529 | 3803  | 5.964109                    | 7.357715                     | 7.415491                                                               |
| 528 | 3797  | 5.962541                    | 7.355781                     | 7.413549                                                               |
| 527 | 3793  | 5.960971                    | 7.353843                     | 7.411602                                                               |
| 526 | 3779  | 5.959400                    | 7.351905                     | 7.409652                                                               |
| 525 | 3769  | 5.957824                    | 7.349959                     | 7.407698                                                               |
| 524 | 3767  | 5.956243                    | 7.348009                     | 7.405740                                                               |
| 523 | 3761  | 5.954663                    | 7.346058                     | 7.403778                                                               |
| 522 | 3739  | 5.953080                    | 7.344105                     | 7.401812                                                               |
| 521 | 3733  | 5.951488                    | 7.342141                     | 7.399843                                                               |
| 520 | 3727  | 5.949894                    | 7.340174                     | 7.397871                                                               |
| 519 | 3719  | 5.948298                    | 7.338205                     | 7.395894                                                               |
| 518 | 3709  | 5.946699                    | 7.336232                     | 7.393913                                                               |
| 517 | 3701  | 5.945096                    | 7.334254                     | 7.391928                                                               |
| 516 | 3697  | 5.943490                    | 7.332272                     | 7.389939                                                               |
| 515 | 3691  | 5.941883                    | 7.330289                     | 7.387947                                                               |

| $k$ | $p_k$ | $\frac{\sigma(N'_k)}{N'_k}$ | $\frac{N'_k}{\varphi(N'_k)}$ | $\frac{e^\gamma}{2} \log \log N'_k + \frac{0.73\dots}{\log \log N'_k}$ |
|-----|-------|-----------------------------|------------------------------|------------------------------------------------------------------------|
| 514 | 3677  | 5.940274                    | 7.328303                     | 7.385950                                                               |
| 513 | 3673  | 5.938659                    | 7.326310                     | 7.383949                                                               |
| 512 | 3671  | 5.937042                    | 7.324315                     | 7.381944                                                               |
| 511 | 3659  | 5.935425                    | 7.322320                     | 7.379935                                                               |
| 510 | 3643  | 5.933804                    | 7.320319                     | 7.377922                                                               |
| 509 | 3637  | 5.932175                    | 7.318309                     | 7.375905                                                               |
| 508 | 3631  | 5.930545                    | 7.316297                     | 7.373884                                                               |
| 507 | 3623  | 5.928912                    | 7.314282                     | 7.371859                                                               |
| 506 | 3617  | 5.927276                    | 7.312263                     | 7.369830                                                               |
| 505 | 3613  | 5.925638                    | 7.310242                     | 7.367797                                                               |
| 504 | 3607  | 5.923998                    | 7.308218                     | 7.365759                                                               |
| 503 | 3593  | 5.922356                    | 7.306192                     | 7.363717                                                               |
| 502 | 3583  | 5.920708                    | 7.304159                     | 7.361671                                                               |
| 501 | 3581  | 5.919056                    | 7.302120                     | 7.359621                                                               |
| 500 | 3571  | 5.917404                    | 7.300081                     | 7.357566                                                               |
| 499 | 3559  | 5.915747                    | 7.298037                     | 7.355508                                                               |
| 498 | 3557  | 5.914085                    | 7.295986                     | 7.353445                                                               |
| 497 | 3547  | 5.912423                    | 7.293935                     | 7.351378                                                               |
| 496 | 3541  | 5.910757                    | 7.291879                     | 7.349306                                                               |
| 495 | 3539  | 5.909088                    | 7.289819                     | 7.347230                                                               |
| 494 | 3533  | 5.907419                    | 7.287760                     | 7.345150                                                               |
| 493 | 3529  | 5.905747                    | 7.285697                     | 7.343065                                                               |
| 492 | 3527  | 5.904074                    | 7.283632                     | 7.340975                                                               |
| 491 | 3517  | 5.902401                    | 7.281567                     | 7.338880                                                               |
| 490 | 3511  | 5.900723                    | 7.279497                     | 7.336781                                                               |
| 489 | 3499  | 5.899043                    | 7.277423                     | 7.334678                                                               |
| 488 | 3491  | 5.897357                    | 7.275344                     | 7.332570                                                               |
| 487 | 3469  | 5.895669                    | 7.273260                     | 7.330458                                                               |
| 486 | 3467  | 5.893969                    | 7.271163                     | 7.328343                                                               |
| 485 | 3463  | 5.892270                    | 7.269066                     | 7.326222                                                               |
| 484 | 3461  | 5.890569                    | 7.266967                     | 7.324097                                                               |
| 483 | 3457  | 5.888867                    | 7.264867                     | 7.321967                                                               |
| 482 | 3449  | 5.887164                    | 7.262765                     | 7.319832                                                               |
| 481 | 3433  | 5.885458                    | 7.260660                     | 7.317692                                                               |
| 480 | 3413  | 5.883744                    | 7.258545                     | 7.315548                                                               |
| 479 | 3407  | 5.882021                    | 7.256418                     | 7.313401                                                               |
| 478 | 3391  | 5.880295                    | 7.254288                     | 7.311249                                                               |
| 477 | 3389  | 5.878561                    | 7.252149                     | 7.309093                                                               |
| 476 | 3373  | 5.876827                    | 7.250009                     | 7.306932                                                               |
| 475 | 3371  | 5.875085                    | 7.247859                     | 7.304767                                                               |
| 474 | 3361  | 5.873343                    | 7.245709                     | 7.302596                                                               |
| 473 | 3359  | 5.871596                    | 7.243554                     | 7.300421                                                               |
| 472 | 3347  | 5.869849                    | 7.241397                     | 7.298241                                                               |
| 471 | 3343  | 5.868095                    | 7.239234                     | 7.296056                                                               |

| $k$ | $p_k$ | $\frac{\sigma(N'_k)}{N'_k}$ | $\frac{N'_k}{\varphi(N'_k)}$ | $\frac{e^\gamma}{2} \log \log N'_k + \frac{0.73\dots}{\log \log N'_k}$ |
|-----|-------|-----------------------------|------------------------------|------------------------------------------------------------------------|
| 470 | 3331  | 5.866340                    | 7.237068                     | 7.293867                                                               |
| 469 | 3329  | 5.864580                    | 7.234895                     | 7.291673                                                               |
| 468 | 3323  | 5.862819                    | 7.232722                     | 7.289473                                                               |
| 467 | 3319  | 5.861055                    | 7.230546                     | 7.287269                                                               |
| 466 | 3313  | 5.859290                    | 7.228367                     | 7.285059                                                               |
| 465 | 3307  | 5.857522                    | 7.226185                     | 7.282844                                                               |
| 464 | 3301  | 5.855751                    | 7.224000                     | 7.280624                                                               |
| 463 | 3299  | 5.853977                    | 7.221812                     | 7.278399                                                               |
| 462 | 3271  | 5.852204                    | 7.219623                     | 7.276169                                                               |
| 461 | 3259  | 5.850415                    | 7.217415                     | 7.273935                                                               |
| 460 | 3257  | 5.848620                    | 7.215201                     | 7.271697                                                               |
| 459 | 3253  | 5.846825                    | 7.212986                     | 7.269453                                                               |
| 458 | 3251  | 5.845028                    | 7.210768                     | 7.267204                                                               |
| 457 | 3229  | 5.843231                    | 7.208550                     | 7.264949                                                               |
| 456 | 3221  | 5.841422                    | 7.206318                     | 7.262690                                                               |
| 455 | 3217  | 5.839609                    | 7.204080                     | 7.260426                                                               |
| 454 | 3209  | 5.837794                    | 7.201841                     | 7.258157                                                               |
| 453 | 3203  | 5.835976                    | 7.199597                     | 7.255882                                                               |
| 452 | 3191  | 5.834154                    | 7.197349                     | 7.253603                                                               |
| 451 | 3187  | 5.832326                    | 7.195094                     | 7.251318                                                               |
| 450 | 3181  | 5.830497                    | 7.192836                     | 7.249028                                                               |
| 449 | 3169  | 5.828665                    | 7.190575                     | 7.246732                                                               |
| 448 | 3167  | 5.826826                    | 7.188306                     | 7.244432                                                               |
| 447 | 3163  | 5.824987                    | 7.186036                     | 7.242125                                                               |
| 446 | 3137  | 5.823146                    | 7.183764                     | 7.239813                                                               |
| 445 | 3121  | 5.821290                    | 7.181474                     | 7.237497                                                               |
| 444 | 3119  | 5.819425                    | 7.179173                     | 7.235177                                                               |
| 443 | 3109  | 5.817560                    | 7.176871                     | 7.232851                                                               |
| 442 | 3089  | 5.815690                    | 7.174563                     | 7.230519                                                               |
| 441 | 3083  | 5.813807                    | 7.172240                     | 7.228183                                                               |
| 440 | 3079  | 5.811922                    | 7.169914                     | 7.225842                                                               |
| 439 | 3067  | 5.810035                    | 7.167585                     | 7.223494                                                               |
| 438 | 3061  | 5.808142                    | 7.165248                     | 7.221142                                                               |
| 437 | 3049  | 5.806245                    | 7.162907                     | 7.218784                                                               |
| 436 | 3041  | 5.804341                    | 7.160558                     | 7.216420                                                               |
| 435 | 3037  | 5.802433                    | 7.158203                     | 7.214051                                                               |
| 434 | 3023  | 5.800523                    | 7.155846                     | 7.211676                                                               |
| 433 | 3019  | 5.798605                    | 7.153479                     | 7.209297                                                               |
| 432 | 3011  | 5.796685                    | 7.151110                     | 7.206911                                                               |
| 431 | 3001  | 5.794760                    | 7.148735                     | 7.204519                                                               |
| 430 | 2999  | 5.792830                    | 7.146353                     | 7.202122                                                               |
| 429 | 2971  | 5.790899                    | 7.143970                     | 7.199718                                                               |
| 428 | 2969  | 5.788951                    | 7.141565                     | 7.197311                                                               |
| 427 | 2963  | 5.787001                    | 7.139160                     | 7.194897                                                               |

| $k$ | $p_k$ | $\frac{\sigma(N'_k)}{N'_k}$ | $\frac{N'_k}{\varphi(N'_k)}$ | $\frac{e^\gamma}{2} \log \log N'_k + \frac{0.73\dots}{\log \log N'_k}$ |
|-----|-------|-----------------------------|------------------------------|------------------------------------------------------------------------|
| 426 | 2957  | 5.785049                    | 7.136750                     | 7.192478                                                               |
| 425 | 2953  | 5.783093                    | 7.134337                     | 7.190052                                                               |
| 424 | 2939  | 5.781136                    | 7.131921                     | 7.187620                                                               |
| 423 | 2927  | 5.779169                    | 7.129494                     | 7.185183                                                               |
| 422 | 2917  | 5.777195                    | 7.127058                     | 7.182740                                                               |
| 421 | 2909  | 5.775216                    | 7.124615                     | 7.180291                                                               |
| 420 | 2903  | 5.773231                    | 7.122166                     | 7.177837                                                               |
| 419 | 2897  | 5.771243                    | 7.119713                     | 7.175376                                                               |
| 418 | 2887  | 5.769251                    | 7.117255                     | 7.172909                                                               |
| 417 | 2879  | 5.767254                    | 7.114790                     | 7.170437                                                               |
| 416 | 2861  | 5.765251                    | 7.112318                     | 7.167958                                                               |
| 415 | 2857  | 5.763237                    | 7.109833                     | 7.165474                                                               |
| 414 | 2851  | 5.761220                    | 7.107344                     | 7.162983                                                               |
| 413 | 2843  | 5.759200                    | 7.104851                     | 7.160487                                                               |
| 412 | 2837  | 5.757175                    | 7.102352                     | 7.157984                                                               |
| 411 | 2833  | 5.755147                    | 7.099848                     | 7.155474                                                               |
| 410 | 2819  | 5.753116                    | 7.097342                     | 7.152958                                                               |
| 409 | 2803  | 5.751076                    | 7.094825                     | 7.150436                                                               |
| 408 | 2801  | 5.749025                    | 7.092294                     | 7.147909                                                               |
| 407 | 2797  | 5.746973                    | 7.089761                     | 7.145374                                                               |
| 406 | 2791  | 5.744919                    | 7.087227                     | 7.142833                                                               |
| 405 | 2789  | 5.742861                    | 7.084687                     | 7.140285                                                               |
| 404 | 2777  | 5.740803                    | 7.082147                     | 7.137730                                                               |
| 403 | 2767  | 5.738737                    | 7.079597                     | 7.135169                                                               |
| 402 | 2753  | 5.736663                    | 7.077038                     | 7.132602                                                               |
| 401 | 2749  | 5.734580                    | 7.074468                     | 7.130029                                                               |
| 400 | 2741  | 5.732495                    | 7.071894                     | 7.127449                                                               |
| 399 | 2731  | 5.730404                    | 7.069314                     | 7.124862                                                               |
| 398 | 2729  | 5.728307                    | 7.066726                     | 7.122269                                                               |
| 397 | 2719  | 5.726209                    | 7.064136                     | 7.119668                                                               |
| 396 | 2713  | 5.724103                    | 7.061538                     | 7.117061                                                               |
| 395 | 2711  | 5.721994                    | 7.058935                     | 7.114447                                                               |
| 394 | 2707  | 5.719884                    | 7.056331                     | 7.111825                                                               |
| 393 | 2699  | 5.717772                    | 7.053725                     | 7.109196                                                               |
| 392 | 2693  | 5.715654                    | 7.051111                     | 7.106561                                                               |
| 391 | 2689  | 5.713533                    | 7.048493                     | 7.103918                                                               |
| 390 | 2687  | 5.711409                    | 7.045872                     | 7.101267                                                               |
| 389 | 2683  | 5.709284                    | 7.043249                     | 7.098609                                                               |
| 388 | 2677  | 5.707157                    | 7.040624                     | 7.095943                                                               |
| 387 | 2671  | 5.705026                    | 7.037994                     | 7.093270                                                               |
| 386 | 2663  | 5.702891                    | 7.035359                     | 7.090590                                                               |
| 385 | 2659  | 5.700750                    | 7.032717                     | 7.087902                                                               |
| 384 | 2657  | 5.698607                    | 7.030073                     | 7.085207                                                               |
| 383 | 2647  | 5.696463                    | 7.027427                     | 7.082504                                                               |

| $k$ | $p_k$ | $\frac{\sigma(N'_k)}{N'_k}$ | $\frac{N'_k}{\varphi(N'_k)}$ | $\frac{e^\gamma}{2} \log \log N'_k + \frac{0.73\dots}{\log \log N'_k}$ |
|-----|-------|-----------------------------|------------------------------|------------------------------------------------------------------------|
| 382 | 2633  | 5.694312                    | 7.024772                     | 7.079793                                                               |
| 381 | 2621  | 5.692150                    | 7.022104                     | 7.077077                                                               |
| 380 | 2617  | 5.689979                    | 7.019425                     | 7.074353                                                               |
| 379 | 2609  | 5.687805                    | 7.016742                     | 7.071621                                                               |
| 378 | 2593  | 5.685626                    | 7.014053                     | 7.068882                                                               |
| 377 | 2591  | 5.683434                    | 7.011348                     | 7.066137                                                               |
| 376 | 2579  | 5.681242                    | 7.008642                     | 7.063383                                                               |
| 375 | 2557  | 5.679040                    | 7.005924                     | 7.060623                                                               |
| 374 | 2551  | 5.676819                    | 7.003184                     | 7.057857                                                               |
| 373 | 2549  | 5.674595                    | 7.000439                     | 7.055082                                                               |
| 372 | 2543  | 5.672370                    | 6.997693                     | 7.052300                                                               |
| 371 | 2539  | 5.670140                    | 6.994941                     | 7.049509                                                               |
| 370 | 2531  | 5.667908                    | 6.992186                     | 7.046710                                                               |
| 369 | 2521  | 5.665669                    | 6.989423                     | 7.043903                                                               |
| 368 | 2503  | 5.663423                    | 6.986651                     | 7.041089                                                               |
| 367 | 2477  | 5.661161                    | 6.983860                     | 7.038269                                                               |
| 366 | 2473  | 5.658876                    | 6.981040                     | 7.035443                                                               |
| 365 | 2467  | 5.656589                    | 6.978217                     | 7.032608                                                               |
| 364 | 2459  | 5.654297                    | 6.975389                     | 7.029765                                                               |
| 363 | 2447  | 5.651999                    | 6.972552                     | 7.026915                                                               |
| 362 | 2441  | 5.649690                    | 6.969703                     | 7.024057                                                               |
| 361 | 2437  | 5.647376                    | 6.966847                     | 7.021190                                                               |
| 360 | 2423  | 5.645060                    | 6.963989                     | 7.018315                                                               |
| 359 | 2417  | 5.642731                    | 6.961114                     | 7.015432                                                               |
| 358 | 2411  | 5.640397                    | 6.958234                     | 7.012541                                                               |
| 357 | 2399  | 5.638059                    | 6.955348                     | 7.009641                                                               |
| 356 | 2393  | 5.635710                    | 6.952449                     | 7.006734                                                               |
| 355 | 2389  | 5.633356                    | 6.949544                     | 7.003818                                                               |
| 354 | 2383  | 5.630998                    | 6.946635                     | 7.000893                                                               |
| 353 | 2381  | 5.628636                    | 6.943720                     | 6.997959                                                               |
| 352 | 2377  | 5.626273                    | 6.940803                     | 6.995015                                                               |
| 351 | 2371  | 5.623908                    | 6.937883                     | 6.992063                                                               |
| 350 | 2357  | 5.621537                    | 6.934957                     | 6.989101                                                               |
| 349 | 2351  | 5.619153                    | 6.932015                     | 6.986132                                                               |
| 348 | 2347  | 5.616763                    | 6.929066                     | 6.983153                                                               |
| 347 | 2341  | 5.614371                    | 6.926114                     | 6.980166                                                               |
| 346 | 2339  | 5.611974                    | 6.923155                     | 6.977169                                                               |
| 345 | 2333  | 5.609576                    | 6.920196                     | 6.974162                                                               |
| 344 | 2311  | 5.607172                    | 6.917229                     | 6.971146                                                               |
| 343 | 2309  | 5.604747                    | 6.914236                     | 6.968123                                                               |
| 342 | 2297  | 5.602321                    | 6.911242                     | 6.965090                                                               |
| 341 | 2293  | 5.599883                    | 6.908233                     | 6.962049                                                               |
| 340 | 2287  | 5.597442                    | 6.905220                     | 6.958997                                                               |
| 339 | 2281  | 5.594995                    | 6.902201                     | 6.955937                                                               |

| $k$ | $p_k$ | $\frac{\sigma(N'_k)}{N'_k}$ | $\frac{N'_k}{\varphi(N'_k)}$ | $\frac{e^\gamma}{2} \log \log N'_k + \frac{0.73\dots}{\log \log N'_k}$ |
|-----|-------|-----------------------------|------------------------------|------------------------------------------------------------------------|
| 338 | 2273  | 5.592544                    | 6.899175                     | 6.952866                                                               |
| 337 | 2269  | 5.590084                    | 6.896140                     | 6.949787                                                               |
| 336 | 2267  | 5.587622                    | 6.893100                     | 6.946697                                                               |
| 335 | 2251  | 5.585158                    | 6.890060                     | 6.943597                                                               |
| 334 | 2243  | 5.582678                    | 6.886999                     | 6.940488                                                               |
| 333 | 2239  | 5.580190                    | 6.883928                     | 6.937370                                                               |
| 332 | 2237  | 5.577699                    | 6.880854                     | 6.934242                                                               |
| 331 | 2221  | 5.575207                    | 6.877778                     | 6.931103                                                               |
| 330 | 2213  | 5.572698                    | 6.874681                     | 6.927956                                                               |
| 329 | 2207  | 5.570180                    | 6.871575                     | 6.924799                                                               |
| 328 | 2203  | 5.567658                    | 6.868461                     | 6.921631                                                               |
| 327 | 2179  | 5.565132                    | 6.865343                     | 6.918453                                                               |
| 326 | 2161  | 5.562579                    | 6.862193                     | 6.915268                                                               |
| 325 | 2153  | 5.560006                    | 6.859017                     | 6.912075                                                               |
| 324 | 2143  | 5.557425                    | 6.855831                     | 6.908872                                                               |
| 323 | 2141  | 5.554833                    | 6.852632                     | 6.905659                                                               |
| 322 | 2137  | 5.552239                    | 6.849432                     | 6.902435                                                               |
| 321 | 2131  | 5.549642                    | 6.846226                     | 6.899200                                                               |
| 320 | 2129  | 5.547039                    | 6.843014                     | 6.895954                                                               |
| 319 | 2113  | 5.544435                    | 6.839800                     | 6.892696                                                               |
| 318 | 2111  | 5.541812                    | 6.836563                     | 6.889430                                                               |
| 317 | 2099  | 5.539188                    | 6.833324                     | 6.886151                                                               |
| 316 | 2089  | 5.536551                    | 6.830068                     | 6.882863                                                               |
| 315 | 2087  | 5.533902                    | 6.826799                     | 6.879565                                                               |
| 314 | 2083  | 5.531251                    | 6.823528                     | 6.876255                                                               |
| 313 | 2081  | 5.528597                    | 6.820252                     | 6.872933                                                               |
| 312 | 2069  | 5.525942                    | 6.816975                     | 6.869599                                                               |
| 311 | 2063  | 5.523272                    | 6.813680                     | 6.866255                                                               |
| 310 | 2053  | 5.520596                    | 6.810377                     | 6.862899                                                               |
| 309 | 2039  | 5.517908                    | 6.807060                     | 6.859533                                                               |
| 308 | 2029  | 5.515204                    | 6.803721                     | 6.856156                                                               |
| 307 | 2027  | 5.512487                    | 6.800368                     | 6.852769                                                               |
| 306 | 2017  | 5.509769                    | 6.797013                     | 6.849370                                                               |
| 305 | 2011  | 5.507038                    | 6.793643                     | 6.845959                                                               |
| 304 | 2003  | 5.504301                    | 6.790265                     | 6.842537                                                               |
| 303 | 1999  | 5.501554                    | 6.786875                     | 6.839103                                                               |
| 302 | 1997  | 5.498804                    | 6.783480                     | 6.835656                                                               |
| 301 | 1993  | 5.496052                    | 6.780083                     | 6.832197                                                               |
| 300 | 1987  | 5.493295                    | 6.776681                     | 6.828724                                                               |
| 299 | 1979  | 5.490532                    | 6.773271                     | 6.825240                                                               |
| 298 | 1973  | 5.487759                    | 6.769848                     | 6.821743                                                               |
| 297 | 1951  | 5.484979                    | 6.766417                     | 6.818234                                                               |
| 296 | 1949  | 5.482169                    | 6.762949                     | 6.814716                                                               |
| 295 | 1933  | 5.479358                    | 6.759479                     | 6.811184                                                               |



| $k$ | $p_k$ | $\frac{\sigma(N'_k)}{N'_k}$ | $\frac{N'_k}{\varphi(N'_k)}$ | $\frac{e^\gamma}{2} \log \log N'_k + \frac{0.73\dots}{\log \log N'_k}$ |
|-----|-------|-----------------------------|------------------------------|------------------------------------------------------------------------|
| 294 | 1931  | 5.476525                    | 6.755982                     | 6.807642                                                               |
| 293 | 1913  | 5.473690                    | 6.752483                     | 6.804086                                                               |
| 292 | 1907  | 5.470830                    | 6.748953                     | 6.800520                                                               |
| 291 | 1901  | 5.467963                    | 6.745414                     | 6.796942                                                               |
| 290 | 1889  | 5.465088                    | 6.741866                     | 6.793350                                                               |
| 289 | 1879  | 5.462196                    | 6.738297                     | 6.789746                                                               |
| 288 | 1877  | 5.459291                    | 6.734711                     | 6.786130                                                               |
| 287 | 1873  | 5.456384                    | 6.731123                     | 6.782500                                                               |
| 286 | 1871  | 5.453472                    | 6.727529                     | 6.778856                                                               |
| 285 | 1867  | 5.450559                    | 6.723933                     | 6.775197                                                               |
| 284 | 1861  | 5.447641                    | 6.720332                     | 6.771524                                                               |
| 283 | 1847  | 5.444716                    | 6.716721                     | 6.767837                                                               |
| 282 | 1831  | 5.441769                    | 6.713084                     | 6.764139                                                               |
| 281 | 1823  | 5.438799                    | 6.709418                     | 6.760429                                                               |
| 280 | 1811  | 5.435817                    | 6.705737                     | 6.756706                                                               |
| 279 | 1801  | 5.432817                    | 6.702035                     | 6.752970                                                               |
| 278 | 1789  | 5.429802                    | 6.698313                     | 6.749221                                                               |
| 277 | 1787  | 5.426769                    | 6.694569                     | 6.745459                                                               |
| 276 | 1783  | 5.423734                    | 6.690823                     | 6.741682                                                               |
| 275 | 1777  | 5.420694                    | 6.687070                     | 6.737889                                                               |
| 274 | 1759  | 5.417645                    | 6.683307                     | 6.734082                                                               |
| 273 | 1753  | 5.414567                    | 6.679508                     | 6.730264                                                               |
| 272 | 1747  | 5.411480                    | 6.675697                     | 6.726431                                                               |
| 271 | 1741  | 5.408384                    | 6.671876                     | 6.722582                                                               |
| 270 | 1733  | 5.405279                    | 6.668044                     | 6.718719                                                               |
| 269 | 1723  | 5.402162                    | 6.664196                     | 6.714841                                                               |
| 268 | 1721  | 5.399028                    | 6.660328                     | 6.710949                                                               |
| 267 | 1709  | 5.395893                    | 6.656458                     | 6.707040                                                               |
| 266 | 1699  | 5.392738                    | 6.652563                     | 6.703118                                                               |
| 265 | 1697  | 5.389565                    | 6.648648                     | 6.699181                                                               |
| 264 | 1693  | 5.386391                    | 6.644730                     | 6.695227                                                               |
| 263 | 1669  | 5.383212                    | 6.640805                     | 6.691256                                                               |
| 262 | 1667  | 5.379988                    | 6.636826                     | 6.687275                                                               |
| 261 | 1663  | 5.376763                    | 6.632845                     | 6.683277                                                               |
| 260 | 1657  | 5.373532                    | 6.628856                     | 6.679262                                                               |
| 259 | 1637  | 5.370291                    | 6.624856                     | 6.675230                                                               |
| 258 | 1627  | 5.367012                    | 6.620809                     | 6.671187                                                               |
| 257 | 1621  | 5.363715                    | 6.616740                     | 6.667128                                                               |
| 256 | 1619  | 5.360408                    | 6.612658                     | 6.663053                                                               |
| 255 | 1613  | 5.357100                    | 6.608573                     | 6.658959                                                               |
| 254 | 1609  | 5.353780                    | 6.604476                     | 6.654848                                                               |
| 253 | 1607  | 5.350455                    | 6.600372                     | 6.650719                                                               |
| 252 | 1601  | 5.347128                    | 6.596264                     | 6.646572                                                               |
| 251 | 1597  | 5.343790                    | 6.592144                     | 6.642407                                                               |

| $k$ | $p_k$ | $\frac{\sigma(N'_k)}{N'_k}$ | $\frac{N'_k}{\varphi(N'_k)}$ | $\frac{e^\gamma}{2} \log \log N'_k + \frac{0.73\dots}{\log \log N'_k}$ |
|-----|-------|-----------------------------|------------------------------|------------------------------------------------------------------------|
| 250 | 1583  | 5.340446                    | 6.588016                     | 6.638223                                                               |
| 249 | 1579  | 5.337074                    | 6.583855                     | 6.634025                                                               |
| 248 | 1571  | 5.333696                    | 6.579685                     | 6.629808                                                               |
| 247 | 1567  | 5.330304                    | 6.575497                     | 6.625574                                                               |
| 246 | 1559  | 5.326904                    | 6.571301                     | 6.621320                                                               |
| 245 | 1553  | 5.323489                    | 6.567086                     | 6.617049                                                               |
| 244 | 1549  | 5.320064                    | 6.562857                     | 6.612760                                                               |
| 243 | 1543  | 5.316631                    | 6.558620                     | 6.608451                                                               |
| 242 | 1531  | 5.313188                    | 6.554369                     | 6.604123                                                               |
| 241 | 1523  | 5.309720                    | 6.550088                     | 6.599778                                                               |
| 240 | 1511  | 5.306236                    | 6.545788                     | 6.595415                                                               |
| 239 | 1499  | 5.302726                    | 6.541455                     | 6.591035                                                               |
| 238 | 1493  | 5.299191                    | 6.537092                     | 6.586638                                                               |
| 237 | 1489  | 5.295644                    | 6.532713                     | 6.582221                                                               |
| 236 | 1487  | 5.292090                    | 6.528326                     | 6.577784                                                               |
| 235 | 1483  | 5.288534                    | 6.523936                     | 6.573325                                                               |
| 234 | 1481  | 5.284970                    | 6.519536                     | 6.568844                                                               |
| 233 | 1471  | 5.281404                    | 6.515134                     | 6.564342                                                               |
| 232 | 1459  | 5.277816                    | 6.510705                     | 6.559821                                                               |
| 231 | 1453  | 5.274201                    | 6.506243                     | 6.555282                                                               |
| 230 | 1451  | 5.270574                    | 6.501765                     | 6.550721                                                               |
| 229 | 1447  | 5.266944                    | 6.497284                     | 6.546138                                                               |
| 228 | 1439  | 5.263306                    | 6.492794                     | 6.541533                                                               |
| 227 | 1433  | 5.259651                    | 6.488282                     | 6.536907                                                               |
| 226 | 1429  | 5.255983                    | 6.483754                     | 6.532259                                                               |
| 225 | 1427  | 5.252308                    | 6.479217                     | 6.527588                                                               |
| 224 | 1423  | 5.248630                    | 6.474676                     | 6.522893                                                               |
| 223 | 1409  | 5.244944                    | 6.470126                     | 6.518175                                                               |
| 222 | 1399  | 5.241224                    | 6.465534                     | 6.513438                                                               |
| 221 | 1381  | 5.237480                    | 6.460913                     | 6.508680                                                               |
| 220 | 1373  | 5.233691                    | 6.456234                     | 6.503905                                                               |
| 219 | 1367  | 5.229882                    | 6.451532                     | 6.499107                                                               |
| 218 | 1361  | 5.226059                    | 6.446813                     | 6.494287                                                               |
| 217 | 1327  | 5.222222                    | 6.442076                     | 6.489442                                                               |
| 216 | 1321  | 5.218289                    | 6.437221                     | 6.484588                                                               |
| 215 | 1319  | 5.214342                    | 6.432348                     | 6.479710                                                               |
| 214 | 1307  | 5.210392                    | 6.427472                     | 6.474806                                                               |
| 213 | 1303  | 5.206408                    | 6.422554                     | 6.469881                                                               |
| 212 | 1301  | 5.202415                    | 6.417625                     | 6.464930                                                               |
| 211 | 1297  | 5.198420                    | 6.412692                     | 6.459952                                                               |
| 210 | 1291  | 5.194415                    | 6.407748                     | 6.454949                                                               |
| 209 | 1289  | 5.190394                    | 6.402784                     | 6.449919                                                               |
| 208 | 1283  | 5.186371                    | 6.397817                     | 6.444862                                                               |
| 207 | 1279  | 5.182332                    | 6.392830                     | 6.439779                                                               |

| $k$ | $p_k$ | $\frac{\sigma(N'_k)}{N'_k}$ | $\frac{N'_k}{\varphi(N'_k)}$ | $\frac{e^\gamma}{2} \log \log N'_k + \frac{0.73\dots}{\log \log N'_k}$ |
|-----|-------|-----------------------------|------------------------------|------------------------------------------------------------------------|
| 206 | 1277  | 5.178283                    | 6.387832                     | 6.434669                                                               |
| 205 | 1259  | 5.174231                    | 6.382830                     | 6.429530                                                               |
| 204 | 1249  | 5.170125                    | 6.377760                     | 6.424371                                                               |
| 203 | 1237  | 5.165988                    | 6.372654                     | 6.419187                                                               |
| 202 | 1231  | 5.161816                    | 6.367502                     | 6.413980                                                               |
| 201 | 1229  | 5.157626                    | 6.362330                     | 6.408746                                                               |
| 200 | 1223  | 5.153433                    | 6.357153                     | 6.403481                                                               |
| 199 | 1217  | 5.149222                    | 6.351955                     | 6.398188                                                               |
| 198 | 1213  | 5.144995                    | 6.346735                     | 6.392867                                                               |
| 197 | 1201  | 5.140757                    | 6.341503                     | 6.387516                                                               |
| 196 | 1193  | 5.136480                    | 6.336223                     | 6.382140                                                               |
| 195 | 1187  | 5.132178                    | 6.330912                     | 6.376736                                                               |
| 194 | 1181  | 5.127858                    | 6.325578                     | 6.371303                                                               |
| 193 | 1171  | 5.123520                    | 6.320222                     | 6.365839                                                               |
| 192 | 1163  | 5.119148                    | 6.314825                     | 6.360349                                                               |
| 191 | 1153  | 5.114750                    | 6.309395                     | 6.354829                                                               |
| 190 | 1151  | 5.110318                    | 6.303923                     | 6.349281                                                               |
| 189 | 1129  | 5.105882                    | 6.298446                     | 6.343699                                                               |
| 188 | 1123  | 5.101363                    | 6.292867                     | 6.338097                                                               |
| 187 | 1117  | 5.096825                    | 6.287264                     | 6.332463                                                               |
| 186 | 1109  | 5.092266                    | 6.281635                     | 6.326797                                                               |
| 185 | 1103  | 5.087678                    | 6.275971                     | 6.321101                                                               |
| 184 | 1097  | 5.083070                    | 6.270281                     | 6.315372                                                               |
| 183 | 1093  | 5.078440                    | 6.264565                     | 6.309609                                                               |
| 182 | 1091  | 5.073798                    | 6.258833                     | 6.303812                                                               |
| 181 | 1087  | 5.069152                    | 6.253097                     | 6.297978                                                               |
| 180 | 1069  | 5.064493                    | 6.247344                     | 6.292108                                                               |
| 179 | 1063  | 5.059760                    | 6.241500                     | 6.286213                                                               |
| 178 | 1061  | 5.055004                    | 6.235628                     | 6.280282                                                               |
| 177 | 1051  | 5.050244                    | 6.229751                     | 6.274314                                                               |
| 176 | 1049  | 5.045444                    | 6.223824                     | 6.268312                                                               |
| 175 | 1039  | 5.040639                    | 6.217891                     | 6.262271                                                               |
| 174 | 1033  | 5.035792                    | 6.211906                     | 6.256197                                                               |
| 173 | 1031  | 5.030922                    | 6.205893                     | 6.250085                                                               |
| 172 | 1021  | 5.026047                    | 6.199873                     | 6.243933                                                               |
| 171 | 1019  | 5.021129                    | 6.193801                     | 6.237745                                                               |
| 170 | 1013  | 5.016206                    | 6.187723                     | 6.231516                                                               |
| 169 | 1009  | 5.011259                    | 6.181614                     | 6.225248                                                               |
| 168 | 997   | 5.006298                    | 6.175488                     | 6.218938                                                               |
| 167 | 991   | 5.001281                    | 6.169294                     | 6.212594                                                               |
| 166 | 983   | 4.996240                    | 6.163068                     | 6.206209                                                               |
| 165 | 977   | 4.991162                    | 6.156799                     | 6.199785                                                               |
| 164 | 971   | 4.986059                    | 6.150497                     | 6.193320                                                               |
| 163 | 967   | 4.980929                    | 6.144163                     | 6.186813                                                               |

| $k$ | $p_k$ | $\frac{\sigma(N'_k)}{N'_k}$ | $\frac{N'_k}{\varphi(N'_k)}$ | $\frac{e^\gamma}{2} \log \log N'_k + \frac{0.73\dots}{\log \log N'_k}$ |
|-----|-------|-----------------------------|------------------------------|------------------------------------------------------------------------|
| 162 | 953   | 4.975783                    | 6.137809                     | 6.180261                                                               |
| 161 | 947   | 4.970568                    | 6.131369                     | 6.173674                                                               |
| 160 | 941   | 4.965325                    | 6.124894                     | 6.167043                                                               |
| 159 | 937   | 4.960054                    | 6.118385                     | 6.160368                                                               |
| 158 | 929   | 4.954766                    | 6.111855                     | 6.153646                                                               |
| 157 | 919   | 4.949438                    | 6.105276                     | 6.146881                                                               |
| 156 | 911   | 4.944058                    | 6.098633                     | 6.140075                                                               |
| 155 | 907   | 4.938637                    | 6.091939                     | 6.133224                                                               |
| 154 | 887   | 4.933198                    | 6.085222                     | 6.126324                                                               |
| 153 | 883   | 4.927643                    | 6.078361                     | 6.119392                                                               |
| 152 | 881   | 4.922068                    | 6.071478                     | 6.112410                                                               |
| 151 | 877   | 4.916488                    | 6.064586                     | 6.105374                                                               |
| 150 | 863   | 4.910888                    | 6.057671                     | 6.098286                                                               |
| 149 | 859   | 4.905204                    | 6.050652                     | 6.091157                                                               |
| 148 | 857   | 4.899500                    | 6.043608                     | 6.083976                                                               |
| 147 | 853   | 4.893790                    | 6.036556                     | 6.076737                                                               |
| 146 | 839   | 4.888060                    | 6.029479                     | 6.069444                                                               |
| 145 | 829   | 4.882240                    | 6.022292                     | 6.062108                                                               |
| 144 | 827   | 4.876358                    | 6.015028                     | 6.054723                                                               |
| 143 | 823   | 4.870469                    | 6.007755                     | 6.047278                                                               |
| 142 | 821   | 4.864558                    | 6.000455                     | 6.039775                                                               |
| 141 | 811   | 4.858640                    | 5.993146                     | 6.032210                                                               |
| 140 | 809   | 4.852657                    | 5.985756                     | 6.024594                                                               |
| 139 | 797   | 4.846666                    | 5.978357                     | 6.016914                                                               |
| 138 | 787   | 4.840592                    | 5.970856                     | 6.009183                                                               |
| 137 | 773   | 4.834449                    | 5.963269                     | 6.001399                                                               |
| 136 | 769   | 4.828203                    | 5.955555                     | 5.993566                                                               |
| 135 | 761   | 4.821933                    | 5.947810                     | 5.985669                                                               |
| 134 | 757   | 4.815605                    | 5.939995                     | 5.977713                                                               |
| 133 | 751   | 4.809252                    | 5.932148                     | 5.969691                                                               |
| 132 | 743   | 4.802857                    | 5.924249                     | 5.961605                                                               |
| 131 | 739   | 4.796401                    | 5.916275                     | 5.953456                                                               |
| 130 | 733   | 4.789920                    | 5.908270                     | 5.945239                                                               |
| 129 | 727   | 4.783394                    | 5.900209                     | 5.936954                                                               |
| 128 | 719   | 4.776823                    | 5.892093                     | 5.928600                                                               |
| 127 | 709   | 4.770189                    | 5.883899                     | 5.920181                                                               |
| 126 | 701   | 4.763470                    | 5.875600                     | 5.911698                                                               |
| 125 | 691   | 4.756685                    | 5.867218                     | 5.903148                                                               |
| 124 | 683   | 4.749811                    | 5.858727                     | 5.894532                                                               |
| 123 | 677   | 4.742867                    | 5.850149                     | 5.885847                                                               |
| 122 | 673   | 4.735871                    | 5.841508                     | 5.877087                                                               |
| 121 | 661   | 4.728845                    | 5.832828                     | 5.868246                                                               |
| 120 | 659   | 4.721701                    | 5.824004                     | 5.859341                                                               |
| 119 | 653   | 4.714547                    | 5.815166                     | 5.850348                                                               |

| $k$ | $p_k$ | $\frac{\sigma(N'_k)}{N'_k}$ | $\frac{N'_k}{\varphi(N'_k)}$ | $\frac{e^\gamma}{2} \log \log N'_k + \frac{0.73\dots}{\log \log N'_k}$ |
|-----|-------|-----------------------------|------------------------------|------------------------------------------------------------------------|
| 118 | 647   | 4.707338                    | 5.806261                     | 5.841276                                                               |
| 117 | 643   | 4.700074                    | 5.797287                     | 5.832122                                                               |
| 116 | 641   | 4.692776                    | 5.788271                     | 5.822880                                                               |
| 115 | 631   | 4.685466                    | 5.779241                     | 5.813545                                                               |
| 114 | 619   | 4.678052                    | 5.770082                     | 5.804132                                                               |
| 113 | 617   | 4.670507                    | 5.760760                     | 5.794646                                                               |
| 112 | 613   | 4.662950                    | 5.751423                     | 5.785061                                                               |
| 111 | 607   | 4.655355                    | 5.742041                     | 5.775380                                                               |
| 110 | 601   | 4.647699                    | 5.732581                     | 5.765607                                                               |
| 109 | 599   | 4.639978                    | 5.723043                     | 5.755739                                                               |
| 108 | 593   | 4.632245                    | 5.713489                     | 5.745763                                                               |
| 107 | 587   | 4.624446                    | 5.703854                     | 5.735689                                                               |
| 106 | 577   | 4.616582                    | 5.694137                     | 5.725515                                                               |
| 105 | 571   | 4.608595                    | 5.684268                     | 5.715249                                                               |
| 104 | 569   | 4.600538                    | 5.674313                     | 5.704879                                                               |
| 103 | 563   | 4.592466                    | 5.664341                     | 5.694390                                                               |
| 102 | 557   | 4.584324                    | 5.654280                     | 5.683793                                                               |
| 101 | 547   | 4.576108                    | 5.644129                     | 5.673085                                                               |
| 100 | 541   | 4.567758                    | 5.633810                     | 5.662275                                                               |
| 99  | 523   | 4.559330                    | 5.623396                     | 5.651350                                                               |
| 98  | 521   | 4.550629                    | 5.612644                     | 5.640347                                                               |
| 97  | 509   | 4.541911                    | 5.601871                     | 5.629211                                                               |
| 96  | 503   | 4.533006                    | 5.590866                     | 5.617974                                                               |
| 95  | 499   | 4.524012                    | 5.579751                     | 5.606613                                                               |
| 94  | 491   | 4.514964                    | 5.568569                     | 5.595119                                                               |
| 93  | 487   | 4.505787                    | 5.557228                     | 5.583502                                                               |
| 92  | 479   | 4.496554                    | 5.545817                     | 5.571744                                                               |
| 91  | 467   | 4.487186                    | 5.534239                     | 5.559860                                                               |
| 90  | 463   | 4.477598                    | 5.522388                     | 5.547861                                                               |
| 89  | 461   | 4.467948                    | 5.510461                     | 5.535714                                                               |
| 88  | 457   | 4.458277                    | 5.498507                     | 5.523405                                                               |
| 87  | 449   | 4.448543                    | 5.486476                     | 5.510938                                                               |
| 86  | 443   | 4.438657                    | 5.474256                     | 5.498329                                                               |
| 85  | 439   | 4.428660                    | 5.461899                     | 5.485563                                                               |
| 84  | 433   | 4.418595                    | 5.449457                     | 5.472629                                                               |
| 83  | 431   | 4.408414                    | 5.436872                     | 5.459531                                                               |
| 82  | 421   | 4.398209                    | 5.424257                     | 5.446245                                                               |
| 81  | 419   | 4.387787                    | 5.411373                     | 5.432806                                                               |
| 80  | 409   | 4.377340                    | 5.398458                     | 5.419170                                                               |
| 79  | 401   | 4.366663                    | 5.385259                     | 5.405373                                                               |
| 78  | 397   | 4.355801                    | 5.371829                     | 5.391403                                                               |
| 77  | 389   | 4.344857                    | 5.358298                     | 5.377230                                                               |
| 76  | 383   | 4.333716                    | 5.344524                     | 5.362874                                                               |
| 75  | 379   | 4.322430                    | 5.330570                     | 5.348317                                                               |

| $k$ | $p_k$ | $\frac{\sigma(N'_k)}{N'_k}$ | $\frac{N'_k}{\varphi(N'_k)}$ | $\frac{e^\gamma}{2} \log \log N'_k + \frac{0.73\dots}{\log \log N'_k}$ |
|-----|-------|-----------------------------|------------------------------|------------------------------------------------------------------------|
| 74  | 373   | 4.311056                    | 5.316505                     | 5.333541                                                               |
| 73  | 367   | 4.299529                    | 5.302251                     | 5.318551                                                               |
| 72  | 359   | 4.287845                    | 5.287804                     | 5.303344                                                               |
| 71  | 353   | 4.275934                    | 5.273075                     | 5.287925                                                               |
| 70  | 349   | 4.263856                    | 5.258137                     | 5.272276                                                               |
| 69  | 347   | 4.251673                    | 5.243070                     | 5.256374                                                               |
| 68  | 337   | 4.239456                    | 5.227961                     | 5.240193                                                               |
| 67  | 331   | 4.226913                    | 5.212447                     | 5.223792                                                               |
| 66  | 317   | 4.214181                    | 5.196700                     | 5.207129                                                               |
| 65  | 313   | 4.200929                    | 5.180306                     | 5.190271                                                               |
| 64  | 311   | 4.187550                    | 5.163756                     | 5.173120                                                               |
| 63  | 307   | 4.174129                    | 5.147152                     | 5.155647                                                               |
| 62  | 293   | 4.160576                    | 5.130386                     | 5.137858                                                               |
| 61  | 283   | 4.146425                    | 5.112876                     | 5.119850                                                               |
| 60  | 281   | 4.131825                    | 5.094810                     | 5.101577                                                               |
| 59  | 277   | 4.117173                    | 5.076679                     | 5.082938                                                               |
| 58  | 271   | 4.102363                    | 5.058351                     | 5.063943                                                               |
| 57  | 269   | 4.087281                    | 5.039686                     | 5.044603                                                               |
| 56  | 263   | 4.072143                    | 5.020951                     | 5.024852                                                               |
| 55  | 257   | 4.056718                    | 5.001860                     | 5.004727                                                               |
| 54  | 251   | 4.040994                    | 4.982397                     | 4.984215                                                               |
| 53  | 241   | 4.024958                    | 4.962547                     | 4.963301                                                               |
| 52  | 239   | 4.008326                    | 4.941956                     | 4.942034                                                               |
| 51  | 233   | 3.991625                    | 4.921278                     | 4.920270                                                               |
| 50  | 229   | 3.974567                    | 4.900157                     | 4.898056                                                               |
| 49  | 227   | 3.957286                    | 4.878759                     | 4.875337                                                               |
| 48  | 223   | 3.939929                    | 4.857266                     | 4.852049                                                               |
| 47  | 211   | 3.922340                    | 4.835485                     | 4.828204                                                               |

## 5 Table 5

Note that the constant  $0.7399\dots$  is determined so that the equality is valid in the case that  $n = 315$ . In the numerical computation, however, we use  $0.7399$  instead of that actual value.

Table 5: In the case which  $n \leq 45045$

| $n$ | $\frac{\sigma(n)}{n}$ | $\frac{e^\gamma}{2} \log \log n + \frac{0.73\dots}{\log \log n}$ |
|-----|-----------------------|------------------------------------------------------------------|
| 3   | 1.333333              | 7.951027                                                         |
| 5   | 1.200000              | 1.978580                                                         |
| 7   | 1.142857              | 1.704268                                                         |
| 9   | 1.444444              | 1.640945                                                         |
| 11  | 1.090909              | 1.624850                                                         |
| 13  | 1.076923              | 1.624338                                                         |

| $n$ | $\frac{\sigma(n)}{n}$ | $\frac{e^\gamma}{2} \log \log n + \frac{0.73...}{\log \log n}$ |
|-----|-----------------------|----------------------------------------------------------------|
| 15  | 1.600000              | 1.629879                                                       |
| 17  | 1.058824              | 1.637893                                                       |
| 19  | 1.052632              | 1.646851                                                       |
| 21  | 1.523810              | 1.656048                                                       |
| 23  | 1.043478              | 1.665145                                                       |
| 25  | 1.240000              | 1.673982                                                       |
| 27  | 1.481481              | 1.682485                                                       |
| 29  | 1.034483              | 1.690627                                                       |
| 31  | 1.032258              | 1.698404                                                       |
| 33  | 1.454545              | 1.705827                                                       |
| 35  | 1.371429              | 1.712912                                                       |
| 37  | 1.027027              | 1.719678                                                       |
| 39  | 1.435897              | 1.726144                                                       |
| 41  | 1.024390              | 1.732329                                                       |
| 43  | 1.023256              | 1.738253                                                       |
| 45  | 1.733333              | 1.743932                                                       |
| 47  | 1.021277              | 1.749384                                                       |
| 49  | 1.163265              | 1.754623                                                       |
| 51  | 1.411765              | 1.759663                                                       |
| 53  | 1.018868              | 1.764517                                                       |
| 55  | 1.309091              | 1.769197                                                       |
| 57  | 1.403509              | 1.773714                                                       |
| 59  | 1.016949              | 1.778077                                                       |
| 61  | 1.016393              | 1.782296                                                       |
| 63  | 1.650794              | 1.786379                                                       |
| 65  | 1.292308              | 1.790334                                                       |
| 67  | 1.014925              | 1.794168                                                       |
| 69  | 1.391304              | 1.797887                                                       |
| 71  | 1.014085              | 1.801498                                                       |
| 73  | 1.013699              | 1.805007                                                       |
| 75  | 1.653333              | 1.808418                                                       |
| 77  | 1.246753              | 1.811737                                                       |
| 79  | 1.012658              | 1.814968                                                       |
| 81  | 1.493827              | 1.818115                                                       |
| 83  | 1.012048              | 1.821183                                                       |
| 85  | 1.270588              | 1.824174                                                       |
| 87  | 1.379310              | 1.827092                                                       |
| 89  | 1.011236              | 1.829942                                                       |
| 91  | 1.230769              | 1.832724                                                       |
| 93  | 1.376344              | 1.835443                                                       |
| 95  | 1.263158              | 1.838102                                                       |
| 97  | 1.010309              | 1.840701                                                       |
| 99  | 1.575758              | 1.843245                                                       |
| 101 | 1.009901              | 1.845735                                                       |

| $n$ | $\frac{\sigma(n)}{n}$ | $\frac{e^\gamma}{2} \log \log n + \frac{0.73...}{\log \log n}$ |
|-----|-----------------------|----------------------------------------------------------------|
| 103 | 1.009709              | 1.848173                                                       |
| 105 | 1.828571              | 1.850561                                                       |
| 107 | 1.009346              | 1.852902                                                       |
| 109 | 1.009174              | 1.855196                                                       |
| 111 | 1.369369              | 1.857446                                                       |
| 113 | 1.008850              | 1.859653                                                       |
| 115 | 1.252174              | 1.861819                                                       |
| 117 | 1.555556              | 1.863945                                                       |
| 119 | 1.210084              | 1.866032                                                       |
| 121 | 1.099174              | 1.868082                                                       |
| 123 | 1.365854              | 1.870096                                                       |
| 125 | 1.248000              | 1.872075                                                       |
| 127 | 1.007874              | 1.874020                                                       |
| 129 | 1.364341              | 1.875933                                                       |
| 131 | 1.007634              | 1.877814                                                       |
| 133 | 1.203008              | 1.879664                                                       |
| 135 | 1.777778              | 1.881485                                                       |
| 137 | 1.007299              | 1.883276                                                       |
| 139 | 1.007194              | 1.885040                                                       |
| 141 | 1.361702              | 1.886776                                                       |
| 143 | 1.174825              | 1.888487                                                       |
| 145 | 1.241379              | 1.890171                                                       |
| 147 | 1.551020              | 1.891831                                                       |
| 149 | 1.006711              | 1.893466                                                       |
| 151 | 1.006623              | 1.895077                                                       |
| 153 | 1.529412              | 1.896666                                                       |
| 155 | 1.238710              | 1.898232                                                       |
| 157 | 1.006369              | 1.899777                                                       |
| 159 | 1.358491              | 1.901300                                                       |
| 161 | 1.192547              | 1.902803                                                       |
| 163 | 1.006135              | 1.904286                                                       |
| 165 | 1.745455              | 1.905749                                                       |
| 167 | 1.005988              | 1.907193                                                       |
| 169 | 1.082840              | 1.908618                                                       |
| 171 | 1.520468              | 1.910025                                                       |
| 173 | 1.005780              | 1.911414                                                       |
| 175 | 1.417143              | 1.912785                                                       |
| 177 | 1.355932              | 1.914140                                                       |
| 179 | 1.005587              | 1.915479                                                       |
| 181 | 1.005525              | 1.916801                                                       |
| 183 | 1.355191              | 1.918107                                                       |
| 185 | 1.232432              | 1.919398                                                       |
| 187 | 1.155080              | 1.920673                                                       |
| 189 | 1.693122              | 1.921934                                                       |



| $n$ | $\frac{\sigma(n)}{n}$ | $\frac{e^\gamma}{2} \log \log n + \frac{0.73...}{\log \log n}$ |
|-----|-----------------------|----------------------------------------------------------------|
| 191 | 1.005236              | 1.923180                                                       |
| 193 | 1.005181              | 1.924413                                                       |
| 195 | 1.723077              | 1.925631                                                       |
| 197 | 1.005076              | 1.926836                                                       |
| 199 | 1.005025              | 1.928027                                                       |
| 201 | 1.353234              | 1.929206                                                       |
| 203 | 1.182266              | 1.930372                                                       |
| 205 | 1.229268              | 1.931525                                                       |
| 207 | 1.507246              | 1.932666                                                       |
| 209 | 1.148325              | 1.933795                                                       |
| 211 | 1.004739              | 1.934912                                                       |
| 213 | 1.352113              | 1.936018                                                       |
| 215 | 1.227907              | 1.937113                                                       |
| 217 | 1.179724              | 1.938196                                                       |
| 219 | 1.351598              | 1.939268                                                       |
| 221 | 1.140271              | 1.940330                                                       |
| 223 | 1.004484              | 1.941382                                                       |
| 225 | 1.791111              | 1.942423                                                       |
| 227 | 1.004405              | 1.943454                                                       |
| 229 | 1.004367              | 1.944475                                                       |
| 231 | 1.662338              | 1.945487                                                       |
| 233 | 1.004292              | 1.946488                                                       |
| 235 | 1.225532              | 1.947481                                                       |
| 237 | 1.350211              | 1.948464                                                       |
| 239 | 1.004184              | 1.949438                                                       |
| 241 | 1.004149              | 1.950404                                                       |
| 243 | 1.497942              | 1.951360                                                       |
| 245 | 1.395918              | 1.952308                                                       |
| 247 | 1.133603              | 1.953248                                                       |
| 249 | 1.349398              | 1.954179                                                       |
| 251 | 1.003984              | 1.955102                                                       |
| 253 | 1.138340              | 1.956017                                                       |
| 255 | 1.694118              | 1.956925                                                       |
| 257 | 1.003891              | 1.957824                                                       |
| 259 | 1.173745              | 1.958716                                                       |
| 261 | 1.494253              | 1.959600                                                       |
| 263 | 1.003802              | 1.960477                                                       |
| 265 | 1.222642              | 1.961346                                                       |
| 267 | 1.348315              | 1.962209                                                       |
| 269 | 1.003717              | 1.963064                                                       |
| 271 | 1.003690              | 1.963912                                                       |
| 273 | 1.641026              | 1.964754                                                       |
| 275 | 1.352727              | 1.965588                                                       |
| 277 | 1.003610              | 1.966417                                                       |

| $n$ | $\frac{\sigma(n)}{n}$ | $\frac{e^\gamma}{2} \log \log n + \frac{0.73...}{\log \log n}$ |
|-----|-----------------------|----------------------------------------------------------------|
| 279 | 1.491039              | 1.967238                                                       |
| 281 | 1.003559              | 1.968053                                                       |
| 283 | 1.003534              | 1.968862                                                       |
| 285 | 1.684211              | 1.969665                                                       |
| 287 | 1.170732              | 1.970461                                                       |
| 289 | 1.062284              | 1.971251                                                       |
| 291 | 1.347079              | 1.972035                                                       |
| 293 | 1.003413              | 1.972814                                                       |
| 295 | 1.220339              | 1.973586                                                       |
| 297 | 1.616162              | 1.974353                                                       |
| 299 | 1.123746              | 1.975114                                                       |
| 301 | 1.169435              | 1.975870                                                       |
| 303 | 1.346535              | 1.976620                                                       |
| 305 | 1.219672              | 1.977365                                                       |
| 307 | 1.003257              | 1.978104                                                       |
| 309 | 1.346278              | 1.978838                                                       |
| 311 | 1.003215              | 1.979567                                                       |
| 313 | 1.003195              | 1.980291                                                       |
| 315 | 1.980952              | 1.981009                                                       |
| 317 | 1.003155              | 1.981723                                                       |
| 319 | 1.128527              | 1.982432                                                       |
| 321 | 1.345794              | 1.983136                                                       |
| 323 | 1.114551              | 1.983835                                                       |
| 325 | 1.335385              | 1.984529                                                       |
| 327 | 1.345566              | 1.985219                                                       |
| 329 | 1.167173              | 1.985904                                                       |
| 331 | 1.003021              | 1.986584                                                       |
| 333 | 1.483483              | 1.987260                                                       |
| 335 | 1.217910              | 1.987931                                                       |
| 337 | 1.002967              | 1.988598                                                       |
| 339 | 1.345133              | 1.989261                                                       |
| 341 | 1.126100              | 1.989919                                                       |
| 343 | 1.166181              | 1.990574                                                       |
| 345 | 1.669565              | 1.991224                                                       |
| 347 | 1.002882              | 1.991870                                                       |
| 349 | 1.002865              | 1.992511                                                       |
| 351 | 1.595442              | 1.993149                                                       |
| 353 | 1.002833              | 1.993783                                                       |
| 355 | 1.216901              | 1.994413                                                       |
| 357 | 1.613445              | 1.995039                                                       |
| 359 | 1.002786              | 1.995661                                                       |
| 361 | 1.055402              | 1.996279                                                       |
| 363 | 1.465565              | 1.996893                                                       |
| 365 | 1.216438              | 1.997504                                                       |

| $n$ | $\frac{\sigma(n)}{n}$ | $\frac{e^\gamma}{2} \log \log n + \frac{0.73...}{\log \log n}$ |
|-----|-----------------------|----------------------------------------------------------------|
| 367 | 1.002725              | 1.998111                                                       |
| 369 | 1.479675              | 1.998715                                                       |
| 371 | 1.164420              | 1.999315                                                       |
| 373 | 1.002681              | 1.999911                                                       |
| 375 | 1.664000              | 2.000504                                                       |
| 377 | 1.114058              | 2.001093                                                       |
| 379 | 1.002639              | 2.001679                                                       |
| 381 | 1.343832              | 2.002262                                                       |
| 383 | 1.002611              | 2.002841                                                       |
| 385 | 1.496104              | 2.003417                                                       |
| 387 | 1.478036              | 2.003989                                                       |
| 389 | 1.002571              | 2.004559                                                       |
| 391 | 1.104859              | 2.005125                                                       |
| 393 | 1.343511              | 2.005688                                                       |
| 395 | 1.215190              | 2.006247                                                       |
| 397 | 1.002519              | 2.006804                                                       |
| 399 | 1.604010              | 2.007358                                                       |
| 401 | 1.002494              | 2.007908                                                       |
| 403 | 1.111663              | 2.008456                                                       |
| 405 | 1.792593              | 2.009000                                                       |
| 407 | 1.120393              | 2.009542                                                       |
| 409 | 1.002445              | 2.010081                                                       |
| 411 | 1.343066              | 2.010616                                                       |
| 413 | 1.162228              | 2.011149                                                       |
| 415 | 1.214458              | 2.011679                                                       |
| 417 | 1.342926              | 2.012206                                                       |
| 419 | 1.002387              | 2.012731                                                       |
| 421 | 1.002375              | 2.013253                                                       |
| 423 | 1.475177              | 2.013772                                                       |
| 425 | 1.312941              | 2.014288                                                       |
| 427 | 1.161593              | 2.014802                                                       |
| 429 | 1.566434              | 2.015313                                                       |
| 431 | 1.002320              | 2.015821                                                       |
| 433 | 1.002309              | 2.016327                                                       |
| 435 | 1.655172              | 2.016830                                                       |
| 437 | 1.098398              | 2.017331                                                       |
| 439 | 1.002278              | 2.017829                                                       |
| 441 | 1.680272              | 2.018324                                                       |
| 443 | 1.002257              | 2.018818                                                       |
| 445 | 1.213483              | 2.019308                                                       |
| 447 | 1.342282              | 2.019797                                                       |
| 449 | 1.002227              | 2.020282                                                       |
| 451 | 1.117517              | 2.020766                                                       |
| 453 | 1.342163              | 2.021247                                                       |

| $n$ | $\frac{\sigma(n)}{n}$ | $\frac{e^\gamma}{2} \log \log n + \frac{0.73\dots}{\log \log n}$ |
|-----|-----------------------|------------------------------------------------------------------|
| 455 | 1.476923              | 2.021726                                                         |
| 457 | 1.002188              | 2.022203                                                         |
| 459 | 1.568627              | 2.022677                                                         |
| 461 | 1.002169              | 2.023149                                                         |
| 463 | 1.002160              | 2.023618                                                         |
| 465 | 1.651613              | 2.024086                                                         |
| 467 | 1.002141              | 2.024551                                                         |
| 469 | 1.159915              | 2.025014                                                         |
| 471 | 1.341826              | 2.025475                                                         |
| 473 | 1.116279              | 2.025934                                                         |
| 475 | 1.305263              | 2.026390                                                         |
| 477 | 1.471698              | 2.026845                                                         |
| 479 | 1.002088              | 2.027297                                                         |
| 481 | 1.106029              | 2.027748                                                         |
| 483 | 1.590062              | 2.028196                                                         |
| 485 | 1.212371              | 2.028642                                                         |
| 487 | 1.002053              | 2.029086                                                         |
| 489 | 1.341513              | 2.029528                                                         |
| 491 | 1.002037              | 2.029969                                                         |
| 493 | 1.095335              | 2.030407                                                         |
| 495 | 1.890909              | 2.030843                                                         |
| 497 | 1.158954              | 2.031277                                                         |
| 499 | 1.002004              | 2.031710                                                         |
| 501 | 1.341317              | 2.032140                                                         |
| 503 | 1.001988              | 2.032569                                                         |
| 505 | 1.211881              | 2.032996                                                         |
| 507 | 1.443787              | 2.033421                                                         |
| 509 | 1.001965              | 2.033844                                                         |
| 511 | 1.158513              | 2.034265                                                         |
| 513 | 1.559454              | 2.034684                                                         |
| 515 | 1.211650              | 2.035102                                                         |
| 517 | 1.114120              | 2.035518                                                         |
| 519 | 1.341040              | 2.035932                                                         |
| 521 | 1.001919              | 2.036344                                                         |
| 523 | 1.001912              | 2.036755                                                         |
| 525 | 1.889524              | 2.037163                                                         |
| 527 | 1.092979              | 2.037570                                                         |
| 529 | 1.045369              | 2.037976                                                         |
| 531 | 1.468927              | 2.038380                                                         |
| 533 | 1.103189              | 2.038782                                                         |
| 535 | 1.211215              | 2.039182                                                         |
| 537 | 1.340782              | 2.039581                                                         |
| 539 | 1.269017              | 2.039978                                                         |
| 541 | 1.001848              | 2.040373                                                         |

| $n$ | $\frac{\sigma(n)}{n}$ | $\frac{e^\gamma}{2} \log \log n + \frac{0.73...}{\log \log n}$ |
|-----|-----------------------|----------------------------------------------------------------|
| 543 | 1.340700              | 2.040767                                                       |
| 545 | 1.211009              | 2.041159                                                       |
| 547 | 1.001828              | 2.041550                                                       |
| 549 | 1.468124              | 2.041939                                                       |
| 551 | 1.088929              | 2.042327                                                       |
| 553 | 1.157324              | 2.042713                                                       |
| 555 | 1.643243              | 2.043097                                                       |
| 557 | 1.001795              | 2.043480                                                       |
| 559 | 1.101968              | 2.043862                                                       |
| 561 | 1.540107              | 2.044242                                                       |
| 563 | 1.001776              | 2.044620                                                       |
| 565 | 1.210619              | 2.044997                                                       |
| 567 | 1.707231              | 2.045372                                                       |
| 569 | 1.001757              | 2.045746                                                       |
| 571 | 1.001751              | 2.046119                                                       |
| 573 | 1.340314              | 2.046490                                                       |
| 575 | 1.293913              | 2.046860                                                       |
| 577 | 1.001733              | 2.047228                                                       |
| 579 | 1.340242              | 2.047595                                                       |
| 581 | 1.156627              | 2.047961                                                       |
| 583 | 1.111492              | 2.048325                                                       |
| 585 | 1.866667              | 2.048688                                                       |
| 587 | 1.001704              | 2.049049                                                       |
| 589 | 1.086587              | 2.049409                                                       |
| 591 | 1.340102              | 2.049768                                                       |
| 593 | 1.001686              | 2.050125                                                       |
| 595 | 1.452101              | 2.050481                                                       |
| 597 | 1.340034              | 2.050836                                                       |
| 599 | 1.001669              | 2.051189                                                       |
| 601 | 1.001664              | 2.051541                                                       |
| 603 | 1.466003              | 2.051892                                                       |
| 605 | 1.319008              | 2.052242                                                       |
| 607 | 1.001647              | 2.052590                                                       |
| 609 | 1.576355              | 2.052937                                                       |
| 611 | 1.099836              | 2.053283                                                       |
| 613 | 1.001631              | 2.053627                                                       |
| 615 | 1.639024              | 2.053970                                                       |
| 617 | 1.001621              | 2.054312                                                       |
| 619 | 1.001616              | 2.054653                                                       |
| 621 | 1.545894              | 2.054993                                                       |
| 623 | 1.155698              | 2.055331                                                       |
| 625 | 1.249600              | 2.055668                                                       |
| 627 | 1.531100              | 2.056004                                                       |
| 629 | 1.087440              | 2.056339                                                       |

| $n$ | $\frac{\sigma(n)}{n}$ | $\frac{e^\gamma}{2} \log \log n + \frac{0.73...}{\log \log n}$ |
|-----|-----------------------|----------------------------------------------------------------|
| 631 | 1.001585              | 2.056673                                                       |
| 633 | 1.339652              | 2.057005                                                       |
| 635 | 1.209449              | 2.057337                                                       |
| 637 | 1.252747              | 2.057667                                                       |
| 639 | 1.464789              | 2.057996                                                       |
| 641 | 1.001560              | 2.058324                                                       |
| 643 | 1.001555              | 2.058651                                                       |
| 645 | 1.637209              | 2.058976                                                       |
| 647 | 1.001546              | 2.059301                                                       |
| 649 | 1.109399              | 2.059624                                                       |
| 651 | 1.572965              | 2.059947                                                       |
| 653 | 1.001531              | 2.060268                                                       |
| 655 | 1.209160              | 2.060588                                                       |
| 657 | 1.464231              | 2.060907                                                       |
| 659 | 1.001517              | 2.061225                                                       |
| 661 | 1.001513              | 2.061542                                                       |
| 663 | 1.520362              | 2.061858                                                       |
| 665 | 1.443609              | 2.062173                                                       |
| 667 | 1.079460              | 2.062487                                                       |
| 669 | 1.339312              | 2.062799                                                       |
| 671 | 1.108793              | 2.063111                                                       |
| 673 | 1.001486              | 2.063422                                                       |
| 675 | 1.837037              | 2.063732                                                       |
| 677 | 1.001477              | 2.064040                                                       |
| 679 | 1.154639              | 2.064348                                                       |
| 681 | 1.339207              | 2.064655                                                       |
| 683 | 1.001464              | 2.064960                                                       |
| 685 | 1.208759              | 2.065265                                                       |
| 687 | 1.339156              | 2.065569                                                       |
| 689 | 1.097242              | 2.065872                                                       |
| 691 | 1.001447              | 2.066174                                                       |
| 693 | 1.800866              | 2.066474                                                       |
| 695 | 1.208633              | 2.066774                                                       |
| 697 | 1.084648              | 2.067073                                                       |
| 699 | 1.339056              | 2.067371                                                       |
| 701 | 1.001427              | 2.067668                                                       |
| 703 | 1.081081              | 2.067964                                                       |
| 705 | 1.634043              | 2.068260                                                       |
| 707 | 1.154173              | 2.068554                                                       |
| 709 | 1.001410              | 2.068847                                                       |
| 711 | 1.462729              | 2.069140                                                       |
| 713 | 1.077139              | 2.069431                                                       |
| 715 | 1.409790              | 2.069722                                                       |
| 717 | 1.338912              | 2.070012                                                       |

| $n$ | $\frac{\sigma(n)}{n}$ | $\frac{e^\gamma}{2} \log \log n + \frac{0.73...}{\log \log n}$ |
|-----|-----------------------|----------------------------------------------------------------|
| 719 | 1.001391              | 2.070300                                                       |
| 721 | 1.153953              | 2.070588                                                       |
| 723 | 1.338866              | 2.070875                                                       |
| 725 | 1.282759              | 2.071162                                                       |
| 727 | 1.001376              | 2.071447                                                       |
| 729 | 1.499314              | 2.071732                                                       |
| 731 | 1.083447              | 2.072015                                                       |
| 733 | 1.001364              | 2.072298                                                       |
| 735 | 1.861224              | 2.072580                                                       |
| 737 | 1.107191              | 2.072861                                                       |
| 739 | 1.001353              | 2.073141                                                       |
| 741 | 1.511471              | 2.073421                                                       |
| 743 | 1.001346              | 2.073699                                                       |
| 745 | 1.208054              | 2.073977                                                       |
| 747 | 1.461847              | 2.074254                                                       |
| 749 | 1.153538              | 2.074530                                                       |
| 751 | 1.001332              | 2.074805                                                       |
| 753 | 1.338645              | 2.075080                                                       |
| 755 | 1.207947              | 2.075353                                                       |
| 757 | 1.001321              | 2.075626                                                       |
| 759 | 1.517787              | 2.075898                                                       |
| 761 | 1.001314              | 2.076170                                                       |
| 763 | 1.153342              | 2.076440                                                       |
| 765 | 1.835294              | 2.076710                                                       |
| 767 | 1.095176              | 2.076979                                                       |
| 769 | 1.001300              | 2.077247                                                       |
| 771 | 1.338521              | 2.077514                                                       |
| 773 | 1.001294              | 2.077781                                                       |
| 775 | 1.280000              | 2.078047                                                       |
| 777 | 1.564994              | 2.078312                                                       |
| 779 | 1.078306              | 2.078577                                                       |
| 781 | 1.106274              | 2.078840                                                       |
| 783 | 1.532567              | 2.079103                                                       |
| 785 | 1.207643              | 2.079365                                                       |
| 787 | 1.001271              | 2.079627                                                       |
| 789 | 1.338403              | 2.079887                                                       |
| 791 | 1.152971              | 2.080147                                                       |
| 793 | 1.094578              | 2.080407                                                       |
| 795 | 1.630189              | 2.080665                                                       |
| 797 | 1.001255              | 2.080923                                                       |
| 799 | 1.081352              | 2.081180                                                       |
| 801 | 1.460674              | 2.081436                                                       |
| 803 | 1.105853              | 2.081692                                                       |
| 805 | 1.431056              | 2.081947                                                       |

| $n$ | $\frac{\sigma(n)}{n}$ | $\frac{e^\gamma}{2} \log \log n + \frac{0.73\dots}{\log \log n}$ |
|-----|-----------------------|------------------------------------------------------------------|
| 807 | 1.338290              | 2.082201                                                         |
| 809 | 1.001236              | 2.082455                                                         |
| 811 | 1.001233              | 2.082708                                                         |
| 813 | 1.338253              | 2.082960                                                         |
| 815 | 1.207362              | 2.083212                                                         |
| 817 | 1.077111              | 2.083462                                                         |
| 819 | 1.777778              | 2.083713                                                         |
| 821 | 1.001218              | 2.083962                                                         |
| 823 | 1.001215              | 2.084211                                                         |
| 825 | 1.803636              | 2.084459                                                         |
| 827 | 1.001209              | 2.084707                                                         |
| 829 | 1.001206              | 2.084953                                                         |
| 831 | 1.338147              | 2.085200                                                         |
| 833 | 1.231693              | 2.085445                                                         |
| 835 | 1.207186              | 2.085690                                                         |
| 837 | 1.529271              | 2.085934                                                         |
| 839 | 1.001192              | 2.086178                                                         |
| 841 | 1.035672              | 2.086421                                                         |
| 843 | 1.338078              | 2.086663                                                         |
| 845 | 1.299408              | 2.086905                                                         |
| 847 | 1.256198              | 2.087146                                                         |
| 849 | 1.338045              | 2.087386                                                         |
| 851 | 1.071680              | 2.087626                                                         |
| 853 | 1.001172              | 2.087865                                                         |
| 855 | 1.824561              | 2.088104                                                         |
| 857 | 1.001167              | 2.088342                                                         |
| 859 | 1.001164              | 2.088579                                                         |
| 861 | 1.560976              | 2.088816                                                         |
| 863 | 1.001159              | 2.089052                                                         |
| 865 | 1.206936              | 2.089288                                                         |
| 867 | 1.416378              | 2.089523                                                         |
| 869 | 1.104718              | 2.089757                                                         |
| 871 | 1.092997              | 2.089991                                                         |
| 873 | 1.459336              | 2.090224                                                         |
| 875 | 1.426286              | 2.090456                                                         |
| 877 | 1.001140              | 2.090688                                                         |
| 879 | 1.337884              | 2.090920                                                         |
| 881 | 1.001135              | 2.091151                                                         |
| 883 | 1.001133              | 2.091381                                                         |
| 885 | 1.627119              | 2.091610                                                         |
| 887 | 1.001127              | 2.091840                                                         |
| 889 | 1.151856              | 2.092068                                                         |
| 891 | 1.629630              | 2.092296                                                         |
| 893 | 1.075028              | 2.092523                                                         |



| $n$ | $\frac{\sigma(n)}{n}$ | $\frac{e^\gamma}{2} \log \log n + \frac{0.73...}{\log \log n}$ |
|-----|-----------------------|----------------------------------------------------------------|
| 895 | 1.206704              | 2.092750                                                       |
| 897 | 1.498328              | 2.092977                                                       |
| 899 | 1.067853              | 2.093202                                                       |
| 901 | 1.078801              | 2.093427                                                       |
| 903 | 1.559247              | 2.093652                                                       |
| 905 | 1.206630              | 2.093876                                                       |
| 907 | 1.001103              | 2.094100                                                       |
| 909 | 1.458746              | 2.094323                                                       |
| 911 | 1.001098              | 2.094545                                                       |
| 913 | 1.104053              | 2.094767                                                       |
| 915 | 1.626230              | 2.094988                                                       |
| 917 | 1.151581              | 2.095209                                                       |
| 919 | 1.001088              | 2.095429                                                       |
| 921 | 1.337676              | 2.095649                                                       |
| 923 | 1.092091              | 2.095869                                                       |
| 925 | 1.273514              | 2.096087                                                       |
| 927 | 1.458468              | 2.096305                                                       |
| 929 | 1.001076              | 2.096523                                                       |
| 931 | 1.224490              | 2.096740                                                       |
| 933 | 1.337621              | 2.096957                                                       |
| 935 | 1.386096              | 2.097173                                                       |
| 937 | 1.001067              | 2.097389                                                       |
| 939 | 1.337593              | 2.097604                                                       |
| 941 | 1.001063              | 2.097819                                                       |
| 943 | 1.068929              | 2.098033                                                       |
| 945 | 2.031746              | 2.098246                                                       |
| 947 | 1.001056              | 2.098459                                                       |
| 949 | 1.091675              | 2.098672                                                       |
| 951 | 1.337539              | 2.098884                                                       |
| 953 | 1.001049              | 2.099096                                                       |
| 955 | 1.206283              | 2.099307                                                       |
| 957 | 1.504702              | 2.099518                                                       |
| 959 | 1.151199              | 2.099728                                                       |
| 961 | 1.033299              | 2.099938                                                       |
| 963 | 1.457944              | 2.100147                                                       |
| 965 | 1.206218              | 2.100356                                                       |
| 967 | 1.001034              | 2.100564                                                       |
| 969 | 1.486068              | 2.100772                                                       |
| 971 | 1.001030              | 2.100979                                                       |
| 973 | 1.151079              | 2.101186                                                       |
| 975 | 1.780513              | 2.101392                                                       |
| 977 | 1.001024              | 2.101598                                                       |
| 979 | 1.103166              | 2.101804                                                       |
| 981 | 1.457696              | 2.102009                                                       |

| $n$  | $\frac{\sigma(n)}{n}$ | $\frac{e^\gamma}{2} \log \log n + \frac{0.73\dots}{\log \log n}$ |
|------|-----------------------|------------------------------------------------------------------|
| 983  | 1.001017              | 2.102213                                                         |
| 985  | 1.206091              | 2.102417                                                         |
| 987  | 1.556231              | 2.102621                                                         |
| 989  | 1.067745              | 2.102824                                                         |
| 991  | 1.001009              | 2.103027                                                         |
| 993  | 1.337362              | 2.103229                                                         |
| 995  | 1.206030              | 2.103431                                                         |
| 997  | 1.001003              | 2.103632                                                         |
| 999  | 1.521522              | 2.103833                                                         |
| 1001 | 1.342657              | 2.104034                                                         |
| 1003 | 1.076770              | 2.104234                                                         |
| 1005 | 1.623881              | 2.104433                                                         |
| 1007 | 1.072493              | 2.104632                                                         |
| 1009 | 1.000991              | 2.104831                                                         |
| 1011 | 1.337290              | 2.105029                                                         |
| 1013 | 1.000987              | 2.105227                                                         |
| 1015 | 1.418719              | 2.105425                                                         |
| 1017 | 1.457227              | 2.105622                                                         |
| 1019 | 1.000981              | 2.105818                                                         |
| 1021 | 1.000979              | 2.106014                                                         |
| 1023 | 1.501466              | 2.106210                                                         |
| 1025 | 1.270244              | 2.106405                                                         |
| 1027 | 1.090555              | 2.106600                                                         |
| 1029 | 1.554908              | 2.106795                                                         |
| 1031 | 1.000970              | 2.106989                                                         |
| 1033 | 1.000968              | 2.107183                                                         |
| 1035 | 1.808696              | 2.107376                                                         |
| 1037 | 1.076181              | 2.107569                                                         |
| 1039 | 1.000962              | 2.107761                                                         |
| 1041 | 1.337176              | 2.107953                                                         |
| 1043 | 1.150527              | 2.108145                                                         |
| 1045 | 1.377990              | 2.108336                                                         |
| 1047 | 1.337154              | 2.108527                                                         |
| 1049 | 1.000953              | 2.108717                                                         |
| 1051 | 1.000951              | 2.108907                                                         |
| 1053 | 1.608737              | 2.109097                                                         |
| 1055 | 1.205687              | 2.109286                                                         |
| 1057 | 1.150426              | 2.109475                                                         |
| 1059 | 1.337110              | 2.109663                                                         |
| 1061 | 1.000943              | 2.109851                                                         |
| 1063 | 1.000941              | 2.110039                                                         |
| 1065 | 1.622535              | 2.110226                                                         |
| 1067 | 1.102156              | 2.110413                                                         |
| 1069 | 1.000935              | 2.110599                                                         |

| $n$  | $\frac{\sigma(n)}{n}$ | $\frac{e^\gamma}{2} \log \log n + \frac{0.73...}{\log \log n}$ |
|------|-----------------------|----------------------------------------------------------------|
| 1071 | 1.747899              | 2.110785                                                       |
| 1073 | 1.062442              | 2.110971                                                       |
| 1075 | 1.268837              | 2.111156                                                       |
| 1077 | 1.337047              | 2.111341                                                       |
| 1079 | 1.089898              | 2.111526                                                       |
| 1081 | 1.065680              | 2.111710                                                       |
| 1083 | 1.407202              | 2.111894                                                       |
| 1085 | 1.415668              | 2.112077                                                       |
| 1087 | 1.000920              | 2.112260                                                       |
| 1089 | 1.587695              | 2.112443                                                       |
| 1091 | 1.000917              | 2.112625                                                       |
| 1093 | 1.000915              | 2.112807                                                       |
| 1095 | 1.621918              | 2.112989                                                       |
| 1097 | 1.000912              | 2.113170                                                       |
| 1099 | 1.150136              | 2.113351                                                       |
| 1101 | 1.336966              | 2.113531                                                       |
| 1103 | 1.000907              | 2.113712                                                       |
| 1105 | 1.368326              | 2.113891                                                       |
| 1107 | 1.517615              | 2.114071                                                       |
| 1109 | 1.000902              | 2.114250                                                       |
| 1111 | 1.101710              | 2.114429                                                       |
| 1113 | 1.552561              | 2.114607                                                       |
| 1115 | 1.205381              | 2.114785                                                       |
| 1117 | 1.000895              | 2.114963                                                       |
| 1119 | 1.336908              | 2.115140                                                       |
| 1121 | 1.070473              | 2.115317                                                       |
| 1123 | 1.000890              | 2.115493                                                       |
| 1125 | 1.802667              | 2.115670                                                       |
| 1127 | 1.213842              | 2.115846                                                       |
| 1129 | 1.000886              | 2.116021                                                       |
| 1131 | 1.485411              | 2.116196                                                       |
| 1133 | 1.101500              | 2.116371                                                       |
| 1135 | 1.205286              | 2.116546                                                       |
| 1137 | 1.336851              | 2.116720                                                       |
| 1139 | 1.074627              | 2.116894                                                       |
| 1141 | 1.149869              | 2.117067                                                       |
| 1143 | 1.455818              | 2.117241                                                       |
| 1145 | 1.205240              | 2.117413                                                       |
| 1147 | 1.060157              | 2.117586                                                       |
| 1149 | 1.336815              | 2.117758                                                       |
| 1151 | 1.000869              | 2.117930                                                       |
| 1153 | 1.000867              | 2.118102                                                       |
| 1155 | 1.994805              | 2.118273                                                       |
| 1157 | 1.089023              | 2.118444                                                       |

| $n$  | $\frac{\sigma(n)}{n}$ | $\frac{e^\gamma}{2} \log \log n + \frac{0.73...}{\log \log n}$ |
|------|-----------------------|----------------------------------------------------------------|
| 1159 | 1.069888              | 2.118614                                                       |
| 1161 | 1.515935              | 2.118785                                                       |
| 1163 | 1.000860              | 2.118954                                                       |
| 1165 | 1.205150              | 2.119124                                                       |
| 1167 | 1.336761              | 2.119293                                                       |
| 1169 | 1.149701              | 2.119462                                                       |
| 1171 | 1.000854              | 2.119631                                                       |
| 1173 | 1.473146              | 2.119799                                                       |
| 1175 | 1.266383              | 2.119967                                                       |
| 1177 | 1.101105              | 2.120135                                                       |
| 1179 | 1.455471              | 2.120302                                                       |
| 1181 | 1.000847              | 2.120469                                                       |
| 1183 | 1.237532              | 2.120636                                                       |
| 1185 | 1.620253              | 2.120803                                                       |
| 1187 | 1.000842              | 2.120969                                                       |
| 1189 | 1.059714              | 2.121135                                                       |
| 1191 | 1.336692              | 2.121300                                                       |
| 1193 | 1.000838              | 2.121465                                                       |
| 1195 | 1.205021              | 2.121630                                                       |
| 1197 | 1.737678              | 2.121795                                                       |
| 1199 | 1.100917              | 2.121959                                                       |
| 1201 | 1.000833              | 2.122123                                                       |
| 1203 | 1.336658              | 2.122287                                                       |
| 1205 | 1.204979              | 2.122450                                                       |
| 1207 | 1.073737              | 2.122613                                                       |
| 1209 | 1.482217              | 2.122776                                                       |
| 1211 | 1.149463              | 2.122939                                                       |
| 1213 | 1.000824              | 2.123101                                                       |
| 1215 | 1.797531              | 2.123263                                                       |
| 1217 | 1.000822              | 2.123424                                                       |
| 1219 | 1.063167              | 2.123586                                                       |
| 1221 | 1.493857              | 2.123747                                                       |
| 1223 | 1.000818              | 2.123908                                                       |
| 1225 | 1.442449              | 2.124068                                                       |
| 1227 | 1.336593              | 2.124228                                                       |
| 1229 | 1.000814              | 2.124388                                                       |
| 1231 | 1.000812              | 2.124548                                                       |
| 1233 | 1.454988              | 2.124707                                                       |
| 1235 | 1.360324              | 2.124866                                                       |
| 1237 | 1.000808              | 2.125025                                                       |
| 1239 | 1.549637              | 2.125183                                                       |
| 1241 | 1.073328              | 2.125341                                                       |
| 1243 | 1.100563              | 2.125499                                                       |
| 1245 | 1.619277              | 2.125657                                                       |

| $n$  | $\frac{\sigma(n)}{n}$ | $\frac{e^\gamma}{2} \log \log n + \frac{0.73...}{\log \log n}$ |
|------|-----------------------|----------------------------------------------------------------|
| 1247 | 1.058540              | 2.125814                                                       |
| 1249 | 1.000801              | 2.125971                                                       |
| 1251 | 1.454836              | 2.126128                                                       |
| 1253 | 1.149242              | 2.126285                                                       |
| 1255 | 1.204781              | 2.126441                                                       |
| 1257 | 1.336516              | 2.126597                                                       |
| 1259 | 1.000794              | 2.126753                                                       |
| 1261 | 1.088025              | 2.126908                                                       |
| 1263 | 1.336500              | 2.127063                                                       |
| 1265 | 1.366008              | 2.127218                                                       |
| 1267 | 1.149171              | 2.127373                                                       |
| 1269 | 1.513002              | 2.127527                                                       |
| 1271 | 1.057435              | 2.127681                                                       |
| 1273 | 1.068342              | 2.127835                                                       |
| 1275 | 1.750588              | 2.127988                                                       |
| 1277 | 1.000783              | 2.128142                                                       |
| 1279 | 1.000782              | 2.128295                                                       |
| 1281 | 1.548790              | 2.128448                                                       |
| 1283 | 1.000779              | 2.128600                                                       |
| 1285 | 1.204669              | 2.128752                                                       |
| 1287 | 1.696970              | 2.128904                                                       |
| 1289 | 1.000776              | 2.129056                                                       |
| 1291 | 1.000775              | 2.129207                                                       |
| 1293 | 1.336427              | 2.129359                                                       |
| 1295 | 1.408494              | 2.129510                                                       |
| 1297 | 1.000771              | 2.129660                                                       |
| 1299 | 1.336413              | 2.129811                                                       |
| 1301 | 1.000769              | 2.129961                                                       |
| 1303 | 1.000767              | 2.130111                                                       |
| 1305 | 1.793103              | 2.130260                                                       |
| 1307 | 1.000765              | 2.130410                                                       |
| 1309 | 1.320092              | 2.130559                                                       |
| 1311 | 1.464531              | 2.130708                                                       |
| 1313 | 1.087586              | 2.130856                                                       |
| 1315 | 1.204563              | 2.131005                                                       |
| 1317 | 1.336371              | 2.131153                                                       |
| 1319 | 1.000758              | 2.131301                                                       |
| 1321 | 1.000757              | 2.131449                                                       |
| 1323 | 1.723356              | 2.131596                                                       |
| 1325 | 1.263396              | 2.131743                                                       |
| 1327 | 1.000754              | 2.131890                                                       |
| 1329 | 1.336343              | 2.132037                                                       |
| 1331 | 1.099925              | 2.132183                                                       |
| 1333 | 1.056264              | 2.132329                                                       |

| $n$  | $\frac{\sigma(n)}{n}$ | $\frac{e^\gamma}{2} \log \log n + \frac{0.73...}{\log \log n}$ |
|------|-----------------------|----------------------------------------------------------------|
| 1335 | 1.617978              | 2.132475                                                       |
| 1337 | 1.148841              | 2.132621                                                       |
| 1339 | 1.087379              | 2.132767                                                       |
| 1341 | 1.454139              | 2.132912                                                       |
| 1343 | 1.072226              | 2.133057                                                       |
| 1345 | 1.204461              | 2.133202                                                       |
| 1347 | 1.336303              | 2.133346                                                       |
| 1349 | 1.067457              | 2.133490                                                       |
| 1351 | 1.148779              | 2.133635                                                       |
| 1353 | 1.490022              | 2.133778                                                       |
| 1355 | 1.204428              | 2.133922                                                       |
| 1357 | 1.061164              | 2.134065                                                       |
| 1359 | 1.454010              | 2.134208                                                       |
| 1361 | 1.000735              | 2.134351                                                       |
| 1363 | 1.056493              | 2.134494                                                       |
| 1365 | 1.969231              | 2.134636                                                       |
| 1367 | 1.000732              | 2.134779                                                       |
| 1369 | 1.027757              | 2.134921                                                       |
| 1371 | 1.336251              | 2.135062                                                       |
| 1373 | 1.000728              | 2.135204                                                       |
| 1375 | 1.361455              | 2.135345                                                       |
| 1377 | 1.581699              | 2.135486                                                       |
| 1379 | 1.148658              | 2.135627                                                       |
| 1381 | 1.000724              | 2.135768                                                       |
| 1383 | 1.336226              | 2.135908                                                       |
| 1385 | 1.204332              | 2.136048                                                       |
| 1387 | 1.067051              | 2.136188                                                       |
| 1389 | 1.336213              | 2.136328                                                       |
| 1391 | 1.086988              | 2.136467                                                       |
| 1393 | 1.148600              | 2.136607                                                       |
| 1395 | 1.789247              | 2.136746                                                       |
| 1397 | 1.099499              | 2.136885                                                       |
| 1399 | 1.000715              | 2.137023                                                       |
| 1401 | 1.336188              | 2.137162                                                       |
| 1403 | 1.060584              | 2.137300                                                       |
| 1405 | 1.204270              | 2.137438                                                       |
| 1407 | 1.546553              | 2.137575                                                       |
| 1409 | 1.000710              | 2.137713                                                       |
| 1411 | 1.071580              | 2.137850                                                       |
| 1413 | 1.453645              | 2.137987                                                       |
| 1415 | 1.204240              | 2.138124                                                       |
| 1417 | 1.086803              | 2.138261                                                       |
| 1419 | 1.488372              | 2.138398                                                       |
| 1421 | 1.203378              | 2.138534                                                       |

| $n$  | $\frac{\sigma(n)}{n}$ | $\frac{e^\gamma}{2} \log \log n + \frac{0.73...}{\log \log n}$ |
|------|-----------------------|----------------------------------------------------------------|
| 1423 | 1.000703              | 2.138670                                                       |
| 1425 | 1.740351              | 2.138806                                                       |
| 1427 | 1.000701              | 2.138941                                                       |
| 1429 | 1.000700              | 2.139077                                                       |
| 1431 | 1.509434              | 2.139212                                                       |
| 1433 | 1.000698              | 2.139347                                                       |
| 1435 | 1.404878              | 2.139482                                                       |
| 1437 | 1.336117              | 2.139616                                                       |
| 1439 | 1.000695              | 2.139751                                                       |
| 1441 | 1.099237              | 2.139885                                                       |
| 1443 | 1.474705              | 2.140019                                                       |
| 1445 | 1.274740              | 2.140153                                                       |
| 1447 | 1.000691              | 2.140286                                                       |
| 1449 | 1.722567              | 2.140420                                                       |
| 1451 | 1.000689              | 2.140553                                                       |
| 1453 | 1.000688              | 2.140686                                                       |
| 1455 | 1.616495              | 2.140818                                                       |
| 1457 | 1.054221              | 2.140951                                                       |
| 1459 | 1.000685              | 2.141083                                                       |
| 1461 | 1.336071              | 2.141216                                                       |
| 1463 | 1.312372              | 2.141347                                                       |
| 1465 | 1.204096              | 2.141479                                                       |
| 1467 | 1.453306              | 2.141611                                                       |
| 1469 | 1.086453              | 2.141742                                                       |
| 1471 | 1.000680              | 2.141873                                                       |
| 1473 | 1.336049              | 2.142004                                                       |
| 1475 | 1.261017              | 2.142135                                                       |
| 1477 | 1.148274              | 2.142266                                                       |
| 1479 | 1.460446              | 2.142396                                                       |
| 1481 | 1.000675              | 2.142526                                                       |
| 1483 | 1.000674              | 2.142656                                                       |
| 1485 | 1.939394              | 2.142786                                                       |
| 1487 | 1.000672              | 2.142916                                                       |
| 1489 | 1.000672              | 2.143045                                                       |
| 1491 | 1.545272              | 2.143174                                                       |
| 1493 | 1.000670              | 2.143303                                                       |
| 1495 | 1.348495              | 2.143432                                                       |
| 1497 | 1.336005              | 2.143561                                                       |
| 1499 | 1.000667              | 2.143689                                                       |
| 1501 | 1.065956              | 2.143818                                                       |
| 1503 | 1.453094              | 2.143946                                                       |
| 1505 | 1.403322              | 2.144074                                                       |
| 1507 | 1.098872              | 2.144201                                                       |
| 1509 | 1.335984              | 2.144329                                                       |

| $n$  | $\frac{\sigma(n)}{n}$ | $\frac{e^\gamma}{2} \log \log n + \frac{0.73...}{\log \log n}$ |
|------|-----------------------|----------------------------------------------------------------|
| 1511 | 1.000662              | 2.144456                                                       |
| 1513 | 1.070720              | 2.144583                                                       |
| 1515 | 1.615842              | 2.144710                                                       |
| 1517 | 1.052076              | 2.144837                                                       |
| 1519 | 1.200790              | 2.144964                                                       |
| 1521 | 1.564103              | 2.145090                                                       |
| 1523 | 1.000657              | 2.145217                                                       |
| 1525 | 1.260328              | 2.145343                                                       |
| 1527 | 1.335953              | 2.145468                                                       |
| 1529 | 1.098757              | 2.145594                                                       |
| 1531 | 1.000653              | 2.145720                                                       |
| 1533 | 1.544684              | 2.145845                                                       |
| 1535 | 1.203909              | 2.145970                                                       |
| 1537 | 1.054001              | 2.146095                                                       |
| 1539 | 1.572450              | 2.146220                                                       |
| 1541 | 1.059053              | 2.146345                                                       |
| 1543 | 1.000648              | 2.146469                                                       |
| 1545 | 1.615534              | 2.146593                                                       |
| 1547 | 1.303167              | 2.146717                                                       |
| 1549 | 1.000646              | 2.146841                                                       |
| 1551 | 1.485493              | 2.146965                                                       |
| 1553 | 1.000644              | 2.147089                                                       |
| 1555 | 1.203859              | 2.147212                                                       |
| 1557 | 1.452794              | 2.147335                                                       |
| 1559 | 1.000641              | 2.147458                                                       |
| 1561 | 1.147982              | 2.147581                                                       |
| 1563 | 1.335893              | 2.147704                                                       |
| 1565 | 1.203834              | 2.147826                                                       |
| 1567 | 1.000638              | 2.147949                                                       |
| 1569 | 1.335883              | 2.148071                                                       |
| 1571 | 1.000637              | 2.148193                                                       |
| 1573 | 1.183725              | 2.148315                                                       |
| 1575 | 2.046984              | 2.148436                                                       |
| 1577 | 1.065314              | 2.148558                                                       |
| 1579 | 1.000633              | 2.148679                                                       |
| 1581 | 1.457306              | 2.148800                                                       |
| 1583 | 1.000632              | 2.148921                                                       |
| 1585 | 1.203785              | 2.149042                                                       |
| 1587 | 1.393825              | 2.149163                                                       |
| 1589 | 1.147892              | 2.149283                                                       |
| 1591 | 1.050911              | 2.149404                                                       |
| 1593 | 1.506591              | 2.149524                                                       |
| 1595 | 1.354232              | 2.149644                                                       |
| 1597 | 1.000626              | 2.149764                                                       |



| $n$  | $\frac{\sigma(n)}{n}$ | $\frac{e^\gamma}{2} \log \log n + \frac{0.73...}{\log \log n}$ |
|------|-----------------------|----------------------------------------------------------------|
| 1599 | 1.470919              | 2.149883                                                       |
| 1601 | 1.000625              | 2.150003                                                       |
| 1603 | 1.147848              | 2.150122                                                       |
| 1605 | 1.614953              | 2.150241                                                       |
| 1607 | 1.000622              | 2.150360                                                       |
| 1609 | 1.000622              | 2.150479                                                       |
| 1611 | 1.452514              | 2.150598                                                       |
| 1613 | 1.000620              | 2.150716                                                       |
| 1615 | 1.337461              | 2.150835                                                       |
| 1617 | 1.692022              | 2.150953                                                       |
| 1619 | 1.000618              | 2.151071                                                       |
| 1621 | 1.000617              | 2.151189                                                       |
| 1623 | 1.335798              | 2.151306                                                       |
| 1625 | 1.344000              | 2.151424                                                       |
| 1627 | 1.000615              | 2.151541                                                       |
| 1629 | 1.452425              | 2.151659                                                       |
| 1631 | 1.147762              | 2.151776                                                       |
| 1633 | 1.058175              | 2.151893                                                       |
| 1635 | 1.614679              | 2.152009                                                       |
| 1637 | 1.000611              | 2.152126                                                       |
| 1639 | 1.098231              | 2.152242                                                       |
| 1641 | 1.335771              | 2.152359                                                       |
| 1643 | 1.051735              | 2.152475                                                       |
| 1645 | 1.400608              | 2.152591                                                       |
| 1647 | 1.505768              | 2.152707                                                       |
| 1649 | 1.069739              | 2.152822                                                       |
| 1651 | 1.085403              | 2.152938                                                       |
| 1653 | 1.451906              | 2.153053                                                       |
| 1655 | 1.203625              | 2.153168                                                       |
| 1657 | 1.000604              | 2.153284                                                       |
| 1659 | 1.543098              | 2.153398                                                       |
| 1661 | 1.098134              | 2.153513                                                       |
| 1663 | 1.000601              | 2.153628                                                       |
| 1665 | 1.780180              | 2.153742                                                       |
| 1667 | 1.000600              | 2.153857                                                       |
| 1669 | 1.000599              | 2.153971                                                       |
| 1671 | 1.335727              | 2.154085                                                       |
| 1673 | 1.147639              | 2.154199                                                       |
| 1675 | 1.258507              | 2.154312                                                       |
| 1677 | 1.469290              | 2.154426                                                       |
| 1679 | 1.057772              | 2.154539                                                       |
| 1681 | 1.024985              | 2.154652                                                       |
| 1683 | 1.668449              | 2.154766                                                       |
| 1685 | 1.203561              | 2.154878                                                       |

| $n$  | $\frac{\sigma(n)}{n}$ | $\frac{e^\gamma}{2} \log \log n + \frac{0.73\dots}{\log \log n}$ |
|------|-----------------------|------------------------------------------------------------------|
| 1687 | 1.147599              | 2.154991                                                         |
| 1689 | 1.335702              | 2.155104                                                         |
| 1691 | 1.064459              | 2.155216                                                         |
| 1693 | 1.000591              | 2.155329                                                         |
| 1695 | 1.614159              | 2.155441                                                         |
| 1697 | 1.000589              | 2.155553                                                         |
| 1699 | 1.000589              | 2.155665                                                         |
| 1701 | 1.711934              | 2.155777                                                         |
| 1703 | 1.085144              | 2.155889                                                         |
| 1705 | 1.351320              | 2.156000                                                         |
| 1707 | 1.335677              | 2.156111                                                         |
| 1709 | 1.000585              | 2.156223                                                         |
| 1711 | 1.052016              | 2.156334                                                         |
| 1713 | 1.335668              | 2.156445                                                         |
| 1715 | 1.399417              | 2.156555                                                         |
| 1717 | 1.069307              | 2.156666                                                         |
| 1719 | 1.452007              | 2.156776                                                         |
| 1721 | 1.000581              | 2.156887                                                         |
| 1723 | 1.000580              | 2.156997                                                         |
| 1725 | 1.725217              | 2.157107                                                         |
| 1727 | 1.097858              | 2.157217                                                         |
| 1729 | 1.295547              | 2.157327                                                         |
| 1731 | 1.335644              | 2.157437                                                         |
| 1733 | 1.000577              | 2.157546                                                         |
| 1735 | 1.203458              | 2.157655                                                         |
| 1737 | 1.451929              | 2.157765                                                         |
| 1739 | 1.048879              | 2.157874                                                         |
| 1741 | 1.000574              | 2.157983                                                         |
| 1743 | 1.542169              | 2.158092                                                         |
| 1745 | 1.203438              | 2.158200                                                         |
| 1747 | 1.000572              | 2.158309                                                         |
| 1749 | 1.481990              | 2.158417                                                         |
| 1751 | 1.069103              | 2.158526                                                         |
| 1753 | 1.000570              | 2.158634                                                         |
| 1755 | 1.914530              | 2.158742                                                         |
| 1757 | 1.147410              | 2.158850                                                         |
| 1759 | 1.000569              | 2.158957                                                         |
| 1761 | 1.335605              | 2.159065                                                         |
| 1763 | 1.048213              | 2.159172                                                         |
| 1765 | 1.203399              | 2.159280                                                         |
| 1767 | 1.448783              | 2.159387                                                         |
| 1769 | 1.051441              | 2.159494                                                         |
| 1771 | 1.300960              | 2.159601                                                         |
| 1773 | 1.451777              | 2.159708                                                         |

| $n$  | $\frac{\sigma(n)}{n}$ | $\frac{e^\gamma}{2} \log \log n + \frac{0.73...}{\log \log n}$ |
|------|-----------------------|----------------------------------------------------------------|
| 1775 | 1.257465              | 2.159814                                                       |
| 1777 | 1.000563              | 2.159921                                                       |
| 1779 | 1.335582              | 2.160027                                                       |
| 1781 | 1.084784              | 2.160134                                                       |
| 1783 | 1.000561              | 2.160240                                                       |
| 1785 | 1.936134              | 2.160346                                                       |
| 1787 | 1.000560              | 2.160452                                                       |
| 1789 | 1.000559              | 2.160557                                                       |
| 1791 | 1.451703              | 2.160663                                                       |
| 1793 | 1.097602              | 2.160768                                                       |
| 1795 | 1.203343              | 2.160874                                                       |
| 1797 | 1.335559              | 2.160979                                                       |
| 1799 | 1.147304              | 2.161084                                                       |
| 1801 | 1.000555              | 2.161189                                                       |
| 1803 | 1.335552              | 2.161294                                                       |
| 1805 | 1.266482              | 2.161399                                                       |
| 1807 | 1.084671              | 2.161503                                                       |
| 1809 | 1.503593              | 2.161608                                                       |
| 1811 | 1.000552              | 2.161712                                                       |
| 1813 | 1.194705              | 2.161816                                                       |
| 1815 | 1.758678              | 2.161920                                                       |
| 1817 | 1.056687              | 2.162024                                                       |
| 1819 | 1.068719              | 2.162128                                                       |
| 1821 | 1.335530              | 2.162232                                                       |
| 1823 | 1.000549              | 2.162336                                                       |
| 1825 | 1.256986              | 2.162439                                                       |
| 1827 | 1.707718              | 2.162542                                                       |
| 1829 | 1.049754              | 2.162646                                                       |
| 1831 | 1.000546              | 2.162749                                                       |
| 1833 | 1.466448              | 2.162852                                                       |
| 1835 | 1.203270              | 2.162954                                                       |
| 1837 | 1.097441              | 2.163057                                                       |
| 1839 | 1.335508              | 2.163160                                                       |
| 1841 | 1.147203              | 2.163262                                                       |
| 1843 | 1.063483              | 2.163365                                                       |
| 1845 | 1.775610              | 2.163467                                                       |
| 1847 | 1.000541              | 2.163569                                                       |
| 1849 | 1.023797              | 2.163671                                                       |
| 1851 | 1.335494              | 2.163773                                                       |
| 1853 | 1.068538              | 2.163874                                                       |
| 1855 | 1.397305              | 2.163976                                                       |
| 1857 | 1.335487              | 2.164078                                                       |
| 1859 | 1.181280              | 2.164179                                                       |
| 1861 | 1.000537              | 2.164280                                                       |

| $n$  | $\frac{\sigma(n)}{n}$ | $\frac{e^\gamma}{2} \log \log n + \frac{0.73...}{\log \log n}$ |
|------|-----------------------|----------------------------------------------------------------|
| 1863 | 1.558776              | 2.164381                                                       |
| 1865 | 1.203217              | 2.164482                                                       |
| 1867 | 1.000536              | 2.164583                                                       |
| 1869 | 1.540931              | 2.164684                                                       |
| 1871 | 1.000534              | 2.164785                                                       |
| 1873 | 1.000534              | 2.164885                                                       |
| 1875 | 1.666133              | 2.164986                                                       |
| 1877 | 1.000533              | 2.165086                                                       |
| 1879 | 1.000532              | 2.165186                                                       |
| 1881 | 1.658692              | 2.165286                                                       |
| 1883 | 1.147106              | 2.165386                                                       |
| 1885 | 1.336870              | 2.165486                                                       |
| 1887 | 1.449921              | 2.165586                                                       |
| 1889 | 1.000529              | 2.165685                                                       |
| 1891 | 1.049180              | 2.165785                                                       |
| 1893 | 1.335446              | 2.165884                                                       |
| 1895 | 1.203166              | 2.165984                                                       |
| 1897 | 1.147074              | 2.166083                                                       |
| 1899 | 1.451290              | 2.166182                                                       |
| 1901 | 1.000526              | 2.166281                                                       |
| 1903 | 1.097215              | 2.166380                                                       |
| 1905 | 1.612598              | 2.166478                                                       |
| 1907 | 1.000524              | 2.166577                                                       |
| 1909 | 1.056050              | 2.166675                                                       |
| 1911 | 1.670330              | 2.166774                                                       |
| 1913 | 1.000523              | 2.166872                                                       |
| 1915 | 1.203133              | 2.166970                                                       |
| 1917 | 1.502347              | 2.167068                                                       |
| 1919 | 1.063054              | 2.167166                                                       |
| 1921 | 1.068194              | 2.167264                                                       |
| 1923 | 1.335413              | 2.167361                                                       |
| 1925 | 1.545974              | 2.167459                                                       |
| 1927 | 1.046186              | 2.167556                                                       |
| 1929 | 1.335407              | 2.167654                                                       |
| 1931 | 1.000518              | 2.167751                                                       |
| 1933 | 1.000517              | 2.167848                                                       |
| 1935 | 1.773643              | 2.167945                                                       |
| 1937 | 1.084151              | 2.168042                                                       |
| 1939 | 1.146983              | 2.168139                                                       |
| 1941 | 1.335394              | 2.168235                                                       |
| 1943 | 1.049923              | 2.168332                                                       |
| 1945 | 1.203085              | 2.168429                                                       |
| 1947 | 1.479199              | 2.168525                                                       |
| 1949 | 1.000513              | 2.168621                                                       |

| $n$  | $\frac{\sigma(n)}{n}$ | $\frac{e^\gamma}{2} \log \log n + \frac{0.73...}{\log \log n}$ |
|------|-----------------------|----------------------------------------------------------------|
| 1951 | 1.000513              | 2.168717                                                       |
| 1953 | 1.704045              | 2.168813                                                       |
| 1955 | 1.325831              | 2.168909                                                       |
| 1957 | 1.062851              | 2.169005                                                       |
| 1959 | 1.335375              | 2.169101                                                       |
| 1961 | 1.046405              | 2.169196                                                       |
| 1963 | 1.084055              | 2.169292                                                       |
| 1965 | 1.612214              | 2.169387                                                       |
| 1967 | 1.146924              | 2.169482                                                       |
| 1969 | 1.097004              | 2.169578                                                       |
| 1971 | 1.501776              | 2.169673                                                       |
| 1973 | 1.000507              | 2.169768                                                       |
| 1975 | 1.255696              | 2.169863                                                       |
| 1977 | 1.335357              | 2.169957                                                       |
| 1979 | 1.000505              | 2.170052                                                       |
| 1981 | 1.146896              | 2.170146                                                       |
| 1983 | 1.335350              | 2.170241                                                       |
| 1985 | 1.203023              | 2.170335                                                       |
| 1987 | 1.000503              | 2.170429                                                       |
| 1989 | 1.647059              | 2.170524                                                       |
| 1991 | 1.096936              | 2.170618                                                       |
| 1993 | 1.000502              | 2.170711                                                       |
| 1995 | 1.924812              | 2.170805                                                       |
| 1997 | 1.000501              | 2.170899                                                       |
| 1999 | 1.000500              | 2.170993                                                       |
| 2001 | 1.439280              | 2.171086                                                       |
| 2003 | 1.000499              | 2.171180                                                       |
| 2005 | 1.202993              | 2.171273                                                       |
| 2007 | 1.450922              | 2.171366                                                       |
| 2009 | 1.191638              | 2.171459                                                       |
| 2011 | 1.000497              | 2.171552                                                       |
| 2013 | 1.478390              | 2.171645                                                       |
| 2015 | 1.333995              | 2.171738                                                       |
| 2017 | 1.000496              | 2.171830                                                       |
| 2019 | 1.335315              | 2.171923                                                       |
| 2021 | 1.045027              | 2.172015                                                       |
| 2023 | 1.214039              | 2.172108                                                       |
| 2025 | 1.852346              | 2.172200                                                       |
| 2027 | 1.000493              | 2.172292                                                       |
| 2029 | 1.000493              | 2.172384                                                       |
| 2031 | 1.335303              | 2.172476                                                       |
| 2033 | 1.062469              | 2.172568                                                       |
| 2035 | 1.344472              | 2.172660                                                       |
| 2037 | 1.539519              | 2.172752                                                       |

| $n$  | $\frac{\sigma(n)}{n}$ | $\frac{e^\gamma}{2} \log \log n + \frac{0.73\dots}{\log \log n}$ |
|------|-----------------------|------------------------------------------------------------------|
| 2039 | 1.000490              | 2.172843                                                         |
| 2041 | 1.083782              | 2.172935                                                         |
| 2043 | 1.450808              | 2.173026                                                         |
| 2045 | 1.202934              | 2.173118                                                         |
| 2047 | 1.055203              | 2.173209                                                         |
| 2049 | 1.335286              | 2.173300                                                         |
| 2051 | 1.146758              | 2.173391                                                         |
| 2053 | 1.000487              | 2.173482                                                         |
| 2055 | 1.611679              | 2.173573                                                         |
| 2057 | 1.163831              | 2.173663                                                         |
| 2059 | 1.049053              | 2.173754                                                         |
| 2061 | 1.450752              | 2.173844                                                         |
| 2063 | 1.000485              | 2.173935                                                         |
| 2065 | 1.394673              | 2.174025                                                         |
| 2067 | 1.462990              | 2.174115                                                         |
| 2069 | 1.000483              | 2.174205                                                         |
| 2071 | 1.062289              | 2.174295                                                         |
| 2073 | 1.335263              | 2.174385                                                         |
| 2075 | 1.254940              | 2.174475                                                         |
| 2077 | 1.047665              | 2.174565                                                         |
| 2079 | 1.847042              | 2.174655                                                         |
| 2081 | 1.000481              | 2.174744                                                         |
| 2083 | 1.000480              | 2.174834                                                         |
| 2085 | 1.611511              | 2.174923                                                         |
| 2087 | 1.000479              | 2.175012                                                         |
| 2089 | 1.000479              | 2.175101                                                         |
| 2091 | 1.446198              | 2.175191                                                         |
| 2093 | 1.284281              | 2.175280                                                         |
| 2095 | 1.202864              | 2.175368                                                         |
| 2097 | 1.450644              | 2.175457                                                         |
| 2099 | 1.000476              | 2.175546                                                         |
| 2101 | 1.096621              | 2.175635                                                         |
| 2103 | 1.335235              | 2.175723                                                         |
| 2105 | 1.202850              | 2.175812                                                         |
| 2107 | 1.190318              | 2.175900                                                         |
| 2109 | 1.441441              | 2.175988                                                         |
| 2111 | 1.000474              | 2.176076                                                         |
| 2113 | 1.000473              | 2.176164                                                         |
| 2115 | 1.770213              | 2.176252                                                         |
| 2117 | 1.048654              | 2.176340                                                         |
| 2119 | 1.083530              | 2.176428                                                         |
| 2121 | 1.538897              | 2.176516                                                         |
| 2123 | 1.096561              | 2.176603                                                         |
| 2125 | 1.321412              | 2.176691                                                         |

| $n$  | $\frac{\sigma(n)}{n}$ | $\frac{e^\gamma}{2} \log \log n + \frac{0.73...}{\log \log n}$ |
|------|-----------------------|----------------------------------------------------------------|
| 2127 | 1.335214              | 2.176778                                                       |
| 2129 | 1.000470              | 2.176866                                                       |
| 2131 | 1.000469              | 2.176953                                                       |
| 2133 | 1.500234              | 2.177040                                                       |
| 2135 | 1.393911              | 2.177127                                                       |
| 2137 | 1.000468              | 2.177214                                                       |
| 2139 | 1.436185              | 2.177301                                                       |
| 2141 | 1.000467              | 2.177388                                                       |
| 2143 | 1.000467              | 2.177474                                                       |
| 2145 | 1.879720              | 2.177561                                                       |
| 2147 | 1.061947              | 2.177648                                                       |
| 2149 | 1.146580              | 2.177734                                                       |
| 2151 | 1.450488              | 2.177820                                                       |
| 2153 | 1.000464              | 2.177907                                                       |
| 2155 | 1.202784              | 2.177993                                                       |
| 2157 | 1.335188              | 2.178079                                                       |
| 2159 | 1.067161              | 2.178165                                                       |
| 2161 | 1.000463              | 2.178251                                                       |
| 2163 | 1.538604              | 2.178337                                                       |
| 2165 | 1.202771              | 2.178422                                                       |
| 2167 | 1.096447              | 2.178508                                                       |
| 2169 | 1.450438              | 2.178594                                                       |
| 2171 | 1.083372              | 2.178679                                                       |
| 2173 | 1.043718              | 2.178765                                                       |
| 2175 | 1.710345              | 2.178850                                                       |
| 2177 | 1.146532              | 2.178935                                                       |
| 2179 | 1.000459              | 2.179020                                                       |
| 2181 | 1.335167              | 2.179105                                                       |
| 2183 | 1.044434              | 2.179190                                                       |
| 2185 | 1.318078              | 2.179275                                                       |
| 2187 | 1.499771              | 2.179360                                                       |
| 2189 | 1.096391              | 2.179445                                                       |
| 2191 | 1.146508              | 2.179529                                                       |
| 2193 | 1.444596              | 2.179614                                                       |
| 2195 | 1.202733              | 2.179698                                                       |
| 2197 | 1.083295              | 2.179783                                                       |
| 2199 | 1.335152              | 2.179867                                                       |
| 2201 | 1.046797              | 2.179951                                                       |
| 2203 | 1.000454              | 2.180035                                                       |
| 2205 | 2.016327              | 2.180119                                                       |
| 2207 | 1.000453              | 2.180203                                                       |
| 2209 | 1.021729              | 2.180287                                                       |
| 2211 | 1.476255              | 2.180371                                                       |
| 2213 | 1.000452              | 2.180455                                                       |

| $n$  | $\frac{\sigma(n)}{n}$ | $\frac{e^\gamma}{2} \log \log n + \frac{0.73\dots}{\log \log n}$ |
|------|-----------------------|------------------------------------------------------------------|
| 2215 | 1.202709              | 2.180538                                                         |
| 2217 | 1.335138              | 2.180622                                                         |
| 2219 | 1.146462              | 2.180705                                                         |
| 2221 | 1.000450              | 2.180789                                                         |
| 2223 | 1.637427              | 2.180872                                                         |
| 2225 | 1.253933              | 2.180955                                                         |
| 2227 | 1.066906              | 2.181038                                                         |
| 2229 | 1.335128              | 2.181121                                                         |
| 2231 | 1.054236              | 2.181204                                                         |
| 2233 | 1.289745              | 2.181287                                                         |
| 2235 | 1.610738              | 2.181370                                                         |
| 2237 | 1.000447              | 2.181453                                                         |
| 2239 | 1.000447              | 2.181535                                                         |
| 2241 | 1.499331              | 2.181618                                                         |
| 2243 | 1.000446              | 2.181700                                                         |
| 2245 | 1.202673              | 2.181783                                                         |
| 2247 | 1.538051              | 2.181865                                                         |
| 2249 | 1.083148              | 2.181947                                                         |
| 2251 | 1.000444              | 2.182029                                                         |
| 2253 | 1.335109              | 2.182112                                                         |
| 2255 | 1.341020              | 2.182194                                                         |
| 2257 | 1.043864              | 2.182275                                                         |
| 2259 | 1.450199              | 2.182357                                                         |
| 2261 | 1.273773              | 2.182439                                                         |
| 2263 | 1.046399              | 2.182521                                                         |
| 2265 | 1.610596              | 2.182602                                                         |
| 2267 | 1.000441              | 2.182684                                                         |
| 2269 | 1.000441              | 2.182765                                                         |
| 2271 | 1.335095              | 2.182847                                                         |
| 2273 | 1.000440              | 2.182928                                                         |
| 2275 | 1.526154              | 2.183009                                                         |
| 2277 | 1.644269              | 2.183090                                                         |
| 2279 | 1.042563              | 2.183171                                                         |
| 2281 | 1.000438              | 2.183252                                                         |
| 2283 | 1.335085              | 2.183333                                                         |
| 2285 | 1.202626              | 2.183414                                                         |
| 2287 | 1.000437              | 2.183495                                                         |
| 2289 | 1.537789              | 2.183575                                                         |
| 2291 | 1.047577              | 2.183656                                                         |
| 2293 | 1.000436              | 2.183736                                                         |
| 2295 | 1.882353              | 2.183817                                                         |
| 2297 | 1.000435              | 2.183897                                                         |
| 2299 | 1.157025              | 2.183977                                                         |
| 2301 | 1.460235              | 2.184058                                                         |



| $n$  | $\frac{\sigma(n)}{n}$ | $\frac{e^\gamma}{2} \log \log n + \frac{0.73...}{\log \log n}$ |
|------|-----------------------|----------------------------------------------------------------|
| 2303 | 1.188016              | 2.184138                                                       |
| 2305 | 1.202603              | 2.184218                                                       |
| 2307 | 1.335067              | 2.184298                                                       |
| 2309 | 1.000433              | 2.184378                                                       |
| 2311 | 1.000433              | 2.184457                                                       |
| 2313 | 1.450065              | 2.184537                                                       |
| 2315 | 1.202592              | 2.184617                                                       |
| 2317 | 1.146310              | 2.184696                                                       |
| 2319 | 1.335058              | 2.184776                                                       |
| 2321 | 1.096079              | 2.184855                                                       |
| 2323 | 1.053810              | 2.184935                                                       |
| 2325 | 1.706667              | 2.185014                                                       |
| 2327 | 1.082939              | 2.185093                                                       |
| 2329 | 1.066552              | 2.185172                                                       |
| 2331 | 1.695410              | 2.185251                                                       |
| 2333 | 1.000429              | 2.185330                                                       |
| 2335 | 1.202570              | 2.185409                                                       |
| 2337 | 1.437741              | 2.185488                                                       |
| 2339 | 1.000428              | 2.185567                                                       |
| 2341 | 1.000427              | 2.185646                                                       |
| 2343 | 1.475032              | 2.185724                                                       |
| 2345 | 1.391898              | 2.185803                                                       |
| 2347 | 1.000426              | 2.185881                                                       |
| 2349 | 1.545338              | 2.185960                                                       |
| 2351 | 1.000425              | 2.186038                                                       |
| 2353 | 1.082873              | 2.186116                                                       |
| 2355 | 1.610191              | 2.186194                                                       |
| 2357 | 1.000424              | 2.186273                                                       |
| 2359 | 1.146248              | 2.186351                                                       |
| 2361 | 1.335028              | 2.186429                                                       |
| 2363 | 1.066441              | 2.186506                                                       |
| 2365 | 1.339535              | 2.186584                                                       |
| 2367 | 1.449937              | 2.186662                                                       |
| 2369 | 1.053609              | 2.186740                                                       |
| 2371 | 1.000422              | 2.186817                                                       |
| 2373 | 1.537295              | 2.186895                                                       |
| 2375 | 1.313684              | 2.186972                                                       |
| 2377 | 1.000421              | 2.187050                                                       |
| 2379 | 1.459437              | 2.187127                                                       |
| 2381 | 1.000420              | 2.187204                                                       |
| 2383 | 1.000420              | 2.187281                                                       |
| 2385 | 1.766038              | 2.187358                                                       |
| 2387 | 1.286971              | 2.187435                                                       |
| 2389 | 1.000419              | 2.187512                                                       |

| $n$  | $\frac{\sigma(n)}{n}$ | $\frac{e^\gamma}{2} \log \log n + \frac{0.73...}{\log \log n}$ |
|------|-----------------------|----------------------------------------------------------------|
| 2391 | 1.335006              | 2.187589                                                       |
| 2393 | 1.000418              | 2.187666                                                       |
| 2395 | 1.202505              | 2.187743                                                       |
| 2397 | 1.441802              | 2.187819                                                       |
| 2399 | 1.000417              | 2.187896                                                       |
| 2401 | 1.166597              | 2.187973                                                       |
| 2403 | 1.498127              | 2.188049                                                       |
| 2405 | 1.327235              | 2.188125                                                       |
| 2407 | 1.046946              | 2.188202                                                       |
| 2409 | 1.474471              | 2.188278                                                       |
| 2411 | 1.000415              | 2.188354                                                       |
| 2413 | 1.060920              | 2.188430                                                       |
| 2415 | 1.908075              | 2.188506                                                       |
| 2417 | 1.000414              | 2.188582                                                       |
| 2419 | 1.041753              | 2.188658                                                       |
| 2421 | 1.449814              | 2.188734                                                       |
| 2423 | 1.000413              | 2.188810                                                       |
| 2425 | 1.252784              | 2.188886                                                       |
| 2427 | 1.334981              | 2.188961                                                       |
| 2429 | 1.146151              | 2.189037                                                       |
| 2431 | 1.243933              | 2.189112                                                       |
| 2433 | 1.334977              | 2.189188                                                       |
| 2435 | 1.202464              | 2.189263                                                       |
| 2437 | 1.000410              | 2.189338                                                       |
| 2439 | 1.449774              | 2.189414                                                       |
| 2441 | 1.000410              | 2.189489                                                       |
| 2443 | 1.146132              | 2.189564                                                       |
| 2445 | 1.609816              | 2.189639                                                       |
| 2447 | 1.000409              | 2.189714                                                       |
| 2449 | 1.045325              | 2.189789                                                       |
| 2451 | 1.436149              | 2.189864                                                       |
| 2453 | 1.095801              | 2.189938                                                       |
| 2455 | 1.202444              | 2.190013                                                       |
| 2457 | 1.823362              | 2.190088                                                       |
| 2459 | 1.000407              | 2.190162                                                       |
| 2461 | 1.053230              | 2.190237                                                       |
| 2463 | 1.334957              | 2.190311                                                       |
| 2465 | 1.314402              | 2.190385                                                       |
| 2467 | 1.000405              | 2.190460                                                       |
| 2469 | 1.334953              | 2.190534                                                       |
| 2471 | 1.146095              | 2.190608                                                       |
| 2473 | 1.000404              | 2.190682                                                       |
| 2475 | 1.953939              | 2.190756                                                       |
| 2477 | 1.000404              | 2.190830                                                       |

| $n$  | $\frac{\sigma(n)}{n}$ | $\frac{e^\gamma}{2} \log \log n + \frac{0.73...}{\log \log n}$ |
|------|-----------------------|----------------------------------------------------------------|
| 2479 | 1.042356              | 2.190904                                                       |
| 2481 | 1.334946              | 2.190978                                                       |
| 2483 | 1.082561              | 2.191052                                                       |
| 2485 | 1.390744              | 2.191125                                                       |
| 2487 | 1.334942              | 2.191199                                                       |
| 2489 | 1.060667              | 2.191273                                                       |
| 2491 | 1.040546              | 2.191346                                                       |
| 2493 | 1.449659              | 2.191419                                                       |
| 2495 | 1.202405              | 2.191493                                                       |
| 2497 | 1.095715              | 2.191566                                                       |
| 2499 | 1.642257              | 2.191639                                                       |
| 2501 | 1.041184              | 2.191713                                                       |
| 2503 | 1.000400              | 2.191786                                                       |
| 2505 | 1.609581              | 2.191859                                                       |
| 2507 | 1.053051              | 2.191932                                                       |
| 2509 | 1.082503              | 2.192005                                                       |
| 2511 | 1.542015              | 2.192078                                                       |
| 2513 | 1.146041              | 2.192150                                                       |
| 2515 | 1.202386              | 2.192223                                                       |
| 2517 | 1.334923              | 2.192296                                                       |
| 2519 | 1.095673              | 2.192368                                                       |
| 2521 | 1.000397              | 2.192441                                                       |
| 2523 | 1.380896              | 2.192513                                                       |
| 2525 | 1.252277              | 2.192586                                                       |
| 2527 | 1.206173              | 2.192658                                                       |
| 2529 | 1.449585              | 2.192730                                                       |
| 2531 | 1.000395              | 2.192803                                                       |
| 2533 | 1.065930              | 2.192875                                                       |
| 2535 | 1.732544              | 2.192947                                                       |
| 2537 | 1.040599              | 2.193019                                                       |
| 2539 | 1.000394              | 2.193091                                                       |
| 2541 | 1.674931              | 2.193163                                                       |
| 2543 | 1.000393              | 2.193235                                                       |
| 2545 | 1.202358              | 2.193306                                                       |
| 2547 | 1.449548              | 2.193378                                                       |
| 2549 | 1.000392              | 2.193450                                                       |
| 2551 | 1.000392              | 2.193522                                                       |
| 2553 | 1.428907              | 2.193593                                                       |
| 2555 | 1.390215              | 2.193665                                                       |
| 2557 | 1.000391              | 2.193736                                                       |
| 2559 | 1.334896              | 2.193807                                                       |
| 2561 | 1.082390              | 2.193879                                                       |
| 2563 | 1.095591              | 2.193950                                                       |
| 2565 | 1.871345              | 2.194021                                                       |

| $n$  | $\frac{\sigma(n)}{n}$ | $\frac{e^\gamma}{2} \log \log n + \frac{0.73...}{\log \log n}$ |
|------|-----------------------|----------------------------------------------------------------|
| 2567 | 1.065836              | 2.194092                                                       |
| 2569 | 1.145971              | 2.194163                                                       |
| 2571 | 1.334889              | 2.194234                                                       |
| 2573 | 1.044695              | 2.194305                                                       |
| 2575 | 1.252039              | 2.194376                                                       |
| 2577 | 1.334886              | 2.194447                                                       |
| 2579 | 1.000388              | 2.194518                                                       |
| 2581 | 1.046106              | 2.194588                                                       |
| 2583 | 1.691057              | 2.194659                                                       |
| 2585 | 1.336944              | 2.194729                                                       |
| 2587 | 1.082335              | 2.194800                                                       |
| 2589 | 1.334878              | 2.194870                                                       |
| 2591 | 1.000386              | 2.194941                                                       |
| 2593 | 1.000386              | 2.195011                                                       |
| 2595 | 1.609249              | 2.195081                                                       |
| 2597 | 1.185214              | 2.195152                                                       |
| 2599 | 1.052713              | 2.195222                                                       |
| 2601 | 1.534410              | 2.195292                                                       |
| 2603 | 1.060315              | 2.195362                                                       |
| 2605 | 1.202303              | 2.195432                                                       |
| 2607 | 1.472957              | 2.195502                                                       |
| 2609 | 1.000383              | 2.195572                                                       |
| 2611 | 1.145921              | 2.195642                                                       |
| 2613 | 1.457329              | 2.195711                                                       |
| 2615 | 1.202294              | 2.195781                                                       |
| 2617 | 1.000382              | 2.195851                                                       |
| 2619 | 1.496754              | 2.195920                                                       |
| 2621 | 1.000382              | 2.195990                                                       |
| 2623 | 1.040030              | 2.196059                                                       |
| 2625 | 1.901714              | 2.196129                                                       |
| 2627 | 1.041492              | 2.196198                                                       |
| 2629 | 1.095474              | 2.196267                                                       |
| 2631 | 1.334854              | 2.196336                                                       |
| 2633 | 1.000380              | 2.196406                                                       |
| 2635 | 1.311575              | 2.196475                                                       |
| 2637 | 1.449374              | 2.196544                                                       |
| 2639 | 1.273210              | 2.196613                                                       |
| 2641 | 1.060204              | 2.196682                                                       |
| 2643 | 1.334847              | 2.196750                                                       |
| 2645 | 1.254442              | 2.196819                                                       |
| 2647 | 1.000378              | 2.196888                                                       |
| 2649 | 1.334843              | 2.196957                                                       |
| 2651 | 1.095436              | 2.197025                                                       |
| 2653 | 1.145873              | 2.197094                                                       |

| $n$  | $\frac{\sigma(n)}{n}$ | $\frac{e^\gamma}{2} \log \log n + \frac{0.73...}{\log \log n}$ |
|------|-----------------------|----------------------------------------------------------------|
| 2655 | 1.762712              | 2.197163                                                       |
| 2657 | 1.000376              | 2.197231                                                       |
| 2659 | 1.000376              | 2.197299                                                       |
| 2661 | 1.334837              | 2.197368                                                       |
| 2663 | 1.000376              | 2.197436                                                       |
| 2665 | 1.323827              | 2.197504                                                       |
| 2667 | 1.535808              | 2.197573                                                       |
| 2669 | 1.065568              | 2.197641                                                       |
| 2671 | 1.000374              | 2.197709                                                       |
| 2673 | 1.634119              | 2.197777                                                       |
| 2675 | 1.251589              | 2.197845                                                       |
| 2677 | 1.000374              | 2.197913                                                       |
| 2679 | 1.433371              | 2.197981                                                       |
| 2681 | 1.145841              | 2.198048                                                       |
| 2683 | 1.000373              | 2.198116                                                       |
| 2685 | 1.608939              | 2.198184                                                       |
| 2687 | 1.000372              | 2.198251                                                       |
| 2689 | 1.000372              | 2.198319                                                       |
| 2691 | 1.623188              | 2.198387                                                       |
| 2693 | 1.000371              | 2.198454                                                       |
| 2695 | 1.522820              | 2.198521                                                       |
| 2697 | 1.423804              | 2.198589                                                       |
| 2699 | 1.000371              | 2.198656                                                       |
| 2701 | 1.041096              | 2.198723                                                       |
| 2703 | 1.438402              | 2.198791                                                       |
| 2705 | 1.202218              | 2.198858                                                       |
| 2707 | 1.000369              | 2.198925                                                       |
| 2709 | 1.689184              | 2.198992                                                       |
| 2711 | 1.000369              | 2.199059                                                       |
| 2713 | 1.000369              | 2.199126                                                       |
| 2715 | 1.608840              | 2.199193                                                       |
| 2717 | 1.236658              | 2.199259                                                       |
| 2719 | 1.000368              | 2.199326                                                       |
| 2721 | 1.334803              | 2.199393                                                       |
| 2723 | 1.145795              | 2.199460                                                       |
| 2725 | 1.251376              | 2.199526                                                       |
| 2727 | 1.496150              | 2.199593                                                       |
| 2729 | 1.000366              | 2.199659                                                       |
| 2731 | 1.000366              | 2.199726                                                       |
| 2733 | 1.334797              | 2.199792                                                       |
| 2735 | 1.202194              | 2.199858                                                       |
| 2737 | 1.262696              | 2.199925                                                       |
| 2739 | 1.472070              | 2.199991                                                       |
| 2741 | 1.000365              | 2.200057                                                       |

| $n$  | $\frac{\sigma(n)}{n}$ | $\frac{e^\gamma}{2} \log \log n + \frac{0.73\dots}{\log \log n}$ |
|------|-----------------------|------------------------------------------------------------------|
| 2743 | 1.082027              | 2.200123                                                         |
| 2745 | 1.761749              | 2.200189                                                         |
| 2747 | 1.039680              | 2.200255                                                         |
| 2749 | 1.000364              | 2.200321                                                         |
| 2751 | 1.535442              | 2.200387                                                         |
| 2753 | 1.000363              | 2.200453                                                         |
| 2755 | 1.306715              | 2.200519                                                         |
| 2757 | 1.334784              | 2.200585                                                         |
| 2759 | 1.043856              | 2.200650                                                         |
| 2761 | 1.095255              | 2.200716                                                         |
| 2763 | 1.449149              | 2.200782                                                         |
| 2765 | 1.388788              | 2.200847                                                         |
| 2767 | 1.000361              | 2.200913                                                         |
| 2769 | 1.456121              | 2.200978                                                         |
| 2771 | 1.065319              | 2.201043                                                         |
| 2773 | 1.038586              | 2.201109                                                         |
| 2775 | 1.698018              | 2.201174                                                         |
| 2777 | 1.000360              | 2.201239                                                         |
| 2779 | 1.145736              | 2.201304                                                         |
| 2781 | 1.495865              | 2.201370                                                         |
| 2783 | 1.146964              | 2.201435                                                         |
| 2785 | 1.202154              | 2.201500                                                         |
| 2787 | 1.334769              | 2.201565                                                         |
| 2789 | 1.000359              | 2.201630                                                         |
| 2791 | 1.000358              | 2.201695                                                         |
| 2793 | 1.632653              | 2.201759                                                         |
| 2795 | 1.322361              | 2.201824                                                         |
| 2797 | 1.000358              | 2.201889                                                         |
| 2799 | 1.449089              | 2.201954                                                         |
| 2801 | 1.000357              | 2.202018                                                         |
| 2803 | 1.000357              | 2.202083                                                         |
| 2805 | 1.848128              | 2.202147                                                         |
| 2807 | 1.145707              | 2.202212                                                         |
| 2809 | 1.019224              | 2.202276                                                         |
| 2811 | 1.334756              | 2.202341                                                         |
| 2813 | 1.045148              | 2.202405                                                         |
| 2815 | 1.202131              | 2.202469                                                         |
| 2817 | 1.449059              | 2.202533                                                         |
| 2819 | 1.000355              | 2.202597                                                         |
| 2821 | 1.270471              | 2.202662                                                         |
| 2823 | 1.334750              | 2.202726                                                         |
| 2825 | 1.250973              | 2.202790                                                         |
| 2827 | 1.095154              | 2.202854                                                         |
| 2829 | 1.425239              | 2.202918                                                         |

| $n$  | $\frac{\sigma(n)}{n}$ | $\frac{e^\gamma}{2} \log \log n + \frac{0.73...}{\log \log n}$ |
|------|-----------------------|----------------------------------------------------------------|
| 2831 | 1.059696              | 2.202981                                                       |
| 2833 | 1.000353              | 2.203045                                                       |
| 2835 | 2.048677              | 2.203109                                                       |
| 2837 | 1.000352              | 2.203173                                                       |
| 2839 | 1.065164              | 2.203236                                                       |
| 2841 | 1.334741              | 2.203300                                                       |
| 2843 | 1.000352              | 2.203364                                                       |
| 2845 | 1.202109              | 2.203427                                                       |
| 2847 | 1.455567              | 2.203491                                                       |
| 2849 | 1.280449              | 2.203554                                                       |
| 2851 | 1.000351              | 2.203618                                                       |
| 2853 | 1.449001              | 2.203681                                                       |
| 2855 | 1.202102              | 2.203744                                                       |
| 2857 | 1.000350              | 2.203807                                                       |
| 2859 | 1.334732              | 2.203871                                                       |
| 2861 | 1.000350              | 2.203934                                                       |
| 2863 | 1.145651              | 2.203997                                                       |
| 2865 | 1.608377              | 2.204060                                                       |
| 2867 | 1.038019              | 2.204123                                                       |
| 2869 | 1.059603              | 2.204186                                                       |
| 2871 | 1.630094              | 2.204249                                                       |
| 2873 | 1.146537              | 2.204312                                                       |
| 2875 | 1.302261              | 2.204374                                                       |
| 2877 | 1.534932              | 2.204437                                                       |
| 2879 | 1.000347              | 2.204500                                                       |
| 2881 | 1.038528              | 2.204562                                                       |
| 2883 | 1.377732              | 2.204625                                                       |
| 2885 | 1.202080              | 2.204688                                                       |
| 2887 | 1.000346              | 2.204750                                                       |
| 2889 | 1.495327              | 2.204813                                                       |
| 2891 | 1.182982              | 2.204875                                                       |
| 2893 | 1.095057              | 2.204937                                                       |
| 2895 | 1.608290              | 2.205000                                                       |
| 2897 | 1.000345              | 2.205062                                                       |
| 2899 | 1.081752              | 2.205124                                                       |
| 2901 | 1.334712              | 2.205186                                                       |
| 2903 | 1.000344              | 2.205249                                                       |
| 2905 | 1.387952              | 2.205311                                                       |
| 2907 | 1.609907              | 2.205373                                                       |
| 2909 | 1.000344              | 2.205435                                                       |
| 2911 | 1.038818              | 2.205497                                                       |
| 2913 | 1.334706              | 2.205559                                                       |
| 2915 | 1.333791              | 2.205620                                                       |
| 2917 | 1.000343              | 2.205682                                                       |

| $n$  | $\frac{\sigma(n)}{n}$ | $\frac{e^\gamma}{2} \log \log n + \frac{0.73...}{\log \log n}$ |
|------|-----------------------|----------------------------------------------------------------|
| 2919 | 1.534772              | 2.205744                                                       |
| 2921 | 1.051695              | 2.205806                                                       |
| 2923 | 1.040027              | 2.205867                                                       |
| 2925 | 1.928889              | 2.205929                                                       |
| 2927 | 1.000342              | 2.205991                                                       |
| 2929 | 1.044725              | 2.206052                                                       |
| 2931 | 1.334698              | 2.206114                                                       |
| 2933 | 1.145585              | 2.206175                                                       |
| 2935 | 1.202044              | 2.206236                                                       |
| 2937 | 1.470889              | 2.206298                                                       |
| 2939 | 1.000340              | 2.206359                                                       |
| 2941 | 1.064944              | 2.206420                                                       |
| 2943 | 1.495073              | 2.206482                                                       |
| 2945 | 1.303905              | 2.206543                                                       |
| 2947 | 1.145572              | 2.206604                                                       |
| 2949 | 1.334690              | 2.206665                                                       |
| 2951 | 1.081667              | 2.206726                                                       |
| 2953 | 1.000339              | 2.206787                                                       |
| 2955 | 1.608122              | 2.206848                                                       |
| 2957 | 1.000338              | 2.206909                                                       |
| 2959 | 1.094965              | 2.206970                                                       |
| 2961 | 1.685917              | 2.207030                                                       |
| 2963 | 1.000337              | 2.207091                                                       |
| 2965 | 1.202024              | 2.207152                                                       |
| 2967 | 1.423660              | 2.207213                                                       |
| 2969 | 1.000337              | 2.207273                                                       |
| 2971 | 1.000337              | 2.207334                                                       |
| 2973 | 1.334679              | 2.207394                                                       |
| 2975 | 1.500504              | 2.207455                                                       |
| 2977 | 1.081626              | 2.207515                                                       |
| 2979 | 1.448808              | 2.207576                                                       |
| 2981 | 1.094935              | 2.207636                                                       |
| 2983 | 1.059336              | 2.207696                                                       |
| 2985 | 1.608040              | 2.207757                                                       |
| 2987 | 1.044526              | 2.207817                                                       |
| 2989 | 1.182335              | 2.207877                                                       |
| 2991 | 1.334671              | 2.207937                                                       |
| 2993 | 1.038423              | 2.207997                                                       |
| 2995 | 1.202003              | 2.208057                                                       |
| 2997 | 1.534201              | 2.208117                                                       |
| 2999 | 1.000333              | 2.208177                                                       |
| 3001 | 1.000333              | 2.208237                                                       |
| 3003 | 1.790210              | 2.208297                                                       |
| 3005 | 1.201997              | 2.208357                                                       |



| $n$  | $\frac{\sigma(n)}{n}$ | $\frac{e^\gamma}{2} \log \log n + \frac{0.73...}{\log \log n}$ |
|------|-----------------------|----------------------------------------------------------------|
| 3007 | 1.042900              | 2.208417                                                       |
| 3009 | 1.435693              | 2.208476                                                       |
| 3011 | 1.000332              | 2.208536                                                       |
| 3013 | 1.051444              | 2.208596                                                       |
| 3015 | 1.759204              | 2.208655                                                       |
| 3017 | 1.145509              | 2.208715                                                       |
| 3019 | 1.000331              | 2.208774                                                       |
| 3021 | 1.429990              | 2.208834                                                       |
| 3023 | 1.000331              | 2.208893                                                       |
| 3025 | 1.362975              | 2.208953                                                       |
| 3027 | 1.334655              | 2.209012                                                       |
| 3029 | 1.081545              | 2.209071                                                       |
| 3031 | 1.145497              | 2.209131                                                       |
| 3033 | 1.448731              | 2.209190                                                       |
| 3035 | 1.201977              | 2.209249                                                       |
| 3037 | 1.000329              | 2.209308                                                       |
| 3039 | 1.334650              | 2.209367                                                       |
| 3041 | 1.000329              | 2.209426                                                       |
| 3043 | 1.064739              | 2.209485                                                       |
| 3045 | 1.891626              | 2.209544                                                       |
| 3047 | 1.094847              | 2.209603                                                       |
| 3049 | 1.000328              | 2.209662                                                       |
| 3051 | 1.494592              | 2.209721                                                       |
| 3053 | 1.037668              | 2.209780                                                       |
| 3055 | 1.319804              | 2.209838                                                       |
| 3057 | 1.334642              | 2.209897                                                       |
| 3059 | 1.255312              | 2.209956                                                       |
| 3061 | 1.000327              | 2.210014                                                       |
| 3063 | 1.334639              | 2.210073                                                       |
| 3065 | 1.201958              | 2.210132                                                       |
| 3067 | 1.000326              | 2.210190                                                       |
| 3069 | 1.626588              | 2.210249                                                       |
| 3071 | 1.039401              | 2.210307                                                       |
| 3073 | 1.145460              | 2.210365                                                       |
| 3075 | 1.693659              | 2.210424                                                       |
| 3077 | 1.064673              | 2.210482                                                       |
| 3079 | 1.000325              | 2.210540                                                       |
| 3081 | 1.454073              | 2.210598                                                       |
| 3083 | 1.000324              | 2.210657                                                       |
| 3085 | 1.201945              | 2.210715                                                       |
| 3087 | 1.684483              | 2.210773                                                       |
| 3089 | 1.000324              | 2.210831                                                       |
| 3091 | 1.094791              | 2.210889                                                       |
| 3093 | 1.334627              | 2.210947                                                       |

| $n$  | $\frac{\sigma(n)}{n}$ | $\frac{e^\gamma}{2} \log \log n + \frac{0.73...}{\log \log n}$ |
|------|-----------------------|----------------------------------------------------------------|
| 3095 | 1.201939              | 2.211005                                                       |
| 3097 | 1.059089              | 2.211063                                                       |
| 3099 | 1.334624              | 2.211120                                                       |
| 3101 | 1.145437              | 2.211178                                                       |
| 3103 | 1.044151              | 2.211236                                                       |
| 3105 | 1.855072              | 2.211294                                                       |
| 3107 | 1.081429              | 2.211351                                                       |
| 3109 | 1.000322              | 2.211409                                                       |
| 3111 | 1.434908              | 2.211467                                                       |
| 3113 | 1.094764              | 2.211524                                                       |
| 3115 | 1.386838              | 2.211582                                                       |
| 3117 | 1.334617              | 2.211639                                                       |
| 3119 | 1.000321              | 2.211697                                                       |
| 3121 | 1.000320              | 2.211754                                                       |
| 3123 | 1.448607              | 2.211811                                                       |
| 3125 | 1.249920              | 2.211869                                                       |
| 3127 | 1.036137              | 2.211926                                                       |
| 3129 | 1.534036              | 2.211983                                                       |
| 3131 | 1.042478              | 2.212040                                                       |
| 3133 | 1.081392              | 2.212098                                                       |
| 3135 | 1.837321              | 2.212155                                                       |
| 3137 | 1.000319              | 2.212212                                                       |
| 3139 | 1.037273              | 2.212269                                                       |
| 3141 | 1.448583              | 2.212326                                                       |
| 3143 | 1.145402              | 2.212383                                                       |
| 3145 | 1.304928              | 2.212440                                                       |
| 3147 | 1.334604              | 2.212497                                                       |
| 3149 | 1.036520              | 2.212553                                                       |
| 3151 | 1.051095              | 2.212610                                                       |
| 3153 | 1.334602              | 2.212667                                                       |
| 3155 | 1.201902              | 2.212724                                                       |
| 3157 | 1.277162              | 2.212780                                                       |
| 3159 | 1.613169              | 2.212837                                                       |
| 3161 | 1.043973              | 2.212894                                                       |
| 3163 | 1.000316              | 2.212950                                                       |
| 3165 | 1.607583              | 2.213007                                                       |
| 3167 | 1.000316              | 2.213063                                                       |
| 3169 | 1.000316              | 2.213120                                                       |
| 3171 | 1.533901              | 2.213176                                                       |
| 3173 | 1.058935              | 2.213232                                                       |
| 3175 | 1.249764              | 2.213289                                                       |
| 3177 | 1.448536              | 2.213345                                                       |
| 3179 | 1.158855              | 2.213401                                                       |
| 3181 | 1.000314              | 2.213457                                                       |

| $n$  | $\frac{\sigma(n)}{n}$ | $\frac{e^\gamma}{2} \log \log n + \frac{0.73...}{\log \log n}$ |
|------|-----------------------|----------------------------------------------------------------|
| 3183 | 1.334590              | 2.213514                                                       |
| 3185 | 1.503297              | 2.213570                                                       |
| 3187 | 1.000314              | 2.213626                                                       |
| 3189 | 1.334588              | 2.213682                                                       |
| 3191 | 1.000313              | 2.213738                                                       |
| 3193 | 1.042280              | 2.213794                                                       |
| 3195 | 1.757746              | 2.213850                                                       |
| 3197 | 1.050985              | 2.213906                                                       |
| 3199 | 1.145358              | 2.213961                                                       |
| 3201 | 1.469541              | 2.214017                                                       |
| 3203 | 1.000312              | 2.214073                                                       |
| 3205 | 1.201872              | 2.214129                                                       |
| 3207 | 1.334581              | 2.214185                                                       |
| 3209 | 1.000312              | 2.214240                                                       |
| 3211 | 1.139832              | 2.214296                                                       |
| 3213 | 1.792717              | 2.214351                                                       |
| 3215 | 1.201866              | 2.214407                                                       |
| 3217 | 1.000311              | 2.214463                                                       |
| 3219 | 1.416589              | 2.214518                                                       |
| 3221 | 1.000310              | 2.214573                                                       |
| 3223 | 1.094632              | 2.214629                                                       |
| 3225 | 1.691783              | 2.214684                                                       |
| 3227 | 1.145336              | 2.214740                                                       |
| 3229 | 1.000310              | 2.214795                                                       |
| 3231 | 1.448468              | 2.214850                                                       |
| 3233 | 1.035571              | 2.214905                                                       |
| 3235 | 1.201855              | 2.214961                                                       |
| 3237 | 1.453197              | 2.215016                                                       |
| 3239 | 1.037357              | 2.215071                                                       |
| 3241 | 1.145326              | 2.215126                                                       |
| 3243 | 1.420907              | 2.215181                                                       |
| 3245 | 1.331279              | 2.215236                                                       |
| 3247 | 1.064367              | 2.215291                                                       |
| 3249 | 1.524469              | 2.215346                                                       |
| 3251 | 1.000308              | 2.215401                                                       |
| 3253 | 1.000307              | 2.215455                                                       |
| 3255 | 1.887558              | 2.215510                                                       |
| 3257 | 1.000307              | 2.215565                                                       |
| 3259 | 1.000307              | 2.215620                                                       |
| 3261 | 1.334560              | 2.215674                                                       |
| 3263 | 1.081214              | 2.215729                                                       |
| 3265 | 1.201838              | 2.215784                                                       |
| 3267 | 1.628405              | 2.215838                                                       |
| 3269 | 1.145304              | 2.215893                                                       |

| $n$  | $\frac{\sigma(n)}{n}$ | $\frac{e^\gamma}{2} \log \log n + \frac{0.73\dots}{\log \log n}$ |
|------|-----------------------|------------------------------------------------------------------|
| 3271 | 1.000306              | 2.215947                                                         |
| 3273 | 1.334555              | 2.216002                                                         |
| 3275 | 1.249466              | 2.216056                                                         |
| 3277 | 1.043637              | 2.216111                                                         |
| 3279 | 1.334553              | 2.216165                                                         |
| 3281 | 1.064310              | 2.216219                                                         |
| 3283 | 1.180627              | 2.216274                                                         |
| 3285 | 1.757078              | 2.216328                                                         |
| 3287 | 1.058716              | 2.216382                                                         |
| 3289 | 1.225905              | 2.216436                                                         |
| 3291 | 1.334549              | 2.216491                                                         |
| 3293 | 1.038567              | 2.216545                                                         |
| 3295 | 1.201821              | 2.216599                                                         |
| 3297 | 1.533515              | 2.216653                                                         |
| 3299 | 1.000303              | 2.216707                                                         |
| 3301 | 1.000303              | 2.216761                                                         |
| 3303 | 1.448380              | 2.216815                                                         |
| 3305 | 1.201815              | 2.216869                                                         |
| 3307 | 1.000302              | 2.216922                                                         |
| 3309 | 1.334542              | 2.216976                                                         |
| 3311 | 1.275748              | 2.217030                                                         |
| 3313 | 1.000302              | 2.217084                                                         |
| 3315 | 1.824434              | 2.217138                                                         |
| 3317 | 1.041905              | 2.217191                                                         |
| 3319 | 1.000301              | 2.217245                                                         |
| 3321 | 1.530262              | 2.217299                                                         |
| 3323 | 1.000301              | 2.217352                                                         |
| 3325 | 1.491729              | 2.217406                                                         |
| 3327 | 1.334536              | 2.217459                                                         |
| 3329 | 1.000300              | 2.217513                                                         |
| 3331 | 1.000300              | 2.217566                                                         |
| 3333 | 1.468947              | 2.217619                                                         |
| 3335 | 1.295352              | 2.217673                                                         |
| 3337 | 1.035661              | 2.217726                                                         |
| 3339 | 1.681941              | 2.217779                                                         |
| 3341 | 1.081113              | 2.217833                                                         |
| 3343 | 1.000299              | 2.217886                                                         |
| 3345 | 1.607175              | 2.217939                                                         |
| 3347 | 1.000299              | 2.217992                                                         |
| 3349 | 1.064198              | 2.218045                                                         |
| 3351 | 1.334527              | 2.218099                                                         |
| 3353 | 1.145243              | 2.218152                                                         |
| 3355 | 1.330551              | 2.218205                                                         |
| 3357 | 1.448317              | 2.218258                                                         |

| $n$  | $\frac{\sigma(n)}{n}$ | $\frac{e^\gamma}{2} \log \log n + \frac{0.73\dots}{\log \log n}$ |
|------|-----------------------|------------------------------------------------------------------|
| 3359 | 1.000298              | 2.218311                                                         |
| 3361 | 1.000298              | 2.218363                                                         |
| 3363 | 1.427297              | 2.218416                                                         |
| 3365 | 1.201783              | 2.218469                                                         |
| 3367 | 1.264033              | 2.218522                                                         |
| 3369 | 1.334521              | 2.218575                                                         |
| 3371 | 1.000297              | 2.218628                                                         |
| 3373 | 1.000296              | 2.218680                                                         |
| 3375 | 1.848889              | 2.218733                                                         |
| 3377 | 1.094463              | 2.218786                                                         |
| 3379 | 1.041728              | 2.218838                                                         |
| 3381 | 1.618456              | 2.218891                                                         |
| 3383 | 1.064144              | 2.218943                                                         |
| 3385 | 1.201773              | 2.218996                                                         |
| 3387 | 1.334514              | 2.219048                                                         |
| 3389 | 1.000295              | 2.219101                                                         |
| 3391 | 1.000295              | 2.219153                                                         |
| 3393 | 1.609195              | 2.219205                                                         |
| 3395 | 1.385567              | 2.219258                                                         |
| 3397 | 1.036208              | 2.219310                                                         |
| 3399 | 1.468667              | 2.219362                                                         |
| 3401 | 1.058512              | 2.219415                                                         |
| 3403 | 1.036732              | 2.219467                                                         |
| 3405 | 1.607048              | 2.219519                                                         |
| 3407 | 1.000294              | 2.219571                                                         |
| 3409 | 1.145204              | 2.219623                                                         |
| 3411 | 1.448256              | 2.219675                                                         |
| 3413 | 1.000293              | 2.219727                                                         |
| 3415 | 1.201757              | 2.219779                                                         |
| 3417 | 1.432836              | 2.219831                                                         |
| 3419 | 1.081018              | 2.219883                                                         |
| 3421 | 1.094417              | 2.219935                                                         |
| 3423 | 1.533158              | 2.219987                                                         |
| 3425 | 1.249051              | 2.220039                                                         |
| 3427 | 1.050481              | 2.220091                                                         |
| 3429 | 1.493147              | 2.220142                                                         |
| 3431 | 1.035267              | 2.220194                                                         |
| 3433 | 1.000291              | 2.220246                                                         |
| 3435 | 1.606987              | 2.220298                                                         |
| 3437 | 1.145185              | 2.220349                                                         |
| 3439 | 1.058447              | 2.220401                                                         |
| 3441 | 1.413543              | 2.220452                                                         |
| 3443 | 1.094394              | 2.220504                                                         |
| 3445 | 1.316691              | 2.220555                                                         |

| $n$  | $\frac{\sigma(n)}{n}$ | $\frac{e^\gamma}{2} \log \log n + \frac{0.73...}{\log \log n}$ |
|------|-----------------------|----------------------------------------------------------------|
| 3447 | 1.448216              | 2.220607                                                       |
| 3449 | 1.000290              | 2.220658                                                       |
| 3451 | 1.251811              | 2.220710                                                       |
| 3453 | 1.334492              | 2.220761                                                       |
| 3455 | 1.201737              | 2.220812                                                       |
| 3457 | 1.000289              | 2.220864                                                       |
| 3459 | 1.334490              | 2.220915                                                       |
| 3461 | 1.000289              | 2.220966                                                       |
| 3463 | 1.000289              | 2.221017                                                       |
| 3465 | 2.161039              | 2.221069                                                       |
| 3467 | 1.000288              | 2.221120                                                       |
| 3469 | 1.000288              | 2.221171                                                       |
| 3471 | 1.452031              | 2.221222                                                       |
| 3473 | 1.050389              | 2.221273                                                       |
| 3475 | 1.248921              | 2.221324                                                       |
| 3477 | 1.426517              | 2.221375                                                       |
| 3479 | 1.179649              | 2.221426                                                       |
| 3481 | 1.017236              | 2.221477                                                       |
| 3483 | 1.528567              | 2.221528                                                       |
| 3485 | 1.301578              | 2.221579                                                       |
| 3487 | 1.094350              | 2.221629                                                       |
| 3489 | 1.334480              | 2.221680                                                       |
| 3491 | 1.000286              | 2.221731                                                       |
| 3493 | 1.145147              | 2.221782                                                       |
| 3495 | 1.606867              | 2.221832                                                       |
| 3497 | 1.080927              | 2.221883                                                       |
| 3499 | 1.000286              | 2.221934                                                       |
| 3501 | 1.448158              | 2.221984                                                       |
| 3503 | 1.041393              | 2.222035                                                       |
| 3505 | 1.201712              | 2.222085                                                       |
| 3507 | 1.532934              | 2.222136                                                       |
| 3509 | 1.137076              | 2.222186                                                       |
| 3511 | 1.000285              | 2.222237                                                       |
| 3513 | 1.334472              | 2.222287                                                       |
| 3515 | 1.297297              | 2.222338                                                       |
| 3517 | 1.000284              | 2.222388                                                       |
| 3519 | 1.595908              | 2.222438                                                       |
| 3521 | 1.145129              | 2.222489                                                       |
| 3523 | 1.080897              | 2.222539                                                       |
| 3525 | 1.688511              | 2.222589                                                       |
| 3527 | 1.000284              | 2.222639                                                       |
| 3529 | 1.000283              | 2.222689                                                       |
| 3531 | 1.468139              | 2.222740                                                       |
| 3533 | 1.000283              | 2.222790                                                       |

| $n$  | $\frac{\sigma(n)}{n}$ | $\frac{e^\gamma}{2} \log \log n + \frac{0.73...}{\log \log n}$ |
|------|-----------------------|----------------------------------------------------------------|
| 3535 | 1.385007              | 2.222840                                                       |
| 3537 | 1.492791              | 2.222890                                                       |
| 3539 | 1.000283              | 2.222940                                                       |
| 3541 | 1.000282              | 2.222990                                                       |
| 3543 | 1.334462              | 2.223040                                                       |
| 3545 | 1.201693              | 2.223090                                                       |
| 3547 | 1.000282              | 2.223140                                                       |
| 3549 | 1.650042              | 2.223189                                                       |
| 3551 | 1.034075              | 2.223239                                                       |
| 3553 | 1.215874              | 2.223289                                                       |
| 3555 | 1.755274              | 2.223339                                                       |
| 3557 | 1.000281              | 2.223388                                                       |
| 3559 | 1.000281              | 2.223438                                                       |
| 3561 | 1.334457              | 2.223488                                                       |
| 3563 | 1.145102              | 2.223537                                                       |
| 3565 | 1.292567              | 2.223587                                                       |
| 3567 | 1.412952              | 2.223637                                                       |
| 3569 | 1.035584              | 2.223686                                                       |
| 3571 | 1.000280              | 2.223736                                                       |
| 3573 | 1.448083              | 2.223785                                                       |
| 3575 | 1.456783              | 2.223835                                                       |
| 3577 | 1.179200              | 2.223884                                                       |
| 3579 | 1.334451              | 2.223933                                                       |
| 3581 | 1.000279              | 2.223983                                                       |
| 3583 | 1.000279              | 2.224032                                                       |
| 3585 | 1.606695              | 2.224082                                                       |
| 3587 | 1.063842              | 2.224131                                                       |
| 3589 | 1.037615              | 2.224180                                                       |
| 3591 | 1.782233              | 2.224229                                                       |
| 3593 | 1.000278              | 2.224278                                                       |
| 3595 | 1.201669              | 2.224328                                                       |
| 3597 | 1.467890              | 2.224377                                                       |
| 3599 | 1.033620              | 2.224426                                                       |
| 3601 | 1.080811              | 2.224475                                                       |
| 3603 | 1.334444              | 2.224524                                                       |
| 3605 | 1.384743              | 2.224573                                                       |
| 3607 | 1.000277              | 2.224622                                                       |
| 3609 | 1.448047              | 2.224671                                                       |
| 3611 | 1.050125              | 2.224720                                                       |
| 3613 | 1.000277              | 2.224769                                                       |
| 3615 | 1.606639              | 2.224817                                                       |
| 3617 | 1.000276              | 2.224866                                                       |
| 3619 | 1.273280              | 2.224915                                                       |
| 3621 | 1.431649              | 2.224964                                                       |

| $n$  | $\frac{\sigma(n)}{n}$ | $\frac{e^\gamma}{2} \log \log n + \frac{0.73...}{\log \log n}$ |
|------|-----------------------|----------------------------------------------------------------|
| 3623 | 1.000276              | 2.225013                                                       |
| 3625 | 1.291034              | 2.225061                                                       |
| 3627 | 1.605735              | 2.225110                                                       |
| 3629 | 1.058143              | 2.225159                                                       |
| 3631 | 1.000275              | 2.225207                                                       |
| 3633 | 1.532618              | 2.225256                                                       |
| 3635 | 1.201651              | 2.225304                                                       |
| 3637 | 1.000275              | 2.225353                                                       |
| 3639 | 1.334433              | 2.225401                                                       |
| 3641 | 1.094205              | 2.225450                                                       |
| 3643 | 1.000274              | 2.225498                                                       |
| 3645 | 1.799177              | 2.225547                                                       |
| 3647 | 1.145051              | 2.225595                                                       |
| 3649 | 1.035900              | 2.225644                                                       |
| 3651 | 1.334429              | 2.225692                                                       |
| 3653 | 1.080756              | 2.225740                                                       |
| 3655 | 1.300137              | 2.225788                                                       |
| 3657 | 1.417555              | 2.225837                                                       |
| 3659 | 1.000273              | 2.225885                                                       |
| 3661 | 1.145042              | 2.225933                                                       |
| 3663 | 1.618346              | 2.225981                                                       |
| 3665 | 1.201637              | 2.226029                                                       |
| 3667 | 1.058086              | 2.226077                                                       |
| 3669 | 1.334424              | 2.226126                                                       |
| 3671 | 1.000272              | 2.226174                                                       |
| 3673 | 1.000272              | 2.226222                                                       |
| 3675 | 1.923265              | 2.226270                                                       |
| 3677 | 1.000272              | 2.226318                                                       |
| 3679 | 1.080728              | 2.226365                                                       |
| 3681 | 1.447976              | 2.226413                                                       |
| 3683 | 1.042628              | 2.226461                                                       |
| 3685 | 1.328630              | 2.226509                                                       |
| 3687 | 1.334418              | 2.226557                                                       |
| 3689 | 1.249119              | 2.226605                                                       |
| 3691 | 1.000271              | 2.226652                                                       |
| 3693 | 1.334416              | 2.226700                                                       |
| 3695 | 1.201624              | 2.226748                                                       |
| 3697 | 1.000270              | 2.226796                                                       |
| 3699 | 1.492295              | 2.226843                                                       |
| 3701 | 1.000270              | 2.226891                                                       |
| 3703 | 1.194707              | 2.226938                                                       |
| 3705 | 1.813765              | 2.226986                                                       |
| 3707 | 1.094146              | 2.227033                                                       |
| 3709 | 1.000270              | 2.227081                                                       |



| $n$  | $\frac{\sigma(n)}{n}$ | $\frac{e^\gamma}{2} \log \log n + \frac{0.73\dots}{\log \log n}$ |
|------|-----------------------|------------------------------------------------------------------|
| 3711 | 1.334411              | 2.227128                                                         |
| 3713 | 1.034204              | 2.227176                                                         |
| 3715 | 1.201615              | 2.227223                                                         |
| 3717 | 1.678773              | 2.227271                                                         |
| 3719 | 1.000269              | 2.227318                                                         |
| 3721 | 1.016662              | 2.227365                                                         |
| 3723 | 1.431104              | 2.227413                                                         |
| 3725 | 1.248322              | 2.227460                                                         |
| 3727 | 1.000268              | 2.227507                                                         |
| 3729 | 1.467418              | 2.227554                                                         |
| 3731 | 1.260788              | 2.227602                                                         |
| 3733 | 1.000268              | 2.227649                                                         |
| 3735 | 1.754217              | 2.227696                                                         |
| 3737 | 1.037196              | 2.227743                                                         |
| 3739 | 1.000267              | 2.227790                                                         |
| 3741 | 1.411387              | 2.227837                                                         |
| 3743 | 1.057975              | 2.227884                                                         |
| 3745 | 1.384246              | 2.227931                                                         |
| 3747 | 1.334401              | 2.227978                                                         |
| 3749 | 1.049880              | 2.228025                                                         |
| 3751 | 1.134631              | 2.228072                                                         |
| 3753 | 1.492140              | 2.228119                                                         |
| 3755 | 1.201598              | 2.228166                                                         |
| 3757 | 1.143998              | 2.228213                                                         |
| 3759 | 1.532322              | 2.228259                                                         |
| 3761 | 1.000266              | 2.228306                                                         |
| 3763 | 1.033218              | 2.228353                                                         |
| 3765 | 1.606375              | 2.228400                                                         |
| 3767 | 1.000265              | 2.228446                                                         |
| 3769 | 1.000265              | 2.228493                                                         |
| 3771 | 1.447892              | 2.228540                                                         |
| 3773 | 1.272197              | 2.228586                                                         |
| 3775 | 1.248212              | 2.228633                                                         |
| 3777 | 1.334392              | 2.228680                                                         |
| 3779 | 1.000265              | 2.228726                                                         |
| 3781 | 1.057921              | 2.228773                                                         |
| 3783 | 1.450701              | 2.228819                                                         |
| 3785 | 1.201585              | 2.228866                                                         |
| 3787 | 1.144970              | 2.228912                                                         |
| 3789 | 1.447875              | 2.228958                                                         |
| 3791 | 1.063572              | 2.229005                                                         |
| 3793 | 1.000264              | 2.229051                                                         |
| 3795 | 1.821344              | 2.229097                                                         |
| 3797 | 1.000263              | 2.229144                                                         |

| $n$  | $\frac{\sigma(n)}{n}$ | $\frac{e^\gamma}{2} \log \log n + \frac{0.73...}{\log \log n}$ |
|------|-----------------------|----------------------------------------------------------------|
| 3799 | 1.042380              | 2.229190                                                       |
| 3801 | 1.532228              | 2.229236                                                       |
| 3803 | 1.000263              | 2.229282                                                       |
| 3805 | 1.201577              | 2.229329                                                       |
| 3807 | 1.525611              | 2.229375                                                       |
| 3809 | 1.080599              | 2.229421                                                       |
| 3811 | 1.036998              | 2.229467                                                       |
| 3813 | 1.409913              | 2.229513                                                       |
| 3815 | 1.384010              | 2.229559                                                       |
| 3817 | 1.094053              | 2.229605                                                       |
| 3819 | 1.424457              | 2.229651                                                       |
| 3821 | 1.000262              | 2.229697                                                       |
| 3823 | 1.000262              | 2.229743                                                       |
| 3825 | 1.896471              | 2.229789                                                       |
| 3827 | 1.034753              | 2.229835                                                       |
| 3829 | 1.144946              | 2.229881                                                       |
| 3831 | 1.334377              | 2.229927                                                       |
| 3833 | 1.000261              | 2.229973                                                       |
| 3835 | 1.314211              | 2.230018                                                       |
| 3837 | 1.334376              | 2.230064                                                       |
| 3839 | 1.094035              | 2.230110                                                       |
| 3841 | 1.049727              | 2.230156                                                       |
| 3843 | 1.677856              | 2.230201                                                       |
| 3845 | 1.201560              | 2.230247                                                       |
| 3847 | 1.000260              | 2.230293                                                       |
| 3849 | 1.334373              | 2.230338                                                       |
| 3851 | 1.000260              | 2.230384                                                       |
| 3853 | 1.000260              | 2.230429                                                       |
| 3855 | 1.606226              | 2.230475                                                       |
| 3857 | 1.244491              | 2.230520                                                       |
| 3859 | 1.063488              | 2.230566                                                       |
| 3861 | 1.740482              | 2.230611                                                       |
| 3863 | 1.000259              | 2.230657                                                       |
| 3865 | 1.201552              | 2.230702                                                       |
| 3867 | 1.334368              | 2.230748                                                       |
| 3869 | 1.032825              | 2.230793                                                       |
| 3871 | 1.177990              | 2.230838                                                       |
| 3873 | 1.334366              | 2.230883                                                       |
| 3875 | 1.288258              | 2.230929                                                       |
| 3877 | 1.000258              | 2.230974                                                       |
| 3879 | 1.447796              | 2.231019                                                       |
| 3881 | 1.000258              | 2.231064                                                       |
| 3883 | 1.093999              | 2.231110                                                       |
| 3885 | 1.877992              | 2.231155                                                       |

| $n$  | $\frac{\sigma(n)}{n}$ | $\frac{e^\gamma}{2} \log \log n + \frac{0.73...}{\log \log n}$ |
|------|-----------------------|----------------------------------------------------------------|
| 3887 | 1.129920              | 2.231200                                                       |
| 3889 | 1.000257              | 2.231245                                                       |
| 3891 | 1.334361              | 2.231290                                                       |
| 3893 | 1.063447              | 2.231335                                                       |
| 3895 | 1.293967              | 2.231380                                                       |
| 3897 | 1.447780              | 2.231425                                                       |
| 3899 | 1.144909              | 2.231470                                                       |
| 3901 | 1.033581              | 2.231515                                                       |
| 3903 | 1.334358              | 2.231560                                                       |
| 3905 | 1.327529              | 2.231605                                                       |
| 3907 | 1.000256              | 2.231650                                                       |
| 3909 | 1.334357              | 2.231695                                                       |
| 3911 | 1.000256              | 2.231739                                                       |
| 3913 | 1.259392              | 2.231784                                                       |
| 3915 | 1.839080              | 2.231829                                                       |
| 3917 | 1.000255              | 2.231874                                                       |
| 3919 | 1.000255              | 2.231918                                                       |
| 3921 | 1.334353              | 2.231963                                                       |
| 3923 | 1.000255              | 2.232008                                                       |
| 3925 | 1.247898              | 2.232052                                                       |
| 3927 | 1.760122              | 2.232097                                                       |
| 3929 | 1.000255              | 2.232142                                                       |
| 3931 | 1.000254              | 2.232186                                                       |
| 3933 | 1.586575              | 2.232231                                                       |
| 3935 | 1.201525              | 2.232275                                                       |
| 3937 | 1.040386              | 2.232320                                                       |
| 3939 | 1.450114              | 2.232364                                                       |
| 3941 | 1.144887              | 2.232409                                                       |
| 3943 | 1.000254              | 2.232453                                                       |
| 3945 | 1.606084              | 2.232498                                                       |
| 3947 | 1.000253              | 2.232542                                                       |
| 3949 | 1.093948              | 2.232586                                                       |
| 3951 | 1.447735              | 2.232631                                                       |
| 3953 | 1.032127              | 2.232675                                                       |
| 3955 | 1.383565              | 2.232719                                                       |
| 3957 | 1.334344              | 2.232763                                                       |
| 3959 | 1.036625              | 2.232808                                                       |
| 3961 | 1.063368              | 2.232852                                                       |
| 3963 | 1.334343              | 2.232896                                                       |
| 3965 | 1.313493              | 2.232940                                                       |
| 3967 | 1.000252              | 2.232984                                                       |
| 3969 | 1.737717              | 2.233028                                                       |
| 3971 | 1.151347              | 2.233073                                                       |
| 3973 | 1.042034              | 2.233117                                                       |

| $n$  | $\frac{\sigma(n)}{n}$ | $\frac{e^\gamma}{2} \log \log n + \frac{0.73...}{\log \log n}$ |
|------|-----------------------|----------------------------------------------------------------|
| 3975 | 1.684528              | 2.233161                                                       |
| 3977 | 1.034951              | 2.233205                                                       |
| 3979 | 1.049510              | 2.233249                                                       |
| 3981 | 1.334338              | 2.233293                                                       |
| 3983 | 1.144866              | 2.233337                                                       |
| 3985 | 1.201506              | 2.233380                                                       |
| 3987 | 1.447705              | 2.233424                                                       |
| 3989 | 1.000251              | 2.233468                                                       |
| 3991 | 1.080431              | 2.233512                                                       |
| 3993 | 1.466566              | 2.233556                                                       |
| 3995 | 1.297622              | 2.233600                                                       |
| 3997 | 1.144859              | 2.233643                                                       |
| 3999 | 1.408352              | 2.233687                                                       |
| 4001 | 1.000250              | 2.233731                                                       |
| 4003 | 1.000250              | 2.233775                                                       |
| 4005 | 1.752809              | 2.233818                                                       |
| 4007 | 1.000250              | 2.233862                                                       |
| 4009 | 1.057620              | 2.233905                                                       |
| 4011 | 1.531788              | 2.233949                                                       |
| 4013 | 1.000249              | 2.233993                                                       |
| 4015 | 1.327024              | 2.234036                                                       |
| 4017 | 1.449838              | 2.234080                                                       |
| 4019 | 1.000249              | 2.234123                                                       |
| 4021 | 1.000249              | 2.234167                                                       |
| 4023 | 1.491424              | 2.234210                                                       |
| 4025 | 1.478758              | 2.234254                                                       |
| 4027 | 1.000248              | 2.234297                                                       |
| 4029 | 1.429635              | 2.234340                                                       |
| 4031 | 1.041925              | 2.234384                                                       |
| 4033 | 1.036449              | 2.234427                                                       |
| 4035 | 1.605948              | 2.234470                                                       |
| 4037 | 1.093882              | 2.234514                                                       |
| 4039 | 1.144838              | 2.234557                                                       |
| 4041 | 1.447661              | 2.234600                                                       |
| 4043 | 1.080386              | 2.234643                                                       |
| 4045 | 1.201483              | 2.234687                                                       |
| 4047 | 1.423277              | 2.234730                                                       |
| 4049 | 1.000247              | 2.234773                                                       |
| 4051 | 1.000247              | 2.234816                                                       |
| 4053 | 1.531705              | 2.234859                                                       |
| 4055 | 1.201480              | 2.234902                                                       |
| 4057 | 1.000246              | 2.234945                                                       |
| 4059 | 1.614191              | 2.234988                                                       |
| 4061 | 1.040138              | 2.235031                                                       |

| $n$  | $\frac{\sigma(n)}{n}$ | $\frac{e^\gamma}{2} \log \log n + \frac{0.73...}{\log \log n}$ |
|------|-----------------------|----------------------------------------------------------------|
| 4063 | 1.063254              | 2.235074                                                       |
| 4065 | 1.605904              | 2.235117                                                       |
| 4067 | 1.177281              | 2.235160                                                       |
| 4069 | 1.080364              | 2.235203                                                       |
| 4071 | 1.414886              | 2.235246                                                       |
| 4073 | 1.000246              | 2.235289                                                       |
| 4075 | 1.247607              | 2.235332                                                       |
| 4077 | 1.491293              | 2.235375                                                       |
| 4079 | 1.000245              | 2.235417                                                       |
| 4081 | 1.270277              | 2.235460                                                       |
| 4083 | 1.334313              | 2.235503                                                       |
| 4085 | 1.292534              | 2.235546                                                       |
| 4087 | 1.031563              | 2.235588                                                       |
| 4089 | 1.408657              | 2.235631                                                       |
| 4091 | 1.000244              | 2.235674                                                       |
| 4093 | 1.000244              | 2.235716                                                       |
| 4095 | 2.133333              | 2.235759                                                       |
| 4097 | 1.063217              | 2.235802                                                       |
| 4099 | 1.000244              | 2.235844                                                       |
| 4101 | 1.334309              | 2.235887                                                       |
| 4103 | 1.093834              | 2.235929                                                       |
| 4105 | 1.201462              | 2.235972                                                       |
| 4107 | 1.370343              | 2.236014                                                       |
| 4109 | 1.144804              | 2.236057                                                       |
| 4111 | 1.000243              | 2.236099                                                       |
| 4113 | 1.447605              | 2.236142                                                       |
| 4115 | 1.201458              | 2.236184                                                       |
| 4117 | 1.049308              | 2.236226                                                       |
| 4119 | 1.334304              | 2.236269                                                       |
| 4121 | 1.080320              | 2.236311                                                       |
| 4123 | 1.241814              | 2.236353                                                       |
| 4125 | 1.815273              | 2.236396                                                       |
| 4127 | 1.000242              | 2.236438                                                       |
| 4129 | 1.000242              | 2.236480                                                       |
| 4131 | 1.586057              | 2.236522                                                       |
| 4133 | 1.000242              | 2.236565                                                       |
| 4135 | 1.201451              | 2.236607                                                       |
| 4137 | 1.531545              | 2.236649                                                       |
| 4139 | 1.000242              | 2.236691                                                       |
| 4141 | 1.034533              | 2.236733                                                       |
| 4143 | 1.334299              | 2.236775                                                       |
| 4145 | 1.201448              | 2.236817                                                       |
| 4147 | 1.215336              | 2.236859                                                       |
| 4149 | 1.447578              | 2.236901                                                       |

| $n$  | $\frac{\sigma(n)}{n}$ | $\frac{e^\gamma}{2} \log \log n + \frac{0.73...}{\log \log n}$ |
|------|-----------------------|----------------------------------------------------------------|
| 4151 | 1.144784              | 2.236943                                                       |
| 4153 | 1.000241              | 2.236985                                                       |
| 4155 | 1.605776              | 2.237027                                                       |
| 4157 | 1.000241              | 2.237069                                                       |
| 4159 | 1.000240              | 2.237111                                                       |
| 4161 | 1.422735              | 2.237153                                                       |
| 4163 | 1.049243              | 2.237195                                                       |
| 4165 | 1.478031              | 2.237237                                                       |
| 4167 | 1.447564              | 2.237278                                                       |
| 4169 | 1.093787              | 2.237320                                                       |
| 4171 | 1.033805              | 2.237362                                                       |
| 4173 | 1.449317              | 2.237404                                                       |
| 4175 | 1.247425              | 2.237446                                                       |
| 4177 | 1.000239              | 2.237487                                                       |
| 4179 | 1.531467              | 2.237529                                                       |
| 4181 | 1.036116              | 2.237571                                                       |
| 4183 | 1.032752              | 2.237612                                                       |
| 4185 | 1.835125              | 2.237654                                                       |
| 4187 | 1.031765              | 2.237695                                                       |
| 4189 | 1.031272              | 2.237737                                                       |
| 4191 | 1.465999              | 2.237779                                                       |
| 4193 | 1.144765              | 2.237820                                                       |
| 4195 | 1.201430              | 2.237862                                                       |
| 4197 | 1.334286              | 2.237903                                                       |
| 4199 | 1.200286              | 2.237945                                                       |
| 4201 | 1.000238              | 2.237986                                                       |
| 4203 | 1.447537              | 2.238027                                                       |
| 4205 | 1.242806              | 2.238069                                                       |
| 4207 | 1.144759              | 2.238110                                                       |
| 4209 | 1.414113              | 2.238152                                                       |
| 4211 | 1.000237              | 2.238193                                                       |
| 4213 | 1.093757              | 2.238234                                                       |
| 4215 | 1.605694              | 2.238276                                                       |
| 4217 | 1.000237              | 2.238317                                                       |
| 4219 | 1.000237              | 2.238358                                                       |
| 4221 | 1.675432              | 2.238399                                                       |
| 4223 | 1.034336              | 2.238440                                                       |
| 4225 | 1.342722              | 2.238482                                                       |
| 4227 | 1.334280              | 2.238523                                                       |
| 4229 | 1.000236              | 2.238564                                                       |
| 4231 | 1.000236              | 2.238605                                                       |
| 4233 | 1.428774              | 2.238646                                                       |
| 4235 | 1.507438              | 2.238687                                                       |
| 4237 | 1.057352              | 2.238728                                                       |

| $n$  | $\frac{\sigma(n)}{n}$ | $\frac{e^\gamma}{2} \log \log n + \frac{0.73...}{\log \log n}$ |
|------|-----------------------|----------------------------------------------------------------|
| 4239 | 1.490918              | 2.238769                                                       |
| 4241 | 1.000236              | 2.238810                                                       |
| 4243 | 1.000236              | 2.238851                                                       |
| 4245 | 1.605654              | 2.238892                                                       |
| 4247 | 1.039793              | 2.238933                                                       |
| 4249 | 1.144740              | 2.238974                                                       |
| 4251 | 1.449071              | 2.239015                                                       |
| 4253 | 1.000235              | 2.239056                                                       |
| 4255 | 1.286016              | 2.239097                                                       |
| 4257 | 1.612403              | 2.239138                                                       |
| 4259 | 1.000235              | 2.239179                                                       |
| 4261 | 1.000235              | 2.239219                                                       |
| 4263 | 1.604504              | 2.239260                                                       |
| 4265 | 1.201407              | 2.239301                                                       |
| 4267 | 1.063042              | 2.239342                                                       |
| 4269 | 1.334270              | 2.239382                                                       |
| 4271 | 1.000234              | 2.239423                                                       |
| 4273 | 1.000234              | 2.239464                                                       |
| 4275 | 1.885380              | 2.239504                                                       |
| 4277 | 1.256956              | 2.239545                                                       |
| 4279 | 1.093713              | 2.239586                                                       |
| 4281 | 1.334268              | 2.239626                                                       |
| 4283 | 1.000233              | 2.239667                                                       |
| 4285 | 1.201400              | 2.239707                                                       |
| 4287 | 1.334266              | 2.239748                                                       |
| 4289 | 1.000233              | 2.239789                                                       |
| 4291 | 1.144722              | 2.239829                                                       |
| 4293 | 1.522013              | 2.239870                                                       |
| 4295 | 1.201397              | 2.239910                                                       |
| 4297 | 1.000233              | 2.239950                                                       |
| 4299 | 1.334264              | 2.239991                                                       |
| 4301 | 1.205301              | 2.240031                                                       |
| 4303 | 1.080177              | 2.240072                                                       |
| 4305 | 1.873171              | 2.240112                                                       |
| 4307 | 1.030880              | 2.240152                                                       |
| 4309 | 1.039684              | 2.240193                                                       |
| 4311 | 1.447460              | 2.240233                                                       |
| 4313 | 1.057269              | 2.240273                                                       |
| 4315 | 1.201390              | 2.240313                                                       |
| 4317 | 1.334260              | 2.240354                                                       |
| 4319 | 1.144709              | 2.240394                                                       |
| 4321 | 1.041426              | 2.240434                                                       |
| 4323 | 1.465649              | 2.240474                                                       |
| 4325 | 1.247168              | 2.240514                                                       |

| $n$  | $\frac{\sigma(n)}{n}$ | $\frac{e^\gamma}{2} \log \log n + \frac{0.73...}{\log \log n}$ |
|------|-----------------------|----------------------------------------------------------------|
| 4327 | 1.000231              | 2.240554                                                       |
| 4329 | 1.597598              | 2.240595                                                       |
| 4331 | 1.030709              | 2.240635                                                       |
| 4333 | 1.144703              | 2.240675                                                       |
| 4335 | 1.699654              | 2.240715                                                       |
| 4337 | 1.000231              | 2.240755                                                       |
| 4339 | 1.000230              | 2.240795                                                       |
| 4341 | 1.334255              | 2.240835                                                       |
| 4343 | 1.033387              | 2.240875                                                       |
| 4345 | 1.325662              | 2.240915                                                       |
| 4347 | 1.766736              | 2.240955                                                       |
| 4349 | 1.000230              | 2.240994                                                       |
| 4351 | 1.057228              | 2.241034                                                       |
| 4353 | 1.334252              | 2.241074                                                       |
| 4355 | 1.311596              | 2.241114                                                       |
| 4357 | 1.000230              | 2.241154                                                       |
| 4359 | 1.334251              | 2.241194                                                       |
| 4361 | 1.176336              | 2.241234                                                       |
| 4363 | 1.000229              | 2.241273                                                       |
| 4365 | 1.751203              | 2.241313                                                       |
| 4367 | 1.093657              | 2.241353                                                       |
| 4369 | 1.062943              | 2.241392                                                       |
| 4371 | 1.405628              | 2.241432                                                       |
| 4373 | 1.000229              | 2.241472                                                       |
| 4375 | 1.428114              | 2.241511                                                       |
| 4377 | 1.334247              | 2.241551                                                       |
| 4379 | 1.041334              | 2.241591                                                       |
| 4381 | 1.080119              | 2.241630                                                       |
| 4383 | 1.447410              | 2.241670                                                       |
| 4385 | 1.201368              | 2.241709                                                       |
| 4387 | 1.033964              | 2.241749                                                       |
| 4389 | 1.749829              | 2.241788                                                       |
| 4391 | 1.000228              | 2.241828                                                       |
| 4393 | 1.048941              | 2.241867                                                       |
| 4395 | 1.605461              | 2.241907                                                       |
| 4397 | 1.000227              | 2.241946                                                       |
| 4399 | 1.031143              | 2.241986                                                       |
| 4401 | 1.490570              | 2.242025                                                       |
| 4403 | 1.242789              | 2.242064                                                       |
| 4405 | 1.201362              | 2.242104                                                       |
| 4407 | 1.448604              | 2.242143                                                       |
| 4409 | 1.000227              | 2.242182                                                       |
| 4411 | 1.093630              | 2.242222                                                       |
| 4413 | 1.334240              | 2.242261                                                       |



| $n$  | $\frac{\sigma(n)}{n}$ | $\frac{e^\gamma}{2} \log \log n + \frac{0.73...}{\log \log n}$ |
|------|-----------------------|----------------------------------------------------------------|
| 4415 | 1.201359              | 2.242300                                                       |
| 4417 | 1.144668              | 2.242339                                                       |
| 4419 | 1.447386              | 2.242379                                                       |
| 4421 | 1.000226              | 2.242418                                                       |
| 4423 | 1.000226              | 2.242457                                                       |
| 4425 | 1.681356              | 2.242496                                                       |
| 4427 | 1.057149              | 2.242535                                                       |
| 4429 | 1.033190              | 2.242574                                                       |
| 4431 | 1.531031              | 2.242614                                                       |
| 4433 | 1.212723              | 2.242653                                                       |
| 4435 | 1.201353              | 2.242692                                                       |
| 4437 | 1.582150              | 2.242731                                                       |
| 4439 | 1.048885              | 2.242770                                                       |
| 4441 | 1.000225              | 2.242809                                                       |
| 4443 | 1.334234              | 2.242848                                                       |
| 4445 | 1.382227              | 2.242887                                                       |
| 4447 | 1.000225              | 2.242926                                                       |
| 4449 | 1.334232              | 2.242965                                                       |
| 4451 | 1.000225              | 2.243003                                                       |
| 4453 | 1.030317              | 2.243042                                                       |
| 4455 | 1.955556              | 2.243081                                                       |
| 4457 | 1.000224              | 2.243120                                                       |
| 4459 | 1.255887              | 2.243159                                                       |
| 4461 | 1.334230              | 2.243198                                                       |
| 4463 | 1.000224              | 2.243236                                                       |
| 4465 | 1.290034              | 2.243275                                                       |
| 4467 | 1.334229              | 2.243314                                                       |
| 4469 | 1.033788              | 2.243353                                                       |
| 4471 | 1.062849              | 2.243391                                                       |
| 4473 | 1.674044              | 2.243430                                                       |
| 4475 | 1.246927              | 2.243469                                                       |
| 4477 | 1.128881              | 2.243507                                                       |
| 4479 | 1.334226              | 2.243546                                                       |
| 4481 | 1.000223              | 2.243585                                                       |
| 4483 | 1.000223              | 2.243623                                                       |
| 4485 | 1.797993              | 2.243662                                                       |
| 4487 | 1.144640              | 2.243700                                                       |
| 4489 | 1.015148              | 2.243739                                                       |
| 4491 | 1.447339              | 2.243778                                                       |
| 4493 | 1.000223              | 2.243816                                                       |
| 4495 | 1.281424              | 2.243855                                                       |
| 4497 | 1.334223              | 2.243893                                                       |
| 4499 | 1.093576              | 2.243931                                                       |
| 4501 | 1.144635              | 2.243970                                                       |

| $n$  | $\frac{\sigma(n)}{n}$ | $\frac{e^\gamma}{2} \log \log n + \frac{0.73\dots}{\log \log n}$ |
|------|-----------------------|------------------------------------------------------------------|
| 4503 | 1.421275              | 2.244008                                                         |
| 4505 | 1.294562              | 2.244047                                                         |
| 4507 | 1.000222              | 2.244085                                                         |
| 4509 | 1.490353              | 2.244123                                                         |
| 4511 | 1.080027              | 2.244162                                                         |
| 4513 | 1.000222              | 2.244200                                                         |
| 4515 | 1.871096              | 2.244238                                                         |
| 4517 | 1.000221              | 2.244277                                                         |
| 4519 | 1.000221              | 2.244315                                                         |
| 4521 | 1.465163              | 2.244353                                                         |
| 4523 | 1.000221              | 2.244391                                                         |
| 4525 | 1.246851              | 2.244430                                                         |
| 4527 | 1.447316              | 2.244468                                                         |
| 4529 | 1.144624              | 2.244506                                                         |
| 4531 | 1.048775              | 2.244544                                                         |
| 4533 | 1.334216              | 2.244582                                                         |
| 4535 | 1.201323              | 2.244620                                                         |
| 4537 | 1.080009              | 2.244659                                                         |
| 4539 | 1.427627              | 2.244697                                                         |
| 4541 | 1.057036              | 2.244735                                                         |
| 4543 | 1.267885              | 2.244773                                                         |
| 4545 | 1.750495              | 2.244811                                                         |
| 4547 | 1.000220              | 2.244849                                                         |
| 4549 | 1.000220              | 2.244887                                                         |
| 4551 | 1.402769              | 2.244925                                                         |
| 4553 | 1.041072              | 2.244963                                                         |
| 4555 | 1.201317              | 2.245001                                                         |
| 4557 | 1.601053              | 2.245038                                                         |
| 4559 | 1.031805              | 2.245076                                                         |
| 4561 | 1.000219              | 2.245114                                                         |
| 4563 | 1.604208              | 2.245152                                                         |
| 4565 | 1.324863              | 2.245190                                                         |
| 4567 | 1.000219              | 2.245228                                                         |
| 4569 | 1.334209              | 2.245266                                                         |
| 4571 | 1.144607              | 2.245303                                                         |
| 4573 | 1.062760              | 2.245341                                                         |
| 4575 | 1.680437              | 2.245379                                                         |
| 4577 | 1.048722              | 2.245417                                                         |
| 4579 | 1.056999              | 2.245454                                                         |
| 4581 | 1.447282              | 2.245492                                                         |
| 4583 | 1.000218              | 2.245530                                                         |
| 4585 | 1.381897              | 2.245567                                                         |
| 4587 | 1.465010              | 2.245605                                                         |
| 4589 | 1.079974              | 2.245643                                                         |

| $n$  | $\frac{\sigma(n)}{n}$ | $\frac{e^\gamma}{2} \log \log n + \frac{0.73...}{\log \log n}$ |
|------|-----------------------|----------------------------------------------------------------|
| 4591 | 1.000218              | 2.245680                                                       |
| 4593 | 1.334204              | 2.245718                                                       |
| 4595 | 1.201306              | 2.245755                                                       |
| 4597 | 1.000218              | 2.245793                                                       |
| 4599 | 1.673407              | 2.245831                                                       |
| 4601 | 1.032819              | 2.245868                                                       |
| 4603 | 1.000217              | 2.245906                                                       |
| 4605 | 1.605212              | 2.245943                                                       |
| 4607 | 1.062731              | 2.245981                                                       |
| 4609 | 1.093513              | 2.246018                                                       |
| 4611 | 1.405335              | 2.246055                                                       |
| 4613 | 1.144591              | 2.246093                                                       |
| 4615 | 1.310509              | 2.246130                                                       |
| 4617 | 1.576781              | 2.246168                                                       |
| 4619 | 1.039186              | 2.246205                                                       |
| 4621 | 1.000216              | 2.246242                                                       |
| 4623 | 1.412070              | 2.246280                                                       |
| 4625 | 1.281730              | 2.246317                                                       |
| 4627 | 1.144586              | 2.246354                                                       |
| 4629 | 1.334197              | 2.246391                                                       |
| 4631 | 1.093500              | 2.246429                                                       |
| 4633 | 1.033456              | 2.246466                                                       |
| 4635 | 1.750162              | 2.246503                                                       |
| 4637 | 1.000216              | 2.246540                                                       |
| 4639 | 1.000216              | 2.246578                                                       |
| 4641 | 1.737557              | 2.246615                                                       |
| 4643 | 1.000215              | 2.246652                                                       |
| 4645 | 1.201292              | 2.246689                                                       |
| 4647 | 1.334194              | 2.246726                                                       |
| 4649 | 1.000215              | 2.246763                                                       |
| 4651 | 1.000215              | 2.246800                                                       |
| 4653 | 1.609284              | 2.246837                                                       |
| 4655 | 1.469388              | 2.246874                                                       |
| 4657 | 1.000215              | 2.246911                                                       |
| 4659 | 1.334192              | 2.246948                                                       |
| 4661 | 1.029822              | 2.246985                                                       |
| 4663 | 1.000214              | 2.247022                                                       |
| 4665 | 1.605145              | 2.247059                                                       |
| 4667 | 1.079923              | 2.247096                                                       |
| 4669 | 1.233669              | 2.247133                                                       |
| 4671 | 1.490045              | 2.247170                                                       |
| 4673 | 1.000214              | 2.247207                                                       |
| 4675 | 1.432299              | 2.247244                                                       |
| 4677 | 1.334189              | 2.247281                                                       |

| $n$  | $\frac{\sigma(n)}{n}$ | $\frac{e^\gamma}{2} \log \log n + \frac{0.73...}{\log \log n}$ |
|------|-----------------------|----------------------------------------------------------------|
| 4679 | 1.000214              | 2.247318                                                       |
| 4681 | 1.039094              | 2.247354                                                       |
| 4683 | 1.530643              | 2.247391                                                       |
| 4685 | 1.201281              | 2.247428                                                       |
| 4687 | 1.032643              | 2.247465                                                       |
| 4689 | 1.447217              | 2.247501                                                       |
| 4691 | 1.000213              | 2.247538                                                       |
| 4693 | 1.136586              | 2.247575                                                       |
| 4695 | 1.605112              | 2.247612                                                       |
| 4697 | 1.267192              | 2.247648                                                       |
| 4699 | 1.035114              | 2.247685                                                       |
| 4701 | 1.334184              | 2.247722                                                       |
| 4703 | 1.000213              | 2.247758                                                       |
| 4705 | 1.201275              | 2.247795                                                       |
| 4707 | 1.447206              | 2.247831                                                       |
| 4709 | 1.062646              | 2.247868                                                       |
| 4711 | 1.144555              | 2.247905                                                       |
| 4713 | 1.334182              | 2.247941                                                       |
| 4715 | 1.282715              | 2.247978                                                       |
| 4717 | 1.030316              | 2.248014                                                       |
| 4719 | 1.578300              | 2.248051                                                       |
| 4721 | 1.000212              | 2.248087                                                       |
| 4723 | 1.000212              | 2.248124                                                       |
| 4725 | 2.099471              | 2.248160                                                       |
| 4727 | 1.040829              | 2.248197                                                       |
| 4729 | 1.000211              | 2.248233                                                       |
| 4731 | 1.420419              | 2.248269                                                       |
| 4733 | 1.000211              | 2.248306                                                       |
| 4735 | 1.201267              | 2.248342                                                       |
| 4737 | 1.334178              | 2.248378                                                       |
| 4739 | 1.144545              | 2.248415                                                       |
| 4741 | 1.093440              | 2.248451                                                       |
| 4743 | 1.578748              | 2.248487                                                       |
| 4745 | 1.310011              | 2.248524                                                       |
| 4747 | 1.031388              | 2.248560                                                       |
| 4749 | 1.334176              | 2.248596                                                       |
| 4751 | 1.000210              | 2.248632                                                       |
| 4753 | 1.175258              | 2.248669                                                       |
| 4755 | 1.605047              | 2.248705                                                       |
| 4757 | 1.029220              | 2.248741                                                       |
| 4759 | 1.000210              | 2.248777                                                       |
| 4761 | 1.509977              | 2.248813                                                       |
| 4763 | 1.093429              | 2.248849                                                       |
| 4765 | 1.201259              | 2.248885                                                       |

| $n$  | $\frac{\sigma(n)}{n}$ | $\frac{e^\gamma}{2} \log \log n + \frac{0.73...}{\log \log n}$ |
|------|-----------------------|----------------------------------------------------------------|
| 4767 | 1.530522              | 2.248922                                                       |
| 4769 | 1.056825              | 2.248958                                                       |
| 4771 | 1.079857              | 2.248994                                                       |
| 4773 | 1.401215              | 2.249030                                                       |
| 4775 | 1.246492              | 2.249066                                                       |
| 4777 | 1.062592              | 2.249102                                                       |
| 4779 | 1.519146              | 2.249138                                                       |
| 4781 | 1.144530              | 2.249174                                                       |
| 4783 | 1.000209              | 2.249210                                                       |
| 4785 | 1.805643              | 2.249246                                                       |
| 4787 | 1.000209              | 2.249282                                                       |
| 4789 | 1.000209              | 2.249317                                                       |
| 4791 | 1.334168              | 2.249353                                                       |
| 4793 | 1.000209              | 2.249389                                                       |
| 4795 | 1.381439              | 2.249425                                                       |
| 4797 | 1.593496              | 2.249461                                                       |
| 4799 | 1.000208              | 2.249497                                                       |
| 4801 | 1.000208              | 2.249533                                                       |
| 4803 | 1.334166              | 2.249568                                                       |
| 4805 | 1.239958              | 2.249604                                                       |
| 4807 | 1.198253              | 2.249640                                                       |
| 4809 | 1.530464              | 2.249676                                                       |
| 4811 | 1.062565              | 2.249711                                                       |
| 4813 | 1.000208              | 2.249747                                                       |
| 4815 | 1.749533              | 2.249783                                                       |
| 4817 | 1.000208              | 2.249819                                                       |
| 4819 | 1.029259              | 2.249854                                                       |
| 4821 | 1.334163              | 2.249890                                                       |
| 4823 | 1.253991              | 2.249925                                                       |
| 4825 | 1.246425              | 2.249961                                                       |
| 4827 | 1.334162              | 2.249997                                                       |
| 4829 | 1.093394              | 2.250032                                                       |
| 4831 | 1.000207              | 2.250068                                                       |
| 4833 | 1.489758              | 2.250103                                                       |
| 4835 | 1.201241              | 2.250139                                                       |
| 4837 | 1.144511              | 2.250174                                                       |
| 4839 | 1.334160              | 2.250210                                                       |
| 4841 | 1.031192              | 2.250245                                                       |
| 4843 | 1.040677              | 2.250281                                                       |
| 4845 | 1.783282              | 2.250316                                                       |
| 4847 | 1.034867              | 2.250352                                                       |
| 4849 | 1.079810              | 2.250387                                                       |
| 4851 | 1.833024              | 2.250423                                                       |
| 4853 | 1.048424              | 2.250458                                                       |

| $n$  | $\frac{\sigma(n)}{n}$ | $\frac{e^\gamma}{2} \log \log n + \frac{0.73...}{\log \log n}$ |
|------|-----------------------|----------------------------------------------------------------|
| 4855 | 1.201236              | 2.250493                                                       |
| 4857 | 1.334157              | 2.250529                                                       |
| 4859 | 1.032311              | 2.250564                                                       |
| 4861 | 1.000206              | 2.250599                                                       |
| 4863 | 1.334156              | 2.250635                                                       |
| 4865 | 1.381295              | 2.250670                                                       |
| 4867 | 1.038833              | 2.250705                                                       |
| 4869 | 1.447114              | 2.250741                                                       |
| 4871 | 1.000205              | 2.250776                                                       |
| 4873 | 1.093372              | 2.250811                                                       |
| 4875 | 1.792000              | 2.250846                                                       |
| 4877 | 1.000205              | 2.250882                                                       |
| 4879 | 1.239598              | 2.250917                                                       |
| 4881 | 1.334153              | 2.250952                                                       |
| 4883 | 1.056727              | 2.250987                                                       |
| 4885 | 1.201228              | 2.251022                                                       |
| 4887 | 1.489666              | 2.251057                                                       |
| 4889 | 1.000205              | 2.251092                                                       |
| 4891 | 1.028828              | 2.251128                                                       |
| 4893 | 1.530349              | 2.251163                                                       |
| 4895 | 1.323800              | 2.251198                                                       |
| 4897 | 1.029202              | 2.251233                                                       |
| 4899 | 1.410900              | 2.251268                                                       |
| 4901 | 1.120180              | 2.251303                                                       |
| 4903 | 1.000204              | 2.251338                                                       |
| 4905 | 1.749235              | 2.251373                                                       |
| 4907 | 1.144487              | 2.251408                                                       |
| 4909 | 1.000204              | 2.251443                                                       |
| 4911 | 1.334148              | 2.251478                                                       |
| 4913 | 1.062487              | 2.251513                                                       |
| 4915 | 1.201221              | 2.251547                                                       |
| 4917 | 1.464308              | 2.251582                                                       |
| 4919 | 1.000203              | 2.251617                                                       |
| 4921 | 1.235521              | 2.251652                                                       |
| 4923 | 1.447085              | 2.251687                                                       |
| 4925 | 1.246294              | 2.251722                                                       |
| 4927 | 1.079765              | 2.251757                                                       |
| 4929 | 1.402313              | 2.251791                                                       |
| 4931 | 1.000203              | 2.251826                                                       |
| 4933 | 1.000203              | 2.251861                                                       |
| 4935 | 1.867477              | 2.251896                                                       |
| 4937 | 1.000203              | 2.251930                                                       |
| 4939 | 1.093339              | 2.251965                                                       |
| 4941 | 1.518316              | 2.252000                                                       |

| $n$  | $\frac{\sigma(n)}{n}$ | $\frac{e^\gamma}{2} \log \log n + \frac{0.73\dots}{\log \log n}$ |
|------|-----------------------|------------------------------------------------------------------|
| 4943 | 1.000202              | 2.252034                                                         |
| 4945 | 1.281294              | 2.252069                                                         |
| 4947 | 1.426319              | 2.252104                                                         |
| 4949 | 1.174783              | 2.252138                                                         |
| 4951 | 1.000202              | 2.252173                                                         |
| 4953 | 1.447204              | 2.252208                                                         |
| 4955 | 1.201211              | 2.252242                                                         |
| 4957 | 1.000202              | 2.252277                                                         |
| 4959 | 1.572898              | 2.252311                                                         |
| 4961 | 1.125983              | 2.252346                                                         |
| 4963 | 1.144469              | 2.252381                                                         |
| 4965 | 1.604834              | 2.252415                                                         |
| 4967 | 1.000201              | 2.252450                                                         |
| 4969 | 1.000201              | 2.252484                                                         |
| 4971 | 1.334138              | 2.252519                                                         |
| 4973 | 1.000201              | 2.252553                                                         |
| 4975 | 1.246231              | 2.252587                                                         |
| 4977 | 1.671690              | 2.252622                                                         |
| 4979 | 1.079735              | 2.252656                                                         |
| 4981 | 1.062437              | 2.252691                                                         |
| 4983 | 1.464178              | 2.252725                                                         |
| 4985 | 1.201204              | 2.252759                                                         |
| 4987 | 1.000201              | 2.252794                                                         |
| 4989 | 1.334135              | 2.252828                                                         |
| 4991 | 1.231016              | 2.252862                                                         |
| 4993 | 1.000200              | 2.252897                                                         |
| 4995 | 1.825826              | 2.252931                                                         |
| 4997 | 1.056634              | 2.252965                                                         |
| 4999 | 1.000200              | 2.253000                                                         |
| 5001 | 1.334133              | 2.253034                                                         |
| 5003 | 1.000200              | 2.253068                                                         |
| 5005 | 1.611189              | 2.253102                                                         |
| 5007 | 1.334132              | 2.253137                                                         |
| 5009 | 1.000200              | 2.253171                                                         |
| 5011 | 1.000200              | 2.253205                                                         |
| 5013 | 1.447038              | 2.253239                                                         |
| 5015 | 1.292124              | 2.253273                                                         |
| 5017 | 1.040462              | 2.253307                                                         |
| 5019 | 1.530185              | 2.253341                                                         |
| 5021 | 1.000199              | 2.253376                                                         |
| 5023 | 1.000199              | 2.253410                                                         |
| 5025 | 1.678010              | 2.253444                                                         |
| 5027 | 1.093296              | 2.253478                                                         |
| 5029 | 1.030821              | 2.253512                                                         |

| $n$  | $\frac{\sigma(n)}{n}$ | $\frac{e^\gamma}{2} \log \log n + \frac{0.73...}{\log \log n}$ |
|------|-----------------------|----------------------------------------------------------------|
| 5031 | 1.591731              | 2.253546                                                       |
| 5033 | 1.144447              | 2.253580                                                       |
| 5035 | 1.286991              | 2.253614                                                       |
| 5037 | 1.410363              | 2.253648                                                       |
| 5039 | 1.000198              | 2.253682                                                       |
| 5041 | 1.014283              | 2.253716                                                       |
| 5043 | 1.366647              | 2.253750                                                       |
| 5045 | 1.201189              | 2.253784                                                       |
| 5047 | 1.174559              | 2.253818                                                       |
| 5049 | 1.711230              | 2.253851                                                       |
| 5051 | 1.000198              | 2.253885                                                       |
| 5053 | 1.038591              | 2.253919                                                       |
| 5055 | 1.604748              | 2.253953                                                       |
| 5057 | 1.079692              | 2.253987                                                       |
| 5059 | 1.000198              | 2.254021                                                       |
| 5061 | 1.530132              | 2.254054                                                       |
| 5063 | 1.028639              | 2.254088                                                       |
| 5065 | 1.201185              | 2.254122                                                       |
| 5067 | 1.447010              | 2.254156                                                       |
| 5069 | 1.034524              | 2.254190                                                       |
| 5071 | 1.093275              | 2.254223                                                       |
| 5073 | 1.419279              | 2.254257                                                       |
| 5075 | 1.466010              | 2.254291                                                       |
| 5077 | 1.000197              | 2.254324                                                       |
| 5079 | 1.334121              | 2.254358                                                       |
| 5081 | 1.000197              | 2.254392                                                       |
| 5083 | 1.189849              | 2.254425                                                       |
| 5085 | 1.748673              | 2.254459                                                       |
| 5087 | 1.000197              | 2.254493                                                       |
| 5089 | 1.144429              | 2.254526                                                       |
| 5091 | 1.334119              | 2.254560                                                       |
| 5093 | 1.093265              | 2.254593                                                       |
| 5095 | 1.201178              | 2.254627                                                       |
| 5097 | 1.334118              | 2.254660                                                       |
| 5099 | 1.000196              | 2.254694                                                       |
| 5101 | 1.000196              | 2.254728                                                       |
| 5103 | 1.713502              | 2.254761                                                       |
| 5105 | 1.201175              | 2.254795                                                       |
| 5107 | 1.000196              | 2.254828                                                       |
| 5109 | 1.446858              | 2.254861                                                       |
| 5111 | 1.056545              | 2.254895                                                       |
| 5113 | 1.000196              | 2.254928                                                       |
| 5115 | 1.801760              | 2.254962                                                       |
| 5117 | 1.238226              | 2.254995                                                       |



| $n$  | $\frac{\sigma(n)}{n}$ | $\frac{e^\gamma}{2} \log \log n + \frac{0.73...}{\log \log n}$ |
|------|-----------------------|----------------------------------------------------------------|
| 5119 | 1.000195              | 2.255029                                                       |
| 5121 | 1.446983              | 2.255062                                                       |
| 5123 | 1.030646              | 2.255095                                                       |
| 5125 | 1.278439              | 2.255129                                                       |
| 5127 | 1.334114              | 2.255162                                                       |
| 5129 | 1.048158              | 2.255195                                                       |
| 5131 | 1.144416              | 2.255229                                                       |
| 5133 | 1.402688              | 2.255262                                                       |
| 5135 | 1.308666              | 2.255295                                                       |
| 5137 | 1.093245              | 2.255328                                                       |
| 5139 | 1.446974              | 2.255362                                                       |
| 5141 | 1.029372              | 2.255395                                                       |
| 5143 | 1.034416              | 2.255428                                                       |
| 5145 | 1.865889              | 2.255461                                                       |
| 5147 | 1.000194              | 2.255494                                                       |
| 5149 | 1.056516              | 2.255528                                                       |
| 5151 | 1.425743              | 2.255561                                                       |
| 5153 | 1.000194              | 2.255594                                                       |
| 5155 | 1.201164              | 2.255627                                                       |
| 5157 | 1.489238              | 2.255660                                                       |
| 5159 | 1.265362              | 2.255693                                                       |
| 5161 | 1.079636              | 2.255726                                                       |
| 5163 | 1.334108              | 2.255759                                                       |
| 5165 | 1.201162              | 2.255793                                                       |
| 5167 | 1.000194              | 2.255826                                                       |
| 5169 | 1.334107              | 2.255859                                                       |
| 5171 | 1.000193              | 2.255892                                                       |
| 5173 | 1.144404              | 2.255925                                                       |
| 5175 | 1.868986              | 2.255958                                                       |
| 5177 | 1.038439              | 2.255991                                                       |
| 5179 | 1.000193              | 2.256024                                                       |
| 5181 | 1.463810              | 2.256057                                                       |
| 5183 | 1.027976              | 2.256089                                                       |
| 5185 | 1.291418              | 2.256122                                                       |
| 5187 | 1.727395              | 2.256155                                                       |
| 5189 | 1.000193              | 2.256188                                                       |
| 5191 | 1.040262              | 2.256221                                                       |
| 5193 | 1.446948              | 2.256254                                                       |
| 5195 | 1.201155              | 2.256287                                                       |
| 5197 | 1.000192              | 2.256320                                                       |
| 5199 | 1.334103              | 2.256352                                                       |
| 5201 | 1.144395              | 2.256385                                                       |
| 5203 | 1.124736              | 2.256418                                                       |
| 5205 | 1.604611              | 2.256451                                                       |

| $n$  | $\frac{\sigma(n)}{n}$ | $\frac{e^\gamma}{2} \log \log n + \frac{0.73\dots}{\log \log n}$ |
|------|-----------------------|------------------------------------------------------------------|
| 5207 | 1.032456              | 2.256484                                                         |
| 5209 | 1.000192              | 2.256516                                                         |
| 5211 | 1.489158              | 2.256549                                                         |
| 5213 | 1.079609              | 2.256582                                                         |
| 5215 | 1.380633              | 2.256615                                                         |
| 5217 | 1.398505              | 2.256647                                                         |
| 5219 | 1.062272              | 2.256680                                                         |
| 5221 | 1.048075              | 2.256713                                                         |
| 5223 | 1.334099              | 2.256745                                                         |
| 5225 | 1.423923              | 2.256778                                                         |
| 5227 | 1.000191              | 2.256811                                                         |
| 5229 | 1.670683              | 2.256843                                                         |
| 5231 | 1.000191              | 2.256876                                                         |
| 5233 | 1.000191              | 2.256908                                                         |
| 5235 | 1.604585              | 2.256941                                                         |
| 5237 | 1.000191              | 2.256974                                                         |
| 5239 | 1.117771              | 2.257006                                                         |
| 5241 | 1.334097              | 2.257039                                                         |
| 5243 | 1.174137              | 2.257071                                                         |
| 5245 | 1.201144              | 2.257104                                                         |
| 5247 | 1.605489              | 2.257136                                                         |
| 5249 | 1.040198              | 2.257169                                                         |
| 5251 | 1.028376              | 2.257201                                                         |
| 5253 | 1.425471              | 2.257234                                                         |
| 5255 | 1.201142              | 2.257266                                                         |
| 5257 | 1.144379              | 2.257298                                                         |
| 5259 | 1.334094              | 2.257331                                                         |
| 5261 | 1.000190              | 2.257363                                                         |
| 5263 | 1.056432              | 2.257396                                                         |
| 5265 | 1.930484              | 2.257428                                                         |
| 5267 | 1.048035              | 2.257460                                                         |
| 5269 | 1.093187              | 2.257493                                                         |
| 5271 | 1.529880              | 2.257525                                                         |
| 5273 | 1.000190              | 2.257557                                                         |
| 5275 | 1.245877              | 2.257590                                                         |
| 5277 | 1.334091              | 2.257622                                                         |
| 5279 | 1.000189              | 2.257654                                                         |
| 5281 | 1.000189              | 2.257687                                                         |
| 5283 | 1.446905              | 2.257719                                                         |
| 5285 | 1.380511              | 2.257751                                                         |
| 5287 | 1.062228              | 2.257783                                                         |
| 5289 | 1.397618              | 2.257816                                                         |
| 5291 | 1.206577              | 2.257848                                                         |
| 5293 | 1.027773              | 2.257880                                                         |

| $n$  | $\frac{\sigma(n)}{n}$ | $\frac{e^\gamma}{2} \log \log n + \frac{0.73...}{\log \log n}$ |
|------|-----------------------|----------------------------------------------------------------|
| 5295 | 1.604533              | 2.257912                                                       |
| 5297 | 1.000189              | 2.257944                                                       |
| 5299 | 1.144367              | 2.257976                                                       |
| 5301 | 1.569515              | 2.258009                                                       |
| 5303 | 1.000189              | 2.258041                                                       |
| 5305 | 1.201131              | 2.258073                                                       |
| 5307 | 1.401922              | 2.258105                                                       |
| 5309 | 1.000188              | 2.258137                                                       |
| 5311 | 1.030314              | 2.258169                                                       |
| 5313 | 1.734613              | 2.258201                                                       |
| 5315 | 1.201129              | 2.258233                                                       |
| 5317 | 1.079556              | 2.258265                                                       |
| 5319 | 1.489002              | 2.258297                                                       |
| 5321 | 1.062206              | 2.258329                                                       |
| 5323 | 1.000188              | 2.258361                                                       |
| 5325 | 1.676620              | 2.258393                                                       |
| 5327 | 1.144359              | 2.258425                                                       |
| 5329 | 1.013886              | 2.258457                                                       |
| 5331 | 1.334084              | 2.258489                                                       |
| 5333 | 1.000188              | 2.258521                                                       |
| 5335 | 1.322587              | 2.258553                                                       |
| 5337 | 1.446880              | 2.258585                                                       |
| 5339 | 1.056378              | 2.258617                                                       |
| 5341 | 1.173937              | 2.258649                                                       |
| 5343 | 1.446378              | 2.258680                                                       |
| 5345 | 1.201123              | 2.258712                                                       |
| 5347 | 1.000187              | 2.258744                                                       |
| 5349 | 1.334081              | 2.258776                                                       |
| 5351 | 1.000187              | 2.258808                                                       |
| 5353 | 1.028956              | 2.258840                                                       |
| 5355 | 2.097479              | 2.258871                                                       |
| 5357 | 1.093149              | 2.258903                                                       |
| 5359 | 1.047957              | 2.258935                                                       |
| 5361 | 1.334079              | 2.258967                                                       |
| 5363 | 1.038225              | 2.258998                                                       |
| 5365 | 1.274930              | 2.259030                                                       |
| 5367 | 1.334079              | 2.259062                                                       |
| 5369 | 1.251630              | 2.259093                                                       |
| 5371 | 1.032210              | 2.259125                                                       |
| 5373 | 1.488926              | 2.259157                                                       |
| 5375 | 1.277023              | 2.259188                                                       |
| 5377 | 1.056351              | 2.259220                                                       |
| 5379 | 1.463469              | 2.259252                                                       |
| 5381 | 1.000186              | 2.259283                                                       |

| $n$  | $\frac{\sigma(n)}{n}$ | $\frac{e^\gamma}{2} \log \log n + \frac{0.73...}{\log \log n}$ |
|------|-----------------------|----------------------------------------------------------------|
| 5383 | 1.144343              | 2.259315                                                       |
| 5385 | 1.604457              | 2.259346                                                       |
| 5387 | 1.000186              | 2.259378                                                       |
| 5389 | 1.062164              | 2.259410                                                       |
| 5391 | 1.446856              | 2.259441                                                       |
| 5393 | 1.000185              | 2.259473                                                       |
| 5395 | 1.307878              | 2.259504                                                       |
| 5397 | 1.529739              | 2.259536                                                       |
| 5399 | 1.000185              | 2.259567                                                       |
| 5401 | 1.093131              | 2.259599                                                       |
| 5403 | 1.334074              | 2.259630                                                       |
| 5405 | 1.278816              | 2.259662                                                       |
| 5407 | 1.000185              | 2.259693                                                       |
| 5409 | 1.446848              | 2.259725                                                       |
| 5411 | 1.144336              | 2.259756                                                       |
| 5413 | 1.000185              | 2.259787                                                       |
| 5415 | 1.688643              | 2.259819                                                       |
| 5417 | 1.000185              | 2.259850                                                       |
| 5419 | 1.000185              | 2.259882                                                       |
| 5421 | 1.446228              | 2.259913                                                       |
| 5423 | 1.194911              | 2.259944                                                       |
| 5425 | 1.462857              | 2.259976                                                       |
| 5427 | 1.516123              | 2.260007                                                       |
| 5429 | 1.027814              | 2.260038                                                       |
| 5431 | 1.000184              | 2.260070                                                       |
| 5433 | 1.334070              | 2.260101                                                       |
| 5435 | 1.201104              | 2.260132                                                       |
| 5437 | 1.000184              | 2.260163                                                       |
| 5439 | 1.592940              | 2.260195                                                       |
| 5441 | 1.000184              | 2.260226                                                       |
| 5443 | 1.000184              | 2.260257                                                       |
| 5445 | 1.905234              | 2.260288                                                       |
| 5447 | 1.079493              | 2.260319                                                       |
| 5449 | 1.000184              | 2.260351                                                       |
| 5451 | 1.408916              | 2.260382                                                       |
| 5453 | 1.232349              | 2.260413                                                       |
| 5455 | 1.201100              | 2.260444                                                       |
| 5457 | 1.424959              | 2.260475                                                       |
| 5459 | 1.028760              | 2.260506                                                       |
| 5461 | 1.031313              | 2.260537                                                       |
| 5463 | 1.446824              | 2.260569                                                       |
| 5465 | 1.201098              | 2.260600                                                       |
| 5467 | 1.264313              | 2.260631                                                       |
| 5469 | 1.334065              | 2.260662                                                       |

| $n$  | $\frac{\sigma(n)}{n}$ | $\frac{e^\gamma}{2} \log \log n + \frac{0.73...}{\log \log n}$ |
|------|-----------------------|----------------------------------------------------------------|
| 5471 | 1.000183              | 2.260693                                                       |
| 5473 | 1.079481              | 2.260724                                                       |
| 5475 | 1.675982              | 2.260755                                                       |
| 5477 | 1.000183              | 2.260786                                                       |
| 5479 | 1.000183              | 2.260817                                                       |
| 5481 | 1.751505              | 2.260848                                                       |
| 5483 | 1.000182              | 2.260879                                                       |
| 5485 | 1.201094              | 2.260910                                                       |
| 5487 | 1.399672              | 2.260941                                                       |
| 5489 | 1.093095              | 2.260972                                                       |
| 5491 | 1.118193              | 2.261003                                                       |
| 5493 | 1.334062              | 2.261034                                                       |
| 5495 | 1.380164              | 2.261064                                                       |
| 5497 | 1.047844              | 2.261095                                                       |
| 5499 | 1.588652              | 2.261126                                                       |
| 5501 | 1.000182              | 2.261157                                                       |
| 5503 | 1.000182              | 2.261188                                                       |
| 5505 | 1.604360              | 2.261219                                                       |
| 5507 | 1.000182              | 2.261250                                                       |
| 5509 | 1.144309              | 2.261280                                                       |
| 5511 | 1.463255              | 2.261311                                                       |
| 5513 | 1.033920              | 2.261342                                                       |
| 5515 | 1.201088              | 2.261373                                                       |
| 5517 | 1.446801              | 2.261404                                                       |
| 5519 | 1.000181              | 2.261434                                                       |
| 5521 | 1.000181              | 2.261465                                                       |
| 5523 | 1.529603              | 2.261496                                                       |
| 5525 | 1.413937              | 2.261526                                                       |
| 5527 | 1.000181              | 2.261557                                                       |
| 5529 | 1.417978              | 2.261588                                                       |
| 5531 | 1.000181              | 2.261619                                                       |
| 5533 | 1.093078              | 2.261649                                                       |
| 5535 | 1.821138              | 2.261680                                                       |
| 5537 | 1.173560              | 2.261710                                                       |
| 5539 | 1.039899              | 2.261741                                                       |
| 5541 | 1.334055              | 2.261772                                                       |
| 5543 | 1.047808              | 2.261802                                                       |
| 5545 | 1.201082              | 2.261833                                                       |
| 5547 | 1.365062              | 2.261864                                                       |
| 5549 | 1.038025              | 2.261894                                                       |
| 5551 | 1.250946              | 2.261925                                                       |
| 5553 | 1.446786              | 2.261955                                                       |
| 5555 | 1.322052              | 2.261986                                                       |
| 5557 | 1.000180              | 2.262016                                                       |

| $n$  | $\frac{\sigma(n)}{n}$ | $\frac{e^\gamma}{2} \log \log n + \frac{0.73\dots}{\log \log n}$ |
|------|-----------------------|------------------------------------------------------------------|
| 5559 | 1.424717              | 2.262047                                                         |
| 5561 | 1.027153              | 2.262077                                                         |
| 5563 | 1.000180              | 2.262108                                                         |
| 5565 | 1.863073              | 2.262138                                                         |
| 5567 | 1.056224              | 2.262169                                                         |
| 5569 | 1.000180              | 2.262199                                                         |
| 5571 | 1.446778              | 2.262230                                                         |
| 5573 | 1.000179              | 2.262260                                                         |
| 5575 | 1.245561              | 2.262290                                                         |
| 5577 | 1.575040              | 2.262321                                                         |
| 5579 | 1.144291              | 2.262351                                                         |
| 5581 | 1.000179              | 2.262382                                                         |
| 5583 | 1.334050              | 2.262412                                                         |
| 5585 | 1.201074              | 2.262442                                                         |
| 5587 | 1.033829              | 2.262473                                                         |
| 5589 | 1.563070              | 2.262503                                                         |
| 5591 | 1.000179              | 2.262533                                                         |
| 5593 | 1.235831              | 2.262564                                                         |
| 5595 | 1.604290              | 2.262594                                                         |
| 5597 | 1.039843              | 2.262624                                                         |
| 5599 | 1.093052              | 2.262654                                                         |
| 5601 | 1.334047              | 2.262685                                                         |
| 5603 | 1.079422              | 2.262715                                                         |
| 5605 | 1.284567              | 2.262745                                                         |
| 5607 | 1.669342              | 2.262775                                                         |
| 5609 | 1.026921              | 2.262806                                                         |
| 5611 | 1.037961              | 2.262836                                                         |
| 5613 | 1.334046              | 2.262866                                                         |
| 5615 | 1.201069              | 2.262896                                                         |
| 5617 | 1.031868              | 2.262926                                                         |
| 5619 | 1.334045              | 2.262957                                                         |
| 5621 | 1.263832              | 2.262987                                                         |
| 5623 | 1.000178              | 2.263017                                                         |
| 5625 | 1.804978              | 2.263047                                                         |
| 5627 | 1.062022              | 2.263077                                                         |
| 5629 | 1.079410              | 2.263107                                                         |
| 5631 | 1.334044              | 2.263137                                                         |
| 5633 | 1.031067              | 2.263167                                                         |
| 5635 | 1.456610              | 2.263197                                                         |
| 5637 | 1.334043              | 2.263227                                                         |
| 5639 | 1.000177              | 2.263257                                                         |
| 5641 | 1.000177              | 2.263287                                                         |
| 5643 | 1.701223              | 2.263317                                                         |
| 5645 | 1.201063              | 2.263347                                                         |

| $n$  | $\frac{\sigma(n)}{n}$ | $\frac{e^\gamma}{2} \log \log n + \frac{0.73...}{\log \log n}$ |
|------|-----------------------|----------------------------------------------------------------|
| 5647 | 1.000177              | 2.263377                                                       |
| 5649 | 1.529474              | 2.263407                                                       |
| 5651 | 1.000177              | 2.263437                                                       |
| 5653 | 1.000177              | 2.263467                                                       |
| 5655 | 1.782493              | 2.263497                                                       |
| 5657 | 1.000177              | 2.263527                                                       |
| 5659 | 1.000177              | 2.263557                                                       |
| 5661 | 1.570747              | 2.263587                                                       |
| 5663 | 1.144270              | 2.263617                                                       |
| 5665 | 1.321801              | 2.263647                                                       |
| 5667 | 1.334039              | 2.263677                                                       |
| 5669 | 1.000176              | 2.263707                                                       |
| 5671 | 1.028390              | 2.263736                                                       |
| 5673 | 1.398907              | 2.263766                                                       |
| 5675 | 1.245463              | 2.263796                                                       |
| 5677 | 1.144266              | 2.263826                                                       |
| 5679 | 1.446734              | 2.263856                                                       |
| 5681 | 1.182890              | 2.263886                                                       |
| 5683 | 1.000176              | 2.263915                                                       |
| 5685 | 1.604222              | 2.263945                                                       |
| 5687 | 1.122560              | 2.263975                                                       |
| 5689 | 1.000176              | 2.264005                                                       |
| 5691 | 1.529432              | 2.264034                                                       |
| 5693 | 1.000176              | 2.264064                                                       |
| 5695 | 1.289552              | 2.264094                                                       |
| 5697 | 1.488503              | 2.264124                                                       |
| 5699 | 1.031760              | 2.264153                                                       |
| 5701 | 1.000175              | 2.264183                                                       |
| 5703 | 1.334035              | 2.264213                                                       |
| 5705 | 1.379842              | 2.264242                                                       |
| 5707 | 1.079376              | 2.264272                                                       |
| 5709 | 1.462953              | 2.264302                                                       |
| 5711 | 1.000175              | 2.264331                                                       |
| 5713 | 1.039734              | 2.264361                                                       |
| 5715 | 1.746982              | 2.264390                                                       |
| 5717 | 1.000175              | 2.264420                                                       |
| 5719 | 1.230984              | 2.264450                                                       |
| 5721 | 1.334033              | 2.264479                                                       |
| 5723 | 1.027433              | 2.264509                                                       |
| 5725 | 1.245415              | 2.264538                                                       |
| 5727 | 1.408067              | 2.264568                                                       |
| 5729 | 1.061965              | 2.264597                                                       |
| 5731 | 1.093003              | 2.264627                                                       |
| 5733 | 1.809524              | 2.264656                                                       |

| $n$  | $\frac{\sigma(n)}{n}$ | $\frac{e^\gamma}{2} \log \log n + \frac{0.73...}{\log \log n}$ |
|------|-----------------------|----------------------------------------------------------------|
| 5735 | 1.272188              | 2.264686                                                       |
| 5737 | 1.000174              | 2.264715                                                       |
| 5739 | 1.334030              | 2.264745                                                       |
| 5741 | 1.000174              | 2.264774                                                       |
| 5743 | 1.000174              | 2.264804                                                       |
| 5745 | 1.604178              | 2.264833                                                       |
| 5747 | 1.144249              | 2.264862                                                       |
| 5749 | 1.000174              | 2.264892                                                       |
| 5751 | 1.514867              | 2.264921                                                       |
| 5753 | 1.092995              | 2.264951                                                       |
| 5755 | 1.201043              | 2.264980                                                       |
| 5757 | 1.417405              | 2.265009                                                       |
| 5759 | 1.079354              | 2.265039                                                       |
| 5761 | 1.144246              | 2.265068                                                       |
| 5763 | 1.424258              | 2.265097                                                       |
| 5765 | 1.201041              | 2.265127                                                       |
| 5767 | 1.026530              | 2.265156                                                       |
| 5769 | 1.446698              | 2.265185                                                       |
| 5771 | 1.039681              | 2.265215                                                       |
| 5773 | 1.047636              | 2.265244                                                       |
| 5775 | 2.061299              | 2.265273                                                       |
| 5777 | 1.028215              | 2.265302                                                       |
| 5779 | 1.000173              | 2.265332                                                       |
| 5781 | 1.394914              | 2.265361                                                       |
| 5783 | 1.000173              | 2.265390                                                       |
| 5785 | 1.306828              | 2.265419                                                       |
| 5787 | 1.446691              | 2.265449                                                       |
| 5789 | 1.144239              | 2.265478                                                       |
| 5791 | 1.000173              | 2.265507                                                       |
| 5793 | 1.334024              | 2.265536                                                       |
| 5795 | 1.283865              | 2.265565                                                       |
| 5797 | 1.192341              | 2.265594                                                       |
| 5799 | 1.334023              | 2.265623                                                       |
| 5801 | 1.000172              | 2.265653                                                       |
| 5803 | 1.144236              | 2.265682                                                       |
| 5805 | 1.819121              | 2.265711                                                       |
| 5807 | 1.000172              | 2.265740                                                       |
| 5809 | 1.033569              | 2.265769                                                       |
| 5811 | 1.445534              | 2.265798                                                       |
| 5813 | 1.000172              | 2.265827                                                       |
| 5815 | 1.201032              | 2.265856                                                       |
| 5817 | 1.529311              | 2.265885                                                       |
| 5819 | 1.140402              | 2.265914                                                       |
| 5821 | 1.000172              | 2.265943                                                       |



| $n$  | $\frac{\sigma(n)}{n}$ | $\frac{e^\gamma}{2} \log \log n + \frac{0.73...}{\log \log n}$ |
|------|-----------------------|----------------------------------------------------------------|
| 5823 | 1.446677              | 2.265972                                                       |
| 5825 | 1.245322              | 2.266001                                                       |
| 5827 | 1.000172              | 2.266030                                                       |
| 5829 | 1.399897              | 2.266059                                                       |
| 5831 | 1.234780              | 2.266088                                                       |
| 5833 | 1.056060              | 2.266117                                                       |
| 5835 | 1.604113              | 2.266146                                                       |
| 5837 | 1.079322              | 2.266175                                                       |
| 5839 | 1.000171              | 2.266204                                                       |
| 5841 | 1.602465              | 2.266233                                                       |
| 5843 | 1.000171              | 2.266262                                                       |
| 5845 | 1.379641              | 2.266291                                                       |
| 5847 | 1.334017              | 2.266319                                                       |
| 5849 | 1.000171              | 2.266348                                                       |
| 5851 | 1.000171              | 2.266377                                                       |
| 5853 | 1.334017              | 2.266406                                                       |
| 5855 | 1.201025              | 2.266435                                                       |
| 5857 | 1.000171              | 2.266464                                                       |
| 5859 | 1.747739              | 2.266492                                                       |
| 5861 | 1.000171              | 2.266521                                                       |
| 5863 | 1.203479              | 2.266550                                                       |
| 5865 | 1.767775              | 2.266579                                                       |
| 5867 | 1.000170              | 2.266608                                                       |
| 5869 | 1.000170              | 2.266636                                                       |
| 5871 | 1.417135              | 2.266665                                                       |
| 5873 | 1.144219              | 2.266694                                                       |
| 5875 | 1.274553              | 2.266723                                                       |
| 5877 | 1.446656              | 2.266751                                                       |
| 5879 | 1.000170              | 2.266780                                                       |
| 5881 | 1.000170              | 2.266809                                                       |
| 5883 | 1.395207              | 2.266837                                                       |
| 5885 | 1.321325              | 2.266866                                                       |
| 5887 | 1.183625              | 2.266895                                                       |
| 5889 | 1.445407              | 2.266923                                                       |
| 5891 | 1.030725              | 2.266952                                                       |
| 5893 | 1.026302              | 2.266981                                                       |
| 5895 | 1.746565              | 2.267009                                                       |
| 5897 | 1.000170              | 2.267038                                                       |
| 5899 | 1.061875              | 2.267066                                                       |
| 5901 | 1.529232              | 2.267095                                                       |
| 5903 | 1.000169              | 2.267123                                                       |
| 5905 | 1.201016              | 2.267152                                                       |
| 5907 | 1.462671              | 2.267181                                                       |
| 5909 | 1.056016              | 2.267209                                                       |

| $n$  | $\frac{\sigma(n)}{n}$ | $\frac{e^\gamma}{2} \log \log n + \frac{0.73...}{\log \log n}$ |
|------|-----------------------|----------------------------------------------------------------|
| 5911 | 1.047538              | 2.267238                                                       |
| 5913 | 1.514291              | 2.267266                                                       |
| 5915 | 1.485038              | 2.267295                                                       |
| 5917 | 1.026872              | 2.267323                                                       |
| 5919 | 1.334009              | 2.267352                                                       |
| 5921 | 1.037663              | 2.267380                                                       |
| 5923 | 1.000169              | 2.267409                                                       |
| 5925 | 1.674262              | 2.267437                                                       |
| 5927 | 1.000169              | 2.267466                                                       |
| 5929 | 1.278630              | 2.267494                                                       |
| 5931 | 1.446636              | 2.267522                                                       |
| 5933 | 1.061857              | 2.267551                                                       |
| 5935 | 1.201011              | 2.267579                                                       |
| 5937 | 1.334007              | 2.267608                                                       |
| 5939 | 1.000168              | 2.267636                                                       |
| 5941 | 1.079280              | 2.267664                                                       |
| 5943 | 1.529194              | 2.267693                                                       |
| 5945 | 1.271657              | 2.267721                                                       |
| 5947 | 1.055995              | 2.267749                                                       |
| 5949 | 1.446630              | 2.267778                                                       |
| 5951 | 1.092926              | 2.267806                                                       |
| 5953 | 1.000168              | 2.267834                                                       |
| 5955 | 1.604030              | 2.267863                                                       |
| 5957 | 1.224778              | 2.267891                                                       |
| 5959 | 1.027018              | 2.267919                                                       |
| 5961 | 1.334004              | 2.267948                                                       |
| 5963 | 1.026329              | 2.267976                                                       |
| 5965 | 1.201006              | 2.268004                                                       |
| 5967 | 1.689291              | 2.268032                                                       |
| 5969 | 1.029318              | 2.268061                                                       |
| 5971 | 1.144197              | 2.268089                                                       |
| 5973 | 1.462582              | 2.268117                                                       |
| 5975 | 1.245188              | 2.268145                                                       |
| 5977 | 1.030617              | 2.268173                                                       |
| 5979 | 1.334002              | 2.268202                                                       |
| 5981 | 1.000167              | 2.268230                                                       |
| 5983 | 1.037607              | 2.268258                                                       |
| 5985 | 2.085213              | 2.268286                                                       |
| 5987 | 1.000167              | 2.268314                                                       |
| 5989 | 1.027884              | 2.268342                                                       |
| 5991 | 1.334001              | 2.268370                                                       |
| 5993 | 1.079259              | 2.268398                                                       |
| 5995 | 1.321101              | 2.268427                                                       |
| 5997 | 1.334000              | 2.268455                                                       |

| $n$  | $\frac{\sigma(n)}{n}$ | $\frac{e^\gamma}{2} \log \log n + \frac{0.73...}{\log \log n}$ |
|------|-----------------------|----------------------------------------------------------------|
| 5999 | 1.144191              | 2.268483                                                       |
| 6001 | 1.061823              | 2.268511                                                       |
| 6003 | 1.559220              | 2.268539                                                       |
| 6005 | 1.200999              | 2.268567                                                       |
| 6007 | 1.000166              | 2.268595                                                       |
| 6009 | 1.333999              | 2.268623                                                       |
| 6011 | 1.000166              | 2.268651                                                       |
| 6013 | 1.144188              | 2.268679                                                       |
| 6015 | 1.603990              | 2.268707                                                       |
| 6017 | 1.092903              | 2.268735                                                       |
| 6019 | 1.079249              | 2.268763                                                       |
| 6021 | 1.488125              | 2.268791                                                       |
| 6023 | 1.055952              | 2.268819                                                       |
| 6025 | 1.245145              | 2.268847                                                       |
| 6027 | 1.588850              | 2.268875                                                       |
| 6029 | 1.000166              | 2.268903                                                       |
| 6031 | 1.033328              | 2.268931                                                       |
| 6033 | 1.333996              | 2.268958                                                       |
| 6035 | 1.288484              | 2.268986                                                       |
| 6037 | 1.000166              | 2.269014                                                       |
| 6039 | 1.601590              | 2.269042                                                       |
| 6041 | 1.144181              | 2.269070                                                       |
| 6043 | 1.000165              | 2.269098                                                       |
| 6045 | 1.778660              | 2.269126                                                       |
| 6047 | 1.000165              | 2.269153                                                       |
| 6049 | 1.047446              | 2.269181                                                       |
| 6051 | 1.333994              | 2.269209                                                       |
| 6053 | 1.000165              | 2.269237                                                       |
| 6055 | 1.379356              | 2.269265                                                       |
| 6057 | 1.446591              | 2.269292                                                       |
| 6059 | 1.025912              | 2.269320                                                       |
| 6061 | 1.187923              | 2.269348                                                       |
| 6063 | 1.393370              | 2.269376                                                       |
| 6065 | 1.200989              | 2.269403                                                       |
| 6067 | 1.000165              | 2.269431                                                       |
| 6069 | 1.618718              | 2.269459                                                       |
| 6071 | 1.079229              | 2.269487                                                       |
| 6073 | 1.000165              | 2.269514                                                       |
| 6075 | 1.857449              | 2.269542                                                       |
| 6077 | 1.026822              | 2.269570                                                       |
| 6079 | 1.000165              | 2.269597                                                       |
| 6081 | 1.333991              | 2.269625                                                       |
| 6083 | 1.262535              | 2.269653                                                       |
| 6085 | 1.200986              | 2.269680                                                       |

| $n$  | $\frac{\sigma(n)}{n}$ | $\frac{e^\gamma}{2} \log \log n + \frac{0.73\dots}{\log \log n}$ |
|------|-----------------------|------------------------------------------------------------------|
| 6087 | 1.333990              | 2.269708                                                         |
| 6089 | 1.000164              | 2.269736                                                         |
| 6091 | 1.000164              | 2.269763                                                         |
| 6093 | 1.446578              | 2.269791                                                         |
| 6095 | 1.275800              | 2.269818                                                         |
| 6097 | 1.249139              | 2.269846                                                         |
| 6099 | 1.416626              | 2.269874                                                         |
| 6101 | 1.000164              | 2.269901                                                         |
| 6103 | 1.061773              | 2.269929                                                         |
| 6105 | 1.792629              | 2.269956                                                         |
| 6107 | 1.037498              | 2.269984                                                         |
| 6109 | 1.031265              | 2.270011                                                         |
| 6111 | 1.667812              | 2.270039                                                         |
| 6113 | 1.000164              | 2.270066                                                         |
| 6115 | 1.200981              | 2.270094                                                         |
| 6117 | 1.333987              | 2.270121                                                         |
| 6119 | 1.039386              | 2.270149                                                         |
| 6121 | 1.000163              | 2.270176                                                         |
| 6123 | 1.445043              | 2.270204                                                         |
| 6125 | 1.451755              | 2.270231                                                         |
| 6127 | 1.092868              | 2.270259                                                         |
| 6129 | 1.488008              | 2.270286                                                         |
| 6131 | 1.000163              | 2.270313                                                         |
| 6133 | 1.000163              | 2.270341                                                         |
| 6135 | 1.603912              | 2.270368                                                         |
| 6137 | 1.117484              | 2.270396                                                         |
| 6139 | 1.144160              | 2.270423                                                         |
| 6141 | 1.406937              | 2.270450                                                         |
| 6143 | 1.000163              | 2.270478                                                         |
| 6145 | 1.200976              | 2.270505                                                         |
| 6147 | 1.446559              | 2.270532                                                         |
| 6149 | 1.202147              | 2.270560                                                         |
| 6151 | 1.000163              | 2.270587                                                         |
| 6153 | 1.529010              | 2.270614                                                         |
| 6155 | 1.200975              | 2.270642                                                         |
| 6157 | 1.029073              | 2.270669                                                         |
| 6159 | 1.333983              | 2.270696                                                         |
| 6161 | 1.026457              | 2.270723                                                         |
| 6163 | 1.000162              | 2.270751                                                         |
| 6165 | 1.745985              | 2.270778                                                         |
| 6167 | 1.144154              | 2.270805                                                         |
| 6169 | 1.037445              | 2.270832                                                         |
| 6171 | 1.551774              | 2.270860                                                         |
| 6173 | 1.000162              | 2.270887                                                         |

| $n$  | $\frac{\sigma(n)}{n}$ | $\frac{e^\gamma}{2} \log \log n + \frac{0.73...}{\log \log n}$ |
|------|-----------------------|----------------------------------------------------------------|
| 6175 | 1.405668              | 2.270914                                                       |
| 6177 | 1.398737              | 2.270941                                                       |
| 6179 | 1.033177              | 2.270968                                                       |
| 6181 | 1.144151              | 2.270996                                                       |
| 6183 | 1.487951              | 2.271023                                                       |
| 6185 | 1.200970              | 2.271050                                                       |
| 6187 | 1.047357              | 2.271077                                                       |
| 6189 | 1.333980              | 2.271104                                                       |
| 6191 | 1.031174              | 2.271131                                                       |
| 6193 | 1.092847              | 2.271158                                                       |
| 6195 | 1.859564              | 2.271186                                                       |
| 6197 | 1.000161              | 2.271213                                                       |
| 6199 | 1.000161              | 2.271240                                                       |
| 6201 | 1.584906              | 2.271267                                                       |
| 6203 | 1.000161              | 2.271294                                                       |
| 6205 | 1.287994              | 2.271321                                                       |
| 6207 | 1.333978              | 2.271348                                                       |
| 6209 | 1.144146              | 2.271375                                                       |
| 6211 | 1.000161              | 2.271402                                                       |
| 6213 | 1.416385              | 2.271429                                                       |
| 6215 | 1.320676              | 2.271456                                                       |
| 6217 | 1.000161              | 2.271483                                                       |
| 6219 | 1.446535              | 2.271510                                                       |
| 6221 | 1.000161              | 2.271537                                                       |
| 6223 | 1.172425              | 2.271564                                                       |
| 6225 | 1.673253              | 2.271591                                                       |
| 6227 | 1.079171              | 2.271618                                                       |
| 6229 | 1.000161              | 2.271645                                                       |
| 6231 | 1.396887              | 2.271672                                                       |
| 6233 | 1.047329              | 2.271699                                                       |
| 6235 | 1.270249              | 2.271726                                                       |
| 6237 | 1.862434              | 2.271753                                                       |
| 6239 | 1.061709              | 2.271779                                                       |
| 6241 | 1.012818              | 2.271806                                                       |
| 6243 | 1.333974              | 2.271833                                                       |
| 6245 | 1.200961              | 2.271860                                                       |
| 6247 | 1.000160              | 2.271887                                                       |
| 6249 | 1.333973              | 2.271914                                                       |
| 6251 | 1.228603              | 2.271941                                                       |
| 6253 | 1.112106              | 2.271967                                                       |
| 6255 | 1.745803              | 2.271994                                                       |
| 6257 | 1.000160              | 2.272021                                                       |
| 6259 | 1.092826              | 2.272048                                                       |
| 6261 | 1.333972              | 2.272075                                                       |

| $n$  | $\frac{\sigma(n)}{n}$ | $\frac{e^\gamma}{2} \log \log n + \frac{0.73...}{\log \log n}$ |
|------|-----------------------|----------------------------------------------------------------|
| 6263 | 1.000160              | 2.272101                                                       |
| 6265 | 1.379090              | 2.272128                                                       |
| 6267 | 1.333972              | 2.272155                                                       |
| 6269 | 1.000160              | 2.272182                                                       |
| 6271 | 1.000159              | 2.272209                                                       |
| 6273 | 1.566714              | 2.272235                                                       |
| 6275 | 1.244940              | 2.272262                                                       |
| 6277 | 1.000159              | 2.272289                                                       |
| 6279 | 1.712375              | 2.272315                                                       |
| 6281 | 1.092820              | 2.272342                                                       |
| 6283 | 1.026261              | 2.272369                                                       |
| 6285 | 1.603819              | 2.272395                                                       |
| 6287 | 1.000159              | 2.272422                                                       |
| 6289 | 1.055812              | 2.272449                                                       |
| 6291 | 1.487840              | 2.272475                                                       |
| 6293 | 1.220404              | 2.272502                                                       |
| 6295 | 1.200953              | 2.272529                                                       |
| 6297 | 1.333969              | 2.272555                                                       |
| 6299 | 1.000159              | 2.272582                                                       |
| 6301 | 1.000159              | 2.272609                                                       |
| 6303 | 1.462161              | 2.272635                                                       |
| 6305 | 1.305630              | 2.272662                                                       |
| 6307 | 1.232916              | 2.272688                                                       |
| 6309 | 1.446505              | 2.272715                                                       |
| 6311 | 1.000158              | 2.272741                                                       |
| 6313 | 1.026453              | 2.272768                                                       |
| 6315 | 1.603800              | 2.272795                                                       |
| 6317 | 1.000158              | 2.272821                                                       |
| 6319 | 1.025479              | 2.272848                                                       |
| 6321 | 1.587091              | 2.272874                                                       |
| 6323 | 1.000158              | 2.272901                                                       |
| 6325 | 1.411542              | 2.272927                                                       |
| 6327 | 1.561562              | 2.272954                                                       |
| 6329 | 1.000158              | 2.272980                                                       |
| 6331 | 1.079134              | 2.273007                                                       |
| 6333 | 1.333965              | 2.273033                                                       |
| 6335 | 1.379006              | 2.273060                                                       |
| 6337 | 1.000158              | 2.273086                                                       |
| 6339 | 1.333964              | 2.273112                                                       |
| 6341 | 1.061662              | 2.273139                                                       |
| 6343 | 1.000158              | 2.273165                                                       |
| 6345 | 1.815603              | 2.273192                                                       |
| 6347 | 1.092800              | 2.273218                                                       |
| 6349 | 1.144117              | 2.273244                                                       |

| $n$  | $\frac{\sigma(n)}{n}$ | $\frac{e^\gamma}{2} \log \log n + \frac{0.73...}{\log \log n}$ |
|------|-----------------------|----------------------------------------------------------------|
| 6351 | 1.398205              | 2.273271                                                       |
| 6353 | 1.000157              | 2.273297                                                       |
| 6355 | 1.268922              | 2.273324                                                       |
| 6357 | 1.444707              | 2.273350                                                       |
| 6359 | 1.000157              | 2.273376                                                       |
| 6361 | 1.000157              | 2.273403                                                       |
| 6363 | 1.667138              | 2.273429                                                       |
| 6365 | 1.282011              | 2.273455                                                       |
| 6367 | 1.000157              | 2.273482                                                       |
| 6369 | 1.462082              | 2.273508                                                       |
| 6371 | 1.047245              | 2.273534                                                       |
| 6373 | 1.000157              | 2.273560                                                       |
| 6375 | 1.761882              | 2.273587                                                       |
| 6377 | 1.144112              | 2.273613                                                       |
| 6379 | 1.000157              | 2.273639                                                       |
| 6381 | 1.446482              | 2.273665                                                       |
| 6383 | 1.079116              | 2.273692                                                       |
| 6385 | 1.200940              | 2.273718                                                       |
| 6387 | 1.333960              | 2.273744                                                       |
| 6389 | 1.000157              | 2.273770                                                       |
| 6391 | 1.261774              | 2.273797                                                       |
| 6393 | 1.333959              | 2.273823                                                       |
| 6395 | 1.200938              | 2.273849                                                       |
| 6397 | 1.000156              | 2.273875                                                       |
| 6399 | 1.512736              | 2.273901                                                       |
| 6401 | 1.032964              | 2.273927                                                       |
| 6403 | 1.055755              | 2.273954                                                       |
| 6405 | 1.858548              | 2.273980                                                       |
| 6407 | 1.030123              | 2.274006                                                       |
| 6409 | 1.179591              | 2.274032                                                       |
| 6411 | 1.333957              | 2.274058                                                       |
| 6413 | 1.119913              | 2.274084                                                       |
| 6415 | 1.200935              | 2.274110                                                       |
| 6417 | 1.555867              | 2.274136                                                       |
| 6419 | 1.172145              | 2.274162                                                       |
| 6421 | 1.000156              | 2.274188                                                       |
| 6423 | 1.333956              | 2.274214                                                       |
| 6425 | 1.244825              | 2.274241                                                       |
| 6427 | 1.000156              | 2.274267                                                       |
| 6429 | 1.333956              | 2.274293                                                       |
| 6431 | 1.026279              | 2.274319                                                       |
| 6433 | 1.144101              | 2.274345                                                       |
| 6435 | 2.036364              | 2.274371                                                       |
| 6437 | 1.030915              | 2.274397                                                       |

| $n$  | $\frac{\sigma(n)}{n}$ | $\frac{e^\gamma}{2} \log \log n + \frac{0.73...}{\log \log n}$ |
|------|-----------------------|----------------------------------------------------------------|
| 6439 | 1.028731              | 2.274423                                                       |
| 6441 | 1.415929              | 2.274449                                                       |
| 6443 | 1.061617              | 2.274475                                                       |
| 6445 | 1.200931              | 2.274501                                                       |
| 6447 | 1.528773              | 2.274526                                                       |
| 6449 | 1.000155              | 2.274552                                                       |
| 6451 | 1.000155              | 2.274578                                                       |
| 6453 | 1.487680              | 2.274604                                                       |
| 6455 | 1.200930              | 2.274630                                                       |
| 6457 | 1.092768              | 2.274656                                                       |
| 6459 | 1.333953              | 2.274682                                                       |
| 6461 | 1.248104              | 2.274708                                                       |
| 6463 | 1.047192              | 2.274734                                                       |
| 6465 | 1.603712              | 2.274760                                                       |
| 6467 | 1.039122              | 2.274786                                                       |
| 6469 | 1.000155              | 2.274811                                                       |
| 6471 | 1.446453              | 2.274837                                                       |
| 6473 | 1.000154              | 2.274863                                                       |
| 6475 | 1.455444              | 2.274889                                                       |
| 6477 | 1.422881              | 2.274915                                                       |
| 6479 | 1.185368              | 2.274941                                                       |
| 6481 | 1.000154              | 2.274966                                                       |
| 6483 | 1.333950              | 2.274992                                                       |
| 6485 | 1.200925              | 2.275018                                                       |
| 6487 | 1.079081              | 2.275044                                                       |
| 6489 | 1.666821              | 2.275069                                                       |
| 6491 | 1.000154              | 2.275095                                                       |
| 6493 | 1.030032              | 2.275121                                                       |
| 6495 | 1.603695              | 2.275147                                                       |
| 6497 | 1.025089              | 2.275172                                                       |
| 6499 | 1.025389              | 2.275198                                                       |
| 6501 | 1.461929              | 2.275224                                                       |
| 6503 | 1.144087              | 2.275250                                                       |
| 6505 | 1.200922              | 2.275275                                                       |
| 6507 | 1.487629              | 2.275301                                                       |
| 6509 | 1.047165              | 2.275327                                                       |
| 6511 | 1.061588              | 2.275352                                                       |
| 6513 | 1.444496              | 2.275378                                                       |
| 6515 | 1.200921              | 2.275404                                                       |
| 6517 | 1.227559              | 2.275429                                                       |
| 6519 | 1.391624              | 2.275455                                                       |
| 6521 | 1.000153              | 2.275481                                                       |
| 6523 | 1.092749              | 2.275506                                                       |
| 6525 | 1.852874              | 2.275532                                                       |



| $n$  | $\frac{\sigma(n)}{n}$ | $\frac{e^\gamma}{2} \log \log n + \frac{0.73...}{\log \log n}$ |
|------|-----------------------|----------------------------------------------------------------|
| 6527 | 1.025892              | 2.275557                                                       |
| 6529 | 1.000153              | 2.275583                                                       |
| 6531 | 1.528709              | 2.275609                                                       |
| 6533 | 1.028624              | 2.275634                                                       |
| 6535 | 1.200918              | 2.275660                                                       |
| 6537 | 1.333945              | 2.275685                                                       |
| 6539 | 1.079064              | 2.275711                                                       |
| 6541 | 1.037150              | 2.275736                                                       |
| 6543 | 1.446431              | 2.275762                                                       |
| 6545 | 1.584110              | 2.275787                                                       |
| 6547 | 1.000153              | 2.275813                                                       |
| 6549 | 1.392579              | 2.275838                                                       |
| 6551 | 1.000153              | 2.275864                                                       |
| 6553 | 1.000153              | 2.275889                                                       |
| 6555 | 1.757437              | 2.275915                                                       |
| 6557 | 1.024859              | 2.275940                                                       |
| 6559 | 1.144077              | 2.275966                                                       |
| 6561 | 1.499924              | 2.275991                                                       |
| 6563 | 1.000152              | 2.276017                                                       |
| 6565 | 1.305103              | 2.276042                                                       |
| 6567 | 1.461855              | 2.276068                                                       |
| 6569 | 1.000152              | 2.276093                                                       |
| 6571 | 1.000152              | 2.276118                                                       |
| 6573 | 1.528678              | 2.276144                                                       |
| 6575 | 1.244715              | 2.276169                                                       |
| 6577 | 1.000152              | 2.276195                                                       |
| 6579 | 1.564979              | 2.276220                                                       |
| 6581 | 1.000152              | 2.276245                                                       |
| 6583 | 1.039040              | 2.276271                                                       |
| 6585 | 1.603645              | 2.276296                                                       |
| 6587 | 1.144072              | 2.276322                                                       |
| 6589 | 1.092730              | 2.276347                                                       |
| 6591 | 1.444394              | 2.276372                                                       |
| 6593 | 1.055665              | 2.276398                                                       |
| 6595 | 1.200910              | 2.276423                                                       |
| 6597 | 1.446415              | 2.276448                                                       |
| 6599 | 1.000152              | 2.276473                                                       |
| 6601 | 1.221633              | 2.276499                                                       |
| 6603 | 1.395729              | 2.276524                                                       |
| 6605 | 1.200908              | 2.276549                                                       |
| 6607 | 1.000151              | 2.276575                                                       |
| 6609 | 1.333939              | 2.276600                                                       |
| 6611 | 1.092724              | 2.276625                                                       |
| 6613 | 1.061545              | 2.276650                                                       |

| $n$  | $\frac{\sigma(n)}{n}$ | $\frac{e^\gamma}{2} \log \log n + \frac{0.73...}{\log \log n}$ |
|------|-----------------------|----------------------------------------------------------------|
| 6615 | 2.068027              | 2.276676                                                       |
| 6617 | 1.079039              | 2.276701                                                       |
| 6619 | 1.000151              | 2.276726                                                       |
| 6621 | 1.333937              | 2.276751                                                       |
| 6623 | 1.032765              | 2.276776                                                       |
| 6625 | 1.271547              | 2.276802                                                       |
| 6627 | 1.362306              | 2.276827                                                       |
| 6629 | 1.144064              | 2.276852                                                       |
| 6631 | 1.055648              | 2.276877                                                       |
| 6633 | 1.599276              | 2.276902                                                       |
| 6635 | 1.200904              | 2.276927                                                       |
| 6637 | 1.000151              | 2.276953                                                       |
| 6639 | 1.333936              | 2.276978                                                       |
| 6641 | 1.039000              | 2.277003                                                       |
| 6643 | 1.247629              | 2.277028                                                       |
| 6645 | 1.603612              | 2.277053                                                       |
| 6647 | 1.108470              | 2.277078                                                       |
| 6649 | 1.025718              | 2.277103                                                       |
| 6651 | 1.446399              | 2.277128                                                       |
| 6653 | 1.000150              | 2.277153                                                       |
| 6655 | 1.319910              | 2.277178                                                       |
| 6657 | 1.528616              | 2.277204                                                       |
| 6659 | 1.000150              | 2.277229                                                       |
| 6661 | 1.000150              | 2.277254                                                       |
| 6663 | 1.333934              | 2.277279                                                       |
| 6665 | 1.267517              | 2.277304                                                       |
| 6667 | 1.025949              | 2.277329                                                       |
| 6669 | 1.679412              | 2.277354                                                       |
| 6671 | 1.144056              | 2.277379                                                       |
| 6673 | 1.000150              | 2.277404                                                       |
| 6675 | 1.671910              | 2.277429                                                       |
| 6677 | 1.092706              | 2.277454                                                       |
| 6679 | 1.000150              | 2.277479                                                       |
| 6681 | 1.422542              | 2.277504                                                       |
| 6683 | 1.030675              | 2.277529                                                       |
| 6685 | 1.378609              | 2.277553                                                       |
| 6687 | 1.446389              | 2.277578                                                       |
| 6689 | 1.000149              | 2.277603                                                       |
| 6691 | 1.000149              | 2.277628                                                       |
| 6693 | 1.405648              | 2.277653                                                       |
| 6695 | 1.304854              | 2.277678                                                       |
| 6697 | 1.032701              | 2.277703                                                       |
| 6699 | 1.719660              | 2.277728                                                       |
| 6701 | 1.000149              | 2.277753                                                       |

| $n$  | $\frac{\sigma(n)}{n}$ | $\frac{e^\gamma}{2} \log \log n + \frac{0.73...}{\log \log n}$ |
|------|-----------------------|----------------------------------------------------------------|
| 6703 | 1.000149              | 2.277778                                                       |
| 6705 | 1.744966              | 2.277802                                                       |
| 6707 | 1.055614              | 2.277827                                                       |
| 6709 | 1.000149              | 2.277852                                                       |
| 6711 | 1.333929              | 2.277877                                                       |
| 6713 | 1.171756              | 2.277902                                                       |
| 6715 | 1.286672              | 2.277927                                                       |
| 6717 | 1.333929              | 2.277951                                                       |
| 6719 | 1.000149              | 2.277976                                                       |
| 6721 | 1.199821              | 2.278001                                                       |
| 6723 | 1.511825              | 2.278026                                                       |
| 6725 | 1.244610              | 2.278051                                                       |
| 6727 | 1.180913              | 2.278075                                                       |
| 6729 | 1.333928              | 2.278100                                                       |
| 6731 | 1.026891              | 2.278125                                                       |
| 6733 | 1.000149              | 2.278150                                                       |
| 6735 | 1.603563              | 2.278174                                                       |
| 6737 | 1.000148              | 2.278199                                                       |
| 6739 | 1.047040              | 2.278224                                                       |
| 6741 | 1.666222              | 2.278249                                                       |
| 6743 | 1.092689              | 2.278273                                                       |
| 6745 | 1.280949              | 2.278298                                                       |
| 6747 | 1.444197              | 2.278323                                                       |
| 6749 | 1.061491              | 2.278347                                                       |
| 6751 | 1.029773              | 2.278372                                                       |
| 6753 | 1.333926              | 2.278397                                                       |
| 6755 | 1.378534              | 2.278421                                                       |
| 6757 | 1.038923              | 2.278446                                                       |
| 6759 | 1.446368              | 2.278471                                                       |
| 6761 | 1.000148              | 2.278495                                                       |
| 6763 | 1.000148              | 2.278520                                                       |
| 6765 | 1.788027              | 2.278545                                                       |
| 6767 | 1.024974              | 2.278569                                                       |
| 6769 | 1.144039              | 2.278594                                                       |
| 6771 | 1.391818              | 2.278618                                                       |
| 6773 | 1.078990              | 2.278643                                                       |
| 6775 | 1.244576              | 2.278668                                                       |
| 6777 | 1.487384              | 2.278692                                                       |
| 6779 | 1.000148              | 2.278717                                                       |
| 6781 | 1.000147              | 2.278741                                                       |
| 6783 | 1.698364              | 2.278766                                                       |
| 6785 | 1.273397              | 2.278790                                                       |
| 6787 | 1.092677              | 2.278815                                                       |
| 6789 | 1.395198              | 2.278839                                                       |

| $n$  | $\frac{\sigma(n)}{n}$ | $\frac{e^\gamma}{2} \log \log n + \frac{0.73...}{\log \log n}$ |
|------|-----------------------|----------------------------------------------------------------|
| 6791 | 1.000147              | 2.278864                                                       |
| 6793 | 1.000147              | 2.278888                                                       |
| 6795 | 1.744812              | 2.278913                                                       |
| 6797 | 1.144034              | 2.278937                                                       |
| 6799 | 1.078982              | 2.278962                                                       |
| 6801 | 1.333921              | 2.278986                                                       |
| 6803 | 1.000147              | 2.279011                                                       |
| 6805 | 1.200882              | 2.279035                                                       |
| 6807 | 1.333921              | 2.279060                                                       |
| 6809 | 1.092671              | 2.279084                                                       |
| 6811 | 1.171634              | 2.279109                                                       |
| 6813 | 1.446353              | 2.279133                                                       |
| 6815 | 1.267792              | 2.279158                                                       |
| 6817 | 1.061464              | 2.279182                                                       |
| 6819 | 1.333920              | 2.279206                                                       |
| 6821 | 1.055564              | 2.279231                                                       |
| 6823 | 1.000147              | 2.279255                                                       |
| 6825 | 2.034872              | 2.279280                                                       |
| 6827 | 1.000146              | 2.279304                                                       |
| 6829 | 1.000146              | 2.279328                                                       |
| 6831 | 1.686430              | 2.279353                                                       |
| 6833 | 1.000146              | 2.279377                                                       |
| 6835 | 1.200878              | 2.279401                                                       |
| 6837 | 1.390083              | 2.279426                                                       |
| 6839 | 1.144027              | 2.279450                                                       |
| 6841 | 1.000146              | 2.279474                                                       |
| 6843 | 1.333918              | 2.279499                                                       |
| 6845 | 1.233309              | 2.279523                                                       |
| 6847 | 1.030524              | 2.279547                                                       |
| 6849 | 1.446343              | 2.279572                                                       |
| 6851 | 1.177054              | 2.279596                                                       |
| 6853 | 1.260762              | 2.279620                                                       |
| 6855 | 1.603501              | 2.279644                                                       |
| 6857 | 1.000146              | 2.279669                                                       |
| 6859 | 1.055547              | 2.279693                                                       |
| 6861 | 1.333916              | 2.279717                                                       |
| 6863 | 1.000146              | 2.279741                                                       |
| 6865 | 1.200874              | 2.279766                                                       |
| 6867 | 1.665939              | 2.279790                                                       |
| 6869 | 1.000146              | 2.279814                                                       |
| 6871 | 1.000146              | 2.279838                                                       |
| 6873 | 1.396770              | 2.279863                                                       |
| 6875 | 1.363200              | 2.279887                                                       |
| 6877 | 1.125782              | 2.279911                                                       |

| $n$  | $\frac{\sigma(n)}{n}$ | $\frac{e^\gamma}{2} \log \log n + \frac{0.73...}{\log \log n}$ |
|------|-----------------------|----------------------------------------------------------------|
| 6879 | 1.333915              | 2.279935                                                       |
| 6881 | 1.144020              | 2.279959                                                       |
| 6883 | 1.000145              | 2.279983                                                       |
| 6885 | 1.898039              | 2.280008                                                       |
| 6887 | 1.024539              | 2.280032                                                       |
| 6889 | 1.012193              | 2.280056                                                       |
| 6891 | 1.333914              | 2.280080                                                       |
| 6893 | 1.025388              | 2.280104                                                       |
| 6895 | 1.378390              | 2.280128                                                       |
| 6897 | 1.542700              | 2.280152                                                       |
| 6899 | 1.000145              | 2.280176                                                       |
| 6901 | 1.024779              | 2.280201                                                       |
| 6903 | 1.581921              | 2.280225                                                       |
| 6905 | 1.200869              | 2.280249                                                       |
| 6907 | 1.000145              | 2.280273                                                       |
| 6909 | 1.584021              | 2.280297                                                       |
| 6911 | 1.000145              | 2.280321                                                       |
| 6913 | 1.036887              | 2.280345                                                       |
| 6915 | 1.603471              | 2.280369                                                       |
| 6917 | 1.000145              | 2.280393                                                       |
| 6919 | 1.186299              | 2.280417                                                       |
| 6921 | 1.446323              | 2.280441                                                       |
| 6923 | 1.220280              | 2.280465                                                       |
| 6925 | 1.244477              | 2.280489                                                       |
| 6927 | 1.333911              | 2.280513                                                       |
| 6929 | 1.109251              | 2.280537                                                       |
| 6931 | 1.038811              | 2.280561                                                       |
| 6933 | 1.333910              | 2.280585                                                       |
| 6935 | 1.280461              | 2.280609                                                       |
| 6937 | 1.144010              | 2.280633                                                       |
| 6939 | 1.487246              | 2.280657                                                       |
| 6941 | 1.092638              | 2.280681                                                       |
| 6943 | 1.026646              | 2.280705                                                       |
| 6945 | 1.603456              | 2.280729                                                       |
| 6947 | 1.000144              | 2.280753                                                       |
| 6949 | 1.000144              | 2.280776                                                       |
| 6951 | 1.528413              | 2.280800                                                       |
| 6953 | 1.061412              | 2.280824                                                       |
| 6955 | 1.304385              | 2.280848                                                       |
| 6957 | 1.446313              | 2.280872                                                       |
| 6959 | 1.000144              | 2.280896                                                       |
| 6961 | 1.000144              | 2.280920                                                       |
| 6963 | 1.461439              | 2.280944                                                       |
| 6965 | 1.378320              | 2.280968                                                       |

| $n$  | $\frac{\sigma(n)}{n}$ | $\frac{e^\gamma}{2} \log \log n + \frac{0.73...}{\log \log n}$ |
|------|-----------------------|----------------------------------------------------------------|
| 6967 | 1.000144              | 2.280991                                                       |
| 6969 | 1.405080              | 2.281015                                                       |
| 6971 | 1.000143              | 2.281039                                                       |
| 6973 | 1.055500              | 2.281063                                                       |
| 6975 | 1.848889              | 2.281087                                                       |
| 6977 | 1.000143              | 2.281110                                                       |
| 6979 | 1.144003              | 2.281134                                                       |
| 6981 | 1.443919              | 2.281158                                                       |
| 6983 | 1.000143              | 2.281182                                                       |
| 6985 | 1.319399              | 2.281206                                                       |
| 6987 | 1.422070              | 2.281229                                                       |
| 6989 | 1.038775              | 2.281253                                                       |
| 6991 | 1.000143              | 2.281277                                                       |
| 6993 | 1.738882              | 2.281301                                                       |
| 6995 | 1.200858              | 2.281324                                                       |
| 6997 | 1.000143              | 2.281348                                                       |
| 6999 | 1.333905              | 2.281372                                                       |
| 7001 | 1.000143              | 2.281396                                                       |
| 7003 | 1.028131              | 2.281419                                                       |
| 7005 | 1.603426              | 2.281443                                                       |
| 7007 | 1.366633              | 2.281467                                                       |
| 7009 | 1.029533              | 2.281490                                                       |
| 7011 | 1.557552              | 2.281514                                                       |
| 7013 | 1.000143              | 2.281538                                                       |
| 7015 | 1.272701              | 2.281561                                                       |
| 7017 | 1.333903              | 2.281585                                                       |
| 7019 | 1.000142              | 2.281609                                                       |
| 7021 | 1.230594              | 2.281632                                                       |
| 7023 | 1.333903              | 2.281656                                                       |
| 7025 | 1.244413              | 2.281680                                                       |
| 7027 | 1.000142              | 2.281703                                                       |
| 7029 | 1.597951              | 2.281727                                                       |
| 7031 | 1.024036              | 2.281750                                                       |
| 7033 | 1.078914              | 2.281774                                                       |
| 7035 | 1.855864              | 2.281798                                                       |
| 7037 | 1.036805              | 2.281821                                                       |
| 7039 | 1.000142              | 2.281845                                                       |
| 7041 | 1.333901              | 2.281868                                                       |
| 7043 | 1.000142              | 2.281892                                                       |
| 7045 | 1.200852              | 2.281916                                                       |
| 7047 | 1.549596              | 2.281939                                                       |
| 7049 | 1.225706              | 2.281963                                                       |
| 7051 | 1.092611              | 2.281986                                                       |
| 7053 | 1.333900              | 2.282010                                                       |

| $n$  | $\frac{\sigma(n)}{n}$ | $\frac{e^\gamma}{2} \log \log n + \frac{0.73...}{\log \log n}$ |
|------|-----------------------|----------------------------------------------------------------|
| 7055 | 1.285897              | 2.282033                                                       |
| 7057 | 1.000142              | 2.282057                                                       |
| 7059 | 1.443831              | 2.282080                                                       |
| 7061 | 1.046877              | 2.282104                                                       |
| 7063 | 1.143990              | 2.282127                                                       |
| 7065 | 1.744374              | 2.282151                                                       |
| 7067 | 1.032404              | 2.282174                                                       |
| 7069 | 1.000141              | 2.282198                                                       |
| 7071 | 1.333899              | 2.282221                                                       |
| 7073 | 1.092606              | 2.282245                                                       |
| 7075 | 1.244382              | 2.282268                                                       |
| 7077 | 1.528331              | 2.282291                                                       |
| 7079 | 1.000141              | 2.282315                                                       |
| 7081 | 1.024149              | 2.282338                                                       |
| 7083 | 1.446280              | 2.282362                                                       |
| 7085 | 1.304164              | 2.282385                                                       |
| 7087 | 1.055454              | 2.282409                                                       |
| 7089 | 1.421921              | 2.282432                                                       |
| 7091 | 1.143985              | 2.282455                                                       |
| 7093 | 1.030312              | 2.282479                                                       |
| 7095 | 1.786047              | 2.282502                                                       |
| 7097 | 1.028040              | 2.282525                                                       |
| 7099 | 1.036766              | 2.282549                                                       |
| 7101 | 1.487114              | 2.282572                                                       |
| 7103 | 1.000141              | 2.282595                                                       |
| 7105 | 1.444053              | 2.282619                                                       |
| 7107 | 1.404812              | 2.282642                                                       |
| 7109 | 1.000141              | 2.282665                                                       |
| 7111 | 1.078892              | 2.282689                                                       |
| 7113 | 1.333896              | 2.282712                                                       |
| 7115 | 1.200843              | 2.282735                                                       |
| 7117 | 1.092595              | 2.282759                                                       |
| 7119 | 1.665402              | 2.282782                                                       |
| 7121 | 1.000140              | 2.282805                                                       |
| 7123 | 1.061351              | 2.282829                                                       |
| 7125 | 1.751579              | 2.282852                                                       |
| 7127 | 1.000140              | 2.282875                                                       |
| 7129 | 1.000140              | 2.282898                                                       |
| 7131 | 1.333894              | 2.282922                                                       |
| 7133 | 1.143979              | 2.282945                                                       |
| 7135 | 1.200841              | 2.282968                                                       |
| 7137 | 1.581056              | 2.282991                                                       |
| 7139 | 1.117804              | 2.283014                                                       |
| 7141 | 1.032348              | 2.283038                                                       |

| $n$  | $\frac{\sigma(n)}{n}$ | $\frac{e^\gamma}{2} \log \log n + \frac{0.73...}{\log \log n}$ |
|------|-----------------------|----------------------------------------------------------------|
| 7143 | 1.333893              | 2.283061                                                       |
| 7145 | 1.200840              | 2.283084                                                       |
| 7147 | 1.143976              | 2.283107                                                       |
| 7149 | 1.333893              | 2.283130                                                       |
| 7151 | 1.000140              | 2.283154                                                       |
| 7153 | 1.046833              | 2.283177                                                       |
| 7155 | 1.811321              | 2.283200                                                       |
| 7157 | 1.061339              | 2.283223                                                       |
| 7159 | 1.000140              | 2.283246                                                       |
| 7161 | 1.715961              | 2.283269                                                       |
| 7163 | 1.172693              | 2.283293                                                       |
| 7165 | 1.200837              | 2.283316                                                       |
| 7167 | 1.333891              | 2.283339                                                       |
| 7169 | 1.024411              | 2.283362                                                       |
| 7171 | 1.024125              | 2.283385                                                       |
| 7173 | 1.446257              | 2.283408                                                       |
| 7175 | 1.451707              | 2.283431                                                       |
| 7177 | 1.000139              | 2.283454                                                       |
| 7179 | 1.333891              | 2.283477                                                       |
| 7181 | 1.029383              | 2.283500                                                       |
| 7183 | 1.092580              | 2.283524                                                       |
| 7185 | 1.603340              | 2.283547                                                       |
| 7187 | 1.000139              | 2.283570                                                       |
| 7189 | 1.246349              | 2.283593                                                       |
| 7191 | 1.561952              | 2.283616                                                       |
| 7193 | 1.000139              | 2.283639                                                       |
| 7195 | 1.200834              | 2.283662                                                       |
| 7197 | 1.333889              | 2.283685                                                       |
| 7199 | 1.046812              | 2.283708                                                       |
| 7201 | 1.055409              | 2.283731                                                       |
| 7203 | 1.555463              | 2.283754                                                       |
| 7205 | 1.319084              | 2.283777                                                       |
| 7207 | 1.000139              | 2.283800                                                       |
| 7209 | 1.510612              | 2.283823                                                       |
| 7211 | 1.000139              | 2.283846                                                       |
| 7213 | 1.000139              | 2.283869                                                       |
| 7215 | 1.769647              | 2.283892                                                       |
| 7217 | 1.143966              | 2.283915                                                       |
| 7219 | 1.000139              | 2.283937                                                       |
| 7221 | 1.395929              | 2.283960                                                       |
| 7223 | 1.036688              | 2.283983                                                       |
| 7225 | 1.317232              | 2.284006                                                       |
| 7227 | 1.597343              | 2.284029                                                       |
| 7229 | 1.000138              | 2.284052                                                       |



| $n$  | $\frac{\sigma(n)}{n}$ | $\frac{e^\gamma}{2} \log \log n + \frac{0.73...}{\log \log n}$ |
|------|-----------------------|----------------------------------------------------------------|
| 7231 | 1.143963              | 2.284075                                                       |
| 7233 | 1.333886              | 2.284098                                                       |
| 7235 | 1.200829              | 2.284121                                                       |
| 7237 | 1.000138              | 2.284144                                                       |
| 7239 | 1.414560              | 2.284166                                                       |
| 7241 | 1.078857              | 2.284189                                                       |
| 7243 | 1.000138              | 2.284212                                                       |
| 7245 | 2.067081              | 2.284235                                                       |
| 7247 | 1.000138              | 2.284258                                                       |
| 7249 | 1.092564              | 2.284281                                                       |
| 7251 | 1.333885              | 2.284304                                                       |
| 7253 | 1.000138              | 2.284326                                                       |
| 7255 | 1.200827              | 2.284349                                                       |
| 7257 | 1.389004              | 2.284372                                                       |
| 7259 | 1.229921              | 2.284395                                                       |
| 7261 | 1.026305              | 2.284418                                                       |
| 7263 | 1.486989              | 2.284440                                                       |
| 7265 | 1.200826              | 2.284463                                                       |
| 7267 | 1.108023              | 2.284486                                                       |
| 7269 | 1.333884              | 2.284509                                                       |
| 7271 | 1.092559              | 2.284531                                                       |
| 7273 | 1.143957              | 2.284554                                                       |
| 7275 | 1.670378              | 2.284577                                                       |
| 7277 | 1.055380              | 2.284600                                                       |
| 7279 | 1.038604              | 2.284622                                                       |
| 7281 | 1.446230              | 2.284645                                                       |
| 7283 | 1.000137              | 2.284668                                                       |
| 7285 | 1.265065              | 2.284691                                                       |
| 7287 | 1.528201              | 2.284713                                                       |
| 7289 | 1.032240              | 2.284736                                                       |
| 7291 | 1.046770              | 2.284759                                                       |
| 7293 | 1.658577              | 2.284781                                                       |
| 7295 | 1.200822              | 2.284804                                                       |
| 7297 | 1.000137              | 2.284827                                                       |
| 7299 | 1.446226              | 2.284849                                                       |
| 7301 | 1.171072              | 2.284872                                                       |
| 7303 | 1.024237              | 2.284895                                                       |
| 7305 | 1.603285              | 2.284917                                                       |
| 7307 | 1.000137              | 2.284940                                                       |
| 7309 | 1.000137              | 2.284963                                                       |
| 7311 | 1.333880              | 2.284985                                                       |
| 7313 | 1.023930              | 2.285008                                                       |
| 7315 | 1.574846              | 2.285030                                                       |
| 7317 | 1.486948              | 2.285053                                                       |

| $n$  | $\frac{\sigma(n)}{n}$ | $\frac{e^\gamma}{2} \log \log n + \frac{0.73...}{\log \log n}$ |
|------|-----------------------|----------------------------------------------------------------|
| 7319 | 1.078836              | 2.285076                                                       |
| 7321 | 1.000137              | 2.285098                                                       |
| 7323 | 1.333880              | 2.285121                                                       |
| 7325 | 1.244232              | 2.285143                                                       |
| 7327 | 1.061280              | 2.285166                                                       |
| 7329 | 1.528176              | 2.285188                                                       |
| 7331 | 1.000136              | 2.285211                                                       |
| 7333 | 1.000136              | 2.285234                                                       |
| 7335 | 1.743967              | 2.285256                                                       |
| 7337 | 1.177593              | 2.285279                                                       |
| 7339 | 1.030113              | 2.285301                                                       |
| 7341 | 1.333878              | 2.285324                                                       |
| 7343 | 1.143947              | 2.285346                                                       |
| 7345 | 1.303744              | 2.285369                                                       |
| 7347 | 1.393766              | 2.285391                                                       |
| 7349 | 1.000136              | 2.285414                                                       |
| 7351 | 1.000136              | 2.285436                                                       |
| 7353 | 1.555828              | 2.285459                                                       |
| 7355 | 1.200816              | 2.285481                                                       |
| 7357 | 1.143945              | 2.285504                                                       |
| 7359 | 1.461068              | 2.285526                                                       |
| 7361 | 1.061269              | 2.285549                                                       |
| 7363 | 1.032188              | 2.285571                                                       |
| 7365 | 1.603259              | 2.285593                                                       |
| 7367 | 1.026198              | 2.285616                                                       |
| 7369 | 1.000136              | 2.285638                                                       |
| 7371 | 1.838557              | 2.285661                                                       |
| 7373 | 1.023735              | 2.285683                                                       |
| 7375 | 1.269153              | 2.285706                                                       |
| 7377 | 1.333876              | 2.285728                                                       |
| 7379 | 1.027782              | 2.285750                                                       |
| 7381 | 1.117193              | 2.285773                                                       |
| 7383 | 1.404307              | 2.285795                                                       |
| 7385 | 1.377928              | 2.285817                                                       |
| 7387 | 1.023420              | 2.285840                                                       |
| 7389 | 1.446204              | 2.285862                                                       |
| 7391 | 1.055338              | 2.285885                                                       |
| 7393 | 1.000135              | 2.285907                                                       |
| 7395 | 1.752535              | 2.285929                                                       |
| 7397 | 1.078816              | 2.285952                                                       |
| 7399 | 1.170969              | 2.285974                                                       |
| 7401 | 1.333874              | 2.285996                                                       |
| 7403 | 1.092530              | 2.286019                                                       |
| 7405 | 1.200810              | 2.286041                                                       |

| $n$  | $\frac{\sigma(n)}{n}$ | $\frac{e^\gamma}{2} \log \log n + \frac{0.73...}{\log \log n}$ |
|------|-----------------------|----------------------------------------------------------------|
| 7407 | 1.446200              | 2.286063                                                       |
| 7409 | 1.036577              | 2.286085                                                       |
| 7411 | 1.000135              | 2.286108                                                       |
| 7413 | 1.528126              | 2.286130                                                       |
| 7415 | 1.200809              | 2.286152                                                       |
| 7417 | 1.000135              | 2.286175                                                       |
| 7419 | 1.333872              | 2.286197                                                       |
| 7421 | 1.030050              | 2.286219                                                       |
| 7423 | 1.078809              | 2.286241                                                       |
| 7425 | 2.004040              | 2.286264                                                       |
| 7427 | 1.143934              | 2.286286                                                       |
| 7429 | 1.163010              | 2.286308                                                       |
| 7431 | 1.333872              | 2.286330                                                       |
| 7433 | 1.000135              | 2.286353                                                       |
| 7435 | 1.200807              | 2.286375                                                       |
| 7437 | 1.389808              | 2.286397                                                       |
| 7439 | 1.029171              | 2.286419                                                       |
| 7441 | 1.143932              | 2.286441                                                       |
| 7443 | 1.446191              | 2.286464                                                       |
| 7445 | 1.200806              | 2.286486                                                       |
| 7447 | 1.092520              | 2.286508                                                       |
| 7449 | 1.443415              | 2.286530                                                       |
| 7451 | 1.000134              | 2.286552                                                       |
| 7453 | 1.038508              | 2.286574                                                       |
| 7455 | 1.854326              | 2.286596                                                       |
| 7457 | 1.000134              | 2.286619                                                       |
| 7459 | 1.000134              | 2.286641                                                       |
| 7461 | 1.446187              | 2.286663                                                       |
| 7463 | 1.061235              | 2.286685                                                       |
| 7465 | 1.200804              | 2.286707                                                       |
| 7467 | 1.414223              | 2.286729                                                       |
| 7469 | 1.259606              | 2.286751                                                       |
| 7471 | 1.036541              | 2.286773                                                       |
| 7473 | 1.387395              | 2.286796                                                       |
| 7475 | 1.393445              | 2.286818                                                       |
| 7477 | 1.000134              | 2.286840                                                       |
| 7479 | 1.486830              | 2.286862                                                       |
| 7481 | 1.000134              | 2.286884                                                       |
| 7483 | 1.143926              | 2.286906                                                       |
| 7485 | 1.603206              | 2.286928                                                       |
| 7487 | 1.000134              | 2.286950                                                       |
| 7489 | 1.000134              | 2.286972                                                       |
| 7491 | 1.460953              | 2.286994                                                       |
| 7493 | 1.024957              | 2.287016                                                       |

| $n$  | $\frac{\sigma(n)}{n}$ | $\frac{e^\gamma}{2} \log \log n + \frac{0.73...}{\log \log n}$ |
|------|-----------------------|----------------------------------------------------------------|
| 7495 | 1.200801              | 2.287038                                                       |
| 7497 | 1.779112              | 2.287060                                                       |
| 7499 | 1.000133              | 2.287082                                                       |
| 7501 | 1.078789              | 2.287104                                                       |
| 7503 | 1.388245              | 2.287126                                                       |
| 7505 | 1.279147              | 2.287148                                                       |
| 7507 | 1.000133              | 2.287170                                                       |
| 7509 | 1.333866              | 2.287192                                                       |
| 7511 | 1.214219              | 2.287214                                                       |
| 7513 | 1.092506              | 2.287236                                                       |
| 7515 | 1.743713              | 2.287258                                                       |
| 7517 | 1.000133              | 2.287280                                                       |
| 7519 | 1.023540              | 2.287302                                                       |
| 7521 | 1.404069              | 2.287324                                                       |
| 7523 | 1.000133              | 2.287346                                                       |
| 7525 | 1.450100              | 2.287368                                                       |
| 7527 | 1.443337              | 2.287389                                                       |
| 7529 | 1.000133              | 2.287411                                                       |
| 7531 | 1.061214              | 2.287433                                                       |
| 7533 | 1.546263              | 2.287455                                                       |
| 7535 | 1.318646              | 2.287477                                                       |
| 7537 | 1.000133              | 2.287499                                                       |
| 7539 | 1.528054              | 2.287521                                                       |
| 7541 | 1.000133              | 2.287543                                                       |
| 7543 | 1.055283              | 2.287565                                                       |
| 7545 | 1.603181              | 2.287586                                                       |
| 7547 | 1.000133              | 2.287608                                                       |
| 7549 | 1.000132              | 2.287630                                                       |
| 7551 | 1.446166              | 2.287652                                                       |
| 7553 | 1.245598              | 2.287674                                                       |
| 7555 | 1.200794              | 2.287696                                                       |
| 7557 | 1.460897              | 2.287717                                                       |
| 7559 | 1.000132              | 2.287739                                                       |
| 7561 | 1.000132              | 2.287761                                                       |
| 7563 | 1.333862              | 2.287783                                                       |
| 7565 | 1.284865              | 2.287805                                                       |
| 7567 | 1.217920              | 2.287826                                                       |
| 7569 | 1.495970              | 2.287848                                                       |
| 7571 | 1.023907              | 2.287870                                                       |
| 7573 | 1.000132              | 2.287892                                                       |
| 7575 | 1.669703              | 2.287914                                                       |
| 7577 | 1.000132              | 2.287935                                                       |
| 7579 | 1.196992              | 2.287957                                                       |
| 7581 | 1.608231              | 2.287979                                                       |

| $n$  | $\frac{\sigma(n)}{n}$ | $\frac{e^\gamma}{2} \log \log n + \frac{0.73...}{\log \log n}$ |
|------|-----------------------|----------------------------------------------------------------|
| 7583 | 1.000132              | 2.288001                                                       |
| 7585 | 1.262492              | 2.288022                                                       |
| 7587 | 1.486754              | 2.288044                                                       |
| 7589 | 1.000132              | 2.288066                                                       |
| 7591 | 1.000132              | 2.288087                                                       |
| 7593 | 1.333860              | 2.288109                                                       |
| 7595 | 1.440948              | 2.288131                                                       |
| 7597 | 1.023562              | 2.288153                                                       |
| 7599 | 1.421240              | 2.288174                                                       |
| 7601 | 1.092488              | 2.288196                                                       |
| 7603 | 1.000132              | 2.288218                                                       |
| 7605 | 1.876923              | 2.288239                                                       |
| 7607 | 1.000131              | 2.288261                                                       |
| 7609 | 1.143909              | 2.288283                                                       |
| 7611 | 1.387466              | 2.288304                                                       |
| 7613 | 1.046631              | 2.288326                                                       |
| 7615 | 1.200788              | 2.288348                                                       |
| 7617 | 1.333858              | 2.288369                                                       |
| 7619 | 1.055257              | 2.288391                                                       |
| 7621 | 1.000131              | 2.288412                                                       |
| 7623 | 1.814509              | 2.288434                                                       |
| 7625 | 1.268459              | 2.288456                                                       |
| 7627 | 1.038416              | 2.288477                                                       |
| 7629 | 1.333858              | 2.288499                                                       |
| 7631 | 1.078758              | 2.288520                                                       |
| 7633 | 1.061182              | 2.288542                                                       |
| 7635 | 1.603143              | 2.288564                                                       |
| 7637 | 1.143905              | 2.288585                                                       |
| 7639 | 1.000131              | 2.288607                                                       |
| 7641 | 1.486716              | 2.288628                                                       |
| 7643 | 1.000131              | 2.288650                                                       |
| 7645 | 1.318509              | 2.288671                                                       |
| 7647 | 1.333856              | 2.288693                                                       |
| 7649 | 1.000131              | 2.288714                                                       |
| 7651 | 1.143903              | 2.288736                                                       |
| 7653 | 1.333856              | 2.288757                                                       |
| 7655 | 1.200784              | 2.288779                                                       |
| 7657 | 1.170171              | 2.288801                                                       |
| 7659 | 1.547983              | 2.288822                                                       |
| 7661 | 1.027542              | 2.288844                                                       |
| 7663 | 1.023098              | 2.288865                                                       |
| 7665 | 1.853620              | 2.288886                                                       |
| 7667 | 1.183253              | 2.288908                                                       |
| 7669 | 1.000130              | 2.288929                                                       |

| $n$  | $\frac{\sigma(n)}{n}$ | $\frac{e^\gamma}{2} \log \log n + \frac{0.73...}{\log \log n}$ |
|------|-----------------------|----------------------------------------------------------------|
| 7671 | 1.333855              | 2.288951                                                       |
| 7673 | 1.000130              | 2.288972                                                       |
| 7675 | 1.244039              | 2.288994                                                       |
| 7677 | 1.446138              | 2.289015                                                       |
| 7679 | 1.143899              | 2.289037                                                       |
| 7681 | 1.000130              | 2.289058                                                       |
| 7683 | 1.443186              | 2.289080                                                       |
| 7685 | 1.264802              | 2.289101                                                       |
| 7687 | 1.000130              | 2.289122                                                       |
| 7689 | 1.460788              | 2.289144                                                       |
| 7691 | 1.000130              | 2.289165                                                       |
| 7693 | 1.170675              | 2.289187                                                       |
| 7695 | 1.886940              | 2.289208                                                       |
| 7697 | 1.028972              | 2.289229                                                       |
| 7699 | 1.000130              | 2.289251                                                       |
| 7701 | 1.421114              | 2.289272                                                       |
| 7703 | 1.000130              | 2.289294                                                       |
| 7705 | 1.270863              | 2.289315                                                       |
| 7707 | 1.527962              | 2.289336                                                       |
| 7709 | 1.078739              | 2.289358                                                       |
| 7711 | 1.092465              | 2.289379                                                       |
| 7713 | 1.446130              | 2.289400                                                       |
| 7715 | 1.200778              | 2.289422                                                       |
| 7717 | 1.000130              | 2.289443                                                       |
| 7719 | 1.392927              | 2.289464                                                       |
| 7721 | 1.143893              | 2.289486                                                       |
| 7723 | 1.000129              | 2.289507                                                       |
| 7725 | 1.669385              | 2.289528                                                       |
| 7727 | 1.000129              | 2.289550                                                       |
| 7729 | 1.024712              | 2.289571                                                       |
| 7731 | 1.446126              | 2.289592                                                       |
| 7733 | 1.179361              | 2.289613                                                       |
| 7735 | 1.563801              | 2.289635                                                       |
| 7737 | 1.333850              | 2.289656                                                       |
| 7739 | 1.023388              | 2.289677                                                       |
| 7741 | 1.000129              | 2.289698                                                       |
| 7743 | 1.394808              | 2.289720                                                       |
| 7745 | 1.200775              | 2.289741                                                       |
| 7747 | 1.024397              | 2.289762                                                       |
| 7749 | 1.734417              | 2.289783                                                       |
| 7751 | 1.046575              | 2.289805                                                       |
| 7753 | 1.000129              | 2.289826                                                       |
| 7755 | 1.782592              | 2.289847                                                       |
| 7757 | 1.000129              | 2.289868                                                       |

| $n$  | $\frac{\sigma(n)}{n}$ | $\frac{e^\gamma}{2} \log \log n + \frac{0.73...}{\log \log n}$ |
|------|-----------------------|----------------------------------------------------------------|
| 7759 | 1.000129              | 2.289889                                                       |
| 7761 | 1.443113              | 2.289911                                                       |
| 7763 | 1.143888              | 2.289932                                                       |
| 7765 | 1.200773              | 2.289953                                                       |
| 7767 | 1.446118              | 2.289974                                                       |
| 7769 | 1.061140              | 2.289995                                                       |
| 7771 | 1.055205              | 2.290017                                                       |
| 7773 | 1.333848              | 2.290038                                                       |
| 7775 | 1.243987              | 2.290059                                                       |
| 7777 | 1.259097              | 2.290080                                                       |
| 7779 | 1.333848              | 2.290101                                                       |
| 7781 | 1.036371              | 2.290122                                                       |
| 7783 | 1.028909              | 2.290143                                                       |
| 7785 | 1.743353              | 2.290165                                                       |
| 7787 | 1.078721              | 2.290186                                                       |
| 7789 | 1.000128              | 2.290207                                                       |
| 7791 | 1.580285              | 2.290228                                                       |
| 7793 | 1.000128              | 2.290249                                                       |
| 7795 | 1.200770              | 2.290270                                                       |
| 7797 | 1.403617              | 2.290291                                                       |
| 7799 | 1.092448              | 2.290312                                                       |
| 7801 | 1.038328              | 2.290333                                                       |
| 7803 | 1.573754              | 2.290354                                                       |
| 7805 | 1.377578              | 2.290375                                                       |
| 7807 | 1.031894              | 2.290397                                                       |
| 7809 | 1.413753              | 2.290418                                                       |
| 7811 | 1.023172              | 2.290439                                                       |
| 7813 | 1.078715              | 2.290460                                                       |
| 7815 | 1.603071              | 2.290481                                                       |
| 7817 | 1.000128              | 2.290502                                                       |
| 7819 | 1.143880              | 2.290523                                                       |
| 7821 | 1.595704              | 2.290544                                                       |
| 7823 | 1.000128              | 2.290565                                                       |
| 7825 | 1.243962              | 2.290586                                                       |
| 7827 | 1.333844              | 2.290607                                                       |
| 7829 | 1.000128              | 2.290628                                                       |
| 7831 | 1.029754              | 2.290649                                                       |
| 7833 | 1.527895              | 2.290670                                                       |
| 7835 | 1.200766              | 2.290691                                                       |
| 7837 | 1.061120              | 2.290712                                                       |
| 7839 | 1.578773              | 2.290733                                                       |
| 7841 | 1.000128              | 2.290754                                                       |
| 7843 | 1.175061              | 2.290775                                                       |
| 7845 | 1.603059              | 2.290796                                                       |

| $n$  | $\frac{\sigma(n)}{n}$ | $\frac{e^\gamma}{2} \log \log n + \frac{0.73...}{\log \log n}$ |
|------|-----------------------|----------------------------------------------------------------|
| 7847 | 1.223397              | 2.290817                                                       |
| 7849 | 1.027392              | 2.290837                                                       |
| 7851 | 1.333843              | 2.290858                                                       |
| 7853 | 1.000127              | 2.290879                                                       |
| 7855 | 1.200764              | 2.290900                                                       |
| 7857 | 1.509227              | 2.290921                                                       |
| 7859 | 1.038300              | 2.290942                                                       |
| 7861 | 1.143875              | 2.290963                                                       |
| 7863 | 1.333842              | 2.290984                                                       |
| 7865 | 1.420470              | 2.291005                                                       |
| 7867 | 1.000127              | 2.291026                                                       |
| 7869 | 1.386707              | 2.291046                                                       |
| 7871 | 1.061110              | 2.291067                                                       |
| 7873 | 1.000127              | 2.291088                                                       |
| 7875 | 2.060190              | 2.291109                                                       |
| 7877 | 1.000127              | 2.291130                                                       |
| 7879 | 1.000127              | 2.291151                                                       |
| 7881 | 1.388656              | 2.291172                                                       |
| 7883 | 1.000127              | 2.291192                                                       |
| 7885 | 1.278377              | 2.291213                                                       |
| 7887 | 1.460631              | 2.291234                                                       |
| 7889 | 1.216884              | 2.291255                                                       |
| 7891 | 1.078697              | 2.291276                                                       |
| 7893 | 1.446091              | 2.291297                                                       |
| 7895 | 1.200760              | 2.291317                                                       |
| 7897 | 1.025706              | 2.291338                                                       |
| 7899 | 1.333840              | 2.291359                                                       |
| 7901 | 1.000127              | 2.291380                                                       |
| 7903 | 1.143869              | 2.291401                                                       |
| 7905 | 1.748767              | 2.291421                                                       |
| 7907 | 1.000126              | 2.291442                                                       |
| 7909 | 1.092426              | 2.291463                                                       |
| 7911 | 1.486538              | 2.291484                                                       |
| 7913 | 1.029698              | 2.291504                                                       |
| 7915 | 1.200758              | 2.291525                                                       |
| 7917 | 1.697613              | 2.291546                                                       |
| 7919 | 1.000126              | 2.291567                                                       |
| 7921 | 1.011362              | 2.291587                                                       |
| 7923 | 1.413606              | 2.291608                                                       |
| 7925 | 1.243912              | 2.291629                                                       |
| 7927 | 1.000126              | 2.291649                                                       |
| 7929 | 1.446084              | 2.291670                                                       |
| 7931 | 1.258858              | 2.291691                                                       |
| 7933 | 1.000126              | 2.291712                                                       |



| $n$  | $\frac{\sigma(n)}{n}$ | $\frac{e^\gamma}{2} \log \log n + \frac{0.73\dots}{\log \log n}$ |
|------|-----------------------|------------------------------------------------------------------|
| 7935 | 1.672590              | 2.291732                                                         |
| 7937 | 1.000126              | 2.291753                                                         |
| 7939 | 1.061091              | 2.291774                                                         |
| 7941 | 1.333837              | 2.291794                                                         |
| 7943 | 1.105879              | 2.291815                                                         |
| 7945 | 1.377470              | 2.291836                                                         |
| 7947 | 1.446080              | 2.291856                                                         |
| 7949 | 1.000126              | 2.291877                                                         |
| 7951 | 1.000126              | 2.291898                                                         |
| 7953 | 1.460581              | 2.291918                                                         |
| 7955 | 1.261094              | 2.291939                                                         |
| 7957 | 1.022999              | 2.291959                                                         |
| 7959 | 1.527830              | 2.291980                                                         |
| 7961 | 1.055144              | 2.292001                                                         |
| 7963 | 1.000126              | 2.292021                                                         |
| 7965 | 1.807910              | 2.292042                                                         |
| 7967 | 1.036275              | 2.292063                                                         |
| 7969 | 1.078680              | 2.292083                                                         |
| 7971 | 1.333835              | 2.292104                                                         |
| 7973 | 1.228145              | 2.292124                                                         |
| 7975 | 1.399373              | 2.292145                                                         |
| 7977 | 1.333835              | 2.292165                                                         |
| 7979 | 1.022685              | 2.292186                                                         |
| 7981 | 1.046485              | 2.292207                                                         |
| 7983 | 1.446073              | 2.292227                                                         |
| 7985 | 1.200751              | 2.292248                                                         |
| 7987 | 1.170402              | 2.292268                                                         |
| 7989 | 1.333834              | 2.292289                                                         |
| 7991 | 1.024152              | 2.292309                                                         |
| 7993 | 1.000125              | 2.292330                                                         |
| 7995 | 1.765103              | 2.292350                                                         |
| 7997 | 1.092410              | 2.292371                                                         |
| 7999 | 1.055132              | 2.292391                                                         |
| 8001 | 1.663792              | 2.292412                                                         |
| 8003 | 1.025615              | 2.292432                                                         |
| 8005 | 1.200750              | 2.292453                                                         |
| 8007 | 1.420757              | 2.292473                                                         |
| 8009 | 1.000125              | 2.292494                                                         |
| 8011 | 1.000125              | 2.292514                                                         |
| 8013 | 1.333833              | 2.292535                                                         |
| 8015 | 1.377417              | 2.292555                                                         |
| 8017 | 1.000125              | 2.292576                                                         |
| 8019 | 1.635615              | 2.292596                                                         |
| 8021 | 1.078668              | 2.292617                                                         |

| $n$  | $\frac{\sigma(n)}{n}$ | $\frac{e^\gamma}{2} \log \log n + \frac{0.73...}{\log \log n}$ |
|------|-----------------------|----------------------------------------------------------------|
| 8023 | 1.023059              | 2.292637                                                       |
| 8025 | 1.668785              | 2.292657                                                       |
| 8027 | 1.046468              | 2.292678                                                       |
| 8029 | 1.211608              | 2.292698                                                       |
| 8031 | 1.333831              | 2.292719                                                       |
| 8033 | 1.038217              | 2.292739                                                       |
| 8035 | 1.200747              | 2.292760                                                       |
| 8037 | 1.552818              | 2.292780                                                       |
| 8039 | 1.000124              | 2.292800                                                       |
| 8041 | 1.181943              | 2.292821                                                       |
| 8043 | 1.527788              | 2.292841                                                       |
| 8045 | 1.200746              | 2.292862                                                       |
| 8047 | 1.078663              | 2.292882                                                       |
| 8049 | 1.333830              | 2.292902                                                       |
| 8051 | 1.022482              | 2.292923                                                       |
| 8053 | 1.000124              | 2.292943                                                       |
| 8055 | 1.743017              | 2.292963                                                       |
| 8057 | 1.143850              | 2.292984                                                       |
| 8059 | 1.000124              | 2.293004                                                       |
| 8061 | 1.333830              | 2.293024                                                       |
| 8063 | 1.092397              | 2.293045                                                       |
| 8065 | 1.200744              | 2.293065                                                       |
| 8067 | 1.333829              | 2.293085                                                       |
| 8069 | 1.000124              | 2.293106                                                       |
| 8071 | 1.143848              | 2.293126                                                       |
| 8073 | 1.664809              | 2.293146                                                       |
| 8075 | 1.382043              | 2.293167                                                       |
| 8077 | 1.029590              | 2.293187                                                       |
| 8079 | 1.333828              | 2.293207                                                       |
| 8081 | 1.000124              | 2.293227                                                       |
| 8083 | 1.024372              | 2.293248                                                       |
| 8085 | 2.030427              | 2.293268                                                       |
| 8087 | 1.000124              | 2.293288                                                       |
| 8089 | 1.000124              | 2.293309                                                       |
| 8091 | 1.542455              | 2.293329                                                       |
| 8093 | 1.000124              | 2.293349                                                       |
| 8095 | 1.200741              | 2.293369                                                       |
| 8097 | 1.333827              | 2.293390                                                       |
| 8099 | 1.244598              | 2.293410                                                       |
| 8101 | 1.000123              | 2.293430                                                       |
| 8103 | 1.388128              | 2.293450                                                       |
| 8105 | 1.200740              | 2.293470                                                       |
| 8107 | 1.115579              | 2.293491                                                       |
| 8109 | 1.558269              | 2.293511                                                       |

| $n$  | $\frac{\sigma(n)}{n}$ | $\frac{e^\gamma}{2} \log \log n + \frac{0.73...}{\log \log n}$ |
|------|-----------------------|----------------------------------------------------------------|
| 8111 | 1.000123              | 2.293531                                                       |
| 8113 | 1.222729              | 2.293551                                                       |
| 8115 | 1.602957              | 2.293571                                                       |
| 8117 | 1.000123              | 2.293592                                                       |
| 8119 | 1.046434              | 2.293612                                                       |
| 8121 | 1.333826              | 2.293632                                                       |
| 8123 | 1.000123              | 2.293652                                                       |
| 8125 | 1.345723              | 2.293672                                                       |
| 8127 | 1.732497              | 2.293692                                                       |
| 8129 | 1.092385              | 2.293713                                                       |
| 8131 | 1.027180              | 2.293733                                                       |
| 8133 | 1.333825              | 2.293753                                                       |
| 8135 | 1.200738              | 2.293773                                                       |
| 8137 | 1.022490              | 2.293793                                                       |
| 8139 | 1.333825              | 2.293813                                                       |
| 8141 | 1.143840              | 2.293833                                                       |
| 8143 | 1.061034              | 2.293854                                                       |
| 8145 | 1.742910              | 2.293874                                                       |
| 8147 | 1.000123              | 2.293894                                                       |
| 8149 | 1.038164              | 2.293914                                                       |
| 8151 | 1.648877              | 2.293934                                                       |
| 8153 | 1.036183              | 2.293954                                                       |
| 8155 | 1.377315              | 2.293974                                                       |
| 8157 | 1.333824              | 2.293994                                                       |
| 8159 | 1.029538              | 2.294014                                                       |
| 8161 | 1.000123              | 2.294034                                                       |
| 8163 | 1.446037              | 2.294054                                                       |
| 8165 | 1.269810              | 2.294074                                                       |
| 8167 | 1.000122              | 2.294094                                                       |
| 8169 | 1.527727              | 2.294115                                                       |
| 8171 | 1.000122              | 2.294135                                                       |
| 8173 | 1.092377              | 2.294155                                                       |
| 8175 | 1.668502              | 2.294175                                                       |
| 8177 | 1.171090              | 2.294195                                                       |
| 8179 | 1.000122              | 2.294215                                                       |
| 8181 | 1.508618              | 2.294235                                                       |
| 8183 | 1.170231              | 2.294255                                                       |
| 8185 | 1.200733              | 2.294275                                                       |
| 8187 | 1.333822              | 2.294295                                                       |
| 8189 | 1.055074              | 2.294315                                                       |
| 8191 | 1.000122              | 2.294335                                                       |
| 8193 | 1.333822              | 2.294355                                                       |
| 8195 | 1.317877              | 2.294375                                                       |
| 8197 | 1.143833              | 2.294395                                                       |

| $n$  | $\frac{\sigma(n)}{n}$ | $\frac{e^\gamma}{2} \log \log n + \frac{0.73...}{\log \log n}$ |
|------|-----------------------|----------------------------------------------------------------|
| 8199 | 1.446030              | 2.294415                                                       |
| 8201 | 1.024265              | 2.294434                                                       |
| 8203 | 1.078630              | 2.294454                                                       |
| 8205 | 1.602925              | 2.294474                                                       |
| 8207 | 1.038138              | 2.294494                                                       |
| 8209 | 1.000122              | 2.294514                                                       |
| 8211 | 1.683595              | 2.294534                                                       |
| 8213 | 1.028613              | 2.294554                                                       |
| 8215 | 1.262082              | 2.294574                                                       |
| 8217 | 1.594743              | 2.294594                                                       |
| 8219 | 1.000122              | 2.294614                                                       |
| 8221 | 1.000122              | 2.294634                                                       |
| 8223 | 1.333820              | 2.294654                                                       |
| 8225 | 1.447295              | 2.294674                                                       |
| 8227 | 1.055063              | 2.294693                                                       |
| 8229 | 1.442703              | 2.294713                                                       |
| 8231 | 1.000121              | 2.294733                                                       |
| 8233 | 1.000121              | 2.294753                                                       |
| 8235 | 1.806922              | 2.294773                                                       |
| 8237 | 1.000121              | 2.294793                                                       |
| 8239 | 1.258405              | 2.294813                                                       |
| 8241 | 1.386240              | 2.294833                                                       |
| 8243 | 1.000121              | 2.294852                                                       |
| 8245 | 1.283687              | 2.294872                                                       |
| 8247 | 1.333818              | 2.294892                                                       |
| 8249 | 1.022669              | 2.294912                                                       |
| 8251 | 1.031633              | 2.294932                                                       |
| 8253 | 1.663395              | 2.294952                                                       |
| 8255 | 1.302483              | 2.294971                                                       |
| 8257 | 1.046385              | 2.294991                                                       |
| 8259 | 1.333818              | 2.295011                                                       |
| 8261 | 1.092362              | 2.295031                                                       |
| 8263 | 1.000121              | 2.295051                                                       |
| 8265 | 1.742287              | 2.295070                                                       |
| 8267 | 1.143825              | 2.295090                                                       |
| 8269 | 1.000121              | 2.295110                                                       |
| 8271 | 1.446016              | 2.295130                                                       |
| 8273 | 1.000121              | 2.295149                                                       |
| 8275 | 1.243746              | 2.295169                                                       |
| 8277 | 1.391809              | 2.295189                                                       |
| 8279 | 1.060998              | 2.295209                                                       |
| 8281 | 1.259630              | 2.295229                                                       |
| 8283 | 1.460340              | 2.295248                                                       |
| 8285 | 1.200724              | 2.295268                                                       |

| $n$  | $\frac{\sigma(n)}{n}$ | $\frac{e^\gamma}{2} \log \log n + \frac{0.73...}{\log \log n}$ |
|------|-----------------------|----------------------------------------------------------------|
| 8287 | 1.000121              | 2.295288                                                       |
| 8289 | 1.486307              | 2.295307                                                       |
| 8291 | 1.000121              | 2.295327                                                       |
| 8293 | 1.000121              | 2.295347                                                       |
| 8295 | 1.851718              | 2.295367                                                       |
| 8297 | 1.000121              | 2.295386                                                       |
| 8299 | 1.028558              | 2.295406                                                       |
| 8301 | 1.333815              | 2.295426                                                       |
| 8303 | 1.101289              | 2.295445                                                       |
| 8305 | 1.317760              | 2.295465                                                       |
| 8307 | 1.577465              | 2.295485                                                       |
| 8309 | 1.143820              | 2.295504                                                       |
| 8311 | 1.000120              | 2.295524                                                       |
| 8313 | 1.420426              | 2.295544                                                       |
| 8315 | 1.200722              | 2.295563                                                       |
| 8317 | 1.000120              | 2.295583                                                       |
| 8319 | 1.384782              | 2.295603                                                       |
| 8321 | 1.025358              | 2.295622                                                       |
| 8323 | 1.211102              | 2.295642                                                       |
| 8325 | 1.839520              | 2.295662                                                       |
| 8327 | 1.092350              | 2.295681                                                       |
| 8329 | 1.000120              | 2.295701                                                       |
| 8331 | 1.333813              | 2.295721                                                       |
| 8333 | 1.078603              | 2.295740                                                       |
| 8335 | 1.200720              | 2.295760                                                       |
| 8337 | 1.527648              | 2.295779                                                       |
| 8339 | 1.036095              | 2.295799                                                       |
| 8341 | 1.055029              | 2.295819                                                       |
| 8343 | 1.508330              | 2.295838                                                       |
| 8345 | 1.200719              | 2.295858                                                       |
| 8347 | 1.060980              | 2.295877                                                       |
| 8349 | 1.529285              | 2.295897                                                       |
| 8351 | 1.143815              | 2.295916                                                       |
| 8353 | 1.000120              | 2.295936                                                       |
| 8355 | 1.602873              | 2.295956                                                       |
| 8357 | 1.023812              | 2.295975                                                       |
| 8359 | 1.078598              | 2.295995                                                       |
| 8361 | 1.445999              | 2.296014                                                       |
| 8363 | 1.000120              | 2.296034                                                       |
| 8365 | 1.377167              | 2.296053                                                       |
| 8367 | 1.333811              | 2.296073                                                       |
| 8369 | 1.000119              | 2.296092                                                       |
| 8371 | 1.092343              | 2.296112                                                       |
| 8373 | 1.333811              | 2.296131                                                       |

| $n$  | $\frac{\sigma(n)}{n}$ | $\frac{e^\gamma}{2} \log \log n + \frac{0.73...}{\log \log n}$ |
|------|-----------------------|----------------------------------------------------------------|
| 8375 | 1.266627              | 2.296151                                                       |
| 8377 | 1.000119              | 2.296170                                                       |
| 8379 | 1.768707              | 2.296190                                                       |
| 8381 | 1.098914              | 2.296209                                                       |
| 8383 | 1.022068              | 2.296229                                                       |
| 8385 | 1.763148              | 2.296248                                                       |
| 8387 | 1.000119              | 2.296268                                                       |
| 8389 | 1.000119              | 2.296287                                                       |
| 8391 | 1.333810              | 2.296307                                                       |
| 8393 | 1.258191              | 2.296326                                                       |
| 8395 | 1.269327              | 2.296346                                                       |
| 8397 | 1.486245              | 2.296365                                                       |
| 8399 | 1.031551              | 2.296385                                                       |
| 8401 | 1.036067              | 2.296404                                                       |
| 8403 | 1.333809              | 2.296423                                                       |
| 8405 | 1.229982              | 2.296443                                                       |
| 8407 | 1.143809              | 2.296462                                                       |
| 8409 | 1.333809              | 2.296482                                                       |
| 8411 | 1.078588              | 2.296501                                                       |
| 8413 | 1.026982              | 2.296521                                                       |
| 8415 | 2.002139              | 2.296540                                                       |
| 8417 | 1.055008              | 2.296559                                                       |
| 8419 | 1.000119              | 2.296579                                                       |
| 8421 | 1.527610              | 2.296598                                                       |
| 8423 | 1.000119              | 2.296618                                                       |
| 8425 | 1.243680              | 2.296637                                                       |
| 8427 | 1.358965              | 2.296656                                                       |
| 8429 | 1.000119              | 2.296676                                                       |
| 8431 | 1.000119              | 2.296695                                                       |
| 8433 | 1.445986              | 2.296714                                                       |
| 8435 | 1.377119              | 2.296734                                                       |
| 8437 | 1.194737              | 2.296753                                                       |
| 8439 | 1.393530              | 2.296772                                                       |
| 8441 | 1.046322              | 2.296792                                                       |
| 8443 | 1.000118              | 2.296811                                                       |
| 8445 | 1.602842              | 2.296830                                                       |
| 8447 | 1.000118              | 2.296850                                                       |
| 8449 | 1.227127              | 2.296869                                                       |
| 8451 | 1.486215              | 2.296888                                                       |
| 8453 | 1.022122              | 2.296908                                                       |
| 8455 | 1.277351              | 2.296927                                                       |
| 8457 | 1.333806              | 2.296946                                                       |
| 8459 | 1.092328              | 2.296966                                                       |
| 8461 | 1.000118              | 2.296985                                                       |

| $n$  | $\frac{\sigma(n)}{n}$ | $\frac{e^\gamma}{2} \log \log n + \frac{0.73...}{\log \log n}$ |
|------|-----------------------|----------------------------------------------------------------|
| 8463 | 1.693962              | 2.297004                                                       |
| 8465 | 1.200709              | 2.297024                                                       |
| 8467 | 1.000118              | 2.297043                                                       |
| 8469 | 1.445979              | 2.297062                                                       |
| 8471 | 1.028450              | 2.297081                                                       |
| 8473 | 1.031512              | 2.297101                                                       |
| 8475 | 1.667965              | 2.297120                                                       |
| 8477 | 1.169989              | 2.297139                                                       |
| 8479 | 1.023706              | 2.297158                                                       |
| 8481 | 1.460205              | 2.297178                                                       |
| 8483 | 1.060945              | 2.297197                                                       |
| 8485 | 1.200707              | 2.297216                                                       |
| 8487 | 1.544008              | 2.297235                                                       |
| 8489 | 1.078572              | 2.297255                                                       |
| 8491 | 1.143799              | 2.297274                                                       |
| 8493 | 1.412928              | 2.297293                                                       |
| 8495 | 1.200706              | 2.297312                                                       |
| 8497 | 1.038013              | 2.297331                                                       |
| 8499 | 1.333804              | 2.297351                                                       |
| 8501 | 1.000118              | 2.297370                                                       |
| 8503 | 1.092320              | 2.297389                                                       |
| 8505 | 2.054321              | 2.297408                                                       |
| 8507 | 1.026919              | 2.297427                                                       |
| 8509 | 1.022917              | 2.297446                                                       |
| 8511 | 1.333803              | 2.297466                                                       |
| 8513 | 1.000117              | 2.297485                                                       |
| 8515 | 1.302173              | 2.297504                                                       |
| 8517 | 1.420218              | 2.297523                                                       |
| 8519 | 1.143796              | 2.297542                                                       |
| 8521 | 1.000117              | 2.297561                                                       |
| 8523 | 1.445970              | 2.297581                                                       |
| 8525 | 1.396364              | 2.297600                                                       |
| 8527 | 1.000117              | 2.297619                                                       |
| 8529 | 1.333802              | 2.297638                                                       |
| 8531 | 1.054976              | 2.297657                                                       |
| 8533 | 1.215047              | 2.297676                                                       |
| 8535 | 1.602812              | 2.297695                                                       |
| 8537 | 1.000117              | 2.297714                                                       |
| 8539 | 1.000117              | 2.297733                                                       |
| 8541 | 1.576865              | 2.297753                                                       |
| 8543 | 1.000117              | 2.297772                                                       |
| 8545 | 1.200702              | 2.297791                                                       |
| 8547 | 1.707266              | 2.297810                                                       |
| 8549 | 1.021874              | 2.297829                                                       |

| $n$  | $\frac{\sigma(n)}{n}$ | $\frac{e^\gamma}{2} \log \log n + \frac{0.73...}{\log \log n}$ |
|------|-----------------------|----------------------------------------------------------------|
| 8551 | 1.060929              | 2.297848                                                       |
| 8553 | 1.333801              | 2.297867                                                       |
| 8555 | 1.262420              | 2.297886                                                       |
| 8557 | 1.028398              | 2.297905                                                       |
| 8559 | 1.486155              | 2.297924                                                       |
| 8561 | 1.143792              | 2.297943                                                       |
| 8563 | 1.000117              | 2.297962                                                       |
| 8565 | 1.602802              | 2.297981                                                       |
| 8567 | 1.078557              | 2.298000                                                       |
| 8569 | 1.176333              | 2.298019                                                       |
| 8571 | 1.333800              | 2.298038                                                       |
| 8573 | 1.000117              | 2.298057                                                       |
| 8575 | 1.446064              | 2.298076                                                       |
| 8577 | 1.445960              | 2.298095                                                       |
| 8579 | 1.046276              | 2.298114                                                       |
| 8581 | 1.000117              | 2.298133                                                       |
| 8583 | 1.333799              | 2.298152                                                       |
| 8585 | 1.283168              | 2.298171                                                       |
| 8587 | 1.035985              | 2.298190                                                       |
| 8589 | 1.527535              | 2.298209                                                       |
| 8591 | 1.114655              | 2.298228                                                       |
| 8593 | 1.078552              | 2.298247                                                       |
| 8595 | 1.742408              | 2.298266                                                       |
| 8597 | 1.000116              | 2.298285                                                       |
| 8599 | 1.000116              | 2.298304                                                       |
| 8601 | 1.384025              | 2.298323                                                       |
| 8603 | 1.143787              | 2.298342                                                       |
| 8605 | 1.200697              | 2.298361                                                       |
| 8607 | 1.412804              | 2.298380                                                       |
| 8609 | 1.000116              | 2.298399                                                       |
| 8611 | 1.021949              | 2.298418                                                       |
| 8613 | 1.671891              | 2.298437                                                       |
| 8615 | 1.200696              | 2.298456                                                       |
| 8617 | 1.143786              | 2.298475                                                       |
| 8619 | 1.528716              | 2.298493                                                       |
| 8621 | 1.031435              | 2.298512                                                       |
| 8623 | 1.000116              | 2.298531                                                       |
| 8625 | 1.736348              | 2.298550                                                       |
| 8627 | 1.000116              | 2.298569                                                       |
| 8629 | 1.000116              | 2.298588                                                       |
| 8631 | 1.662843              | 2.298607                                                       |
| 8633 | 1.021661              | 2.298626                                                       |
| 8635 | 1.317429              | 2.298645                                                       |
| 8637 | 1.333796              | 2.298663                                                       |



| $n$  | $\frac{\sigma(n)}{n}$ | $\frac{e^\gamma}{2} \log \log n + \frac{0.73...}{\log \log n}$ |
|------|-----------------------|----------------------------------------------------------------|
| 8639 | 1.025119              | 2.298682                                                       |
| 8641 | 1.000116              | 2.298701                                                       |
| 8643 | 1.384704              | 2.298720                                                       |
| 8645 | 1.554656              | 2.298739                                                       |
| 8647 | 1.000116              | 2.298758                                                       |
| 8649 | 1.492542              | 2.298777                                                       |
| 8651 | 1.029245              | 2.298795                                                       |
| 8653 | 1.060904              | 2.298814                                                       |
| 8655 | 1.602773              | 2.298833                                                       |
| 8657 | 1.092295              | 2.298852                                                       |
| 8659 | 1.143781              | 2.298871                                                       |
| 8661 | 1.333795              | 2.298889                                                       |
| 8663 | 1.000115              | 2.298908                                                       |
| 8665 | 1.200692              | 2.298927                                                       |
| 8667 | 1.507788              | 2.298946                                                       |
| 8669 | 1.000115              | 2.298965                                                       |
| 8671 | 1.162496              | 2.298983                                                       |
| 8673 | 1.577309              | 2.299002                                                       |
| 8675 | 1.243573              | 2.299021                                                       |
| 8677 | 1.000115              | 2.299040                                                       |
| 8679 | 1.460076              | 2.299058                                                       |
| 8681 | 1.000115              | 2.299077                                                       |
| 8683 | 1.054935              | 2.299096                                                       |
| 8685 | 1.742314              | 2.299115                                                       |
| 8687 | 1.226661              | 2.299133                                                       |
| 8689 | 1.000115              | 2.299152                                                       |
| 8691 | 1.333794              | 2.299171                                                       |
| 8693 | 1.000115              | 2.299190                                                       |
| 8695 | 1.258654              | 2.299208                                                       |
| 8697 | 1.442336              | 2.299227                                                       |
| 8699 | 1.000115              | 2.299246                                                       |
| 8701 | 1.257786              | 2.299265                                                       |
| 8703 | 1.445938              | 2.299283                                                       |
| 8705 | 1.200689              | 2.299302                                                       |
| 8707 | 1.000115              | 2.299321                                                       |
| 8709 | 1.333793              | 2.299339                                                       |
| 8711 | 1.035932              | 2.299358                                                       |
| 8713 | 1.000115              | 2.299377                                                       |
| 8715 | 1.850602              | 2.299395                                                       |
| 8717 | 1.046232              | 2.299414                                                       |
| 8719 | 1.000115              | 2.299433                                                       |
| 8721 | 1.651187              | 2.299451                                                       |
| 8723 | 1.194085              | 2.299470                                                       |
| 8725 | 1.243553              | 2.299489                                                       |

| $n$  | $\frac{\sigma(n)}{n}$ | $\frac{e^\gamma}{2} \log \log n + \frac{0.73...}{\log \log n}$ |
|------|-----------------------|----------------------------------------------------------------|
| 8727 | 1.333792              | 2.299507                                                       |
| 8729 | 1.209761              | 2.299526                                                       |
| 8731 | 1.000115              | 2.299545                                                       |
| 8733 | 1.385091              | 2.299563                                                       |
| 8735 | 1.200687              | 2.299582                                                       |
| 8737 | 1.000114              | 2.299601                                                       |
| 8739 | 1.445932              | 2.299619                                                       |
| 8741 | 1.000114              | 2.299638                                                       |
| 8743 | 1.143772              | 2.299656                                                       |
| 8745 | 1.778388              | 2.299675                                                       |
| 8747 | 1.000114              | 2.299694                                                       |
| 8749 | 1.078523              | 2.299712                                                       |
| 8751 | 1.333790              | 2.299731                                                       |
| 8753 | 1.000114              | 2.299749                                                       |
| 8755 | 1.282924              | 2.299768                                                       |
| 8757 | 1.662670              | 2.299787                                                       |
| 8759 | 1.054915              | 2.299805                                                       |
| 8761 | 1.000114              | 2.299824                                                       |
| 8763 | 1.402260              | 2.299842                                                       |
| 8765 | 1.200685              | 2.299861                                                       |
| 8767 | 1.092278              | 2.299879                                                       |
| 8769 | 1.386703              | 2.299898                                                       |
| 8771 | 1.169764              | 2.299917                                                       |
| 8773 | 1.035906              | 2.299935                                                       |
| 8775 | 1.978348              | 2.299954                                                       |
| 8777 | 1.022673              | 2.299972                                                       |
| 8779 | 1.000114              | 2.299991                                                       |
| 8781 | 1.333789              | 2.300009                                                       |
| 8783 | 1.000114              | 2.300028                                                       |
| 8785 | 1.376892              | 2.300046                                                       |
| 8787 | 1.392967              | 2.300065                                                       |
| 8789 | 1.179656              | 2.300083                                                       |
| 8791 | 1.023774              | 2.300102                                                       |
| 8793 | 1.445923              | 2.300120                                                       |
| 8795 | 1.200682              | 2.300139                                                       |
| 8797 | 1.054905              | 2.300157                                                       |
| 8799 | 1.527446              | 2.300176                                                       |
| 8801 | 1.078514              | 2.300194                                                       |
| 8803 | 1.000114              | 2.300213                                                       |
| 8805 | 1.602726              | 2.300231                                                       |
| 8807 | 1.000114              | 2.300250                                                       |
| 8809 | 1.046203              | 2.300268                                                       |
| 8811 | 1.593463              | 2.300287                                                       |
| 8813 | 1.143765              | 2.300305                                                       |

| $n$  | $\frac{\sigma(n)}{n}$ | $\frac{e^\gamma}{2} \log \log n + \frac{0.73\dots}{\log \log n}$ |
|------|-----------------------|------------------------------------------------------------------|
| 8815 | 1.257856              | 2.300323                                                         |
| 8817 | 1.333787              | 2.300342                                                         |
| 8819 | 1.000113              | 2.300360                                                         |
| 8821 | 1.000113              | 2.300379                                                         |
| 8823 | 1.419925              | 2.300397                                                         |
| 8825 | 1.243513              | 2.300416                                                         |
| 8827 | 1.243458              | 2.300434                                                         |
| 8829 | 1.507532              | 2.300452                                                         |
| 8831 | 1.000113              | 2.300471                                                         |
| 8833 | 1.114231              | 2.300489                                                         |
| 8835 | 1.738540              | 2.300508                                                         |
| 8837 | 1.000113              | 2.300526                                                         |
| 8839 | 1.000113              | 2.300544                                                         |
| 8841 | 1.527429              | 2.300563                                                         |
| 8843 | 1.031324              | 2.300581                                                         |
| 8845 | 1.261730              | 2.300600                                                         |
| 8847 | 1.445914              | 2.300618                                                         |
| 8849 | 1.000113              | 2.300636                                                         |
| 8851 | 1.024969              | 2.300655                                                         |
| 8853 | 1.442223              | 2.300673                                                         |
| 8855 | 1.561152              | 2.300691                                                         |
| 8857 | 1.060856              | 2.300710                                                         |
| 8859 | 1.333785              | 2.300728                                                         |
| 8861 | 1.000113              | 2.300747                                                         |
| 8863 | 1.000113              | 2.300765                                                         |
| 8865 | 1.742132              | 2.300783                                                         |
| 8867 | 1.000113              | 2.300802                                                         |
| 8869 | 1.169692              | 2.300820                                                         |
| 8871 | 1.333784              | 2.300838                                                         |
| 8873 | 1.054886              | 2.300857                                                         |
| 8875 | 1.265577              | 2.300875                                                         |
| 8877 | 1.459953              | 2.300893                                                         |
| 8879 | 1.078500              | 2.300911                                                         |
| 8881 | 1.021507              | 2.300930                                                         |
| 8883 | 1.729146              | 2.300948                                                         |
| 8885 | 1.200675              | 2.300966                                                         |
| 8887 | 1.000113              | 2.300985                                                         |
| 8889 | 1.333783              | 2.301003                                                         |
| 8891 | 1.060848              | 2.301021                                                         |
| 8893 | 1.000112              | 2.301039                                                         |
| 8895 | 1.602698              | 2.301058                                                         |
| 8897 | 1.208497              | 2.301076                                                         |
| 8899 | 1.092258              | 2.301094                                                         |
| 8901 | 1.542299              | 2.301112                                                         |

| $n$  | $\frac{\sigma(n)}{n}$ | $\frac{e^\gamma}{2} \log \log n + \frac{0.73...}{\log \log n}$ |
|------|-----------------------|----------------------------------------------------------------|
| 8903 | 1.037852              | 2.301131                                                       |
| 8905 | 1.301741              | 2.301149                                                       |
| 8907 | 1.333782              | 2.301167                                                       |
| 8909 | 1.023684              | 2.301185                                                       |
| 8911 | 1.220963              | 2.301204                                                       |
| 8913 | 1.333782              | 2.301222                                                       |
| 8915 | 1.200673              | 2.301240                                                       |
| 8917 | 1.031289              | 2.301258                                                       |
| 8919 | 1.445902              | 2.301277                                                       |
| 8921 | 1.092254              | 2.301295                                                       |
| 8923 | 1.000112              | 2.301313                                                       |
| 8925 | 2.000672              | 2.301331                                                       |
| 8927 | 1.021620              | 2.301349                                                       |
| 8929 | 1.000112              | 2.301368                                                       |
| 8931 | 1.442168              | 2.301386                                                       |
| 8933 | 1.000112              | 2.301404                                                       |
| 8935 | 1.200672              | 2.301422                                                       |
| 8937 | 1.485957              | 2.301440                                                       |
| 8939 | 1.143752              | 2.301458                                                       |
| 8941 | 1.000112              | 2.301477                                                       |
| 8943 | 1.459913              | 2.301495                                                       |
| 8945 | 1.200671              | 2.301513                                                       |
| 8947 | 1.046161              | 2.301531                                                       |
| 8949 | 1.412448              | 2.301549                                                       |
| 8951 | 1.000112              | 2.301567                                                       |
| 8953 | 1.143751              | 2.301586                                                       |
| 8955 | 1.742044              | 2.301604                                                       |
| 8957 | 1.103271              | 2.301622                                                       |
| 8959 | 1.096551              | 2.301640                                                       |
| 8961 | 1.392702              | 2.301658                                                       |
| 8963 | 1.000112              | 2.301676                                                       |
| 8965 | 1.317122              | 2.301694                                                       |
| 8967 | 1.576447              | 2.301712                                                       |
| 8969 | 1.000111              | 2.301730                                                       |
| 8971 | 1.000111              | 2.301749                                                       |
| 8973 | 1.445893              | 2.301767                                                       |
| 8975 | 1.243454              | 2.301785                                                       |
| 8977 | 1.026624              | 2.301803                                                       |
| 8979 | 1.384564              | 2.301821                                                       |
| 8981 | 1.143748              | 2.301839                                                       |
| 8983 | 1.078482              | 2.301857                                                       |
| 8985 | 1.602671              | 2.301875                                                       |
| 8987 | 1.175031              | 2.301893                                                       |
| 8989 | 1.021248              | 2.301911                                                       |

| $n$  | $\frac{\sigma(n)}{n}$ | $\frac{e^\gamma}{2} \log \log n + \frac{0.73\dots}{\log \log n}$ |
|------|-----------------------|------------------------------------------------------------------|
| 8991 | 1.538427              | 2.301929                                                         |
| 8993 | 1.106861              | 2.301947                                                         |
| 8995 | 1.376765              | 2.301965                                                         |
| 8997 | 1.333778              | 2.301983                                                         |
| 8999 | 1.000111              | 2.302002                                                         |
| 9001 | 1.000111              | 2.302020                                                         |
| 9003 | 1.333778              | 2.302038                                                         |
| 9005 | 1.200666              | 2.302056                                                         |
| 9007 | 1.000111              | 2.302074                                                         |
| 9009 | 1.939394              | 2.302092                                                         |
| 9011 | 1.000111              | 2.302110                                                         |
| 9013 | 1.000111              | 2.302128                                                         |
| 9015 | 1.602662              | 2.302146                                                         |
| 9017 | 1.022069              | 2.302164                                                         |
| 9019 | 1.037809              | 2.302182                                                         |
| 9021 | 1.390533              | 2.302200                                                         |
| 9023 | 1.143744              | 2.302218                                                         |
| 9025 | 1.308698              | 2.302236                                                         |
| 9027 | 1.555334              | 2.302254                                                         |
| 9029 | 1.000111              | 2.302272                                                         |
| 9031 | 1.092238              | 2.302290                                                         |
| 9033 | 1.333776              | 2.302307                                                         |
| 9035 | 1.301605              | 2.302325                                                         |
| 9037 | 1.143742              | 2.302343                                                         |
| 9039 | 1.401925              | 2.302361                                                         |
| 9041 | 1.000111              | 2.302379                                                         |
| 9043 | 1.000111              | 2.302397                                                         |
| 9045 | 1.804312              | 2.302415                                                         |
| 9047 | 1.021333              | 2.302433                                                         |
| 9049 | 1.000111              | 2.302451                                                         |
| 9051 | 1.527345              | 2.302469                                                         |
| 9053 | 1.092235              | 2.302487                                                         |
| 9055 | 1.200663              | 2.302505                                                         |
| 9057 | 1.333775              | 2.302523                                                         |
| 9059 | 1.000110              | 2.302541                                                         |
| 9061 | 1.168083              | 2.302559                                                         |
| 9063 | 1.549156              | 2.302576                                                         |
| 9065 | 1.433646              | 2.302594                                                         |
| 9067 | 1.000110              | 2.302612                                                         |
| 9069 | 1.333774              | 2.302630                                                         |
| 9071 | 1.026568              | 2.302648                                                         |
| 9073 | 1.028105              | 2.302666                                                         |
| 9075 | 1.817300              | 2.302684                                                         |
| 9077 | 1.037788              | 2.302702                                                         |

| $n$  | $\frac{\sigma(n)}{n}$ | $\frac{e^\gamma}{2} \log \log n + \frac{0.73\dots}{\log \log n}$ |
|------|-----------------------|------------------------------------------------------------------|
| 9079 | 1.143738              | 2.302719                                                         |
| 9081 | 1.445876              | 2.302737                                                         |
| 9083 | 1.035781              | 2.302755                                                         |
| 9085 | 1.268024              | 2.302773                                                         |
| 9087 | 1.442060              | 2.302791                                                         |
| 9089 | 1.023215              | 2.302809                                                         |
| 9091 | 1.000110              | 2.302827                                                         |
| 9093 | 1.527329              | 2.302844                                                         |
| 9095 | 1.282463              | 2.302862                                                         |
| 9097 | 1.092228              | 2.302880                                                         |
| 9099 | 1.485878              | 2.302898                                                         |
| 9101 | 1.054829              | 2.302916                                                         |
| 9103 | 1.000110              | 2.302934                                                         |
| 9105 | 1.602636              | 2.302951                                                         |
| 9107 | 1.143736              | 2.302969                                                         |
| 9109 | 1.000110              | 2.302987                                                         |
| 9111 | 1.333772              | 2.303005                                                         |
| 9113 | 1.078459              | 2.303023                                                         |
| 9115 | 1.200658              | 2.303040                                                         |
| 9117 | 1.445870              | 2.303058                                                         |
| 9119 | 1.092225              | 2.303076                                                         |
| 9121 | 1.143734              | 2.303094                                                         |
| 9123 | 1.333772              | 2.303111                                                         |
| 9125 | 1.265096              | 2.303129                                                         |
| 9127 | 1.000110              | 2.303147                                                         |
| 9129 | 1.419652              | 2.303165                                                         |
| 9131 | 1.046107              | 2.303182                                                         |
| 9133 | 1.000109              | 2.303200                                                         |
| 9135 | 2.049261              | 2.303218                                                         |
| 9137 | 1.000109              | 2.303236                                                         |
| 9139 | 1.164241              | 2.303253                                                         |
| 9141 | 1.459797              | 2.303271                                                         |
| 9143 | 1.028984              | 2.303289                                                         |
| 9145 | 1.259705              | 2.303307                                                         |
| 9147 | 1.333771              | 2.303324                                                         |
| 9149 | 1.143732              | 2.303342                                                         |
| 9151 | 1.000109              | 2.303360                                                         |
| 9153 | 1.507047              | 2.303377                                                         |
| 9155 | 1.200655              | 2.303395                                                         |
| 9157 | 1.000109              | 2.303413                                                         |
| 9159 | 1.383557              | 2.303431                                                         |
| 9161 | 1.000109              | 2.303448                                                         |
| 9163 | 1.343665              | 2.303466                                                         |
| 9165 | 1.759738              | 2.303484                                                         |

| $n$  | $\frac{\sigma(n)}{n}$ | $\frac{e^\gamma}{2} \log \log n + \frac{0.73...}{\log \log n}$ |
|------|-----------------------|----------------------------------------------------------------|
| 9167 | 1.021054              | 2.303501                                                       |
| 9169 | 1.024757              | 2.303519                                                       |
| 9171 | 1.445862              | 2.303537                                                       |
| 9173 | 1.000109              | 2.303554                                                       |
| 9175 | 1.243379              | 2.303572                                                       |
| 9177 | 1.673750              | 2.303590                                                       |
| 9179 | 1.022334              | 2.303607                                                       |
| 9181 | 1.000109              | 2.303625                                                       |
| 9183 | 1.333769              | 2.303643                                                       |
| 9185 | 1.316930              | 2.303660                                                       |
| 9187 | 1.000109              | 2.303678                                                       |
| 9189 | 1.445859              | 2.303696                                                       |
| 9191 | 1.242955              | 2.303713                                                       |
| 9193 | 1.037746              | 2.303731                                                       |
| 9195 | 1.602610              | 2.303748                                                       |
| 9197 | 1.060781              | 2.303766                                                       |
| 9199 | 1.000109              | 2.303784                                                       |
| 9201 | 1.333768              | 2.303801                                                       |
| 9203 | 1.000109              | 2.303819                                                       |
| 9205 | 1.376643              | 2.303836                                                       |
| 9207 | 1.668296              | 2.303854                                                       |
| 9209 | 1.000109              | 2.303872                                                       |
| 9211 | 1.023125              | 2.303889                                                       |
| 9213 | 1.385868              | 2.303907                                                       |
| 9215 | 1.276180              | 2.303924                                                       |
| 9217 | 1.078442              | 2.303942                                                       |
| 9219 | 1.527281              | 2.303959                                                       |
| 9221 | 1.000108              | 2.303977                                                       |
| 9223 | 1.046080              | 2.303995                                                       |
| 9225 | 1.834797              | 2.304012                                                       |
| 9227 | 1.000108              | 2.304030                                                       |
| 9229 | 1.092209              | 2.304047                                                       |
| 9231 | 1.419565              | 2.304065                                                       |
| 9233 | 1.143724              | 2.304082                                                       |
| 9235 | 1.200650              | 2.304100                                                       |
| 9237 | 1.333766              | 2.304117                                                       |
| 9239 | 1.000108              | 2.304135                                                       |
| 9241 | 1.000108              | 2.304152                                                       |
| 9243 | 1.575246              | 2.304170                                                       |
| 9245 | 1.228556              | 2.304188                                                       |
| 9247 | 1.143722              | 2.304205                                                       |
| 9249 | 1.333766              | 2.304223                                                       |
| 9251 | 1.129824              | 2.304240                                                       |
| 9253 | 1.054793              | 2.304258                                                       |

| $n$  | $\frac{\sigma(n)}{n}$ | $\frac{e^\gamma}{2} \log \log n + \frac{0.73\dots}{\log \log n}$ |
|------|-----------------------|------------------------------------------------------------------|
| 9255 | 1.602593              | 2.304275                                                         |
| 9257 | 1.000108              | 2.304293                                                         |
| 9259 | 1.026461              | 2.304310                                                         |
| 9261 | 1.727675              | 2.304327                                                         |
| 9263 | 1.023427              | 2.304345                                                         |
| 9265 | 1.282245              | 2.304362                                                         |
| 9267 | 1.333765              | 2.304380                                                         |
| 9269 | 1.159996              | 2.304397                                                         |
| 9271 | 1.021681              | 2.304415                                                         |
| 9273 | 1.459722              | 2.304432                                                         |
| 9275 | 1.443881              | 2.304450                                                         |
| 9277 | 1.000108              | 2.304467                                                         |
| 9279 | 1.445845              | 2.304485                                                         |
| 9281 | 1.000108              | 2.304502                                                         |
| 9283 | 1.000108              | 2.304520                                                         |
| 9285 | 1.602585              | 2.304537                                                         |
| 9287 | 1.031119              | 2.304554                                                         |
| 9289 | 1.143718              | 2.304572                                                         |
| 9291 | 1.412119              | 2.304589                                                         |
| 9293 | 1.000108              | 2.304607                                                         |
| 9295 | 1.417536              | 2.304624                                                         |
| 9297 | 1.445843              | 2.304641                                                         |
| 9299 | 1.060759              | 2.304659                                                         |
| 9301 | 1.021826              | 2.304676                                                         |
| 9303 | 1.527249              | 2.304694                                                         |
| 9305 | 1.200645              | 2.304711                                                         |
| 9307 | 1.028903              | 2.304728                                                         |
| 9309 | 1.392201              | 2.304746                                                         |
| 9311 | 1.000107              | 2.304763                                                         |
| 9313 | 1.022227              | 2.304781                                                         |
| 9315 | 1.870531              | 2.304798                                                         |
| 9317 | 1.257057              | 2.304815                                                         |
| 9319 | 1.000107              | 2.304833                                                         |
| 9321 | 1.441905              | 2.304850                                                         |
| 9323 | 1.000107              | 2.304867                                                         |
| 9325 | 1.243324              | 2.304885                                                         |
| 9327 | 1.333762              | 2.304902                                                         |
| 9329 | 1.054775              | 2.304919                                                         |
| 9331 | 1.207159              | 2.304937                                                         |
| 9333 | 1.554484              | 2.304954                                                         |
| 9335 | 1.200643              | 2.304971                                                         |
| 9337 | 1.000107              | 2.304989                                                         |
| 9339 | 1.459685              | 2.305006                                                         |
| 9341 | 1.000107              | 2.305023                                                         |



| $n$  | $\frac{\sigma(n)}{n}$ | $\frac{e^\gamma}{2} \log \log n + \frac{0.73\dots}{\log \log n}$ |
|------|-----------------------|------------------------------------------------------------------|
| 9343 | 1.000107              | 2.305041                                                         |
| 9345 | 1.849117              | 2.305058                                                         |
| 9347 | 1.078421              | 2.305075                                                         |
| 9349 | 1.000107              | 2.305093                                                         |
| 9351 | 1.445835              | 2.305110                                                         |
| 9353 | 1.026409              | 2.305127                                                         |
| 9355 | 1.200641              | 2.305145                                                         |
| 9357 | 1.333761              | 2.305162                                                         |
| 9359 | 1.169356              | 2.305179                                                         |
| 9361 | 1.169106              | 2.305196                                                         |
| 9363 | 1.333761              | 2.305214                                                         |
| 9365 | 1.200641              | 2.305231                                                         |
| 9367 | 1.152984              | 2.305248                                                         |
| 9369 | 1.485751              | 2.305266                                                         |
| 9371 | 1.000107              | 2.305283                                                         |
| 9373 | 1.242718              | 2.305300                                                         |
| 9375 | 1.666560              | 2.305317                                                         |
| 9377 | 1.000107              | 2.305335                                                         |
| 9379 | 1.021004              | 2.305352                                                         |
| 9381 | 1.381516              | 2.305369                                                         |
| 9383 | 1.092188              | 2.305386                                                         |
| 9385 | 1.200639              | 2.305403                                                         |
| 9387 | 1.661873              | 2.305421                                                         |
| 9389 | 1.028864              | 2.305438                                                         |
| 9391 | 1.000106              | 2.305455                                                         |
| 9393 | 1.389971              | 2.305472                                                         |
| 9395 | 1.200639              | 2.305490                                                         |
| 9397 | 1.000106              | 2.305507                                                         |
| 9399 | 1.441856              | 2.305524                                                         |
| 9401 | 1.225402              | 2.305541                                                         |
| 9403 | 1.000106              | 2.305558                                                         |
| 9405 | 1.990431              | 2.305576                                                         |
| 9407 | 1.046030              | 2.305593                                                         |
| 9409 | 1.010416              | 2.305610                                                         |
| 9411 | 1.333758              | 2.305627                                                         |
| 9413 | 1.000106              | 2.305644                                                         |
| 9415 | 1.376527              | 2.305661                                                         |
| 9417 | 1.383031              | 2.305679                                                         |
| 9419 | 1.000106              | 2.305696                                                         |
| 9421 | 1.000106              | 2.305713                                                         |
| 9423 | 1.485726              | 2.305730                                                         |
| 9425 | 1.381432              | 2.305747                                                         |
| 9427 | 1.092182              | 2.305764                                                         |
| 9429 | 1.527203              | 2.305782                                                         |

| $n$  | $\frac{\sigma(n)}{n}$ | $\frac{e^\gamma}{2} \log \log n + \frac{0.73...}{\log \log n}$ |
|------|-----------------------|----------------------------------------------------------------|
| 9431 | 1.000106              | 2.305799                                                       |
| 9433 | 1.000106              | 2.305816                                                       |
| 9435 | 1.739905              | 2.305833                                                       |
| 9437 | 1.000106              | 2.305850                                                       |
| 9439 | 1.000106              | 2.305867                                                       |
| 9441 | 1.445821              | 2.305884                                                       |
| 9443 | 1.219951              | 2.305901                                                       |
| 9445 | 1.200635              | 2.305919                                                       |
| 9447 | 1.382026              | 2.305936                                                       |
| 9449 | 1.092179              | 2.305953                                                       |
| 9451 | 1.078404              | 2.305970                                                       |
| 9453 | 1.401460              | 2.305987                                                       |
| 9455 | 1.259016              | 2.306004                                                       |
| 9457 | 1.169293              | 2.306021                                                       |
| 9459 | 1.445819              | 2.306038                                                       |
| 9461 | 1.000106              | 2.306055                                                       |
| 9463 | 1.000106              | 2.306072                                                       |
| 9465 | 1.602536              | 2.306089                                                       |
| 9467 | 1.000106              | 2.306107                                                       |
| 9469 | 1.060724              | 2.306124                                                       |
| 9471 | 1.702882              | 2.306141                                                       |
| 9473 | 1.000106              | 2.306158                                                       |
| 9475 | 1.243272              | 2.306175                                                       |
| 9477 | 1.614646              | 2.306192                                                       |
| 9479 | 1.000105              | 2.306209                                                       |
| 9481 | 1.054741              | 2.306226                                                       |
| 9483 | 1.391965              | 2.306243                                                       |
| 9485 | 1.376489              | 2.306260                                                       |
| 9487 | 1.024560              | 2.306277                                                       |
| 9489 | 1.333755              | 2.306294                                                       |
| 9491 | 1.000105              | 2.306311                                                       |
| 9493 | 1.092173              | 2.306328                                                       |
| 9495 | 1.741548              | 2.306345                                                       |
| 9497 | 1.000105              | 2.306362                                                       |
| 9499 | 1.212759              | 2.306379                                                       |
| 9501 | 1.333754              | 2.306396                                                       |
| 9503 | 1.166789              | 2.306413                                                       |
| 9505 | 1.200631              | 2.306430                                                       |
| 9507 | 1.333754              | 2.306447                                                       |
| 9509 | 1.031023              | 2.306464                                                       |
| 9511 | 1.000105              | 2.306481                                                       |
| 9513 | 1.661726              | 2.306498                                                       |
| 9515 | 1.316658              | 2.306515                                                       |
| 9517 | 1.035620              | 2.306532                                                       |

| $n$  | $\frac{\sigma(n)}{n}$ | $\frac{e^\gamma}{2} \log \log n + \frac{0.73...}{\log \log n}$ |
|------|-----------------------|----------------------------------------------------------------|
| 9519 | 1.411913              | 2.306549                                                       |
| 9521 | 1.000105              | 2.306566                                                       |
| 9523 | 1.020687              | 2.306583                                                       |
| 9525 | 1.666352              | 2.306600                                                       |
| 9527 | 1.143697              | 2.306617                                                       |
| 9529 | 1.078392              | 2.306634                                                       |
| 9531 | 1.485678              | 2.306651                                                       |
| 9533 | 1.000105              | 2.306668                                                       |
| 9535 | 1.200629              | 2.306685                                                       |
| 9537 | 1.545140              | 2.306701                                                       |
| 9539 | 1.000105              | 2.306718                                                       |
| 9541 | 1.207421              | 2.306735                                                       |
| 9543 | 1.333752              | 2.306752                                                       |
| 9545 | 1.267260              | 2.306769                                                       |
| 9547 | 1.000105              | 2.306786                                                       |
| 9549 | 1.445806              | 2.306803                                                       |
| 9551 | 1.000105              | 2.306820                                                       |
| 9553 | 1.028787              | 2.306837                                                       |
| 9555 | 2.004396              | 2.306854                                                       |
| 9557 | 1.054724              | 2.306871                                                       |
| 9559 | 1.113087              | 2.306887                                                       |
| 9561 | 1.333752              | 2.306904                                                       |
| 9563 | 1.021437              | 2.306921                                                       |
| 9565 | 1.200627              | 2.306938                                                       |
| 9567 | 1.445803              | 2.306955                                                       |
| 9569 | 1.143693              | 2.306972                                                       |
| 9571 | 1.060704              | 2.306989                                                       |
| 9573 | 1.333751              | 2.307006                                                       |
| 9575 | 1.243238              | 2.307022                                                       |
| 9577 | 1.022867              | 2.307039                                                       |
| 9579 | 1.389707              | 2.307056                                                       |
| 9581 | 1.192360              | 2.307073                                                       |
| 9583 | 1.174580              | 2.307090                                                       |
| 9585 | 1.802817              | 2.307107                                                       |
| 9587 | 1.000104              | 2.307124                                                       |
| 9589 | 1.027844              | 2.307140                                                       |
| 9591 | 1.401314              | 2.307157                                                       |
| 9593 | 1.024497              | 2.307174                                                       |
| 9595 | 1.275664              | 2.307191                                                       |
| 9597 | 1.527144              | 2.307208                                                       |
| 9599 | 1.037608              | 2.307224                                                       |
| 9601 | 1.000104              | 2.307241                                                       |
| 9603 | 1.592002              | 2.307258                                                       |
| 9605 | 1.281832              | 2.307275                                                       |

| $n$  | $\frac{\sigma(n)}{n}$ | $\frac{e^\gamma}{2} \log \log n + \frac{0.73...}{\log \log n}$ |
|------|-----------------------|----------------------------------------------------------------|
| 9607 | 1.078380              | 2.307292                                                       |
| 9609 | 1.333750              | 2.307308                                                       |
| 9611 | 1.143690              | 2.307325                                                       |
| 9613 | 1.000104              | 2.307342                                                       |
| 9615 | 1.602496              | 2.307359                                                       |
| 9617 | 1.023188              | 2.307376                                                       |
| 9619 | 1.000104              | 2.307392                                                       |
| 9621 | 1.445796              | 2.307409                                                       |
| 9623 | 1.000104              | 2.307426                                                       |
| 9625 | 1.555948              | 2.307443                                                       |
| 9627 | 1.333749              | 2.307459                                                       |
| 9629 | 1.000104              | 2.307476                                                       |
| 9631 | 1.000104              | 2.307493                                                       |
| 9633 | 1.519776              | 2.307510                                                       |
| 9635 | 1.255423              | 2.307526                                                       |
| 9637 | 1.045969              | 2.307543                                                       |
| 9639 | 1.807656              | 2.307560                                                       |
| 9641 | 1.035577              | 2.307577                                                       |
| 9643 | 1.000104              | 2.307593                                                       |
| 9645 | 1.602488              | 2.307610                                                       |
| 9647 | 1.092153              | 2.307627                                                       |
| 9649 | 1.000104              | 2.307644                                                       |
| 9651 | 1.333748              | 2.307660                                                       |
| 9653 | 1.169170              | 2.307677                                                       |
| 9655 | 1.200621              | 2.307694                                                       |
| 9657 | 1.534638              | 2.307710                                                       |
| 9659 | 1.078373              | 2.307727                                                       |
| 9661 | 1.000104              | 2.307744                                                       |
| 9663 | 1.333747              | 2.307760                                                       |
| 9665 | 1.200621              | 2.307777                                                       |
| 9667 | 1.143685              | 2.307794                                                       |
| 9669 | 1.459510              | 2.307811                                                       |
| 9671 | 1.054700              | 2.307827                                                       |
| 9673 | 1.060684              | 2.307844                                                       |
| 9675 | 1.832765              | 2.307861                                                       |
| 9677 | 1.000103              | 2.307877                                                       |
| 9679 | 1.000103              | 2.307894                                                       |
| 9681 | 1.527115              | 2.307911                                                       |
| 9683 | 1.045957              | 2.307927                                                       |
| 9685 | 1.300981              | 2.307944                                                       |
| 9687 | 1.333746              | 2.307961                                                       |
| 9689 | 1.000103              | 2.307977                                                       |
| 9691 | 1.092147              | 2.307994                                                       |
| 9693 | 1.485608              | 2.308010                                                       |

| $n$  | $\frac{\sigma(n)}{n}$ | $\frac{e^\gamma}{2} \log \log n + \frac{0.73...}{\log \log n}$ |
|------|-----------------------|----------------------------------------------------------------|
| 9695 | 1.376380              | 2.308027                                                       |
| 9697 | 1.000103              | 2.308044                                                       |
| 9699 | 1.380761              | 2.308060                                                       |
| 9701 | 1.020513              | 2.308077                                                       |
| 9703 | 1.035556              | 2.308094                                                       |
| 9705 | 1.602473              | 2.308110                                                       |
| 9707 | 1.060678              | 2.308127                                                       |
| 9709 | 1.219487              | 2.308143                                                       |
| 9711 | 1.574297              | 2.308160                                                       |
| 9713 | 1.092145              | 2.308177                                                       |
| 9715 | 1.259907              | 2.308193                                                       |
| 9717 | 1.383143              | 2.308210                                                       |
| 9719 | 1.000103              | 2.308226                                                       |
| 9721 | 1.000103              | 2.308243                                                       |
| 9723 | 1.527101              | 2.308260                                                       |
| 9725 | 1.243188              | 2.308276                                                       |
| 9727 | 1.021487              | 2.308293                                                       |
| 9729 | 1.539315              | 2.308309                                                       |
| 9731 | 1.030932              | 2.308326                                                       |
| 9733 | 1.000103              | 2.308342                                                       |
| 9735 | 1.775039              | 2.308359                                                       |
| 9737 | 1.242272              | 2.308375                                                       |
| 9739 | 1.000103              | 2.308392                                                       |
| 9741 | 1.419156              | 2.308409                                                       |
| 9743 | 1.000103              | 2.308425                                                       |
| 9745 | 1.200616              | 2.308442                                                       |
| 9747 | 1.563558              | 2.308458                                                       |
| 9749 | 1.000103              | 2.308475                                                       |
| 9751 | 1.169111              | 2.308491                                                       |
| 9753 | 1.333743              | 2.308508                                                       |
| 9755 | 1.200615              | 2.308524                                                       |
| 9757 | 1.092139              | 2.308541                                                       |
| 9759 | 1.333743              | 2.308557                                                       |
| 9761 | 1.027764              | 2.308574                                                       |
| 9763 | 1.078357              | 2.308590                                                       |
| 9765 | 2.044854              | 2.308607                                                       |
| 9767 | 1.000102              | 2.308623                                                       |
| 9769 | 1.000102              | 2.308640                                                       |
| 9771 | 1.333743              | 2.308656                                                       |
| 9773 | 1.037552              | 2.308673                                                       |
| 9775 | 1.370026              | 2.308689                                                       |
| 9777 | 1.333742              | 2.308706                                                       |
| 9779 | 1.256570              | 2.308722                                                       |
| 9781 | 1.000102              | 2.308739                                                       |

| $n$  | $\frac{\sigma(n)}{n}$ | $\frac{e^\gamma}{2} \log \log n + \frac{0.73\dots}{\log \log n}$ |
|------|-----------------------|------------------------------------------------------------------|
| 9783 | 1.445773              | 2.308755                                                         |
| 9785 | 1.275422              | 2.308772                                                         |
| 9787 | 1.000102              | 2.308788                                                         |
| 9789 | 1.441618              | 2.308805                                                         |
| 9791 | 1.000102              | 2.308821                                                         |
| 9793 | 1.143674              | 2.308837                                                         |
| 9795 | 1.602450              | 2.308854                                                         |
| 9797 | 1.020312              | 2.308870                                                         |
| 9799 | 1.028676              | 2.308887                                                         |
| 9801 | 1.641975              | 2.308903                                                         |
| 9803 | 1.000102              | 2.308920                                                         |
| 9805 | 1.255686              | 2.308936                                                         |
| 9807 | 1.527072              | 2.308953                                                         |
| 9809 | 1.060659              | 2.308969                                                         |
| 9811 | 1.000102              | 2.308985                                                         |
| 9813 | 1.333741              | 2.309002                                                         |
| 9815 | 1.300866              | 2.309018                                                         |
| 9817 | 1.000102              | 2.309035                                                         |
| 9819 | 1.445768              | 2.309051                                                         |
| 9821 | 1.212097              | 2.309067                                                         |
| 9823 | 1.172758              | 2.309084                                                         |
| 9825 | 1.665954              | 2.309100                                                         |
| 9827 | 1.035514              | 2.309117                                                         |
| 9829 | 1.000102              | 2.309133                                                         |
| 9831 | 1.391517              | 2.309149                                                         |
| 9833 | 1.000102              | 2.309166                                                         |
| 9835 | 1.376309              | 2.309182                                                         |
| 9837 | 1.445766              | 2.309198                                                         |
| 9839 | 1.000102              | 2.309215                                                         |
| 9841 | 1.078346              | 2.309231                                                         |
| 9843 | 1.419080              | 2.309248                                                         |
| 9845 | 1.316404              | 2.309264                                                         |
| 9847 | 1.027724              | 2.309280                                                         |
| 9849 | 1.574170              | 2.309297                                                         |
| 9851 | 1.000102              | 2.309313                                                         |
| 9853 | 1.023039              | 2.309329                                                         |
| 9855 | 1.802131              | 2.309346                                                         |
| 9857 | 1.000101              | 2.309362                                                         |
| 9859 | 1.000101              | 2.309378                                                         |
| 9861 | 1.411622              | 2.309395                                                         |
| 9863 | 1.143668              | 2.309411                                                         |
| 9865 | 1.200608              | 2.309427                                                         |
| 9867 | 1.634539              | 2.309444                                                         |
| 9869 | 1.021380              | 2.309460                                                         |

| $n$  | $\frac{\sigma(n)}{n}$ | $\frac{e^\gamma}{2} \log \log n + \frac{0.73...}{\log \log n}$ |
|------|-----------------------|----------------------------------------------------------------|
| 9871 | 1.000101              | 2.309476                                                       |
| 9873 | 1.445761              | 2.309493                                                       |
| 9875 | 1.263797              | 2.309509                                                       |
| 9877 | 1.224663              | 2.309525                                                       |
| 9879 | 1.384756              | 2.309541                                                       |
| 9881 | 1.028641              | 2.309558                                                       |
| 9883 | 1.000101              | 2.309574                                                       |
| 9885 | 1.602428              | 2.309590                                                       |
| 9887 | 1.000101              | 2.309607                                                       |
| 9889 | 1.164931              | 2.309623                                                       |
| 9891 | 1.661308              | 2.309639                                                       |
| 9893 | 1.078338              | 2.309655                                                       |
| 9895 | 1.200606              | 2.309672                                                       |
| 9897 | 1.333737              | 2.309688                                                       |
| 9899 | 1.054652              | 2.309704                                                       |
| 9901 | 1.000101              | 2.309720                                                       |
| 9903 | 1.333737              | 2.309737                                                       |
| 9905 | 1.376275              | 2.309753                                                       |
| 9907 | 1.000101              | 2.309769                                                       |
| 9909 | 1.485518              | 2.309785                                                       |
| 9911 | 1.176874              | 2.309802                                                       |
| 9913 | 1.045899              | 2.309818                                                       |
| 9915 | 1.602421              | 2.309834                                                       |
| 9917 | 1.026117              | 2.309850                                                       |
| 9919 | 1.242061              | 2.309867                                                       |
| 9921 | 1.333737              | 2.309883                                                       |
| 9923 | 1.000101              | 2.309899                                                       |
| 9925 | 1.243123              | 2.309915                                                       |
| 9927 | 1.445754              | 2.309931                                                       |
| 9929 | 1.000101              | 2.309948                                                       |
| 9931 | 1.000101              | 2.309964                                                       |
| 9933 | 1.700997              | 2.309980                                                       |
| 9935 | 1.200604              | 2.309996                                                       |
| 9937 | 1.054644              | 2.310012                                                       |
| 9939 | 1.333736              | 2.310029                                                       |
| 9941 | 1.000101              | 2.310045                                                       |
| 9943 | 1.022629              | 2.310061                                                       |
| 9945 | 1.976471              | 2.310077                                                       |
| 9947 | 1.206394              | 2.310093                                                       |
| 9949 | 1.000101              | 2.310110                                                       |
| 9951 | 1.389207              | 2.310126                                                       |
| 9953 | 1.030845              | 2.310142                                                       |
| 9955 | 1.316323              | 2.310158                                                       |
| 9957 | 1.333735              | 2.310174                                                       |

| $n$   | $\frac{\sigma(n)}{n}$ | $\frac{e^\gamma}{2} \log \log n + \frac{0.73...}{\log \log n}$ |
|-------|-----------------------|----------------------------------------------------------------|
| 9959  | 1.045888              | 2.310190                                                       |
| 9961  | 1.143660              | 2.310206                                                       |
| 9963  | 1.534478              | 2.310223                                                       |
| 9965  | 1.200602              | 2.310239                                                       |
| 9967  | 1.000100              | 2.310255                                                       |
| 9969  | 1.333735              | 2.310271                                                       |
| 9971  | 1.101193              | 2.310287                                                       |
| 9973  | 1.000100              | 2.310303                                                       |
| 9975  | 1.988972              | 2.310319                                                       |
| 9977  | 1.092112              | 2.310336                                                       |
| 9979  | 1.060627              | 2.310352                                                       |
| 9981  | 1.445747              | 2.310368                                                       |
| 9983  | 1.021737              | 2.310384                                                       |
| 9985  | 1.200601              | 2.310400                                                       |
| 9987  | 1.333734              | 2.310416                                                       |
| 9989  | 1.143658              | 2.310432                                                       |
| 9991  | 1.020118              | 2.310448                                                       |
| 9993  | 1.333734              | 2.310464                                                       |
| 9995  | 1.200600              | 2.310480                                                       |
| 9997  | 1.078323              | 2.310497                                                       |
| 9999  | 1.591359              | 2.310513                                                       |
| 10001 | 1.021098              | 2.310529                                                       |
| 10003 | 1.143657              | 2.310545                                                       |
| 10005 | 1.727136              | 2.310561                                                       |
| 10007 | 1.000100              | 2.310577                                                       |
| 10009 | 1.000100              | 2.310593                                                       |
| 10011 | 1.380881              | 2.310609                                                       |
| 10013 | 1.150504              | 2.310625                                                       |
| 10015 | 1.200599              | 2.310641                                                       |
| 10017 | 1.725067              | 2.310657                                                       |
| 10019 | 1.027647              | 2.310673                                                       |
| 10021 | 1.092107              | 2.310689                                                       |
| 10023 | 1.441485              | 2.310705                                                       |
| 10025 | 1.243092              | 2.310721                                                       |
| 10027 | 1.030817              | 2.310737                                                       |
| 10029 | 1.333732              | 2.310753                                                       |
| 10031 | 1.143655              | 2.310769                                                       |
| 10033 | 1.020632              | 2.310785                                                       |
| 10035 | 1.741106              | 2.310801                                                       |
| 10037 | 1.000100              | 2.310818                                                       |
| 10039 | 1.000100              | 2.310834                                                       |
| 10041 | 1.333732              | 2.310850                                                       |
| 10043 | 1.112417              | 2.310866                                                       |
| 10045 | 1.429965              | 2.310882                                                       |



| $n$   | $\frac{\sigma(n)}{n}$ | $\frac{e^\gamma}{2} \log \log n + \frac{0.73\dots}{\log \log n}$ |
|-------|-----------------------|------------------------------------------------------------------|
| 10047 | 1.418931              | 2.310898                                                         |
| 10049 | 1.078316              | 2.310914                                                         |
| 10051 | 1.100388              | 2.310930                                                         |
| 10053 | 1.445738              | 2.310946                                                         |
| 10055 | 1.200597              | 2.310961                                                         |
| 10057 | 1.020185              | 2.310977                                                         |
| 10059 | 1.526991              | 2.310993                                                         |
| 10061 | 1.000099              | 2.311009                                                         |
| 10063 | 1.037464              | 2.311025                                                         |
| 10065 | 1.774069              | 2.311041                                                         |
| 10067 | 1.000099              | 2.311057                                                         |
| 10069 | 1.000099              | 2.311073                                                         |
| 10071 | 1.485453              | 2.311089                                                         |
| 10073 | 1.143651              | 2.311105                                                         |
| 10075 | 1.378462              | 2.311121                                                         |
| 10077 | 1.333730              | 2.311137                                                         |
| 10079 | 1.000099              | 2.311153                                                         |
| 10081 | 1.060609              | 2.311169                                                         |
| 10083 | 1.333730              | 2.311185                                                         |
| 10085 | 1.200595              | 2.311201                                                         |
| 10087 | 1.256270              | 2.311217                                                         |
| 10089 | 1.546238              | 2.311233                                                         |
| 10091 | 1.000099              | 2.311249                                                         |
| 10093 | 1.000099              | 2.311265                                                         |
| 10095 | 1.602377              | 2.311280                                                         |
| 10097 | 1.045855              | 2.311296                                                         |
| 10099 | 1.000099              | 2.311312                                                         |
| 10101 | 1.685378              | 2.311328                                                         |
| 10103 | 1.000099              | 2.311344                                                         |
| 10105 | 1.254033              | 2.311360                                                         |
| 10107 | 1.445731              | 2.311376                                                         |
| 10109 | 1.092096              | 2.311392                                                         |
| 10111 | 1.000099              | 2.311408                                                         |
| 10113 | 1.333729              | 2.311424                                                         |
| 10115 | 1.456846              | 2.311439                                                         |
| 10117 | 1.021647              | 2.311455                                                         |
| 10119 | 1.333729              | 2.311471                                                         |
| 10121 | 1.037447              | 2.311487                                                         |
| 10123 | 1.024202              | 2.311503                                                         |
| 10125 | 1.864296              | 2.311519                                                         |
| 10127 | 1.161252              | 2.311535                                                         |
| 10129 | 1.143647              | 2.311551                                                         |
| 10131 | 1.459283              | 2.311566                                                         |
| 10133 | 1.000099              | 2.311582                                                         |

| $n$   | $\frac{\sigma(n)}{n}$ | $\frac{e^\gamma}{2} \log \log n + \frac{0.73...}{\log \log n}$ |
|-------|-----------------------|----------------------------------------------------------------|
| 10135 | 1.200592              | 2.311598                                                       |
| 10137 | 1.388971              | 2.311614                                                       |
| 10139 | 1.000099              | 2.311630                                                       |
| 10141 | 1.000099              | 2.311646                                                       |
| 10143 | 1.753327              | 2.311661                                                       |
| 10145 | 1.200591              | 2.311677                                                       |
| 10147 | 1.020991              | 2.311693                                                       |
| 10149 | 1.418859              | 2.311709                                                       |
| 10151 | 1.000099              | 2.311725                                                       |
| 10153 | 1.191372              | 2.311741                                                       |
| 10155 | 1.602363              | 2.311756                                                       |
| 10157 | 1.143645              | 2.311772                                                       |
| 10159 | 1.000098              | 2.311788                                                       |
| 10161 | 1.445724              | 2.311804                                                       |
| 10163 | 1.000098              | 2.311820                                                       |
| 10165 | 1.274963              | 2.311835                                                       |
| 10167 | 1.333727              | 2.311851                                                       |
| 10169 | 1.000098              | 2.311867                                                       |
| 10171 | 1.143644              | 2.311883                                                       |
| 10173 | 1.333727              | 2.311899                                                       |
| 10175 | 1.389287              | 2.311914                                                       |
| 10177 | 1.000098              | 2.311930                                                       |
| 10179 | 1.650457              | 2.311946                                                       |
| 10181 | 1.000098              | 2.311962                                                       |
| 10183 | 1.060591              | 2.311977                                                       |
| 10185 | 1.847423              | 2.311993                                                       |
| 10187 | 1.022480              | 2.312009                                                       |
| 10189 | 1.045834              | 2.312025                                                       |
| 10191 | 1.381611              | 2.312040                                                       |
| 10193 | 1.000098              | 2.312056                                                       |
| 10195 | 1.200589              | 2.312072                                                       |
| 10197 | 1.591056              | 2.312088                                                       |
| 10199 | 1.204824              | 2.312103                                                       |
| 10201 | 1.009999              | 2.312119                                                       |
| 10203 | 1.411350              | 2.312135                                                       |
| 10205 | 1.300539              | 2.312151                                                       |
| 10207 | 1.022827              | 2.312166                                                       |
| 10209 | 1.382310              | 2.312182                                                       |
| 10211 | 1.000098              | 2.312198                                                       |
| 10213 | 1.143640              | 2.312213                                                       |
| 10215 | 1.740969              | 2.312229                                                       |
| 10217 | 1.060585              | 2.312245                                                       |
| 10219 | 1.092083              | 2.312261                                                       |
| 10221 | 1.333725              | 2.312276                                                       |

| $n$   | $\frac{\sigma(n)}{n}$ | $\frac{e^\gamma}{2} \log \log n + \frac{0.73...}{\log \log n}$ |
|-------|-----------------------|----------------------------------------------------------------|
| 10223 | 1.000098              | 2.312292                                                       |
| 10225 | 1.243032              | 2.312308                                                       |
| 10227 | 1.526938              | 2.312323                                                       |
| 10229 | 1.024147              | 2.312339                                                       |
| 10231 | 1.078291              | 2.312355                                                       |
| 10233 | 1.485390              | 2.312370                                                       |
| 10235 | 1.266243              | 2.312386                                                       |
| 10237 | 1.037413              | 2.312402                                                       |
| 10239 | 1.333724              | 2.312417                                                       |
| 10241 | 1.335807              | 2.312433                                                       |
| 10243 | 1.000098              | 2.312449                                                       |
| 10245 | 1.602343              | 2.312464                                                       |
| 10247 | 1.000098              | 2.312480                                                       |
| 10249 | 1.030735              | 2.312496                                                       |
| 10251 | 1.552239              | 2.312511                                                       |
| 10253 | 1.000098              | 2.312527                                                       |
| 10255 | 1.376109              | 2.312543                                                       |
| 10257 | 1.441357              | 2.312558                                                       |
| 10259 | 1.000097              | 2.312574                                                       |
| 10261 | 1.035377              | 2.312590                                                       |
| 10263 | 1.459222              | 2.312605                                                       |
| 10265 | 1.200585              | 2.312621                                                       |
| 10267 | 1.000097              | 2.312637                                                       |
| 10269 | 1.660921              | 2.312652                                                       |
| 10271 | 1.000097              | 2.312668                                                       |
| 10273 | 1.000097              | 2.312683                                                       |
| 10275 | 1.665401              | 2.312699                                                       |
| 10277 | 1.027537              | 2.312715                                                       |
| 10279 | 1.054577              | 2.312730                                                       |
| 10281 | 1.400642              | 2.312746                                                       |
| 10283 | 1.241661              | 2.312761                                                       |
| 10285 | 1.396597              | 2.312777                                                       |
| 10287 | 1.505590              | 2.312793                                                       |
| 10289 | 1.000097              | 2.312808                                                       |
| 10291 | 1.028471              | 2.312824                                                       |
| 10293 | 1.380356              | 2.312839                                                       |
| 10295 | 1.258864              | 2.312855                                                       |
| 10297 | 1.143634              | 2.312871                                                       |
| 10299 | 1.333722              | 2.312886                                                       |
| 10301 | 1.000097              | 2.312902                                                       |
| 10303 | 1.000097              | 2.312917                                                       |
| 10305 | 1.740902              | 2.312933                                                       |
| 10307 | 1.092073              | 2.312948                                                       |
| 10309 | 1.100592              | 2.312964                                                       |

| $n$   | $\frac{\sigma(n)}{n}$ | $\frac{e^\gamma}{2} \log \log n + \frac{0.73\dots}{\log \log n}$ |
|-------|-----------------------|------------------------------------------------------------------|
| 10311 | 1.526913              | 2.312979                                                         |
| 10313 | 1.000097              | 2.312995                                                         |
| 10315 | 1.200582              | 2.313011                                                         |
| 10317 | 1.411263              | 2.313026                                                         |
| 10319 | 1.060568              | 2.313042                                                         |
| 10321 | 1.000097              | 2.313057                                                         |
| 10323 | 1.531338              | 2.313073                                                         |
| 10325 | 1.441162              | 2.313088                                                         |
| 10327 | 1.045802              | 2.313104                                                         |
| 10329 | 1.459193              | 2.313119                                                         |
| 10331 | 1.000097              | 2.313135                                                         |
| 10333 | 1.000097              | 2.313150                                                         |
| 10335 | 1.755588              | 2.313166                                                         |
| 10337 | 1.000097              | 2.313181                                                         |
| 10339 | 1.168778              | 2.313197                                                         |
| 10341 | 1.485350              | 2.313212                                                         |
| 10343 | 1.000097              | 2.313228                                                         |
| 10345 | 1.200580              | 2.313243                                                         |
| 10347 | 1.333720              | 2.313259                                                         |
| 10349 | 1.020388              | 2.313274                                                         |
| 10351 | 1.092068              | 2.313290                                                         |
| 10353 | 1.669081              | 2.313305                                                         |
| 10355 | 1.274746              | 2.313321                                                         |
| 10357 | 1.000097              | 2.313336                                                         |
| 10359 | 1.445699              | 2.313352                                                         |
| 10361 | 1.078274              | 2.313367                                                         |
| 10363 | 1.027502              | 2.313383                                                         |
| 10365 | 1.602315              | 2.313398                                                         |
| 10367 | 1.143629              | 2.313414                                                         |
| 10369 | 1.000096              | 2.313429                                                         |
| 10371 | 1.333719              | 2.313445                                                         |
| 10373 | 1.166104              | 2.313460                                                         |
| 10375 | 1.263036              | 2.313475                                                         |
| 10377 | 1.445697              | 2.313491                                                         |
| 10379 | 1.019751              | 2.313506                                                         |
| 10381 | 1.143628              | 2.313522                                                         |
| 10383 | 1.333719              | 2.313537                                                         |
| 10385 | 1.257198              | 2.313553                                                         |
| 10387 | 1.164533              | 2.313568                                                         |
| 10389 | 1.333718              | 2.313583                                                         |
| 10391 | 1.000096              | 2.313599                                                         |
| 10393 | 1.054556              | 2.313614                                                         |
| 10395 | 2.216450              | 2.313630                                                         |
| 10397 | 1.030682              | 2.313645                                                         |

| $n$   | $\frac{\sigma(n)}{n}$ | $\frac{e^\gamma}{2} \log \log n + \frac{0.73...}{\log \log n}$ |
|-------|-----------------------|----------------------------------------------------------------|
| 10399 | 1.000096              | 2.313661                                                       |
| 10401 | 1.333718              | 2.313676                                                       |
| 10403 | 1.019706              | 2.313691                                                       |
| 10405 | 1.200577              | 2.313707                                                       |
| 10407 | 1.333718              | 2.313722                                                       |
| 10409 | 1.143626              | 2.313738                                                       |
| 10411 | 1.037364              | 2.313753                                                       |
| 10413 | 1.573034              | 2.313768                                                       |
| 10415 | 1.200576              | 2.313784                                                       |
| 10417 | 1.092061              | 2.313799                                                       |
| 10419 | 1.400518              | 2.313814                                                       |
| 10421 | 1.060551              | 2.313830                                                       |
| 10423 | 1.143625              | 2.313845                                                       |
| 10425 | 1.665228              | 2.313861                                                       |
| 10427 | 1.000096              | 2.313876                                                       |
| 10429 | 1.000096              | 2.313891                                                       |
| 10431 | 1.545394              | 2.313907                                                       |
| 10433 | 1.000096              | 2.313922                                                       |
| 10435 | 1.200575              | 2.313937                                                       |
| 10437 | 1.572866              | 2.313953                                                       |
| 10439 | 1.190919              | 2.313968                                                       |
| 10441 | 1.024040              | 2.313983                                                       |
| 10443 | 1.356315              | 2.313999                                                       |
| 10445 | 1.200574              | 2.314014                                                       |
| 10447 | 1.035321              | 2.314029                                                       |
| 10449 | 1.532778              | 2.314045                                                       |
| 10451 | 1.143623              | 2.314060                                                       |
| 10453 | 1.000096              | 2.314075                                                       |
| 10455 | 1.735438              | 2.314091                                                       |
| 10457 | 1.000096              | 2.314106                                                       |
| 10459 | 1.000096              | 2.314121                                                       |
| 10461 | 1.459134              | 2.314137                                                       |
| 10463 | 1.000096              | 2.314152                                                       |
| 10465 | 1.541137              | 2.314167                                                       |
| 10467 | 1.445686              | 2.314183                                                       |
| 10469 | 1.091795              | 2.314198                                                       |
| 10471 | 1.030656              | 2.314213                                                       |
| 10473 | 1.333715              | 2.314228                                                       |
| 10475 | 1.242959              | 2.314244                                                       |
| 10477 | 1.000095              | 2.314259                                                       |
| 10479 | 1.526863              | 2.314274                                                       |
| 10481 | 1.025856              | 2.314290                                                       |
| 10483 | 1.092054              | 2.314305                                                       |
| 10485 | 1.740773              | 2.314320                                                       |

| $n$   | $\frac{\sigma(n)}{n}$ | $\frac{e^\gamma}{2} \log \log n + \frac{0.73...}{\log \log n}$ |
|-------|-----------------------|----------------------------------------------------------------|
| 10487 | 1.000095              | 2.314335                                                       |
| 10489 | 1.060540              | 2.314351                                                       |
| 10491 | 1.441235              | 2.314366                                                       |
| 10493 | 1.143620              | 2.314381                                                       |
| 10495 | 1.200572              | 2.314396                                                       |
| 10497 | 1.333714              | 2.314412                                                       |
| 10499 | 1.000095              | 2.314427                                                       |
| 10501 | 1.000095              | 2.314442                                                       |
| 10503 | 1.485290              | 2.314457                                                       |
| 10505 | 1.315945              | 2.314473                                                       |
| 10507 | 1.218235              | 2.314488                                                       |
| 10509 | 1.388524              | 2.314503                                                       |
| 10511 | 1.045762              | 2.314518                                                       |
| 10513 | 1.000095              | 2.314534                                                       |
| 10515 | 1.602282              | 2.314549                                                       |
| 10517 | 1.078254              | 2.314564                                                       |
| 10519 | 1.021390              | 2.314579                                                       |
| 10521 | 1.660679              | 2.314595                                                       |
| 10523 | 1.060534              | 2.314610                                                       |
| 10525 | 1.242945              | 2.314625                                                       |
| 10527 | 1.516101              | 2.314640                                                       |
| 10529 | 1.000095              | 2.314655                                                       |
| 10531 | 1.000095              | 2.314671                                                       |
| 10533 | 1.333713              | 2.314686                                                       |
| 10535 | 1.428382              | 2.314701                                                       |
| 10537 | 1.028376              | 2.314716                                                       |
| 10539 | 1.445678              | 2.314731                                                       |
| 10541 | 1.020017              | 2.314746                                                       |
| 10543 | 1.078251              | 2.314762                                                       |
| 10545 | 1.729730              | 2.314777                                                       |
| 10547 | 1.023988              | 2.314792                                                       |
| 10549 | 1.255854              | 2.314807                                                       |
| 10551 | 1.333712              | 2.314822                                                       |
| 10553 | 1.022269              | 2.314838                                                       |
| 10555 | 1.200568              | 2.314853                                                       |
| 10557 | 1.636829              | 2.314868                                                       |
| 10559 | 1.000095              | 2.314883                                                       |
| 10561 | 1.022630              | 2.314898                                                       |
| 10563 | 1.526839              | 2.314913                                                       |
| 10565 | 1.200568              | 2.314928                                                       |
| 10567 | 1.000095              | 2.314944                                                       |
| 10569 | 1.441196              | 2.314959                                                       |
| 10571 | 1.127235              | 2.314974                                                       |
| 10573 | 1.019578              | 2.314989                                                       |

| $n$   | $\frac{\sigma(n)}{n}$ | $\frac{e^\gamma}{2} \log \log n + \frac{0.73...}{\log \log n}$ |
|-------|-----------------------|----------------------------------------------------------------|
| 10575 | 1.829220              | 2.315004                                                       |
| 10577 | 1.143614              | 2.315019                                                       |
| 10579 | 1.020890              | 2.315034                                                       |
| 10581 | 1.333711              | 2.315050                                                       |
| 10583 | 1.054521              | 2.315065                                                       |
| 10585 | 1.258385              | 2.315080                                                       |
| 10587 | 1.333711              | 2.315095                                                       |
| 10589 | 1.000094              | 2.315110                                                       |
| 10591 | 1.223680              | 2.315125                                                       |
| 10593 | 1.590484              | 2.315140                                                       |
| 10595 | 1.300236              | 2.315155                                                       |
| 10597 | 1.000094              | 2.315170                                                       |
| 10599 | 1.333711              | 2.315185                                                       |
| 10601 | 1.000094              | 2.315201                                                       |
| 10603 | 1.045742              | 2.315216                                                       |
| 10605 | 1.846676              | 2.315231                                                       |
| 10607 | 1.000094              | 2.315246                                                       |
| 10609 | 1.009803              | 2.315261                                                       |
| 10611 | 1.505230              | 2.315276                                                       |
| 10613 | 1.000094              | 2.315291                                                       |
| 10615 | 1.315874              | 2.315306                                                       |
| 10617 | 1.333710              | 2.315321                                                       |
| 10619 | 1.202373              | 2.315336                                                       |
| 10621 | 1.159966              | 2.315351                                                       |
| 10623 | 1.333710              | 2.315366                                                       |
| 10625 | 1.323106              | 2.315381                                                       |
| 10627 | 1.000094              | 2.315396                                                       |
| 10629 | 1.445668              | 2.315411                                                       |
| 10631 | 1.000094              | 2.315427                                                       |
| 10633 | 1.203799              | 2.315442                                                       |
| 10635 | 1.602257              | 2.315457                                                       |
| 10637 | 1.092037              | 2.315472                                                       |
| 10639 | 1.000094              | 2.315487                                                       |
| 10641 | 1.333709              | 2.315502                                                       |
| 10643 | 1.037302              | 2.315517                                                       |
| 10645 | 1.200564              | 2.315532                                                       |
| 10647 | 1.787546              | 2.315547                                                       |
| 10649 | 1.045732              | 2.315562                                                       |
| 10651 | 1.000094              | 2.315577                                                       |
| 10653 | 1.378767              | 2.315592                                                       |
| 10655 | 1.200563              | 2.315607                                                       |
| 10657 | 1.000094              | 2.315622                                                       |
| 10659 | 1.621165              | 2.315637                                                       |
| 10661 | 1.143608              | 2.315652                                                       |

| $n$   | $\frac{\sigma(n)}{n}$ | $\frac{e^\gamma}{2} \log \log n + \frac{0.73...}{\log \log n}$ |
|-------|-----------------------|----------------------------------------------------------------|
| 10663 | 1.000094              | 2.315667                                                       |
| 10665 | 1.800281              | 2.315682                                                       |
| 10667 | 1.000094              | 2.315697                                                       |
| 10669 | 1.025776              | 2.315712                                                       |
| 10671 | 1.333708              | 2.315727                                                       |
| 10673 | 1.078235              | 2.315742                                                       |
| 10675 | 1.440375              | 2.315757                                                       |
| 10677 | 1.333708              | 2.315772                                                       |
| 10679 | 1.022568              | 2.315787                                                       |
| 10681 | 1.092033              | 2.315802                                                       |
| 10683 | 1.445661              | 2.315817                                                       |
| 10685 | 1.200562              | 2.315832                                                       |
| 10687 | 1.000094              | 2.315847                                                       |
| 10689 | 1.526803              | 2.315861                                                       |
| 10691 | 1.000094              | 2.315876                                                       |
| 10693 | 1.090994              | 2.315891                                                       |
| 10695 | 1.723422              | 2.315906                                                       |
| 10697 | 1.054501              | 2.315921                                                       |
| 10699 | 1.078232              | 2.315936                                                       |
| 10701 | 1.530698              | 2.315951                                                       |
| 10703 | 1.255723              | 2.315966                                                       |
| 10705 | 1.200560              | 2.315981                                                       |
| 10707 | 1.380779              | 2.315996                                                       |
| 10709 | 1.000093              | 2.316011                                                       |
| 10711 | 1.000093              | 2.316026                                                       |
| 10713 | 1.333707              | 2.316041                                                       |
| 10715 | 1.200560              | 2.316056                                                       |
| 10717 | 1.143604              | 2.316071                                                       |
| 10719 | 1.485213              | 2.316085                                                       |
| 10721 | 1.020800              | 2.316100                                                       |
| 10723 | 1.000093              | 2.316115                                                       |
| 10725 | 1.942378              | 2.316130                                                       |
| 10727 | 1.060502              | 2.316145                                                       |
| 10729 | 1.000093              | 2.316160                                                       |
| 10731 | 1.572267              | 2.316175                                                       |
| 10733 | 1.000093              | 2.316190                                                       |
| 10735 | 1.274336              | 2.316205                                                       |
| 10737 | 1.445655              | 2.316220                                                       |
| 10739 | 1.000093              | 2.316234                                                       |
| 10741 | 1.045713              | 2.316249                                                       |
| 10743 | 1.333706              | 2.316264                                                       |
| 10745 | 1.375896              | 2.316279                                                       |
| 10747 | 1.092026              | 2.316294                                                       |
| 10749 | 1.333705              | 2.316309                                                       |



| $n$   | $\frac{\sigma(n)}{n}$ | $\frac{e^\gamma}{2} \log \log n + \frac{0.73...}{\log \log n}$ |
|-------|-----------------------|----------------------------------------------------------------|
| 10751 | 1.078225              | 2.316324                                                       |
| 10753 | 1.000093              | 2.316338                                                       |
| 10755 | 1.740586              | 2.316353                                                       |
| 10757 | 1.035233              | 2.316368                                                       |
| 10759 | 1.204573              | 2.316383                                                       |
| 10761 | 1.418456              | 2.316398                                                       |
| 10763 | 1.025736              | 2.316413                                                       |
| 10765 | 1.200557              | 2.316428                                                       |
| 10767 | 1.383487              | 2.316442                                                       |
| 10769 | 1.111524              | 2.316457                                                       |
| 10771 | 1.000093              | 2.316472                                                       |
| 10773 | 1.797085              | 2.316487                                                       |
| 10775 | 1.242877              | 2.316502                                                       |
| 10777 | 1.078222              | 2.316517                                                       |
| 10779 | 1.333704              | 2.316531                                                       |
| 10781 | 1.000093              | 2.316546                                                       |
| 10783 | 1.028285              | 2.316561                                                       |
| 10785 | 1.602225              | 2.316576                                                       |
| 10787 | 1.210346              | 2.316591                                                       |
| 10789 | 1.000093              | 2.316605                                                       |
| 10791 | 1.590214              | 2.316620                                                       |
| 10793 | 1.027333              | 2.316635                                                       |
| 10795 | 1.280593              | 2.316650                                                       |
| 10797 | 1.378161              | 2.316665                                                       |
| 10799 | 1.000093              | 2.316679                                                       |
| 10801 | 1.143598              | 2.316694                                                       |
| 10803 | 1.441081              | 2.316709                                                       |
| 10805 | 1.200555              | 2.316724                                                       |
| 10807 | 1.019339              | 2.316738                                                       |
| 10809 | 1.445647              | 2.316753                                                       |
| 10811 | 1.054482              | 2.316768                                                       |
| 10813 | 1.092019              | 2.316783                                                       |
| 10815 | 1.846325              | 2.316798                                                       |
| 10817 | 1.037256              | 2.316812                                                       |
| 10819 | 1.035216              | 2.316827                                                       |
| 10821 | 1.333703              | 2.316842                                                       |
| 10823 | 1.020050              | 2.316857                                                       |
| 10825 | 1.242864              | 2.316871                                                       |
| 10827 | 1.485176              | 2.316886                                                       |
| 10829 | 1.326438              | 2.316901                                                       |
| 10831 | 1.000092              | 2.316916                                                       |
| 10833 | 1.400166              | 2.316930                                                       |
| 10835 | 1.315736              | 2.316945                                                       |
| 10837 | 1.000092              | 2.316960                                                       |

| $n$   | $\frac{\sigma(n)}{n}$ | $\frac{e^\gamma}{2} \log \log n + \frac{0.73...}{\log \log n}$ |
|-------|-----------------------|----------------------------------------------------------------|
| 10839 | 1.333702              | 2.316975                                                       |
| 10841 | 1.030532              | 2.316989                                                       |
| 10843 | 1.143595              | 2.317004                                                       |
| 10845 | 1.740526              | 2.317019                                                       |
| 10847 | 1.000092              | 2.317033                                                       |
| 10849 | 1.054475              | 2.317048                                                       |
| 10851 | 1.333702              | 2.317063                                                       |
| 10853 | 1.000092              | 2.317078                                                       |
| 10855 | 1.300046              | 2.317092                                                       |
| 10857 | 1.697707              | 2.317107                                                       |
| 10859 | 1.000092              | 2.317122                                                       |
| 10861 | 1.000092              | 2.317136                                                       |
| 10863 | 1.550953              | 2.317151                                                       |
| 10865 | 1.252462              | 2.317166                                                       |
| 10867 | 1.000092              | 2.317180                                                       |
| 10869 | 1.333701              | 2.317195                                                       |
| 10871 | 1.143593              | 2.317210                                                       |
| 10873 | 1.019774              | 2.317225                                                       |
| 10875 | 1.721379              | 2.317239                                                       |
| 10877 | 1.020502              | 2.317254                                                       |
| 10879 | 1.164813              | 2.317269                                                       |
| 10881 | 1.646907              | 2.317283                                                       |
| 10883 | 1.000092              | 2.317298                                                       |
| 10885 | 1.375838              | 2.317313                                                       |
| 10887 | 1.410857              | 2.317327                                                       |
| 10889 | 1.000092              | 2.317342                                                       |
| 10891 | 1.000092              | 2.317356                                                       |
| 10893 | 1.333701              | 2.317371                                                       |
| 10895 | 1.200551              | 2.317386                                                       |
| 10897 | 1.060475              | 2.317400                                                       |
| 10899 | 1.660336              | 2.317415                                                       |
| 10901 | 1.092010              | 2.317430                                                       |
| 10903 | 1.000092              | 2.317444                                                       |
| 10905 | 1.602201              | 2.317459                                                       |
| 10907 | 1.078207              | 2.317474                                                       |
| 10909 | 1.000092              | 2.317488                                                       |
| 10911 | 1.333700              | 2.317503                                                       |
| 10913 | 1.143590              | 2.317517                                                       |
| 10915 | 1.253321              | 2.317532                                                       |
| 10917 | 1.445635              | 2.317547                                                       |
| 10919 | 1.022072              | 2.317561                                                       |
| 10921 | 1.021152              | 2.317576                                                       |
| 10923 | 1.458940              | 2.317591                                                       |
| 10925 | 1.362014              | 2.317605                                                       |

| $n$   | $\frac{\sigma(n)}{n}$ | $\frac{e^\gamma}{2} \log \log n + \frac{0.73\dots}{\log \log n}$ |
|-------|-----------------------|------------------------------------------------------------------|
| 10927 | 1.168482              | 2.317620                                                         |
| 10929 | 1.333699              | 2.317634                                                         |
| 10931 | 1.060470              | 2.317649                                                         |
| 10933 | 1.115339              | 2.317664                                                         |
| 10935 | 1.799726              | 2.317678                                                         |
| 10937 | 1.000091              | 2.317693                                                         |
| 10939 | 1.000091              | 2.317707                                                         |
| 10941 | 1.526734              | 2.317722                                                         |
| 10943 | 1.035182              | 2.317736                                                         |
| 10945 | 1.315669              | 2.317751                                                         |
| 10947 | 1.381200              | 2.317766                                                         |
| 10949 | 1.000091              | 2.317780                                                         |
| 10951 | 1.025660              | 2.317795                                                         |
| 10953 | 1.445631              | 2.317809                                                         |
| 10955 | 1.375810              | 2.317824                                                         |
| 10957 | 1.000091              | 2.317838                                                         |
| 10959 | 1.441007              | 2.317853                                                         |
| 10961 | 1.019250              | 2.317868                                                         |
| 10963 | 1.054456              | 2.317882                                                         |
| 10965 | 1.733516              | 2.317897                                                         |
| 10967 | 1.092003              | 2.317911                                                         |
| 10969 | 1.143586              | 2.317926                                                         |
| 10971 | 1.535685              | 2.317940                                                         |
| 10973 | 1.000091              | 2.317955                                                         |
| 10975 | 1.242825              | 2.317969                                                         |
| 10977 | 1.333698              | 2.317984                                                         |
| 10979 | 1.000091              | 2.317998                                                         |
| 10981 | 1.019944              | 2.318013                                                         |
| 10983 | 1.526723              | 2.318027                                                         |
| 10985 | 1.299954              | 2.318042                                                         |
| 10987 | 1.000091              | 2.318056                                                         |
| 10989 | 1.659842              | 2.318071                                                         |
| 10991 | 1.037212              | 2.318085                                                         |
| 10993 | 1.000091              | 2.318100                                                         |
| 10995 | 1.602183              | 2.318114                                                         |
| 10997 | 1.143585              | 2.318129                                                         |
| 10999 | 1.060460              | 2.318143                                                         |
| 11001 | 1.410781              | 2.318158                                                         |
| 11003 | 1.000091              | 2.318172                                                         |
| 11005 | 1.256156              | 2.318187                                                         |
| 11007 | 1.445626              | 2.318201                                                         |
| 11009 | 1.019166              | 2.318216                                                         |
| 11011 | 1.352829              | 2.318230                                                         |
| 11013 | 1.333697              | 2.318245                                                         |

| $n$   | $\frac{\sigma(n)}{n}$ | $\frac{e^\gamma}{2} \log \log n + \frac{0.73...}{\log \log n}$ |
|-------|-----------------------|----------------------------------------------------------------|
| 11015 | 1.200545              | 2.318259                                                       |
| 11017 | 1.045657              | 2.318274                                                       |
| 11019 | 1.333696              | 2.318288                                                       |
| 11021 | 1.019145              | 2.318303                                                       |
| 11023 | 1.020412              | 2.318317                                                       |
| 11025 | 2.083537              | 2.318332                                                       |
| 11027 | 1.000091              | 2.318346                                                       |
| 11029 | 1.028198              | 2.318361                                                       |
| 11031 | 1.333696              | 2.318375                                                       |
| 11033 | 1.174658              | 2.318389                                                       |
| 11035 | 1.200544              | 2.318404                                                       |
| 11037 | 1.440971              | 2.318418                                                       |
| 11039 | 1.217502              | 2.318433                                                       |
| 11041 | 1.022009              | 2.318447                                                       |
| 11043 | 1.485104              | 2.318462                                                       |
| 11045 | 1.226075              | 2.318476                                                       |
| 11047 | 1.000091              | 2.318491                                                       |
| 11049 | 1.390171              | 2.318505                                                       |
| 11051 | 1.027237              | 2.318519                                                       |
| 11053 | 1.143581              | 2.318534                                                       |
| 11055 | 1.771506              | 2.318548                                                       |
| 11057 | 1.000090              | 2.318563                                                       |
| 11059 | 1.000090              | 2.318577                                                       |
| 11061 | 1.445620              | 2.318591                                                       |
| 11063 | 1.154117              | 2.318606                                                       |
| 11065 | 1.200542              | 2.318620                                                       |
| 11067 | 1.665492              | 2.318635                                                       |
| 11069 | 1.000090              | 2.318649                                                       |
| 11071 | 1.000090              | 2.318663                                                       |
| 11073 | 1.333695              | 2.318678                                                       |
| 11075 | 1.242799              | 2.318692                                                       |
| 11077 | 1.169992              | 2.318707                                                       |
| 11079 | 1.445618              | 2.318721                                                       |
| 11081 | 1.143579              | 2.318735                                                       |
| 11083 | 1.000090              | 2.318750                                                       |
| 11085 | 1.602165              | 2.318764                                                       |
| 11087 | 1.000090              | 2.318779                                                       |
| 11089 | 1.078186              | 2.318793                                                       |
| 11091 | 1.333694              | 2.318807                                                       |
| 11093 | 1.000090              | 2.318822                                                       |
| 11095 | 1.375755              | 2.318836                                                       |
| 11097 | 1.504731              | 2.318850                                                       |
| 11099 | 1.091990              | 2.318865                                                       |
| 11101 | 1.060445              | 2.318879                                                       |

| $n$   | $\frac{\sigma(n)}{n}$ | $\frac{e^\gamma}{2} \log \log n + \frac{0.73\dots}{\log \log n}$ |
|-------|-----------------------|------------------------------------------------------------------|
| 11103 | 1.333694              | 2.318893                                                         |
| 11105 | 1.200540              | 2.318908                                                         |
| 11107 | 1.037184              | 2.318922                                                         |
| 11109 | 1.592943              | 2.318936                                                         |
| 11111 | 1.028170              | 2.318951                                                         |
| 11113 | 1.000090              | 2.318965                                                         |
| 11115 | 1.964912              | 2.318979                                                         |
| 11117 | 1.000090              | 2.318994                                                         |
| 11119 | 1.000090              | 2.319008                                                         |
| 11121 | 1.458862              | 2.319022                                                         |
| 11123 | 1.168390              | 2.319037                                                         |
| 11125 | 1.262022              | 2.319051                                                         |
| 11127 | 1.333693              | 2.319065                                                         |
| 11129 | 1.035133              | 2.319080                                                         |
| 11131 | 1.000090              | 2.319094                                                         |
| 11133 | 1.445612              | 2.319108                                                         |
| 11135 | 1.280287              | 2.319123                                                         |
| 11137 | 1.201042              | 2.319137                                                         |
| 11139 | 1.378939              | 2.319151                                                         |
| 11141 | 1.078180              | 2.319165                                                         |
| 11143 | 1.091986              | 2.319180                                                         |
| 11145 | 1.602153              | 2.319194                                                         |
| 11147 | 1.020544              | 2.319208                                                         |
| 11149 | 1.000090              | 2.319223                                                         |
| 11151 | 1.721819              | 2.319237                                                         |
| 11153 | 1.054425              | 2.319251                                                         |
| 11155 | 1.265083              | 2.319265                                                         |
| 11157 | 1.333692              | 2.319280                                                         |
| 11159 | 1.000090              | 2.319294                                                         |
| 11161 | 1.000090              | 2.319308                                                         |
| 11163 | 1.355550              | 2.319323                                                         |
| 11165 | 1.547694              | 2.319337                                                         |
| 11167 | 1.078177              | 2.319351                                                         |
| 11169 | 1.550363              | 2.319365                                                         |
| 11171 | 1.000090              | 2.319380                                                         |
| 11173 | 1.000090              | 2.319394                                                         |
| 11175 | 1.664430              | 2.319408                                                         |
| 11177 | 1.000089              | 2.319422                                                         |
| 11179 | 1.143573              | 2.319437                                                         |
| 11181 | 1.333691              | 2.319451                                                         |
| 11183 | 1.023697              | 2.319465                                                         |
| 11185 | 1.200536              | 2.319479                                                         |
| 11187 | 1.589702              | 2.319494                                                         |
| 11189 | 1.021003              | 2.319508                                                         |

| $n$   | $\frac{\sigma(n)}{n}$ | $\frac{e^\gamma}{2} \log \log n + \frac{0.73\dots}{\log \log n}$ |
|-------|-----------------------|------------------------------------------------------------------|
| 11191 | 1.089447              | 2.319522                                                         |
| 11193 | 1.681051              | 2.319536                                                         |
| 11195 | 1.200536              | 2.319550                                                         |
| 11197 | 1.000089              | 2.319565                                                         |
| 11199 | 1.333691              | 2.319579                                                         |
| 11201 | 1.045621              | 2.319593                                                         |
| 11203 | 1.060430              | 2.319607                                                         |
| 11205 | 1.799197              | 2.319622                                                         |
| 11207 | 1.143571              | 2.319636                                                         |
| 11209 | 1.091980              | 2.319650                                                         |
| 11211 | 1.382927              | 2.319664                                                         |
| 11213 | 1.000089              | 2.319678                                                         |
| 11215 | 1.200535              | 2.319693                                                         |
| 11217 | 1.333690              | 2.319707                                                         |
| 11219 | 1.078171              | 2.319721                                                         |
| 11221 | 1.168345              | 2.319735                                                         |
| 11223 | 1.529003              | 2.319749                                                         |
| 11225 | 1.242762              | 2.319763                                                         |
| 11227 | 1.018972              | 2.319778                                                         |
| 11229 | 1.410633              | 2.319792                                                         |
| 11231 | 1.091978              | 2.319806                                                         |
| 11233 | 1.025550              | 2.319820                                                         |
| 11235 | 1.845661              | 2.319834                                                         |
| 11237 | 1.060425              | 2.319848                                                         |
| 11239 | 1.000089              | 2.319863                                                         |
| 11241 | 1.445601              | 2.319877                                                         |
| 11243 | 1.000089              | 2.319891                                                         |
| 11245 | 1.299778              | 2.319905                                                         |
| 11247 | 1.399840              | 2.319919                                                         |
| 11249 | 1.143568              | 2.319933                                                         |
| 11251 | 1.000089              | 2.319948                                                         |
| 11253 | 1.512841              | 2.319962                                                         |
| 11255 | 1.200533              | 2.319976                                                         |
| 11257 | 1.000089              | 2.319990                                                         |
| 11259 | 1.504574              | 2.320004                                                         |
| 11261 | 1.000089              | 2.320018                                                         |
| 11263 | 1.143567              | 2.320032                                                         |
| 11265 | 1.602130              | 2.320046                                                         |
| 11267 | 1.054407              | 2.320061                                                         |
| 11269 | 1.022273              | 2.320075                                                         |
| 11271 | 1.525330              | 2.320089                                                         |
| 11273 | 1.000089              | 2.320103                                                         |
| 11275 | 1.385721              | 2.320117                                                         |
| 11277 | 1.660016              | 2.320131                                                         |

| $n$   | $\frac{\sigma(n)}{n}$ | $\frac{e^\gamma}{2} \log \log n + \frac{0.73\dots}{\log \log n}$ |
|-------|-----------------------|------------------------------------------------------------------|
| 11279 | 1.000089              | 2.320145                                                         |
| 11281 | 1.037142              | 2.320159                                                         |
| 11283 | 1.333688              | 2.320173                                                         |
| 11285 | 1.252636              | 2.320188                                                         |
| 11287 | 1.000089              | 2.320202                                                         |
| 11289 | 1.377624              | 2.320216                                                         |
| 11291 | 1.143566              | 2.320230                                                         |
| 11293 | 1.045603              | 2.320244                                                         |
| 11295 | 1.740239              | 2.320258                                                         |
| 11297 | 1.189696              | 2.320272                                                         |
| 11299 | 1.000089              | 2.320286                                                         |
| 11301 | 1.333687              | 2.320300                                                         |
| 11303 | 1.019198              | 2.320314                                                         |
| 11305 | 1.528527              | 2.320328                                                         |
| 11307 | 1.333687              | 2.320342                                                         |
| 11309 | 1.027147              | 2.320357                                                         |
| 11311 | 1.000088              | 2.320371                                                         |
| 11313 | 1.485017              | 2.320385                                                         |
| 11315 | 1.255678              | 2.320399                                                         |
| 11317 | 1.000088              | 2.320413                                                         |
| 11319 | 1.696263              | 2.320427                                                         |
| 11321 | 1.000088              | 2.320441                                                         |
| 11323 | 1.099002              | 2.320455                                                         |
| 11325 | 1.664283              | 2.320469                                                         |
| 11327 | 1.025514              | 2.320483                                                         |
| 11329 | 1.000088              | 2.320497                                                         |
| 11331 | 1.445592              | 2.320511                                                         |
| 11333 | 1.143563              | 2.320525                                                         |
| 11335 | 1.200529              | 2.320539                                                         |
| 11337 | 1.333686              | 2.320553                                                         |
| 11339 | 1.142958              | 2.320567                                                         |
| 11341 | 1.091967              | 2.320581                                                         |
| 11343 | 1.410562              | 2.320595                                                         |
| 11345 | 1.200529              | 2.320609                                                         |
| 11347 | 1.143562              | 2.320623                                                         |
| 11349 | 1.571592              | 2.320637                                                         |
| 11351 | 1.000088              | 2.320651                                                         |
| 11353 | 1.000088              | 2.320665                                                         |
| 11355 | 1.602114              | 2.320679                                                         |
| 11357 | 1.028088              | 2.320693                                                         |
| 11359 | 1.030372              | 2.320707                                                         |
| 11361 | 1.526626              | 2.320721                                                         |
| 11363 | 1.091965              | 2.320735                                                         |
| 11365 | 1.200528              | 2.320749                                                         |

| $n$   | $\frac{\sigma(n)}{n}$ | $\frac{e^\gamma}{2} \log \log n + \frac{0.73...}{\log \log n}$ |
|-------|-----------------------|----------------------------------------------------------------|
| 11367 | 1.485000              | 2.320763                                                       |
| 11369 | 1.000088              | 2.320777                                                       |
| 11371 | 1.019435              | 2.320791                                                       |
| 11373 | 1.418095              | 2.320805                                                       |
| 11375 | 1.536000              | 2.320819                                                       |
| 11377 | 1.035071              | 2.320833                                                       |
| 11379 | 1.333685              | 2.320847                                                       |
| 11381 | 1.054389              | 2.320861                                                       |
| 11383 | 1.000088              | 2.320875                                                       |
| 11385 | 1.973123              | 2.320889                                                       |
| 11387 | 1.022218              | 2.320903                                                       |
| 11389 | 1.143560              | 2.320917                                                       |
| 11391 | 1.333684              | 2.320931                                                       |
| 11393 | 1.000088              | 2.320945                                                       |
| 11395 | 1.251075              | 2.320959                                                       |
| 11397 | 1.389839              | 2.320973                                                       |
| 11399 | 1.000088              | 2.320987                                                       |
| 11401 | 1.078151              | 2.321001                                                       |
| 11403 | 1.659914              | 2.321015                                                       |
| 11405 | 1.200526              | 2.321028                                                       |
| 11407 | 1.174016              | 2.321042                                                       |
| 11409 | 1.333684              | 2.321056                                                       |
| 11411 | 1.000088              | 2.321070                                                       |
| 11413 | 1.018838              | 2.321084                                                       |
| 11415 | 1.602102              | 2.321098                                                       |
| 11417 | 1.168258              | 2.321112                                                       |
| 11419 | 1.054383              | 2.321126                                                       |
| 11421 | 1.529814              | 2.321140                                                       |
| 11423 | 1.000088              | 2.321154                                                       |
| 11425 | 1.242713              | 2.321168                                                       |
| 11427 | 1.440798              | 2.321182                                                       |
| 11429 | 1.091959              | 2.321196                                                       |
| 11431 | 1.209343              | 2.321209                                                       |
| 11433 | 1.382664              | 2.321223                                                       |
| 11435 | 1.200525              | 2.321237                                                       |
| 11437 | 1.000087              | 2.321251                                                       |
| 11439 | 1.527406              | 2.321265                                                       |
| 11441 | 1.060397              | 2.321279                                                       |
| 11443 | 1.000087              | 2.321293                                                       |
| 11445 | 1.845347              | 2.321307                                                       |
| 11447 | 1.000087              | 2.321321                                                       |
| 11449 | 1.009433              | 2.321334                                                       |
| 11451 | 1.458737              | 2.321348                                                       |
| 11453 | 1.078145              | 2.321362                                                       |



| $n$   | $\frac{\sigma(n)}{n}$ | $\frac{e^\gamma}{2} \log \log n + \frac{0.73...}{\log \log n}$ |
|-------|-----------------------|----------------------------------------------------------------|
| 11455 | 1.257093              | 2.321376                                                       |
| 11457 | 1.543161              | 2.321390                                                       |
| 11459 | 1.143555              | 2.321404                                                       |
| 11461 | 1.020155              | 2.321418                                                       |
| 11463 | 1.333682              | 2.321431                                                       |
| 11465 | 1.200523              | 2.321445                                                       |
| 11467 | 1.000087              | 2.321459                                                       |
| 11469 | 1.333682              | 2.321473                                                       |
| 11471 | 1.000087              | 2.321487                                                       |
| 11473 | 1.255121              | 2.321501                                                       |
| 11475 | 1.945098              | 2.321515                                                       |
| 11477 | 1.045569              | 2.321528                                                       |
| 11479 | 1.078143              | 2.321542                                                       |
| 11481 | 1.379671              | 2.321556                                                       |
| 11483 | 1.000087              | 2.321570                                                       |
| 11485 | 1.200522              | 2.321584                                                       |
| 11487 | 1.526595              | 2.321598                                                       |
| 11489 | 1.000087              | 2.321611                                                       |
| 11491 | 1.000087              | 2.321625                                                       |
| 11493 | 1.445576              | 2.321639                                                       |
| 11495 | 1.388430              | 2.321653                                                       |
| 11497 | 1.000087              | 2.321667                                                       |
| 11499 | 1.333681              | 2.321681                                                       |
| 11501 | 1.201982              | 2.321694                                                       |
| 11503 | 1.000087              | 2.321708                                                       |
| 11505 | 1.752282              | 2.321722                                                       |
| 11507 | 1.030329              | 2.321736                                                       |
| 11509 | 1.060388              | 2.321750                                                       |
| 11511 | 1.445574              | 2.321763                                                       |
| 11513 | 1.037089              | 2.321777                                                       |
| 11515 | 1.425619              | 2.321791                                                       |
| 11517 | 1.458713              | 2.321805                                                       |
| 11519 | 1.000087              | 2.321818                                                       |
| 11521 | 1.028036              | 2.321832                                                       |
| 11523 | 1.399636              | 2.321846                                                       |
| 11525 | 1.242690              | 2.321860                                                       |
| 11527 | 1.000087              | 2.321874                                                       |
| 11529 | 1.720878              | 2.321887                                                       |
| 11531 | 1.078137              | 2.321901                                                       |
| 11533 | 1.054366              | 2.321915                                                       |
| 11535 | 1.602081              | 2.321929                                                       |
| 11537 | 1.019329              | 2.321942                                                       |
| 11539 | 1.091949              | 2.321956                                                       |
| 11541 | 1.333680              | 2.321970                                                       |

| $n$   | $\frac{\sigma(n)}{n}$ | $\frac{e^\gamma}{2} \log \log n + \frac{0.73\dots}{\log \log n}$ |
|-------|-----------------------|------------------------------------------------------------------|
| 11543 | 1.222559              | 2.321984                                                         |
| 11545 | 1.200520              | 2.321997                                                         |
| 11547 | 1.445570              | 2.322011                                                         |
| 11549 | 1.000087              | 2.322025                                                         |
| 11551 | 1.000087              | 2.322039                                                         |
| 11553 | 1.333680              | 2.322052                                                         |
| 11555 | 1.200519              | 2.322066                                                         |
| 11557 | 1.240460              | 2.322080                                                         |
| 11559 | 1.333679              | 2.322094                                                         |
| 11561 | 1.091947              | 2.322107                                                         |
| 11563 | 1.035026              | 2.322121                                                         |
| 11565 | 1.740078              | 2.322135                                                         |
| 11567 | 1.027060              | 2.322149                                                         |
| 11569 | 1.045553              | 2.322162                                                         |
| 11571 | 1.659321              | 2.322176                                                         |
| 11573 | 1.020306              | 2.322190                                                         |
| 11575 | 1.242678              | 2.322203                                                         |
| 11577 | 1.417984              | 2.322217                                                         |
| 11579 | 1.000086              | 2.322231                                                         |
| 11581 | 1.030308              | 2.322245                                                         |
| 11583 | 1.754986              | 2.322258                                                         |
| 11585 | 1.375572              | 2.322272                                                         |
| 11587 | 1.000086              | 2.322286                                                         |
| 11589 | 1.333678              | 2.322299                                                         |
| 11591 | 1.020792              | 2.322313                                                         |
| 11593 | 1.000086              | 2.322327                                                         |
| 11595 | 1.602070              | 2.322340                                                         |
| 11597 | 1.000086              | 2.322354                                                         |
| 11599 | 1.143547              | 2.322368                                                         |
| 11601 | 1.445565              | 2.322382                                                         |
| 11603 | 1.028010              | 2.322395                                                         |
| 11605 | 1.315295              | 2.322409                                                         |
| 11607 | 1.377100              | 2.322423                                                         |
| 11609 | 1.157722              | 2.322436                                                         |
| 11611 | 1.060374              | 2.322450                                                         |
| 11613 | 1.570654              | 2.322464                                                         |
| 11615 | 1.264572              | 2.322477                                                         |
| 11617 | 1.000086              | 2.322491                                                         |
| 11619 | 1.445563              | 2.322505                                                         |
| 11621 | 1.000086              | 2.322518                                                         |
| 11623 | 1.022111              | 2.322532                                                         |
| 11625 | 1.717677              | 2.322545                                                         |
| 11627 | 1.255010              | 2.322559                                                         |
| 11629 | 1.037063              | 2.322573                                                         |

| $n$   | $\frac{\sigma(n)}{n}$ | $\frac{e^\gamma}{2} \log \log n + \frac{0.73\dots}{\log \log n}$ |
|-------|-----------------------|------------------------------------------------------------------|
| 11631 | 1.333677              | 2.322586                                                         |
| 11633 | 1.000086              | 2.322600                                                         |
| 11635 | 1.299527              | 2.322614                                                         |
| 11637 | 1.484919              | 2.322627                                                         |
| 11639 | 1.018644              | 2.322641                                                         |
| 11641 | 1.143544              | 2.322655                                                         |
| 11643 | 1.333677              | 2.322668                                                         |
| 11645 | 1.279863              | 2.322682                                                         |
| 11647 | 1.054349              | 2.322695                                                         |
| 11649 | 1.458666              | 2.322709                                                         |
| 11651 | 1.021715              | 2.322723                                                         |
| 11653 | 1.027032              | 2.322736                                                         |
| 11655 | 2.034492              | 2.322750                                                         |
| 11657 | 1.000086              | 2.322764                                                         |
| 11659 | 1.018955              | 2.322777                                                         |
| 11661 | 1.506560              | 2.322791                                                         |
| 11663 | 1.018606              | 2.322804                                                         |
| 11665 | 1.200514              | 2.322818                                                         |
| 11667 | 1.333676              | 2.322832                                                         |
| 11669 | 1.143543              | 2.322845                                                         |
| 11671 | 1.091937              | 2.322859                                                         |
| 11673 | 1.445558              | 2.322872                                                         |
| 11675 | 1.242655              | 2.322886                                                         |
| 11677 | 1.000086              | 2.322899                                                         |
| 11679 | 1.417930              | 2.322913                                                         |
| 11681 | 1.000086              | 2.322927                                                         |
| 11683 | 1.143542              | 2.322940                                                         |
| 11685 | 1.725289              | 2.322954                                                         |
| 11687 | 1.149996              | 2.322967                                                         |
| 11689 | 1.000086              | 2.322981                                                         |
| 11691 | 1.484903              | 2.322994                                                         |
| 11693 | 1.091935              | 2.323008                                                         |
| 11695 | 1.200513              | 2.323022                                                         |
| 11697 | 1.526545              | 2.323035                                                         |
| 11699 | 1.000085              | 2.323049                                                         |
| 11701 | 1.000085              | 2.323062                                                         |
| 11703 | 1.378108              | 2.323076                                                         |
| 11705 | 1.200513              | 2.323089                                                         |
| 11707 | 1.045528              | 2.323103                                                         |
| 11709 | 1.445555              | 2.323116                                                         |
| 11711 | 1.168133              | 2.323130                                                         |
| 11713 | 1.161786              | 2.323144                                                         |
| 11715 | 1.770038              | 2.323157                                                         |
| 11717 | 1.000085              | 2.323171                                                         |

| $n$   | $\frac{\sigma(n)}{n}$ | $\frac{e^\gamma}{2} \log \log n + \frac{0.73\dots}{\log \log n}$ |
|-------|-----------------------|------------------------------------------------------------------|
| 11719 | 1.000085              | 2.323184                                                         |
| 11721 | 1.333675              | 2.323198                                                         |
| 11723 | 1.054338              | 2.323211                                                         |
| 11725 | 1.438294              | 2.323225                                                         |
| 11727 | 1.445553              | 2.323238                                                         |
| 11729 | 1.030267              | 2.323252                                                         |
| 11731 | 1.000085              | 2.323265                                                         |
| 11733 | 1.333674              | 2.323279                                                         |
| 11735 | 1.200511              | 2.323292                                                         |
| 11737 | 1.110505              | 2.323306                                                         |
| 11739 | 1.679189              | 2.323319                                                         |
| 11741 | 1.022059              | 2.323333                                                         |
| 11743 | 1.000085              | 2.323346                                                         |
| 11745 | 1.854406              | 2.323360                                                         |
| 11747 | 1.060356              | 2.323373                                                         |
| 11749 | 1.034982              | 2.323387                                                         |
| 11751 | 1.333674              | 2.323400                                                         |
| 11753 | 1.208883              | 2.323414                                                         |
| 11755 | 1.200510              | 2.323427                                                         |
| 11757 | 1.333674              | 2.323441                                                         |
| 11759 | 1.091930              | 2.323454                                                         |
| 11761 | 1.054332              | 2.323468                                                         |
| 11763 | 1.445550              | 2.323481                                                         |
| 11765 | 1.299448              | 2.323495                                                         |
| 11767 | 1.171412              | 2.323508                                                         |
| 11769 | 1.333673              | 2.323522                                                         |
| 11771 | 1.019455              | 2.323535                                                         |
| 11773 | 1.021660              | 2.323549                                                         |
| 11775 | 1.663864              | 2.323562                                                         |
| 11777 | 1.000085              | 2.323575                                                         |
| 11779 | 1.000085              | 2.323589                                                         |
| 11781 | 1.906799              | 2.323602                                                         |
| 11783 | 1.000085              | 2.323616                                                         |
| 11785 | 1.200509              | 2.323629                                                         |
| 11787 | 1.333673              | 2.323643                                                         |
| 11789 | 1.000085              | 2.323656                                                         |
| 11791 | 1.078110              | 2.323670                                                         |
| 11793 | 1.333673              | 2.323683                                                         |
| 11795 | 1.375498              | 2.323696                                                         |
| 11797 | 1.025345              | 2.323710                                                         |
| 11799 | 1.627257              | 2.323723                                                         |
| 11801 | 1.000085              | 2.323737                                                         |
| 11803 | 1.159027              | 2.323750                                                         |
| 11805 | 1.602033              | 2.323764                                                         |

| $n$   | $\frac{\sigma(n)}{n}$ | $\frac{e^\gamma}{2} \log \log n + \frac{0.73...}{\log \log n}$ |
|-------|-----------------------|----------------------------------------------------------------|
| 11807 | 1.000085              | 2.323777                                                       |
| 11809 | 1.168092              | 2.323790                                                       |
| 11811 | 1.387181              | 2.323804                                                       |
| 11813 | 1.000085              | 2.323817                                                       |
| 11815 | 1.279729              | 2.323831                                                       |
| 11817 | 1.570957              | 2.323844                                                       |
| 11819 | 1.023437              | 2.323858                                                       |
| 11821 | 1.000085              | 2.323871                                                       |
| 11823 | 1.526516              | 2.323884                                                       |
| 11825 | 1.384186              | 2.323898                                                       |
| 11827 | 1.000085              | 2.323911                                                       |
| 11829 | 1.333671              | 2.323924                                                       |
| 11831 | 1.000085              | 2.323938                                                       |
| 11833 | 1.000085              | 2.323951                                                       |
| 11835 | 1.739924              | 2.323965                                                       |
| 11837 | 1.216524              | 2.323978                                                       |
| 11839 | 1.000084              | 2.323991                                                       |
| 11841 | 1.333671              | 2.324005                                                       |
| 11843 | 1.078105              | 2.324018                                                       |
| 11845 | 1.264331              | 2.324032                                                       |
| 11847 | 1.458597              | 2.324045                                                       |
| 11849 | 1.088193              | 2.324058                                                       |
| 11851 | 1.143532              | 2.324072                                                       |
| 11853 | 1.484856              | 2.324085                                                       |
| 11855 | 1.200506              | 2.324098                                                       |
| 11857 | 1.020157              | 2.324112                                                       |
| 11859 | 1.376170              | 2.324125                                                       |
| 11861 | 1.037012              | 2.324138                                                       |
| 11863 | 1.000084              | 2.324152                                                       |
| 11865 | 1.844753              | 2.324165                                                       |
| 11867 | 1.000084              | 2.324179                                                       |
| 11869 | 1.188980              | 2.324192                                                       |
| 11871 | 1.445540              | 2.324205                                                       |
| 11873 | 1.034953              | 2.324219                                                       |
| 11875 | 1.315368              | 2.324232                                                       |
| 11877 | 1.382167              | 2.324245                                                       |
| 11879 | 1.143531              | 2.324259                                                       |
| 11881 | 1.009258              | 2.324272                                                       |
| 11883 | 1.417824              | 2.324285                                                       |
| 11885 | 1.200505              | 2.324299                                                       |
| 11887 | 1.000084              | 2.324312                                                       |
| 11889 | 1.445538              | 2.324325                                                       |
| 11891 | 1.162560              | 2.324338                                                       |
| 11893 | 1.143530              | 2.324352                                                       |

| $n$   | $\frac{\sigma(n)}{n}$ | $\frac{e^\gamma}{2} \log \log n + \frac{0.73...}{\log \log n}$ |
|-------|-----------------------|----------------------------------------------------------------|
| 11895 | 1.751324              | 2.324365                                                       |
| 11897 | 1.000084              | 2.324378                                                       |
| 11899 | 1.019918              | 2.324392                                                       |
| 11901 | 1.333669              | 2.324405                                                       |
| 11903 | 1.000084              | 2.324418                                                       |
| 11905 | 1.200504              | 2.324432                                                       |
| 11907 | 1.742504              | 2.324445                                                       |
| 11909 | 1.000084              | 2.324458                                                       |
| 11911 | 1.026950              | 2.324472                                                       |
| 11913 | 1.535130              | 2.324485                                                       |
| 11915 | 1.200504              | 2.324498                                                       |
| 11917 | 1.060334              | 2.324511                                                       |
| 11919 | 1.389378              | 2.324525                                                       |
| 11921 | 1.240164              | 2.324538                                                       |
| 11923 | 1.000084              | 2.324551                                                       |
| 11925 | 1.824906              | 2.324565                                                       |
| 11927 | 1.000084              | 2.324578                                                       |
| 11929 | 1.019365              | 2.324591                                                       |
| 11931 | 1.379935              | 2.324604                                                       |
| 11933 | 1.000084              | 2.324618                                                       |
| 11935 | 1.544365              | 2.324631                                                       |
| 11937 | 1.399347              | 2.324644                                                       |
| 11939 | 1.000084              | 2.324657                                                       |
| 11941 | 1.000084              | 2.324671                                                       |
| 11943 | 1.445533              | 2.324684                                                       |
| 11945 | 1.200502              | 2.324697                                                       |
| 11947 | 1.078095              | 2.324710                                                       |
| 11949 | 1.526488              | 2.324724                                                       |
| 11951 | 1.144674              | 2.324737                                                       |
| 11953 | 1.000084              | 2.324750                                                       |
| 11955 | 1.602008              | 2.324763                                                       |
| 11957 | 1.091913              | 2.324777                                                       |
| 11959 | 1.000084              | 2.324790                                                       |
| 11961 | 1.484826              | 2.324803                                                       |
| 11963 | 1.143526              | 2.324816                                                       |
| 11965 | 1.200501              | 2.324830                                                       |
| 11967 | 1.333668              | 2.324843                                                       |
| 11969 | 1.000084              | 2.324856                                                       |
| 11971 | 1.000084              | 2.324869                                                       |
| 11973 | 1.440575              | 2.324882                                                       |
| 11975 | 1.242589              | 2.324896                                                       |
| 11977 | 1.202304              | 2.324909                                                       |
| 11979 | 1.588780              | 2.324922                                                       |
| 11981 | 1.000083              | 2.324935                                                       |

| $n$   | $\frac{\sigma(n)}{n}$ | $\frac{e^\gamma}{2} \log \log n + \frac{0.73\dots}{\log \log n}$ |
|-------|-----------------------|------------------------------------------------------------------|
| 11983 | 1.045481              | 2.324948                                                         |
| 11985 | 1.730163              | 2.324962                                                         |
| 11987 | 1.000083              | 2.324975                                                         |
| 11989 | 1.054300              | 2.324988                                                         |
| 11991 | 1.526478              | 2.325001                                                         |
| 11993 | 1.020595              | 2.325014                                                         |
| 11995 | 1.200500              | 2.325028                                                         |
| 11997 | 1.525715              | 2.325041                                                         |
| 11999 | 1.098092              | 2.325054                                                         |
| 12001 | 1.091909              | 2.325067                                                         |
| 12003 | 1.333667              | 2.325080                                                         |
| 12005 | 1.399917              | 2.325094                                                         |
| 12007 | 1.000083              | 2.325107                                                         |
| 12009 | 1.333666              | 2.325120                                                         |
| 12011 | 1.000083              | 2.325133                                                         |
| 12013 | 1.027886              | 2.325146                                                         |
| 12015 | 1.797753              | 2.325159                                                         |
| 12017 | 1.021553              | 2.325173                                                         |
| 12019 | 1.222065              | 2.325186                                                         |
| 12021 | 1.333666              | 2.325199                                                         |
| 12023 | 1.091907              | 2.325212                                                         |
| 12025 | 1.371476              | 2.325225                                                         |
| 12027 | 1.410160              | 2.325238                                                         |
| 12029 | 1.045473              | 2.325252                                                         |
| 12031 | 1.023356              | 2.325265                                                         |
| 12033 | 1.659437              | 2.325278                                                         |
| 12035 | 1.256336              | 2.325291                                                         |
| 12037 | 1.000083              | 2.325304                                                         |
| 12039 | 1.333666              | 2.325317                                                         |
| 12041 | 1.000083              | 2.325330                                                         |
| 12043 | 1.000083              | 2.325344                                                         |
| 12045 | 1.769365              | 2.325357                                                         |
| 12047 | 1.143521              | 2.325370                                                         |
| 12049 | 1.000083              | 2.325383                                                         |
| 12051 | 1.570658              | 2.325396                                                         |
| 12053 | 1.060317              | 2.325409                                                         |
| 12055 | 1.200498              | 2.325422                                                         |
| 12057 | 1.333665              | 2.325435                                                         |
| 12059 | 1.034912              | 2.325449                                                         |
| 12061 | 1.143520              | 2.325462                                                         |
| 12063 | 1.333665              | 2.325475                                                         |
| 12065 | 1.273104              | 2.325488                                                         |
| 12067 | 1.091904              | 2.325501                                                         |
| 12069 | 1.503853              | 2.325514                                                         |

| $n$   | $\frac{\sigma(n)}{n}$ | $\frac{e^\gamma}{2} \log \log n + \frac{0.73\dots}{\log \log n}$ |
|-------|-----------------------|------------------------------------------------------------------|
| 12071 | 1.000083              | 2.325527                                                         |
| 12073 | 1.000083              | 2.325540                                                         |
| 12075 | 1.971677              | 2.325553                                                         |
| 12077 | 1.078082              | 2.325567                                                         |
| 12079 | 1.025250              | 2.325580                                                         |
| 12081 | 1.333664              | 2.325593                                                         |
| 12083 | 1.026897              | 2.325606                                                         |
| 12085 | 1.200496              | 2.325619                                                         |
| 12087 | 1.548771              | 2.325632                                                         |
| 12089 | 1.254694              | 2.325645                                                         |
| 12091 | 1.018278              | 2.325658                                                         |
| 12093 | 1.389233              | 2.325671                                                         |
| 12095 | 1.250103              | 2.325684                                                         |
| 12097 | 1.000083              | 2.325697                                                         |
| 12099 | 1.381932              | 2.325710                                                         |
| 12101 | 1.000083              | 2.325723                                                         |
| 12103 | 1.318681              | 2.325737                                                         |
| 12105 | 1.739777              | 2.325750                                                         |
| 12107 | 1.000083              | 2.325763                                                         |
| 12109 | 1.000083              | 2.325776                                                         |
| 12111 | 1.458509              | 2.325789                                                         |
| 12113 | 1.000083              | 2.325802                                                         |
| 12115 | 1.200495              | 2.325815                                                         |
| 12117 | 1.526450              | 2.325828                                                         |
| 12119 | 1.000083              | 2.325841                                                         |
| 12121 | 1.140500              | 2.325854                                                         |
| 12123 | 1.484781              | 2.325867                                                         |
| 12125 | 1.260866              | 2.325880                                                         |
| 12127 | 1.020533              | 2.325893                                                         |
| 12129 | 1.440514              | 2.325906                                                         |
| 12131 | 1.143517              | 2.325919                                                         |
| 12133 | 1.091898              | 2.325932                                                         |
| 12135 | 1.601978              | 2.325945                                                         |
| 12137 | 1.023317              | 2.325958                                                         |
| 12139 | 1.021501              | 2.325971                                                         |
| 12141 | 1.541883              | 2.325984                                                         |
| 12143 | 1.000082              | 2.325997                                                         |
| 12145 | 1.375381              | 2.326010                                                         |
| 12147 | 1.333663              | 2.326023                                                         |
| 12149 | 1.000082              | 2.326036                                                         |
| 12151 | 1.036952              | 2.326049                                                         |
| 12153 | 1.333662              | 2.326062                                                         |
| 12155 | 1.492719              | 2.326075                                                         |
| 12157 | 1.000082              | 2.326088                                                         |



| $n$   | $\frac{\sigma(n)}{n}$ | $\frac{e^\gamma}{2} \log \log n + \frac{0.73...}{\log \log n}$ |
|-------|-----------------------|----------------------------------------------------------------|
| 12159 | 1.659347              | 2.326101                                                       |
| 12161 | 1.000082              | 2.326114                                                       |
| 12163 | 1.000082              | 2.326127                                                       |
| 12165 | 1.601973              | 2.326140                                                       |
| 12167 | 1.045451              | 2.326153                                                       |
| 12169 | 1.026872              | 2.326166                                                       |
| 12171 | 1.333662              | 2.326179                                                       |
| 12173 | 1.198718              | 2.326192                                                       |
| 12175 | 1.242546              | 2.326205                                                       |
| 12177 | 1.655580              | 2.326218                                                       |
| 12179 | 1.054274              | 2.326231                                                       |
| 12181 | 1.078072              | 2.326244                                                       |
| 12183 | 1.386851              | 2.326257                                                       |
| 12185 | 1.200492              | 2.326270                                                       |
| 12187 | 1.143514              | 2.326283                                                       |
| 12189 | 1.417672              | 2.326296                                                       |
| 12191 | 1.019769              | 2.326309                                                       |
| 12193 | 1.018617              | 2.326322                                                       |
| 12195 | 1.739729              | 2.326335                                                       |
| 12197 | 1.000082              | 2.326348                                                       |
| 12199 | 1.091893              | 2.326361                                                       |
| 12201 | 1.569707              | 2.326374                                                       |
| 12203 | 1.000082              | 2.326387                                                       |
| 12205 | 1.200492              | 2.326400                                                       |
| 12207 | 1.440485              | 2.326413                                                       |
| 12209 | 1.036940              | 2.326426                                                       |
| 12211 | 1.000082              | 2.326439                                                       |
| 12213 | 1.532793              | 2.326451                                                       |
| 12215 | 1.375358              | 2.326464                                                       |
| 12217 | 1.054269              | 2.326477                                                       |
| 12219 | 1.333661              | 2.326490                                                       |
| 12221 | 1.110056              | 2.326503                                                       |
| 12223 | 1.060296              | 2.326516                                                       |
| 12225 | 1.663476              | 2.326529                                                       |
| 12227 | 1.000082              | 2.326542                                                       |
| 12229 | 1.143511              | 2.326555                                                       |
| 12231 | 1.503720              | 2.326568                                                       |
| 12233 | 1.078068              | 2.326581                                                       |
| 12235 | 1.200490              | 2.326594                                                       |
| 12237 | 1.333660              | 2.326607                                                       |
| 12239 | 1.000082              | 2.326619                                                       |
| 12241 | 1.000082              | 2.326632                                                       |
| 12243 | 1.693703              | 2.326645                                                       |
| 12245 | 1.254390              | 2.326658                                                       |

| $n$   | $\frac{\sigma(n)}{n}$ | $\frac{e^\gamma}{2} \log \log n + \frac{0.73\dots}{\log \log n}$ |
|-------|-----------------------|------------------------------------------------------------------|
| 12247 | 1.030130              | 2.326671                                                         |
| 12249 | 1.445506              | 2.326684                                                         |
| 12251 | 1.000082              | 2.326697                                                         |
| 12253 | 1.000082              | 2.326710                                                         |
| 12255 | 1.723378              | 2.326723                                                         |
| 12257 | 1.221832              | 2.326736                                                         |
| 12259 | 1.151154              | 2.326748                                                         |
| 12261 | 1.375418              | 2.326761                                                         |
| 12263 | 1.000082              | 2.326774                                                         |
| 12265 | 1.314961              | 2.326787                                                         |
| 12267 | 1.526045              | 2.326800                                                         |
| 12269 | 1.000082              | 2.326813                                                         |
| 12271 | 1.143509              | 2.326826                                                         |
| 12273 | 1.333659              | 2.326839                                                         |
| 12275 | 1.242525              | 2.326851                                                         |
| 12277 | 1.000081              | 2.326864                                                         |
| 12279 | 1.333659              | 2.326877                                                         |
| 12281 | 1.000081              | 2.326890                                                         |
| 12283 | 1.019946              | 2.326903                                                         |
| 12285 | 2.188034              | 2.326916                                                         |
| 12287 | 1.091886              | 2.326929                                                         |
| 12289 | 1.000081              | 2.326941                                                         |
| 12291 | 1.417623              | 2.326954                                                         |
| 12293 | 1.054259              | 2.326967                                                         |
| 12295 | 1.200488              | 2.326980                                                         |
| 12297 | 1.333659              | 2.326993                                                         |
| 12299 | 1.167900              | 2.327006                                                         |
| 12301 | 1.000081              | 2.327018                                                         |
| 12303 | 1.445501              | 2.327031                                                         |
| 12305 | 1.263876              | 2.327044                                                         |
| 12307 | 1.034858              | 2.327057                                                         |
| 12309 | 1.458445              | 2.327070                                                         |
| 12311 | 1.078060              | 2.327083                                                         |
| 12313 | 1.143507              | 2.327095                                                         |
| 12315 | 1.601949              | 2.327108                                                         |
| 12317 | 1.018105              | 2.327121                                                         |
| 12319 | 1.018264              | 2.327134                                                         |
| 12321 | 1.484539              | 2.327147                                                         |
| 12323 | 1.000081              | 2.327159                                                         |
| 12325 | 1.358215              | 2.327172                                                         |
| 12327 | 1.526405              | 2.327185                                                         |
| 12329 | 1.000081              | 2.327198                                                         |
| 12331 | 1.167789              | 2.327211                                                         |
| 12333 | 1.333658              | 2.327223                                                         |

| $n$   | $\frac{\sigma(n)}{n}$ | $\frac{e^\gamma}{2} \log \log n + \frac{0.73\dots}{\log \log n}$ |
|-------|-----------------------|------------------------------------------------------------------|
| 12335 | 1.200486              | 2.327236                                                         |
| 12337 | 1.097674              | 2.327249                                                         |
| 12339 | 1.484723              | 2.327262                                                         |
| 12341 | 1.197958              | 2.327275                                                         |
| 12343 | 1.000081              | 2.327287                                                         |
| 12345 | 1.601944              | 2.327300                                                         |
| 12347 | 1.000081              | 2.327313                                                         |
| 12349 | 1.023241              | 2.327326                                                         |
| 12351 | 1.399077              | 2.327339                                                         |
| 12353 | 1.091881              | 2.327351                                                         |
| 12355 | 1.375314              | 2.327364                                                         |
| 12357 | 1.445496              | 2.327377                                                         |
| 12359 | 1.060280              | 2.327390                                                         |
| 12361 | 1.025160              | 2.327402                                                         |
| 12363 | 1.440427              | 2.327415                                                         |
| 12365 | 1.200485              | 2.327428                                                         |
| 12367 | 1.018840              | 2.327441                                                         |
| 12369 | 1.655752              | 2.327454                                                         |
| 12371 | 1.018511              | 2.327466                                                         |
| 12373 | 1.000081              | 2.327479                                                         |
| 12375 | 1.966545              | 2.327492                                                         |
| 12377 | 1.000081              | 2.327505                                                         |
| 12379 | 1.000081              | 2.327517                                                         |
| 12381 | 1.333656              | 2.327530                                                         |
| 12383 | 1.201647              | 2.327543                                                         |
| 12385 | 1.200484              | 2.327555                                                         |
| 12387 | 1.333656              | 2.327568                                                         |
| 12389 | 1.078053              | 2.327581                                                         |
| 12391 | 1.000081              | 2.327594                                                         |
| 12393 | 1.587509              | 2.327606                                                         |
| 12395 | 1.250827              | 2.327619                                                         |
| 12397 | 1.324191              | 2.327632                                                         |
| 12399 | 1.333656              | 2.327645                                                         |
| 12401 | 1.000081              | 2.327657                                                         |
| 12403 | 1.019108              | 2.327670                                                         |
| 12405 | 1.601935              | 2.327683                                                         |
| 12407 | 1.054244              | 2.327696                                                         |
| 12409 | 1.000081              | 2.327708                                                         |
| 12411 | 1.659173              | 2.327721                                                         |
| 12413 | 1.000081              | 2.327734                                                         |
| 12415 | 1.299074              | 2.327746                                                         |
| 12417 | 1.333655              | 2.327759                                                         |
| 12419 | 1.091875              | 2.327772                                                         |
| 12421 | 1.000081              | 2.327784                                                         |

| $n$   | $\frac{\sigma(n)}{n}$ | $\frac{e^\gamma}{2} \log \log n + \frac{0.73\dots}{\log \log n}$ |
|-------|-----------------------|------------------------------------------------------------------|
| 12423 | 1.379377              | 2.327797                                                         |
| 12425 | 1.437103              | 2.327810                                                         |
| 12427 | 1.086988              | 2.327823                                                         |
| 12429 | 1.445490              | 2.327835                                                         |
| 12431 | 1.034832              | 2.327848                                                         |
| 12433 | 1.000080              | 2.327861                                                         |
| 12435 | 1.601930              | 2.327873                                                         |
| 12437 | 1.000080              | 2.327886                                                         |
| 12439 | 1.143500              | 2.327899                                                         |
| 12441 | 1.620449              | 2.327911                                                         |
| 12443 | 1.045407              | 2.327924                                                         |
| 12445 | 1.272800              | 2.327937                                                         |
| 12447 | 1.484695              | 2.327949                                                         |
| 12449 | 1.021769              | 2.327962                                                         |
| 12451 | 1.000080              | 2.327975                                                         |
| 12453 | 1.526379              | 2.327987                                                         |
| 12455 | 1.248655              | 2.328000                                                         |
| 12457 | 1.000080              | 2.328013                                                         |
| 12459 | 1.333654              | 2.328025                                                         |
| 12461 | 1.060268              | 2.328038                                                         |
| 12463 | 1.109845              | 2.328051                                                         |
| 12465 | 1.739591              | 2.328063                                                         |
| 12467 | 1.239753              | 2.328076                                                         |
| 12469 | 1.030075              | 2.328089                                                         |
| 12471 | 1.333654              | 2.328101                                                         |
| 12473 | 1.000080              | 2.328114                                                         |
| 12475 | 1.242485              | 2.328127                                                         |
| 12477 | 1.333654              | 2.328139                                                         |
| 12479 | 1.000080              | 2.328152                                                         |
| 12481 | 1.143498              | 2.328164                                                         |
| 12483 | 1.541296              | 2.328177                                                         |
| 12485 | 1.314858              | 2.328190                                                         |
| 12487 | 1.000080              | 2.328202                                                         |
| 12489 | 1.398991              | 2.328215                                                         |
| 12491 | 1.000080              | 2.328228                                                         |
| 12493 | 1.112783              | 2.328240                                                         |
| 12495 | 1.970708              | 2.328253                                                         |
| 12497 | 1.000080              | 2.328265                                                         |
| 12499 | 1.036883              | 2.328278                                                         |
| 12501 | 1.484681              | 2.328291                                                         |
| 12503 | 1.000080              | 2.328303                                                         |
| 12505 | 1.249420              | 2.328316                                                         |
| 12507 | 1.458383              | 2.328329                                                         |
| 12509 | 1.143497              | 2.328341                                                         |

| $n$   | $\frac{\sigma(n)}{n}$ | $\frac{e^\gamma}{2} \log \log n + \frac{0.73\dots}{\log \log n}$ |
|-------|-----------------------|------------------------------------------------------------------|
| 12511 | 1.000080              | 2.328354                                                         |
| 12513 | 1.378406              | 2.328366                                                         |
| 12515 | 1.200479              | 2.328379                                                         |
| 12517 | 1.000080              | 2.328392                                                         |
| 12519 | 1.570093              | 2.328404                                                         |
| 12521 | 1.054229              | 2.328417                                                         |
| 12523 | 1.143496              | 2.328429                                                         |
| 12525 | 1.663234              | 2.328442                                                         |
| 12527 | 1.000080              | 2.328454                                                         |
| 12529 | 1.172320              | 2.328467                                                         |
| 12531 | 1.333653              | 2.328480                                                         |
| 12533 | 1.018750              | 2.328492                                                         |
| 12535 | 1.263662              | 2.328505                                                         |
| 12537 | 1.659089              | 2.328517                                                         |
| 12539 | 1.000080              | 2.328530                                                         |
| 12541 | 1.000080              | 2.328542                                                         |
| 12543 | 1.381488              | 2.328555                                                         |
| 12545 | 1.299004              | 2.328568                                                         |
| 12547 | 1.000080              | 2.328580                                                         |
| 12549 | 1.377002              | 2.328593                                                         |
| 12551 | 1.254402              | 2.328605                                                         |
| 12553 | 1.000080              | 2.328618                                                         |
| 12555 | 1.850418              | 2.328630                                                         |
| 12557 | 1.036872              | 2.328643                                                         |
| 12559 | 1.054224              | 2.328655                                                         |
| 12561 | 1.375687              | 2.328668                                                         |
| 12563 | 1.060256              | 2.328681                                                         |
| 12565 | 1.375249              | 2.328693                                                         |
| 12567 | 1.375030              | 2.328706                                                         |
| 12569 | 1.000080              | 2.328718                                                         |
| 12571 | 1.078037              | 2.328731                                                         |
| 12573 | 1.588165              | 2.328743                                                         |
| 12575 | 1.242465              | 2.328756                                                         |
| 12577 | 1.000080              | 2.328768                                                         |
| 12579 | 1.526353              | 2.328781                                                         |
| 12581 | 1.045386              | 2.328793                                                         |
| 12583 | 1.000079              | 2.328806                                                         |
| 12585 | 1.601907              | 2.328818                                                         |
| 12587 | 1.027727              | 2.328831                                                         |
| 12589 | 1.000079              | 2.328843                                                         |
| 12591 | 1.445477              | 2.328856                                                         |
| 12593 | 1.167792              | 2.328869                                                         |
| 12595 | 1.314807              | 2.328881                                                         |
| 12597 | 1.600381              | 2.328894                                                         |

| $n$   | $\frac{\sigma(n)}{n}$ | $\frac{e^\gamma}{2} \log \log n + \frac{0.73...}{\log \log n}$ |
|-------|-----------------------|----------------------------------------------------------------|
| 12599 | 1.026748              | 2.328906                                                       |
| 12601 | 1.000079              | 2.328919                                                       |
| 12603 | 1.333651              | 2.328931                                                       |
| 12605 | 1.200476              | 2.328944                                                       |
| 12607 | 1.143492              | 2.328956                                                       |
| 12609 | 1.484654              | 2.328969                                                       |
| 12611 | 1.000079              | 2.328981                                                       |
| 12613 | 1.000079              | 2.328994                                                       |
| 12615 | 1.657075              | 2.329006                                                       |
| 12617 | 1.156535              | 2.329018                                                       |
| 12619 | 1.000079              | 2.329031                                                       |
| 12621 | 1.526345              | 2.329043                                                       |
| 12623 | 1.078032              | 2.329056                                                       |
| 12625 | 1.260356              | 2.329068                                                       |
| 12627 | 1.531955              | 2.329081                                                       |
| 12629 | 1.019558              | 2.329093                                                       |
| 12631 | 1.060249              | 2.329106                                                       |
| 12633 | 1.333650              | 2.329118                                                       |
| 12635 | 1.447408              | 2.329131                                                       |
| 12637 | 1.000079              | 2.329143                                                       |
| 12639 | 1.458343              | 2.329156                                                       |
| 12641 | 1.000079              | 2.329168                                                       |
| 12643 | 1.025073              | 2.329181                                                       |
| 12645 | 1.739502              | 2.329193                                                       |
| 12647 | 1.000079              | 2.329206                                                       |
| 12649 | 1.239624              | 2.329218                                                       |
| 12651 | 1.333650              | 2.329230                                                       |
| 12653 | 1.000079              | 2.329243                                                       |
| 12655 | 1.200474              | 2.329255                                                       |
| 12657 | 1.333649              | 2.329268                                                       |
| 12659 | 1.000079              | 2.329280                                                       |
| 12661 | 1.091857              | 2.329293                                                       |
| 12663 | 1.718392              | 2.329305                                                       |
| 12665 | 1.279116              | 2.329318                                                       |
| 12667 | 1.023131              | 2.329330                                                       |
| 12669 | 1.379114              | 2.329342                                                       |
| 12671 | 1.000079              | 2.329355                                                       |
| 12673 | 1.136274              | 2.329367                                                       |
| 12675 | 1.790296              | 2.329380                                                       |
| 12677 | 1.143488              | 2.329392                                                       |
| 12679 | 1.034782              | 2.329405                                                       |
| 12681 | 1.445470              | 2.329417                                                       |
| 12683 | 1.091855              | 2.329429                                                       |
| 12685 | 1.248719              | 2.329442                                                       |

| $n$   | $\frac{\sigma(n)}{n}$ | $\frac{e^\gamma}{2} \log \log n + \frac{0.73...}{\log \log n}$ |
|-------|-----------------------|----------------------------------------------------------------|
| 12687 | 1.333649              | 2.329454                                                       |
| 12689 | 1.000079              | 2.329467                                                       |
| 12691 | 1.197699              | 2.329479                                                       |
| 12693 | 1.333648              | 2.329491                                                       |
| 12695 | 1.200473              | 2.329504                                                       |
| 12697 | 1.000079              | 2.329516                                                       |
| 12699 | 1.547838              | 2.329529                                                       |
| 12701 | 1.078025              | 2.329541                                                       |
| 12703 | 1.000079              | 2.329553                                                       |
| 12705 | 2.009917              | 2.329566                                                       |
| 12707 | 1.018022              | 2.329578                                                       |
| 12709 | 1.019750              | 2.329591                                                       |
| 12711 | 1.409803              | 2.329603                                                       |
| 12713 | 1.000079              | 2.329615                                                       |
| 12715 | 1.200472              | 2.329628                                                       |
| 12717 | 1.503342              | 2.329640                                                       |
| 12719 | 1.207642              | 2.329652                                                       |
| 12721 | 1.000079              | 2.329665                                                       |
| 12723 | 1.333648              | 2.329677                                                       |
| 12725 | 1.242436              | 2.329690                                                       |
| 12727 | 1.188025              | 2.329702                                                       |
| 12729 | 1.333648              | 2.329714                                                       |
| 12731 | 1.036839              | 2.329727                                                       |
| 12733 | 1.221393              | 2.329739                                                       |
| 12735 | 1.739458              | 2.329751                                                       |
| 12737 | 1.025045              | 2.329764                                                       |
| 12739 | 1.000078              | 2.329776                                                       |
| 12741 | 1.386390              | 2.329788                                                       |
| 12743 | 1.000078              | 2.329801                                                       |
| 12745 | 1.200471              | 2.329813                                                       |
| 12747 | 1.526320              | 2.329826                                                       |
| 12749 | 1.167150              | 2.329838                                                       |
| 12751 | 1.027684              | 2.329850                                                       |
| 12753 | 1.569827              | 2.329863                                                       |
| 12755 | 1.200470              | 2.329875                                                       |
| 12757 | 1.000078              | 2.329887                                                       |
| 12759 | 1.333647              | 2.329900                                                       |
| 12761 | 1.143484              | 2.329912                                                       |
| 12763 | 1.000078              | 2.329924                                                       |
| 12765 | 1.714689              | 2.329937                                                       |
| 12767 | 1.060233              | 2.329949                                                       |
| 12769 | 1.008928              | 2.329961                                                       |
| 12771 | 1.653747              | 2.329974                                                       |
| 12773 | 1.023096              | 2.329986                                                       |

| $n$   | $\frac{\sigma(n)}{n}$ | $\frac{e^\gamma}{2} \log \log n + \frac{0.73\dots}{\log \log n}$ |
|-------|-----------------------|------------------------------------------------------------------|
| 12775 | 1.436556              | 2.329998                                                         |
| 12777 | 1.333646              | 2.330011                                                         |
| 12779 | 1.078019              | 2.330023                                                         |
| 12781 | 1.000078              | 2.330035                                                         |
| 12783 | 1.333646              | 2.330047                                                         |
| 12785 | 1.200469              | 2.330060                                                         |
| 12787 | 1.054196              | 2.330072                                                         |
| 12789 | 1.738213              | 2.330084                                                         |
| 12791 | 1.000078              | 2.330097                                                         |
| 12793 | 1.091847              | 2.330109                                                         |
| 12795 | 1.601876              | 2.330121                                                         |
| 12797 | 1.020239              | 2.330134                                                         |
| 12799 | 1.000078              | 2.330146                                                         |
| 12801 | 1.417389              | 2.330158                                                         |
| 12803 | 1.199719              | 2.330170                                                         |
| 12805 | 1.298868              | 2.330183                                                         |
| 12807 | 1.445460              | 2.330195                                                         |
| 12809 | 1.000078              | 2.330207                                                         |
| 12811 | 1.045352              | 2.330220                                                         |
| 12813 | 1.333646              | 2.330232                                                         |
| 12815 | 1.314709              | 2.330244                                                         |
| 12817 | 1.143481              | 2.330256                                                         |
| 12819 | 1.333645              | 2.330269                                                         |
| 12821 | 1.000078              | 2.330281                                                         |
| 12823 | 1.000078              | 2.330293                                                         |
| 12825 | 1.933723              | 2.330305                                                         |
| 12827 | 1.017853              | 2.330318                                                         |
| 12829 | 1.000078              | 2.330330                                                         |
| 12831 | 1.675941              | 2.330342                                                         |
| 12833 | 1.027663              | 2.330355                                                         |
| 12835 | 1.279003              | 2.330367                                                         |
| 12837 | 1.458285              | 2.330379                                                         |
| 12839 | 1.029987              | 2.330391                                                         |
| 12841 | 1.000078              | 2.330404                                                         |
| 12843 | 1.445457              | 2.330416                                                         |
| 12845 | 1.375165              | 2.330428                                                         |
| 12847 | 1.036818              | 2.330440                                                         |
| 12849 | 1.333645              | 2.330453                                                         |
| 12851 | 1.019687              | 2.330465                                                         |
| 12853 | 1.000078              | 2.330477                                                         |
| 12855 | 1.601867              | 2.330489                                                         |
| 12857 | 1.149879              | 2.330501                                                         |
| 12859 | 1.254219              | 2.330514                                                         |
| 12861 | 1.445455              | 2.330526                                                         |



| $n$   | $\frac{\sigma(n)}{n}$ | $\frac{e^\gamma}{2} \log \log n + \frac{0.73\dots}{\log \log n}$ |
|-------|-----------------------|------------------------------------------------------------------|
| 12863 | 1.054186              | 2.330538                                                         |
| 12865 | 1.253634              | 2.330550                                                         |
| 12867 | 1.333644              | 2.330563                                                         |
| 12869 | 1.060222              | 2.330575                                                         |
| 12871 | 1.021210              | 2.330587                                                         |
| 12873 | 1.526295              | 2.330599                                                         |
| 12875 | 1.260117              | 2.330611                                                         |
| 12877 | 1.018871              | 2.330624                                                         |
| 12879 | 1.526205              | 2.330636                                                         |
| 12881 | 1.091841              | 2.330648                                                         |
| 12883 | 1.078010              | 2.330660                                                         |
| 12885 | 1.601863              | 2.330673                                                         |
| 12887 | 1.167688              | 2.330685                                                         |
| 12889 | 1.000078              | 2.330697                                                         |
| 12891 | 1.333644              | 2.330709                                                         |
| 12893 | 1.000078              | 2.330721                                                         |
| 12895 | 1.200465              | 2.330734                                                         |
| 12897 | 1.445452              | 2.330746                                                         |
| 12899 | 1.000078              | 2.330758                                                         |
| 12901 | 1.215410              | 2.330770                                                         |
| 12903 | 1.607068              | 2.330782                                                         |
| 12905 | 1.255327              | 2.330794                                                         |
| 12907 | 1.000077              | 2.330807                                                         |
| 12909 | 1.440235              | 2.330819                                                         |
| 12911 | 1.000077              | 2.330831                                                         |
| 12913 | 1.029970              | 2.330843                                                         |
| 12915 | 2.029268              | 2.330855                                                         |
| 12917 | 1.000077              | 2.330868                                                         |
| 12919 | 1.000077              | 2.330880                                                         |
| 12921 | 1.374507              | 2.330892                                                         |
| 12923 | 1.000077              | 2.330904                                                         |
| 12925 | 1.381509              | 2.330916                                                         |
| 12927 | 1.386246              | 2.330928                                                         |
| 12929 | 1.143476              | 2.330940                                                         |
| 12931 | 1.020184              | 2.330953                                                         |
| 12933 | 1.484574              | 2.330965                                                         |
| 12935 | 1.298802              | 2.330977                                                         |
| 12937 | 1.060215              | 2.330989                                                         |
| 12939 | 1.409692              | 2.331001                                                         |
| 12941 | 1.000077              | 2.331013                                                         |
| 12943 | 1.170053              | 2.331026                                                         |
| 12945 | 1.601854              | 2.331038                                                         |
| 12947 | 1.109446              | 2.331050                                                         |
| 12949 | 1.045332              | 2.331062                                                         |

| $n$   | $\frac{\sigma(n)}{n}$ | $\frac{e^\gamma}{2} \log \log n + \frac{0.73\dots}{\log \log n}$ |
|-------|-----------------------|------------------------------------------------------------------|
| 12951 | 1.445448              | 2.331074                                                         |
| 12953 | 1.000077              | 2.331086                                                         |
| 12955 | 1.200463              | 2.331098                                                         |
| 12957 | 1.526279              | 2.331111                                                         |
| 12959 | 1.000077              | 2.331123                                                         |
| 12961 | 1.078003              | 2.331135                                                         |
| 12963 | 1.388567              | 2.331147                                                         |
| 12965 | 1.200463              | 2.331159                                                         |
| 12967 | 1.000077              | 2.331171                                                         |
| 12969 | 1.587786              | 2.331183                                                         |
| 12971 | 1.221186              | 2.331195                                                         |
| 12973 | 1.000077              | 2.331207                                                         |
| 12975 | 1.662890              | 2.331220                                                         |
| 12977 | 1.054173              | 2.331232                                                         |
| 12979 | 1.000077              | 2.331244                                                         |
| 12981 | 1.333641              | 2.331256                                                         |
| 12983 | 1.000077              | 2.331268                                                         |
| 12985 | 1.422256              | 2.331280                                                         |
| 12987 | 1.638562              | 2.331292                                                         |
| 12989 | 1.034722              | 2.331304                                                         |
| 12991 | 1.091833              | 2.331316                                                         |
| 12993 | 1.374278              | 2.331329                                                         |
| 12995 | 1.263255              | 2.331341                                                         |
| 12997 | 1.027622              | 2.331353                                                         |
| 12999 | 1.526271              | 2.331365                                                         |
| 13001 | 1.000077              | 2.331377                                                         |
| 13003 | 1.000077              | 2.331389                                                         |
| 13005 | 1.841292              | 2.331401                                                         |
| 13007 | 1.000077              | 2.331413                                                         |
| 13009 | 1.000077              | 2.331425                                                         |
| 13011 | 1.333641              | 2.331437                                                         |
| 13013 | 1.350035              | 2.331449                                                         |
| 13015 | 1.272378              | 2.331461                                                         |
| 13017 | 1.333641              | 2.331473                                                         |
| 13019 | 1.024964              | 2.331486                                                         |
| 13021 | 1.036787              | 2.331498                                                         |
| 13023 | 1.445443              | 2.331510                                                         |
| 13025 | 1.242380              | 2.331522                                                         |
| 13027 | 1.143471              | 2.331534                                                         |
| 13029 | 1.377849              | 2.331546                                                         |
| 13031 | 1.018494              | 2.331558                                                         |
| 13033 | 1.000077              | 2.331570                                                         |
| 13035 | 1.767549              | 2.331582                                                         |
| 13037 | 1.000077              | 2.331594                                                         |

| $n$   | $\frac{\sigma(n)}{n}$ | $\frac{e^\gamma}{2} \log \log n + \frac{0.73\dots}{\log \log n}$ |
|-------|-----------------------|------------------------------------------------------------------|
| 13039 | 1.159598              | 2.331606                                                         |
| 13041 | 1.781458              | 2.331618                                                         |
| 13043 | 1.000077              | 2.331630                                                         |
| 13045 | 1.200460              | 2.331642                                                         |
| 13047 | 1.333640              | 2.331654                                                         |
| 13049 | 1.000077              | 2.331666                                                         |
| 13051 | 1.034710              | 2.331678                                                         |
| 13053 | 1.409638              | 2.331690                                                         |
| 13055 | 1.375105              | 2.331702                                                         |
| 13057 | 1.091828              | 2.331714                                                         |
| 13059 | 1.445440              | 2.331726                                                         |
| 13061 | 1.029936              | 2.331739                                                         |
| 13063 | 1.000077              | 2.331751                                                         |
| 13065 | 1.748794              | 2.331763                                                         |
| 13067 | 1.019362              | 2.331775                                                         |
| 13069 | 1.143469              | 2.331787                                                         |
| 13071 | 1.333639              | 2.331799                                                         |
| 13073 | 1.060200              | 2.331811                                                         |
| 13075 | 1.242371              | 2.331823                                                         |
| 13077 | 1.445439              | 2.331835                                                         |
| 13079 | 1.156052              | 2.331847                                                         |
| 13081 | 1.017659              | 2.331859                                                         |
| 13083 | 1.568448              | 2.331871                                                         |
| 13085 | 1.200459              | 2.331883                                                         |
| 13087 | 1.045312              | 2.331895                                                         |
| 13089 | 1.333639              | 2.331907                                                         |
| 13091 | 1.154992              | 2.331919                                                         |
| 13093 | 1.000076              | 2.331931                                                         |
| 13095 | 1.796105              | 2.331943                                                         |
| 13097 | 1.143468              | 2.331955                                                         |
| 13099 | 1.000076              | 2.331967                                                         |
| 13101 | 1.458209              | 2.331979                                                         |
| 13103 | 1.000076              | 2.331991                                                         |
| 13105 | 1.200458              | 2.332003                                                         |
| 13107 | 1.417258              | 2.332015                                                         |
| 13109 | 1.000076              | 2.332027                                                         |
| 13111 | 1.143467              | 2.332039                                                         |
| 13113 | 1.522764              | 2.332050                                                         |
| 13115 | 1.248037              | 2.332062                                                         |
| 13117 | 1.077990              | 2.332074                                                         |
| 13119 | 1.333638              | 2.332086                                                         |
| 13121 | 1.000076              | 2.332098                                                         |
| 13123 | 1.091824              | 2.332110                                                         |
| 13125 | 1.904152              | 2.332122                                                         |

| $n$   | $\frac{\sigma(n)}{n}$ | $\frac{e^\gamma}{2} \log \log n + \frac{0.73\dots}{\log \log n}$ |
|-------|-----------------------|------------------------------------------------------------------|
| 13127 | 1.000076              | 2.332134                                                         |
| 13129 | 1.054155              | 2.332146                                                         |
| 13131 | 1.445434              | 2.332158                                                         |
| 13133 | 1.045306              | 2.332170                                                         |
| 13135 | 1.249791              | 2.332182                                                         |
| 13137 | 1.388445              | 2.332194                                                         |
| 13139 | 1.143466              | 2.332206                                                         |
| 13141 | 1.060193              | 2.332218                                                         |
| 13143 | 1.440158              | 2.332230                                                         |
| 13145 | 1.314568              | 2.332242                                                         |
| 13147 | 1.000076              | 2.332254                                                         |
| 13149 | 1.484524              | 2.332266                                                         |
| 13151 | 1.000076              | 2.332278                                                         |
| 13153 | 1.143465              | 2.332290                                                         |
| 13155 | 1.601824              | 2.332301                                                         |
| 13157 | 1.021509              | 2.332313                                                         |
| 13159 | 1.000076              | 2.332325                                                         |
| 13161 | 1.378619              | 2.332337                                                         |
| 13163 | 1.000076              | 2.332349                                                         |
| 13165 | 1.200456              | 2.332361                                                         |
| 13167 | 1.895648              | 2.332373                                                         |
| 13169 | 1.077986              | 2.332385                                                         |
| 13171 | 1.000076              | 2.332397                                                         |
| 13173 | 1.333637              | 2.332409                                                         |
| 13175 | 1.355294              | 2.332421                                                         |
| 13177 | 1.000076              | 2.332433                                                         |
| 13179 | 1.398589              | 2.332445                                                         |
| 13181 | 1.167590              | 2.332456                                                         |
| 13183 | 1.000076              | 2.332468                                                         |
| 13185 | 1.739249              | 2.332480                                                         |
| 13187 | 1.000076              | 2.332492                                                         |
| 13189 | 1.109258              | 2.332504                                                         |
| 13191 | 1.333637              | 2.332516                                                         |
| 13193 | 1.018722              | 2.332528                                                         |
| 13195 | 1.527851              | 2.332540                                                         |
| 13197 | 1.374858              | 2.332552                                                         |
| 13199 | 1.020077              | 2.332564                                                         |
| 13201 | 1.026589              | 2.332575                                                         |
| 13203 | 1.502992              | 2.332587                                                         |
| 13205 | 1.272245              | 2.332599                                                         |
| 13207 | 1.024911              | 2.332611                                                         |
| 13209 | 1.657052              | 2.332623                                                         |
| 13211 | 1.091817              | 2.332635                                                         |
| 13213 | 1.019299              | 2.332647                                                         |

| $n$   | $\frac{\sigma(n)}{n}$ | $\frac{e^\gamma}{2} \log \log n + \frac{0.73...}{\log \log n}$ |
|-------|-----------------------|----------------------------------------------------------------|
| 13215 | 1.601816              | 2.332659                                                       |
| 13217 | 1.000076              | 2.332670                                                       |
| 13219 | 1.000076              | 2.332682                                                       |
| 13221 | 1.569322              | 2.332694                                                       |
| 13223 | 1.143462              | 2.332706                                                       |
| 13225 | 1.296257              | 2.332718                                                       |
| 13227 | 1.333636              | 2.332730                                                       |
| 13229 | 1.000076              | 2.332742                                                       |
| 13231 | 1.017610              | 2.332753                                                       |
| 13233 | 1.458173              | 2.332765                                                       |
| 13235 | 1.200453              | 2.332777                                                       |
| 13237 | 1.199063              | 2.332789                                                       |
| 13239 | 1.445426              | 2.332801                                                       |
| 13241 | 1.000076              | 2.332813                                                       |
| 13243 | 1.141735              | 2.332825                                                       |
| 13245 | 1.601812              | 2.332836                                                       |
| 13247 | 1.077980              | 2.332848                                                       |
| 13249 | 1.000075              | 2.332860                                                       |
| 13251 | 1.526224              | 2.332872                                                       |
| 13253 | 1.036746              | 2.332884                                                       |
| 13255 | 1.314523              | 2.332896                                                       |
| 13257 | 1.484499              | 2.332907                                                       |
| 13259 | 1.000075              | 2.332919                                                       |
| 13261 | 1.018023              | 2.332931                                                       |
| 13263 | 1.333635              | 2.332943                                                       |
| 13265 | 1.375047              | 2.332955                                                       |
| 13267 | 1.000075              | 2.332967                                                       |
| 13269 | 1.333635              | 2.332978                                                       |
| 13271 | 1.045287              | 2.332990                                                       |
| 13273 | 1.077978              | 2.333002                                                       |
| 13275 | 1.821469              | 2.333014                                                       |
| 13277 | 1.171349              | 2.333026                                                       |
| 13279 | 1.167558              | 2.333037                                                       |
| 13281 | 1.409532              | 2.333049                                                       |
| 13283 | 1.029888              | 2.333061                                                       |
| 13285 | 1.200452              | 2.333073                                                       |
| 13287 | 1.377587              | 2.333085                                                       |
| 13289 | 1.017684              | 2.333097                                                       |
| 13291 | 1.000075              | 2.333108                                                       |
| 13293 | 1.658617              | 2.333120                                                       |
| 13295 | 1.200451              | 2.333132                                                       |
| 13297 | 1.000075              | 2.333144                                                       |
| 13299 | 1.616964              | 2.333155                                                       |
| 13301 | 1.024885              | 2.333167                                                       |

| $n$   | $\frac{\sigma(n)}{n}$ | $\frac{e^\gamma}{2} \log \log n + \frac{0.73...}{\log \log n}$ |
|-------|-----------------------|----------------------------------------------------------------|
| 13303 | 1.022927              | 2.333179                                                       |
| 13305 | 1.601804              | 2.333191                                                       |
| 13307 | 1.143458              | 2.333203                                                       |
| 13309 | 1.000075              | 2.333214                                                       |
| 13311 | 1.622718              | 2.333226                                                       |
| 13313 | 1.000075              | 2.333238                                                       |
| 13315 | 1.200451              | 2.333250                                                       |
| 13317 | 1.398513              | 2.333262                                                       |
| 13319 | 1.054133              | 2.333273                                                       |
| 13321 | 1.253960              | 2.333285                                                       |
| 13323 | 1.333634              | 2.333297                                                       |
| 13325 | 1.367955              | 2.333309                                                       |
| 13327 | 1.000075              | 2.333320                                                       |
| 13329 | 1.445420              | 2.333332                                                       |
| 13331 | 1.000075              | 2.333344                                                       |
| 13333 | 1.020026              | 2.333356                                                       |
| 13335 | 1.842970              | 2.333367                                                       |
| 13337 | 1.000075              | 2.333379                                                       |
| 13339 | 1.000075              | 2.333391                                                       |
| 13341 | 1.333633              | 2.333403                                                       |
| 13343 | 1.091808              | 2.333414                                                       |
| 13345 | 1.278681              | 2.333426                                                       |
| 13347 | 1.445418              | 2.333438                                                       |
| 13349 | 1.143456              | 2.333450                                                       |
| 13351 | 1.096547              | 2.333461                                                       |
| 13353 | 1.333633              | 2.333473                                                       |
| 13355 | 1.200449              | 2.333485                                                       |
| 13357 | 1.083926              | 2.333497                                                       |
| 13359 | 1.373756              | 2.333508                                                       |
| 13361 | 1.034653              | 2.333520                                                       |
| 13363 | 1.206915              | 2.333532                                                       |
| 13365 | 1.960943              | 2.333544                                                       |
| 13367 | 1.000075              | 2.333555                                                       |
| 13369 | 1.036727              | 2.333567                                                       |
| 13371 | 1.333632              | 2.333579                                                       |
| 13373 | 1.026546              | 2.333590                                                       |
| 13375 | 1.259664              | 2.333602                                                       |
| 13377 | 1.674516              | 2.333614                                                       |
| 13379 | 1.060169              | 2.333626                                                       |
| 13381 | 1.000075              | 2.333637                                                       |
| 13383 | 1.445416              | 2.333649                                                       |
| 13385 | 1.200448              | 2.333661                                                       |
| 13387 | 1.091805              | 2.333672                                                       |
| 13389 | 1.333632              | 2.333684                                                       |

| $n$   | $\frac{\sigma(n)}{n}$ | $\frac{e^\gamma}{2} \log \log n + \frac{0.73...}{\log \log n}$ |
|-------|-----------------------|----------------------------------------------------------------|
| 13391 | 1.143455              | 2.333696                                                       |
| 13393 | 1.021429              | 2.333708                                                       |
| 13395 | 1.720045              | 2.333719                                                       |
| 13397 | 1.000075              | 2.333731                                                       |
| 13399 | 1.000075              | 2.333743                                                       |
| 13401 | 1.445415              | 2.333754                                                       |
| 13403 | 1.077968              | 2.333766                                                       |
| 13405 | 1.375009              | 2.333778                                                       |
| 13407 | 1.378384              | 2.333789                                                       |
| 13409 | 1.159818              | 2.333801                                                       |
| 13411 | 1.000075              | 2.333813                                                       |
| 13413 | 1.417133              | 2.333824                                                       |
| 13415 | 1.200447              | 2.333836                                                       |
| 13417 | 1.000075              | 2.333848                                                       |
| 13419 | 1.716968              | 2.333860                                                       |
| 13421 | 1.000075              | 2.333871                                                       |
| 13423 | 1.034642              | 2.333883                                                       |
| 13425 | 1.662570              | 2.333895                                                       |
| 13427 | 1.036717              | 2.333906                                                       |
| 13429 | 1.077966              | 2.333918                                                       |
| 13431 | 1.505175              | 2.333930                                                       |
| 13433 | 1.214918              | 2.333941                                                       |
| 13435 | 1.200447              | 2.333953                                                       |
| 13437 | 1.445412              | 2.333965                                                       |
| 13439 | 1.017933              | 2.333976                                                       |
| 13441 | 1.000074              | 2.333988                                                       |
| 13443 | 1.333631              | 2.333999                                                       |
| 13445 | 1.200446              | 2.334011                                                       |
| 13447 | 1.220793              | 2.334023                                                       |
| 13449 | 1.333631              | 2.334034                                                       |
| 13451 | 1.000074              | 2.334046                                                       |
| 13453 | 1.091801              | 2.334058                                                       |
| 13455 | 1.947826              | 2.334069                                                       |
| 13457 | 1.000074              | 2.334081                                                       |
| 13459 | 1.026525              | 2.334093                                                       |
| 13461 | 1.526187              | 2.334104                                                       |
| 13463 | 1.000074              | 2.334116                                                       |
| 13465 | 1.200446              | 2.334128                                                       |
| 13467 | 1.353531              | 2.334139                                                       |
| 13469 | 1.000074              | 2.334151                                                       |
| 13471 | 1.054116              | 2.334162                                                       |
| 13473 | 1.484450              | 2.334174                                                       |
| 13475 | 1.573581              | 2.334186                                                       |
| 13477 | 1.000074              | 2.334197                                                       |

| $n$   | $\frac{\sigma(n)}{n}$ | $\frac{e^\gamma}{2} \log \log n + \frac{0.73...}{\log \log n}$ |
|-------|-----------------------|----------------------------------------------------------------|
| 13479 | 1.333630              | 2.334209                                                       |
| 13481 | 1.158964              | 2.334221                                                       |
| 13483 | 1.017578              | 2.334232                                                       |
| 13485 | 1.708565              | 2.334244                                                       |
| 13487 | 1.000074              | 2.334255                                                       |
| 13489 | 1.195641              | 2.334267                                                       |
| 13491 | 1.445408              | 2.334279                                                       |
| 13493 | 1.017416              | 2.334290                                                       |
| 13495 | 1.200445              | 2.334302                                                       |
| 13497 | 1.458102              | 2.334313                                                       |
| 13499 | 1.000074              | 2.334325                                                       |
| 13501 | 1.045256              | 2.334337                                                       |
| 13503 | 1.526179              | 2.334348                                                       |
| 13505 | 1.249315              | 2.334360                                                       |
| 13507 | 1.077960              | 2.334371                                                       |
| 13509 | 1.539714              | 2.334383                                                       |
| 13511 | 1.021390              | 2.334395                                                       |
| 13513 | 1.000074              | 2.334406                                                       |
| 13515 | 1.726082              | 2.334418                                                       |
| 13517 | 1.143449              | 2.334429                                                       |
| 13519 | 1.091797              | 2.334441                                                       |
| 13521 | 1.333629              | 2.334453                                                       |
| 13523 | 1.000074              | 2.334464                                                       |
| 13525 | 1.242292              | 2.334476                                                       |
| 13527 | 1.502772              | 2.334487                                                       |
| 13529 | 1.018257              | 2.334499                                                       |
| 13531 | 1.143448              | 2.334510                                                       |
| 13533 | 1.440035              | 2.334522                                                       |
| 13535 | 1.200443              | 2.334534                                                       |
| 13537 | 1.000074              | 2.334545                                                       |
| 13539 | 1.333629              | 2.334557                                                       |
| 13541 | 1.091795              | 2.334568                                                       |
| 13543 | 1.036698              | 2.334580                                                       |
| 13545 | 2.027021              | 2.334591                                                       |
| 13547 | 1.133830              | 2.334603                                                       |
| 13549 | 1.060152              | 2.334615                                                       |
| 13551 | 1.333629              | 2.334626                                                       |
| 13553 | 1.000074              | 2.334638                                                       |
| 13555 | 1.200443              | 2.334649                                                       |
| 13557 | 1.333628              | 2.334661                                                       |
| 13559 | 1.239029              | 2.334672                                                       |
| 13561 | 1.019394              | 2.334684                                                       |
| 13563 | 1.587259              | 2.334695                                                       |
| 13565 | 1.200442              | 2.334707                                                       |



| $n$   | $\frac{\sigma(n)}{n}$ | $\frac{e^\gamma}{2} \log \log n + \frac{0.73...}{\log \log n}$ |
|-------|-----------------------|----------------------------------------------------------------|
| 13567 | 1.000074              | 2.334718                                                       |
| 13569 | 1.333628              | 2.334730                                                       |
| 13571 | 1.027485              | 2.334741                                                       |
| 13573 | 1.167465              | 2.334753                                                       |
| 13575 | 1.662468              | 2.334765                                                       |
| 13577 | 1.000074              | 2.334776                                                       |
| 13579 | 1.029825              | 2.334788                                                       |
| 13581 | 1.484427              | 2.334799                                                       |
| 13583 | 1.084886              | 2.334811                                                       |
| 13585 | 1.483990              | 2.334822                                                       |
| 13587 | 1.526165              | 2.334834                                                       |
| 13589 | 1.017293              | 2.334845                                                       |
| 13591 | 1.000074              | 2.334857                                                       |
| 13593 | 1.398367              | 2.334868                                                       |
| 13595 | 1.200441              | 2.334880                                                       |
| 13597 | 1.000074              | 2.334891                                                       |
| 13599 | 1.445400              | 2.334903                                                       |
| 13601 | 1.199912              | 2.334914                                                       |
| 13603 | 1.020951              | 2.334926                                                       |
| 13605 | 1.601764              | 2.334937                                                       |
| 13607 | 1.091791              | 2.334949                                                       |
| 13609 | 1.034609              | 2.334960                                                       |
| 13611 | 1.440012              | 2.334972                                                       |
| 13613 | 1.000073              | 2.334983                                                       |
| 13615 | 1.374954              | 2.334995                                                       |
| 13617 | 1.546596              | 2.335006                                                       |
| 13619 | 1.000073              | 2.335018                                                       |
| 13621 | 1.022832              | 2.335029                                                       |
| 13623 | 1.409381              | 2.335041                                                       |
| 13625 | 1.259450              | 2.335052                                                       |
| 13627 | 1.000073              | 2.335064                                                       |
| 13629 | 1.690513              | 2.335075                                                       |
| 13631 | 1.026484              | 2.335087                                                       |
| 13633 | 1.000073              | 2.335098                                                       |
| 13635 | 1.795380              | 2.335110                                                       |
| 13637 | 1.077950              | 2.335121                                                       |
| 13639 | 1.045238              | 2.335133                                                       |
| 13641 | 1.333627              | 2.335144                                                       |
| 13643 | 1.143444              | 2.335156                                                       |
| 13645 | 1.200440              | 2.335167                                                       |
| 13647 | 1.333626              | 2.335178                                                       |
| 13649 | 1.000073              | 2.335190                                                       |
| 13651 | 1.170903              | 2.335201                                                       |
| 13653 | 1.519666              | 2.335213                                                       |

| $n$   | $\frac{\sigma(n)}{n}$ | $\frac{e^\gamma}{2} \log \log n + \frac{0.73...}{\log \log n}$ |
|-------|-----------------------|----------------------------------------------------------------|
| 13655 | 1.200439              | 2.335224                                                       |
| 13657 | 1.143443              | 2.335236                                                       |
| 13659 | 1.388096              | 2.335247                                                       |
| 13661 | 1.054096              | 2.335259                                                       |
| 13663 | 1.077948              | 2.335270                                                       |
| 13665 | 1.601756              | 2.335282                                                       |
| 13667 | 1.018512              | 2.335293                                                       |
| 13669 | 1.000073              | 2.335304                                                       |
| 13671 | 1.734474              | 2.335316                                                       |
| 13673 | 1.108901              | 2.335327                                                       |
| 13675 | 1.242267              | 2.335339                                                       |
| 13677 | 1.375740              | 2.335350                                                       |
| 13679 | 1.000073              | 2.335362                                                       |
| 13681 | 1.000073              | 2.335373                                                       |
| 13683 | 1.333626              | 2.335385                                                       |
| 13685 | 1.515236              | 2.335396                                                       |
| 13687 | 1.000073              | 2.335407                                                       |
| 13689 | 1.617576              | 2.335419                                                       |
| 13691 | 1.000073              | 2.335430                                                       |
| 13693 | 1.000073              | 2.335442                                                       |
| 13695 | 1.766484              | 2.335453                                                       |
| 13697 | 1.000073              | 2.335465                                                       |
| 13699 | 1.214687              | 2.335476                                                       |
| 13701 | 1.333625              | 2.335487                                                       |
| 13703 | 1.019339              | 2.335499                                                       |
| 13705 | 1.200438              | 2.335510                                                       |
| 13707 | 1.445393              | 2.335522                                                       |
| 13709 | 1.000073              | 2.335533                                                       |
| 13711 | 1.000073              | 2.335544                                                       |
| 13713 | 1.526143              | 2.335556                                                       |
| 13715 | 1.298432              | 2.335567                                                       |
| 13717 | 1.154771              | 2.335579                                                       |
| 13719 | 1.417013              | 2.335590                                                       |
| 13721 | 1.000073              | 2.335601                                                       |
| 13723 | 1.000073              | 2.335613                                                       |
| 13725 | 1.820474              | 2.335624                                                       |
| 13727 | 1.195891              | 2.335636                                                       |
| 13729 | 1.000073              | 2.335647                                                       |
| 13731 | 1.398296              | 2.335658                                                       |
| 13733 | 1.034588              | 2.335670                                                       |
| 13735 | 1.247616              | 2.335681                                                       |
| 13737 | 1.409332              | 2.335693                                                       |
| 13739 | 1.091783              | 2.335704                                                       |
| 13741 | 1.238920              | 2.335715                                                       |

| $n$   | $\frac{\sigma(n)}{n}$ | $\frac{e^\gamma}{2} \log \log n + \frac{0.73...}{\log \log n}$ |
|-------|-----------------------|----------------------------------------------------------------|
| 13743 | 1.484392              | 2.335727                                                       |
| 13745 | 1.200437              | 2.335738                                                       |
| 13747 | 1.021314              | 2.335749                                                       |
| 13749 | 1.333624              | 2.335761                                                       |
| 13751 | 1.000073              | 2.335772                                                       |
| 13753 | 1.060132              | 2.335784                                                       |
| 13755 | 1.842530              | 2.335795                                                       |
| 13757 | 1.000073              | 2.335806                                                       |
| 13759 | 1.000073              | 2.335818                                                       |
| 13761 | 1.587094              | 2.335829                                                       |
| 13763 | 1.000073              | 2.335840                                                       |
| 13765 | 1.200436              | 2.335852                                                       |
| 13767 | 1.439965              | 2.335863                                                       |
| 13769 | 1.167405              | 2.335874                                                       |
| 13771 | 1.024762              | 2.335886                                                       |
| 13773 | 1.333624              | 2.335897                                                       |
| 13775 | 1.350272              | 2.335909                                                       |
| 13777 | 1.045220              | 2.335920                                                       |
| 13779 | 1.445388              | 2.335931                                                       |
| 13781 | 1.000073              | 2.335943                                                       |
| 13783 | 1.253718              | 2.335954                                                       |
| 13785 | 1.601741              | 2.335965                                                       |
| 13787 | 1.060129              | 2.335977                                                       |
| 13789 | 1.000073              | 2.335988                                                       |
| 13791 | 1.333623              | 2.335999                                                       |
| 13793 | 1.077938              | 2.336011                                                       |
| 13795 | 1.252628              | 2.336022                                                       |
| 13797 | 1.716315              | 2.336033                                                       |
| 13799 | 1.000072              | 2.336045                                                       |
| 13801 | 1.029780              | 2.336056                                                       |
| 13803 | 1.377092              | 2.336067                                                       |
| 13805 | 1.314306              | 2.336079                                                       |
| 13807 | 1.000072              | 2.336090                                                       |
| 13809 | 1.333623              | 2.336101                                                       |
| 13811 | 1.143436              | 2.336112                                                       |
| 13813 | 1.054079              | 2.336124                                                       |
| 13815 | 1.738979              | 2.336135                                                       |
| 13817 | 1.027430              | 2.336146                                                       |
| 13819 | 1.077936              | 2.336158                                                       |
| 13821 | 1.416974              | 2.336169                                                       |
| 13823 | 1.045214              | 2.336180                                                       |
| 13825 | 1.435081              | 2.336192                                                       |
| 13827 | 1.458017              | 2.336203                                                       |
| 13829 | 1.000072              | 2.336214                                                       |

| $n$   | $\frac{\sigma(n)}{n}$ | $\frac{e^\gamma}{2} \log \log n + \frac{0.73...}{\log \log n}$ |
|-------|-----------------------|----------------------------------------------------------------|
| 13831 | 1.000072              | 2.336226                                                       |
| 13833 | 1.522446              | 2.336237                                                       |
| 13835 | 1.200434              | 2.336248                                                       |
| 13837 | 1.017273              | 2.336259                                                       |
| 13839 | 1.526122              | 2.336271                                                       |
| 13841 | 1.000072              | 2.336282                                                       |
| 13843 | 1.017121              | 2.336293                                                       |
| 13845 | 1.747346              | 2.336305                                                       |
| 13847 | 1.020871              | 2.336316                                                       |
| 13849 | 1.091776              | 2.336327                                                       |
| 13851 | 1.578225              | 2.336338                                                       |
| 13853 | 1.143435              | 2.336350                                                       |
| 13855 | 1.278383              | 2.336361                                                       |
| 13857 | 1.385581              | 2.336372                                                       |
| 13859 | 1.000072              | 2.336384                                                       |
| 13861 | 1.018108              | 2.336395                                                       |
| 13863 | 1.333622              | 2.336406                                                       |
| 13865 | 1.246304              | 2.336417                                                       |
| 13867 | 1.167376              | 2.336429                                                       |
| 13869 | 1.529743              | 2.336440                                                       |
| 13871 | 1.186937              | 2.336451                                                       |
| 13873 | 1.000072              | 2.336462                                                       |
| 13875 | 1.708973              | 2.336474                                                       |
| 13877 | 1.000072              | 2.336485                                                       |
| 13879 | 1.000072              | 2.336496                                                       |
| 13881 | 1.526115              | 2.336507                                                       |
| 13883 | 1.000072              | 2.336519                                                       |
| 13885 | 1.200432              | 2.336530                                                       |
| 13887 | 1.445381              | 2.336541                                                       |
| 13889 | 1.140471              | 2.336552                                                       |
| 13891 | 1.036642              | 2.336564                                                       |
| 13893 | 1.458000              | 2.336575                                                       |
| 13895 | 1.374883              | 2.336586                                                       |
| 13897 | 1.077930              | 2.336597                                                       |
| 13899 | 1.377941              | 2.336609                                                       |
| 13901 | 1.000072              | 2.336620                                                       |
| 13903 | 1.000072              | 2.336631                                                       |
| 13905 | 1.795038              | 2.336642                                                       |
| 13907 | 1.000072              | 2.336654                                                       |
| 13909 | 1.143432              | 2.336665                                                       |
| 13911 | 1.333621              | 2.336676                                                       |
| 13913 | 1.000072              | 2.336687                                                       |
| 13915 | 1.376356              | 2.336699                                                       |
| 13917 | 1.333621              | 2.336710                                                       |

| $n$   | $\frac{\sigma(n)}{n}$ | $\frac{e^\gamma}{2} \log \log n + \frac{0.73\dots}{\log \log n}$ |
|-------|-----------------------|------------------------------------------------------------------|
| 13919 | 1.034557              | 2.336721                                                         |
| 13921 | 1.000072              | 2.336732                                                         |
| 13923 | 1.882353              | 2.336743                                                         |
| 13925 | 1.242226              | 2.336755                                                         |
| 13927 | 1.054068              | 2.336766                                                         |
| 13929 | 1.333621              | 2.336777                                                         |
| 13931 | 1.000072              | 2.336788                                                         |
| 13933 | 1.000072              | 2.336800                                                         |
| 13935 | 1.601722              | 2.336811                                                         |
| 13937 | 1.253641              | 2.336822                                                         |
| 13939 | 1.022742              | 2.336833                                                         |
| 13941 | 1.445377              | 2.336844                                                         |
| 13943 | 1.019006              | 2.336856                                                         |
| 13945 | 1.200430              | 2.336867                                                         |
| 13947 | 1.333620              | 2.336878                                                         |
| 13949 | 1.144168              | 2.336889                                                         |
| 13951 | 1.143431              | 2.336900                                                         |
| 13953 | 1.333620              | 2.336912                                                         |
| 13955 | 1.200430              | 2.336923                                                         |
| 13957 | 1.060113              | 2.336934                                                         |
| 13959 | 1.650548              | 2.336945                                                         |
| 13961 | 1.045197              | 2.336956                                                         |
| 13963 | 1.000072              | 2.336967                                                         |
| 13965 | 1.959184              | 2.336979                                                         |
| 13967 | 1.000072              | 2.336990                                                         |
| 13969 | 1.020832              | 2.337001                                                         |
| 13971 | 1.333620              | 2.337012                                                         |
| 13973 | 1.017677              | 2.337023                                                         |
| 13975 | 1.366440              | 2.337035                                                         |
| 13977 | 1.445375              | 2.337046                                                         |
| 13979 | 1.143429              | 2.337057                                                         |
| 13981 | 1.153566              | 2.337068                                                         |
| 13983 | 1.373096              | 2.337079                                                         |
| 13985 | 1.200429              | 2.337090                                                         |
| 13987 | 1.019232              | 2.337102                                                         |
| 13989 | 1.333619              | 2.337113                                                         |
| 13991 | 1.060110              | 2.337124                                                         |
| 13993 | 1.143429              | 2.337135                                                         |
| 13995 | 1.738907              | 2.337146                                                         |
| 13997 | 1.000071              | 2.337157                                                         |
| 13999 | 1.000071              | 2.337168                                                         |
| 14001 | 1.439897              | 2.337180                                                         |
| 14003 | 1.165465              | 2.337191                                                         |
| 14005 | 1.200428              | 2.337202                                                         |

| $n$   | $\frac{\sigma(n)}{n}$ | $\frac{e^\gamma}{2} \log \log n + \frac{0.73...}{\log \log n}$ |
|-------|-----------------------|----------------------------------------------------------------|
| 14007 | 1.644892              | 2.337213                                                       |
| 14009 | 1.000071              | 2.337224                                                       |
| 14011 | 1.000071              | 2.337235                                                       |
| 14013 | 1.502462              | 2.337246                                                       |
| 14015 | 1.200428              | 2.337258                                                       |
| 14017 | 1.017051              | 2.337269                                                       |
| 14019 | 1.333619              | 2.337280                                                       |
| 14021 | 1.143428              | 2.337291                                                       |
| 14023 | 1.029737              | 2.337302                                                       |
| 14025 | 1.909733              | 2.337313                                                       |
| 14027 | 1.095887              | 2.337324                                                       |
| 14029 | 1.000071              | 2.337336                                                       |
| 14031 | 1.445371              | 2.337347                                                       |
| 14033 | 1.000071              | 2.337358                                                       |
| 14035 | 1.374849              | 2.337369                                                       |
| 14037 | 1.333618              | 2.337380                                                       |
| 14039 | 1.017166              | 2.337391                                                       |
| 14041 | 1.054056              | 2.337402                                                       |
| 14043 | 1.385459              | 2.337413                                                       |
| 14045 | 1.223069              | 2.337425                                                       |
| 14047 | 1.091763              | 2.337436                                                       |
| 14049 | 1.658196              | 2.337447                                                       |
| 14051 | 1.000071              | 2.337458                                                       |
| 14053 | 1.147655              | 2.337469                                                       |
| 14055 | 1.601708              | 2.337480                                                       |
| 14057 | 1.000071              | 2.337491                                                       |
| 14059 | 1.060104              | 2.337502                                                       |
| 14061 | 1.376858              | 2.337513                                                       |
| 14063 | 1.194624              | 2.337524                                                       |
| 14065 | 1.254177              | 2.337536                                                       |
| 14067 | 1.484325              | 2.337547                                                       |
| 14069 | 1.091762              | 2.337558                                                       |
| 14071 | 1.000071              | 2.337569                                                       |
| 14073 | 1.333618              | 2.337580                                                       |
| 14075 | 1.242202              | 2.337591                                                       |
| 14077 | 1.143425              | 2.337602                                                       |
| 14079 | 1.515449              | 2.337613                                                       |
| 14081 | 1.000071              | 2.337624                                                       |
| 14083 | 1.000071              | 2.337635                                                       |
| 14085 | 1.738871              | 2.337646                                                       |
| 14087 | 1.000071              | 2.337657                                                       |
| 14089 | 1.018951              | 2.337669                                                       |
| 14091 | 1.689589              | 2.337680                                                       |
| 14093 | 1.060101              | 2.337691                                                       |

| $n$   | $\frac{\sigma(n)}{n}$ | $\frac{e^\gamma}{2} \log \log n + \frac{0.73\dots}{\log \log n}$ |
|-------|-----------------------|------------------------------------------------------------------|
| 14095 | 1.200426              | 2.337702                                                         |
| 14097 | 1.380152              | 2.337713                                                         |
| 14099 | 1.045181              | 2.337724                                                         |
| 14101 | 1.021204              | 2.337735                                                         |
| 14103 | 1.445366              | 2.337746                                                         |
| 14105 | 1.524566              | 2.337757                                                         |
| 14107 | 1.000071              | 2.337768                                                         |
| 14109 | 1.333617              | 2.337779                                                         |
| 14111 | 1.017079              | 2.337790                                                         |
| 14113 | 1.091759              | 2.337801                                                         |
| 14115 | 1.601700              | 2.337812                                                         |
| 14117 | 1.054048              | 2.337823                                                         |
| 14119 | 1.143424              | 2.337834                                                         |
| 14121 | 1.484314              | 2.337846                                                         |
| 14123 | 1.036607              | 2.337857                                                         |
| 14125 | 1.259044              | 2.337868                                                         |
| 14127 | 1.416861              | 2.337879                                                         |
| 14129 | 1.019180              | 2.337890                                                         |
| 14131 | 1.077914              | 2.337901                                                         |
| 14133 | 1.526074              | 2.337912                                                         |
| 14135 | 1.314185              | 2.337923                                                         |
| 14137 | 1.019735              | 2.337934                                                         |
| 14139 | 1.445364              | 2.337945                                                         |
| 14141 | 1.018316              | 2.337956                                                         |
| 14143 | 1.000071              | 2.337967                                                         |
| 14145 | 1.710286              | 2.337978                                                         |
| 14147 | 1.194317              | 2.337989                                                         |
| 14149 | 1.000071              | 2.338000                                                         |
| 14151 | 1.373755              | 2.338011                                                         |
| 14153 | 1.000071              | 2.338022                                                         |
| 14155 | 1.271635              | 2.338033                                                         |
| 14157 | 1.709826              | 2.338044                                                         |
| 14159 | 1.000071              | 2.338055                                                         |
| 14161 | 1.235718              | 2.338066                                                         |
| 14163 | 1.333616              | 2.338077                                                         |
| 14165 | 1.200424              | 2.338088                                                         |
| 14167 | 1.034517              | 2.338099                                                         |
| 14169 | 1.333616              | 2.338110                                                         |
| 14171 | 1.029709              | 2.338121                                                         |
| 14173 | 1.000071              | 2.338132                                                         |
| 14175 | 2.116966              | 2.338143                                                         |
| 14177 | 1.000071              | 2.338154                                                         |
| 14179 | 1.091755              | 2.338165                                                         |
| 14181 | 1.387772              | 2.338176                                                         |

| $n$   | $\frac{\sigma(n)}{n}$ | $\frac{e^\gamma}{2} \log \log n + \frac{0.73...}{\log \log n}$ |
|-------|-----------------------|----------------------------------------------------------------|
| 14183 | 1.077910              | 2.338187                                                       |
| 14185 | 1.200423              | 2.338198                                                       |
| 14187 | 1.333615              | 2.338209                                                       |
| 14189 | 1.143421              | 2.338220                                                       |
| 14191 | 1.045169              | 2.338231                                                       |
| 14193 | 1.538787              | 2.338242                                                       |
| 14195 | 1.278197              | 2.338253                                                       |
| 14197 | 1.000070              | 2.338264                                                       |
| 14199 | 1.333615              | 2.338275                                                       |
| 14201 | 1.091754              | 2.338286                                                       |
| 14203 | 1.143420              | 2.338297                                                       |
| 14205 | 1.601690              | 2.338308                                                       |
| 14207 | 1.000070              | 2.338319                                                       |
| 14209 | 1.077908              | 2.338330                                                       |
| 14211 | 1.445359              | 2.338341                                                       |
| 14213 | 1.020756              | 2.338352                                                       |
| 14215 | 1.200422              | 2.338363                                                       |
| 14217 | 1.526060              | 2.338374                                                       |
| 14219 | 1.021169              | 2.338385                                                       |
| 14221 | 1.000070              | 2.338396                                                       |
| 14223 | 1.457920              | 2.338407                                                       |
| 14225 | 1.242179              | 2.338418                                                       |
| 14227 | 1.027342              | 2.338429                                                       |
| 14229 | 1.619228              | 2.338440                                                       |
| 14231 | 1.214251              | 2.338451                                                       |
| 14233 | 1.026347              | 2.338462                                                       |
| 14235 | 1.746681              | 2.338472                                                       |
| 14237 | 1.045164              | 2.338483                                                       |
| 14239 | 1.036590              | 2.338494                                                       |
| 14241 | 1.375184              | 2.338505                                                       |
| 14243 | 1.000070              | 2.338516                                                       |
| 14245 | 1.536539              | 2.338527                                                       |
| 14247 | 1.445357              | 2.338538                                                       |
| 14249 | 1.000070              | 2.338549                                                       |
| 14251 | 1.000070              | 2.338560                                                       |
| 14253 | 1.333614              | 2.338571                                                       |
| 14255 | 1.200421              | 2.338582                                                       |
| 14257 | 1.022656              | 2.338593                                                       |
| 14259 | 1.567010              | 2.338604                                                       |
| 14261 | 1.077905              | 2.338615                                                       |
| 14263 | 1.060086              | 2.338626                                                       |
| 14265 | 1.738801              | 2.338637                                                       |
| 14267 | 1.091750              | 2.338647                                                       |
| 14269 | 1.054033              | 2.338658                                                       |



| $n$   | $\frac{\sigma(n)}{n}$ | $\frac{e^\gamma}{2} \log \log n + \frac{0.73\dots}{\log \log n}$ |
|-------|-----------------------|------------------------------------------------------------------|
| 14271 | 1.372293              | 2.338669                                                         |
| 14273 | 1.143418              | 2.338680                                                         |
| 14275 | 1.242172              | 2.338691                                                         |
| 14277 | 1.333614              | 2.338702                                                         |
| 14279 | 1.016878              | 2.338713                                                         |
| 14281 | 1.000070              | 2.338724                                                         |
| 14283 | 1.548694              | 2.338735                                                         |
| 14285 | 1.200420              | 2.338746                                                         |
| 14287 | 1.238609              | 2.338757                                                         |
| 14289 | 1.457905              | 2.338768                                                         |
| 14291 | 1.034497              | 2.338778                                                         |
| 14293 | 1.000070              | 2.338789                                                         |
| 14295 | 1.601679              | 2.338800                                                         |
| 14297 | 1.096594              | 2.338811                                                         |
| 14299 | 1.018253              | 2.338822                                                         |
| 14301 | 1.658066              | 2.338833                                                         |
| 14303 | 1.000070              | 2.338844                                                         |
| 14305 | 1.200419              | 2.338855                                                         |
| 14307 | 1.409100              | 2.338866                                                         |
| 14309 | 1.027325              | 2.338877                                                         |
| 14311 | 1.091748              | 2.338887                                                         |
| 14313 | 1.439810              | 2.338898                                                         |
| 14315 | 1.374782              | 2.338909                                                         |
| 14317 | 1.016973              | 2.338920                                                         |
| 14319 | 1.517983              | 2.338931                                                         |
| 14321 | 1.000070              | 2.338942                                                         |
| 14323 | 1.000070              | 2.338953                                                         |
| 14325 | 1.661990              | 2.338964                                                         |
| 14327 | 1.000070              | 2.338974                                                         |
| 14329 | 1.205946              | 2.338985                                                         |
| 14331 | 1.416789              | 2.338996                                                         |
| 14333 | 1.091746              | 2.339007                                                         |
| 14335 | 1.245623              | 2.339018                                                         |
| 14337 | 1.523331              | 2.339029                                                         |
| 14339 | 1.077899              | 2.339040                                                         |
| 14341 | 1.000070              | 2.339051                                                         |
| 14343 | 1.526041              | 2.339061                                                         |
| 14345 | 1.271523              | 2.339072                                                         |
| 14347 | 1.000070              | 2.339083                                                         |
| 14349 | 1.333612              | 2.339094                                                         |
| 14351 | 1.016793              | 2.339105                                                         |
| 14353 | 1.034488              | 2.339116                                                         |
| 14355 | 1.956113              | 2.339127                                                         |
| 14357 | 1.167235              | 2.339137                                                         |

| $n$   | $\frac{\sigma(n)}{n}$ | $\frac{e^\gamma}{2} \log \log n + \frac{0.73...}{\log \log n}$ |
|-------|-----------------------|----------------------------------------------------------------|
| 14359 | 1.017898              | 2.339148                                                       |
| 14361 | 1.333612              | 2.339159                                                       |
| 14363 | 1.022628              | 2.339170                                                       |
| 14365 | 1.375844              | 2.339181                                                       |
| 14367 | 1.333612              | 2.339192                                                       |
| 14369 | 1.000070              | 2.339202                                                       |
| 14371 | 1.143414              | 2.339213                                                       |
| 14373 | 1.445349              | 2.339224                                                       |
| 14375 | 1.303930              | 2.339235                                                       |
| 14377 | 1.091744              | 2.339246                                                       |
| 14379 | 1.333612              | 2.339257                                                       |
| 14381 | 1.018844              | 2.339267                                                       |
| 14383 | 1.054022              | 2.339278                                                       |
| 14385 | 1.841919              | 2.339289                                                       |
| 14387 | 1.000070              | 2.339300                                                       |
| 14389 | 1.000069              | 2.339311                                                       |
| 14391 | 1.634355              | 2.339322                                                       |
| 14393 | 1.029667              | 2.339332                                                       |
| 14395 | 1.200417              | 2.339343                                                       |
| 14397 | 1.333611              | 2.339354                                                       |
| 14399 | 1.330092              | 2.339365                                                       |
| 14401 | 1.000069              | 2.339376                                                       |
| 14403 | 1.333611              | 2.339386                                                       |
| 14405 | 1.246234              | 2.339397                                                       |
| 14407 | 1.000069              | 2.339408                                                       |
| 14409 | 1.445347              | 2.339419                                                       |
| 14411 | 1.000069              | 2.339430                                                       |
| 14413 | 1.198918              | 2.339441                                                       |
| 14415 | 1.653278              | 2.339451                                                       |
| 14417 | 1.077894              | 2.339462                                                       |
| 14419 | 1.000069              | 2.339473                                                       |
| 14421 | 1.597670              | 2.339484                                                       |
| 14423 | 1.000069              | 2.339495                                                       |
| 14425 | 1.242149              | 2.339505                                                       |
| 14427 | 1.658002              | 2.339516                                                       |
| 14429 | 1.024603              | 2.339527                                                       |
| 14431 | 1.000069              | 2.339538                                                       |
| 14433 | 1.416753              | 2.339548                                                       |
| 14435 | 1.200416              | 2.339559                                                       |
| 14437 | 1.000069              | 2.339570                                                       |
| 14439 | 1.333610              | 2.339581                                                       |
| 14441 | 1.143411              | 2.339592                                                       |
| 14443 | 1.186457              | 2.339602                                                       |
| 14445 | 1.794393              | 2.339613                                                       |

| $n$   | $\frac{\sigma(n)}{n}$ | $\frac{e^\gamma}{2} \log \log n + \frac{0.73...}{\log \log n}$ |
|-------|-----------------------|----------------------------------------------------------------|
| 14447 | 1.000069              | 2.339624                                                       |
| 14449 | 1.000069              | 2.339635                                                       |
| 14451 | 1.333610              | 2.339646                                                       |
| 14453 | 1.017090              | 2.339656                                                       |
| 14455 | 1.419578              | 2.339667                                                       |
| 14457 | 1.372346              | 2.339678                                                       |
| 14459 | 1.054015              | 2.339689                                                       |
| 14461 | 1.000069              | 2.339699                                                       |
| 14463 | 1.445343              | 2.339710                                                       |
| 14465 | 1.314068              | 2.339721                                                       |
| 14467 | 1.134720              | 2.339732                                                       |
| 14469 | 1.671988              | 2.339742                                                       |
| 14471 | 1.036556              | 2.339753                                                       |
| 14473 | 1.027292              | 2.339764                                                       |
| 14475 | 1.661900              | 2.339775                                                       |
| 14477 | 1.034468              | 2.339785                                                       |
| 14479 | 1.000069              | 2.339796                                                       |
| 14481 | 1.445342              | 2.339807                                                       |
| 14483 | 1.143410              | 2.339818                                                       |
| 14485 | 1.200414              | 2.339828                                                       |
| 14487 | 1.457859              | 2.339839                                                       |
| 14489 | 1.000069              | 2.339850                                                       |
| 14491 | 1.026292              | 2.339861                                                       |
| 14493 | 1.333609              | 2.339871                                                       |
| 14495 | 1.298103              | 2.339882                                                       |
| 14497 | 1.214044              | 2.339893                                                       |
| 14499 | 1.502173              | 2.339904                                                       |
| 14501 | 1.060065              | 2.339914                                                       |
| 14503 | 1.000069              | 2.339925                                                       |
| 14505 | 1.601655              | 2.339936                                                       |
| 14507 | 1.017440              | 2.339947                                                       |
| 14509 | 1.091736              | 2.339957                                                       |
| 14511 | 1.526015              | 2.339968                                                       |
| 14513 | 1.045132              | 2.339979                                                       |
| 14515 | 1.200413              | 2.339989                                                       |
| 14517 | 1.445340              | 2.340000                                                       |
| 14519 | 1.000069              | 2.340011                                                       |
| 14521 | 1.077887              | 2.340022                                                       |
| 14523 | 1.374923              | 2.340032                                                       |
| 14525 | 1.434217              | 2.340043                                                       |
| 14527 | 1.018793              | 2.340054                                                       |
| 14529 | 1.387570              | 2.340064                                                       |
| 14531 | 1.091735              | 2.340075                                                       |
| 14533 | 1.000069              | 2.340086                                                       |

| $n$   | $\frac{\sigma(n)}{n}$ | $\frac{e^\gamma}{2} \log \log n + \frac{0.73...}{\log \log n}$ |
|-------|-----------------------|----------------------------------------------------------------|
| 14535 | 1.931889              | 2.340097                                                       |
| 14537 | 1.000069              | 2.340107                                                       |
| 14539 | 1.197331              | 2.340118                                                       |
| 14541 | 1.379823              | 2.340129                                                       |
| 14543 | 1.000069              | 2.340139                                                       |
| 14545 | 1.200413              | 2.340150                                                       |
| 14547 | 1.439747              | 2.340161                                                       |
| 14549 | 1.000069              | 2.340171                                                       |
| 14551 | 1.000069              | 2.340182                                                       |
| 14553 | 1.880025              | 2.340193                                                       |
| 14555 | 1.246582              | 2.340204                                                       |
| 14557 | 1.000069              | 2.340214                                                       |
| 14559 | 1.397898              | 2.340225                                                       |
| 14561 | 1.000069              | 2.340236                                                       |
| 14563 | 1.000069              | 2.340246                                                       |
| 14565 | 1.601648              | 2.340257                                                       |
| 14567 | 1.143406              | 2.340268                                                       |
| 14569 | 1.060059              | 2.340278                                                       |
| 14571 | 1.445337              | 2.340289                                                       |
| 14573 | 1.152817              | 2.340300                                                       |
| 14575 | 1.378250              | 2.340310                                                       |
| 14577 | 1.376415              | 2.340321                                                       |
| 14579 | 1.020646              | 2.340332                                                       |
| 14581 | 1.143406              | 2.340342                                                       |
| 14583 | 1.333608              | 2.340353                                                       |
| 14585 | 1.200411              | 2.340364                                                       |
| 14587 | 1.036539              | 2.340374                                                       |
| 14589 | 1.445336              | 2.340385                                                       |
| 14591 | 1.000069              | 2.340396                                                       |
| 14593 | 1.000069              | 2.340406                                                       |
| 14595 | 1.841727              | 2.340417                                                       |
| 14597 | 1.091731              | 2.340428                                                       |
| 14599 | 1.077882              | 2.340438                                                       |
| 14601 | 1.385111              | 2.340449                                                       |
| 14603 | 1.060056              | 2.340460                                                       |
| 14605 | 1.262034              | 2.340470                                                       |
| 14607 | 1.484220              | 2.340481                                                       |
| 14609 | 1.143405              | 2.340492                                                       |
| 14611 | 1.054000              | 2.340502                                                       |
| 14613 | 1.333607              | 2.340513                                                       |
| 14615 | 1.248033              | 2.340524                                                       |
| 14617 | 1.024560              | 2.340534                                                       |
| 14619 | 1.457829              | 2.340545                                                       |
| 14621 | 1.000068              | 2.340555                                                       |

| $n$   | $\frac{\sigma(n)}{n}$ | $\frac{e^\gamma}{2} \log \log n + \frac{0.73...}{\log \log n}$ |
|-------|-----------------------|----------------------------------------------------------------|
| 14623 | 1.143404              | 2.340566                                                       |
| 14625 | 1.941333              | 2.340577                                                       |
| 14627 | 1.000068              | 2.340587                                                       |
| 14629 | 1.000068              | 2.340598                                                       |
| 14631 | 1.333607              | 2.340609                                                       |
| 14633 | 1.000068              | 2.340619                                                       |
| 14635 | 1.200410              | 2.340630                                                       |
| 14637 | 1.652798              | 2.340640                                                       |
| 14639 | 1.000068              | 2.340651                                                       |
| 14641 | 1.099993              | 2.340662                                                       |
| 14643 | 1.445332              | 2.340672                                                       |
| 14645 | 1.253670              | 2.340683                                                       |
| 14647 | 1.017000              | 2.340694                                                       |
| 14649 | 1.408970              | 2.340704                                                       |
| 14651 | 1.307215              | 2.340715                                                       |
| 14653 | 1.000068              | 2.340725                                                       |
| 14655 | 1.601638              | 2.340736                                                       |
| 14657 | 1.000068              | 2.340747                                                       |
| 14659 | 1.016713              | 2.340757                                                       |
| 14661 | 1.502080              | 2.340768                                                       |
| 14663 | 1.152288              | 2.340778                                                       |
| 14665 | 1.374702              | 2.340789                                                       |
| 14667 | 1.333606              | 2.340800                                                       |
| 14669 | 1.000068              | 2.340810                                                       |
| 14671 | 1.060050              | 2.340821                                                       |
| 14673 | 1.371771              | 2.340831                                                       |
| 14675 | 1.242112              | 2.340842                                                       |
| 14677 | 1.077877              | 2.340853                                                       |
| 14679 | 1.657879              | 2.340863                                                       |
| 14681 | 1.022546              | 2.340874                                                       |
| 14683 | 1.000068              | 2.340884                                                       |
| 14685 | 1.765066              | 2.340895                                                       |
| 14687 | 1.053993              | 2.340906                                                       |
| 14689 | 1.029614              | 2.340916                                                       |
| 14691 | 1.372269              | 2.340927                                                       |
| 14693 | 1.143402              | 2.340937                                                       |
| 14695 | 1.200408              | 2.340948                                                       |
| 14697 | 1.528475              | 2.340959                                                       |
| 14699 | 1.000068              | 2.340969                                                       |
| 14701 | 1.020611              | 2.340980                                                       |
| 14703 | 1.493573              | 2.340990                                                       |
| 14705 | 1.277933              | 2.341001                                                       |
| 14707 | 1.253281              | 2.341011                                                       |
| 14709 | 1.333605              | 2.341022                                                       |

| $n$   | $\frac{\sigma(n)}{n}$ | $\frac{e^\gamma}{2} \log \log n + \frac{0.73\dots}{\log \log n}$ |
|-------|-----------------------|------------------------------------------------------------------|
| 14711 | 1.024539              | 2.341033                                                         |
| 14713 | 1.000068              | 2.341043                                                         |
| 14715 | 1.794088              | 2.341054                                                         |
| 14717 | 1.000068              | 2.341064                                                         |
| 14719 | 1.027244              | 2.341075                                                         |
| 14721 | 1.525983              | 2.341085                                                         |
| 14723 | 1.000068              | 2.341096                                                         |
| 14725 | 1.347368              | 2.341106                                                         |
| 14727 | 1.333605              | 2.341117                                                         |
| 14729 | 1.186231              | 2.341128                                                         |
| 14731 | 1.000068              | 2.341138                                                         |
| 14733 | 1.445327              | 2.341149                                                         |
| 14735 | 1.374686              | 2.341159                                                         |
| 14737 | 1.000068              | 2.341170                                                         |
| 14739 | 1.416650              | 2.341180                                                         |
| 14741 | 1.000068              | 2.341191                                                         |
| 14743 | 1.045106              | 2.341201                                                         |
| 14745 | 1.601628              | 2.341212                                                         |
| 14747 | 1.000068              | 2.341222                                                         |
| 14749 | 1.193301              | 2.341233                                                         |
| 14751 | 1.586333              | 2.341244                                                         |
| 14753 | 1.000068              | 2.341254                                                         |
| 14755 | 1.298001              | 2.341265                                                         |
| 14757 | 1.333604              | 2.341275                                                         |
| 14759 | 1.000068              | 2.341286                                                         |
| 14761 | 1.036515              | 2.341296                                                         |
| 14763 | 1.647362              | 2.341307                                                         |
| 14765 | 1.200406              | 2.341317                                                         |
| 14767 | 1.000068              | 2.341328                                                         |
| 14769 | 1.484190              | 2.341338                                                         |
| 14771 | 1.000068              | 2.341349                                                         |
| 14773 | 1.169701              | 2.341359                                                         |
| 14775 | 1.661726              | 2.341370                                                         |
| 14777 | 1.143399              | 2.341380                                                         |
| 14779 | 1.000068              | 2.341391                                                         |
| 14781 | 1.439686              | 2.341401                                                         |
| 14783 | 1.000068              | 2.341412                                                         |
| 14785 | 1.200406              | 2.341422                                                         |
| 14787 | 1.519172              | 2.341433                                                         |
| 14789 | 1.045101              | 2.341443                                                         |
| 14791 | 1.143398              | 2.341454                                                         |
| 14793 | 1.333604              | 2.341464                                                         |
| 14795 | 1.313957              | 2.341475                                                         |
| 14797 | 1.000068              | 2.341485                                                         |

| $n$   | $\frac{\sigma(n)}{n}$ | $\frac{e^\gamma}{2} \log \log n + \frac{0.73\dots}{\log \log n}$ |
|-------|-----------------------|------------------------------------------------------------------|
| 14799 | 1.333604              | 2.341496                                                         |
| 14801 | 1.081143              | 2.341506                                                         |
| 14803 | 1.016551              | 2.341517                                                         |
| 14805 | 2.023100              | 2.341527                                                         |
| 14807 | 1.157290              | 2.341538                                                         |
| 14809 | 1.021001              | 2.341548                                                         |
| 14811 | 1.333603              | 2.341559                                                         |
| 14813 | 1.000068              | 2.341569                                                         |
| 14815 | 1.200405              | 2.341580                                                         |
| 14817 | 1.457785              | 2.341590                                                         |
| 14819 | 1.198461              | 2.341601                                                         |
| 14821 | 1.000067              | 2.341611                                                         |
| 14823 | 1.522499              | 2.341622                                                         |
| 14825 | 1.242091              | 2.341632                                                         |
| 14827 | 1.000067              | 2.341643                                                         |
| 14829 | 1.333603              | 2.341653                                                         |
| 14831 | 1.000067              | 2.341664                                                         |
| 14833 | 1.238320              | 2.341674                                                         |
| 14835 | 1.708392              | 2.341685                                                         |
| 14837 | 1.029588              | 2.341695                                                         |
| 14839 | 1.164499              | 2.341706                                                         |
| 14841 | 1.545179              | 2.341716                                                         |
| 14843 | 1.000067              | 2.341727                                                         |
| 14845 | 1.200404              | 2.341737                                                         |
| 14847 | 1.566377              | 2.341747                                                         |
| 14849 | 1.034413              | 2.341758                                                         |
| 14851 | 1.000067              | 2.341768                                                         |
| 14853 | 1.333603              | 2.341779                                                         |
| 14855 | 1.200404              | 2.341789                                                         |
| 14857 | 1.017702              | 2.341800                                                         |
| 14859 | 1.567804              | 2.341810                                                         |
| 14861 | 1.253213              | 2.341821                                                         |
| 14863 | 1.017291              | 2.341831                                                         |
| 14865 | 1.601615              | 2.341842                                                         |
| 14867 | 1.000067              | 2.341852                                                         |
| 14869 | 1.000067              | 2.341862                                                         |
| 14871 | 1.333602              | 2.341873                                                         |
| 14873 | 1.016607              | 2.341883                                                         |
| 14875 | 1.510185              | 2.341894                                                         |
| 14877 | 1.613228              | 2.341904                                                         |
| 14879 | 1.000067              | 2.341915                                                         |
| 14881 | 1.045091              | 2.341925                                                         |
| 14883 | 1.501310              | 2.341936                                                         |
| 14885 | 1.297951              | 2.341946                                                         |

| $n$   | $\frac{\sigma(n)}{n}$ | $\frac{e^\gamma}{2} \log \log n + \frac{0.73\dots}{\log \log n}$ |
|-------|-----------------------|------------------------------------------------------------------|
| 14887 | 1.000067              | 2.341956                                                         |
| 14889 | 1.525959              | 2.341967                                                         |
| 14891 | 1.000067              | 2.341977                                                         |
| 14893 | 1.022494              | 2.341988                                                         |
| 14895 | 1.738570              | 2.341998                                                         |
| 14897 | 1.000067              | 2.342009                                                         |
| 14899 | 1.024498              | 2.342019                                                         |
| 14901 | 1.333602              | 2.342029                                                         |
| 14903 | 1.143394              | 2.342040                                                         |
| 14905 | 1.313922              | 2.342050                                                         |
| 14907 | 1.333602              | 2.342061                                                         |
| 14909 | 1.060031              | 2.342071                                                         |
| 14911 | 1.141707              | 2.342081                                                         |
| 14913 | 1.445316              | 2.342092                                                         |
| 14915 | 1.271203              | 2.342102                                                         |
| 14917 | 1.143393              | 2.342113                                                         |
| 14919 | 1.333601              | 2.342123                                                         |
| 14921 | 1.026205              | 2.342133                                                         |
| 14923 | 1.000067              | 2.342144                                                         |
| 14925 | 1.661642              | 2.342154                                                         |
| 14927 | 1.157634              | 2.342165                                                         |
| 14929 | 1.000067              | 2.342175                                                         |
| 14931 | 1.714554              | 2.342186                                                         |
| 14933 | 1.016541              | 2.342196                                                         |
| 14935 | 1.253432              | 2.342206                                                         |
| 14937 | 1.439647              | 2.342217                                                         |
| 14939 | 1.000067              | 2.342227                                                         |
| 14941 | 1.019477              | 2.342237                                                         |
| 14943 | 1.416583              | 2.342248                                                         |
| 14945 | 1.418802              | 2.342258                                                         |
| 14947 | 1.000067              | 2.342269                                                         |
| 14949 | 1.586193              | 2.342279                                                         |
| 14951 | 1.000067              | 2.342289                                                         |
| 14953 | 1.053969              | 2.342300                                                         |
| 14955 | 1.601605              | 2.342310                                                         |
| 14957 | 1.000067              | 2.342321                                                         |
| 14959 | 1.143392              | 2.342331                                                         |
| 14961 | 1.333601              | 2.342341                                                         |
| 14963 | 1.077859              | 2.342352                                                         |
| 14965 | 1.246108              | 2.342362                                                         |
| 14967 | 1.445313              | 2.342372                                                         |
| 14969 | 1.000067              | 2.342383                                                         |
| 14971 | 1.091711              | 2.342393                                                         |
| 14973 | 1.641354              | 2.342404                                                         |



| $n$   | $\frac{\sigma(n)}{n}$ | $\frac{e^\gamma}{2} \log \log n + \frac{0.73\dots}{\log \log n}$ |
|-------|-----------------------|------------------------------------------------------------------|
| 14975 | 1.242070              | 2.342414                                                         |
| 14977 | 1.060025              | 2.342424                                                         |
| 14979 | 1.333600              | 2.342435                                                         |
| 14981 | 1.018891              | 2.342445                                                         |
| 14983 | 1.000067              | 2.342455                                                         |
| 14985 | 1.841041              | 2.342466                                                         |
| 14987 | 1.143391              | 2.342476                                                         |
| 14989 | 1.077857              | 2.342486                                                         |
| 14991 | 1.408845              | 2.342497                                                         |
| 14993 | 1.152538              | 2.342507                                                         |
| 14995 | 1.200400              | 2.342517                                                         |
| 14997 | 1.333600              | 2.342528                                                         |
| 14999 | 1.022468              | 2.342538                                                         |
| 15001 | 1.143390              | 2.342548                                                         |
| 15003 | 1.445311              | 2.342559                                                         |
| 15005 | 1.200400              | 2.342569                                                         |
| 15007 | 1.026188              | 2.342580                                                         |
| 15009 | 1.333600              | 2.342590                                                         |
| 15011 | 1.060023              | 2.342600                                                         |
| 15013 | 1.000067              | 2.342611                                                         |
| 15015 | 2.148252              | 2.342621                                                         |
| 15017 | 1.000067              | 2.342631                                                         |
| 15019 | 1.045076              | 2.342642                                                         |
| 15021 | 1.445310              | 2.342652                                                         |
| 15023 | 1.017640              | 2.342662                                                         |
| 15025 | 1.242063              | 2.342673                                                         |
| 15027 | 1.333600              | 2.342683                                                         |
| 15029 | 1.213654              | 2.342693                                                         |
| 15031 | 1.000067              | 2.342704                                                         |
| 15033 | 1.333599              | 2.342714                                                         |
| 15035 | 1.251480              | 2.342724                                                         |
| 15037 | 1.091707              | 2.342734                                                         |
| 15039 | 1.484141              | 2.342745                                                         |
| 15041 | 1.095007              | 2.342755                                                         |
| 15043 | 1.167054              | 2.342765                                                         |
| 15045 | 1.722832              | 2.342776                                                         |
| 15047 | 1.027181              | 2.342786                                                         |
| 15049 | 1.016679              | 2.342796                                                         |
| 15051 | 1.387283              | 2.342807                                                         |
| 15053 | 1.000066              | 2.342817                                                         |
| 15055 | 1.200399              | 2.342827                                                         |
| 15057 | 1.657701              | 2.342838                                                         |
| 15059 | 1.121190              | 2.342848                                                         |
| 15061 | 1.000066              | 2.342858                                                         |

| $n$   | $\frac{\sigma(n)}{n}$ | $\frac{e^\gamma}{2} \log \log n + \frac{0.73...}{\log \log n}$ |
|-------|-----------------------|----------------------------------------------------------------|
| 15063 | 1.333599              | 2.342868                                                       |
| 15065 | 1.261732              | 2.342879                                                       |
| 15067 | 1.152187              | 2.342889                                                       |
| 15069 | 1.333599              | 2.342899                                                       |
| 15071 | 1.143388              | 2.342910                                                       |
| 15073 | 1.000066              | 2.342920                                                       |
| 15075 | 1.817844              | 2.342930                                                       |
| 15077 | 1.000066              | 2.342941                                                       |
| 15079 | 1.060017              | 2.342951                                                       |
| 15081 | 1.457728              | 2.342961                                                       |
| 15083 | 1.000066              | 2.342971                                                       |
| 15085 | 1.374611              | 2.342982                                                       |
| 15087 | 1.374428              | 2.342992                                                       |
| 15089 | 1.017960              | 2.343002                                                       |
| 15091 | 1.000066              | 2.343013                                                       |
| 15093 | 1.632545              | 2.343023                                                       |
| 15095 | 1.200397              | 2.343033                                                       |
| 15097 | 1.034378              | 2.343043                                                       |
| 15099 | 1.525929              | 2.343054                                                       |
| 15101 | 1.000066              | 2.343064                                                       |
| 15103 | 1.091704              | 2.343074                                                       |
| 15105 | 1.715988              | 2.343084                                                       |
| 15107 | 1.000066              | 2.343095                                                       |
| 15109 | 1.036468              | 2.343105                                                       |
| 15111 | 1.527894              | 2.343115                                                       |
| 15113 | 1.219612              | 2.343125                                                       |
| 15115 | 1.200397              | 2.343136                                                       |
| 15117 | 1.333598              | 2.343146                                                       |
| 15119 | 1.077849              | 2.343156                                                       |
| 15121 | 1.000066              | 2.343167                                                       |
| 15123 | 1.352377              | 2.343177                                                       |
| 15125 | 1.371769              | 2.343187                                                       |
| 15127 | 1.143386              | 2.343197                                                       |
| 15129 | 1.480534              | 2.343208                                                       |
| 15131 | 1.000066              | 2.343218                                                       |
| 15133 | 1.029538              | 2.343228                                                       |
| 15135 | 1.601586              | 2.343238                                                       |
| 15137 | 1.000066              | 2.343249                                                       |
| 15139 | 1.000066              | 2.343259                                                       |
| 15141 | 1.566079              | 2.343269                                                       |
| 15143 | 1.053952              | 2.343279                                                       |
| 15145 | 1.297854              | 2.343289                                                       |
| 15147 | 1.725490              | 2.343300                                                       |
| 15149 | 1.000066              | 2.343310                                                       |

| $n$   | $\frac{\sigma(n)}{n}$ | $\frac{e^\gamma}{2} \log \log n + \frac{0.73\dots}{\log \log n}$ |
|-------|-----------------------|------------------------------------------------------------------|
| 15151 | 1.016435              | 2.343320                                                         |
| 15153 | 1.333597              | 2.343330                                                         |
| 15155 | 1.374596              | 2.343341                                                         |
| 15157 | 1.045062              | 2.343351                                                         |
| 15159 | 1.384788              | 2.343361                                                         |
| 15161 | 1.000066              | 2.343371                                                         |
| 15163 | 1.020906              | 2.343382                                                         |
| 15165 | 1.738477              | 2.343392                                                         |
| 15167 | 1.036461              | 2.343402                                                         |
| 15169 | 1.253082              | 2.343412                                                         |
| 15171 | 1.439589              | 2.343422                                                         |
| 15173 | 1.000066              | 2.343433                                                         |
| 15175 | 1.242043              | 2.343443                                                         |
| 15177 | 1.333597              | 2.343453                                                         |
| 15179 | 1.026155              | 2.343463                                                         |
| 15181 | 1.138265              | 2.343474                                                         |
| 15183 | 1.657643              | 2.343484                                                         |
| 15185 | 1.200395              | 2.343494                                                         |
| 15187 | 1.000066              | 2.343504                                                         |
| 15189 | 1.371519              | 2.343514                                                         |
| 15191 | 1.091699              | 2.343525                                                         |
| 15193 | 1.000066              | 2.343535                                                         |
| 15195 | 1.601579              | 2.343545                                                         |
| 15197 | 1.238139              | 2.343555                                                         |
| 15199 | 1.000066              | 2.343565                                                         |
| 15201 | 1.484113              | 2.343576                                                         |
| 15203 | 1.045057              | 2.343586                                                         |
| 15205 | 1.200395              | 2.343596                                                         |
| 15207 | 1.379365              | 2.343606                                                         |
| 15209 | 1.019396              | 2.343616                                                         |
| 15211 | 1.192821              | 2.343627                                                         |
| 15213 | 1.457701              | 2.343637                                                         |
| 15215 | 1.277686              | 2.343647                                                         |
| 15217 | 1.000066              | 2.343657                                                         |
| 15219 | 1.537552              | 2.343667                                                         |
| 15221 | 1.034360              | 2.343677                                                         |
| 15223 | 1.077843              | 2.343688                                                         |
| 15225 | 1.954680              | 2.343698                                                         |
| 15227 | 1.000066              | 2.343708                                                         |
| 15229 | 1.016744              | 2.343718                                                         |
| 15231 | 1.333596              | 2.343728                                                         |
| 15233 | 1.000066              | 2.343739                                                         |
| 15235 | 1.313817              | 2.343749                                                         |
| 15237 | 1.445298              | 2.343759                                                         |

| $n$   | $\frac{\sigma(n)}{n}$ | $\frac{e^\gamma}{2} \log \log n + \frac{0.73\dots}{\log \log n}$ |
|-------|-----------------------|------------------------------------------------------------------|
| 15239 | 1.167006              | 2.343769                                                         |
| 15241 | 1.000066              | 2.343779                                                         |
| 15243 | 1.333596              | 2.343789                                                         |
| 15245 | 1.200394              | 2.343800                                                         |
| 15247 | 1.017905              | 2.343810                                                         |
| 15249 | 1.586465              | 2.343820                                                         |
| 15251 | 1.016589              | 2.343830                                                         |
| 15253 | 1.143382              | 2.343840                                                         |
| 15255 | 1.793510              | 2.343850                                                         |
| 15257 | 1.164056              | 2.343861                                                         |
| 15259 | 1.000066              | 2.343871                                                         |
| 15261 | 1.333595              | 2.343881                                                         |
| 15263 | 1.000066              | 2.343891                                                         |
| 15265 | 1.245201              | 2.343901                                                         |
| 15267 | 1.525906              | 2.343911                                                         |
| 15269 | 1.000065              | 2.343921                                                         |
| 15271 | 1.000065              | 2.343932                                                         |
| 15273 | 1.445296              | 2.343942                                                         |
| 15275 | 1.363797              | 2.343952                                                         |
| 15277 | 1.000065              | 2.343962                                                         |
| 15279 | 1.457687              | 2.343972                                                         |
| 15281 | 1.193639              | 2.343982                                                         |
| 15283 | 1.130668              | 2.343992                                                         |
| 15285 | 1.601570              | 2.344003                                                         |
| 15287 | 1.000065              | 2.344013                                                         |
| 15289 | 1.000065              | 2.344023                                                         |
| 15291 | 1.445295              | 2.344033                                                         |
| 15293 | 1.027137              | 2.344043                                                         |
| 15295 | 1.506375              | 2.344053                                                         |
| 15297 | 1.333595              | 2.344063                                                         |
| 15299 | 1.000065              | 2.344073                                                         |
| 15301 | 1.185805              | 2.344084                                                         |
| 15303 | 1.333595              | 2.344094                                                         |
| 15305 | 1.200392              | 2.344104                                                         |
| 15307 | 1.000065              | 2.344114                                                         |
| 15309 | 1.714024              | 2.344124                                                         |
| 15311 | 1.020443              | 2.344134                                                         |
| 15313 | 1.000065              | 2.344144                                                         |
| 15315 | 1.601567              | 2.344154                                                         |
| 15317 | 1.082327              | 2.344165                                                         |
| 15319 | 1.000065              | 2.344175                                                         |
| 15321 | 1.333594              | 2.344185                                                         |
| 15323 | 1.253018              | 2.344195                                                         |
| 15325 | 1.242023              | 2.344205                                                         |

| $n$   | $\frac{\sigma(n)}{n}$ | $\frac{e^\gamma}{2} \log \log n + \frac{0.73...}{\log \log n}$ |
|-------|-----------------------|----------------------------------------------------------------|
| 15327 | 1.567430              | 2.344215                                                       |
| 15329 | 1.000065              | 2.344225                                                       |
| 15331 | 1.000065              | 2.344235                                                       |
| 15333 | 1.408726              | 2.344245                                                       |
| 15335 | 1.200391              | 2.344256                                                       |
| 15337 | 1.166982              | 2.344266                                                       |
| 15339 | 1.333594              | 2.344276                                                       |
| 15341 | 1.081416              | 2.344286                                                       |
| 15343 | 1.019357              | 2.344296                                                       |
| 15345 | 1.951906              | 2.344306                                                       |
| 15347 | 1.016485              | 2.344316                                                       |
| 15349 | 1.000065              | 2.344326                                                       |
| 15351 | 1.650967              | 2.344336                                                       |
| 15353 | 1.077835              | 2.344346                                                       |
| 15355 | 1.247281              | 2.344356                                                       |
| 15357 | 1.333594              | 2.344367                                                       |
| 15359 | 1.000065              | 2.344377                                                       |
| 15361 | 1.000065              | 2.344387                                                       |
| 15363 | 1.484085              | 2.344397                                                       |
| 15365 | 1.374553              | 2.344407                                                       |
| 15367 | 1.107828              | 2.344417                                                       |
| 15369 | 1.374195              | 2.344427                                                       |
| 15371 | 1.053933              | 2.344437                                                       |
| 15373 | 1.000065              | 2.344447                                                       |
| 15375 | 1.704585              | 2.344457                                                       |
| 15377 | 1.000065              | 2.344467                                                       |
| 15379 | 1.238052              | 2.344477                                                       |
| 15381 | 1.445290              | 2.344487                                                       |
| 15383 | 1.000065              | 2.344498                                                       |
| 15385 | 1.277608              | 2.344508                                                       |
| 15387 | 1.397543              | 2.344518                                                       |
| 15389 | 1.091689              | 2.344528                                                       |
| 15391 | 1.000065              | 2.344538                                                       |
| 15393 | 1.525888              | 2.344548                                                       |
| 15395 | 1.200390              | 2.344558                                                       |
| 15397 | 1.017081              | 2.344568                                                       |
| 15399 | 1.519579              | 2.344578                                                       |
| 15401 | 1.000065              | 2.344588                                                       |
| 15403 | 1.018503              | 2.344598                                                       |
| 15405 | 1.744888              | 2.344608                                                       |
| 15407 | 1.196339              | 2.344618                                                       |
| 15409 | 1.053930              | 2.344628                                                       |
| 15411 | 1.457660              | 2.344638                                                       |
| 15413 | 1.000065              | 2.344648                                                       |

| $n$   | $\frac{\sigma(n)}{n}$ | $\frac{e^\gamma}{2} \log \log n + \frac{0.73...}{\log \log n}$ |
|-------|-----------------------|----------------------------------------------------------------|
| 15415 | 1.200389              | 2.344658                                                       |
| 15417 | 1.484076              | 2.344668                                                       |
| 15419 | 1.059991              | 2.344678                                                       |
| 15421 | 1.143376              | 2.344689                                                       |
| 15423 | 1.372496              | 2.344699                                                       |
| 15425 | 1.242010              | 2.344709                                                       |
| 15427 | 1.000065              | 2.344719                                                       |
| 15429 | 1.379221              | 2.344729                                                       |
| 15431 | 1.077830              | 2.344739                                                       |
| 15433 | 1.157001              | 2.344749                                                       |
| 15435 | 2.021380              | 2.344759                                                       |
| 15437 | 1.026106              | 2.344769                                                       |
| 15439 | 1.000065              | 2.344779                                                       |
| 15441 | 1.333592              | 2.344789                                                       |
| 15443 | 1.000065              | 2.344799                                                       |
| 15445 | 1.200388              | 2.344809                                                       |
| 15447 | 1.408688              | 2.344819                                                       |
| 15449 | 1.143375              | 2.344829                                                       |
| 15451 | 1.000065              | 2.344839                                                       |
| 15453 | 1.544554              | 2.344849                                                       |
| 15455 | 1.313750              | 2.344859                                                       |
| 15457 | 1.141231              | 2.344869                                                       |
| 15459 | 1.333592              | 2.344879                                                       |
| 15461 | 1.000065              | 2.344889                                                       |
| 15463 | 1.167691              | 2.344899                                                       |
| 15465 | 1.601552              | 2.344909                                                       |
| 15467 | 1.000065              | 2.344919                                                       |
| 15469 | 1.034327              | 2.344929                                                       |
| 15471 | 1.501648              | 2.344939                                                       |
| 15473 | 1.000065              | 2.344949                                                       |
| 15475 | 1.242003              | 2.344959                                                       |
| 15477 | 1.687149              | 2.344969                                                       |
| 15479 | 1.045029              | 2.344979                                                       |
| 15481 | 1.016213              | 2.344989                                                       |
| 15483 | 1.439514              | 2.344999                                                       |
| 15485 | 1.270907              | 2.345009                                                       |
| 15487 | 1.059986              | 2.345019                                                       |
| 15489 | 1.445284              | 2.345029                                                       |
| 15491 | 1.143374              | 2.345039                                                       |
| 15493 | 1.000065              | 2.345049                                                       |
| 15495 | 1.601549              | 2.345059                                                       |
| 15497 | 1.000065              | 2.345069                                                       |
| 15499 | 1.091683              | 2.345079                                                       |
| 15501 | 1.333591              | 2.345089                                                       |

| $n$   | $\frac{\sigma(n)}{n}$ | $\frac{e^\gamma}{2} \log \log n + \frac{0.73\dots}{\log \log n}$ |
|-------|-----------------------|------------------------------------------------------------------|
| 15503 | 1.029478              | 2.345099                                                         |
| 15505 | 1.374524              | 2.345109                                                         |
| 15507 | 1.445283              | 2.345119                                                         |
| 15509 | 1.077826              | 2.345129                                                         |
| 15511 | 1.000064              | 2.345139                                                         |
| 15513 | 1.333591              | 2.345149                                                         |
| 15515 | 1.252981              | 2.345159                                                         |
| 15517 | 1.020816              | 2.345169                                                         |
| 15519 | 1.525872              | 2.345179                                                         |
| 15521 | 1.168997              | 2.345189                                                         |
| 15523 | 1.079946              | 2.345199                                                         |
| 15525 | 1.916908              | 2.345209                                                         |
| 15527 | 1.000064              | 2.345219                                                         |
| 15529 | 1.022345              | 2.345229                                                         |
| 15531 | 1.384586              | 2.345239                                                         |
| 15533 | 1.166935              | 2.345249                                                         |
| 15535 | 1.297715              | 2.345258                                                         |
| 15537 | 1.333591              | 2.345268                                                         |
| 15539 | 1.027093              | 2.345278                                                         |
| 15541 | 1.000064              | 2.345288                                                         |
| 15543 | 1.585794              | 2.345298                                                         |
| 15545 | 1.200386              | 2.345308                                                         |
| 15547 | 1.143372              | 2.345318                                                         |
| 15549 | 1.370635              | 2.345328                                                         |
| 15551 | 1.000064              | 2.345338                                                         |
| 15553 | 1.016396              | 2.345348                                                         |
| 15555 | 1.721890              | 2.345358                                                         |
| 15557 | 1.024362              | 2.345368                                                         |
| 15559 | 1.000064              | 2.345378                                                         |
| 15561 | 1.871345              | 2.345388                                                         |
| 15563 | 1.017799              | 2.345398                                                         |
| 15565 | 1.313717              | 2.345408                                                         |
| 15567 | 1.333590              | 2.345418                                                         |
| 15569 | 1.000064              | 2.345428                                                         |
| 15571 | 1.045020              | 2.345438                                                         |
| 15573 | 1.387016              | 2.345447                                                         |
| 15575 | 1.433066              | 2.345457                                                         |
| 15577 | 1.029467              | 2.345467                                                         |
| 15579 | 1.484049              | 2.345477                                                         |
| 15581 | 1.000064              | 2.345487                                                         |
| 15583 | 1.000064              | 2.345497                                                         |
| 15585 | 1.601540              | 2.345507                                                         |
| 15587 | 1.185603              | 2.345517                                                         |
| 15589 | 1.219321              | 2.345527                                                         |

| $n$   | $\frac{\sigma(n)}{n}$ | $\frac{e^\gamma}{2} \log \log n + \frac{0.73...}{\log \log n}$ |
|-------|-----------------------|----------------------------------------------------------------|
| 15591 | 1.333590              | 2.345537                                                       |
| 15593 | 1.034310              | 2.345547                                                       |
| 15595 | 1.200385              | 2.345557                                                       |
| 15597 | 1.445278              | 2.345567                                                       |
| 15599 | 1.053914              | 2.345576                                                       |
| 15601 | 1.000064              | 2.345586                                                       |
| 15603 | 1.525860              | 2.345596                                                       |
| 15605 | 1.200384              | 2.345606                                                       |
| 15607 | 1.000064              | 2.345616                                                       |
| 15609 | 1.499648              | 2.345626                                                       |
| 15611 | 1.019281              | 2.345636                                                       |
| 15613 | 1.077820              | 2.345646                                                       |
| 15615 | 1.738329              | 2.345656                                                       |
| 15617 | 1.204841              | 2.345666                                                       |
| 15619 | 1.000064              | 2.345676                                                       |
| 15621 | 1.376608              | 2.345685                                                       |
| 15623 | 1.059976              | 2.345695                                                       |
| 15625 | 1.249984              | 2.345705                                                       |
| 15627 | 1.333589              | 2.345715                                                       |
| 15629 | 1.000064              | 2.345725                                                       |
| 15631 | 1.312776              | 2.345735                                                       |
| 15633 | 1.501567              | 2.345745                                                       |
| 15635 | 1.243364              | 2.345755                                                       |
| 15637 | 1.053911              | 2.345765                                                       |
| 15639 | 1.439478              | 2.345774                                                       |
| 15641 | 1.000064              | 2.345784                                                       |
| 15643 | 1.000064              | 2.345794                                                       |
| 15645 | 1.840844              | 2.345804                                                       |
| 15647 | 1.000064              | 2.345814                                                       |
| 15649 | 1.000064              | 2.345824                                                       |
| 15651 | 1.515047              | 2.345834                                                       |
| 15653 | 1.091676              | 2.345844                                                       |
| 15655 | 1.250974              | 2.345854                                                       |
| 15657 | 1.416363              | 2.345863                                                       |
| 15659 | 1.143368              | 2.345873                                                       |
| 15661 | 1.000064              | 2.345883                                                       |
| 15663 | 1.397433              | 2.345893                                                       |
| 15665 | 1.297670              | 2.345903                                                       |
| 15667 | 1.000064              | 2.345913                                                       |
| 15669 | 1.445274              | 2.345923                                                       |
| 15671 | 1.000064              | 2.345932                                                       |
| 15673 | 1.143368              | 2.345942                                                       |
| 15675 | 1.898565              | 2.345952                                                       |
| 15677 | 1.020348              | 2.345962                                                       |



| $n$   | $\frac{\sigma(n)}{n}$ | $\frac{e^\gamma}{2} \log \log n + \frac{0.73\dots}{\log \log n}$ |
|-------|-----------------------|------------------------------------------------------------------|
| 15679 | 1.000064              | 2.345972                                                         |
| 15681 | 1.333588              | 2.345982                                                         |
| 15683 | 1.000064              | 2.345992                                                         |
| 15685 | 1.200383              | 2.346002                                                         |
| 15687 | 1.713521              | 2.346011                                                         |
| 15689 | 1.036395              | 2.346021                                                         |
| 15691 | 1.156332              | 2.346031                                                         |
| 15693 | 1.333588              | 2.346041                                                         |
| 15695 | 1.244728              | 2.346051                                                         |
| 15697 | 1.091674              | 2.346061                                                         |
| 15699 | 1.333588              | 2.346070                                                         |
| 15701 | 1.143367              | 2.346080                                                         |
| 15703 | 1.027065              | 2.346090                                                         |
| 15705 | 1.738300              | 2.346100                                                         |
| 15707 | 1.016107              | 2.346110                                                         |
| 15709 | 1.045006              | 2.346120                                                         |
| 15711 | 1.333588              | 2.346130                                                         |
| 15713 | 1.053904              | 2.346139                                                         |
| 15715 | 1.374483              | 2.346149                                                         |
| 15717 | 1.490361              | 2.346159                                                         |
| 15719 | 1.091672              | 2.346169                                                         |
| 15721 | 1.017747              | 2.346179                                                         |
| 15723 | 1.445271              | 2.346189                                                         |
| 15725 | 1.348426              | 2.346198                                                         |
| 15727 | 1.000064              | 2.346208                                                         |
| 15729 | 1.565516              | 2.346218                                                         |
| 15731 | 1.000064              | 2.346228                                                         |
| 15733 | 1.000064              | 2.346238                                                         |
| 15735 | 1.601525              | 2.346247                                                         |
| 15737 | 1.000064              | 2.346257                                                         |
| 15739 | 1.000064              | 2.346267                                                         |
| 15741 | 1.646655              | 2.346277                                                         |
| 15743 | 1.237884              | 2.346287                                                         |
| 15745 | 1.243823              | 2.346297                                                         |
| 15747 | 1.386931              | 2.346306                                                         |
| 15749 | 1.000063              | 2.346316                                                         |
| 15751 | 1.053901              | 2.346326                                                         |
| 15753 | 1.371167              | 2.346336                                                         |
| 15755 | 1.261314              | 2.346346                                                         |
| 15757 | 1.143365              | 2.346355                                                         |
| 15759 | 1.544260              | 2.346365                                                         |
| 15761 | 1.000063              | 2.346375                                                         |
| 15763 | 1.091670              | 2.346385                                                         |
| 15765 | 1.601522              | 2.346395                                                         |

| $n$   | $\frac{\sigma(n)}{n}$ | $\frac{e^\gamma}{2} \log \log n + \frac{0.73\dots}{\log \log n}$ |
|-------|-----------------------|------------------------------------------------------------------|
| 15767 | 1.000063              | 2.346404                                                         |
| 15769 | 1.077811              | 2.346414                                                         |
| 15771 | 1.525839              | 2.346424                                                         |
| 15773 | 1.000063              | 2.346434                                                         |
| 15775 | 1.241965              | 2.346444                                                         |
| 15777 | 1.445268              | 2.346453                                                         |
| 15779 | 1.034286              | 2.346463                                                         |
| 15781 | 1.026044              | 2.346473                                                         |
| 15783 | 1.333587              | 2.346483                                                         |
| 15785 | 1.532594              | 2.346493                                                         |
| 15787 | 1.000063              | 2.346502                                                         |
| 15789 | 1.408576              | 2.346512                                                         |
| 15791 | 1.000063              | 2.346522                                                         |
| 15793 | 1.059963              | 2.346532                                                         |
| 15795 | 1.935802              | 2.346542                                                         |
| 15797 | 1.000063              | 2.346551                                                         |
| 15799 | 1.192987              | 2.346561                                                         |
| 15801 | 1.397380              | 2.346571                                                         |
| 15803 | 1.000063              | 2.346581                                                         |
| 15805 | 1.252768              | 2.346590                                                         |
| 15807 | 1.457582              | 2.346600                                                         |
| 15809 | 1.000063              | 2.346610                                                         |
| 15811 | 1.016507              | 2.346620                                                         |
| 15813 | 1.657371              | 2.346630                                                         |
| 15815 | 1.200379              | 2.346639                                                         |
| 15817 | 1.000063              | 2.346649                                                         |
| 15819 | 1.333586              | 2.346659                                                         |
| 15821 | 1.077808              | 2.346669                                                         |
| 15823 | 1.000063              | 2.346678                                                         |
| 15825 | 1.661169              | 2.346688                                                         |
| 15827 | 1.296519              | 2.346698                                                         |
| 15829 | 1.091667              | 2.346708                                                         |
| 15831 | 1.445266              | 2.346717                                                         |
| 15833 | 1.018632              | 2.346727                                                         |
| 15835 | 1.200379              | 2.346737                                                         |
| 15837 | 1.333586              | 2.346747                                                         |
| 15839 | 1.024307              | 2.346756                                                         |
| 15841 | 1.195884              | 2.346766                                                         |
| 15843 | 1.333586              | 2.346776                                                         |
| 15845 | 1.200379              | 2.346786                                                         |
| 15847 | 1.144949              | 2.346795                                                         |
| 15849 | 1.484005              | 2.346805                                                         |
| 15851 | 1.107564              | 2.346815                                                         |
| 15853 | 1.017347              | 2.346825                                                         |

| $n$   | $\frac{\sigma(n)}{n}$ | $\frac{e^\gamma}{2} \log \log n + \frac{0.73...}{\log \log n}$ |
|-------|-----------------------|----------------------------------------------------------------|
| 15855 | 1.840681              | 2.346834                                                       |
| 15857 | 1.016333              | 2.346844                                                       |
| 15859 | 1.000063              | 2.346854                                                       |
| 15861 | 1.416304              | 2.346864                                                       |
| 15863 | 1.036374              | 2.346873                                                       |
| 15865 | 1.270722              | 2.346883                                                       |
| 15867 | 1.514086              | 2.346893                                                       |
| 15869 | 1.143361              | 2.346903                                                       |
| 15871 | 1.020730              | 2.346912                                                       |
| 15873 | 1.608770              | 2.346922                                                       |
| 15875 | 1.257827              | 2.346932                                                       |
| 15877 | 1.000063              | 2.346941                                                       |
| 15879 | 1.370363              | 2.346951                                                       |
| 15881 | 1.000063              | 2.346961                                                       |
| 15883 | 1.143361              | 2.346971                                                       |
| 15885 | 1.738244              | 2.346980                                                       |
| 15887 | 1.000063              | 2.346990                                                       |
| 15889 | 1.000063              | 2.347000                                                       |
| 15891 | 1.333585              | 2.347009                                                       |
| 15893 | 1.044988              | 2.347019                                                       |
| 15895 | 1.390626              | 2.347029                                                       |
| 15897 | 1.525822              | 2.347039                                                       |
| 15899 | 1.077804              | 2.347048                                                       |
| 15901 | 1.000063              | 2.347058                                                       |
| 15903 | 1.609759              | 2.347068                                                       |
| 15905 | 1.200377              | 2.347077                                                       |
| 15907 | 1.000063              | 2.347087                                                       |
| 15909 | 1.333585              | 2.347097                                                       |
| 15911 | 1.143360              | 2.347107                                                       |
| 15913 | 1.000063              | 2.347116                                                       |
| 15915 | 1.601508              | 2.347126                                                       |
| 15917 | 1.091663              | 2.347136                                                       |
| 15919 | 1.000063              | 2.347145                                                       |
| 15921 | 1.518749              | 2.347155                                                       |
| 15923 | 1.000063              | 2.347165                                                       |
| 15925 | 1.553407              | 2.347174                                                       |
| 15927 | 1.333584              | 2.347184                                                       |
| 15929 | 1.059954              | 2.347194                                                       |
| 15931 | 1.016885              | 2.347204                                                       |
| 15933 | 1.373753              | 2.347213                                                       |
| 15935 | 1.200377              | 2.347223                                                       |
| 15937 | 1.000063              | 2.347233                                                       |
| 15939 | 1.879164              | 2.347242                                                       |
| 15941 | 1.053886              | 2.347252                                                       |

| $n$   | $\frac{\sigma(n)}{n}$ | $\frac{e^\gamma}{2} \log \log n + \frac{0.73\dots}{\log \log n}$ |
|-------|-----------------------|------------------------------------------------------------------|
| 15943 | 1.016120              | 2.347262                                                         |
| 15945 | 1.601505              | 2.347271                                                         |
| 15947 | 1.029410              | 2.347281                                                         |
| 15949 | 1.027024              | 2.347291                                                         |
| 15951 | 1.439408              | 2.347300                                                         |
| 15953 | 1.191500              | 2.347310                                                         |
| 15955 | 1.200376              | 2.347320                                                         |
| 15957 | 1.501410              | 2.347329                                                         |
| 15959 | 1.000063              | 2.347339                                                         |
| 15961 | 1.091661              | 2.347349                                                         |
| 15963 | 1.416275              | 2.347358                                                         |
| 15965 | 1.250736              | 2.347368                                                         |
| 15967 | 1.143358              | 2.347378                                                         |
| 15969 | 1.333584              | 2.347387                                                         |
| 15971 | 1.000063              | 2.347397                                                         |
| 15973 | 1.000063              | 2.347407                                                         |
| 15975 | 1.816338              | 2.347416                                                         |
| 15977 | 1.077799              | 2.347426                                                         |
| 15979 | 1.090181              | 2.347436                                                         |
| 15981 | 1.525812              | 2.347445                                                         |
| 15983 | 1.091660              | 2.347455                                                         |
| 15985 | 1.261182              | 2.347465                                                         |
| 15987 | 1.351848              | 2.347474                                                         |
| 15989 | 1.020702              | 2.347484                                                         |
| 15991 | 1.000063              | 2.347494                                                         |
| 15993 | 1.445257              | 2.347503                                                         |
| 15995 | 1.374430              | 2.347513                                                         |
| 15997 | 1.059949              | 2.347523                                                         |
| 15999 | 1.333583              | 2.347532                                                         |
| 16001 | 1.000062              | 2.347542                                                         |
| 16003 | 1.077798              | 2.347552                                                         |
| 16005 | 1.763449              | 2.347561                                                         |
| 16007 | 1.000062              | 2.347571                                                         |
| 16009 | 1.143357              | 2.347581                                                         |
| 16011 | 1.483980              | 2.347590                                                         |
| 16013 | 1.019172              | 2.347600                                                         |
| 16015 | 1.200375              | 2.347609                                                         |
| 16017 | 1.408503              | 2.347619                                                         |
| 16019 | 1.017292              | 2.347629                                                         |
| 16021 | 1.029399              | 2.347638                                                         |
| 16023 | 1.565250              | 2.347648                                                         |
| 16025 | 1.241934              | 2.347658                                                         |
| 16027 | 1.150059              | 2.347667                                                         |
| 16029 | 1.566910              | 2.347677                                                         |

| $n$   | $\frac{\sigma(n)}{n}$ | $\frac{e^\gamma}{2} \log \log n + \frac{0.73...}{\log \log n}$ |
|-------|-----------------------|----------------------------------------------------------------|
| 16031 | 1.131807              | 2.347686                                                       |
| 16033 | 1.000062              | 2.347696                                                       |
| 16035 | 1.601497              | 2.347706                                                       |
| 16037 | 1.197231              | 2.347715                                                       |
| 16039 | 1.025999              | 2.347725                                                       |
| 16041 | 1.333583              | 2.347735                                                       |
| 16043 | 1.020258              | 2.347744                                                       |
| 16045 | 1.200374              | 2.347754                                                       |
| 16047 | 1.445255              | 2.347763                                                       |
| 16049 | 1.091657              | 2.347773                                                       |
| 16051 | 1.143356              | 2.347783                                                       |
| 16053 | 1.333583              | 2.347792                                                       |
| 16055 | 1.367798              | 2.347802                                                       |
| 16057 | 1.000062              | 2.347811                                                       |
| 16059 | 1.371941              | 2.347821                                                       |
| 16061 | 1.000062              | 2.347831                                                       |
| 16063 | 1.000062              | 2.347840                                                       |
| 16065 | 2.151261              | 2.347850                                                       |
| 16067 | 1.000062              | 2.347859                                                       |
| 16069 | 1.000062              | 2.347869                                                       |
| 16071 | 1.457532              | 2.347879                                                       |
| 16073 | 1.000062              | 2.347888                                                       |
| 16075 | 1.241928              | 2.347898                                                       |
| 16077 | 1.397276              | 2.347907                                                       |
| 16079 | 1.143355              | 2.347917                                                       |
| 16081 | 1.077794              | 2.347927                                                       |
| 16083 | 1.445253              | 2.347936                                                       |
| 16085 | 1.200373              | 2.347946                                                       |
| 16087 | 1.000062              | 2.347955                                                       |
| 16089 | 1.384300              | 2.347965                                                       |
| 16091 | 1.000062              | 2.347975                                                       |
| 16093 | 1.322314              | 2.347984                                                       |
| 16095 | 1.699907              | 2.347994                                                       |
| 16097 | 1.000062              | 2.348003                                                       |
| 16099 | 1.059942              | 2.348013                                                       |
| 16101 | 1.445252              | 2.348023                                                       |
| 16103 | 1.000062              | 2.348032                                                       |
| 16105 | 1.200373              | 2.348042                                                       |
| 16107 | 1.668840              | 2.348051                                                       |
| 16109 | 1.016823              | 2.348061                                                       |
| 16111 | 1.000062              | 2.348070                                                       |
| 16113 | 1.376280              | 2.348080                                                       |
| 16115 | 1.313559              | 2.348090                                                       |
| 16117 | 1.018552              | 2.348099                                                       |

| $n$   | $\frac{\sigma(n)}{n}$ | $\frac{e^\gamma}{2} \log \log n + \frac{0.73...}{\log \log n}$ |
|-------|-----------------------|----------------------------------------------------------------|
| 16119 | 1.501334              | 2.348109                                                       |
| 16121 | 1.190993              | 2.348118                                                       |
| 16123 | 1.044967              | 2.348128                                                       |
| 16125 | 1.702698              | 2.348137                                                       |
| 16127 | 1.000062              | 2.348147                                                       |
| 16129 | 1.007936              | 2.348157                                                       |
| 16131 | 1.408468              | 2.348166                                                       |
| 16133 | 1.155892              | 2.348176                                                       |
| 16135 | 1.374403              | 2.348185                                                       |
| 16137 | 1.585425              | 2.348195                                                       |
| 16139 | 1.000062              | 2.348204                                                       |
| 16141 | 1.000062              | 2.348214                                                       |
| 16143 | 1.333581              | 2.348223                                                       |
| 16145 | 1.200372              | 2.348233                                                       |
| 16147 | 1.019137              | 2.348243                                                       |
| 16149 | 1.525791              | 2.348252                                                       |
| 16151 | 1.034239              | 2.348262                                                       |
| 16153 | 1.036340              | 2.348271                                                       |
| 16155 | 1.738162              | 2.348281                                                       |
| 16157 | 1.016030              | 2.348290                                                       |
| 16159 | 1.185222              | 2.348300                                                       |
| 16161 | 1.333581              | 2.348309                                                       |
| 16163 | 1.143352              | 2.348319                                                       |
| 16165 | 1.242685              | 2.348328                                                       |
| 16167 | 1.416218              | 2.348338                                                       |
| 16169 | 1.128085              | 2.348348                                                       |
| 16171 | 1.016140              | 2.348357                                                       |
| 16173 | 1.483955              | 2.348367                                                       |
| 16175 | 1.241917              | 2.348376                                                       |
| 16177 | 1.143352              | 2.348386                                                       |
| 16179 | 1.333581              | 2.348395                                                       |
| 16181 | 1.091651              | 2.348405                                                       |
| 16183 | 1.000062              | 2.348414                                                       |
| 16185 | 1.743837              | 2.348424                                                       |
| 16187 | 1.000062              | 2.348433                                                       |
| 16189 | 1.000062              | 2.348443                                                       |
| 16191 | 1.657217              | 2.348452                                                       |
| 16193 | 1.000062              | 2.348462                                                       |
| 16195 | 1.244829              | 2.348471                                                       |
| 16197 | 1.333580              | 2.348481                                                       |
| 16199 | 1.016359              | 2.348490                                                       |
| 16201 | 1.059935              | 2.348500                                                       |
| 16203 | 1.457508              | 2.348509                                                       |
| 16205 | 1.374391              | 2.348519                                                       |

| $n$   | $\frac{\sigma(n)}{n}$ | $\frac{e^\gamma}{2} \log \log n + \frac{0.73...}{\log \log n}$ |
|-------|-----------------------|----------------------------------------------------------------|
| 16207 | 1.053866              | 2.348528                                                       |
| 16209 | 1.445246              | 2.348538                                                       |
| 16211 | 1.139967              | 2.348547                                                       |
| 16213 | 1.034232              | 2.348557                                                       |
| 16215 | 1.705088              | 2.348566                                                       |
| 16217 | 1.000062              | 2.348576                                                       |
| 16219 | 1.166780              | 2.348586                                                       |
| 16221 | 1.333580              | 2.348595                                                       |
| 16223 | 1.000062              | 2.348605                                                       |
| 16225 | 1.375655              | 2.348614                                                       |
| 16227 | 1.483947              | 2.348624                                                       |
| 16229 | 1.000062              | 2.348633                                                       |
| 16231 | 1.000062              | 2.348643                                                       |
| 16233 | 1.525781              | 2.348652                                                       |
| 16235 | 1.277241              | 2.348661                                                       |
| 16237 | 1.077785              | 2.348671                                                       |
| 16239 | 1.333580              | 2.348680                                                       |
| 16241 | 1.015947              | 2.348690                                                       |
| 16243 | 1.029366              | 2.348699                                                       |
| 16245 | 1.829363              | 2.348709                                                       |
| 16247 | 1.252662              | 2.348718                                                       |
| 16249 | 1.000062              | 2.348728                                                       |
| 16251 | 1.333579              | 2.348737                                                       |
| 16253 | 1.000062              | 2.348747                                                       |
| 16255 | 1.200369              | 2.348756                                                       |
| 16257 | 1.333579              | 2.348766                                                       |
| 16259 | 1.018513              | 2.348775                                                       |
| 16261 | 1.204354              | 2.348785                                                       |
| 16263 | 1.566747              | 2.348794                                                       |
| 16265 | 1.200369              | 2.348804                                                       |
| 16267 | 1.000061              | 2.348813                                                       |
| 16269 | 1.593214              | 2.348823                                                       |
| 16271 | 1.022187              | 2.348832                                                       |
| 16273 | 1.000061              | 2.348842                                                       |
| 16275 | 1.950476              | 2.348851                                                       |
| 16277 | 1.026971              | 2.348861                                                       |
| 16279 | 1.018244              | 2.348870                                                       |
| 16281 | 1.520300              | 2.348880                                                       |
| 16283 | 1.053860              | 2.348889                                                       |
| 16285 | 1.200368              | 2.348898                                                       |
| 16287 | 1.370418              | 2.348908                                                       |
| 16289 | 1.237645              | 2.348917                                                       |
| 16291 | 1.091646              | 2.348927                                                       |
| 16293 | 1.333579              | 2.348936                                                       |

| $n$   | $\frac{\sigma(n)}{n}$ | $\frac{e^\gamma}{2} \log \log n + \frac{0.73...}{\log \log n}$ |
|-------|-----------------------|----------------------------------------------------------------|
| 16295 | 1.200368              | 2.348946                                                       |
| 16297 | 1.025956              | 2.348955                                                       |
| 16299 | 1.445242              | 2.348965                                                       |
| 16301 | 1.000061              | 2.348974                                                       |
| 16303 | 1.218917              | 2.348984                                                       |
| 16305 | 1.601472              | 2.348993                                                       |
| 16307 | 1.044950              | 2.349002                                                       |
| 16309 | 1.024220              | 2.349012                                                       |
| 16311 | 1.333579              | 2.349021                                                       |
| 16313 | 1.091645              | 2.349031                                                       |
| 16315 | 1.297456              | 2.349040                                                       |
| 16317 | 1.725685              | 2.349050                                                       |
| 16319 | 1.000061              | 2.349059                                                       |
| 16321 | 1.053857              | 2.349069                                                       |
| 16323 | 1.333578              | 2.349078                                                       |
| 16325 | 1.241899              | 2.349087                                                       |
| 16327 | 1.036320              | 2.349097                                                       |
| 16329 | 1.333578              | 2.349106                                                       |
| 16331 | 1.143347              | 2.349116                                                       |
| 16333 | 1.000061              | 2.349125                                                       |
| 16335 | 1.954086              | 2.349135                                                       |
| 16337 | 1.094081              | 2.349144                                                       |
| 16339 | 1.000061              | 2.349153                                                       |
| 16341 | 1.439324              | 2.349163                                                       |
| 16343 | 1.020620              | 2.349172                                                       |
| 16345 | 1.374365              | 2.349182                                                       |
| 16347 | 1.333578              | 2.349191                                                       |
| 16349 | 1.000061              | 2.349201                                                       |
| 16351 | 1.017185              | 2.349210                                                       |
| 16353 | 1.526325              | 2.349219                                                       |
| 16355 | 1.200367              | 2.349229                                                       |
| 16357 | 1.091643              | 2.349238                                                       |
| 16359 | 1.643132              | 2.349248                                                       |
| 16361 | 1.000061              | 2.349257                                                       |
| 16363 | 1.000061              | 2.349267                                                       |
| 16365 | 1.601467              | 2.349276                                                       |
| 16367 | 1.077778              | 2.349285                                                       |
| 16369 | 1.000061              | 2.349295                                                       |
| 16371 | 1.543705              | 2.349304                                                       |
| 16373 | 1.143346              | 2.349314                                                       |
| 16375 | 1.257527              | 2.349323                                                       |
| 16377 | 1.371680              | 2.349332                                                       |
| 16379 | 1.091642              | 2.349342                                                       |
| 16381 | 1.000061              | 2.349351                                                       |



| $n$   | $\frac{\sigma(n)}{n}$ | $\frac{e^\gamma}{2} \log \log n + \frac{0.73...}{\log \log n}$ |
|-------|-----------------------|----------------------------------------------------------------|
| 16383 | 1.375084              | 2.349361                                                       |
| 16385 | 1.252365              | 2.349370                                                       |
| 16387 | 1.143345              | 2.349379                                                       |
| 16389 | 1.483922              | 2.349389                                                       |
| 16391 | 1.029345              | 2.349398                                                       |
| 16393 | 1.094004              | 2.349408                                                       |
| 16395 | 1.601464              | 2.349417                                                       |
| 16397 | 1.053851              | 2.349426                                                       |
| 16399 | 1.079090              | 2.349436                                                       |
| 16401 | 1.685751              | 2.349445                                                       |
| 16403 | 1.024203              | 2.349455                                                       |
| 16405 | 1.277172              | 2.349464                                                       |
| 16407 | 1.445237              | 2.349473                                                       |
| 16409 | 1.020172              | 2.349483                                                       |
| 16411 | 1.000061              | 2.349492                                                       |
| 16413 | 1.333577              | 2.349501                                                       |
| 16415 | 1.416753              | 2.349511                                                       |
| 16417 | 1.000061              | 2.349520                                                       |
| 16419 | 1.439308              | 2.349530                                                       |
| 16421 | 1.000061              | 2.349539                                                       |
| 16423 | 1.091640              | 2.349548                                                       |
| 16425 | 1.815647              | 2.349558                                                       |
| 16427 | 1.000061              | 2.349567                                                       |
| 16429 | 1.143344              | 2.349576                                                       |
| 16431 | 1.333577              | 2.349586                                                       |
| 16433 | 1.000061              | 2.349595                                                       |
| 16435 | 1.270459              | 2.349605                                                       |
| 16437 | 1.333577              | 2.349614                                                       |
| 16439 | 1.059918              | 2.349623                                                       |
| 16441 | 1.026945              | 2.349633                                                       |
| 16443 | 1.766101              | 2.349642                                                       |
| 16445 | 1.471085              | 2.349651                                                       |
| 16447 | 1.000061              | 2.349661                                                       |
| 16449 | 1.333577              | 2.349670                                                       |
| 16451 | 1.000061              | 2.349679                                                       |
| 16453 | 1.000061              | 2.349689                                                       |
| 16455 | 1.601459              | 2.349698                                                       |
| 16457 | 1.143343              | 2.349708                                                       |
| 16459 | 1.015858              | 2.349717                                                       |
| 16461 | 1.516311              | 2.349726                                                       |
| 16463 | 1.016097              | 2.349736                                                       |
| 16465 | 1.246280              | 2.349745                                                       |
| 16467 | 1.457460              | 2.349754                                                       |
| 16469 | 1.025928              | 2.349764                                                       |

| $n$   | $\frac{\sigma(n)}{n}$ | $\frac{e^\gamma}{2} \log \log n + \frac{0.73...}{\log \log n}$ |
|-------|-----------------------|----------------------------------------------------------------|
| 16471 | 1.237569              | 2.349773                                                       |
| 16473 | 1.490925              | 2.349782                                                       |
| 16475 | 1.241882              | 2.349792                                                       |
| 16477 | 1.000061              | 2.349801                                                       |
| 16479 | 1.445233              | 2.349810                                                       |
| 16481 | 1.000061              | 2.349820                                                       |
| 16483 | 1.022144              | 2.349829                                                       |
| 16485 | 1.840218              | 2.349838                                                       |
| 16487 | 1.000061              | 2.349848                                                       |
| 16489 | 1.091637              | 2.349857                                                       |
| 16491 | 1.397126              | 2.349866                                                       |
| 16493 | 1.000061              | 2.349876                                                       |
| 16495 | 1.200364              | 2.349885                                                       |
| 16497 | 1.629387              | 2.349894                                                       |
| 16499 | 1.143342              | 2.349904                                                       |
| 16501 | 1.036301              | 2.349913                                                       |
| 16503 | 1.333576              | 2.349922                                                       |
| 16505 | 1.200364              | 2.349932                                                       |
| 16507 | 1.059914              | 2.349941                                                       |
| 16509 | 1.333576              | 2.349950                                                       |
| 16511 | 1.162861              | 2.349960                                                       |
| 16513 | 1.166717              | 2.349969                                                       |
| 16515 | 1.738056              | 2.349978                                                       |
| 16517 | 1.017134              | 2.349988                                                       |
| 16519 | 1.000061              | 2.349997                                                       |
| 16521 | 1.333575              | 2.350006                                                       |
| 16523 | 1.138776              | 2.350016                                                       |
| 16525 | 1.241876              | 2.350025                                                       |
| 16527 | 1.525746              | 2.350034                                                       |
| 16529 | 1.000060              | 2.350044                                                       |
| 16531 | 1.020144              | 2.350053                                                       |
| 16533 | 1.585193              | 2.350062                                                       |
| 16535 | 1.200363              | 2.350071                                                       |
| 16537 | 1.044930              | 2.350081                                                       |
| 16539 | 1.378560              | 2.350090                                                       |
| 16541 | 1.218790              | 2.350099                                                       |
| 16543 | 1.018437              | 2.350109                                                       |
| 16545 | 1.601451              | 2.350118                                                       |
| 16547 | 1.000060              | 2.350127                                                       |
| 16549 | 1.150523              | 2.350137                                                       |
| 16551 | 1.483898              | 2.350146                                                       |
| 16553 | 1.000060              | 2.350155                                                       |
| 16555 | 1.530897              | 2.350164                                                       |
| 16557 | 1.333575              | 2.350174                                                       |

| $n$   | $\frac{\sigma(n)}{n}$ | $\frac{e^\gamma}{2} \log \log n + \frac{0.73...}{\log \log n}$ |
|-------|-----------------------|----------------------------------------------------------------|
| 16559 | 1.036294              | 2.350183                                                       |
| 16561 | 1.000060              | 2.350192                                                       |
| 16563 | 1.333575              | 2.350202                                                       |
| 16565 | 1.200362              | 2.350211                                                       |
| 16567 | 1.000060              | 2.350220                                                       |
| 16569 | 1.657070              | 2.350230                                                       |
| 16571 | 1.018164              | 2.350239                                                       |
| 16573 | 1.000060              | 2.350248                                                       |
| 16575 | 1.885249              | 2.350257                                                       |
| 16577 | 1.107197              | 2.350267                                                       |
| 16579 | 1.020568              | 2.350276                                                       |
| 16581 | 1.333575              | 2.350285                                                       |
| 16583 | 1.204125              | 2.350294                                                       |
| 16585 | 1.250286              | 2.350304                                                       |
| 16587 | 1.536143              | 2.350313                                                       |
| 16589 | 1.022123              | 2.350322                                                       |
| 16591 | 1.024170              | 2.350332                                                       |
| 16593 | 1.333574              | 2.350341                                                       |
| 16595 | 1.200362              | 2.350350                                                       |
| 16597 | 1.143339              | 2.350359                                                       |
| 16599 | 1.457437              | 2.350369                                                       |
| 16601 | 1.077766              | 2.350378                                                       |
| 16603 | 1.000060              | 2.350387                                                       |
| 16605 | 1.836314              | 2.350396                                                       |
| 16607 | 1.000060              | 2.350406                                                       |
| 16609 | 1.059907              | 2.350415                                                       |
| 16611 | 1.564746              | 2.350424                                                       |
| 16613 | 1.029314              | 2.350434                                                       |
| 16615 | 1.200361              | 2.350443                                                       |
| 16617 | 1.386532              | 2.350452                                                       |
| 16619 | 1.000060              | 2.350461                                                       |
| 16621 | 1.091631              | 2.350471                                                       |
| 16623 | 1.445226              | 2.350480                                                       |
| 16625 | 1.501353              | 2.350489                                                       |
| 16627 | 1.077765              | 2.350498                                                       |
| 16629 | 1.397077              | 2.350508                                                       |
| 16631 | 1.000060              | 2.350517                                                       |
| 16633 | 1.000060              | 2.350526                                                       |
| 16635 | 1.601443              | 2.350535                                                       |
| 16637 | 1.015568              | 2.350545                                                       |
| 16639 | 1.143338              | 2.350554                                                       |
| 16641 | 1.478817              | 2.350563                                                       |
| 16643 | 1.168059              | 2.350572                                                       |
| 16645 | 1.200360              | 2.350582                                                       |

| $n$   | $\frac{\sigma(n)}{n}$ | $\frac{e^\gamma}{2} \log \log n + \frac{0.73...}{\log \log n}$ |
|-------|-----------------------|----------------------------------------------------------------|
| 16647 | 1.384033              | 2.350591                                                       |
| 16649 | 1.000060              | 2.350600                                                       |
| 16651 | 1.000060              | 2.350609                                                       |
| 16653 | 1.667928              | 2.350618                                                       |
| 16655 | 1.200360              | 2.350628                                                       |
| 16657 | 1.000060              | 2.350637                                                       |
| 16659 | 1.483883              | 2.350646                                                       |
| 16661 | 1.000060              | 2.350655                                                       |
| 16663 | 1.053832              | 2.350665                                                       |
| 16665 | 1.762736              | 2.350674                                                       |
| 16667 | 1.143337              | 2.350683                                                       |
| 16669 | 1.017458              | 2.350692                                                       |
| 16671 | 1.333573              | 2.350702                                                       |
| 16673 | 1.000060              | 2.350711                                                       |
| 16675 | 1.338531              | 2.350720                                                       |
| 16677 | 1.543443              | 2.350729                                                       |
| 16679 | 1.077762              | 2.350738                                                       |
| 16681 | 1.143337              | 2.350748                                                       |
| 16683 | 1.369538              | 2.350757                                                       |
| 16685 | 1.242793              | 2.350766                                                       |
| 16687 | 1.147720              | 2.350775                                                       |
| 16689 | 1.333573              | 2.350784                                                       |
| 16691 | 1.000060              | 2.350794                                                       |
| 16693 | 1.000060              | 2.350803                                                       |
| 16695 | 2.018329              | 2.350812                                                       |
| 16697 | 1.020543              | 2.350821                                                       |
| 16699 | 1.000060              | 2.350831                                                       |
| 16701 | 1.408299              | 2.350840                                                       |
| 16703 | 1.000060              | 2.350849                                                       |
| 16705 | 1.297336              | 2.350858                                                       |
| 16707 | 1.333573              | 2.350867                                                       |
| 16709 | 1.309953              | 2.350877                                                       |
| 16711 | 1.059901              | 2.350886                                                       |
| 16713 | 1.483875              | 2.350895                                                       |
| 16715 | 1.200359              | 2.350904                                                       |
| 16717 | 1.018125              | 2.350913                                                       |
| 16719 | 1.333573              | 2.350923                                                       |
| 16721 | 1.044914              | 2.350932                                                       |
| 16723 | 1.143336              | 2.350941                                                       |
| 16725 | 1.660747              | 2.350950                                                       |
| 16727 | 1.025886              | 2.350959                                                       |
| 16729 | 1.000060              | 2.350969                                                       |
| 16731 | 1.706294              | 2.350978                                                       |
| 16733 | 1.036276              | 2.350987                                                       |

| $n$   | $\frac{\sigma(n)}{n}$ | $\frac{e^\gamma}{2} \log \log n + \frac{0.73...}{\log \log n}$ |
|-------|-----------------------|----------------------------------------------------------------|
| 16735 | 1.200359              | 2.350996                                                       |
| 16737 | 1.525721              | 2.351005                                                       |
| 16739 | 1.053826              | 2.351014                                                       |
| 16741 | 1.000060              | 2.351024                                                       |
| 16743 | 1.333572              | 2.351033                                                       |
| 16745 | 1.277038              | 2.351042                                                       |
| 16747 | 1.000060              | 2.351051                                                       |
| 16749 | 1.445221              | 2.351060                                                       |
| 16751 | 1.143335              | 2.351070                                                       |
| 16753 | 1.091625              | 2.351079                                                       |
| 16755 | 1.601432              | 2.351088                                                       |
| 16757 | 1.077759              | 2.351097                                                       |
| 16759 | 1.000060              | 2.351106                                                       |
| 16761 | 1.378438              | 2.351115                                                       |
| 16763 | 1.000060              | 2.351125                                                       |
| 16765 | 1.374292              | 2.351134                                                       |
| 16767 | 1.564502              | 2.351143                                                       |
| 16769 | 1.026895              | 2.351152                                                       |
| 16771 | 1.034166              | 2.351161                                                       |
| 16773 | 1.333572              | 2.351170                                                       |
| 16775 | 1.374903              | 2.351180                                                       |
| 16777 | 1.053824              | 2.351189                                                       |
| 16779 | 1.647774              | 2.351198                                                       |
| 16781 | 1.016149              | 2.351207                                                       |
| 16783 | 1.077757              | 2.351216                                                       |
| 16785 | 1.737980              | 2.351225                                                       |
| 16787 | 1.000060              | 2.351235                                                       |
| 16789 | 1.015903              | 2.351244                                                       |
| 16791 | 1.386457              | 2.351253                                                       |
| 16793 | 1.143334              | 2.351262                                                       |
| 16795 | 1.200357              | 2.351271                                                       |
| 16797 | 1.457403              | 2.351280                                                       |
| 16799 | 1.015775              | 2.351289                                                       |
| 16801 | 1.022082              | 2.351299                                                       |
| 16803 | 1.445218              | 2.351308                                                       |
| 16805 | 1.200357              | 2.351317                                                       |
| 16807 | 1.166657              | 2.351326                                                       |
| 16809 | 1.439229              | 2.351335                                                       |
| 16811 | 1.000059              | 2.351344                                                       |
| 16813 | 1.130554              | 2.351353                                                       |
| 16815 | 1.712756              | 2.351363                                                       |
| 16817 | 1.018969              | 2.351372                                                       |
| 16819 | 1.107081              | 2.351381                                                       |
| 16821 | 1.712146              | 2.351390                                                       |

| $n$   | $\frac{\sigma(n)}{n}$ | $\frac{e^\gamma}{2} \log \log n + \frac{0.73...}{\log \log n}$ |
|-------|-----------------------|----------------------------------------------------------------|
| 16823 | 1.000059              | 2.351399                                                       |
| 16825 | 1.241842              | 2.351408                                                       |
| 16827 | 1.369228              | 2.351417                                                       |
| 16829 | 1.000059              | 2.351427                                                       |
| 16831 | 1.000059              | 2.351436                                                       |
| 16833 | 1.383948              | 2.351445                                                       |
| 16835 | 1.516840              | 2.351454                                                       |
| 16837 | 1.015620              | 2.351463                                                       |
| 16839 | 1.445216              | 2.351472                                                       |
| 16841 | 1.091622              | 2.351481                                                       |
| 16843 | 1.000059              | 2.351490                                                       |
| 16845 | 1.601425              | 2.351500                                                       |
| 16847 | 1.059892              | 2.351509                                                       |
| 16849 | 1.196510              | 2.351518                                                       |
| 16851 | 1.375823              | 2.351527                                                       |
| 16853 | 1.053818              | 2.351536                                                       |
| 16855 | 1.200356              | 2.351545                                                       |
| 16857 | 1.445216              | 2.351554                                                       |
| 16859 | 1.044902              | 2.351563                                                       |
| 16861 | 1.077753              | 2.351572                                                       |
| 16863 | 1.685109              | 2.351582                                                       |
| 16865 | 1.200356              | 2.351591                                                       |
| 16867 | 1.015948              | 2.351600                                                       |
| 16869 | 1.333570              | 2.351609                                                       |
| 16871 | 1.000059              | 2.351618                                                       |
| 16873 | 1.024121              | 2.351627                                                       |
| 16875 | 1.851259              | 2.351636                                                       |
| 16877 | 1.143331              | 2.351645                                                       |
| 16879 | 1.000059              | 2.351654                                                       |
| 16881 | 1.416030              | 2.351664                                                       |
| 16883 | 1.000059              | 2.351673                                                       |
| 16885 | 1.313355              | 2.351682                                                       |
| 16887 | 1.439214              | 2.351691                                                       |
| 16889 | 1.000059              | 2.351700                                                       |
| 16891 | 1.212480              | 2.351709                                                       |
| 16893 | 1.445214              | 2.351718                                                       |
| 16895 | 1.250074              | 2.351727                                                       |
| 16897 | 1.020063              | 2.351736                                                       |
| 16899 | 1.374756              | 2.351745                                                       |
| 16901 | 1.000059              | 2.351754                                                       |
| 16903 | 1.000059              | 2.351764                                                       |
| 16905 | 1.942147              | 2.351773                                                       |
| 16907 | 1.149820              | 2.351782                                                       |
| 16909 | 1.029274              | 2.351791                                                       |

| $n$   | $\frac{\sigma(n)}{n}$ | $\frac{e^\gamma}{2} \log \log n + \frac{0.73\dots}{\log \log n}$ |
|-------|-----------------------|------------------------------------------------------------------|
| 16911 | 1.445213              | 2.351800                                                         |
| 16913 | 1.077751              | 2.351809                                                         |
| 16915 | 1.276973              | 2.351818                                                         |
| 16917 | 1.333570              | 2.351827                                                         |
| 16919 | 1.143330              | 2.351836                                                         |
| 16921 | 1.000059              | 2.351845                                                         |
| 16923 | 1.333570              | 2.351854                                                         |
| 16925 | 1.241832              | 2.351863                                                         |
| 16927 | 1.000059              | 2.351873                                                         |
| 16929 | 1.715400              | 2.351882                                                         |
| 16931 | 1.000059              | 2.351891                                                         |
| 16933 | 1.190575              | 2.351900                                                         |
| 16935 | 1.601417              | 2.351909                                                         |
| 16937 | 1.000059              | 2.351918                                                         |
| 16939 | 1.077750              | 2.351927                                                         |
| 16941 | 1.333569              | 2.351936                                                         |
| 16943 | 1.000059              | 2.351945                                                         |
| 16945 | 1.200354              | 2.351954                                                         |
| 16947 | 1.656930              | 2.351963                                                         |
| 16949 | 1.059886              | 2.351972                                                         |
| 16951 | 1.155330              | 2.351981                                                         |
| 16953 | 1.333569              | 2.351990                                                         |
| 16955 | 1.200354              | 2.351999                                                         |
| 16957 | 1.034145              | 2.352008                                                         |
| 16959 | 1.333569              | 2.352018                                                         |
| 16961 | 1.143329              | 2.352027                                                         |
| 16963 | 1.000059              | 2.352036                                                         |
| 16965 | 1.931034              | 2.352045                                                         |
| 16967 | 1.077857              | 2.352054                                                         |
| 16969 | 1.018328              | 2.352063                                                         |
| 16971 | 1.333569              | 2.352072                                                         |
| 16973 | 1.091616              | 2.352081                                                         |
| 16975 | 1.431753              | 2.352090                                                         |
| 16977 | 1.333569              | 2.352099                                                         |
| 16979 | 1.000059              | 2.352108                                                         |
| 16981 | 1.000059              | 2.352117                                                         |
| 16983 | 1.611023              | 2.352126                                                         |
| 16985 | 1.243450              | 2.352135                                                         |
| 16987 | 1.000059              | 2.352144                                                         |
| 16989 | 1.525693              | 2.352153                                                         |
| 16991 | 1.077747              | 2.352162                                                         |
| 16993 | 1.000059              | 2.352171                                                         |
| 16995 | 1.762401              | 2.352180                                                         |
| 16997 | 1.044890              | 2.352189                                                         |

| $n$   | $\frac{\sigma(n)}{n}$ | $\frac{e^\gamma}{2} \log \log n + \frac{0.73\dots}{\log \log n}$ |
|-------|-----------------------|------------------------------------------------------------------|
| 16999 | 1.016530              | 2.352198                                                         |
| 17001 | 1.445209              | 2.352207                                                         |
| 17003 | 1.166618              | 2.352216                                                         |
| 17005 | 1.270215              | 2.352226                                                         |
| 17007 | 1.333569              | 2.352235                                                         |
| 17009 | 1.018049              | 2.352244                                                         |
| 17011 | 1.000059              | 2.352253                                                         |
| 17013 | 1.371187              | 2.352262                                                         |
| 17015 | 1.244079              | 2.352271                                                         |
| 17017 | 1.421637              | 2.352280                                                         |
| 17019 | 1.515483              | 2.352289                                                         |
| 17021 | 1.000059              | 2.352298                                                         |
| 17023 | 1.036245              | 2.352307                                                         |
| 17025 | 1.660617              | 2.352316                                                         |
| 17027 | 1.000059              | 2.352325                                                         |
| 17029 | 1.000059              | 2.352334                                                         |
| 17031 | 1.525688              | 2.352343                                                         |
| 17033 | 1.000059              | 2.352352                                                         |
| 17035 | 1.200352              | 2.352361                                                         |
| 17037 | 1.483829              | 2.352370                                                         |
| 17039 | 1.091613              | 2.352379                                                         |
| 17041 | 1.000059              | 2.352388                                                         |
| 17043 | 1.577187              | 2.352397                                                         |
| 17045 | 1.374245              | 2.352406                                                         |
| 17047 | 1.000059              | 2.352415                                                         |
| 17049 | 1.333568              | 2.352424                                                         |
| 17051 | 1.080289              | 2.352433                                                         |
| 17053 | 1.000059              | 2.352442                                                         |
| 17055 | 1.737907              | 2.352451                                                         |
| 17057 | 1.029255              | 2.352460                                                         |
| 17059 | 1.143326              | 2.352469                                                         |
| 17061 | 1.496747              | 2.352478                                                         |
| 17063 | 1.015531              | 2.352487                                                         |
| 17065 | 1.200352              | 2.352496                                                         |
| 17067 | 1.333568              | 2.352505                                                         |
| 17069 | 1.093561              | 2.352514                                                         |
| 17071 | 1.025833              | 2.352523                                                         |
| 17073 | 1.656885              | 2.352532                                                         |
| 17075 | 1.241816              | 2.352541                                                         |
| 17077 | 1.000059              | 2.352550                                                         |
| 17079 | 1.333568              | 2.352559                                                         |
| 17081 | 1.124056              | 2.352568                                                         |
| 17083 | 1.091612              | 2.352577                                                         |
| 17085 | 1.719403              | 2.352586                                                         |



| $n$   | $\frac{\sigma(n)}{n}$ | $\frac{e^\gamma}{2} \log \log n + \frac{0.73\dots}{\log \log n}$ |
|-------|-----------------------|------------------------------------------------------------------|
| 17087 | 1.143325              | 2.352595                                                         |
| 17089 | 1.044883              | 2.352604                                                         |
| 17091 | 1.500907              | 2.352613                                                         |
| 17093 | 1.000059              | 2.352622                                                         |
| 17095 | 1.297221              | 2.352631                                                         |
| 17097 | 1.375680              | 2.352640                                                         |
| 17099 | 1.000058              | 2.352649                                                         |
| 17101 | 1.166598              | 2.352658                                                         |
| 17103 | 1.333567              | 2.352667                                                         |
| 17105 | 1.313300              | 2.352675                                                         |
| 17107 | 1.000058              | 2.352684                                                         |
| 17109 | 1.445204              | 2.352693                                                         |
| 17111 | 1.018292              | 2.352702                                                         |
| 17113 | 1.015602              | 2.352711                                                         |
| 17115 | 1.839790              | 2.352720                                                         |
| 17117 | 1.000058              | 2.352729                                                         |
| 17119 | 1.135580              | 2.352738                                                         |
| 17121 | 1.439168              | 2.352747                                                         |
| 17123 | 1.000058              | 2.352756                                                         |
| 17125 | 1.257109              | 2.352765                                                         |
| 17127 | 1.584866              | 2.352774                                                         |
| 17129 | 1.143324              | 2.352783                                                         |
| 17131 | 1.029245              | 2.352792                                                         |
| 17133 | 1.333567              | 2.352801                                                         |
| 17135 | 1.260578              | 2.352810                                                         |
| 17137 | 1.000058              | 2.352819                                                         |
| 17139 | 1.386312              | 2.352828                                                         |
| 17141 | 1.020011              | 2.352837                                                         |
| 17143 | 1.194657              | 2.352846                                                         |
| 17145 | 1.791776              | 2.352855                                                         |
| 17147 | 1.077740              | 2.352864                                                         |
| 17149 | 1.091609              | 2.352873                                                         |
| 17151 | 1.333567              | 2.352882                                                         |
| 17153 | 1.059873              | 2.352890                                                         |
| 17155 | 1.242320              | 2.352899                                                         |
| 17157 | 1.641313              | 2.352908                                                         |
| 17159 | 1.000058              | 2.352917                                                         |
| 17161 | 1.007692              | 2.352926                                                         |
| 17163 | 1.445202              | 2.352935                                                         |
| 17165 | 1.200350              | 2.352944                                                         |
| 17167 | 1.000058              | 2.352953                                                         |
| 17169 | 1.369911              | 2.352962                                                         |
| 17171 | 1.252344              | 2.352971                                                         |
| 17173 | 1.077738              | 2.352980                                                         |

| $n$   | $\frac{\sigma(n)}{n}$ | $\frac{e^\gamma}{2} \log \log n + \frac{0.73...}{\log \log n}$ |
|-------|-----------------------|----------------------------------------------------------------|
| 17175 | 1.660553              | 2.352989                                                       |
| 17177 | 1.016476              | 2.352998                                                       |
| 17179 | 1.026835              | 2.353007                                                       |
| 17181 | 1.525406              | 2.353016                                                       |
| 17183 | 1.000058              | 2.353024                                                       |
| 17185 | 1.374222              | 2.353033                                                       |
| 17187 | 1.415954              | 2.353042                                                       |
| 17189 | 1.000058              | 2.353051                                                       |
| 17191 | 1.000058              | 2.353060                                                       |
| 17193 | 1.457337              | 2.353069                                                       |
| 17195 | 1.270137              | 2.353078                                                       |
| 17197 | 1.036227              | 2.353087                                                       |
| 17199 | 1.855922              | 2.353096                                                       |
| 17201 | 1.015755              | 2.353105                                                       |
| 17203 | 1.000058              | 2.353114                                                       |
| 17205 | 1.696251              | 2.353123                                                       |
| 17207 | 1.000058              | 2.353132                                                       |
| 17209 | 1.000058              | 2.353140                                                       |
| 17211 | 1.333566              | 2.353149                                                       |
| 17213 | 1.143322              | 2.353158                                                       |
| 17215 | 1.313273              | 2.353167                                                       |
| 17217 | 1.445200              | 2.353176                                                       |
| 17219 | 1.018874              | 2.353185                                                       |
| 17221 | 1.059869              | 2.353194                                                       |
| 17223 | 1.333566              | 2.353203                                                       |
| 17225 | 1.360581              | 2.353212                                                       |
| 17227 | 1.203692              | 2.353221                                                       |
| 17229 | 1.333566              | 2.353229                                                       |
| 17231 | 1.000058              | 2.353238                                                       |
| 17233 | 1.053792              | 2.353247                                                       |
| 17235 | 1.737859              | 2.353256                                                       |
| 17237 | 1.091605              | 2.353265                                                       |
| 17239 | 1.000058              | 2.353274                                                       |
| 17241 | 1.525666              | 2.353283                                                       |
| 17243 | 1.025808              | 2.353292                                                       |
| 17245 | 1.200348              | 2.353301                                                       |
| 17247 | 1.333565              | 2.353310                                                       |
| 17249 | 1.024059              | 2.353318                                                       |
| 17251 | 1.077735              | 2.353327                                                       |
| 17253 | 1.519040              | 2.353336                                                       |
| 17255 | 1.502173              | 2.353345                                                       |
| 17257 | 1.000058              | 2.353354                                                       |
| 17259 | 1.457327              | 2.353363                                                       |
| 17261 | 1.026823              | 2.353372                                                       |

| $n$   | $\frac{\sigma(n)}{n}$ | $\frac{e^\gamma}{2} \log \log n + \frac{0.73\dots}{\log \log n}$ |
|-------|-----------------------|------------------------------------------------------------------|
| 17263 | 1.019985              | 2.353381                                                         |
| 17265 | 1.601390              | 2.353390                                                         |
| 17267 | 1.034111              | 2.353398                                                         |
| 17269 | 1.143320              | 2.353407                                                         |
| 17271 | 1.535522              | 2.353416                                                         |
| 17273 | 1.044868              | 2.353425                                                         |
| 17275 | 1.241795              | 2.353434                                                         |
| 17277 | 1.439139              | 2.353443                                                         |
| 17279 | 1.029226              | 2.353452                                                         |
| 17281 | 1.091603              | 2.353461                                                         |
| 17283 | 1.525661              | 2.353469                                                         |
| 17285 | 1.200347              | 2.353478                                                         |
| 17287 | 1.020420              | 2.353487                                                         |
| 17289 | 1.542946              | 2.353496                                                         |
| 17291 | 1.000058              | 2.353505                                                         |
| 17293 | 1.000058              | 2.353514                                                         |
| 17295 | 1.601388              | 2.353523                                                         |
| 17297 | 1.166561              | 2.353531                                                         |
| 17299 | 1.000058              | 2.353540                                                         |
| 17301 | 1.368707              | 2.353549                                                         |
| 17303 | 1.184534              | 2.353558                                                         |
| 17305 | 1.200347              | 2.353567                                                         |
| 17307 | 1.483793              | 2.353576                                                         |
| 17309 | 1.053787              | 2.353585                                                         |
| 17311 | 1.143319              | 2.353593                                                         |
| 17313 | 1.386242              | 2.353602                                                         |
| 17315 | 1.200347              | 2.353611                                                         |
| 17317 | 1.000058              | 2.353620                                                         |
| 17319 | 1.396847              | 2.353629                                                         |
| 17321 | 1.000058              | 2.353638                                                         |
| 17323 | 1.059863              | 2.353647                                                         |
| 17325 | 2.233074              | 2.353655                                                         |
| 17327 | 1.000058              | 2.353664                                                         |
| 17329 | 1.137515              | 2.353673                                                         |
| 17331 | 1.370954              | 2.353682                                                         |
| 17333 | 1.000058              | 2.353691                                                         |
| 17335 | 1.200346              | 2.353700                                                         |
| 17337 | 1.333564              | 2.353708                                                         |
| 17339 | 1.143319              | 2.353717                                                         |
| 17341 | 1.000058              | 2.353726                                                         |
| 17343 | 1.511157              | 2.353735                                                         |
| 17345 | 1.200346              | 2.353744                                                         |
| 17347 | 1.162161              | 2.353753                                                         |
| 17349 | 1.333564              | 2.353762                                                         |

| $n$   | $\frac{\sigma(n)}{n}$ | $\frac{e^\gamma}{2} \log \log n + \frac{0.73\dots}{\log \log n}$ |
|-------|-----------------------|------------------------------------------------------------------|
| 17351 | 1.000058              | 2.353770                                                         |
| 17353 | 1.191264              | 2.353779                                                         |
| 17355 | 1.742437              | 2.353788                                                         |
| 17357 | 1.059861              | 2.353797                                                         |
| 17359 | 1.000058              | 2.353806                                                         |
| 17361 | 1.483785              | 2.353815                                                         |
| 17363 | 1.015953              | 2.353823                                                         |
| 17365 | 1.260466              | 2.353832                                                         |
| 17367 | 1.525652              | 2.353841                                                         |
| 17369 | 1.091600              | 2.353850                                                         |
| 17371 | 1.036210              | 2.353859                                                         |
| 17373 | 1.333564              | 2.353867                                                         |
| 17375 | 1.256978              | 2.353876                                                         |
| 17377 | 1.000058              | 2.353885                                                         |
| 17379 | 1.445192              | 2.353894                                                         |
| 17381 | 1.237213              | 2.353903                                                         |
| 17383 | 1.000058              | 2.353912                                                         |
| 17385 | 1.711821              | 2.353920                                                         |
| 17387 | 1.000058              | 2.353929                                                         |
| 17389 | 1.000058              | 2.353938                                                         |
| 17391 | 1.589788              | 2.353947                                                         |
| 17393 | 1.000057              | 2.353956                                                         |
| 17395 | 1.415579              | 2.353964                                                         |
| 17397 | 1.445192              | 2.353973                                                         |
| 17399 | 1.015231              | 2.353982                                                         |
| 17401 | 1.000057              | 2.353991                                                         |
| 17403 | 1.333563              | 2.354000                                                         |
| 17405 | 1.220684              | 2.354008                                                         |
| 17407 | 1.093353              | 2.354017                                                         |
| 17409 | 1.525648              | 2.354026                                                         |
| 17411 | 1.044857              | 2.354035                                                         |
| 17413 | 1.091598              | 2.354044                                                         |
| 17415 | 1.834281              | 2.354052                                                         |
| 17417 | 1.000057              | 2.354061                                                         |
| 17419 | 1.000057              | 2.354070                                                         |
| 17421 | 1.333563              | 2.354079                                                         |
| 17423 | 1.212191              | 2.354088                                                         |
| 17425 | 1.344964              | 2.354096                                                         |
| 17427 | 1.378091              | 2.354105                                                         |
| 17429 | 1.036204              | 2.354114                                                         |
| 17431 | 1.000057              | 2.354123                                                         |
| 17433 | 1.565996              | 2.354132                                                         |
| 17435 | 1.313221              | 2.354140                                                         |
| 17437 | 1.189195              | 2.354149                                                         |

| $n$   | $\frac{\sigma(n)}{n}$ | $\frac{e^\gamma}{2} \log \log n + \frac{0.73\dots}{\log \log n}$ |
|-------|-----------------------|------------------------------------------------------------------|
| 17439 | 1.333563              | 2.354158                                                         |
| 17441 | 1.015538              | 2.354167                                                         |
| 17443 | 1.000057              | 2.354175                                                         |
| 17445 | 1.601376              | 2.354184                                                         |
| 17447 | 1.017940              | 2.354193                                                         |
| 17449 | 1.000057              | 2.354202                                                         |
| 17451 | 1.656753              | 2.354211                                                         |
| 17453 | 1.034092              | 2.354219                                                         |
| 17455 | 1.200344              | 2.354228                                                         |
| 17457 | 1.520536              | 2.354237                                                         |
| 17459 | 1.154705              | 2.354246                                                         |
| 17461 | 1.053777              | 2.354254                                                         |
| 17463 | 1.333562              | 2.354263                                                         |
| 17465 | 1.374177              | 2.354272                                                         |
| 17467 | 1.000057              | 2.354281                                                         |
| 17469 | 1.483771              | 2.354290                                                         |
| 17471 | 1.000057              | 2.354298                                                         |
| 17473 | 1.015739              | 2.354307                                                         |
| 17475 | 1.660429              | 2.354316                                                         |
| 17477 | 1.000057              | 2.354325                                                         |
| 17479 | 1.252246              | 2.354333                                                         |
| 17481 | 1.333562              | 2.354342                                                         |
| 17483 | 1.000057              | 2.354351                                                         |
| 17485 | 1.297112              | 2.354360                                                         |
| 17487 | 1.516555              | 2.354368                                                         |
| 17489 | 1.000057              | 2.354377                                                         |
| 17491 | 1.000057              | 2.354386                                                         |
| 17493 | 1.646373              | 2.354395                                                         |
| 17495 | 1.200343              | 2.354403                                                         |
| 17497 | 1.000057              | 2.354412                                                         |
| 17499 | 1.408080              | 2.354421                                                         |
| 17501 | 1.146449              | 2.354430                                                         |
| 17503 | 1.044849              | 2.354438                                                         |
| 17505 | 1.737789              | 2.354447                                                         |
| 17507 | 1.189924              | 2.354456                                                         |
| 17509 | 1.000057              | 2.354465                                                         |
| 17511 | 1.439095              | 2.354473                                                         |
| 17513 | 1.016845              | 2.354482                                                         |
| 17515 | 1.249672              | 2.354491                                                         |
| 17517 | 1.333562              | 2.354500                                                         |
| 17519 | 1.000057              | 2.354508                                                         |
| 17521 | 1.143314              | 2.354517                                                         |
| 17523 | 1.643554              | 2.354526                                                         |
| 17525 | 1.241769              | 2.354535                                                         |

| $n$   | $\frac{\sigma(n)}{n}$ | $\frac{e^\gamma}{2} \log \log n + \frac{0.73\dots}{\log \log n}$ |
|-------|-----------------------|------------------------------------------------------------------|
| 17527 | 1.059851              | 2.354543                                                         |
| 17529 | 1.333562              | 2.354552                                                         |
| 17531 | 1.024015              | 2.354561                                                         |
| 17533 | 1.016369              | 2.354570                                                         |
| 17535 | 1.839521              | 2.354578                                                         |
| 17537 | 1.149569              | 2.354587                                                         |
| 17539 | 1.000057              | 2.354596                                                         |
| 17541 | 1.445186              | 2.354605                                                         |
| 17543 | 1.021946              | 2.354613                                                         |
| 17545 | 1.364491              | 2.354622                                                         |
| 17547 | 1.333561              | 2.354631                                                         |
| 17549 | 1.203487              | 2.354639                                                         |
| 17551 | 1.000057              | 2.354648                                                         |
| 17553 | 1.333561              | 2.354657                                                         |
| 17555 | 1.200342              | 2.354666                                                         |
| 17557 | 1.015891              | 2.354674                                                         |
| 17559 | 1.445185              | 2.354683                                                         |
| 17561 | 1.059849              | 2.354692                                                         |
| 17563 | 1.237146              | 2.354700                                                         |
| 17565 | 1.601366              | 2.354709                                                         |
| 17567 | 1.091592              | 2.354718                                                         |
| 17569 | 1.000057              | 2.354727                                                         |
| 17571 | 1.333561              | 2.354735                                                         |
| 17573 | 1.000057              | 2.354744                                                         |
| 17575 | 1.340541              | 2.354753                                                         |
| 17577 | 1.762303              | 2.354761                                                         |
| 17579 | 1.000057              | 2.354770                                                         |
| 17581 | 1.000057              | 2.354779                                                         |
| 17583 | 1.333561              | 2.354788                                                         |
| 17585 | 1.200341              | 2.354796                                                         |
| 17587 | 1.025758              | 2.354805                                                         |
| 17589 | 1.604639              | 2.354814                                                         |
| 17591 | 1.166506              | 2.354822                                                         |
| 17593 | 1.017905              | 2.354831                                                         |
| 17595 | 1.915090              | 2.354840                                                         |
| 17597 | 1.000057              | 2.354849                                                         |
| 17599 | 1.000057              | 2.354857                                                         |
| 17601 | 1.333561              | 2.354866                                                         |
| 17603 | 1.036187              | 2.354875                                                         |
| 17605 | 1.374155              | 2.354883                                                         |
| 17607 | 1.333561              | 2.354892                                                         |
| 17609 | 1.000057              | 2.354901                                                         |
| 17611 | 1.091590              | 2.354909                                                         |
| 17613 | 1.535230              | 2.354918                                                         |

| $n$   | $\frac{\sigma(n)}{n}$ | $\frac{e^\gamma}{2} \log \log n + \frac{0.73...}{\log \log n}$ |
|-------|-----------------------|----------------------------------------------------------------|
| 17615 | 1.297076              | 2.354927                                                       |
| 17617 | 1.017199              | 2.354935                                                       |
| 17619 | 1.525626              | 2.354944                                                       |
| 17621 | 1.018784              | 2.354953                                                       |
| 17623 | 1.000057              | 2.354962                                                       |
| 17625 | 1.699404              | 2.354970                                                       |
| 17627 | 1.000057              | 2.354979                                                       |
| 17629 | 1.079698              | 2.354988                                                       |
| 17631 | 1.483750              | 2.354996                                                       |
| 17633 | 1.252198              | 2.355005                                                       |
| 17635 | 1.200340              | 2.355014                                                       |
| 17637 | 1.333560              | 2.355022                                                       |
| 17639 | 1.034072              | 2.355031                                                       |
| 17641 | 1.142792              | 2.355040                                                       |
| 17643 | 1.333560              | 2.355048                                                       |
| 17645 | 1.200340              | 2.355057                                                       |
| 17647 | 1.143310              | 2.355066                                                       |
| 17649 | 1.511474              | 2.355074                                                       |
| 17651 | 1.053765              | 2.355083                                                       |
| 17653 | 1.015125              | 2.355092                                                       |
| 17655 | 1.761767              | 2.355100                                                       |
| 17657 | 1.000057              | 2.355109                                                       |
| 17659 | 1.000057              | 2.355118                                                       |
| 17661 | 1.578167              | 2.355126                                                       |
| 17663 | 1.059843              | 2.355135                                                       |
| 17665 | 1.200340              | 2.355144                                                       |
| 17667 | 1.565857              | 2.355152                                                       |
| 17669 | 1.000057              | 2.355161                                                       |
| 17671 | 1.026767              | 2.355170                                                       |
| 17673 | 1.374300              | 2.355178                                                       |
| 17675 | 1.431174              | 2.355187                                                       |
| 17677 | 1.091588              | 2.355196                                                       |
| 17679 | 1.368403              | 2.355204                                                       |
| 17681 | 1.000057              | 2.355213                                                       |
| 17683 | 1.000057              | 2.355222                                                       |
| 17685 | 1.791349              | 2.355230                                                       |
| 17687 | 1.044835              | 2.355239                                                       |
| 17689 | 1.227712              | 2.355248                                                       |
| 17691 | 1.333559              | 2.355256                                                       |
| 17693 | 1.077714              | 2.355265                                                       |
| 17695 | 1.200339              | 2.355273                                                       |
| 17697 | 1.415833              | 2.355282                                                       |
| 17699 | 1.091587              | 2.355291                                                       |
| 17701 | 1.034066              | 2.355299                                                       |

| $n$   | $\frac{\sigma(n)}{n}$ | $\frac{e^\gamma}{2} \log \log n + \frac{0.73...}{\log \log n}$ |
|-------|-----------------------|----------------------------------------------------------------|
| 17703 | 1.656668              | 2.355308                                                       |
| 17705 | 1.200339              | 2.355317                                                       |
| 17707 | 1.000056              | 2.355325                                                       |
| 17709 | 1.333559              | 2.355334                                                       |
| 17711 | 1.016318              | 2.355343                                                       |
| 17713 | 1.000056              | 2.355351                                                       |
| 17715 | 1.601355              | 2.355360                                                       |
| 17717 | 1.143309              | 2.355369                                                       |
| 17719 | 1.137762              | 2.355377                                                       |
| 17721 | 1.584561              | 2.355386                                                       |
| 17723 | 1.029171              | 2.355394                                                       |
| 17725 | 1.241749              | 2.355403                                                       |
| 17727 | 1.408022              | 2.355412                                                       |
| 17729 | 1.000056              | 2.355420                                                       |
| 17731 | 1.218205              | 2.355429                                                       |
| 17733 | 1.396718              | 2.355438                                                       |
| 17735 | 1.200338              | 2.355446                                                       |
| 17737 | 1.000056              | 2.355455                                                       |
| 17739 | 1.518462              | 2.355463                                                       |
| 17741 | 1.015275              | 2.355472                                                       |
| 17743 | 1.091585              | 2.355481                                                       |
| 17745 | 1.980051              | 2.355489                                                       |
| 17747 | 1.000056              | 2.355498                                                       |
| 17749 | 1.000056              | 2.355507                                                       |
| 17751 | 1.369162              | 2.355515                                                       |
| 17753 | 1.026756              | 2.355524                                                       |
| 17755 | 1.240890              | 2.355532                                                       |
| 17757 | 1.445177              | 2.355541                                                       |
| 17759 | 1.189256              | 2.355550                                                       |
| 17761 | 1.000056              | 2.355558                                                       |
| 17763 | 1.383550              | 2.355567                                                       |
| 17765 | 1.459049              | 2.355575                                                       |
| 17767 | 1.015366              | 2.355584                                                       |
| 17769 | 1.333558              | 2.355593                                                       |
| 17771 | 1.077711              | 2.355601                                                       |
| 17773 | 1.143307              | 2.355610                                                       |
| 17775 | 1.813783              | 2.355618                                                       |
| 17777 | 1.036170              | 2.355627                                                       |
| 17779 | 1.044828              | 2.355636                                                       |
| 17781 | 1.333558              | 2.355644                                                       |
| 17783 | 1.000056              | 2.355653                                                       |
| 17785 | 1.200337              | 2.355662                                                       |
| 17787 | 1.704841              | 2.355670                                                       |
| 17789 | 1.000056              | 2.355679                                                       |



| $n$   | $\frac{\sigma(n)}{n}$ | $\frac{e^\gamma}{2} \log \log n + \frac{0.73...}{\log \log n}$ |
|-------|-----------------------|----------------------------------------------------------------|
| 17791 | 1.000056              | 2.355687                                                       |
| 17793 | 1.483730              | 2.355696                                                       |
| 17795 | 1.200337              | 2.355704                                                       |
| 17797 | 1.106816              | 2.355713                                                       |
| 17799 | 1.415810              | 2.355722                                                       |
| 17801 | 1.143307              | 2.355730                                                       |
| 17803 | 1.053755              | 2.355739                                                       |
| 17805 | 1.601348              | 2.355747                                                       |
| 17807 | 1.000056              | 2.355756                                                       |
| 17809 | 1.091583              | 2.355765                                                       |
| 17811 | 1.445174              | 2.355773                                                       |
| 17813 | 1.023971              | 2.355782                                                       |
| 17815 | 1.374123              | 2.355790                                                       |
| 17817 | 1.333558              | 2.355799                                                       |
| 17819 | 1.015545              | 2.355808                                                       |
| 17821 | 1.018125              | 2.355816                                                       |
| 17823 | 1.439039              | 2.355825                                                       |
| 17825 | 1.335652              | 2.355833                                                       |
| 17827 | 1.000056              | 2.355842                                                       |
| 17829 | 1.656627              | 2.355850                                                       |
| 17831 | 1.091582              | 2.355859                                                       |
| 17833 | 1.059833              | 2.355868                                                       |
| 17835 | 1.695542              | 2.355876                                                       |
| 17837 | 1.000056              | 2.355885                                                       |
| 17839 | 1.000056              | 2.355893                                                       |
| 17841 | 1.407993              | 2.355902                                                       |
| 17843 | 1.143305              | 2.355910                                                       |
| 17845 | 1.242701              | 2.355919                                                       |
| 17847 | 1.483723              | 2.355928                                                       |
| 17849 | 1.077707              | 2.355936                                                       |
| 17851 | 1.000056              | 2.355945                                                       |
| 17853 | 1.457234              | 2.355953                                                       |
| 17855 | 1.200336              | 2.355962                                                       |
| 17857 | 1.143305              | 2.355970                                                       |
| 17859 | 1.333557              | 2.355979                                                       |
| 17861 | 1.021891              | 2.355988                                                       |
| 17863 | 1.000056              | 2.355996                                                       |
| 17865 | 1.737699              | 2.356005                                                       |
| 17867 | 1.059831              | 2.356013                                                       |
| 17869 | 1.015390              | 2.356022                                                       |
| 17871 | 1.633037              | 2.356030                                                       |
| 17873 | 1.019862              | 2.356039                                                       |
| 17875 | 1.466182              | 2.356047                                                       |
| 17877 | 1.369357              | 2.356056                                                       |

| $n$   | $\frac{\sigma(n)}{n}$ | $\frac{e^\gamma}{2} \log \log n + \frac{0.73\dots}{\log \log n}$ |
|-------|-----------------------|------------------------------------------------------------------|
| 17879 | 1.053750              | 2.356065                                                         |
| 17881 | 1.000056              | 2.356073                                                         |
| 17883 | 1.445171              | 2.356082                                                         |
| 17885 | 1.415041              | 2.356090                                                         |
| 17887 | 1.034047              | 2.356099                                                         |
| 17889 | 1.368439              | 2.356107                                                         |
| 17891 | 1.000056              | 2.356116                                                         |
| 17893 | 1.036159              | 2.356124                                                         |
| 17895 | 1.601341              | 2.356133                                                         |
| 17897 | 1.091580              | 2.356141                                                         |
| 17899 | 1.143304              | 2.356150                                                         |
| 17901 | 1.703369              | 2.356158                                                         |
| 17903 | 1.000056              | 2.356167                                                         |
| 17905 | 1.200335              | 2.356176                                                         |
| 17907 | 1.372424              | 2.356184                                                         |
| 17909 | 1.000056              | 2.356193                                                         |
| 17911 | 1.000056              | 2.356201                                                         |
| 17913 | 1.525596              | 2.356210                                                         |
| 17915 | 1.200335              | 2.356218                                                         |
| 17917 | 1.125188              | 2.356227                                                         |
| 17919 | 1.584463              | 2.356235                                                         |
| 17921 | 1.000056              | 2.356244                                                         |
| 17923 | 1.000056              | 2.356252                                                         |
| 17925 | 1.660251              | 2.356261                                                         |
| 17927 | 1.237017              | 2.356269                                                         |
| 17929 | 1.000056              | 2.356278                                                         |
| 17931 | 1.374156              | 2.356286                                                         |
| 17933 | 1.017119              | 2.356295                                                         |
| 17935 | 1.276610              | 2.356304                                                         |
| 17937 | 1.445169              | 2.356312                                                         |
| 17939 | 1.000056              | 2.356321                                                         |
| 17941 | 1.252104              | 2.356329                                                         |
| 17943 | 1.333556              | 2.356338                                                         |
| 17945 | 1.245138              | 2.356346                                                         |
| 17947 | 1.014989              | 2.356355                                                         |
| 17949 | 1.383475              | 2.356363                                                         |
| 17951 | 1.036154              | 2.356372                                                         |
| 17953 | 1.077703              | 2.356380                                                         |
| 17955 | 2.138680              | 2.356389                                                         |
| 17957 | 1.000056              | 2.356397                                                         |
| 17959 | 1.000056              | 2.356406                                                         |
| 17961 | 1.333556              | 2.356414                                                         |
| 17963 | 1.154373              | 2.356423                                                         |
| 17965 | 1.200334              | 2.356431                                                         |

| $n$   | $\frac{\sigma(n)}{n}$ | $\frac{e^\gamma}{2} \log \log n + \frac{0.73...}{\log \log n}$ |
|-------|-----------------------|----------------------------------------------------------------|
| 17967 | 1.370513              | 2.356440                                                       |
| 17969 | 1.218098              | 2.356448                                                       |
| 17971 | 1.000056              | 2.356457                                                       |
| 17973 | 1.445168              | 2.356465                                                       |
| 17975 | 1.241725              | 2.356474                                                       |
| 17977 | 1.000056              | 2.356482                                                       |
| 17979 | 1.439012              | 2.356491                                                       |
| 17981 | 1.000056              | 2.356499                                                       |
| 17983 | 1.166435              | 2.356508                                                       |
| 17985 | 1.761468              | 2.356516                                                       |
| 17987 | 1.000056              | 2.356525                                                       |
| 17989 | 1.000056              | 2.356533                                                       |
| 17991 | 1.445167              | 2.356542                                                       |
| 17993 | 1.053743              | 2.356550                                                       |
| 17995 | 1.240345              | 2.356559                                                       |
| 17997 | 1.525588              | 2.356567                                                       |
| 17999 | 1.026724              | 2.356576                                                       |
| 18001 | 1.023943              | 2.356584                                                       |
| 18003 | 1.415764              | 2.356593                                                       |
| 18005 | 1.296973              | 2.356601                                                       |
| 18007 | 1.091575              | 2.356610                                                       |
| 18009 | 1.599200              | 2.356618                                                       |
| 18011 | 1.193937              | 2.356627                                                       |
| 18013 | 1.000056              | 2.356635                                                       |
| 18015 | 1.601332              | 2.356644                                                       |
| 18017 | 1.025698              | 2.356652                                                       |
| 18019 | 1.029136              | 2.356660                                                       |
| 18021 | 1.333555              | 2.356669                                                       |
| 18023 | 1.018698              | 2.356677                                                       |
| 18025 | 1.430902              | 2.356686                                                       |
| 18027 | 1.445166              | 2.356694                                                       |
| 18029 | 1.106551              | 2.356703                                                       |
| 18031 | 1.149132              | 2.356711                                                       |
| 18033 | 1.333555              | 2.356720                                                       |
| 18035 | 1.200333              | 2.356728                                                       |
| 18037 | 1.059821              | 2.356737                                                       |
| 18039 | 1.525583              | 2.356745                                                       |
| 18041 | 1.000055              | 2.356754                                                       |
| 18043 | 1.000055              | 2.356762                                                       |
| 18045 | 1.737656              | 2.356771                                                       |
| 18047 | 1.000055              | 2.356779                                                       |
| 18049 | 1.000055              | 2.356788                                                       |
| 18051 | 1.457205              | 2.356796                                                       |
| 18053 | 1.143300              | 2.356804                                                       |

| $n$   | $\frac{\sigma(n)}{n}$ | $\frac{e^\gamma}{2} \log \log n + \frac{0.73\dots}{\log \log n}$ |
|-------|-----------------------|------------------------------------------------------------------|
| 18055 | 1.260150              | 2.356813                                                         |
| 18057 | 1.438999              | 2.356821                                                         |
| 18059 | 1.000055              | 2.356830                                                         |
| 18061 | 1.000055              | 2.356838                                                         |
| 18063 | 1.500526              | 2.356847                                                         |
| 18065 | 1.200332              | 2.356855                                                         |
| 18067 | 1.195550              | 2.356864                                                         |
| 18069 | 1.407936              | 2.356872                                                         |
| 18071 | 1.059820              | 2.356881                                                         |
| 18073 | 1.147347              | 2.356889                                                         |
| 18075 | 1.660194              | 2.356897                                                         |
| 18077 | 1.000055              | 2.356906                                                         |
| 18079 | 1.015543              | 2.356914                                                         |
| 18081 | 1.721254              | 2.356923                                                         |
| 18083 | 1.092960              | 2.356931                                                         |
| 18085 | 1.200332              | 2.356940                                                         |
| 18087 | 1.333554              | 2.356948                                                         |
| 18089 | 1.000055              | 2.356957                                                         |
| 18091 | 1.017080              | 2.356965                                                         |
| 18093 | 1.377770              | 2.356973                                                         |
| 18095 | 1.527936              | 2.356982                                                         |
| 18097 | 1.000055              | 2.356990                                                         |
| 18099 | 1.445163              | 2.356999                                                         |
| 18101 | 1.044804              | 2.357007                                                         |
| 18103 | 1.025686              | 2.357016                                                         |
| 18105 | 1.717978              | 2.357024                                                         |
| 18107 | 1.053736              | 2.357033                                                         |
| 18109 | 1.236954              | 2.357041                                                         |
| 18111 | 1.333554              | 2.357049                                                         |
| 18113 | 1.020262              | 2.357058                                                         |
| 18115 | 1.200331              | 2.357066                                                         |
| 18117 | 1.642656              | 2.357075                                                         |
| 18119 | 1.000055              | 2.357083                                                         |
| 18121 | 1.000055              | 2.357092                                                         |
| 18123 | 1.525575              | 2.357100                                                         |
| 18125 | 1.292690              | 2.357108                                                         |
| 18127 | 1.000055              | 2.357117                                                         |
| 18129 | 1.333554              | 2.357125                                                         |
| 18131 | 1.000055              | 2.357134                                                         |
| 18133 | 1.000055              | 2.357142                                                         |
| 18135 | 1.926882              | 2.357151                                                         |
| 18137 | 1.143298              | 2.357159                                                         |
| 18139 | 1.166988              | 2.357167                                                         |
| 18141 | 1.333554              | 2.357176                                                         |

| $n$   | $\frac{\sigma(n)}{n}$ | $\frac{e^\gamma}{2} \log \log n + \frac{0.73...}{\log \log n}$ |
|-------|-----------------------|----------------------------------------------------------------|
| 18143 | 1.000055              | 2.357184                                                       |
| 18145 | 1.269771              | 2.357193                                                       |
| 18147 | 1.396594              | 2.357201                                                       |
| 18149 | 1.000055              | 2.357209                                                       |
| 18151 | 1.143298              | 2.357218                                                       |
| 18153 | 1.445161              | 2.357226                                                       |
| 18155 | 1.200330              | 2.357235                                                       |
| 18157 | 1.018670              | 2.357243                                                       |
| 18159 | 1.333554              | 2.357251                                                       |
| 18161 | 1.184076              | 2.357260                                                       |
| 18163 | 1.026703              | 2.357268                                                       |
| 18165 | 1.839141              | 2.357277                                                       |
| 18167 | 1.029119              | 2.357285                                                       |
| 18169 | 1.000055              | 2.357293                                                       |
| 18171 | 1.483683              | 2.357302                                                       |
| 18173 | 1.059814              | 2.357310                                                       |
| 18175 | 1.241706              | 2.357319                                                       |
| 18177 | 1.367882              | 2.357327                                                       |
| 18179 | 1.188184              | 2.357335                                                       |
| 18181 | 1.000055              | 2.357344                                                       |
| 18183 | 1.583897              | 2.357352                                                       |
| 18185 | 1.200330              | 2.357361                                                       |
| 18187 | 1.077693              | 2.357369                                                       |
| 18189 | 1.509484              | 2.357377                                                       |
| 18191 | 1.000055              | 2.357386                                                       |
| 18193 | 1.203100              | 2.357394                                                       |
| 18195 | 1.601319              | 2.357403                                                       |
| 18197 | 1.034017              | 2.357411                                                       |
| 18199 | 1.000055              | 2.357419                                                       |
| 18201 | 1.333553              | 2.357428                                                       |
| 18203 | 1.015217              | 2.357436                                                       |
| 18205 | 1.313046              | 2.357445                                                       |
| 18207 | 1.753611              | 2.357453                                                       |
| 18209 | 1.014883              | 2.357461                                                       |
| 18211 | 1.000055              | 2.357470                                                       |
| 18213 | 1.438972              | 2.357478                                                       |
| 18215 | 1.200329              | 2.357486                                                       |
| 18217 | 1.000055              | 2.357495                                                       |
| 18219 | 1.333553              | 2.357503                                                       |
| 18221 | 1.211789              | 2.357512                                                       |
| 18223 | 1.000055              | 2.357520                                                       |
| 18225 | 1.859150              | 2.357528                                                       |
| 18227 | 1.091567              | 2.357537                                                       |
| 18229 | 1.000055              | 2.357545                                                       |

| $n$   | $\frac{\sigma(n)}{n}$ | $\frac{e^\gamma}{2} \log \log n + \frac{0.73...}{\log \log n}$ |
|-------|-----------------------|----------------------------------------------------------------|
| 18231 | 1.369097              | 2.357553                                                       |
| 18233 | 1.000055              | 2.357562                                                       |
| 18235 | 1.374061              | 2.357570                                                       |
| 18237 | 1.333553              | 2.357579                                                       |
| 18239 | 1.142168              | 2.357587                                                       |
| 18241 | 1.124938              | 2.357595                                                       |
| 18243 | 1.445157              | 2.357604                                                       |
| 18245 | 1.243080              | 2.357612                                                       |
| 18247 | 1.018030              | 2.357620                                                       |
| 18249 | 1.683380              | 2.357629                                                       |
| 18251 | 1.000055              | 2.357637                                                       |
| 18253 | 1.000055              | 2.357645                                                       |
| 18255 | 1.601315              | 2.357654                                                       |
| 18257 | 1.000055              | 2.357662                                                       |
| 18259 | 1.087683              | 2.357671                                                       |
| 18261 | 1.445156              | 2.357679                                                       |
| 18263 | 1.143295              | 2.357687                                                       |
| 18265 | 1.296907              | 2.357696                                                       |
| 18267 | 1.333552              | 2.357704                                                       |
| 18269 | 1.000055              | 2.357712                                                       |
| 18271 | 1.106453              | 2.357721                                                       |
| 18273 | 1.333552              | 2.357729                                                       |
| 18275 | 1.343475              | 2.357737                                                       |
| 18277 | 1.166384              | 2.357746                                                       |
| 18279 | 1.483670              | 2.357754                                                       |
| 18281 | 1.015481              | 2.357762                                                       |
| 18283 | 1.023902              | 2.357771                                                       |
| 18285 | 1.701066              | 2.357779                                                       |
| 18287 | 1.000055              | 2.357787                                                       |
| 18289 | 1.000055              | 2.357796                                                       |
| 18291 | 1.665519              | 2.357804                                                       |
| 18293 | 1.091565              | 2.357812                                                       |
| 18295 | 1.200328              | 2.357821                                                       |
| 18297 | 1.534678              | 2.357829                                                       |
| 18299 | 1.036122              | 2.357838                                                       |
| 18301 | 1.000055              | 2.357846                                                       |
| 18303 | 1.333552              | 2.357854                                                       |
| 18305 | 1.374051              | 2.357863                                                       |
| 18307 | 1.000055              | 2.357871                                                       |
| 18309 | 1.415697              | 2.357879                                                       |
| 18311 | 1.000055              | 2.357888                                                       |
| 18313 | 1.000055              | 2.357896                                                       |
| 18315 | 1.942015              | 2.357904                                                       |
| 18317 | 1.077687              | 2.357913                                                       |

| $n$   | $\frac{\sigma(n)}{n}$ | $\frac{e^\gamma}{2} \log \log n + \frac{0.73...}{\log \log n}$ |
|-------|-----------------------|----------------------------------------------------------------|
| 18319 | 1.143294              | 2.357921                                                       |
| 18321 | 1.383331              | 2.357929                                                       |
| 18323 | 1.017737              | 2.357937                                                       |
| 18325 | 1.241692              | 2.357946                                                       |
| 18327 | 1.375020              | 2.357954                                                       |
| 18329 | 1.000055              | 2.357962                                                       |
| 18331 | 1.044788              | 2.357971                                                       |
| 18333 | 1.710577              | 2.357979                                                       |
| 18335 | 1.269703              | 2.357987                                                       |
| 18337 | 1.091564              | 2.357996                                                       |
| 18339 | 1.333551              | 2.358004                                                       |
| 18341 | 1.000055              | 2.358012                                                       |
| 18343 | 1.154010              | 2.358021                                                       |
| 18345 | 1.601308              | 2.358029                                                       |
| 18347 | 1.143293              | 2.358037                                                       |
| 18349 | 1.020219              | 2.358046                                                       |
| 18351 | 1.445153              | 2.358054                                                       |
| 18353 | 1.000054              | 2.358062                                                       |
| 18355 | 1.200327              | 2.358071                                                       |
| 18357 | 1.385847              | 2.358079                                                       |
| 18359 | 1.091563              | 2.358087                                                       |
| 18361 | 1.188606              | 2.358096                                                       |
| 18363 | 1.333551              | 2.358104                                                       |
| 18365 | 1.200327              | 2.358112                                                       |
| 18367 | 1.000054              | 2.358120                                                       |
| 18369 | 1.565464              | 2.358129                                                       |
| 18371 | 1.000054              | 2.358137                                                       |
| 18373 | 1.053720              | 2.358145                                                       |
| 18375 | 1.935673              | 2.358154                                                       |
| 18377 | 1.128367              | 2.358162                                                       |
| 18379 | 1.000054              | 2.358170                                                       |
| 18381 | 1.457157              | 2.358179                                                       |
| 18383 | 1.033999              | 2.358187                                                       |
| 18385 | 1.200326              | 2.358195                                                       |
| 18387 | 1.500408              | 2.358203                                                       |
| 18389 | 1.190277              | 2.358212                                                       |
| 18391 | 1.021804              | 2.358220                                                       |
| 18393 | 1.333551              | 2.358228                                                       |
| 18395 | 1.296874              | 2.358237                                                       |
| 18397 | 1.000054              | 2.358245                                                       |
| 18399 | 1.333551              | 2.358253                                                       |
| 18401 | 1.000054              | 2.358261                                                       |
| 18403 | 1.251970              | 2.358270                                                       |
| 18405 | 1.737571              | 2.358278                                                       |

| $n$   | $\frac{\sigma(n)}{n}$ | $\frac{e^\gamma}{2} \log \log n + \frac{0.73...}{\log \log n}$ |
|-------|-----------------------|----------------------------------------------------------------|
| 18407 | 1.017004              | 2.358286                                                       |
| 18409 | 1.026672              | 2.358295                                                       |
| 18411 | 1.489979              | 2.358303                                                       |
| 18413 | 1.000054              | 2.358311                                                       |
| 18415 | 1.251154              | 2.358319                                                       |
| 18417 | 1.525547              | 2.358328                                                       |
| 18419 | 1.015039              | 2.358336                                                       |
| 18421 | 1.092775              | 2.358344                                                       |
| 18423 | 1.524182              | 2.358353                                                       |
| 18425 | 1.372917              | 2.358361                                                       |
| 18427 | 1.000054              | 2.358369                                                       |
| 18429 | 1.333550              | 2.358377                                                       |
| 18431 | 1.143291              | 2.358386                                                       |
| 18433 | 1.000054              | 2.358394                                                       |
| 18435 | 1.601302              | 2.358402                                                       |
| 18437 | 1.015350              | 2.358410                                                       |
| 18439 | 1.000054              | 2.358419                                                       |
| 18441 | 1.483651              | 2.358427                                                       |
| 18443 | 1.000054              | 2.358435                                                       |
| 18445 | 1.498943              | 2.358444                                                       |
| 18447 | 1.602862              | 2.358452                                                       |
| 18449 | 1.053716              | 2.358460                                                       |
| 18451 | 1.000054              | 2.358468                                                       |
| 18453 | 1.333550              | 2.358477                                                       |
| 18455 | 1.200325              | 2.358485                                                       |
| 18457 | 1.000054              | 2.358493                                                       |
| 18459 | 1.656428              | 2.358501                                                       |
| 18461 | 1.000054              | 2.358510                                                       |
| 18463 | 1.029085              | 2.358518                                                       |
| 18465 | 1.601300              | 2.358526                                                       |
| 18467 | 1.020198              | 2.358534                                                       |
| 18469 | 1.153934              | 2.358543                                                       |
| 18471 | 1.372097              | 2.358551                                                       |
| 18473 | 1.295945              | 2.358559                                                       |
| 18475 | 1.241678              | 2.358567                                                       |
| 18477 | 1.445148              | 2.358576                                                       |
| 18479 | 1.059798              | 2.358584                                                       |
| 18481 | 1.000054              | 2.358592                                                       |
| 18483 | 1.368609              | 2.358600                                                       |
| 18485 | 1.200325              | 2.358609                                                       |
| 18487 | 1.211662              | 2.358617                                                       |
| 18489 | 1.333550              | 2.358625                                                       |
| 18491 | 1.118166              | 2.358633                                                       |
| 18493 | 1.000054              | 2.358642                                                       |



| $n$   | $\frac{\sigma(n)}{n}$ | $\frac{e^\gamma}{2} \log \log n + \frac{0.73\dots}{\log \log n}$ |
|-------|-----------------------|------------------------------------------------------------------|
| 18495 | 1.790754              | 2.358650                                                         |
| 18497 | 1.021787              | 2.358658                                                         |
| 18499 | 1.077680              | 2.358666                                                         |
| 18501 | 1.525539              | 2.358675                                                         |
| 18503 | 1.000054              | 2.358683                                                         |
| 18505 | 1.200324              | 2.358691                                                         |
| 18507 | 1.383260              | 2.358699                                                         |
| 18509 | 1.016587              | 2.358708                                                         |
| 18511 | 1.015180              | 2.358716                                                         |
| 18513 | 1.681089              | 2.358724                                                         |
| 18515 | 1.433648              | 2.358732                                                         |
| 18517 | 1.000054              | 2.358740                                                         |
| 18519 | 1.333549              | 2.358749                                                         |
| 18521 | 1.000054              | 2.358757                                                         |
| 18523 | 1.000054              | 2.358765                                                         |
| 18525 | 1.874224              | 2.358773                                                         |
| 18527 | 1.015599              | 2.358782                                                         |
| 18529 | 1.143289              | 2.358790                                                         |
| 18531 | 1.515299              | 2.358798                                                         |
| 18533 | 1.025630              | 2.358806                                                         |
| 18535 | 1.312975              | 2.358815                                                         |
| 18537 | 1.377569              | 2.358823                                                         |
| 18539 | 1.000054              | 2.358831                                                         |
| 18541 | 1.000054              | 2.358839                                                         |
| 18543 | 1.525535              | 2.358847                                                         |
| 18545 | 1.200324              | 2.358856                                                         |
| 18547 | 1.059794              | 2.358864                                                         |
| 18549 | 1.500350              | 2.358872                                                         |
| 18551 | 1.077678              | 2.358880                                                         |
| 18553 | 1.000054              | 2.358888                                                         |
| 18555 | 1.601293              | 2.358897                                                         |
| 18557 | 1.251926              | 2.358905                                                         |
| 18559 | 1.018589              | 2.358913                                                         |
| 18561 | 1.396476              | 2.358921                                                         |
| 18563 | 1.053709              | 2.358930                                                         |
| 18565 | 1.241045              | 2.358938                                                         |
| 18567 | 1.445145              | 2.358946                                                         |
| 18569 | 1.033981              | 2.358954                                                         |
| 18571 | 1.166335              | 2.358962                                                         |
| 18573 | 1.374899              | 2.358971                                                         |
| 18575 | 1.241669              | 2.358979                                                         |
| 18577 | 1.077677              | 2.358987                                                         |
| 18579 | 1.457129              | 2.358995                                                         |
| 18581 | 1.059792              | 2.359003                                                         |

| $n$   | $\frac{\sigma(n)}{n}$ | $\frac{e^\gamma}{2} \log \log n + \frac{0.73\dots}{\log \log n}$ |
|-------|-----------------------|------------------------------------------------------------------|
| 18583 | 1.000054              | 2.359012                                                         |
| 18585 | 2.014528              | 2.359020                                                         |
| 18587 | 1.000054              | 2.359028                                                         |
| 18589 | 1.036097              | 2.359036                                                         |
| 18591 | 1.333548              | 2.359044                                                         |
| 18593 | 1.000054              | 2.359053                                                         |
| 18595 | 1.200323              | 2.359061                                                         |
| 18597 | 1.333548              | 2.359069                                                         |
| 18599 | 1.143287              | 2.359077                                                         |
| 18601 | 1.161228              | 2.359085                                                         |
| 18603 | 1.625544              | 2.359094                                                         |
| 18605 | 1.219995              | 2.359102                                                         |
| 18607 | 1.044768              | 2.359110                                                         |
| 18609 | 1.333548              | 2.359118                                                         |
| 18611 | 1.029069              | 2.359126                                                         |
| 18613 | 1.143287              | 2.359134                                                         |
| 18615 | 1.717325              | 2.359143                                                         |
| 18617 | 1.000054              | 2.359151                                                         |
| 18619 | 1.025619              | 2.359159                                                         |
| 18621 | 1.445143              | 2.359167                                                         |
| 18623 | 1.091553              | 2.359175                                                         |
| 18625 | 1.256376              | 2.359184                                                         |
| 18627 | 1.525527              | 2.359192                                                         |
| 18629 | 1.077675              | 2.359200                                                         |
| 18631 | 1.033976              | 2.359208                                                         |
| 18633 | 1.333548              | 2.359216                                                         |
| 18635 | 1.200322              | 2.359224                                                         |
| 18637 | 1.000054              | 2.359233                                                         |
| 18639 | 1.534417              | 2.359241                                                         |
| 18641 | 1.143286              | 2.359249                                                         |
| 18643 | 1.015287              | 2.359257                                                         |
| 18645 | 1.760901              | 2.359265                                                         |
| 18647 | 1.036092              | 2.359273                                                         |
| 18649 | 1.059789              | 2.359282                                                         |
| 18651 | 1.333548              | 2.359290                                                         |
| 18653 | 1.044765              | 2.359298                                                         |
| 18655 | 1.512946              | 2.359306                                                         |
| 18657 | 1.483625              | 2.359314                                                         |
| 18659 | 1.023849              | 2.359322                                                         |
| 18661 | 1.000054              | 2.359331                                                         |
| 18663 | 1.333548              | 2.359339                                                         |
| 18665 | 1.200321              | 2.359347                                                         |
| 18667 | 1.091552              | 2.359355                                                         |
| 18669 | 1.563233              | 2.359363                                                         |

| $n$   | $\frac{\sigma(n)}{n}$ | $\frac{e^\gamma}{2} \log \log n + \frac{0.73\dots}{\log \log n}$ |
|-------|-----------------------|------------------------------------------------------------------|
| 18671 | 1.000054              | 2.359371                                                         |
| 18673 | 1.017940              | 2.359380                                                         |
| 18675 | 1.812691              | 2.359388                                                         |
| 18677 | 1.053702              | 2.359396                                                         |
| 18679 | 1.000054              | 2.359404                                                         |
| 18681 | 1.438895              | 2.359412                                                         |
| 18683 | 1.217792              | 2.359420                                                         |
| 18685 | 1.244635              | 2.359428                                                         |
| 18687 | 1.333547              | 2.359437                                                         |
| 18689 | 1.091551              | 2.359445                                                         |
| 18691 | 1.000054              | 2.359453                                                         |
| 18693 | 1.513294              | 2.359461                                                         |
| 18695 | 1.200321              | 2.359469                                                         |
| 18697 | 1.143285              | 2.359477                                                         |
| 18699 | 1.396438              | 2.359486                                                         |
| 18701 | 1.000053              | 2.359494                                                         |
| 18703 | 1.020157              | 2.359502                                                         |
| 18705 | 1.693665              | 2.359510                                                         |
| 18707 | 1.077671              | 2.359518                                                         |
| 18709 | 1.021754              | 2.359526                                                         |
| 18711 | 1.867565              | 2.359534                                                         |
| 18713 | 1.000053              | 2.359542                                                         |
| 18715 | 1.269570              | 2.359551                                                         |
| 18717 | 1.415611              | 2.359559                                                         |
| 18719 | 1.000053              | 2.359567                                                         |
| 18721 | 1.015544              | 2.359575                                                         |
| 18723 | 1.350425              | 2.359583                                                         |
| 18725 | 1.430387              | 2.359591                                                         |
| 18727 | 1.019704              | 2.359599                                                         |
| 18729 | 1.445139              | 2.359608                                                         |
| 18731 | 1.000053              | 2.359616                                                         |
| 18733 | 1.183793              | 2.359624                                                         |
| 18735 | 1.601281              | 2.359632                                                         |
| 18737 | 1.026632              | 2.359640                                                         |
| 18739 | 1.143284              | 2.359648                                                         |
| 18741 | 1.333547              | 2.359656                                                         |
| 18743 | 1.000053              | 2.359664                                                         |
| 18745 | 1.259856              | 2.359673                                                         |
| 18747 | 1.445138              | 2.359681                                                         |
| 18749 | 1.000053              | 2.359689                                                         |
| 18751 | 1.059783              | 2.359697                                                         |
| 18753 | 1.638138              | 2.359705                                                         |
| 18755 | 1.361557              | 2.359713                                                         |
| 18757 | 1.000053              | 2.359721                                                         |

| $n$   | $\frac{\sigma(n)}{n}$ | $\frac{e^\gamma}{2} \log \log n + \frac{0.73...}{\log \log n}$ |
|-------|-----------------------|----------------------------------------------------------------|
| 18759 | 1.482808              | 2.359729                                                       |
| 18761 | 1.017643              | 2.359738                                                       |
| 18763 | 1.036082              | 2.359746                                                       |
| 18765 | 1.790568              | 2.359754                                                       |
| 18767 | 1.166303              | 2.359762                                                       |
| 18769 | 1.007353              | 2.359770                                                       |
| 18771 | 1.333546              | 2.359778                                                       |
| 18773 | 1.000053              | 2.359786                                                       |
| 18775 | 1.241651              | 2.359794                                                       |
| 18777 | 1.457102              | 2.359802                                                       |
| 18779 | 1.016029              | 2.359811                                                       |
| 18781 | 1.143283              | 2.359819                                                       |
| 18783 | 1.445137              | 2.359827                                                       |
| 18785 | 1.372797              | 2.359835                                                       |
| 18787 | 1.000053              | 2.359843                                                       |
| 18789 | 1.333546              | 2.359851                                                       |
| 18791 | 1.123942              | 2.359859                                                       |
| 18793 | 1.000053              | 2.359867                                                       |
| 18795 | 1.838787              | 2.359875                                                       |
| 18797 | 1.000053              | 2.359883                                                       |
| 18799 | 1.091547              | 2.359892                                                       |
| 18801 | 1.445136              | 2.359900                                                       |
| 18803 | 1.000053              | 2.359908                                                       |
| 18805 | 1.200319              | 2.359916                                                       |
| 18807 | 1.333546              | 2.359924                                                       |
| 18809 | 1.143282              | 2.359932                                                       |
| 18811 | 1.077667              | 2.359940                                                       |
| 18813 | 1.333546              | 2.359948                                                       |
| 18815 | 1.239862              | 2.359956                                                       |
| 18817 | 1.033959              | 2.359964                                                       |
| 18819 | 1.606887              | 2.359972                                                       |
| 18821 | 1.147654              | 2.359981                                                       |
| 18823 | 1.143282              | 2.359989                                                       |
| 18825 | 1.659920              | 2.359997                                                       |
| 18827 | 1.018537              | 2.360005                                                       |
| 18829 | 1.053694              | 2.360013                                                       |
| 18831 | 1.333546              | 2.360021                                                       |
| 18833 | 1.029045              | 2.360029                                                       |
| 18835 | 1.200319              | 2.360037                                                       |
| 18837 | 1.855072              | 2.360045                                                       |
| 18839 | 1.000053              | 2.360053                                                       |
| 18841 | 1.016507              | 2.360061                                                       |
| 18843 | 1.457093              | 2.360069                                                       |
| 18845 | 1.200318              | 2.360078                                                       |

| $n$   | $\frac{\sigma(n)}{n}$ | $\frac{e^\gamma}{2} \log \log n + \frac{0.73\dots}{\log \log n}$ |
|-------|-----------------------|------------------------------------------------------------------|
| 18847 | 1.023823              | 2.360086                                                         |
| 18849 | 1.368348              | 2.360094                                                         |
| 18851 | 1.143282              | 2.360102                                                         |
| 18853 | 1.059778              | 2.360110                                                         |
| 18855 | 1.737470              | 2.360118                                                         |
| 18857 | 1.015008              | 2.360126                                                         |
| 18859 | 1.000053              | 2.360134                                                         |
| 18861 | 1.333545              | 2.360142                                                         |
| 18863 | 1.077665              | 2.360150                                                         |
| 18865 | 1.526637              | 2.360158                                                         |
| 18867 | 1.407749              | 2.360166                                                         |
| 18869 | 1.000053              | 2.360174                                                         |
| 18871 | 1.014891              | 2.360182                                                         |
| 18873 | 1.500238              | 2.360190                                                         |
| 18875 | 1.256265              | 2.360199                                                         |
| 18877 | 1.025587              | 2.360207                                                         |
| 18879 | 1.627205              | 2.360215                                                         |
| 18881 | 1.016895              | 2.360223                                                         |
| 18883 | 1.044749              | 2.360231                                                         |
| 18885 | 1.601271              | 2.360239                                                         |
| 18887 | 1.166517              | 2.360247                                                         |
| 18889 | 1.077664              | 2.360255                                                         |
| 18891 | 1.445133              | 2.360263                                                         |
| 18893 | 1.143281              | 2.360271                                                         |
| 18895 | 1.200318              | 2.360279                                                         |
| 18897 | 1.333545              | 2.360287                                                         |
| 18899 | 1.000053              | 2.360295                                                         |
| 18901 | 1.026612              | 2.360303                                                         |
| 18903 | 1.333545              | 2.360311                                                         |
| 18905 | 1.269505              | 2.360319                                                         |
| 18907 | 1.189824              | 2.360327                                                         |
| 18909 | 1.584008              | 2.360335                                                         |
| 18911 | 1.000053              | 2.360344                                                         |
| 18913 | 1.000053              | 2.360352                                                         |
| 18915 | 1.740841              | 2.360360                                                         |
| 18917 | 1.000053              | 2.360368                                                         |
| 18919 | 1.000053              | 2.360376                                                         |
| 18921 | 1.643888              | 2.360384                                                         |
| 18923 | 1.014638              | 2.360392                                                         |
| 18925 | 1.241638              | 2.360400                                                         |
| 18927 | 1.483595              | 2.360408                                                         |
| 18929 | 1.044746              | 2.360416                                                         |
| 18931 | 1.091543              | 2.360424                                                         |
| 18933 | 1.333545              | 2.360432                                                         |

| $n$   | $\frac{\sigma(n)}{n}$ | $\frac{e^\gamma}{2} \log \log n + \frac{0.73\dots}{\log \log n}$ |
|-------|-----------------------|------------------------------------------------------------------|
| 18935 | 1.373964              | 2.360440                                                         |
| 18937 | 1.036067              | 2.360448                                                         |
| 18939 | 1.368604              | 2.360456                                                         |
| 18941 | 1.135315              | 2.360464                                                         |
| 18943 | 1.053687              | 2.360472                                                         |
| 18945 | 1.737451              | 2.360480                                                         |
| 18947 | 1.000053              | 2.360488                                                         |
| 18949 | 1.143279              | 2.360496                                                         |
| 18951 | 1.333544              | 2.360504                                                         |
| 18953 | 1.091542              | 2.360512                                                         |
| 18955 | 1.276286              | 2.360520                                                         |
| 18957 | 1.367305              | 2.360528                                                         |
| 18959 | 1.000053              | 2.360536                                                         |
| 18961 | 1.018512              | 2.360544                                                         |
| 18963 | 1.719348              | 2.360552                                                         |
| 18965 | 1.200316              | 2.360560                                                         |
| 18967 | 1.077661              | 2.360568                                                         |
| 18969 | 1.333544              | 2.360576                                                         |
| 18971 | 1.019662              | 2.360584                                                         |
| 18973 | 1.000053              | 2.360592                                                         |
| 18975 | 1.882055              | 2.360600                                                         |
| 18977 | 1.143279              | 2.360609                                                         |
| 18979 | 1.000053              | 2.360617                                                         |
| 18981 | 1.601602              | 2.360625                                                         |
| 18983 | 1.026603              | 2.360633                                                         |
| 18985 | 1.200316              | 2.360641                                                         |
| 18987 | 1.333544              | 2.360649                                                         |
| 18989 | 1.059771              | 2.360657                                                         |
| 18991 | 1.143278              | 2.360665                                                         |
| 18993 | 1.438846              | 2.360673                                                         |
| 18995 | 1.250855              | 2.360681                                                         |
| 18997 | 1.106175              | 2.360689                                                         |
| 18999 | 1.445129              | 2.360697                                                         |
| 19001 | 1.000053              | 2.360705                                                         |
| 19003 | 1.033942              | 2.360713                                                         |
| 19005 | 1.838674              | 2.360721                                                         |
| 19007 | 1.016468              | 2.360729                                                         |
| 19009 | 1.000053              | 2.360737                                                         |
| 19011 | 1.333544              | 2.360745                                                         |
| 19013 | 1.000053              | 2.360753                                                         |
| 19015 | 1.200316              | 2.360761                                                         |
| 19017 | 1.445128              | 2.360769                                                         |
| 19019 | 1.413324              | 2.360777                                                         |
| 19021 | 1.044740              | 2.360785                                                         |

| $n$   | $\frac{\sigma(n)}{n}$ | $\frac{e^\gamma}{2} \log \log n + \frac{0.73...}{\log \log n}$ |
|-------|-----------------------|----------------------------------------------------------------|
| 19023 | 1.415550              | 2.360793                                                       |
| 19025 | 1.241629              | 2.360801                                                       |
| 19027 | 1.021706              | 2.360809                                                       |
| 19029 | 1.333544              | 2.360817                                                       |
| 19031 | 1.000053              | 2.360825                                                       |
| 19033 | 1.143277              | 2.360833                                                       |
| 19035 | 1.830733              | 2.360841                                                       |
| 19037 | 1.000053              | 2.360849                                                       |
| 19039 | 1.016860              | 2.360857                                                       |
| 19041 | 1.457066              | 2.360865                                                       |
| 19043 | 1.014546              | 2.360872                                                       |
| 19045 | 1.296718              | 2.360880                                                       |
| 19047 | 1.525490              | 2.360888                                                       |
| 19049 | 1.025566              | 2.360896                                                       |
| 19051 | 1.000052              | 2.360904                                                       |
| 19053 | 1.514722              | 2.360912                                                       |
| 19055 | 1.244398              | 2.360920                                                       |
| 19057 | 1.133442              | 2.360928                                                       |
| 19059 | 1.333543              | 2.360936                                                       |
| 19061 | 1.166256              | 2.360944                                                       |
| 19063 | 1.091539              | 2.360952                                                       |
| 19065 | 1.691896              | 2.360960                                                       |
| 19067 | 1.044737              | 2.360968                                                       |
| 19069 | 1.000052              | 2.360976                                                       |
| 19071 | 1.565099              | 2.360984                                                       |
| 19073 | 1.000052              | 2.360992                                                       |
| 19075 | 1.430144              | 2.361000                                                       |
| 19077 | 1.333543              | 2.361008                                                       |
| 19079 | 1.000052              | 2.361016                                                       |
| 19081 | 1.000052              | 2.361024                                                       |
| 19083 | 1.333543              | 2.361032                                                       |
| 19085 | 1.312864              | 2.361040                                                       |
| 19087 | 1.000052              | 2.361048                                                       |
| 19089 | 1.709885              | 2.361056                                                       |
| 19091 | 1.059766              | 2.361064                                                       |
| 19093 | 1.019641              | 2.361072                                                       |
| 19095 | 1.709348              | 2.361080                                                       |
| 19097 | 1.092423              | 2.361088                                                       |
| 19099 | 1.017854              | 2.361096                                                       |
| 19101 | 1.333543              | 2.361104                                                       |
| 19103 | 1.143276              | 2.361112                                                       |
| 19105 | 1.200314              | 2.361120                                                       |
| 19107 | 1.583922              | 2.361128                                                       |
| 19109 | 1.015438              | 2.361135                                                       |

| $n$   | $\frac{\sigma(n)}{n}$ | $\frac{e^\gamma}{2} \log \log n + \frac{0.73...}{\log \log n}$ |
|-------|-----------------------|----------------------------------------------------------------|
| 19111 | 1.036053              | 2.361143                                                       |
| 19113 | 1.396327              | 2.361151                                                       |
| 19115 | 1.200314              | 2.361159                                                       |
| 19117 | 1.143276              | 2.361167                                                       |
| 19119 | 1.333543              | 2.361175                                                       |
| 19121 | 1.000052              | 2.361183                                                       |
| 19123 | 1.077655              | 2.361191                                                       |
| 19125 | 1.908706              | 2.361199                                                       |
| 19127 | 1.033931              | 2.361207                                                       |
| 19129 | 1.144231              | 2.361215                                                       |
| 19131 | 1.525482              | 2.361223                                                       |
| 19133 | 1.075315              | 2.361231                                                       |
| 19135 | 1.241704              | 2.361239                                                       |
| 19137 | 1.333542              | 2.361247                                                       |
| 19139 | 1.000052              | 2.361255                                                       |
| 19141 | 1.000052              | 2.361263                                                       |
| 19143 | 1.483571              | 2.361271                                                       |
| 19145 | 1.373936              | 2.361279                                                       |
| 19147 | 1.026584              | 2.361286                                                       |
| 19149 | 1.438822              | 2.361294                                                       |
| 19151 | 1.091536              | 2.361302                                                       |
| 19153 | 1.014985              | 2.361310                                                       |
| 19155 | 1.601253              | 2.361318                                                       |
| 19157 | 1.000052              | 2.361326                                                       |
| 19159 | 1.285245              | 2.361334                                                       |
| 19161 | 1.445123              | 2.361342                                                       |
| 19163 | 1.000052              | 2.361350                                                       |
| 19165 | 1.200313              | 2.361358                                                       |
| 19167 | 1.333542              | 2.361366                                                       |
| 19169 | 1.036048              | 2.361374                                                       |
| 19171 | 1.053675              | 2.361382                                                       |
| 19173 | 1.682366              | 2.361390                                                       |
| 19175 | 1.358018              | 2.361398                                                       |
| 19177 | 1.014549              | 2.361405                                                       |
| 19179 | 1.445122              | 2.361413                                                       |
| 19181 | 1.000052              | 2.361421                                                       |
| 19183 | 1.000052              | 2.361429                                                       |
| 19185 | 1.601251              | 2.361437                                                       |
| 19187 | 1.143274              | 2.361445                                                       |
| 19189 | 1.033926              | 2.361453                                                       |
| 19191 | 1.333542              | 2.361461                                                       |
| 19193 | 1.059761              | 2.361469                                                       |
| 19195 | 1.312842              | 2.361477                                                       |
| 19197 | 1.516904              | 2.361485                                                       |



| $n$   | $\frac{\sigma(n)}{n}$ | $\frac{e^\gamma}{2} \log \log n + \frac{0.73\dots}{\log \log n}$ |
|-------|-----------------------|------------------------------------------------------------------|
| 19199 | 1.017553              | 2.361493                                                         |
| 19201 | 1.236602              | 2.361500                                                         |
| 19203 | 1.377285              | 2.361508                                                         |
| 19205 | 1.259672              | 2.361516                                                         |
| 19207 | 1.000052              | 2.361524                                                         |
| 19209 | 1.407673              | 2.361532                                                         |
| 19211 | 1.000052              | 2.361540                                                         |
| 19213 | 1.000052              | 2.361548                                                         |
| 19215 | 2.013427              | 2.361556                                                         |
| 19217 | 1.091534              | 2.361564                                                         |
| 19219 | 1.000052              | 2.361572                                                         |
| 19221 | 1.373498              | 2.361580                                                         |
| 19223 | 1.023774              | 2.361587                                                         |
| 19225 | 1.241612              | 2.361595                                                         |
| 19227 | 1.572788              | 2.361603                                                         |
| 19229 | 1.188205              | 2.361611                                                         |
| 19231 | 1.000052              | 2.361619                                                         |
| 19233 | 1.445120              | 2.361627                                                         |
| 19235 | 1.200312              | 2.361635                                                         |
| 19237 | 1.000052              | 2.361643                                                         |
| 19239 | 1.493217              | 2.361651                                                         |
| 19241 | 1.017827              | 2.361659                                                         |
| 19243 | 1.143273              | 2.361666                                                         |
| 19245 | 1.601247              | 2.361674                                                         |
| 19247 | 1.053671              | 2.361682                                                         |
| 19249 | 1.000052              | 2.361690                                                         |
| 19251 | 1.595761              | 2.361698                                                         |
| 19253 | 1.077650              | 2.361706                                                         |
| 19255 | 1.200312              | 2.361714                                                         |
| 19257 | 1.562860              | 2.361722                                                         |
| 19259 | 1.000052              | 2.361730                                                         |
| 19261 | 1.166295              | 2.361737                                                         |
| 19263 | 1.333541              | 2.361745                                                         |
| 19265 | 1.200311              | 2.361753                                                         |
| 19267 | 1.000052              | 2.361761                                                         |
| 19269 | 1.445119              | 2.361769                                                         |
| 19271 | 1.143272              | 2.361777                                                         |
| 19273 | 1.000052              | 2.361785                                                         |
| 19275 | 1.659767              | 2.361793                                                         |
| 19277 | 1.028998              | 2.361801                                                         |
| 19279 | 1.077649              | 2.361808                                                         |
| 19281 | 1.333541              | 2.361816                                                         |
| 19283 | 1.091531              | 2.361824                                                         |
| 19285 | 1.493389              | 2.361832                                                         |

| $n$   | $\frac{\sigma(n)}{n}$ | $\frac{e^\gamma}{2} \log \log n + \frac{0.73...}{\log \log n}$ |
|-------|-----------------------|----------------------------------------------------------------|
| 19287 | 1.445118              | 2.361840                                                       |
| 19289 | 1.000052              | 2.361848                                                       |
| 19291 | 1.015188              | 2.361856                                                       |
| 19293 | 1.368372              | 2.361864                                                       |
| 19295 | 1.276186              | 2.361871                                                       |
| 19297 | 1.044722              | 2.361879                                                       |
| 19299 | 1.525468              | 2.361887                                                       |
| 19301 | 1.000052              | 2.361895                                                       |
| 19303 | 1.015386              | 2.361903                                                       |
| 19305 | 2.088578              | 2.361911                                                       |
| 19307 | 1.025535              | 2.361919                                                       |
| 19309 | 1.000052              | 2.361926                                                       |
| 19311 | 1.374553              | 2.361934                                                       |
| 19313 | 1.192979              | 2.361942                                                       |
| 19315 | 1.200311              | 2.361950                                                       |
| 19317 | 1.371642              | 2.361958                                                       |
| 19319 | 1.000052              | 2.361966                                                       |
| 19321 | 1.007246              | 2.361974                                                       |
| 19323 | 1.533923              | 2.361982                                                       |
| 19325 | 1.241604              | 2.361989                                                       |
| 19327 | 1.251720              | 2.361997                                                       |
| 19329 | 1.415490              | 2.362005                                                       |
| 19331 | 1.077647              | 2.362013                                                       |
| 19333 | 1.000052              | 2.362021                                                       |
| 19335 | 1.601241              | 2.362029                                                       |
| 19337 | 1.019600              | 2.362037                                                       |
| 19339 | 1.016392              | 2.362044                                                       |
| 19341 | 1.656171              | 2.362052                                                       |
| 19343 | 1.080701              | 2.362060                                                       |
| 19345 | 1.239390              | 2.362068                                                       |
| 19347 | 1.333540              | 2.362076                                                       |
| 19349 | 1.091529              | 2.362084                                                       |
| 19351 | 1.028991              | 2.362091                                                       |
| 19353 | 1.333540              | 2.362099                                                       |
| 19355 | 1.413588              | 2.362107                                                       |
| 19357 | 1.077646              | 2.362115                                                       |
| 19359 | 1.500077              | 2.362123                                                       |
| 19361 | 1.053665              | 2.362131                                                       |
| 19363 | 1.078139              | 2.362139                                                       |
| 19365 | 1.601239              | 2.362146                                                       |
| 19367 | 1.014922              | 2.362154                                                       |
| 19369 | 1.143270              | 2.362162                                                       |
| 19371 | 1.457023              | 2.362170                                                       |
| 19373 | 1.000052              | 2.362178                                                       |

| $n$   | $\frac{\sigma(n)}{n}$ | $\frac{e^\gamma}{2} \log \log n + \frac{0.73\dots}{\log \log n}$ |
|-------|-----------------------|------------------------------------------------------------------|
| 19375 | 1.289910              | 2.362186                                                         |
| 19377 | 1.445115              | 2.362193                                                         |
| 19379 | 1.000052              | 2.362201                                                         |
| 19381 | 1.000052              | 2.362209                                                         |
| 19383 | 1.664139              | 2.362217                                                         |
| 19385 | 1.200310              | 2.362225                                                         |
| 19387 | 1.000052              | 2.362233                                                         |
| 19389 | 1.396256              | 2.362240                                                         |
| 19391 | 1.000052              | 2.362248                                                         |
| 19393 | 1.143505              | 2.362256                                                         |
| 19395 | 1.737355              | 2.362264                                                         |
| 19397 | 1.217508              | 2.362272                                                         |
| 19399 | 1.053663              | 2.362280                                                         |
| 19401 | 1.385496              | 2.362287                                                         |
| 19403 | 1.000052              | 2.362295                                                         |
| 19405 | 1.200309              | 2.362303                                                         |
| 19407 | 1.333539              | 2.362311                                                         |
| 19409 | 1.077644              | 2.362319                                                         |
| 19411 | 1.186956              | 2.362326                                                         |
| 19413 | 1.483542              | 2.362334                                                         |
| 19415 | 1.312799              | 2.362342                                                         |
| 19417 | 1.000052              | 2.362350                                                         |
| 19419 | 1.333539              | 2.362358                                                         |
| 19421 | 1.000051              | 2.362366                                                         |
| 19423 | 1.000051              | 2.362373                                                         |
| 19425 | 1.940592              | 2.362381                                                         |
| 19427 | 1.000051              | 2.362389                                                         |
| 19429 | 1.000051              | 2.362397                                                         |
| 19431 | 1.541454              | 2.362405                                                         |
| 19433 | 1.000051              | 2.362412                                                         |
| 19435 | 1.355904              | 2.362420                                                         |
| 19437 | 1.580491              | 2.362428                                                         |
| 19439 | 1.143269              | 2.362436                                                         |
| 19441 | 1.000051              | 2.362444                                                         |
| 19443 | 1.333539              | 2.362451                                                         |
| 19445 | 1.200309              | 2.362459                                                         |
| 19447 | 1.000051              | 2.362467                                                         |
| 19449 | 1.445113              | 2.362475                                                         |
| 19451 | 1.021644              | 2.362483                                                         |
| 19453 | 1.166195              | 2.362491                                                         |
| 19455 | 1.601234              | 2.362498                                                         |
| 19457 | 1.000051              | 2.362506                                                         |
| 19459 | 1.147027              | 2.362514                                                         |
| 19461 | 1.438775              | 2.362522                                                         |

| $n$   | $\frac{\sigma(n)}{n}$ | $\frac{e^\gamma}{2} \log \log n + \frac{0.73...}{\log \log n}$ |
|-------|-----------------------|----------------------------------------------------------------|
| 19463 | 1.000051              | 2.362530                                                       |
| 19465 | 1.276137              | 2.362537                                                       |
| 19467 | 1.709560              | 2.362545                                                       |
| 19469 | 1.000051              | 2.362553                                                       |
| 19471 | 1.000051              | 2.362561                                                       |
| 19473 | 1.333539              | 2.362568                                                       |
| 19475 | 1.337099              | 2.362576                                                       |
| 19477 | 1.000051              | 2.362584                                                       |
| 19479 | 1.373376              | 2.362592                                                       |
| 19481 | 1.310816              | 2.362600                                                       |
| 19483 | 1.000051              | 2.362607                                                       |
| 19485 | 1.737336              | 2.362615                                                       |
| 19487 | 1.077642              | 2.362623                                                       |
| 19489 | 1.000051              | 2.362631                                                       |
| 19491 | 1.366785              | 2.362639                                                       |
| 19493 | 1.015134              | 2.362646                                                       |
| 19495 | 1.373891              | 2.362654                                                       |
| 19497 | 1.367185              | 2.362662                                                       |
| 19499 | 1.122519              | 2.362670                                                       |
| 19501 | 1.000051              | 2.362678                                                       |
| 19503 | 1.583756              | 2.362685                                                       |
| 19505 | 1.240297              | 2.362693                                                       |
| 19507 | 1.000051              | 2.362701                                                       |
| 19509 | 1.525450              | 2.362709                                                       |
| 19511 | 1.014812              | 2.362716                                                       |
| 19513 | 1.147953              | 2.362724                                                       |
| 19515 | 1.601230              | 2.362732                                                       |
| 19517 | 1.036020              | 2.362740                                                       |
| 19519 | 1.014396              | 2.362748                                                       |
| 19521 | 1.500026              | 2.362755                                                       |
| 19523 | 1.143267              | 2.362763                                                       |
| 19525 | 1.371780              | 2.362771                                                       |
| 19527 | 1.396221              | 2.362779                                                       |
| 19529 | 1.020022              | 2.362786                                                       |
| 19531 | 1.000051              | 2.362794                                                       |
| 19533 | 1.415451              | 2.362802                                                       |
| 19535 | 1.200307              | 2.362810                                                       |
| 19537 | 1.143267              | 2.362817                                                       |
| 19539 | 1.564870              | 2.362825                                                       |
| 19541 | 1.000051              | 2.362833                                                       |
| 19543 | 1.000051              | 2.362841                                                       |
| 19545 | 1.601228              | 2.362848                                                       |
| 19547 | 1.091523              | 2.362856                                                       |
| 19549 | 1.014681              | 2.362864                                                       |

| $n$   | $\frac{\sigma(n)}{n}$ | $\frac{e^\gamma}{2} \log \log n + \frac{0.73...}{\log \log n}$ |
|-------|-----------------------|----------------------------------------------------------------|
| 19551 | 1.636745              | 2.362872                                                       |
| 19553 | 1.000051              | 2.362880                                                       |
| 19555 | 1.200307              | 2.362887                                                       |
| 19557 | 1.507593              | 2.362895                                                       |
| 19559 | 1.000051              | 2.362903                                                       |
| 19561 | 1.033894              | 2.362911                                                       |
| 19563 | 1.333538              | 2.362918                                                       |
| 19565 | 1.511270              | 2.362926                                                       |
| 19567 | 1.059743              | 2.362934                                                       |
| 19569 | 1.456998              | 2.362942                                                       |
| 19571 | 1.000051              | 2.362949                                                       |
| 19573 | 1.073622              | 2.362957                                                       |
| 19575 | 1.900383              | 2.362965                                                       |
| 19577 | 1.000051              | 2.362973                                                       |
| 19579 | 1.143266              | 2.362980                                                       |
| 19581 | 1.367857              | 2.362988                                                       |
| 19583 | 1.000051              | 2.362996                                                       |
| 19585 | 1.200306              | 2.363004                                                       |
| 19587 | 1.333538              | 2.363011                                                       |
| 19589 | 1.053653              | 2.363019                                                       |
| 19591 | 1.183401              | 2.363027                                                       |
| 19593 | 1.656102              | 2.363035                                                       |
| 19595 | 1.200306              | 2.363042                                                       |
| 19597 | 1.000051              | 2.363050                                                       |
| 19599 | 1.371499              | 2.363058                                                       |
| 19601 | 1.059742              | 2.363065                                                       |
| 19603 | 1.000051              | 2.363073                                                       |
| 19605 | 1.601224              | 2.363081                                                       |
| 19607 | 1.143265              | 2.363089                                                       |
| 19609 | 1.000051              | 2.363096                                                       |
| 19611 | 1.445107              | 2.363104                                                       |
| 19613 | 1.091521              | 2.363112                                                       |
| 19615 | 1.200306              | 2.363120                                                       |
| 19617 | 1.438752              | 2.363127                                                       |
| 19619 | 1.044702              | 2.363135                                                       |
| 19621 | 1.143265              | 2.363143                                                       |
| 19623 | 1.382867              | 2.363151                                                       |
| 19625 | 1.255949              | 2.363158                                                       |
| 19627 | 1.053651              | 2.363166                                                       |
| 19629 | 1.483519              | 2.363174                                                       |
| 19631 | 1.018389              | 2.363181                                                       |
| 19633 | 1.036011              | 2.363189                                                       |
| 19635 | 2.112147              | 2.363197                                                       |
| 19637 | 1.017467              | 2.363205                                                       |

| $n$   | $\frac{\sigma(n)}{n}$ | $\frac{e^\gamma}{2} \log \log n + \frac{0.73\dots}{\log \log n}$ |
|-------|-----------------------|------------------------------------------------------------------|
| 19639 | 1.026529              | 2.363212                                                         |
| 19641 | 1.333537              | 2.363220                                                         |
| 19643 | 1.077636              | 2.363228                                                         |
| 19645 | 1.200305              | 2.363236                                                         |
| 19647 | 1.508627              | 2.363243                                                         |
| 19649 | 1.166166              | 2.363251                                                         |
| 19651 | 1.025495              | 2.363259                                                         |
| 19653 | 1.333537              | 2.363266                                                         |
| 19655 | 1.200305              | 2.363274                                                         |
| 19657 | 1.091520              | 2.363282                                                         |
| 19659 | 1.333537              | 2.363290                                                         |
| 19661 | 1.000051              | 2.363297                                                         |
| 19663 | 1.164827              | 2.363305                                                         |
| 19665 | 1.903890              | 2.363313                                                         |
| 19667 | 1.017745              | 2.363320                                                         |
| 19669 | 1.153084              | 2.363328                                                         |
| 19671 | 1.366479              | 2.363336                                                         |
| 19673 | 1.014995              | 2.363344                                                         |
| 19675 | 1.241576              | 2.363351                                                         |
| 19677 | 1.525436              | 2.363359                                                         |
| 19679 | 1.091519              | 2.363367                                                         |
| 19681 | 1.000051              | 2.363374                                                         |
| 19683 | 1.499975              | 2.363382                                                         |
| 19685 | 1.248463              | 2.363390                                                         |
| 19687 | 1.000051              | 2.363397                                                         |
| 19689 | 1.333536              | 2.363405                                                         |
| 19691 | 1.194454              | 2.363413                                                         |
| 19693 | 1.023714              | 2.363421                                                         |
| 19695 | 1.740137              | 2.363428                                                         |
| 19697 | 1.000051              | 2.363436                                                         |
| 19699 | 1.000051              | 2.363444                                                         |
| 19701 | 1.583676              | 2.363451                                                         |
| 19703 | 1.132822              | 2.363459                                                         |
| 19705 | 1.373865              | 2.363467                                                         |
| 19707 | 1.333536              | 2.363474                                                         |
| 19709 | 1.000051              | 2.363482                                                         |
| 19711 | 1.044696              | 2.363490                                                         |
| 19713 | 1.333536              | 2.363498                                                         |
| 19715 | 1.200304              | 2.363505                                                         |
| 19717 | 1.000051              | 2.363513                                                         |
| 19719 | 1.656068              | 2.363521                                                         |
| 19721 | 1.133005              | 2.363528                                                         |
| 19723 | 1.105917              | 2.363536                                                         |
| 19725 | 1.659620              | 2.363544                                                         |

| $n$   | $\frac{\sigma(n)}{n}$ | $\frac{e^\gamma}{2} \log \log n + \frac{0.73...}{\log \log n}$ |
|-------|-----------------------|----------------------------------------------------------------|
| 19727 | 1.000051              | 2.363551                                                       |
| 19729 | 1.014750              | 2.363559                                                       |
| 19731 | 1.333536              | 2.363567                                                       |
| 19733 | 1.143263              | 2.363574                                                       |
| 19735 | 1.200304              | 2.363582                                                       |
| 19737 | 1.605107              | 2.363590                                                       |
| 19739 | 1.000051              | 2.363597                                                       |
| 19741 | 1.053645              | 2.363605                                                       |
| 19743 | 1.333536              | 2.363613                                                       |
| 19745 | 1.312737              | 2.363620                                                       |
| 19747 | 1.293158              | 2.363628                                                       |
| 19749 | 1.385387              | 2.363636                                                       |
| 19751 | 1.000051              | 2.363643                                                       |
| 19753 | 1.000051              | 2.363651                                                       |
| 19755 | 1.737282              | 2.363659                                                       |
| 19757 | 1.044693              | 2.363666                                                       |
| 19759 | 1.000051              | 2.363674                                                       |
| 19761 | 1.525429              | 2.363682                                                       |
| 19763 | 1.000051              | 2.363690                                                       |
| 19765 | 1.238553              | 2.363697                                                       |
| 19767 | 1.456974              | 2.363705                                                       |
| 19769 | 1.021599              | 2.363713                                                       |
| 19771 | 1.059734              | 2.363720                                                       |
| 19773 | 1.564760              | 2.363728                                                       |
| 19775 | 1.429684              | 2.363736                                                       |
| 19777 | 1.000051              | 2.363743                                                       |
| 19779 | 1.407553              | 2.363751                                                       |
| 19781 | 1.014307              | 2.363759                                                       |
| 19783 | 1.017439              | 2.363766                                                       |
| 19785 | 1.601213              | 2.363774                                                       |
| 19787 | 1.023702              | 2.363781                                                       |
| 19789 | 1.251604              | 2.363789                                                       |
| 19791 | 1.483503              | 2.363797                                                       |
| 19793 | 1.000051              | 2.363804                                                       |
| 19795 | 1.243950              | 2.363812                                                       |
| 19797 | 1.333535              | 2.363820                                                       |
| 19799 | 1.077630              | 2.363827                                                       |
| 19801 | 1.000051              | 2.363835                                                       |
| 19803 | 1.628844              | 2.363843                                                       |
| 19805 | 1.276041              | 2.363850                                                       |
| 19807 | 1.035997              | 2.363858                                                       |
| 19809 | 1.512040              | 2.363866                                                       |
| 19811 | 1.091515              | 2.363873                                                       |
| 19813 | 1.000050              | 2.363881                                                       |

| $n$   | $\frac{\sigma(n)}{n}$ | $\frac{e^\gamma}{2} \log \log n + \frac{0.73\dots}{\log \log n}$ |
|-------|-----------------------|------------------------------------------------------------------|
| 19815 | 1.601211              | 2.363889                                                         |
| 19817 | 1.211081              | 2.363896                                                         |
| 19819 | 1.000050              | 2.363904                                                         |
| 19821 | 1.333535              | 2.363912                                                         |
| 19823 | 1.025475              | 2.363919                                                         |
| 19825 | 1.357276              | 2.363927                                                         |
| 19827 | 1.445100              | 2.363935                                                         |
| 19829 | 1.016693              | 2.363942                                                         |
| 19831 | 1.143261              | 2.363950                                                         |
| 19833 | 1.456966              | 2.363957                                                         |
| 19835 | 1.200302              | 2.363965                                                         |
| 19837 | 1.016283              | 2.363973                                                         |
| 19839 | 1.415394              | 2.363980                                                         |
| 19841 | 1.000050              | 2.363988                                                         |
| 19843 | 1.000050              | 2.363996                                                         |
| 19845 | 2.085261              | 2.364003                                                         |
| 19847 | 1.015771              | 2.364011                                                         |
| 19849 | 1.044687              | 2.364019                                                         |
| 19851 | 1.438718              | 2.364026                                                         |
| 19853 | 1.000050              | 2.364034                                                         |
| 19855 | 1.381617              | 2.364041                                                         |
| 19857 | 1.333535              | 2.364049                                                         |
| 19859 | 1.143260              | 2.364057                                                         |
| 19861 | 1.000050              | 2.364064                                                         |
| 19863 | 1.445099              | 2.364072                                                         |
| 19865 | 1.250440              | 2.364080                                                         |
| 19867 | 1.000050              | 2.364087                                                         |
| 19869 | 1.377019              | 2.364095                                                         |
| 19871 | 1.033868              | 2.364102                                                         |
| 19873 | 1.217330              | 2.364110                                                         |
| 19875 | 1.695396              | 2.364118                                                         |
| 19877 | 1.183277              | 2.364125                                                         |
| 19879 | 1.014940              | 2.364133                                                         |
| 19881 | 1.475831              | 2.364141                                                         |
| 19883 | 1.019967              | 2.364148                                                         |
| 19885 | 1.241941              | 2.364156                                                         |
| 19887 | 1.525419              | 2.364163                                                         |
| 19889 | 1.000050              | 2.364171                                                         |
| 19891 | 1.000050              | 2.364179                                                         |
| 19893 | 1.407530              | 2.364186                                                         |
| 19895 | 1.259412              | 2.364194                                                         |
| 19897 | 1.015027              | 2.364201                                                         |
| 19899 | 1.640283              | 2.364209                                                         |
| 19901 | 1.143259              | 2.364217                                                         |



| $n$   | $\frac{\sigma(n)}{n}$ | $\frac{e^\gamma}{2} \log \log n + \frac{0.73\dots}{\log \log n}$ |
|-------|-----------------------|------------------------------------------------------------------|
| 19903 | 1.077626              | 2.364224                                                         |
| 19905 | 1.601206              | 2.364232                                                         |
| 19907 | 1.059728              | 2.364240                                                         |
| 19909 | 1.025466              | 2.364247                                                         |
| 19911 | 1.333534              | 2.364255                                                         |
| 19913 | 1.000050              | 2.364262                                                         |
| 19915 | 1.373839              | 2.364270                                                         |
| 19917 | 1.445097              | 2.364278                                                         |
| 19919 | 1.000050              | 2.364285                                                         |
| 19921 | 1.091511              | 2.364293                                                         |
| 19923 | 1.385334              | 2.364300                                                         |
| 19925 | 1.241556              | 2.364308                                                         |
| 19927 | 1.000050              | 2.364316                                                         |
| 19929 | 1.663505              | 2.364323                                                         |
| 19931 | 1.053635              | 2.364331                                                         |
| 19933 | 1.033863              | 2.364338                                                         |
| 19935 | 1.737246              | 2.364346                                                         |
| 19937 | 1.000050              | 2.364354                                                         |
| 19939 | 1.014294              | 2.364361                                                         |
| 19941 | 1.477960              | 2.364369                                                         |
| 19943 | 1.303314              | 2.364376                                                         |
| 19945 | 1.200301              | 2.364384                                                         |
| 19947 | 1.367624              | 2.364392                                                         |
| 19949 | 1.000050              | 2.364399                                                         |
| 19951 | 1.017693              | 2.364407                                                         |
| 19953 | 1.483486              | 2.364414                                                         |
| 19955 | 1.296517              | 2.364422                                                         |
| 19957 | 1.143258              | 2.364430                                                         |
| 19959 | 1.333534              | 2.364437                                                         |
| 19961 | 1.000050              | 2.364445                                                         |
| 19963 | 1.000050              | 2.364452                                                         |
| 19965 | 1.759880              | 2.364460                                                         |
| 19967 | 1.026494              | 2.364467                                                         |
| 19969 | 1.053633              | 2.364475                                                         |
| 19971 | 1.656001              | 2.364483                                                         |
| 19973 | 1.000050              | 2.364490                                                         |
| 19975 | 1.340876              | 2.364498                                                         |
| 19977 | 1.333534              | 2.364505                                                         |
| 19979 | 1.000050              | 2.364513                                                         |
| 19981 | 1.135078              | 2.364521                                                         |
| 19983 | 1.333534              | 2.364528                                                         |
| 19985 | 1.373830              | 2.364536                                                         |
| 19987 | 1.152749              | 2.364543                                                         |
| 19989 | 1.445095              | 2.364551                                                         |

| $n$   | $\frac{\sigma(n)}{n}$ | $\frac{e^\gamma}{2} \log \log n + \frac{0.73...}{\log \log n}$ |
|-------|-----------------------|----------------------------------------------------------------|
| 19991 | 1.000050              | 2.364558                                                       |
| 19993 | 1.000050              | 2.364566                                                       |
| 19995 | 1.690023              | 2.364574                                                       |
| 19997 | 1.000050              | 2.364581                                                       |
| 19999 | 1.143257              | 2.364589                                                       |
| 20001 | 1.367932              | 2.364596                                                       |
| 20003 | 1.016248              | 2.364604                                                       |
| 20005 | 1.200300              | 2.364611                                                       |
| 20007 | 1.693407              | 2.364619                                                       |
| 20009 | 1.165875              | 2.364627                                                       |
| 20011 | 1.000050              | 2.364634                                                       |
| 20013 | 1.525408              | 2.364642                                                       |
| 20015 | 1.200300              | 2.364649                                                       |
| 20017 | 1.028925              | 2.364657                                                       |
| 20019 | 1.333533              | 2.364664                                                       |
| 20021 | 1.000050              | 2.364672                                                       |
| 20023 | 1.000050              | 2.364680                                                       |
| 20025 | 1.811236              | 2.364687                                                       |
| 20027 | 1.143257              | 2.364695                                                       |
| 20029 | 1.000050              | 2.364702                                                       |
| 20031 | 1.456942              | 2.364710                                                       |
| 20033 | 1.140518              | 2.364717                                                       |
| 20035 | 1.200299              | 2.364725                                                       |
| 20037 | 1.333533              | 2.364732                                                       |
| 20039 | 1.035980              | 2.364740                                                       |
| 20041 | 1.166109              | 2.364748                                                       |
| 20043 | 1.541087              | 2.364755                                                       |
| 20045 | 1.269144              | 2.364763                                                       |
| 20047 | 1.000050              | 2.364770                                                       |
| 20049 | 1.374233              | 2.364778                                                       |
| 20051 | 1.000050              | 2.364785                                                       |
| 20053 | 1.091508              | 2.364793                                                       |
| 20055 | 1.838145              | 2.364800                                                       |
| 20057 | 1.033854              | 2.364808                                                       |
| 20059 | 1.077621              | 2.364815                                                       |
| 20061 | 1.483475              | 2.364823                                                       |
| 20063 | 1.000050              | 2.364831                                                       |
| 20065 | 1.200299              | 2.364838                                                       |
| 20067 | 1.333533              | 2.364846                                                       |
| 20069 | 1.186307              | 2.364853                                                       |
| 20071 | 1.000050              | 2.364861                                                       |
| 20073 | 1.333533              | 2.364868                                                       |
| 20075 | 1.371258              | 2.364876                                                       |
| 20077 | 1.059720              | 2.364883                                                       |

| $n$   | $\frac{\sigma(n)}{n}$ | $\frac{e^\gamma}{2} \log \log n + \frac{0.73...}{\log \log n}$ |
|-------|-----------------------|----------------------------------------------------------------|
| 20079 | 1.522785              | 2.364891                                                       |
| 20081 | 1.025447              | 2.364898                                                       |
| 20083 | 1.210974              | 2.364906                                                       |
| 20085 | 1.739806              | 2.364914                                                       |
| 20087 | 1.021556              | 2.364921                                                       |
| 20089 | 1.000050              | 2.364929                                                       |
| 20091 | 1.376935              | 2.364936                                                       |
| 20093 | 1.017668              | 2.364944                                                       |
| 20095 | 1.200299              | 2.364951                                                       |
| 20097 | 1.862965              | 2.364959                                                       |
| 20099 | 1.014976              | 2.364966                                                       |
| 20101 | 1.000050              | 2.364974                                                       |
| 20103 | 1.333532              | 2.364981                                                       |
| 20105 | 1.200298              | 2.364989                                                       |
| 20107 | 1.000050              | 2.364996                                                       |
| 20109 | 1.333532              | 2.365004                                                       |
| 20111 | 1.310328              | 2.365011                                                       |
| 20113 | 1.000050              | 2.365019                                                       |
| 20115 | 1.789709              | 2.365026                                                       |
| 20117 | 1.000050              | 2.365034                                                       |
| 20119 | 1.145186              | 2.365042                                                       |
| 20121 | 1.407485              | 2.365049                                                       |
| 20123 | 1.000050              | 2.365057                                                       |
| 20125 | 1.488298              | 2.365064                                                       |
| 20127 | 1.333532              | 2.365072                                                       |
| 20129 | 1.000050              | 2.365079                                                       |
| 20131 | 1.026477              | 2.365087                                                       |
| 20133 | 1.445090              | 2.365094                                                       |
| 20135 | 1.200298              | 2.365102                                                       |
| 20137 | 1.077618              | 2.365109                                                       |
| 20139 | 1.562342              | 2.365117                                                       |
| 20141 | 1.091505              | 2.365124                                                       |
| 20143 | 1.000050              | 2.365132                                                       |
| 20145 | 1.715562              | 2.365139                                                       |
| 20147 | 1.000050              | 2.365147                                                       |
| 20149 | 1.000050              | 2.365154                                                       |
| 20151 | 1.445090              | 2.365162                                                       |
| 20153 | 1.143254              | 2.365169                                                       |
| 20155 | 1.250310              | 2.365177                                                       |
| 20157 | 1.333532              | 2.365184                                                       |
| 20159 | 1.053624              | 2.365192                                                       |
| 20161 | 1.000050              | 2.365199                                                       |
| 20163 | 1.599762              | 2.365207                                                       |
| 20165 | 1.243739              | 2.365214                                                       |

| $n$   | $\frac{\sigma(n)}{n}$ | $\frac{e^\gamma}{2} \log \log n + \frac{0.73...}{\log \log n}$ |
|-------|-----------------------|----------------------------------------------------------------|
| 20167 | 1.186889              | 2.365222                                                       |
| 20169 | 1.515990              | 2.365229                                                       |
| 20171 | 1.044668              | 2.365237                                                       |
| 20173 | 1.000050              | 2.365244                                                       |
| 20175 | 1.659480              | 2.365252                                                       |
| 20177 | 1.000050              | 2.365259                                                       |
| 20179 | 1.059716              | 2.365267                                                       |
| 20181 | 1.574550              | 2.365274                                                       |
| 20183 | 1.000050              | 2.365282                                                       |
| 20185 | 1.312658              | 2.365289                                                       |
| 20187 | 1.445088              | 2.365297                                                       |
| 20189 | 1.077617              | 2.365304                                                       |
| 20191 | 1.019464              | 2.365312                                                       |
| 20193 | 1.369187              | 2.365319                                                       |
| 20195 | 1.373805              | 2.365327                                                       |
| 20197 | 1.053622              | 2.365334                                                       |
| 20199 | 1.333531              | 2.365342                                                       |
| 20201 | 1.000050              | 2.365349                                                       |
| 20203 | 1.015691              | 2.365357                                                       |
| 20205 | 1.737194              | 2.365364                                                       |
| 20207 | 1.105755              | 2.365372                                                       |
| 20209 | 1.143253              | 2.365379                                                       |
| 20211 | 1.333531              | 2.365387                                                       |
| 20213 | 1.122050              | 2.365394                                                       |
| 20215 | 1.296463              | 2.365402                                                       |
| 20217 | 1.396053              | 2.365409                                                       |
| 20219 | 1.000049              | 2.365417                                                       |
| 20221 | 1.017358              | 2.365424                                                       |
| 20223 | 1.708945              | 2.365432                                                       |
| 20225 | 1.241533              | 2.365439                                                       |
| 20227 | 1.014486              | 2.365447                                                       |
| 20229 | 1.456918              | 2.365454                                                       |
| 20231 | 1.000049              | 2.365462                                                       |
| 20233 | 1.000049              | 2.365469                                                       |
| 20235 | 1.707932              | 2.365476                                                       |
| 20237 | 1.185947              | 2.365484                                                       |
| 20239 | 1.028905              | 2.365491                                                       |
| 20241 | 1.564547              | 2.365499                                                       |
| 20243 | 1.033839              | 2.365506                                                       |
| 20245 | 1.200296              | 2.365514                                                       |
| 20247 | 1.415321              | 2.365521                                                       |
| 20249 | 1.000049              | 2.365529                                                       |
| 20251 | 1.251494              | 2.365536                                                       |
| 20253 | 1.373031              | 2.365544                                                       |

| $n$   | $\frac{\sigma(n)}{n}$ | $\frac{e^\gamma}{2} \log \log n + \frac{0.73...}{\log \log n}$ |
|-------|-----------------------|----------------------------------------------------------------|
| 20255 | 1.200296              | 2.365551                                                       |
| 20257 | 1.023646              | 2.365559                                                       |
| 20259 | 1.445086              | 2.365566                                                       |
| 20261 | 1.000049              | 2.365574                                                       |
| 20263 | 1.044663              | 2.365581                                                       |
| 20265 | 1.838046              | 2.365589                                                       |
| 20267 | 1.077614              | 2.365596                                                       |
| 20269 | 1.000049              | 2.365603                                                       |
| 20271 | 1.385230              | 2.365611                                                       |
| 20273 | 1.160164              | 2.365618                                                       |
| 20275 | 1.241529              | 2.365626                                                       |
| 20277 | 1.483454              | 2.365633                                                       |
| 20279 | 1.143252              | 2.365641                                                       |
| 20281 | 1.059711              | 2.365648                                                       |
| 20283 | 1.333531              | 2.365656                                                       |
| 20285 | 1.200296              | 2.365663                                                       |
| 20287 | 1.000049              | 2.365671                                                       |
| 20289 | 1.333530              | 2.365678                                                       |
| 20291 | 1.014834              | 2.365685                                                       |
| 20293 | 1.236288              | 2.365693                                                       |
| 20295 | 1.937029              | 2.365700                                                       |
| 20297 | 1.000049              | 2.365708                                                       |
| 20299 | 1.021528              | 2.365715                                                       |
| 20301 | 1.366632              | 2.365723                                                       |
| 20303 | 1.016599              | 2.365730                                                       |
| 20305 | 1.248165              | 2.365738                                                       |
| 20307 | 1.525385              | 2.365745                                                       |
| 20309 | 1.044660              | 2.365753                                                       |
| 20311 | 1.053616              | 2.365760                                                       |
| 20313 | 1.507803              | 2.365767                                                       |
| 20315 | 1.275905              | 2.365775                                                       |
| 20317 | 1.091500              | 2.365782                                                       |
| 20319 | 1.438653              | 2.365790                                                       |
| 20321 | 1.143251              | 2.365797                                                       |
| 20323 | 1.000049              | 2.365805                                                       |
| 20325 | 1.659434              | 2.365812                                                       |
| 20327 | 1.000049              | 2.365820                                                       |
| 20329 | 1.035958              | 2.365827                                                       |
| 20331 | 1.499779              | 2.365834                                                       |
| 20333 | 1.000049              | 2.365842                                                       |
| 20335 | 1.412737              | 2.365849                                                       |
| 20337 | 1.333530              | 2.365857                                                       |
| 20339 | 1.116869              | 2.365864                                                       |
| 20341 | 1.000049              | 2.365872                                                       |

| $n$   | $\frac{\sigma(n)}{n}$ | $\frac{e^\gamma}{2} \log \log n + \frac{0.73...}{\log \log n}$ |
|-------|-----------------------|----------------------------------------------------------------|
| 20343 | 1.333530              | 2.365879                                                       |
| 20345 | 1.296436              | 2.365886                                                       |
| 20347 | 1.000049              | 2.365894                                                       |
| 20349 | 1.839894              | 2.365901                                                       |
| 20351 | 1.023635              | 2.365909                                                       |
| 20353 | 1.000049              | 2.365916                                                       |
| 20355 | 1.697863              | 2.365924                                                       |
| 20357 | 1.000049              | 2.365931                                                       |
| 20359 | 1.000049              | 2.365938                                                       |
| 20361 | 1.456903              | 2.365946                                                       |
| 20363 | 1.143250              | 2.365953                                                       |
| 20365 | 1.200295              | 2.365961                                                       |
| 20367 | 1.511465              | 2.365968                                                       |
| 20369 | 1.000049              | 2.365976                                                       |
| 20371 | 1.077610              | 2.365983                                                       |
| 20373 | 1.333530              | 2.365990                                                       |
| 20375 | 1.255656              | 2.365998                                                       |
| 20377 | 1.187221              | 2.366005                                                       |
| 20379 | 1.333530              | 2.366013                                                       |
| 20381 | 1.015652              | 2.366020                                                       |
| 20383 | 1.165677              | 2.366027                                                       |
| 20385 | 1.789551              | 2.366035                                                       |
| 20387 | 1.118360              | 2.366042                                                       |
| 20389 | 1.000049              | 2.366050                                                       |
| 20391 | 1.525379              | 2.366057                                                       |
| 20393 | 1.000049              | 2.366065                                                       |
| 20395 | 1.200294              | 2.366072                                                       |
| 20397 | 1.438643              | 2.366079                                                       |
| 20399 | 1.000049              | 2.366087                                                       |
| 20401 | 1.044655              | 2.366094                                                       |
| 20403 | 1.445082              | 2.366102                                                       |
| 20405 | 1.524332              | 2.366109                                                       |
| 20407 | 1.000049              | 2.366116                                                       |
| 20409 | 1.333529              | 2.366124                                                       |
| 20411 | 1.000049              | 2.366131                                                       |
| 20413 | 1.014060              | 2.366139                                                       |
| 20415 | 1.601176              | 2.366146                                                       |
| 20417 | 1.059705              | 2.366153                                                       |
| 20419 | 1.143249              | 2.366161                                                       |
| 20421 | 1.445081              | 2.366168                                                       |
| 20423 | 1.077609              | 2.366176                                                       |
| 20425 | 1.335618              | 2.366183                                                       |
| 20427 | 1.456895              | 2.366190                                                       |
| 20429 | 1.033824              | 2.366198                                                       |

| $n$   | $\frac{\sigma(n)}{n}$ | $\frac{e^\gamma}{2} \log \log n + \frac{0.73...}{\log \log n}$ |
|-------|-----------------------|----------------------------------------------------------------|
| 20431 | 1.000049              | 2.366205                                                       |
| 20433 | 1.562179              | 2.366213                                                       |
| 20435 | 1.237876              | 2.366220                                                       |
| 20437 | 1.014630              | 2.366227                                                       |
| 20439 | 1.483439              | 2.366235                                                       |
| 20441 | 1.000049              | 2.366242                                                       |
| 20443 | 1.000049              | 2.366250                                                       |
| 20445 | 1.690389              | 2.366257                                                       |
| 20447 | 1.201937              | 2.366264                                                       |
| 20449 | 1.190229              | 2.366272                                                       |
| 20451 | 1.415285              | 2.366279                                                       |
| 20453 | 1.014423              | 2.366287                                                       |
| 20455 | 1.200293              | 2.366294                                                       |
| 20457 | 1.445080              | 2.366301                                                       |
| 20459 | 1.026443              | 2.366309                                                       |
| 20461 | 1.188603              | 2.366316                                                       |
| 20463 | 1.407418              | 2.366324                                                       |
| 20465 | 1.200293              | 2.366331                                                       |
| 20467 | 1.015097              | 2.366338                                                       |
| 20469 | 1.333529              | 2.366346                                                       |
| 20471 | 1.091495              | 2.366353                                                       |
| 20473 | 1.019880              | 2.366360                                                       |
| 20475 | 2.204444              | 2.366368                                                       |
| 20477 | 1.000049              | 2.366375                                                       |
| 20479 | 1.000049              | 2.366383                                                       |
| 20481 | 1.333529              | 2.366390                                                       |
| 20483 | 1.000049              | 2.366397                                                       |
| 20485 | 1.275860              | 2.366405                                                       |
| 20487 | 1.333529              | 2.366412                                                       |
| 20489 | 1.143248              | 2.366419                                                       |
| 20491 | 1.033820              | 2.366427                                                       |
| 20493 | 1.700483              | 2.366434                                                       |
| 20495 | 1.200293              | 2.366442                                                       |
| 20497 | 1.014783              | 2.366449                                                       |
| 20499 | 1.333528              | 2.366456                                                       |
| 20501 | 1.147261              | 2.366464                                                       |
| 20503 | 1.193972              | 2.366471                                                       |
| 20505 | 1.601170              | 2.366478                                                       |
| 20507 | 1.000049              | 2.366486                                                       |
| 20509 | 1.000049              | 2.366493                                                       |
| 20511 | 1.505924              | 2.366501                                                       |
| 20513 | 1.017306              | 2.366508                                                       |
| 20515 | 1.312601              | 2.366515                                                       |
| 20517 | 1.525369              | 2.366523                                                       |

| $n$   | $\frac{\sigma(n)}{n}$ | $\frac{e^\gamma}{2} \log \log n + \frac{0.73...}{\log \log n}$ |
|-------|-----------------------|----------------------------------------------------------------|
| 20519 | 1.077245              | 2.366530                                                       |
| 20521 | 1.000049              | 2.366537                                                       |
| 20523 | 1.333528              | 2.366545                                                       |
| 20525 | 1.241510              | 2.366552                                                       |
| 20527 | 1.077605              | 2.366559                                                       |
| 20529 | 1.445078              | 2.366567                                                       |
| 20531 | 1.166042              | 2.366574                                                       |
| 20533 | 1.000049              | 2.366582                                                       |
| 20535 | 1.644412              | 2.366589                                                       |
| 20537 | 1.091493              | 2.366596                                                       |
| 20539 | 1.121768              | 2.366604                                                       |
| 20541 | 1.374032              | 2.366611                                                       |
| 20543 | 1.000049              | 2.366618                                                       |
| 20545 | 1.373765              | 2.366626                                                       |
| 20547 | 1.483428              | 2.366633                                                       |
| 20549 | 1.000049              | 2.366640                                                       |
| 20551 | 1.000049              | 2.366648                                                       |
| 20553 | 1.569406              | 2.366655                                                       |
| 20555 | 1.200292              | 2.366662                                                       |
| 20557 | 1.019409              | 2.366670                                                       |
| 20559 | 1.681016              | 2.366677                                                       |
| 20561 | 1.035942              | 2.366684                                                       |
| 20563 | 1.000049              | 2.366692                                                       |
| 20565 | 1.737126              | 2.366699                                                       |
| 20567 | 1.014052              | 2.366707                                                       |
| 20569 | 1.018231              | 2.366714                                                       |
| 20571 | 1.333528              | 2.366721                                                       |
| 20573 | 1.143246              | 2.366729                                                       |
| 20575 | 1.241507              | 2.366736                                                       |
| 20577 | 1.407397              | 2.366743                                                       |
| 20579 | 1.077603              | 2.366751                                                       |
| 20581 | 1.091492              | 2.366758                                                       |
| 20583 | 1.445076              | 2.366765                                                       |
| 20585 | 1.259169              | 2.366773                                                       |
| 20587 | 1.217079              | 2.366780                                                       |
| 20589 | 1.333528              | 2.366787                                                       |
| 20591 | 1.019863              | 2.366795                                                       |
| 20593 | 1.000049              | 2.366802                                                       |
| 20595 | 1.601165              | 2.366809                                                       |
| 20597 | 1.025392              | 2.366817                                                       |
| 20599 | 1.000049              | 2.366824                                                       |
| 20601 | 1.708655              | 2.366831                                                       |
| 20603 | 1.091492              | 2.366839                                                       |
| 20605 | 1.296384              | 2.366846                                                       |



| $n$   | $\frac{\sigma(n)}{n}$ | $\frac{e^\gamma}{2} \log \log n + \frac{0.73...}{\log \log n}$ |
|-------|-----------------------|----------------------------------------------------------------|
| 20607 | 1.333527              | 2.366853                                                       |
| 20609 | 1.028871              | 2.366861                                                       |
| 20611 | 1.000049              | 2.366868                                                       |
| 20613 | 1.333527              | 2.366875                                                       |
| 20615 | 1.490177              | 2.366883                                                       |
| 20617 | 1.021487              | 2.366890                                                       |
| 20619 | 1.513167              | 2.366897                                                       |
| 20621 | 1.059696              | 2.366905                                                       |
| 20623 | 1.026427              | 2.366912                                                       |
| 20625 | 1.817600              | 2.366919                                                       |
| 20627 | 1.000048              | 2.366927                                                       |
| 20629 | 1.166028              | 2.366934                                                       |
| 20631 | 1.501042              | 2.366941                                                       |
| 20633 | 1.023603              | 2.366948                                                       |
| 20635 | 1.200291              | 2.366956                                                       |
| 20637 | 1.445074              | 2.366963                                                       |
| 20639 | 1.000048              | 2.366970                                                       |
| 20641 | 1.000048              | 2.366978                                                       |
| 20643 | 1.525360              | 2.366985                                                       |
| 20645 | 1.200291              | 2.366992                                                       |
| 20647 | 1.091490              | 2.367000                                                       |
| 20649 | 1.333527              | 2.367007                                                       |
| 20651 | 1.014576              | 2.367014                                                       |
| 20653 | 1.053600              | 2.367022                                                       |
| 20655 | 1.903268              | 2.367029                                                       |
| 20657 | 1.236191              | 2.367036                                                       |
| 20659 | 1.017281              | 2.367044                                                       |
| 20661 | 1.366052              | 2.367051                                                       |
| 20663 | 1.000048              | 2.367058                                                       |
| 20665 | 1.200290              | 2.367066                                                       |
| 20667 | 1.349591              | 2.367073                                                       |
| 20669 | 1.091490              | 2.367080                                                       |
| 20671 | 1.143244              | 2.367087                                                       |
| 20673 | 1.445073              | 2.367095                                                       |
| 20675 | 1.241499              | 2.367102                                                       |
| 20677 | 1.114282              | 2.367109                                                       |
| 20679 | 1.367184              | 2.367117                                                       |
| 20681 | 1.000048              | 2.367124                                                       |
| 20683 | 1.131751              | 2.367131                                                       |
| 20685 | 1.837854              | 2.367139                                                       |
| 20687 | 1.013970              | 2.367146                                                       |
| 20689 | 1.059694              | 2.367153                                                       |
| 20691 | 1.671258              | 2.367160                                                       |
| 20693 | 1.000048              | 2.367168                                                       |

| $n$   | $\frac{\sigma(n)}{n}$ | $\frac{e^\gamma}{2} \log \log n + \frac{0.73\dots}{\log \log n}$ |
|-------|-----------------------|------------------------------------------------------------------|
| 20695 | 1.200290              | 2.367175                                                         |
| 20697 | 1.333527              | 2.367182                                                         |
| 20699 | 1.143244              | 2.367190                                                         |
| 20701 | 1.014057              | 2.367197                                                         |
| 20703 | 1.366372              | 2.367204                                                         |
| 20705 | 1.241439              | 2.367212                                                         |
| 20707 | 1.000048              | 2.367219                                                         |
| 20709 | 1.622483              | 2.367226                                                         |
| 20711 | 1.013954              | 2.367233                                                         |
| 20713 | 1.251388              | 2.367241                                                         |
| 20715 | 1.601159              | 2.367248                                                         |
| 20717 | 1.000048              | 2.367255                                                         |
| 20719 | 1.000048              | 2.367263                                                         |
| 20721 | 1.333526              | 2.367270                                                         |
| 20723 | 1.125706              | 2.367277                                                         |
| 20725 | 1.241496              | 2.367284                                                         |
| 20727 | 1.716023              | 2.367292                                                         |
| 20729 | 1.053596              | 2.367299                                                         |
| 20731 | 1.000048              | 2.367306                                                         |
| 20733 | 1.333526              | 2.367314                                                         |
| 20735 | 1.458404              | 2.367321                                                         |
| 20737 | 1.015576              | 2.367328                                                         |
| 20739 | 1.382516              | 2.367335                                                         |
| 20741 | 1.143243              | 2.367343                                                         |
| 20743 | 1.000048              | 2.367350                                                         |
| 20745 | 1.737093              | 2.367357                                                         |
| 20747 | 1.000048              | 2.367364                                                         |
| 20749 | 1.000048              | 2.367372                                                         |
| 20751 | 1.333526              | 2.367379                                                         |
| 20753 | 1.000048              | 2.367386                                                         |
| 20755 | 1.373741              | 2.367394                                                         |
| 20757 | 1.581731              | 2.367401                                                         |
| 20759 | 1.000048              | 2.367408                                                         |
| 20761 | 1.077597              | 2.367415                                                         |
| 20763 | 1.483408              | 2.367423                                                         |
| 20765 | 1.200289              | 2.367430                                                         |
| 20767 | 1.053595              | 2.367437                                                         |
| 20769 | 1.627040              | 2.367444                                                         |
| 20771 | 1.000048              | 2.367452                                                         |
| 20773 | 1.000048              | 2.367459                                                         |
| 20775 | 1.659302              | 2.367466                                                         |
| 20777 | 1.016509              | 2.367474                                                         |
| 20779 | 1.091487              | 2.367481                                                         |
| 20781 | 1.445070              | 2.367488                                                         |

| $n$   | $\frac{\sigma(n)}{n}$ | $\frac{e^\gamma}{2} \log \log n + \frac{0.73\dots}{\log \log n}$ |
|-------|-----------------------|------------------------------------------------------------------|
| 20783 | 1.143242              | 2.367495                                                         |
| 20785 | 1.200289              | 2.367503                                                         |
| 20787 | 1.479001              | 2.367510                                                         |
| 20789 | 1.000048              | 2.367517                                                         |
| 20791 | 1.059689              | 2.367524                                                         |
| 20793 | 1.385082              | 2.367532                                                         |
| 20795 | 1.200289              | 2.367539                                                         |
| 20797 | 1.143242              | 2.367546                                                         |
| 20799 | 1.445069              | 2.367553                                                         |
| 20801 | 1.144560              | 2.367561                                                         |
| 20803 | 1.017546              | 2.367568                                                         |
| 20805 | 1.707282              | 2.367575                                                         |
| 20807 | 1.000048              | 2.367582                                                         |
| 20809 | 1.000048              | 2.367590                                                         |
| 20811 | 1.525347              | 2.367597                                                         |
| 20813 | 1.077596              | 2.367604                                                         |
| 20815 | 1.259092              | 2.367611                                                         |
| 20817 | 1.499640              | 2.367619                                                         |
| 20819 | 1.014458              | 2.367626                                                         |
| 20821 | 1.023582              | 2.367633                                                         |
| 20823 | 1.456851              | 2.367640                                                         |
| 20825 | 1.527299              | 2.367648                                                         |
| 20827 | 1.019830              | 2.367655                                                         |
| 20829 | 1.368861              | 2.367662                                                         |
| 20831 | 1.028851              | 2.367669                                                         |
| 20833 | 1.016080              | 2.367677                                                         |
| 20835 | 1.737077              | 2.367684                                                         |
| 20837 | 1.018189              | 2.367691                                                         |
| 20839 | 1.236144              | 2.367698                                                         |
| 20841 | 1.333525              | 2.367706                                                         |
| 20843 | 1.053591              | 2.367713                                                         |
| 20845 | 1.312545              | 2.367720                                                         |
| 20847 | 1.333525              | 2.367727                                                         |
| 20849 | 1.000048              | 2.367735                                                         |
| 20851 | 1.035922              | 2.367742                                                         |
| 20853 | 1.655781              | 2.367749                                                         |
| 20855 | 1.240566              | 2.367756                                                         |
| 20857 | 1.000048              | 2.367763                                                         |
| 20859 | 1.415216              | 2.367771                                                         |
| 20861 | 1.044629              | 2.367778                                                         |
| 20863 | 1.033792              | 2.367785                                                         |
| 20865 | 1.739180              | 2.367792                                                         |
| 20867 | 1.251354              | 2.367800                                                         |
| 20869 | 1.026403              | 2.367807                                                         |

| $n$   | $\frac{\sigma(n)}{n}$ | $\frac{e^\gamma}{2} \log \log n + \frac{0.73...}{\log \log n}$ |
|-------|-----------------------|----------------------------------------------------------------|
| 20871 | 1.483398              | 2.367814                                                       |
| 20873 | 1.000048              | 2.367821                                                       |
| 20875 | 1.255473              | 2.367829                                                       |
| 20877 | 1.333525              | 2.367836                                                       |
| 20879 | 1.000048              | 2.367843                                                       |
| 20881 | 1.210670              | 2.367850                                                       |
| 20883 | 1.333525              | 2.367857                                                       |
| 20885 | 1.200287              | 2.367865                                                       |
| 20887 | 1.000048              | 2.367872                                                       |
| 20889 | 1.583226              | 2.367879                                                       |
| 20891 | 1.077593              | 2.367886                                                       |
| 20893 | 1.059685              | 2.367894                                                       |
| 20895 | 1.837760              | 2.367901                                                       |
| 20897 | 1.000048              | 2.367908                                                       |
| 20899 | 1.000048              | 2.367915                                                       |
| 20901 | 1.333525              | 2.367922                                                       |
| 20903 | 1.000048              | 2.367930                                                       |
| 20905 | 1.243339              | 2.367937                                                       |
| 20907 | 1.522170              | 2.367944                                                       |
| 20909 | 1.193744              | 2.367951                                                       |
| 20911 | 1.091483              | 2.367959                                                       |
| 20913 | 1.333525              | 2.367966                                                       |
| 20915 | 1.239302              | 2.367973                                                       |
| 20917 | 1.077592              | 2.367980                                                       |
| 20919 | 1.407333              | 2.367987                                                       |
| 20921 | 1.000048              | 2.367995                                                       |
| 20923 | 1.185298              | 2.368002                                                       |
| 20925 | 1.896296              | 2.368009                                                       |
| 20927 | 1.059684              | 2.368016                                                       |
| 20929 | 1.000048              | 2.368023                                                       |
| 20931 | 1.333524              | 2.368031                                                       |
| 20933 | 1.105527              | 2.368038                                                       |
| 20935 | 1.238118              | 2.368045                                                       |
| 20937 | 1.525338              | 2.368052                                                       |
| 20939 | 1.000048              | 2.368059                                                       |
| 20941 | 1.025357              | 2.368067                                                       |
| 20943 | 1.564246              | 2.368074                                                       |
| 20945 | 1.237527              | 2.368081                                                       |
| 20947 | 1.000048              | 2.368088                                                       |
| 20949 | 1.333524              | 2.368095                                                       |
| 20951 | 1.186769              | 2.368103                                                       |
| 20953 | 1.044624              | 2.368110                                                       |
| 20955 | 1.759198              | 2.368117                                                       |
| 20957 | 1.053586              | 2.368124                                                       |

| $n$   | $\frac{\sigma(n)}{n}$ | $\frac{e^\gamma}{2} \log \log n + \frac{0.73\dots}{\log \log n}$ |
|-------|-----------------------|------------------------------------------------------------------|
| 20959 | 1.000048              | 2.368131                                                         |
| 20961 | 1.540575              | 2.368139                                                         |
| 20963 | 1.000048              | 2.368146                                                         |
| 20965 | 1.373718              | 2.368153                                                         |
| 20967 | 1.385034              | 2.368160                                                         |
| 20969 | 1.077591              | 2.368167                                                         |
| 20971 | 1.018168              | 2.368175                                                         |
| 20973 | 1.333524              | 2.368182                                                         |
| 20975 | 1.241478              | 2.368189                                                         |
| 20977 | 1.091481              | 2.368196                                                         |
| 20979 | 1.753372              | 2.368203                                                         |
| 20981 | 1.000048              | 2.368211                                                         |
| 20983 | 1.000048              | 2.368218                                                         |
| 20985 | 1.601144              | 2.368225                                                         |
| 20987 | 1.033783              | 2.368232                                                         |
| 20989 | 1.013864              | 2.368239                                                         |
| 20991 | 1.333524              | 2.368247                                                         |
| 20993 | 1.143238              | 2.368254                                                         |
| 20995 | 1.440343              | 2.368261                                                         |
| 20997 | 1.445064              | 2.368268                                                         |
| 20999 | 1.152055              | 2.368275                                                         |
| 21001 | 1.000048              | 2.368282                                                         |
| 21003 | 1.333524              | 2.368290                                                         |
| 21005 | 1.200286              | 2.368297                                                         |
| 21007 | 1.143238              | 2.368304                                                         |
| 21009 | 1.370841              | 2.368311                                                         |
| 21011 | 1.000048              | 2.368318                                                         |
| 21013 | 1.000048              | 2.368325                                                         |
| 21015 | 1.737045              | 2.368333                                                         |
| 21017 | 1.000048              | 2.368340                                                         |
| 21019 | 1.000048              | 2.368347                                                         |
| 21021 | 1.822178              | 2.368354                                                         |
| 21023 | 1.000048              | 2.368361                                                         |
| 21025 | 1.284233              | 2.368369                                                         |
| 21027 | 1.372711              | 2.368376                                                         |
| 21029 | 1.059679              | 2.368383                                                         |
| 21031 | 1.000048              | 2.368390                                                         |
| 21033 | 1.597490              | 2.368397                                                         |
| 21035 | 1.373710              | 2.368404                                                         |
| 21037 | 1.014403              | 2.368412                                                         |
| 21039 | 1.333523              | 2.368419                                                         |
| 21041 | 1.021434              | 2.368426                                                         |
| 21043 | 1.091479              | 2.368433                                                         |
| 21045 | 1.696935              | 2.368440                                                         |

| $n$   | $\frac{\sigma(n)}{n}$ | $\frac{e^\gamma}{2} \log \log n + \frac{0.73...}{\log \log n}$ |
|-------|-----------------------|----------------------------------------------------------------|
| 21047 | 1.077588              | 2.368447                                                       |
| 21049 | 1.191886              | 2.368455                                                       |
| 21051 | 1.445062              | 2.368462                                                       |
| 21053 | 1.028832              | 2.368469                                                       |
| 21055 | 1.200285              | 2.368476                                                       |
| 21057 | 1.333523              | 2.368483                                                       |
| 21059 | 1.000047              | 2.368490                                                       |
| 21061 | 1.000047              | 2.368498                                                       |
| 21063 | 1.640792              | 2.368505                                                       |
| 21065 | 1.312509              | 2.368512                                                       |
| 21067 | 1.000047              | 2.368519                                                       |
| 21069 | 1.445061              | 2.368526                                                       |
| 21071 | 1.053581              | 2.368533                                                       |
| 21073 | 1.077587              | 2.368540                                                       |
| 21075 | 1.659217              | 2.368548                                                       |
| 21077 | 1.143237              | 2.368555                                                       |
| 21079 | 1.014469              | 2.368562                                                       |
| 21081 | 1.333523              | 2.368569                                                       |
| 21083 | 1.035906              | 2.368576                                                       |
| 21085 | 1.200285              | 2.368583                                                       |
| 21087 | 1.638924              | 2.368591                                                       |
| 21089 | 1.000047              | 2.368598                                                       |
| 21091 | 1.201650              | 2.368605                                                       |
| 21093 | 1.365382              | 2.368612                                                       |
| 21095 | 1.200284              | 2.368619                                                       |
| 21097 | 1.076836              | 2.368626                                                       |
| 21099 | 1.438552              | 2.368633                                                       |
| 21101 | 1.000047              | 2.368641                                                       |
| 21103 | 1.023551              | 2.368648                                                       |
| 21105 | 2.010519              | 2.368655                                                       |
| 21107 | 1.000047              | 2.368662                                                       |
| 21109 | 1.159695              | 2.368669                                                       |
| 21111 | 1.382407              | 2.368676                                                       |
| 21113 | 1.025340              | 2.368683                                                       |
| 21115 | 1.241203              | 2.368691                                                       |
| 21117 | 1.333523              | 2.368698                                                       |
| 21119 | 1.165964              | 2.368705                                                       |
| 21121 | 1.000047              | 2.368712                                                       |
| 21123 | 1.445060              | 2.368719                                                       |
| 21125 | 1.351385              | 2.368726                                                       |
| 21127 | 1.028826              | 2.368733                                                       |
| 21129 | 1.333523              | 2.368740                                                       |
| 21131 | 1.165302              | 2.368748                                                       |
| 21133 | 1.143236              | 2.368755                                                       |

| $n$   | $\frac{\sigma(n)}{n}$ | $\frac{e^\gamma}{2} \log \log n + \frac{0.73...}{\log \log n}$ |
|-------|-----------------------|----------------------------------------------------------------|
| 21135 | 1.601136              | 2.368762                                                       |
| 21137 | 1.044614              | 2.368769                                                       |
| 21139 | 1.000047              | 2.368776                                                       |
| 21141 | 1.551015              | 2.368783                                                       |
| 21143 | 1.000047              | 2.368790                                                       |
| 21145 | 1.200284              | 2.368798                                                       |
| 21147 | 1.634274              | 2.368805                                                       |
| 21149 | 1.000047              | 2.368812                                                       |
| 21151 | 1.077585              | 2.368819                                                       |
| 21153 | 1.456815              | 2.368826                                                       |
| 21155 | 1.200284              | 2.368833                                                       |
| 21157 | 1.000047              | 2.368840                                                       |
| 21159 | 1.445059              | 2.368847                                                       |
| 21161 | 1.143235              | 2.368855                                                       |
| 21163 | 1.000047              | 2.368862                                                       |
| 21165 | 1.714529              | 2.368869                                                       |
| 21167 | 1.019323              | 2.368876                                                       |
| 21169 | 1.000047              | 2.368883                                                       |
| 21171 | 1.333522              | 2.368890                                                       |
| 21173 | 1.033769              | 2.368897                                                       |
| 21175 | 1.557686              | 2.368904                                                       |
| 21177 | 1.564150              | 2.368911                                                       |
| 21179 | 1.000047              | 2.368919                                                       |
| 21181 | 1.019782              | 2.368926                                                       |
| 21183 | 1.395836              | 2.368933                                                       |
| 21185 | 1.268822              | 2.368940                                                       |
| 21187 | 1.000047              | 2.368947                                                       |
| 21189 | 1.525320              | 2.368954                                                       |
| 21191 | 1.000047              | 2.368961                                                       |
| 21193 | 1.000047              | 2.368968                                                       |
| 21195 | 1.789101              | 2.368975                                                       |
| 21197 | 1.141294              | 2.368983                                                       |
| 21199 | 1.120808              | 2.368990                                                       |
| 21201 | 1.376539              | 2.368997                                                       |
| 21203 | 1.236052              | 2.369004                                                       |
| 21205 | 1.200283              | 2.369011                                                       |
| 21207 | 1.333522              | 2.369018                                                       |
| 21209 | 1.013909              | 2.369025                                                       |
| 21211 | 1.000047              | 2.369032                                                       |
| 21213 | 1.445057              | 2.369039                                                       |
| 21215 | 1.200283              | 2.369047                                                       |
| 21217 | 1.165952              | 2.369054                                                       |
| 21219 | 1.456808              | 2.369061                                                       |
| 21221 | 1.000047              | 2.369068                                                       |

| $n$   | $\frac{\sigma(n)}{n}$ | $\frac{e^\gamma}{2} \log \log n + \frac{0.73\dots}{\log \log n}$ |
|-------|-----------------------|------------------------------------------------------------------|
| 21223 | 1.053574              | 2.369075                                                         |
| 21225 | 1.659176              | 2.369082                                                         |
| 21227 | 1.000047              | 2.369089                                                         |
| 21229 | 1.139573              | 2.369096                                                         |
| 21231 | 1.655692              | 2.369103                                                         |
| 21233 | 1.059671              | 2.369110                                                         |
| 21235 | 1.247751              | 2.369118                                                         |
| 21237 | 1.333522              | 2.369125                                                         |
| 21239 | 1.018127              | 2.369132                                                         |
| 21241 | 1.091474              | 2.369139                                                         |
| 21243 | 1.365532              | 2.369146                                                         |
| 21245 | 1.373688              | 2.369153                                                         |
| 21247 | 1.000047              | 2.369160                                                         |
| 21249 | 1.483364              | 2.369167                                                         |
| 21251 | 1.016423              | 2.369174                                                         |
| 21253 | 1.021409              | 2.369181                                                         |
| 21255 | 1.738885              | 2.369188                                                         |
| 21257 | 1.035894              | 2.369196                                                         |
| 21259 | 1.143233              | 2.369203                                                         |
| 21261 | 1.407272              | 2.369210                                                         |
| 21263 | 1.091473              | 2.369217                                                         |
| 21265 | 1.200282              | 2.369224                                                         |
| 21267 | 1.540415              | 2.369231                                                         |
| 21269 | 1.000047              | 2.369238                                                         |
| 21271 | 1.015467              | 2.369245                                                         |
| 21273 | 1.525314              | 2.369252                                                         |
| 21275 | 1.328884              | 2.369259                                                         |
| 21277 | 1.000047              | 2.369266                                                         |
| 21279 | 1.373749              | 2.369273                                                         |
| 21281 | 1.077581              | 2.369281                                                         |
| 21283 | 1.000047              | 2.369288                                                         |
| 21285 | 1.934884              | 2.369295                                                         |
| 21287 | 1.143233              | 2.369302                                                         |
| 21289 | 1.019306              | 2.369309                                                         |
| 21291 | 1.370720              | 2.369316                                                         |
| 21293 | 1.014418              | 2.369323                                                         |
| 21295 | 1.200282              | 2.369330                                                         |
| 21297 | 1.382354              | 2.369337                                                         |
| 21299 | 1.073290              | 2.369344                                                         |
| 21301 | 1.216844              | 2.369351                                                         |
| 21303 | 1.499507              | 2.369358                                                         |
| 21305 | 1.200282              | 2.369365                                                         |
| 21307 | 1.182710              | 2.369372                                                         |
| 21309 | 1.333521              | 2.369380                                                         |



| $n$   | $\frac{\sigma(n)}{n}$ | $\frac{e^\gamma}{2} \log \log n + \frac{0.73\dots}{\log \log n}$ |
|-------|-----------------------|------------------------------------------------------------------|
| 21311 | 1.014687              | 2.369387                                                         |
| 21313 | 1.000047              | 2.369394                                                         |
| 21315 | 1.925405              | 2.369401                                                         |
| 21317 | 1.000047              | 2.369408                                                         |
| 21319 | 1.000047              | 2.369415                                                         |
| 21321 | 1.521880              | 2.369422                                                         |
| 21323 | 1.000047              | 2.369429                                                         |
| 21325 | 1.241454              | 2.369436                                                         |
| 21327 | 1.333521              | 2.369443                                                         |
| 21329 | 1.251254              | 2.369450                                                         |
| 21331 | 1.015986              | 2.369457                                                         |
| 21333 | 1.438522              | 2.369464                                                         |
| 21335 | 1.275650              | 2.369471                                                         |
| 21337 | 1.053569              | 2.369478                                                         |
| 21339 | 1.445054              | 2.369485                                                         |
| 21341 | 1.000047              | 2.369493                                                         |
| 21343 | 1.143232              | 2.369500                                                         |
| 21345 | 1.601124              | 2.369507                                                         |
| 21347 | 1.000047              | 2.369514                                                         |
| 21349 | 1.028807              | 2.369521                                                         |
| 21351 | 1.456794              | 2.369528                                                         |
| 21353 | 1.013815              | 2.369535                                                         |
| 21355 | 1.200281              | 2.369542                                                         |
| 21357 | 1.708105              | 2.369549                                                         |
| 21359 | 1.132637              | 2.369556                                                         |
| 21361 | 1.026356              | 2.369563                                                         |
| 21363 | 1.333521              | 2.369570                                                         |
| 21365 | 1.200281              | 2.369577                                                         |
| 21367 | 1.044601              | 2.369584                                                         |
| 21369 | 1.415134              | 2.369591                                                         |
| 21371 | 1.185906              | 2.369598                                                         |
| 21373 | 1.145370              | 2.369605                                                         |
| 21375 | 1.897544              | 2.369612                                                         |
| 21377 | 1.000047              | 2.369619                                                         |
| 21379 | 1.000047              | 2.369626                                                         |
| 21381 | 1.333520              | 2.369634                                                         |
| 21383 | 1.000047              | 2.369641                                                         |
| 21385 | 1.508347              | 2.369648                                                         |
| 21387 | 1.333520              | 2.369655                                                         |
| 21389 | 1.017158              | 2.369662                                                         |
| 21391 | 1.000047              | 2.369669                                                         |
| 21393 | 1.445052              | 2.369676                                                         |
| 21395 | 1.312456              | 2.369683                                                         |
| 21397 | 1.000047              | 2.369690                                                         |

| $n$   | $\frac{\sigma(n)}{n}$ | $\frac{e^\gamma}{2} \log \log n + \frac{0.73...}{\log \log n}$ |
|-------|-----------------------|----------------------------------------------------------------|
| 21399 | 1.525305              | 2.369697                                                       |
| 21401 | 1.000047              | 2.369704                                                       |
| 21403 | 1.059665              | 2.369711                                                       |
| 21405 | 1.601121              | 2.369718                                                       |
| 21407 | 1.000047              | 2.369725                                                       |
| 21409 | 1.016395              | 2.369732                                                       |
| 21411 | 1.621596              | 2.369739                                                       |
| 21413 | 1.277728              | 2.369746                                                       |
| 21415 | 1.200280              | 2.369753                                                       |
| 21417 | 1.490405              | 2.369760                                                       |
| 21419 | 1.000047              | 2.369767                                                       |
| 21421 | 1.033752              | 2.369774                                                       |
| 21423 | 1.376465              | 2.369781                                                       |
| 21425 | 1.241447              | 2.369788                                                       |
| 21427 | 1.143231              | 2.369795                                                       |
| 21429 | 1.445051              | 2.369802                                                       |
| 21431 | 1.035883              | 2.369809                                                       |
| 21433 | 1.000047              | 2.369816                                                       |
| 21435 | 1.601120              | 2.369823                                                       |
| 21437 | 1.152027              | 2.369830                                                       |
| 21439 | 1.091469              | 2.369837                                                       |
| 21441 | 1.525302              | 2.369844                                                       |
| 21443 | 1.026349              | 2.369851                                                       |
| 21445 | 1.200280              | 2.369859                                                       |
| 21447 | 1.445051              | 2.369866                                                       |
| 21449 | 1.015432              | 2.369873                                                       |
| 21451 | 1.053564              | 2.369880                                                       |
| 21453 | 1.333520              | 2.369887                                                       |
| 21455 | 1.373666              | 2.369894                                                       |
| 21457 | 1.025306              | 2.369901                                                       |
| 21459 | 1.395778              | 2.369908                                                       |
| 21461 | 1.091468              | 2.369915                                                       |
| 21463 | 1.091367              | 2.369922                                                       |
| 21465 | 1.826415              | 2.369929                                                       |
| 21467 | 1.000047              | 2.369936                                                       |
| 21469 | 1.143230              | 2.369943                                                       |
| 21471 | 1.415118              | 2.369950                                                       |
| 21473 | 1.014297              | 2.369957                                                       |
| 21475 | 1.241444              | 2.369964                                                       |
| 21477 | 1.333520              | 2.369971                                                       |
| 21479 | 1.023511              | 2.369978                                                       |
| 21481 | 1.000047              | 2.369985                                                       |
| 21483 | 1.858958              | 2.369992                                                       |
| 21485 | 1.200279              | 2.369999                                                       |

| $n$   | $\frac{\sigma(n)}{n}$ | $\frac{e^\gamma}{2} \log \log n + \frac{0.73\dots}{\log \log n}$ |
|-------|-----------------------|------------------------------------------------------------------|
| 21487 | 1.000047              | 2.370006                                                         |
| 21489 | 1.563591              | 2.370013                                                         |
| 21491 | 1.000047              | 2.370020                                                         |
| 21493 | 1.000047              | 2.370027                                                         |
| 21495 | 1.601117              | 2.370034                                                         |
| 21497 | 1.187887              | 2.370041                                                         |
| 21499 | 1.000047              | 2.370048                                                         |
| 21501 | 1.445049              | 2.370055                                                         |
| 21503 | 1.000047              | 2.370062                                                         |
| 21505 | 1.446361              | 2.370069                                                         |
| 21507 | 1.365881              | 2.370076                                                         |
| 21509 | 1.013715              | 2.370083                                                         |
| 21511 | 1.165915              | 2.370090                                                         |
| 21513 | 1.365500              | 2.370097                                                         |
| 21515 | 1.296212              | 2.370104                                                         |
| 21517 | 1.000046              | 2.370111                                                         |
| 21519 | 1.483340              | 2.370118                                                         |
| 21521 | 1.000046              | 2.370125                                                         |
| 21523 | 1.000046              | 2.370132                                                         |
| 21525 | 1.935610              | 2.370139                                                         |
| 21527 | 1.159474              | 2.370146                                                         |
| 21529 | 1.000046              | 2.370153                                                         |
| 21531 | 1.333519              | 2.370160                                                         |
| 21533 | 1.019273              | 2.370167                                                         |
| 21535 | 1.237056              | 2.370174                                                         |
| 21537 | 1.445048              | 2.370181                                                         |
| 21539 | 1.216770              | 2.370188                                                         |
| 21541 | 1.077573              | 2.370195                                                         |
| 21543 | 1.372511              | 2.370202                                                         |
| 21545 | 1.247621              | 2.370209                                                         |
| 21547 | 1.035875              | 2.370216                                                         |
| 21549 | 1.456773              | 2.370223                                                         |
| 21551 | 1.044592              | 2.370230                                                         |
| 21553 | 1.143228              | 2.370237                                                         |
| 21555 | 1.736952              | 2.370244                                                         |
| 21557 | 1.000046              | 2.370250                                                         |
| 21559 | 1.000046              | 2.370257                                                         |
| 21561 | 1.333519              | 2.370264                                                         |
| 21563 | 1.000046              | 2.370271                                                         |
| 21565 | 1.268722              | 2.370278                                                         |
| 21567 | 1.661798              | 2.370285                                                         |
| 21569 | 1.000046              | 2.370292                                                         |
| 21571 | 1.141533              | 2.370299                                                         |
| 21573 | 1.602003              | 2.370306                                                         |

| $n$   | $\frac{\sigma(n)}{n}$ | $\frac{e^\gamma}{2} \log \log n + \frac{0.73...}{\log \log n}$ |
|-------|-----------------------|----------------------------------------------------------------|
| 21575 | 1.241437              | 2.370313                                                       |
| 21577 | 1.000046              | 2.370320                                                       |
| 21579 | 1.333519              | 2.370327                                                       |
| 21581 | 1.143228              | 2.370334                                                       |
| 21583 | 1.014131              | 2.370341                                                       |
| 21585 | 1.601112              | 2.370348                                                       |
| 21587 | 1.000046              | 2.370355                                                       |
| 21589 | 1.000046              | 2.370362                                                       |
| 21591 | 1.445047              | 2.370369                                                       |
| 21593 | 1.182605              | 2.370376                                                       |
| 21595 | 1.373651              | 2.370383                                                       |
| 21597 | 1.395749              | 2.370390                                                       |
| 21599 | 1.000046              | 2.370397                                                       |
| 21601 | 1.000046              | 2.370404                                                       |
| 21603 | 1.407212              | 2.370411                                                       |
| 21605 | 1.249711              | 2.370418                                                       |
| 21607 | 1.119637              | 2.370425                                                       |
| 21609 | 1.685085              | 2.370432                                                       |
| 21611 | 1.000046              | 2.370439                                                       |
| 21613 | 1.000046              | 2.370446                                                       |
| 21615 | 1.758779              | 2.370453                                                       |
| 21617 | 1.000046              | 2.370460                                                       |
| 21619 | 1.077571              | 2.370467                                                       |
| 21621 | 1.333518              | 2.370473                                                       |
| 21623 | 1.143227              | 2.370480                                                       |
| 21625 | 1.255214              | 2.370487                                                       |
| 21627 | 1.514773              | 2.370494                                                       |
| 21629 | 1.025290              | 2.370501                                                       |
| 21631 | 1.014840              | 2.370508                                                       |
| 21633 | 1.333518              | 2.370515                                                       |
| 21635 | 1.200277              | 2.370522                                                       |
| 21637 | 1.251190              | 2.370529                                                       |
| 21639 | 1.333518              | 2.370536                                                       |
| 21641 | 1.131186              | 2.370543                                                       |
| 21643 | 1.044587              | 2.370550                                                       |
| 21645 | 1.917117              | 2.370557                                                       |
| 21647 | 1.000046              | 2.370564                                                       |
| 21649 | 1.000046              | 2.370571                                                       |
| 21651 | 1.525288              | 2.370578                                                       |
| 21653 | 1.019720              | 2.370585                                                       |
| 21655 | 1.236851              | 2.370592                                                       |
| 21657 | 1.333518              | 2.370599                                                       |
| 21659 | 1.105314              | 2.370606                                                       |
| 21661 | 1.000046              | 2.370613                                                       |

| $n$   | $\frac{\sigma(n)}{n}$ | $\frac{e^\gamma}{2} \log \log n + \frac{0.73\dots}{\log \log n}$ |
|-------|-----------------------|------------------------------------------------------------------|
| 21663 | 1.512256              | 2.370619                                                         |
| 21665 | 1.373644              | 2.370626                                                         |
| 21667 | 1.023492              | 2.370633                                                         |
| 21669 | 1.382251              | 2.370640                                                         |
| 21671 | 1.077569              | 2.370647                                                         |
| 21673 | 1.000046              | 2.370654                                                         |
| 21675 | 1.756309              | 2.370661                                                         |
| 21677 | 1.021359              | 2.370668                                                         |
| 21679 | 1.210388              | 2.370675                                                         |
| 21681 | 1.638301              | 2.370682                                                         |
| 21683 | 1.000046              | 2.370689                                                         |
| 21685 | 1.200277              | 2.370696                                                         |
| 21687 | 1.333518              | 2.370703                                                         |
| 21689 | 1.070865              | 2.370710                                                         |
| 21691 | 1.014246              | 2.370717                                                         |
| 21693 | 1.525285              | 2.370724                                                         |
| 21695 | 1.200277              | 2.370730                                                         |
| 21697 | 1.077568              | 2.370737                                                         |
| 21699 | 1.445044              | 2.370744                                                         |
| 21701 | 1.000046              | 2.370751                                                         |
| 21703 | 1.091462              | 2.370758                                                         |
| 21705 | 1.601106              | 2.370765                                                         |
| 21707 | 1.165891              | 2.370772                                                         |
| 21709 | 1.059653              | 2.370779                                                         |
| 21711 | 1.333518              | 2.370786                                                         |
| 21713 | 1.000046              | 2.370793                                                         |
| 21715 | 1.240064              | 2.370800                                                         |
| 21717 | 1.532440              | 2.370807                                                         |
| 21719 | 1.028777              | 2.370814                                                         |
| 21721 | 1.193315              | 2.370821                                                         |
| 21723 | 1.438475              | 2.370827                                                         |
| 21725 | 1.369850              | 2.370834                                                         |
| 21727 | 1.000046              | 2.370841                                                         |
| 21729 | 1.333517              | 2.370848                                                         |
| 21731 | 1.033731              | 2.370855                                                         |
| 21733 | 1.014494              | 2.370862                                                         |
| 21735 | 2.120083              | 2.370869                                                         |
| 21737 | 1.000046              | 2.370876                                                         |
| 21739 | 1.000046              | 2.370883                                                         |
| 21741 | 1.333517              | 2.370890                                                         |
| 21743 | 1.059651              | 2.370897                                                         |
| 21745 | 1.200276              | 2.370904                                                         |
| 21747 | 1.456753              | 2.370910                                                         |
| 21749 | 1.235919              | 2.370917                                                         |

| $n$   | $\frac{\sigma(n)}{n}$ | $\frac{e^\gamma}{2} \log \log n + \frac{0.73...}{\log \log n}$ |
|-------|-----------------------|----------------------------------------------------------------|
| 21751 | 1.000046              | 2.370924                                                       |
| 21753 | 1.445042              | 2.370931                                                       |
| 21755 | 1.268674              | 2.370938                                                       |
| 21757 | 1.000046              | 2.370945                                                       |
| 21759 | 1.333517              | 2.370952                                                       |
| 21761 | 1.023482              | 2.370959                                                       |
| 21763 | 1.143225              | 2.370966                                                       |
| 21765 | 1.601103              | 2.370973                                                       |
| 21767 | 1.000046              | 2.370980                                                       |
| 21769 | 1.091460              | 2.370986                                                       |
| 21771 | 1.504754              | 2.370993                                                       |
| 21773 | 1.000046              | 2.371000                                                       |
| 21775 | 1.355316              | 2.371007                                                       |
| 21777 | 1.639895              | 2.371014                                                       |
| 21779 | 1.035860              | 2.371021                                                       |
| 21781 | 1.044580              | 2.371028                                                       |
| 21783 | 1.368407              | 2.371035                                                       |
| 21785 | 1.200275              | 2.371042                                                       |
| 21787 | 1.000046              | 2.371049                                                       |
| 21789 | 1.499380              | 2.371055                                                       |
| 21791 | 1.251159              | 2.371062                                                       |
| 21793 | 1.115955              | 2.371069                                                       |
| 21795 | 1.601101              | 2.371076                                                       |
| 21797 | 1.017388              | 2.371083                                                       |
| 21799 | 1.000046              | 2.371090                                                       |
| 21801 | 1.477363              | 2.371097                                                       |
| 21803 | 1.000046              | 2.371104                                                       |
| 21805 | 1.411603              | 2.371111                                                       |
| 21807 | 1.445041              | 2.371118                                                       |
| 21809 | 1.014077              | 2.371124                                                       |
| 21811 | 1.059649              | 2.371131                                                       |
| 21813 | 1.456746              | 2.371138                                                       |
| 21815 | 1.200275              | 2.371145                                                       |
| 21817 | 1.000046              | 2.371152                                                       |
| 21819 | 1.525276              | 2.371159                                                       |
| 21821 | 1.000046              | 2.371166                                                       |
| 21823 | 1.013609              | 2.371173                                                       |
| 21825 | 1.809576              | 2.371180                                                       |
| 21827 | 1.139140              | 2.371186                                                       |
| 21829 | 1.015896              | 2.371193                                                       |
| 21831 | 1.407173              | 2.371200                                                       |
| 21833 | 1.143224              | 2.371207                                                       |
| 21835 | 1.312388              | 2.371214                                                       |
| 21837 | 1.384806              | 2.371221                                                       |

| $n$   | $\frac{\sigma(n)}{n}$ | $\frac{e^\gamma}{2} \log \log n + \frac{0.73...}{\log \log n}$ |
|-------|-----------------------|----------------------------------------------------------------|
| 21839 | 1.000046              | 2.371228                                                       |
| 21841 | 1.000046              | 2.371235                                                       |
| 21843 | 1.483313              | 2.371242                                                       |
| 21845 | 1.275532              | 2.371248                                                       |
| 21847 | 1.143223              | 2.371255                                                       |
| 21849 | 1.333516              | 2.371262                                                       |
| 21851 | 1.000046              | 2.371269                                                       |
| 21853 | 1.103830              | 2.371276                                                       |
| 21855 | 1.686754              | 2.371283                                                       |
| 21857 | 1.091458              | 2.371290                                                       |
| 21859 | 1.000046              | 2.371297                                                       |
| 21861 | 1.655551              | 2.371303                                                       |
| 21863 | 1.000046              | 2.371310                                                       |
| 21865 | 1.200274              | 2.371317                                                       |
| 21867 | 1.376320              | 2.371324                                                       |
| 21869 | 1.053546              | 2.371331                                                       |
| 21871 | 1.000046              | 2.371338                                                       |
| 21873 | 1.395693              | 2.371345                                                       |
| 21875 | 1.428480              | 2.371352                                                       |
| 21877 | 1.013667              | 2.371358                                                       |
| 21879 | 1.796791              | 2.371365                                                       |
| 21881 | 1.000046              | 2.371372                                                       |
| 21883 | 1.016314              | 2.371379                                                       |
| 21885 | 1.601097              | 2.371386                                                       |
| 21887 | 1.025266              | 2.371393                                                       |
| 21889 | 1.184156              | 2.371400                                                       |
| 21891 | 1.333516              | 2.371406                                                       |
| 21893 | 1.000046              | 2.371413                                                       |
| 21895 | 1.249600              | 2.371420                                                       |
| 21897 | 1.483308              | 2.371427                                                       |
| 21899 | 1.019225              | 2.371434                                                       |
| 21901 | 1.105246              | 2.371441                                                       |
| 21903 | 1.561430              | 2.371448                                                       |
| 21905 | 1.296142              | 2.371455                                                       |
| 21907 | 1.053545              | 2.371461                                                       |
| 21909 | 1.365649              | 2.371468                                                       |
| 21911 | 1.000046              | 2.371475                                                       |
| 21913 | 1.059645              | 2.371482                                                       |
| 21915 | 1.736893              | 2.371489                                                       |
| 21917 | 1.191404              | 2.371496                                                       |
| 21919 | 1.044573              | 2.371503                                                       |
| 21921 | 1.333516              | 2.371509                                                       |
| 21923 | 1.091456              | 2.371516                                                       |
| 21925 | 1.241414              | 2.371523                                                       |

| $n$   | $\frac{\sigma(n)}{n}$ | $\frac{e^\gamma}{2} \log \log n + \frac{0.73...}{\log \log n}$ |
|-------|-----------------------|----------------------------------------------------------------|
| 21927 | 1.333516              | 2.371530                                                       |
| 21929 | 1.000046              | 2.371537                                                       |
| 21931 | 1.235876              | 2.371544                                                       |
| 21933 | 1.445037              | 2.371550                                                       |
| 21935 | 1.240757              | 2.371557                                                       |
| 21937 | 1.000046              | 2.371564                                                       |
| 21939 | 1.365240              | 2.371571                                                       |
| 21941 | 1.028759              | 2.371578                                                       |
| 21943 | 1.000046              | 2.371585                                                       |
| 21945 | 2.099795              | 2.371592                                                       |
| 21947 | 1.059644              | 2.371598                                                       |
| 21949 | 1.023463              | 2.371605                                                       |
| 21951 | 1.499339              | 2.371612                                                       |
| 21953 | 1.035849              | 2.371619                                                       |
| 21955 | 1.200273              | 2.371626                                                       |
| 21957 | 1.438448              | 2.371633                                                       |
| 21959 | 1.143221              | 2.371639                                                       |
| 21961 | 1.000046              | 2.371646                                                       |
| 21963 | 1.333515              | 2.371653                                                       |
| 21965 | 1.258730              | 2.371660                                                       |
| 21967 | 1.091455              | 2.371667                                                       |
| 21969 | 1.445036              | 2.371674                                                       |
| 21971 | 1.013700              | 2.371681                                                       |
| 21973 | 1.185455              | 2.371687                                                       |
| 21975 | 1.658976              | 2.371694                                                       |
| 21977 | 1.000046              | 2.371701                                                       |
| 21979 | 1.033714              | 2.371708                                                       |
| 21981 | 1.415040              | 2.371715                                                       |
| 21983 | 1.146340              | 2.371722                                                       |
| 21985 | 1.200273              | 2.371728                                                       |
| 21987 | 1.655524              | 2.371735                                                       |
| 21989 | 1.091455              | 2.371742                                                       |
| 21991 | 1.000045              | 2.371749                                                       |
| 21993 | 1.333515              | 2.371756                                                       |
| 21995 | 1.237372              | 2.371763                                                       |
| 21997 | 1.000045              | 2.371769                                                       |
| 21999 | 1.333515              | 2.371776                                                       |
| 22001 | 1.165856              | 2.371783                                                       |
| 22003 | 1.000045              | 2.371790                                                       |
| 22005 | 1.788684              | 2.371797                                                       |
| 22007 | 1.019676              | 2.371803                                                       |
| 22009 | 1.077559              | 2.371810                                                       |
| 22011 | 1.570124              | 2.371817                                                       |
| 22013 | 1.000045              | 2.371824                                                       |



| $n$   | $\frac{\sigma(n)}{n}$ | $\frac{e^\gamma}{2} \log \log n + \frac{0.73\dots}{\log \log n}$ |
|-------|-----------------------|------------------------------------------------------------------|
| 22015 | 1.491347              | 2.371831                                                         |
| 22017 | 1.373484              | 2.371838                                                         |
| 22019 | 1.014760              | 2.371844                                                         |
| 22021 | 1.072703              | 2.371851                                                         |
| 22023 | 1.445035              | 2.371858                                                         |
| 22025 | 1.241407              | 2.371865                                                         |
| 22027 | 1.000045              | 2.371872                                                         |
| 22029 | 1.525262              | 2.371879                                                         |
| 22031 | 1.000045              | 2.371885                                                         |
| 22033 | 1.091454              | 2.371892                                                         |
| 22035 | 1.738325              | 2.371899                                                         |
| 22037 | 1.000045              | 2.371906                                                         |
| 22039 | 1.000045              | 2.371913                                                         |
| 22041 | 1.509913              | 2.371919                                                         |
| 22043 | 1.184594              | 2.371926                                                         |
| 22045 | 1.200272              | 2.371933                                                         |
| 22047 | 1.333515              | 2.371940                                                         |
| 22049 | 1.059640              | 2.371947                                                         |
| 22051 | 1.000045              | 2.371953                                                         |
| 22053 | 1.333515              | 2.371960                                                         |
| 22055 | 1.312355              | 2.371967                                                         |
| 22057 | 1.201251              | 2.371974                                                         |
| 22059 | 1.595721              | 2.371981                                                         |
| 22061 | 1.077558              | 2.371988                                                         |
| 22063 | 1.000045              | 2.371994                                                         |
| 22065 | 1.601088              | 2.372001                                                         |
| 22067 | 1.000045              | 2.372008                                                         |
| 22069 | 1.035842              | 2.372015                                                         |
| 22071 | 1.525259              | 2.372022                                                         |
| 22073 | 1.000045              | 2.372028                                                         |
| 22075 | 1.241404              | 2.372035                                                         |
| 22077 | 1.582824              | 2.372042                                                         |
| 22079 | 1.000045              | 2.372049                                                         |
| 22081 | 1.017345              | 2.372056                                                         |
| 22083 | 1.415025              | 2.372062                                                         |
| 22085 | 1.373602              | 2.372069                                                         |
| 22087 | 1.077557              | 2.372076                                                         |
| 22089 | 1.376251              | 2.372083                                                         |
| 22091 | 1.000045              | 2.372090                                                         |
| 22093 | 1.000045              | 2.372096                                                         |
| 22095 | 1.736864              | 2.372103                                                         |
| 22097 | 1.053537              | 2.372110                                                         |
| 22099 | 1.299968              | 2.372117                                                         |
| 22101 | 1.368264              | 2.372124                                                         |

| $n$   | $\frac{\sigma(n)}{n}$ | $\frac{e^\gamma}{2} \log \log n + \frac{0.73...}{\log \log n}$ |
|-------|-----------------------|----------------------------------------------------------------|
| 22103 | 1.078225              | 2.372130                                                       |
| 22105 | 1.200271              | 2.372137                                                       |
| 22107 | 1.333514              | 2.372144                                                       |
| 22109 | 1.000045              | 2.372151                                                       |
| 22111 | 1.000045              | 2.372158                                                       |
| 22113 | 1.843621              | 2.372164                                                       |
| 22115 | 1.200271              | 2.372171                                                       |
| 22117 | 1.059637              | 2.372178                                                       |
| 22119 | 1.364980              | 2.372185                                                       |
| 22121 | 1.091452              | 2.372191                                                       |
| 22123 | 1.000045              | 2.372198                                                       |
| 22125 | 1.692203              | 2.372205                                                       |
| 22127 | 1.193112              | 2.372212                                                       |
| 22129 | 1.000045              | 2.372219                                                       |
| 22131 | 1.445032              | 2.372225                                                       |
| 22133 | 1.000045              | 2.372232                                                       |
| 22135 | 1.268579              | 2.372239                                                       |
| 22137 | 1.370375              | 2.372246                                                       |
| 22139 | 1.091106              | 2.372253                                                       |
| 22141 | 1.143218              | 2.372259                                                       |
| 22143 | 1.489590              | 2.372266                                                       |
| 22145 | 1.239828              | 2.372273                                                       |
| 22147 | 1.000045              | 2.372280                                                       |
| 22149 | 1.521333              | 2.372286                                                       |
| 22151 | 1.059636              | 2.372293                                                       |
| 22153 | 1.000045              | 2.372300                                                       |
| 22155 | 1.837238              | 2.372307                                                       |
| 22157 | 1.000045              | 2.372314                                                       |
| 22159 | 1.000045              | 2.372320                                                       |
| 22161 | 1.364559              | 2.372327                                                       |
| 22163 | 1.028742              | 2.372334                                                       |
| 22165 | 1.455267              | 2.372341                                                       |
| 22167 | 1.483286              | 2.372347                                                       |
| 22169 | 1.143218              | 2.372354                                                       |
| 22171 | 1.000045              | 2.372361                                                       |
| 22173 | 1.407117              | 2.372368                                                       |
| 22175 | 1.241398              | 2.372374                                                       |
| 22177 | 1.017992              | 2.372381                                                       |
| 22179 | 1.333514              | 2.372388                                                       |
| 22181 | 1.026284              | 2.372395                                                       |
| 22183 | 1.143218              | 2.372402                                                       |
| 22185 | 1.898580              | 2.372408                                                       |
| 22187 | 1.091450              | 2.372415                                                       |
| 22189 | 1.000045              | 2.372422                                                       |

| $n$   | $\frac{\sigma(n)}{n}$ | $\frac{e^\gamma}{2} \log \log n + \frac{0.73...}{\log \log n}$ |
|-------|-----------------------|----------------------------------------------------------------|
| 22191 | 1.438421              | 2.372429                                                       |
| 22193 | 1.000045              | 2.372435                                                       |
| 22195 | 1.258662              | 2.372442                                                       |
| 22197 | 1.561292              | 2.372449                                                       |
| 22199 | 1.016262              | 2.372456                                                       |
| 22201 | 1.006756              | 2.372462                                                       |
| 22203 | 1.445030              | 2.372469                                                       |
| 22205 | 1.200270              | 2.372476                                                       |
| 22207 | 1.021300              | 2.372483                                                       |
| 22209 | 1.456707              | 2.372489                                                       |
| 22211 | 1.210211              | 2.372496                                                       |
| 22213 | 1.014721              | 2.372503                                                       |
| 22215 | 1.601080              | 2.372510                                                       |
| 22217 | 1.077553              | 2.372516                                                       |
| 22219 | 1.059634              | 2.372523                                                       |
| 22221 | 1.483282              | 2.372530                                                       |
| 22223 | 1.017324              | 2.372537                                                       |
| 22225 | 1.428301              | 2.372543                                                       |
| 22227 | 1.382103              | 2.372550                                                       |
| 22229 | 1.000045              | 2.372557                                                       |
| 22231 | 1.140030              | 2.372564                                                       |
| 22233 | 1.333513              | 2.372571                                                       |
| 22235 | 1.200270              | 2.372577                                                       |
| 22237 | 1.028736              | 2.372584                                                       |
| 22239 | 1.655470              | 2.372591                                                       |
| 22241 | 1.044557              | 2.372597                                                       |
| 22243 | 1.132941              | 2.372604                                                       |
| 22245 | 1.601079              | 2.372611                                                       |
| 22247 | 1.000045              | 2.372618                                                       |
| 22249 | 1.053530              | 2.372624                                                       |
| 22251 | 1.333513              | 2.372631                                                       |
| 22253 | 1.324406              | 2.372638                                                       |
| 22255 | 1.200270              | 2.372645                                                       |
| 22257 | 1.445029              | 2.372651                                                       |
| 22259 | 1.000045              | 2.372658                                                       |
| 22261 | 1.013971              | 2.372665                                                       |
| 22263 | 1.373400              | 2.372672                                                       |
| 22265 | 1.236380              | 2.372678                                                       |
| 22267 | 1.143216              | 2.372685                                                       |
| 22269 | 1.438412              | 2.372692                                                       |
| 22271 | 1.000045              | 2.372699                                                       |
| 22273 | 1.000045              | 2.372705                                                       |
| 22275 | 2.020741              | 2.372712                                                       |
| 22277 | 1.000045              | 2.372719                                                       |

| $n$   | $\frac{\sigma(n)}{n}$ | $\frac{e^\gamma}{2} \log \log n + \frac{0.73\dots}{\log \log n}$ |
|-------|-----------------------|------------------------------------------------------------------|
| 22279 | 1.000045              | 2.372726                                                         |
| 22281 | 1.525246              | 2.372732                                                         |
| 22283 | 1.000045              | 2.372739                                                         |
| 22285 | 1.200269              | 2.372746                                                         |
| 22287 | 1.550680              | 2.372753                                                         |
| 22289 | 1.033694              | 2.372759                                                         |
| 22291 | 1.000045              | 2.372766                                                         |
| 22293 | 1.445028              | 2.372773                                                         |
| 22295 | 1.507064              | 2.372779                                                         |
| 22297 | 1.091447              | 2.372786                                                         |
| 22299 | 1.333513              | 2.372793                                                         |
| 22301 | 1.035828              | 2.372800                                                         |
| 22303 | 1.000045              | 2.372806                                                         |
| 22305 | 1.601076              | 2.372813                                                         |
| 22307 | 1.000045              | 2.372820                                                         |
| 22309 | 1.143216              | 2.372827                                                         |
| 22311 | 1.505625              | 2.372833                                                         |
| 22313 | 1.021288              | 2.372840                                                         |
| 22315 | 1.200269              | 2.372847                                                         |
| 22317 | 1.372227              | 2.372853                                                         |
| 22319 | 1.091447              | 2.372860                                                         |
| 22321 | 1.151561              | 2.372867                                                         |
| 22323 | 1.525243              | 2.372874                                                         |
| 22325 | 1.333035              | 2.372880                                                         |
| 22327 | 1.015810              | 2.372887                                                         |
| 22329 | 1.483273              | 2.372894                                                         |
| 22331 | 1.013479              | 2.372900                                                         |
| 22333 | 1.044553              | 2.372907                                                         |
| 22335 | 1.601075              | 2.372914                                                         |
| 22337 | 1.143215              | 2.372921                                                         |
| 22339 | 1.015265              | 2.372927                                                         |
| 22341 | 1.456694              | 2.372934                                                         |
| 22343 | 1.000045              | 2.372941                                                         |
| 22345 | 1.240546              | 2.372947                                                         |
| 22347 | 1.563700              | 2.372954                                                         |
| 22349 | 1.000045              | 2.372961                                                         |
| 22351 | 1.191177              | 2.372968                                                         |
| 22353 | 1.333512              | 2.372974                                                         |
| 22355 | 1.275419              | 2.372981                                                         |
| 22357 | 1.016237              | 2.372988                                                         |
| 22359 | 1.384677              | 2.372994                                                         |
| 22361 | 1.019632              | 2.373001                                                         |
| 22363 | 1.159057              | 2.373008                                                         |
| 22365 | 2.008853              | 2.373015                                                         |

| $n$   | $\frac{\sigma(n)}{n}$ | $\frac{e^\gamma}{2} \log \log n + \frac{0.73...}{\log \log n}$ |
|-------|-----------------------|----------------------------------------------------------------|
| 22367 | 1.000045              | 2.373021                                                       |
| 22369 | 1.000045              | 2.373028                                                       |
| 22371 | 1.333512              | 2.373035                                                       |
| 22373 | 1.077549              | 2.373041                                                       |
| 22375 | 1.254972              | 2.373048                                                       |
| 22377 | 1.333512              | 2.373055                                                       |
| 22379 | 1.201126              | 2.373062                                                       |
| 22381 | 1.000045              | 2.373068                                                       |
| 22383 | 1.483269              | 2.373075                                                       |
| 22385 | 1.354657              | 2.373082                                                       |
| 22387 | 1.019163              | 2.373088                                                       |
| 22389 | 1.414981              | 2.373095                                                       |
| 22391 | 1.000045              | 2.373102                                                       |
| 22393 | 1.165811              | 2.373108                                                       |
| 22395 | 1.601072              | 2.373115                                                       |
| 22397 | 1.000045              | 2.373122                                                       |
| 22399 | 1.077548              | 2.373129                                                       |
| 22401 | 1.532074              | 2.373135                                                       |
| 22403 | 1.025220              | 2.373142                                                       |
| 22405 | 1.200268              | 2.373149                                                       |
| 22407 | 1.679475              | 2.373155                                                       |
| 22409 | 1.000045              | 2.373162                                                       |
| 22411 | 1.017001              | 2.373169                                                       |
| 22413 | 1.382055              | 2.373175                                                       |
| 22415 | 1.200268              | 2.373182                                                       |
| 22417 | 1.035821              | 2.373189                                                       |
| 22419 | 1.503011              | 2.373195                                                       |
| 22421 | 1.143214              | 2.373202                                                       |
| 22423 | 1.059626              | 2.373209                                                       |
| 22425 | 1.857926              | 2.373216                                                       |
| 22427 | 1.026263              | 2.373222                                                       |
| 22429 | 1.091444              | 2.373229                                                       |
| 22431 | 1.333512              | 2.373236                                                       |
| 22433 | 1.000045              | 2.373242                                                       |
| 22435 | 1.373568              | 2.373249                                                       |
| 22437 | 1.499220              | 2.373256                                                       |
| 22439 | 1.053523              | 2.373262                                                       |
| 22441 | 1.000045              | 2.373269                                                       |
| 22443 | 1.333512              | 2.373276                                                       |
| 22445 | 1.218178              | 2.373282                                                       |
| 22447 | 1.000045              | 2.373289                                                       |
| 22449 | 1.525235              | 2.373296                                                       |
| 22451 | 1.182308              | 2.373302                                                       |
| 22453 | 1.000045              | 2.373309                                                       |

| $n$   | $\frac{\sigma(n)}{n}$ | $\frac{e^\gamma}{2} \log \log n + \frac{0.73\dots}{\log \log n}$ |
|-------|-----------------------|------------------------------------------------------------------|
| 22455 | 1.736807              | 2.373316                                                         |
| 22457 | 1.059625              | 2.373322                                                         |
| 22459 | 1.028719              | 2.373329                                                         |
| 22461 | 1.333511              | 2.373336                                                         |
| 22463 | 1.143213              | 2.373342                                                         |
| 22465 | 1.200267              | 2.373349                                                         |
| 22467 | 1.333511              | 2.373356                                                         |
| 22469 | 1.000045              | 2.373362                                                         |
| 22471 | 1.044546              | 2.373369                                                         |
| 22473 | 1.582699              | 2.373376                                                         |
| 22475 | 1.324138              | 2.373383                                                         |
| 22477 | 1.302665              | 2.373389                                                         |
| 22479 | 1.366609              | 2.373396                                                         |
| 22481 | 1.000044              | 2.373403                                                         |
| 22483 | 1.000044              | 2.373409                                                         |
| 22485 | 1.601067              | 2.373416                                                         |
| 22487 | 1.013919              | 2.373423                                                         |
| 22489 | 1.025212              | 2.373429                                                         |
| 22491 | 1.824730              | 2.373436                                                         |
| 22493 | 1.015783              | 2.373443                                                         |
| 22495 | 1.312292              | 2.373449                                                         |
| 22497 | 1.333511              | 2.373456                                                         |
| 22499 | 1.013378              | 2.373463                                                         |
| 22501 | 1.000044              | 2.373469                                                         |
| 22503 | 1.438386              | 2.373476                                                         |
| 22505 | 1.373561              | 2.373483                                                         |
| 22507 | 1.017284              | 2.373489                                                         |
| 22509 | 1.503932              | 2.373496                                                         |
| 22511 | 1.000044              | 2.373502                                                         |
| 22513 | 1.023409              | 2.373509                                                         |
| 22515 | 1.705530              | 2.373516                                                         |
| 22517 | 1.151130              | 2.373522                                                         |
| 22519 | 1.143212              | 2.373529                                                         |
| 22521 | 1.333511              | 2.373536                                                         |
| 22523 | 1.014430              | 2.373542                                                         |
| 22525 | 1.337714              | 2.373549                                                         |
| 22527 | 1.445022              | 2.373556                                                         |
| 22529 | 1.077544              | 2.373562                                                         |
| 22531 | 1.000044              | 2.373569                                                         |
| 22533 | 1.618959              | 2.373576                                                         |
| 22535 | 1.200266              | 2.373582                                                         |
| 22537 | 1.033678              | 2.373589                                                         |
| 22539 | 1.456675              | 2.373596                                                         |
| 22541 | 1.000044              | 2.373602                                                         |

| $n$   | $\frac{\sigma(n)}{n}$ | $\frac{e^\gamma}{2} \log \log n + \frac{0.73...}{\log \log n}$ |
|-------|-----------------------|----------------------------------------------------------------|
| 22543 | 1.000044              | 2.373609                                                       |
| 22545 | 1.788423              | 2.373616                                                       |
| 22547 | 1.143212              | 2.373622                                                       |
| 22549 | 1.000044              | 2.373629                                                       |
| 22551 | 1.333511              | 2.373636                                                       |
| 22553 | 1.053518              | 2.373642                                                       |
| 22555 | 1.296032              | 2.373649                                                       |
| 22557 | 1.364720              | 2.373655                                                       |
| 22559 | 1.059621              | 2.373662                                                       |
| 22561 | 1.251008              | 2.373669                                                       |
| 22563 | 1.521074              | 2.373675                                                       |
| 22565 | 1.200266              | 2.373682                                                       |
| 22567 | 1.000044              | 2.373689                                                       |
| 22569 | 1.333511              | 2.373695                                                       |
| 22571 | 1.000044              | 2.373702                                                       |
| 22573 | 1.000044              | 2.373709                                                       |
| 22575 | 1.933466              | 2.373715                                                       |
| 22577 | 1.014129              | 2.373722                                                       |
| 22579 | 1.017937              | 2.373729                                                       |
| 22581 | 1.563615              | 2.373735                                                       |
| 22583 | 1.091440              | 2.373742                                                       |
| 22585 | 1.200266              | 2.373748                                                       |
| 22587 | 1.333510              | 2.373755                                                       |
| 22589 | 1.165789              | 2.373762                                                       |
| 22591 | 1.115488              | 2.373768                                                       |
| 22593 | 1.414952              | 2.373775                                                       |
| 22595 | 1.200266              | 2.373782                                                       |
| 22597 | 1.019604              | 2.373788                                                       |
| 22599 | 1.547679              | 2.373795                                                       |
| 22601 | 1.014645              | 2.373802                                                       |
| 22603 | 1.143211              | 2.373808                                                       |
| 22605 | 1.758195              | 2.373815                                                       |
| 22607 | 1.129562              | 2.373821                                                       |
| 22609 | 1.044540              | 2.373828                                                       |
| 22611 | 1.333510              | 2.373835                                                       |
| 22613 | 1.000044              | 2.373841                                                       |
| 22615 | 1.200265              | 2.373848                                                       |
| 22617 | 1.655392              | 2.373855                                                       |
| 22619 | 1.000044              | 2.373861                                                       |
| 22621 | 1.000044              | 2.373868                                                       |
| 22623 | 1.333510              | 2.373874                                                       |
| 22625 | 1.254895              | 2.373881                                                       |
| 22627 | 1.164626              | 2.373888                                                       |
| 22629 | 1.407044              | 2.373894                                                       |

| $n$   | $\frac{\sigma(n)}{n}$ | $\frac{e^\gamma}{2} \log \log n + \frac{0.73...}{\log \log n}$ |
|-------|-----------------------|----------------------------------------------------------------|
| 22631 | 1.183509              | 2.373901                                                       |
| 22633 | 1.077542              | 2.373908                                                       |
| 22635 | 1.736779              | 2.373914                                                       |
| 22637 | 1.000044              | 2.373921                                                       |
| 22639 | 1.000044              | 2.373927                                                       |
| 22641 | 1.333510              | 2.373934                                                       |
| 22643 | 1.000044              | 2.373941                                                       |
| 22645 | 1.373548              | 2.373947                                                       |
| 22647 | 1.333510              | 2.373954                                                       |
| 22649 | 1.144421              | 2.373961                                                       |
| 22651 | 1.000044              | 2.373967                                                       |
| 22653 | 1.483247              | 2.373974                                                       |
| 22655 | 1.258530              | 2.373980                                                       |
| 22657 | 1.013373              | 2.373987                                                       |
| 22659 | 1.660797              | 2.373994                                                       |
| 22661 | 1.118397              | 2.374000                                                       |
| 22663 | 1.013458              | 2.374007                                                       |
| 22665 | 1.601059              | 2.374013                                                       |
| 22667 | 1.053514              | 2.374020                                                       |
| 22669 | 1.000044              | 2.374027                                                       |
| 22671 | 1.582639              | 2.374033                                                       |
| 22673 | 1.185551              | 2.374040                                                       |
| 22675 | 1.241367              | 2.374046                                                       |
| 22677 | 1.333510              | 2.374053                                                       |
| 22679 | 1.000044              | 2.374060                                                       |
| 22681 | 1.028702              | 2.374066                                                       |
| 22683 | 1.333510              | 2.374073                                                       |
| 22685 | 1.296011              | 2.374079                                                       |
| 22687 | 1.165778              | 2.374086                                                       |
| 22689 | 1.445017              | 2.374093                                                       |
| 22691 | 1.000044              | 2.374099                                                       |
| 22693 | 1.091438              | 2.374106                                                       |
| 22695 | 1.713153              | 2.374113                                                       |
| 22697 | 1.000044              | 2.374119                                                       |
| 22699 | 1.000044              | 2.374126                                                       |
| 22701 | 1.623893              | 2.374132                                                       |
| 22703 | 1.016958              | 2.374139                                                       |
| 22705 | 1.268443              | 2.374146                                                       |
| 22707 | 1.534329              | 2.374152                                                       |
| 22709 | 1.000044              | 2.374159                                                       |
| 22711 | 1.077540              | 2.374165                                                       |
| 22713 | 1.365209              | 2.374172                                                       |
| 22715 | 1.521462              | 2.374178                                                       |
| 22717 | 1.000044              | 2.374185                                                       |



| $n$   | $\frac{\sigma(n)}{n}$ | $\frac{e^\gamma}{2} \log \log n + \frac{0.73\dots}{\log \log n}$ |
|-------|-----------------------|------------------------------------------------------------------|
| 22719 | 1.333509              | 2.374192                                                         |
| 22721 | 1.000044              | 2.374198                                                         |
| 22723 | 1.033666              | 2.374205                                                         |
| 22725 | 1.808845              | 2.374211                                                         |
| 22727 | 1.000044              | 2.374218                                                         |
| 22729 | 1.216420              | 2.374225                                                         |
| 22731 | 1.333509              | 2.374231                                                         |
| 22733 | 1.013505              | 2.374238                                                         |
| 22735 | 1.200264              | 2.374244                                                         |
| 22737 | 1.595989              | 2.374251                                                         |
| 22739 | 1.000044              | 2.374258                                                         |
| 22741 | 1.000044              | 2.374264                                                         |
| 22743 | 1.742250              | 2.374271                                                         |
| 22745 | 1.200264              | 2.374277                                                         |
| 22747 | 1.069680              | 2.374284                                                         |
| 22749 | 1.333509              | 2.374291                                                         |
| 22751 | 1.000044              | 2.374297                                                         |
| 22753 | 1.019118              | 2.374304                                                         |
| 22755 | 1.683322              | 2.374310                                                         |
| 22757 | 1.143209              | 2.374317                                                         |
| 22759 | 1.091436              | 2.374323                                                         |
| 22761 | 1.499143              | 2.374330                                                         |
| 22763 | 1.151342              | 2.374337                                                         |
| 22765 | 1.249286              | 2.374343                                                         |
| 22767 | 1.333509              | 2.374350                                                         |
| 22769 | 1.000044              | 2.374356                                                         |
| 22771 | 1.143208              | 2.374363                                                         |
| 22773 | 1.333509              | 2.374369                                                         |
| 22775 | 1.241361              | 2.374376                                                         |
| 22777 | 1.000044              | 2.374383                                                         |
| 22779 | 1.445015              | 2.374389                                                         |
| 22781 | 1.158860              | 2.374396                                                         |
| 22783 | 1.000044              | 2.374402                                                         |
| 22785 | 1.921264              | 2.374409                                                         |
| 22787 | 1.000044              | 2.374416                                                         |
| 22789 | 1.077537              | 2.374422                                                         |
| 22791 | 1.364749              | 2.374429                                                         |
| 22793 | 1.044531              | 2.374435                                                         |
| 22795 | 1.238166              | 2.374442                                                         |
| 22797 | 1.539676              | 2.374448                                                         |
| 22799 | 1.143208              | 2.374455                                                         |
| 22801 | 1.006666              | 2.374462                                                         |
| 22803 | 1.456650              | 2.374468                                                         |
| 22805 | 1.200263              | 2.374475                                                         |

| $n$   | $\frac{\sigma(n)}{n}$ | $\frac{e^\gamma}{2} \log \log n + \frac{0.73...}{\log \log n}$ |
|-------|-----------------------|----------------------------------------------------------------|
| 22807 | 1.000044              | 2.374481                                                       |
| 22809 | 1.333509              | 2.374488                                                       |
| 22811 | 1.000044              | 2.374494                                                       |
| 22813 | 1.143208              | 2.374501                                                       |
| 22815 | 1.925049              | 2.374507                                                       |
| 22817 | 1.000044              | 2.374514                                                       |
| 22819 | 1.053508              | 2.374521                                                       |
| 22821 | 1.333509              | 2.374527                                                       |
| 22823 | 1.035797              | 2.374534                                                       |
| 22825 | 1.369025              | 2.374540                                                       |
| 22827 | 1.525211              | 2.374547                                                       |
| 22829 | 1.028692              | 2.374553                                                       |
| 22831 | 1.075730              | 2.374560                                                       |
| 22833 | 1.503088              | 2.374567                                                       |
| 22835 | 1.200263              | 2.374573                                                       |
| 22837 | 1.026229              | 2.374580                                                       |
| 22839 | 1.395508              | 2.374586                                                       |
| 22841 | 1.235673              | 2.374593                                                       |
| 22843 | 1.021232              | 2.374599                                                       |
| 22845 | 1.601051              | 2.374606                                                       |
| 22847 | 1.142907              | 2.374612                                                       |
| 22849 | 1.016937              | 2.374619                                                       |
| 22851 | 1.445013              | 2.374626                                                       |
| 22853 | 1.000044              | 2.374632                                                       |
| 22855 | 1.373529              | 2.374639                                                       |
| 22857 | 1.407009              | 2.374645                                                       |
| 22859 | 1.000044              | 2.374652                                                       |
| 22861 | 1.000044              | 2.374658                                                       |
| 22863 | 1.333508              | 2.374665                                                       |
| 22865 | 1.275312              | 2.374671                                                       |
| 22867 | 1.077535              | 2.374678                                                       |
| 22869 | 1.861035              | 2.374684                                                       |
| 22871 | 1.000044              | 2.374691                                                       |
| 22873 | 1.015171              | 2.374698                                                       |
| 22875 | 1.691279              | 2.374704                                                       |
| 22877 | 1.000044              | 2.374711                                                       |
| 22879 | 1.013331              | 2.374717                                                       |
| 22881 | 1.384555              | 2.374724                                                       |
| 22883 | 1.165756              | 2.374730                                                       |
| 22885 | 1.258466              | 2.374737                                                       |
| 22887 | 1.445012              | 2.374743                                                       |
| 22889 | 1.023374              | 2.374750                                                       |
| 22891 | 1.091433              | 2.374756                                                       |
| 22893 | 1.438344              | 2.374763                                                       |

| $n$   | $\frac{\sigma(n)}{n}$ | $\frac{e^\gamma}{2} \log \log n + \frac{0.73...}{\log \log n}$ |
|-------|-----------------------|----------------------------------------------------------------|
| 22895 | 1.268399              | 2.374770                                                       |
| 22897 | 1.143207              | 2.374776                                                       |
| 22899 | 1.414909              | 2.374783                                                       |
| 22901 | 1.000044              | 2.374789                                                       |
| 22903 | 1.028686              | 2.374796                                                       |
| 22905 | 1.736739              | 2.374802                                                       |
| 22907 | 1.000044              | 2.374809                                                       |
| 22909 | 1.033655              | 2.374815                                                       |
| 22911 | 1.525206              | 2.374822                                                       |
| 22913 | 1.091433              | 2.374828                                                       |
| 22915 | 1.200262              | 2.374835                                                       |
| 22917 | 1.333508              | 2.374841                                                       |
| 22919 | 1.128845              | 2.374848                                                       |
| 22921 | 1.000044              | 2.374854                                                       |
| 22923 | 1.499106              | 2.374861                                                       |
| 22925 | 1.427961              | 2.374868                                                       |
| 22927 | 1.014350              | 2.374874                                                       |
| 22929 | 1.333508              | 2.374881                                                       |
| 22931 | 1.044525              | 2.374887                                                       |
| 22933 | 1.130249              | 2.374894                                                       |
| 22935 | 1.758012              | 2.374900                                                       |
| 22937 | 1.000044              | 2.374907                                                       |
| 22939 | 1.192729              | 2.374913                                                       |
| 22941 | 1.445011              | 2.374920                                                       |
| 22943 | 1.000044              | 2.374926                                                       |
| 22945 | 1.295969              | 2.374933                                                       |
| 22947 | 1.333508              | 2.374939                                                       |
| 22949 | 1.021221              | 2.374946                                                       |
| 22951 | 1.019563              | 2.374952                                                       |
| 22953 | 1.525204              | 2.374959                                                       |
| 22955 | 1.200261              | 2.374965                                                       |
| 22957 | 1.091432              | 2.374972                                                       |
| 22959 | 1.445011              | 2.374978                                                       |
| 22961 | 1.000044              | 2.374985                                                       |
| 22963 | 1.000044              | 2.374991                                                       |
| 22965 | 1.601045              | 2.374998                                                       |
| 22967 | 1.216354              | 2.375005                                                       |
| 22969 | 1.014237              | 2.375011                                                       |
| 22971 | 1.560228              | 2.375018                                                       |
| 22973 | 1.000044              | 2.375024                                                       |
| 22975 | 1.241349              | 2.375031                                                       |
| 22977 | 1.587675              | 2.375037                                                       |
| 22979 | 1.091431              | 2.375044                                                       |
| 22981 | 1.183586              | 2.375050                                                       |

| $n$   | $\frac{\sigma(n)}{n}$ | $\frac{e^\gamma}{2} \log \log n + \frac{0.73\dots}{\log \log n}$ |
|-------|-----------------------|------------------------------------------------------------------|
| 22983 | 1.370056              | 2.375057                                                         |
| 22985 | 1.200261              | 2.375063                                                         |
| 22987 | 1.013442              | 2.375070                                                         |
| 22989 | 1.364131              | 2.375076                                                         |
| 22991 | 1.015702              | 2.375083                                                         |
| 22993 | 1.000043              | 2.375089                                                         |
| 22995 | 2.008089              | 2.375096                                                         |
| 22997 | 1.132322              | 2.375102                                                         |
| 22999 | 1.013957              | 2.375109                                                         |
| 23001 | 1.577671              | 2.375115                                                         |
| 23003 | 1.000043              | 2.375122                                                         |
| 23005 | 1.239383              | 2.375128                                                         |
| 23007 | 1.333507              | 2.375135                                                         |
| 23009 | 1.209961              | 2.375141                                                         |
| 23011 | 1.000043              | 2.375148                                                         |
| 23013 | 1.445009              | 2.375154                                                         |
| 23015 | 1.200261              | 2.375161                                                         |
| 23017 | 1.000043              | 2.375167                                                         |
| 23019 | 1.333507              | 2.375174                                                         |
| 23021 | 1.000043              | 2.375180                                                         |
| 23023 | 1.401034              | 2.375187                                                         |
| 23025 | 1.658719              | 2.375193                                                         |
| 23027 | 1.000043              | 2.375200                                                         |
| 23029 | 1.000043              | 2.375206                                                         |
| 23031 | 1.483218              | 2.375213                                                         |
| 23033 | 1.033647              | 2.375219                                                         |
| 23035 | 1.275277              | 2.375226                                                         |
| 23037 | 1.525199              | 2.375232                                                         |
| 23039 | 1.000043              | 2.375239                                                         |
| 23041 | 1.000043              | 2.375245                                                         |
| 23043 | 1.333507              | 2.375252                                                         |
| 23045 | 1.312215              | 2.375258                                                         |
| 23047 | 1.053499              | 2.375265                                                         |
| 23049 | 1.563452              | 2.375271                                                         |
| 23051 | 1.186933              | 2.375278                                                         |
| 23053 | 1.000043              | 2.375284                                                         |
| 23055 | 1.686402              | 2.375291                                                         |
| 23057 | 1.000043              | 2.375297                                                         |
| 23059 | 1.000043              | 2.375304                                                         |
| 23061 | 1.333507              | 2.375310                                                         |
| 23063 | 1.000043              | 2.375317                                                         |
| 23065 | 1.373510              | 2.375323                                                         |
| 23067 | 1.582520              | 2.375330                                                         |
| 23069 | 1.123586              | 2.375336                                                         |

| $n$   | $\frac{\sigma(n)}{n}$ | $\frac{e^\gamma}{2} \log \log n + \frac{0.73\dots}{\log \log n}$ |
|-------|-----------------------|------------------------------------------------------------------|
| 23071 | 1.000043              | 2.375343                                                         |
| 23073 | 1.333507              | 2.375349                                                         |
| 23075 | 1.354193              | 2.375356                                                         |
| 23077 | 1.023357              | 2.375362                                                         |
| 23079 | 1.560900              | 2.375369                                                         |
| 23081 | 1.000043              | 2.375375                                                         |
| 23083 | 1.026210              | 2.375381                                                         |
| 23085 | 1.892138              | 2.375388                                                         |
| 23087 | 1.000043              | 2.375394                                                         |
| 23089 | 1.091429              | 2.375401                                                         |
| 23091 | 1.371963              | 2.375407                                                         |
| 23093 | 1.143204              | 2.375414                                                         |
| 23095 | 1.247023              | 2.375420                                                         |
| 23097 | 1.333507              | 2.375427                                                         |
| 23099 | 1.000043              | 2.375433                                                         |
| 23101 | 1.077529              | 2.375440                                                         |
| 23103 | 1.539540              | 2.375446                                                         |
| 23105 | 1.200260              | 2.375453                                                         |
| 23107 | 1.143203              | 2.375459                                                         |
| 23109 | 1.333506              | 2.375466                                                         |
| 23111 | 1.104928              | 2.375472                                                         |
| 23113 | 1.035781              | 2.375479                                                         |
| 23115 | 1.694484              | 2.375485                                                         |
| 23117 | 1.000043              | 2.375492                                                         |
| 23119 | 1.019075              | 2.375498                                                         |
| 23121 | 1.655292              | 2.375505                                                         |
| 23123 | 1.053497              | 2.375511                                                         |
| 23125 | 1.283373              | 2.375517                                                         |
| 23127 | 1.438319              | 2.375524                                                         |
| 23129 | 1.014311              | 2.375530                                                         |
| 23131 | 1.000043              | 2.375537                                                         |
| 23133 | 1.456620              | 2.375543                                                         |
| 23135 | 1.373503              | 2.375550                                                         |
| 23137 | 1.059602              | 2.375556                                                         |
| 23139 | 1.483210              | 2.375563                                                         |
| 23141 | 1.016896              | 2.375569                                                         |
| 23143 | 1.000043              | 2.375576                                                         |
| 23145 | 1.601037              | 2.375582                                                         |
| 23147 | 1.016114              | 2.375589                                                         |
| 23149 | 1.143203              | 2.375595                                                         |
| 23151 | 1.333506              | 2.375601                                                         |
| 23153 | 1.090744              | 2.375608                                                         |
| 23155 | 1.312200              | 2.375614                                                         |
| 23157 | 1.509004              | 2.375621                                                         |

| $n$   | $\frac{\sigma(n)}{n}$ | $\frac{e^\gamma}{2} \log \log n + \frac{0.73...}{\log \log n}$ |
|-------|-----------------------|----------------------------------------------------------------|
| 23159 | 1.000043              | 2.375627                                                       |
| 23161 | 1.119123              | 2.375634                                                       |
| 23163 | 1.525191              | 2.375640                                                       |
| 23165 | 1.240147              | 2.375647                                                       |
| 23167 | 1.000043              | 2.375653                                                       |
| 23169 | 1.333506              | 2.375660                                                       |
| 23171 | 1.118640              | 2.375666                                                       |
| 23173 | 1.000043              | 2.375673                                                       |
| 23175 | 1.808501              | 2.375679                                                       |
| 23177 | 1.298529              | 2.375685                                                       |
| 23179 | 1.077527              | 2.375692                                                       |
| 23181 | 1.333506              | 2.375698                                                       |
| 23183 | 1.014537              | 2.375705                                                       |
| 23185 | 1.200259              | 2.375711                                                       |
| 23187 | 1.366283              | 2.375718                                                       |
| 23189 | 1.000043              | 2.375724                                                       |
| 23191 | 1.143202              | 2.375731                                                       |
| 23193 | 1.483206              | 2.375737                                                       |
| 23195 | 1.200259              | 2.375743                                                       |
| 23197 | 1.000043              | 2.375750                                                       |
| 23199 | 1.572482              | 2.375756                                                       |
| 23201 | 1.000043              | 2.375763                                                       |
| 23203 | 1.000043              | 2.375769                                                       |
| 23205 | 2.085068              | 2.375776                                                       |
| 23207 | 1.044512              | 2.375782                                                       |
| 23209 | 1.000043              | 2.375789                                                       |
| 23211 | 1.445005              | 2.375795                                                       |
| 23213 | 1.013225              | 2.375801                                                       |
| 23215 | 1.200258              | 2.375808                                                       |
| 23217 | 1.364517              | 2.375814                                                       |
| 23219 | 1.190749              | 2.375821                                                       |
| 23221 | 1.091426              | 2.375827                                                       |
| 23223 | 1.333506              | 2.375834                                                       |
| 23225 | 1.241335              | 2.375840                                                       |
| 23227 | 1.000043              | 2.375847                                                       |
| 23229 | 1.511042              | 2.375853                                                       |
| 23231 | 1.077526              | 2.375859                                                       |
| 23233 | 1.143201              | 2.375866                                                       |
| 23235 | 1.601033              | 2.375872                                                       |
| 23237 | 1.053492              | 2.375879                                                       |
| 23239 | 1.059598              | 2.375885                                                       |
| 23241 | 1.365862              | 2.375892                                                       |
| 23243 | 1.091425              | 2.375898                                                       |
| 23245 | 1.200258              | 2.375904                                                       |

| $n$   | $\frac{\sigma(n)}{n}$ | $\frac{e^\gamma}{2} \log \log n + \frac{0.73...}{\log \log n}$ |
|-------|-----------------------|----------------------------------------------------------------|
| 23247 | 1.748871              | 2.375911                                                       |
| 23249 | 1.017850              | 2.375917                                                       |
| 23251 | 1.000043              | 2.375924                                                       |
| 23253 | 1.395433              | 2.375930                                                       |
| 23255 | 1.200258              | 2.375937                                                       |
| 23257 | 1.077525              | 2.375943                                                       |
| 23259 | 1.333505              | 2.375949                                                       |
| 23261 | 1.143201              | 2.375956                                                       |
| 23263 | 1.025147              | 2.375962                                                       |
| 23265 | 1.931141              | 2.375969                                                       |
| 23267 | 1.021189              | 2.375975                                                       |
| 23269 | 1.000043              | 2.375982                                                       |
| 23271 | 1.333505              | 2.375988                                                       |
| 23273 | 1.088214              | 2.375994                                                       |
| 23275 | 1.518367              | 2.376001                                                       |
| 23277 | 1.333505              | 2.376007                                                       |
| 23279 | 1.000043              | 2.376014                                                       |
| 23281 | 1.033633              | 2.376020                                                       |
| 23283 | 1.563372              | 2.376027                                                       |
| 23285 | 1.200258              | 2.376033                                                       |
| 23287 | 1.143986              | 2.376039                                                       |
| 23289 | 1.525184              | 2.376046                                                       |
| 23291 | 1.000043              | 2.376052                                                       |
| 23293 | 1.000043              | 2.376059                                                       |
| 23295 | 1.601030              | 2.376065                                                       |
| 23297 | 1.000043              | 2.376072                                                       |
| 23299 | 1.044508              | 2.376078                                                       |
| 23301 | 1.483198              | 2.376084                                                       |
| 23303 | 1.143200              | 2.376091                                                       |
| 23305 | 1.235786              | 2.376097                                                       |
| 23307 | 1.414854              | 2.376104                                                       |
| 23309 | 1.182033              | 2.376110                                                       |
| 23311 | 1.000043              | 2.376116                                                       |
| 23313 | 1.406940              | 2.376123                                                       |
| 23315 | 1.200257              | 2.376129                                                       |
| 23317 | 1.143200              | 2.376136                                                       |
| 23319 | 1.445002              | 2.376142                                                       |
| 23321 | 1.000043              | 2.376148                                                       |
| 23323 | 1.015650              | 2.376155                                                       |
| 23325 | 1.658650              | 2.376161                                                       |
| 23327 | 1.000043              | 2.376168                                                       |
| 23329 | 1.026191              | 2.376174                                                       |
| 23331 | 1.678796              | 2.376181                                                       |
| 23333 | 1.000043              | 2.376187                                                       |

| $n$   | $\frac{\sigma(n)}{n}$ | $\frac{e^\gamma}{2} \log \log n + \frac{0.73\dots}{\log \log n}$ |
|-------|-----------------------|------------------------------------------------------------------|
| 23335 | 1.295907              | 2.376193                                                         |
| 23337 | 1.445001              | 2.376200                                                         |
| 23339 | 1.000043              | 2.376206                                                         |
| 23341 | 1.059595              | 2.376213                                                         |
| 23343 | 1.381828              | 2.376219                                                         |
| 23345 | 1.480403              | 2.376225                                                         |
| 23347 | 1.028655              | 2.376232                                                         |
| 23349 | 1.371879              | 2.376238                                                         |
| 23351 | 1.053488              | 2.376245                                                         |
| 23353 | 1.104869              | 2.376251                                                         |
| 23355 | 1.788054              | 2.376257                                                         |
| 23357 | 1.000043              | 2.376264                                                         |
| 23359 | 1.183612              | 2.376270                                                         |
| 23361 | 1.438295              | 2.376277                                                         |
| 23363 | 1.019047              | 2.376283                                                         |
| 23365 | 1.200257              | 2.376289                                                         |
| 23367 | 1.333505              | 2.376296                                                         |
| 23369 | 1.000043              | 2.376302                                                         |
| 23371 | 1.000043              | 2.376309                                                         |
| 23373 | 1.711975              | 2.376315                                                         |
| 23375 | 1.441540              | 2.376321                                                         |
| 23377 | 1.014501              | 2.376328                                                         |
| 23379 | 1.333504              | 2.376334                                                         |
| 23381 | 1.014157              | 2.376340                                                         |
| 23383 | 1.017833              | 2.376347                                                         |
| 23385 | 1.601026              | 2.376353                                                         |
| 23387 | 1.235558              | 2.376360                                                         |
| 23389 | 1.053487              | 2.376366                                                         |
| 23391 | 1.520585              | 2.376372                                                         |
| 23393 | 1.013124              | 2.376379                                                         |
| 23395 | 1.200256              | 2.376385                                                         |
| 23397 | 1.456597              | 2.376392                                                         |
| 23399 | 1.000043              | 2.376398                                                         |
| 23401 | 1.143199              | 2.376404                                                         |
| 23403 | 1.384438              | 2.376411                                                         |
| 23405 | 1.246913              | 2.376417                                                         |
| 23407 | 1.015081              | 2.376424                                                         |
| 23409 | 1.586868              | 2.376430                                                         |
| 23411 | 1.026184              | 2.376436                                                         |
| 23413 | 1.077521              | 2.376443                                                         |
| 23415 | 1.836771              | 2.376449                                                         |
| 23417 | 1.000043              | 2.376455                                                         |
| 23419 | 1.091421              | 2.376462                                                         |
| 23421 | 1.375859              | 2.376468                                                         |



| $n$   | $\frac{\sigma(n)}{n}$ | $\frac{e^\gamma}{2} \log \log n + \frac{0.73\dots}{\log \log n}$ |
|-------|-----------------------|------------------------------------------------------------------|
| 23423 | 1.019511              | 2.376475                                                         |
| 23425 | 1.241323              | 2.376481                                                         |
| 23427 | 1.531566              | 2.376487                                                         |
| 23429 | 1.143199              | 2.376494                                                         |
| 23431 | 1.000043              | 2.376500                                                         |
| 23433 | 1.364230              | 2.376506                                                         |
| 23435 | 1.239172              | 2.376513                                                         |
| 23437 | 1.044502              | 2.376519                                                         |
| 23439 | 1.438287              | 2.376526                                                         |
| 23441 | 1.091421              | 2.376532                                                         |
| 23443 | 1.216227              | 2.376538                                                         |
| 23445 | 1.736660              | 2.376545                                                         |
| 23447 | 1.000043              | 2.376551                                                         |
| 23449 | 1.013263              | 2.376557                                                         |
| 23451 | 1.333504              | 2.376564                                                         |
| 23453 | 1.023323              | 2.376570                                                         |
| 23455 | 1.200256              | 2.376577                                                         |
| 23457 | 1.525174              | 2.376583                                                         |
| 23459 | 1.000043              | 2.376589                                                         |
| 23461 | 1.035761              | 2.376596                                                         |
| 23463 | 1.636619              | 2.376602                                                         |
| 23465 | 1.363904              | 2.376608                                                         |
| 23467 | 1.033622              | 2.376615                                                         |
| 23469 | 1.333504              | 2.376621                                                         |
| 23471 | 1.165694              | 2.376628                                                         |
| 23473 | 1.000043              | 2.376634                                                         |
| 23475 | 1.658616              | 2.376640                                                         |
| 23477 | 1.059590              | 2.376647                                                         |
| 23479 | 1.021168              | 2.376653                                                         |
| 23481 | 1.444998              | 2.376659                                                         |
| 23483 | 1.044500              | 2.376666                                                         |
| 23485 | 1.520630              | 2.376672                                                         |
| 23487 | 1.333504              | 2.376678                                                         |
| 23489 | 1.015624              | 2.376685                                                         |
| 23491 | 1.090630              | 2.376691                                                         |
| 23493 | 1.373005              | 2.376698                                                         |
| 23495 | 1.242137              | 2.376704                                                         |
| 23497 | 1.000043              | 2.376710                                                         |
| 23499 | 1.655219              | 2.376717                                                         |
| 23501 | 1.017148              | 2.376723                                                         |
| 23503 | 1.053483              | 2.376729                                                         |
| 23505 | 1.601021              | 2.376736                                                         |
| 23507 | 1.091420              | 2.376742                                                         |
| 23509 | 1.000043              | 2.376748                                                         |

| $n$   | $\frac{\sigma(n)}{n}$ | $\frac{e^\gamma}{2} \log \log n + \frac{0.73...}{\log \log n}$ |
|-------|-----------------------|----------------------------------------------------------------|
| 23511 | 1.414827              | 2.376755                                                       |
| 23513 | 1.143197              | 2.376761                                                       |
| 23515 | 1.200255              | 2.376767                                                       |
| 23517 | 1.619254              | 2.376774                                                       |
| 23519 | 1.035758              | 2.376780                                                       |
| 23521 | 1.025126              | 2.376786                                                       |
| 23523 | 1.333503              | 2.376793                                                       |
| 23525 | 1.241318              | 2.376799                                                       |
| 23527 | 1.143197              | 2.376806                                                       |
| 23529 | 1.566747              | 2.376812                                                       |
| 23531 | 1.000042              | 2.376818                                                       |
| 23533 | 1.014235              | 2.376825                                                       |
| 23535 | 1.736648              | 2.376831                                                       |
| 23537 | 1.000042              | 2.376837                                                       |
| 23539 | 1.000042              | 2.376844                                                       |
| 23541 | 1.631197              | 2.376850                                                       |
| 23543 | 1.077518              | 2.376856                                                       |
| 23545 | 1.275175              | 2.376863                                                       |
| 23547 | 1.369856              | 2.376869                                                       |
| 23549 | 1.000042              | 2.376875                                                       |
| 23551 | 1.091419              | 2.376882                                                       |
| 23553 | 1.444996              | 2.376888                                                       |
| 23555 | 1.373466              | 2.376894                                                       |
| 23557 | 1.000042              | 2.376901                                                       |
| 23559 | 1.333503              | 2.376907                                                       |
| 23561 | 1.000042              | 2.376913                                                       |
| 23563 | 1.000042              | 2.376920                                                       |
| 23565 | 1.601018              | 2.376926                                                       |
| 23567 | 1.000042              | 2.376932                                                       |
| 23569 | 1.286605              | 2.376939                                                       |
| 23571 | 1.513385              | 2.376945                                                       |
| 23573 | 1.091418              | 2.376951                                                       |
| 23575 | 1.325472              | 2.376958                                                       |
| 23577 | 1.384400              | 2.376964                                                       |
| 23579 | 1.129819              | 2.376970                                                       |
| 23581 | 1.000042              | 2.376977                                                       |
| 23583 | 1.525166              | 2.376983                                                       |
| 23585 | 1.236379              | 2.376989                                                       |
| 23587 | 1.014118              | 2.376996                                                       |
| 23589 | 1.444996              | 2.377002                                                       |
| 23591 | 1.033615              | 2.377008                                                       |
| 23593 | 1.000042              | 2.377015                                                       |
| 23595 | 1.893961              | 2.377021                                                       |
| 23597 | 1.143196              | 2.377027                                                       |

| $n$   | $\frac{\sigma(n)}{n}$ | $\frac{e^\gamma}{2} \log \log n + \frac{0.73...}{\log \log n}$ |
|-------|-----------------------|----------------------------------------------------------------|
| 23599 | 1.000042              | 2.377034                                                       |
| 23601 | 1.333503              | 2.377040                                                       |
| 23603 | 1.000042              | 2.377046                                                       |
| 23605 | 1.200254              | 2.377053                                                       |
| 23607 | 1.502266              | 2.377059                                                       |
| 23609 | 1.000042              | 2.377065                                                       |
| 23611 | 1.143196              | 2.377072                                                       |
| 23613 | 1.414814              | 2.377078                                                       |
| 23615 | 1.200254              | 2.377084                                                       |
| 23617 | 1.158488              | 2.377091                                                       |
| 23619 | 1.333503              | 2.377097                                                       |
| 23621 | 1.137970              | 2.377103                                                       |
| 23623 | 1.000042              | 2.377110                                                       |
| 23625 | 2.113016              | 2.377116                                                       |
| 23627 | 1.000042              | 2.377122                                                       |
| 23629 | 1.000042              | 2.377129                                                       |
| 23631 | 1.333503              | 2.377135                                                       |
| 23633 | 1.000042              | 2.377141                                                       |
| 23635 | 1.248995              | 2.377148                                                       |
| 23637 | 1.333503              | 2.377154                                                       |
| 23639 | 1.250814              | 2.377160                                                       |
| 23641 | 1.023307              | 2.377166                                                       |
| 23643 | 1.504378              | 2.377173                                                       |
| 23645 | 1.200254              | 2.377179                                                       |
| 23647 | 1.150928              | 2.377185                                                       |
| 23649 | 1.333502              | 2.377192                                                       |
| 23651 | 1.017801              | 2.377198                                                       |
| 23653 | 1.190547              | 2.377204                                                       |
| 23655 | 1.704502              | 2.377211                                                       |
| 23657 | 1.026166              | 2.377217                                                       |
| 23659 | 1.019485              | 2.377223                                                       |
| 23661 | 1.582351              | 2.377230                                                       |
| 23663 | 1.000042              | 2.377236                                                       |
| 23665 | 1.200254              | 2.377242                                                       |
| 23667 | 1.622512              | 2.377249                                                       |
| 23669 | 1.000042              | 2.377255                                                       |
| 23671 | 1.000042              | 2.377261                                                       |
| 23673 | 1.438263              | 2.377267                                                       |
| 23675 | 1.241309              | 2.377274                                                       |
| 23677 | 1.000042              | 2.377280                                                       |
| 23679 | 1.483171              | 2.377286                                                       |
| 23681 | 1.216165              | 2.377293                                                       |
| 23683 | 1.091416              | 2.377299                                                       |
| 23685 | 1.601013              | 2.377305                                                       |

| $n$   | $\frac{\sigma(n)}{n}$ | $\frac{e^\gamma}{2} \log \log n + \frac{0.73...}{\log \log n}$ |
|-------|-----------------------|----------------------------------------------------------------|
| 23687 | 1.000042              | 2.377312                                                       |
| 23689 | 1.000042              | 2.377318                                                       |
| 23691 | 1.367608              | 2.377324                                                       |
| 23693 | 1.114253              | 2.377330                                                       |
| 23695 | 1.373454              | 2.377337                                                       |
| 23697 | 1.444993              | 2.377343                                                       |
| 23699 | 1.077514              | 2.377349                                                       |
| 23701 | 1.013122              | 2.377356                                                       |
| 23703 | 1.333502              | 2.377362                                                       |
| 23705 | 1.312128              | 2.377368                                                       |
| 23707 | 1.013034              | 2.377375                                                       |
| 23709 | 1.525159              | 2.377381                                                       |
| 23711 | 1.013201              | 2.377387                                                       |
| 23713 | 1.044490              | 2.377393                                                       |
| 23715 | 1.894497              | 2.377400                                                       |
| 23717 | 1.028629              | 2.377406                                                       |
| 23719 | 1.000042              | 2.377412                                                       |
| 23721 | 1.333502              | 2.377419                                                       |
| 23723 | 1.143194              | 2.377425                                                       |
| 23725 | 1.353678              | 2.377431                                                       |
| 23727 | 1.456568              | 2.377438                                                       |
| 23729 | 1.019006              | 2.377444                                                       |
| 23731 | 1.053474              | 2.377450                                                       |
| 23733 | 1.498926              | 2.377456                                                       |
| 23735 | 1.237666              | 2.377463                                                       |
| 23737 | 1.143194              | 2.377469                                                       |
| 23739 | 1.372931              | 2.377475                                                       |
| 23741 | 1.000042              | 2.377482                                                       |
| 23743 | 1.000042              | 2.377488                                                       |
| 23745 | 1.601011              | 2.377494                                                       |
| 23747 | 1.000042              | 2.377500                                                       |
| 23749 | 1.164175              | 2.377507                                                       |
| 23751 | 1.839080              | 2.377513                                                       |
| 23753 | 1.000042              | 2.377519                                                       |
| 23755 | 1.200253              | 2.377526                                                       |
| 23757 | 1.333502              | 2.377532                                                       |
| 23759 | 1.044488              | 2.377538                                                       |
| 23761 | 1.000042              | 2.377544                                                       |
| 23763 | 1.348483              | 2.377551                                                       |
| 23765 | 1.410309              | 2.377557                                                       |
| 23767 | 1.000042              | 2.377563                                                       |
| 23769 | 1.531406              | 2.377569                                                       |
| 23771 | 1.091414              | 2.377576                                                       |
| 23773 | 1.000042              | 2.377582                                                       |

| $n$   | $\frac{\sigma(n)}{n}$ | $\frac{e^\gamma}{2} \log \log n + \frac{0.73...}{\log \log n}$ |
|-------|-----------------------|----------------------------------------------------------------|
| 23775 | 1.658549              | 2.377588                                                       |
| 23777 | 1.130504              | 2.377595                                                       |
| 23779 | 1.184238              | 2.377601                                                       |
| 23781 | 1.333502              | 2.377607                                                       |
| 23783 | 1.059580              | 2.377613                                                       |
| 23785 | 1.235064              | 2.377620                                                       |
| 23787 | 1.483163              | 2.377626                                                       |
| 23789 | 1.000042              | 2.377632                                                       |
| 23791 | 1.028624              | 2.377639                                                       |
| 23793 | 1.678477              | 2.377645                                                       |
| 23795 | 1.200252              | 2.377651                                                       |
| 23797 | 1.021137              | 2.377657                                                       |
| 23799 | 1.333501              | 2.377664                                                       |
| 23801 | 1.000042              | 2.377670                                                       |
| 23803 | 1.077511              | 2.377676                                                       |
| 23805 | 1.811972              | 2.377682                                                       |
| 23807 | 1.209728              | 2.377689                                                       |
| 23809 | 1.035743              | 2.377695                                                       |
| 23811 | 1.333501              | 2.377701                                                       |
| 23813 | 1.000042              | 2.377707                                                       |
| 23815 | 1.312114              | 2.377714                                                       |
| 23817 | 1.414788              | 2.377720                                                       |
| 23819 | 1.000042              | 2.377726                                                       |
| 23821 | 1.184837              | 2.377733                                                       |
| 23823 | 1.444990              | 2.377739                                                       |
| 23825 | 1.241301              | 2.377745                                                       |
| 23827 | 1.000042              | 2.377751                                                       |
| 23829 | 1.474506              | 2.377758                                                       |
| 23831 | 1.000042              | 2.377764                                                       |
| 23833 | 1.000042              | 2.377770                                                       |
| 23835 | 1.836627              | 2.377776                                                       |
| 23837 | 1.104753              | 2.377783                                                       |
| 23839 | 1.033600              | 2.377789                                                       |
| 23841 | 1.483159              | 2.377795                                                       |
| 23843 | 1.013631              | 2.377801                                                       |
| 23845 | 1.268190              | 2.377808                                                       |
| 23847 | 1.333501              | 2.377814                                                       |
| 23849 | 1.143193              | 2.377820                                                       |
| 23851 | 1.122972              | 2.377826                                                       |
| 23853 | 1.333501              | 2.377833                                                       |
| 23855 | 1.295829              | 2.377839                                                       |
| 23857 | 1.000042              | 2.377845                                                       |
| 23859 | 1.582296              | 2.377851                                                       |
| 23861 | 1.013872              | 2.377858                                                       |

| $n$   | $\frac{\sigma(n)}{n}$ | $\frac{e^\gamma}{2} \log \log n + \frac{0.73...}{\log \log n}$ |
|-------|-----------------------|----------------------------------------------------------------|
| 23863 | 1.165654              | 2.377864                                                       |
| 23865 | 1.681458              | 2.377870                                                       |
| 23867 | 1.035740              | 2.377876                                                       |
| 23869 | 1.000042              | 2.377883                                                       |
| 23871 | 1.363998              | 2.377889                                                       |
| 23873 | 1.000042              | 2.377895                                                       |
| 23875 | 1.254534              | 2.377901                                                       |
| 23877 | 1.655149              | 2.377908                                                       |
| 23879 | 1.000042              | 2.377914                                                       |
| 23881 | 1.181860              | 2.377920                                                       |
| 23883 | 1.406858              | 2.377926                                                       |
| 23885 | 1.275110              | 2.377933                                                       |
| 23887 | 1.000042              | 2.377939                                                       |
| 23889 | 1.333501              | 2.377945                                                       |
| 23891 | 1.143192              | 2.377951                                                       |
| 23893 | 1.000042              | 2.377958                                                       |
| 23895 | 1.822976              | 2.377964                                                       |
| 23897 | 1.044483              | 2.377970                                                       |
| 23899 | 1.000042              | 2.377976                                                       |
| 23901 | 1.381700              | 2.377983                                                       |
| 23903 | 1.138602              | 2.377989                                                       |
| 23905 | 1.373437              | 2.377995                                                       |
| 23907 | 1.438240              | 2.378001                                                       |
| 23909 | 1.000042              | 2.378008                                                       |
| 23911 | 1.000042              | 2.378014                                                       |
| 23913 | 1.444988              | 2.378020                                                       |
| 23915 | 1.200251              | 2.378026                                                       |
| 23917 | 1.000042              | 2.378033                                                       |
| 23919 | 1.637527              | 2.378039                                                       |
| 23921 | 1.053468              | 2.378045                                                       |
| 23923 | 1.023283              | 2.378051                                                       |
| 23925 | 1.865831              | 2.378058                                                       |
| 23927 | 1.017094              | 2.378064                                                       |
| 23929 | 1.000042              | 2.378070                                                       |
| 23931 | 1.444988              | 2.378076                                                       |
| 23933 | 1.235449              | 2.378082                                                       |
| 23935 | 1.200251              | 2.378089                                                       |
| 23937 | 1.363579              | 2.378095                                                       |
| 23939 | 1.028614              | 2.378101                                                       |
| 23941 | 1.014995              | 2.378107                                                       |
| 23943 | 1.395314              | 2.378114                                                       |
| 23945 | 1.200251              | 2.378120                                                       |
| 23947 | 1.250762              | 2.378126                                                       |
| 23949 | 1.483152              | 2.378132                                                       |

| $n$   | $\frac{\sigma(n)}{n}$ | $\frac{e^\gamma}{2} \log \log n + \frac{0.73\dots}{\log \log n}$ |
|-------|-----------------------|------------------------------------------------------------------|
| 23951 | 1.025093              | 2.378139                                                         |
| 23953 | 1.059575              | 2.378145                                                         |
| 23955 | 1.601002              | 2.378151                                                         |
| 23957 | 1.000042              | 2.378157                                                         |
| 23959 | 1.145290              | 2.378163                                                         |
| 23961 | 1.560536              | 2.378170                                                         |
| 23963 | 1.033593              | 2.378176                                                         |
| 23965 | 1.200250              | 2.378182                                                         |
| 23967 | 1.444987              | 2.378188                                                         |
| 23969 | 1.091410              | 2.378195                                                         |
| 23971 | 1.000042              | 2.378201                                                         |
| 23973 | 1.365536              | 2.378207                                                         |
| 23975 | 1.427487              | 2.378213                                                         |
| 23977 | 1.000042              | 2.378219                                                         |
| 23979 | 1.333500              | 2.378226                                                         |
| 23981 | 1.000042              | 2.378232                                                         |
| 23983 | 1.035734              | 2.378238                                                         |
| 23985 | 1.912195              | 2.378244                                                         |
| 23987 | 1.075082              | 2.378251                                                         |
| 23989 | 1.200550              | 2.378257                                                         |
| 23991 | 1.456546              | 2.378263                                                         |
| 23993 | 1.000042              | 2.378269                                                         |
| 23995 | 1.200250              | 2.378275                                                         |
| 23997 | 1.406843              | 2.378282                                                         |
| 23999 | 1.014042              | 2.378288                                                         |
| 24001 | 1.000042              | 2.378294                                                         |
| 24003 | 1.706453              | 2.378300                                                         |
| 24005 | 1.200250              | 2.378306                                                         |
| 24007 | 1.000042              | 2.378313                                                         |
| 24009 | 1.367487              | 2.378319                                                         |
| 24011 | 1.077506              | 2.378325                                                         |
| 24013 | 1.139383              | 2.378331                                                         |
| 24015 | 1.600999              | 2.378338                                                         |
| 24017 | 1.183162              | 2.378344                                                         |
| 24019 | 1.000042              | 2.378350                                                         |
| 24021 | 1.539153              | 2.378356                                                         |
| 24023 | 1.000042              | 2.378362                                                         |
| 24025 | 1.281290              | 2.378369                                                         |
| 24027 | 1.333500              | 2.378375                                                         |
| 24029 | 1.000042              | 2.378381                                                         |
| 24031 | 1.143190              | 2.378387                                                         |
| 24033 | 1.333500              | 2.378393                                                         |
| 24035 | 1.437903              | 2.378400                                                         |
| 24037 | 1.102550              | 2.378406                                                         |

| $n$   | $\frac{\sigma(n)}{n}$ | $\frac{e^\gamma}{2} \log \log n + \frac{0.73...}{\log \log n}$ |
|-------|-----------------------|----------------------------------------------------------------|
| 24039 | 1.444985              | 2.378412                                                       |
| 24041 | 1.035731              | 2.378418                                                       |
| 24043 | 1.000042              | 2.378424                                                       |
| 24045 | 1.836556              | 2.378431                                                       |
| 24047 | 1.013016              | 2.378437                                                       |
| 24049 | 1.000042              | 2.378443                                                       |
| 24051 | 1.333500              | 2.378449                                                       |
| 24053 | 1.017752              | 2.378455                                                       |
| 24055 | 1.275078              | 2.378462                                                       |
| 24057 | 1.636114              | 2.378468                                                       |
| 24059 | 1.165634              | 2.378474                                                       |
| 24061 | 1.000042              | 2.378480                                                       |
| 24063 | 1.438225              | 2.378486                                                       |
| 24065 | 1.200249              | 2.378493                                                       |
| 24067 | 1.026135              | 2.378499                                                       |
| 24069 | 1.364078              | 2.378505                                                       |
| 24071 | 1.000042              | 2.378511                                                       |
| 24073 | 1.209654              | 2.378517                                                       |
| 24075 | 1.807850              | 2.378524                                                       |
| 24077 | 1.000042              | 2.378530                                                       |
| 24079 | 1.104697              | 2.378536                                                       |
| 24081 | 1.395291              | 2.378542                                                       |
| 24083 | 1.000042              | 2.378548                                                       |
| 24085 | 1.200249              | 2.378554                                                       |
| 24087 | 1.615477              | 2.378561                                                       |
| 24089 | 1.150733              | 2.378567                                                       |
| 24091 | 1.000042              | 2.378573                                                       |
| 24093 | 1.444984              | 2.378579                                                       |
| 24095 | 1.235111              | 2.378585                                                       |
| 24097 | 1.000041              | 2.378592                                                       |
| 24099 | 1.384290              | 2.378598                                                       |
| 24101 | 1.250736              | 2.378604                                                       |
| 24103 | 1.000041              | 2.378610                                                       |
| 24105 | 1.600996              | 2.378616                                                       |
| 24107 | 1.000041              | 2.378623                                                       |
| 24109 | 1.000041              | 2.378629                                                       |
| 24111 | 1.592634              | 2.378635                                                       |
| 24113 | 1.000041              | 2.378641                                                       |
| 24115 | 1.504790              | 2.378647                                                       |
| 24117 | 1.333499              | 2.378653                                                       |
| 24119 | 1.014967              | 2.378660                                                       |
| 24121 | 1.000041              | 2.378666                                                       |
| 24123 | 1.575923              | 2.378672                                                       |
| 24125 | 1.254466              | 2.378678                                                       |



| $n$   | $\frac{\sigma(n)}{n}$ | $\frac{e^\gamma}{2} \log \log n + \frac{0.73\dots}{\log \log n}$ |
|-------|-----------------------|------------------------------------------------------------------|
| 24127 | 1.044473              | 2.378684                                                         |
| 24129 | 1.655104              | 2.378691                                                         |
| 24131 | 1.019436              | 2.378697                                                         |
| 24133 | 1.000041              | 2.378703                                                         |
| 24135 | 1.600994              | 2.378709                                                         |
| 24137 | 1.000041              | 2.378715                                                         |
| 24139 | 1.014127              | 2.378721                                                         |
| 24141 | 1.438217              | 2.378728                                                         |
| 24143 | 1.143189              | 2.378734                                                         |
| 24145 | 1.312073              | 2.378740                                                         |
| 24147 | 1.444983              | 2.378746                                                         |
| 24149 | 1.113090              | 2.378752                                                         |
| 24151 | 1.000041              | 2.378758                                                         |
| 24153 | 1.363309              | 2.378765                                                         |
| 24155 | 1.200248              | 2.378771                                                         |
| 24157 | 1.274165              | 2.378777                                                         |
| 24159 | 1.333499              | 2.378783                                                         |
| 24161 | 1.028600              | 2.378789                                                         |
| 24163 | 1.016761              | 2.378795                                                         |
| 24165 | 1.787709              | 2.378802                                                         |
| 24167 | 1.181777              | 2.378808                                                         |
| 24169 | 1.000041              | 2.378814                                                         |
| 24171 | 1.525133              | 2.378820                                                         |
| 24173 | 1.044471              | 2.378826                                                         |
| 24175 | 1.241282              | 2.378832                                                         |
| 24177 | 1.333499              | 2.378839                                                         |
| 24179 | 1.000041              | 2.378845                                                         |
| 24181 | 1.000041              | 2.378851                                                         |
| 24183 | 1.444982              | 2.378857                                                         |
| 24185 | 1.373413              | 2.378863                                                         |
| 24187 | 1.071154              | 2.378869                                                         |
| 24189 | 1.456530              | 2.378876                                                         |
| 24191 | 1.059568              | 2.378882                                                         |
| 24193 | 1.077502              | 2.378888                                                         |
| 24195 | 1.600992              | 2.378894                                                         |
| 24197 | 1.000041              | 2.378900                                                         |
| 24199 | 1.143188              | 2.378906                                                         |
| 24201 | 1.444982              | 2.378913                                                         |
| 24203 | 1.000041              | 2.378919                                                         |
| 24205 | 1.237430              | 2.378925                                                         |
| 24207 | 1.333499              | 2.378931                                                         |
| 24209 | 1.025073              | 2.378937                                                         |
| 24211 | 1.141960              | 2.378943                                                         |
| 24213 | 1.525131              | 2.378949                                                         |

| $n$   | $\frac{\sigma(n)}{n}$ | $\frac{e^\gamma}{2} \log \log n + \frac{0.73...}{\log \log n}$ |
|-------|-----------------------|----------------------------------------------------------------|
| 24215 | 1.248813              | 2.378956                                                       |
| 24217 | 1.018954              | 2.378962                                                       |
| 24219 | 1.678682              | 2.378968                                                       |
| 24221 | 1.021097              | 2.378974                                                       |
| 24223 | 1.000041              | 2.378980                                                       |
| 24225 | 1.842724              | 2.378986                                                       |
| 24227 | 1.143187              | 2.378993                                                       |
| 24229 | 1.000041              | 2.378999                                                       |
| 24231 | 1.372787              | 2.379005                                                       |
| 24233 | 1.091404              | 2.379011                                                       |
| 24235 | 1.241840              | 2.379017                                                       |
| 24237 | 1.444981              | 2.379023                                                       |
| 24239 | 1.000041              | 2.379029                                                       |
| 24241 | 1.143187              | 2.379036                                                       |
| 24243 | 1.333498              | 2.379042                                                       |
| 24245 | 1.295772              | 2.379048                                                       |
| 24247 | 1.000041              | 2.379054                                                       |
| 24249 | 1.365830              | 2.379060                                                       |
| 24251 | 1.000041              | 2.379066                                                       |
| 24253 | 1.015957              | 2.379072                                                       |
| 24255 | 2.199629              | 2.379079                                                       |
| 24257 | 1.013151              | 2.379085                                                       |
| 24259 | 1.059566              | 2.379091                                                       |
| 24261 | 1.333498              | 2.379097                                                       |
| 24263 | 1.053456              | 2.379103                                                       |
| 24265 | 1.258108              | 2.379109                                                       |
| 24267 | 1.333498              | 2.379115                                                       |
| 24269 | 1.143187              | 2.379122                                                       |
| 24271 | 1.077500              | 2.379128                                                       |
| 24273 | 1.582005              | 2.379134                                                       |
| 24275 | 1.241277              | 2.379140                                                       |
| 24277 | 1.091403              | 2.379146                                                       |
| 24279 | 1.333498              | 2.379152                                                       |
| 24281 | 1.000041              | 2.379158                                                       |
| 24283 | 1.143187              | 2.379165                                                       |
| 24285 | 1.600988              | 2.379171                                                       |
| 24287 | 1.012888              | 2.379177                                                       |
| 24289 | 1.013792              | 2.379183                                                       |
| 24291 | 1.444980              | 2.379189                                                       |
| 24293 | 1.059564              | 2.379195                                                       |
| 24295 | 1.238773              | 2.379201                                                       |
| 24297 | 1.659464              | 2.379207                                                       |
| 24299 | 1.114614              | 2.379214                                                       |
| 24301 | 1.053455              | 2.379220                                                       |

| $n$   | $\frac{\sigma(n)}{n}$ | $\frac{e^\gamma}{2} \log \log n + \frac{0.73...}{\log \log n}$ |
|-------|-----------------------|----------------------------------------------------------------|
| 24303 | 1.333498              | 2.379226                                                       |
| 24305 | 1.200247              | 2.379232                                                       |
| 24307 | 1.013700              | 2.379238                                                       |
| 24309 | 1.503805              | 2.379244                                                       |
| 24311 | 1.200444              | 2.379250                                                       |
| 24313 | 1.026118              | 2.379257                                                       |
| 24315 | 1.600987              | 2.379263                                                       |
| 24317 | 1.000041              | 2.379269                                                       |
| 24319 | 1.015502              | 2.379275                                                       |
| 24321 | 1.487439              | 2.379281                                                       |
| 24323 | 1.077499              | 2.379287                                                       |
| 24325 | 1.427338              | 2.379293                                                       |
| 24327 | 1.598224              | 2.379299                                                       |
| 24329 | 1.000041              | 2.379306                                                       |
| 24331 | 1.035716              | 2.379312                                                       |
| 24333 | 1.333498              | 2.379318                                                       |
| 24335 | 1.246600              | 2.379324                                                       |
| 24337 | 1.000041              | 2.379330                                                       |
| 24339 | 1.630305              | 2.379336                                                       |
| 24341 | 1.014091              | 2.379342                                                       |
| 24343 | 1.091402              | 2.379348                                                       |
| 24345 | 1.736537              | 2.379354                                                       |
| 24347 | 1.014334              | 2.379361                                                       |
| 24349 | 1.077498              | 2.379367                                                       |
| 24351 | 1.333498              | 2.379373                                                       |
| 24353 | 1.182606              | 2.379379                                                       |
| 24355 | 1.200246              | 2.379385                                                       |
| 24357 | 1.395246              | 2.379391                                                       |
| 24359 | 1.000041              | 2.379397                                                       |
| 24361 | 1.059562              | 2.379403                                                       |
| 24363 | 1.444978              | 2.379410                                                       |
| 24365 | 1.312046              | 2.379416                                                       |
| 24367 | 1.162556              | 2.379422                                                       |
| 24369 | 1.333497              | 2.379428                                                       |
| 24371 | 1.000041              | 2.379434                                                       |
| 24373 | 1.000041              | 2.379440                                                       |
| 24375 | 1.794297              | 2.379446                                                       |
| 24377 | 1.053452              | 2.379452                                                       |
| 24379 | 1.000041              | 2.379458                                                       |
| 24381 | 1.746934              | 2.379465                                                       |
| 24383 | 1.028585              | 2.379471                                                       |
| 24385 | 1.200246              | 2.379477                                                       |
| 24387 | 1.456514              | 2.379483                                                       |
| 24389 | 1.035713              | 2.379489                                                       |

| $n$   | $\frac{\sigma(n)}{n}$ | $\frac{e^\gamma}{2} \log \log n + \frac{0.73\dots}{\log \log n}$ |
|-------|-----------------------|------------------------------------------------------------------|
| 24391 | 1.000041              | 2.379495                                                         |
| 24393 | 1.369573              | 2.379501                                                         |
| 24395 | 1.487518              | 2.379507                                                         |
| 24397 | 1.033570              | 2.379513                                                         |
| 24399 | 1.444977              | 2.379519                                                         |
| 24401 | 1.077497              | 2.379526                                                         |
| 24403 | 1.044462              | 2.379532                                                         |
| 24405 | 1.600983              | 2.379538                                                         |
| 24407 | 1.000041              | 2.379544                                                         |
| 24409 | 1.250686              | 2.379550                                                         |
| 24411 | 1.363320              | 2.379556                                                         |
| 24413 | 1.000041              | 2.379562                                                         |
| 24415 | 1.268073              | 2.379568                                                         |
| 24417 | 1.444977              | 2.379574                                                         |
| 24419 | 1.000041              | 2.379580                                                         |
| 24421 | 1.000041              | 2.379587                                                         |
| 24423 | 1.525120              | 2.379593                                                         |
| 24425 | 1.241269              | 2.379599                                                         |
| 24427 | 1.077496              | 2.379605                                                         |
| 24429 | 1.414712              | 2.379611                                                         |
| 24431 | 1.091400              | 2.379617                                                         |
| 24433 | 1.021078              | 2.379623                                                         |
| 24435 | 1.787600              | 2.379629                                                         |
| 24437 | 1.143185              | 2.379635                                                         |
| 24439 | 1.000041              | 2.379641                                                         |
| 24441 | 1.333497              | 2.379648                                                         |
| 24443 | 1.000041              | 2.379654                                                         |
| 24445 | 1.200245              | 2.379660                                                         |
| 24447 | 1.384219              | 2.379666                                                         |
| 24449 | 1.044460              | 2.379672                                                         |
| 24451 | 1.165596              | 2.379678                                                         |
| 24453 | 1.786284              | 2.379684                                                         |
| 24455 | 1.234594              | 2.379690                                                         |
| 24457 | 1.028581              | 2.379696                                                         |
| 24459 | 1.381577              | 2.379702                                                         |
| 24461 | 1.018928              | 2.379708                                                         |
| 24463 | 1.059559              | 2.379714                                                         |
| 24465 | 1.836419              | 2.379721                                                         |
| 24467 | 1.025054              | 2.379727                                                         |
| 24469 | 1.000041              | 2.379733                                                         |
| 24471 | 1.444976              | 2.379739                                                         |
| 24473 | 1.000041              | 2.379745                                                         |
| 24475 | 1.367926              | 2.379751                                                         |
| 24477 | 1.372717              | 2.379757                                                         |

| $n$   | $\frac{\sigma(n)}{n}$ | $\frac{e^\gamma}{2} \log \log n + \frac{0.73...}{\log \log n}$ |
|-------|-----------------------|----------------------------------------------------------------|
| 24479 | 1.235345              | 2.379763                                                       |
| 24481 | 1.000041              | 2.379769                                                       |
| 24483 | 1.333497              | 2.379775                                                       |
| 24485 | 1.235042              | 2.379781                                                       |
| 24487 | 1.023237              | 2.379787                                                       |
| 24489 | 1.483115              | 2.379794                                                       |
| 24491 | 1.053448              | 2.379800                                                       |
| 24493 | 1.143184              | 2.379806                                                       |
| 24495 | 1.693080              | 2.379812                                                       |
| 24497 | 1.163898              | 2.379818                                                       |
| 24499 | 1.000041              | 2.379824                                                       |
| 24501 | 1.333497              | 2.379830                                                       |
| 24503 | 1.013753              | 2.379836                                                       |
| 24505 | 1.344215              | 2.379842                                                       |
| 24507 | 1.655037              | 2.379848                                                       |
| 24509 | 1.000041              | 2.379854                                                       |
| 24511 | 1.013096              | 2.379860                                                       |
| 24513 | 1.333497              | 2.379866                                                       |
| 24515 | 1.200245              | 2.379873                                                       |
| 24517 | 1.000041              | 2.379879                                                       |
| 24519 | 1.456503              | 2.379885                                                       |
| 24521 | 1.190164              | 2.379891                                                       |
| 24523 | 1.012927              | 2.379897                                                       |
| 24525 | 1.807543              | 2.379903                                                       |
| 24527 | 1.000041              | 2.379909                                                       |
| 24529 | 1.053447              | 2.379915                                                       |
| 24531 | 1.561453              | 2.379921                                                       |
| 24533 | 1.000041              | 2.379927                                                       |
| 24535 | 1.373385              | 2.379933                                                       |
| 24537 | 1.333496              | 2.379939                                                       |
| 24539 | 1.021069              | 2.379945                                                       |
| 24541 | 1.150075              | 2.379951                                                       |
| 24543 | 1.512773              | 2.379958                                                       |
| 24545 | 1.200244              | 2.379964                                                       |
| 24547 | 1.000041              | 2.379970                                                       |
| 24549 | 1.560308              | 2.379976                                                       |
| 24551 | 1.000041              | 2.379982                                                       |
| 24553 | 1.025048              | 2.379988                                                       |
| 24555 | 1.600977              | 2.379994                                                       |
| 24557 | 1.077493              | 2.380000                                                       |
| 24559 | 1.026100              | 2.380006                                                       |
| 24561 | 1.444974              | 2.380012                                                       |
| 24563 | 1.299516              | 2.380018                                                       |
| 24565 | 1.274985              | 2.380024                                                       |

| $n$   | $\frac{\sigma(n)}{n}$ | $\frac{e^\gamma}{2} \log \log n + \frac{0.73\dots}{\log \log n}$ |
|-------|-----------------------|------------------------------------------------------------------|
| 24567 | 1.406765              | 2.380030                                                         |
| 24569 | 1.015914              | 2.380036                                                         |
| 24571 | 1.000041              | 2.380042                                                         |
| 24573 | 1.333496              | 2.380048                                                         |
| 24575 | 1.241261              | 2.380054                                                         |
| 24577 | 1.143183              | 2.380061                                                         |
| 24579 | 1.444973              | 2.380067                                                         |
| 24581 | 1.023229              | 2.380073                                                         |
| 24583 | 1.129887              | 2.380079                                                         |
| 24585 | 1.757169              | 2.380085                                                         |
| 24587 | 1.044454              | 2.380091                                                         |
| 24589 | 1.017691              | 2.380097                                                         |
| 24591 | 1.525111              | 2.380103                                                         |
| 24593 | 1.000041              | 2.380109                                                         |
| 24595 | 1.200244              | 2.380115                                                         |
| 24597 | 1.483108              | 2.380121                                                         |
| 24599 | 1.059555              | 2.380127                                                         |
| 24601 | 1.016707              | 2.380133                                                         |
| 24603 | 1.365687              | 2.380139                                                         |
| 24605 | 1.482625              | 2.380145                                                         |
| 24607 | 1.091397              | 2.380151                                                         |
| 24609 | 1.438173              | 2.380157                                                         |
| 24611 | 1.000041              | 2.380163                                                         |
| 24613 | 1.012798              | 2.380169                                                         |
| 24615 | 1.736502              | 2.380175                                                         |
| 24617 | 1.013933              | 2.380182                                                         |
| 24619 | 1.143182              | 2.380188                                                         |
| 24621 | 1.384184              | 2.380194                                                         |
| 24623 | 1.000041              | 2.380200                                                         |
| 24625 | 1.254335              | 2.380206                                                         |
| 24627 | 1.333496              | 2.380212                                                         |
| 24629 | 1.091396              | 2.380218                                                         |
| 24631 | 1.000041              | 2.380224                                                         |
| 24633 | 1.823895              | 2.380230                                                         |
| 24635 | 1.295717              | 2.380236                                                         |
| 24637 | 1.017007              | 2.380242                                                         |
| 24639 | 1.371484              | 2.380248                                                         |
| 24641 | 1.026095              | 2.380254                                                         |
| 24643 | 1.053443              | 2.380260                                                         |
| 24645 | 1.682775              | 2.380266                                                         |
| 24647 | 1.165578              | 2.380272                                                         |
| 24649 | 1.006410              | 2.380278                                                         |
| 24651 | 1.635633              | 2.380284                                                         |
| 24653 | 1.014887              | 2.380290                                                         |

| $n$   | $\frac{\sigma(n)}{n}$ | $\frac{e^\gamma}{2} \log \log n + \frac{0.73\dots}{\log \log n}$ |
|-------|-----------------------|------------------------------------------------------------------|
| 24655 | 1.200243              | 2.380296                                                         |
| 24657 | 1.333496              | 2.380302                                                         |
| 24659 | 1.000041              | 2.380308                                                         |
| 24661 | 1.235311              | 2.380314                                                         |
| 24663 | 1.333496              | 2.380320                                                         |
| 24665 | 1.200243              | 2.380326                                                         |
| 24667 | 1.059553              | 2.380333                                                         |
| 24669 | 1.444971              | 2.380339                                                         |
| 24671 | 1.000041              | 2.380345                                                         |
| 24673 | 1.091395              | 2.380351                                                         |
| 24675 | 1.929726              | 2.380357                                                         |
| 24677 | 1.000041              | 2.380363                                                         |
| 24679 | 1.108635              | 2.380369                                                         |
| 24681 | 1.406750              | 2.380375                                                         |
| 24683 | 1.000041              | 2.380381                                                         |
| 24685 | 1.200243              | 2.380387                                                         |
| 24687 | 1.562928              | 2.380393                                                         |
| 24689 | 1.143181              | 2.380399                                                         |
| 24691 | 1.000041              | 2.380405                                                         |
| 24693 | 1.333495              | 2.380411                                                         |
| 24695 | 1.312006              | 2.380417                                                         |
| 24697 | 1.000040              | 2.380423                                                         |
| 24699 | 1.333495              | 2.380429                                                         |
| 24701 | 1.059552              | 2.380435                                                         |
| 24703 | 1.143181              | 2.380441                                                         |
| 24705 | 1.821979              | 2.380447                                                         |
| 24707 | 1.033553              | 2.380453                                                         |
| 24709 | 1.000040              | 2.380459                                                         |
| 24711 | 1.333495              | 2.380465                                                         |
| 24713 | 1.077490              | 2.380471                                                         |
| 24715 | 1.200243              | 2.380477                                                         |
| 24717 | 1.677874              | 2.380483                                                         |
| 24719 | 1.053441              | 2.380489                                                         |
| 24721 | 1.019376              | 2.380495                                                         |
| 24723 | 1.501759              | 2.380501                                                         |
| 24725 | 1.324004              | 2.380507                                                         |
| 24727 | 1.015894              | 2.380513                                                         |
| 24729 | 1.333495              | 2.380519                                                         |
| 24731 | 1.143181              | 2.380525                                                         |
| 24733 | 1.000040              | 2.380531                                                         |
| 24735 | 1.711583              | 2.380537                                                         |
| 24737 | 1.035696              | 2.380543                                                         |
| 24739 | 1.181616              | 2.380549                                                         |
| 24741 | 1.444970              | 2.380555                                                         |

| $n$   | $\frac{\sigma(n)}{n}$ | $\frac{e^\gamma}{2} \log \log n + \frac{0.73...}{\log \log n}$ |
|-------|-----------------------|----------------------------------------------------------------|
| 24743 | 1.013620              | 2.380561                                                       |
| 24745 | 1.409739              | 2.380567                                                       |
| 24747 | 1.363559              | 2.380573                                                       |
| 24749 | 1.000040              | 2.380579                                                       |
| 24751 | 1.021050              | 2.380585                                                       |
| 24753 | 1.375510              | 2.380591                                                       |
| 24755 | 1.200242              | 2.380597                                                       |
| 24757 | 1.053439              | 2.380603                                                       |
| 24759 | 1.706046              | 2.380609                                                       |
| 24761 | 1.091394              | 2.380615                                                       |
| 24763 | 1.000040              | 2.380621                                                       |
| 24765 | 1.736644              | 2.380627                                                       |
| 24767 | 1.000040              | 2.380633                                                       |
| 24769 | 1.116234              | 2.380639                                                       |
| 24771 | 1.395180              | 2.380645                                                       |
| 24773 | 1.143180              | 2.380651                                                       |
| 24775 | 1.241251              | 2.380657                                                       |
| 24777 | 1.444969              | 2.380663                                                       |
| 24779 | 1.016990              | 2.380669                                                       |
| 24781 | 1.000040              | 2.380675                                                       |
| 24783 | 1.456482              | 2.380681                                                       |
| 24785 | 1.200242              | 2.380687                                                       |
| 24787 | 1.143180              | 2.380693                                                       |
| 24789 | 1.333495              | 2.380699                                                       |
| 24791 | 1.077488              | 2.380705                                                       |
| 24793 | 1.000040              | 2.380711                                                       |
| 24795 | 1.887477              | 2.380717                                                       |
| 24797 | 1.012864              | 2.380723                                                       |
| 24799 | 1.000040              | 2.380729                                                       |
| 24801 | 1.525100              | 2.380735                                                       |
| 24803 | 1.059549              | 2.380741                                                       |
| 24805 | 1.351179              | 2.380747                                                       |
| 24807 | 1.333495              | 2.380753                                                       |
| 24809 | 1.000040              | 2.380759                                                       |
| 24811 | 1.025029              | 2.380765                                                       |
| 24813 | 1.483094              | 2.380771                                                       |
| 24815 | 1.373363              | 2.380777                                                       |
| 24817 | 1.137285              | 2.380783                                                       |
| 24819 | 1.333495              | 2.380789                                                       |
| 24821 | 1.000040              | 2.380795                                                       |
| 24823 | 1.013898              | 2.380801                                                       |
| 24825 | 1.658328              | 2.380807                                                       |
| 24827 | 1.138760              | 2.380813                                                       |
| 24829 | 1.143179              | 2.380819                                                       |



| $n$   | $\frac{\sigma(n)}{n}$ | $\frac{e^\gamma}{2} \log \log n + \frac{0.73...}{\log \log n}$ |
|-------|-----------------------|----------------------------------------------------------------|
| 24831 | 1.507793              | 2.380825                                                       |
| 24833 | 1.053437              | 2.380831                                                       |
| 24835 | 1.200242              | 2.380837                                                       |
| 24837 | 1.414664              | 2.380843                                                       |
| 24839 | 1.019365              | 2.380849                                                       |
| 24841 | 1.000040              | 2.380855                                                       |
| 24843 | 1.679507              | 2.380861                                                       |
| 24845 | 1.200241              | 2.380867                                                       |
| 24847 | 1.000040              | 2.380873                                                       |
| 24849 | 1.582035              | 2.380879                                                       |
| 24851 | 1.000040              | 2.380885                                                       |
| 24853 | 1.035690              | 2.380891                                                       |
| 24855 | 1.600966              | 2.380897                                                       |
| 24857 | 1.181800              | 2.380903                                                       |
| 24859 | 1.000040              | 2.380909                                                       |
| 24861 | 1.333494              | 2.380915                                                       |
| 24863 | 1.067611              | 2.380921                                                       |
| 24865 | 1.200241              | 2.380927                                                       |
| 24867 | 1.498693              | 2.380933                                                       |
| 24869 | 1.077486              | 2.380939                                                       |
| 24871 | 1.389570              | 2.380945                                                       |
| 24873 | 1.333494              | 2.380951                                                       |
| 24875 | 1.254271              | 2.380957                                                       |
| 24877 | 1.000040              | 2.380963                                                       |
| 24879 | 1.333494              | 2.380969                                                       |
| 24881 | 1.012821              | 2.380975                                                       |
| 24883 | 1.012740              | 2.380981                                                       |
| 24885 | 2.006028              | 2.380987                                                       |
| 24887 | 1.026078              | 2.380993                                                       |
| 24889 | 1.000040              | 2.380999                                                       |
| 24891 | 1.333494              | 2.381005                                                       |
| 24893 | 1.141526              | 2.381011                                                       |
| 24895 | 1.295682              | 2.381017                                                       |
| 24897 | 1.371410              | 2.381023                                                       |
| 24899 | 1.143178              | 2.381029                                                       |
| 24901 | 1.028553              | 2.381035                                                       |
| 24903 | 1.444966              | 2.381041                                                       |
| 24905 | 1.274925              | 2.381047                                                       |
| 24907 | 1.000040              | 2.381053                                                       |
| 24909 | 1.468385              | 2.381058                                                       |
| 24911 | 1.035687              | 2.381064                                                       |
| 24913 | 1.143178              | 2.381070                                                       |
| 24915 | 1.757014              | 2.381076                                                       |
| 24917 | 1.000040              | 2.381082                                                       |

| $n$   | $\frac{\sigma(n)}{n}$ | $\frac{e^\gamma}{2} \log \log n + \frac{0.73...}{\log \log n}$ |
|-------|-----------------------|----------------------------------------------------------------|
| 24919 | 1.000040              | 2.381088                                                       |
| 24921 | 1.617913              | 2.381094                                                       |
| 24923 | 1.000040              | 2.381100                                                       |
| 24925 | 1.241244              | 2.381106                                                       |
| 24927 | 1.525093              | 2.381112                                                       |
| 24929 | 1.014240              | 2.381118                                                       |
| 24931 | 1.013678              | 2.381124                                                       |
| 24933 | 1.333494              | 2.381130                                                       |
| 24935 | 1.200241              | 2.381136                                                       |
| 24937 | 1.091390              | 2.381142                                                       |
| 24939 | 1.538795              | 2.381148                                                       |
| 24941 | 1.165551              | 2.381154                                                       |
| 24943 | 1.000040              | 2.381160                                                       |
| 24945 | 1.600962              | 2.381166                                                       |
| 24947 | 1.144827              | 2.381172                                                       |
| 24949 | 1.018879              | 2.381178                                                       |
| 24951 | 1.333494              | 2.381184                                                       |
| 24953 | 1.000040              | 2.381190                                                       |
| 24955 | 1.477219              | 2.381196                                                       |
| 24957 | 1.500180              | 2.381202                                                       |
| 24959 | 1.091390              | 2.381208                                                       |
| 24961 | 1.013581              | 2.381213                                                       |
| 24963 | 1.367143              | 2.381219                                                       |
| 24965 | 1.200240              | 2.381225                                                       |
| 24967 | 1.000040              | 2.381231                                                       |
| 24969 | 1.614802              | 2.381237                                                       |
| 24971 | 1.000040              | 2.381243                                                       |
| 24973 | 1.150362              | 2.381249                                                       |
| 24975 | 1.886687              | 2.381255                                                       |
| 24977 | 1.000040              | 2.381261                                                       |
| 24979 | 1.000040              | 2.381267                                                       |
| 24981 | 1.456467              | 2.381273                                                       |
| 24983 | 1.183525              | 2.381279                                                       |
| 24985 | 1.267961              | 2.381285                                                       |
| 24987 | 1.333493              | 2.381291                                                       |
| 24989 | 1.000040              | 2.381297                                                       |
| 24991 | 1.017646              | 2.381303                                                       |
| 24993 | 1.444965              | 2.381309                                                       |
| 24995 | 1.200240              | 2.381315                                                       |
| 24997 | 1.143177              | 2.381321                                                       |
| 24999 | 1.438138              | 2.381327                                                       |
| 25001 | 1.044438              | 2.381332                                                       |
| 25003 | 1.091389              | 2.381338                                                       |
| 25005 | 1.600960              | 2.381344                                                       |

| $n$   | $\frac{\sigma(n)}{n}$ | $\frac{e^\gamma}{2} \log \log n + \frac{0.73...}{\log \log n}$ |
|-------|-----------------------|----------------------------------------------------------------|
| 25007 | 1.059543              | 2.381350                                                       |
| 25009 | 1.014835              | 2.381356                                                       |
| 25011 | 1.654952              | 2.381362                                                       |
| 25013 | 1.000040              | 2.381368                                                       |
| 25015 | 1.200240              | 2.381374                                                       |
| 25017 | 1.381461              | 2.381380                                                       |
| 25019 | 1.012990              | 2.381386                                                       |
| 25021 | 1.012909              | 2.381392                                                       |
| 25023 | 1.406706              | 2.381398                                                       |
| 25025 | 1.664895              | 2.381404                                                       |
| 25027 | 1.035681              | 2.381410                                                       |
| 25029 | 1.512486              | 2.381416                                                       |
| 25031 | 1.000040              | 2.381422                                                       |
| 25033 | 1.000040              | 2.381428                                                       |
| 25035 | 1.600959              | 2.381433                                                       |
| 25037 | 1.000040              | 2.381439                                                       |
| 25039 | 1.182156              | 2.381445                                                       |
| 25041 | 1.414640              | 2.381451                                                       |
| 25043 | 1.015853              | 2.381457                                                       |
| 25045 | 1.200240              | 2.381463                                                       |
| 25047 | 1.656725              | 2.381469                                                       |
| 25049 | 1.028544              | 2.381475                                                       |
| 25051 | 1.126662              | 2.381481                                                       |
| 25053 | 1.525087              | 2.381487                                                       |
| 25055 | 1.200239              | 2.381493                                                       |
| 25057 | 1.000040              | 2.381499                                                       |
| 25059 | 1.333493              | 2.381505                                                       |
| 25061 | 1.053430              | 2.381511                                                       |
| 25063 | 1.016957              | 2.381516                                                       |
| 25065 | 1.736445              | 2.381522                                                       |
| 25067 | 1.143176              | 2.381528                                                       |
| 25069 | 1.137341              | 2.381534                                                       |
| 25071 | 1.365083              | 2.381540                                                       |
| 25073 | 1.000040              | 2.381546                                                       |
| 25075 | 1.335194              | 2.381552                                                       |
| 25077 | 1.438131              | 2.381558                                                       |
| 25079 | 1.033534              | 2.381564                                                       |
| 25081 | 1.143176              | 2.381570                                                       |
| 25083 | 1.483076              | 2.381576                                                       |
| 25085 | 1.248555              | 2.381582                                                       |
| 25087 | 1.000040              | 2.381588                                                       |
| 25089 | 1.333493              | 2.381594                                                       |
| 25091 | 1.091387              | 2.381599                                                       |
| 25093 | 1.044435              | 2.381605                                                       |

| $n$   | $\frac{\sigma(n)}{n}$ | $\frac{e^\gamma}{2} \log \log n + \frac{0.73...}{\log \log n}$ |
|-------|-----------------------|----------------------------------------------------------------|
| 25095 | 1.836222              | 2.381611                                                       |
| 25097 | 1.000040              | 2.381617                                                       |
| 25099 | 1.053428              | 2.381623                                                       |
| 25101 | 1.444962              | 2.381629                                                       |
| 25103 | 1.077481              | 2.381635                                                       |
| 25105 | 1.200239              | 2.381641                                                       |
| 25107 | 1.333493              | 2.381647                                                       |
| 25109 | 1.215819              | 2.381653                                                       |
| 25111 | 1.000040              | 2.381659                                                       |
| 25113 | 1.456457              | 2.381665                                                       |
| 25115 | 1.200239              | 2.381670                                                       |
| 25117 | 1.000040              | 2.381676                                                       |
| 25119 | 1.444962              | 2.381682                                                       |
| 25121 | 1.000040              | 2.381688                                                       |
| 25123 | 1.185846              | 2.381694                                                       |
| 25125 | 1.688836              | 2.381700                                                       |
| 25127 | 1.000040              | 2.381706                                                       |
| 25129 | 1.077480              | 2.381712                                                       |
| 25131 | 1.333492              | 2.381718                                                       |
| 25133 | 1.026061              | 2.381724                                                       |
| 25135 | 1.311955              | 2.381730                                                       |
| 25137 | 1.814059              | 2.381736                                                       |
| 25139 | 1.044433              | 2.381741                                                       |
| 25141 | 1.033531              | 2.381747                                                       |
| 25143 | 1.465219              | 2.381753                                                       |
| 25145 | 1.236985              | 2.381759                                                       |
| 25147 | 1.000040              | 2.381765                                                       |
| 25149 | 1.362758              | 2.381771                                                       |
| 25151 | 1.143175              | 2.381777                                                       |
| 25153 | 1.000040              | 2.381783                                                       |
| 25155 | 1.910078              | 2.381789                                                       |
| 25157 | 1.091386              | 2.381795                                                       |
| 25159 | 1.012759              | 2.381800                                                       |
| 25161 | 1.333492              | 2.381806                                                       |
| 25163 | 1.000040              | 2.381812                                                       |
| 25165 | 1.373336              | 2.381818                                                       |
| 25167 | 1.333492              | 2.381824                                                       |
| 25169 | 1.000040              | 2.381830                                                       |
| 25171 | 1.000040              | 2.381836                                                       |
| 25173 | 1.444961              | 2.381842                                                       |
| 25175 | 1.329891              | 2.381848                                                       |
| 25177 | 1.059538              | 2.381854                                                       |
| 25179 | 1.677588              | 2.381859                                                       |
| 25181 | 1.090108              | 2.381865                                                       |

| $n$   | $\frac{\sigma(n)}{n}$ | $\frac{e^\gamma}{2} \log \log n + \frac{0.73...}{\log \log n}$ |
|-------|-----------------------|----------------------------------------------------------------|
| 25183 | 1.000040              | 2.381871                                                       |
| 25185 | 1.692436              | 2.381877                                                       |
| 25187 | 1.014809              | 2.381883                                                       |
| 25189 | 1.000040              | 2.381889                                                       |
| 25191 | 1.498630              | 2.381895                                                       |
| 25193 | 1.181281              | 2.381901                                                       |
| 25195 | 1.200238              | 2.381907                                                       |
| 25197 | 1.375402              | 2.381913                                                       |
| 25199 | 1.013374              | 2.381918                                                       |
| 25201 | 1.142812              | 2.381924                                                       |
| 25203 | 1.381423              | 2.381930                                                       |
| 25205 | 1.217139              | 2.381936                                                       |
| 25207 | 1.235212              | 2.381942                                                       |
| 25209 | 1.444960              | 2.381948                                                       |
| 25211 | 1.059538              | 2.381954                                                       |
| 25213 | 1.053425              | 2.381960                                                       |
| 25215 | 1.639976              | 2.381966                                                       |
| 25217 | 1.012650              | 2.381971                                                       |
| 25219 | 1.000040              | 2.381977                                                       |
| 25221 | 1.525078              | 2.381983                                                       |
| 25223 | 1.091385              | 2.381989                                                       |
| 25225 | 1.241229              | 2.381995                                                       |
| 25227 | 1.444960              | 2.382001                                                       |
| 25229 | 1.000040              | 2.382007                                                       |
| 25231 | 1.044429              | 2.382013                                                       |
| 25233 | 1.438117              | 2.382019                                                       |
| 25235 | 1.409471              | 2.382024                                                       |
| 25237 | 1.000040              | 2.382030                                                       |
| 25239 | 1.369309              | 2.382036                                                       |
| 25241 | 1.024999              | 2.382042                                                       |
| 25243 | 1.000040              | 2.382048                                                       |
| 25245 | 2.053476              | 2.382054                                                       |
| 25247 | 1.000040              | 2.382060                                                       |
| 25249 | 1.143174              | 2.382066                                                       |
| 25251 | 1.406677              | 2.382072                                                       |
| 25253 | 1.000040              | 2.382077                                                       |
| 25255 | 1.200238              | 2.382083                                                       |
| 25257 | 1.333492              | 2.382089                                                       |
| 25259 | 1.130686              | 2.382095                                                       |
| 25261 | 1.000040              | 2.382101                                                       |
| 25263 | 1.654910              | 2.382107                                                       |
| 25265 | 1.246309              | 2.382113                                                       |
| 25267 | 1.091384              | 2.382119                                                       |
| 25269 | 1.333492              | 2.382124                                                       |

| $n$   | $\frac{\sigma(n)}{n}$ | $\frac{e^\gamma}{2} \log \log n + \frac{0.73\dots}{\log \log n}$ |
|-------|-----------------------|------------------------------------------------------------------|
| 25271 | 1.028531              | 2.382130                                                         |
| 25273 | 1.012939              | 2.382136                                                         |
| 25275 | 1.658239              | 2.382142                                                         |
| 25277 | 1.200142              | 2.382148                                                         |
| 25279 | 1.059536              | 2.382154                                                         |
| 25281 | 1.472212              | 2.382160                                                         |
| 25283 | 1.012854              | 2.382166                                                         |
| 25285 | 1.295630              | 2.382171                                                         |
| 25287 | 1.333492              | 2.382177                                                         |
| 25289 | 1.157816              | 2.382183                                                         |
| 25291 | 1.143173              | 2.382189                                                         |
| 25293 | 1.333491              | 2.382195                                                         |
| 25295 | 1.200237              | 2.382201                                                         |
| 25297 | 1.026051              | 2.382207                                                         |
| 25299 | 1.483063              | 2.382213                                                         |
| 25301 | 1.000040              | 2.382218                                                         |
| 25303 | 1.000040              | 2.382224                                                         |
| 25305 | 1.836159              | 2.382230                                                         |
| 25307 | 1.000040              | 2.382236                                                         |
| 25309 | 1.000040              | 2.382242                                                         |
| 25311 | 1.592983              | 2.382248                                                         |
| 25313 | 1.059535              | 2.382254                                                         |
| 25315 | 1.234367              | 2.382259                                                         |
| 25317 | 1.509658              | 2.382265                                                         |
| 25319 | 1.143173              | 2.382271                                                         |
| 25321 | 1.000039              | 2.382277                                                         |
| 25323 | 1.395095              | 2.382283                                                         |
| 25325 | 1.241224              | 2.382289                                                         |
| 25327 | 1.111857              | 2.382295                                                         |
| 25329 | 1.333491              | 2.382300                                                         |
| 25331 | 1.016620              | 2.382306                                                         |
| 25333 | 1.296017              | 2.382312                                                         |
| 25335 | 1.736412              | 2.382318                                                         |
| 25337 | 1.077476              | 2.382324                                                         |
| 25339 | 1.000039              | 2.382330                                                         |
| 25341 | 1.333491              | 2.382336                                                         |
| 25343 | 1.000039              | 2.382342                                                         |
| 25345 | 1.241428              | 2.382347                                                         |
| 25347 | 1.636170              | 2.382353                                                         |
| 25349 | 1.000039              | 2.382359                                                         |
| 25351 | 1.013925              | 2.382365                                                         |
| 25353 | 1.498600              | 2.382371                                                         |
| 25355 | 1.311931              | 2.382377                                                         |
| 25357 | 1.000039              | 2.382382                                                         |

| $n$   | $\frac{\sigma(n)}{n}$ | $\frac{e^\gamma}{2} \log \log n + \frac{0.73\dots}{\log \log n}$ |
|-------|-----------------------|------------------------------------------------------------------|
| 25359 | 1.362830              | 2.382388                                                         |
| 25361 | 1.143173              | 2.382394                                                         |
| 25363 | 1.077475              | 2.382400                                                         |
| 25365 | 1.703134              | 2.382406                                                         |
| 25367 | 1.000039              | 2.382412                                                         |
| 25369 | 1.044424              | 2.382418                                                         |
| 25371 | 1.444957              | 2.382423                                                         |
| 25373 | 1.000039              | 2.382429                                                         |
| 25375 | 1.475468              | 2.382435                                                         |
| 25377 | 1.456437              | 2.382441                                                         |
| 25379 | 1.026045              | 2.382447                                                         |
| 25381 | 1.059533              | 2.382453                                                         |
| 25383 | 1.333491              | 2.382459                                                         |
| 25385 | 1.200236              | 2.382464                                                         |
| 25387 | 1.020995              | 2.382470                                                         |
| 25389 | 1.835125              | 2.382476                                                         |
| 25391 | 1.000039              | 2.382482                                                         |
| 25393 | 1.017603              | 2.382488                                                         |
| 25395 | 1.600945              | 2.382494                                                         |
| 25397 | 1.013506              | 2.382499                                                         |
| 25399 | 1.091382              | 2.382505                                                         |
| 25401 | 1.333491              | 2.382511                                                         |
| 25403 | 1.209306              | 2.382517                                                         |
| 25405 | 1.200236              | 2.382523                                                         |
| 25407 | 1.483056              | 2.382529                                                         |
| 25409 | 1.000039              | 2.382535                                                         |
| 25411 | 1.000039              | 2.382540                                                         |
| 25413 | 1.371267              | 2.382546                                                         |
| 25415 | 1.427818              | 2.382552                                                         |
| 25417 | 1.143172              | 2.382558                                                         |
| 25419 | 1.375349              | 2.382564                                                         |
| 25421 | 1.091381              | 2.382570                                                         |
| 25423 | 1.000039              | 2.382575                                                         |
| 25425 | 1.806962              | 2.382581                                                         |
| 25427 | 1.023164              | 2.382587                                                         |
| 25429 | 1.019309              | 2.382593                                                         |
| 25431 | 1.559986              | 2.382599                                                         |
| 25433 | 1.035662              | 2.382605                                                         |
| 25435 | 1.200236              | 2.382610                                                         |
| 25437 | 1.364941              | 2.382616                                                         |
| 25439 | 1.000039              | 2.382622                                                         |
| 25441 | 1.144609              | 2.382628                                                         |
| 25443 | 1.581889              | 2.382634                                                         |
| 25445 | 1.373315              | 2.382640                                                         |

| $n$   | $\frac{\sigma(n)}{n}$ | $\frac{e^\gamma}{2} \log \log n + \frac{0.73...}{\log \log n}$ |
|-------|-----------------------|----------------------------------------------------------------|
| 25447 | 1.000039              | 2.382645                                                       |
| 25449 | 1.414594              | 2.382651                                                       |
| 25451 | 1.033515              | 2.382657                                                       |
| 25453 | 1.000039              | 2.382663                                                       |
| 25455 | 1.600943              | 2.382669                                                       |
| 25457 | 1.000039              | 2.382675                                                       |
| 25459 | 1.143171              | 2.382680                                                       |
| 25461 | 1.583598              | 2.382686                                                       |
| 25463 | 1.000039              | 2.382692                                                       |
| 25465 | 1.311918              | 2.382698                                                       |
| 25467 | 1.438096              | 2.382704                                                       |
| 25469 | 1.000039              | 2.382710                                                       |
| 25471 | 1.000039              | 2.382715                                                       |
| 25473 | 1.525066              | 2.382721                                                       |
| 25475 | 1.241217              | 2.382727                                                       |
| 25477 | 1.016603              | 2.382733                                                       |
| 25479 | 1.530672              | 2.382739                                                       |
| 25481 | 1.015345              | 2.382744                                                       |
| 25483 | 1.059530              | 2.382750                                                       |
| 25485 | 1.600942              | 2.382756                                                       |
| 25487 | 1.250520              | 2.382762                                                       |
| 25489 | 1.016909              | 2.382768                                                       |
| 25491 | 1.384018              | 2.382774                                                       |
| 25493 | 1.126898              | 2.382779                                                       |
| 25495 | 1.200235              | 2.382785                                                       |
| 25497 | 1.444954              | 2.382791                                                       |
| 25499 | 1.024981              | 2.382797                                                       |
| 25501 | 1.143171              | 2.382803                                                       |
| 25503 | 1.333490              | 2.382809                                                       |
| 25505 | 1.200235              | 2.382814                                                       |
| 25507 | 1.044419              | 2.382820                                                       |
| 25509 | 1.456427              | 2.382826                                                       |
| 25511 | 1.014151              | 2.382832                                                       |
| 25513 | 1.033512              | 2.382838                                                       |
| 25515 | 2.056202              | 2.382843                                                       |
| 25517 | 1.128659              | 2.382849                                                       |
| 25519 | 1.090011              | 2.382855                                                       |
| 25521 | 1.369225              | 2.382861                                                       |
| 25523 | 1.000039              | 2.382867                                                       |
| 25525 | 1.241214              | 2.382872                                                       |
| 25527 | 1.363889              | 2.382878                                                       |
| 25529 | 1.165498              | 2.382884                                                       |
| 25531 | 1.104383              | 2.382890                                                       |
| 25533 | 1.444954              | 2.382896                                                       |



| $n$   | $\frac{\sigma(n)}{n}$ | $\frac{e^\gamma}{2} \log \log n + \frac{0.73\dots}{\log \log n}$ |
|-------|-----------------------|------------------------------------------------------------------|
| 25535 | 1.200235              | 2.382902                                                         |
| 25537 | 1.000039              | 2.382907                                                         |
| 25539 | 1.333490              | 2.382913                                                         |
| 25541 | 1.000039              | 2.382919                                                         |
| 25543 | 1.183886              | 2.382925                                                         |
| 25545 | 1.736230              | 2.382931                                                         |
| 25547 | 1.019298              | 2.382936                                                         |
| 25549 | 1.035657              | 2.382942                                                         |
| 25551 | 1.538570              | 2.382948                                                         |
| 25553 | 1.149611              | 2.382954                                                         |
| 25555 | 1.267854              | 2.382960                                                         |
| 25557 | 1.525062              | 2.382965                                                         |
| 25559 | 1.018819              | 2.382971                                                         |
| 25561 | 1.000039              | 2.382977                                                         |
| 25563 | 1.333490              | 2.382983                                                         |
| 25565 | 1.200235              | 2.382989                                                         |
| 25567 | 1.028513              | 2.382994                                                         |
| 25569 | 1.483046              | 2.383000                                                         |
| 25571 | 1.235149              | 2.383006                                                         |
| 25573 | 1.013569              | 2.383012                                                         |
| 25575 | 1.861818              | 2.383018                                                         |
| 25577 | 1.000039              | 2.383023                                                         |
| 25579 | 1.000039              | 2.383029                                                         |
| 25581 | 1.333490              | 2.383035                                                         |
| 25583 | 1.000039              | 2.383041                                                         |
| 25585 | 1.485871              | 2.383047                                                         |
| 25587 | 1.444953              | 2.383052                                                         |
| 25589 | 1.000039              | 2.383058                                                         |
| 25591 | 1.012543              | 2.383064                                                         |
| 25593 | 1.406635              | 2.383070                                                         |
| 25595 | 1.200234              | 2.383076                                                         |
| 25597 | 1.181388              | 2.383081                                                         |
| 25599 | 1.620063              | 2.383087                                                         |
| 25601 | 1.000039              | 2.383093                                                         |
| 25603 | 1.000039              | 2.383099                                                         |
| 25605 | 1.736380              | 2.383105                                                         |
| 25607 | 1.035654              | 2.383110                                                         |
| 25609 | 1.000039              | 2.383116                                                         |
| 25611 | 1.333490              | 2.383122                                                         |
| 25613 | 1.143169              | 2.383128                                                         |
| 25615 | 1.236775              | 2.383134                                                         |
| 25617 | 1.333489              | 2.383139                                                         |
| 25619 | 1.163511              | 2.383145                                                         |
| 25621 | 1.000039              | 2.383151                                                         |

| $n$   | $\frac{\sigma(n)}{n}$ | $\frac{e^\gamma}{2} \log \log n + \frac{0.73...}{\log \log n}$ |
|-------|-----------------------|----------------------------------------------------------------|
| 25623 | 1.617297              | 2.383157                                                       |
| 25625 | 1.280078              | 2.383162                                                       |
| 25627 | 1.165490              | 2.383168                                                       |
| 25629 | 1.333489              | 2.383174                                                       |
| 25631 | 1.070266              | 2.383180                                                       |
| 25633 | 1.000039              | 2.383186                                                       |
| 25635 | 1.600936              | 2.383191                                                       |
| 25637 | 1.033506              | 2.383197                                                       |
| 25639 | 1.000039              | 2.383203                                                       |
| 25641 | 1.849538              | 2.383209                                                       |
| 25643 | 1.000039              | 2.383215                                                       |
| 25645 | 1.257789              | 2.383220                                                       |
| 25647 | 1.362499              | 2.383226                                                       |
| 25649 | 1.077469              | 2.383232                                                       |
| 25651 | 1.013294              | 2.383238                                                       |
| 25653 | 1.414571              | 2.383243                                                       |
| 25655 | 1.373300              | 2.383249                                                       |
| 25657 | 1.000039              | 2.383255                                                       |
| 25659 | 1.444951              | 2.383261                                                       |
| 25661 | 1.017575              | 2.383267                                                       |
| 25663 | 1.091377              | 2.383272                                                       |
| 25665 | 1.683226              | 2.383278                                                       |
| 25667 | 1.000039              | 2.383284                                                       |
| 25669 | 1.209241              | 2.383290                                                       |
| 25671 | 1.371197              | 2.383295                                                       |
| 25673 | 1.000039              | 2.383301                                                       |
| 25675 | 1.352288              | 2.383307                                                       |
| 25677 | 1.498540              | 2.383313                                                       |
| 25679 | 1.000039              | 2.383319                                                       |
| 25681 | 1.018808              | 2.383324                                                       |
| 25683 | 1.525055              | 2.383330                                                       |
| 25685 | 1.311894              | 2.383336                                                       |
| 25687 | 1.059524              | 2.383342                                                       |
| 25689 | 1.333489              | 2.383347                                                       |
| 25691 | 1.044412              | 2.383353                                                       |
| 25693 | 1.000039              | 2.383359                                                       |
| 25695 | 1.736369              | 2.383365                                                       |
| 25697 | 1.143168              | 2.383371                                                       |
| 25699 | 1.033503              | 2.383376                                                       |
| 25701 | 1.438076              | 2.383382                                                       |
| 25703 | 1.000039              | 2.383388                                                       |
| 25705 | 1.235246              | 2.383394                                                       |
| 25707 | 1.568444              | 2.383399                                                       |
| 25709 | 1.023144              | 2.383405                                                       |

| $n$   | $\frac{\sigma(n)}{n}$ | $\frac{e^\gamma}{2} \log \log n + \frac{0.73...}{\log \log n}$ |
|-------|-----------------------|----------------------------------------------------------------|
| 25711 | 1.143168              | 2.383411                                                       |
| 25713 | 1.444950              | 2.383417                                                       |
| 25715 | 1.241299              | 2.383422                                                       |
| 25717 | 1.000039              | 2.383428                                                       |
| 25719 | 1.333489              | 2.383434                                                       |
| 25721 | 1.074220              | 2.383440                                                       |
| 25723 | 1.035649              | 2.383446                                                       |
| 25725 | 1.928086              | 2.383451                                                       |
| 25727 | 1.077467              | 2.383457                                                       |
| 25729 | 1.091375              | 2.383463                                                       |
| 25731 | 1.483036              | 2.383469                                                       |
| 25733 | 1.000039              | 2.383474                                                       |
| 25735 | 1.200233              | 2.383480                                                       |
| 25737 | 1.395034              | 2.383486                                                       |
| 25739 | 1.143168              | 2.383492                                                       |
| 25741 | 1.000039              | 2.383497                                                       |
| 25743 | 1.333489              | 2.383503                                                       |
| 25745 | 1.267819              | 2.383509                                                       |
| 25747 | 1.000039              | 2.383515                                                       |
| 25749 | 1.444949              | 2.383520                                                       |
| 25751 | 1.091375              | 2.383526                                                       |
| 25753 | 1.235118              | 2.383532                                                       |
| 25755 | 1.710891              | 2.383538                                                       |
| 25757 | 1.024964              | 2.383543                                                       |
| 25759 | 1.000039              | 2.383549                                                       |
| 25761 | 1.381313              | 2.383555                                                       |
| 25763 | 1.000039              | 2.383561                                                       |
| 25765 | 1.200233              | 2.383566                                                       |
| 25767 | 1.654830              | 2.383572                                                       |
| 25769 | 1.016570              | 2.383578                                                       |
| 25771 | 1.000039              | 2.383584                                                       |
| 25773 | 1.486206              | 2.383589                                                       |
| 25775 | 1.241203              | 2.383595                                                       |
| 25777 | 1.012531              | 2.383601                                                       |
| 25779 | 1.438070              | 2.383607                                                       |
| 25781 | 1.191575              | 2.383612                                                       |
| 25783 | 1.117015              | 2.383618                                                       |
| 25785 | 1.787086              | 2.383624                                                       |
| 25787 | 1.013534              | 2.383630                                                       |
| 25789 | 1.113963              | 2.383635                                                       |
| 25791 | 1.333488              | 2.383641                                                       |
| 25793 | 1.000039              | 2.383647                                                       |
| 25795 | 1.518434              | 2.383653                                                       |
| 25797 | 1.333488              | 2.383658                                                       |

| $n$   | $\frac{\sigma(n)}{n}$ | $\frac{e^\gamma}{2} \log \log n + \frac{0.73...}{\log \log n}$ |
|-------|-----------------------|----------------------------------------------------------------|
| 25799 | 1.000039              | 2.383664                                                       |
| 25801 | 1.000039              | 2.383670                                                       |
| 25803 | 1.499361              | 2.383676                                                       |
| 25805 | 1.295563              | 2.383681                                                       |
| 25807 | 1.012748              | 2.383687                                                       |
| 25809 | 1.525049              | 2.383693                                                       |
| 25811 | 1.020960              | 2.383699                                                       |
| 25813 | 1.015302              | 2.383704                                                       |
| 25815 | 1.600930              | 2.383710                                                       |
| 25817 | 1.091374              | 2.383716                                                       |
| 25819 | 1.000039              | 2.383722                                                       |
| 25821 | 1.530537              | 2.383727                                                       |
| 25823 | 1.271425              | 2.383733                                                       |
| 25825 | 1.241200              | 2.383739                                                       |
| 25827 | 1.333488              | 2.383745                                                       |
| 25829 | 1.044407              | 2.383750                                                       |
| 25831 | 1.077465              | 2.383756                                                       |
| 25833 | 1.362598              | 2.383762                                                       |
| 25835 | 1.200232              | 2.383768                                                       |
| 25837 | 1.143167              | 2.383773                                                       |
| 25839 | 1.685824              | 2.383779                                                       |
| 25841 | 1.000039              | 2.383785                                                       |
| 25843 | 1.024958              | 2.383790                                                       |
| 25845 | 1.600929              | 2.383796                                                       |
| 25847 | 1.000039              | 2.383802                                                       |
| 25849 | 1.000039              | 2.383808                                                       |
| 25851 | 1.525047              | 2.383813                                                       |
| 25853 | 1.013731              | 2.383819                                                       |
| 25855 | 1.200232              | 2.383825                                                       |
| 25857 | 1.656109              | 2.383831                                                       |
| 25859 | 1.053405              | 2.383836                                                       |
| 25861 | 1.091373              | 2.383842                                                       |
| 25863 | 1.375246              | 2.383848                                                       |
| 25865 | 1.373284              | 2.383854                                                       |
| 25867 | 1.000039              | 2.383859                                                       |
| 25869 | 1.333488              | 2.383865                                                       |
| 25871 | 1.026014              | 2.383871                                                       |
| 25873 | 1.000039              | 2.383876                                                       |
| 25875 | 1.881043              | 2.383882                                                       |
| 25877 | 1.013255              | 2.383888                                                       |
| 25879 | 1.143166              | 2.383894                                                       |
| 25881 | 1.333488              | 2.383899                                                       |
| 25883 | 1.181316              | 2.383905                                                       |
| 25885 | 1.246127              | 2.383911                                                       |

| $n$   | $\frac{\sigma(n)}{n}$ | $\frac{e^\gamma}{2} \log \log n + \frac{0.73...}{\log \log n}$ |
|-------|-----------------------|----------------------------------------------------------------|
| 25887 | 1.333488              | 2.383917                                                       |
| 25889 | 1.000039              | 2.383922                                                       |
| 25891 | 1.059519              | 2.383928                                                       |
| 25893 | 1.705480              | 2.383934                                                       |
| 25895 | 1.200232              | 2.383939                                                       |
| 25897 | 1.112098              | 2.383945                                                       |
| 25899 | 1.362215              | 2.383951                                                       |
| 25901 | 1.019266              | 2.383957                                                       |
| 25903 | 1.000039              | 2.383962                                                       |
| 25905 | 1.756572              | 2.383968                                                       |
| 25907 | 1.143166              | 2.383974                                                       |
| 25909 | 1.077463              | 2.383979                                                       |
| 25911 | 1.444946              | 2.383985                                                       |
| 25913 | 1.000039              | 2.383991                                                       |
| 25915 | 1.233571              | 2.383997                                                       |
| 25917 | 1.366825              | 2.384002                                                       |
| 25919 | 1.000039              | 2.384008                                                       |
| 25921 | 1.216041              | 2.384014                                                       |
| 25923 | 1.333488              | 2.384019                                                       |
| 25925 | 1.334465              | 2.384025                                                       |
| 25927 | 1.091372              | 2.384031                                                       |
| 25929 | 1.500096              | 2.384037                                                       |
| 25931 | 1.000039              | 2.384042                                                       |
| 25933 | 1.000039              | 2.384048                                                       |
| 25935 | 2.072874              | 2.384054                                                       |
| 25937 | 1.028492              | 2.384059                                                       |
| 25939 | 1.000039              | 2.384065                                                       |
| 25941 | 1.333488              | 2.384071                                                       |
| 25943 | 1.000039              | 2.384077                                                       |
| 25945 | 1.200231              | 2.384082                                                       |
| 25947 | 1.530813              | 2.384088                                                       |
| 25949 | 1.250453              | 2.384094                                                       |
| 25951 | 1.000039              | 2.384099                                                       |
| 25953 | 1.372327              | 2.384105                                                       |
| 25955 | 1.248314              | 2.384111                                                       |
| 25957 | 1.013831              | 2.384117                                                       |
| 25959 | 1.414538              | 2.384122                                                       |
| 25961 | 1.077462              | 2.384128                                                       |
| 25963 | 1.143165              | 2.384134                                                       |
| 25965 | 1.736337              | 2.384139                                                       |
| 25967 | 1.044403              | 2.384145                                                       |
| 25969 | 1.000039              | 2.384151                                                       |
| 25971 | 1.456394              | 2.384157                                                       |
| 25973 | 1.053402              | 2.384162                                                       |

| $n$   | $\frac{\sigma(n)}{n}$ | $\frac{e^\gamma}{2} \log \log n + \frac{0.73\dots}{\log \log n}$ |
|-------|-----------------------|------------------------------------------------------------------|
| 25975 | 1.241193              | 2.384168                                                         |
| 25977 | 1.525041              | 2.384174                                                         |
| 25979 | 1.015282              | 2.384179                                                         |
| 25981 | 1.000038              | 2.384185                                                         |
| 25983 | 1.444945              | 2.384191                                                         |
| 25985 | 1.200231              | 2.384196                                                         |
| 25987 | 1.077462              | 2.384202                                                         |
| 25989 | 1.333487              | 2.384208                                                         |
| 25991 | 1.181948              | 2.384214                                                         |
| 25993 | 1.163390              | 2.384219                                                         |
| 25995 | 1.600923              | 2.384225                                                         |
| 25997 | 1.000038              | 2.384231                                                         |
| 25999 | 1.000038              | 2.384236                                                         |
| 26001 | 1.511942              | 2.384242                                                         |
| 26003 | 1.000038              | 2.384248                                                         |
| 26005 | 1.373274              | 2.384253                                                         |
| 26007 | 1.333487              | 2.384259                                                         |
| 26009 | 1.033488              | 2.384265                                                         |
| 26011 | 1.081850              | 2.384271                                                         |
| 26013 | 1.549994              | 2.384276                                                         |
| 26015 | 1.349683              | 2.384282                                                         |
| 26017 | 1.000038              | 2.384288                                                         |
| 26019 | 1.708751              | 2.384293                                                         |
| 26021 | 1.000038              | 2.384299                                                         |
| 26023 | 1.020943              | 2.384305                                                         |
| 26025 | 1.658098              | 2.384310                                                         |
| 26027 | 1.059515              | 2.384316                                                         |
| 26029 | 1.000038              | 2.384322                                                         |
| 26031 | 1.333487              | 2.384327                                                         |
| 26033 | 1.143164              | 2.384333                                                         |
| 26035 | 1.238948              | 2.384339                                                         |
| 26037 | 1.581749              | 2.384345                                                         |
| 26039 | 1.077461              | 2.384350                                                         |
| 26041 | 1.000038              | 2.384356                                                         |
| 26043 | 1.333487              | 2.384362                                                         |
| 26045 | 1.200230              | 2.384367                                                         |
| 26047 | 1.161900              | 2.384373                                                         |
| 26049 | 1.406580              | 2.384379                                                         |
| 26051 | 1.013397              | 2.384384                                                         |
| 26053 | 1.000038              | 2.384390                                                         |
| 26055 | 1.786989              | 2.384396                                                         |
| 26057 | 1.016848              | 2.384401                                                         |
| 26059 | 1.149392              | 2.384407                                                         |
| 26061 | 1.635547              | 2.384413                                                         |

| $n$   | $\frac{\sigma(n)}{n}$ | $\frac{e^\gamma}{2} \log \log n + \frac{0.73\dots}{\log \log n}$ |
|-------|-----------------------|------------------------------------------------------------------|
| 26063 | 1.017534              | 2.384418                                                         |
| 26065 | 1.295530              | 2.384424                                                         |
| 26067 | 1.333487              | 2.384430                                                         |
| 26069 | 1.012697              | 2.384435                                                         |
| 26071 | 1.069081              | 2.384441                                                         |
| 26073 | 1.444943              | 2.384447                                                         |
| 26075 | 1.426654              | 2.384453                                                         |
| 26077 | 1.014687              | 2.384458                                                         |
| 26079 | 1.333487              | 2.384464                                                         |
| 26081 | 1.091369              | 2.384470                                                         |
| 26083 | 1.000038              | 2.384475                                                         |
| 26085 | 1.678206              | 2.384481                                                         |
| 26087 | 1.053398              | 2.384487                                                         |
| 26089 | 1.143164              | 2.384492                                                         |
| 26091 | 1.562531              | 2.384498                                                         |
| 26093 | 1.014065              | 2.384504                                                         |
| 26095 | 1.274727              | 2.384509                                                         |
| 26097 | 1.333487              | 2.384515                                                         |
| 26099 | 1.000038              | 2.384521                                                         |
| 26101 | 1.024942              | 2.384526                                                         |
| 26103 | 1.677049              | 2.384532                                                         |
| 26105 | 1.257690              | 2.384538                                                         |
| 26107 | 1.000038              | 2.384543                                                         |
| 26109 | 1.483014              | 2.384549                                                         |
| 26111 | 1.000038              | 2.384555                                                         |
| 26113 | 1.000038              | 2.384560                                                         |
| 26115 | 1.600919              | 2.384566                                                         |
| 26117 | 1.283302              | 2.384572                                                         |
| 26119 | 1.000038              | 2.384577                                                         |
| 26121 | 1.333486              | 2.384583                                                         |
| 26123 | 1.012441              | 2.384589                                                         |
| 26125 | 1.433110              | 2.384594                                                         |
| 26127 | 1.444942              | 2.384600                                                         |
| 26129 | 1.116001              | 2.384606                                                         |
| 26131 | 1.143163              | 2.384611                                                         |
| 26133 | 1.381242              | 2.384617                                                         |
| 26135 | 1.200230              | 2.384623                                                         |
| 26137 | 1.019245              | 2.384628                                                         |
| 26139 | 1.333486              | 2.384634                                                         |
| 26141 | 1.000038              | 2.384640                                                         |
| 26143 | 1.077459              | 2.384645                                                         |
| 26145 | 2.004819              | 2.384651                                                         |
| 26147 | 1.091368              | 2.384657                                                         |
| 26149 | 1.015718              | 2.384662                                                         |

| $n$   | $\frac{\sigma(n)}{n}$ | $\frac{e^\gamma}{2} \log \log n + \frac{0.73...}{\log \log n}$ |
|-------|-----------------------|----------------------------------------------------------------|
| 26151 | 1.394975              | 2.384668                                                       |
| 26153 | 1.000038              | 2.384674                                                       |
| 26155 | 1.200229              | 2.384679                                                       |
| 26157 | 1.333486              | 2.384685                                                       |
| 26159 | 1.185366              | 2.384691                                                       |
| 26161 | 1.000038              | 2.384696                                                       |
| 26163 | 1.664947              | 2.384702                                                       |
| 26165 | 1.200229              | 2.384708                                                       |
| 26167 | 1.012573              | 2.384713                                                       |
| 26169 | 1.592113              | 2.384719                                                       |
| 26171 | 1.000038              | 2.384725                                                       |
| 26173 | 1.143163              | 2.384730                                                       |
| 26175 | 1.658071              | 2.384736                                                       |
| 26177 | 1.000038              | 2.384742                                                       |
| 26179 | 1.023110              | 2.384747                                                       |
| 26181 | 1.444941              | 2.384753                                                       |
| 26183 | 1.000038              | 2.384759                                                       |
| 26185 | 1.200229              | 2.384764                                                       |
| 26187 | 1.613014              | 2.384770                                                       |
| 26189 | 1.000038              | 2.384775                                                       |
| 26191 | 1.091367              | 2.384781                                                       |
| 26193 | 1.333486              | 2.384787                                                       |
| 26195 | 1.341325              | 2.384792                                                       |
| 26197 | 1.121350              | 2.384798                                                       |
| 26199 | 1.500515              | 2.384804                                                       |
| 26201 | 1.209114              | 2.384809                                                       |
| 26203 | 1.000038              | 2.384815                                                       |
| 26205 | 1.600916              | 2.384821                                                       |
| 26207 | 1.016522              | 2.384826                                                       |
| 26209 | 1.000038              | 2.384832                                                       |
| 26211 | 1.333486              | 2.384838                                                       |
| 26213 | 1.091367              | 2.384843                                                       |
| 26215 | 1.408964              | 2.384849                                                       |
| 26217 | 1.483007              | 2.384855                                                       |
| 26219 | 1.012396              | 2.384860                                                       |
| 26221 | 1.077457              | 2.384866                                                       |
| 26223 | 1.333486              | 2.384872                                                       |
| 26225 | 1.241182              | 2.384877                                                       |
| 26227 | 1.000038              | 2.384883                                                       |
| 26229 | 1.525030              | 2.384888                                                       |
| 26231 | 1.059510              | 2.384894                                                       |
| 26233 | 1.028476              | 2.384900                                                       |
| 26235 | 1.926587              | 2.384905                                                       |
| 26237 | 1.000038              | 2.384911                                                       |



| $n$   | $\frac{\sigma(n)}{n}$ | $\frac{e^\gamma}{2} \log \log n + \frac{0.73...}{\log \log n}$ |
|-------|-----------------------|----------------------------------------------------------------|
| 26239 | 1.053394              | 2.384917                                                       |
| 26241 | 1.333486              | 2.384922                                                       |
| 26243 | 1.199863              | 2.384928                                                       |
| 26245 | 1.248238              | 2.384934                                                       |
| 26247 | 1.438031              | 2.384939                                                       |
| 26249 | 1.000038              | 2.384945                                                       |
| 26251 | 1.000038              | 2.384951                                                       |
| 26253 | 1.444940              | 2.384956                                                       |
| 26255 | 1.234051              | 2.384962                                                       |
| 26257 | 1.296721              | 2.384967                                                       |
| 26259 | 1.333486              | 2.384973                                                       |
| 26261 | 1.000038              | 2.384979                                                       |
| 26263 | 1.000038              | 2.384984                                                       |
| 26265 | 1.710565              | 2.384990                                                       |
| 26267 | 1.000038              | 2.384996                                                       |
| 26269 | 1.013362              | 2.385001                                                       |
| 26271 | 1.705302              | 2.385007                                                       |
| 26273 | 1.125414              | 2.385013                                                       |
| 26275 | 1.241180              | 2.385018                                                       |
| 26277 | 1.406553              | 2.385024                                                       |
| 26279 | 1.091366              | 2.385029                                                       |
| 26281 | 1.025988              | 2.385035                                                       |
| 26283 | 1.333486              | 2.385041                                                       |
| 26285 | 1.373255              | 2.385046                                                       |
| 26287 | 1.014037              | 2.385052                                                       |
| 26289 | 1.519114              | 2.385058                                                       |
| 26291 | 1.018752              | 2.385063                                                       |
| 26293 | 1.000038              | 2.385069                                                       |
| 26295 | 1.600913              | 2.385074                                                       |
| 26297 | 1.000038              | 2.385080                                                       |
| 26299 | 1.307426              | 2.385086                                                       |
| 26301 | 1.456370              | 2.385091                                                       |
| 26303 | 1.035623              | 2.385097                                                       |
| 26305 | 1.200228              | 2.385103                                                       |
| 26307 | 1.502262              | 2.385108                                                       |
| 26309 | 1.000038              | 2.385114                                                       |
| 26311 | 1.015241              | 2.385119                                                       |
| 26313 | 1.559685              | 2.385125                                                       |
| 26315 | 1.267718              | 2.385131                                                       |
| 26317 | 1.000038              | 2.385136                                                       |
| 26319 | 1.381207              | 2.385142                                                       |
| 26321 | 1.000038              | 2.385148                                                       |
| 26323 | 1.091365              | 2.385153                                                       |
| 26325 | 1.994834              | 2.385159                                                       |

| $n$   | $\frac{\sigma(n)}{n}$ | $\frac{e^\gamma}{2} \log \log n + \frac{0.73...}{\log \log n}$ |
|-------|-----------------------|----------------------------------------------------------------|
| 26327 | 1.143161              | 2.385164                                                       |
| 26329 | 1.013179              | 2.385170                                                       |
| 26331 | 1.363564              | 2.385176                                                       |
| 26333 | 1.059507              | 2.385181                                                       |
| 26335 | 1.257642              | 2.385187                                                       |
| 26337 | 1.333485              | 2.385193                                                       |
| 26339 | 1.000038              | 2.385198                                                       |
| 26341 | 1.180821              | 2.385204                                                       |
| 26343 | 1.444938              | 2.385209                                                       |
| 26345 | 1.311824              | 2.385215                                                       |
| 26347 | 1.000038              | 2.385221                                                       |
| 26349 | 1.333485              | 2.385226                                                       |
| 26351 | 1.077454              | 2.385232                                                       |
| 26353 | 1.069859              | 2.385237                                                       |
| 26355 | 1.835857              | 2.385243                                                       |
| 26357 | 1.000038              | 2.385249                                                       |
| 26359 | 1.024925              | 2.385254                                                       |
| 26361 | 1.509047              | 2.385260                                                       |
| 26363 | 1.025983              | 2.385266                                                       |
| 26365 | 1.200228              | 2.385271                                                       |
| 26367 | 1.572875              | 2.385277                                                       |
| 26369 | 1.143161              | 2.385282                                                       |
| 26371 | 1.000038              | 2.385288                                                       |
| 26373 | 1.365032              | 2.385294                                                       |
| 26375 | 1.253915              | 2.385299                                                       |
| 26377 | 1.077454              | 2.385305                                                       |
| 26379 | 1.482998              | 2.385310                                                       |
| 26381 | 1.106251              | 2.385316                                                       |
| 26383 | 1.143160              | 2.385322                                                       |
| 26385 | 1.600910              | 2.385327                                                       |
| 26387 | 1.000038              | 2.385333                                                       |
| 26389 | 1.091364              | 2.385338                                                       |
| 26391 | 1.406540              | 2.385344                                                       |
| 26393 | 1.000038              | 2.385350                                                       |
| 26395 | 1.200227              | 2.385355                                                       |
| 26397 | 1.654733              | 2.385361                                                       |
| 26399 | 1.000038              | 2.385366                                                       |
| 26401 | 1.059505              | 2.385372                                                       |
| 26403 | 1.438018              | 2.385378                                                       |
| 26405 | 1.200227              | 2.385383                                                       |
| 26407 | 1.000038              | 2.385389                                                       |
| 26409 | 1.333485              | 2.385395                                                       |
| 26411 | 1.272652              | 2.385400                                                       |
| 26413 | 1.018741              | 2.385406                                                       |

| $n$   | $\frac{\sigma(n)}{n}$ | $\frac{e^\gamma}{2} \log \log n + \frac{0.73\dots}{\log \log n}$ |
|-------|-----------------------|------------------------------------------------------------------|
| 26415 | 1.736286              | 2.385411                                                         |
| 26417 | 1.000038              | 2.385417                                                         |
| 26419 | 1.035618              | 2.385423                                                         |
| 26421 | 1.333485              | 2.385428                                                         |
| 26423 | 1.000038              | 2.385434                                                         |
| 26425 | 1.426528              | 2.385439                                                         |
| 26427 | 1.394937              | 2.385445                                                         |
| 26429 | 1.144198              | 2.385451                                                         |
| 26431 | 1.000038              | 2.385456                                                         |
| 26433 | 1.634321              | 2.385462                                                         |
| 26435 | 1.274674              | 2.385467                                                         |
| 26437 | 1.000038              | 2.385473                                                         |
| 26439 | 1.525020              | 2.385478                                                         |
| 26441 | 1.012518              | 2.385484                                                         |
| 26443 | 1.033468              | 2.385490                                                         |
| 26445 | 1.677141              | 2.385495                                                         |
| 26447 | 1.020910              | 2.385501                                                         |
| 26449 | 1.000038              | 2.385506                                                         |
| 26451 | 1.444936              | 2.385512                                                         |
| 26453 | 1.143160              | 2.385518                                                         |
| 26455 | 1.447893              | 2.385523                                                         |
| 26457 | 1.333485              | 2.385529                                                         |
| 26459 | 1.000038              | 2.385534                                                         |
| 26461 | 1.023091              | 2.385540                                                         |
| 26463 | 1.333484              | 2.385546                                                         |
| 26465 | 1.233327              | 2.385551                                                         |
| 26467 | 1.209053              | 2.385557                                                         |
| 26469 | 1.538252              | 2.385562                                                         |
| 26471 | 1.013638              | 2.385568                                                         |
| 26473 | 1.044385              | 2.385574                                                         |
| 26475 | 1.658017              | 2.385579                                                         |
| 26477 | 1.142123              | 2.385585                                                         |
| 26479 | 1.000038              | 2.385590                                                         |
| 26481 | 1.657943              | 2.385596                                                         |
| 26483 | 1.016803              | 2.385601                                                         |
| 26485 | 1.200227              | 2.385607                                                         |
| 26487 | 1.511685              | 2.385613                                                         |
| 26489 | 1.000038              | 2.385618                                                         |
| 26491 | 1.019214              | 2.385624                                                         |
| 26493 | 1.333484              | 2.385629                                                         |
| 26495 | 1.373240              | 2.385635                                                         |
| 26497 | 1.000038              | 2.385641                                                         |
| 26499 | 1.485641              | 2.385646                                                         |
| 26501 | 1.000038              | 2.385652                                                         |

| $n$   | $\frac{\sigma(n)}{n}$ | $\frac{e^\gamma}{2} \log \log n + \frac{0.73...}{\log \log n}$ |
|-------|-----------------------|----------------------------------------------------------------|
| 26503 | 1.059503              | 2.385657                                                       |
| 26505 | 1.883418              | 2.385663                                                       |
| 26507 | 1.077451              | 2.385668                                                       |
| 26509 | 1.165416              | 2.385674                                                       |
| 26511 | 1.333484              | 2.385680                                                       |
| 26513 | 1.000038              | 2.385685                                                       |
| 26515 | 1.200226              | 2.385691                                                       |
| 26517 | 1.333484              | 2.385696                                                       |
| 26519 | 1.044383              | 2.385702                                                       |
| 26521 | 1.091362              | 2.385708                                                       |
| 26523 | 1.654715              | 2.385713                                                       |
| 26525 | 1.241169              | 2.385719                                                       |
| 26527 | 1.025974              | 2.385724                                                       |
| 26529 | 1.375099              | 2.385730                                                       |
| 26531 | 1.024914              | 2.385735                                                       |
| 26533 | 1.089737              | 2.385741                                                       |
| 26535 | 1.682306              | 2.385747                                                       |
| 26537 | 1.215510              | 2.385752                                                       |
| 26539 | 1.000038              | 2.385758                                                       |
| 26541 | 1.482989              | 2.385763                                                       |
| 26543 | 1.157367              | 2.385769                                                       |
| 26545 | 1.200226              | 2.385774                                                       |
| 26547 | 1.333484              | 2.385780                                                       |
| 26549 | 1.012468              | 2.385786                                                       |
| 26551 | 1.143158              | 2.385791                                                       |
| 26553 | 1.366625              | 2.385797                                                       |
| 26555 | 1.236377              | 2.385802                                                       |
| 26557 | 1.000038              | 2.385808                                                       |
| 26559 | 1.562408              | 2.385813                                                       |
| 26561 | 1.000038              | 2.385819                                                       |
| 26563 | 1.013741              | 2.385825                                                       |
| 26565 | 2.081536              | 2.385830                                                       |
| 26567 | 1.033463              | 2.385836                                                       |
| 26569 | 1.006173              | 2.385841                                                       |
| 26571 | 1.414474              | 2.385847                                                       |
| 26573 | 1.000038              | 2.385852                                                       |
| 26575 | 1.241167              | 2.385858                                                       |
| 26577 | 1.444934              | 2.385863                                                       |
| 26579 | 1.143158              | 2.385869                                                       |
| 26581 | 1.053384              | 2.385875                                                       |
| 26583 | 1.333484              | 2.385880                                                       |
| 26585 | 1.295467              | 2.385886                                                       |
| 26587 | 1.091360              | 2.385891                                                       |
| 26589 | 1.333484              | 2.385897                                                       |

| $n$   | $\frac{\sigma(n)}{n}$ | $\frac{e^\gamma}{2} \log \log n + \frac{0.73...}{\log \log n}$ |
|-------|-----------------------|----------------------------------------------------------------|
| 26591 | 1.000038              | 2.385902                                                       |
| 26593 | 1.191291              | 2.385908                                                       |
| 26595 | 1.786802              | 2.385914                                                       |
| 26597 | 1.000038              | 2.385919                                                       |
| 26599 | 1.017482              | 2.385925                                                       |
| 26601 | 1.333484              | 2.385930                                                       |
| 26603 | 1.028455              | 2.385936                                                       |
| 26605 | 1.274648              | 2.385941                                                       |
| 26607 | 1.559590              | 2.385947                                                       |
| 26609 | 1.136458              | 2.385952                                                       |
| 26611 | 1.136372              | 2.385958                                                       |
| 26613 | 1.444933              | 2.385964                                                       |
| 26615 | 1.200225              | 2.385969                                                       |
| 26617 | 1.024909              | 2.385975                                                       |
| 26619 | 1.406514              | 2.385980                                                       |
| 26621 | 1.143158              | 2.385986                                                       |
| 26623 | 1.015663              | 2.385991                                                       |
| 26625 | 1.687437              | 2.385997                                                       |
| 26627 | 1.000038              | 2.386002                                                       |
| 26629 | 1.033460              | 2.386008                                                       |
| 26631 | 1.581615              | 2.386014                                                       |
| 26633 | 1.000038              | 2.386019                                                       |
| 26635 | 1.373231              | 2.386025                                                       |
| 26637 | 1.438000              | 2.386030                                                       |
| 26639 | 1.059499              | 2.386036                                                       |
| 26641 | 1.000038              | 2.386041                                                       |
| 26643 | 1.362009              | 2.386047                                                       |
| 26645 | 1.216664              | 2.386052                                                       |
| 26647 | 1.000038              | 2.386058                                                       |
| 26649 | 1.743555              | 2.386063                                                       |
| 26651 | 1.035608              | 2.386069                                                       |
| 26653 | 1.091359              | 2.386075                                                       |
| 26655 | 1.600900              | 2.386080                                                       |
| 26657 | 1.116405              | 2.386086                                                       |
| 26659 | 1.020894              | 2.386091                                                       |
| 26661 | 1.333483              | 2.386097                                                       |
| 26663 | 1.234970              | 2.386102                                                       |
| 26665 | 1.200225              | 2.386108                                                       |
| 26667 | 1.444932              | 2.386113                                                       |
| 26669 | 1.000037              | 2.386119                                                       |
| 26671 | 1.012335              | 2.386124                                                       |
| 26673 | 1.414464              | 2.386130                                                       |
| 26675 | 1.366673              | 2.386136                                                       |
| 26677 | 1.185141              | 2.386141                                                       |

| $n$   | $\frac{\sigma(n)}{n}$ | $\frac{e^\gamma}{2} \log \log n + \frac{0.73\dots}{\log \log n}$ |
|-------|-----------------------|------------------------------------------------------------------|
| 26679 | 1.333483              | 2.386147                                                         |
| 26681 | 1.000037              | 2.386152                                                         |
| 26683 | 1.000037              | 2.386158                                                         |
| 26685 | 1.736256              | 2.386163                                                         |
| 26687 | 1.000037              | 2.386169                                                         |
| 26689 | 1.077448              | 2.386174                                                         |
| 26691 | 1.611330              | 2.386180                                                         |
| 26693 | 1.000037              | 2.386185                                                         |
| 26695 | 1.267653              | 2.386191                                                         |
| 26697 | 1.456343              | 2.386196                                                         |
| 26699 | 1.000037              | 2.386202                                                         |
| 26701 | 1.000037              | 2.386208                                                         |
| 26703 | 1.581845              | 2.386213                                                         |
| 26705 | 1.408725              | 2.386219                                                         |
| 26707 | 1.059498              | 2.386224                                                         |
| 26709 | 1.383803              | 2.386230                                                         |
| 26711 | 1.000037              | 2.386235                                                         |
| 26713 | 1.000037              | 2.386241                                                         |
| 26715 | 1.735654              | 2.386246                                                         |
| 26717 | 1.000037              | 2.386252                                                         |
| 26719 | 1.250346              | 2.386257                                                         |
| 26721 | 1.444931              | 2.386263                                                         |
| 26723 | 1.000037              | 2.386268                                                         |
| 26725 | 1.241160              | 2.386274                                                         |
| 26727 | 1.364912              | 2.386279                                                         |
| 26729 | 1.000037              | 2.386285                                                         |
| 26731 | 1.000037              | 2.386291                                                         |
| 26733 | 1.627950              | 2.386296                                                         |
| 26735 | 1.200224              | 2.386302                                                         |
| 26737 | 1.000037              | 2.386307                                                         |
| 26739 | 1.444931              | 2.386313                                                         |
| 26741 | 1.253356              | 2.386318                                                         |
| 26743 | 1.023071              | 2.386324                                                         |
| 26745 | 1.600897              | 2.386329                                                         |
| 26747 | 1.143156              | 2.386335                                                         |
| 26749 | 1.044375              | 2.386340                                                         |
| 26751 | 1.375051              | 2.386346                                                         |
| 26753 | 1.033454              | 2.386351                                                         |
| 26755 | 1.200224              | 2.386357                                                         |
| 26757 | 1.482976              | 2.386362                                                         |
| 26759 | 1.000037              | 2.386368                                                         |
| 26761 | 1.143156              | 2.386373                                                         |
| 26763 | 1.456339              | 2.386379                                                         |
| 26765 | 1.234747              | 2.386384                                                         |

| $n$   | $\frac{\sigma(n)}{n}$ | $\frac{e^\gamma}{2} \log \log n + \frac{0.73\dots}{\log \log n}$ |
|-------|-----------------------|------------------------------------------------------------------|
| 26767 | 1.129749              | 2.386390                                                         |
| 26769 | 1.333483              | 2.386395                                                         |
| 26771 | 1.053379              | 2.386401                                                         |
| 26773 | 1.025959              | 2.386407                                                         |
| 26775 | 2.167395              | 2.386412                                                         |
| 26777 | 1.000037              | 2.386418                                                         |
| 26779 | 1.018709              | 2.386423                                                         |
| 26781 | 1.362160              | 2.386429                                                         |
| 26783 | 1.000037              | 2.386434                                                         |
| 26785 | 1.311779              | 2.386440                                                         |
| 26787 | 1.333483              | 2.386445                                                         |
| 26789 | 1.182575              | 2.386451                                                         |
| 26791 | 1.016461              | 2.386456                                                         |
| 26793 | 1.562348              | 2.386462                                                         |
| 26795 | 1.257548              | 2.386467                                                         |
| 26797 | 1.012651              | 2.386473                                                         |
| 26799 | 1.333483              | 2.386478                                                         |
| 26801 | 1.000037              | 2.386484                                                         |
| 26803 | 1.165392              | 2.386489                                                         |
| 26805 | 1.600895              | 2.386495                                                         |
| 26807 | 1.091357              | 2.386500                                                         |
| 26809 | 1.127979              | 2.386506                                                         |
| 26811 | 1.498340              | 2.386511                                                         |
| 26813 | 1.000037              | 2.386517                                                         |
| 26815 | 1.245870              | 2.386522                                                         |
| 26817 | 1.525003              | 2.386528                                                         |
| 26819 | 1.077445              | 2.386533                                                         |
| 26821 | 1.000037              | 2.386539                                                         |
| 26823 | 1.333482              | 2.386544                                                         |
| 26825 | 1.317428              | 2.386550                                                         |
| 26827 | 1.012413              | 2.386555                                                         |
| 26829 | 1.581572              | 2.386561                                                         |
| 26831 | 1.143155              | 2.386566                                                         |
| 26833 | 1.000037              | 2.386572                                                         |
| 26835 | 1.600894              | 2.386577                                                         |
| 26837 | 1.023065              | 2.386583                                                         |
| 26839 | 1.000037              | 2.386588                                                         |
| 26841 | 1.394881              | 2.386594                                                         |
| 26843 | 1.059494              | 2.386599                                                         |
| 26845 | 1.501956              | 2.386605                                                         |
| 26847 | 1.530152              | 2.386610                                                         |
| 26849 | 1.000037              | 2.386616                                                         |
| 26851 | 1.091356              | 2.386621                                                         |
| 26853 | 1.333482              | 2.386627                                                         |

| $n$   | $\frac{\sigma(n)}{n}$ | $\frac{e^\gamma}{2} \log \log n + \frac{0.73...}{\log \log n}$ |
|-------|-----------------------|----------------------------------------------------------------|
| 26855 | 1.238652              | 2.386632                                                       |
| 26857 | 1.013367              | 2.386638                                                       |
| 26859 | 1.525001              | 2.386643                                                       |
| 26861 | 1.000037              | 2.386649                                                       |
| 26863 | 1.000037              | 2.386654                                                       |
| 26865 | 1.786711              | 2.386660                                                       |
| 26867 | 1.017456              | 2.386665                                                       |
| 26869 | 1.013957              | 2.386671                                                       |
| 26871 | 1.471028              | 2.386676                                                       |
| 26873 | 1.250326              | 2.386682                                                       |
| 26875 | 1.278660              | 2.386687                                                       |
| 26877 | 1.462068              | 2.386693                                                       |
| 26879 | 1.000037              | 2.386698                                                       |
| 26881 | 1.000037              | 2.386704                                                       |
| 26883 | 1.508760              | 2.386709                                                       |
| 26885 | 1.267621              | 2.386715                                                       |
| 26887 | 1.199688              | 2.386720                                                       |
| 26889 | 1.333482              | 2.386726                                                       |
| 26891 | 1.000037              | 2.386731                                                       |
| 26893 | 1.000037              | 2.386737                                                       |
| 26895 | 1.756163              | 2.386742                                                       |
| 26897 | 1.077444              | 2.386748                                                       |
| 26899 | 1.028440              | 2.386753                                                       |
| 26901 | 1.707818              | 2.386759                                                       |
| 26903 | 1.000037              | 2.386764                                                       |
| 26905 | 1.200223              | 2.386770                                                       |
| 26907 | 1.333482              | 2.386775                                                       |
| 26909 | 1.016760              | 2.386781                                                       |
| 26911 | 1.059492              | 2.386786                                                       |
| 26913 | 1.333482              | 2.386792                                                       |
| 26915 | 1.373212              | 2.386797                                                       |
| 26917 | 1.091355              | 2.386803                                                       |
| 26919 | 1.482967              | 2.386808                                                       |
| 26921 | 1.000037              | 2.386814                                                       |
| 26923 | 1.144003              | 2.386819                                                       |
| 26925 | 1.657939              | 2.386825                                                       |
| 26927 | 1.000037              | 2.386830                                                       |
| 26929 | 1.143154              | 2.386836                                                       |
| 26931 | 1.368831              | 2.386841                                                       |
| 26933 | 1.044369              | 2.386847                                                       |
| 26935 | 1.200223              | 2.386852                                                       |
| 26937 | 1.499944              | 2.386858                                                       |
| 26939 | 1.140354              | 2.386863                                                       |
| 26941 | 1.035596              | 2.386869                                                       |



| $n$   | $\frac{\sigma(n)}{n}$ | $\frac{e^\gamma}{2} \log \log n + \frac{0.73...}{\log \log n}$ |
|-------|-----------------------|----------------------------------------------------------------|
| 26943 | 1.524997              | 2.386874                                                       |
| 26945 | 1.274596              | 2.386880                                                       |
| 26947 | 1.000037              | 2.386885                                                       |
| 26949 | 1.437975              | 2.386891                                                       |
| 26951 | 1.000037              | 2.386896                                                       |
| 26953 | 1.000037              | 2.386901                                                       |
| 26955 | 1.736227              | 2.386907                                                       |
| 26957 | 1.143154              | 2.386912                                                       |
| 26959 | 1.000037              | 2.386918                                                       |
| 26961 | 1.566707              | 2.386923                                                       |
| 26963 | 1.019174              | 2.386929                                                       |
| 26965 | 1.200223              | 2.386934                                                       |
| 26967 | 1.361664              | 2.386940                                                       |
| 26969 | 1.012273              | 2.386945                                                       |
| 26971 | 1.143154              | 2.386951                                                       |
| 26973 | 1.539836              | 2.386956                                                       |
| 26975 | 1.351474              | 2.386962                                                       |
| 26977 | 1.020870              | 2.386967                                                       |
| 26979 | 1.475815              | 2.386973                                                       |
| 26981 | 1.000037              | 2.386978                                                       |
| 26983 | 1.104103              | 2.386984                                                       |
| 26985 | 1.835686              | 2.386989                                                       |
| 26987 | 1.000037              | 2.386995                                                       |
| 26989 | 1.012412              | 2.387000                                                       |
| 26991 | 1.444926              | 2.387006                                                       |
| 26993 | 1.000037              | 2.387011                                                       |
| 26995 | 1.200222              | 2.387016                                                       |
| 26997 | 1.333481              | 2.387022                                                       |
| 26999 | 1.266714              | 2.387027                                                       |
| 27001 | 1.128255              | 2.387033                                                       |
| 27003 | 1.333481              | 2.387038                                                       |
| 27005 | 1.311757              | 2.387044                                                       |
| 27007 | 1.013071              | 2.387049                                                       |
| 27009 | 1.444926              | 2.387055                                                       |
| 27011 | 1.000037              | 2.387060                                                       |
| 27013 | 1.215415              | 2.387066                                                       |
| 27015 | 1.600888              | 2.387071                                                       |
| 27017 | 1.000037              | 2.387077                                                       |
| 27019 | 1.025945              | 2.387082                                                       |
| 27021 | 1.333481              | 2.387088                                                       |
| 27023 | 1.018688              | 2.387093                                                       |
| 27025 | 1.321443              | 2.387098                                                       |
| 27027 | 1.989122              | 2.387104                                                       |
| 27029 | 1.012246              | 2.387109                                                       |

| $n$   | $\frac{\sigma(n)}{n}$ | $\frac{e^\gamma}{2} \log \log n + \frac{0.73...}{\log \log n}$ |
|-------|-----------------------|----------------------------------------------------------------|
| 27031 | 1.000037              | 2.387115                                                       |
| 27033 | 1.333481              | 2.387120                                                       |
| 27035 | 1.200222              | 2.387126                                                       |
| 27037 | 1.053371              | 2.387131                                                       |
| 27039 | 1.333481              | 2.387137                                                       |
| 27041 | 1.143153              | 2.387142                                                       |
| 27043 | 1.000037              | 2.387148                                                       |
| 27045 | 1.736217              | 2.387153                                                       |
| 27047 | 1.112730              | 2.387159                                                       |
| 27049 | 1.091353              | 2.387164                                                       |
| 27051 | 1.362759              | 2.387169                                                       |
| 27053 | 1.077441              | 2.387175                                                       |
| 27055 | 1.373203              | 2.387180                                                       |
| 27057 | 1.383745              | 2.387186                                                       |
| 27059 | 1.000037              | 2.387191                                                       |
| 27061 | 1.000037              | 2.387197                                                       |
| 27063 | 1.506411              | 2.387202                                                       |
| 27065 | 1.200222              | 2.387208                                                       |
| 27067 | 1.000037              | 2.387213                                                       |
| 27069 | 1.524992              | 2.387219                                                       |
| 27071 | 1.148979              | 2.387224                                                       |
| 27073 | 1.000037              | 2.387229                                                       |
| 27075 | 1.744931              | 2.387235                                                       |
| 27077 | 1.000037              | 2.387240                                                       |
| 27079 | 1.077440              | 2.387246                                                       |
| 27081 | 1.595214              | 2.387251                                                       |
| 27083 | 1.180371              | 2.387257                                                       |
| 27085 | 1.200222              | 2.387262                                                       |
| 27087 | 1.333481              | 2.387268                                                       |
| 27089 | 1.013548              | 2.387273                                                       |
| 27091 | 1.000037              | 2.387279                                                       |
| 27093 | 1.456317              | 2.387284                                                       |
| 27095 | 1.200221              | 2.387289                                                       |
| 27097 | 1.180943              | 2.387295                                                       |
| 27099 | 1.444924              | 2.387300                                                       |
| 27101 | 1.025940              | 2.387306                                                       |
| 27103 | 1.000037              | 2.387311                                                       |
| 27105 | 1.735473              | 2.387317                                                       |
| 27107 | 1.000037              | 2.387322                                                       |
| 27109 | 1.000037              | 2.387328                                                       |
| 27111 | 1.524990              | 2.387333                                                       |
| 27113 | 1.053369              | 2.387338                                                       |
| 27115 | 1.433893              | 2.387344                                                       |
| 27117 | 1.518752              | 2.387349                                                       |

| $n$   | $\frac{\sigma(n)}{n}$ | $\frac{e^\gamma}{2} \log \log n + \frac{0.73...}{\log \log n}$ |
|-------|-----------------------|----------------------------------------------------------------|
| 27119 | 1.023047              | 2.387355                                                       |
| 27121 | 1.028428              | 2.387360                                                       |
| 27123 | 1.333481              | 2.387366                                                       |
| 27125 | 1.472295              | 2.387371                                                       |
| 27127 | 1.000037              | 2.387377                                                       |
| 27129 | 1.333481              | 2.387382                                                       |
| 27131 | 1.077439              | 2.387387                                                       |
| 27133 | 1.024877              | 2.387393                                                       |
| 27135 | 1.819348              | 2.387398                                                       |
| 27137 | 1.091351              | 2.387404                                                       |
| 27139 | 1.143152              | 2.387409                                                       |
| 27141 | 1.361777              | 2.387415                                                       |
| 27143 | 1.000037              | 2.387420                                                       |
| 27145 | 1.233376              | 2.387426                                                       |
| 27147 | 1.333481              | 2.387431                                                       |
| 27149 | 1.059487              | 2.387436                                                       |
| 27151 | 1.053368              | 2.387442                                                       |
| 27153 | 1.654624              | 2.387447                                                       |
| 27155 | 1.200221              | 2.387453                                                       |
| 27157 | 1.077439              | 2.387458                                                       |
| 27159 | 1.456313              | 2.387464                                                       |
| 27161 | 1.012187              | 2.387469                                                       |
| 27163 | 1.044362              | 2.387474                                                       |
| 27165 | 1.600883              | 2.387480                                                       |
| 27167 | 1.143152              | 2.387485                                                       |
| 27169 | 1.013655              | 2.387491                                                       |
| 27171 | 1.444923              | 2.387496                                                       |
| 27173 | 1.035587              | 2.387502                                                       |
| 27175 | 1.241141              | 2.387507                                                       |
| 27177 | 1.333481              | 2.387512                                                       |
| 27179 | 1.000037              | 2.387518                                                       |
| 27181 | 1.250285              | 2.387523                                                       |
| 27183 | 1.557444              | 2.387529                                                       |
| 27185 | 1.200221              | 2.387534                                                       |
| 27187 | 1.033435              | 2.387540                                                       |
| 27189 | 1.588878              | 2.387545                                                       |
| 27191 | 1.000037              | 2.387550                                                       |
| 27193 | 1.016732              | 2.387556                                                       |
| 27195 | 1.911528              | 2.387561                                                       |
| 27197 | 1.000037              | 2.387567                                                       |
| 27199 | 1.019155              | 2.387572                                                       |
| 27201 | 1.333480              | 2.387578                                                       |
| 27203 | 1.091350              | 2.387583                                                       |
| 27205 | 1.200221              | 2.387588                                                       |

| $n$   | $\frac{\sigma(n)}{n}$ | $\frac{e^\gamma}{2} \log \log n + \frac{0.73...}{\log \log n}$ |
|-------|-----------------------|----------------------------------------------------------------|
| 27207 | 1.444922              | 2.387594                                                       |
| 27209 | 1.291337              | 2.387599                                                       |
| 27211 | 1.000037              | 2.387605                                                       |
| 27213 | 1.368758              | 2.387610                                                       |
| 27215 | 1.200220              | 2.387616                                                       |
| 27217 | 1.059485              | 2.387621                                                       |
| 27219 | 1.370807              | 2.387626                                                       |
| 27221 | 1.012160              | 2.387632                                                       |
| 27223 | 1.143151              | 2.387637                                                       |
| 27225 | 1.968742              | 2.387643                                                       |
| 27227 | 1.053366              | 2.387648                                                       |
| 27229 | 1.016416              | 2.387654                                                       |
| 27231 | 1.383717              | 2.387659                                                       |
| 27233 | 1.013036              | 2.387664                                                       |
| 27235 | 1.295392              | 2.387670                                                       |
| 27237 | 1.524984              | 2.387675                                                       |
| 27239 | 1.000037              | 2.387681                                                       |
| 27241 | 1.000037              | 2.387686                                                       |
| 27243 | 1.482950              | 2.387691                                                       |
| 27245 | 1.200220              | 2.387697                                                       |
| 27247 | 1.091350              | 2.387702                                                       |
| 27249 | 1.381042              | 2.387708                                                       |
| 27251 | 1.215368              | 2.387713                                                       |
| 27253 | 1.000037              | 2.387719                                                       |
| 27255 | 1.690699              | 2.387724                                                       |
| 27257 | 1.013905              | 2.387729                                                       |
| 27259 | 1.000037              | 2.387735                                                       |
| 27261 | 1.562232              | 2.387740                                                       |
| 27263 | 1.012361              | 2.387746                                                       |
| 27265 | 1.478819              | 2.387751                                                       |
| 27267 | 1.364287              | 2.387756                                                       |
| 27269 | 1.137115              | 2.387762                                                       |
| 27271 | 1.000037              | 2.387767                                                       |
| 27273 | 1.333480              | 2.387773                                                       |
| 27275 | 1.241137              | 2.387778                                                       |
| 27277 | 1.000037              | 2.387783                                                       |
| 27279 | 1.654606              | 2.387789                                                       |
| 27281 | 1.000037              | 2.387794                                                       |
| 27283 | 1.000037              | 2.387800                                                       |
| 27285 | 1.709951              | 2.387805                                                       |
| 27287 | 1.077436              | 2.387811                                                       |
| 27289 | 1.035582              | 2.387816                                                       |
| 27291 | 1.456304              | 2.387821                                                       |
| 27293 | 1.165354              | 2.387827                                                       |

| $n$   | $\frac{\sigma(n)}{n}$ | $\frac{e^\gamma}{2} \log \log n + \frac{0.73...}{\log \log n}$ |
|-------|-----------------------|----------------------------------------------------------------|
| 27295 | 1.234512              | 2.387832                                                       |
| 27297 | 1.498260              | 2.387838                                                       |
| 27299 | 1.000037              | 2.387843                                                       |
| 27301 | 1.044357              | 2.387848                                                       |
| 27303 | 1.406439              | 2.387854                                                       |
| 27305 | 1.237576              | 2.387859                                                       |
| 27307 | 1.181236              | 2.387865                                                       |
| 27309 | 1.333480              | 2.387870                                                       |
| 27311 | 1.033430              | 2.387875                                                       |
| 27313 | 1.180976              | 2.387881                                                       |
| 27315 | 1.736189              | 2.387886                                                       |
| 27317 | 1.019146              | 2.387892                                                       |
| 27319 | 1.059482              | 2.387897                                                       |
| 27321 | 1.524981              | 2.387902                                                       |
| 27323 | 1.014530              | 2.387908                                                       |
| 27325 | 1.241134              | 2.387913                                                       |
| 27327 | 1.333480              | 2.387919                                                       |
| 27329 | 1.000037              | 2.387924                                                       |
| 27331 | 1.012184              | 2.387929                                                       |
| 27333 | 1.444920              | 2.387935                                                       |
| 27335 | 1.517176              | 2.387940                                                       |
| 27337 | 1.000037              | 2.387946                                                       |
| 27339 | 1.437946              | 2.387951                                                       |
| 27341 | 1.053363              | 2.387956                                                       |
| 27343 | 1.028417              | 2.387962                                                       |
| 27345 | 1.600878              | 2.387967                                                       |
| 27347 | 1.105789              | 2.387973                                                       |
| 27349 | 1.143150              | 2.387978                                                       |
| 27351 | 1.482944              | 2.387983                                                       |
| 27353 | 1.059482              | 2.387989                                                       |
| 27355 | 1.200219              | 2.387994                                                       |
| 27357 | 1.456300              | 2.387999                                                       |
| 27359 | 1.013195              | 2.388005                                                       |
| 27361 | 1.000037              | 2.388010                                                       |
| 27363 | 1.524979              | 2.388016                                                       |
| 27365 | 1.295377              | 2.388021                                                       |
| 27367 | 1.000037              | 2.388026                                                       |
| 27369 | 1.444919              | 2.388032                                                       |
| 27371 | 1.013628              | 2.388037                                                       |
| 27373 | 1.033427              | 2.388043                                                       |
| 27375 | 1.686795              | 2.388048                                                       |
| 27377 | 1.143149              | 2.388053                                                       |
| 27379 | 1.157091              | 2.388059                                                       |
| 27381 | 1.333479              | 2.388064                                                       |

| $n$   | $\frac{\sigma(n)}{n}$ | $\frac{e^\gamma}{2} \log \log n + \frac{0.73\dots}{\log \log n}$ |
|-------|-----------------------|------------------------------------------------------------------|
| 27383 | 1.012307              | 2.388070                                                         |
| 27385 | 1.200219              | 2.388075                                                         |
| 27387 | 1.537956              | 2.388080                                                         |
| 27389 | 1.018657              | 2.388086                                                         |
| 27391 | 1.281881              | 2.388091                                                         |
| 27393 | 1.394809              | 2.388096                                                         |
| 27395 | 1.200219              | 2.388102                                                         |
| 27397 | 1.000037              | 2.388107                                                         |
| 27399 | 1.333479              | 2.388113                                                         |
| 27401 | 1.135141              | 2.388118                                                         |
| 27403 | 1.017407              | 2.388123                                                         |
| 27405 | 2.101806              | 2.388129                                                         |
| 27407 | 1.000036              | 2.388134                                                         |
| 27409 | 1.000036              | 2.388140                                                         |
| 27411 | 1.333479              | 2.388145                                                         |
| 27413 | 1.015577              | 2.388150                                                         |
| 27415 | 1.200219              | 2.388156                                                         |
| 27417 | 1.552322              | 2.388161                                                         |
| 27419 | 1.143149              | 2.388166                                                         |
| 27421 | 1.059480              | 2.388172                                                         |
| 27423 | 1.581446              | 2.388177                                                         |
| 27425 | 1.241130              | 2.388183                                                         |
| 27427 | 1.000036              | 2.388188                                                         |
| 27429 | 1.371979              | 2.388193                                                         |
| 27431 | 1.000036              | 2.388199                                                         |
| 27433 | 1.143149              | 2.388204                                                         |
| 27435 | 1.679606              | 2.388209                                                         |
| 27437 | 1.000036              | 2.388215                                                         |
| 27439 | 1.044353              | 2.388220                                                         |
| 27441 | 1.444918              | 2.388226                                                         |
| 27443 | 1.077433              | 2.388231                                                         |
| 27445 | 1.311714              | 2.388236                                                         |
| 27447 | 1.524975              | 2.388242                                                         |
| 27449 | 1.000036              | 2.388247                                                         |
| 27451 | 1.013879              | 2.388252                                                         |
| 27453 | 1.333479              | 2.388258                                                         |
| 27455 | 1.341832              | 2.388263                                                         |
| 27457 | 1.000036              | 2.388269                                                         |
| 27459 | 1.511199              | 2.388274                                                         |
| 27461 | 1.143148              | 2.388279                                                         |
| 27463 | 1.035575              | 2.388285                                                         |
| 27465 | 1.600874              | 2.388290                                                         |
| 27467 | 1.104016              | 2.388295                                                         |
| 27469 | 1.077433              | 2.388301                                                         |

| $n$   | $\frac{\sigma(n)}{n}$ | $\frac{e^\gamma}{2} \log \log n + \frac{0.73\dots}{\log \log n}$ |
|-------|-----------------------|------------------------------------------------------------------|
| 27471 | 1.333479              | 2.388306                                                         |
| 27473 | 1.015106              | 2.388312                                                         |
| 27475 | 1.426169              | 2.388317                                                         |
| 27477 | 1.498854              | 2.388322                                                         |
| 27479 | 1.000036              | 2.388328                                                         |
| 27481 | 1.000036              | 2.388333                                                         |
| 27483 | 1.333479              | 2.388338                                                         |
| 27485 | 1.257413              | 2.388344                                                         |
| 27487 | 1.000036              | 2.388349                                                         |
| 27489 | 1.791553              | 2.388354                                                         |
| 27491 | 1.028409              | 2.388360                                                         |
| 27493 | 1.053359              | 2.388365                                                         |
| 27495 | 1.906383              | 2.388371                                                         |
| 27497 | 1.033422              | 2.388376                                                         |
| 27499 | 1.013273              | 2.388381                                                         |
| 27501 | 1.361405              | 2.388387                                                         |
| 27503 | 1.143148              | 2.388392                                                         |
| 27505 | 1.200218              | 2.388397                                                         |
| 27507 | 1.366343              | 2.388403                                                         |
| 27509 | 1.000036              | 2.388408                                                         |
| 27511 | 1.135837              | 2.388413                                                         |
| 27513 | 1.482935              | 2.388419                                                         |
| 27515 | 1.200218              | 2.388424                                                         |
| 27517 | 1.143148              | 2.388430                                                         |
| 27519 | 1.333479              | 2.388435                                                         |
| 27521 | 1.129319              | 2.388440                                                         |
| 27523 | 1.059478              | 2.388446                                                         |
| 27525 | 1.657838              | 2.388451                                                         |
| 27527 | 1.000036              | 2.388456                                                         |
| 27529 | 1.000036              | 2.388462                                                         |
| 27531 | 1.813229              | 2.388467                                                         |
| 27533 | 1.091345              | 2.388472                                                         |
| 27535 | 1.200218              | 2.388478                                                         |
| 27537 | 1.363111              | 2.388483                                                         |
| 27539 | 1.000036              | 2.388488                                                         |
| 27541 | 1.000036              | 2.388494                                                         |
| 27543 | 1.333479              | 2.388499                                                         |
| 27545 | 1.373171              | 2.388504                                                         |
| 27547 | 1.089483              | 2.388510                                                         |
| 27549 | 1.444916              | 2.388515                                                         |
| 27551 | 1.000036              | 2.388521                                                         |
| 27553 | 1.019127              | 2.388526                                                         |
| 27555 | 1.755906              | 2.388531                                                         |
| 27557 | 1.059477              | 2.388537                                                         |

| $n$   | $\frac{\sigma(n)}{n}$ | $\frac{e^\gamma}{2} \log \log n + \frac{0.73...}{\log \log n}$ |
|-------|-----------------------|----------------------------------------------------------------|
| 27559 | 1.189013              | 2.388542                                                       |
| 27561 | 1.333478              | 2.388547                                                       |
| 27563 | 1.024852              | 2.388553                                                       |
| 27565 | 1.240704              | 2.388558                                                       |
| 27567 | 1.482932              | 2.388563                                                       |
| 27569 | 1.053357              | 2.388569                                                       |
| 27571 | 1.015560              | 2.388574                                                       |
| 27573 | 1.657273              | 2.388579                                                       |
| 27575 | 1.241124              | 2.388585                                                       |
| 27577 | 1.148783              | 2.388590                                                       |
| 27579 | 1.383661              | 2.388595                                                       |
| 27581 | 1.000036              | 2.388601                                                       |
| 27583 | 1.000036              | 2.388606                                                       |
| 27585 | 1.736161              | 2.388611                                                       |
| 27587 | 1.165331              | 2.388617                                                       |
| 27589 | 1.023016              | 2.388622                                                       |
| 27591 | 1.414374              | 2.388627                                                       |
| 27593 | 1.025912              | 2.388633                                                       |
| 27595 | 1.200217              | 2.388638                                                       |
| 27597 | 1.333478              | 2.388643                                                       |
| 27599 | 1.180912              | 2.388649                                                       |
| 27601 | 1.143147              | 2.388654                                                       |
| 27603 | 1.444915              | 2.388660                                                       |
| 27605 | 1.200217              | 2.388665                                                       |
| 27607 | 1.053356              | 2.388670                                                       |
| 27609 | 1.333478              | 2.388676                                                       |
| 27611 | 1.000036              | 2.388681                                                       |
| 27613 | 1.020824              | 2.388686                                                       |
| 27615 | 1.835524              | 2.388692                                                       |
| 27617 | 1.000036              | 2.388697                                                       |
| 27619 | 1.016691              | 2.388702                                                       |
| 27621 | 1.682198              | 2.388708                                                       |
| 27623 | 1.044347              | 2.388713                                                       |
| 27625 | 1.423059              | 2.388718                                                       |
| 27627 | 1.333478              | 2.388724                                                       |
| 27629 | 1.143147              | 2.388729                                                       |
| 27631 | 1.000036              | 2.388734                                                       |
| 27633 | 1.364166              | 2.388740                                                       |
| 27635 | 1.200217              | 2.388745                                                       |
| 27637 | 1.035568              | 2.388750                                                       |
| 27639 | 1.501357              | 2.388756                                                       |
| 27641 | 1.012409              | 2.388761                                                       |
| 27643 | 1.250226              | 2.388766                                                       |
| 27645 | 1.701574              | 2.388772                                                       |



| $n$   | $\frac{\sigma(n)}{n}$ | $\frac{e^\gamma}{2} \log \log n + \frac{0.73\dots}{\log \log n}$ |
|-------|-----------------------|------------------------------------------------------------------|
| 27647 | 1.000036              | 2.388777                                                         |
| 27649 | 1.024847              | 2.388782                                                         |
| 27651 | 1.437923              | 2.388788                                                         |
| 27653 | 1.000036              | 2.388793                                                         |
| 27655 | 1.200217              | 2.388798                                                         |
| 27657 | 1.654554              | 2.388804                                                         |
| 27659 | 1.059474              | 2.388809                                                         |
| 27661 | 1.012256              | 2.388814                                                         |
| 27663 | 1.333478              | 2.388820                                                         |
| 27665 | 1.311693              | 2.388825                                                         |
| 27667 | 1.016373              | 2.388830                                                         |
| 27669 | 1.394774              | 2.388836                                                         |
| 27671 | 1.179574              | 2.388841                                                         |
| 27673 | 1.000036              | 2.388846                                                         |
| 27675 | 1.881843              | 2.388851                                                         |
| 27677 | 1.077429              | 2.388857                                                         |
| 27679 | 1.014488              | 2.388862                                                         |
| 27681 | 1.333478              | 2.388867                                                         |
| 27683 | 1.109706              | 2.388873                                                         |
| 27685 | 1.408272              | 2.388878                                                         |
| 27687 | 1.456279              | 2.388883                                                         |
| 27689 | 1.000036              | 2.388889                                                         |
| 27691 | 1.000036              | 2.388894                                                         |
| 27693 | 1.537862              | 2.388899                                                         |
| 27695 | 1.247879              | 2.388905                                                         |
| 27697 | 1.000036              | 2.388910                                                         |
| 27699 | 1.524965              | 2.388915                                                         |
| 27701 | 1.000036              | 2.388921                                                         |
| 27703 | 1.077428              | 2.388926                                                         |
| 27705 | 1.600866              | 2.388931                                                         |
| 27707 | 1.013462              | 2.388937                                                         |
| 27709 | 1.103973              | 2.388942                                                         |
| 27711 | 1.444914              | 2.388947                                                         |
| 27713 | 1.184715              | 2.388953                                                         |
| 27715 | 1.257370              | 2.388958                                                         |
| 27717 | 1.333478              | 2.388963                                                         |
| 27719 | 1.020816              | 2.388969                                                         |
| 27721 | 1.053353              | 2.388974                                                         |
| 27723 | 1.333478              | 2.388979                                                         |
| 27725 | 1.241118              | 2.388984                                                         |
| 27727 | 1.215278              | 2.388990                                                         |
| 27729 | 1.615637              | 2.388995                                                         |
| 27731 | 1.091342              | 2.389000                                                         |
| 27733 | 1.000036              | 2.389006                                                         |

| $n$   | $\frac{\sigma(n)}{n}$ | $\frac{e^\gamma}{2} \log \log n + \frac{0.73\dots}{\log \log n}$ |
|-------|-----------------------|------------------------------------------------------------------|
| 27735 | 1.638075              | 2.389011                                                         |
| 27737 | 1.000036              | 2.389016                                                         |
| 27739 | 1.000036              | 2.389022                                                         |
| 27741 | 1.524963              | 2.389027                                                         |
| 27743 | 1.000036              | 2.389032                                                         |
| 27745 | 1.245630              | 2.389038                                                         |
| 27747 | 1.444913              | 2.389043                                                         |
| 27749 | 1.000036              | 2.389048                                                         |
| 27751 | 1.000036              | 2.389054                                                         |
| 27753 | 1.506432              | 2.389059                                                         |
| 27755 | 1.501135              | 2.389064                                                         |
| 27757 | 1.025903              | 2.389069                                                         |
| 27759 | 1.406391              | 2.389075                                                         |
| 27761 | 1.120421              | 2.389080                                                         |
| 27763 | 1.000036              | 2.389085                                                         |
| 27765 | 1.736143              | 2.389091                                                         |
| 27767 | 1.000036              | 2.389096                                                         |
| 27769 | 1.143145              | 2.389101                                                         |
| 27771 | 1.333477              | 2.389107                                                         |
| 27773 | 1.000036              | 2.389112                                                         |
| 27775 | 1.366121              | 2.389117                                                         |
| 27777 | 1.368614              | 2.389123                                                         |
| 27779 | 1.000036              | 2.389128                                                         |
| 27781 | 1.077427              | 2.389133                                                         |
| 27783 | 1.742072              | 2.389138                                                         |
| 27785 | 1.200216              | 2.389144                                                         |
| 27787 | 1.028395              | 2.389149                                                         |
| 27789 | 1.364569              | 2.389154                                                         |
| 27791 | 1.000036              | 2.389160                                                         |
| 27793 | 1.000036              | 2.389165                                                         |
| 27795 | 1.709660              | 2.389170                                                         |
| 27797 | 1.315825              | 2.389176                                                         |
| 27799 | 1.000036              | 2.389181                                                         |
| 27801 | 1.444912              | 2.389186                                                         |
| 27803 | 1.000036              | 2.389191                                                         |
| 27805 | 1.232584              | 2.389197                                                         |
| 27807 | 1.546661              | 2.389202                                                         |
| 27809 | 1.000036              | 2.389207                                                         |
| 27811 | 1.190896              | 2.389213                                                         |
| 27813 | 1.362241              | 2.389218                                                         |
| 27815 | 1.200216              | 2.389223                                                         |
| 27817 | 1.000036              | 2.389229                                                         |
| 27819 | 1.581365              | 2.389234                                                         |
| 27821 | 1.024837              | 2.389239                                                         |

| $n$   | $\frac{\sigma(n)}{n}$ | $\frac{e^\gamma}{2} \log \log n + \frac{0.73\dots}{\log \log n}$ |
|-------|-----------------------|------------------------------------------------------------------|
| 27823 | 1.000036              | 2.389244                                                         |
| 27825 | 1.925175              | 2.389250                                                         |
| 27827 | 1.000036              | 2.389255                                                         |
| 27829 | 1.059470              | 2.389260                                                         |
| 27831 | 1.333477              | 2.389266                                                         |
| 27833 | 1.077426              | 2.389271                                                         |
| 27835 | 1.267469              | 2.389276                                                         |
| 27837 | 1.482918              | 2.389281                                                         |
| 27839 | 1.182801              | 2.389287                                                         |
| 27841 | 1.091340              | 2.389292                                                         |
| 27843 | 1.333477              | 2.389297                                                         |
| 27845 | 1.200215              | 2.389303                                                         |
| 27847 | 1.000036              | 2.389308                                                         |
| 27849 | 1.333477              | 2.389313                                                         |
| 27851 | 1.000036              | 2.389318                                                         |
| 27853 | 1.199440              | 2.389324                                                         |
| 27855 | 1.736134              | 2.389329                                                         |
| 27857 | 1.014467              | 2.389334                                                         |
| 27859 | 1.077426              | 2.389340                                                         |
| 27861 | 1.374825              | 2.389345                                                         |
| 27863 | 1.162832              | 2.389350                                                         |
| 27865 | 1.200215              | 2.389356                                                         |
| 27867 | 1.524958              | 2.389361                                                         |
| 27869 | 1.068930              | 2.389366                                                         |
| 27871 | 1.022999              | 2.389371                                                         |
| 27873 | 1.529796              | 2.389377                                                         |
| 27875 | 1.253596              | 2.389382                                                         |
| 27877 | 1.018617              | 2.389387                                                         |
| 27879 | 1.333477              | 2.389392                                                         |
| 27881 | 1.165310              | 2.389398                                                         |
| 27883 | 1.000036              | 2.389403                                                         |
| 27885 | 1.890048              | 2.389408                                                         |
| 27887 | 1.015527              | 2.389414                                                         |
| 27889 | 1.006024              | 2.389419                                                         |
| 27891 | 1.482916              | 2.389424                                                         |
| 27893 | 1.000036              | 2.389429                                                         |
| 27895 | 1.373149              | 2.389435                                                         |
| 27897 | 1.414346              | 2.389440                                                         |
| 27899 | 1.044339              | 2.389445                                                         |
| 27901 | 1.000036              | 2.389451                                                         |
| 27903 | 1.362434              | 2.389456                                                         |
| 27905 | 1.200215              | 2.389461                                                         |
| 27907 | 1.135199              | 2.389466                                                         |
| 27909 | 1.654520              | 2.389472                                                         |

| $n$   | $\frac{\sigma(n)}{n}$ | $\frac{e^\gamma}{2} \log \log n + \frac{0.73...}{\log \log n}$ |
|-------|-----------------------|----------------------------------------------------------------|
| 27911 | 1.143635              | 2.389477                                                       |
| 27913 | 1.013435              | 2.389482                                                       |
| 27915 | 1.600860              | 2.389488                                                       |
| 27917 | 1.000036              | 2.389493                                                       |
| 27919 | 1.000036              | 2.389498                                                       |
| 27921 | 1.371871              | 2.389503                                                       |
| 27923 | 1.143144              | 2.389509                                                       |
| 27925 | 1.241110              | 2.389514                                                       |
| 27927 | 1.508218              | 2.389519                                                       |
| 27929 | 1.091339              | 2.389524                                                       |
| 27931 | 1.113601              | 2.389530                                                       |
| 27933 | 1.333477              | 2.389535                                                       |
| 27935 | 1.240594              | 2.389540                                                       |
| 27937 | 1.234778              | 2.389546                                                       |
| 27939 | 1.362969              | 2.389551                                                       |
| 27941 | 1.000036              | 2.389556                                                       |
| 27943 | 1.000036              | 2.389561                                                       |
| 27945 | 1.875684              | 2.389567                                                       |
| 27947 | 1.000036              | 2.389572                                                       |
| 27949 | 1.053347              | 2.389577                                                       |
| 27951 | 1.676076              | 2.389582                                                       |
| 27953 | 1.000036              | 2.389588                                                       |
| 27955 | 1.200215              | 2.389593                                                       |
| 27957 | 1.333476              | 2.389598                                                       |
| 27959 | 1.016345              | 2.389603                                                       |
| 27961 | 1.000036              | 2.389609                                                       |
| 27963 | 1.562064              | 2.389614                                                       |
| 27965 | 1.482997              | 2.389619                                                       |
| 27967 | 1.000036              | 2.389625                                                       |
| 27969 | 1.333476              | 2.389630                                                       |
| 27971 | 1.015051              | 2.389635                                                       |
| 27973 | 1.091338              | 2.389640                                                       |
| 27975 | 1.657766              | 2.389646                                                       |
| 27977 | 1.013547              | 2.389651                                                       |
| 27979 | 1.165303              | 2.389656                                                       |
| 27981 | 1.444909              | 2.389661                                                       |
| 27983 | 1.000036              | 2.389667                                                       |
| 27985 | 1.247811              | 2.389672                                                       |
| 27987 | 1.406367              | 2.389677                                                       |
| 27989 | 1.077423              | 2.389682                                                       |
| 27991 | 1.044336              | 2.389688                                                       |
| 27993 | 1.609545              | 2.389693                                                       |
| 27995 | 1.311663              | 2.389698                                                       |
| 27997 | 1.000036              | 2.389703                                                       |

| $n$   | $\frac{\sigma(n)}{n}$ | $\frac{e^\gamma}{2} \log \log n + \frac{0.73...}{\log \log n}$ |
|-------|-----------------------|----------------------------------------------------------------|
| 27999 | 1.594343              | 2.389709                                                       |
| 28001 | 1.000036              | 2.389714                                                       |
| 28003 | 1.025890              | 2.389719                                                       |
| 28005 | 1.600857              | 2.389725                                                       |
| 28007 | 1.143143              | 2.389730                                                       |
| 28009 | 1.028384              | 2.389735                                                       |
| 28011 | 1.333476              | 2.389740                                                       |
| 28013 | 1.013101              | 2.389746                                                       |
| 28015 | 1.295306              | 2.389751                                                       |
| 28017 | 1.581326              | 2.389756                                                       |
| 28019 | 1.000036              | 2.389761                                                       |
| 28021 | 1.143143              | 2.389767                                                       |
| 28023 | 1.333476              | 2.389772                                                       |
| 28025 | 1.327386              | 2.389777                                                       |
| 28027 | 1.000036              | 2.389782                                                       |
| 28029 | 1.333476              | 2.389788                                                       |
| 28031 | 1.000036              | 2.389793                                                       |
| 28033 | 1.073235              | 2.389798                                                       |
| 28035 | 2.003210              | 2.389803                                                       |
| 28037 | 1.065093              | 2.389809                                                       |
| 28039 | 1.091337              | 2.389814                                                       |
| 28041 | 1.437895              | 2.389819                                                       |
| 28043 | 1.035553              | 2.389824                                                       |
| 28045 | 1.232305              | 2.389830                                                       |
| 28047 | 1.333476              | 2.389835                                                       |
| 28049 | 1.143142              | 2.389840                                                       |
| 28051 | 1.000036              | 2.389845                                                       |
| 28053 | 1.482907              | 2.389851                                                       |
| 28055 | 1.245553              | 2.389856                                                       |
| 28057 | 1.000036              | 2.389861                                                       |
| 28059 | 1.368545              | 2.389866                                                       |
| 28061 | 1.091337              | 2.389872                                                       |
| 28063 | 1.208709              | 2.389877                                                       |
| 28065 | 1.600855              | 2.389882                                                       |
| 28067 | 1.149250              | 2.389887                                                       |
| 28069 | 1.000036              | 2.389893                                                       |
| 28071 | 1.444908              | 2.389898                                                       |
| 28073 | 1.017348              | 2.389903                                                       |
| 28075 | 1.241104              | 2.389908                                                       |
| 28077 | 1.559141              | 2.389914                                                       |
| 28079 | 1.024823              | 2.389919                                                       |
| 28081 | 1.000036              | 2.389924                                                       |
| 28083 | 1.558808              | 2.389929                                                       |
| 28085 | 1.238241              | 2.389934                                                       |

| $n$   | $\frac{\sigma(n)}{n}$ | $\frac{e^\gamma}{2} \log \log n + \frac{0.73\dots}{\log \log n}$ |
|-------|-----------------------|------------------------------------------------------------------|
| 28087 | 1.000036              | 2.389940                                                         |
| 28089 | 1.444907              | 2.389945                                                         |
| 28091 | 1.143142              | 2.389950                                                         |
| 28093 | 1.077421              | 2.389955                                                         |
| 28095 | 1.600854              | 2.389961                                                         |
| 28097 | 1.000036              | 2.389966                                                         |
| 28099 | 1.000036              | 2.389971                                                         |
| 28101 | 1.537312              | 2.389976                                                         |
| 28103 | 1.011992              | 2.389982                                                         |
| 28105 | 1.516598              | 2.389987                                                         |
| 28107 | 1.498132              | 2.389992                                                         |
| 28109 | 1.000036              | 2.389997                                                         |
| 28111 | 1.000036              | 2.390003                                                         |
| 28113 | 1.333476              | 2.390008                                                         |
| 28115 | 1.200213              | 2.390013                                                         |
| 28117 | 1.033396              | 2.390018                                                         |
| 28119 | 1.656958              | 2.390024                                                         |
| 28121 | 1.018598              | 2.390029                                                         |
| 28123 | 1.000036              | 2.390034                                                         |
| 28125 | 1.805440              | 2.390039                                                         |
| 28127 | 1.091336              | 2.390044                                                         |
| 28129 | 1.044331              | 2.390050                                                         |
| 28131 | 1.333476              | 2.390055                                                         |
| 28133 | 1.143142              | 2.390060                                                         |
| 28135 | 1.274427              | 2.390065                                                         |
| 28137 | 1.361339              | 2.390071                                                         |
| 28139 | 1.053342              | 2.390076                                                         |
| 28141 | 1.013184              | 2.390081                                                         |
| 28143 | 1.496642              | 2.390086                                                         |
| 28145 | 1.295292              | 2.390092                                                         |
| 28147 | 1.143141              | 2.390097                                                         |
| 28149 | 1.456251              | 2.390102                                                         |
| 28151 | 1.000036              | 2.390107                                                         |
| 28153 | 1.022982              | 2.390112                                                         |
| 28155 | 1.600852              | 2.390118                                                         |
| 28157 | 1.028377              | 2.390123                                                         |
| 28159 | 1.035548              | 2.390128                                                         |
| 28161 | 1.704485              | 2.390133                                                         |
| 28163 | 1.000036              | 2.390139                                                         |
| 28165 | 1.237280              | 2.390144                                                         |
| 28167 | 1.371818              | 2.390149                                                         |
| 28169 | 1.059463              | 2.390154                                                         |
| 28171 | 1.180789              | 2.390159                                                         |
| 28173 | 1.333475              | 2.390165                                                         |

| $n$   | $\frac{\sigma(n)}{n}$ | $\frac{e^\gamma}{2} \log \log n + \frac{0.73\dots}{\log \log n}$ |
|-------|-----------------------|------------------------------------------------------------------|
| 28175 | 1.505164              | 2.390170                                                         |
| 28177 | 1.053341              | 2.390175                                                         |
| 28179 | 1.505802              | 2.390180                                                         |
| 28181 | 1.000035              | 2.390186                                                         |
| 28183 | 1.000035              | 2.390191                                                         |
| 28185 | 1.600852              | 2.390196                                                         |
| 28187 | 1.016639              | 2.390201                                                         |
| 28189 | 1.143141              | 2.390206                                                         |
| 28191 | 1.333475              | 2.390212                                                         |
| 28193 | 1.103891              | 2.390217                                                         |
| 28195 | 1.200213              | 2.390222                                                         |
| 28197 | 1.562010              | 2.390227                                                         |
| 28199 | 1.011951              | 2.390233                                                         |
| 28201 | 1.000035              | 2.390238                                                         |
| 28203 | 1.633869              | 2.390243                                                         |
| 28205 | 1.200213              | 2.390248                                                         |
| 28207 | 1.017336              | 2.390253                                                         |
| 28209 | 1.333475              | 2.390259                                                         |
| 28211 | 1.000035              | 2.390264                                                         |
| 28213 | 1.014426              | 2.390269                                                         |
| 28215 | 2.041467              | 2.390274                                                         |
| 28217 | 1.190772              | 2.390279                                                         |
| 28219 | 1.000035              | 2.390285                                                         |
| 28221 | 1.394706              | 2.390290                                                         |
| 28223 | 1.089324              | 2.390295                                                         |
| 28225 | 1.241098              | 2.390300                                                         |
| 28227 | 1.347221              | 2.390306                                                         |
| 28229 | 1.000035              | 2.390311                                                         |
| 28231 | 1.184513              | 2.390316                                                         |
| 28233 | 1.444905              | 2.390321                                                         |
| 28235 | 1.200213              | 2.390326                                                         |
| 28237 | 1.162730              | 2.390332                                                         |
| 28239 | 1.333475              | 2.390337                                                         |
| 28241 | 1.033391              | 2.390342                                                         |
| 28243 | 1.018589              | 2.390347                                                         |
| 28245 | 1.835369              | 2.390352                                                         |
| 28247 | 1.022976              | 2.390358                                                         |
| 28249 | 1.124004              | 2.390363                                                         |
| 28251 | 1.498283              | 2.390368                                                         |
| 28253 | 1.053339              | 2.390373                                                         |
| 28255 | 1.200212              | 2.390379                                                         |
| 28257 | 1.333475              | 2.390384                                                         |
| 28259 | 1.250150              | 2.390389                                                         |
| 28261 | 1.019072              | 2.390394                                                         |

| $n$   | $\frac{\sigma(n)}{n}$ | $\frac{e^\gamma}{2} \log \log n + \frac{0.73\dots}{\log \log n}$ |
|-------|-----------------------|------------------------------------------------------------------|
| 28263 | 1.333475              | 2.390399                                                         |
| 28265 | 1.200212              | 2.390405                                                         |
| 28267 | 1.044327              | 2.390410                                                         |
| 28269 | 1.498107              | 2.390415                                                         |
| 28271 | 1.059460              | 2.390420                                                         |
| 28273 | 1.165281              | 2.390425                                                         |
| 28275 | 1.841910              | 2.390431                                                         |
| 28277 | 1.000035              | 2.390436                                                         |
| 28279 | 1.000035              | 2.390441                                                         |
| 28281 | 1.456243              | 2.390446                                                         |
| 28283 | 1.000035              | 2.390451                                                         |
| 28285 | 1.200212              | 2.390457                                                         |
| 28287 | 1.654470              | 2.390462                                                         |
| 28289 | 1.000035              | 2.390467                                                         |
| 28291 | 1.053339              | 2.390472                                                         |
| 28293 | 1.333475              | 2.390477                                                         |
| 28295 | 1.200212              | 2.390483                                                         |
| 28297 | 1.000035              | 2.390488                                                         |
| 28299 | 1.333475              | 2.390493                                                         |
| 28301 | 1.234727              | 2.390498                                                         |
| 28303 | 1.139667              | 2.390503                                                         |
| 28305 | 1.884897              | 2.390509                                                         |
| 28307 | 1.000035              | 2.390514                                                         |
| 28309 | 1.000035              | 2.390519                                                         |
| 28311 | 1.333475              | 2.390524                                                         |
| 28313 | 1.044326              | 2.390529                                                         |
| 28315 | 1.373124              | 2.390535                                                         |
| 28317 | 1.333475              | 2.390540                                                         |
| 28319 | 1.000035              | 2.390545                                                         |
| 28321 | 1.012394              | 2.390550                                                         |
| 28323 | 1.482894              | 2.390555                                                         |
| 28325 | 1.365861              | 2.390560                                                         |
| 28327 | 1.077417              | 2.390566                                                         |
| 28329 | 1.626602              | 2.390571                                                         |
| 28331 | 1.025873              | 2.390576                                                         |
| 28333 | 1.035542              | 2.390581                                                         |
| 28335 | 1.600847              | 2.390586                                                         |
| 28337 | 1.024809              | 2.390592                                                         |
| 28339 | 1.059459              | 2.390597                                                         |
| 28341 | 1.497195              | 2.390602                                                         |
| 28343 | 1.143139              | 2.390607                                                         |
| 28345 | 1.200212              | 2.390612                                                         |
| 28347 | 1.456239              | 2.390618                                                         |
| 28349 | 1.000035              | 2.390623                                                         |



| $n$   | $\frac{\sigma(n)}{n}$ | $\frac{e^\gamma}{2} \log \log n + \frac{0.73...}{\log \log n}$ |
|-------|-----------------------|----------------------------------------------------------------|
| 28351 | 1.000035              | 2.390628                                                       |
| 28353 | 1.437873              | 2.390633                                                       |
| 28355 | 1.234068              | 2.390638                                                       |
| 28357 | 1.143139              | 2.390644                                                       |
| 28359 | 1.518248              | 2.390649                                                       |
| 28361 | 1.015479              | 2.390654                                                       |
| 28363 | 1.012869              | 2.390659                                                       |
| 28365 | 1.678689              | 2.390664                                                       |
| 28367 | 1.053337              | 2.390669                                                       |
| 28369 | 1.091332              | 2.390675                                                       |
| 28371 | 1.559057              | 2.390680                                                       |
| 28373 | 1.059458              | 2.390685                                                       |
| 28375 | 1.253498              | 2.390690                                                       |
| 28377 | 1.482891              | 2.390695                                                       |
| 28379 | 1.124775              | 2.390701                                                       |
| 28381 | 1.013495              | 2.390706                                                       |
| 28383 | 1.333474              | 2.390711                                                       |
| 28385 | 1.373120              | 2.390716                                                       |
| 28387 | 1.000035              | 2.390721                                                       |
| 28389 | 1.333474              | 2.390726                                                       |
| 28391 | 1.141207              | 2.390732                                                       |
| 28393 | 1.000035              | 2.390737                                                       |
| 28395 | 1.736080              | 2.390742                                                       |
| 28397 | 1.016305              | 2.390747                                                       |
| 28399 | 1.143139              | 2.390752                                                       |
| 28401 | 1.333474              | 2.390758                                                       |
| 28403 | 1.000035              | 2.390763                                                       |
| 28405 | 1.419468              | 2.390768                                                       |
| 28407 | 1.414299              | 2.390773                                                       |
| 28409 | 1.000035              | 2.390778                                                       |
| 28411 | 1.000035              | 2.390783                                                       |
| 28413 | 1.844789              | 2.390789                                                       |
| 28415 | 1.200211              | 2.390794                                                       |
| 28417 | 1.011929              | 2.390799                                                       |
| 28419 | 1.333474              | 2.390804                                                       |
| 28421 | 1.013757              | 2.390809                                                       |
| 28423 | 1.024804              | 2.390814                                                       |
| 28425 | 1.657696              | 2.390820                                                       |
| 28427 | 1.188729              | 2.390825                                                       |
| 28429 | 1.000035              | 2.390830                                                       |
| 28431 | 1.615138              | 2.390835                                                       |
| 28433 | 1.000035              | 2.390840                                                       |
| 28435 | 1.347072              | 2.390846                                                       |
| 28437 | 1.333474              | 2.390851                                                       |

| $n$   | $\frac{\sigma(n)}{n}$ | $\frac{e^\gamma}{2} \log \log n + \frac{0.73...}{\log \log n}$ |
|-------|-----------------------|----------------------------------------------------------------|
| 28439 | 1.000035              | 2.390856                                                       |
| 28441 | 1.215147              | 2.390861                                                       |
| 28443 | 1.406321              | 2.390866                                                       |
| 28445 | 1.200211              | 2.390871                                                       |
| 28447 | 1.000035              | 2.390877                                                       |
| 28449 | 1.507962              | 2.390882                                                       |
| 28451 | 1.044322              | 2.390887                                                       |
| 28453 | 1.028363              | 2.390892                                                       |
| 28455 | 1.835319              | 2.390897                                                       |
| 28457 | 1.180729              | 2.390902                                                       |
| 28459 | 1.011982              | 2.390908                                                       |
| 28461 | 1.366080              | 2.390913                                                       |
| 28463 | 1.000035              | 2.390918                                                       |
| 28465 | 1.200211              | 2.390923                                                       |
| 28467 | 1.444901              | 2.390928                                                       |
| 28469 | 1.180231              | 2.390933                                                       |
| 28471 | 1.016613              | 2.390939                                                       |
| 28473 | 1.333474              | 2.390944                                                       |
| 28475 | 1.332537              | 2.390949                                                       |
| 28477 | 1.000035              | 2.390954                                                       |
| 28479 | 1.456231              | 2.390959                                                       |
| 28481 | 1.053334              | 2.390964                                                       |
| 28483 | 1.234701              | 2.390970                                                       |
| 28485 | 1.786203              | 2.390975                                                       |
| 28487 | 1.018570              | 2.390980                                                       |
| 28489 | 1.033381              | 2.390985                                                       |
| 28491 | 1.333474              | 2.390990                                                       |
| 28493 | 1.000035              | 2.390995                                                       |
| 28495 | 1.238112              | 2.391000                                                       |
| 28497 | 1.617012              | 2.391006                                                       |
| 28499 | 1.000035              | 2.391011                                                       |
| 28501 | 1.091330              | 2.391016                                                       |
| 28503 | 1.444901              | 2.391021                                                       |
| 28505 | 1.200210              | 2.391026                                                       |
| 28507 | 1.035535              | 2.391031                                                       |
| 28509 | 1.555719              | 2.391037                                                       |
| 28511 | 1.143138              | 2.391042                                                       |
| 28513 | 1.000035              | 2.391047                                                       |
| 28515 | 1.600842              | 2.391052                                                       |
| 28517 | 1.000035              | 2.391057                                                       |
| 28519 | 1.068761              | 2.391062                                                       |
| 28521 | 1.444900              | 2.391068                                                       |
| 28523 | 1.091330              | 2.391073                                                       |
| 28525 | 1.425837              | 2.391078                                                       |

| $n$   | $\frac{\sigma(n)}{n}$ | $\frac{e^\gamma}{2} \log \log n + \frac{0.73...}{\log \log n}$ |
|-------|-----------------------|----------------------------------------------------------------|
| 28527 | 1.374698              | 2.391083                                                       |
| 28529 | 1.022959              | 2.391088                                                       |
| 28531 | 1.013354              | 2.391093                                                       |
| 28533 | 1.333474              | 2.391098                                                       |
| 28535 | 1.295251              | 2.391104                                                       |
| 28537 | 1.000035              | 2.391109                                                       |
| 28539 | 1.704334              | 2.391114                                                       |
| 28541 | 1.000035              | 2.391119                                                       |
| 28543 | 1.119994              | 2.391124                                                       |
| 28545 | 1.755544              | 2.391129                                                       |
| 28547 | 1.000035              | 2.391134                                                       |
| 28549 | 1.000035              | 2.391140                                                       |
| 28551 | 1.380827              | 2.391145                                                       |
| 28553 | 1.143137              | 2.391150                                                       |
| 28555 | 1.200210              | 2.391155                                                       |
| 28557 | 1.529572              | 2.391160                                                       |
| 28559 | 1.000035              | 2.391165                                                       |
| 28561 | 1.083330              | 2.391171                                                       |
| 28563 | 1.333473              | 2.391176                                                       |
| 28565 | 1.247681              | 2.391181                                                       |
| 28567 | 1.292960              | 2.391186                                                       |
| 28569 | 1.360916              | 2.391191                                                       |
| 28571 | 1.000035              | 2.391196                                                       |
| 28573 | 1.000035              | 2.391201                                                       |
| 28575 | 1.805214              | 2.391207                                                       |
| 28577 | 1.085278              | 2.391212                                                       |
| 28579 | 1.000035              | 2.391217                                                       |
| 28581 | 1.524929              | 2.391222                                                       |
| 28583 | 1.013470              | 2.391227                                                       |
| 28585 | 1.200210              | 2.391232                                                       |
| 28587 | 1.437856              | 2.391237                                                       |
| 28589 | 1.148414              | 2.391243                                                       |
| 28591 | 1.000035              | 2.391248                                                       |
| 28593 | 1.498059              | 2.391253                                                       |
| 28595 | 1.477181              | 2.391258                                                       |
| 28597 | 1.000035              | 2.391263                                                       |
| 28599 | 1.333473              | 2.391268                                                       |
| 28601 | 1.028356              | 2.391273                                                       |
| 28603 | 1.000035              | 2.391279                                                       |
| 28605 | 1.600839              | 2.391284                                                       |
| 28607 | 1.000035              | 2.391289                                                       |
| 28609 | 1.178930              | 2.391294                                                       |
| 28611 | 1.673902              | 2.391299                                                       |
| 28613 | 1.127320              | 2.391304                                                       |

| $n$   | $\frac{\sigma(n)}{n}$ | $\frac{e^\gamma}{2} \log \log n + \frac{0.73...}{\log \log n}$ |
|-------|-----------------------|----------------------------------------------------------------|
| 28615 | 1.232920              | 2.391309                                                       |
| 28617 | 1.333473              | 2.391314                                                       |
| 28619 | 1.000035              | 2.391320                                                       |
| 28621 | 1.000035              | 2.391325                                                       |
| 28623 | 1.609894              | 2.391330                                                       |
| 28625 | 1.253450              | 2.391335                                                       |
| 28627 | 1.000035              | 2.391340                                                       |
| 28629 | 1.444899              | 2.391345                                                       |
| 28631 | 1.000035              | 2.391350                                                       |
| 28633 | 1.156707              | 2.391356                                                       |
| 28635 | 1.689680              | 2.391361                                                       |
| 28637 | 1.143137              | 2.391366                                                       |
| 28639 | 1.077412              | 2.391371                                                       |
| 28641 | 1.333473              | 2.391376                                                       |
| 28643 | 1.000035              | 2.391381                                                       |
| 28645 | 1.274359              | 2.391386                                                       |
| 28647 | 1.482878              | 2.391391                                                       |
| 28649 | 1.000035              | 2.391397                                                       |
| 28651 | 1.143136              | 2.391402                                                       |
| 28653 | 1.333473              | 2.391407                                                       |
| 28655 | 1.311604              | 2.391412                                                       |
| 28657 | 1.000035              | 2.391417                                                       |
| 28659 | 1.371716              | 2.391422                                                       |
| 28661 | 1.000035              | 2.391427                                                       |
| 28663 | 1.000035              | 2.391432                                                       |
| 28665 | 2.171429              | 2.391438                                                       |
| 28667 | 1.013011              | 2.391443                                                       |
| 28669 | 1.000035              | 2.391448                                                       |
| 28671 | 1.406299              | 2.391453                                                       |
| 28673 | 1.020751              | 2.391458                                                       |
| 28675 | 1.314595              | 2.391463                                                       |
| 28677 | 1.484116              | 2.391468                                                       |
| 28679 | 1.215105              | 2.391473                                                       |
| 28681 | 1.104564              | 2.391479                                                       |
| 28683 | 1.444898              | 2.391484                                                       |
| 28685 | 1.200209              | 2.391489                                                       |
| 28687 | 1.000035              | 2.391494                                                       |
| 28689 | 1.361916              | 2.391499                                                       |
| 28691 | 1.077411              | 2.391504                                                       |
| 28693 | 1.143136              | 2.391509                                                       |
| 28695 | 1.600836              | 2.391514                                                       |
| 28697 | 1.000035              | 2.391520                                                       |
| 28699 | 1.091327              | 2.391525                                                       |
| 28701 | 1.482875              | 2.391530                                                       |

| $n$   | $\frac{\sigma(n)}{n}$ | $\frac{e^\gamma}{2} \log \log n + \frac{0.73...}{\log \log n}$ |
|-------|-----------------------|----------------------------------------------------------------|
| 28703 | 1.000035              | 2.391535                                                       |
| 28705 | 1.200209              | 2.391540                                                       |
| 28707 | 1.524924              | 2.391545                                                       |
| 28709 | 1.053328              | 2.391550                                                       |
| 28711 | 1.000035              | 2.391555                                                       |
| 28713 | 1.414272              | 2.391561                                                       |
| 28715 | 1.200209              | 2.391566                                                       |
| 28717 | 1.100324              | 2.391571                                                       |
| 28719 | 1.444897              | 2.391576                                                       |
| 28721 | 1.250096              | 2.391581                                                       |
| 28723 | 1.000035              | 2.391586                                                       |
| 28725 | 1.657650              | 2.391591                                                       |
| 28727 | 1.044314              | 2.391596                                                       |
| 28729 | 1.000035              | 2.391601                                                       |
| 28731 | 1.363823              | 2.391607                                                       |
| 28733 | 1.019037              | 2.391612                                                       |
| 28735 | 1.373099              | 2.391617                                                       |
| 28737 | 1.505516              | 2.391622                                                       |
| 28739 | 1.035527              | 2.391627                                                       |
| 28741 | 1.025852              | 2.391632                                                       |
| 28743 | 1.589813              | 2.391637                                                       |
| 28745 | 1.200209              | 2.391642                                                       |
| 28747 | 1.127074              | 2.391647                                                       |
| 28749 | 1.566107              | 2.391653                                                       |
| 28751 | 1.000035              | 2.391658                                                       |
| 28753 | 1.000035              | 2.391663                                                       |
| 28755 | 1.817840              | 2.391668                                                       |
| 28757 | 1.011928              | 2.391673                                                       |
| 28759 | 1.000035              | 2.391678                                                       |
| 28761 | 1.333472              | 2.391683                                                       |
| 28763 | 1.165247              | 2.391688                                                       |
| 28765 | 1.311594              | 2.391693                                                       |
| 28767 | 1.370459              | 2.391699                                                       |
| 28769 | 1.077410              | 2.391704                                                       |
| 28771 | 1.000035              | 2.391709                                                       |
| 28773 | 1.518090              | 2.391714                                                       |
| 28775 | 1.241077              | 2.391719                                                       |
| 28777 | 1.143135              | 2.391724                                                       |
| 28779 | 1.365996              | 2.391729                                                       |
| 28781 | 1.059449              | 2.391734                                                       |
| 28783 | 1.013098              | 2.391739                                                       |
| 28785 | 1.700886              | 2.391744                                                       |
| 28787 | 1.091326              | 2.391750                                                       |
| 28789 | 1.000035              | 2.391755                                                       |

| $n$   | $\frac{\sigma(n)}{n}$ | $\frac{e^\gamma}{2} \log \log n + \frac{0.73...}{\log \log n}$ |
|-------|-----------------------|----------------------------------------------------------------|
| 28791 | 1.654406              | 2.391760                                                       |
| 28793 | 1.000035              | 2.391765                                                       |
| 28795 | 1.295225              | 2.391770                                                       |
| 28797 | 1.383477              | 2.391775                                                       |
| 28799 | 1.033369              | 2.391780                                                       |
| 28801 | 1.014965              | 2.391785                                                       |
| 28803 | 1.333472              | 2.391790                                                       |
| 28805 | 1.373095              | 2.391796                                                       |
| 28807 | 1.000035              | 2.391801                                                       |
| 28809 | 1.632823              | 2.391806                                                       |
| 28811 | 1.022943              | 2.391811                                                       |
| 28813 | 1.000035              | 2.391816                                                       |
| 28815 | 1.709110              | 2.391821                                                       |
| 28817 | 1.000035              | 2.391826                                                       |
| 28819 | 1.199209              | 2.391831                                                       |
| 28821 | 1.437840              | 2.391836                                                       |
| 28823 | 1.107449              | 2.391841                                                       |
| 28825 | 1.241075              | 2.391846                                                       |
| 28827 | 1.444895              | 2.391852                                                       |
| 28829 | 1.012314              | 2.391857                                                       |
| 28831 | 1.091325              | 2.391862                                                       |
| 28833 | 1.524919              | 2.391867                                                       |
| 28835 | 1.231836              | 2.391872                                                       |
| 28837 | 1.000035              | 2.391877                                                       |
| 28839 | 1.333472              | 2.391882                                                       |
| 28841 | 1.011893              | 2.391887                                                       |
| 28843 | 1.000035              | 2.391892                                                       |
| 28845 | 1.736037              | 2.391897                                                       |
| 28847 | 1.234652              | 2.391903                                                       |
| 28849 | 1.059447              | 2.391908                                                       |
| 28851 | 1.364251              | 2.391913                                                       |
| 28853 | 1.134579              | 2.391918                                                       |
| 28855 | 1.247617              | 2.391923                                                       |
| 28857 | 1.333472              | 2.391928                                                       |
| 28859 | 1.000035              | 2.391933                                                       |
| 28861 | 1.263989              | 2.391938                                                       |
| 28863 | 1.482867              | 2.391943                                                       |
| 28865 | 1.257163              | 2.391948                                                       |
| 28867 | 1.000035              | 2.391953                                                       |
| 28869 | 1.333472              | 2.391958                                                       |
| 28871 | 1.000035              | 2.391964                                                       |
| 28873 | 1.077408              | 2.391969                                                       |
| 28875 | 2.074597              | 2.391974                                                       |
| 28877 | 1.017280              | 2.391979                                                       |

| $n$   | $\frac{\sigma(n)}{n}$ | $\frac{e^\gamma}{2} \log \log n + \frac{0.73...}{\log \log n}$ |
|-------|-----------------------|----------------------------------------------------------------|
| 28879 | 1.000035              | 2.391984                                                       |
| 28881 | 1.444895              | 2.391989                                                       |
| 28883 | 1.059447              | 2.391994                                                       |
| 28885 | 1.233858              | 2.391999                                                       |
| 28887 | 1.333472              | 2.392004                                                       |
| 28889 | 1.143134              | 2.392009                                                       |
| 28891 | 1.011803              | 2.392014                                                       |
| 28893 | 1.333472              | 2.392020                                                       |
| 28895 | 1.200208              | 2.392025                                                       |
| 28897 | 1.136173              | 2.392030                                                       |
| 28899 | 1.646424              | 2.392035                                                       |
| 28901 | 1.000035              | 2.392040                                                       |
| 28903 | 1.143134              | 2.392045                                                       |
| 28905 | 1.673897              | 2.392050                                                       |
| 28907 | 1.012073              | 2.392055                                                       |
| 28909 | 1.000035              | 2.392060                                                       |
| 28911 | 1.394625              | 2.392065                                                       |
| 28913 | 1.035520              | 2.392070                                                       |
| 28915 | 1.200208              | 2.392075                                                       |
| 28917 | 1.812636              | 2.392080                                                       |
| 28919 | 1.103773              | 2.392086                                                       |
| 28921 | 1.000035              | 2.392091                                                       |
| 28923 | 1.380770              | 2.392096                                                       |
| 28925 | 1.350389              | 2.392101                                                       |
| 28927 | 1.000035              | 2.392106                                                       |
| 28929 | 1.333472              | 2.392111                                                       |
| 28931 | 1.143134              | 2.392116                                                       |
| 28933 | 1.000035              | 2.392121                                                       |
| 28935 | 1.736029              | 2.392126                                                       |
| 28937 | 1.053323              | 2.392131                                                       |
| 28939 | 1.024776              | 2.392136                                                       |
| 28941 | 1.456204              | 2.392141                                                       |
| 28943 | 1.013302              | 2.392146                                                       |
| 28945 | 1.373087              | 2.392152                                                       |
| 28947 | 1.333472              | 2.392157                                                       |
| 28949 | 1.000035              | 2.392162                                                       |
| 28951 | 1.148976              | 2.392167                                                       |
| 28953 | 1.444893              | 2.392172                                                       |
| 28955 | 1.200207              | 2.392177                                                       |
| 28957 | 1.044307              | 2.392182                                                       |
| 28959 | 1.558894              | 2.392187                                                       |
| 28961 | 1.000035              | 2.392192                                                       |
| 28963 | 1.091323              | 2.392197                                                       |
| 28965 | 1.600829              | 2.392202                                                       |

| $n$   | $\frac{\sigma(n)}{n}$ | $\frac{e^\gamma}{2} \log \log n + \frac{0.73\dots}{\log \log n}$ |
|-------|-----------------------|------------------------------------------------------------------|
| 28967 | 1.014948              | 2.392207                                                         |
| 28969 | 1.019020              | 2.392212                                                         |
| 28971 | 1.573988              | 2.392217                                                         |
| 28973 | 1.143133              | 2.392223                                                         |
| 28975 | 1.326661              | 2.392228                                                         |
| 28977 | 1.437830              | 2.392233                                                         |
| 28979 | 1.000035              | 2.392238                                                         |
| 28981 | 1.016252              | 2.392243                                                         |
| 28983 | 1.333471              | 2.392248                                                         |
| 28985 | 1.430809              | 2.392253                                                         |
| 28987 | 1.182323              | 2.392258                                                         |
| 28989 | 1.444893              | 2.392263                                                         |
| 28991 | 1.020731              | 2.392268                                                         |
| 28993 | 1.015418              | 2.392273                                                         |
| 28995 | 1.600828              | 2.392278                                                         |
| 28997 | 1.013070              | 2.392283                                                         |
| 28999 | 1.022932              | 2.392288                                                         |
| 29001 | 1.524913              | 2.392293                                                         |
| 29003 | 1.135331              | 2.392298                                                         |
| 29005 | 1.200207              | 2.392304                                                         |
| 29007 | 1.581136              | 2.392309                                                         |
| 29009 | 1.000034              | 2.392314                                                         |
| 29011 | 1.017269              | 2.392319                                                         |
| 29013 | 1.406266              | 2.392324                                                         |
| 29015 | 1.373083              | 2.392329                                                         |
| 29017 | 1.000034              | 2.392334                                                         |
| 29019 | 1.414246              | 2.392339                                                         |
| 29021 | 1.000034              | 2.392344                                                         |
| 29023 | 1.000034              | 2.392349                                                         |
| 29025 | 1.879759              | 2.392354                                                         |
| 29027 | 1.000034              | 2.392359                                                         |
| 29029 | 1.388956              | 2.392364                                                         |
| 29031 | 1.333471              | 2.392369                                                         |
| 29033 | 1.000034              | 2.392374                                                         |
| 29035 | 1.200207              | 2.392379                                                         |
| 29037 | 1.333471              | 2.392384                                                         |
| 29039 | 1.016564              | 2.392390                                                         |
| 29041 | 1.012775              | 2.392395                                                         |
| 29043 | 1.654375              | 2.392400                                                         |
| 29045 | 1.240282              | 2.392405                                                         |
| 29047 | 1.033360              | 2.392410                                                         |
| 29049 | 1.394609              | 2.392415                                                         |
| 29051 | 1.156587              | 2.392420                                                         |
| 29053 | 1.059443              | 2.392425                                                         |



| $n$   | $\frac{\sigma(n)}{n}$ | $\frac{e^\gamma}{2} \log \log n + \frac{0.73...}{\log \log n}$ |
|-------|-----------------------|----------------------------------------------------------------|
| 29055 | 1.734641              | 2.392430                                                       |
| 29057 | 1.165227              | 2.392435                                                       |
| 29059 | 1.000034              | 2.392440                                                       |
| 29061 | 1.444892              | 2.392445                                                       |
| 29063 | 1.000034              | 2.392450                                                       |
| 29065 | 1.200206              | 2.392455                                                       |
| 29067 | 1.333471              | 2.392460                                                       |
| 29069 | 1.025835              | 2.392465                                                       |
| 29071 | 1.143132              | 2.392470                                                       |
| 29073 | 1.456196              | 2.392475                                                       |
| 29075 | 1.241066              | 2.392480                                                       |
| 29077 | 1.000034              | 2.392485                                                       |
| 29079 | 1.497988              | 2.392491                                                       |
| 29081 | 1.077404              | 2.392496                                                       |
| 29083 | 1.012275              | 2.392501                                                       |
| 29085 | 1.835173              | 2.392506                                                       |
| 29087 | 1.113900              | 2.392511                                                       |
| 29089 | 1.053319              | 2.392516                                                       |
| 29091 | 1.333471              | 2.392521                                                       |
| 29093 | 1.022926              | 2.392526                                                       |
| 29095 | 1.368483              | 2.392531                                                       |
| 29097 | 1.495824              | 2.392536                                                       |
| 29099 | 1.143132              | 2.392541                                                       |
| 29101 | 1.000034              | 2.392546                                                       |
| 29103 | 1.360684              | 2.392551                                                       |
| 29105 | 1.200206              | 2.392556                                                       |
| 29107 | 1.077404              | 2.392561                                                       |
| 29109 | 1.380741              | 2.392566                                                       |
| 29111 | 1.024767              | 2.392571                                                       |
| 29113 | 1.143132              | 2.392576                                                       |
| 29115 | 1.736012              | 2.392581                                                       |
| 29117 | 1.091321              | 2.392586                                                       |
| 29119 | 1.028332              | 2.392591                                                       |
| 29121 | 1.414237              | 2.392596                                                       |
| 29123 | 1.000034              | 2.392601                                                       |
| 29125 | 1.253356              | 2.392607                                                       |
| 29127 | 1.625983              | 2.392612                                                       |
| 29129 | 1.000034              | 2.392617                                                       |
| 29131 | 1.000034              | 2.392622                                                       |
| 29133 | 1.614664              | 2.392627                                                       |
| 29135 | 1.200206              | 2.392632                                                       |
| 29137 | 1.000034              | 2.392637                                                       |
| 29139 | 1.456193              | 2.392642                                                       |
| 29141 | 1.199135              | 2.392647                                                       |

| $n$   | $\frac{\sigma(n)}{n}$ | $\frac{e^\gamma}{2} \log \log n + \frac{0.73...}{\log \log n}$ |
|-------|-----------------------|----------------------------------------------------------------|
| 29143 | 1.011838              | 2.392652                                                       |
| 29145 | 1.679876              | 2.392657                                                       |
| 29147 | 1.000034              | 2.392662                                                       |
| 29149 | 1.013277              | 2.392667                                                       |
| 29151 | 1.498405              | 2.392672                                                       |
| 29153 | 1.000034              | 2.392677                                                       |
| 29155 | 1.481736              | 2.392682                                                       |
| 29157 | 1.333471              | 2.392687                                                       |
| 29159 | 1.077403              | 2.392692                                                       |
| 29161 | 1.103734              | 2.392697                                                       |
| 29163 | 1.333470              | 2.392702                                                       |
| 29165 | 1.267272              | 2.392707                                                       |
| 29167 | 1.000034              | 2.392712                                                       |
| 29169 | 1.654359              | 2.392717                                                       |
| 29171 | 1.033355              | 2.392722                                                       |
| 29173 | 1.000034              | 2.392727                                                       |
| 29175 | 1.657584              | 2.392732                                                       |
| 29177 | 1.011756              | 2.392737                                                       |
| 29179 | 1.000034              | 2.392742                                                       |
| 29181 | 1.361982              | 2.392747                                                       |
| 29183 | 1.250043              | 2.392752                                                       |
| 29185 | 1.295186              | 2.392758                                                       |
| 29187 | 1.578785              | 2.392763                                                       |
| 29189 | 1.072801              | 2.392768                                                       |
| 29191 | 1.000034              | 2.392773                                                       |
| 29193 | 1.374576              | 2.392778                                                       |
| 29195 | 1.200206              | 2.392783                                                       |
| 29197 | 1.181491              | 2.392788                                                       |
| 29199 | 1.333470              | 2.392793                                                       |
| 29201 | 1.000034              | 2.392798                                                       |
| 29203 | 1.109475              | 2.392803                                                       |
| 29205 | 1.922958              | 2.392808                                                       |
| 29207 | 1.000034              | 2.392813                                                       |
| 29209 | 1.000034              | 2.392818                                                       |
| 29211 | 1.656362              | 2.392823                                                       |
| 29213 | 1.012152              | 2.392828                                                       |
| 29215 | 1.200205              | 2.392833                                                       |
| 29217 | 1.333470              | 2.392838                                                       |
| 29219 | 1.018515              | 2.392843                                                       |
| 29221 | 1.000034              | 2.392848                                                       |
| 29223 | 1.537419              | 2.392853                                                       |
| 29225 | 1.425629              | 2.392858                                                       |
| 29227 | 1.091320              | 2.392863                                                       |
| 29229 | 1.333470              | 2.392868                                                       |

| $n$   | $\frac{\sigma(n)}{n}$ | $\frac{e^\gamma}{2} \log \log n + \frac{0.73...}{\log \log n}$ |
|-------|-----------------------|----------------------------------------------------------------|
| 29231 | 1.000034              | 2.392873                                                       |
| 29233 | 1.103411              | 2.392878                                                       |
| 29235 | 1.600821              | 2.392883                                                       |
| 29237 | 1.089099              | 2.392888                                                       |
| 29239 | 1.143131              | 2.392893                                                       |
| 29241 | 1.576588              | 2.392898                                                       |
| 29243 | 1.000034              | 2.392903                                                       |
| 29245 | 1.200205              | 2.392908                                                       |
| 29247 | 1.333470              | 2.392913                                                       |
| 29249 | 1.091319              | 2.392918                                                       |
| 29251 | 1.000034              | 2.392923                                                       |
| 29253 | 1.558814              | 2.392928                                                       |
| 29255 | 1.200205              | 2.392933                                                       |
| 29257 | 1.059439              | 2.392938                                                       |
| 29259 | 1.444889              | 2.392943                                                       |
| 29261 | 1.035508              | 2.392948                                                       |
| 29263 | 1.077401              | 2.392953                                                       |
| 29265 | 1.600820              | 2.392958                                                       |
| 29267 | 1.184132              | 2.392963                                                       |
| 29269 | 1.000034              | 2.392968                                                       |
| 29271 | 1.456185              | 2.392973                                                       |
| 29273 | 1.016227              | 2.392978                                                       |
| 29275 | 1.241059              | 2.392983                                                       |
| 29277 | 1.444888              | 2.392988                                                       |
| 29279 | 1.114792              | 2.392993                                                       |
| 29281 | 1.180288              | 2.392998                                                       |
| 29283 | 1.370351              | 2.393003                                                       |
| 29285 | 1.200205              | 2.393008                                                       |
| 29287 | 1.000034              | 2.393013                                                       |
| 29289 | 1.437809              | 2.393018                                                       |
| 29291 | 1.059438              | 2.393023                                                       |
| 29293 | 1.091319              | 2.393028                                                       |
| 29295 | 2.097286              | 2.393033                                                       |
| 29297 | 1.000034              | 2.393038                                                       |
| 29299 | 1.014915              | 2.393043                                                       |
| 29301 | 1.333470              | 2.393048                                                       |
| 29303 | 1.000034              | 2.393054                                                       |
| 29305 | 1.200205              | 2.393059                                                       |
| 29307 | 1.333470              | 2.393064                                                       |
| 29309 | 1.179160              | 2.393069                                                       |
| 29311 | 1.000034              | 2.393074                                                       |
| 29313 | 1.444888              | 2.393079                                                       |
| 29315 | 1.444175              | 2.393084                                                       |
| 29317 | 1.053314              | 2.393089                                                       |

| $n$   | $\frac{\sigma(n)}{n}$ | $\frac{e^\gamma}{2} \log \log n + \frac{0.73\dots}{\log \log n}$ |
|-------|-----------------------|------------------------------------------------------------------|
| 29319 | 1.383403              | 2.393094                                                         |
| 29321 | 1.012926              | 2.393099                                                         |
| 29323 | 1.178597              | 2.393104                                                         |
| 29325 | 1.826701              | 2.393109                                                         |
| 29327 | 1.000034              | 2.393114                                                         |
| 29329 | 1.011968              | 2.393119                                                         |
| 29331 | 1.444888              | 2.393124                                                         |
| 29333 | 1.000034              | 2.393129                                                         |
| 29335 | 1.200205              | 2.393134                                                         |
| 29337 | 1.675427              | 2.393139                                                         |
| 29339 | 1.000034              | 2.393144                                                         |
| 29341 | 1.124161              | 2.393149                                                         |
| 29343 | 1.333470              | 2.393154                                                         |
| 29345 | 1.200204              | 2.393159                                                         |
| 29347 | 1.000034              | 2.393164                                                         |
| 29349 | 1.482844              | 2.393169                                                         |
| 29351 | 1.165207              | 2.393174                                                         |
| 29353 | 1.011822              | 2.393179                                                         |
| 29355 | 1.700562              | 2.393184                                                         |
| 29357 | 1.033348              | 2.393189                                                         |
| 29359 | 1.162437              | 2.393194                                                         |
| 29361 | 1.333470              | 2.393199                                                         |
| 29363 | 1.000034              | 2.393204                                                         |
| 29365 | 1.373063              | 2.393208                                                         |
| 29367 | 1.561753              | 2.393213                                                         |
| 29369 | 1.024754              | 2.393218                                                         |
| 29371 | 1.044295              | 2.393223                                                         |
| 29373 | 1.333470              | 2.393228                                                         |
| 29375 | 1.276187              | 2.393233                                                         |
| 29377 | 1.035504              | 2.393238                                                         |
| 29379 | 1.524899              | 2.393243                                                         |
| 29381 | 1.091318              | 2.393248                                                         |
| 29383 | 1.000034              | 2.393253                                                         |
| 29385 | 1.735988              | 2.393258                                                         |
| 29387 | 1.000034              | 2.393263                                                         |
| 29389 | 1.000034              | 2.393268                                                         |
| 29391 | 1.360416              | 2.393273                                                         |
| 29393 | 1.371755              | 2.393278                                                         |
| 29395 | 1.200204              | 2.393283                                                         |
| 29397 | 1.371569              | 2.393288                                                         |
| 29399 | 1.000034              | 2.393293                                                         |
| 29401 | 1.000034              | 2.393298                                                         |
| 29403 | 1.646499              | 2.393303                                                         |
| 29405 | 1.200204              | 2.393308                                                         |

| $n$   | $\frac{\sigma(n)}{n}$ | $\frac{e^\gamma}{2} \log \log n + \frac{0.73\dots}{\log \log n}$ |
|-------|-----------------------|------------------------------------------------------------------|
| 29407 | 1.143129              | 2.393313                                                         |
| 29409 | 1.333469              | 2.393318                                                         |
| 29411 | 1.000034              | 2.393323                                                         |
| 29413 | 1.017237              | 2.393328                                                         |
| 29415 | 1.674248              | 2.393333                                                         |
| 29417 | 1.044294              | 2.393338                                                         |
| 29419 | 1.126891              | 2.393343                                                         |
| 29421 | 1.654329              | 2.393348                                                         |
| 29423 | 1.000034              | 2.393353                                                         |
| 29425 | 1.365370              | 2.393358                                                         |
| 29427 | 1.414211              | 2.393363                                                         |
| 29429 | 1.000034              | 2.393368                                                         |
| 29431 | 1.053311              | 2.393373                                                         |
| 29433 | 1.333469              | 2.393378                                                         |
| 29435 | 1.420350              | 2.393383                                                         |
| 29437 | 1.000034              | 2.393388                                                         |
| 29439 | 1.444886              | 2.393393                                                         |
| 29441 | 1.018987              | 2.393398                                                         |
| 29443 | 1.000034              | 2.393403                                                         |
| 29445 | 1.734488              | 2.393408                                                         |
| 29447 | 1.091317              | 2.393413                                                         |
| 29449 | 1.165201              | 2.393418                                                         |
| 29451 | 1.333469              | 2.393423                                                         |
| 29453 | 1.000034              | 2.393428                                                         |
| 29455 | 1.236870              | 2.393433                                                         |
| 29457 | 1.482839              | 2.393438                                                         |
| 29459 | 1.014291              | 2.393443                                                         |
| 29461 | 1.059435              | 2.393448                                                         |
| 29463 | 1.616129              | 2.393453                                                         |
| 29465 | 1.231563              | 2.393458                                                         |
| 29467 | 1.015373              | 2.393463                                                         |
| 29469 | 1.563677              | 2.393468                                                         |
| 29471 | 1.077398              | 2.393473                                                         |
| 29473 | 1.000034              | 2.393478                                                         |
| 29475 | 1.804784              | 2.393483                                                         |
| 29477 | 1.143129              | 2.393488                                                         |
| 29479 | 1.025815              | 2.393493                                                         |
| 29481 | 1.380686              | 2.393498                                                         |
| 29483 | 1.000034              | 2.393503                                                         |
| 29485 | 1.200203              | 2.393507                                                         |
| 29487 | 1.333469              | 2.393512                                                         |
| 29489 | 1.028316              | 2.393517                                                         |
| 29491 | 1.250008              | 2.393522                                                         |
| 29493 | 1.507476              | 2.393527                                                         |

| $n$   | $\frac{\sigma(n)}{n}$ | $\frac{e^\gamma}{2} \log \log n + \frac{0.73\dots}{\log \log n}$ |
|-------|-----------------------|------------------------------------------------------------------|
| 29495 | 1.274250              | 2.393532                                                         |
| 29497 | 1.077398              | 2.393537                                                         |
| 29499 | 1.333469              | 2.393542                                                         |
| 29501 | 1.000034              | 2.393547                                                         |
| 29503 | 1.011694              | 2.393552                                                         |
| 29505 | 1.835079              | 2.393557                                                         |
| 29507 | 1.053309              | 2.393562                                                         |
| 29509 | 1.044292              | 2.393567                                                         |
| 29511 | 1.482837              | 2.393572                                                         |
| 29513 | 1.091316              | 2.393577                                                         |
| 29515 | 1.200203              | 2.393582                                                         |
| 29517 | 1.333469              | 2.393587                                                         |
| 29519 | 1.143128              | 2.393592                                                         |
| 29521 | 1.020697              | 2.393597                                                         |
| 29523 | 1.437794              | 2.393602                                                         |
| 29525 | 1.241050              | 2.393607                                                         |
| 29527 | 1.000034              | 2.393612                                                         |
| 29529 | 1.537336              | 2.393617                                                         |
| 29531 | 1.000034              | 2.393622                                                         |
| 29533 | 1.143128              | 2.393627                                                         |
| 29535 | 1.755206              | 2.393632                                                         |
| 29537 | 1.000034              | 2.393637                                                         |
| 29539 | 1.012898              | 2.393642                                                         |
| 29541 | 1.370299              | 2.393647                                                         |
| 29543 | 1.033341              | 2.393652                                                         |
| 29545 | 1.267219              | 2.393656                                                         |
| 29547 | 1.705351              | 2.393661                                                         |
| 29549 | 1.077397              | 2.393666                                                         |
| 29551 | 1.035498              | 2.393671                                                         |
| 29553 | 1.333469              | 2.393676                                                         |
| 29555 | 1.257046              | 2.393681                                                         |
| 29557 | 1.091315              | 2.393686                                                         |
| 29559 | 1.364052              | 2.393691                                                         |
| 29561 | 1.182098              | 2.393696                                                         |
| 29563 | 1.110577              | 2.393701                                                         |
| 29565 | 1.817149              | 2.393706                                                         |
| 29567 | 1.000034              | 2.393711                                                         |
| 29569 | 1.000034              | 2.393716                                                         |
| 29571 | 1.333469              | 2.393721                                                         |
| 29573 | 1.000034              | 2.393726                                                         |
| 29575 | 1.534539              | 2.393731                                                         |
| 29577 | 1.333469              | 2.393736                                                         |
| 29579 | 1.091315              | 2.393741                                                         |
| 29581 | 1.000034              | 2.393746                                                         |

| $n$   | $\frac{\sigma(n)}{n}$ | $\frac{e^\gamma}{2} \log \log n + \frac{0.73...}{\log \log n}$ |
|-------|-----------------------|----------------------------------------------------------------|
| 29583 | 1.529257              | 2.393751                                                       |
| 29585 | 1.232246              | 2.393756                                                       |
| 29587 | 1.000034              | 2.393761                                                       |
| 29589 | 1.524891              | 2.393766                                                       |
| 29591 | 1.012200              | 2.393771                                                       |
| 29593 | 1.013348              | 2.393775                                                       |
| 29595 | 1.600811              | 2.393780                                                       |
| 29597 | 1.059432              | 2.393785                                                       |
| 29599 | 1.000034              | 2.393790                                                       |
| 29601 | 1.770751              | 2.393795                                                       |
| 29603 | 1.143127              | 2.393800                                                       |
| 29605 | 1.245195              | 2.393805                                                       |
| 29607 | 1.361840              | 2.393810                                                       |
| 29609 | 1.035496              | 2.393815                                                       |
| 29611 | 1.000034              | 2.393820                                                       |
| 29613 | 1.333468              | 2.393825                                                       |
| 29615 | 1.200203              | 2.393830                                                       |
| 29617 | 1.143127              | 2.393835                                                       |
| 29619 | 1.482832              | 2.393840                                                       |
| 29621 | 1.053307              | 2.393845                                                       |
| 29623 | 1.091314              | 2.393850                                                       |
| 29625 | 1.685063              | 2.393855                                                       |
| 29627 | 1.122760              | 2.393860                                                       |
| 29629 | 1.000034              | 2.393865                                                       |
| 29631 | 1.632884              | 2.393869                                                       |
| 29633 | 1.000034              | 2.393874                                                       |
| 29635 | 1.200202              | 2.393879                                                       |
| 29637 | 1.500152              | 2.393884                                                       |
| 29639 | 1.012990              | 2.393889                                                       |
| 29641 | 1.000034              | 2.393894                                                       |
| 29643 | 1.371521              | 2.393899                                                       |
| 29645 | 1.534357              | 2.393904                                                       |
| 29647 | 1.044288              | 2.393909                                                       |
| 29649 | 1.333468              | 2.393914                                                       |
| 29651 | 1.011770              | 2.393919                                                       |
| 29653 | 1.077395              | 2.393924                                                       |
| 29655 | 1.735964              | 2.393929                                                       |
| 29657 | 1.022895              | 2.393934                                                       |
| 29659 | 1.208402              | 2.393939                                                       |
| 29661 | 1.333468              | 2.393944                                                       |
| 29663 | 1.000034              | 2.393949                                                       |
| 29665 | 1.274229              | 2.393954                                                       |
| 29667 | 1.553241              | 2.393958                                                       |
| 29669 | 1.000034              | 2.393963                                                       |

| $n$   | $\frac{\sigma(n)}{n}$ | $\frac{e^\gamma}{2} \log \log n + \frac{0.73...}{\log \log n}$ |
|-------|-----------------------|----------------------------------------------------------------|
| 29671 | 1.000034              | 2.393968                                                       |
| 29673 | 1.703906              | 2.393973                                                       |
| 29675 | 1.241045              | 2.393978                                                       |
| 29677 | 1.018971              | 2.393983                                                       |
| 29679 | 1.437784              | 2.393988                                                       |
| 29681 | 1.017216              | 2.393993                                                       |
| 29683 | 1.000034              | 2.393998                                                       |
| 29685 | 1.600808              | 2.394003                                                       |
| 29687 | 1.143127              | 2.394008                                                       |
| 29689 | 1.091313              | 2.394013                                                       |
| 29691 | 1.444882              | 2.394018                                                       |
| 29693 | 1.044287              | 2.394023                                                       |
| 29695 | 1.200202              | 2.394028                                                       |
| 29697 | 1.406203              | 2.394032                                                       |
| 29699 | 1.059430              | 2.394037                                                       |
| 29701 | 1.143126              | 2.394042                                                       |
| 29703 | 1.333468              | 2.394047                                                       |
| 29705 | 1.295135              | 2.394052                                                       |
| 29707 | 1.018480              | 2.394057                                                       |
| 29709 | 1.444882              | 2.394062                                                       |
| 29711 | 1.135741              | 2.394067                                                       |
| 29713 | 1.024737              | 2.394072                                                       |
| 29715 | 1.835033              | 2.394077                                                       |
| 29717 | 1.000034              | 2.394082                                                       |
| 29719 | 1.012685              | 2.394087                                                       |
| 29721 | 1.333468              | 2.394092                                                       |
| 29723 | 1.000034              | 2.394097                                                       |
| 29725 | 1.314045              | 2.394102                                                       |
| 29727 | 1.497898              | 2.394106                                                       |
| 29729 | 1.188335              | 2.394111                                                       |
| 29731 | 1.077394              | 2.394116                                                       |
| 29733 | 1.569166              | 2.394121                                                       |
| 29735 | 1.267194              | 2.394126                                                       |
| 29737 | 1.012073              | 2.394131                                                       |
| 29739 | 1.394532              | 2.394136                                                       |
| 29741 | 1.000034              | 2.394141                                                       |
| 29743 | 1.165182              | 2.394146                                                       |
| 29745 | 1.735956              | 2.394151                                                       |
| 29747 | 1.011732              | 2.394156                                                       |
| 29749 | 1.016505              | 2.394161                                                       |
| 29751 | 1.368156              | 2.394166                                                       |
| 29753 | 1.000034              | 2.394171                                                       |
| 29755 | 1.311511              | 2.394175                                                       |
| 29757 | 1.656081              | 2.394180                                                       |



| $n$   | $\frac{\sigma(n)}{n}$ | $\frac{e^\gamma}{2} \log \log n + \frac{0.73...}{\log \log n}$ |
|-------|-----------------------|----------------------------------------------------------------|
| 29759 | 1.000034              | 2.394185                                                       |
| 29761 | 1.000034              | 2.394190                                                       |
| 29763 | 1.444881              | 2.394195                                                       |
| 29765 | 1.200202              | 2.394200                                                       |
| 29767 | 1.072597              | 2.394205                                                       |
| 29769 | 1.333468              | 2.394210                                                       |
| 29771 | 1.143126              | 2.394215                                                       |
| 29773 | 1.053303              | 2.394220                                                       |
| 29775 | 1.657498              | 2.394225                                                       |
| 29777 | 1.091312              | 2.394230                                                       |
| 29779 | 1.013600              | 2.394234                                                       |
| 29781 | 1.482825              | 2.394239                                                       |
| 29783 | 1.128160              | 2.394244                                                       |
| 29785 | 1.469733              | 2.394249                                                       |
| 29787 | 1.333468              | 2.394254                                                       |
| 29789 | 1.000034              | 2.394259                                                       |
| 29791 | 1.033332              | 2.394264                                                       |
| 29793 | 1.333468              | 2.394269                                                       |
| 29795 | 1.232422              | 2.394274                                                       |
| 29797 | 1.014867              | 2.394279                                                       |
| 29799 | 1.842746              | 2.394284                                                       |
| 29801 | 1.059428              | 2.394289                                                       |
| 29803 | 1.000034              | 2.394293                                                       |
| 29805 | 1.600805              | 2.394298                                                       |
| 29807 | 1.025799              | 2.394303                                                       |
| 29809 | 1.077393              | 2.394308                                                       |
| 29811 | 1.406192              | 2.394313                                                       |
| 29813 | 1.143125              | 2.394318                                                       |
| 29815 | 1.231595              | 2.394323                                                       |
| 29817 | 1.444880              | 2.394328                                                       |
| 29819 | 1.000034              | 2.394333                                                       |
| 29821 | 1.091311              | 2.394338                                                       |
| 29823 | 1.333467              | 2.394343                                                       |
| 29825 | 1.241039              | 2.394348                                                       |
| 29827 | 1.143125              | 2.394352                                                       |
| 29829 | 1.363505              | 2.394357                                                       |
| 29831 | 1.044283              | 2.394362                                                       |
| 29833 | 1.000034              | 2.394367                                                       |
| 29835 | 2.027149              | 2.394372                                                       |
| 29837 | 1.000034              | 2.394377                                                       |
| 29839 | 1.020678              | 2.394382                                                       |
| 29841 | 1.608525              | 2.394387                                                       |
| 29843 | 1.091311              | 2.394392                                                       |
| 29845 | 1.235182              | 2.394397                                                       |

| $n$   | $\frac{\sigma(n)}{n}$ | $\frac{e^\gamma}{2} \log \log n + \frac{0.73\dots}{\log \log n}$ |
|-------|-----------------------|------------------------------------------------------------------|
| 29847 | 1.333467              | 2.394402                                                         |
| 29849 | 1.053302              | 2.394406                                                         |
| 29851 | 1.000033              | 2.394411                                                         |
| 29853 | 1.504974              | 2.394416                                                         |
| 29855 | 1.373036              | 2.394421                                                         |
| 29857 | 1.016177              | 2.394426                                                         |
| 29859 | 1.374460              | 2.394431                                                         |
| 29861 | 1.077392              | 2.394436                                                         |
| 29863 | 1.000033              | 2.394441                                                         |
| 29865 | 1.755098              | 2.394446                                                         |
| 29867 | 1.000033              | 2.394451                                                         |
| 29869 | 1.214905              | 2.394455                                                         |
| 29871 | 1.444880              | 2.394460                                                         |
| 29873 | 1.000033              | 2.394465                                                         |
| 29875 | 1.253222              | 2.394470                                                         |
| 29877 | 1.394518              | 2.394475                                                         |
| 29879 | 1.000033              | 2.394480                                                         |
| 29881 | 1.000033              | 2.394485                                                         |
| 29883 | 1.524880              | 2.394490                                                         |
| 29885 | 1.236741              | 2.394495                                                         |
| 29887 | 1.246027              | 2.394500                                                         |
| 29889 | 1.535883              | 2.394504                                                         |
| 29891 | 1.016493              | 2.394509                                                         |
| 29893 | 1.011608              | 2.394514                                                         |
| 29895 | 1.600803              | 2.394519                                                         |
| 29897 | 1.143125              | 2.394524                                                         |
| 29899 | 1.035486              | 2.394529                                                         |
| 29901 | 1.333467              | 2.394534                                                         |
| 29903 | 1.059425              | 2.394539                                                         |
| 29905 | 1.200201              | 2.394544                                                         |
| 29907 | 1.444879              | 2.394549                                                         |
| 29909 | 1.091310              | 2.394553                                                         |
| 29911 | 1.143125              | 2.394558                                                         |
| 29913 | 1.468258              | 2.394563                                                         |
| 29915 | 1.245128              | 2.394568                                                         |
| 29917 | 1.000033              | 2.394573                                                         |
| 29919 | 1.333467              | 2.394578                                                         |
| 29921 | 1.000033              | 2.394583                                                         |
| 29923 | 1.044280              | 2.394588                                                         |
| 29925 | 2.154720              | 2.394593                                                         |
| 29927 | 1.000033              | 2.394598                                                         |
| 29929 | 1.005814              | 2.394602                                                         |
| 29931 | 1.456149              | 2.394607                                                         |
| 29933 | 1.028297              | 2.394612                                                         |

| $n$   | $\frac{\sigma(n)}{n}$ | $\frac{e^\gamma}{2} \log \log n + \frac{0.73...}{\log \log n}$ |
|-------|-----------------------|----------------------------------------------------------------|
| 29935 | 1.200200              | 2.394617                                                       |
| 29937 | 1.414170              | 2.394622                                                       |
| 29939 | 1.279401              | 2.394627                                                       |
| 29941 | 1.015330              | 2.394632                                                       |
| 29943 | 1.482817              | 2.394637                                                       |
| 29945 | 1.233461              | 2.394642                                                       |
| 29947 | 1.000033              | 2.394646                                                       |
| 29949 | 1.362316              | 2.394651                                                       |
| 29951 | 1.018463              | 2.394656                                                       |
| 29953 | 1.249958              | 2.394661                                                       |
| 29955 | 1.600801              | 2.394666                                                       |
| 29957 | 1.035484              | 2.394671                                                       |
| 29959 | 1.000033              | 2.394676                                                       |
| 29961 | 1.444878              | 2.394681                                                       |
| 29963 | 1.068117              | 2.394686                                                       |
| 29965 | 1.295111              | 2.394690                                                       |
| 29967 | 1.524877              | 2.394695                                                       |
| 29969 | 1.044279              | 2.394700                                                       |
| 29971 | 1.109873              | 2.394705                                                       |
| 29973 | 1.360157              | 2.394710                                                       |
| 29975 | 1.365138              | 2.394715                                                       |
| 29977 | 1.033326              | 2.394720                                                       |
| 29979 | 1.444878              | 2.394725                                                       |
| 29981 | 1.143124              | 2.394729                                                       |
| 29983 | 1.000033              | 2.394734                                                       |
| 29985 | 1.600800              | 2.394739                                                       |
| 29987 | 1.011638              | 2.394744                                                       |
| 29989 | 1.000033              | 2.394749                                                       |
| 29991 | 1.437765              | 2.394754                                                       |
| 29993 | 1.014237              | 2.394759                                                       |
| 29995 | 1.373029              | 2.394764                                                       |
| 29997 | 1.632163              | 2.394769                                                       |
| 29999 | 1.012034              | 2.394773                                                       |
| 30001 | 1.053298              | 2.394778                                                       |
| 30003 | 1.361464              | 2.394783                                                       |
| 30005 | 1.274188              | 2.394788                                                       |
| 30007 | 1.028293              | 2.394793                                                       |
| 30009 | 1.524876              | 2.394798                                                       |
| 30011 | 1.000033              | 2.394803                                                       |
| 30013 | 1.000033              | 2.394808                                                       |
| 30015 | 1.871064              | 2.394812                                                       |
| 30017 | 1.077389              | 2.394817                                                       |
| 30019 | 1.091309              | 2.394822                                                       |
| 30021 | 1.333467              | 2.394827                                                       |

| $n$   | $\frac{\sigma(n)}{n}$ | $\frac{e^\gamma}{2} \log \log n + \frac{0.73...}{\log \log n}$ |
|-------|-----------------------|----------------------------------------------------------------|
| 30023 | 1.143124              | 2.394832                                                       |
| 30025 | 1.241032              | 2.394837                                                       |
| 30027 | 1.333467              | 2.394842                                                       |
| 30029 | 1.000033              | 2.394847                                                       |
| 30031 | 1.018947              | 2.394851                                                       |
| 30033 | 1.495954              | 2.394856                                                       |
| 30035 | 1.200200              | 2.394861                                                       |
| 30037 | 1.165163              | 2.394866                                                       |
| 30039 | 1.534006              | 2.394871                                                       |
| 30041 | 1.091309              | 2.394876                                                       |
| 30043 | 1.077389              | 2.394881                                                       |
| 30045 | 1.600799              | 2.394886                                                       |
| 30047 | 1.000033              | 2.394890                                                       |
| 30049 | 1.011681              | 2.394895                                                       |
| 30051 | 1.739443              | 2.394900                                                       |
| 30053 | 1.025788              | 2.394905                                                       |
| 30055 | 1.200200              | 2.394910                                                       |
| 30057 | 1.370197              | 2.394915                                                       |
| 30059 | 1.000033              | 2.394920                                                       |
| 30061 | 1.044277              | 2.394925                                                       |
| 30063 | 1.456142              | 2.394929                                                       |
| 30065 | 1.373025              | 2.394934                                                       |
| 30067 | 1.012938              | 2.394939                                                       |
| 30069 | 1.561608              | 2.394944                                                       |
| 30071 | 1.000033              | 2.394949                                                       |
| 30073 | 1.113291              | 2.394954                                                       |
| 30075 | 1.657456              | 2.394959                                                       |
| 30077 | 1.053297              | 2.394963                                                       |
| 30079 | 1.143123              | 2.394968                                                       |
| 30081 | 1.374422              | 2.394973                                                       |
| 30083 | 1.017186              | 2.394978                                                       |
| 30085 | 1.311484              | 2.394983                                                       |
| 30087 | 1.444877              | 2.394988                                                       |
| 30089 | 1.000033              | 2.394993                                                       |
| 30091 | 1.000033              | 2.394998                                                       |
| 30093 | 1.524873              | 2.395002                                                       |
| 30095 | 1.295099              | 2.395007                                                       |
| 30097 | 1.000033              | 2.395012                                                       |
| 30099 | 1.360843              | 2.395017                                                       |
| 30101 | 1.033321              | 2.395022                                                       |
| 30103 | 1.000033              | 2.395027                                                       |
| 30105 | 1.785750              | 2.395032                                                       |
| 30107 | 1.377487              | 2.395036                                                       |
| 30109 | 1.000033              | 2.395041                                                       |

| $n$   | $\frac{\sigma(n)}{n}$ | $\frac{e^\gamma}{2} \log \log n + \frac{0.73\dots}{\log \log n}$ |
|-------|-----------------------|------------------------------------------------------------------|
| 30111 | 1.333466              | 2.395046                                                         |
| 30113 | 1.000033              | 2.395051                                                         |
| 30115 | 1.267143              | 2.395056                                                         |
| 30117 | 1.333466              | 2.395061                                                         |
| 30119 | 1.000033              | 2.395066                                                         |
| 30121 | 1.234488              | 2.395070                                                         |
| 30123 | 1.444876              | 2.395075                                                         |
| 30125 | 1.253178              | 2.395080                                                         |
| 30127 | 1.022870              | 2.395085                                                         |
| 30129 | 1.483222              | 2.395090                                                         |
| 30131 | 1.035478              | 2.395095                                                         |
| 30133 | 1.000033              | 2.395100                                                         |
| 30135 | 1.906620              | 2.395104                                                         |
| 30137 | 1.000033              | 2.395109                                                         |
| 30139 | 1.000033              | 2.395114                                                         |
| 30141 | 1.537175              | 2.395119                                                         |
| 30143 | 1.024716              | 2.395124                                                         |
| 30145 | 1.200199              | 2.395129                                                         |
| 30147 | 1.437755              | 2.395134                                                         |
| 30149 | 1.178149              | 2.395138                                                         |
| 30151 | 1.091307              | 2.395143                                                         |
| 30153 | 1.467184              | 2.395148                                                         |
| 30155 | 1.239993              | 2.395153                                                         |
| 30157 | 1.020659              | 2.395158                                                         |
| 30159 | 1.482808              | 2.395163                                                         |
| 30161 | 1.000033              | 2.395168                                                         |
| 30163 | 1.188211              | 2.395172                                                         |
| 30165 | 1.600796              | 2.395177                                                         |
| 30167 | 1.013558              | 2.395182                                                         |
| 30169 | 1.000033              | 2.395187                                                         |
| 30171 | 1.360247              | 2.395192                                                         |
| 30173 | 1.180393              | 2.395197                                                         |
| 30175 | 1.331433              | 2.395202                                                         |
| 30177 | 1.654240              | 2.395206                                                         |
| 30179 | 1.013155              | 2.395211                                                         |
| 30181 | 1.000033              | 2.395216                                                         |
| 30183 | 1.333466              | 2.395221                                                         |
| 30185 | 1.200199              | 2.395226                                                         |
| 30187 | 1.000033              | 2.395231                                                         |
| 30189 | 1.383285              | 2.395235                                                         |
| 30191 | 1.208307              | 2.395240                                                         |
| 30193 | 1.012818              | 2.395245                                                         |
| 30195 | 1.921908              | 2.395250                                                         |
| 30197 | 1.000033              | 2.395255                                                         |

| $n$   | $\frac{\sigma(n)}{n}$ | $\frac{e^\gamma}{2} \log \log n + \frac{0.73\dots}{\log \log n}$ |
|-------|-----------------------|------------------------------------------------------------------|
| 30199 | 1.134872              | 2.395260                                                         |
| 30201 | 1.333466              | 2.395265                                                         |
| 30203 | 1.000033              | 2.395269                                                         |
| 30205 | 1.373018              | 2.395274                                                         |
| 30207 | 1.333466              | 2.395279                                                         |
| 30209 | 1.059419              | 2.395284                                                         |
| 30211 | 1.000033              | 2.395289                                                         |
| 30213 | 1.497832              | 2.395294                                                         |
| 30215 | 1.200199              | 2.395298                                                         |
| 30217 | 1.134196              | 2.395303                                                         |
| 30219 | 1.524868              | 2.395308                                                         |
| 30221 | 1.022865              | 2.395313                                                         |
| 30223 | 1.000033              | 2.395318                                                         |
| 30225 | 1.837949              | 2.395323                                                         |
| 30227 | 1.011546              | 2.395327                                                         |
| 30229 | 1.106223              | 2.395332                                                         |
| 30231 | 1.444874              | 2.395337                                                         |
| 30233 | 1.165151              | 2.395342                                                         |
| 30235 | 1.200198              | 2.395347                                                         |
| 30237 | 1.333466              | 2.395352                                                         |
| 30239 | 1.091306              | 2.395357                                                         |
| 30241 | 1.000033              | 2.395361                                                         |
| 30243 | 1.414145              | 2.395366                                                         |
| 30245 | 1.256935              | 2.395371                                                         |
| 30247 | 1.190201              | 2.395376                                                         |
| 30249 | 1.444874              | 2.395381                                                         |
| 30251 | 1.088890              | 2.395386                                                         |
| 30253 | 1.000033              | 2.395390                                                         |
| 30255 | 1.600793              | 2.395395                                                         |
| 30257 | 1.015302              | 2.395400                                                         |
| 30259 | 1.000033              | 2.395405                                                         |
| 30261 | 1.675027              | 2.395410                                                         |
| 30263 | 1.020652              | 2.395415                                                         |
| 30265 | 1.200198              | 2.395419                                                         |
| 30267 | 1.585886              | 2.395424                                                         |
| 30269 | 1.000033              | 2.395429                                                         |
| 30271 | 1.000033              | 2.395434                                                         |
| 30273 | 1.333465              | 2.395439                                                         |
| 30275 | 1.425334              | 2.395444                                                         |
| 30277 | 1.148595              | 2.395448                                                         |
| 30279 | 1.333465              | 2.395453                                                         |
| 30281 | 1.012912              | 2.395458                                                         |
| 30283 | 1.091305              | 2.395463                                                         |
| 30285 | 1.735909              | 2.395468                                                         |

| $n$   | $\frac{\sigma(n)}{n}$ | $\frac{e^\gamma}{2} \log \log n + \frac{0.73...}{\log \log n}$ |
|-------|-----------------------|----------------------------------------------------------------|
| 30287 | 1.033315              | 2.395473                                                       |
| 30289 | 1.143121              | 2.395477                                                       |
| 30291 | 1.394474              | 2.395482                                                       |
| 30293 | 1.000033              | 2.395487                                                       |
| 30295 | 1.231094              | 2.395492                                                       |
| 30297 | 1.333465              | 2.395497                                                       |
| 30299 | 1.025776              | 2.395502                                                       |
| 30301 | 1.011584              | 2.395506                                                       |
| 30303 | 1.825826              | 2.395511                                                       |
| 30305 | 1.425507              | 2.395516                                                       |
| 30307 | 1.000033              | 2.395521                                                       |
| 30309 | 1.333465              | 2.395526                                                       |
| 30311 | 1.059417              | 2.395530                                                       |
| 30313 | 1.000033              | 2.395535                                                       |
| 30315 | 1.672044              | 2.395540                                                       |
| 30317 | 1.177953              | 2.395545                                                       |
| 30319 | 1.000033              | 2.395550                                                       |
| 30321 | 1.482801              | 2.395555                                                       |
| 30323 | 1.000033              | 2.395559                                                       |
| 30325 | 1.241022              | 2.395564                                                       |
| 30327 | 1.456128              | 2.395569                                                       |
| 30329 | 1.077385              | 2.395574                                                       |
| 30331 | 1.165145              | 2.395579                                                       |
| 30333 | 1.333465              | 2.395584                                                       |
| 30335 | 1.200198              | 2.395588                                                       |
| 30337 | 1.044269              | 2.395593                                                       |
| 30339 | 1.444873              | 2.395598                                                       |
| 30341 | 1.000033              | 2.395603                                                       |
| 30343 | 1.053291              | 2.395608                                                       |
| 30345 | 1.942462              | 2.395612                                                       |
| 30347 | 1.000033              | 2.395617                                                       |
| 30349 | 1.138753              | 2.395622                                                       |
| 30351 | 1.362196              | 2.395627                                                       |
| 30353 | 1.012091              | 2.395632                                                       |
| 30355 | 1.295075              | 2.395637                                                       |
| 30357 | 1.444873              | 2.395641                                                       |
| 30359 | 1.143121              | 2.395646                                                       |
| 30361 | 1.013537              | 2.395651                                                       |
| 30363 | 1.383263              | 2.395656                                                       |
| 30365 | 1.200198              | 2.395661                                                       |
| 30367 | 1.000033              | 2.395665                                                       |
| 30369 | 1.365603              | 2.395670                                                       |
| 30371 | 1.103553              | 2.395675                                                       |
| 30373 | 1.143121              | 2.395680                                                       |

| $n$   | $\frac{\sigma(n)}{n}$ | $\frac{e^\gamma}{2} \log \log n + \frac{0.73...}{\log \log n}$ |
|-------|-----------------------|----------------------------------------------------------------|
| 30375 | 1.869432              | 2.395685                                                       |
| 30377 | 1.028278              | 2.395690                                                       |
| 30379 | 1.059416              | 2.395694                                                       |
| 30381 | 1.548336              | 2.395699                                                       |
| 30383 | 1.044268              | 2.395704                                                       |
| 30385 | 1.232187              | 2.395709                                                       |
| 30387 | 1.524863              | 2.395714                                                       |
| 30389 | 1.000033              | 2.395718                                                       |
| 30391 | 1.000033              | 2.395723                                                       |
| 30393 | 1.580890              | 2.395728                                                       |
| 30395 | 1.200197              | 2.395733                                                       |
| 30397 | 1.012600              | 2.395738                                                       |
| 30399 | 1.333465              | 2.395742                                                       |
| 30401 | 1.181014              | 2.395747                                                       |
| 30403 | 1.000033              | 2.395752                                                       |
| 30405 | 1.600789              | 2.395757                                                       |
| 30407 | 1.077383              | 2.395762                                                       |
| 30409 | 1.022855              | 2.395767                                                       |
| 30411 | 1.504719              | 2.395771                                                       |
| 30413 | 1.059415              | 2.395776                                                       |
| 30415 | 1.515042              | 2.395781                                                       |
| 30417 | 1.333465              | 2.395786                                                       |
| 30419 | 1.053289              | 2.395791                                                       |
| 30421 | 1.035469              | 2.395795                                                       |
| 30423 | 1.333465              | 2.395800                                                       |
| 30425 | 1.241019              | 2.395805                                                       |
| 30427 | 1.000033              | 2.395810                                                       |
| 30429 | 1.798285              | 2.395815                                                       |
| 30431 | 1.000033              | 2.395819                                                       |
| 30433 | 1.077383              | 2.395824                                                       |
| 30435 | 1.600789              | 2.395829                                                       |
| 30437 | 1.091303              | 2.395834                                                       |
| 30439 | 1.018430              | 2.395839                                                       |
| 30441 | 1.361322              | 2.395843                                                       |
| 30443 | 1.143120              | 2.395848                                                       |
| 30445 | 1.200197              | 2.395853                                                       |
| 30447 | 1.537097              | 2.395858                                                       |
| 30449 | 1.000033              | 2.395863                                                       |
| 30451 | 1.028275              | 2.395867                                                       |
| 30453 | 1.333465              | 2.395872                                                       |
| 30455 | 1.200197              | 2.395877                                                       |
| 30457 | 1.208261              | 2.395882                                                       |
| 30459 | 1.588496              | 2.395887                                                       |
| 30461 | 1.014806              | 2.395891                                                       |



| $n$   | $\frac{\sigma(n)}{n}$ | $\frac{e^\gamma}{2} \log \log n + \frac{0.73...}{\log \log n}$ |
|-------|-----------------------|----------------------------------------------------------------|
| 30463 | 1.025769              | 2.395896                                                       |
| 30465 | 1.735894              | 2.395901                                                       |
| 30467 | 1.000033              | 2.395906                                                       |
| 30469 | 1.000033              | 2.395911                                                       |
| 30471 | 1.524860              | 2.395915                                                       |
| 30473 | 1.033308              | 2.395920                                                       |
| 30475 | 1.318326              | 2.395925                                                       |
| 30477 | 1.333465              | 2.395930                                                       |
| 30479 | 1.035467              | 2.395935                                                       |
| 30481 | 1.162167              | 2.395939                                                       |
| 30483 | 1.482794              | 2.395944                                                       |
| 30485 | 1.498967              | 2.395949                                                       |
| 30487 | 1.024699              | 2.395954                                                       |
| 30489 | 1.333465              | 2.395959                                                       |
| 30491 | 1.000033              | 2.395963                                                       |
| 30493 | 1.000033              | 2.395968                                                       |
| 30495 | 1.699951              | 2.395973                                                       |
| 30497 | 1.000033              | 2.395978                                                       |
| 30499 | 1.143119              | 2.395983                                                       |
| 30501 | 1.444871              | 2.395987                                                       |
| 30503 | 1.133003              | 2.395992                                                       |
| 30505 | 1.200197              | 2.395997                                                       |
| 30507 | 1.333464              | 2.396002                                                       |
| 30509 | 1.000033              | 2.396007                                                       |
| 30511 | 1.077382              | 2.396011                                                       |
| 30513 | 1.524858              | 2.396016                                                       |
| 30515 | 1.274127              | 2.396021                                                       |
| 30517 | 1.000033              | 2.396026                                                       |
| 30519 | 1.444870              | 2.396030                                                       |
| 30521 | 1.044265              | 2.396035                                                       |
| 30523 | 1.011958              | 2.396040                                                       |
| 30525 | 1.852383              | 2.396045                                                       |
| 30527 | 1.179284              | 2.396050                                                       |
| 30529 | 1.000033              | 2.396054                                                       |
| 30531 | 1.333464              | 2.396059                                                       |
| 30533 | 1.053287              | 2.396064                                                       |
| 30535 | 1.244998              | 2.396069                                                       |
| 30537 | 1.664211              | 2.396074                                                       |
| 30539 | 1.000033              | 2.396078                                                       |
| 30541 | 1.143119              | 2.396083                                                       |
| 30543 | 1.333464              | 2.396088                                                       |
| 30545 | 1.237518              | 2.396093                                                       |
| 30547 | 1.091302              | 2.396098                                                       |
| 30549 | 1.414122              | 2.396102                                                       |

| $n$   | $\frac{\sigma(n)}{n}$ | $\frac{e^\gamma}{2} \log \log n + \frac{0.73\dots}{\log \log n}$ |
|-------|-----------------------|------------------------------------------------------------------|
| 30551 | 1.011816              | 2.396107                                                         |
| 30553 | 1.000033              | 2.396112                                                         |
| 30555 | 2.001375              | 2.396117                                                         |
| 30557 | 1.000033              | 2.396121                                                         |
| 30559 | 1.000033              | 2.396126                                                         |
| 30561 | 1.363306              | 2.396131                                                         |
| 30563 | 1.077381              | 2.396136                                                         |
| 30565 | 1.200196              | 2.396141                                                         |
| 30567 | 1.394445              | 2.396145                                                         |
| 30569 | 1.249894              | 2.396150                                                         |
| 30571 | 1.053286              | 2.396155                                                         |
| 30573 | 1.496745              | 2.396160                                                         |
| 30575 | 1.241014              | 2.396164                                                         |
| 30577 | 1.000033              | 2.396169                                                         |
| 30579 | 1.333464              | 2.396174                                                         |
| 30581 | 1.020634              | 2.396179                                                         |
| 30583 | 1.214793              | 2.396184                                                         |
| 30585 | 1.600785              | 2.396188                                                         |
| 30587 | 1.016118              | 2.396193                                                         |
| 30589 | 1.088823              | 2.396198                                                         |
| 30591 | 1.631853              | 2.396203                                                         |
| 30593 | 1.000033              | 2.396207                                                         |
| 30595 | 1.247263              | 2.396212                                                         |
| 30597 | 1.606432              | 2.396217                                                         |
| 30599 | 1.028269              | 2.396222                                                         |
| 30601 | 1.016437              | 2.396227                                                         |
| 30603 | 1.346665              | 2.396231                                                         |
| 30605 | 1.200196              | 2.396236                                                         |
| 30607 | 1.012056              | 2.396241                                                         |
| 30609 | 1.528962              | 2.396246                                                         |
| 30611 | 1.143118              | 2.396250                                                         |
| 30613 | 1.147748              | 2.396255                                                         |
| 30615 | 1.734052              | 2.396260                                                         |
| 30617 | 1.059411              | 2.396265                                                         |
| 30619 | 1.017146              | 2.396270                                                         |
| 30621 | 1.363770              | 2.396274                                                         |
| 30623 | 1.012572              | 2.396279                                                         |
| 30625 | 1.453616              | 2.396284                                                         |
| 30627 | 1.497502              | 2.396289                                                         |
| 30629 | 1.012766              | 2.396293                                                         |
| 30631 | 1.000033              | 2.396298                                                         |
| 30633 | 1.333464              | 2.396303                                                         |
| 30635 | 1.311441              | 2.396308                                                         |
| 30637 | 1.000033              | 2.396313                                                         |

| $n$   | $\frac{\sigma(n)}{n}$ | $\frac{e^\gamma}{2} \log \log n + \frac{0.73...}{\log \log n}$ |
|-------|-----------------------|----------------------------------------------------------------|
| 30639 | 1.524854              | 2.396317                                                       |
| 30641 | 1.077380              | 2.396322                                                       |
| 30643 | 1.000033              | 2.396327                                                       |
| 30645 | 1.785609              | 2.396332                                                       |
| 30647 | 1.053284              | 2.396336                                                       |
| 30649 | 1.000033              | 2.396341                                                       |
| 30651 | 1.414114              | 2.396346                                                       |
| 30653 | 1.190096              | 2.396351                                                       |
| 30655 | 1.200196              | 2.396355                                                       |
| 30657 | 1.456111              | 2.396360                                                       |
| 30659 | 1.102189              | 2.396365                                                       |
| 30661 | 1.000033              | 2.396370                                                       |
| 30663 | 1.444868              | 2.396375                                                       |
| 30665 | 1.200196              | 2.396379                                                       |
| 30667 | 1.234421              | 2.396384                                                       |
| 30669 | 1.333464              | 2.396389                                                       |
| 30671 | 1.000033              | 2.396394                                                       |
| 30673 | 1.028266              | 2.396398                                                       |
| 30675 | 1.657376              | 2.396403                                                       |
| 30677 | 1.000033              | 2.396408                                                       |
| 30679 | 1.091300              | 2.396413                                                       |
| 30681 | 1.654183              | 2.396417                                                       |
| 30683 | 1.018414              | 2.396422                                                       |
| 30685 | 1.340981              | 2.396427                                                       |
| 30687 | 1.365529              | 2.396432                                                       |
| 30689 | 1.000033              | 2.396436                                                       |
| 30691 | 1.022841              | 2.396441                                                       |
| 30693 | 1.437722              | 2.396446                                                       |
| 30695 | 1.372992              | 2.396451                                                       |
| 30697 | 1.000033              | 2.396455                                                       |
| 30699 | 1.497769              | 2.396460                                                       |
| 30701 | 1.091300              | 2.396465                                                       |
| 30703 | 1.000033              | 2.396470                                                       |
| 30705 | 1.688324              | 2.396475                                                       |
| 30707 | 1.000033              | 2.396479                                                       |
| 30709 | 1.181673              | 2.396484                                                       |
| 30711 | 1.383218              | 2.396489                                                       |
| 30713 | 1.000033              | 2.396494                                                       |
| 30715 | 1.200195              | 2.396498                                                       |
| 30717 | 1.444868              | 2.396503                                                       |
| 30719 | 1.148475              | 2.396508                                                       |
| 30721 | 1.033300              | 2.396513                                                       |
| 30723 | 1.781076              | 2.396517                                                       |
| 30725 | 1.241009              | 2.396522                                                       |

| $n$   | $\frac{\sigma(n)}{n}$ | $\frac{e^\gamma}{2} \log \log n + \frac{0.73...}{\log \log n}$ |
|-------|-----------------------|----------------------------------------------------------------|
| 30727 | 1.000033              | 2.396527                                                       |
| 30729 | 1.333464              | 2.396532                                                       |
| 30731 | 1.015261              | 2.396536                                                       |
| 30733 | 1.016106              | 2.396541                                                       |
| 30735 | 1.735871              | 2.396546                                                       |
| 30737 | 1.143117              | 2.396551                                                       |
| 30739 | 1.018901              | 2.396555                                                       |
| 30741 | 1.333463              | 2.396560                                                       |
| 30743 | 1.016427              | 2.396565                                                       |
| 30745 | 1.442576              | 2.396570                                                       |
| 30747 | 1.374313              | 2.396574                                                       |
| 30749 | 1.013496              | 2.396579                                                       |
| 30751 | 1.198790              | 2.396584                                                       |
| 30753 | 1.592040              | 2.396589                                                       |
| 30755 | 1.200195              | 2.396593                                                       |
| 30757 | 1.000033              | 2.396598                                                       |
| 30759 | 1.333463              | 2.396603                                                       |
| 30761 | 1.053282              | 2.396608                                                       |
| 30763 | 1.000033              | 2.396612                                                       |
| 30765 | 1.834812              | 2.396617                                                       |
| 30767 | 1.091299              | 2.396622                                                       |
| 30769 | 1.035458              | 2.396627                                                       |
| 30771 | 1.561470              | 2.396631                                                       |
| 30773 | 1.000032              | 2.396636                                                       |
| 30775 | 1.241007              | 2.396641                                                       |
| 30777 | 1.333463              | 2.396646                                                       |
| 30779 | 1.143117              | 2.396650                                                       |
| 30781 | 1.000032              | 2.396655                                                       |
| 30783 | 1.380502              | 2.396660                                                       |
| 30785 | 1.234887              | 2.396665                                                       |
| 30787 | 1.059408              | 2.396669                                                       |
| 30789 | 1.580824              | 2.396674                                                       |
| 30791 | 1.025754              | 2.396679                                                       |
| 30793 | 1.178450              | 2.396684                                                       |
| 30795 | 1.600779              | 2.396688                                                       |
| 30797 | 1.134656              | 2.396693                                                       |
| 30799 | 1.053281              | 2.396698                                                       |
| 30801 | 1.333463              | 2.396703                                                       |
| 30803 | 1.000032              | 2.396707                                                       |
| 30805 | 1.231748              | 2.396712                                                       |
| 30807 | 1.703509              | 2.396717                                                       |
| 30809 | 1.000032              | 2.396722                                                       |
| 30811 | 1.091299              | 2.396726                                                       |
| 30813 | 1.333463              | 2.396731                                                       |

| $n$   | $\frac{\sigma(n)}{n}$ | $\frac{e^\gamma}{2} \log \log n + \frac{0.73...}{\log \log n}$ |
|-------|-----------------------|----------------------------------------------------------------|
| 30815 | 1.200195              | 2.396736                                                       |
| 30817 | 1.000032              | 2.396740                                                       |
| 30819 | 1.333463              | 2.396745                                                       |
| 30821 | 1.264982              | 2.396750                                                       |
| 30823 | 1.077377              | 2.396755                                                       |
| 30825 | 1.804185              | 2.396759                                                       |
| 30827 | 1.035456              | 2.396764                                                       |
| 30829 | 1.000032              | 2.396769                                                       |
| 30831 | 1.370050              | 2.396774                                                       |
| 30833 | 1.091298              | 2.396778                                                       |
| 30835 | 1.372985              | 2.396783                                                       |
| 30837 | 1.406103              | 2.396788                                                       |
| 30839 | 1.000032              | 2.396793                                                       |
| 30841 | 1.000032              | 2.396797                                                       |
| 30843 | 1.517362              | 2.396802                                                       |
| 30845 | 1.244934              | 2.396807                                                       |
| 30847 | 1.012740              | 2.396812                                                       |
| 30849 | 1.655548              | 2.396816                                                       |
| 30851 | 1.000032              | 2.396821                                                       |
| 30853 | 1.000032              | 2.396826                                                       |
| 30855 | 1.862129              | 2.396830                                                       |
| 30857 | 1.018894              | 2.396835                                                       |
| 30859 | 1.000032              | 2.396840                                                       |
| 30861 | 1.509737              | 2.396845                                                       |
| 30863 | 1.143116              | 2.396849                                                       |
| 30865 | 1.200194              | 2.396854                                                       |
| 30867 | 1.333463              | 2.396859                                                       |
| 30869 | 1.000032              | 2.396864                                                       |
| 30871 | 1.000032              | 2.396868                                                       |
| 30873 | 1.371295              | 2.396873                                                       |
| 30875 | 1.414737              | 2.396878                                                       |
| 30877 | 1.249862              | 2.396883                                                       |
| 30879 | 1.495385              | 2.396887                                                       |
| 30881 | 1.000032              | 2.396892                                                       |
| 30883 | 1.014150              | 2.396897                                                       |
| 30885 | 1.678485              | 2.396901                                                       |
| 30887 | 1.017127              | 2.396906                                                       |
| 30889 | 1.118845              | 2.396911                                                       |
| 30891 | 1.524845              | 2.396916                                                       |
| 30893 | 1.000032              | 2.396920                                                       |
| 30895 | 1.239812              | 2.396925                                                       |
| 30897 | 1.444865              | 2.396930                                                       |
| 30899 | 1.111881              | 2.396935                                                       |
| 30901 | 1.077376              | 2.396939                                                       |

| $n$   | $\frac{\sigma(n)}{n}$ | $\frac{e^\gamma}{2} \log \log n + \frac{0.73...}{\log \log n}$ |
|-------|-----------------------|----------------------------------------------------------------|
| 30903 | 1.333463              | 2.396944                                                       |
| 30905 | 1.372982              | 2.396949                                                       |
| 30907 | 1.033293              | 2.396953                                                       |
| 30909 | 1.333463              | 2.396958                                                       |
| 30911 | 1.000032              | 2.396963                                                       |
| 30913 | 1.053279              | 2.396968                                                       |
| 30915 | 1.785541              | 2.396972                                                       |
| 30917 | 1.024679              | 2.396977                                                       |
| 30919 | 1.165109              | 2.396982                                                       |
| 30921 | 1.456098              | 2.396987                                                       |
| 30923 | 1.072212              | 2.396991                                                       |
| 30925 | 1.241002              | 2.396996                                                       |
| 30927 | 1.467456              | 2.397001                                                       |
| 30929 | 1.011478              | 2.397005                                                       |
| 30931 | 1.000032              | 2.397010                                                       |
| 30933 | 1.654156              | 2.397015                                                       |
| 30935 | 1.256829              | 2.397020                                                       |
| 30937 | 1.000032              | 2.397024                                                       |
| 30939 | 1.333463              | 2.397029                                                       |
| 30941 | 1.000032              | 2.397034                                                       |
| 30943 | 1.140161              | 2.397038                                                       |
| 30945 | 1.600776              | 2.397043                                                       |
| 30947 | 1.143116              | 2.397048                                                       |
| 30949 | 1.000032              | 2.397053                                                       |
| 30951 | 1.528868              | 2.397057                                                       |
| 30953 | 1.077375              | 2.397062                                                       |
| 30955 | 1.237409              | 2.397067                                                       |
| 30957 | 1.414091              | 2.397071                                                       |
| 30959 | 1.014761              | 2.397076                                                       |
| 30961 | 1.143116              | 2.397081                                                       |
| 30963 | 1.333463              | 2.397086                                                       |
| 30965 | 1.311416              | 2.397090                                                       |
| 30967 | 1.011399              | 2.397095                                                       |
| 30969 | 1.570603              | 2.397100                                                       |
| 30971 | 1.000032              | 2.397104                                                       |
| 30973 | 1.022826              | 2.397109                                                       |
| 30975 | 1.921550              | 2.397114                                                       |
| 30977 | 1.000032              | 2.397119                                                       |
| 30979 | 1.077375              | 2.397123                                                       |
| 30981 | 1.394403              | 2.397128                                                       |
| 30983 | 1.000032              | 2.397133                                                       |
| 30985 | 1.200194              | 2.397137                                                       |
| 30987 | 1.580792              | 2.397142                                                       |
| 30989 | 1.208171              | 2.397147                                                       |

| $n$   | $\frac{\sigma(n)}{n}$ | $\frac{e^\gamma}{2} \log \log n + \frac{0.73...}{\log \log n}$ |
|-------|-----------------------|----------------------------------------------------------------|
| 30991 | 1.059404              | 2.397152                                                       |
| 30993 | 1.333462              | 2.397156                                                       |
| 30995 | 1.200194              | 2.397161                                                       |
| 30997 | 1.011711              | 2.397166                                                       |
| 30999 | 1.333462              | 2.397170                                                       |
| 31001 | 1.035450              | 2.397175                                                       |
| 31003 | 1.180789              | 2.397180                                                       |
| 31005 | 1.901887              | 2.397185                                                       |
| 31007 | 1.013191              | 2.397189                                                       |
| 31009 | 1.091296              | 2.397194                                                       |
| 31011 | 1.333462              | 2.397199                                                       |
| 31013 | 1.000032              | 2.397203                                                       |
| 31015 | 1.200193              | 2.397208                                                       |
| 31017 | 1.558371              | 2.397213                                                       |
| 31019 | 1.000032              | 2.397218                                                       |
| 31021 | 1.017117              | 2.397222                                                       |
| 31023 | 1.497727              | 2.397227                                                       |
| 31025 | 1.330927              | 2.397232                                                       |
| 31027 | 1.113869              | 2.397236                                                       |
| 31029 | 1.333462              | 2.397241                                                       |
| 31031 | 1.385969              | 2.397246                                                       |
| 31033 | 1.000032              | 2.397250                                                       |
| 31035 | 1.600773              | 2.397255                                                       |
| 31037 | 1.025743              | 2.397260                                                       |
| 31039 | 1.000032              | 2.397265                                                       |
| 31041 | 1.444863              | 2.397269                                                       |
| 31043 | 1.028251              | 2.397274                                                       |
| 31045 | 1.372975              | 2.397279                                                       |
| 31047 | 1.360518              | 2.397283                                                       |
| 31049 | 1.018390              | 2.397288                                                       |
| 31051 | 1.000032              | 2.397293                                                       |
| 31053 | 1.456091              | 2.397298                                                       |
| 31055 | 1.200193              | 2.397302                                                       |
| 31057 | 1.077374              | 2.397307                                                       |
| 31059 | 1.808172              | 2.397312                                                       |
| 31061 | 1.014133              | 2.397316                                                       |
| 31063 | 1.000032              | 2.397321                                                       |
| 31065 | 1.699662              | 2.397326                                                       |
| 31067 | 1.022822              | 2.397330                                                       |
| 31069 | 1.000032              | 2.397335                                                       |
| 31071 | 1.333462              | 2.397340                                                       |
| 31073 | 1.198726              | 2.397345                                                       |
| 31075 | 1.364698              | 2.397349                                                       |
| 31077 | 1.482769              | 2.397354                                                       |

| $n$   | $\frac{\sigma(n)}{n}$ | $\frac{e^\gamma}{2} \log \log n + \frac{0.73...}{\log \log n}$ |
|-------|-----------------------|----------------------------------------------------------------|
| 31079 | 1.000032              | 2.397359                                                       |
| 31081 | 1.000032              | 2.397363                                                       |
| 31083 | 1.437699              | 2.397368                                                       |
| 31085 | 1.200193              | 2.397373                                                       |
| 31087 | 1.143114              | 2.397377                                                       |
| 31089 | 1.370002              | 2.397382                                                       |
| 31091 | 1.000032              | 2.397387                                                       |
| 31093 | 1.111504              | 2.397391                                                       |
| 31095 | 1.735842              | 2.397396                                                       |
| 31097 | 1.103450              | 2.397401                                                       |
| 31099 | 1.011737              | 2.397406                                                       |
| 31101 | 1.524838              | 2.397410                                                       |
| 31103 | 1.053275              | 2.397415                                                       |
| 31105 | 1.200193              | 2.397420                                                       |
| 31107 | 1.333462              | 2.397424                                                       |
| 31109 | 1.077373              | 2.397429                                                       |
| 31111 | 1.020604              | 2.397434                                                       |
| 31113 | 1.444862              | 2.397438                                                       |
| 31115 | 1.406910              | 2.397443                                                       |
| 31117 | 1.063663              | 2.397448                                                       |
| 31119 | 1.554806              | 2.397452                                                       |
| 31121 | 1.000032              | 2.397457                                                       |
| 31123 | 1.000032              | 2.397462                                                       |
| 31125 | 1.684048              | 2.397467                                                       |
| 31127 | 1.059402              | 2.397471                                                       |
| 31129 | 1.143114              | 2.397476                                                       |
| 31131 | 1.482766              | 2.397481                                                       |
| 31133 | 1.011403              | 2.397485                                                       |
| 31135 | 1.295006              | 2.397490                                                       |
| 31137 | 1.359669              | 2.397495                                                       |
| 31139 | 1.000032              | 2.397499                                                       |
| 31141 | 1.156032              | 2.397504                                                       |
| 31143 | 1.524837              | 2.397509                                                       |
| 31145 | 1.200193              | 2.397513                                                       |
| 31147 | 1.000032              | 2.397518                                                       |
| 31149 | 1.444862              | 2.397523                                                       |
| 31151 | 1.000032              | 2.397527                                                       |
| 31153 | 1.000032              | 2.397532                                                       |
| 31155 | 1.676264              | 2.397537                                                       |
| 31157 | 1.143114              | 2.397542                                                       |
| 31159 | 1.000032              | 2.397546                                                       |
| 31161 | 1.552710              | 2.397551                                                       |
| 31163 | 1.091294              | 2.397556                                                       |
| 31165 | 1.256794              | 2.397560                                                       |



| $n$   | $\frac{\sigma(n)}{n}$ | $\frac{e^\gamma}{2} \log \log n + \frac{0.73...}{\log \log n}$ |
|-------|-----------------------|----------------------------------------------------------------|
| 31167 | 1.444862              | 2.397565                                                       |
| 31169 | 1.016394              | 2.397570                                                       |
| 31171 | 1.177505              | 2.397574                                                       |
| 31173 | 1.333462              | 2.397579                                                       |
| 31175 | 1.312590              | 2.397584                                                       |
| 31177 | 1.000032              | 2.397588                                                       |
| 31179 | 1.406075              | 2.397593                                                       |
| 31181 | 1.000032              | 2.397598                                                       |
| 31183 | 1.000032              | 2.397602                                                       |
| 31185 | 2.234921              | 2.397607                                                       |
| 31187 | 1.077372              | 2.397612                                                       |
| 31189 | 1.000032              | 2.397616                                                       |
| 31191 | 1.374243              | 2.397621                                                       |
| 31193 | 1.000032              | 2.397626                                                       |
| 31195 | 1.274050              | 2.397630                                                       |
| 31197 | 1.333462              | 2.397635                                                       |
| 31199 | 1.143114              | 2.397640                                                       |
| 31201 | 1.025736              | 2.397644                                                       |
| 31203 | 1.444861              | 2.397649                                                       |
| 31205 | 1.215382              | 2.397654                                                       |
| 31207 | 1.091294              | 2.397659                                                       |
| 31209 | 1.359608              | 2.397663                                                       |
| 31211 | 1.063087              | 2.397668                                                       |
| 31213 | 1.256336              | 2.397673                                                       |
| 31215 | 1.600769              | 2.397677                                                       |
| 31217 | 1.107089              | 2.397682                                                       |
| 31219 | 1.000032              | 2.397687                                                       |
| 31221 | 1.444861              | 2.397691                                                       |
| 31223 | 1.000032              | 2.397696                                                       |
| 31225 | 1.240993              | 2.397701                                                       |
| 31227 | 1.524834              | 2.397705                                                       |
| 31229 | 1.161997              | 2.397710                                                       |
| 31231 | 1.000032              | 2.397715                                                       |
| 31233 | 1.383152              | 2.397719                                                       |
| 31235 | 1.200192              | 2.397724                                                       |
| 31237 | 1.000032              | 2.397729                                                       |
| 31239 | 1.613368              | 2.397733                                                       |
| 31241 | 1.143113              | 2.397738                                                       |
| 31243 | 1.011427              | 2.397743                                                       |
| 31245 | 1.600768              | 2.397747                                                       |
| 31247 | 1.000032              | 2.397752                                                       |
| 31249 | 1.000032              | 2.397757                                                       |
| 31251 | 1.456081              | 2.397761                                                       |
| 31253 | 1.000032              | 2.397766                                                       |

| $n$   | $\frac{\sigma(n)}{n}$ | $\frac{e^\gamma}{2} \log \log n + \frac{0.73...}{\log \log n}$ |
|-------|-----------------------|----------------------------------------------------------------|
| 31255 | 1.474324              | 2.397771                                                       |
| 31257 | 1.517228              | 2.397775                                                       |
| 31259 | 1.000032              | 2.397780                                                       |
| 31261 | 1.024663              | 2.397785                                                       |
| 31263 | 1.414068              | 2.397789                                                       |
| 31265 | 1.334527              | 2.397794                                                       |
| 31267 | 1.000032              | 2.397799                                                       |
| 31269 | 1.524833              | 2.397803                                                       |
| 31271 | 1.000032              | 2.397808                                                       |
| 31273 | 1.091293              | 2.397813                                                       |
| 31275 | 1.803997              | 2.397817                                                       |
| 31277 | 1.000032              | 2.397822                                                       |
| 31279 | 1.033281              | 2.397827                                                       |
| 31281 | 1.333461              | 2.397831                                                       |
| 31283 | 1.181472              | 2.397836                                                       |
| 31285 | 1.200192              | 2.397841                                                       |
| 31287 | 1.333461              | 2.397845                                                       |
| 31289 | 1.017099              | 2.397850                                                       |
| 31291 | 1.127481              | 2.397855                                                       |
| 31293 | 1.585019              | 2.397859                                                       |
| 31295 | 1.311392              | 2.397864                                                       |
| 31297 | 1.214685              | 2.397869                                                       |
| 31299 | 1.333461              | 2.397873                                                       |
| 31301 | 1.012492              | 2.397878                                                       |
| 31303 | 1.044245              | 2.397883                                                       |
| 31305 | 1.600767              | 2.397887                                                       |
| 31307 | 1.000032              | 2.397892                                                       |
| 31309 | 1.011850              | 2.397897                                                       |
| 31311 | 1.703938              | 2.397901                                                       |
| 31313 | 1.011337              | 2.397906                                                       |
| 31315 | 1.200192              | 2.397911                                                       |
| 31317 | 1.587892              | 2.397915                                                       |
| 31319 | 1.000032              | 2.397920                                                       |
| 31321 | 1.000032              | 2.397925                                                       |
| 31323 | 1.365386              | 2.397929                                                       |
| 31325 | 1.425060              | 2.397934                                                       |
| 31327 | 1.000032              | 2.397939                                                       |
| 31329 | 1.469342              | 2.397943                                                       |
| 31331 | 1.126041              | 2.397948                                                       |
| 31333 | 1.000032              | 2.397952                                                       |
| 31335 | 1.600766              | 2.397957                                                       |
| 31337 | 1.000032              | 2.397962                                                       |
| 31339 | 1.290150              | 2.397966                                                       |
| 31341 | 1.380428              | 2.397971                                                       |

| $n$   | $\frac{\sigma(n)}{n}$ | $\frac{e^\gamma}{2} \log \log n + \frac{0.73...}{\log \log n}$ |
|-------|-----------------------|----------------------------------------------------------------|
| 31343 | 1.077370              | 2.397976                                                       |
| 31345 | 1.200191              | 2.397980                                                       |
| 31347 | 1.534182              | 2.397985                                                       |
| 31349 | 1.102428              | 2.397990                                                       |
| 31351 | 1.012791              | 2.397994                                                       |
| 31353 | 1.524830              | 2.397999                                                       |
| 31355 | 1.200191              | 2.398004                                                       |
| 31357 | 1.000032              | 2.398008                                                       |
| 31359 | 1.333461              | 2.398013                                                       |
| 31361 | 1.091292              | 2.398018                                                       |
| 31363 | 1.015209              | 2.398022                                                       |
| 31365 | 1.880057              | 2.398027                                                       |
| 31367 | 1.143112              | 2.398032                                                       |
| 31369 | 1.142529              | 2.398036                                                       |
| 31371 | 1.333461              | 2.398041                                                       |
| 31373 | 1.011698              | 2.398046                                                       |
| 31375 | 1.252972              | 2.398050                                                       |
| 31377 | 1.333461              | 2.398055                                                       |
| 31379 | 1.000032              | 2.398059                                                       |
| 31381 | 1.143112              | 2.398064                                                       |
| 31383 | 1.580728              | 2.398069                                                       |
| 31385 | 1.200191              | 2.398073                                                       |
| 31387 | 1.000032              | 2.398078                                                       |
| 31389 | 1.333461              | 2.398083                                                       |
| 31391 | 1.000032              | 2.398087                                                       |
| 31393 | 1.000032              | 2.398092                                                       |
| 31395 | 2.054849              | 2.398097                                                       |
| 31397 | 1.000032              | 2.398101                                                       |
| 31399 | 1.059397              | 2.398106                                                       |
| 31401 | 1.482755              | 2.398111                                                       |
| 31403 | 1.033277              | 2.398115                                                       |
| 31405 | 1.311384              | 2.398120                                                       |
| 31407 | 1.455726              | 2.398125                                                       |
| 31409 | 1.165080              | 2.398129                                                       |
| 31411 | 1.013148              | 2.398134                                                       |
| 31413 | 1.374208              | 2.398138                                                       |
| 31415 | 1.231514              | 2.398143                                                       |
| 31417 | 1.014101              | 2.398148                                                       |
| 31419 | 1.444858              | 2.398152                                                       |
| 31421 | 1.077369              | 2.398157                                                       |
| 31423 | 1.160169              | 2.398162                                                       |
| 31425 | 1.657279              | 2.398166                                                       |
| 31427 | 1.091291              | 2.398171                                                       |
| 31429 | 1.020586              | 2.398176                                                       |

| $n$   | $\frac{\sigma(n)}{n}$ | $\frac{e^\gamma}{2} \log \log n + \frac{0.73\dots}{\log \log n}$ |
|-------|-----------------------|------------------------------------------------------------------|
| 31431 | 1.333461              | 2.398180                                                         |
| 31433 | 1.084020              | 2.398185                                                         |
| 31435 | 1.200191              | 2.398189                                                         |
| 31437 | 1.654102              | 2.398194                                                         |
| 31439 | 1.011483              | 2.398199                                                         |
| 31441 | 1.044242              | 2.398203                                                         |
| 31443 | 1.367808              | 2.398208                                                         |
| 31445 | 1.266974              | 2.398213                                                         |
| 31447 | 1.121888              | 2.398217                                                         |
| 31449 | 1.456072              | 2.398222                                                         |
| 31451 | 1.143112              | 2.398227                                                         |
| 31453 | 1.016374              | 2.398231                                                         |
| 31455 | 1.785408              | 2.398236                                                         |
| 31457 | 1.014719              | 2.398241                                                         |
| 31459 | 1.011348              | 2.398245                                                         |
| 31461 | 1.333460              | 2.398250                                                         |
| 31463 | 1.016051              | 2.398254                                                         |
| 31465 | 1.464484              | 2.398259                                                         |
| 31467 | 1.414053              | 2.398264                                                         |
| 31469 | 1.000032              | 2.398268                                                         |
| 31471 | 1.091290              | 2.398273                                                         |
| 31473 | 1.561338              | 2.398278                                                         |
| 31475 | 1.240985              | 2.398282                                                         |
| 31477 | 1.000032              | 2.398287                                                         |
| 31479 | 1.524826              | 2.398291                                                         |
| 31481 | 1.000032              | 2.398296                                                         |
| 31483 | 1.053267              | 2.398301                                                         |
| 31485 | 1.600762              | 2.398305                                                         |
| 31487 | 1.072443              | 2.398310                                                         |
| 31489 | 1.000032              | 2.398315                                                         |
| 31491 | 1.444857              | 2.398319                                                         |
| 31493 | 1.249802              | 2.398324                                                         |
| 31495 | 1.200191              | 2.398329                                                         |
| 31497 | 1.333460              | 2.398333                                                         |
| 31499 | 1.077368              | 2.398338                                                         |
| 31501 | 1.072029              | 2.398342                                                         |
| 31503 | 1.333460              | 2.398347                                                         |
| 31505 | 1.200190              | 2.398352                                                         |
| 31507 | 1.165074              | 2.398356                                                         |
| 31509 | 1.497667              | 2.398361                                                         |
| 31511 | 1.000032              | 2.398366                                                         |
| 31513 | 1.000032              | 2.398370                                                         |
| 31515 | 1.754593              | 2.398375                                                         |
| 31517 | 1.000032              | 2.398379                                                         |

| $n$   | $\frac{\sigma(n)}{n}$ | $\frac{e^\gamma}{2} \log \log n + \frac{0.73\dots}{\log \log n}$ |
|-------|-----------------------|------------------------------------------------------------------|
| 31519 | 1.024652              | 2.398384                                                         |
| 31521 | 1.624314              | 2.398389                                                         |
| 31523 | 1.035434              | 2.398393                                                         |
| 31525 | 1.349151              | 2.398398                                                         |
| 31527 | 1.504234              | 2.398403                                                         |
| 31529 | 1.025722              | 2.398407                                                         |
| 31531 | 1.000032              | 2.398412                                                         |
| 31533 | 1.394349              | 2.398416                                                         |
| 31535 | 1.479499              | 2.398421                                                         |
| 31537 | 1.132384              | 2.398426                                                         |
| 31539 | 1.333460              | 2.398430                                                         |
| 31541 | 1.000032              | 2.398435                                                         |
| 31543 | 1.000032              | 2.398440                                                         |
| 31545 | 1.735806              | 2.398444                                                         |
| 31547 | 1.000032              | 2.398449                                                         |
| 31549 | 1.143111              | 2.398453                                                         |
| 31551 | 1.437672              | 2.398458                                                         |
| 31553 | 1.011631              | 2.398463                                                         |
| 31555 | 1.200190              | 2.398467                                                         |
| 31557 | 1.361853              | 2.398472                                                         |
| 31559 | 1.155930              | 2.398477                                                         |
| 31561 | 1.028231              | 2.398481                                                         |
| 31563 | 1.703260              | 2.398486                                                         |
| 31565 | 1.231744              | 2.398490                                                         |
| 31567 | 1.000032              | 2.398495                                                         |
| 31569 | 1.414045              | 2.398500                                                         |
| 31571 | 1.011815              | 2.398504                                                         |
| 31573 | 1.000032              | 2.398509                                                         |
| 31575 | 1.657260              | 2.398513                                                         |
| 31577 | 1.234316              | 2.398518                                                         |
| 31579 | 1.044238              | 2.398523                                                         |
| 31581 | 1.642443              | 2.398527                                                         |
| 31583 | 1.000032              | 2.398532                                                         |
| 31585 | 1.200190              | 2.398537                                                         |
| 31587 | 1.333460              | 2.398541                                                         |
| 31589 | 1.033271              | 2.398546                                                         |
| 31591 | 1.143110              | 2.398550                                                         |
| 31593 | 1.333460              | 2.398555                                                         |
| 31595 | 1.230574              | 2.398560                                                         |
| 31597 | 1.053265              | 2.398564                                                         |
| 31599 | 1.444856              | 2.398569                                                         |
| 31601 | 1.000032              | 2.398573                                                         |
| 31603 | 1.250767              | 2.398578                                                         |
| 31605 | 1.904509              | 2.398583                                                         |

| $n$   | $\frac{\sigma(n)}{n}$ | $\frac{e^\gamma}{2} \log \log n + \frac{0.73\dots}{\log \log n}$ |
|-------|-----------------------|------------------------------------------------------------------|
| 31607 | 1.000032              | 2.398587                                                         |
| 31609 | 1.016040              | 2.398592                                                         |
| 31611 | 1.371168              | 2.398597                                                         |
| 31613 | 1.013128              | 2.398601                                                         |
| 31615 | 1.200190              | 2.398606                                                         |
| 31617 | 1.482747              | 2.398610                                                         |
| 31619 | 1.143110              | 2.398615                                                         |
| 31621 | 1.012998              | 2.398620                                                         |
| 31623 | 1.360023              | 2.398624                                                         |
| 31625 | 1.420648              | 2.398629                                                         |
| 31627 | 1.000032              | 2.398633                                                         |
| 31629 | 1.437668              | 2.398638                                                         |
| 31631 | 1.022794              | 2.398643                                                         |
| 31633 | 1.143110              | 2.398647                                                         |
| 31635 | 1.873874              | 2.398652                                                         |
| 31637 | 1.059392              | 2.398656                                                         |
| 31639 | 1.035431              | 2.398661                                                         |
| 31641 | 1.365317              | 2.398666                                                         |
| 31643 | 1.000032              | 2.398670                                                         |
| 31645 | 1.200190              | 2.398675                                                         |
| 31647 | 1.674472              | 2.398679                                                         |
| 31649 | 1.000032              | 2.398684                                                         |
| 31651 | 1.033269              | 2.398689                                                         |
| 31653 | 1.444855              | 2.398693                                                         |
| 31655 | 1.294961              | 2.398698                                                         |
| 31657 | 1.000032              | 2.398703                                                         |
| 31659 | 1.363025              | 2.398707                                                         |
| 31661 | 1.143110              | 2.398712                                                         |
| 31663 | 1.000032              | 2.398716                                                         |
| 31665 | 1.600758              | 2.398721                                                         |
| 31667 | 1.000032              | 2.398726                                                         |
| 31669 | 1.091288              | 2.398730                                                         |
| 31671 | 1.650469              | 2.398735                                                         |
| 31673 | 1.053263              | 2.398739                                                         |
| 31675 | 1.424972              | 2.398744                                                         |
| 31677 | 1.333460              | 2.398749                                                         |
| 31679 | 1.015184              | 2.398753                                                         |
| 31681 | 1.077365              | 2.398758                                                         |
| 31683 | 1.363507              | 2.398762                                                         |
| 31685 | 1.200189              | 2.398767                                                         |
| 31687 | 1.000032              | 2.398772                                                         |
| 31689 | 1.654076              | 2.398776                                                         |
| 31691 | 1.132940              | 2.398781                                                         |
| 31693 | 1.025715              | 2.398785                                                         |

| $n$   | $\frac{\sigma(n)}{n}$ | $\frac{e^\gamma}{2} \log \log n + \frac{0.73...}{\log \log n}$ |
|-------|-----------------------|----------------------------------------------------------------|
| 31695 | 1.600757              | 2.398790                                                       |
| 31697 | 1.035429              | 2.398795                                                       |
| 31699 | 1.000032              | 2.398799                                                       |
| 31701 | 1.333460              | 2.398804                                                       |
| 31703 | 1.165063              | 2.398808                                                       |
| 31705 | 1.273995              | 2.398813                                                       |
| 31707 | 1.561296              | 2.398818                                                       |
| 31709 | 1.028225              | 2.398822                                                       |
| 31711 | 1.053262              | 2.398827                                                       |
| 31713 | 1.502980              | 2.398831                                                       |
| 31715 | 1.200189              | 2.398836                                                       |
| 31717 | 1.198600              | 2.398840                                                       |
| 31719 | 1.359438              | 2.398845                                                       |
| 31721 | 1.000032              | 2.398850                                                       |
| 31723 | 1.000032              | 2.398854                                                       |
| 31725 | 1.876123              | 2.398859                                                       |
| 31727 | 1.000032              | 2.398863                                                       |
| 31729 | 1.000032              | 2.398868                                                       |
| 31731 | 1.524818              | 2.398873                                                       |
| 31733 | 1.077364              | 2.398877                                                       |
| 31735 | 1.311360              | 2.398882                                                       |
| 31737 | 1.361187              | 2.398886                                                       |
| 31739 | 1.059391              | 2.398891                                                       |
| 31741 | 1.000032              | 2.398896                                                       |
| 31743 | 1.444854              | 2.398900                                                       |
| 31745 | 1.372941              | 2.398905                                                       |
| 31747 | 1.020569              | 2.398909                                                       |
| 31749 | 1.406029              | 2.398914                                                       |
| 31751 | 1.000031              | 2.398919                                                       |
| 31753 | 1.012440              | 2.398923                                                       |
| 31755 | 1.677846              | 2.398928                                                       |
| 31757 | 1.091287              | 2.398932                                                       |
| 31759 | 1.234296              | 2.398937                                                       |
| 31761 | 1.444854              | 2.398941                                                       |
| 31763 | 1.044234              | 2.398946                                                       |
| 31765 | 1.200189              | 2.398951                                                       |
| 31767 | 1.333459              | 2.398955                                                       |
| 31769 | 1.000031              | 2.398960                                                       |
| 31771 | 1.000031              | 2.398964                                                       |
| 31773 | 1.631574              | 2.398969                                                       |
| 31775 | 1.311220              | 2.398974                                                       |
| 31777 | 1.024640              | 2.398978                                                       |
| 31779 | 1.631266              | 2.398983                                                       |
| 31781 | 1.018344              | 2.398987                                                       |

| $n$   | $\frac{\sigma(n)}{n}$ | $\frac{e^\gamma}{2} \log \log n + \frac{0.73\dots}{\log \log n}$ |
|-------|-----------------------|------------------------------------------------------------------|
| 31783 | 1.028223              | 2.398992                                                         |
| 31785 | 1.733648              | 2.398997                                                         |
| 31787 | 1.208041              | 2.399001                                                         |
| 31789 | 1.014691              | 2.399006                                                         |
| 31791 | 1.333459              | 2.399010                                                         |
| 31793 | 1.000031              | 2.399015                                                         |
| 31795 | 1.200189              | 2.399019                                                         |
| 31797 | 1.444853              | 2.399024                                                         |
| 31799 | 1.000031              | 2.399029                                                         |
| 31801 | 1.290525              | 2.399033                                                         |
| 31803 | 1.333459              | 2.399038                                                         |
| 31805 | 1.200189              | 2.399042                                                         |
| 31807 | 1.059389              | 2.399047                                                         |
| 31809 | 1.394322              | 2.399052                                                         |
| 31811 | 1.077363              | 2.399056                                                         |
| 31813 | 1.035426              | 2.399061                                                         |
| 31815 | 2.000566              | 2.399065                                                         |
| 31817 | 1.000031              | 2.399070                                                         |
| 31819 | 1.022785              | 2.399074                                                         |
| 31821 | 1.333459              | 2.399079                                                         |
| 31823 | 1.103353              | 2.399084                                                         |
| 31825 | 1.324745              | 2.399088                                                         |
| 31827 | 1.346404              | 2.399093                                                         |
| 31829 | 1.143108              | 2.399097                                                         |
| 31831 | 1.011592              | 2.399102                                                         |
| 31833 | 1.509377              | 2.399106                                                         |
| 31835 | 1.200188              | 2.399111                                                         |
| 31837 | 1.125734              | 2.399116                                                         |
| 31839 | 1.333459              | 2.399120                                                         |
| 31841 | 1.059389              | 2.399125                                                         |
| 31843 | 1.143108              | 2.399129                                                         |
| 31845 | 1.754498              | 2.399134                                                         |
| 31847 | 1.000031              | 2.399138                                                         |
| 31849 | 1.000031              | 2.399143                                                         |
| 31851 | 1.444853              | 2.399148                                                         |
| 31853 | 1.020563              | 2.399152                                                         |
| 31855 | 1.256694              | 2.399157                                                         |
| 31857 | 1.603164              | 2.399161                                                         |
| 31859 | 1.000031              | 2.399166                                                         |
| 31861 | 1.011393              | 2.399170                                                         |
| 31863 | 1.546621              | 2.399175                                                         |
| 31865 | 1.200188              | 2.399180                                                         |
| 31867 | 1.091286              | 2.399184                                                         |
| 31869 | 1.444852              | 2.399189                                                         |



| $n$   | $\frac{\sigma(n)}{n}$ | $\frac{e^\gamma}{2} \log \log n + \frac{0.73\dots}{\log \log n}$ |
|-------|-----------------------|------------------------------------------------------------------|
| 31871 | 1.189796              | 2.399193                                                         |
| 31873 | 1.000031              | 2.399198                                                         |
| 31875 | 1.764141              | 2.399202                                                         |
| 31877 | 1.011889              | 2.399207                                                         |
| 31879 | 1.016343              | 2.399212                                                         |
| 31881 | 1.333459              | 2.399216                                                         |
| 31883 | 1.000031              | 2.399221                                                         |
| 31885 | 1.372934              | 2.399225                                                         |
| 31887 | 1.482736              | 2.399230                                                         |
| 31889 | 1.180093              | 2.399234                                                         |
| 31891 | 1.000031              | 2.399239                                                         |
| 31893 | 1.333459              | 2.399244                                                         |
| 31895 | 1.200188              | 2.399248                                                         |
| 31897 | 1.011255              | 2.399253                                                         |
| 31899 | 1.605066              | 2.399257                                                         |
| 31901 | 1.113445              | 2.399262                                                         |
| 31903 | 1.018337              | 2.399266                                                         |
| 31905 | 1.735778              | 2.399271                                                         |
| 31907 | 1.000031              | 2.399276                                                         |
| 31909 | 1.059388              | 2.399280                                                         |
| 31911 | 1.456050              | 2.399285                                                         |
| 31913 | 1.179206              | 2.399289                                                         |
| 31915 | 1.294940              | 2.399294                                                         |
| 31917 | 1.333459              | 2.399298                                                         |
| 31919 | 1.018829              | 2.399303                                                         |
| 31921 | 1.011622              | 2.399308                                                         |
| 31923 | 1.444852              | 2.399312                                                         |
| 31925 | 1.240971              | 2.399317                                                         |
| 31927 | 1.143108              | 2.399321                                                         |
| 31929 | 1.383069              | 2.399326                                                         |
| 31931 | 1.028217              | 2.399330                                                         |
| 31933 | 1.091285              | 2.399335                                                         |
| 31935 | 1.600752              | 2.399339                                                         |
| 31937 | 1.012619              | 2.399344                                                         |
| 31939 | 1.078932              | 2.399349                                                         |
| 31941 | 1.833380              | 2.399353                                                         |
| 31943 | 1.059387              | 2.399358                                                         |
| 31945 | 1.200188              | 2.399362                                                         |
| 31947 | 1.394309              | 2.399367                                                         |
| 31949 | 1.024633              | 2.399371                                                         |
| 31951 | 1.014053              | 2.399376                                                         |
| 31953 | 1.333459              | 2.399380                                                         |
| 31955 | 1.514129              | 2.399385                                                         |
| 31957 | 1.000031              | 2.399390                                                         |

| $n$   | $\frac{\sigma(n)}{n}$ | $\frac{e^\gamma}{2} \log \log n + \frac{0.73\dots}{\log \log n}$ |
|-------|-----------------------|------------------------------------------------------------------|
| 31959 | 1.493664              | 2.399394                                                         |
| 31961 | 1.033259              | 2.399399                                                         |
| 31963 | 1.000031              | 2.399403                                                         |
| 31965 | 1.600751              | 2.399408                                                         |
| 31967 | 1.077361              | 2.399412                                                         |
| 31969 | 1.143107              | 2.399417                                                         |
| 31971 | 1.333458              | 2.399422                                                         |
| 31973 | 1.000031              | 2.399426                                                         |
| 31975 | 1.240970              | 2.399431                                                         |
| 31977 | 1.756262              | 2.399435                                                         |
| 31979 | 1.012414              | 2.399440                                                         |
| 31981 | 1.000031              | 2.399444                                                         |
| 31983 | 1.524810              | 2.399449                                                         |
| 31985 | 1.200188              | 2.399453                                                         |
| 31987 | 1.035421              | 2.399458                                                         |
| 31989 | 1.333458              | 2.399462                                                         |
| 31991 | 1.000031              | 2.399467                                                         |
| 31993 | 1.134248              | 2.399472                                                         |
| 31995 | 1.815284              | 2.399476                                                         |
| 31997 | 1.165047              | 2.399481                                                         |
| 31999 | 1.091284              | 2.399485                                                         |
| 32001 | 1.333458              | 2.399490                                                         |
| 32003 | 1.000031              | 2.399494                                                         |
| 32005 | 1.239556              | 2.399499                                                         |
| 32007 | 1.367701              | 2.399503                                                         |
| 32009 | 1.000031              | 2.399508                                                         |
| 32011 | 1.214582              | 2.399513                                                         |
| 32013 | 1.444851              | 2.399517                                                         |
| 32015 | 1.266906              | 2.399522                                                         |
| 32017 | 1.013087              | 2.399526                                                         |
| 32019 | 1.437646              | 2.399531                                                         |
| 32021 | 1.133256              | 2.399535                                                         |
| 32023 | 1.033257              | 2.399540                                                         |
| 32025 | 1.920500              | 2.399544                                                         |
| 32027 | 1.000031              | 2.399549                                                         |
| 32029 | 1.000031              | 2.399553                                                         |
| 32031 | 1.444850              | 2.399558                                                         |
| 32033 | 1.012955              | 2.399563                                                         |
| 32035 | 1.236148              | 2.399567                                                         |
| 32037 | 1.363424              | 2.399572                                                         |
| 32039 | 1.198539              | 2.399576                                                         |
| 32041 | 1.005618              | 2.399581                                                         |
| 32043 | 1.456043              | 2.399585                                                         |
| 32045 | 1.415509              | 2.399590                                                         |

| $n$   | $\frac{\sigma(n)}{n}$ | $\frac{e^\gamma}{2} \log \log n + \frac{0.73\dots}{\log \log n}$ |
|-------|-----------------------|------------------------------------------------------------------|
| 32047 | 1.016008              | 2.399594                                                         |
| 32049 | 1.482730              | 2.399599                                                         |
| 32051 | 1.000031              | 2.399603                                                         |
| 32053 | 1.207999              | 2.399608                                                         |
| 32055 | 1.600749              | 2.399613                                                         |
| 32057 | 1.000031              | 2.399617                                                         |
| 32059 | 1.000031              | 2.399622                                                         |
| 32061 | 1.333458              | 2.399626                                                         |
| 32063 | 1.000031              | 2.399631                                                         |
| 32065 | 1.343895              | 2.399635                                                         |
| 32067 | 1.654037              | 2.399640                                                         |
| 32069 | 1.000031              | 2.399644                                                         |
| 32071 | 1.077360              | 2.399649                                                         |
| 32073 | 1.333458              | 2.399653                                                         |
| 32075 | 1.240966              | 2.399658                                                         |
| 32077 | 1.000031              | 2.399663                                                         |
| 32079 | 1.454659              | 2.399667                                                         |
| 32081 | 1.143107              | 2.399672                                                         |
| 32083 | 1.000031              | 2.399676                                                         |
| 32085 | 1.867041              | 2.399681                                                         |
| 32087 | 1.091283              | 2.399685                                                         |
| 32089 | 1.000031              | 2.399690                                                         |
| 32091 | 1.406002              | 2.399694                                                         |
| 32093 | 1.017044              | 2.399699                                                         |
| 32095 | 1.406574              | 2.399703                                                         |
| 32097 | 1.437642              | 2.399708                                                         |
| 32099 | 1.000031              | 2.399712                                                         |
| 32101 | 1.022772              | 2.399717                                                         |
| 32103 | 1.569947              | 2.399721                                                         |
| 32105 | 1.200187              | 2.399726                                                         |
| 32107 | 1.013362              | 2.399731                                                         |
| 32109 | 1.674297              | 2.399735                                                         |
| 32111 | 1.011242              | 2.399740                                                         |
| 32113 | 1.059384              | 2.399744                                                         |
| 32115 | 1.600747              | 2.399749                                                         |
| 32117 | 1.000031              | 2.399753                                                         |
| 32119 | 1.000031              | 2.399758                                                         |
| 32121 | 1.495844              | 2.399762                                                         |
| 32123 | 1.234256              | 2.399767                                                         |
| 32125 | 1.252856              | 2.399771                                                         |
| 32127 | 1.333458              | 2.399776                                                         |
| 32129 | 1.067260              | 2.399780                                                         |
| 32131 | 1.147303              | 2.399785                                                         |
| 32133 | 1.333458              | 2.399789                                                         |

| $n$   | $\frac{\sigma(n)}{n}$ | $\frac{e^\gamma}{2} \log \log n + \frac{0.73\dots}{\log \log n}$ |
|-------|-----------------------|------------------------------------------------------------------|
| 32135 | 1.200187              | 2.399794                                                         |
| 32137 | 1.143106              | 2.399799                                                         |
| 32139 | 1.444849              | 2.399803                                                         |
| 32141 | 1.000031              | 2.399808                                                         |
| 32143 | 1.000031              | 2.399812                                                         |
| 32145 | 1.600747              | 2.399817                                                         |
| 32147 | 1.110897              | 2.399821                                                         |
| 32149 | 1.077359              | 2.399826                                                         |
| 32151 | 1.524805              | 2.399830                                                         |
| 32153 | 1.134575              | 2.399835                                                         |
| 32155 | 1.231535              | 2.399839                                                         |
| 32157 | 1.497590              | 2.399844                                                         |
| 32159 | 1.000031              | 2.399848                                                         |
| 32161 | 1.035416              | 2.399853                                                         |
| 32163 | 1.361067              | 2.399857                                                         |
| 32165 | 1.372921              | 2.399862                                                         |
| 32167 | 1.053253              | 2.399866                                                         |
| 32169 | 1.333458              | 2.399871                                                         |
| 32171 | 1.020546              | 2.399875                                                         |
| 32173 | 1.000031              | 2.399880                                                         |
| 32175 | 2.104242              | 2.399885                                                         |
| 32177 | 1.044224              | 2.399889                                                         |
| 32179 | 1.143106              | 2.399894                                                         |
| 32181 | 1.414002              | 2.399898                                                         |
| 32183 | 1.000031              | 2.399903                                                         |
| 32185 | 1.237098              | 2.399907                                                         |
| 32187 | 1.333458              | 2.399912                                                         |
| 32189 | 1.000031              | 2.399916                                                         |
| 32191 | 1.000031              | 2.399921                                                         |
| 32193 | 1.703290              | 2.399925                                                         |
| 32195 | 1.234477              | 2.399930                                                         |
| 32197 | 1.091282              | 2.399934                                                         |
| 32199 | 1.333458              | 2.399939                                                         |
| 32201 | 1.077358              | 2.399943                                                         |
| 32203 | 1.000031              | 2.399948                                                         |
| 32205 | 1.699115              | 2.399952                                                         |
| 32207 | 1.180365              | 2.399957                                                         |
| 32209 | 1.033252              | 2.399961                                                         |
| 32211 | 1.482723              | 2.399966                                                         |
| 32213 | 1.000031              | 2.399970                                                         |
| 32215 | 1.273941              | 2.399975                                                         |
| 32217 | 1.333457              | 2.399979                                                         |
| 32219 | 1.139700              | 2.399984                                                         |
| 32221 | 1.143105              | 2.399989                                                         |

| $n$   | $\frac{\sigma(n)}{n}$ | $\frac{e^\gamma}{2} \log \log n + \frac{0.73\dots}{\log \log n}$ |
|-------|-----------------------|------------------------------------------------------------------|
| 32223 | 1.394284              | 2.399993                                                         |
| 32225 | 1.240962              | 2.399998                                                         |
| 32227 | 1.122537              | 2.400002                                                         |
| 32229 | 1.444848              | 2.400007                                                         |
| 32231 | 1.011200              | 2.400011                                                         |
| 32233 | 1.000031              | 2.400016                                                         |
| 32235 | 1.834528              | 2.400020                                                         |
| 32237 | 1.000031              | 2.400025                                                         |
| 32239 | 1.012935              | 2.400029                                                         |
| 32241 | 1.456034              | 2.400034                                                         |
| 32243 | 1.053252              | 2.400038                                                         |
| 32245 | 1.200186              | 2.400043                                                         |
| 32247 | 1.444848              | 2.400047                                                         |
| 32249 | 1.214549              | 2.400052                                                         |
| 32251 | 1.000031              | 2.400056                                                         |
| 32253 | 1.437634              | 2.400061                                                         |
| 32255 | 1.200186              | 2.400065                                                         |
| 32257 | 1.000031              | 2.400070                                                         |
| 32259 | 1.333457              | 2.400074                                                         |
| 32261 | 1.000031              | 2.400079                                                         |
| 32263 | 1.249729              | 2.400083                                                         |
| 32265 | 1.785216              | 2.400088                                                         |
| 32267 | 1.025692              | 2.400092                                                         |
| 32269 | 1.062506              | 2.400097                                                         |
| 32271 | 1.380310              | 2.400101                                                         |
| 32273 | 1.018808              | 2.400106                                                         |
| 32275 | 1.240960              | 2.400110                                                         |
| 32277 | 1.606097              | 2.400115                                                         |
| 32279 | 1.088510              | 2.400119                                                         |
| 32281 | 1.053251              | 2.400124                                                         |
| 32283 | 1.536660              | 2.400128                                                         |
| 32285 | 1.311321              | 2.400133                                                         |
| 32287 | 1.014650              | 2.400137                                                         |
| 32289 | 1.367648              | 2.400142                                                         |
| 32291 | 1.165031              | 2.400146                                                         |
| 32293 | 1.024618              | 2.400151                                                         |
| 32295 | 1.600743              | 2.400155                                                         |
| 32297 | 1.000031              | 2.400160                                                         |
| 32299 | 1.000031              | 2.400164                                                         |
| 32301 | 1.498777              | 2.400169                                                         |
| 32303 | 1.000031              | 2.400173                                                         |
| 32305 | 1.497725              | 2.400178                                                         |
| 32307 | 1.482032              | 2.400182                                                         |
| 32309 | 1.000031              | 2.400187                                                         |

| $n$   | $\frac{\sigma(n)}{n}$ | $\frac{e^\gamma}{2} \log \log n + \frac{0.73\dots}{\log \log n}$ |
|-------|-----------------------|------------------------------------------------------------------|
| 32311 | 1.015134              | 2.400191                                                         |
| 32313 | 1.333457              | 2.400196                                                         |
| 32315 | 1.256630              | 2.400200                                                         |
| 32317 | 1.059381              | 2.400205                                                         |
| 32319 | 1.802036              | 2.400209                                                         |
| 32321 | 1.000031              | 2.400214                                                         |
| 32323 | 1.000031              | 2.400218                                                         |
| 32325 | 1.657169              | 2.400223                                                         |
| 32327 | 1.000031              | 2.400227                                                         |
| 32329 | 1.091280              | 2.400232                                                         |
| 32331 | 1.437630              | 2.400236                                                         |
| 32333 | 1.187641              | 2.400241                                                         |
| 32335 | 1.246946              | 2.400246                                                         |
| 32337 | 1.444846              | 2.400250                                                         |
| 32339 | 1.015987              | 2.400254                                                         |
| 32341 | 1.000031              | 2.400259                                                         |
| 32343 | 1.333457              | 2.400263                                                         |
| 32345 | 1.200186              | 2.400268                                                         |
| 32347 | 1.143104              | 2.400272                                                         |
| 32349 | 1.371047              | 2.400277                                                         |
| 32351 | 1.161757              | 2.400281                                                         |
| 32353 | 1.000031              | 2.400286                                                         |
| 32355 | 1.735744              | 2.400290                                                         |
| 32357 | 1.142257              | 2.400295                                                         |
| 32359 | 1.000031              | 2.400299                                                         |
| 32361 | 1.613794              | 2.400304                                                         |
| 32363 | 1.000031              | 2.400308                                                         |
| 32365 | 1.200185              | 2.400313                                                         |
| 32367 | 1.333457              | 2.400317                                                         |
| 32369 | 1.000031              | 2.400322                                                         |
| 32371 | 1.000031              | 2.400326                                                         |
| 32373 | 1.630989              | 2.400331                                                         |
| 32375 | 1.464834              | 2.400335                                                         |
| 32377 | 1.000031              | 2.400340                                                         |
| 32379 | 1.369777              | 2.400344                                                         |
| 32381 | 1.000031              | 2.400349                                                         |
| 32383 | 1.120588              | 2.400353                                                         |
| 32385 | 1.707457              | 2.400358                                                         |
| 32387 | 1.011517              | 2.400362                                                         |
| 32389 | 1.165025              | 2.400367                                                         |
| 32391 | 1.493007              | 2.400371                                                         |
| 32393 | 1.035409              | 2.400376                                                         |
| 32395 | 1.422442              | 2.400380                                                         |
| 32397 | 1.333457              | 2.400385                                                         |

| $n$   | $\frac{\sigma(n)}{n}$ | $\frac{e^\gamma}{2} \log \log n + \frac{0.73...}{\log \log n}$ |
|-------|-----------------------|----------------------------------------------------------------|
| 32399 | 1.011142              | 2.400389                                                       |
| 32401 | 1.000031              | 2.400394                                                       |
| 32403 | 1.524797              | 2.400398                                                       |
| 32405 | 1.200185              | 2.400403                                                       |
| 32407 | 1.044219              | 2.400407                                                       |
| 32409 | 1.561171              | 2.400412                                                       |
| 32411 | 1.000031              | 2.400416                                                       |
| 32413 | 1.000031              | 2.400421                                                       |
| 32415 | 1.600740              | 2.400425                                                       |
| 32417 | 1.249715              | 2.400430                                                       |
| 32419 | 1.059379              | 2.400434                                                       |
| 32421 | 1.359119              | 2.400439                                                       |
| 32423 | 1.000031              | 2.400443                                                       |
| 32425 | 1.240956              | 2.400448                                                       |
| 32427 | 1.482715              | 2.400452                                                       |
| 32429 | 1.000031              | 2.400457                                                       |
| 32431 | 1.181092              | 2.400461                                                       |
| 32433 | 1.405975              | 2.400466                                                       |
| 32435 | 1.294897              | 2.400470                                                       |
| 32437 | 1.011191              | 2.400475                                                       |
| 32439 | 1.456025              | 2.400479                                                       |
| 32441 | 1.000031              | 2.400484                                                       |
| 32443 | 1.000031              | 2.400488                                                       |
| 32445 | 2.000185              | 2.400493                                                       |
| 32447 | 1.016304              | 2.400497                                                       |
| 32449 | 1.028198              | 2.400502                                                       |
| 32451 | 1.383008              | 2.400506                                                       |
| 32453 | 1.118171              | 2.400510                                                       |
| 32455 | 1.200185              | 2.400515                                                       |
| 32457 | 1.380288              | 2.400519                                                       |
| 32459 | 1.143104              | 2.400524                                                       |
| 32461 | 1.180001              | 2.400528                                                       |
| 32463 | 1.444845              | 2.400533                                                       |
| 32465 | 1.236039              | 2.400537                                                       |
| 32467 | 1.000031              | 2.400542                                                       |
| 32469 | 1.360067              | 2.400546                                                       |
| 32471 | 1.053248              | 2.400551                                                       |
| 32473 | 1.143104              | 2.400555                                                       |
| 32475 | 1.657152              | 2.400560                                                       |
| 32477 | 1.022755              | 2.400564                                                       |
| 32479 | 1.000031              | 2.400569                                                       |
| 32481 | 1.497552              | 2.400573                                                       |
| 32483 | 1.091279              | 2.400578                                                       |
| 32485 | 1.230106              | 2.400582                                                       |

| $n$   | $\frac{\sigma(n)}{n}$ | $\frac{e^\gamma}{2} \log \log n + \frac{0.73...}{\log \log n}$ |
|-------|-----------------------|----------------------------------------------------------------|
| 32487 | 1.768584              | 2.400587                                                       |
| 32489 | 1.020530              | 2.400591                                                       |
| 32491 | 1.000031              | 2.400596                                                       |
| 32493 | 1.333456              | 2.400600                                                       |
| 32495 | 1.230466              | 2.400605                                                       |
| 32497 | 1.000031              | 2.400609                                                       |
| 32499 | 1.516847              | 2.400613                                                       |
| 32501 | 1.143103              | 2.400618                                                       |
| 32503 | 1.000031              | 2.400622                                                       |
| 32505 | 1.754315              | 2.400627                                                       |
| 32507 | 1.000031              | 2.400631                                                       |
| 32509 | 1.107386              | 2.400636                                                       |
| 32511 | 1.333456              | 2.400640                                                       |
| 32513 | 1.121275              | 2.400645                                                       |
| 32515 | 1.372905              | 2.400649                                                       |
| 32517 | 1.444844              | 2.400654                                                       |
| 32519 | 1.033242              | 2.400658                                                       |
| 32521 | 1.059377              | 2.400663                                                       |
| 32523 | 1.374043              | 2.400667                                                       |
| 32525 | 1.240953              | 2.400672                                                       |
| 32527 | 1.091278              | 2.400676                                                       |
| 32529 | 1.524793              | 2.400681                                                       |
| 32531 | 1.000031              | 2.400685                                                       |
| 32533 | 1.000031              | 2.400690                                                       |
| 32535 | 1.785154              | 2.400694                                                       |
| 32537 | 1.000031              | 2.400698                                                       |
| 32539 | 1.077353              | 2.400703                                                       |
| 32541 | 1.333456              | 2.400707                                                       |
| 32543 | 1.143103              | 2.400712                                                       |
| 32545 | 1.256599              | 2.400716                                                       |
| 32547 | 1.405967              | 2.400721                                                       |
| 32549 | 1.103260              | 2.400725                                                       |
| 32551 | 1.024608              | 2.400730                                                       |
| 32553 | 1.444844              | 2.400734                                                       |
| 32555 | 1.273906              | 2.400739                                                       |
| 32557 | 1.143103              | 2.400743                                                       |
| 32559 | 1.333456              | 2.400748                                                       |
| 32561 | 1.000031              | 2.400752                                                       |
| 32563 | 1.000031              | 2.400757                                                       |
| 32565 | 1.733395              | 2.400761                                                       |
| 32567 | 1.035404              | 2.400765                                                       |
| 32569 | 1.000031              | 2.400770                                                       |
| 32571 | 1.839182              | 2.400774                                                       |
| 32573 | 1.000031              | 2.400779                                                       |



| $n$   | $\frac{\sigma(n)}{n}$ | $\frac{e^\gamma}{2} \log \log n + \frac{0.73...}{\log \log n}$ |
|-------|-----------------------|----------------------------------------------------------------|
| 32575 | 1.240952              | 2.400783                                                       |
| 32577 | 1.333456              | 2.400788                                                       |
| 32579 | 1.000031              | 2.400792                                                       |
| 32581 | 1.033240              | 2.400797                                                       |
| 32583 | 1.333456              | 2.400801                                                       |
| 32585 | 1.473070              | 2.400806                                                       |
| 32587 | 1.000031              | 2.400810                                                       |
| 32589 | 1.590721              | 2.400815                                                       |
| 32591 | 1.134055              | 2.400819                                                       |
| 32593 | 1.091277              | 2.400823                                                       |
| 32595 | 1.669949              | 2.400828                                                       |
| 32597 | 1.028193              | 2.400832                                                       |
| 32599 | 1.143103              | 2.400837                                                       |
| 32601 | 1.333456              | 2.400841                                                       |
| 32603 | 1.000031              | 2.400846                                                       |
| 32605 | 1.200184              | 2.400850                                                       |
| 32607 | 1.444843              | 2.400855                                                       |
| 32609 | 1.000031              | 2.400859                                                       |
| 32611 | 1.000031              | 2.400864                                                       |
| 32613 | 1.524791              | 2.400868                                                       |
| 32615 | 1.311298              | 2.400873                                                       |
| 32617 | 1.088451              | 2.400877                                                       |
| 32619 | 1.359698              | 2.400881                                                       |
| 32621 | 1.000031              | 2.400886                                                       |
| 32623 | 1.125586              | 2.400890                                                       |
| 32625 | 1.864828              | 2.400895                                                       |
| 32627 | 1.176939              | 2.400899                                                       |
| 32629 | 1.017009              | 2.400904                                                       |
| 32631 | 1.360669              | 2.400908                                                       |
| 32633 | 1.000031              | 2.400913                                                       |
| 32635 | 1.231071              | 2.400917                                                       |
| 32637 | 1.553084              | 2.400922                                                       |
| 32639 | 1.011796              | 2.400926                                                       |
| 32641 | 1.143102              | 2.400930                                                       |
| 32643 | 1.660632              | 2.400935                                                       |
| 32645 | 1.200184              | 2.400939                                                       |
| 32647 | 1.000031              | 2.400944                                                       |
| 32649 | 1.333456              | 2.400948                                                       |
| 32651 | 1.012894              | 2.400953                                                       |
| 32653 | 1.000031              | 2.400957                                                       |
| 32655 | 1.834451              | 2.400962                                                       |
| 32657 | 1.071684              | 2.400966                                                       |
| 32659 | 1.091277              | 2.400971                                                       |
| 32661 | 1.528428              | 2.400975                                                       |

| $n$   | $\frac{\sigma(n)}{n}$ | $\frac{e^\gamma}{2} \log \log n + \frac{0.73...}{\log \log n}$ |
|-------|-----------------------|----------------------------------------------------------------|
| 32663 | 1.013991              | 2.400979                                                       |
| 32665 | 1.234349              | 2.400984                                                       |
| 32667 | 1.333456              | 2.400988                                                       |
| 32669 | 1.234198              | 2.400993                                                       |
| 32671 | 1.028190              | 2.400997                                                       |
| 32673 | 1.333456              | 2.401002                                                       |
| 32675 | 1.240949              | 2.401006                                                       |
| 32677 | 1.025676              | 2.401011                                                       |
| 32679 | 1.444842              | 2.401015                                                       |
| 32681 | 1.091276              | 2.401019                                                       |
| 32683 | 1.255699              | 2.401024                                                       |
| 32685 | 1.600734              | 2.401028                                                       |
| 32687 | 1.000031              | 2.401033                                                       |
| 32689 | 1.013307              | 2.401037                                                       |
| 32691 | 1.413967              | 2.401042                                                       |
| 32693 | 1.000031              | 2.401046                                                       |
| 32695 | 1.294877              | 2.401051                                                       |
| 32697 | 1.702909              | 2.401055                                                       |
| 32699 | 1.053243              | 2.401060                                                       |
| 32701 | 1.020519              | 2.401064                                                       |
| 32703 | 1.456013              | 2.401068                                                       |
| 32705 | 1.244580              | 2.401073                                                       |
| 32707 | 1.000031              | 2.401077                                                       |
| 32709 | 1.333456              | 2.401082                                                       |
| 32711 | 1.143102              | 2.401086                                                       |
| 32713 | 1.000031              | 2.401091                                                       |
| 32715 | 1.735718              | 2.401095                                                       |
| 32717 | 1.000031              | 2.401100                                                       |
| 32719 | 1.000031              | 2.401104                                                       |
| 32721 | 1.437609              | 2.401108                                                       |
| 32723 | 1.024600              | 2.401113                                                       |
| 32725 | 1.636914              | 2.401117                                                       |
| 32727 | 1.333456              | 2.401122                                                       |
| 32729 | 1.044212              | 2.401126                                                       |
| 32731 | 1.016284              | 2.401131                                                       |
| 32733 | 1.444842              | 2.401135                                                       |
| 32735 | 1.200183              | 2.401139                                                       |
| 32737 | 1.053243              | 2.401144                                                       |
| 32739 | 1.524787              | 2.401148                                                       |
| 32741 | 1.035399              | 2.401153                                                       |
| 32743 | 1.011514              | 2.401157                                                       |
| 32745 | 1.671095              | 2.401162                                                       |
| 32747 | 1.179955              | 2.401166                                                       |
| 32749 | 1.000031              | 2.401171                                                       |

| $n$   | $\frac{\sigma(n)}{n}$ | $\frac{e^\gamma}{2} \log \log n + \frac{0.73...}{\log \log n}$ |
|-------|-----------------------|----------------------------------------------------------------|
| 32751 | 1.482703              | 2.401175                                                       |
| 32753 | 1.143101              | 2.401179                                                       |
| 32755 | 1.200183              | 2.401184                                                       |
| 32757 | 1.362762              | 2.401188                                                       |
| 32759 | 1.107726              | 2.401193                                                       |
| 32761 | 1.005555              | 2.401197                                                       |
| 32763 | 1.361536              | 2.401202                                                       |
| 32765 | 1.200183              | 2.401206                                                       |
| 32767 | 1.187536              | 2.401211                                                       |
| 32769 | 1.580518              | 2.401215                                                       |
| 32771 | 1.000031              | 2.401219                                                       |
| 32773 | 1.077350              | 2.401224                                                       |
| 32775 | 1.816018              | 2.401228                                                       |
| 32777 | 1.015956              | 2.401233                                                       |
| 32779 | 1.000031              | 2.401237                                                       |
| 32781 | 1.557976              | 2.401242                                                       |
| 32783 | 1.000031              | 2.401246                                                       |
| 32785 | 1.229831              | 2.401250                                                       |
| 32787 | 1.444841              | 2.401255                                                       |
| 32789 | 1.000030              | 2.401259                                                       |
| 32791 | 1.103230              | 2.401264                                                       |
| 32793 | 1.413960              | 2.401268                                                       |
| 32795 | 1.372892              | 2.401273                                                       |
| 32797 | 1.000030              | 2.401277                                                       |
| 32799 | 1.487119              | 2.401281                                                       |
| 32801 | 1.000030              | 2.401286                                                       |
| 32803 | 1.000030              | 2.401290                                                       |
| 32805 | 1.799909              | 2.401295                                                       |
| 32807 | 1.020514              | 2.401299                                                       |
| 32809 | 1.180164              | 2.401304                                                       |
| 32811 | 1.333455              | 2.401308                                                       |
| 32813 | 1.155640              | 2.401312                                                       |
| 32815 | 1.200183              | 2.401317                                                       |
| 32817 | 1.333455              | 2.401321                                                       |
| 32819 | 1.028185              | 2.401326                                                       |
| 32821 | 1.044210              | 2.401330                                                       |
| 32823 | 1.653962              | 2.401335                                                       |
| 32825 | 1.348606              | 2.401339                                                       |
| 32827 | 1.059372              | 2.401343                                                       |
| 32829 | 1.380243              | 2.401348                                                       |
| 32831 | 1.000030              | 2.401352                                                       |
| 32833 | 1.000030              | 2.401357                                                       |
| 32835 | 1.754226              | 2.401361                                                       |
| 32837 | 1.143101              | 2.401366                                                       |

| $n$   | $\frac{\sigma(n)}{n}$ | $\frac{e^\gamma}{2} \log \log n + \frac{0.73...}{\log \log n}$ |
|-------|-----------------------|----------------------------------------------------------------|
| 32839 | 1.000030              | 2.401370                                                       |
| 32841 | 1.496300              | 2.401374                                                       |
| 32843 | 1.000030              | 2.401379                                                       |
| 32845 | 1.200183              | 2.401383                                                       |
| 32847 | 1.333455              | 2.401388                                                       |
| 32849 | 1.012634              | 2.401392                                                       |
| 32851 | 1.298956              | 2.401397                                                       |
| 32853 | 1.367546              | 2.401401                                                       |
| 32855 | 1.200183              | 2.401405                                                       |
| 32857 | 1.139483              | 2.401410                                                       |
| 32859 | 1.482699              | 2.401414                                                       |
| 32861 | 1.059371              | 2.401419                                                       |
| 32863 | 1.018775              | 2.401423                                                       |
| 32865 | 1.834414              | 2.401428                                                       |
| 32867 | 1.044208              | 2.401432                                                       |
| 32869 | 1.000030              | 2.401436                                                       |
| 32871 | 1.333455              | 2.401441                                                       |
| 32873 | 1.016275              | 2.401445                                                       |
| 32875 | 1.252745              | 2.401450                                                       |
| 32877 | 1.561091              | 2.401454                                                       |
| 32879 | 1.289820              | 2.401458                                                       |
| 32881 | 1.011648              | 2.401463                                                       |
| 32883 | 1.359000              | 2.401467                                                       |
| 32885 | 1.200182              | 2.401472                                                       |
| 32887 | 1.000030              | 2.401476                                                       |
| 32889 | 1.405941              | 2.401481                                                       |
| 32891 | 1.033231              | 2.401485                                                       |
| 32893 | 1.182987              | 2.401489                                                       |
| 32895 | 1.877975              | 2.401494                                                       |
| 32897 | 1.016992              | 2.401498                                                       |
| 32899 | 1.011095              | 2.401503                                                       |
| 32901 | 1.456004              | 2.401507                                                       |
| 32903 | 1.077349              | 2.401511                                                       |
| 32905 | 1.200182              | 2.401516                                                       |
| 32907 | 1.524782              | 2.401520                                                       |
| 32909 | 1.000030              | 2.401525                                                       |
| 32911 | 1.000030              | 2.401529                                                       |
| 32913 | 1.575062              | 2.401534                                                       |
| 32915 | 1.246848              | 2.401538                                                       |
| 32917 | 1.000030              | 2.401542                                                       |
| 32919 | 1.333455              | 2.401547                                                       |
| 32921 | 1.143100              | 2.401551                                                       |
| 32923 | 1.132825              | 2.401556                                                       |
| 32925 | 1.657099              | 2.401560                                                       |

| $n$   | $\frac{\sigma(n)}{n}$ | $\frac{e^\gamma}{2} \log \log n + \frac{0.73...}{\log \log n}$ |
|-------|-----------------------|----------------------------------------------------------------|
| 32927 | 1.053239              | 2.401564                                                       |
| 32929 | 1.147924              | 2.401569                                                       |
| 32931 | 1.444839              | 2.401573                                                       |
| 32933 | 1.000030              | 2.401578                                                       |
| 32935 | 1.372886              | 2.401582                                                       |
| 32937 | 1.333455              | 2.401586                                                       |
| 32939 | 1.000030              | 2.401591                                                       |
| 32941 | 1.000030              | 2.401595                                                       |
| 32943 | 1.359925              | 2.401600                                                       |
| 32945 | 1.311276              | 2.401604                                                       |
| 32947 | 1.022733              | 2.401609                                                       |
| 32949 | 1.653950              | 2.401613                                                       |
| 32951 | 1.014597              | 2.401617                                                       |
| 32953 | 1.033229              | 2.401622                                                       |
| 32955 | 1.733273              | 2.401626                                                       |
| 32957 | 1.000030              | 2.401631                                                       |
| 32959 | 1.044206              | 2.401635                                                       |
| 32961 | 1.333455              | 2.401639                                                       |
| 32963 | 1.214453              | 2.401644                                                       |
| 32965 | 1.266798              | 2.401648                                                       |
| 32967 | 1.673674              | 2.401653                                                       |
| 32969 | 1.000030              | 2.401657                                                       |
| 32971 | 1.000030              | 2.401661                                                       |
| 32973 | 1.382950              | 2.401666                                                       |
| 32975 | 1.240940              | 2.401670                                                       |
| 32977 | 1.164994              | 2.401675                                                       |
| 32979 | 1.333455              | 2.401679                                                       |
| 32981 | 1.120645              | 2.401683                                                       |
| 32983 | 1.000030              | 2.401688                                                       |
| 32985 | 1.735698              | 2.401692                                                       |
| 32987 | 1.000030              | 2.401697                                                       |
| 32989 | 1.091273              | 2.401701                                                       |
| 32991 | 1.524779              | 2.401705                                                       |
| 32993 | 1.000030              | 2.401710                                                       |
| 32995 | 1.200182              | 2.401714                                                       |
| 32997 | 1.413947              | 2.401719                                                       |
| 32999 | 1.000030              | 2.401723                                                       |
| 33001 | 1.018272              | 2.401727                                                       |
| 33003 | 1.528346              | 2.401732                                                       |
| 33005 | 1.465960              | 2.401736                                                       |
| 33007 | 1.077347              | 2.401741                                                       |
| 33009 | 1.333455              | 2.401745                                                       |
| 33011 | 1.091273              | 2.401749                                                       |
| 33013 | 1.000030              | 2.401754                                                       |

| $n$   | $\frac{\sigma(n)}{n}$ | $\frac{e^\gamma}{2} \log \log n + \frac{0.73...}{\log \log n}$ |
|-------|-----------------------|----------------------------------------------------------------|
| 33015 | 1.674875              | 2.401758                                                       |
| 33017 | 1.011479              | 2.401763                                                       |
| 33019 | 1.177504              | 2.401767                                                       |
| 33021 | 1.482693              | 2.401771                                                       |
| 33023 | 1.000030              | 2.401776                                                       |
| 33025 | 1.240939              | 2.401780                                                       |
| 33027 | 1.358888              | 2.401785                                                       |
| 33029 | 1.000030              | 2.401789                                                       |
| 33031 | 1.111683              | 2.401793                                                       |
| 33033 | 1.803772              | 2.401798                                                       |
| 33035 | 1.200182              | 2.401802                                                       |
| 33037 | 1.000030              | 2.401807                                                       |
| 33039 | 1.444838              | 2.401811                                                       |
| 33041 | 1.104083              | 2.401815                                                       |
| 33043 | 1.011046              | 2.401820                                                       |
| 33045 | 1.600726              | 2.401824                                                       |
| 33047 | 1.143099              | 2.401829                                                       |
| 33049 | 1.000030              | 2.401833                                                       |
| 33051 | 1.394209              | 2.401837                                                       |
| 33053 | 1.000030              | 2.401842                                                       |
| 33055 | 1.311269              | 2.401846                                                       |
| 33057 | 1.444838              | 2.401851                                                       |
| 33059 | 1.077347              | 2.401855                                                       |
| 33061 | 1.143099              | 2.401859                                                       |
| 33063 | 1.358860              | 2.401864                                                       |
| 33065 | 1.273855              | 2.401868                                                       |
| 33067 | 1.024586              | 2.401873                                                       |
| 33069 | 1.360549              | 2.401877                                                       |
| 33071 | 1.000030              | 2.401881                                                       |
| 33073 | 1.000030              | 2.401886                                                       |
| 33075 | 2.136961              | 2.401890                                                       |
| 33077 | 1.137709              | 2.401895                                                       |
| 33079 | 1.053236              | 2.401899                                                       |
| 33081 | 1.333454              | 2.401903                                                       |
| 33083 | 1.000030              | 2.401908                                                       |
| 33085 | 1.294847              | 2.401912                                                       |
| 33087 | 1.370931              | 2.401916                                                       |
| 33089 | 1.189519              | 2.401921                                                       |
| 33091 | 1.000030              | 2.401925                                                       |
| 33093 | 1.444837              | 2.401930                                                       |
| 33095 | 1.200181              | 2.401934                                                       |
| 33097 | 1.044203              | 2.401938                                                       |
| 33099 | 1.566210              | 2.401943                                                       |
| 33101 | 1.015075              | 2.401947                                                       |

| $n$   | $\frac{\sigma(n)}{n}$ | $\frac{e^\gamma}{2} \log \log n + \frac{0.73...}{\log \log n}$ |
|-------|-----------------------|----------------------------------------------------------------|
| 33103 | 1.143099              | 2.401952                                                       |
| 33105 | 1.600725              | 2.401956                                                       |
| 33107 | 1.000030              | 2.401960                                                       |
| 33109 | 1.012293              | 2.401965                                                       |
| 33111 | 1.561052              | 2.401969                                                       |
| 33113 | 1.000030              | 2.401974                                                       |
| 33115 | 1.239318              | 2.401978                                                       |
| 33117 | 1.623335              | 2.401982                                                       |
| 33119 | 1.000030              | 2.401987                                                       |
| 33121 | 1.091271              | 2.401991                                                       |
| 33123 | 1.362679              | 2.401995                                                       |
| 33125 | 1.273177              | 2.402000                                                       |
| 33127 | 1.011139              | 2.402004                                                       |
| 33129 | 1.497480              | 2.402009                                                       |
| 33131 | 1.143099              | 2.402013                                                       |
| 33133 | 1.059367              | 2.402017                                                       |
| 33135 | 1.634767              | 2.402022                                                       |
| 33137 | 1.077346              | 2.402026                                                       |
| 33139 | 1.033224              | 2.402031                                                       |
| 33141 | 1.333454              | 2.402035                                                       |
| 33143 | 1.147030              | 2.402039                                                       |
| 33145 | 1.372877              | 2.402044                                                       |
| 33147 | 1.506019              | 2.402048                                                       |
| 33149 | 1.000030              | 2.402052                                                       |
| 33151 | 1.000030              | 2.402057                                                       |
| 33153 | 1.369650              | 2.402061                                                       |
| 33155 | 1.266777              | 2.402066                                                       |
| 33157 | 1.016256              | 2.402070                                                       |
| 33159 | 1.524775              | 2.402074                                                       |
| 33161 | 1.000030              | 2.402079                                                       |
| 33163 | 1.077345              | 2.402083                                                       |
| 33165 | 1.919132              | 2.402087                                                       |
| 33167 | 1.059366              | 2.402092                                                       |
| 33169 | 1.025656              | 2.402096                                                       |
| 33171 | 1.333454              | 2.402101                                                       |
| 33173 | 1.164984              | 2.402105                                                       |
| 33175 | 1.240934              | 2.402109                                                       |
| 33177 | 1.333454              | 2.402114                                                       |
| 33179 | 1.000030              | 2.402118                                                       |
| 33181 | 1.000030              | 2.402122                                                       |
| 33183 | 1.482687              | 2.402127                                                       |
| 33185 | 1.200181              | 2.402131                                                       |
| 33187 | 1.249646              | 2.402136                                                       |
| 33189 | 1.538823              | 2.402140                                                       |

| $n$   | $\frac{\sigma(n)}{n}$ | $\frac{e^\gamma}{2} \log \log n + \frac{0.73...}{\log \log n}$ |
|-------|-----------------------|----------------------------------------------------------------|
| 33191 | 1.000030              | 2.402144                                                       |
| 33193 | 1.053234              | 2.402149                                                       |
| 33195 | 1.600723              | 2.402153                                                       |
| 33197 | 1.013947              | 2.402157                                                       |
| 33199 | 1.000030              | 2.402162                                                       |
| 33201 | 1.804283              | 2.402166                                                       |
| 33203 | 1.000030              | 2.402171                                                       |
| 33205 | 1.246800              | 2.402175                                                       |
| 33207 | 1.333454              | 2.402179                                                       |
| 33209 | 1.091270              | 2.402184                                                       |
| 33211 | 1.000030              | 2.402188                                                       |
| 33213 | 1.333454              | 2.402192                                                       |
| 33215 | 1.497155              | 2.402197                                                       |
| 33217 | 1.018755              | 2.402201                                                       |
| 33219 | 1.444836              | 2.402206                                                       |
| 33221 | 1.011408              | 2.402210                                                       |
| 33223 | 1.000030              | 2.402214                                                       |
| 33225 | 1.657065              | 2.402219                                                       |
| 33227 | 1.011226              | 2.402223                                                       |
| 33229 | 1.178729              | 2.402227                                                       |
| 33231 | 1.559989              | 2.402232                                                       |
| 33233 | 1.011043              | 2.402236                                                       |
| 33235 | 1.330164              | 2.402241                                                       |
| 33237 | 1.482685              | 2.402245                                                       |
| 33239 | 1.024580              | 2.402249                                                       |
| 33241 | 1.077344              | 2.402254                                                       |
| 33243 | 1.524772              | 2.402258                                                       |
| 33245 | 1.230862              | 2.402262                                                       |
| 33247 | 1.000030              | 2.402267                                                       |
| 33249 | 1.333454              | 2.402271                                                       |
| 33251 | 1.025653              | 2.402275                                                       |
| 33253 | 1.091270              | 2.402280                                                       |
| 33255 | 1.735679              | 2.402284                                                       |
| 33257 | 1.143098              | 2.402289                                                       |
| 33259 | 1.015064              | 2.402293                                                       |
| 33261 | 1.333454              | 2.402297                                                       |
| 33263 | 1.096714              | 2.402302                                                       |
| 33265 | 1.200180              | 2.402306                                                       |
| 33267 | 1.437581              | 2.402310                                                       |
| 33269 | 1.125372              | 2.402315                                                       |
| 33271 | 1.178203              | 2.402319                                                       |
| 33273 | 1.444835              | 2.402323                                                       |
| 33275 | 1.363907              | 2.402328                                                       |
| 33277 | 1.012591              | 2.402332                                                       |



| $n$   | $\frac{\sigma(n)}{n}$ | $\frac{e^\gamma}{2} \log \log n + \frac{0.73...}{\log \log n}$ |
|-------|-----------------------|----------------------------------------------------------------|
| 33279 | 1.333454              | 2.402337                                                       |
| 33281 | 1.044199              | 2.402341                                                       |
| 33283 | 1.014572              | 2.402345                                                       |
| 33285 | 1.834340              | 2.402350                                                       |
| 33287 | 1.000030              | 2.402354                                                       |
| 33289 | 1.000030              | 2.402358                                                       |
| 33291 | 1.508876              | 2.402363                                                       |
| 33293 | 1.088337              | 2.402367                                                       |
| 33295 | 1.200180              | 2.402371                                                       |
| 33297 | 1.455987              | 2.402376                                                       |
| 33299 | 1.176252              | 2.402380                                                       |
| 33301 | 1.000030              | 2.402385                                                       |
| 33303 | 1.413927              | 2.402389                                                       |
| 33305 | 1.200180              | 2.402393                                                       |
| 33307 | 1.053232              | 2.402398                                                       |
| 33309 | 1.444835              | 2.402402                                                       |
| 33311 | 1.000030              | 2.402406                                                       |
| 33313 | 1.143097              | 2.402411                                                       |
| 33315 | 1.600720              | 2.402415                                                       |
| 33317 | 1.000030              | 2.402419                                                       |
| 33319 | 1.179867              | 2.402424                                                       |
| 33321 | 1.382912              | 2.402428                                                       |
| 33323 | 1.022717              | 2.402432                                                       |
| 33325 | 1.309767              | 2.402437                                                       |
| 33327 | 1.725688              | 2.402441                                                       |
| 33329 | 1.000030              | 2.402446                                                       |
| 33331 | 1.000030              | 2.402450                                                       |
| 33333 | 1.370894              | 2.402454                                                       |
| 33335 | 1.231138              | 2.402459                                                       |
| 33337 | 1.107958              | 2.402463                                                       |
| 33339 | 1.333453              | 2.402467                                                       |
| 33341 | 1.249633              | 2.402472                                                       |
| 33343 | 1.000030              | 2.402476                                                       |
| 33345 | 2.015295              | 2.402480                                                       |
| 33347 | 1.000030              | 2.402485                                                       |
| 33349 | 1.000030              | 2.402489                                                       |
| 33351 | 1.333453              | 2.402493                                                       |
| 33353 | 1.000030              | 2.402498                                                       |
| 33355 | 1.372868              | 2.402502                                                       |
| 33357 | 1.333453              | 2.402506                                                       |
| 33359 | 1.000030              | 2.402511                                                       |
| 33361 | 1.015917              | 2.402515                                                       |
| 33363 | 1.580433              | 2.402520                                                       |
| 33365 | 1.200180              | 2.402524                                                       |

| $n$   | $\frac{\sigma(n)}{n}$ | $\frac{e^\gamma}{2} \log \log n + \frac{0.73...}{\log \log n}$ |
|-------|-----------------------|----------------------------------------------------------------|
| 33367 | 1.018252              | 2.402528                                                       |
| 33369 | 1.557853              | 2.402533                                                       |
| 33371 | 1.147823              | 2.402537                                                       |
| 33373 | 1.044197              | 2.402541                                                       |
| 33375 | 1.682697              | 2.402546                                                       |
| 33377 | 1.000030              | 2.402550                                                       |
| 33379 | 1.035382              | 2.402554                                                       |
| 33381 | 1.444834              | 2.402559                                                       |
| 33383 | 1.207800              | 2.402563                                                       |
| 33385 | 1.311248              | 2.402567                                                       |
| 33387 | 1.380178              | 2.402572                                                       |
| 33389 | 1.010992              | 2.402576                                                       |
| 33391 | 1.000030              | 2.402580                                                       |
| 33393 | 1.333453              | 2.402585                                                       |
| 33395 | 1.200180              | 2.402589                                                       |
| 33397 | 1.234123              | 2.402593                                                       |
| 33399 | 1.482679              | 2.402598                                                       |
| 33401 | 1.011706              | 2.402602                                                       |
| 33403 | 1.000030              | 2.402606                                                       |
| 33405 | 1.707050              | 2.402611                                                       |
| 33407 | 1.091268              | 2.402615                                                       |
| 33409 | 1.000030              | 2.402619                                                       |
| 33411 | 1.601389              | 2.402624                                                       |
| 33413 | 1.000030              | 2.402628                                                       |
| 33415 | 1.236810              | 2.402633                                                       |
| 33417 | 1.493850              | 2.402637                                                       |
| 33419 | 1.044196              | 2.402641                                                       |
| 33421 | 1.053230              | 2.402646                                                       |
| 33423 | 1.437573              | 2.402650                                                       |
| 33425 | 1.424562              | 2.402654                                                       |
| 33427 | 1.000030              | 2.402659                                                       |
| 33429 | 1.455981              | 2.402663                                                       |
| 33431 | 1.012952              | 2.402667                                                       |
| 33433 | 1.016959              | 2.402672                                                       |
| 33435 | 1.735666              | 2.402676                                                       |
| 33437 | 1.035380              | 2.402680                                                       |
| 33439 | 1.214390              | 2.402685                                                       |
| 33441 | 1.360725              | 2.402689                                                       |
| 33443 | 1.020483              | 2.402693                                                       |
| 33445 | 1.200179              | 2.402698                                                       |
| 33447 | 1.333453              | 2.402702                                                       |
| 33449 | 1.125056              | 2.402706                                                       |
| 33451 | 1.091268              | 2.402711                                                       |
| 33453 | 1.736167              | 2.402715                                                       |

| $n$   | $\frac{\sigma(n)}{n}$ | $\frac{e^\gamma}{2} \log \log n + \frac{0.73...}{\log \log n}$ |
|-------|-----------------------|----------------------------------------------------------------|
| 33455 | 1.200179              | 2.402719                                                       |
| 33457 | 1.000030              | 2.402724                                                       |
| 33459 | 1.405900              | 2.402728                                                       |
| 33461 | 1.000030              | 2.402732                                                       |
| 33463 | 1.012462              | 2.402737                                                       |
| 33465 | 1.686777              | 2.402741                                                       |
| 33467 | 1.164968              | 2.402745                                                       |
| 33469 | 1.000030              | 2.402750                                                       |
| 33471 | 1.444833              | 2.402754                                                       |
| 33473 | 1.161533              | 2.402758                                                       |
| 33475 | 1.348350              | 2.402763                                                       |
| 33477 | 1.333453              | 2.402767                                                       |
| 33479 | 1.000030              | 2.402771                                                       |
| 33481 | 1.143096              | 2.402776                                                       |
| 33483 | 1.333453              | 2.402780                                                       |
| 33485 | 1.239241              | 2.402784                                                       |
| 33487 | 1.000030              | 2.402789                                                       |
| 33489 | 1.468512              | 2.402793                                                       |
| 33491 | 1.012571              | 2.402797                                                       |
| 33493 | 1.000030              | 2.402802                                                       |
| 33495 | 2.063592              | 2.402806                                                       |
| 33497 | 1.103382              | 2.402810                                                       |
| 33499 | 1.011373              | 2.402815                                                       |
| 33501 | 1.437569              | 2.402819                                                       |
| 33503 | 1.000030              | 2.402823                                                       |
| 33505 | 1.200179              | 2.402828                                                       |
| 33507 | 1.590115              | 2.402832                                                       |
| 33509 | 1.143096              | 2.402836                                                       |
| 33511 | 1.100057              | 2.402841                                                       |
| 33513 | 1.333453              | 2.402845                                                       |
| 33515 | 1.200179              | 2.402849                                                       |
| 33517 | 1.103142              | 2.402854                                                       |
| 33519 | 1.333453              | 2.402858                                                       |
| 33521 | 1.000030              | 2.402862                                                       |
| 33523 | 1.143096              | 2.402867                                                       |
| 33525 | 1.803132              | 2.402871                                                       |
| 33527 | 1.077341              | 2.402875                                                       |
| 33529 | 1.000030              | 2.402880                                                       |
| 33531 | 1.333453              | 2.402884                                                       |
| 33533 | 1.000030              | 2.402888                                                       |
| 33535 | 1.266736              | 2.402893                                                       |
| 33537 | 1.524764              | 2.402897                                                       |
| 33539 | 1.091267              | 2.402901                                                       |
| 33541 | 1.059360              | 2.402906                                                       |

| $n$   | $\frac{\sigma(n)}{n}$ | $\frac{e^\gamma}{2} \log \log n + \frac{0.73...}{\log \log n}$ |
|-------|-----------------------|----------------------------------------------------------------|
| 33543 | 1.444832              | 2.402910                                                       |
| 33545 | 1.200179              | 2.402914                                                       |
| 33547 | 1.000030              | 2.402919                                                       |
| 33549 | 1.364929              | 2.402923                                                       |
| 33551 | 1.143096              | 2.402927                                                       |
| 33553 | 1.126576              | 2.402931                                                       |
| 33555 | 1.600715              | 2.402936                                                       |
| 33557 | 1.044193              | 2.402940                                                       |
| 33559 | 1.028159              | 2.402944                                                       |
| 33561 | 1.630464              | 2.402949                                                       |
| 33563 | 1.000030              | 2.402953                                                       |
| 33565 | 1.406108              | 2.402957                                                       |
| 33567 | 1.361337              | 2.402962                                                       |
| 33569 | 1.000030              | 2.402966                                                       |
| 33571 | 1.018736              | 2.402970                                                       |
| 33573 | 1.452596              | 2.402975                                                       |
| 33575 | 1.329561              | 2.402979                                                       |
| 33577 | 1.000030              | 2.402983                                                       |
| 33579 | 1.821138              | 2.402988                                                       |
| 33581 | 1.000030              | 2.402992                                                       |
| 33583 | 1.132001              | 2.402996                                                       |
| 33585 | 1.600715              | 2.403001                                                       |
| 33587 | 1.000030              | 2.403005                                                       |
| 33589 | 1.000030              | 2.403009                                                       |
| 33591 | 1.333452              | 2.403014                                                       |
| 33593 | 1.143095              | 2.403018                                                       |
| 33595 | 1.200179              | 2.403022                                                       |
| 33597 | 1.444831              | 2.403027                                                       |
| 33599 | 1.000030              | 2.403031                                                       |
| 33601 | 1.000030              | 2.403035                                                       |
| 33603 | 1.394161              | 2.403039                                                       |
| 33605 | 1.439786              | 2.403044                                                       |
| 33607 | 1.143095              | 2.403048                                                       |
| 33609 | 1.413907              | 2.403052                                                       |
| 33611 | 1.106781              | 2.403057                                                       |
| 33613 | 1.000030              | 2.403061                                                       |
| 33615 | 1.814190              | 2.403065                                                       |
| 33617 | 1.000030              | 2.403070                                                       |
| 33619 | 1.000030              | 2.403074                                                       |
| 33621 | 1.524761              | 2.403078                                                       |
| 33623 | 1.000030              | 2.403083                                                       |
| 33625 | 1.252639              | 2.403087                                                       |
| 33627 | 1.455973              | 2.403091                                                       |
| 33629 | 1.000030              | 2.403096                                                       |

| $n$   | $\frac{\sigma(n)}{n}$ | $\frac{e^\gamma}{2} \log \log n + \frac{0.73...}{\log \log n}$ |
|-------|-----------------------|----------------------------------------------------------------|
| 33631 | 1.088282              | 2.403100                                                       |
| 33633 | 1.498171              | 2.403104                                                       |
| 33635 | 1.417095              | 2.403109                                                       |
| 33637 | 1.000030              | 2.403113                                                       |
| 33639 | 1.333452              | 2.403117                                                       |
| 33641 | 1.000030              | 2.403121                                                       |
| 33643 | 1.059359              | 2.403126                                                       |
| 33645 | 1.600713              | 2.403130                                                       |
| 33647 | 1.000030              | 2.403134                                                       |
| 33649 | 1.369431              | 2.403139                                                       |
| 33651 | 1.444831              | 2.403143                                                       |
| 33653 | 1.015898              | 2.403147                                                       |
| 33655 | 1.232269              | 2.403152                                                       |
| 33657 | 1.437561              | 2.403156                                                       |
| 33659 | 1.013221              | 2.403160                                                       |
| 33661 | 1.025638              | 2.403165                                                       |
| 33663 | 1.557793              | 2.403169                                                       |
| 33665 | 1.200178              | 2.403173                                                       |
| 33667 | 1.011554              | 2.403177                                                       |
| 33669 | 1.568208              | 2.403182                                                       |
| 33671 | 1.091265              | 2.403186                                                       |
| 33673 | 1.011137              | 2.403190                                                       |
| 33675 | 1.657016              | 2.403195                                                       |
| 33677 | 1.214360              | 2.403199                                                       |
| 33679 | 1.000030              | 2.403203                                                       |
| 33681 | 1.358629              | 2.403208                                                       |
| 33683 | 1.077339              | 2.403212                                                       |
| 33685 | 1.200178              | 2.403216                                                       |
| 33687 | 1.528186              | 2.403221                                                       |
| 33689 | 1.018730              | 2.403225                                                       |
| 33691 | 1.143095              | 2.403229                                                       |
| 33693 | 1.455970              | 2.403233                                                       |
| 33695 | 1.256448              | 2.403238                                                       |
| 33697 | 1.033208              | 2.403242                                                       |
| 33699 | 1.367400              | 2.403246                                                       |
| 33701 | 1.016943              | 2.403251                                                       |
| 33703 | 1.000030              | 2.403255                                                       |
| 33705 | 1.999466              | 2.403259                                                       |
| 33707 | 1.028154              | 2.403264                                                       |
| 33709 | 1.077338              | 2.403268                                                       |
| 33711 | 1.413901              | 2.403272                                                       |
| 33713 | 1.000030              | 2.403276                                                       |
| 33715 | 1.311226              | 2.403281                                                       |
| 33717 | 1.333452              | 2.403285                                                       |

| $n$   | $\frac{\sigma(n)}{n}$ | $\frac{e^\gamma}{2} \log \log n + \frac{0.73...}{\log \log n}$ |
|-------|-----------------------|----------------------------------------------------------------|
| 33719 | 1.143094              | 2.403289                                                       |
| 33721 | 1.000030              | 2.403294                                                       |
| 33723 | 1.482668              | 2.403298                                                       |
| 33725 | 1.323647              | 2.403302                                                       |
| 33727 | 1.035372              | 2.403307                                                       |
| 33729 | 1.333452              | 2.403311                                                       |
| 33731 | 1.013904              | 2.403315                                                       |
| 33733 | 1.176296              | 2.403319                                                       |
| 33735 | 1.733037              | 2.403324                                                       |
| 33737 | 1.091265              | 2.403328                                                       |
| 33739 | 1.000030              | 2.403332                                                       |
| 33741 | 1.516493              | 2.403337                                                       |
| 33743 | 1.025635              | 2.403341                                                       |
| 33745 | 1.273789              | 2.403345                                                       |
| 33747 | 1.524758              | 2.403350                                                       |
| 33749 | 1.000030              | 2.403354                                                       |
| 33751 | 1.000030              | 2.403358                                                       |
| 33753 | 1.333452              | 2.403362                                                       |
| 33755 | 1.235728              | 2.403367                                                       |
| 33757 | 1.000030              | 2.403371                                                       |
| 33759 | 1.638911              | 2.403375                                                       |
| 33761 | 1.276384              | 2.403380                                                       |
| 33763 | 1.053224              | 2.403384                                                       |
| 33765 | 1.600711              | 2.403388                                                       |
| 33767 | 1.000030              | 2.403393                                                       |
| 33769 | 1.000030              | 2.403397                                                       |
| 33771 | 1.333452              | 2.403401                                                       |
| 33773 | 1.000030              | 2.403405                                                       |
| 33775 | 1.424486              | 2.403410                                                       |
| 33777 | 1.508719              | 2.403414                                                       |
| 33779 | 1.059356              | 2.403418                                                       |
| 33781 | 1.133892              | 2.403423                                                       |
| 33783 | 1.333452              | 2.403427                                                       |
| 33785 | 1.246707              | 2.403431                                                       |
| 33787 | 1.133690              | 2.403435                                                       |
| 33789 | 1.524757              | 2.403440                                                       |
| 33791 | 1.000030              | 2.403444                                                       |
| 33793 | 1.022697              | 2.403448                                                       |
| 33795 | 1.735641              | 2.403453                                                       |
| 33797 | 1.000030              | 2.403457                                                       |
| 33799 | 1.015888              | 2.403461                                                       |
| 33801 | 1.405876              | 2.403465                                                       |
| 33803 | 1.249593              | 2.403470                                                       |
| 33805 | 1.200177              | 2.403474                                                       |

| $n$   | $\frac{\sigma(n)}{n}$ | $\frac{e^\gamma}{2} \log \log n + \frac{0.73...}{\log \log n}$ |
|-------|-----------------------|----------------------------------------------------------------|
| 33807 | 1.363031              | 2.403478                                                       |
| 33809 | 1.000030              | 2.403483                                                       |
| 33811 | 1.000030              | 2.403487                                                       |
| 33813 | 1.652441              | 2.403491                                                       |
| 33815 | 1.200177              | 2.403495                                                       |
| 33817 | 1.143094              | 2.403500                                                       |
| 33819 | 1.333452              | 2.403504                                                       |
| 33821 | 1.033204              | 2.403508                                                       |
| 33823 | 1.011146              | 2.403513                                                       |
| 33825 | 1.847627              | 2.403517                                                       |
| 33827 | 1.000030              | 2.403521                                                       |
| 33829 | 1.000030              | 2.403525                                                       |
| 33831 | 1.702580              | 2.403530                                                       |
| 33833 | 1.044188              | 2.403534                                                       |
| 33835 | 1.229969              | 2.403538                                                       |
| 33837 | 1.333452              | 2.403543                                                       |
| 33839 | 1.141878              | 2.403547                                                       |
| 33841 | 1.024556              | 2.403551                                                       |
| 33843 | 1.382856              | 2.403555                                                       |
| 33845 | 1.372847              | 2.403560                                                       |
| 33847 | 1.161462              | 2.403564                                                       |
| 33849 | 1.444829              | 2.403568                                                       |
| 33851 | 1.000030              | 2.403573                                                       |
| 33853 | 1.013204              | 2.403577                                                       |
| 33855 | 1.670182              | 2.403581                                                       |
| 33857 | 1.000030              | 2.403585                                                       |
| 33859 | 1.164949              | 2.403590                                                       |
| 33861 | 1.333451              | 2.403594                                                       |
| 33863 | 1.000030              | 2.403598                                                       |
| 33865 | 1.294788              | 2.403603                                                       |
| 33867 | 1.492426              | 2.403607                                                       |
| 33869 | 1.091263              | 2.403611                                                       |
| 33871 | 1.000030              | 2.403615                                                       |
| 33873 | 1.524754              | 2.403620                                                       |
| 33875 | 1.252605              | 2.403624                                                       |
| 33877 | 1.053222              | 2.403628                                                       |
| 33879 | 1.394138              | 2.403633                                                       |
| 33881 | 1.059355              | 2.403637                                                       |
| 33883 | 1.033202              | 2.403641                                                       |
| 33885 | 1.784861              | 2.403645                                                       |
| 33887 | 1.178505              | 2.403650                                                       |
| 33889 | 1.000030              | 2.403654                                                       |
| 33891 | 1.586262              | 2.403658                                                       |
| 33893 | 1.000030              | 2.403662                                                       |

| $n$   | $\frac{\sigma(n)}{n}$ | $\frac{e^\gamma}{2} \log \log n + \frac{0.73...}{\log \log n}$ |
|-------|-----------------------|----------------------------------------------------------------|
| 33895 | 1.200177              | 2.403667                                                       |
| 33897 | 1.333451              | 2.403671                                                       |
| 33899 | 1.012419              | 2.403675                                                       |
| 33901 | 1.189345              | 2.403680                                                       |
| 33903 | 1.444828              | 2.403684                                                       |
| 33905 | 1.200177              | 2.403688                                                       |
| 33907 | 1.025629              | 2.403692                                                       |
| 33909 | 1.358931              | 2.403697                                                       |
| 33911 | 1.000029              | 2.403701                                                       |
| 33913 | 1.091263              | 2.403705                                                       |
| 33915 | 2.038036              | 2.403710                                                       |
| 33917 | 1.077336              | 2.403714                                                       |
| 33919 | 1.012530              | 2.403718                                                       |
| 33921 | 1.444828              | 2.403722                                                       |
| 33923 | 1.000029              | 2.403727                                                       |
| 33925 | 1.315844              | 2.403731                                                       |
| 33927 | 1.369529              | 2.403735                                                       |
| 33929 | 1.182705              | 2.403739                                                       |
| 33931 | 1.000029              | 2.403744                                                       |
| 33933 | 1.333451              | 2.403748                                                       |
| 33935 | 1.311213              | 2.403752                                                       |
| 33937 | 1.000029              | 2.403756                                                       |
| 33939 | 1.497392              | 2.403761                                                       |
| 33941 | 1.000029              | 2.403765                                                       |
| 33943 | 1.234069              | 2.403769                                                       |
| 33945 | 1.674238              | 2.403774                                                       |
| 33947 | 1.014523              | 2.403778                                                       |
| 33949 | 1.059354              | 2.403782                                                       |
| 33951 | 1.333451              | 2.403786                                                       |
| 33953 | 1.053221              | 2.403791                                                       |
| 33955 | 1.200177              | 2.403795                                                       |
| 33957 | 1.837618              | 2.403799                                                       |
| 33959 | 1.035366              | 2.403803                                                       |
| 33961 | 1.000029              | 2.403808                                                       |
| 33963 | 1.333451              | 2.403812                                                       |
| 33965 | 1.200177              | 2.403816                                                       |
| 33967 | 1.000029              | 2.403821                                                       |
| 33969 | 1.465336              | 2.403825                                                       |
| 33971 | 1.198198              | 2.403829                                                       |
| 33973 | 1.020457              | 2.403833                                                       |
| 33975 | 1.802973              | 2.403838                                                       |
| 33977 | 1.018218              | 2.403842                                                       |
| 33979 | 1.091262              | 2.403846                                                       |
| 33981 | 1.367352              | 2.403850                                                       |



| $n$   | $\frac{\sigma(n)}{n}$ | $\frac{e^\gamma}{2} \log \log n + \frac{0.73...}{\log \log n}$ |
|-------|-----------------------|----------------------------------------------------------------|
| 33983 | 1.059353              | 2.403855                                                       |
| 33985 | 1.372841              | 2.403859                                                       |
| 33987 | 1.333451              | 2.403863                                                       |
| 33989 | 1.025626              | 2.403867                                                       |
| 33991 | 1.053220              | 2.403872                                                       |
| 33993 | 1.482658              | 2.403876                                                       |
| 33995 | 1.294779              | 2.403880                                                       |
| 33997 | 1.000029              | 2.403884                                                       |
| 33999 | 1.524751              | 2.403889                                                       |
| 34001 | 1.103085              | 2.403893                                                       |
| 34003 | 1.028145              | 2.403897                                                       |
| 34005 | 1.600706              | 2.403902                                                       |
| 34007 | 1.033199              | 2.403906                                                       |
| 34009 | 1.016202              | 2.403910                                                       |
| 34011 | 1.444827              | 2.403914                                                       |
| 34013 | 1.179784              | 2.403919                                                       |
| 34015 | 1.200176              | 2.403923                                                       |
| 34017 | 1.523944              | 2.403927                                                       |
| 34019 | 1.000029              | 2.403931                                                       |
| 34021 | 1.077335              | 2.403936                                                       |
| 34023 | 1.455956              | 2.403940                                                       |
| 34025 | 1.240911              | 2.403944                                                       |
| 34027 | 1.143092              | 2.403948                                                       |
| 34029 | 1.528108              | 2.403953                                                       |
| 34031 | 1.000029              | 2.403957                                                       |
| 34033 | 1.000029              | 2.403961                                                       |
| 34035 | 1.600705              | 2.403965                                                       |
| 34037 | 1.012898              | 2.403970                                                       |
| 34039 | 1.000029              | 2.403974                                                       |
| 34041 | 1.524750              | 2.403978                                                       |
| 34043 | 1.018712              | 2.403982                                                       |
| 34045 | 1.311206              | 2.403987                                                       |
| 34047 | 1.611889              | 2.403991                                                       |
| 34049 | 1.015008              | 2.403995                                                       |
| 34051 | 1.059352              | 2.403999                                                       |
| 34053 | 1.333451              | 2.404004                                                       |
| 34055 | 1.405961              | 2.404008                                                       |
| 34057 | 1.000029              | 2.404012                                                       |
| 34059 | 1.333451              | 2.404016                                                       |
| 34061 | 1.000029              | 2.404021                                                       |
| 34063 | 1.044183              | 2.404025                                                       |
| 34065 | 1.735623              | 2.404029                                                       |
| 34067 | 1.155370              | 2.404034                                                       |
| 34069 | 1.187238              | 2.404038                                                       |

| $n$   | $\frac{\sigma(n)}{n}$ | $\frac{e^\gamma}{2} \log \log n + \frac{0.73...}{\log \log n}$ |
|-------|-----------------------|----------------------------------------------------------------|
| 34071 | 1.370785              | 2.404042                                                       |
| 34073 | 1.077334              | 2.404046                                                       |
| 34075 | 1.310051              | 2.404051                                                       |
| 34077 | 1.373830              | 2.404055                                                       |
| 34079 | 1.020452              | 2.404059                                                       |
| 34081 | 1.010886              | 2.404063                                                       |
| 34083 | 1.653845              | 2.404068                                                       |
| 34085 | 1.273757              | 2.404072                                                       |
| 34087 | 1.013876              | 2.404076                                                       |
| 34089 | 1.455954              | 2.404080                                                       |
| 34091 | 1.015869              | 2.404085                                                       |
| 34093 | 1.012759              | 2.404089                                                       |
| 34095 | 1.600704              | 2.404093                                                       |
| 34097 | 1.143092              | 2.404097                                                       |
| 34099 | 1.120033              | 2.404102                                                       |
| 34101 | 1.497375              | 2.404106                                                       |
| 34103 | 1.016919              | 2.404110                                                       |
| 34105 | 1.266676              | 2.404114                                                       |
| 34107 | 1.333451              | 2.404119                                                       |
| 34109 | 1.044182              | 2.404123                                                       |
| 34111 | 1.249568              | 2.404127                                                       |
| 34113 | 1.359247              | 2.404131                                                       |
| 34115 | 1.200176              | 2.404136                                                       |
| 34117 | 1.012399              | 2.404140                                                       |
| 34119 | 1.536270              | 2.404144                                                       |
| 34121 | 1.011108              | 2.404148                                                       |
| 34123 | 1.000029              | 2.404152                                                       |
| 34125 | 2.048000              | 2.404157                                                       |
| 34127 | 1.000029              | 2.404161                                                       |
| 34129 | 1.000029              | 2.404165                                                       |
| 34131 | 1.380094              | 2.404169                                                       |
| 34133 | 1.139074              | 2.404174                                                       |
| 34135 | 1.200176              | 2.404178                                                       |
| 34137 | 1.444825              | 2.404182                                                       |
| 34139 | 1.143091              | 2.404186                                                       |
| 34141 | 1.000029              | 2.404191                                                       |
| 34143 | 1.405852              | 2.404195                                                       |
| 34145 | 1.200176              | 2.404199                                                       |
| 34147 | 1.000029              | 2.404203                                                       |
| 34149 | 1.333450              | 2.404208                                                       |
| 34151 | 1.121607              | 2.404212                                                       |
| 34153 | 1.261734              | 2.404216                                                       |
| 34155 | 2.023715              | 2.404220                                                       |
| 34157 | 1.000029              | 2.404225                                                       |

| $n$   | $\frac{\sigma(n)}{n}$ | $\frac{e^\gamma}{2} \log \log n + \frac{0.73...}{\log \log n}$ |
|-------|-----------------------|----------------------------------------------------------------|
| 34159 | 1.000029              | 2.404229                                                       |
| 34161 | 1.362958              | 2.404233                                                       |
| 34163 | 1.011621              | 2.404237                                                       |
| 34165 | 1.200176              | 2.404242                                                       |
| 34167 | 1.524746              | 2.404246                                                       |
| 34169 | 1.022681              | 2.404250                                                       |
| 34171 | 1.000029              | 2.404254                                                       |
| 34173 | 1.444825              | 2.404259                                                       |
| 34175 | 1.240907              | 2.404263                                                       |
| 34177 | 1.179741              | 2.404267                                                       |
| 34179 | 1.333450              | 2.404271                                                       |
| 34181 | 1.207688              | 2.404275                                                       |
| 34183 | 1.000029              | 2.404280                                                       |
| 34185 | 1.668100              | 2.404284                                                       |
| 34187 | 1.059350              | 2.404288                                                       |
| 34189 | 1.010851              | 2.404292                                                       |
| 34191 | 1.505659              | 2.404297                                                       |
| 34193 | 1.033194              | 2.404301                                                       |
| 34195 | 1.372832              | 2.404305                                                       |
| 34197 | 1.333450              | 2.404309                                                       |
| 34199 | 1.091260              | 2.404314                                                       |
| 34201 | 1.044180              | 2.404318                                                       |
| 34203 | 1.437535              | 2.404322                                                       |
| 34205 | 1.200175              | 2.404326                                                       |
| 34207 | 1.014997              | 2.404331                                                       |
| 34209 | 1.702476              | 2.404335                                                       |
| 34211 | 1.000029              | 2.404339                                                       |
| 34213 | 1.000029              | 2.404343                                                       |
| 34215 | 1.600701              | 2.404347                                                       |
| 34217 | 1.000029              | 2.404352                                                       |
| 34219 | 1.053216              | 2.404356                                                       |
| 34221 | 1.565355              | 2.404360                                                       |
| 34223 | 1.143091              | 2.404364                                                       |
| 34225 | 1.274419              | 2.404369                                                       |
| 34227 | 1.444824              | 2.404373                                                       |
| 34229 | 1.077332              | 2.404377                                                       |
| 34231 | 1.000029              | 2.404381                                                       |
| 34233 | 1.333450              | 2.404386                                                       |
| 34235 | 1.236629              | 2.404390                                                       |
| 34237 | 1.175804              | 2.404394                                                       |
| 34239 | 1.358451              | 2.404398                                                       |
| 34241 | 1.013171              | 2.404402                                                       |
| 34243 | 1.103058              | 2.404407                                                       |
| 34245 | 1.735611              | 2.404411                                                       |

| $n$   | $\frac{\sigma(n)}{n}$ | $\frac{e^\gamma}{2} \log \log n + \frac{0.73...}{\log \log n}$ |
|-------|-----------------------|----------------------------------------------------------------|
| 34247 | 1.044179              | 2.404415                                                       |
| 34249 | 1.035359              | 2.404419                                                       |
| 34251 | 1.557677              | 2.404424                                                       |
| 34253 | 1.000029              | 2.404428                                                       |
| 34255 | 1.412465              | 2.404432                                                       |
| 34257 | 1.405844              | 2.404436                                                       |
| 34259 | 1.000029              | 2.404441                                                       |
| 34261 | 1.000029              | 2.404445                                                       |
| 34263 | 1.531214              | 2.404449                                                       |
| 34265 | 1.512914              | 2.404453                                                       |
| 34267 | 1.000029              | 2.404457                                                       |
| 34269 | 1.333450              | 2.404462                                                       |
| 34271 | 1.024540              | 2.404466                                                       |
| 34273 | 1.000029              | 2.404470                                                       |
| 34275 | 1.656951              | 2.404474                                                       |
| 34277 | 1.011057              | 2.404479                                                       |
| 34279 | 1.176230              | 2.404483                                                       |
| 34281 | 1.560865              | 2.404487                                                       |
| 34283 | 1.000029              | 2.404491                                                       |
| 34285 | 1.200175              | 2.404495                                                       |
| 34287 | 1.455945              | 2.404500                                                       |
| 34289 | 1.059348              | 2.404504                                                       |
| 34291 | 1.020443              | 2.404508                                                       |
| 34293 | 1.612457              | 2.404512                                                       |
| 34295 | 1.266657              | 2.404517                                                       |
| 34297 | 1.000029              | 2.404521                                                       |
| 34299 | 1.497886              | 2.404525                                                       |
| 34301 | 1.000029              | 2.404529                                                       |
| 34303 | 1.000029              | 2.404533                                                       |
| 34305 | 1.600700              | 2.404538                                                       |
| 34307 | 1.280205              | 2.404542                                                       |
| 34309 | 1.091259              | 2.404546                                                       |
| 34311 | 1.333450              | 2.404550                                                       |
| 34313 | 1.000029              | 2.404555                                                       |
| 34315 | 1.200175              | 2.404559                                                       |
| 34317 | 1.566571              | 2.404563                                                       |
| 34319 | 1.000029              | 2.404567                                                       |
| 34321 | 1.143090              | 2.404571                                                       |
| 34323 | 1.413862              | 2.404576                                                       |
| 34325 | 1.240903              | 2.404580                                                       |
| 34327 | 1.000029              | 2.404584                                                       |
| 34329 | 1.333450              | 2.404588                                                       |
| 34331 | 1.091259              | 2.404593                                                       |
| 34333 | 1.141759              | 2.404597                                                       |

| $n$   | $\frac{\sigma(n)}{n}$ | $\frac{e^\gamma}{2} \log \log n + \frac{0.73...}{\log \log n}$ |
|-------|-----------------------|----------------------------------------------------------------|
| 34335 | 1.999126              | 2.404601                                                       |
| 34337 | 1.000029              | 2.404605                                                       |
| 34339 | 1.044177              | 2.404609                                                       |
| 34341 | 1.333450              | 2.404614                                                       |
| 34343 | 1.018199              | 2.404618                                                       |
| 34345 | 1.200175              | 2.404622                                                       |
| 34347 | 1.345911              | 2.404626                                                       |
| 34349 | 1.164925              | 2.404631                                                       |
| 34351 | 1.000029              | 2.404635                                                       |
| 34353 | 1.580299              | 2.404639                                                       |
| 34355 | 1.200175              | 2.404643                                                       |
| 34357 | 1.106499              | 2.404647                                                       |
| 34359 | 1.437527              | 2.404652                                                       |
| 34361 | 1.000029              | 2.404656                                                       |
| 34363 | 1.143090              | 2.404660                                                       |
| 34365 | 1.676124              | 2.404664                                                       |
| 34367 | 1.000029              | 2.404668                                                       |
| 34369 | 1.000029              | 2.404673                                                       |
| 34371 | 1.582730              | 2.404677                                                       |
| 34373 | 1.028133              | 2.404681                                                       |
| 34375 | 1.363549              | 2.404685                                                       |
| 34377 | 1.524740              | 2.404689                                                       |
| 34379 | 1.033189              | 2.404694                                                       |
| 34381 | 1.000029              | 2.404698                                                       |
| 34383 | 1.360207              | 2.404702                                                       |
| 34385 | 1.350938              | 2.404706                                                       |
| 34387 | 1.011312              | 2.404711                                                       |
| 34389 | 1.444822              | 2.404715                                                       |
| 34391 | 1.214271              | 2.404719                                                       |
| 34393 | 1.010903              | 2.404723                                                       |
| 34395 | 1.600698              | 2.404727                                                       |
| 34397 | 1.130331              | 2.404732                                                       |
| 34399 | 1.025611              | 2.404736                                                       |
| 34401 | 1.333450              | 2.404740                                                       |
| 34403 | 1.000029              | 2.404744                                                       |
| 34405 | 1.372824              | 2.404748                                                       |
| 34407 | 1.444822              | 2.404753                                                       |
| 34409 | 1.053213              | 2.404757                                                       |
| 34411 | 1.077330              | 2.404761                                                       |
| 34413 | 1.333450              | 2.404765                                                       |
| 34415 | 1.200174              | 2.404769                                                       |
| 34417 | 1.011593              | 2.404774                                                       |
| 34419 | 1.673494              | 2.404778                                                       |
| 34421 | 1.000029              | 2.404782                                                       |

| $n$   | $\frac{\sigma(n)}{n}$ | $\frac{e^\gamma}{2} \log \log n + \frac{0.73...}{\log \log n}$ |
|-------|-----------------------|----------------------------------------------------------------|
| 34423 | 1.035354              | 2.404786                                                       |
| 34425 | 1.961307              | 2.404790                                                       |
| 34427 | 1.010835              | 2.404795                                                       |
| 34429 | 1.000029              | 2.404799                                                       |
| 34431 | 1.394093              | 2.404803                                                       |
| 34433 | 1.143089              | 2.404807                                                       |
| 34435 | 1.229447              | 2.404812                                                       |
| 34437 | 1.437524              | 2.404816                                                       |
| 34439 | 1.000029              | 2.404820                                                       |
| 34441 | 1.137249              | 2.404824                                                       |
| 34443 | 1.494643              | 2.404828                                                       |
| 34445 | 1.214632              | 2.404833                                                       |
| 34447 | 1.257584              | 2.404837                                                       |
| 34449 | 1.333449              | 2.404841                                                       |
| 34451 | 1.022670              | 2.404845                                                       |
| 34453 | 1.011465              | 2.404849                                                       |
| 34455 | 1.600697              | 2.404854                                                       |
| 34457 | 1.000029              | 2.404858                                                       |
| 34459 | 1.059346              | 2.404862                                                       |
| 34461 | 1.653812              | 2.404866                                                       |
| 34463 | 1.179700              | 2.404870                                                       |
| 34465 | 1.230466              | 2.404875                                                       |
| 34467 | 1.333449              | 2.404879                                                       |
| 34469 | 1.000029              | 2.404883                                                       |
| 34471 | 1.000029              | 2.404887                                                       |
| 34473 | 1.333449              | 2.404891                                                       |
| 34475 | 1.424336              | 2.404896                                                       |
| 34477 | 1.044174              | 2.404900                                                       |
| 34479 | 1.482642              | 2.404904                                                       |
| 34481 | 1.060932              | 2.404908                                                       |
| 34483 | 1.000029              | 2.404912                                                       |
| 34485 | 1.851240              | 2.404917                                                       |
| 34487 | 1.000029              | 2.404921                                                       |
| 34489 | 1.234017              | 2.404925                                                       |
| 34491 | 1.333449              | 2.404929                                                       |
| 34493 | 1.059345              | 2.404933                                                       |
| 34495 | 1.200174              | 2.404938                                                       |
| 34497 | 1.444821              | 2.404942                                                       |
| 34499 | 1.000029              | 2.404946                                                       |
| 34501 | 1.000029              | 2.404950                                                       |
| 34503 | 1.602643              | 2.404954                                                       |
| 34505 | 1.229735              | 2.404958                                                       |
| 34507 | 1.091257              | 2.404963                                                       |
| 34509 | 1.333449              | 2.404967                                                       |

| $n$   | $\frac{\sigma(n)}{n}$ | $\frac{e^\gamma}{2} \log \log n + \frac{0.73...}{\log \log n}$ |
|-------|-----------------------|----------------------------------------------------------------|
| 34511 | 1.000029              | 2.404971                                                       |
| 34513 | 1.000029              | 2.404975                                                       |
| 34515 | 1.898305              | 2.404979                                                       |
| 34517 | 1.143089              | 2.404984                                                       |
| 34519 | 1.000029              | 2.404988                                                       |
| 34521 | 1.373772              | 2.404992                                                       |
| 34523 | 1.112302              | 2.404996                                                       |
| 34525 | 1.240898              | 2.405000                                                       |
| 34527 | 1.413850              | 2.405005                                                       |
| 34529 | 1.131571              | 2.405009                                                       |
| 34531 | 1.143089              | 2.405013                                                       |
| 34533 | 1.482640              | 2.405017                                                       |
| 34535 | 1.200174              | 2.405021                                                       |
| 34537 | 1.000029              | 2.405026                                                       |
| 34539 | 1.382785              | 2.405030                                                       |
| 34541 | 1.077328              | 2.405034                                                       |
| 34543 | 1.000029              | 2.405038                                                       |
| 34545 | 1.900825              | 2.405042                                                       |
| 34547 | 1.010797              | 2.405047                                                       |
| 34549 | 1.000029              | 2.405051                                                       |
| 34551 | 1.580273              | 2.405055                                                       |
| 34553 | 1.012358              | 2.405059                                                       |
| 34555 | 1.200174              | 2.405063                                                       |
| 34557 | 1.333449              | 2.405067                                                       |
| 34559 | 1.143089              | 2.405072                                                       |
| 34561 | 1.124967              | 2.405076                                                       |
| 34563 | 1.370714              | 2.405080                                                       |
| 34565 | 1.244264              | 2.405084                                                       |
| 34567 | 1.077328              | 2.405088                                                       |
| 34569 | 1.516272              | 2.405093                                                       |
| 34571 | 1.010789              | 2.405097                                                       |
| 34573 | 1.249530              | 2.405101                                                       |
| 34575 | 1.656920              | 2.405105                                                       |
| 34577 | 1.016167              | 2.405109                                                       |
| 34579 | 1.011018              | 2.405114                                                       |
| 34581 | 1.333449              | 2.405118                                                       |
| 34583 | 1.000029              | 2.405122                                                       |
| 34585 | 1.200173              | 2.405126                                                       |
| 34587 | 1.735218              | 2.405130                                                       |
| 34589 | 1.000029              | 2.405134                                                       |
| 34591 | 1.000029              | 2.405139                                                       |
| 34593 | 1.437516              | 2.405143                                                       |
| 34595 | 1.423558              | 2.405147                                                       |
| 34597 | 1.035350              | 2.405151                                                       |

| $n$   | $\frac{\sigma(n)}{n}$ | $\frac{e^\gamma}{2} \log \log n + \frac{0.73\dots}{\log \log n}$ |
|-------|-----------------------|------------------------------------------------------------------|
| 34599 | 1.405821              | 2.405155                                                         |
| 34601 | 1.143088              | 2.405160                                                         |
| 34603 | 1.000029              | 2.405164                                                         |
| 34605 | 1.735587              | 2.405168                                                         |
| 34607 | 1.000029              | 2.405172                                                         |
| 34609 | 1.020428              | 2.405176                                                         |
| 34611 | 1.359105              | 2.405180                                                         |
| 34613 | 1.000029              | 2.405185                                                         |
| 34615 | 1.464336              | 2.405189                                                         |
| 34617 | 1.455932              | 2.405193                                                         |
| 34619 | 1.077327              | 2.405197                                                         |
| 34621 | 1.013836              | 2.405201                                                         |
| 34623 | 1.444820              | 2.405206                                                         |
| 34625 | 1.252505              | 2.405210                                                         |
| 34627 | 1.033182              | 2.405214                                                         |
| 34629 | 1.630079              | 2.405218                                                         |
| 34631 | 1.000029              | 2.405222                                                         |
| 34633 | 1.018682              | 2.405226                                                         |
| 34635 | 1.600693              | 2.405231                                                         |
| 34637 | 1.053209              | 2.405235                                                         |
| 34639 | 1.130749              | 2.405239                                                         |
| 34641 | 1.482636              | 2.405243                                                         |
| 34643 | 1.177727              | 2.405247                                                         |
| 34645 | 1.331101              | 2.405251                                                         |
| 34647 | 1.333449              | 2.405256                                                         |
| 34649 | 1.000029              | 2.405260                                                         |
| 34651 | 1.000029              | 2.405264                                                         |
| 34653 | 1.333449              | 2.405268                                                         |
| 34655 | 1.246573              | 2.405272                                                         |
| 34657 | 1.143088              | 2.405277                                                         |
| 34659 | 1.444820              | 2.405281                                                         |
| 34661 | 1.146649              | 2.405285                                                         |
| 34663 | 1.059343              | 2.405289                                                         |
| 34665 | 1.600692              | 2.405293                                                         |
| 34667 | 1.000029              | 2.405297                                                         |
| 34669 | 1.028123              | 2.405302                                                         |
| 34671 | 1.653947              | 2.405306                                                         |
| 34673 | 1.000029              | 2.405310                                                         |
| 34675 | 1.323143              | 2.405314                                                         |
| 34677 | 1.444819              | 2.405318                                                         |
| 34679 | 1.000029              | 2.405322                                                         |
| 34681 | 1.014965              | 2.405327                                                         |
| 34683 | 1.455929              | 2.405331                                                         |
| 34685 | 1.372812              | 2.405335                                                         |



| $n$   | $\frac{\sigma(n)}{n}$ | $\frac{e^\gamma}{2} \log \log n + \frac{0.73...}{\log \log n}$ |
|-------|-----------------------|----------------------------------------------------------------|
| 34687 | 1.000029              | 2.405339                                                       |
| 34689 | 1.380034              | 2.405343                                                       |
| 34691 | 1.012136              | 2.405347                                                       |
| 34693 | 1.000029              | 2.405352                                                       |
| 34695 | 1.784695              | 2.405356                                                       |
| 34697 | 1.147534              | 2.405360                                                       |
| 34699 | 1.143088              | 2.405364                                                       |
| 34701 | 1.369413              | 2.405368                                                       |
| 34703 | 1.000029              | 2.405372                                                       |
| 34705 | 1.311166              | 2.405377                                                       |
| 34707 | 1.394070              | 2.405381                                                       |
| 34709 | 1.018180              | 2.405385                                                       |
| 34711 | 1.012705              | 2.405389                                                       |
| 34713 | 1.797597              | 2.405393                                                       |
| 34715 | 1.231975              | 2.405397                                                       |
| 34717 | 1.011032              | 2.405402                                                       |
| 34719 | 1.360408              | 2.405406                                                       |
| 34721 | 1.000029              | 2.405410                                                       |
| 34723 | 1.077326              | 2.405414                                                       |
| 34725 | 1.656904              | 2.405418                                                       |
| 34727 | 1.286837              | 2.405422                                                       |
| 34729 | 1.000029              | 2.405427                                                       |
| 34731 | 1.536149              | 2.405431                                                       |
| 34733 | 1.022659              | 2.405435                                                       |
| 34735 | 1.200173              | 2.405439                                                       |
| 34737 | 1.333448              | 2.405443                                                       |
| 34739 | 1.000029              | 2.405447                                                       |
| 34741 | 1.164906              | 2.405452                                                       |
| 34743 | 1.373744              | 2.405456                                                       |
| 34745 | 1.200173              | 2.405460                                                       |
| 34747 | 1.000029              | 2.405464                                                       |
| 34749 | 1.759820              | 2.405468                                                       |
| 34751 | 1.105004              | 2.405472                                                       |
| 34753 | 1.044169              | 2.405477                                                       |
| 34755 | 1.834096              | 2.405481                                                       |
| 34757 | 1.000029              | 2.405485                                                       |
| 34759 | 1.000029              | 2.405489                                                       |
| 34761 | 1.333448              | 2.405493                                                       |
| 34763 | 1.000029              | 2.405497                                                       |
| 34765 | 1.273695              | 2.405502                                                       |
| 34767 | 1.444818              | 2.405506                                                       |
| 34769 | 1.143087              | 2.405510                                                       |
| 34771 | 1.138880              | 2.405514                                                       |
| 34773 | 1.361056              | 2.405518                                                       |

| $n$   | $\frac{\sigma(n)}{n}$ | $\frac{e^\gamma}{2} \log \log n + \frac{0.73\dots}{\log \log n}$ |
|-------|-----------------------|------------------------------------------------------------------|
| 34775 | 1.347865              | 2.405522                                                         |
| 34777 | 1.014464              | 2.405527                                                         |
| 34779 | 1.333448              | 2.405531                                                         |
| 34781 | 1.000029              | 2.405535                                                         |
| 34783 | 1.143087              | 2.405539                                                         |
| 34785 | 1.735576              | 2.405543                                                         |
| 34787 | 1.024521              | 2.405547                                                         |
| 34789 | 1.053206              | 2.405551                                                         |
| 34791 | 1.333448              | 2.405556                                                         |
| 34793 | 1.091254              | 2.405560                                                         |
| 34795 | 1.200172              | 2.405564                                                         |
| 34797 | 1.524729              | 2.405568                                                         |
| 34799 | 1.117273              | 2.405572                                                         |
| 34801 | 1.077325              | 2.405576                                                         |
| 34803 | 1.482631              | 2.405581                                                         |
| 34805 | 1.200172              | 2.405585                                                         |
| 34807 | 1.000029              | 2.405589                                                         |
| 34809 | 1.370680              | 2.405593                                                         |
| 34811 | 1.143087              | 2.405597                                                         |
| 34813 | 1.033177              | 2.405601                                                         |
| 34815 | 1.753727              | 2.405606                                                         |
| 34817 | 1.028118              | 2.405610                                                         |
| 34819 | 1.000029              | 2.405614                                                         |
| 34821 | 1.491858              | 2.405618                                                         |
| 34823 | 1.013124              | 2.405622                                                         |
| 34825 | 1.424264              | 2.405626                                                         |
| 34827 | 1.543630              | 2.405630                                                         |
| 34829 | 1.035344              | 2.405635                                                         |
| 34831 | 1.018173              | 2.405639                                                         |
| 34833 | 1.413832              | 2.405643                                                         |
| 34835 | 1.200172              | 2.405647                                                         |
| 34837 | 1.091254              | 2.405651                                                         |
| 34839 | 1.701541              | 2.405655                                                         |
| 34841 | 1.000029              | 2.405659                                                         |
| 34843 | 1.000029              | 2.405664                                                         |
| 34845 | 1.686096              | 2.405668                                                         |
| 34847 | 1.000029              | 2.405672                                                         |
| 34849 | 1.000029              | 2.405676                                                         |
| 34851 | 1.333448              | 2.405680                                                         |
| 34853 | 1.233983              | 2.405684                                                         |
| 34855 | 1.200172              | 2.405689                                                         |
| 34857 | 1.482629              | 2.405693                                                         |
| 34859 | 1.091253              | 2.405697                                                         |
| 34861 | 1.016150              | 2.405701                                                         |

| $n$   | $\frac{\sigma(n)}{n}$ | $\frac{e^\gamma}{2} \log \log n + \frac{0.73...}{\log \log n}$ |
|-------|-----------------------|----------------------------------------------------------------|
| 34863 | 1.333448              | 2.405705                                                       |
| 34865 | 1.266600              | 2.405709                                                       |
| 34867 | 1.214214              | 2.405713                                                       |
| 34869 | 1.362815              | 2.405718                                                       |
| 34871 | 1.000029              | 2.405722                                                       |
| 34873 | 1.024518              | 2.405726                                                       |
| 34875 | 1.860817              | 2.405730                                                       |
| 34877 | 1.000029              | 2.405734                                                       |
| 34879 | 1.077324              | 2.405738                                                       |
| 34881 | 1.673347              | 2.405742                                                       |
| 34883 | 1.000029              | 2.405747                                                       |
| 34885 | 1.200172              | 2.405751                                                       |
| 34887 | 1.382750              | 2.405755                                                       |
| 34889 | 1.011207              | 2.405759                                                       |
| 34891 | 1.097819              | 2.405763                                                       |
| 34893 | 1.444817              | 2.405767                                                       |
| 34895 | 1.372804              | 2.405771                                                       |
| 34897 | 1.000029              | 2.405776                                                       |
| 34899 | 1.333448              | 2.405780                                                       |
| 34901 | 1.059339              | 2.405784                                                       |
| 34903 | 1.155202              | 2.405788                                                       |
| 34905 | 1.732703              | 2.405792                                                       |
| 34907 | 1.016873              | 2.405796                                                       |
| 34909 | 1.143086              | 2.405800                                                       |
| 34911 | 1.497293              | 2.405805                                                       |
| 34913 | 1.000029              | 2.405809                                                       |
| 34915 | 1.200172              | 2.405813                                                       |
| 34917 | 1.358192              | 2.405817                                                       |
| 34919 | 1.000029              | 2.405821                                                       |
| 34921 | 1.022651              | 2.405825                                                       |
| 34923 | 1.524726              | 2.405829                                                       |
| 34925 | 1.363379              | 2.405834                                                       |
| 34927 | 1.020414              | 2.405838                                                       |
| 34929 | 1.444817              | 2.405842                                                       |
| 34931 | 1.077324              | 2.405846                                                       |
| 34933 | 1.010735              | 2.405850                                                       |
| 34935 | 1.706483              | 2.405854                                                       |
| 34937 | 1.252998              | 2.405858                                                       |
| 34939 | 1.000029              | 2.405863                                                       |
| 34941 | 1.405798              | 2.405867                                                       |
| 34943 | 1.014452              | 2.405871                                                       |
| 34945 | 1.246530              | 2.405875                                                       |
| 34947 | 1.580221              | 2.405879                                                       |
| 34949 | 1.000029              | 2.405883                                                       |

| $n$   | $\frac{\sigma(n)}{n}$ | $\frac{e^\gamma}{2} \log \log n + \frac{0.73\dots}{\log \log n}$ |
|-------|-----------------------|------------------------------------------------------------------|
| 34951 | 1.143086              | 2.405887                                                         |
| 34953 | 1.362286              | 2.405892                                                         |
| 34955 | 1.200172              | 2.405896                                                         |
| 34957 | 1.077324              | 2.405900                                                         |
| 34959 | 1.369376              | 2.405904                                                         |
| 34961 | 1.000029              | 2.405908                                                         |
| 34963 | 1.000029              | 2.405912                                                         |
| 34965 | 2.086658              | 2.405916                                                         |
| 34967 | 1.015815              | 2.405920                                                         |
| 34969 | 1.167634              | 2.405925                                                         |
| 34971 | 1.333448              | 2.405929                                                         |
| 34973 | 1.025591              | 2.405933                                                         |
| 34975 | 1.240886              | 2.405937                                                         |
| 34977 | 1.358607              | 2.405941                                                         |
| 34979 | 1.207582              | 2.405945                                                         |
| 34981 | 1.000029              | 2.405949                                                         |
| 34983 | 1.632107              | 2.405954                                                         |
| 34985 | 1.200172              | 2.405958                                                         |
| 34987 | 1.018664              | 2.405962                                                         |
| 34989 | 1.358141              | 2.405966                                                         |
| 34991 | 1.091252              | 2.405970                                                         |
| 34993 | 1.143086              | 2.405974                                                         |
| 34995 | 1.600686              | 2.405978                                                         |
| 34997 | 1.014944              | 2.405982                                                         |
| 34999 | 1.033172              | 2.405987                                                         |
| 35001 | 1.444816              | 2.405991                                                         |
| 35003 | 1.110762              | 2.405995                                                         |
| 35005 | 1.200171              | 2.405999                                                         |
| 35007 | 1.524724              | 2.406003                                                         |
| 35009 | 1.077323              | 2.406007                                                         |
| 35011 | 1.010882              | 2.406011                                                         |
| 35013 | 1.455916              | 2.406016                                                         |
| 35015 | 1.233757              | 2.406020                                                         |
| 35017 | 1.066282              | 2.406024                                                         |
| 35019 | 1.482624              | 2.406028                                                         |
| 35021 | 1.143086              | 2.406032                                                         |
| 35023 | 1.000029              | 2.406036                                                         |
| 35025 | 1.656874              | 2.406040                                                         |
| 35027 | 1.000029              | 2.406044                                                         |
| 35029 | 1.044163              | 2.406049                                                         |
| 35031 | 1.333448              | 2.406053                                                         |
| 35033 | 1.020409              | 2.406057                                                         |
| 35035 | 1.639960              | 2.406061                                                         |
| 35037 | 1.536090              | 2.406065                                                         |

| $n$   | $\frac{\sigma(n)}{n}$ | $\frac{e^\gamma}{2} \log \log n + \frac{0.73...}{\log \log n}$ |
|-------|-----------------------|----------------------------------------------------------------|
| 35039 | 1.028112              | 2.406069                                                       |
| 35041 | 1.016866              | 2.406073                                                       |
| 35043 | 1.333447              | 2.406077                                                       |
| 35045 | 1.235440              | 2.406082                                                       |
| 35047 | 1.012811              | 2.406086                                                       |
| 35049 | 1.524723              | 2.406090                                                       |
| 35051 | 1.000029              | 2.406094                                                       |
| 35053 | 1.000029              | 2.406098                                                       |
| 35055 | 1.869063              | 2.406102                                                       |
| 35057 | 1.091251              | 2.406106                                                       |
| 35059 | 1.000029              | 2.406110                                                       |
| 35061 | 1.533328              | 2.406115                                                       |
| 35063 | 1.143085              | 2.406119                                                       |
| 35065 | 1.200171              | 2.406123                                                       |
| 35067 | 1.333447              | 2.406127                                                       |
| 35069 | 1.000029              | 2.406131                                                       |
| 35071 | 1.059337              | 2.406135                                                       |
| 35073 | 1.497277              | 2.406139                                                       |
| 35075 | 1.315125              | 2.406143                                                       |
| 35077 | 1.143085              | 2.406148                                                       |
| 35079 | 1.455914              | 2.406152                                                       |
| 35081 | 1.000029              | 2.406156                                                       |
| 35083 | 1.000029              | 2.406160                                                       |
| 35085 | 1.600684              | 2.406164                                                       |
| 35087 | 1.077322              | 2.406168                                                       |
| 35089 | 1.000028              | 2.406172                                                       |
| 35091 | 1.653757              | 2.406176                                                       |
| 35093 | 1.053201              | 2.406180                                                       |
| 35095 | 1.200171              | 2.406185                                                       |
| 35097 | 1.333447              | 2.406189                                                       |
| 35099 | 1.000028              | 2.406193                                                       |
| 35101 | 1.091251              | 2.406197                                                       |
| 35103 | 1.333447              | 2.406201                                                       |
| 35105 | 1.476713              | 2.406205                                                       |
| 35107 | 1.000028              | 2.406209                                                       |
| 35109 | 1.492951              | 2.406213                                                       |
| 35111 | 1.000028              | 2.406218                                                       |
| 35113 | 1.121180              | 2.406222                                                       |
| 35115 | 1.600683              | 2.406226                                                       |
| 35117 | 1.000028              | 2.406230                                                       |
| 35119 | 1.189100              | 2.406234                                                       |
| 35121 | 1.394038              | 2.406238                                                       |
| 35123 | 1.137033              | 2.406242                                                       |
| 35125 | 1.252441              | 2.406246                                                       |

| $n$   | $\frac{\sigma(n)}{n}$ | $\frac{e^\gamma}{2} \log \log n + \frac{0.73...}{\log \log n}$ |
|-------|-----------------------|----------------------------------------------------------------|
| 35127 | 1.482620              | 2.406250                                                       |
| 35129 | 1.000028              | 2.406255                                                       |
| 35131 | 1.077681              | 2.406259                                                       |
| 35133 | 1.557510              | 2.406263                                                       |
| 35135 | 1.200171              | 2.406267                                                       |
| 35137 | 1.025586              | 2.406271                                                       |
| 35139 | 1.549048              | 2.406275                                                       |
| 35141 | 1.000028              | 2.406279                                                       |
| 35143 | 1.012093              | 2.406283                                                       |
| 35145 | 1.917542              | 2.406287                                                       |
| 35147 | 1.143085              | 2.406292                                                       |
| 35149 | 1.000028              | 2.406296                                                       |
| 35151 | 1.333447              | 2.406300                                                       |
| 35153 | 1.000028              | 2.406304                                                       |
| 35155 | 1.228844              | 2.406308                                                       |
| 35157 | 1.333447              | 2.406312                                                       |
| 35159 | 1.000028              | 2.406316                                                       |
| 35161 | 1.143085              | 2.406320                                                       |
| 35163 | 1.444814              | 2.406324                                                       |
| 35165 | 1.294696              | 2.406329                                                       |
| 35167 | 1.146529              | 2.406333                                                       |
| 35169 | 1.405784              | 2.406337                                                       |
| 35171 | 1.000028              | 2.406341                                                       |
| 35173 | 1.059335              | 2.406345                                                       |
| 35175 | 1.917726              | 2.406349                                                       |
| 35177 | 1.035336              | 2.406353                                                       |
| 35179 | 1.011513              | 2.406357                                                       |
| 35181 | 1.482618              | 2.406361                                                       |
| 35183 | 1.010943              | 2.406366                                                       |
| 35185 | 1.244167              | 2.406370                                                       |
| 35187 | 1.373689              | 2.406374                                                       |
| 35189 | 1.249481              | 2.406378                                                       |
| 35191 | 1.077321              | 2.406382                                                       |
| 35193 | 1.333447              | 2.406386                                                       |
| 35195 | 1.200170              | 2.406390                                                       |
| 35197 | 1.018155              | 2.406394                                                       |
| 35199 | 1.444814              | 2.406398                                                       |
| 35201 | 1.000028              | 2.406403                                                       |
| 35203 | 1.178081              | 2.406407                                                       |
| 35205 | 1.600682              | 2.406411                                                       |
| 35207 | 1.124776              | 2.406415                                                       |
| 35209 | 1.011219              | 2.406419                                                       |
| 35211 | 1.480674              | 2.406423                                                       |
| 35213 | 1.044160              | 2.406427                                                       |

| $n$   | $\frac{\sigma(n)}{n}$ | $\frac{e^\gamma}{2} \log \log n + \frac{0.73\dots}{\log \log n}$ |
|-------|-----------------------|------------------------------------------------------------------|
| 35215 | 1.200170              | 2.406431                                                         |
| 35217 | 1.819121              | 2.406435                                                         |
| 35219 | 1.025583              | 2.406439                                                         |
| 35221 | 1.000028              | 2.406444                                                         |
| 35223 | 1.362746              | 2.406448                                                         |
| 35225 | 1.240880              | 2.406452                                                         |
| 35227 | 1.000028              | 2.406456                                                         |
| 35229 | 1.333447              | 2.406460                                                         |
| 35231 | 1.164883              | 2.406464                                                         |
| 35233 | 1.091250              | 2.406468                                                         |
| 35235 | 1.859515              | 2.406472                                                         |
| 35237 | 1.010756              | 2.406476                                                         |
| 35239 | 1.011379              | 2.406480                                                         |
| 35241 | 1.413808              | 2.406485                                                         |
| 35243 | 1.077320              | 2.406489                                                         |
| 35245 | 1.470847              | 2.406493                                                         |
| 35247 | 1.379976              | 2.406497                                                         |
| 35249 | 1.012795              | 2.406501                                                         |
| 35251 | 1.000028              | 2.406505                                                         |
| 35253 | 1.444813              | 2.406509                                                         |
| 35255 | 1.311133              | 2.406513                                                         |
| 35257 | 1.000028              | 2.406517                                                         |
| 35259 | 1.611844              | 2.406521                                                         |
| 35261 | 1.028105              | 2.406526                                                         |
| 35263 | 1.010691              | 2.406530                                                         |
| 35265 | 1.600681              | 2.406534                                                         |
| 35267 | 1.000028              | 2.406538                                                         |
| 35269 | 1.077320              | 2.406542                                                         |
| 35271 | 1.444813              | 2.406546                                                         |
| 35273 | 1.143084              | 2.406550                                                         |
| 35275 | 1.328760              | 2.406554                                                         |
| 35277 | 1.455906              | 2.406558                                                         |
| 35279 | 1.000028              | 2.406562                                                         |
| 35281 | 1.000028              | 2.406567                                                         |
| 35283 | 1.405776              | 2.406571                                                         |
| 35285 | 1.200170              | 2.406575                                                         |
| 35287 | 1.159180              | 2.406579                                                         |
| 35289 | 1.482615              | 2.406583                                                         |
| 35291 | 1.000028              | 2.406587                                                         |
| 35293 | 1.035333              | 2.406591                                                         |
| 35295 | 1.732597              | 2.406595                                                         |
| 35297 | 1.022636              | 2.406599                                                         |
| 35299 | 1.091249              | 2.406603                                                         |
| 35301 | 1.561882              | 2.406607                                                         |

| $n$   | $\frac{\sigma(n)}{n}$ | $\frac{e^\gamma}{2} \log \log n + \frac{0.73\dots}{\log \log n}$ |
|-------|-----------------------|------------------------------------------------------------------|
| 35303 | 1.024502              | 2.406612                                                         |
| 35305 | 1.256253              | 2.406616                                                         |
| 35307 | 1.444813              | 2.406620                                                         |
| 35309 | 1.109292              | 2.406624                                                         |
| 35311 | 1.000028              | 2.406628                                                         |
| 35313 | 1.359273              | 2.406632                                                         |
| 35315 | 1.372788              | 2.406636                                                         |
| 35317 | 1.000028              | 2.406640                                                         |
| 35319 | 1.362213              | 2.406644                                                         |
| 35321 | 1.243453              | 2.406648                                                         |
| 35323 | 1.000028              | 2.406652                                                         |
| 35325 | 1.802519              | 2.406657                                                         |
| 35327 | 1.000028              | 2.406661                                                         |
| 35329 | 1.177503              | 2.406665                                                         |
| 35331 | 1.333447              | 2.406669                                                         |
| 35333 | 1.013783              | 2.406673                                                         |
| 35335 | 1.238885              | 2.406677                                                         |
| 35337 | 1.333447              | 2.406681                                                         |
| 35339 | 1.000028              | 2.406685                                                         |
| 35341 | 1.018647              | 2.406689                                                         |
| 35343 | 1.955691              | 2.406693                                                         |
| 35345 | 1.200170              | 2.406697                                                         |
| 35347 | 1.077319              | 2.406702                                                         |
| 35349 | 1.333446              | 2.406706                                                         |
| 35351 | 1.099827              | 2.406710                                                         |
| 35353 | 1.000028              | 2.406714                                                         |
| 35355 | 1.600679              | 2.406718                                                         |
| 35357 | 1.143083              | 2.406722                                                         |
| 35359 | 1.053197              | 2.406726                                                         |
| 35361 | 1.444812              | 2.406730                                                         |
| 35363 | 1.000028              | 2.406734                                                         |
| 35365 | 1.311127              | 2.406738                                                         |
| 35367 | 1.333446              | 2.406742                                                         |
| 35369 | 1.012073              | 2.406746                                                         |
| 35371 | 1.186961              | 2.406751                                                         |
| 35373 | 1.437481              | 2.406755                                                         |
| 35375 | 1.252410              | 2.406759                                                         |
| 35377 | 1.059332              | 2.406763                                                         |
| 35379 | 1.444812              | 2.406767                                                         |
| 35381 | 1.000028              | 2.406771                                                         |
| 35383 | 1.025577              | 2.406775                                                         |
| 35385 | 1.833997              | 2.406779                                                         |
| 35387 | 1.091248              | 2.406783                                                         |
| 35389 | 1.024499              | 2.406787                                                         |



| $n$   | $\frac{\sigma(n)}{n}$ | $\frac{e^\gamma}{2} \log \log n + \frac{0.73\dots}{\log \log n}$ |
|-------|-----------------------|------------------------------------------------------------------|
| 35391 | 1.367127              | 2.406791                                                         |
| 35393 | 1.000028              | 2.406795                                                         |
| 35395 | 1.200170              | 2.406800                                                         |
| 35397 | 1.640817              | 2.406804                                                         |
| 35399 | 1.233933              | 2.406808                                                         |
| 35401 | 1.000028              | 2.406812                                                         |
| 35403 | 1.333446              | 2.406816                                                         |
| 35405 | 1.228979              | 2.406820                                                         |
| 35407 | 1.000028              | 2.406824                                                         |
| 35409 | 1.545370              | 2.406828                                                         |
| 35411 | 1.059332              | 2.406832                                                         |
| 35413 | 1.143083              | 2.406836                                                         |
| 35415 | 1.735536              | 2.406840                                                         |
| 35417 | 1.012395              | 2.406844                                                         |
| 35419 | 1.000028              | 2.406848                                                         |
| 35421 | 1.333446              | 2.406853                                                         |
| 35423 | 1.000028              | 2.406857                                                         |
| 35425 | 1.347636              | 2.406861                                                         |
| 35427 | 1.557456              | 2.406865                                                         |
| 35429 | 1.016117              | 2.406869                                                         |
| 35431 | 1.091248              | 2.406873                                                         |
| 35433 | 1.502780              | 2.406877                                                         |
| 35435 | 1.266544              | 2.406881                                                         |
| 35437 | 1.000028              | 2.406885                                                         |
| 35439 | 1.333446              | 2.406889                                                         |
| 35441 | 1.175588              | 2.406893                                                         |
| 35443 | 1.060971              | 2.406897                                                         |
| 35445 | 1.706306              | 2.406901                                                         |
| 35447 | 1.000028              | 2.406906                                                         |
| 35449 | 1.000028              | 2.406910                                                         |
| 35451 | 1.611238              | 2.406914                                                         |
| 35453 | 1.102925              | 2.406918                                                         |
| 35455 | 1.372782              | 2.406922                                                         |
| 35457 | 1.364582              | 2.406926                                                         |
| 35459 | 1.018641              | 2.406930                                                         |
| 35461 | 1.000028              | 2.406934                                                         |
| 35463 | 1.333446              | 2.406938                                                         |
| 35465 | 1.236374              | 2.406942                                                         |
| 35467 | 1.035329              | 2.406946                                                         |
| 35469 | 1.653726              | 2.406950                                                         |
| 35471 | 1.014914              | 2.406954                                                         |
| 35473 | 1.053195              | 2.406958                                                         |
| 35475 | 1.845581              | 2.406963                                                         |
| 35477 | 1.077318              | 2.406967                                                         |

| $n$   | $\frac{\sigma(n)}{n}$ | $\frac{e^\gamma}{2} \log \log n + \frac{0.73...}{\log \log n}$ |
|-------|-----------------------|----------------------------------------------------------------|
| 35479 | 1.059331              | 2.406971                                                       |
| 35481 | 1.333446              | 2.406975                                                       |
| 35483 | 1.182313              | 2.406979                                                       |
| 35485 | 1.233648              | 2.406983                                                       |
| 35487 | 1.444811              | 2.406987                                                       |
| 35489 | 1.044155              | 2.406991                                                       |
| 35491 | 1.000028              | 2.406995                                                       |
| 35493 | 1.333446              | 2.406999                                                       |
| 35495 | 1.244119              | 2.407003                                                       |
| 35497 | 1.249458              | 2.407007                                                       |
| 35499 | 1.333446              | 2.407011                                                       |
| 35501 | 1.011352              | 2.407015                                                       |
| 35503 | 1.077317              | 2.407020                                                       |
| 35505 | 1.784537              | 2.407024                                                       |
| 35507 | 1.000028              | 2.407028                                                       |
| 35509 | 1.000028              | 2.407032                                                       |
| 35511 | 1.622033              | 2.407036                                                       |
| 35513 | 1.059330              | 2.407040                                                       |
| 35515 | 1.200169              | 2.407044                                                       |
| 35517 | 1.333446              | 2.407048                                                       |
| 35519 | 1.091247              | 2.407052                                                       |
| 35521 | 1.000028              | 2.407056                                                       |
| 35523 | 1.444810              | 2.407060                                                       |
| 35525 | 1.492189              | 2.407064                                                       |
| 35527 | 1.000028              | 2.407068                                                       |
| 35529 | 1.437474              | 2.407072                                                       |
| 35531 | 1.000028              | 2.407076                                                       |
| 35533 | 1.000028              | 2.407080                                                       |
| 35535 | 1.685775              | 2.407085                                                       |
| 35537 | 1.000028              | 2.407089                                                       |
| 35539 | 1.143082              | 2.407093                                                       |
| 35541 | 1.580147              | 2.407097                                                       |
| 35543 | 1.000028              | 2.407101                                                       |
| 35545 | 1.200169              | 2.407105                                                       |
| 35547 | 1.450924              | 2.407109                                                       |
| 35549 | 1.053194              | 2.407113                                                       |
| 35551 | 1.015780              | 2.407117                                                       |
| 35553 | 1.524710              | 2.407121                                                       |
| 35555 | 1.294670              | 2.407125                                                       |
| 35557 | 1.061226              | 2.407129                                                       |
| 35559 | 1.497230              | 2.407133                                                       |
| 35561 | 1.024493              | 2.407137                                                       |
| 35563 | 1.129713              | 2.407141                                                       |
| 35565 | 1.600675              | 2.407145                                                       |

| $n$   | $\frac{\sigma(n)}{n}$ | $\frac{e^\gamma}{2} \log \log n + \frac{0.73...}{\log \log n}$ |
|-------|-----------------------|----------------------------------------------------------------|
| 35567 | 1.143082              | 2.407150                                                       |
| 35569 | 1.000028              | 2.407154                                                       |
| 35571 | 1.360209              | 2.407158                                                       |
| 35573 | 1.000028              | 2.407162                                                       |
| 35575 | 1.240871              | 2.407166                                                       |
| 35577 | 1.490851              | 2.407170                                                       |
| 35579 | 1.022626              | 2.407174                                                       |
| 35581 | 1.359827              | 2.407178                                                       |
| 35583 | 1.382683              | 2.407182                                                       |
| 35585 | 1.311114              | 2.407186                                                       |
| 35587 | 1.053194              | 2.407190                                                       |
| 35589 | 1.333446              | 2.407194                                                       |
| 35591 | 1.000028              | 2.407198                                                       |
| 35593 | 1.000028              | 2.407202                                                       |
| 35595 | 1.998483              | 2.407206                                                       |
| 35597 | 1.000028              | 2.407210                                                       |
| 35599 | 1.013062              | 2.407214                                                       |
| 35601 | 1.333446              | 2.407219                                                       |
| 35603 | 1.000028              | 2.407223                                                       |
| 35605 | 1.200169              | 2.407227                                                       |
| 35607 | 1.585306              | 2.407231                                                       |
| 35609 | 1.143082              | 2.407235                                                       |
| 35611 | 1.010924              | 2.407239                                                       |
| 35613 | 1.482605              | 2.407243                                                       |
| 35615 | 1.273621              | 2.407247                                                       |
| 35617 | 1.000028              | 2.407251                                                       |
| 35619 | 1.379938              | 2.407255                                                       |
| 35621 | 1.010640              | 2.407259                                                       |
| 35623 | 1.164865              | 2.407263                                                       |
| 35625 | 1.753825              | 2.407267                                                       |
| 35627 | 1.044152              | 2.407271                                                       |
| 35629 | 1.131662              | 2.407275                                                       |
| 35631 | 1.497348              | 2.407279                                                       |
| 35633 | 1.077316              | 2.407283                                                       |
| 35635 | 1.200168              | 2.407287                                                       |
| 35637 | 1.524707              | 2.407291                                                       |
| 35639 | 1.010803              | 2.407296                                                       |
| 35641 | 1.035324              | 2.407300                                                       |
| 35643 | 1.345678              | 2.407304                                                       |
| 35645 | 1.200168              | 2.407308                                                       |
| 35647 | 1.024490              | 2.407312                                                       |
| 35649 | 1.535976              | 2.407316                                                       |
| 35651 | 1.249446              | 2.407320                                                       |
| 35653 | 1.012762              | 2.407324                                                       |

| $n$   | $\frac{\sigma(n)}{n}$ | $\frac{e^\gamma}{2} \log \log n + \frac{0.73...}{\log \log n}$ |
|-------|-----------------------|----------------------------------------------------------------|
| 35655 | 1.600673              | 2.407328                                                       |
| 35657 | 1.010629              | 2.407332                                                       |
| 35659 | 1.087972              | 2.407336                                                       |
| 35661 | 1.333446              | 2.407340                                                       |
| 35663 | 1.053192              | 2.407344                                                       |
| 35665 | 1.372774              | 2.407348                                                       |
| 35667 | 1.482603              | 2.407352                                                       |
| 35669 | 1.020382              | 2.407356                                                       |
| 35671 | 1.000028              | 2.407360                                                       |
| 35673 | 1.550080              | 2.407364                                                       |
| 35675 | 1.240869              | 2.407368                                                       |
| 35677 | 1.000028              | 2.407372                                                       |
| 35679 | 1.524706              | 2.407376                                                       |
| 35681 | 1.033155              | 2.407381                                                       |
| 35683 | 1.059328              | 2.407385                                                       |
| 35685 | 1.897268              | 2.407389                                                       |
| 35687 | 1.011461              | 2.407393                                                       |
| 35689 | 1.013758              | 2.407397                                                       |
| 35691 | 1.333445              | 2.407401                                                       |
| 35693 | 1.143081              | 2.407405                                                       |
| 35695 | 1.341364              | 2.407409                                                       |
| 35697 | 1.359890              | 2.407413                                                       |
| 35699 | 1.035323              | 2.407417                                                       |
| 35701 | 1.053192              | 2.407421                                                       |
| 35703 | 1.444809              | 2.407425                                                       |
| 35705 | 1.238818              | 2.407429                                                       |
| 35707 | 1.143081              | 2.407433                                                       |
| 35709 | 1.333445              | 2.407437                                                       |
| 35711 | 1.119655              | 2.407441                                                       |
| 35713 | 1.016101              | 2.407445                                                       |
| 35715 | 1.600672              | 2.407449                                                       |
| 35717 | 1.161128              | 2.407453                                                       |
| 35719 | 1.044150              | 2.407457                                                       |
| 35721 | 1.744100              | 2.407461                                                       |
| 35723 | 1.011113              | 2.407465                                                       |
| 35725 | 1.240868              | 2.407469                                                       |
| 35727 | 1.333445              | 2.407473                                                       |
| 35729 | 1.000028              | 2.407478                                                       |
| 35731 | 1.000028              | 2.407482                                                       |
| 35733 | 1.369267              | 2.407486                                                       |
| 35735 | 1.372772              | 2.407490                                                       |
| 35737 | 1.077315              | 2.407494                                                       |
| 35739 | 1.663057              | 2.407498                                                       |
| 35741 | 1.012619              | 2.407502                                                       |

| $n$   | $\frac{\sigma(n)}{n}$ | $\frac{e^\gamma}{2} \log \log n + \frac{0.73...}{\log \log n}$ |
|-------|-----------------------|----------------------------------------------------------------|
| 35743 | 1.033153              | 2.407506                                                       |
| 35745 | 1.600671              | 2.407510                                                       |
| 35747 | 1.000028              | 2.407514                                                       |
| 35749 | 1.143081              | 2.407518                                                       |
| 35751 | 1.413779              | 2.407522                                                       |
| 35753 | 1.000028              | 2.407526                                                       |
| 35755 | 1.200168              | 2.407530                                                       |
| 35757 | 1.505160              | 2.407534                                                       |
| 35759 | 1.000028              | 2.407538                                                       |
| 35761 | 1.091245              | 2.407542                                                       |
| 35763 | 1.653553              | 2.407546                                                       |
| 35765 | 1.256200              | 2.407550                                                       |
| 35767 | 1.022619              | 2.407554                                                       |
| 35769 | 1.333445              | 2.407558                                                       |
| 35771 | 1.000028              | 2.407562                                                       |
| 35773 | 1.014396              | 2.407566                                                       |
| 35775 | 1.871698              | 2.407570                                                       |
| 35777 | 1.207480              | 2.407574                                                       |
| 35779 | 1.028089              | 2.407578                                                       |
| 35781 | 1.333445              | 2.407582                                                       |
| 35783 | 1.091244              | 2.407587                                                       |
| 35785 | 1.273606              | 2.407591                                                       |
| 35787 | 1.359153              | 2.407595                                                       |
| 35789 | 1.077314              | 2.407599                                                       |
| 35791 | 1.143081              | 2.407603                                                       |
| 35793 | 1.494929              | 2.407607                                                       |
| 35795 | 1.200168              | 2.407611                                                       |
| 35797 | 1.000028              | 2.407615                                                       |
| 35799 | 1.333445              | 2.407619                                                       |
| 35801 | 1.000028              | 2.407623                                                       |
| 35803 | 1.000028              | 2.407627                                                       |
| 35805 | 2.059154              | 2.407631                                                       |
| 35807 | 1.018125              | 2.407635                                                       |
| 35809 | 1.000028              | 2.407639                                                       |
| 35811 | 1.515959              | 2.407643                                                       |
| 35813 | 1.018625              | 2.407647                                                       |
| 35815 | 1.407232              | 2.407651                                                       |
| 35817 | 1.333445              | 2.407655                                                       |
| 35819 | 1.260337              | 2.407659                                                       |
| 35821 | 1.012032              | 2.407663                                                       |
| 35823 | 1.333445              | 2.407667                                                       |
| 35825 | 1.240865              | 2.407671                                                       |
| 35827 | 1.091244              | 2.407675                                                       |
| 35829 | 1.482598              | 2.407679                                                       |

| $n$   | $\frac{\sigma(n)}{n}$ | $\frac{e^\gamma}{2} \log \log n + \frac{0.73...}{\log \log n}$ |
|-------|-----------------------|----------------------------------------------------------------|
| 35831 | 1.000028              | 2.407683                                                       |
| 35833 | 1.143080              | 2.407687                                                       |
| 35835 | 1.600670              | 2.407691                                                       |
| 35837 | 1.000028              | 2.407695                                                       |
| 35839 | 1.000028              | 2.407699                                                       |
| 35841 | 1.437460              | 2.407703                                                       |
| 35843 | 1.015763              | 2.407707                                                       |
| 35845 | 1.229293              | 2.407711                                                       |
| 35847 | 1.653695              | 2.407715                                                       |
| 35849 | 1.091244              | 2.407719                                                       |
| 35851 | 1.000028              | 2.407723                                                       |
| 35853 | 1.526232              | 2.407728                                                       |
| 35855 | 1.228950              | 2.407732                                                       |
| 35857 | 1.044148              | 2.407736                                                       |
| 35859 | 1.333445              | 2.407740                                                       |
| 35861 | 1.177881              | 2.407744                                                       |
| 35863 | 1.000028              | 2.407748                                                       |
| 35865 | 1.735508              | 2.407752                                                       |
| 35867 | 1.124153              | 2.407756                                                       |
| 35869 | 1.000028              | 2.407760                                                       |
| 35871 | 1.455884              | 2.407764                                                       |
| 35873 | 1.035319              | 2.407768                                                       |
| 35875 | 1.461073              | 2.407772                                                       |
| 35877 | 1.333445              | 2.407776                                                       |
| 35879 | 1.000028              | 2.407780                                                       |
| 35881 | 1.020373              | 2.407784                                                       |
| 35883 | 1.497199              | 2.407788                                                       |
| 35885 | 1.200167              | 2.407792                                                       |
| 35887 | 1.059325              | 2.407796                                                       |
| 35889 | 1.524701              | 2.407800                                                       |
| 35891 | 1.053189              | 2.407804                                                       |
| 35893 | 1.179506              | 2.407808                                                       |
| 35895 | 1.600669              | 2.407812                                                       |
| 35897 | 1.000028              | 2.407816                                                       |
| 35899 | 1.000028              | 2.407820                                                       |
| 35901 | 1.444807              | 2.407824                                                       |
| 35903 | 1.197894              | 2.407828                                                       |
| 35905 | 1.235260              | 2.407832                                                       |
| 35907 | 1.333445              | 2.407836                                                       |
| 35909 | 1.010889              | 2.407840                                                       |
| 35911 | 1.000028              | 2.407844                                                       |
| 35913 | 1.333445              | 2.407848                                                       |
| 35915 | 1.311096              | 2.407852                                                       |
| 35917 | 1.164852              | 2.407856                                                       |

| $n$   | $\frac{\sigma(n)}{n}$ | $\frac{e^\gamma}{2} \log \log n + \frac{0.73...}{\log \log n}$ |
|-------|-----------------------|----------------------------------------------------------------|
| 35919 | 1.560623              | 2.407860                                                       |
| 35921 | 1.059325              | 2.407864                                                       |
| 35923 | 1.000028              | 2.407868                                                       |
| 35925 | 1.656785              | 2.407872                                                       |
| 35927 | 1.028085              | 2.407876                                                       |
| 35929 | 1.104400              | 2.407880                                                       |
| 35931 | 1.603073              | 2.407884                                                       |
| 35933 | 1.000028              | 2.407888                                                       |
| 35935 | 1.200167              | 2.407892                                                       |
| 35937 | 1.629518              | 2.407896                                                       |
| 35939 | 1.014385              | 2.407900                                                       |
| 35941 | 1.011435              | 2.407904                                                       |
| 35943 | 1.333445              | 2.407908                                                       |
| 35945 | 1.495618              | 2.407912                                                       |
| 35947 | 1.012602              | 2.407916                                                       |
| 35949 | 1.393975              | 2.407920                                                       |
| 35951 | 1.000028              | 2.407924                                                       |
| 35953 | 1.010764              | 2.407928                                                       |
| 35955 | 1.874343              | 2.407932                                                       |
| 35957 | 1.025558              | 2.407936                                                       |
| 35959 | 1.249423              | 2.407940                                                       |
| 35961 | 1.333445              | 2.407944                                                       |
| 35963 | 1.000028              | 2.407948                                                       |
| 35965 | 1.200167              | 2.407952                                                       |
| 35967 | 1.405733              | 2.407957                                                       |
| 35969 | 1.000028              | 2.407961                                                       |
| 35971 | 1.077312              | 2.407965                                                       |
| 35973 | 1.653685              | 2.407969                                                       |
| 35975 | 1.240862              | 2.407973                                                       |
| 35977 | 1.000028              | 2.407977                                                       |
| 35979 | 1.360794              | 2.407981                                                       |
| 35981 | 1.091243              | 2.407985                                                       |
| 35983 | 1.000028              | 2.407989                                                       |
| 35985 | 1.600667              | 2.407993                                                       |
| 35987 | 1.176425              | 2.407997                                                       |
| 35989 | 1.110339              | 2.408001                                                       |
| 35991 | 1.564836              | 2.408005                                                       |
| 35993 | 1.000028              | 2.408009                                                       |
| 35995 | 1.256174              | 2.408013                                                       |
| 35997 | 1.464122              | 2.408017                                                       |
| 35999 | 1.000028              | 2.408021                                                       |
| 36001 | 1.182189              | 2.408025                                                       |
| 36003 | 1.455879              | 2.408029                                                       |
| 36005 | 1.266491              | 2.408033                                                       |

| $n$   | $\frac{\sigma(n)}{n}$ | $\frac{e^\gamma}{2} \log \log n + \frac{0.73...}{\log \log n}$ |
|-------|-----------------------|----------------------------------------------------------------|
| 36007 | 1.000028              | 2.408037                                                       |
| 36009 | 1.444805              | 2.408041                                                       |
| 36011 | 1.000028              | 2.408045                                                       |
| 36013 | 1.000028              | 2.408049                                                       |
| 36015 | 1.866556              | 2.408053                                                       |
| 36017 | 1.000028              | 2.408057                                                       |
| 36019 | 1.010578              | 2.408061                                                       |
| 36021 | 1.333444              | 2.408065                                                       |
| 36023 | 1.147267              | 2.408069                                                       |
| 36025 | 1.363053              | 2.408073                                                       |
| 36027 | 1.444805              | 2.408077                                                       |
| 36029 | 1.143079              | 2.408081                                                       |
| 36031 | 1.011129              | 2.408085                                                       |
| 36033 | 1.333444              | 2.408089                                                       |
| 36035 | 1.200167              | 2.408093                                                       |
| 36037 | 1.000028              | 2.408097                                                       |
| 36039 | 1.370515              | 2.408101                                                       |
| 36041 | 1.044144              | 2.408105                                                       |
| 36043 | 1.207447              | 2.408109                                                       |
| 36045 | 1.812734              | 2.408113                                                       |
| 36047 | 1.138514              | 2.408117                                                       |
| 36049 | 1.118478              | 2.408121                                                       |
| 36051 | 1.362070              | 2.408125                                                       |
| 36053 | 1.033146              | 2.408129                                                       |
| 36055 | 1.200166              | 2.408133                                                       |
| 36057 | 1.629420              | 2.408137                                                       |
| 36059 | 1.012341              | 2.408141                                                       |
| 36061 | 1.000028              | 2.408145                                                       |
| 36063 | 1.444805              | 2.408149                                                       |
| 36065 | 1.200166              | 2.408153                                                       |
| 36067 | 1.000028              | 2.408157                                                       |
| 36069 | 1.455876              | 2.408161                                                       |
| 36071 | 1.143079              | 2.408165                                                       |
| 36073 | 1.000028              | 2.408169                                                       |
| 36075 | 1.828635              | 2.408173                                                       |
| 36077 | 1.024475              | 2.408177                                                       |
| 36079 | 1.012223              | 2.408181                                                       |
| 36081 | 1.527674              | 2.408185                                                       |
| 36083 | 1.000028              | 2.408189                                                       |
| 36085 | 1.372759              | 2.408193                                                       |
| 36087 | 1.393965              | 2.408197                                                       |
| 36089 | 1.010834              | 2.408201                                                       |
| 36091 | 1.161065              | 2.408205                                                       |
| 36093 | 1.364475              | 2.408209                                                       |



| $n$   | $\frac{\sigma(n)}{n}$ | $\frac{e^\gamma}{2} \log \log n + \frac{0.73\dots}{\log \log n}$ |
|-------|-----------------------|------------------------------------------------------------------|
| 36095 | 1.200166              | 2.408213                                                         |
| 36097 | 1.000028              | 2.408217                                                         |
| 36099 | 1.701986              | 2.408221                                                         |
| 36101 | 1.077311              | 2.408225                                                         |
| 36103 | 1.014874              | 2.408229                                                         |
| 36105 | 1.675114              | 2.408233                                                         |
| 36107 | 1.000028              | 2.408237                                                         |
| 36109 | 1.000028              | 2.408241                                                         |
| 36111 | 1.333444              | 2.408245                                                         |
| 36113 | 1.287957              | 2.408249                                                         |
| 36115 | 1.244026              | 2.408253                                                         |
| 36117 | 1.444804              | 2.408257                                                         |
| 36119 | 1.053185              | 2.408261                                                         |
| 36121 | 1.025553              | 2.408265                                                         |
| 36123 | 1.333444              | 2.408269                                                         |
| 36125 | 1.325730              | 2.408273                                                         |
| 36127 | 1.233869              | 2.408277                                                         |
| 36129 | 1.333444              | 2.408281                                                         |
| 36131 | 1.000028              | 2.408285                                                         |
| 36133 | 1.044142              | 2.408289                                                         |
| 36135 | 1.916812              | 2.408293                                                         |
| 36137 | 1.000028              | 2.408297                                                         |
| 36139 | 1.016077              | 2.408301                                                         |
| 36141 | 1.524695              | 2.408305                                                         |
| 36143 | 1.022605              | 2.408309                                                         |
| 36145 | 1.200166              | 2.408312                                                         |
| 36147 | 1.333444              | 2.408316                                                         |
| 36149 | 1.028078              | 2.408320                                                         |
| 36151 | 1.000028              | 2.408324                                                         |
| 36153 | 1.610931              | 2.408328                                                         |
| 36155 | 1.372756              | 2.408332                                                         |
| 36157 | 1.154963              | 2.408336                                                         |
| 36159 | 1.413756              | 2.408340                                                         |
| 36161 | 1.000028              | 2.408344                                                         |
| 36163 | 1.059757              | 2.408348                                                         |
| 36165 | 1.600664              | 2.408352                                                         |
| 36167 | 1.018608              | 2.408356                                                         |
| 36169 | 1.143078              | 2.408360                                                         |
| 36171 | 1.444804              | 2.408364                                                         |
| 36173 | 1.018107              | 2.408368                                                         |
| 36175 | 1.240857              | 2.408372                                                         |
| 36177 | 1.379882              | 2.408376                                                         |
| 36179 | 1.235192              | 2.408380                                                         |
| 36181 | 1.013018              | 2.408384                                                         |

| $n$   | $\frac{\sigma(n)}{n}$ | $\frac{e^\gamma}{2} \log \log n + \frac{0.73\dots}{\log \log n}$ |
|-------|-----------------------|------------------------------------------------------------------|
| 36183 | 1.524694              | 2.408388                                                         |
| 36185 | 1.200166              | 2.408392                                                         |
| 36187 | 1.000028              | 2.408396                                                         |
| 36189 | 1.444804              | 2.408400                                                         |
| 36191 | 1.000028              | 2.408404                                                         |
| 36193 | 1.059321              | 2.408408                                                         |
| 36195 | 1.697472              | 2.408412                                                         |
| 36197 | 1.143078              | 2.408416                                                         |
| 36199 | 1.020360              | 2.408420                                                         |
| 36201 | 1.455871              | 2.408424                                                         |
| 36203 | 1.025550              | 2.408428                                                         |
| 36205 | 1.294628              | 2.408432                                                         |
| 36207 | 1.507996              | 2.408436                                                         |
| 36209 | 1.000028              | 2.408440                                                         |
| 36211 | 1.164839              | 2.408444                                                         |
| 36213 | 1.333444              | 2.408448                                                         |
| 36215 | 1.200166              | 2.408452                                                         |
| 36217 | 1.000028              | 2.408456                                                         |
| 36219 | 1.333444              | 2.408460                                                         |
| 36221 | 1.035311              | 2.408464                                                         |
| 36223 | 1.132982              | 2.408468                                                         |
| 36225 | 2.135983              | 2.408472                                                         |
| 36227 | 1.059320              | 2.408476                                                         |
| 36229 | 1.000028              | 2.408480                                                         |
| 36231 | 1.437443              | 2.408484                                                         |
| 36233 | 1.053184              | 2.408488                                                         |
| 36235 | 1.200166              | 2.408492                                                         |
| 36237 | 1.367001              | 2.408496                                                         |
| 36239 | 1.186788              | 2.408500                                                         |
| 36241 | 1.000028              | 2.408504                                                         |
| 36243 | 1.444803              | 2.408508                                                         |
| 36245 | 1.311077              | 2.408512                                                         |
| 36247 | 1.016801              | 2.408516                                                         |
| 36249 | 1.369196              | 2.408520                                                         |
| 36251 | 1.000028              | 2.408524                                                         |
| 36253 | 1.143078              | 2.408528                                                         |
| 36255 | 1.600662              | 2.408532                                                         |
| 36257 | 1.077309              | 2.408536                                                         |
| 36259 | 1.012714              | 2.408539                                                         |
| 36261 | 1.588483              | 2.408543                                                         |
| 36263 | 1.000028              | 2.408547                                                         |
| 36265 | 1.200165              | 2.408551                                                         |
| 36267 | 1.672926              | 2.408555                                                         |
| 36269 | 1.000028              | 2.408559                                                         |

| $n$   | $\frac{\sigma(n)}{n}$ | $\frac{e^\gamma}{2} \log \log n + \frac{0.73...}{\log \log n}$ |
|-------|-----------------------|----------------------------------------------------------------|
| 36271 | 1.111632              | 2.408563                                                       |
| 36273 | 1.357704              | 2.408567                                                       |
| 36275 | 1.240855              | 2.408571                                                       |
| 36277 | 1.000028              | 2.408575                                                       |
| 36279 | 1.505003              | 2.408579                                                       |
| 36281 | 1.174830              | 2.408583                                                       |
| 36283 | 1.077309              | 2.408587                                                       |
| 36285 | 1.666804              | 2.408591                                                       |
| 36287 | 1.011271              | 2.408595                                                       |
| 36289 | 1.091240              | 2.408599                                                       |
| 36291 | 1.333444              | 2.408603                                                       |
| 36293 | 1.000028              | 2.408607                                                       |
| 36295 | 1.475906              | 2.408611                                                       |
| 36297 | 1.497093              | 2.408615                                                       |
| 36299 | 1.000028              | 2.408619                                                       |
| 36301 | 1.033140              | 2.408623                                                       |
| 36303 | 1.333444              | 2.408627                                                       |
| 36305 | 1.231566              | 2.408631                                                       |
| 36307 | 1.000028              | 2.408635                                                       |
| 36309 | 1.758242              | 2.408639                                                       |
| 36311 | 1.091240              | 2.408643                                                       |
| 36313 | 1.000028              | 2.408647                                                       |
| 36315 | 1.784387              | 2.408651                                                       |
| 36317 | 1.044139              | 2.408655                                                       |
| 36319 | 1.000028              | 2.408659                                                       |
| 36321 | 1.333443              | 2.408663                                                       |
| 36323 | 1.143077              | 2.408667                                                       |
| 36325 | 1.240853              | 2.408671                                                       |
| 36327 | 1.333443              | 2.408675                                                       |
| 36329 | 1.059319              | 2.408679                                                       |
| 36331 | 1.022598              | 2.408682                                                       |
| 36333 | 1.580051              | 2.408686                                                       |
| 36335 | 1.329627              | 2.408690                                                       |
| 36337 | 1.188871              | 2.408694                                                       |
| 36339 | 1.333443              | 2.408698                                                       |
| 36341 | 1.000028              | 2.408702                                                       |
| 36343 | 1.000028              | 2.408706                                                       |
| 36345 | 1.600660              | 2.408710                                                       |
| 36347 | 1.053182              | 2.408714                                                       |
| 36349 | 1.010647              | 2.408718                                                       |
| 36351 | 1.653655              | 2.408722                                                       |
| 36353 | 1.000028              | 2.408726                                                       |
| 36355 | 1.311071              | 2.408730                                                       |
| 36357 | 1.333443              | 2.408734                                                       |

| $n$   | $\frac{\sigma(n)}{n}$ | $\frac{e^\gamma}{2} \log \log n + \frac{0.73...}{\log \log n}$ |
|-------|-----------------------|----------------------------------------------------------------|
| 36359 | 1.012569              | 2.408738                                                       |
| 36361 | 1.077308              | 2.408742                                                       |
| 36363 | 1.520667              | 2.408746                                                       |
| 36365 | 1.372749              | 2.408750                                                       |
| 36367 | 1.025545              | 2.408754                                                       |
| 36369 | 1.497154              | 2.408758                                                       |
| 36371 | 1.028072              | 2.408762                                                       |
| 36373 | 1.000027              | 2.408766                                                       |
| 36375 | 1.681155              | 2.408770                                                       |
| 36377 | 1.091239              | 2.408774                                                       |
| 36379 | 1.143077              | 2.408778                                                       |
| 36381 | 1.360710              | 2.408782                                                       |
| 36383 | 1.000027              | 2.408786                                                       |
| 36385 | 1.266456              | 2.408789                                                       |
| 36387 | 1.560557              | 2.408793                                                       |
| 36389 | 1.000027              | 2.408797                                                       |
| 36391 | 1.010799              | 2.408801                                                       |
| 36393 | 1.524689              | 2.408805                                                       |
| 36395 | 1.246325              | 2.408809                                                       |
| 36397 | 1.059318              | 2.408813                                                       |
| 36399 | 1.455864              | 2.408817                                                       |
| 36401 | 1.013708              | 2.408821                                                       |
| 36403 | 1.018597              | 2.408825                                                       |
| 36405 | 1.735476              | 2.408829                                                       |
| 36407 | 1.164831              | 2.408833                                                       |
| 36409 | 1.044137              | 2.408837                                                       |
| 36411 | 1.364423              | 2.408841                                                       |
| 36413 | 1.077308              | 2.408845                                                       |
| 36415 | 1.200165              | 2.408849                                                       |
| 36417 | 1.362001              | 2.408853                                                       |
| 36419 | 1.014855              | 2.408857                                                       |
| 36421 | 1.285412              | 2.408861                                                       |
| 36423 | 1.581418              | 2.408865                                                       |
| 36425 | 1.307234              | 2.408869                                                       |
| 36427 | 1.015730              | 2.408873                                                       |
| 36429 | 1.333443              | 2.408877                                                       |
| 36431 | 1.059318              | 2.408881                                                       |
| 36433 | 1.000027              | 2.408884                                                       |
| 36435 | 1.833841              | 2.408888                                                       |
| 36437 | 1.014354              | 2.408892                                                       |
| 36439 | 1.077307              | 2.408896                                                       |
| 36441 | 1.444801              | 2.408900                                                       |
| 36443 | 1.091238              | 2.408904                                                       |
| 36445 | 1.238688              | 2.408908                                                       |

| $n$   | $\frac{\sigma(n)}{n}$ | $\frac{e^\gamma}{2} \log \log n + \frac{0.73\dots}{\log \log n}$ |
|-------|-----------------------|------------------------------------------------------------------|
| 36447 | 1.333443              | 2.408912                                                         |
| 36449 | 1.179950              | 2.408916                                                         |
| 36451 | 1.000027              | 2.408920                                                         |
| 36453 | 1.382602              | 2.408924                                                         |
| 36455 | 1.256124              | 2.408928                                                         |
| 36457 | 1.000027              | 2.408932                                                         |
| 36459 | 1.444801              | 2.408936                                                         |
| 36461 | 1.065851              | 2.408940                                                         |
| 36463 | 1.143077              | 2.408944                                                         |
| 36465 | 1.990292              | 2.408948                                                         |
| 36467 | 1.000027              | 2.408952                                                         |
| 36469 | 1.000027              | 2.408956                                                         |
| 36471 | 1.333443              | 2.408960                                                         |
| 36473 | 1.000027              | 2.408964                                                         |
| 36475 | 1.240850              | 2.408967                                                         |
| 36477 | 1.701894              | 2.408971                                                         |
| 36479 | 1.000027              | 2.408975                                                         |
| 36481 | 1.005263              | 2.408979                                                         |
| 36483 | 1.333443              | 2.408983                                                         |
| 36485 | 1.200164              | 2.408987                                                         |
| 36487 | 1.136624              | 2.408991                                                         |
| 36489 | 1.333443              | 2.408995                                                         |
| 36491 | 1.233838              | 2.408999                                                         |
| 36493 | 1.000027              | 2.409003                                                         |
| 36495 | 1.735471              | 2.409007                                                         |
| 36497 | 1.000027              | 2.409011                                                         |
| 36499 | 1.124414              | 2.409015                                                         |
| 36501 | 1.393934              | 2.409019                                                         |
| 36503 | 1.010547              | 2.409023                                                         |
| 36505 | 1.405287              | 2.409027                                                         |
| 36507 | 1.369162              | 2.409031                                                         |
| 36509 | 1.091238              | 2.409035                                                         |
| 36511 | 1.035304              | 2.409039                                                         |
| 36513 | 1.444800              | 2.409043                                                         |
| 36515 | 1.229084              | 2.409046                                                         |
| 36517 | 1.097626              | 2.409050                                                         |
| 36519 | 1.598291              | 2.409054                                                         |
| 36521 | 1.018592              | 2.409058                                                         |
| 36523 | 1.000027              | 2.409062                                                         |
| 36525 | 1.656728              | 2.409066                                                         |
| 36527 | 1.000027              | 2.409070                                                         |
| 36529 | 1.000027              | 2.409074                                                         |
| 36531 | 1.669377              | 2.409078                                                         |
| 36533 | 1.214026              | 2.409082                                                         |

| $n$   | $\frac{\sigma(n)}{n}$ | $\frac{e^\gamma}{2} \log \log n + \frac{0.73...}{\log \log n}$ |
|-------|-----------------------|----------------------------------------------------------------|
| 36535 | 1.200164              | 2.409086                                                       |
| 36537 | 1.405698              | 2.409090                                                       |
| 36539 | 1.018090              | 2.409094                                                       |
| 36541 | 1.000027              | 2.409098                                                       |
| 36543 | 1.437430              | 2.409102                                                       |
| 36545 | 1.200164              | 2.409106                                                       |
| 36547 | 1.197800              | 2.409110                                                       |
| 36549 | 1.502421              | 2.409113                                                       |
| 36551 | 1.000027              | 2.409117                                                       |
| 36553 | 1.091237              | 2.409121                                                       |
| 36555 | 1.600657              | 2.409125                                                       |
| 36557 | 1.011024              | 2.409129                                                       |
| 36559 | 1.000027              | 2.409133                                                       |
| 36561 | 1.524685              | 2.409137                                                       |
| 36563 | 1.000027              | 2.409141                                                       |
| 36565 | 1.228716              | 2.409145                                                       |
| 36567 | 1.535811              | 2.409149                                                       |
| 36569 | 1.125543              | 2.409153                                                       |
| 36571 | 1.000027              | 2.409157                                                       |
| 36573 | 1.359692              | 2.409161                                                       |
| 36575 | 1.627341              | 2.409165                                                       |
| 36577 | 1.014845              | 2.409169                                                       |
| 36579 | 1.358156              | 2.409173                                                       |
| 36581 | 1.010689              | 2.409177                                                       |
| 36583 | 1.000027              | 2.409180                                                       |
| 36585 | 1.784338              | 2.409184                                                       |
| 36587 | 1.000027              | 2.409188                                                       |
| 36589 | 1.143076              | 2.409192                                                       |
| 36591 | 1.333443              | 2.409196                                                       |
| 36593 | 1.096603              | 2.409200                                                       |
| 36595 | 1.294603              | 2.409204                                                       |
| 36597 | 1.455857              | 2.409208                                                       |
| 36599 | 1.000027              | 2.409212                                                       |
| 36601 | 1.059315              | 2.409216                                                       |
| 36603 | 1.700516              | 2.409220                                                       |
| 36605 | 1.200164              | 2.409224                                                       |
| 36607 | 1.000027              | 2.409228                                                       |
| 36609 | 1.333443              | 2.409232                                                       |
| 36611 | 1.033132              | 2.409236                                                       |
| 36613 | 1.101248              | 2.409240                                                       |
| 36615 | 1.600655              | 2.409243                                                       |
| 36617 | 1.143076              | 2.409247                                                       |
| 36619 | 1.091237              | 2.409251                                                       |
| 36621 | 1.560525              | 2.409255                                                       |

| $n$   | $\frac{\sigma(n)}{n}$ | $\frac{e^\gamma}{2} \log \log n + \frac{0.73...}{\log \log n}$ |
|-------|-----------------------|----------------------------------------------------------------|
| 36623 | 1.020342              | 2.409259                                                       |
| 36625 | 1.252259              | 2.409263                                                       |
| 36627 | 1.382587              | 2.409267                                                       |
| 36629 | 1.000027              | 2.409271                                                       |
| 36631 | 1.143076              | 2.409275                                                       |
| 36633 | 1.333443              | 2.409279                                                       |
| 36635 | 1.273536              | 2.409283                                                       |
| 36637 | 1.000027              | 2.409287                                                       |
| 36639 | 1.572095              | 2.409291                                                       |
| 36641 | 1.091237              | 2.409295                                                       |
| 36643 | 1.000027              | 2.409298                                                       |
| 36645 | 1.833811              | 2.409302                                                       |
| 36647 | 1.077305              | 2.409306                                                       |
| 36649 | 1.016781              | 2.409310                                                       |
| 36651 | 1.405692              | 2.409314                                                       |
| 36653 | 1.000027              | 2.409318                                                       |
| 36655 | 1.200164              | 2.409322                                                       |
| 36657 | 1.444799              | 2.409326                                                       |
| 36659 | 1.143075              | 2.409330                                                       |
| 36661 | 1.018085              | 2.409334                                                       |
| 36663 | 1.480075              | 2.409338                                                       |
| 36665 | 1.200164              | 2.409342                                                       |
| 36667 | 1.028063              | 2.409346                                                       |
| 36669 | 1.413728              | 2.409350                                                       |
| 36671 | 1.000027              | 2.409353                                                       |
| 36673 | 1.277452              | 2.409357                                                       |
| 36675 | 1.802100              | 2.409361                                                       |
| 36677 | 1.000027              | 2.409365                                                       |
| 36679 | 1.024455              | 2.409369                                                       |
| 36681 | 1.333442              | 2.409373                                                       |
| 36683 | 1.000027              | 2.409377                                                       |
| 36685 | 1.413112              | 2.409381                                                       |
| 36687 | 1.524682              | 2.409385                                                       |
| 36689 | 1.053177              | 2.409389                                                       |
| 36691 | 1.000027              | 2.409393                                                       |
| 36693 | 1.507863              | 2.409397                                                       |
| 36695 | 1.236136              | 2.409401                                                       |
| 36697 | 1.000027              | 2.409405                                                       |
| 36699 | 1.437423              | 2.409408                                                       |
| 36701 | 1.177080              | 2.409412                                                       |
| 36703 | 1.070648              | 2.409416                                                       |
| 36705 | 1.600654              | 2.409420                                                       |
| 36707 | 1.129812              | 2.409424                                                       |
| 36709 | 1.000027              | 2.409428                                                       |

| $n$   | $\frac{\sigma(n)}{n}$ | $\frac{e^\gamma}{2} \log \log n + \frac{0.73\dots}{\log \log n}$ |
|-------|-----------------------|------------------------------------------------------------------|
| 36711 | 1.444799              | 2.409432                                                         |
| 36713 | 1.000027              | 2.409436                                                         |
| 36715 | 1.372736              | 2.409440                                                         |
| 36717 | 1.333442              | 2.409444                                                         |
| 36719 | 1.015714              | 2.409448                                                         |
| 36721 | 1.000027              | 2.409452                                                         |
| 36723 | 1.333442              | 2.409456                                                         |
| 36725 | 1.347202              | 2.409459                                                         |
| 36727 | 1.053176              | 2.409463                                                         |
| 36729 | 1.834844              | 2.409467                                                         |
| 36731 | 1.044132              | 2.409471                                                         |
| 36733 | 1.012169              | 2.409475                                                         |
| 36735 | 1.672519              | 2.409479                                                         |
| 36737 | 1.059313              | 2.409483                                                         |
| 36739 | 1.000027              | 2.409487                                                         |
| 36741 | 1.373506              | 2.409491                                                         |
| 36743 | 1.188798              | 2.409495                                                         |
| 36745 | 1.200163              | 2.409499                                                         |
| 36747 | 1.482570              | 2.409503                                                         |
| 36749 | 1.000027              | 2.409506                                                         |
| 36751 | 1.179396              | 2.409510                                                         |
| 36753 | 1.333442              | 2.409514                                                         |
| 36755 | 1.200163              | 2.409518                                                         |
| 36757 | 1.175286              | 2.409522                                                         |
| 36759 | 1.333442              | 2.409526                                                         |
| 36761 | 1.000027              | 2.409530                                                         |
| 36763 | 1.012975              | 2.409534                                                         |
| 36765 | 1.866993              | 2.409538                                                         |
| 36767 | 1.000027              | 2.409542                                                         |
| 36769 | 1.014333              | 2.409546                                                         |
| 36771 | 1.629110              | 2.409550                                                         |
| 36773 | 1.091235              | 2.409553                                                         |
| 36775 | 1.240843              | 2.409557                                                         |
| 36777 | 1.534872              | 2.409561                                                         |
| 36779 | 1.000027              | 2.409565                                                         |
| 36781 | 1.000027              | 2.409569                                                         |
| 36783 | 1.490036              | 2.409573                                                         |
| 36785 | 1.372733              | 2.409577                                                         |
| 36787 | 1.000027              | 2.409581                                                         |
| 36789 | 1.333442              | 2.409585                                                         |
| 36791 | 1.000027              | 2.409589                                                         |
| 36793 | 1.000027              | 2.409593                                                         |
| 36795 | 1.753282              | 2.409597                                                         |
| 36797 | 1.033128              | 2.409600                                                         |



| $n$   | $\frac{\sigma(n)}{n}$ | $\frac{e^\gamma}{2} \log \log n + \frac{0.73\dots}{\log \log n}$ |
|-------|-----------------------|------------------------------------------------------------------|
| 36799 | 1.164814              | 2.409604                                                         |
| 36801 | 1.565175              | 2.409608                                                         |
| 36803 | 1.141211              | 2.409612                                                         |
| 36805 | 1.273523              | 2.409616                                                         |
| 36807 | 1.333442              | 2.409620                                                         |
| 36809 | 1.000027              | 2.409624                                                         |
| 36811 | 1.011219              | 2.409628                                                         |
| 36813 | 1.524679              | 2.409632                                                         |
| 36815 | 1.238626              | 2.409636                                                         |
| 36817 | 1.091235              | 2.409640                                                         |
| 36819 | 1.444798              | 2.409643                                                         |
| 36821 | 1.000027              | 2.409647                                                         |
| 36823 | 1.044130              | 2.409651                                                         |
| 36825 | 1.656701              | 2.409655                                                         |
| 36827 | 1.143074              | 2.409659                                                         |
| 36829 | 1.077303              | 2.409663                                                         |
| 36831 | 1.333442              | 2.409667                                                         |
| 36833 | 1.000027              | 2.409671                                                         |
| 36835 | 1.231437              | 2.409675                                                         |
| 36837 | 1.444797              | 2.409679                                                         |
| 36839 | 1.160944              | 2.409683                                                         |
| 36841 | 1.207351              | 2.409686                                                         |
| 36843 | 1.333442              | 2.409690                                                         |
| 36845 | 1.200163              | 2.409694                                                         |
| 36847 | 1.000027              | 2.409698                                                         |
| 36849 | 1.359928              | 2.409702                                                         |
| 36851 | 1.024450              | 2.409706                                                         |
| 36853 | 1.011044              | 2.409710                                                         |
| 36855 | 2.206268              | 2.409714                                                         |
| 36857 | 1.000027              | 2.409718                                                         |
| 36859 | 1.093898              | 2.409722                                                         |
| 36861 | 1.455848              | 2.409726                                                         |
| 36863 | 1.010444              | 2.409729                                                         |
| 36865 | 1.228482              | 2.409733                                                         |
| 36867 | 1.333442              | 2.409737                                                         |
| 36869 | 1.197754              | 2.409741                                                         |
| 36871 | 1.000027              | 2.409745                                                         |
| 36873 | 1.535758              | 2.409749                                                         |
| 36875 | 1.270780              | 2.409753                                                         |
| 36877 | 1.000027              | 2.409757                                                         |
| 36879 | 1.405678              | 2.409761                                                         |
| 36881 | 1.077303              | 2.409765                                                         |
| 36883 | 1.249356              | 2.409769                                                         |
| 36885 | 1.600651              | 2.409772                                                         |

| $n$   | $\frac{\sigma(n)}{n}$ | $\frac{e^\gamma}{2} \log \log n + \frac{0.73...}{\log \log n}$ |
|-------|-----------------------|----------------------------------------------------------------|
| 36887 | 1.000027              | 2.409776                                                       |
| 36889 | 1.028057              | 2.409780                                                       |
| 36891 | 1.444797              | 2.409784                                                       |
| 36893 | 1.014827              | 2.409788                                                       |
| 36895 | 1.233338              | 2.409792                                                       |
| 36897 | 1.557200              | 2.409796                                                       |
| 36899 | 1.000027              | 2.409800                                                       |
| 36901 | 1.000027              | 2.409804                                                       |
| 36903 | 1.333442              | 2.409808                                                       |
| 36905 | 1.340631              | 2.409811                                                       |
| 36907 | 1.147099              | 2.409815                                                       |
| 36909 | 1.482565              | 2.409819                                                       |
| 36911 | 1.143074              | 2.409823                                                       |
| 36913 | 1.000027              | 2.409827                                                       |
| 36915 | 1.685169              | 2.409831                                                       |
| 36917 | 1.105182              | 2.409835                                                       |
| 36919 | 1.000027              | 2.409839                                                       |
| 36921 | 1.379811              | 2.409843                                                       |
| 36923 | 1.000027              | 2.409847                                                       |
| 36925 | 1.423859              | 2.409850                                                       |
| 36927 | 1.579982              | 2.409854                                                       |
| 36929 | 1.000027              | 2.409858                                                       |
| 36931 | 1.000027              | 2.409862                                                       |
| 36933 | 1.437414              | 2.409866                                                       |
| 36935 | 1.228103              | 2.409870                                                       |
| 36937 | 1.024447              | 2.409874                                                       |
| 36939 | 1.524676              | 2.409878                                                       |
| 36941 | 1.105114              | 2.409882                                                       |
| 36943 | 1.000027              | 2.409885                                                       |
| 36945 | 1.735445              | 2.409889                                                       |
| 36947 | 1.000027              | 2.409893                                                       |
| 36949 | 1.091234              | 2.409897                                                       |
| 36951 | 1.357473              | 2.409901                                                       |
| 36953 | 1.143074              | 2.409905                                                       |
| 36955 | 1.266405              | 2.409909                                                       |
| 36957 | 1.357686              | 2.409913                                                       |
| 36959 | 1.077302              | 2.409917                                                       |
| 36961 | 1.044128              | 2.409921                                                       |
| 36963 | 1.522604              | 2.409924                                                       |
| 36965 | 1.200162              | 2.409928                                                       |
| 36967 | 1.143074              | 2.409932                                                       |
| 36969 | 1.333442              | 2.409936                                                       |
| 36971 | 1.091234              | 2.409940                                                       |
| 36973 | 1.000027              | 2.409944                                                       |

| $n$   | $\frac{\sigma(n)}{n}$ | $\frac{e^\gamma}{2} \log \log n + \frac{0.73\dots}{\log \log n}$ |
|-------|-----------------------|------------------------------------------------------------------|
| 36975 | 1.810953              | 2.409948                                                         |
| 36977 | 1.012521              | 2.409952                                                         |
| 36979 | 1.000027              | 2.409956                                                         |
| 36981 | 1.653606              | 2.409959                                                         |
| 36983 | 1.033123              | 2.409963                                                         |
| 36985 | 1.294579              | 2.409967                                                         |
| 36987 | 1.333441              | 2.409971                                                         |
| 36989 | 1.022574              | 2.409975                                                         |
| 36991 | 1.016031              | 2.409979                                                         |
| 36993 | 1.557051              | 2.409983                                                         |
| 36995 | 1.405163              | 2.409987                                                         |
| 36997 | 1.000027              | 2.409991                                                         |
| 36999 | 1.444796              | 2.409995                                                         |
| 37001 | 1.010567              | 2.409998                                                         |
| 37003 | 1.000027              | 2.410002                                                         |
| 37005 | 1.600649              | 2.410006                                                         |
| 37007 | 1.044127              | 2.410010                                                         |
| 37009 | 1.213975              | 2.410014                                                         |
| 37011 | 1.463565              | 2.410018                                                         |
| 37013 | 1.000027              | 2.410022                                                         |
| 37015 | 1.311036              | 2.410026                                                         |
| 37017 | 1.497096              | 2.410030                                                         |
| 37019 | 1.000027              | 2.410033                                                         |
| 37021 | 1.000027              | 2.410037                                                         |
| 37023 | 1.597277              | 2.410041                                                         |
| 37025 | 1.240837              | 2.410045                                                         |
| 37027 | 1.018068              | 2.410049                                                         |
| 37029 | 1.333441              | 2.410053                                                         |
| 37031 | 1.053172              | 2.410057                                                         |
| 37033 | 1.035293              | 2.410061                                                         |
| 37035 | 1.735439              | 2.410064                                                         |
| 37037 | 1.378945              | 2.410068                                                         |
| 37039 | 1.000027              | 2.410072                                                         |
| 37041 | 1.333441              | 2.410076                                                         |
| 37043 | 1.059309              | 2.410080                                                         |
| 37045 | 1.243893              | 2.410084                                                         |
| 37047 | 1.364321              | 2.410088                                                         |
| 37049 | 1.000027              | 2.410092                                                         |
| 37051 | 1.174597              | 2.410096                                                         |
| 37053 | 1.515667              | 2.410099                                                         |
| 37055 | 1.200162              | 2.410103                                                         |
| 37057 | 1.000027              | 2.410107                                                         |
| 37059 | 1.455841              | 2.410111                                                         |
| 37061 | 1.000027              | 2.410115                                                         |

| $n$   | $\frac{\sigma(n)}{n}$ | $\frac{e^\gamma}{2} \log \log n + \frac{0.73...}{\log \log n}$ |
|-------|-----------------------|----------------------------------------------------------------|
| 37063 | 1.077301              | 2.410119                                                       |
| 37065 | 1.833752              | 2.410123                                                       |
| 37067 | 1.012653              | 2.410127                                                       |
| 37069 | 1.053171              | 2.410131                                                       |
| 37071 | 1.482560              | 2.410134                                                       |
| 37073 | 1.011194              | 2.410138                                                       |
| 37075 | 1.240836              | 2.410142                                                       |
| 37077 | 1.413707              | 2.410146                                                       |
| 37079 | 1.143073              | 2.410150                                                       |
| 37081 | 1.091233              | 2.410154                                                       |
| 37083 | 1.366880              | 2.410158                                                       |
| 37085 | 1.200162              | 2.410162                                                       |
| 37087 | 1.000027              | 2.410165                                                       |
| 37089 | 1.560463              | 2.410169                                                       |
| 37091 | 1.035292              | 2.410173                                                       |
| 37093 | 1.164802              | 2.410177                                                       |
| 37095 | 1.600647              | 2.410181                                                       |
| 37097 | 1.000027              | 2.410185                                                       |
| 37099 | 1.044125              | 2.410189                                                       |
| 37101 | 1.358454              | 2.410193                                                       |
| 37103 | 1.091233              | 2.410196                                                       |
| 37105 | 1.236060              | 2.410200                                                       |
| 37107 | 1.793732              | 2.410204                                                       |
| 37109 | 1.024442              | 2.410208                                                       |
| 37111 | 1.105872              | 2.410212                                                       |
| 37113 | 1.358015              | 2.410216                                                       |
| 37115 | 1.294571              | 2.410220                                                       |
| 37117 | 1.000027              | 2.410224                                                       |
| 37119 | 1.333441              | 2.410227                                                       |
| 37121 | 1.143073              | 2.410231                                                       |
| 37123 | 1.000027              | 2.410235                                                       |
| 37125 | 2.016970              | 2.410239                                                       |
| 37127 | 1.011016              | 2.410243                                                       |
| 37129 | 1.012255              | 2.410247                                                       |
| 37131 | 1.333441              | 2.410251                                                       |
| 37133 | 1.016023              | 2.410255                                                       |
| 37135 | 1.372721              | 2.410258                                                       |
| 37137 | 1.333441              | 2.410262                                                       |
| 37139 | 1.000027              | 2.410266                                                       |
| 37141 | 1.077300              | 2.410270                                                       |
| 37143 | 1.444794              | 2.410274                                                       |
| 37145 | 1.395612              | 2.410278                                                       |
| 37147 | 1.102754              | 2.410282                                                       |
| 37149 | 1.602197              | 2.410286                                                       |

| $n$   | $\frac{\sigma(n)}{n}$ | $\frac{e^\gamma}{2} \log \log n + \frac{0.73...}{\log \log n}$ |
|-------|-----------------------|----------------------------------------------------------------|
| 37151 | 1.012947              | 2.410289                                                       |
| 37153 | 1.020321              | 2.410293                                                       |
| 37155 | 1.600646              | 2.410297                                                       |
| 37157 | 1.015690              | 2.410301                                                       |
| 37159 | 1.000027              | 2.410305                                                       |
| 37161 | 1.444794              | 2.410309                                                       |
| 37163 | 1.143072              | 2.410313                                                       |
| 37165 | 1.200161              | 2.410317                                                       |
| 37167 | 1.437404              | 2.410320                                                       |
| 37169 | 1.136431              | 2.410324                                                       |
| 37171 | 1.000027              | 2.410328                                                       |
| 37173 | 1.333441              | 2.410332                                                       |
| 37175 | 1.240834              | 2.410336                                                       |
| 37177 | 1.177502              | 2.410340                                                       |
| 37179 | 1.587993              | 2.410344                                                       |
| 37181 | 1.000027              | 2.410348                                                       |
| 37183 | 1.065648              | 2.410351                                                       |
| 37185 | 1.667769              | 2.410355                                                       |
| 37187 | 1.025520              | 2.410359                                                       |
| 37189 | 1.000027              | 2.410363                                                       |
| 37191 | 1.765588              | 2.410367                                                       |
| 37193 | 1.077299              | 2.410371                                                       |
| 37195 | 1.235005              | 2.410375                                                       |
| 37197 | 1.444794              | 2.410378                                                       |
| 37199 | 1.000027              | 2.410382                                                       |
| 37201 | 1.000027              | 2.410386                                                       |
| 37203 | 1.333441              | 2.410390                                                       |
| 37205 | 1.372719              | 2.410394                                                       |
| 37207 | 1.035289              | 2.410398                                                       |
| 37209 | 1.358811              | 2.410402                                                       |
| 37211 | 1.011314              | 2.410406                                                       |
| 37213 | 1.160885              | 2.410409                                                       |
| 37215 | 1.735429              | 2.410413                                                       |
| 37217 | 1.000027              | 2.410417                                                       |
| 37219 | 1.233778              | 2.410421                                                       |
| 37221 | 1.405658              | 2.410425                                                       |
| 37223 | 1.000027              | 2.410429                                                       |
| 37225 | 1.240833              | 2.410433                                                       |
| 37227 | 1.333441              | 2.410436                                                       |
| 37229 | 1.018561              | 2.410440                                                       |
| 37231 | 1.033118              | 2.410444                                                       |
| 37233 | 1.701716              | 2.410448                                                       |
| 37235 | 1.311025              | 2.410452                                                       |
| 37237 | 1.044123              | 2.410456                                                       |

| $n$   | $\frac{\sigma(n)}{n}$ | $\frac{e^\gamma}{2} \log \log n + \frac{0.73\dots}{\log \log n}$ |
|-------|-----------------------|------------------------------------------------------------------|
| 37239 | 1.333441              | 2.410460                                                         |
| 37241 | 1.010499              | 2.410464                                                         |
| 37243 | 1.000027              | 2.410467                                                         |
| 37245 | 1.732098              | 2.410471                                                         |
| 37247 | 1.213950              | 2.410475                                                         |
| 37249 | 1.005208              | 2.410479                                                         |
| 37251 | 1.444793              | 2.410483                                                         |
| 37253 | 1.000027              | 2.410487                                                         |
| 37255 | 1.200161              | 2.410491                                                         |
| 37257 | 1.455834              | 2.410494                                                         |
| 37259 | 1.101479              | 2.410498                                                         |
| 37261 | 1.143072              | 2.410502                                                         |
| 37263 | 1.333441              | 2.410506                                                         |
| 37265 | 1.246210              | 2.410510                                                         |
| 37267 | 1.014302              | 2.410514                                                         |
| 37269 | 1.494325              | 2.410518                                                         |
| 37271 | 1.117866              | 2.410521                                                         |
| 37273 | 1.000027              | 2.410525                                                         |
| 37275 | 1.916137              | 2.410529                                                         |
| 37277 | 1.000027              | 2.410533                                                         |
| 37279 | 1.091231              | 2.410537                                                         |
| 37281 | 1.449317              | 2.410541                                                         |
| 37283 | 1.044122              | 2.410545                                                         |
| 37285 | 1.200161              | 2.410548                                                         |
| 37287 | 1.482554              | 2.410552                                                         |
| 37289 | 1.164794              | 2.410556                                                         |
| 37291 | 1.013649              | 2.410560                                                         |
| 37293 | 1.379776              | 2.410564                                                         |
| 37295 | 1.200161              | 2.410568                                                         |
| 37297 | 1.141111              | 2.410572                                                         |
| 37299 | 1.333441              | 2.410575                                                         |
| 37301 | 1.091231              | 2.410579                                                         |
| 37303 | 1.158727              | 2.410583                                                         |
| 37305 | 1.735424              | 2.410587                                                         |
| 37307 | 1.000027              | 2.410591                                                         |
| 37309 | 1.000027              | 2.410595                                                         |
| 37311 | 1.333441              | 2.410599                                                         |
| 37313 | 1.000027              | 2.410602                                                         |
| 37315 | 1.273483              | 2.410606                                                         |
| 37317 | 1.524667              | 2.410610                                                         |
| 37319 | 1.016748              | 2.410614                                                         |
| 37321 | 1.000027              | 2.410618                                                         |
| 37323 | 1.755486              | 2.410622                                                         |
| 37325 | 1.240831              | 2.410626                                                         |

| $n$   | $\frac{\sigma(n)}{n}$ | $\frac{e^\gamma}{2} \log \log n + \frac{0.73...}{\log \log n}$ |
|-------|-----------------------|----------------------------------------------------------------|
| 37327 | 1.010529              | 2.410629                                                       |
| 37329 | 1.393876              | 2.410633                                                       |
| 37331 | 1.143071              | 2.410637                                                       |
| 37333 | 1.028045              | 2.410641                                                       |
| 37335 | 1.697067              | 2.410645                                                       |
| 37337 | 1.000027              | 2.410649                                                       |
| 37339 | 1.000027              | 2.410653                                                       |
| 37341 | 1.497068              | 2.410656                                                       |
| 37343 | 1.012238              | 2.410660                                                       |
| 37345 | 1.511528              | 2.410664                                                       |
| 37347 | 1.362358              | 2.410668                                                       |
| 37349 | 1.147019              | 2.410672                                                       |
| 37351 | 1.025515              | 2.410676                                                       |
| 37353 | 1.333440              | 2.410679                                                       |
| 37355 | 1.243850              | 2.410683                                                       |
| 37357 | 1.000027              | 2.410687                                                       |
| 37359 | 1.653577              | 2.410691                                                       |
| 37361 | 1.000027              | 2.410695                                                       |
| 37363 | 1.000027              | 2.410699                                                       |
| 37365 | 1.664874              | 2.410703                                                       |
| 37367 | 1.130409              | 2.410706                                                       |
| 37369 | 1.000027              | 2.410710                                                       |
| 37371 | 1.333440              | 2.410714                                                       |
| 37373 | 1.207289              | 2.410718                                                       |
| 37375 | 1.402435              | 2.410722                                                       |
| 37377 | 1.444792              | 2.410726                                                       |
| 37379 | 1.000027              | 2.410729                                                       |
| 37381 | 1.035285              | 2.410733                                                       |
| 37383 | 1.413691              | 2.410737                                                       |
| 37385 | 1.200160              | 2.410741                                                       |
| 37387 | 1.176880              | 2.410745                                                       |
| 37389 | 1.479794              | 2.410749                                                       |
| 37391 | 1.010938              | 2.410753                                                       |
| 37393 | 1.018052              | 2.410756                                                       |
| 37395 | 1.784196              | 2.410760                                                       |
| 37397 | 1.000027              | 2.410764                                                       |
| 37399 | 1.010722              | 2.410768                                                       |
| 37401 | 1.653004              | 2.410772                                                       |
| 37403 | 1.011897              | 2.410776                                                       |
| 37405 | 1.200160              | 2.410779                                                       |
| 37407 | 1.373433              | 2.410783                                                       |
| 37409 | 1.000027              | 2.410787                                                       |
| 37411 | 1.154741              | 2.410791                                                       |
| 37413 | 1.444792              | 2.410795                                                       |

| $n$   | $\frac{\sigma(n)}{n}$ | $\frac{e^\gamma}{2} \log \log n + \frac{0.73\dots}{\log \log n}$ |
|-------|-----------------------|------------------------------------------------------------------|
| 37415 | 1.372711              | 2.410799                                                         |
| 37417 | 1.108373              | 2.410803                                                         |
| 37419 | 1.333440              | 2.410806                                                         |
| 37421 | 1.044120              | 2.410810                                                         |
| 37423 | 1.000027              | 2.410814                                                         |
| 37425 | 1.656647              | 2.410818                                                         |
| 37427 | 1.077297              | 2.410822                                                         |
| 37429 | 1.143071              | 2.410826                                                         |
| 37431 | 1.444792              | 2.410829                                                         |
| 37433 | 1.130981              | 2.410833                                                         |
| 37435 | 1.200160              | 2.410837                                                         |
| 37437 | 1.333440              | 2.410841                                                         |
| 37439 | 1.035284              | 2.410845                                                         |
| 37441 | 1.000027              | 2.410849                                                         |
| 37443 | 1.524664              | 2.410852                                                         |
| 37445 | 1.200160              | 2.410856                                                         |
| 37447 | 1.000027              | 2.410860                                                         |
| 37449 | 1.580817              | 2.410864                                                         |
| 37451 | 1.059304              | 2.410868                                                         |
| 37453 | 1.118415              | 2.410872                                                         |
| 37455 | 1.753144              | 2.410876                                                         |
| 37457 | 1.143071              | 2.410879                                                         |
| 37459 | 1.022558              | 2.410883                                                         |
| 37461 | 1.333440              | 2.410887                                                         |
| 37463 | 1.000027              | 2.410891                                                         |
| 37465 | 1.229948              | 2.410895                                                         |
| 37467 | 1.515574              | 2.410899                                                         |
| 37469 | 1.013638              | 2.410902                                                         |
| 37471 | 1.175949              | 2.410906                                                         |
| 37473 | 1.333440              | 2.410910                                                         |
| 37475 | 1.240827              | 2.410914                                                         |
| 37477 | 1.091229              | 2.410918                                                         |
| 37479 | 1.483711              | 2.410922                                                         |
| 37481 | 1.028041              | 2.410925                                                         |
| 37483 | 1.000027              | 2.410929                                                         |
| 37485 | 2.134934              | 2.410933                                                         |
| 37487 | 1.053165              | 2.410937                                                         |
| 37489 | 1.000027              | 2.410941                                                         |
| 37491 | 1.333440              | 2.410945                                                         |
| 37493 | 1.000027              | 2.410948                                                         |
| 37495 | 1.200160              | 2.410952                                                         |
| 37497 | 1.382511              | 2.410956                                                         |
| 37499 | 1.249313              | 2.410960                                                         |
| 37501 | 1.000027              | 2.410964                                                         |



| $n$   | $\frac{\sigma(n)}{n}$ | $\frac{e^\gamma}{2} \log \log n + \frac{0.73...}{\log \log n}$ |
|-------|-----------------------|----------------------------------------------------------------|
| 37503 | 1.497054              | 2.410968                                                       |
| 37505 | 1.294547              | 2.410971                                                       |
| 37507 | 1.000027              | 2.410975                                                       |
| 37509 | 1.333440              | 2.410979                                                       |
| 37511 | 1.000027              | 2.410983                                                       |
| 37513 | 1.197665              | 2.410987                                                       |
| 37515 | 1.665894              | 2.410991                                                       |
| 37517 | 1.000027              | 2.410994                                                       |
| 37519 | 1.059303              | 2.410998                                                       |
| 37521 | 1.579915              | 2.411002                                                       |
| 37523 | 1.010580              | 2.411006                                                       |
| 37525 | 1.321785              | 2.411010                                                       |
| 37527 | 1.524662              | 2.411014                                                       |
| 37529 | 1.000027              | 2.411017                                                       |
| 37531 | 1.077296              | 2.411021                                                       |
| 37533 | 1.333440              | 2.411025                                                       |
| 37535 | 1.200160              | 2.411029                                                       |
| 37537 | 1.000027              | 2.411033                                                       |
| 37539 | 1.493274              | 2.411037                                                       |
| 37541 | 1.186543              | 2.411040                                                       |
| 37543 | 1.091229              | 2.411044                                                       |
| 37545 | 1.600639              | 2.411048                                                       |
| 37547 | 1.000027              | 2.411052                                                       |
| 37549 | 1.000027              | 2.411056                                                       |
| 37551 | 1.333440              | 2.411060                                                       |
| 37553 | 1.081831              | 2.411063                                                       |
| 37555 | 1.457063              | 2.411067                                                       |
| 37557 | 1.610352              | 2.411071                                                       |
| 37559 | 1.060092              | 2.411075                                                       |
| 37561 | 1.000027              | 2.411079                                                       |
| 37563 | 1.405639              | 2.411082                                                       |
| 37565 | 1.311008              | 2.411086                                                       |
| 37567 | 1.000027              | 2.411090                                                       |
| 37569 | 1.524661              | 2.411094                                                       |
| 37571 | 1.000027              | 2.411098                                                       |
| 37573 | 1.000027              | 2.411102                                                       |
| 37575 | 1.801836              | 2.411105                                                       |
| 37577 | 1.020305              | 2.411109                                                       |
| 37579 | 1.000027              | 2.411113                                                       |
| 37581 | 1.333440              | 2.411117                                                       |
| 37583 | 1.273980              | 2.411121                                                       |
| 37585 | 1.200160              | 2.411125                                                       |
| 37587 | 1.563094              | 2.411128                                                       |
| 37589 | 1.000027              | 2.411132                                                       |

| $n$   | $\frac{\sigma(n)}{n}$ | $\frac{e^\gamma}{2} \log \log n + \frac{0.73...}{\log \log n}$ |
|-------|-----------------------|----------------------------------------------------------------|
| 37591 | 1.000027              | 2.411136                                                       |
| 37593 | 1.444790              | 2.411140                                                       |
| 37595 | 1.228248              | 2.411144                                                       |
| 37597 | 1.179669              | 2.411148                                                       |
| 37599 | 1.358334              | 2.411151                                                       |
| 37601 | 1.053163              | 2.411155                                                       |
| 37603 | 1.033109              | 2.411159                                                       |
| 37605 | 1.684882              | 2.411163                                                       |
| 37607 | 1.000027              | 2.411167                                                       |
| 37609 | 1.179292              | 2.411170                                                       |
| 37611 | 1.701630              | 2.411174                                                       |
| 37613 | 1.035280              | 2.411178                                                       |
| 37615 | 1.200160              | 2.411182                                                       |
| 37617 | 1.333440              | 2.411186                                                       |
| 37619 | 1.000027              | 2.411190                                                       |
| 37621 | 1.059302              | 2.411193                                                       |
| 37623 | 1.333440              | 2.411197                                                       |
| 37625 | 1.459455              | 2.411201                                                       |
| 37627 | 1.010338              | 2.411205                                                       |
| 37629 | 1.496612              | 2.411209                                                       |
| 37631 | 1.102708              | 2.411212                                                       |
| 37633 | 1.000027              | 2.411216                                                       |
| 37635 | 1.732005              | 2.411220                                                       |
| 37637 | 1.018041              | 2.411224                                                       |
| 37639 | 1.207258              | 2.411228                                                       |
| 37641 | 1.333440              | 2.411232                                                       |
| 37643 | 1.000027              | 2.411235                                                       |
| 37645 | 1.200159              | 2.411239                                                       |
| 37647 | 1.491752              | 2.411243                                                       |
| 37649 | 1.000027              | 2.411247                                                       |
| 37651 | 1.044116              | 2.411251                                                       |
| 37653 | 1.672536              | 2.411254                                                       |
| 37655 | 1.273456              | 2.411258                                                       |
| 37657 | 1.000027              | 2.411262                                                       |
| 37659 | 1.333440              | 2.411266                                                       |
| 37661 | 1.077295              | 2.411270                                                       |
| 37663 | 1.000027              | 2.411274                                                       |
| 37665 | 1.855516              | 2.411277                                                       |
| 37667 | 1.143070              | 2.411281                                                       |
| 37669 | 1.010911              | 2.411285                                                       |
| 37671 | 1.382496              | 2.411289                                                       |
| 37673 | 1.012608              | 2.411293                                                       |
| 37675 | 1.362601              | 2.411296                                                       |
| 37677 | 1.405632              | 2.411300                                                       |

| $n$   | $\frac{\sigma(n)}{n}$ | $\frac{e^\gamma}{2} \log \log n + \frac{0.73\dots}{\log \log n}$ |
|-------|-----------------------|------------------------------------------------------------------|
| 37679 | 1.025505              | 2.411304                                                         |
| 37681 | 1.164778              | 2.411308                                                         |
| 37683 | 1.490327              | 2.411312                                                         |
| 37685 | 1.200159              | 2.411316                                                         |
| 37687 | 1.087696              | 2.411319                                                         |
| 37689 | 1.413675              | 2.411323                                                         |
| 37691 | 1.000027              | 2.411327                                                         |
| 37693 | 1.000027              | 2.411331                                                         |
| 37695 | 1.833665              | 2.411335                                                         |
| 37697 | 1.145980              | 2.411338                                                         |
| 37699 | 1.000027              | 2.411342                                                         |
| 37701 | 1.489616              | 2.411346                                                         |
| 37703 | 1.028035              | 2.411350                                                         |
| 37705 | 1.200159              | 2.411354                                                         |
| 37707 | 1.333439              | 2.411357                                                         |
| 37709 | 1.143069              | 2.411361                                                         |
| 37711 | 1.024423              | 2.411365                                                         |
| 37713 | 1.437382              | 2.411369                                                         |
| 37715 | 1.266340              | 2.411373                                                         |
| 37717 | 1.000027              | 2.411376                                                         |
| 37719 | 1.628887              | 2.411380                                                         |
| 37721 | 1.016728              | 2.411384                                                         |
| 37723 | 1.213901              | 2.411388                                                         |
| 37725 | 1.656620              | 2.411392                                                         |
| 37727 | 1.033106              | 2.411396                                                         |
| 37729 | 1.035278              | 2.411399                                                         |
| 37731 | 1.333439              | 2.411403                                                         |
| 37733 | 1.012906              | 2.411407                                                         |
| 37735 | 1.200159              | 2.411411                                                         |
| 37737 | 1.653550              | 2.411415                                                         |
| 37739 | 1.077294              | 2.411418                                                         |
| 37741 | 1.129382              | 2.411422                                                         |
| 37743 | 1.393848              | 2.411426                                                         |
| 37745 | 1.200159              | 2.411430                                                         |
| 37747 | 1.000026              | 2.411434                                                         |
| 37749 | 1.333439              | 2.411437                                                         |
| 37751 | 1.143069              | 2.411441                                                         |
| 37753 | 1.053161              | 2.411445                                                         |
| 37755 | 1.735399              | 2.411449                                                         |
| 37757 | 1.059300              | 2.411453                                                         |
| 37759 | 1.018035              | 2.411456                                                         |
| 37761 | 1.370303              | 2.411460                                                         |
| 37763 | 1.091227              | 2.411464                                                         |
| 37765 | 1.494717              | 2.411468                                                         |

| $n$   | $\frac{\sigma(n)}{n}$ | $\frac{e^\gamma}{2} \log \log n + \frac{0.73...}{\log \log n}$ |
|-------|-----------------------|----------------------------------------------------------------|
| 37767 | 1.333439              | 2.411472                                                       |
| 37769 | 1.010352              | 2.411475                                                       |
| 37771 | 1.012205              | 2.411479                                                       |
| 37773 | 1.482540              | 2.411483                                                       |
| 37775 | 1.240821              | 2.411487                                                       |
| 37777 | 1.028033              | 2.411491                                                       |
| 37779 | 1.557056              | 2.411494                                                       |
| 37781 | 1.000026              | 2.411498                                                       |
| 37783 | 1.000026              | 2.411502                                                       |
| 37785 | 1.753077              | 2.411506                                                       |
| 37787 | 1.035277              | 2.411510                                                       |
| 37789 | 1.097462              | 2.411514                                                       |
| 37791 | 1.733746              | 2.411517                                                       |
| 37793 | 1.143069              | 2.411521                                                       |
| 37795 | 1.200159              | 2.411525                                                       |
| 37797 | 1.368998              | 2.411529                                                       |
| 37799 | 1.000026              | 2.411533                                                       |
| 37801 | 1.012460              | 2.411536                                                       |
| 37803 | 1.333439              | 2.411540                                                       |
| 37805 | 1.200159              | 2.411544                                                       |
| 37807 | 1.249292              | 2.411548                                                       |
| 37809 | 1.444788              | 2.411552                                                       |
| 37811 | 1.000026              | 2.411555                                                       |
| 37813 | 1.000026              | 2.411559                                                       |
| 37815 | 1.600635              | 2.411563                                                       |
| 37817 | 1.077293              | 2.411567                                                       |
| 37819 | 1.018536              | 2.411571                                                       |
| 37821 | 1.524656              | 2.411574                                                       |
| 37823 | 1.012083              | 2.411578                                                       |
| 37825 | 1.327693              | 2.411582                                                       |
| 37827 | 1.497026              | 2.411586                                                       |
| 37829 | 1.154670              | 2.411590                                                       |
| 37831 | 1.000026              | 2.411593                                                       |
| 37833 | 1.333439              | 2.411597                                                       |
| 37835 | 1.461504              | 2.411601                                                       |
| 37837 | 1.010545              | 2.411605                                                       |
| 37839 | 1.333439              | 2.411608                                                       |
| 37841 | 1.014772              | 2.411612                                                       |
| 37843 | 1.118727              | 2.411616                                                       |
| 37845 | 1.795164              | 2.411620                                                       |
| 37847 | 1.000026              | 2.411624                                                       |
| 37849 | 1.143069              | 2.411627                                                       |
| 37851 | 1.542046              | 2.411631                                                       |
| 37853 | 1.000026              | 2.411635                                                       |

| $n$   | $\frac{\sigma(n)}{n}$ | $\frac{e^\gamma}{2} \log \log n + \frac{0.73\dots}{\log \log n}$ |
|-------|-----------------------|------------------------------------------------------------------|
| 37855 | 1.228688              | 2.411639                                                         |
| 37857 | 1.333439              | 2.411643                                                         |
| 37859 | 1.070393              | 2.411646                                                         |
| 37861 | 1.000026              | 2.411650                                                         |
| 37863 | 1.653540              | 2.411654                                                         |
| 37865 | 1.200158              | 2.411658                                                         |
| 37867 | 1.053160              | 2.411662                                                         |
| 37869 | 1.437376              | 2.411665                                                         |
| 37871 | 1.000026              | 2.411669                                                         |
| 37873 | 1.102685              | 2.411673                                                         |
| 37875 | 1.680475              | 2.411677                                                         |
| 37877 | 1.164770              | 2.411681                                                         |
| 37879 | 1.000026              | 2.411684                                                         |
| 37881 | 1.571236              | 2.411688                                                         |
| 37883 | 1.024417              | 2.411692                                                         |
| 37885 | 1.200158              | 2.411696                                                         |
| 37887 | 1.359411              | 2.411700                                                         |
| 37889 | 1.000026              | 2.411703                                                         |
| 37891 | 1.143068              | 2.411707                                                         |
| 37893 | 1.413665              | 2.411711                                                         |
| 37895 | 1.436390              | 2.411715                                                         |
| 37897 | 1.000026              | 2.411718                                                         |
| 37899 | 1.444787              | 2.411722                                                         |
| 37901 | 1.010633              | 2.411726                                                         |
| 37903 | 1.035274              | 2.411730                                                         |
| 37905 | 1.929877              | 2.411734                                                         |
| 37907 | 1.000026              | 2.411737                                                         |
| 37909 | 1.010420              | 2.411741                                                         |
| 37911 | 1.333439              | 2.411745                                                         |
| 37913 | 1.033102              | 2.411749                                                         |
| 37915 | 1.200158              | 2.411753                                                         |
| 37917 | 1.579872              | 2.411756                                                         |
| 37919 | 1.143068              | 2.411760                                                         |
| 37921 | 1.077292              | 2.411764                                                         |
| 37923 | 1.333439              | 2.411768                                                         |
| 37925 | 1.304575              | 2.411772                                                         |
| 37927 | 1.116250              | 2.411775                                                         |
| 37929 | 1.366764              | 2.411779                                                         |
| 37931 | 1.014263              | 2.411783                                                         |
| 37933 | 1.143068              | 2.411787                                                         |
| 37935 | 1.784104              | 2.411790                                                         |
| 37937 | 1.018531              | 2.411794                                                         |
| 37939 | 1.091225              | 2.411798                                                         |
| 37941 | 1.333439              | 2.411802                                                         |

| $n$   | $\frac{\sigma(n)}{n}$ | $\frac{e^\gamma}{2} \log \log n + \frac{0.73...}{\log \log n}$ |
|-------|-----------------------|----------------------------------------------------------------|
| 37943 | 1.053159              | 2.411806                                                       |
| 37945 | 1.200158              | 2.411809                                                       |
| 37947 | 1.652832              | 2.411813                                                       |
| 37949 | 1.010936              | 2.411817                                                       |
| 37951 | 1.000026              | 2.411821                                                       |
| 37953 | 1.444787              | 2.411825                                                       |
| 37955 | 1.200158              | 2.411828                                                       |
| 37957 | 1.000026              | 2.411832                                                       |
| 37959 | 1.333439              | 2.411836                                                       |
| 37961 | 1.365612              | 2.411840                                                       |
| 37963 | 1.000026              | 2.411843                                                       |
| 37965 | 1.600632              | 2.411847                                                       |
| 37967 | 1.000026              | 2.411851                                                       |
| 37969 | 1.024415              | 2.411855                                                       |
| 37971 | 1.444787              | 2.411859                                                       |
| 37973 | 1.132594              | 2.411862                                                       |
| 37975 | 1.488980              | 2.411866                                                       |
| 37977 | 1.333439              | 2.411870                                                       |
| 37979 | 1.010453              | 2.411874                                                       |
| 37981 | 1.053158              | 2.411877                                                       |
| 37983 | 1.455809              | 2.411881                                                       |
| 37985 | 1.228274              | 2.411885                                                       |
| 37987 | 1.000026              | 2.411889                                                       |
| 37989 | 1.732712              | 2.411893                                                       |
| 37991 | 1.000026              | 2.411896                                                       |
| 37993 | 1.000026              | 2.411900                                                       |
| 37995 | 1.705488              | 2.411904                                                       |
| 37997 | 1.000026              | 2.411908                                                       |
| 37999 | 1.120029              | 2.411912                                                       |
| 38001 | 1.364175              | 2.411915                                                       |
| 38003 | 1.174644              | 2.411919                                                       |
| 38005 | 1.310985              | 2.411923                                                       |
| 38007 | 1.494041              | 2.411927                                                       |
| 38009 | 1.010287              | 2.411930                                                       |
| 38011 | 1.000026              | 2.411934                                                       |
| 38013 | 1.333439              | 2.411938                                                       |
| 38015 | 1.200158              | 2.411942                                                       |
| 38017 | 1.143068              | 2.411946                                                       |
| 38019 | 1.515032              | 2.411949                                                       |
| 38021 | 1.010284              | 2.411953                                                       |
| 38023 | 1.022539              | 2.411957                                                       |
| 38025 | 1.939487              | 2.411961                                                       |
| 38027 | 1.091225              | 2.411964                                                       |
| 38029 | 1.059297              | 2.411968                                                       |

| $n$   | $\frac{\sigma(n)}{n}$ | $\frac{e^\gamma}{2} \log \log n + \frac{0.73\dots}{\log \log n}$ |
|-------|-----------------------|------------------------------------------------------------------|
| 38031 | 1.524651              | 2.411972                                                         |
| 38033 | 1.015644              | 2.411976                                                         |
| 38035 | 1.200158              | 2.411980                                                         |
| 38037 | 1.379709              | 2.411983                                                         |
| 38039 | 1.000026              | 2.411987                                                         |
| 38041 | 1.012066              | 2.411991                                                         |
| 38043 | 1.482533              | 2.411995                                                         |
| 38045 | 1.372690              | 2.411998                                                         |
| 38047 | 1.000026              | 2.412002                                                         |
| 38049 | 1.455807              | 2.412006                                                         |
| 38051 | 1.077291              | 2.412010                                                         |
| 38053 | 1.000026              | 2.412013                                                         |
| 38055 | 1.664959              | 2.412017                                                         |
| 38057 | 1.053157              | 2.412021                                                         |
| 38059 | 1.143067              | 2.412025                                                         |
| 38061 | 1.444786              | 2.412029                                                         |
| 38063 | 1.059296              | 2.412032                                                         |
| 38065 | 1.255957              | 2.412036                                                         |
| 38067 | 1.333438              | 2.412040                                                         |
| 38069 | 1.000026              | 2.412044                                                         |
| 38071 | 1.091224              | 2.412047                                                         |
| 38073 | 1.596932              | 2.412051                                                         |
| 38075 | 1.240814              | 2.412055                                                         |
| 38077 | 1.125089              | 2.412059                                                         |
| 38079 | 1.444786              | 2.412063                                                         |
| 38081 | 1.011843              | 2.412066                                                         |
| 38083 | 1.000026              | 2.412070                                                         |
| 38085 | 1.600630              | 2.412074                                                         |
| 38087 | 1.143067              | 2.412078                                                         |
| 38089 | 1.025493              | 2.412081                                                         |
| 38091 | 1.333438              | 2.412085                                                         |
| 38093 | 1.091224              | 2.412089                                                         |
| 38095 | 1.266308              | 2.412093                                                         |
| 38097 | 1.587527              | 2.412096                                                         |
| 38099 | 1.033098              | 2.412100                                                         |
| 38101 | 1.143067              | 2.412104                                                         |
| 38103 | 1.437367              | 2.412108                                                         |
| 38105 | 1.200157              | 2.412112                                                         |
| 38107 | 1.020285              | 2.412115                                                         |
| 38109 | 1.333438              | 2.412119                                                         |
| 38111 | 1.044108              | 2.412123                                                         |
| 38113 | 1.000026              | 2.412127                                                         |
| 38115 | 2.177410              | 2.412130                                                         |
| 38117 | 1.022536              | 2.412134                                                         |

| $n$   | $\frac{\sigma(n)}{n}$ | $\frac{e^\gamma}{2} \log \log n + \frac{0.73...}{\log \log n}$ |
|-------|-----------------------|----------------------------------------------------------------|
| 38119 | 1.000026              | 2.412138                                                       |
| 38121 | 1.357362              | 2.412142                                                       |
| 38123 | 1.016709              | 2.412145                                                       |
| 38125 | 1.270085              | 2.412149                                                       |
| 38127 | 1.359666              | 2.412153                                                       |
| 38129 | 1.233707              | 2.412157                                                       |
| 38131 | 1.059296              | 2.412160                                                       |
| 38133 | 1.527286              | 2.412164                                                       |
| 38135 | 1.246099              | 2.412168                                                       |
| 38137 | 1.091224              | 2.412172                                                       |
| 38139 | 1.333438              | 2.412176                                                       |
| 38141 | 1.024409              | 2.412179                                                       |
| 38143 | 1.143067              | 2.412183                                                       |
| 38145 | 1.600629              | 2.412187                                                       |
| 38147 | 1.028023              | 2.412191                                                       |
| 38149 | 1.000026              | 2.412194                                                       |
| 38151 | 1.507483              | 2.412198                                                       |
| 38153 | 1.000026              | 2.412202                                                       |
| 38155 | 1.294509              | 2.412206                                                       |
| 38157 | 1.610189              | 2.412209                                                       |
| 38159 | 1.091224              | 2.412213                                                       |
| 38161 | 1.033097              | 2.412217                                                       |
| 38163 | 1.333438              | 2.412221                                                       |
| 38165 | 1.273418              | 2.412224                                                       |
| 38167 | 1.000026              | 2.412228                                                       |
| 38169 | 1.444785              | 2.412232                                                       |
| 38171 | 1.254355              | 2.412236                                                       |
| 38173 | 1.018521              | 2.412240                                                       |
| 38175 | 1.656582              | 2.412243                                                       |
| 38177 | 1.000026              | 2.412247                                                       |
| 38179 | 1.015637              | 2.412251                                                       |
| 38181 | 1.584034              | 2.412255                                                       |
| 38183 | 1.000026              | 2.412258                                                       |
| 38185 | 1.372686              | 2.412262                                                       |
| 38187 | 1.444785              | 2.412266                                                       |
| 38189 | 1.000026              | 2.412270                                                       |
| 38191 | 1.010290              | 2.412273                                                       |
| 38193 | 1.382452              | 2.412277                                                       |
| 38195 | 1.200157              | 2.412281                                                       |
| 38197 | 1.000026              | 2.412285                                                       |
| 38199 | 1.628524              | 2.412288                                                       |
| 38201 | 1.000026              | 2.412292                                                       |
| 38203 | 1.145879              | 2.412296                                                       |
| 38205 | 1.784060              | 2.412300                                                       |



| $n$   | $\frac{\sigma(n)}{n}$ | $\frac{e^\gamma}{2} \log \log n + \frac{0.73...}{\log \log n}$ |
|-------|-----------------------|----------------------------------------------------------------|
| 38207 | 1.077290              | 2.412303                                                       |
| 38209 | 1.053155              | 2.412307                                                       |
| 38211 | 1.366727              | 2.412311                                                       |
| 38213 | 1.175726              | 2.412315                                                       |
| 38215 | 1.200157              | 2.412318                                                       |
| 38217 | 1.333438              | 2.412322                                                       |
| 38219 | 1.000026              | 2.412326                                                       |
| 38221 | 1.028021              | 2.412330                                                       |
| 38223 | 1.501923              | 2.412333                                                       |
| 38225 | 1.362459              | 2.412337                                                       |
| 38227 | 1.178643              | 2.412341                                                       |
| 38229 | 1.333438              | 2.412345                                                       |
| 38231 | 1.000026              | 2.412348                                                       |
| 38233 | 1.146863              | 2.412352                                                       |
| 38235 | 1.600628              | 2.412356                                                       |
| 38237 | 1.000026              | 2.412360                                                       |
| 38239 | 1.000026              | 2.412363                                                       |
| 38241 | 1.653513              | 2.412367                                                       |
| 38243 | 1.010381              | 2.412371                                                       |
| 38245 | 1.200157              | 2.412375                                                       |
| 38247 | 1.556200              | 2.412379                                                       |
| 38249 | 1.044106              | 2.412382                                                       |
| 38251 | 1.035267              | 2.412386                                                       |
| 38253 | 1.370245              | 2.412390                                                       |
| 38255 | 1.372683              | 2.412394                                                       |
| 38257 | 1.016703              | 2.412397                                                       |
| 38259 | 1.610079              | 2.412401                                                       |
| 38261 | 1.000026              | 2.412405                                                       |
| 38263 | 1.014244              | 2.412409                                                       |
| 38265 | 1.600627              | 2.412412                                                       |
| 38267 | 1.059294              | 2.412416                                                       |
| 38269 | 1.286890              | 2.412420                                                       |
| 38271 | 1.333438              | 2.412424                                                       |
| 38273 | 1.000026              | 2.412427                                                       |
| 38275 | 1.240810              | 2.412431                                                       |
| 38277 | 1.444784              | 2.412435                                                       |
| 38279 | 1.012566              | 2.412439                                                       |
| 38281 | 1.000026              | 2.412442                                                       |
| 38283 | 1.524645              | 2.412446                                                       |
| 38285 | 1.404205              | 2.412450                                                       |
| 38287 | 1.000026              | 2.412454                                                       |
| 38289 | 1.333438              | 2.412457                                                       |
| 38291 | 1.109712              | 2.412461                                                       |
| 38293 | 1.010629              | 2.412465                                                       |

| $n$   | $\frac{\sigma(n)}{n}$ | $\frac{e^\gamma}{2} \log \log n + \frac{0.73...}{\log \log n}$ |
|-------|-----------------------|----------------------------------------------------------------|
| 38295 | 1.857579              | 2.412469                                                       |
| 38297 | 1.143066              | 2.412472                                                       |
| 38299 | 1.000026              | 2.412476                                                       |
| 38301 | 1.413645              | 2.412480                                                       |
| 38303 | 1.000026              | 2.412484                                                       |
| 38305 | 1.233051              | 2.412487                                                       |
| 38307 | 1.345237              | 2.412491                                                       |
| 38309 | 1.035266              | 2.412495                                                       |
| 38311 | 1.233693              | 2.412498                                                       |
| 38313 | 1.667528              | 2.412502                                                       |
| 38315 | 1.227718              | 2.412506                                                       |
| 38317 | 1.000026              | 2.412510                                                       |
| 38319 | 1.364127              | 2.412513                                                       |
| 38321 | 1.000026              | 2.412517                                                       |
| 38323 | 1.053153              | 2.412521                                                       |
| 38325 | 1.915408              | 2.412525                                                       |
| 38327 | 1.000026              | 2.412528                                                       |
| 38329 | 1.000026              | 2.412532                                                       |
| 38331 | 1.444784              | 2.412536                                                       |
| 38333 | 1.000026              | 2.412540                                                       |
| 38335 | 1.419903              | 2.412543                                                       |
| 38337 | 1.437358              | 2.412547                                                       |
| 38339 | 1.143066              | 2.412551                                                       |
| 38341 | 1.044104              | 2.412555                                                       |
| 38343 | 1.333438              | 2.412558                                                       |
| 38345 | 1.200156              | 2.412562                                                       |
| 38347 | 1.033093              | 2.412566                                                       |
| 38349 | 1.444783              | 2.412570                                                       |
| 38351 | 1.000026              | 2.412573                                                       |
| 38353 | 1.143066              | 2.412577                                                       |
| 38355 | 1.600626              | 2.412581                                                       |
| 38357 | 1.102641              | 2.412585                                                       |
| 38359 | 1.013582              | 2.412588                                                       |
| 38361 | 1.405594              | 2.412592                                                       |
| 38363 | 1.087610              | 2.412596                                                       |
| 38365 | 1.200156              | 2.412600                                                       |
| 38367 | 1.782782              | 2.412603                                                       |
| 38369 | 1.105267              | 2.412607                                                       |
| 38371 | 1.000026              | 2.412611                                                       |
| 38373 | 1.333438              | 2.412615                                                       |
| 38375 | 1.252065              | 2.412618                                                       |
| 38377 | 1.000026              | 2.412622                                                       |
| 38379 | 1.455796              | 2.412626                                                       |
| 38381 | 1.143066              | 2.412629                                                       |

| $n$   | $\frac{\sigma(n)}{n}$ | $\frac{e^\gamma}{2} \log \log n + \frac{0.73...}{\log \log n}$ |
|-------|-----------------------|----------------------------------------------------------------|
| 38383 | 1.011073              | 2.412633                                                       |
| 38385 | 1.735365              | 2.412637                                                       |
| 38387 | 1.044103              | 2.412641                                                       |
| 38389 | 1.077288              | 2.412644                                                       |
| 38391 | 1.360319              | 2.412648                                                       |
| 38393 | 1.000026              | 2.412652                                                       |
| 38395 | 1.372679              | 2.412656                                                       |
| 38397 | 1.333438              | 2.412659                                                       |
| 38399 | 1.100029              | 2.412663                                                       |
| 38401 | 1.091222              | 2.412667                                                       |
| 38403 | 1.535505              | 2.412671                                                       |
| 38405 | 1.200156              | 2.412674                                                       |
| 38407 | 1.010233              | 2.412678                                                       |
| 38409 | 1.599625              | 2.412682                                                       |
| 38411 | 1.015959              | 2.412686                                                       |
| 38413 | 1.012157              | 2.412689                                                       |
| 38415 | 1.731824              | 2.412693                                                       |
| 38417 | 1.025484              | 2.412697                                                       |
| 38419 | 1.012416              | 2.412700                                                       |
| 38421 | 1.482523              | 2.412704                                                       |
| 38423 | 1.249252              | 2.412708                                                       |
| 38425 | 1.306962              | 2.412712                                                       |
| 38427 | 1.333437              | 2.412715                                                       |
| 38429 | 1.014234              | 2.412719                                                       |
| 38431 | 1.000026              | 2.412723                                                       |
| 38433 | 1.393802              | 2.412727                                                       |
| 38435 | 1.200156              | 2.412730                                                       |
| 38437 | 1.277935              | 2.412734                                                       |
| 38439 | 1.444783              | 2.412738                                                       |
| 38441 | 1.077287              | 2.412742                                                       |
| 38443 | 1.028016              | 2.412745                                                       |
| 38445 | 1.752946              | 2.412749                                                       |
| 38447 | 1.000026              | 2.412753                                                       |
| 38449 | 1.000026              | 2.412756                                                       |
| 38451 | 1.524642              | 2.412760                                                       |
| 38453 | 1.000026              | 2.412764                                                       |
| 38455 | 1.200156              | 2.412768                                                       |
| 38457 | 1.444782              | 2.412771                                                       |
| 38459 | 1.000026              | 2.412775                                                       |
| 38461 | 1.000026              | 2.412779                                                       |
| 38463 | 1.333437              | 2.412783                                                       |
| 38465 | 1.404810              | 2.412786                                                       |
| 38467 | 1.179193              | 2.412790                                                       |
| 38469 | 1.333437              | 2.412794                                                       |

| $n$   | $\frac{\sigma(n)}{n}$ | $\frac{e^\gamma}{2} \log \log n + \frac{0.73...}{\log \log n}$ |
|-------|-----------------------|----------------------------------------------------------------|
| 38471 | 1.107951              | 2.412797                                                       |
| 38473 | 1.014738              | 2.412801                                                       |
| 38475 | 1.949838              | 2.412805                                                       |
| 38477 | 1.012033              | 2.412809                                                       |
| 38479 | 1.197536              | 2.412812                                                       |
| 38481 | 1.357137              | 2.412816                                                       |
| 38483 | 1.035262              | 2.412820                                                       |
| 38485 | 1.234767              | 2.412824                                                       |
| 38487 | 1.333437              | 2.412827                                                       |
| 38489 | 1.091221              | 2.412831                                                       |
| 38491 | 1.018004              | 2.412835                                                       |
| 38493 | 1.815603              | 2.412839                                                       |
| 38495 | 1.200156              | 2.412842                                                       |
| 38497 | 1.010884              | 2.412846                                                       |
| 38499 | 1.370217              | 2.412850                                                       |
| 38501 | 1.000026              | 2.412853                                                       |
| 38503 | 1.010830              | 2.412857                                                       |
| 38505 | 1.705337              | 2.412861                                                       |
| 38507 | 1.143065              | 2.412865                                                       |
| 38509 | 1.012854              | 2.412868                                                       |
| 38511 | 1.579808              | 2.412872                                                       |
| 38513 | 1.053151              | 2.412876                                                       |
| 38515 | 1.200156              | 2.412879                                                       |
| 38517 | 1.373316              | 2.412883                                                       |
| 38519 | 1.077287              | 2.412887                                                       |
| 38521 | 1.143065              | 2.412891                                                       |
| 38523 | 1.333437              | 2.412894                                                       |
| 38525 | 1.313225              | 2.412898                                                       |
| 38527 | 1.018507              | 2.412902                                                       |
| 38529 | 1.482520              | 2.412906                                                       |
| 38531 | 1.020269              | 2.412909                                                       |
| 38533 | 1.136065              | 2.412913                                                       |
| 38535 | 1.833554              | 2.412917                                                       |
| 38537 | 1.013571              | 2.412920                                                       |
| 38539 | 1.059291              | 2.412924                                                       |
| 38541 | 1.382424              | 2.412928                                                       |
| 38543 | 1.000026              | 2.412932                                                       |
| 38545 | 1.294487              | 2.412935                                                       |
| 38547 | 1.444782              | 2.412939                                                       |
| 38549 | 1.143065              | 2.412943                                                       |
| 38551 | 1.053150              | 2.412946                                                       |
| 38553 | 1.359583              | 2.412950                                                       |
| 38555 | 1.310958              | 2.412954                                                       |
| 38557 | 1.000026              | 2.412958                                                       |

| $n$   | $\frac{\sigma(n)}{n}$ | $\frac{e^\gamma}{2} \log \log n + \frac{0.73\dots}{\log \log n}$ |
|-------|-----------------------|------------------------------------------------------------------|
| 38559 | 1.333437              | 2.412961                                                         |
| 38561 | 1.000026              | 2.412965                                                         |
| 38563 | 1.164743              | 2.412969                                                         |
| 38565 | 1.735356              | 2.412973                                                         |
| 38567 | 1.000026              | 2.412976                                                         |
| 38569 | 1.000026              | 2.412980                                                         |
| 38571 | 1.533173              | 2.412984                                                         |
| 38573 | 1.059290              | 2.412987                                                         |
| 38575 | 1.240804              | 2.412991                                                         |
| 38577 | 1.672292              | 2.412995                                                         |
| 38579 | 1.010291              | 2.412999                                                         |
| 38581 | 1.025479              | 2.413002                                                         |
| 38583 | 1.482518              | 2.413006                                                         |
| 38585 | 1.200156              | 2.413010                                                         |
| 38587 | 1.022521              | 2.413013                                                         |
| 38589 | 1.405582              | 2.413017                                                         |
| 38591 | 1.181623              | 2.413021                                                         |
| 38593 | 1.000026              | 2.413025                                                         |
| 38595 | 1.671512              | 2.413028                                                         |
| 38597 | 1.077286              | 2.413032                                                         |
| 38599 | 1.137853              | 2.413036                                                         |
| 38601 | 1.444781              | 2.413039                                                         |
| 38603 | 1.000026              | 2.413043                                                         |
| 38605 | 1.372672              | 2.413047                                                         |
| 38607 | 1.413630              | 2.413051                                                         |
| 38609 | 1.000026              | 2.413054                                                         |
| 38611 | 1.000026              | 2.413058                                                         |
| 38613 | 1.361614              | 2.413062                                                         |
| 38615 | 1.200155              | 2.413065                                                         |
| 38617 | 1.059689              | 2.413069                                                         |
| 38619 | 1.653487              | 2.413073                                                         |
| 38621 | 1.091220              | 2.413077                                                         |
| 38623 | 1.077286              | 2.413080                                                         |
| 38625 | 1.680155              | 2.413084                                                         |
| 38627 | 1.065265              | 2.413088                                                         |
| 38629 | 1.000026              | 2.413091                                                         |
| 38631 | 1.358494              | 2.413095                                                         |
| 38633 | 1.143064              | 2.413099                                                         |
| 38635 | 1.200155              | 2.413103                                                         |
| 38637 | 1.527603              | 2.413106                                                         |
| 38639 | 1.000026              | 2.413110                                                         |
| 38641 | 1.059289              | 2.413114                                                         |
| 38643 | 1.455788              | 2.413117                                                         |
| 38645 | 1.229655              | 2.413121                                                         |

| $n$   | $\frac{\sigma(n)}{n}$ | $\frac{e^\gamma}{2} \log \log n + \frac{0.73...}{\log \log n}$ |
|-------|-----------------------|----------------------------------------------------------------|
| 38647 | 1.143064              | 2.413125                                                       |
| 38649 | 1.437346              | 2.413129                                                       |
| 38651 | 1.000026              | 2.413132                                                       |
| 38653 | 1.000026              | 2.413136                                                       |
| 38655 | 1.735351              | 2.413140                                                       |
| 38657 | 1.092687              | 2.413143                                                       |
| 38659 | 1.016684              | 2.413147                                                       |
| 38661 | 1.556918              | 2.413151                                                       |
| 38663 | 1.069550              | 2.413155                                                       |
| 38665 | 1.415233              | 2.413158                                                       |
| 38667 | 1.333437              | 2.413162                                                       |
| 38669 | 1.000026              | 2.413166                                                       |
| 38671 | 1.000026              | 2.413169                                                       |
| 38673 | 1.444781              | 2.413173                                                       |
| 38675 | 1.615928              | 2.413177                                                       |
| 38677 | 1.000026              | 2.413180                                                       |
| 38679 | 1.333437              | 2.413184                                                       |
| 38681 | 1.022518              | 2.413188                                                       |
| 38683 | 1.012538              | 2.413192                                                       |
| 38685 | 1.600620              | 2.413195                                                       |
| 38687 | 1.091219              | 2.413199                                                       |
| 38689 | 1.143064              | 2.413203                                                       |
| 38691 | 1.482515              | 2.413206                                                       |
| 38693 | 1.000026              | 2.413210                                                       |
| 38695 | 1.228066              | 2.413214                                                       |
| 38697 | 1.333437              | 2.413218                                                       |
| 38699 | 1.000026              | 2.413221                                                       |
| 38701 | 1.087569              | 2.413225                                                       |
| 38703 | 1.620546              | 2.413229                                                       |
| 38705 | 1.200155              | 2.413232                                                       |
| 38707 | 1.000026              | 2.413236                                                       |
| 38709 | 1.740990              | 2.413240                                                       |
| 38711 | 1.000026              | 2.413243                                                       |
| 38713 | 1.000026              | 2.413247                                                       |
| 38715 | 1.673770              | 2.413251                                                       |
| 38717 | 1.143064              | 2.413255                                                       |
| 38719 | 1.033085              | 2.413258                                                       |
| 38721 | 1.333437              | 2.413262                                                       |
| 38723 | 1.000026              | 2.413266                                                       |
| 38725 | 1.240801              | 2.413269                                                       |
| 38727 | 1.560255              | 2.413273                                                       |
| 38729 | 1.000026              | 2.413277                                                       |
| 38731 | 1.249232              | 2.413281                                                       |
| 38733 | 1.333437              | 2.413284                                                       |

| $n$   | $\frac{\sigma(n)}{n}$ | $\frac{e^\gamma}{2} \log \log n + \frac{0.73...}{\log \log n}$ |
|-------|-----------------------|----------------------------------------------------------------|
| 38735 | 1.229276              | 2.413288                                                       |
| 38737 | 1.000026              | 2.413292                                                       |
| 38739 | 1.373293              | 2.413295                                                       |
| 38741 | 1.053148              | 2.413299                                                       |
| 38743 | 1.103890              | 2.413303                                                       |
| 38745 | 2.081301              | 2.413306                                                       |
| 38747 | 1.000026              | 2.413310                                                       |
| 38749 | 1.000026              | 2.413314                                                       |
| 38751 | 1.333437              | 2.413318                                                       |
| 38753 | 1.179160              | 2.413321                                                       |
| 38755 | 1.255890              | 2.413325                                                       |
| 38757 | 1.333437              | 2.413329                                                       |
| 38759 | 1.176501              | 2.413332                                                       |
| 38761 | 1.014215              | 2.413336                                                       |
| 38763 | 1.489049              | 2.413340                                                       |
| 38765 | 1.200155              | 2.413343                                                       |
| 38767 | 1.000026              | 2.413347                                                       |
| 38769 | 1.333437              | 2.413351                                                       |
| 38771 | 1.010859              | 2.413355                                                       |
| 38773 | 1.188456              | 2.413358                                                       |
| 38775 | 1.842012              | 2.413362                                                       |
| 38777 | 1.059288              | 2.413366                                                       |
| 38779 | 1.140824              | 2.413369                                                       |
| 38781 | 1.501766              | 2.413373                                                       |
| 38783 | 1.000026              | 2.413377                                                       |
| 38785 | 1.200155              | 2.413380                                                       |
| 38787 | 1.524635              | 2.413384                                                       |
| 38789 | 1.014721              | 2.413388                                                       |
| 38791 | 1.000026              | 2.413392                                                       |
| 38793 | 1.360245              | 2.413395                                                       |
| 38795 | 1.200155              | 2.413399                                                       |
| 38797 | 1.091218              | 2.413403                                                       |
| 38799 | 1.496946              | 2.413406                                                       |
| 38801 | 1.197495              | 2.413410                                                       |
| 38803 | 1.000026              | 2.413414                                                       |
| 38805 | 1.731736              | 2.413417                                                       |
| 38807 | 1.010539              | 2.413421                                                       |
| 38809 | 1.005102              | 2.413425                                                       |
| 38811 | 1.413620              | 2.413428                                                       |
| 38813 | 1.028006              | 2.413432                                                       |
| 38815 | 1.372665              | 2.413436                                                       |
| 38817 | 1.527166              | 2.413440                                                       |
| 38819 | 1.091218              | 2.413443                                                       |
| 38821 | 1.000026              | 2.413447                                                       |

| $n$   | $\frac{\sigma(n)}{n}$ | $\frac{e^\gamma}{2} \log \log n + \frac{0.73\dots}{\log \log n}$ |
|-------|-----------------------|------------------------------------------------------------------|
| 38823 | 1.333436              | 2.413451                                                         |
| 38825 | 1.240798              | 2.413454                                                         |
| 38827 | 1.025472              | 2.413458                                                         |
| 38829 | 1.560071              | 2.413462                                                         |
| 38831 | 1.124874              | 2.413465                                                         |
| 38833 | 1.000026              | 2.413469                                                         |
| 38835 | 1.735342              | 2.413473                                                         |
| 38837 | 1.015938              | 2.413476                                                         |
| 38839 | 1.000026              | 2.413480                                                         |
| 38841 | 1.479262              | 2.413484                                                         |
| 38843 | 1.186314              | 2.413488                                                         |
| 38845 | 1.273369              | 2.413491                                                         |
| 38847 | 1.393776              | 2.413495                                                         |
| 38849 | 1.020258              | 2.413499                                                         |
| 38851 | 1.000026              | 2.413502                                                         |
| 38853 | 1.482511              | 2.413506                                                         |
| 38855 | 1.266246              | 2.413510                                                         |
| 38857 | 1.273284              | 2.413513                                                         |
| 38859 | 1.333436              | 2.413517                                                         |
| 38861 | 1.000026              | 2.413521                                                         |
| 38863 | 1.091218              | 2.413524                                                         |
| 38865 | 1.600618              | 2.413528                                                         |
| 38867 | 1.000026              | 2.413532                                                         |
| 38869 | 1.022512              | 2.413535                                                         |
| 38871 | 1.653469              | 2.413539                                                         |
| 38873 | 1.000026              | 2.413543                                                         |
| 38875 | 1.252013              | 2.413547                                                         |
| 38877 | 1.333436              | 2.413550                                                         |
| 38879 | 1.059287              | 2.413554                                                         |
| 38881 | 1.018492              | 2.413558                                                         |
| 38883 | 1.437338              | 2.413561                                                         |
| 38885 | 1.510917              | 2.413565                                                         |
| 38887 | 1.028004              | 2.413569                                                         |
| 38889 | 1.504281              | 2.413572                                                         |
| 38891 | 1.000026              | 2.413576                                                         |
| 38893 | 1.110740              | 2.413580                                                         |
| 38895 | 1.600617              | 2.413583                                                         |
| 38897 | 1.012829              | 2.413587                                                         |
| 38899 | 1.143063              | 2.413591                                                         |
| 38901 | 1.333436              | 2.413594                                                         |
| 38903 | 1.000026              | 2.413598                                                         |
| 38905 | 1.243645              | 2.413602                                                         |
| 38907 | 1.628499              | 2.413606                                                         |
| 38909 | 1.118302              | 2.413609                                                         |



| $n$   | $\frac{\sigma(n)}{n}$ | $\frac{e^\gamma}{2} \log \log n + \frac{0.73\dots}{\log \log n}$ |
|-------|-----------------------|------------------------------------------------------------------|
| 38911 | 1.010306              | 2.413613                                                         |
| 38913 | 1.628248              | 2.413617                                                         |
| 38915 | 1.234691              | 2.413620                                                         |
| 38917 | 1.000026              | 2.413624                                                         |
| 38919 | 1.333436              | 2.413628                                                         |
| 38921 | 1.000026              | 2.413631                                                         |
| 38923 | 1.000026              | 2.413635                                                         |
| 38925 | 1.801464              | 2.413639                                                         |
| 38927 | 1.173890              | 2.413642                                                         |
| 38929 | 1.091217              | 2.413646                                                         |
| 38931 | 1.405564              | 2.413650                                                         |
| 38933 | 1.000026              | 2.413653                                                         |
| 38935 | 1.294465              | 2.413657                                                         |
| 38937 | 1.333436              | 2.413661                                                         |
| 38939 | 1.044095              | 2.413664                                                         |
| 38941 | 1.143063              | 2.413668                                                         |
| 38943 | 1.444778              | 2.413672                                                         |
| 38945 | 1.200154              | 2.413675                                                         |
| 38947 | 1.109200              | 2.413679                                                         |
| 38949 | 1.333436              | 2.413683                                                         |
| 38951 | 1.091217              | 2.413687                                                         |
| 38953 | 1.000026              | 2.413690                                                         |
| 38955 | 1.896342              | 2.413694                                                         |
| 38957 | 1.010345              | 2.413698                                                         |
| 38959 | 1.000026              | 2.413701                                                         |
| 38961 | 1.652216              | 2.413705                                                         |
| 38963 | 1.022509              | 2.413709                                                         |
| 38965 | 1.200154              | 2.413712                                                         |
| 38967 | 1.379629              | 2.413716                                                         |
| 38969 | 1.207113              | 2.413720                                                         |
| 38971 | 1.000026              | 2.413723                                                         |
| 38973 | 1.455777              | 2.413727                                                         |
| 38975 | 1.240795              | 2.413731                                                         |
| 38977 | 1.000026              | 2.413734                                                         |
| 38979 | 1.488802              | 2.413738                                                         |
| 38981 | 1.059285              | 2.413742                                                         |
| 38983 | 1.143062              | 2.413745                                                         |
| 38985 | 1.684340              | 2.413749                                                         |
| 38987 | 1.077282              | 2.413753                                                         |
| 38989 | 1.011157              | 2.413756                                                         |
| 38991 | 1.370162              | 2.413760                                                         |
| 38993 | 1.000026              | 2.413764                                                         |
| 38995 | 1.310937              | 2.413767                                                         |
| 38997 | 1.653461              | 2.413771                                                         |

| $n$   | $\frac{\sigma(n)}{n}$ | $\frac{e^\gamma}{2} \log \log n + \frac{0.73...}{\log \log n}$ |
|-------|-----------------------|----------------------------------------------------------------|
| 38999 | 1.018488              | 2.413775                                                       |
| 39001 | 1.024384              | 2.413778                                                       |
| 39003 | 1.333436              | 2.413782                                                       |
| 39005 | 1.245994              | 2.413786                                                       |
| 39007 | 1.053144              | 2.413789                                                       |
| 39009 | 1.333436              | 2.413793                                                       |
| 39011 | 1.143062              | 2.413797                                                       |
| 39013 | 1.077282              | 2.413800                                                       |
| 39015 | 1.888504              | 2.413804                                                       |
| 39017 | 1.091217              | 2.413808                                                       |
| 39019 | 1.000026              | 2.413812                                                       |
| 39021 | 1.333436              | 2.413815                                                       |
| 39023 | 1.000026              | 2.413819                                                       |
| 39025 | 1.423498              | 2.413823                                                       |
| 39027 | 1.333436              | 2.413826                                                       |
| 39029 | 1.033078              | 2.413830                                                       |
| 39031 | 1.044093              | 2.413834                                                       |
| 39033 | 1.444777              | 2.413837                                                       |
| 39035 | 1.238273              | 2.413841                                                       |
| 39037 | 1.012373              | 2.413845                                                       |
| 39039 | 1.800046              | 2.413848                                                       |
| 39041 | 1.000026              | 2.413852                                                       |
| 39043 | 1.000026              | 2.413856                                                       |
| 39045 | 1.696504              | 2.413859                                                       |
| 39047 | 1.000026              | 2.413863                                                       |
| 39049 | 1.059284              | 2.413867                                                       |
| 39051 | 1.444777              | 2.413870                                                       |
| 39053 | 1.164725              | 2.413874                                                       |
| 39055 | 1.227807              | 2.413878                                                       |
| 39057 | 1.366618              | 2.413881                                                       |
| 39059 | 1.010779              | 2.413885                                                       |
| 39061 | 1.128082              | 2.413889                                                       |
| 39063 | 1.382382              | 2.413892                                                       |
| 39065 | 1.294458              | 2.413896                                                       |
| 39067 | 1.143062              | 2.413900                                                       |
| 39069 | 1.482505              | 2.413903                                                       |
| 39071 | 1.013539              | 2.413907                                                       |
| 39073 | 1.025465              | 2.413911                                                       |
| 39075 | 1.656507              | 2.413914                                                       |
| 39077 | 1.044092              | 2.413918                                                       |
| 39079 | 1.000026              | 2.413922                                                       |
| 39081 | 1.524628              | 2.413925                                                       |
| 39083 | 1.225085              | 2.413929                                                       |
| 39085 | 1.200154              | 2.413933                                                       |

| $n$   | $\frac{\sigma(n)}{n}$ | $\frac{e^\gamma}{2} \log \log n + \frac{0.73...}{\log \log n}$ |
|-------|-----------------------|----------------------------------------------------------------|
| 39087 | 1.492670              | 2.413936                                                       |
| 39089 | 1.000026              | 2.413940                                                       |
| 39091 | 1.123123              | 2.413944                                                       |
| 39093 | 1.357992              | 2.413947                                                       |
| 39095 | 1.372656              | 2.413951                                                       |
| 39097 | 1.000026              | 2.413955                                                       |
| 39099 | 1.333436              | 2.413958                                                       |
| 39101 | 1.017979              | 2.413962                                                       |
| 39103 | 1.000026              | 2.413966                                                       |
| 39105 | 1.914845              | 2.413969                                                       |
| 39107 | 1.000026              | 2.413973                                                       |
| 39109 | 1.181518              | 2.413977                                                       |
| 39111 | 1.333436              | 2.413980                                                       |
| 39113 | 1.000026              | 2.413984                                                       |
| 39115 | 1.200153              | 2.413988                                                       |
| 39117 | 1.546131              | 2.413991                                                       |
| 39119 | 1.000026              | 2.413995                                                       |
| 39121 | 1.104266              | 2.413999                                                       |
| 39123 | 1.786366              | 2.414002                                                       |
| 39125 | 1.251987              | 2.414006                                                       |
| 39127 | 1.091216              | 2.414010                                                       |
| 39129 | 1.333436              | 2.414013                                                       |
| 39131 | 1.011985              | 2.414017                                                       |
| 39133 | 1.000026              | 2.414021                                                       |
| 39135 | 1.600613              | 2.414024                                                       |
| 39137 | 1.143062              | 2.414028                                                       |
| 39139 | 1.000026              | 2.414032                                                       |
| 39141 | 1.444777              | 2.414035                                                       |
| 39143 | 1.077281              | 2.414039                                                       |
| 39145 | 1.200153              | 2.414042                                                       |
| 39147 | 1.333436              | 2.414046                                                       |
| 39149 | 1.091216              | 2.414050                                                       |
| 39151 | 1.257899              | 2.414053                                                       |
| 39153 | 1.379613              | 2.414057                                                       |
| 39155 | 1.235704              | 2.414061                                                       |
| 39157 | 1.000026              | 2.414064                                                       |
| 39159 | 1.527107              | 2.414068                                                       |
| 39161 | 1.000026              | 2.414072                                                       |
| 39163 | 1.000026              | 2.414075                                                       |
| 39165 | 1.833474              | 2.414079                                                       |
| 39167 | 1.020247              | 2.414083                                                       |
| 39169 | 1.132324              | 2.414086                                                       |
| 39171 | 1.455771              | 2.414090                                                       |
| 39173 | 1.024379              | 2.414094                                                       |

| $n$   | $\frac{\sigma(n)}{n}$ | $\frac{e^\gamma}{2} \log \log n + \frac{0.73...}{\log \log n}$ |
|-------|-----------------------|----------------------------------------------------------------|
| 39175 | 1.240791              | 2.414097                                                       |
| 39177 | 1.482502              | 2.414101                                                       |
| 39179 | 1.188392              | 2.414105                                                       |
| 39181 | 1.000026              | 2.414108                                                       |
| 39183 | 1.373249              | 2.414112                                                       |
| 39185 | 1.273344              | 2.414116                                                       |
| 39187 | 1.010539              | 2.414119                                                       |
| 39189 | 1.333435              | 2.414123                                                       |
| 39191 | 1.000026              | 2.414127                                                       |
| 39193 | 1.249203              | 2.414130                                                       |
| 39195 | 1.894527              | 2.414134                                                       |
| 39197 | 1.053142              | 2.414138                                                       |
| 39199 | 1.000026              | 2.414141                                                       |
| 39201 | 1.359149              | 2.414145                                                       |
| 39203 | 1.010127              | 2.414149                                                       |
| 39205 | 1.200153              | 2.414152                                                       |
| 39207 | 1.524626              | 2.414156                                                       |
| 39209 | 1.000026              | 2.414160                                                       |
| 39211 | 1.011757              | 2.414163                                                       |
| 39213 | 1.444776              | 2.414167                                                       |
| 39215 | 1.410073              | 2.414170                                                       |
| 39217 | 1.000025              | 2.414174                                                       |
| 39219 | 1.413601              | 2.414178                                                       |
| 39221 | 1.233625              | 2.414181                                                       |
| 39223 | 1.017974              | 2.414185                                                       |
| 39225 | 1.656495              | 2.414189                                                       |
| 39227 | 1.000025              | 2.414192                                                       |
| 39229 | 1.000025              | 2.414196                                                       |
| 39231 | 1.482501              | 2.414200                                                       |
| 39233 | 1.000025              | 2.414203                                                       |
| 39235 | 1.468077              | 2.414207                                                       |
| 39237 | 1.541402              | 2.414211                                                       |
| 39239 | 1.000025              | 2.414214                                                       |
| 39241 | 1.000025              | 2.414218                                                       |
| 39243 | 1.356879              | 2.414222                                                       |
| 39245 | 1.232870              | 2.414225                                                       |
| 39247 | 1.077280              | 2.414229                                                       |
| 39249 | 1.699152              | 2.414233                                                       |
| 39251 | 1.000025              | 2.414236                                                       |
| 39253 | 1.059282              | 2.414240                                                       |
| 39255 | 1.600611              | 2.414243                                                       |
| 39257 | 1.027995              | 2.414247                                                       |
| 39259 | 1.129728              | 2.414251                                                       |
| 39261 | 1.393750              | 2.414254                                                       |

| $n$   | $\frac{\sigma(n)}{n}$ | $\frac{e^\gamma}{2} \log \log n + \frac{0.73...}{\log \log n}$ |
|-------|-----------------------|----------------------------------------------------------------|
| 39263 | 1.173624              | 2.414258                                                       |
| 39265 | 1.200153              | 2.414262                                                       |
| 39267 | 1.444776              | 2.414265                                                       |
| 39269 | 1.012096              | 2.414269                                                       |
| 39271 | 1.010211              | 2.414273                                                       |
| 39273 | 1.539989              | 2.414276                                                       |
| 39275 | 1.240789              | 2.414280                                                       |
| 39277 | 1.186241              | 2.414284                                                       |
| 39279 | 1.333435              | 2.414287                                                       |
| 39281 | 1.091215              | 2.414291                                                       |
| 39283 | 1.010310              | 2.414295                                                       |
| 39285 | 1.811073              | 2.414298                                                       |
| 39287 | 1.059282              | 2.414302                                                       |
| 39289 | 1.012497              | 2.414305                                                       |
| 39291 | 1.524624              | 2.414309                                                       |
| 39293 | 1.000025              | 2.414313                                                       |
| 39295 | 1.245960              | 2.414316                                                       |
| 39297 | 1.333435              | 2.414320                                                       |
| 39299 | 1.077279              | 2.414324                                                       |
| 39301 | 1.000025              | 2.414327                                                       |
| 39303 | 1.579727              | 2.414331                                                       |
| 39305 | 1.372650              | 2.414335                                                       |
| 39307 | 1.044089              | 2.414338                                                       |
| 39309 | 1.333435              | 2.414342                                                       |
| 39311 | 1.053140              | 2.414346                                                       |
| 39313 | 1.000025              | 2.414349                                                       |
| 39315 | 1.600610              | 2.414353                                                       |
| 39317 | 1.000025              | 2.414356                                                       |
| 39319 | 1.179277              | 2.414360                                                       |
| 39321 | 1.535363              | 2.414364                                                       |
| 39323 | 1.000025              | 2.414367                                                       |
| 39325 | 1.467819              | 2.414371                                                       |
| 39327 | 1.333435              | 2.414375                                                       |
| 39329 | 1.016654              | 2.414378                                                       |
| 39331 | 1.027993              | 2.414382                                                       |
| 39333 | 1.524623              | 2.414386                                                       |
| 39335 | 1.200153              | 2.414389                                                       |
| 39337 | 1.010753              | 2.414393                                                       |
| 39339 | 1.561809              | 2.414397                                                       |
| 39341 | 1.000025              | 2.414400                                                       |
| 39343 | 1.000025              | 2.414404                                                       |
| 39345 | 1.664049              | 2.414407                                                       |
| 39347 | 1.286400              | 2.414411                                                       |
| 39349 | 1.065084              | 2.414415                                                       |

| $n$   | $\frac{\sigma(n)}{n}$ | $\frac{e^\gamma}{2} \log \log n + \frac{0.73\dots}{\log \log n}$ |
|-------|-----------------------|------------------------------------------------------------------|
| 39351 | 1.437321              | 2.414418                                                         |
| 39353 | 1.097756              | 2.414422                                                         |
| 39355 | 1.273332              | 2.414426                                                         |
| 39357 | 1.444775              | 2.414429                                                         |
| 39359 | 1.000025              | 2.414433                                                         |
| 39361 | 1.143060              | 2.414437                                                         |
| 39363 | 1.333435              | 2.414440                                                         |
| 39365 | 1.200152              | 2.414444                                                         |
| 39367 | 1.000025              | 2.414447                                                         |
| 39369 | 1.455765              | 2.414451                                                         |
| 39371 | 1.000025              | 2.414455                                                         |
| 39373 | 1.000025              | 2.414458                                                         |
| 39375 | 2.062832              | 2.414462                                                         |
| 39377 | 1.087488              | 2.414466                                                         |
| 39379 | 1.020239              | 2.414469                                                         |
| 39381 | 1.333435              | 2.414473                                                         |
| 39383 | 1.000025              | 2.414477                                                         |
| 39385 | 1.200152              | 2.414480                                                         |
| 39387 | 1.405540              | 2.414484                                                         |
| 39389 | 1.213740              | 2.414487                                                         |
| 39391 | 1.091214              | 2.414491                                                         |
| 39393 | 1.482497              | 2.414495                                                         |
| 39395 | 1.200152              | 2.414498                                                         |
| 39397 | 1.000025              | 2.414502                                                         |
| 39399 | 1.393741              | 2.414506                                                         |
| 39401 | 1.058501              | 2.414509                                                         |
| 39403 | 1.233612              | 2.414513                                                         |
| 39405 | 1.666388              | 2.414517                                                         |
| 39407 | 1.010379              | 2.414520                                                         |
| 39409 | 1.000025              | 2.414524                                                         |
| 39411 | 1.504149              | 2.414527                                                         |
| 39413 | 1.091214              | 2.414531                                                         |
| 39415 | 1.200152              | 2.414535                                                         |
| 39417 | 1.524621              | 2.414538                                                         |
| 39419 | 1.000025              | 2.414542                                                         |
| 39421 | 1.014688              | 2.414546                                                         |
| 39423 | 1.413591              | 2.414549                                                         |
| 39425 | 1.320989              | 2.414553                                                         |
| 39427 | 1.013519              | 2.414557                                                         |
| 39429 | 1.560171              | 2.414560                                                         |
| 39431 | 1.178362              | 2.414564                                                         |
| 39433 | 1.022494              | 2.414567                                                         |
| 39435 | 1.752758              | 2.414571                                                         |
| 39437 | 1.011740              | 2.414575                                                         |

| $n$   | $\frac{\sigma(n)}{n}$ | $\frac{e^\gamma}{2} \log \log n + \frac{0.73...}{\log \log n}$ |
|-------|-----------------------|----------------------------------------------------------------|
| 39439 | 1.000025              | 2.414578                                                       |
| 39441 | 1.333435              | 2.414582                                                       |
| 39443 | 1.000025              | 2.414586                                                       |
| 39445 | 1.460261              | 2.414589                                                       |
| 39447 | 1.496895              | 2.414593                                                       |
| 39449 | 1.012345              | 2.414596                                                       |
| 39451 | 1.000025              | 2.414600                                                       |
| 39453 | 1.333435              | 2.414604                                                       |
| 39455 | 1.294437              | 2.414607                                                       |
| 39457 | 1.160555              | 2.414611                                                       |
| 39459 | 1.524620              | 2.414615                                                       |
| 39461 | 1.000025              | 2.414618                                                       |
| 39463 | 1.102805              | 2.414622                                                       |
| 39465 | 1.735310              | 2.414625                                                       |
| 39467 | 1.017964              | 2.414629                                                       |
| 39469 | 1.035243              | 2.414633                                                       |
| 39471 | 1.362013              | 2.414636                                                       |
| 39473 | 1.143060              | 2.414640                                                       |
| 39475 | 1.240785              | 2.414644                                                       |
| 39477 | 1.333435              | 2.414647                                                       |
| 39479 | 1.131944              | 2.414651                                                       |
| 39481 | 1.077278              | 2.414655                                                       |
| 39483 | 1.493504              | 2.414658                                                       |
| 39485 | 1.230847              | 2.414662                                                       |
| 39487 | 1.143060              | 2.414665                                                       |
| 39489 | 1.333435              | 2.414669                                                       |
| 39491 | 1.115799              | 2.414673                                                       |
| 39493 | 1.015572              | 2.414676                                                       |
| 39495 | 1.600608              | 2.414680                                                       |
| 39497 | 1.011115              | 2.414684                                                       |
| 39499 | 1.000025              | 2.414687                                                       |
| 39501 | 1.944255              | 2.414691                                                       |
| 39503 | 1.000025              | 2.414694                                                       |
| 39505 | 1.200152              | 2.414698                                                       |
| 39507 | 1.437315              | 2.414702                                                       |
| 39509 | 1.000025              | 2.414705                                                       |
| 39511 | 1.000025              | 2.414709                                                       |
| 39513 | 1.333435              | 2.414713                                                       |
| 39515 | 1.372643              | 2.414716                                                       |
| 39517 | 1.024369              | 2.414720                                                       |
| 39519 | 1.444773              | 2.414723                                                       |
| 39521 | 1.000025              | 2.414727                                                       |
| 39523 | 1.091213              | 2.414731                                                       |
| 39525 | 1.807059              | 2.414734                                                       |

| $n$   | $\frac{\sigma(n)}{n}$ | $\frac{e^\gamma}{2} \log \log n + \frac{0.73...}{\log \log n}$ |
|-------|-----------------------|----------------------------------------------------------------|
| 39527 | 1.057707              | 2.414738                                                       |
| 39529 | 1.143060              | 2.414741                                                       |
| 39531 | 1.333435              | 2.414745                                                       |
| 39533 | 1.077277              | 2.414749                                                       |
| 39535 | 1.200152              | 2.414752                                                       |
| 39537 | 1.515138              | 2.414756                                                       |
| 39539 | 1.053137              | 2.414760                                                       |
| 39541 | 1.000025              | 2.414763                                                       |
| 39543 | 1.556786              | 2.414767                                                       |
| 39545 | 1.310912              | 2.414770                                                       |
| 39547 | 1.015905              | 2.414774                                                       |
| 39549 | 1.333434              | 2.414778                                                       |
| 39551 | 1.000025              | 2.414781                                                       |
| 39553 | 1.027988              | 2.414785                                                       |
| 39555 | 1.783845              | 2.414789                                                       |
| 39557 | 1.143059              | 2.414792                                                       |
| 39559 | 1.146642              | 2.414796                                                       |
| 39561 | 1.333434              | 2.414799                                                       |
| 39563 | 1.000025              | 2.414803                                                       |
| 39565 | 1.235638              | 2.414807                                                       |
| 39567 | 1.479010              | 2.414810                                                       |
| 39569 | 1.000025              | 2.414814                                                       |
| 39571 | 1.143059              | 2.414817                                                       |
| 39573 | 1.444773              | 2.414821                                                       |
| 39575 | 1.240783              | 2.414825                                                       |
| 39577 | 1.053137              | 2.414828                                                       |
| 39579 | 1.358296              | 2.414832                                                       |
| 39581 | 1.000025              | 2.414836                                                       |
| 39583 | 1.044085              | 2.414839                                                       |
| 39585 | 2.037135              | 2.414843                                                       |
| 39587 | 1.033066              | 2.414846                                                       |
| 39589 | 1.127586              | 2.414850                                                       |
| 39591 | 1.489429              | 2.414854                                                       |
| 39593 | 1.070038              | 2.414857                                                       |
| 39595 | 1.200152              | 2.414861                                                       |
| 39597 | 1.360103              | 2.414865                                                       |
| 39599 | 1.143059              | 2.414868                                                       |
| 39601 | 1.005050              | 2.414872                                                       |
| 39603 | 1.368785              | 2.414875                                                       |
| 39605 | 1.213635              | 2.414879                                                       |
| 39607 | 1.000025              | 2.414883                                                       |
| 39609 | 1.507132              | 2.414886                                                       |
| 39611 | 1.179066              | 2.414890                                                       |
| 39613 | 1.143059              | 2.414893                                                       |



| $n$   | $\frac{\sigma(n)}{n}$ | $\frac{e^\gamma}{2} \log \log n + \frac{0.73...}{\log \log n}$ |
|-------|-----------------------|----------------------------------------------------------------|
| 39615 | 1.696327              | 2.414897                                                       |
| 39617 | 1.010172              | 2.414901                                                       |
| 39619 | 1.000025              | 2.414904                                                       |
| 39621 | 1.366548              | 2.414908                                                       |
| 39623 | 1.000025              | 2.414911                                                       |
| 39625 | 1.251937              | 2.414915                                                       |
| 39627 | 1.795140              | 2.414919                                                       |
| 39629 | 1.044084              | 2.414922                                                       |
| 39631 | 1.000025              | 2.414926                                                       |
| 39633 | 1.455757              | 2.414930                                                       |
| 39635 | 1.200151              | 2.414933                                                       |
| 39637 | 1.077276              | 2.414937                                                       |
| 39639 | 1.359066              | 2.414940                                                       |
| 39641 | 1.164703              | 2.414944                                                       |
| 39643 | 1.035240              | 2.414948                                                       |
| 39645 | 1.735301              | 2.414951                                                       |
| 39647 | 1.025450              | 2.414955                                                       |
| 39649 | 1.033065              | 2.414958                                                       |
| 39651 | 1.333434              | 2.414962                                                       |
| 39653 | 1.053136              | 2.414966                                                       |
| 39655 | 1.510629              | 2.414969                                                       |
| 39657 | 1.333434              | 2.414973                                                       |
| 39659 | 1.000025              | 2.414976                                                       |
| 39661 | 1.059277              | 2.414980                                                       |
| 39663 | 1.609561              | 2.414984                                                       |
| 39665 | 1.200151              | 2.414987                                                       |
| 39667 | 1.000025              | 2.414991                                                       |
| 39669 | 1.524616              | 2.414995                                                       |
| 39671 | 1.000025              | 2.414998                                                       |
| 39673 | 1.012779              | 2.415002                                                       |
| 39675 | 1.728343              | 2.415005                                                       |
| 39677 | 1.091212              | 2.415009                                                       |
| 39679 | 1.000025              | 2.415013                                                       |
| 39681 | 1.444772              | 2.415016                                                       |
| 39683 | 1.143059              | 2.415020                                                       |
| 39685 | 1.200151              | 2.415023                                                       |
| 39687 | 1.333434              | 2.415027                                                       |
| 39689 | 1.117488              | 2.415031                                                       |
| 39691 | 1.053135              | 2.415034                                                       |
| 39693 | 1.356814              | 2.415038                                                       |
| 39695 | 1.273309              | 2.415041                                                       |
| 39697 | 1.175303              | 2.415045                                                       |
| 39699 | 1.579687              | 2.415049                                                       |
| 39701 | 1.063197              | 2.415052                                                       |

| $n$   | $\frac{\sigma(n)}{n}$ | $\frac{e^\gamma}{2} \log \log n + \frac{0.73...}{\log \log n}$ |
|-------|-----------------------|----------------------------------------------------------------|
| 39703 | 1.000025              | 2.415056                                                       |
| 39705 | 1.600604              | 2.415059                                                       |
| 39707 | 1.018460              | 2.415063                                                       |
| 39709 | 1.000025              | 2.415067                                                       |
| 39711 | 1.598751              | 2.415070                                                       |
| 39713 | 1.010450              | 2.415074                                                       |
| 39715 | 1.327055              | 2.415077                                                       |
| 39717 | 1.482489              | 2.415081                                                       |
| 39719 | 1.000025              | 2.415085                                                       |
| 39721 | 1.145590              | 2.415088                                                       |
| 39723 | 1.333434              | 2.415092                                                       |
| 39725 | 1.423386              | 2.415095                                                       |
| 39727 | 1.000025              | 2.415099                                                       |
| 39729 | 1.522314              | 2.415103                                                       |
| 39731 | 1.016637              | 2.415106                                                       |
| 39733 | 1.000025              | 2.415110                                                       |
| 39735 | 1.735296              | 2.415113                                                       |
| 39737 | 1.014671              | 2.415117                                                       |
| 39739 | 1.164700              | 2.415121                                                       |
| 39741 | 1.437307              | 2.415124                                                       |
| 39743 | 1.091211              | 2.415128                                                       |
| 39745 | 1.200151              | 2.415131                                                       |
| 39747 | 1.333434              | 2.415135                                                       |
| 39749 | 1.000025              | 2.415139                                                       |
| 39751 | 1.011094              | 2.415142                                                       |
| 39753 | 1.653410              | 2.415146                                                       |
| 39755 | 1.200151              | 2.415149                                                       |
| 39757 | 1.014161              | 2.415153                                                       |
| 39759 | 1.382329              | 2.415157                                                       |
| 39761 | 1.000025              | 2.415160                                                       |
| 39763 | 1.059276              | 2.415164                                                       |
| 39765 | 1.752697              | 2.415167                                                       |
| 39767 | 1.351875              | 2.415171                                                       |
| 39769 | 1.000025              | 2.415175                                                       |
| 39771 | 1.496870              | 2.415178                                                       |
| 39773 | 1.033063              | 2.415182                                                       |
| 39775 | 1.303130              | 2.415185                                                       |
| 39777 | 1.333434              | 2.415189                                                       |
| 39779 | 1.000025              | 2.415193                                                       |
| 39781 | 1.143058              | 2.415196                                                       |
| 39783 | 1.357364              | 2.415200                                                       |
| 39785 | 1.227598              | 2.415203                                                       |
| 39787 | 1.091211              | 2.415207                                                       |
| 39789 | 1.444771              | 2.415211                                                       |

| $n$   | $\frac{\sigma(n)}{n}$ | $\frac{e^\gamma}{2} \log \log n + \frac{0.73...}{\log \log n}$ |
|-------|-----------------------|----------------------------------------------------------------|
| 39791 | 1.000025              | 2.415214                                                       |
| 39793 | 1.077275              | 2.415218                                                       |
| 39795 | 1.833396              | 2.415221                                                       |
| 39797 | 1.059276              | 2.415225                                                       |
| 39799 | 1.000025              | 2.415229                                                       |
| 39801 | 1.333434              | 2.415232                                                       |
| 39803 | 1.020225              | 2.415236                                                       |
| 39805 | 1.266173              | 2.415239                                                       |
| 39807 | 1.444771              | 2.415243                                                       |
| 39809 | 1.282926              | 2.415247                                                       |
| 39811 | 1.025445              | 2.415250                                                       |
| 39813 | 1.393716              | 2.415254                                                       |
| 39815 | 1.200151              | 2.415257                                                       |
| 39817 | 1.035236              | 2.415261                                                       |
| 39819 | 1.437304              | 2.415265                                                       |
| 39821 | 1.000025              | 2.415268                                                       |
| 39823 | 1.143058              | 2.415272                                                       |
| 39825 | 1.868173              | 2.415275                                                       |
| 39827 | 1.000025              | 2.415279                                                       |
| 39829 | 1.000025              | 2.415282                                                       |
| 39831 | 1.561799              | 2.415286                                                       |
| 39833 | 1.017950              | 2.415290                                                       |
| 39835 | 1.243530              | 2.415293                                                       |
| 39837 | 1.556744              | 2.415297                                                       |
| 39839 | 1.000025              | 2.415300                                                       |
| 39841 | 1.000025              | 2.415304                                                       |
| 39843 | 1.526993              | 2.415308                                                       |
| 39845 | 1.294416              | 2.415311                                                       |
| 39847 | 1.000025              | 2.415315                                                       |
| 39849 | 1.373184              | 2.415318                                                       |
| 39851 | 1.143058              | 2.415322                                                       |
| 39853 | 1.091210              | 2.415326                                                       |
| 39855 | 1.600602              | 2.415329                                                       |
| 39857 | 1.000025              | 2.415333                                                       |
| 39859 | 1.044080              | 2.415336                                                       |
| 39861 | 1.492386              | 2.415340                                                       |
| 39863 | 1.000025              | 2.415344                                                       |
| 39865 | 1.473774              | 2.415347                                                       |
| 39867 | 1.356912              | 2.415351                                                       |
| 39869 | 1.000025              | 2.415354                                                       |
| 39871 | 1.077274              | 2.415358                                                       |
| 39873 | 1.333434              | 2.415361                                                       |
| 39875 | 1.408401              | 2.415365                                                       |
| 39877 | 1.000025              | 2.415369                                                       |

| $n$   | $\frac{\sigma(n)}{n}$ | $\frac{e^\gamma}{2} \log \log n + \frac{0.73...}{\log \log n}$ |
|-------|-----------------------|----------------------------------------------------------------|
| 39879 | 1.701146              | 2.415372                                                       |
| 39881 | 1.053133              | 2.415376                                                       |
| 39883 | 1.000025              | 2.415379                                                       |
| 39885 | 1.600602              | 2.415383                                                       |
| 39887 | 1.000025              | 2.415387                                                       |
| 39889 | 1.011707              | 2.415390                                                       |
| 39891 | 1.333434              | 2.415394                                                       |
| 39893 | 1.179154              | 2.415397                                                       |
| 39895 | 1.227221              | 2.415401                                                       |
| 39897 | 1.751711              | 2.415405                                                       |
| 39899 | 1.059275              | 2.415408                                                       |
| 39901 | 1.000025              | 2.415412                                                       |
| 39903 | 1.366514              | 2.415415                                                       |
| 39905 | 1.255782              | 2.415419                                                       |
| 39907 | 1.143058              | 2.415422                                                       |
| 39909 | 1.363903              | 2.415426                                                       |
| 39911 | 1.012052              | 2.415430                                                       |
| 39913 | 1.010197              | 2.415433                                                       |
| 39915 | 1.735287              | 2.415437                                                       |
| 39917 | 1.010096              | 2.415440                                                       |
| 39919 | 1.154338              | 2.415444                                                       |
| 39921 | 1.524611              | 2.415448                                                       |
| 39923 | 1.119355              | 2.415451                                                       |
| 39925 | 1.240776              | 2.415455                                                       |
| 39927 | 1.333434              | 2.415458                                                       |
| 39929 | 1.000025              | 2.415462                                                       |
| 39931 | 1.015552              | 2.415465                                                       |
| 39933 | 1.636241              | 2.415469                                                       |
| 39935 | 1.404482              | 2.415473                                                       |
| 39937 | 1.000025              | 2.415476                                                       |
| 39939 | 1.333433              | 2.415480                                                       |
| 39941 | 1.091210              | 2.415483                                                       |
| 39943 | 1.018451              | 2.415487                                                       |
| 39945 | 1.600601              | 2.415491                                                       |
| 39947 | 1.024357              | 2.415494                                                       |
| 39949 | 1.233573              | 2.415498                                                       |
| 39951 | 1.515056              | 2.415501                                                       |
| 39953 | 1.000025              | 2.415505                                                       |
| 39955 | 1.228983              | 2.415508                                                       |
| 39957 | 1.405511              | 2.415512                                                       |
| 39959 | 1.033059              | 2.415516                                                       |
| 39961 | 1.013488              | 2.415519                                                       |
| 39963 | 1.671947              | 2.415523                                                       |
| 39965 | 1.200150              | 2.415526                                                       |

| $n$   | $\frac{\sigma(n)}{n}$ | $\frac{e^\gamma}{2} \log \log n + \frac{0.73...}{\log \log n}$ |
|-------|-----------------------|----------------------------------------------------------------|
| 39967 | 1.059274              | 2.415530                                                       |
| 39969 | 1.444770              | 2.415533                                                       |
| 39971 | 1.000025              | 2.415537                                                       |
| 39973 | 1.015886              | 2.415541                                                       |
| 39975 | 1.823940              | 2.415544                                                       |
| 39977 | 1.143057              | 2.415548                                                       |
| 39979 | 1.000025              | 2.415551                                                       |
| 39981 | 1.333433              | 2.415555                                                       |
| 39983 | 1.000025              | 2.415559                                                       |
| 39985 | 1.310892              | 2.415562                                                       |
| 39987 | 1.482482              | 2.415566                                                       |
| 39989 | 1.000025              | 2.415569                                                       |
| 39991 | 1.188267              | 2.415573                                                       |
| 39993 | 1.333433              | 2.415576                                                       |
| 39995 | 1.266158              | 2.415580                                                       |
| 39997 | 1.094482              | 2.415584                                                       |
| 39999 | 1.360034              | 2.415587                                                       |
| 40001 | 1.146571              | 2.415591                                                       |
| 40003 | 1.011924              | 2.415594                                                       |
| 40005 | 1.996550              | 2.415598                                                       |
| 40007 | 1.091209              | 2.415601                                                       |
| 40009 | 1.000025              | 2.415605                                                       |
| 40011 | 1.333433              | 2.415609                                                       |
| 40013 | 1.000025              | 2.415612                                                       |
| 40015 | 1.230738              | 2.415616                                                       |
| 40017 | 1.333433              | 2.415619                                                       |
| 40019 | 1.143057              | 2.415623                                                       |
| 40021 | 1.033058              | 2.415626                                                       |
| 40023 | 1.444769              | 2.415630                                                       |
| 40025 | 1.240775              | 2.415634                                                       |
| 40027 | 1.077273              | 2.415637                                                       |
| 40029 | 1.455745              | 2.415641                                                       |
| 40031 | 1.000025              | 2.415644                                                       |
| 40033 | 1.252966              | 2.415648                                                       |
| 40035 | 1.704908              | 2.415651                                                       |
| 40037 | 1.000025              | 2.415655                                                       |
| 40039 | 1.000025              | 2.415659                                                       |
| 40041 | 1.482480              | 2.415662                                                       |
| 40043 | 1.044078              | 2.415666                                                       |
| 40045 | 1.200150              | 2.415669                                                       |
| 40047 | 1.524609              | 2.415673                                                       |
| 40049 | 1.035232              | 2.415676                                                       |
| 40051 | 1.102494              | 2.415680                                                       |
| 40053 | 1.462063              | 2.415684                                                       |

| $n$   | $\frac{\sigma(n)}{n}$ | $\frac{e^\gamma}{2} \log \log n + \frac{0.73...}{\log \log n}$ |
|-------|-----------------------|----------------------------------------------------------------|
| 40055 | 1.200150              | 2.415687                                                       |
| 40057 | 1.025439              | 2.415691                                                       |
| 40059 | 1.444769              | 2.415694                                                       |
| 40061 | 1.174209              | 2.415698                                                       |
| 40063 | 1.000025              | 2.415701                                                       |
| 40065 | 1.600599              | 2.415705                                                       |
| 40067 | 1.012304              | 2.415709                                                       |
| 40069 | 1.059273              | 2.415712                                                       |
| 40071 | 1.445235              | 2.415716                                                       |
| 40073 | 1.091209              | 2.415719                                                       |
| 40075 | 1.423331              | 2.415723                                                       |
| 40077 | 1.488235              | 2.415726                                                       |
| 40079 | 1.077272              | 2.415730                                                       |
| 40081 | 1.010454              | 2.415734                                                       |
| 40083 | 1.379537              | 2.415737                                                       |
| 40085 | 1.200150              | 2.415741                                                       |
| 40087 | 1.000025              | 2.415744                                                       |
| 40089 | 1.609219              | 2.415748                                                       |
| 40091 | 1.022474              | 2.415751                                                       |
| 40093 | 1.000025              | 2.415755                                                       |
| 40095 | 1.962738              | 2.415759                                                       |
| 40097 | 1.012445              | 2.415762                                                       |
| 40099 | 1.000025              | 2.415766                                                       |
| 40101 | 1.333433              | 2.415769                                                       |
| 40103 | 1.213675              | 2.415773                                                       |
| 40105 | 1.294402              | 2.415776                                                       |
| 40107 | 1.382302              | 2.415780                                                       |
| 40109 | 1.053130              | 2.415783                                                       |
| 40111 | 1.000025              | 2.415787                                                       |
| 40113 | 1.444769              | 2.415791                                                       |
| 40115 | 1.227670              | 2.415794                                                       |
| 40117 | 1.249146              | 2.415798                                                       |
| 40119 | 1.368728              | 2.415801                                                       |
| 40121 | 1.020214              | 2.415805                                                       |
| 40123 | 1.000025              | 2.415808                                                       |
| 40125 | 1.679551              | 2.415812                                                       |
| 40127 | 1.000025              | 2.415816                                                       |
| 40129 | 1.000025              | 2.415819                                                       |
| 40131 | 1.814059              | 2.415823                                                       |
| 40133 | 1.016620              | 2.415826                                                       |
| 40135 | 1.255762              | 2.415830                                                       |
| 40137 | 1.413559              | 2.415833                                                       |
| 40139 | 1.130073              | 2.415837                                                       |
| 40141 | 1.010737              | 2.415840                                                       |

| $n$   | $\frac{\sigma(n)}{n}$ | $\frac{e^\gamma}{2} \log \log n + \frac{0.73...}{\log \log n}$ |
|-------|-----------------------|----------------------------------------------------------------|
| 40143 | 1.333433              | 2.415844                                                       |
| 40145 | 1.453930              | 2.415848                                                       |
| 40147 | 1.053130              | 2.415851                                                       |
| 40149 | 1.482478              | 2.415855                                                       |
| 40151 | 1.000025              | 2.415858                                                       |
| 40153 | 1.000025              | 2.415862                                                       |
| 40155 | 1.600598              | 2.415865                                                       |
| 40157 | 1.077272              | 2.415869                                                       |
| 40159 | 1.143056              | 2.415873                                                       |
| 40161 | 1.455741              | 2.415876                                                       |
| 40163 | 1.000025              | 2.415880                                                       |
| 40165 | 1.245861              | 2.415883                                                       |
| 40167 | 1.444768              | 2.415887                                                       |
| 40169 | 1.000025              | 2.415890                                                       |
| 40171 | 1.069926              | 2.415894                                                       |
| 40173 | 1.524606              | 2.415897                                                       |
| 40175 | 1.240772              | 2.415901                                                       |
| 40177 | 1.000025              | 2.415905                                                       |
| 40179 | 1.361905              | 2.415908                                                       |
| 40181 | 1.044076              | 2.415912                                                       |
| 40183 | 1.179006              | 2.415915                                                       |
| 40185 | 1.863382              | 2.415919                                                       |
| 40187 | 1.143056              | 2.415922                                                       |
| 40189 | 1.000025              | 2.415926                                                       |
| 40191 | 1.333433              | 2.415929                                                       |
| 40193 | 1.000025              | 2.415933                                                       |
| 40195 | 1.200149              | 2.415937                                                       |
| 40197 | 1.333433              | 2.415940                                                       |
| 40199 | 1.017936              | 2.415944                                                       |
| 40201 | 1.143056              | 2.415947                                                       |
| 40203 | 1.482476              | 2.415951                                                       |
| 40205 | 1.418331              | 2.415954                                                       |
| 40207 | 1.033054              | 2.415958                                                       |
| 40209 | 1.437290              | 2.415961                                                       |
| 40211 | 1.014648              | 2.415965                                                       |
| 40213 | 1.000025              | 2.415969                                                       |
| 40215 | 1.833346              | 2.415972                                                       |
| 40217 | 1.010916              | 2.415976                                                       |
| 40219 | 1.027972              | 2.415979                                                       |
| 40221 | 1.493250              | 2.415983                                                       |
| 40223 | 1.103846              | 2.415986                                                       |
| 40225 | 1.240771              | 2.415990                                                       |
| 40227 | 1.546424              | 2.415993                                                       |
| 40229 | 1.164682              | 2.415997                                                       |

| $n$   | $\frac{\sigma(n)}{n}$ | $\frac{e^\gamma}{2} \log \log n + \frac{0.73...}{\log \log n}$ |
|-------|-----------------------|----------------------------------------------------------------|
| 40231 | 1.000025              | 2.416001                                                       |
| 40233 | 1.333433              | 2.416004                                                       |
| 40235 | 1.294395              | 2.416008                                                       |
| 40237 | 1.000025              | 2.416011                                                       |
| 40239 | 1.535227              | 2.416015                                                       |
| 40241 | 1.000025              | 2.416018                                                       |
| 40243 | 1.143056              | 2.416022                                                       |
| 40245 | 1.600596              | 2.416025                                                       |
| 40247 | 1.010162              | 2.416029                                                       |
| 40249 | 1.091207              | 2.416033                                                       |
| 40251 | 1.333433              | 2.416036                                                       |
| 40253 | 1.000025              | 2.416040                                                       |
| 40255 | 1.226978              | 2.416043                                                       |
| 40257 | 1.731277              | 2.416047                                                       |
| 40259 | 1.011053              | 2.416050                                                       |
| 40261 | 1.140558              | 2.416054                                                       |
| 40263 | 1.333433              | 2.416057                                                       |
| 40265 | 1.200149              | 2.416061                                                       |
| 40267 | 1.016614              | 2.416065                                                       |
| 40269 | 1.379523              | 2.416068                                                       |
| 40271 | 1.249137              | 2.416072                                                       |
| 40273 | 1.115586              | 2.416075                                                       |
| 40275 | 1.801117              | 2.416079                                                       |
| 40277 | 1.000025              | 2.416082                                                       |
| 40279 | 1.022468              | 2.416086                                                       |
| 40281 | 1.382289              | 2.416089                                                       |
| 40283 | 1.000025              | 2.416093                                                       |
| 40285 | 1.372620              | 2.416096                                                       |
| 40287 | 1.437287              | 2.416100                                                       |
| 40289 | 1.000025              | 2.416104                                                       |
| 40291 | 1.024348              | 2.416107                                                       |
| 40293 | 1.630606              | 2.416111                                                       |
| 40295 | 1.200149              | 2.416114                                                       |
| 40297 | 1.018438              | 2.416118                                                       |
| 40299 | 1.619891              | 2.416121                                                       |
| 40301 | 1.010000              | 2.416125                                                       |
| 40303 | 1.025432              | 2.416128                                                       |
| 40305 | 1.600595              | 2.416132                                                       |
| 40307 | 1.059270              | 2.416135                                                       |
| 40309 | 1.010097              | 2.416139                                                       |
| 40311 | 1.482474              | 2.416143                                                       |
| 40313 | 1.233547              | 2.416146                                                       |
| 40315 | 1.310877              | 2.416150                                                       |
| 40317 | 1.357244              | 2.416153                                                       |



| $n$   | $\frac{\sigma(n)}{n}$ | $\frac{e^\gamma}{2} \log \log n + \frac{0.73...}{\log \log n}$ |
|-------|-----------------------|----------------------------------------------------------------|
| 40319 | 1.044074              | 2.416157                                                       |
| 40321 | 1.017931              | 2.416160                                                       |
| 40323 | 1.333433              | 2.416164                                                       |
| 40325 | 1.240769              | 2.416167                                                       |
| 40327 | 1.164679              | 2.416171                                                       |
| 40329 | 1.444767              | 2.416174                                                       |
| 40331 | 1.033051              | 2.416178                                                       |
| 40333 | 1.020207              | 2.416182                                                       |
| 40335 | 1.600595              | 2.416185                                                       |
| 40337 | 1.154275              | 2.416189                                                       |
| 40339 | 1.124470              | 2.416192                                                       |
| 40341 | 1.627724              | 2.416196                                                       |
| 40343 | 1.000025              | 2.416199                                                       |
| 40345 | 1.200149              | 2.416203                                                       |
| 40347 | 1.444767              | 2.416206                                                       |
| 40349 | 1.010285              | 2.416210                                                       |
| 40351 | 1.000025              | 2.416213                                                       |
| 40353 | 1.333432              | 2.416217                                                       |
| 40355 | 1.372618              | 2.416221                                                       |
| 40357 | 1.000025              | 2.416224                                                       |
| 40359 | 1.455735              | 2.416228                                                       |
| 40361 | 1.000025              | 2.416231                                                       |
| 40363 | 1.010034              | 2.416235                                                       |
| 40365 | 1.997770              | 2.416238                                                       |
| 40367 | 1.027968              | 2.416242                                                       |
| 40369 | 1.173177              | 2.416245                                                       |
| 40371 | 1.333432              | 2.416249                                                       |
| 40373 | 1.022466              | 2.416252                                                       |
| 40375 | 1.390960              | 2.416256                                                       |
| 40377 | 1.368700              | 2.416259                                                       |
| 40379 | 1.010426              | 2.416263                                                       |
| 40381 | 1.091206              | 2.416267                                                       |
| 40383 | 1.653369              | 2.416270                                                       |
| 40385 | 1.235508              | 2.416274                                                       |
| 40387 | 1.000025              | 2.416277                                                       |
| 40389 | 1.333432              | 2.416281                                                       |
| 40391 | 1.087371              | 2.416284                                                       |
| 40393 | 1.033050              | 2.416288                                                       |
| 40395 | 1.600594              | 2.416291                                                       |
| 40397 | 1.188207              | 2.416295                                                       |
| 40399 | 1.015867              | 2.416298                                                       |
| 40401 | 1.466325              | 2.416302                                                       |
| 40403 | 1.091206              | 2.416305                                                       |
| 40405 | 1.200148              | 2.416309                                                       |

| $n$   | $\frac{\sigma(n)}{n}$ | $\frac{e^\gamma}{2} \log \log n + \frac{0.73...}{\log \log n}$ |
|-------|-----------------------|----------------------------------------------------------------|
| 40407 | 1.333432              | 2.416313                                                       |
| 40409 | 1.059269              | 2.416316                                                       |
| 40411 | 1.197298              | 2.416320                                                       |
| 40413 | 1.405488              | 2.416323                                                       |
| 40415 | 1.229247              | 2.416327                                                       |
| 40417 | 1.077269              | 2.416330                                                       |
| 40419 | 1.496821              | 2.416334                                                       |
| 40421 | 1.014126              | 2.416337                                                       |
| 40423 | 1.000025              | 2.416341                                                       |
| 40425 | 2.098108              | 2.416344                                                       |
| 40427 | 1.000025              | 2.416348                                                       |
| 40429 | 1.000025              | 2.416351                                                       |
| 40431 | 1.333432              | 2.416355                                                       |
| 40433 | 1.000025              | 2.416358                                                       |
| 40435 | 1.200148              | 2.416362                                                       |
| 40437 | 1.444766              | 2.416366                                                       |
| 40439 | 1.175103              | 2.416369                                                       |
| 40441 | 1.027967              | 2.416373                                                       |
| 40443 | 1.545286              | 2.416376                                                       |
| 40445 | 1.200148              | 2.416380                                                       |
| 40447 | 1.091206              | 2.416383                                                       |
| 40449 | 1.356770              | 2.416387                                                       |
| 40451 | 1.053126              | 2.416390                                                       |
| 40453 | 1.143055              | 2.416394                                                       |
| 40455 | 1.850945              | 2.416397                                                       |
| 40457 | 1.044071              | 2.416401                                                       |
| 40459 | 1.000025              | 2.416404                                                       |
| 40461 | 1.333432              | 2.416408                                                       |
| 40463 | 1.024343              | 2.416411                                                       |
| 40465 | 1.200148              | 2.416415                                                       |
| 40467 | 1.594188              | 2.416419                                                       |
| 40469 | 1.178977              | 2.416422                                                       |
| 40471 | 1.000025              | 2.416426                                                       |
| 40473 | 1.482470              | 2.416429                                                       |
| 40475 | 1.240766              | 2.416433                                                       |
| 40477 | 1.059268              | 2.416436                                                       |
| 40479 | 1.356555              | 2.416440                                                       |
| 40481 | 1.143055              | 2.416443                                                       |
| 40483 | 1.000025              | 2.416447                                                       |
| 40485 | 1.600593              | 2.416450                                                       |
| 40487 | 1.000025              | 2.416454                                                       |
| 40489 | 1.053126              | 2.416457                                                       |
| 40491 | 1.579610              | 2.416461                                                       |
| 40493 | 1.000025              | 2.416464                                                       |

| $n$   | $\frac{\sigma(n)}{n}$ | $\frac{e^\gamma}{2} \log \log n + \frac{0.73\dots}{\log \log n}$ |
|-------|-----------------------|------------------------------------------------------------------|
| 40495 | 1.493518              | 2.416468                                                         |
| 40497 | 1.333432              | 2.416471                                                         |
| 40499 | 1.000025              | 2.416475                                                         |
| 40501 | 1.012419              | 2.416479                                                         |
| 40503 | 1.393675              | 2.416482                                                         |
| 40505 | 1.200148              | 2.416486                                                         |
| 40507 | 1.000025              | 2.416489                                                         |
| 40509 | 1.653361              | 2.416493                                                         |
| 40511 | 1.059268              | 2.416496                                                         |
| 40513 | 1.137413              | 2.416500                                                         |
| 40515 | 1.665753              | 2.416503                                                         |
| 40517 | 1.033048              | 2.416507                                                         |
| 40519 | 1.000025              | 2.416510                                                         |
| 40521 | 1.437279              | 2.416514                                                         |
| 40523 | 1.164672              | 2.416517                                                         |
| 40525 | 1.240765              | 2.416521                                                         |
| 40527 | 1.579194              | 2.416524                                                         |
| 40529 | 1.000025              | 2.416528                                                         |
| 40531 | 1.000025              | 2.416531                                                         |
| 40533 | 1.361853              | 2.416535                                                         |
| 40535 | 1.338695              | 2.416538                                                         |
| 40537 | 1.143054              | 2.416542                                                         |
| 40539 | 1.333432              | 2.416546                                                         |
| 40541 | 1.015860              | 2.416549                                                         |
| 40543 | 1.000025              | 2.416553                                                         |
| 40545 | 1.869922              | 2.416556                                                         |
| 40547 | 1.077268              | 2.416560                                                         |
| 40549 | 1.093788              | 2.416563                                                         |
| 40551 | 1.524599              | 2.416567                                                         |
| 40553 | 1.012009              | 2.416570                                                         |
| 40555 | 1.200148              | 2.416574                                                         |
| 40557 | 1.455729              | 2.416577                                                         |
| 40559 | 1.000025              | 2.416581                                                         |
| 40561 | 1.022460              | 2.416584                                                         |
| 40563 | 1.444765              | 2.416588                                                         |
| 40565 | 1.467275              | 2.416591                                                         |
| 40567 | 1.011660              | 2.416595                                                         |
| 40569 | 1.333432              | 2.416598                                                         |
| 40571 | 1.035222              | 2.416602                                                         |
| 40573 | 1.077268              | 2.416605                                                         |
| 40575 | 1.656389              | 2.416609                                                         |
| 40577 | 1.000025              | 2.416612                                                         |
| 40579 | 1.362675              | 2.416616                                                         |
| 40581 | 1.506912              | 2.416619                                                         |

| $n$   | $\frac{\sigma(n)}{n}$ | $\frac{e^\gamma}{2} \log \log n + \frac{0.73...}{\log \log n}$ |
|-------|-----------------------|----------------------------------------------------------------|
| 40583 | 1.000025              | 2.416623                                                       |
| 40585 | 1.200148              | 2.416627                                                       |
| 40587 | 1.357676              | 2.416630                                                       |
| 40589 | 1.027963              | 2.416634                                                       |
| 40591 | 1.000025              | 2.416637                                                       |
| 40593 | 1.524598              | 2.416641                                                       |
| 40595 | 1.255721              | 2.416644                                                       |
| 40597 | 1.000025              | 2.416648                                                       |
| 40599 | 1.560038              | 2.416651                                                       |
| 40601 | 1.091205              | 2.416655                                                       |
| 40603 | 1.053124              | 2.416658                                                       |
| 40605 | 1.600591              | 2.416662                                                       |
| 40607 | 1.143054              | 2.416665                                                       |
| 40609 | 1.000025              | 2.416669                                                       |
| 40611 | 1.333432              | 2.416672                                                       |
| 40613 | 1.059267              | 2.416676                                                       |
| 40615 | 1.200148              | 2.416679                                                       |
| 40617 | 1.444765              | 2.416683                                                       |
| 40619 | 1.010365              | 2.416686                                                       |
| 40621 | 1.164669              | 2.416690                                                       |
| 40623 | 1.455727              | 2.416693                                                       |
| 40625 | 1.346068              | 2.416697                                                       |
| 40627 | 1.000025              | 2.416700                                                       |
| 40629 | 1.382264              | 2.416704                                                       |
| 40631 | 1.025424              | 2.416707                                                       |
| 40633 | 1.010016              | 2.416711                                                       |
| 40635 | 2.078996              | 2.416714                                                       |
| 40637 | 1.000025              | 2.416718                                                       |
| 40639 | 1.000025              | 2.416721                                                       |
| 40641 | 1.511774              | 2.416725                                                       |
| 40643 | 1.012721              | 2.416729                                                       |
| 40645 | 1.310862              | 2.416732                                                       |
| 40647 | 1.413536              | 2.416736                                                       |
| 40649 | 1.143054              | 2.416739                                                       |
| 40651 | 1.115840              | 2.416743                                                       |
| 40653 | 1.444764              | 2.416746                                                       |
| 40655 | 1.232616              | 2.416750                                                       |
| 40657 | 1.011880              | 2.416753                                                       |
| 40659 | 1.333432              | 2.416757                                                       |
| 40661 | 1.015519              | 2.416760                                                       |
| 40663 | 1.181221              | 2.416764                                                       |
| 40665 | 1.600590              | 2.416767                                                       |
| 40667 | 1.091204              | 2.416771                                                       |
| 40669 | 1.016597              | 2.416774                                                       |

| $n$   | $\frac{\sigma(n)}{n}$ | $\frac{e^\gamma}{2} \log \log n + \frac{0.73...}{\log \log n}$ |
|-------|-----------------------|----------------------------------------------------------------|
| 40671 | 1.444764              | 2.416778                                                       |
| 40673 | 1.013449              | 2.416781                                                       |
| 40675 | 1.240762              | 2.416785                                                       |
| 40677 | 1.652039              | 2.416788                                                       |
| 40679 | 1.053123              | 2.416792                                                       |
| 40681 | 1.059266              | 2.416795                                                       |
| 40683 | 1.359192              | 2.416799                                                       |
| 40685 | 1.226988              | 2.416802                                                       |
| 40687 | 1.097156              | 2.416806                                                       |
| 40689 | 1.627958              | 2.416809                                                       |
| 40691 | 1.143054              | 2.416813                                                       |
| 40693 | 1.000025              | 2.416816                                                       |
| 40695 | 1.600590              | 2.416820                                                       |
| 40697 | 1.000025              | 2.416823                                                       |
| 40699 | 1.000025              | 2.416827                                                       |
| 40701 | 1.333432              | 2.416830                                                       |
| 40703 | 1.122669              | 2.416834                                                       |
| 40705 | 1.372608              | 2.416837                                                       |
| 40707 | 1.444764              | 2.416841                                                       |
| 40709 | 1.000025              | 2.416844                                                       |
| 40711 | 1.091204              | 2.416848                                                       |
| 40713 | 1.369980              | 2.416851                                                       |
| 40715 | 1.273241              | 2.416855                                                       |
| 40717 | 1.053123              | 2.416858                                                       |
| 40719 | 1.556620              | 2.416862                                                       |
| 40721 | 1.024336              | 2.416865                                                       |
| 40723 | 1.009945              | 2.416869                                                       |
| 40725 | 1.801007              | 2.416872                                                       |
| 40727 | 1.010632              | 2.416876                                                       |
| 40729 | 1.087333              | 2.416879                                                       |
| 40731 | 1.333432              | 2.416883                                                       |
| 40733 | 1.303317              | 2.416886                                                       |
| 40735 | 1.200147              | 2.416890                                                       |
| 40737 | 1.373101              | 2.416893                                                       |
| 40739 | 1.000025              | 2.416897                                                       |
| 40741 | 1.010874              | 2.416901                                                       |
| 40743 | 1.496797              | 2.416904                                                       |
| 40745 | 1.245797              | 2.416908                                                       |
| 40747 | 1.143053              | 2.416911                                                       |
| 40749 | 1.446514              | 2.416915                                                       |
| 40751 | 1.000025              | 2.416918                                                       |
| 40753 | 1.014109              | 2.416922                                                       |
| 40755 | 1.978653              | 2.416925                                                       |
| 40757 | 1.020193              | 2.416929                                                       |

| $n$   | $\frac{\sigma(n)}{n}$ | $\frac{e^\gamma}{2} \log \log n + \frac{0.73...}{\log \log n}$ |
|-------|-----------------------|----------------------------------------------------------------|
| 40759 | 1.000025              | 2.416932                                                       |
| 40761 | 1.653345              | 2.416936                                                       |
| 40763 | 1.000025              | 2.416939                                                       |
| 40765 | 1.243420              | 2.416943                                                       |
| 40767 | 1.356391              | 2.416946                                                       |
| 40769 | 1.018421              | 2.416950                                                       |
| 40771 | 1.000025              | 2.416953                                                       |
| 40773 | 1.333431              | 2.416957                                                       |
| 40775 | 1.423225              | 2.416960                                                       |
| 40777 | 1.102435              | 2.416964                                                       |
| 40779 | 1.514897              | 2.416967                                                       |
| 40781 | 1.077266              | 2.416971                                                       |
| 40783 | 1.059265              | 2.416974                                                       |
| 40785 | 1.600588              | 2.416978                                                       |
| 40787 | 1.000025              | 2.416981                                                       |
| 40789 | 1.143053              | 2.416985                                                       |
| 40791 | 1.333431              | 2.416988                                                       |
| 40793 | 1.064741              | 2.416992                                                       |
| 40795 | 1.235446              | 2.416995                                                       |
| 40797 | 1.482462              | 2.416999                                                       |
| 40799 | 1.091203              | 2.417002                                                       |
| 40801 | 1.000025              | 2.417006                                                       |
| 40803 | 1.599882              | 2.417009                                                       |
| 40805 | 1.200147              | 2.417013                                                       |
| 40807 | 1.117063              | 2.417016                                                       |
| 40809 | 1.361268              | 2.417020                                                       |
| 40811 | 1.027958              | 2.417023                                                       |
| 40813 | 1.000025              | 2.417027                                                       |
| 40815 | 1.735244              | 2.417030                                                       |
| 40817 | 1.235221              | 2.417034                                                       |
| 40819 | 1.000024              | 2.417037                                                       |
| 40821 | 1.455721              | 2.417041                                                       |
| 40823 | 1.000024              | 2.417044                                                       |
| 40825 | 1.312137              | 2.417048                                                       |
| 40827 | 1.379479              | 2.417051                                                       |
| 40829 | 1.000024              | 2.417055                                                       |
| 40831 | 1.206926              | 2.417058                                                       |
| 40833 | 1.560013              | 2.417062                                                       |
| 40835 | 1.200147              | 2.417065                                                       |
| 40837 | 1.012709              | 2.417069                                                       |
| 40839 | 1.333431              | 2.417072                                                       |
| 40841 | 1.000024              | 2.417076                                                       |
| 40843 | 1.128223              | 2.417079                                                       |
| 40845 | 1.833272              | 2.417083                                                       |

| $n$   | $\frac{\sigma(n)}{n}$ | $\frac{e^\gamma}{2} \log \log n + \frac{0.73...}{\log \log n}$ |
|-------|-----------------------|----------------------------------------------------------------|
| 40847 | 1.000024              | 2.417086                                                       |
| 40849 | 1.000024              | 2.417090                                                       |
| 40851 | 1.586252              | 2.417093                                                       |
| 40853 | 1.000024              | 2.417097                                                       |
| 40855 | 1.200147              | 2.417100                                                       |
| 40857 | 1.333431              | 2.417103                                                       |
| 40859 | 1.233510              | 2.417107                                                       |
| 40861 | 1.035217              | 2.417110                                                       |
| 40863 | 1.363777              | 2.417114                                                       |
| 40865 | 1.310853              | 2.417117                                                       |
| 40867 | 1.000024              | 2.417121                                                       |
| 40869 | 1.526830              | 2.417124                                                       |
| 40871 | 1.044065              | 2.417128                                                       |
| 40873 | 1.143053              | 2.417131                                                       |
| 40875 | 1.679266              | 2.417135                                                       |
| 40877 | 1.025418              | 2.417138                                                       |
| 40879 | 1.000024              | 2.417142                                                       |
| 40881 | 1.333431              | 2.417145                                                       |
| 40883 | 1.000024              | 2.417149                                                       |
| 40885 | 1.405308              | 2.417152                                                       |
| 40887 | 1.831389              | 2.417156                                                       |
| 40889 | 1.033041              | 2.417159                                                       |
| 40891 | 1.012252              | 2.417163                                                       |
| 40893 | 1.368645              | 2.417166                                                       |
| 40895 | 1.200147              | 2.417170                                                       |
| 40897 | 1.000024              | 2.417173                                                       |
| 40899 | 1.333431              | 2.417177                                                       |
| 40901 | 1.143053              | 2.417180                                                       |
| 40903 | 1.000024              | 2.417184                                                       |
| 40905 | 1.810341              | 2.417187                                                       |
| 40907 | 1.053120              | 2.417191                                                       |
| 40909 | 1.091202              | 2.417194                                                       |
| 40911 | 1.437266              | 2.417198                                                       |
| 40913 | 1.010143              | 2.417201                                                       |
| 40915 | 1.404277              | 2.417205                                                       |
| 40917 | 1.393651              | 2.417208                                                       |
| 40919 | 1.108531              | 2.417212                                                       |
| 40921 | 1.010337              | 2.417215                                                       |
| 40923 | 1.444762              | 2.417219                                                       |
| 40925 | 1.240757              | 2.417222                                                       |
| 40927 | 1.000024              | 2.417226                                                       |
| 40929 | 1.524591              | 2.417229                                                       |
| 40931 | 1.109086              | 2.417233                                                       |
| 40933 | 1.000024              | 2.417236                                                       |

| $n$   | $\frac{\sigma(n)}{n}$ | $\frac{e^\gamma}{2} \log \log n + \frac{0.73\dots}{\log \log n}$ |
|-------|-----------------------|------------------------------------------------------------------|
| 40935 | 1.600586              | 2.417240                                                         |
| 40937 | 1.116252              | 2.417243                                                         |
| 40939 | 1.000024              | 2.417247                                                         |
| 40941 | 1.444762              | 2.417250                                                         |
| 40943 | 1.143053              | 2.417254                                                         |
| 40945 | 1.266089              | 2.417257                                                         |
| 40947 | 1.333431              | 2.417261                                                         |
| 40949 | 1.000024              | 2.417264                                                         |
| 40951 | 1.033039              | 2.417268                                                         |
| 40953 | 1.561204              | 2.417271                                                         |
| 40955 | 1.200147              | 2.417275                                                         |
| 40957 | 1.143052              | 2.417278                                                         |
| 40959 | 1.558632              | 2.417281                                                         |
| 40961 | 1.000024              | 2.417285                                                         |
| 40963 | 1.131948              | 2.417288                                                         |
| 40965 | 1.600586              | 2.417292                                                         |
| 40967 | 1.015842              | 2.417295                                                         |
| 40969 | 1.020186              | 2.417299                                                         |
| 40971 | 1.524591              | 2.417302                                                         |
| 40973 | 1.000024              | 2.417306                                                         |
| 40975 | 1.361806              | 2.417309                                                         |
| 40977 | 1.503770              | 2.417313                                                         |
| 40979 | 1.024330              | 2.417316                                                         |
| 40981 | 1.011981              | 2.417320                                                         |
| 40983 | 1.405461              | 2.417323                                                         |
| 40985 | 1.372600              | 2.417327                                                         |
| 40987 | 1.059263              | 2.417330                                                         |
| 40989 | 1.437264              | 2.417334                                                         |
| 40991 | 1.009978              | 2.417337                                                         |
| 40993 | 1.000024              | 2.417341                                                         |
| 40995 | 1.735236              | 2.417344                                                         |
| 40997 | 1.091202              | 2.417348                                                         |
| 40999 | 1.143052              | 2.417351                                                         |
| 41001 | 1.358016              | 2.417355                                                         |
| 41003 | 1.010853              | 2.417358                                                         |
| 41005 | 1.229118              | 2.417362                                                         |
| 41007 | 1.333431              | 2.417365                                                         |
| 41009 | 1.044063              | 2.417369                                                         |
| 41011 | 1.000024              | 2.417372                                                         |
| 41013 | 1.778948              | 2.417376                                                         |
| 41015 | 1.294356              | 2.417379                                                         |
| 41017 | 1.000024              | 2.417382                                                         |
| 41019 | 1.478534              | 2.417386                                                         |
| 41021 | 1.123327              | 2.417389                                                         |



| $n$   | $\frac{\sigma(n)}{n}$ | $\frac{e^\gamma}{2} \log \log n + \frac{0.73...}{\log \log n}$ |
|-------|-----------------------|----------------------------------------------------------------|
| 41023 | 1.000024              | 2.417393                                                       |
| 41025 | 1.656356              | 2.417396                                                       |
| 41027 | 1.143052              | 2.417400                                                       |
| 41029 | 1.013430              | 2.417403                                                       |
| 41031 | 1.490385              | 2.417407                                                       |
| 41033 | 1.027953              | 2.417410                                                       |
| 41035 | 1.245766              | 2.417414                                                       |
| 41037 | 1.333431              | 2.417417                                                       |
| 41039 | 1.000024              | 2.417421                                                       |
| 41041 | 1.375405              | 2.417424                                                       |
| 41043 | 1.333431              | 2.417428                                                       |
| 41045 | 1.200146              | 2.417431                                                       |
| 41047 | 1.000024              | 2.417435                                                       |
| 41049 | 1.444761              | 2.417438                                                       |
| 41051 | 1.000024              | 2.417442                                                       |
| 41053 | 1.017904              | 2.417445                                                       |
| 41055 | 2.020314              | 2.417449                                                       |
| 41057 | 1.000024              | 2.417452                                                       |
| 41059 | 1.053119              | 2.417456                                                       |
| 41061 | 1.333431              | 2.417459                                                       |
| 41063 | 1.091201              | 2.417462                                                       |
| 41065 | 1.234336              | 2.417466                                                       |
| 41067 | 1.622032              | 2.417469                                                       |
| 41069 | 1.143052              | 2.417473                                                       |
| 41071 | 1.016581              | 2.417476                                                       |
| 41073 | 1.333431              | 2.417480                                                       |
| 41075 | 1.304151              | 2.417483                                                       |
| 41077 | 1.000024              | 2.417487                                                       |
| 41079 | 1.333431              | 2.417490                                                       |
| 41081 | 1.000024              | 2.417494                                                       |
| 41083 | 1.143052              | 2.417497                                                       |
| 41085 | 1.913691              | 2.417501                                                       |
| 41087 | 1.009954              | 2.417504                                                       |
| 41089 | 1.059262              | 2.417508                                                       |
| 41091 | 1.333431              | 2.417511                                                       |
| 41093 | 1.124279              | 2.417515                                                       |
| 41095 | 1.200146              | 2.417518                                                       |
| 41097 | 1.619583              | 2.417522                                                       |
| 41099 | 1.015499              | 2.417525                                                       |
| 41101 | 1.044062              | 2.417528                                                       |
| 41103 | 1.444761              | 2.417532                                                       |
| 41105 | 1.200146              | 2.417535                                                       |
| 41107 | 1.131486              | 2.417539                                                       |
| 41109 | 1.359118              | 2.417542                                                       |

| $n$   | $\frac{\sigma(n)}{n}$ | $\frac{e^\gamma}{2} \log \log n + \frac{0.73...}{\log \log n}$ |
|-------|-----------------------|----------------------------------------------------------------|
| 41111 | 1.164652              | 2.417546                                                       |
| 41113 | 1.000024              | 2.417549                                                       |
| 41115 | 1.600584              | 2.417553                                                       |
| 41117 | 1.000024              | 2.417556                                                       |
| 41119 | 1.077264              | 2.417560                                                       |
| 41121 | 1.482454              | 2.417563                                                       |
| 41123 | 1.103032              | 2.417567                                                       |
| 41125 | 1.456632              | 2.417570                                                       |
| 41127 | 1.333431              | 2.417574                                                       |
| 41129 | 1.091201              | 2.417577                                                       |
| 41131 | 1.000024              | 2.417581                                                       |
| 41133 | 1.333431              | 2.417584                                                       |
| 41135 | 1.266075              | 2.417587                                                       |
| 41137 | 1.033036              | 2.417591                                                       |
| 41139 | 1.653322              | 2.417594                                                       |
| 41141 | 1.000024              | 2.417598                                                       |
| 41143 | 1.000024              | 2.417601                                                       |
| 41145 | 1.731243              | 2.417605                                                       |
| 41147 | 1.044062              | 2.417608                                                       |
| 41149 | 1.000024              | 2.417612                                                       |
| 41151 | 1.539695              | 2.417615                                                       |
| 41153 | 1.143052              | 2.417619                                                       |
| 41155 | 1.200146              | 2.417622                                                       |
| 41157 | 1.535097              | 2.417626                                                       |
| 41159 | 1.014602              | 2.417629                                                       |
| 41161 | 1.000024              | 2.417633                                                       |
| 41163 | 1.333431              | 2.417636                                                       |
| 41165 | 1.200146              | 2.417639                                                       |
| 41167 | 1.143051              | 2.417643                                                       |
| 41169 | 1.333430              | 2.417646                                                       |
| 41171 | 1.077263              | 2.417650                                                       |
| 41173 | 1.154154              | 2.417653                                                       |
| 41175 | 1.867152              | 2.417657                                                       |
| 41177 | 1.000024              | 2.417660                                                       |
| 41179 | 1.000024              | 2.417664                                                       |
| 41181 | 1.594522              | 2.417667                                                       |
| 41183 | 1.000024              | 2.417671                                                       |
| 41185 | 1.200146              | 2.417674                                                       |
| 41187 | 1.333430              | 2.417678                                                       |
| 41189 | 1.000024              | 2.417681                                                       |
| 41191 | 1.059261              | 2.417685                                                       |
| 41193 | 1.514820              | 2.417688                                                       |
| 41195 | 1.510086              | 2.417691                                                       |
| 41197 | 1.077263              | 2.417695                                                       |

| $n$   | $\frac{\sigma(n)}{n}$ | $\frac{e^\gamma}{2} \log \log n + \frac{0.73...}{\log \log n}$ |
|-------|-----------------------|----------------------------------------------------------------|
| 41199 | 1.379451              | 2.417698                                                       |
| 41201 | 1.000024              | 2.417702                                                       |
| 41203 | 1.000024              | 2.417705                                                       |
| 41205 | 1.663487              | 2.417709                                                       |
| 41207 | 1.013420              | 2.417712                                                       |
| 41209 | 1.204761              | 2.417716                                                       |
| 41211 | 1.526777              | 2.417719                                                       |
| 41213 | 1.000024              | 2.417723                                                       |
| 41215 | 1.200146              | 2.417726                                                       |
| 41217 | 1.455710              | 2.417730                                                       |
| 41219 | 1.022441              | 2.417733                                                       |
| 41221 | 1.000024              | 2.417736                                                       |
| 41223 | 1.651893              | 2.417740                                                       |
| 41225 | 1.326477              | 2.417743                                                       |
| 41227 | 1.000024              | 2.417747                                                       |
| 41229 | 1.496762              | 2.417750                                                       |
| 41231 | 1.000024              | 2.417754                                                       |
| 41233 | 1.000024              | 2.417757                                                       |
| 41235 | 1.600582              | 2.417761                                                       |
| 41237 | 1.177971              | 2.417764                                                       |
| 41239 | 1.145324              | 2.417768                                                       |
| 41241 | 1.361752              | 2.417771                                                       |
| 41243 | 1.000024              | 2.417775                                                       |
| 41245 | 1.227203              | 2.417778                                                       |
| 41247 | 1.444760              | 2.417781                                                       |
| 41249 | 1.140391              | 2.417785                                                       |
| 41251 | 1.172917              | 2.417788                                                       |
| 41253 | 1.333430              | 2.417792                                                       |
| 41255 | 1.237959              | 2.417795                                                       |
| 41257 | 1.000024              | 2.417799                                                       |
| 41259 | 1.413510              | 2.417802                                                       |
| 41261 | 1.135406              | 2.417806                                                       |
| 41263 | 1.000024              | 2.417809                                                       |
| 41265 | 1.996074              | 2.417813                                                       |
| 41267 | 1.035210              | 2.417816                                                       |
| 41269 | 1.000024              | 2.417819                                                       |
| 41271 | 1.333430              | 2.417823                                                       |
| 41273 | 1.010346              | 2.417826                                                       |
| 41275 | 1.345899              | 2.417830                                                       |
| 41277 | 1.333430              | 2.417833                                                       |
| 41279 | 1.143051              | 2.417837                                                       |
| 41281 | 1.000024              | 2.417840                                                       |
| 41283 | 1.627789              | 2.417844                                                       |
| 41285 | 1.255662              | 2.417847                                                       |

| $n$   | $\frac{\sigma(n)}{n}$ | $\frac{e^\gamma}{2} \log \log n + \frac{0.73...}{\log \log n}$ |
|-------|-----------------------|----------------------------------------------------------------|
| 41287 | 1.098651              | 2.417851                                                       |
| 41289 | 1.333430              | 2.417854                                                       |
| 41291 | 1.010196              | 2.417857                                                       |
| 41293 | 1.213571              | 2.417861                                                       |
| 41295 | 1.600581              | 2.417864                                                       |
| 41297 | 1.017895              | 2.417868                                                       |
| 41299 | 1.000024              | 2.417871                                                       |
| 41301 | 1.559962              | 2.417875                                                       |
| 41303 | 1.012227              | 2.417878                                                       |
| 41305 | 1.310834              | 2.417882                                                       |
| 41307 | 1.556540              | 2.417885                                                       |
| 41309 | 1.012370              | 2.417889                                                       |
| 41311 | 1.011837              | 2.417892                                                       |
| 41313 | 1.366350              | 2.417895                                                       |
| 41315 | 1.200145              | 2.417899                                                       |
| 41317 | 1.014594              | 2.417902                                                       |
| 41319 | 1.444759              | 2.417906                                                       |
| 41321 | 1.143051              | 2.417909                                                       |
| 41323 | 1.057329              | 2.417913                                                       |
| 41325 | 1.800363              | 2.417916                                                       |
| 41327 | 1.247998              | 2.417920                                                       |
| 41329 | 1.027946              | 2.417923                                                       |
| 41331 | 1.393627              | 2.417927                                                       |
| 41333 | 1.000024              | 2.417930                                                       |
| 41335 | 1.372590              | 2.417933                                                       |
| 41337 | 1.482449              | 2.417937                                                       |
| 41339 | 1.016570              | 2.417940                                                       |
| 41341 | 1.000024              | 2.417944                                                       |
| 41343 | 1.333430              | 2.417947                                                       |
| 41345 | 1.200145              | 2.417951                                                       |
| 41347 | 1.009989              | 2.417954                                                       |
| 41349 | 1.671624              | 2.417958                                                       |
| 41351 | 1.000024              | 2.417961                                                       |
| 41353 | 1.077262              | 2.417964                                                       |
| 41355 | 1.735219              | 2.417968                                                       |
| 41357 | 1.000024              | 2.417971                                                       |
| 41359 | 1.018400              | 2.417975                                                       |
| 41361 | 1.413505              | 2.417978                                                       |
| 41363 | 1.206876              | 2.417982                                                       |
| 41365 | 1.200145              | 2.417985                                                       |
| 41367 | 1.333430              | 2.417989                                                       |
| 41369 | 1.025405              | 2.417992                                                       |
| 41371 | 1.091199              | 2.417996                                                       |
| 41373 | 1.444759              | 2.417999                                                       |

| $n$   | $\frac{\sigma(n)}{n}$ | $\frac{e^\gamma}{2} \log \log n + \frac{0.73\dots}{\log \log n}$ |
|-------|-----------------------|------------------------------------------------------------------|
| 41375 | 1.251770              | 2.418002                                                         |
| 41377 | 1.197187              | 2.418006                                                         |
| 41379 | 1.437251              | 2.418009                                                         |
| 41381 | 1.000024              | 2.418013                                                         |
| 41383 | 1.035208              | 2.418016                                                         |
| 41385 | 1.670170              | 2.418020                                                         |
| 41387 | 1.000024              | 2.418023                                                         |
| 41389 | 1.000024              | 2.418027                                                         |
| 41391 | 1.730618              | 2.418030                                                         |
| 41393 | 1.127147              | 2.418033                                                         |
| 41395 | 1.273197              | 2.418037                                                         |
| 41397 | 1.333430              | 2.418040                                                         |
| 41399 | 1.000024              | 2.418044                                                         |
| 41401 | 1.053115              | 2.418047                                                         |
| 41403 | 1.373041              | 2.418051                                                         |
| 41405 | 1.511557              | 2.418054                                                         |
| 41407 | 1.022436              | 2.418058                                                         |
| 41409 | 1.491850              | 2.418061                                                         |
| 41411 | 1.000024              | 2.418064                                                         |
| 41413 | 1.000024              | 2.418068                                                         |
| 41415 | 1.752409              | 2.418071                                                         |
| 41417 | 1.014076              | 2.418075                                                         |
| 41419 | 1.173568              | 2.418078                                                         |
| 41421 | 1.333430              | 2.418082                                                         |
| 41423 | 1.044058              | 2.418085                                                         |
| 41425 | 1.240748              | 2.418089                                                         |
| 41427 | 1.444758              | 2.418092                                                         |
| 41429 | 1.059258              | 2.418095                                                         |
| 41431 | 1.077261              | 2.418099                                                         |
| 41433 | 1.524582              | 2.418102                                                         |
| 41435 | 1.200145              | 2.418106                                                         |
| 41437 | 1.091199              | 2.418109                                                         |
| 41439 | 1.405439              | 2.418113                                                         |
| 41441 | 1.035207              | 2.418116                                                         |
| 41443 | 1.000024              | 2.418120                                                         |
| 41445 | 1.783569              | 2.418123                                                         |
| 41447 | 1.185900              | 2.418126                                                         |
| 41449 | 1.009916              | 2.418130                                                         |
| 41451 | 1.369907              | 2.418133                                                         |
| 41453 | 1.000024              | 2.418137                                                         |
| 41455 | 1.200145              | 2.418140                                                         |
| 41457 | 1.437248              | 2.418144                                                         |
| 41459 | 1.091199              | 2.418147                                                         |
| 41461 | 1.143050              | 2.418150                                                         |

| $n$   | $\frac{\sigma(n)}{n}$ | $\frac{e^\gamma}{2} \log \log n + \frac{0.73...}{\log \log n}$ |
|-------|-----------------------|----------------------------------------------------------------|
| 41463 | 1.535055              | 2.418154                                                       |
| 41465 | 1.200145              | 2.418157                                                       |
| 41467 | 1.000024              | 2.418161                                                       |
| 41469 | 1.393619              | 2.418164                                                       |
| 41471 | 1.011598              | 2.418168                                                       |
| 41473 | 1.016565              | 2.418171                                                       |
| 41475 | 1.913442              | 2.418175                                                       |
| 41477 | 1.099404              | 2.418178                                                       |
| 41479 | 1.000024              | 2.418181                                                       |
| 41481 | 1.579518              | 2.418185                                                       |
| 41483 | 1.077261              | 2.418188                                                       |
| 41485 | 1.200145              | 2.418192                                                       |
| 41487 | 1.333430              | 2.418195                                                       |
| 41489 | 1.143050              | 2.418199                                                       |
| 41491 | 1.000024              | 2.418202                                                       |
| 41493 | 1.333430              | 2.418206                                                       |
| 41495 | 1.234269              | 2.418209                                                       |
| 41497 | 1.059257              | 2.418212                                                       |
| 41499 | 1.561483              | 2.418216                                                       |
| 41501 | 1.022433              | 2.418219                                                       |
| 41503 | 1.281835              | 2.418223                                                       |
| 41505 | 1.600578              | 2.418226                                                       |
| 41507 | 1.000024              | 2.418230                                                       |
| 41509 | 1.122455              | 2.418233                                                       |
| 41511 | 1.356363              | 2.418236                                                       |
| 41513 | 1.000024              | 2.418240                                                       |
| 41515 | 1.321546              | 2.418243                                                       |
| 41517 | 1.653299              | 2.418247                                                       |
| 41519 | 1.000024              | 2.418250                                                       |
| 41521 | 1.000024              | 2.418254                                                       |
| 41523 | 1.333430              | 2.418257                                                       |
| 41525 | 1.361686              | 2.418260                                                       |
| 41527 | 1.010812              | 2.418264                                                       |
| 41529 | 1.356161              | 2.418267                                                       |
| 41531 | 1.213551              | 2.418271                                                       |
| 41533 | 1.025401              | 2.418274                                                       |
| 41535 | 1.892958              | 2.418278                                                       |
| 41537 | 1.015480              | 2.418281                                                       |
| 41539 | 1.000024              | 2.418284                                                       |
| 41541 | 1.361161              | 2.418288                                                       |
| 41543 | 1.000024              | 2.418291                                                       |
| 41545 | 1.372584              | 2.418295                                                       |
| 41547 | 1.455701              | 2.418298                                                       |
| 41549 | 1.000024              | 2.418302                                                       |

| $n$   | $\frac{\sigma(n)}{n}$ | $\frac{e^\gamma}{2} \log \log n + \frac{0.73...}{\log \log n}$ |
|-------|-----------------------|----------------------------------------------------------------|
| 41551 | 1.027942              | 2.418305                                                       |
| 41553 | 1.578707              | 2.418309                                                       |
| 41555 | 1.200144              | 2.418312                                                       |
| 41557 | 1.035205              | 2.418315                                                       |
| 41559 | 1.524580              | 2.418319                                                       |
| 41561 | 1.131830              | 2.418322                                                       |
| 41563 | 1.013401              | 2.418326                                                       |
| 41565 | 1.704511              | 2.418329                                                       |
| 41567 | 1.009840              | 2.418333                                                       |
| 41569 | 1.091198              | 2.418336                                                       |
| 41571 | 1.501046              | 2.418339                                                       |
| 41573 | 1.143050              | 2.418343                                                       |
| 41575 | 1.240746              | 2.418346                                                       |
| 41577 | 1.333430              | 2.418350                                                       |
| 41579 | 1.000024              | 2.418353                                                       |
| 41581 | 1.024314              | 2.418357                                                       |
| 41583 | 1.357478              | 2.418360                                                       |
| 41585 | 1.200144              | 2.418363                                                       |
| 41587 | 1.233462              | 2.418367                                                       |
| 41589 | 1.444757              | 2.418370                                                       |
| 41591 | 1.154096              | 2.418374                                                       |
| 41593 | 1.000024              | 2.418377                                                       |
| 41595 | 1.661738              | 2.418381                                                       |
| 41597 | 1.000024              | 2.418384                                                       |
| 41599 | 1.059256              | 2.418387                                                       |
| 41601 | 1.556501              | 2.418391                                                       |
| 41603 | 1.000024              | 2.418394                                                       |
| 41605 | 1.230429              | 2.418398                                                       |
| 41607 | 1.568967              | 2.418401                                                       |
| 41609 | 1.000024              | 2.418405                                                       |
| 41611 | 1.000024              | 2.418408                                                       |
| 41613 | 1.582582              | 2.418411                                                       |
| 41615 | 1.453322              | 2.418415                                                       |
| 41617 | 1.000024              | 2.418418                                                       |
| 41619 | 1.333429              | 2.418422                                                       |
| 41621 | 1.000024              | 2.418425                                                       |
| 41623 | 1.011941              | 2.418429                                                       |
| 41625 | 1.851387              | 2.418432                                                       |
| 41627 | 1.000024              | 2.418435                                                       |
| 41629 | 1.206851              | 2.418439                                                       |
| 41631 | 1.333429              | 2.418442                                                       |
| 41633 | 1.106814              | 2.418446                                                       |
| 41635 | 1.310820              | 2.418449                                                       |
| 41637 | 1.333429              | 2.418452                                                       |

| $n$   | $\frac{\sigma(n)}{n}$ | $\frac{e^\gamma}{2} \log \log n + \frac{0.73\dots}{\log \log n}$ |
|-------|-----------------------|------------------------------------------------------------------|
| 41639 | 1.077259              | 2.418456                                                         |
| 41641 | 1.000024              | 2.418459                                                         |
| 41643 | 1.653291              | 2.418463                                                         |
| 41645 | 1.200144              | 2.418466                                                         |
| 41647 | 1.000024              | 2.418470                                                         |
| 41649 | 1.333429              | 2.418473                                                         |
| 41651 | 1.000024              | 2.418476                                                         |
| 41653 | 1.044054              | 2.418480                                                         |
| 41655 | 1.600576              | 2.418483                                                         |
| 41657 | 1.249058              | 2.418487                                                         |
| 41659 | 1.000024              | 2.418490                                                         |
| 41661 | 1.482442              | 2.418494                                                         |
| 41663 | 1.017882              | 2.418497                                                         |
| 41665 | 1.294324              | 2.418500                                                         |
| 41667 | 1.520628              | 2.418504                                                         |
| 41669 | 1.000024              | 2.418507                                                         |
| 41671 | 1.143049              | 2.418511                                                         |
| 41673 | 1.382190              | 2.418514                                                         |
| 41675 | 1.240744              | 2.418517                                                         |
| 41677 | 1.015812              | 2.418521                                                         |
| 41679 | 1.579500              | 2.418524                                                         |
| 41681 | 1.000024              | 2.418528                                                         |
| 41683 | 1.015474              | 2.418531                                                         |
| 41685 | 1.833177              | 2.418535                                                         |
| 41687 | 1.000024              | 2.418538                                                         |
| 41689 | 1.022428              | 2.418541                                                         |
| 41691 | 1.437241              | 2.418545                                                         |
| 41693 | 1.009954              | 2.418548                                                         |
| 41695 | 1.243315              | 2.418552                                                         |
| 41697 | 1.492769              | 2.418555                                                         |
| 41699 | 1.246649              | 2.418559                                                         |
| 41701 | 1.160260              | 2.418562                                                         |
| 41703 | 1.333429              | 2.418565                                                         |
| 41705 | 1.266035              | 2.418569                                                         |
| 41707 | 1.009902              | 2.418572                                                         |
| 41709 | 1.333429              | 2.418576                                                         |
| 41711 | 1.020163              | 2.418579                                                         |
| 41713 | 1.173735              | 2.418582                                                         |
| 41715 | 1.809996              | 2.418586                                                         |
| 41717 | 1.077259              | 2.418589                                                         |
| 41719 | 1.000024              | 2.418593                                                         |
| 41721 | 1.333429              | 2.418596                                                         |
| 41723 | 1.091197              | 2.418600                                                         |
| 41725 | 1.240743              | 2.418603                                                         |



| $n$   | $\frac{\sigma(n)}{n}$ | $\frac{e^\gamma}{2} \log \log n + \frac{0.73...}{\log \log n}$ |
|-------|-----------------------|----------------------------------------------------------------|
| 41727 | 1.524576              | 2.418606                                                       |
| 41729 | 1.000024              | 2.418610                                                       |
| 41731 | 1.035202              | 2.418613                                                       |
| 41733 | 1.444756              | 2.418617                                                       |
| 41735 | 1.273176              | 2.418620                                                       |
| 41737 | 1.000024              | 2.418623                                                       |
| 41739 | 1.333429              | 2.418627                                                       |
| 41741 | 1.172947              | 2.418630                                                       |
| 41743 | 1.140311              | 2.418634                                                       |
| 41745 | 1.835142              | 2.418637                                                       |
| 41747 | 1.011809              | 2.418641                                                       |
| 41749 | 1.014060              | 2.418644                                                       |
| 41751 | 1.444756              | 2.418647                                                       |
| 41753 | 1.024310              | 2.418651                                                       |
| 41755 | 1.372578              | 2.418654                                                       |
| 41757 | 1.379409              | 2.418658                                                       |
| 41759 | 1.000024              | 2.418661                                                       |
| 41761 | 1.000024              | 2.418664                                                       |
| 41763 | 1.333429              | 2.418668                                                       |
| 41765 | 1.200144              | 2.418671                                                       |
| 41767 | 1.091196              | 2.418675                                                       |
| 41769 | 1.930618              | 2.418678                                                       |
| 41771 | 1.000024              | 2.418681                                                       |
| 41773 | 1.027937              | 2.418685                                                       |
| 41775 | 1.656302              | 2.418688                                                       |
| 41777 | 1.000024              | 2.418692                                                       |
| 41779 | 1.025396              | 2.418695                                                       |
| 41781 | 1.405424              | 2.418699                                                       |
| 41783 | 1.176364              | 2.418702                                                       |
| 41785 | 1.228575              | 2.418705                                                       |
| 41787 | 1.444756              | 2.418709                                                       |
| 41789 | 1.137141              | 2.418712                                                       |
| 41791 | 1.058601              | 2.418716                                                       |
| 41793 | 1.333429              | 2.418719                                                       |
| 41795 | 1.294318              | 2.418722                                                       |
| 41797 | 1.164629              | 2.418726                                                       |
| 41799 | 1.333429              | 2.418729                                                       |
| 41801 | 1.000024              | 2.418733                                                       |
| 41803 | 1.059254              | 2.418736                                                       |
| 41805 | 1.735199              | 2.418739                                                       |
| 41807 | 1.012653              | 2.418743                                                       |
| 41809 | 1.000024              | 2.418746                                                       |
| 41811 | 1.671522              | 2.418750                                                       |
| 41813 | 1.000024              | 2.418753                                                       |

| $n$   | $\frac{\sigma(n)}{n}$ | $\frac{e^\gamma}{2} \log \log n + \frac{0.73...}{\log \log n}$ |
|-------|-----------------------|----------------------------------------------------------------|
| 41815 | 1.200143              | 2.418756                                                       |
| 41817 | 1.363656              | 2.418760                                                       |
| 41819 | 1.101891              | 2.418763                                                       |
| 41821 | 1.077258              | 2.418767                                                       |
| 41823 | 1.482438              | 2.418770                                                       |
| 41825 | 1.423072              | 2.418774                                                       |
| 41827 | 1.010257              | 2.418777                                                       |
| 41829 | 1.358675              | 2.418780                                                       |
| 41831 | 1.018383              | 2.418784                                                       |
| 41833 | 1.091196              | 2.418787                                                       |
| 41835 | 1.600574              | 2.418791                                                       |
| 41837 | 1.115185              | 2.418794                                                       |
| 41839 | 1.177848              | 2.418797                                                       |
| 41841 | 1.444755              | 2.418801                                                       |
| 41843 | 1.000024              | 2.418804                                                       |
| 41845 | 1.200143              | 2.418808                                                       |
| 41847 | 1.525557              | 2.418811                                                       |
| 41849 | 1.000024              | 2.418814                                                       |
| 41851 | 1.000024              | 2.418818                                                       |
| 41853 | 1.524574              | 2.418821                                                       |
| 41855 | 1.310811              | 2.418825                                                       |
| 41857 | 1.053109              | 2.418828                                                       |
| 41859 | 1.444755              | 2.418831                                                       |
| 41861 | 1.025394              | 2.418835                                                       |
| 41863 | 1.000024              | 2.418838                                                       |
| 41865 | 1.600573              | 2.418842                                                       |
| 41867 | 1.143048              | 2.418845                                                       |
| 41869 | 1.010294              | 2.418848                                                       |
| 41871 | 1.413484              | 2.418852                                                       |
| 41873 | 1.077257              | 2.418855                                                       |
| 41875 | 1.268251              | 2.418859                                                       |
| 41877 | 1.664303              | 2.418862                                                       |
| 41879 | 1.000024              | 2.418865                                                       |
| 41881 | 1.185836              | 2.418869                                                       |
| 41883 | 1.393596              | 2.418872                                                       |
| 41885 | 1.200143              | 2.418876                                                       |
| 41887 | 1.000024              | 2.418879                                                       |
| 41889 | 1.333429              | 2.418882                                                       |
| 41891 | 1.010050              | 2.418886                                                       |
| 41893 | 1.000024              | 2.418889                                                       |
| 41895 | 2.122449              | 2.418893                                                       |
| 41897 | 1.000024              | 2.418896                                                       |
| 41899 | 1.178835              | 2.418899                                                       |
| 41901 | 1.333429              | 2.418903                                                       |

| $n$   | $\frac{\sigma(n)}{n}$ | $\frac{e^\gamma}{2} \log \log n + \frac{0.73...}{\log \log n}$ |
|-------|-----------------------|----------------------------------------------------------------|
| 41903 | 1.000024              | 2.418906                                                       |
| 41905 | 1.318697              | 2.418910                                                       |
| 41907 | 1.361109              | 2.418913                                                       |
| 41909 | 1.143048              | 2.418916                                                       |
| 41911 | 1.000024              | 2.418920                                                       |
| 41913 | 1.444755              | 2.418923                                                       |
| 41915 | 1.226482              | 2.418927                                                       |
| 41917 | 1.009996              | 2.418930                                                       |
| 41919 | 1.356903              | 2.418933                                                       |
| 41921 | 1.131271              | 2.418937                                                       |
| 41923 | 1.174725              | 2.418940                                                       |
| 41925 | 1.821920              | 2.418944                                                       |
| 41927 | 1.000024              | 2.418947                                                       |
| 41929 | 1.044051              | 2.418950                                                       |
| 41931 | 1.482435              | 2.418954                                                       |
| 41933 | 1.053109              | 2.418957                                                       |
| 41935 | 1.200143              | 2.418961                                                       |
| 41937 | 1.524573              | 2.418964                                                       |
| 41939 | 1.059253              | 2.418967                                                       |
| 41941 | 1.000024              | 2.418971                                                       |
| 41943 | 1.538087              | 2.418974                                                       |
| 41945 | 1.200143              | 2.418978                                                       |
| 41947 | 1.000024              | 2.418981                                                       |
| 41949 | 1.487521              | 2.418984                                                       |
| 41951 | 1.233439              | 2.418988                                                       |
| 41953 | 1.000024              | 2.418991                                                       |
| 41955 | 1.600572              | 2.418995                                                       |
| 41957 | 1.000024              | 2.418998                                                       |
| 41959 | 1.000024              | 2.419001                                                       |
| 41961 | 1.358976              | 2.419005                                                       |
| 41963 | 1.035198              | 2.419008                                                       |
| 41965 | 1.509830              | 2.419012                                                       |
| 41967 | 1.444754              | 2.419015                                                       |
| 41969 | 1.000024              | 2.419018                                                       |
| 41971 | 1.075505              | 2.419022                                                       |
| 41973 | 1.413480              | 2.419025                                                       |
| 41975 | 1.311638              | 2.419029                                                       |
| 41977 | 1.077257              | 2.419032                                                       |
| 41979 | 1.524572              | 2.419035                                                       |
| 41981 | 1.000024              | 2.419039                                                       |
| 41983 | 1.000024              | 2.419042                                                       |
| 41985 | 1.783494              | 2.419046                                                       |
| 41987 | 1.102341              | 2.419049                                                       |
| 41989 | 1.009788              | 2.419052                                                       |

| $n$   | $\frac{\sigma(n)}{n}$ | $\frac{e^\gamma}{2} \log \log n + \frac{0.73...}{\log \log n}$ |
|-------|-----------------------|----------------------------------------------------------------|
| 41991 | 1.333429              | 2.419056                                                       |
| 41993 | 1.164623              | 2.419059                                                       |
| 41995 | 1.237862              | 2.419063                                                       |
| 41997 | 1.333429              | 2.419066                                                       |
| 41999 | 1.000024              | 2.419069                                                       |
| 42001 | 1.012643              | 2.419073                                                       |
| 42003 | 1.559889              | 2.419076                                                       |
| 42005 | 1.243281              | 2.419079                                                       |
| 42007 | 1.213512              | 2.419083                                                       |
| 42009 | 1.553953              | 2.419086                                                       |
| 42011 | 1.024303              | 2.419090                                                       |
| 42013 | 1.000024              | 2.419093                                                       |
| 42015 | 1.600571              | 2.419096                                                       |
| 42017 | 1.000024              | 2.419100                                                       |
| 42019 | 1.000024              | 2.419103                                                       |
| 42021 | 1.781966              | 2.419107                                                       |
| 42023 | 1.000024              | 2.419110                                                       |
| 42025 | 1.270982              | 2.419113                                                       |
| 42027 | 1.333429              | 2.419117                                                       |
| 42029 | 1.115230              | 2.419120                                                       |
| 42031 | 1.091195              | 2.419124                                                       |
| 42033 | 1.333428              | 2.419127                                                       |
| 42035 | 1.372570              | 2.419130                                                       |
| 42037 | 1.010919              | 2.419134                                                       |
| 42039 | 1.506601              | 2.419137                                                       |
| 42041 | 1.059252              | 2.419140                                                       |
| 42043 | 1.000024              | 2.419144                                                       |
| 42045 | 1.600571              | 2.419147                                                       |
| 42047 | 1.053107              | 2.419151                                                       |
| 42049 | 1.143047              | 2.419154                                                       |
| 42051 | 1.356068              | 2.419157                                                       |
| 42053 | 1.091194              | 2.419161                                                       |
| 42055 | 1.294305              | 2.419164                                                       |
| 42057 | 1.444754              | 2.419168                                                       |
| 42059 | 1.010580              | 2.419171                                                       |
| 42061 | 1.000024              | 2.419174                                                       |
| 42063 | 1.524570              | 2.419178                                                       |
| 42065 | 1.232378              | 2.419181                                                       |
| 42067 | 1.095395              | 2.419185                                                       |
| 42069 | 1.372982              | 2.419188                                                       |
| 42071 | 1.000024              | 2.419191                                                       |
| 42073 | 1.000024              | 2.419195                                                       |
| 42075 | 2.068877              | 2.419198                                                       |
| 42077 | 1.143047              | 2.419201                                                       |

| $n$   | $\frac{\sigma(n)}{n}$ | $\frac{e^\gamma}{2} \log \log n + \frac{0.73\dots}{\log \log n}$ |
|-------|-----------------------|------------------------------------------------------------------|
| 42079 | 1.035196              | 2.419205                                                         |
| 42081 | 1.461182              | 2.419208                                                         |
| 42083 | 1.000024              | 2.419212                                                         |
| 42085 | 1.266009              | 2.419215                                                         |
| 42087 | 1.333428              | 2.419218                                                         |
| 42089 | 1.000024              | 2.419222                                                         |
| 42091 | 1.164620              | 2.419225                                                         |
| 42093 | 1.482432              | 2.419229                                                         |
| 42095 | 1.200143              | 2.419232                                                         |
| 42097 | 1.128822              | 2.419235                                                         |
| 42099 | 1.333428              | 2.419239                                                         |
| 42101 | 1.000024              | 2.419242                                                         |
| 42103 | 1.015795              | 2.419245                                                         |
| 42105 | 1.833131              | 2.419249                                                         |
| 42107 | 1.117154              | 2.419252                                                         |
| 42109 | 1.059251              | 2.419256                                                         |
| 42111 | 1.444753              | 2.419259                                                         |
| 42113 | 1.044048              | 2.419262                                                         |
| 42115 | 1.200142              | 2.419266                                                         |
| 42117 | 1.356222              | 2.419269                                                         |
| 42119 | 1.249033              | 2.419272                                                         |
| 42121 | 1.015455              | 2.419276                                                         |
| 42123 | 1.405408              | 2.419279                                                         |
| 42125 | 1.251703              | 2.419283                                                         |
| 42127 | 1.012177              | 2.419286                                                         |
| 42129 | 1.500914              | 2.419289                                                         |
| 42131 | 1.000024              | 2.419293                                                         |
| 42133 | 1.233427              | 2.419296                                                         |
| 42135 | 1.630758              | 2.419300                                                         |
| 42137 | 1.035195              | 2.419303                                                         |
| 42139 | 1.000024              | 2.419306                                                         |
| 42141 | 1.455684              | 2.419310                                                         |
| 42143 | 1.103671              | 2.419313                                                         |
| 42145 | 1.200142              | 2.419316                                                         |
| 42147 | 1.700714              | 2.419320                                                         |
| 42149 | 1.011554              | 2.419323                                                         |
| 42151 | 1.017864              | 2.419327                                                         |
| 42153 | 1.333428              | 2.419330                                                         |
| 42155 | 1.200142              | 2.419333                                                         |
| 42157 | 1.000024              | 2.419337                                                         |
| 42159 | 1.530207              | 2.419340                                                         |
| 42161 | 1.206802              | 2.419343                                                         |
| 42163 | 1.091194              | 2.419347                                                         |
| 42165 | 1.735183              | 2.419350                                                         |

| $n$   | $\frac{\sigma(n)}{n}$ | $\frac{e^\gamma}{2} \log \log n + \frac{0.73...}{\log \log n}$ |
|-------|-----------------------|----------------------------------------------------------------|
| 42167 | 1.010269              | 2.419354                                                       |
| 42169 | 1.000024              | 2.419357                                                       |
| 42171 | 1.333428              | 2.419360                                                       |
| 42173 | 1.009840              | 2.419364                                                       |
| 42175 | 1.423023              | 2.419367                                                       |
| 42177 | 1.413472              | 2.419370                                                       |
| 42179 | 1.000024              | 2.419374                                                       |
| 42181 | 1.000024              | 2.419377                                                       |
| 42183 | 1.491596              | 2.419381                                                       |
| 42185 | 1.433685              | 2.419384                                                       |
| 42187 | 1.000024              | 2.419387                                                       |
| 42189 | 1.592832              | 2.419391                                                       |
| 42191 | 1.033017              | 2.419394                                                       |
| 42193 | 1.000024              | 2.419397                                                       |
| 42195 | 1.672236              | 2.419401                                                       |
| 42197 | 1.000024              | 2.419404                                                       |
| 42199 | 1.053106              | 2.419408                                                       |
| 42201 | 1.496694              | 2.419411                                                       |
| 42203 | 1.143047              | 2.419414                                                       |
| 42205 | 1.255586              | 2.419418                                                       |
| 42207 | 1.455683              | 2.419421                                                       |
| 42209 | 1.000024              | 2.419424                                                       |
| 42211 | 1.146242              | 2.419428                                                       |
| 42213 | 1.333428              | 2.419431                                                       |
| 42215 | 1.200142              | 2.419435                                                       |
| 42217 | 1.180946              | 2.419438                                                       |
| 42219 | 1.444752              | 2.419441                                                       |
| 42221 | 1.000024              | 2.419445                                                       |
| 42223 | 1.000024              | 2.419448                                                       |
| 42225 | 1.656270              | 2.419451                                                       |
| 42227 | 1.000024              | 2.419455                                                       |
| 42229 | 1.102323              | 2.419458                                                       |
| 42231 | 1.524567              | 2.419462                                                       |
| 42233 | 1.010111              | 2.419465                                                       |
| 42235 | 1.200142              | 2.419468                                                       |
| 42237 | 1.641736              | 2.419472                                                       |
| 42239 | 1.000024              | 2.419475                                                       |
| 42241 | 1.020146              | 2.419478                                                       |
| 42243 | 1.333428              | 2.419482                                                       |
| 42245 | 1.472553              | 2.419485                                                       |
| 42247 | 1.014036              | 2.419489                                                       |
| 42249 | 1.333428              | 2.419492                                                       |
| 42251 | 1.145156              | 2.419495                                                       |
| 42253 | 1.090573              | 2.419499                                                       |

| $n$   | $\frac{\sigma(n)}{n}$ | $\frac{e^\gamma}{2} \log \log n + \frac{0.73\dots}{\log \log n}$ |
|-------|-----------------------|------------------------------------------------------------------|
| 42255 | 1.783458              | 2.419502                                                         |
| 42257 | 1.000024              | 2.419505                                                         |
| 42259 | 1.143046              | 2.419509                                                         |
| 42261 | 1.333428              | 2.419512                                                         |
| 42263 | 1.077254              | 2.419516                                                         |
| 42265 | 1.226547              | 2.419519                                                         |
| 42267 | 1.358601              | 2.419522                                                         |
| 42269 | 1.024297              | 2.419526                                                         |
| 42271 | 1.025384              | 2.419529                                                         |
| 42273 | 1.830388              | 2.419532                                                         |
| 42275 | 1.319929              | 2.419536                                                         |
| 42277 | 1.016534              | 2.419539                                                         |
| 42279 | 1.413468              | 2.419542                                                         |
| 42281 | 1.000024              | 2.419546                                                         |
| 42283 | 1.000024              | 2.419549                                                         |
| 42285 | 1.600568              | 2.419553                                                         |
| 42287 | 1.164613              | 2.419556                                                         |
| 42289 | 1.077254              | 2.419559                                                         |
| 42291 | 1.495164              | 2.419563                                                         |
| 42293 | 1.000024              | 2.419566                                                         |
| 42295 | 1.310793              | 2.419569                                                         |
| 42297 | 1.393574              | 2.419573                                                         |
| 42299 | 1.000024              | 2.419576                                                         |
| 42301 | 1.143046              | 2.419580                                                         |
| 42303 | 1.361606              | 2.419583                                                         |
| 42305 | 1.200142              | 2.419586                                                         |
| 42307 | 1.000024              | 2.419590                                                         |
| 42309 | 1.482427              | 2.419593                                                         |
| 42311 | 1.035192              | 2.419596                                                         |
| 42313 | 1.123059              | 2.419600                                                         |
| 42315 | 2.032754              | 2.419603                                                         |
| 42317 | 1.091193              | 2.419606                                                         |
| 42319 | 1.012311              | 2.419610                                                         |
| 42321 | 1.333428              | 2.419613                                                         |
| 42323 | 1.000024              | 2.419617                                                         |
| 42325 | 1.240732              | 2.419620                                                         |
| 42327 | 1.444752              | 2.419623                                                         |
| 42329 | 1.143046              | 2.419627                                                         |
| 42331 | 1.000024              | 2.419630                                                         |
| 42333 | 1.356105              | 2.419633                                                         |
| 42335 | 1.200142              | 2.419637                                                         |
| 42337 | 1.000024              | 2.419640                                                         |
| 42339 | 1.455679              | 2.419643                                                         |
| 42341 | 1.077254              | 2.419647                                                         |

| $n$   | $\frac{\sigma(n)}{n}$ | $\frac{e^\gamma}{2} \log \log n + \frac{0.73...}{\log \log n}$ |
|-------|-----------------------|----------------------------------------------------------------|
| 42343 | 1.197081              | 2.419650                                                       |
| 42345 | 1.735175              | 2.419654                                                       |
| 42347 | 1.101755              | 2.419657                                                       |
| 42349 | 1.000024              | 2.419660                                                       |
| 42351 | 1.405398              | 2.419664                                                       |
| 42353 | 1.025382              | 2.419667                                                       |
| 42355 | 1.234140              | 2.419670                                                       |
| 42357 | 1.524565              | 2.419674                                                       |
| 42359 | 1.000024              | 2.419677                                                       |
| 42361 | 1.091192              | 2.419680                                                       |
| 42363 | 1.496683              | 2.419684                                                       |
| 42365 | 1.237814              | 2.419687                                                       |
| 42367 | 1.077254              | 2.419690                                                       |
| 42369 | 1.382143              | 2.419694                                                       |
| 42371 | 1.143046              | 2.419697                                                       |
| 42373 | 1.000024              | 2.419701                                                       |
| 42375 | 1.678726              | 2.419704                                                       |
| 42377 | 1.033013              | 2.419707                                                       |
| 42379 | 1.000024              | 2.419711                                                       |
| 42381 | 1.534933              | 2.419714                                                       |
| 42383 | 1.091192              | 2.419717                                                       |
| 42385 | 1.403987              | 2.419721                                                       |
| 42387 | 1.358907              | 2.419724                                                       |
| 42389 | 1.109722              | 2.419727                                                       |
| 42391 | 1.000024              | 2.419731                                                       |
| 42393 | 1.437218              | 2.419734                                                       |
| 42395 | 1.228447              | 2.419738                                                       |
| 42397 | 1.000024              | 2.419741                                                       |
| 42399 | 1.653247              | 2.419744                                                       |
| 42401 | 1.011769              | 2.419748                                                       |
| 42403 | 1.000024              | 2.419751                                                       |
| 42405 | 1.752246              | 2.419754                                                       |
| 42407 | 1.000024              | 2.419758                                                       |
| 42409 | 1.000024              | 2.419761                                                       |
| 42411 | 1.359647              | 2.419764                                                       |
| 42413 | 1.172471              | 2.419768                                                       |
| 42415 | 1.273135              | 2.419771                                                       |
| 42417 | 1.482424              | 2.419774                                                       |
| 42419 | 1.087154              | 2.419778                                                       |
| 42421 | 1.018364              | 2.419781                                                       |
| 42423 | 1.357754              | 2.419784                                                       |
| 42425 | 1.240731              | 2.419788                                                       |
| 42427 | 1.357626              | 2.419791                                                       |
| 42429 | 1.333428              | 2.419795                                                       |



| $n$   | $\frac{\sigma(n)}{n}$ | $\frac{e^\gamma}{2} \log \log n + \frac{0.73...}{\log \log n}$ |
|-------|-----------------------|----------------------------------------------------------------|
| 42431 | 1.010205              | 2.419798                                                       |
| 42433 | 1.000024              | 2.419801                                                       |
| 42435 | 1.852810              | 2.419805                                                       |
| 42437 | 1.000024              | 2.419808                                                       |
| 42439 | 1.060911              | 2.419811                                                       |
| 42441 | 1.592422              | 2.419815                                                       |
| 42443 | 1.000024              | 2.419818                                                       |
| 42445 | 1.294287              | 2.419821                                                       |
| 42447 | 1.333428              | 2.419825                                                       |
| 42449 | 1.160169              | 2.419828                                                       |
| 42451 | 1.000024              | 2.419831                                                       |
| 42453 | 1.488234              | 2.419835                                                       |
| 42455 | 1.372559              | 2.419838                                                       |
| 42457 | 1.000024              | 2.419842                                                       |
| 42459 | 1.333428              | 2.419845                                                       |
| 42461 | 1.000024              | 2.419848                                                       |
| 42463 | 1.000024              | 2.419852                                                       |
| 42465 | 1.695514              | 2.419855                                                       |
| 42467 | 1.000024              | 2.419858                                                       |
| 42469 | 1.143046              | 2.419862                                                       |
| 42471 | 1.753667              | 2.419865                                                       |
| 42473 | 1.000024              | 2.419868                                                       |
| 42475 | 1.240730              | 2.419872                                                       |
| 42477 | 1.333428              | 2.419875                                                       |
| 42479 | 1.011888              | 2.419878                                                       |
| 42481 | 1.044043              | 2.419882                                                       |
| 42483 | 1.647624              | 2.419885                                                       |
| 42485 | 1.245616              | 2.419888                                                       |
| 42487 | 1.000024              | 2.419892                                                       |
| 42489 | 1.444750              | 2.419895                                                       |
| 42491 | 1.000024              | 2.419898                                                       |
| 42493 | 1.091191              | 2.419902                                                       |
| 42495 | 1.600565              | 2.419905                                                       |
| 42497 | 1.233405              | 2.419909                                                       |
| 42499 | 1.000024              | 2.419912                                                       |
| 42501 | 1.379356              | 2.419915                                                       |
| 42503 | 1.053102              | 2.419919                                                       |
| 42505 | 1.200141              | 2.419922                                                       |
| 42507 | 1.444750              | 2.419925                                                       |
| 42509 | 1.000024              | 2.419929                                                       |
| 42511 | 1.143045              | 2.419932                                                       |
| 42513 | 1.372945              | 2.419935                                                       |
| 42515 | 1.310784              | 2.419939                                                       |
| 42517 | 1.102430              | 2.419942                                                       |

| $n$   | $\frac{\sigma(n)}{n}$ | $\frac{e^\gamma}{2} \log \log n + \frac{0.73\dots}{\log \log n}$ |
|-------|-----------------------|------------------------------------------------------------------|
| 42519 | 1.333427              | 2.419945                                                         |
| 42521 | 1.012300              | 2.419949                                                         |
| 42523 | 1.077252              | 2.419952                                                         |
| 42525 | 2.122798              | 2.419955                                                         |
| 42527 | 1.068310              | 2.419959                                                         |
| 42529 | 1.015777              | 2.419962                                                         |
| 42531 | 1.333427              | 2.419965                                                         |
| 42533 | 1.000024              | 2.419969                                                         |
| 42535 | 1.232303              | 2.419972                                                         |
| 42537 | 1.455674              | 2.419975                                                         |
| 42539 | 1.173511              | 2.419979                                                         |
| 42541 | 1.053102              | 2.419982                                                         |
| 42543 | 1.503420              | 2.419986                                                         |
| 42545 | 1.227500              | 2.419989                                                         |
| 42547 | 1.010083              | 2.419992                                                         |
| 42549 | 1.437214              | 2.419996                                                         |
| 42551 | 1.059247              | 2.419999                                                         |
| 42553 | 1.143045              | 2.420002                                                         |
| 42555 | 1.600564              | 2.420006                                                         |
| 42557 | 1.000023              | 2.420009                                                         |
| 42559 | 1.126718              | 2.420012                                                         |
| 42561 | 1.444750              | 2.420016                                                         |
| 42563 | 1.033010              | 2.420019                                                         |
| 42565 | 1.200141              | 2.420022                                                         |
| 42567 | 1.524561              | 2.420026                                                         |
| 42569 | 1.000023              | 2.420029                                                         |
| 42571 | 1.000023              | 2.420032                                                         |
| 42573 | 1.393559              | 2.420036                                                         |
| 42575 | 1.345578              | 2.420039                                                         |
| 42577 | 1.000023              | 2.420042                                                         |
| 42579 | 1.578243              | 2.420046                                                         |
| 42581 | 1.285080              | 2.420049                                                         |
| 42583 | 1.012611              | 2.420052                                                         |
| 42585 | 1.704262              | 2.420056                                                         |
| 42587 | 1.027919              | 2.420059                                                         |
| 42589 | 1.000023              | 2.420062                                                         |
| 42591 | 1.333427              | 2.420066                                                         |
| 42593 | 1.009743              | 2.420069                                                         |
| 42595 | 1.372555              | 2.420072                                                         |
| 42597 | 1.444750              | 2.420076                                                         |
| 42599 | 1.025376              | 2.420079                                                         |
| 42601 | 1.123917              | 2.420082                                                         |
| 42603 | 1.455672              | 2.420086                                                         |
| 42605 | 1.200141              | 2.420089                                                         |

| $n$   | $\frac{\sigma(n)}{n}$ | $\frac{e^\gamma}{2} \log \log n + \frac{0.73...}{\log \log n}$ |
|-------|-----------------------|----------------------------------------------------------------|
| 42607 | 1.010538              | 2.420092                                                       |
| 42609 | 1.524561              | 2.420096                                                       |
| 42611 | 1.000023              | 2.420099                                                       |
| 42613 | 1.024288              | 2.420102                                                       |
| 42615 | 1.735164              | 2.420106                                                       |
| 42617 | 1.053101              | 2.420109                                                       |
| 42619 | 1.114996              | 2.420113                                                       |
| 42621 | 1.333427              | 2.420116                                                       |
| 42623 | 1.143045              | 2.420119                                                       |
| 42625 | 1.405372              | 2.420123                                                       |
| 42627 | 1.437211              | 2.420126                                                       |
| 42629 | 1.022403              | 2.420129                                                       |
| 42631 | 1.013347              | 2.420133                                                       |
| 42633 | 1.482420              | 2.420136                                                       |
| 42635 | 1.200141              | 2.420139                                                       |
| 42637 | 1.143045              | 2.420143                                                       |
| 42639 | 1.361008              | 2.420146                                                       |
| 42641 | 1.000023              | 2.420149                                                       |
| 42643 | 1.000023              | 2.420153                                                       |
| 42645 | 1.600563              | 2.420156                                                       |
| 42647 | 1.091190              | 2.420159                                                       |
| 42649 | 1.000023              | 2.420163                                                       |
| 42651 | 1.653232              | 2.420166                                                       |
| 42653 | 1.146180              | 2.420169                                                       |
| 42655 | 1.265971              | 2.420173                                                       |
| 42657 | 1.361558              | 2.420176                                                       |
| 42659 | 1.035186              | 2.420179                                                       |
| 42661 | 1.027918              | 2.420183                                                       |
| 42663 | 1.333427              | 2.420186                                                       |
| 42665 | 1.458057              | 2.420189                                                       |
| 42667 | 1.000023              | 2.420193                                                       |
| 42669 | 1.579414              | 2.420196                                                       |
| 42671 | 1.015772              | 2.420199                                                       |
| 42673 | 1.010475              | 2.420203                                                       |
| 42675 | 1.656239              | 2.420206                                                       |
| 42677 | 1.000023              | 2.420209                                                       |
| 42679 | 1.271445              | 2.420213                                                       |
| 42681 | 1.369790              | 2.420216                                                       |
| 42683 | 1.000023              | 2.420219                                                       |
| 42685 | 1.200141              | 2.420223                                                       |
| 42687 | 1.632722              | 2.420226                                                       |
| 42689 | 1.000023              | 2.420229                                                       |
| 42691 | 1.091190              | 2.420233                                                       |
| 42693 | 1.619001              | 2.420236                                                       |

| $n$   | $\frac{\sigma(n)}{n}$ | $\frac{e^\gamma}{2} \log \log n + \frac{0.73...}{\log \log n}$ |
|-------|-----------------------|----------------------------------------------------------------|
| 42695 | 1.200141              | 2.420239                                                       |
| 42697 | 1.000023              | 2.420243                                                       |
| 42699 | 1.368463              | 2.420246                                                       |
| 42701 | 1.000023              | 2.420249                                                       |
| 42703 | 1.000023              | 2.420253                                                       |
| 42705 | 1.892237              | 2.420256                                                       |
| 42707 | 1.143044              | 2.420259                                                       |
| 42709 | 1.000023              | 2.420263                                                       |
| 42711 | 1.393552              | 2.420266                                                       |
| 42713 | 1.102287              | 2.420269                                                       |
| 42715 | 1.200140              | 2.420273                                                       |
| 42717 | 1.382120              | 2.420276                                                       |
| 42719 | 1.000023              | 2.420279                                                       |
| 42721 | 1.213455              | 2.420283                                                       |
| 42723 | 1.489783              | 2.420286                                                       |
| 42725 | 1.240726              | 2.420289                                                       |
| 42727 | 1.000023              | 2.420293                                                       |
| 42729 | 1.333427              | 2.420296                                                       |
| 42731 | 1.140156              | 2.420299                                                       |
| 42733 | 1.010179              | 2.420303                                                       |
| 42735 | 2.048719              | 2.420306                                                       |
| 42737 | 1.000023              | 2.420309                                                       |
| 42739 | 1.014530              | 2.420313                                                       |
| 42741 | 1.482417              | 2.420316                                                       |
| 42743 | 1.000023              | 2.420319                                                       |
| 42745 | 1.226249              | 2.420323                                                       |
| 42747 | 1.333427              | 2.420326                                                       |
| 42749 | 1.185712              | 2.420329                                                       |
| 42751 | 1.000023              | 2.420332                                                       |
| 42753 | 1.333427              | 2.420336                                                       |
| 42755 | 1.273114              | 2.420339                                                       |
| 42757 | 1.232640              | 2.420342                                                       |
| 42759 | 1.444748              | 2.420346                                                       |
| 42761 | 1.017843              | 2.420349                                                       |
| 42763 | 1.178589              | 2.420352                                                       |
| 42765 | 1.600561              | 2.420356                                                       |
| 42767 | 1.000023              | 2.420359                                                       |
| 42769 | 1.053099              | 2.420362                                                       |
| 42771 | 1.363541              | 2.420366                                                       |
| 42773 | 1.000023              | 2.420369                                                       |
| 42775 | 1.304500              | 2.420372                                                       |
| 42777 | 1.697595              | 2.420376                                                       |
| 42779 | 1.091190              | 2.420379                                                       |
| 42781 | 1.009794              | 2.420382                                                       |

| $n$   | $\frac{\sigma(n)}{n}$ | $\frac{e^\gamma}{2} \log \log n + \frac{0.73...}{\log \log n}$ |
|-------|-----------------------|----------------------------------------------------------------|
| 42783 | 1.437206              | 2.420386                                                       |
| 42785 | 1.234077              | 2.420389                                                       |
| 42787 | 1.000023              | 2.420392                                                       |
| 42789 | 1.413447              | 2.420396                                                       |
| 42791 | 1.143044              | 2.420399                                                       |
| 42793 | 1.000023              | 2.420402                                                       |
| 42795 | 1.783386              | 2.420406                                                       |
| 42797 | 1.000023              | 2.420409                                                       |
| 42799 | 1.010865              | 2.420412                                                       |
| 42801 | 1.455667              | 2.420416                                                       |
| 42803 | 1.044039              | 2.420419                                                       |
| 42805 | 1.372550              | 2.420422                                                       |
| 42807 | 1.405378              | 2.420426                                                       |
| 42809 | 1.118456              | 2.420429                                                       |
| 42811 | 1.033006              | 2.420432                                                       |
| 42813 | 1.486651              | 2.420436                                                       |
| 42815 | 1.200140              | 2.420439                                                       |
| 42817 | 1.022398              | 2.420442                                                       |
| 42819 | 1.524557              | 2.420446                                                       |
| 42821 | 1.000023              | 2.420449                                                       |
| 42823 | 1.160124              | 2.420452                                                       |
| 42825 | 1.656229              | 2.420455                                                       |
| 42827 | 1.011511              | 2.420459                                                       |
| 42829 | 1.000023              | 2.420462                                                       |
| 42831 | 1.444748              | 2.420465                                                       |
| 42833 | 1.187869              | 2.420469                                                       |
| 42835 | 1.294269              | 2.420472                                                       |
| 42837 | 1.355837              | 2.420475                                                       |
| 42839 | 1.000023              | 2.420479                                                       |
| 42841 | 1.000023              | 2.420482                                                       |
| 42843 | 1.333427              | 2.420485                                                       |
| 42845 | 1.411600              | 2.420489                                                       |
| 42847 | 1.143044              | 2.420492                                                       |
| 42849 | 1.561600              | 2.420495                                                       |
| 42851 | 1.015426              | 2.420499                                                       |
| 42853 | 1.000023              | 2.420502                                                       |
| 42855 | 1.600560              | 2.420505                                                       |
| 42857 | 1.059244              | 2.420509                                                       |
| 42859 | 1.000023              | 2.420512                                                       |
| 42861 | 1.651478              | 2.420515                                                       |
| 42863 | 1.000023              | 2.420519                                                       |
| 42865 | 1.200140              | 2.420522                                                       |
| 42867 | 1.579397              | 2.420525                                                       |
| 42869 | 1.009961              | 2.420529                                                       |

| $n$   | $\frac{\sigma(n)}{n}$ | $\frac{e^\gamma}{2} \log \log n + \frac{0.73...}{\log \log n}$ |
|-------|-----------------------|----------------------------------------------------------------|
| 42871 | 1.024282              | 2.420532                                                       |
| 42873 | 1.379330              | 2.420535                                                       |
| 42875 | 1.455394              | 2.420538                                                       |
| 42877 | 1.020127              | 2.420542                                                       |
| 42879 | 1.333427              | 2.420545                                                       |
| 42881 | 1.010517              | 2.420548                                                       |
| 42883 | 1.098804              | 2.420552                                                       |
| 42885 | 1.735152              | 2.420555                                                       |
| 42887 | 1.077250              | 2.420558                                                       |
| 42889 | 1.248992              | 2.420562                                                       |
| 42891 | 1.462125              | 2.420565                                                       |
| 42893 | 1.018348              | 2.420568                                                       |
| 42895 | 1.255531              | 2.420572                                                       |
| 42897 | 1.357671              | 2.420575                                                       |
| 42899 | 1.000023              | 2.420578                                                       |
| 42901 | 1.000023              | 2.420582                                                       |
| 42903 | 1.700580              | 2.420585                                                       |
| 42905 | 1.200140              | 2.420588                                                       |
| 42907 | 1.011863              | 2.420592                                                       |
| 42909 | 1.333427              | 2.420595                                                       |
| 42911 | 1.127543              | 2.420598                                                       |
| 42913 | 1.077249              | 2.420601                                                       |
| 42915 | 1.600559              | 2.420605                                                       |
| 42917 | 1.143044              | 2.420608                                                       |
| 42919 | 1.009902              | 2.420611                                                       |
| 42921 | 1.526525              | 2.420615                                                       |
| 42923 | 1.000023              | 2.420618                                                       |
| 42925 | 1.325941              | 2.420621                                                       |
| 42927 | 1.369767              | 2.420625                                                       |
| 42929 | 1.000023              | 2.420628                                                       |
| 42931 | 1.143043              | 2.420631                                                       |
| 42933 | 1.455663              | 2.420635                                                       |
| 42935 | 1.243182              | 2.420638                                                       |
| 42937 | 1.000023              | 2.420641                                                       |
| 42939 | 1.559794              | 2.420645                                                       |
| 42941 | 1.044037              | 2.420648                                                       |
| 42943 | 1.000023              | 2.420651                                                       |
| 42945 | 1.833042              | 2.420654                                                       |
| 42947 | 1.016509              | 2.420658                                                       |
| 42949 | 1.035181              | 2.420661                                                       |
| 42951 | 1.355964              | 2.420664                                                       |
| 42953 | 1.000023              | 2.420668                                                       |
| 42955 | 1.337586              | 2.420671                                                       |
| 42957 | 1.556906              | 2.420674                                                       |

| $n$   | $\frac{\sigma(n)}{n}$ | $\frac{e^\gamma}{2} \log \log n + \frac{0.73...}{\log \log n}$ |
|-------|-----------------------|----------------------------------------------------------------|
| 42959 | 1.277125              | 2.420678                                                       |
| 42961 | 1.000023              | 2.420681                                                       |
| 42963 | 1.333426              | 2.420684                                                       |
| 42965 | 1.294263              | 2.420688                                                       |
| 42967 | 1.000023              | 2.420691                                                       |
| 42969 | 1.333426              | 2.420694                                                       |
| 42971 | 1.012590              | 2.420698                                                       |
| 42973 | 1.164592              | 2.420701                                                       |
| 42975 | 1.800489              | 2.420704                                                       |
| 42977 | 1.091188              | 2.420707                                                       |
| 42979 | 1.000023              | 2.420711                                                       |
| 42981 | 1.333426              | 2.420714                                                       |
| 42983 | 1.020124              | 2.420717                                                       |
| 42985 | 1.200140              | 2.420721                                                       |
| 42987 | 1.607928              | 2.420724                                                       |
| 42989 | 1.000023              | 2.420727                                                       |
| 42991 | 1.077249              | 2.420731                                                       |
| 42993 | 1.534855              | 2.420734                                                       |
| 42995 | 1.200140              | 2.420737                                                       |
| 42997 | 1.101472              | 2.420741                                                       |
| 42999 | 1.455662              | 2.420744                                                       |
| 43001 | 1.143043              | 2.420747                                                       |
| 43003 | 1.000023              | 2.420750                                                       |
| 43005 | 1.660830              | 2.420754                                                       |
| 43007 | 1.035180              | 2.420757                                                       |
| 43009 | 1.025367              | 2.420760                                                       |
| 43011 | 1.524726              | 2.420764                                                       |
| 43013 | 1.000023              | 2.420767                                                       |
| 43015 | 1.372544              | 2.420770                                                       |
| 43017 | 1.437199              | 2.420774                                                       |
| 43019 | 1.000023              | 2.420777                                                       |
| 43021 | 1.091188              | 2.420780                                                       |
| 43023 | 1.333426              | 2.420783                                                       |
| 43025 | 1.240721              | 2.420787                                                       |
| 43027 | 1.059242              | 2.420790                                                       |
| 43029 | 1.653211              | 2.420793                                                       |
| 43031 | 1.027910              | 2.420797                                                       |
| 43033 | 1.044036              | 2.420800                                                       |
| 43035 | 1.695364              | 2.420803                                                       |
| 43037 | 1.000023              | 2.420807                                                       |
| 43039 | 1.009689              | 2.420810                                                       |
| 43041 | 1.333426              | 2.420813                                                       |
| 43043 | 1.373882              | 2.420817                                                       |
| 43045 | 1.200139              | 2.420820                                                       |

| $n$   | $\frac{\sigma(n)}{n}$ | $\frac{e^\gamma}{2} \log \log n + \frac{0.73...}{\log \log n}$ |
|-------|-----------------------|----------------------------------------------------------------|
| 43047 | 1.444746              | 2.420823                                                       |
| 43049 | 1.000023              | 2.420826                                                       |
| 43051 | 1.000023              | 2.420830                                                       |
| 43053 | 1.355724              | 2.420833                                                       |
| 43055 | 1.226338              | 2.420836                                                       |
| 43057 | 1.143043              | 2.420840                                                       |
| 43059 | 1.379317              | 2.420843                                                       |
| 43061 | 1.069413              | 2.420846                                                       |
| 43063 | 1.000023              | 2.420850                                                       |
| 43065 | 2.006270              | 2.420853                                                       |
| 43067 | 1.000023              | 2.420856                                                       |
| 43069 | 1.077248              | 2.420859                                                       |
| 43071 | 1.556314              | 2.420863                                                       |
| 43073 | 1.053096              | 2.420866                                                       |
| 43075 | 1.240720              | 2.420869                                                       |
| 43077 | 1.357198              | 2.420873                                                       |
| 43079 | 1.044035              | 2.420876                                                       |
| 43081 | 1.016504              | 2.420879                                                       |
| 43083 | 1.444746              | 2.420883                                                       |
| 43085 | 1.372543              | 2.420886                                                       |
| 43087 | 1.091188              | 2.420889                                                       |
| 43089 | 1.363503              | 2.420892                                                       |
| 43091 | 1.025365              | 2.420896                                                       |
| 43093 | 1.000023              | 2.420899                                                       |
| 43095 | 1.834459              | 2.420902                                                       |
| 43097 | 1.015755              | 2.420906                                                       |
| 43099 | 1.176083              | 2.420909                                                       |
| 43101 | 1.444746              | 2.420912                                                       |
| 43103 | 1.000023              | 2.420916                                                       |
| 43105 | 1.237722              | 2.420919                                                       |
| 43107 | 1.333426              | 2.420922                                                       |
| 43109 | 1.091187              | 2.420925                                                       |
| 43111 | 1.053095              | 2.420929                                                       |
| 43113 | 1.524552              | 2.420932                                                       |
| 43115 | 1.200139              | 2.420935                                                       |
| 43117 | 1.000023              | 2.420939                                                       |
| 43119 | 1.482409              | 2.420942                                                       |
| 43121 | 1.122052              | 2.420945                                                       |
| 43123 | 1.035178              | 2.420949                                                       |
| 43125 | 1.738574              | 2.420952                                                       |
| 43127 | 1.173093              | 2.420955                                                       |
| 43129 | 1.101811              | 2.420958                                                       |
| 43131 | 1.455658              | 2.420962                                                       |
| 43133 | 1.000023              | 2.420965                                                       |



| $n$   | $\frac{\sigma(n)}{n}$ | $\frac{e^\gamma}{2} \log \log n + \frac{0.73...}{\log \log n}$ |
|-------|-----------------------|----------------------------------------------------------------|
| 43135 | 1.200139              | 2.420968                                                       |
| 43137 | 1.444746              | 2.420972                                                       |
| 43139 | 1.009759              | 2.420975                                                       |
| 43141 | 1.143043              | 2.420978                                                       |
| 43143 | 1.358459              | 2.420981                                                       |
| 43145 | 1.200139              | 2.420985                                                       |
| 43147 | 1.077248              | 2.420988                                                       |
| 43149 | 1.405363              | 2.420991                                                       |
| 43151 | 1.000023              | 2.420995                                                       |
| 43153 | 1.091187              | 2.420998                                                       |
| 43155 | 1.995412              | 2.421001                                                       |
| 43157 | 1.012119              | 2.421005                                                       |
| 43159 | 1.000023              | 2.421008                                                       |
| 43161 | 1.333426              | 2.421011                                                       |
| 43163 | 1.059241              | 2.421014                                                       |
| 43165 | 1.225993              | 2.421018                                                       |
| 43167 | 1.333426              | 2.421021                                                       |
| 43169 | 1.164586              | 2.421024                                                       |
| 43171 | 1.044034              | 2.421028                                                       |
| 43173 | 1.647974              | 2.421031                                                       |
| 43175 | 1.361343              | 2.421034                                                       |
| 43177 | 1.000023              | 2.421037                                                       |
| 43179 | 1.372890              | 2.421041                                                       |
| 43181 | 1.035178              | 2.421044                                                       |
| 43183 | 1.185652              | 2.421047                                                       |
| 43185 | 1.600556              | 2.421051                                                       |
| 43187 | 1.053095              | 2.421054                                                       |
| 43189 | 1.000023              | 2.421057                                                       |
| 43191 | 1.444745              | 2.421061                                                       |
| 43193 | 1.022388              | 2.421064                                                       |
| 43195 | 1.230142              | 2.421067                                                       |
| 43197 | 1.773456              | 2.421070                                                       |
| 43199 | 1.077247              | 2.421074                                                       |
| 43201 | 1.000023              | 2.421077                                                       |
| 43203 | 1.333426              | 2.421080                                                       |
| 43205 | 1.200139              | 2.421084                                                       |
| 43207 | 1.000023              | 2.421087                                                       |
| 43209 | 1.444745              | 2.421090                                                       |
| 43211 | 1.143042              | 2.421093                                                       |
| 43213 | 1.014510              | 2.421097                                                       |
| 43215 | 1.661645              | 2.421100                                                       |
| 43217 | 1.044034              | 2.421103                                                       |
| 43219 | 1.091187              | 2.421107                                                       |
| 43221 | 1.333426              | 2.421110                                                       |

| $n$   | $\frac{\sigma(n)}{n}$ | $\frac{e^\gamma}{2} \log \log n + \frac{0.73...}{\log \log n}$ |
|-------|-----------------------|----------------------------------------------------------------|
| 43223 | 1.000023              | 2.421113                                                       |
| 43225 | 1.606478              | 2.421116                                                       |
| 43227 | 1.482407              | 2.421120                                                       |
| 43229 | 1.010433              | 2.421123                                                       |
| 43231 | 1.059240              | 2.421126                                                       |
| 43233 | 1.333426              | 2.421130                                                       |
| 43235 | 1.200139              | 2.421133                                                       |
| 43237 | 1.000023              | 2.421136                                                       |
| 43239 | 1.598557              | 2.421139                                                       |
| 43241 | 1.091187              | 2.421143                                                       |
| 43243 | 1.013991              | 2.421146                                                       |
| 43245 | 1.791051              | 2.421149                                                       |
| 43247 | 1.018337              | 2.421153                                                       |
| 43249 | 1.017827              | 2.421156                                                       |
| 43251 | 1.437192              | 2.421159                                                       |
| 43253 | 1.180774              | 2.421162                                                       |
| 43255 | 1.235094              | 2.421166                                                       |
| 43257 | 1.333426              | 2.421169                                                       |
| 43259 | 1.009732              | 2.421172                                                       |
| 43261 | 1.000023              | 2.421176                                                       |
| 43263 | 1.730809              | 2.421179                                                       |
| 43265 | 1.273084              | 2.421182                                                       |
| 43267 | 1.164583              | 2.421185                                                       |
| 43269 | 1.333426              | 2.421189                                                       |
| 43271 | 1.000023              | 2.421192                                                       |
| 43273 | 1.011716              | 2.421195                                                       |
| 43275 | 1.656199              | 2.421199                                                       |
| 43277 | 1.077247              | 2.421202                                                       |
| 43279 | 1.011484              | 2.421205                                                       |
| 43281 | 1.700515              | 2.421208                                                       |
| 43283 | 1.000023              | 2.421212                                                       |
| 43285 | 1.310754              | 2.421215                                                       |
| 43287 | 1.366138              | 2.421218                                                       |
| 43289 | 1.015408              | 2.421222                                                       |
| 43291 | 1.000023              | 2.421225                                                       |
| 43293 | 1.333426              | 2.421228                                                       |
| 43295 | 1.372537              | 2.421231                                                       |
| 43297 | 1.035176              | 2.421235                                                       |
| 43299 | 1.534816              | 2.421238                                                       |
| 43301 | 1.097434              | 2.421241                                                       |
| 43303 | 1.077246              | 2.421245                                                       |
| 43305 | 1.600554              | 2.421248                                                       |
| 43307 | 1.134967              | 2.421251                                                       |
| 43309 | 1.196980              | 2.421254                                                       |

| $n$   | $\frac{\sigma(n)}{n}$ | $\frac{e^\gamma}{2} \log \log n + \frac{0.73...}{\log \log n}$ |
|-------|-----------------------|----------------------------------------------------------------|
| 43311 | 1.333426              | 2.421258                                                       |
| 43313 | 1.000023              | 2.421261                                                       |
| 43315 | 1.200139              | 2.421264                                                       |
| 43317 | 1.444745              | 2.421268                                                       |
| 43319 | 1.000023              | 2.421271                                                       |
| 43321 | 1.000023              | 2.421274                                                       |
| 43323 | 1.524548              | 2.421277                                                       |
| 43325 | 1.240716              | 2.421281                                                       |
| 43327 | 1.027904              | 2.421284                                                       |
| 43329 | 1.581943              | 2.421287                                                       |
| 43331 | 1.000023              | 2.421290                                                       |
| 43333 | 1.059239              | 2.421294                                                       |
| 43335 | 1.809346              | 2.421297                                                       |
| 43337 | 1.178485              | 2.421300                                                       |
| 43339 | 1.053093              | 2.421304                                                       |
| 43341 | 1.333426              | 2.421307                                                       |
| 43343 | 1.013312              | 2.421310                                                       |
| 43345 | 1.200138              | 2.421313                                                       |
| 43347 | 1.333426              | 2.421317                                                       |
| 43349 | 1.016494              | 2.421320                                                       |
| 43351 | 1.248968              | 2.421323                                                       |
| 43353 | 1.444744              | 2.421327                                                       |
| 43355 | 1.394995              | 2.421330                                                       |
| 43357 | 1.009664              | 2.421333                                                       |
| 43359 | 1.356120              | 2.421336                                                       |
| 43361 | 1.010678              | 2.421340                                                       |
| 43363 | 1.012107              | 2.421343                                                       |
| 43365 | 1.892771              | 2.421346                                                       |
| 43367 | 1.059239              | 2.421349                                                       |
| 43369 | 1.032996              | 2.421353                                                       |
| 43371 | 1.486708              | 2.421356                                                       |
| 43373 | 1.091186              | 2.421359                                                       |
| 43375 | 1.251597              | 2.421363                                                       |
| 43377 | 1.405353              | 2.421366                                                       |
| 43379 | 1.143042              | 2.421369                                                       |
| 43381 | 1.115327              | 2.421372                                                       |
| 43383 | 1.333426              | 2.421376                                                       |
| 43385 | 1.200138              | 2.421379                                                       |
| 43387 | 1.024270              | 2.421382                                                       |
| 43389 | 1.482403              | 2.421386                                                       |
| 43391 | 1.000023              | 2.421389                                                       |
| 43393 | 1.143042              | 2.421392                                                       |
| 43395 | 1.752091              | 2.421395                                                       |
| 43397 | 1.000023              | 2.421399                                                       |

| $n$   | $\frac{\sigma(n)}{n}$ | $\frac{e^\gamma}{2} \log \log n + \frac{0.73...}{\log \log n}$ |
|-------|-----------------------|----------------------------------------------------------------|
| 43399 | 1.000023              | 2.421402                                                       |
| 43401 | 1.512961              | 2.421405                                                       |
| 43403 | 1.000023              | 2.421408                                                       |
| 43405 | 1.200138              | 2.421412                                                       |
| 43407 | 1.811321              | 2.421415                                                       |
| 43409 | 1.013983              | 2.421418                                                       |
| 43411 | 1.000023              | 2.421422                                                       |
| 43413 | 1.382074              | 2.421425                                                       |
| 43415 | 1.265922              | 2.421428                                                       |
| 43417 | 1.091185              | 2.421431                                                       |
| 43419 | 1.369723              | 2.421435                                                       |
| 43421 | 1.143041              | 2.421438                                                       |
| 43423 | 1.009787              | 2.421441                                                       |
| 43425 | 1.800391              | 2.421444                                                       |
| 43427 | 1.000023              | 2.421448                                                       |
| 43429 | 1.010477              | 2.421451                                                       |
| 43431 | 1.379291              | 2.421454                                                       |
| 43433 | 1.087054              | 2.421458                                                       |
| 43435 | 1.471993              | 2.421461                                                       |
| 43437 | 1.333425              | 2.421464                                                       |
| 43439 | 1.102235              | 2.421467                                                       |
| 43441 | 1.000023              | 2.421471                                                       |
| 43443 | 1.482402              | 2.421474                                                       |
| 43445 | 1.200138              | 2.421477                                                       |
| 43447 | 1.044031              | 2.421480                                                       |
| 43449 | 1.524546              | 2.421484                                                       |
| 43451 | 1.000023              | 2.421487                                                       |
| 43453 | 1.053092              | 2.421490                                                       |
| 43455 | 1.600552              | 2.421493                                                       |
| 43457 | 1.000023              | 2.421497                                                       |
| 43459 | 1.077245              | 2.421500                                                       |
| 43461 | 1.579347              | 2.421503                                                       |
| 43463 | 1.164577              | 2.421507                                                       |
| 43465 | 1.200138              | 2.421510                                                       |
| 43467 | 1.333425              | 2.421513                                                       |
| 43469 | 1.059238              | 2.421516                                                       |
| 43471 | 1.035173              | 2.421520                                                       |
| 43473 | 1.368390              | 2.421523                                                       |
| 43475 | 1.300610              | 2.421526                                                       |
| 43477 | 1.143041              | 2.421529                                                       |
| 43479 | 1.444743              | 2.421533                                                       |
| 43481 | 1.000023              | 2.421536                                                       |
| 43483 | 1.125957              | 2.421539                                                       |
| 43485 | 1.730804              | 2.421543                                                       |

| $n$   | $\frac{\sigma(n)}{n}$ | $\frac{e^\gamma}{2} \log \log n + \frac{0.73\dots}{\log \log n}$ |
|-------|-----------------------|------------------------------------------------------------------|
| 43487 | 1.000023              | 2.421546                                                         |
| 43489 | 1.010003              | 2.421549                                                         |
| 43491 | 1.618726              | 2.421552                                                         |
| 43493 | 1.094797              | 2.421556                                                         |
| 43495 | 1.200138              | 2.421559                                                         |
| 43497 | 1.506311              | 2.421562                                                         |
| 43499 | 1.000023              | 2.421565                                                         |
| 43501 | 1.025356              | 2.421569                                                         |
| 43503 | 1.413420              | 2.421572                                                         |
| 43505 | 1.509344              | 2.421575                                                         |
| 43507 | 1.010412              | 2.421578                                                         |
| 43509 | 1.333425              | 2.421582                                                         |
| 43511 | 1.077245              | 2.421585                                                         |
| 43513 | 1.020109              | 2.421588                                                         |
| 43515 | 1.735126              | 2.421592                                                         |
| 43517 | 1.000023              | 2.421595                                                         |
| 43519 | 1.143041              | 2.421598                                                         |
| 43521 | 1.356586              | 2.421601                                                         |
| 43523 | 1.015739              | 2.421605                                                         |
| 43525 | 1.240712              | 2.421608                                                         |
| 43527 | 1.455648              | 2.421611                                                         |
| 43529 | 1.102713              | 2.421614                                                         |
| 43531 | 1.012244              | 2.421618                                                         |
| 43533 | 1.653183              | 2.421621                                                         |
| 43535 | 1.200138              | 2.421624                                                         |
| 43537 | 1.146060              | 2.421627                                                         |
| 43539 | 1.393509              | 2.421631                                                         |
| 43541 | 1.000023              | 2.421634                                                         |
| 43543 | 1.000023              | 2.421637                                                         |
| 43545 | 1.600551              | 2.421640                                                         |
| 43547 | 1.143041              | 2.421644                                                         |
| 43549 | 1.130864              | 2.421647                                                         |
| 43551 | 1.482400              | 2.421650                                                         |
| 43553 | 1.012559              | 2.421653                                                         |
| 43555 | 1.243118              | 2.421657                                                         |
| 43557 | 1.333425              | 2.421660                                                         |
| 43559 | 1.024266              | 2.421663                                                         |
| 43561 | 1.175363              | 2.421667                                                         |
| 43563 | 1.437183              | 2.421670                                                         |
| 43565 | 1.200138              | 2.421673                                                         |
| 43567 | 1.053091              | 2.421676                                                         |
| 43569 | 1.489499              | 2.421680                                                         |
| 43571 | 1.160038              | 2.421683                                                         |
| 43573 | 1.000023              | 2.421686                                                         |

| $n$   | $\frac{\sigma(n)}{n}$ | $\frac{e^\gamma}{2} \log \log n + \frac{0.73...}{\log \log n}$ |
|-------|-----------------------|----------------------------------------------------------------|
| 43575 | 1.912289              | 2.421689                                                       |
| 43577 | 1.000023              | 2.421693                                                       |
| 43579 | 1.000023              | 2.421696                                                       |
| 43581 | 1.358390              | 2.421699                                                       |
| 43583 | 1.025354              | 2.421702                                                       |
| 43585 | 1.255478              | 2.421706                                                       |
| 43587 | 1.503200              | 2.421709                                                       |
| 43589 | 1.233339              | 2.421712                                                       |
| 43591 | 1.000023              | 2.421715                                                       |
| 43593 | 1.455647              | 2.421719                                                       |
| 43595 | 1.200138              | 2.421722                                                       |
| 43597 | 1.000023              | 2.421725                                                       |
| 43599 | 1.333425              | 2.421728                                                       |
| 43601 | 1.018325              | 2.421732                                                       |
| 43603 | 1.143041              | 2.421735                                                       |
| 43605 | 1.981424              | 2.421738                                                       |
| 43607 | 1.000023              | 2.421741                                                       |
| 43609 | 1.000023              | 2.421745                                                       |
| 43611 | 1.333425              | 2.421748                                                       |
| 43613 | 1.000023              | 2.421751                                                       |
| 43615 | 1.432902              | 2.421755                                                       |
| 43617 | 1.596442              | 2.421758                                                       |
| 43619 | 1.020106              | 2.421761                                                       |
| 43621 | 1.009697              | 2.421764                                                       |
| 43623 | 1.494808              | 2.421768                                                       |
| 43625 | 1.251576              | 2.421771                                                       |
| 43627 | 1.000023              | 2.421774                                                       |
| 43629 | 1.333425              | 2.421777                                                       |
| 43631 | 1.196947              | 2.421781                                                       |
| 43633 | 1.000023              | 2.421784                                                       |
| 43635 | 1.600550              | 2.421787                                                       |
| 43637 | 1.091184              | 2.421790                                                       |
| 43639 | 1.069319              | 2.421794                                                       |
| 43641 | 1.559726              | 2.421797                                                       |
| 43643 | 1.053090              | 2.421800                                                       |
| 43645 | 1.451713              | 2.421803                                                       |
| 43647 | 1.333425              | 2.421807                                                       |
| 43649 | 1.000023              | 2.421810                                                       |
| 43651 | 1.000023              | 2.421813                                                       |
| 43653 | 1.333425              | 2.421816                                                       |
| 43655 | 1.200137              | 2.421820                                                       |
| 43657 | 1.010147              | 2.421823                                                       |
| 43659 | 1.895692              | 2.421826                                                       |
| 43661 | 1.000023              | 2.421829                                                       |

| $n$   | $\frac{\sigma(n)}{n}$ | $\frac{e^\gamma}{2} \log \log n + \frac{0.73...}{\log \log n}$ |
|-------|-----------------------|----------------------------------------------------------------|
| 43663 | 1.022376              | 2.421833                                                       |
| 43665 | 1.662109              | 2.421836                                                       |
| 43667 | 1.077244              | 2.421839                                                       |
| 43669 | 1.000023              | 2.421842                                                       |
| 43671 | 1.333425              | 2.421846                                                       |
| 43673 | 1.213381              | 2.421849                                                       |
| 43675 | 1.240710              | 2.421852                                                       |
| 43677 | 1.514390              | 2.421855                                                       |
| 43679 | 1.032991              | 2.421859                                                       |
| 43681 | 1.160070              | 2.421862                                                       |
| 43683 | 1.333425              | 2.421865                                                       |
| 43685 | 1.200137              | 2.421868                                                       |
| 43687 | 1.157507              | 2.421872                                                       |
| 43689 | 1.333425              | 2.421875                                                       |
| 43691 | 1.000023              | 2.421878                                                       |
| 43693 | 1.077243              | 2.421881                                                       |
| 43695 | 1.735118              | 2.421885                                                       |
| 43697 | 1.027897              | 2.421888                                                       |
| 43699 | 1.013295              | 2.421891                                                       |
| 43701 | 1.524542              | 2.421894                                                       |
| 43703 | 1.136764              | 2.421898                                                       |
| 43705 | 1.200137              | 2.421901                                                       |
| 43707 | 1.413412              | 2.421904                                                       |
| 43709 | 1.011691              | 2.421907                                                       |
| 43711 | 1.000023              | 2.421911                                                       |
| 43713 | 1.482397              | 2.421914                                                       |
| 43715 | 1.372527              | 2.421917                                                       |
| 43717 | 1.000023              | 2.421920                                                       |
| 43719 | 1.537089              | 2.421924                                                       |
| 43721 | 1.000023              | 2.421927                                                       |
| 43723 | 1.044027              | 2.421930                                                       |
| 43725 | 1.837667              | 2.421933                                                       |
| 43727 | 1.015391              | 2.421937                                                       |
| 43729 | 1.143040              | 2.421940                                                       |
| 43731 | 1.491116              | 2.421943                                                       |
| 43733 | 1.012233              | 2.421946                                                       |
| 43735 | 1.200137              | 2.421950                                                       |
| 43737 | 1.360862              | 2.421953                                                       |
| 43739 | 1.009625              | 2.421956                                                       |
| 43741 | 1.106148              | 2.421959                                                       |
| 43743 | 1.524541              | 2.421963                                                       |
| 43745 | 1.294228              | 2.421966                                                       |
| 43747 | 1.129037              | 2.421969                                                       |
| 43749 | 1.444742              | 2.421972                                                       |

| $n$   | $\frac{\sigma(n)}{n}$ | $\frac{e^\gamma}{2} \log \log n + \frac{0.73...}{\log \log n}$ |
|-------|-----------------------|----------------------------------------------------------------|
| 43751 | 1.016480              | 2.421976                                                       |
| 43753 | 1.000023              | 2.421979                                                       |
| 43755 | 1.600549              | 2.421982                                                       |
| 43757 | 1.250543              | 2.421985                                                       |
| 43759 | 1.000023              | 2.421989                                                       |
| 43761 | 1.382053              | 2.421992                                                       |
| 43763 | 1.011814              | 2.421995                                                       |
| 43765 | 1.200137              | 2.421998                                                       |
| 43767 | 1.482395              | 2.422002                                                       |
| 43769 | 1.144920              | 2.422005                                                       |
| 43771 | 1.270979              | 2.422008                                                       |
| 43773 | 1.333425              | 2.422011                                                       |
| 43775 | 1.325688              | 2.422015                                                       |
| 43777 | 1.000023              | 2.422018                                                       |
| 43779 | 1.333425              | 2.422021                                                       |
| 43781 | 1.000023              | 2.422024                                                       |
| 43783 | 1.000023              | 2.422027                                                       |
| 43785 | 1.995204              | 2.422031                                                       |
| 43787 | 1.000023              | 2.422034                                                       |
| 43789 | 1.000023              | 2.422037                                                       |
| 43791 | 1.455642              | 2.422040                                                       |
| 43793 | 1.000023              | 2.422044                                                       |
| 43795 | 1.265898              | 2.422047                                                       |
| 43797 | 1.437176              | 2.422050                                                       |
| 43799 | 1.143040              | 2.422053                                                       |
| 43801 | 1.000023              | 2.422057                                                       |
| 43803 | 1.500536              | 2.422060                                                       |
| 43805 | 1.200137              | 2.422063                                                       |
| 43807 | 1.015728              | 2.422066                                                       |
| 43809 | 1.413408              | 2.422070                                                       |
| 43811 | 1.009609              | 2.422073                                                       |
| 43813 | 1.248944              | 2.422076                                                       |
| 43815 | 1.682711              | 2.422079                                                       |
| 43817 | 1.024260              | 2.422083                                                       |
| 43819 | 1.035167              | 2.422086                                                       |
| 43821 | 1.496588              | 2.422089                                                       |
| 43823 | 1.077243              | 2.422092                                                       |
| 43825 | 1.240707              | 2.422096                                                       |
| 43827 | 1.524540              | 2.422099                                                       |
| 43829 | 1.025349              | 2.422102                                                       |
| 43831 | 1.020100              | 2.422105                                                       |
| 43833 | 1.405334              | 2.422109                                                       |
| 43835 | 1.310733              | 2.422112                                                       |
| 43837 | 1.018318              | 2.422115                                                       |



| $n$   | $\frac{\sigma(n)}{n}$ | $\frac{e^\gamma}{2} \log \log n + \frac{0.73...}{\log \log n}$ |
|-------|-----------------------|----------------------------------------------------------------|
| 43839 | 1.444741              | 2.422118                                                       |
| 43841 | 1.143040              | 2.422121                                                       |
| 43843 | 1.059234              | 2.422125                                                       |
| 43845 | 1.664044              | 2.422128                                                       |
| 43847 | 1.009875              | 2.422131                                                       |
| 43849 | 1.077242              | 2.422134                                                       |
| 43851 | 1.366081              | 2.422138                                                       |
| 43853 | 1.000023              | 2.422141                                                       |
| 43855 | 1.403717              | 2.422144                                                       |
| 43857 | 1.579315              | 2.422147                                                       |
| 43859 | 1.017807              | 2.422151                                                       |
| 43861 | 1.044025              | 2.422154                                                       |
| 43863 | 1.333425              | 2.422157                                                       |
| 43865 | 1.243087              | 2.422160                                                       |
| 43867 | 1.000023              | 2.422164                                                       |
| 43869 | 1.524539              | 2.422167                                                       |
| 43871 | 1.053087              | 2.422170                                                       |
| 43873 | 1.015385              | 2.422173                                                       |
| 43875 | 1.991111              | 2.422177                                                       |
| 43877 | 1.107642              | 2.422180                                                       |
| 43879 | 1.091183              | 2.422183                                                       |
| 43881 | 1.333424              | 2.422186                                                       |
| 43883 | 1.143039              | 2.422189                                                       |
| 43885 | 1.227207              | 2.422193                                                       |
| 43887 | 1.333424              | 2.422196                                                       |
| 43889 | 1.000023              | 2.422199                                                       |
| 43891 | 1.000023              | 2.422202                                                       |
| 43893 | 1.444741              | 2.422206                                                       |
| 43895 | 1.200137              | 2.422209                                                       |
| 43897 | 1.143039              | 2.422212                                                       |
| 43899 | 1.333424              | 2.422215                                                       |
| 43901 | 1.178652              | 2.422219                                                       |
| 43903 | 1.024258              | 2.422222                                                       |
| 43905 | 1.600547              | 2.422225                                                       |
| 43907 | 1.057963              | 2.422228                                                       |
| 43909 | 1.053087              | 2.422231                                                       |
| 43911 | 1.790531              | 2.422235                                                       |
| 43913 | 1.000023              | 2.422238                                                       |
| 43915 | 1.200137              | 2.422241                                                       |
| 43917 | 1.333424              | 2.422244                                                       |
| 43919 | 1.027892              | 2.422248                                                       |
| 43921 | 1.009813              | 2.422251                                                       |
| 43923 | 1.466658              | 2.422254                                                       |
| 43925 | 1.422789              | 2.422257                                                       |

| $n$   | $\frac{\sigma(n)}{n}$ | $\frac{e^\gamma}{2} \log \log n + \frac{0.73...}{\log \log n}$ |
|-------|-----------------------|----------------------------------------------------------------|
| 43927 | 1.121861              | 2.422261                                                       |
| 43929 | 1.482392              | 2.422264                                                       |
| 43931 | 1.009583              | 2.422267                                                       |
| 43933 | 1.000023              | 2.422270                                                       |
| 43935 | 1.671560              | 2.422274                                                       |
| 43937 | 1.020097              | 2.422277                                                       |
| 43939 | 1.143039              | 2.422280                                                       |
| 43941 | 1.356000              | 2.422283                                                       |
| 43943 | 1.000023              | 2.422286                                                       |
| 43945 | 1.415588              | 2.422290                                                       |
| 43947 | 1.526384              | 2.422293                                                       |
| 43949 | 1.015723              | 2.422296                                                       |
| 43951 | 1.000023              | 2.422299                                                       |
| 43953 | 1.742953              | 2.422303                                                       |
| 43955 | 1.228529              | 2.422306                                                       |
| 43957 | 1.011443              | 2.422309                                                       |
| 43959 | 1.333424              | 2.422312                                                       |
| 43961 | 1.000023              | 2.422315                                                       |
| 43963 | 1.000023              | 2.422319                                                       |
| 43965 | 1.735107              | 2.422322                                                       |
| 43967 | 1.248937              | 2.422325                                                       |
| 43969 | 1.000023              | 2.422328                                                       |
| 43971 | 1.333424              | 2.422332                                                       |
| 43973 | 1.000023              | 2.422335                                                       |
| 43975 | 1.240705              | 2.422338                                                       |
| 43977 | 1.355618              | 2.422341                                                       |
| 43979 | 1.146002              | 2.422345                                                       |
| 43981 | 1.172870              | 2.422348                                                       |
| 43983 | 1.506218              | 2.422351                                                       |
| 43985 | 1.265886              | 2.422354                                                       |
| 43987 | 1.000023              | 2.422357                                                       |
| 43989 | 1.536384              | 2.422361                                                       |
| 43991 | 1.000023              | 2.422364                                                       |
| 43993 | 1.088355              | 2.422367                                                       |
| 43995 | 1.832936              | 2.422370                                                       |
| 43997 | 1.000023              | 2.422374                                                       |
| 43999 | 1.044024              | 2.422377                                                       |
| 44001 | 1.444740              | 2.422380                                                       |
| 44003 | 1.014476              | 2.422383                                                       |
| 44005 | 1.294217              | 2.422386                                                       |
| 44007 | 1.333424              | 2.422390                                                       |
| 44009 | 1.143039              | 2.422393                                                       |
| 44011 | 1.091182              | 2.422396                                                       |
| 44013 | 1.413401              | 2.422399                                                       |

| $n$   | $\frac{\sigma(n)}{n}$ | $\frac{e^\gamma}{2} \log \log n + \frac{0.73...}{\log \log n}$ |
|-------|-----------------------|----------------------------------------------------------------|
| 44015 | 1.200136              | 2.422403                                                       |
| 44017 | 1.000023              | 2.422406                                                       |
| 44019 | 1.486086              | 2.422409                                                       |
| 44021 | 1.000023              | 2.422412                                                       |
| 44023 | 1.206642              | 2.422416                                                       |
| 44025 | 1.656150              | 2.422419                                                       |
| 44027 | 1.000023              | 2.422422                                                       |
| 44029 | 1.000023              | 2.422425                                                       |
| 44031 | 1.437169              | 2.422428                                                       |
| 44033 | 1.091182              | 2.422432                                                       |
| 44035 | 1.200136              | 2.422435                                                       |
| 44037 | 1.700388              | 2.422438                                                       |
| 44039 | 1.022367              | 2.422441                                                       |
| 44041 | 1.000023              | 2.422445                                                       |
| 44043 | 1.363395              | 2.422448                                                       |
| 44045 | 1.255443              | 2.422451                                                       |
| 44047 | 1.059232              | 2.422454                                                       |
| 44049 | 1.333424              | 2.422457                                                       |
| 44051 | 1.242197              | 2.422461                                                       |
| 44053 | 1.000023              | 2.422464                                                       |
| 44055 | 1.912155              | 2.422467                                                       |
| 44057 | 1.077241              | 2.422470                                                       |
| 44059 | 1.000023              | 2.422474                                                       |
| 44061 | 1.405324              | 2.422477                                                       |
| 44063 | 1.010372              | 2.422480                                                       |
| 44065 | 1.372518              | 2.422483                                                       |
| 44067 | 1.372819              | 2.422486                                                       |
| 44069 | 1.010779              | 2.422490                                                       |
| 44071 | 1.000023              | 2.422493                                                       |
| 44073 | 1.486624              | 2.422496                                                       |
| 44075 | 1.299784              | 2.422499                                                       |
| 44077 | 1.091181              | 2.422502                                                       |
| 44079 | 1.524535              | 2.422506                                                       |
| 44081 | 1.059232              | 2.422509                                                       |
| 44083 | 1.077241              | 2.422512                                                       |
| 44085 | 1.600544              | 2.422515                                                       |
| 44087 | 1.000023              | 2.422519                                                       |
| 44089 | 1.000023              | 2.422522                                                       |
| 44091 | 1.567667              | 2.422525                                                       |
| 44093 | 1.143039              | 2.422528                                                       |
| 44095 | 1.200136              | 2.422531                                                       |
| 44097 | 1.333424              | 2.422535                                                       |
| 44099 | 1.153768              | 2.422538                                                       |
| 44101 | 1.000023              | 2.422541                                                       |

| $n$   | $\frac{\sigma(n)}{n}$ | $\frac{e^\gamma}{2} \log \log n + \frac{0.73...}{\log \log n}$ |
|-------|-----------------------|----------------------------------------------------------------|
| 44103 | 1.360814              | 2.422544                                                       |
| 44105 | 1.200136              | 2.422548                                                       |
| 44107 | 1.143039              | 2.422551                                                       |
| 44109 | 1.618037              | 2.422554                                                       |
| 44111 | 1.000023              | 2.422557                                                       |
| 44113 | 1.032983              | 2.422560                                                       |
| 44115 | 1.703910              | 2.422564                                                       |
| 44117 | 1.009951              | 2.422567                                                       |
| 44119 | 1.000023              | 2.422570                                                       |
| 44121 | 1.671041              | 2.422573                                                       |
| 44123 | 1.000023              | 2.422577                                                       |
| 44125 | 1.251535              | 2.422580                                                       |
| 44127 | 1.444739              | 2.422583                                                       |
| 44129 | 1.000023              | 2.422586                                                       |
| 44131 | 1.000023              | 2.422589                                                       |
| 44133 | 1.366053              | 2.422593                                                       |
| 44135 | 1.492149              | 2.422596                                                       |
| 44137 | 1.109273              | 2.422599                                                       |
| 44139 | 1.333424              | 2.422602                                                       |
| 44141 | 1.027888              | 2.422605                                                       |
| 44143 | 1.091181              | 2.422609                                                       |
| 44145 | 1.809038              | 2.422612                                                       |
| 44147 | 1.010624              | 2.422615                                                       |
| 44149 | 1.254932              | 2.422618                                                       |
| 44151 | 1.333424              | 2.422622                                                       |
| 44153 | 1.016465              | 2.422625                                                       |
| 44155 | 1.200136              | 2.422628                                                       |
| 44157 | 1.369658              | 2.422631                                                       |
| 44159 | 1.000023              | 2.422634                                                       |
| 44161 | 1.115917              | 2.422638                                                       |
| 44163 | 1.653149              | 2.422641                                                       |
| 44165 | 1.337077              | 2.422644                                                       |
| 44167 | 1.035162              | 2.422647                                                       |
| 44169 | 1.333424              | 2.422650                                                       |
| 44171 | 1.000023              | 2.422654                                                       |
| 44173 | 1.009848              | 2.422657                                                       |
| 44175 | 1.796491              | 2.422660                                                       |
| 44177 | 1.143038              | 2.422663                                                       |
| 44179 | 1.000023              | 2.422666                                                       |
| 44181 | 1.444739              | 2.422670                                                       |
| 44183 | 1.114637              | 2.422673                                                       |
| 44185 | 1.200136              | 2.422676                                                       |
| 44187 | 1.581642              | 2.422679                                                       |
| 44189 | 1.000023              | 2.422683                                                       |

| $n$   | $\frac{\sigma(n)}{n}$ | $\frac{e^\gamma}{2} \log \log n + \frac{0.73...}{\log \log n}$ |
|-------|-----------------------|----------------------------------------------------------------|
| 44191 | 1.173090              | 2.422686                                                       |
| 44193 | 1.333424              | 2.422689                                                       |
| 44195 | 1.200136              | 2.422692                                                       |
| 44197 | 1.009571              | 2.422695                                                       |
| 44199 | 1.482386              | 2.422699                                                       |
| 44201 | 1.000023              | 2.422702                                                       |
| 44203 | 1.000023              | 2.422705                                                       |
| 44205 | 1.832915              | 2.422708                                                       |
| 44207 | 1.000023              | 2.422711                                                       |
| 44209 | 1.091181              | 2.422715                                                       |
| 44211 | 1.333424              | 2.422718                                                       |
| 44213 | 1.139936              | 2.422721                                                       |
| 44215 | 1.237589              | 2.422724                                                       |
| 44217 | 1.534704              | 2.422727                                                       |
| 44219 | 1.143038              | 2.422731                                                       |
| 44221 | 1.000023              | 2.422734                                                       |
| 44223 | 1.333424              | 2.422737                                                       |
| 44225 | 1.303787              | 2.422740                                                       |
| 44227 | 1.022362              | 2.422744                                                       |
| 44229 | 1.393475              | 2.422747                                                       |
| 44231 | 1.091180              | 2.422750                                                       |
| 44233 | 1.171976              | 2.422753                                                       |
| 44235 | 1.735097              | 2.422756                                                       |
| 44237 | 1.032981              | 2.422760                                                       |
| 44239 | 1.116481              | 2.422763                                                       |
| 44241 | 1.333424              | 2.422766                                                       |
| 44243 | 1.010058              | 2.422769                                                       |
| 44245 | 1.200136              | 2.422772                                                       |
| 44247 | 1.591068              | 2.422776                                                       |
| 44249 | 1.000023              | 2.422779                                                       |
| 44251 | 1.122686              | 2.422782                                                       |
| 44253 | 1.627008              | 2.422785                                                       |
| 44255 | 1.229963              | 2.422788                                                       |
| 44257 | 1.000023              | 2.422792                                                       |
| 44259 | 1.333424              | 2.422795                                                       |
| 44261 | 1.143038              | 2.422798                                                       |
| 44263 | 1.000023              | 2.422801                                                       |
| 44265 | 1.730668              | 2.422804                                                       |
| 44267 | 1.000023              | 2.422808                                                       |
| 44269 | 1.000023              | 2.422811                                                       |
| 44271 | 1.444738              | 2.422814                                                       |
| 44273 | 1.000023              | 2.422817                                                       |
| 44275 | 1.613190              | 2.422820                                                       |
| 44277 | 1.333424              | 2.422824                                                       |

| $n$   | $\frac{\sigma(n)}{n}$ | $\frac{e^\gamma}{2} \log \log n + \frac{0.73...}{\log \log n}$ |
|-------|-----------------------|----------------------------------------------------------------|
| 44279 | 1.000023              | 2.422827                                                       |
| 44281 | 1.000023              | 2.422830                                                       |
| 44283 | 1.382020              | 2.422833                                                       |
| 44285 | 1.273027              | 2.422836                                                       |
| 44287 | 1.016461              | 2.422840                                                       |
| 44289 | 1.784642              | 2.422843                                                       |
| 44291 | 1.077239              | 2.422846                                                       |
| 44293 | 1.000023              | 2.422849                                                       |
| 44295 | 1.600542              | 2.422852                                                       |
| 44297 | 1.091180              | 2.422856                                                       |
| 44299 | 1.032980              | 2.422859                                                       |
| 44301 | 1.333424              | 2.422862                                                       |
| 44303 | 1.143038              | 2.422865                                                       |
| 44305 | 1.200135              | 2.422869                                                       |
| 44307 | 1.496558              | 2.422872                                                       |
| 44309 | 1.018303              | 2.422875                                                       |
| 44311 | 1.015369              | 2.422878                                                       |
| 44313 | 1.333424              | 2.422881                                                       |
| 44315 | 1.200135              | 2.422885                                                       |
| 44317 | 1.233296              | 2.422888                                                       |
| 44319 | 1.559602              | 2.422891                                                       |
| 44321 | 1.091672              | 2.422894                                                       |
| 44323 | 1.010762              | 2.422897                                                       |
| 44325 | 1.800203              | 2.422901                                                       |
| 44327 | 1.053083              | 2.422904                                                       |
| 44329 | 1.012520              | 2.422907                                                       |
| 44331 | 1.524531              | 2.422910                                                       |
| 44333 | 1.024248              | 2.422913                                                       |
| 44335 | 1.200135              | 2.422917                                                       |
| 44337 | 1.333424              | 2.422920                                                       |
| 44339 | 1.012201              | 2.422923                                                       |
| 44341 | 1.136646              | 2.422926                                                       |
| 44343 | 1.559660              | 2.422929                                                       |
| 44345 | 1.403631              | 2.422933                                                       |
| 44347 | 1.017792              | 2.422936                                                       |
| 44349 | 1.333424              | 2.422939                                                       |
| 44351 | 1.000023              | 2.422942                                                       |
| 44353 | 1.059229              | 2.422945                                                       |
| 44355 | 1.600541              | 2.422948                                                       |
| 44357 | 1.000023              | 2.422952                                                       |
| 44359 | 1.143037              | 2.422955                                                       |
| 44361 | 1.558125              | 2.422958                                                       |
| 44363 | 1.130672              | 2.422961                                                       |
| 44365 | 1.265863              | 2.422964                                                       |

| $n$   | $\frac{\sigma(n)}{n}$ | $\frac{e^\gamma}{2} \log \log n + \frac{0.73...}{\log \log n}$ |
|-------|-----------------------|----------------------------------------------------------------|
| 44367 | 1.393468              | 2.422968                                                       |
| 44369 | 1.077239              | 2.422971                                                       |
| 44371 | 1.000023              | 2.422974                                                       |
| 44373 | 1.524531              | 2.422977                                                       |
| 44375 | 1.267200              | 2.422980                                                       |
| 44377 | 1.009532              | 2.422984                                                       |
| 44379 | 1.444737              | 2.422987                                                       |
| 44381 | 1.000023              | 2.422990                                                       |
| 44383 | 1.000023              | 2.422993                                                       |
| 44385 | 1.751943              | 2.422996                                                       |
| 44387 | 1.213328              | 2.423000                                                       |
| 44389 | 1.000023              | 2.423003                                                       |
| 44391 | 1.333423              | 2.423006                                                       |
| 44393 | 1.012051              | 2.423009                                                       |
| 44395 | 1.294200              | 2.423012                                                       |
| 44397 | 1.444737              | 2.423016                                                       |
| 44399 | 1.035158              | 2.423019                                                       |
| 44401 | 1.143037              | 2.423022                                                       |
| 44403 | 1.441524              | 2.423025                                                       |
| 44405 | 1.225808              | 2.423028                                                       |
| 44407 | 1.102169              | 2.423032                                                       |
| 44409 | 1.355401              | 2.423035                                                       |
| 44411 | 1.013262              | 2.423038                                                       |
| 44413 | 1.044019              | 2.423041                                                       |
| 44415 | 2.074975              | 2.423044                                                       |
| 44417 | 1.000023              | 2.423048                                                       |
| 44419 | 1.024246              | 2.423051                                                       |
| 44421 | 1.543054              | 2.423054                                                       |
| 44423 | 1.032978              | 2.423057                                                       |
| 44425 | 1.240698              | 2.423060                                                       |
| 44427 | 1.361334              | 2.423064                                                       |
| 44429 | 1.248914              | 2.423067                                                       |
| 44431 | 1.009926              | 2.423070                                                       |
| 44433 | 1.444737              | 2.423073                                                       |
| 44435 | 1.200135              | 2.423076                                                       |
| 44437 | 1.027882              | 2.423079                                                       |
| 44439 | 1.333423              | 2.423083                                                       |
| 44441 | 1.053082              | 2.423086                                                       |
| 44443 | 1.164548              | 2.423089                                                       |
| 44445 | 1.600540              | 2.423092                                                       |
| 44447 | 1.086957              | 2.423095                                                       |
| 44449 | 1.000022              | 2.423099                                                       |
| 44451 | 1.579267              | 2.423102                                                       |
| 44453 | 1.000022              | 2.423105                                                       |

| $n$   | $\frac{\sigma(n)}{n}$ | $\frac{e^\gamma}{2} \log \log n + \frac{0.73...}{\log \log n}$ |
|-------|-----------------------|----------------------------------------------------------------|
| 44455 | 1.273018              | 2.423108                                                       |
| 44457 | 1.597949              | 2.423111                                                       |
| 44459 | 1.044018              | 2.423115                                                       |
| 44461 | 1.009694              | 2.423118                                                       |
| 44463 | 1.333423              | 2.423121                                                       |
| 44465 | 1.200135              | 2.423124                                                       |
| 44467 | 1.020082              | 2.423127                                                       |
| 44469 | 1.523893              | 2.423131                                                       |
| 44471 | 1.143037              | 2.423134                                                       |
| 44473 | 1.178603              | 2.423137                                                       |
| 44475 | 1.656121              | 2.423140                                                       |
| 44477 | 1.014457              | 2.423143                                                       |
| 44479 | 1.053081              | 2.423146                                                       |
| 44481 | 1.333423              | 2.423150                                                       |
| 44483 | 1.000022              | 2.423153                                                       |
| 44485 | 1.450197              | 2.423156                                                       |
| 44487 | 1.444737              | 2.423159                                                       |
| 44489 | 1.059228              | 2.423162                                                       |
| 44491 | 1.000022              | 2.423166                                                       |
| 44493 | 1.333423              | 2.423169                                                       |
| 44495 | 1.310709              | 2.423172                                                       |
| 44497 | 1.000022              | 2.423175                                                       |
| 44499 | 1.651093              | 2.423178                                                       |
| 44501 | 1.000022              | 2.423182                                                       |
| 44503 | 1.009550              | 2.423185                                                       |
| 44505 | 1.850758              | 2.423188                                                       |
| 44507 | 1.000022              | 2.423191                                                       |
| 44509 | 1.022355              | 2.423194                                                       |
| 44511 | 1.372784              | 2.423197                                                       |
| 44513 | 1.143037              | 2.423201                                                       |
| 44515 | 1.245423              | 2.423204                                                       |
| 44517 | 1.552665              | 2.423207                                                       |
| 44519 | 1.000022              | 2.423210                                                       |
| 44521 | 1.004762              | 2.423213                                                       |
| 44523 | 1.584799              | 2.423217                                                       |
| 44525 | 1.345132              | 2.423220                                                       |
| 44527 | 1.143037              | 2.423223                                                       |
| 44529 | 1.333423              | 2.423226                                                       |
| 44531 | 1.000022              | 2.423229                                                       |
| 44533 | 1.000022              | 2.423232                                                       |
| 44535 | 1.600539              | 2.423236                                                       |
| 44537 | 1.000022              | 2.423239                                                       |
| 44539 | 1.091179              | 2.423242                                                       |
| 44541 | 1.696908              | 2.423245                                                       |



| $n$   | $\frac{\sigma(n)}{n}$ | $\frac{e^\gamma}{2} \log \log n + \frac{0.73...}{\log \log n}$ |
|-------|-----------------------|----------------------------------------------------------------|
| 44543 | 1.000022              | 2.423248                                                       |
| 44545 | 1.228421              | 2.423252                                                       |
| 44547 | 1.379217              | 2.423255                                                       |
| 44549 | 1.000022              | 2.423258                                                       |
| 44551 | 1.131288              | 2.423261                                                       |
| 44553 | 1.333423              | 2.423264                                                       |
| 44555 | 1.465155              | 2.423268                                                       |
| 44557 | 1.059228              | 2.423271                                                       |
| 44559 | 1.444736              | 2.423274                                                       |
| 44561 | 1.091178              | 2.423277                                                       |
| 44563 | 1.000022              | 2.423280                                                       |
| 44565 | 1.600539              | 2.423283                                                       |
| 44567 | 1.025333              | 2.423287                                                       |
| 44569 | 1.143037              | 2.423290                                                       |
| 44571 | 1.356936              | 2.423293                                                       |
| 44573 | 1.055213              | 2.423296                                                       |
| 44575 | 1.240695              | 2.423299                                                       |
| 44577 | 1.608004              | 2.423302                                                       |
| 44579 | 1.000022              | 2.423306                                                       |
| 44581 | 1.011642              | 2.423309                                                       |
| 44583 | 1.670951              | 2.423312                                                       |
| 44585 | 1.237546              | 2.423315                                                       |
| 44587 | 1.000022              | 2.423318                                                       |
| 44589 | 1.356388              | 2.423322                                                       |
| 44591 | 1.101209              | 2.423325                                                       |
| 44593 | 1.053080              | 2.423328                                                       |
| 44595 | 1.735082              | 2.423331                                                       |
| 44597 | 1.196852              | 2.423334                                                       |
| 44599 | 1.012041              | 2.423337                                                       |
| 44601 | 1.333423              | 2.423341                                                       |
| 44603 | 1.114903              | 2.423344                                                       |
| 44605 | 1.310705              | 2.423347                                                       |
| 44607 | 1.333423              | 2.423350                                                       |
| 44609 | 1.032975              | 2.423353                                                       |
| 44611 | 1.143036              | 2.423357                                                       |
| 44613 | 1.444736              | 2.423360                                                       |
| 44615 | 1.200134              | 2.423363                                                       |
| 44617 | 1.000022              | 2.423366                                                       |
| 44619 | 1.355476              | 2.423369                                                       |
| 44621 | 1.000022              | 2.423372                                                       |
| 44623 | 1.000022              | 2.423376                                                       |
| 44625 | 2.013580              | 2.423379                                                       |
| 44627 | 1.091178              | 2.423382                                                       |
| 44629 | 1.077237              | 2.423385                                                       |

| $n$   | $\frac{\sigma(n)}{n}$ | $\frac{e^\gamma}{2} \log \log n + \frac{0.73...}{\log \log n}$ |
|-------|-----------------------|----------------------------------------------------------------|
| 44631 | 1.626672              | 2.423388                                                       |
| 44633 | 1.000022              | 2.423391                                                       |
| 44635 | 1.225944              | 2.423395                                                       |
| 44637 | 1.333423              | 2.423398                                                       |
| 44639 | 1.164542              | 2.423401                                                       |
| 44641 | 1.000022              | 2.423404                                                       |
| 44643 | 1.393455              | 2.423407                                                       |
| 44645 | 1.200134              | 2.423411                                                       |
| 44647 | 1.000022              | 2.423414                                                       |
| 44649 | 1.626419              | 2.423417                                                       |
| 44651 | 1.000022              | 2.423420                                                       |
| 44653 | 1.143036              | 2.423423                                                       |
| 44655 | 1.730601              | 2.423426                                                       |
| 44657 | 1.000022              | 2.423430                                                       |
| 44659 | 1.102756              | 2.423433                                                       |
| 44661 | 1.333423              | 2.423436                                                       |
| 44663 | 1.018293              | 2.423439                                                       |
| 44665 | 1.200134              | 2.423442                                                       |
| 44667 | 1.653122              | 2.423445                                                       |
| 44669 | 1.053079              | 2.423449                                                       |
| 44671 | 1.134696              | 2.423452                                                       |
| 44673 | 1.333423              | 2.423455                                                       |
| 44675 | 1.240694              | 2.423458                                                       |
| 44677 | 1.024241              | 2.423461                                                       |
| 44679 | 1.363325              | 2.423465                                                       |
| 44681 | 1.233276              | 2.423468                                                       |
| 44683 | 1.000022              | 2.423471                                                       |
| 44685 | 1.783149              | 2.423474                                                       |
| 44687 | 1.000022              | 2.423477                                                       |
| 44689 | 1.095572              | 2.423480                                                       |
| 44691 | 1.333423              | 2.423484                                                       |
| 44693 | 1.159913              | 2.423487                                                       |
| 44695 | 1.372503              | 2.423490                                                       |
| 44697 | 1.365998              | 2.423493                                                       |
| 44699 | 1.000022              | 2.423496                                                       |
| 44701 | 1.000022              | 2.423499                                                       |
| 44703 | 1.444735              | 2.423503                                                       |
| 44705 | 1.200134              | 2.423506                                                       |
| 44707 | 1.139866              | 2.423509                                                       |
| 44709 | 1.524525              | 2.423512                                                       |
| 44711 | 1.000022              | 2.423515                                                       |
| 44713 | 1.017780              | 2.423518                                                       |
| 44715 | 1.751895              | 2.423522                                                       |
| 44717 | 1.012501              | 2.423525                                                       |

| $n$   | $\frac{\sigma(n)}{n}$ | $\frac{e^\gamma}{2} \log \log n + \frac{0.73...}{\log \log n}$ |
|-------|-----------------------|----------------------------------------------------------------|
| 44719 | 1.009504              | 2.423528                                                       |
| 44721 | 1.444735              | 2.423531                                                       |
| 44723 | 1.143036              | 2.423534                                                       |
| 44725 | 1.240693              | 2.423537                                                       |
| 44727 | 1.413374              | 2.423541                                                       |
| 44729 | 1.000022              | 2.423544                                                       |
| 44731 | 1.025329              | 2.423547                                                       |
| 44733 | 1.522277              | 2.423550                                                       |
| 44735 | 1.255393              | 2.423553                                                       |
| 44737 | 1.284306              | 2.423556                                                       |
| 44739 | 1.482376              | 2.423560                                                       |
| 44741 | 1.000022              | 2.423563                                                       |
| 44743 | 1.012181              | 2.423566                                                       |
| 44745 | 1.694938              | 2.423569                                                       |
| 44747 | 1.035153              | 2.423572                                                       |
| 44749 | 1.015352              | 2.423575                                                       |
| 44751 | 1.524525              | 2.423579                                                       |
| 44753 | 1.000022              | 2.423582                                                       |
| 44755 | 1.200134              | 2.423585                                                       |
| 44757 | 1.444735              | 2.423588                                                       |
| 44759 | 1.178579              | 2.423591                                                       |
| 44761 | 1.059226              | 2.423594                                                       |
| 44763 | 1.368273              | 2.423598                                                       |
| 44765 | 1.372501              | 2.423601                                                       |
| 44767 | 1.013246              | 2.423604                                                       |
| 44769 | 1.333423              | 2.423607                                                       |
| 44771 | 1.000022              | 2.423610                                                       |
| 44773 | 1.000022              | 2.423613                                                       |
| 44775 | 1.800112              | 2.423617                                                       |
| 44777 | 1.000022              | 2.423620                                                       |
| 44779 | 1.143036              | 2.423623                                                       |
| 44781 | 1.543512              | 2.423626                                                       |
| 44783 | 1.053078              | 2.423629                                                       |
| 44785 | 1.323925              | 2.423632                                                       |
| 44787 | 1.333423              | 2.423636                                                       |
| 44789 | 1.000022              | 2.423639                                                       |
| 44791 | 1.022348              | 2.423642                                                       |
| 44793 | 1.728842              | 2.423645                                                       |
| 44795 | 1.315861              | 2.423648                                                       |
| 44797 | 1.000022              | 2.423651                                                       |
| 44799 | 1.355387              | 2.423655                                                       |
| 44801 | 1.015692              | 2.423658                                                       |
| 44803 | 1.091177              | 2.423661                                                       |
| 44805 | 1.671242              | 2.423664                                                       |

| $n$   | $\frac{\sigma(n)}{n}$ | $\frac{e^\gamma}{2} \log \log n + \frac{0.73...}{\log \log n}$ |
|-------|-----------------------|----------------------------------------------------------------|
| 44807 | 1.180530              | 2.423667                                                       |
| 44809 | 1.000022              | 2.423670                                                       |
| 44811 | 1.559617              | 2.423674                                                       |
| 44813 | 1.025327              | 2.423677                                                       |
| 44815 | 1.200134              | 2.423680                                                       |
| 44817 | 1.333423              | 2.423683                                                       |
| 44819 | 1.000022              | 2.423686                                                       |
| 44821 | 1.206577              | 2.423689                                                       |
| 44823 | 1.359302              | 2.423693                                                       |
| 44825 | 1.361026              | 2.423696                                                       |
| 44827 | 1.044014              | 2.423699                                                       |
| 44829 | 1.534632              | 2.423702                                                       |
| 44831 | 1.010729              | 2.423705                                                       |
| 44833 | 1.011755              | 2.423708                                                       |
| 44835 | 1.891736              | 2.423712                                                       |
| 44837 | 1.077235              | 2.423715                                                       |
| 44839 | 1.000022              | 2.423718                                                       |
| 44841 | 1.333423              | 2.423721                                                       |
| 44843 | 1.000022              | 2.423724                                                       |
| 44845 | 1.200134              | 2.423727                                                       |
| 44847 | 1.626865              | 2.423730                                                       |
| 44849 | 1.177284              | 2.423734                                                       |
| 44851 | 1.000022              | 2.423737                                                       |
| 44853 | 1.333423              | 2.423740                                                       |
| 44855 | 1.200134              | 2.423743                                                       |
| 44857 | 1.032971              | 2.423746                                                       |
| 44859 | 1.405292              | 2.423749                                                       |
| 44861 | 1.011391              | 2.423753                                                       |
| 44863 | 1.348104              | 2.423756                                                       |
| 44865 | 1.735072              | 2.423759                                                       |
| 44867 | 1.000022              | 2.423762                                                       |
| 44869 | 1.091177              | 2.423765                                                       |
| 44871 | 1.333422              | 2.423768                                                       |
| 44873 | 1.044013              | 2.423772                                                       |
| 44875 | 1.251476              | 2.423775                                                       |
| 44877 | 1.524523              | 2.423778                                                       |
| 44879 | 1.000022              | 2.423781                                                       |
| 44881 | 1.027874              | 2.423784                                                       |
| 44883 | 1.444734              | 2.423787                                                       |
| 44885 | 1.231948              | 2.423790                                                       |
| 44887 | 1.000022              | 2.423794                                                       |
| 44889 | 1.437145              | 2.423797                                                       |
| 44891 | 1.279900              | 2.423800                                                       |
| 44893 | 1.000022              | 2.423803                                                       |

| $n$   | $\frac{\sigma(n)}{n}$ | $\frac{e^\gamma}{2} \log \log n + \frac{0.73...}{\log \log n}$ |
|-------|-----------------------|----------------------------------------------------------------|
| 44895 | 1.661477              | 2.423806                                                       |
| 44897 | 1.122569              | 2.423809                                                       |
| 44899 | 1.018285              | 2.423813                                                       |
| 44901 | 1.482372              | 2.423816                                                       |
| 44903 | 1.013919              | 2.423819                                                       |
| 44905 | 1.372497              | 2.423822                                                       |
| 44907 | 1.333422              | 2.423825                                                       |
| 44909 | 1.000022              | 2.423828                                                       |
| 44911 | 1.012491              | 2.423832                                                       |
| 44913 | 1.455614              | 2.423835                                                       |
| 44915 | 1.294178              | 2.423838                                                       |
| 44917 | 1.000022              | 2.423841                                                       |
| 44919 | 1.778134              | 2.423844                                                       |
| 44921 | 1.035151              | 2.423847                                                       |
| 44923 | 1.009728              | 2.423850                                                       |
| 44925 | 1.656093              | 2.423854                                                       |
| 44927 | 1.000022              | 2.423857                                                       |
| 44929 | 1.009593              | 2.423860                                                       |
| 44931 | 1.413367              | 2.423863                                                       |
| 44933 | 1.175083              | 2.423866                                                       |
| 44935 | 1.410037              | 2.423869                                                       |
| 44937 | 1.444734              | 2.423873                                                       |
| 44939 | 1.000022              | 2.423876                                                       |
| 44941 | 1.077235              | 2.423879                                                       |
| 44943 | 1.358521              | 2.423882                                                       |
| 44945 | 1.225498              | 2.423885                                                       |
| 44947 | 1.143035              | 2.423888                                                       |
| 44949 | 1.333422              | 2.423891                                                       |
| 44951 | 1.014438              | 2.423895                                                       |
| 44953 | 1.000022              | 2.423898                                                       |
| 44955 | 1.846113              | 2.423901                                                       |
| 44957 | 1.125342              | 2.423904                                                       |
| 44959 | 1.000022              | 2.423907                                                       |
| 44961 | 1.524521              | 2.423910                                                       |
| 44963 | 1.000022              | 2.423914                                                       |
| 44965 | 1.328233              | 2.423917                                                       |
| 44967 | 1.437143              | 2.423920                                                       |
| 44969 | 1.009495              | 2.423923                                                       |
| 44971 | 1.000022              | 2.423926                                                       |
| 44973 | 1.526249              | 2.423929                                                       |
| 44975 | 1.422657              | 2.423932                                                       |
| 44977 | 1.025324              | 2.423936                                                       |
| 44979 | 1.536717              | 2.423939                                                       |
| 44981 | 1.032969              | 2.423942                                                       |

| $n$   | $\frac{\sigma(n)}{n}$ | $\frac{e^\gamma}{2} \log \log n + \frac{0.73...}{\log \log n}$ |
|-------|-----------------------|----------------------------------------------------------------|
| 44983 | 1.000022              | 2.423945                                                       |
| 44985 | 1.600534              | 2.423948                                                       |
| 44987 | 1.000022              | 2.423951                                                       |
| 44989 | 1.143035              | 2.423954                                                       |
| 44991 | 1.444733              | 2.423958                                                       |
| 44993 | 1.077234              | 2.423961                                                       |
| 44995 | 1.200133              | 2.423964                                                       |
| 44997 | 1.363291              | 2.423967                                                       |
| 44999 | 1.059224              | 2.423970                                                       |
| 45001 | 1.091176              | 2.423973                                                       |
| 45003 | 1.524521              | 2.423976                                                       |
| 45005 | 1.200133              | 2.423980                                                       |
| 45007 | 1.000022              | 2.423983                                                       |
| 45009 | 1.482370              | 2.423986                                                       |
| 45011 | 1.109062              | 2.423989                                                       |
| 45013 | 1.000022              | 2.423992                                                       |
| 45015 | 1.600533              | 2.423995                                                       |
| 45017 | 1.172890              | 2.423999                                                       |
| 45019 | 1.077234              | 2.424002                                                       |
| 45021 | 1.368250              | 2.424005                                                       |
| 45023 | 1.091176              | 2.424008                                                       |
| 45025 | 1.240689              | 2.424011                                                       |
| 45027 | 1.444733              | 2.424014                                                       |
| 45029 | 1.027871              | 2.424017                                                       |
| 45031 | 1.164531              | 2.424021                                                       |
| 45033 | 1.413364              | 2.424024                                                       |
| 45035 | 1.200133              | 2.424027                                                       |
| 45037 | 1.035149              | 2.424030                                                       |
| 45039 | 1.333422              | 2.424033                                                       |
| 45041 | 1.015342              | 2.424036                                                       |
| 45043 | 1.032968              | 2.424039                                                       |
| 45045 | 2.327273              | 2.424043                                                       |
